# Supplementary material for: Two-Loop Anomalous Dimensions in the LEFT: Dimension-Six Four-Fermion Operators in NDR
Source: arXiv:2501.08384 ancillary file (2026-01-17)
Supplement: Supplementary file 1 [file Beta_Functions_at_NLO.pdf]

# Appendix:

## Four-Fermion Beta Functions in the LEFT

Jason Aebischer<sup>a</sup>, Pol Morell<sup>b,c</sup>, Marko Pesut<sup>d</sup> and Javier Virto<sup>b,c</sup>

<sup>a</sup> *Theoretical Physics Department, CERN, 1211 Geneva 23, Switzerland*

<sup>b</sup> *Departament de Física Quàntica i Astrofísica, Universitat de Barcelona,  
Martí Franquès 1, E08028 Barcelona, Catalunya*

<sup>c</sup> *Institut de Ciències del Cosmos (ICCUB), Universitat de Barcelona,  
Martí Franquès 1, E08028 Barcelona, Catalunya*

<sup>d</sup> *Physik-Institut, Universität Zürich, CH-8057 Zürich, Switzerland*

### Abstract

This is the collection of all the contributions from four-fermion operators to the beta functions of four-fermion operators in the LEFT, up to NLO in both  $\alpha_s$  and  $\alpha$ . In the following expressions, different flavor indices  $i, j, k, l$  are always indicate different fermions (e.g.  $\bar{\psi}_i \chi_j$  will imply  $i \neq j$  if  $\psi = \chi$ ; and any pair  $i, j$  if  $\psi \neq \chi$ ). The particular arrangements of flavor indices in each sector follow the description in the main text.

# Contents

|          |                                                                                                              |            |
|----------|--------------------------------------------------------------------------------------------------------------|------------|
| <b>1</b> | <b>Five Flavor LEFT</b>                                                                                      | <b>4</b>   |
| 1.1      | $\Delta F = 2$ Transitions $(\bar{f}_i f_j \bar{f}_i f_j)$                                                   | 4          |
| 1.2      | $\Delta F = 1.5$ Transitions $(\bar{f}_i f_j \bar{f}_k f_j)$                                                 | 6          |
| 1.3      | $\Delta F = 1$ Transitions $(\bar{f}_i f_j \bar{f}'_k f'_l)$                                                 | 9          |
| 1.4      | $\Delta F = 1^{\bar{f}f}$ Transitions $(\bar{f}_i f_j \bar{f}'_k f'_k)$                                      | 14         |
| 1.5      | $\Delta F = 1^{\bar{f}f} : d\text{-type}$ $(\bar{d}_i d_j \bar{f}_k f_k)$                                    | 14         |
| 1.6      | $\Delta F = 1^{\bar{f}f} : u\text{-type}$ $(\bar{u}_i u_j \bar{f}_k f_k)$                                    | 57         |
| 1.7      | $\Delta F = 1^{\bar{f}f} : e\text{-type}$ $(\bar{e}_i e_j \bar{f}_k f_k)$                                    | 99         |
| 1.8      | $\Delta F = 1^{\bar{f}f} : \nu\text{-type}$ $(\bar{\nu}_i \nu_j \bar{f}_k f_k)$                              | 121        |
| 1.9      | $\Delta F = 0$ Transitions $(\bar{f}_i f_i \bar{f}_j f_j)$                                                   | 133        |
| 1.10     | $\Delta L = 2$ Transitions $(\bar{\nu}_i^c \nu_j \bar{f}_k f_l \text{ or } \bar{\nu}_i^c e_j \bar{d}_k u_l)$ | 229        |
| 1.11     | $\Delta L = 4$ Transitions $(\bar{\nu}_i^c \nu_j \bar{\nu}_k^c \nu_l)$                                       | 231        |
| 1.12     | $ \Delta B  =  \Delta L  = 1$ Transitions: Baryon Number Violation                                           | 231        |
| <b>2</b> | <b>Four Flavor LEFT</b>                                                                                      | <b>234</b> |
| 2.1      | $\Delta F = 2$ Transitions $(\bar{f}_i f_j \bar{f}_i f_j)$                                                   | 234        |
| 2.2      | $\Delta F = 1.5$ Transitions $(\bar{f}_i f_j \bar{f}_k f_j)$                                                 | 236        |
| 2.3      | $\Delta F = 1$ Transitions $(\bar{f}_i f_j \bar{f}'_k f'_l)$                                                 | 237        |
| 2.4      | $\Delta F = 1^{\bar{f}f}$ Transitions $(\bar{f}_i f_j \bar{f}'_k f'_k)$                                      | 242        |
| 2.5      | $\Delta F = 1^{\bar{f}f} : d\text{-type}$ $(\bar{d}_i d_j \bar{f}_k f_k)$                                    | 242        |
| 2.6      | $\Delta F = 1^{\bar{f}f} : u\text{-type}$ $(\bar{u}_i u_j \bar{f}_k f_k)$                                    | 272        |
| 2.7      | $\Delta F = 1^{\bar{f}f} : e\text{-type}$ $(\bar{e}_i e_j \bar{f}_k f_k)$                                    | 303        |
| 2.8      | $\Delta F = 1^{\bar{f}f} : \nu\text{-type}$ $(\bar{\nu}_i \nu_j \bar{f}_k f_k)$                              | 321        |
| 2.9      | $\Delta F = 0$ Transitions $(\bar{f}_i f_i \bar{f}_j f_j)$                                                   | 330        |
| 2.10     | $\Delta L = 2$ Transitions $(\bar{\nu}_i^c \nu_j \bar{f}_k f_l \text{ or } \bar{\nu}_i^c e_j \bar{d}_k u_l)$ | 413        |
| 2.11     | $\Delta L = 4$ Transitions $(\bar{\nu}_i^c \nu_j \bar{\nu}_k^c \nu_l)$                                       | 414        |
| 2.12     | $ \Delta B  =  \Delta L  = 1$ Transitions: Baryon Number Violation                                           | 414        |
| <b>3</b> | <b>Three Flavor LEFT</b>                                                                                     | <b>417</b> |
| 3.1      | $\Delta F = 2$ Transitions $(\bar{f}_i f_j \bar{f}_i f_j)$                                                   | 417        |
| 3.2      | $\Delta F = 1.5$ Transitions $(\bar{f}_i f_j \bar{f}_k f_j)$                                                 | 418        |
| 3.3      | $\Delta F = 1$ Transitions $(\bar{f}_i f_j \bar{f}'_k f'_l)$                                                 | 418        |
| 3.4      | $\Delta F = 1^{\bar{f}f}$ Transitions $(\bar{f}_i f_j \bar{f}'_k f'_k)$                                      | 420        |
| 3.5      | $\Delta F = 1^{\bar{f}f} : d\text{-type}$ $(\bar{d}_i d_j \bar{f}_k f_k)$                                    | 420        |
| 3.6      | $\Delta F = 1^{\bar{f}f} : e\text{-type}$ $(\bar{e}_i e_j \bar{f}_k f_k)$                                    | 438        |
| 3.7      | $\Delta F = 1^{\bar{f}f} : \nu\text{-type}$ $(\bar{\nu}_i \nu_j \bar{f}_k f_k)$                              | 448        |

|      |                                                                                                                        |     |
|------|------------------------------------------------------------------------------------------------------------------------|-----|
| 3.8  | $\Delta F = 0$ Transitions $(\bar{f}_i f_i \bar{f}_j f_j)$ . . . . .                                                   | 453 |
| 3.9  | $\Delta L = 2$ Transitions $(\bar{\nu}_i^c \nu_j \bar{f}_k f_l \text{ or } \bar{\nu}_i^c e_j \bar{d}_k u_l)$ . . . . . | 510 |
| 3.10 | $\Delta L = 4$ Transitions $(\bar{\nu}_i^c \nu_j \bar{\nu}_k^c \nu_l)$ . . . . .                                       | 511 |
| 3.11 | $ \Delta B  =  \Delta L  = 1$ Transitions: Baryon Number Violation . . . . .                                           | 511 |

# 1 Five Flavor LEFT

## 1.1 $\Delta F = 2$ Transitions ( $\bar{f}_i f_j \bar{f}_i f_j$ )

### 1.1.1 $\Delta F = 2 : d\text{-type } (\bar{d}_i d_j \bar{d}_i d_j)$

$$\begin{aligned}
\dot{L}_{dd,ijij}^{V,LL} &= 4g_s^2 L_{dd,ijij}^{V,LL} + \frac{4}{3}e^2 L_{dd,ijij}^{V,LL} - \frac{43}{9}\alpha_s^2 L_{dd,ijij}^{V,LL} - \frac{148}{9}\alpha_s \alpha L_{dd,ijij}^{V,LL} \\
&\quad + \frac{46}{81}\alpha^2 L_{dd,ijij}^{V,LL} ; \\
\dot{L}_{dd,ijij}^{V,RR} &= 4g_s^2 L_{dd,ijij}^{V,RR} + \frac{4}{3}e^2 L_{dd,ijij}^{V,RR} - \frac{43}{9}\alpha_s^2 L_{dd,ijij}^{V,RR} - \frac{148}{9}\alpha_s \alpha L_{dd,ijij}^{V,RR} \\
&\quad + \frac{46}{81}\alpha^2 L_{dd,ijij}^{V,RR} ; \\
\dot{L}_{dd,ijij}^{V1,LR} &= -\frac{8}{3}g_s^2 L_{dd,ijij}^{V8,LR} - \frac{4}{3}e^2 L_{dd,ijij}^{V1,LR} + \alpha_s^2 \left[ -\frac{28}{3}L_{dd,ijij}^{V1,LR} - \frac{2044}{27}L_{dd,ijij}^{V8,LR} \right] \\
&\quad + \alpha_s \alpha \left[ \frac{32}{3}L_{dd,ijij}^{V1,LR} - \frac{8}{27}L_{dd,ijij}^{V8,LR} \right] + \frac{1790}{81}\alpha^2 L_{dd,ijij}^{V1,LR} ; \\
\dot{L}_{dd,ijij}^{V8,LR} &= g_s^2 \left[ -12L_{dd,ijij}^{V1,LR} - 14L_{dd,ijij}^{V8,LR} \right] - \frac{4}{3}e^2 L_{dd,ijij}^{V8,LR} + \alpha_s^2 \left[ -\frac{374}{3}L_{dd,ijij}^{V1,LR} \right. \\
&\quad \left. - \frac{2975}{18}L_{dd,ijij}^{V8,LR} \right] + \alpha_s \alpha \left[ -\frac{4}{3}L_{dd,ijij}^{V1,LR} - \frac{26}{9}L_{dd,ijij}^{V8,LR} \right] + \frac{1790}{81}\alpha^2 L_{dd,ijij}^{V8,LR} ; \\
\dot{L}_{dd,ijij}^{S1,RR} &= g_s^2 \left[ \frac{160}{27}L_{dd,ijij}^{S8,RR} - \frac{80}{9}L_{dd,ijij}^{S1,RR} \right] + e^2 \left[ \frac{4}{27}L_{dd,ijij}^{S1,RR} + \frac{64}{81}L_{dd,ijij}^{S8,RR} \right] \\
&\quad + \alpha_s^2 \left[ \frac{19360}{243}L_{dd,ijij}^{S8,RR} - \frac{9608}{81}L_{dd,ijij}^{S1,RR} \right] + \alpha_s \alpha \left[ \frac{352}{243}L_{dd,ijij}^{S8,RR} - \frac{1040}{81}L_{dd,ijij}^{S1,RR} \right] \\
&\quad + \alpha^2 \left[ \frac{4634}{729}L_{dd,ijij}^{S1,RR} - \frac{3328}{2187}L_{dd,ijij}^{S8,RR} \right] ; \\
\dot{L}_{dd,ijij}^{S8,RR} &= g_s^2 \left[ \frac{8}{3}L_{dd,ijij}^{S1,RR} + \frac{92}{9}L_{dd,ijij}^{S8,RR} \right] + e^2 \left[ \frac{32}{9}L_{dd,ijij}^{S1,RR} - \frac{28}{27}L_{dd,ijij}^{S8,RR} \right] \\
&\quad + \alpha_s^2 \left[ \frac{6479}{81}L_{dd,ijij}^{S8,RR} - \frac{112}{27}L_{dd,ijij}^{S1,RR} \right] + \alpha_s \alpha \left[ -\frac{1840}{27}L_{dd,ijij}^{S1,RR} - \frac{208}{81}L_{dd,ijij}^{S8,RR} \right]
\end{aligned}$$

$$+ \alpha^2 \left[ \frac{6298}{729} L_{ijij}^{S8,RR} - \frac{1664}{243} L_{ijij}^{S1,RR} \right];$$

### 1.1.2 $\Delta F = 2$ : $u$ -type ( $\bar{u}_i u_j \bar{u}_i u_j$ )

$$\begin{aligned} \dot{L}_{ijij}^{V,LL} &= 4g_s^2 L_{ijij}^{V,LL} + \frac{16}{3} e^2 L_{ijij}^{V,LL} - \frac{43}{9} \alpha_s^2 L_{ijij}^{V,LL} - \frac{592}{9} \alpha_s \alpha L_{ijij}^{V,LL} \\ &\quad - \frac{1184}{81} \alpha^2 L_{ijij}^{V,LL}; \end{aligned}$$

$$\begin{aligned} \dot{L}_{ijij}^{V,RR} &= 4g_s^2 L_{ijij}^{V,RR} + \frac{16}{3} e^2 L_{ijij}^{V,RR} - \frac{43}{9} \alpha_s^2 L_{ijij}^{V,RR} - \frac{592}{9} \alpha_s \alpha L_{ijij}^{V,RR} \\ &\quad - \frac{1184}{81} \alpha^2 L_{ijij}^{V,RR}; \end{aligned}$$

$$\begin{aligned} \dot{L}_{ijij}^{V1,LR} &= -\frac{8}{3} g_s^2 L_{ijij}^{V8,LR} - \frac{16}{3} e^2 L_{ijij}^{V1,LR} + \alpha_s^2 \left[ -\frac{28}{3} L_{ijij}^{V1,LR} - \frac{2044}{27} L_{ijij}^{V8,LR} \right] \\ &\quad + \alpha_s \alpha \left[ \frac{128}{3} L_{ijij}^{V1,LR} - \frac{32}{27} L_{ijij}^{V8,LR} \right] + \frac{7520}{81} \alpha^2 L_{ijij}^{V1,LR}; \end{aligned}$$

$$\begin{aligned} \dot{L}_{ijij}^{V8,LR} &= g_s^2 \left[ -12 L_{ijij}^{V1,LR} - 14 L_{ijij}^{V8,LR} \right] - \frac{16}{3} e^2 L_{ijij}^{V8,LR} + \alpha_s^2 \left[ -\frac{374}{3} L_{ijij}^{V1,LR} \right. \\ &\quad \left. - \frac{2975}{18} L_{ijij}^{V8,LR} \right] + \alpha_s \alpha \left[ -\frac{16}{3} L_{ijij}^{V1,LR} - \frac{104}{9} L_{ijij}^{V8,LR} \right] + \frac{7520}{81} \alpha^2 L_{ijij}^{V8,LR}; \end{aligned}$$

$$\begin{aligned} \dot{L}_{ijij}^{S1,RR} &= g_s^2 \left[ \frac{160}{27} L_{ijij}^{S8,RR} - \frac{80}{9} L_{ijij}^{S1,RR} \right] + e^2 \left[ \frac{16}{27} L_{ijij}^{S1,RR} + \frac{256}{81} L_{ijij}^{S8,RR} \right] \\ &\quad + \alpha_s^2 \left[ \frac{19360}{243} L_{ijij}^{S8,RR} - \frac{9608}{81} L_{ijij}^{S1,RR} \right] + \alpha_s \alpha \left[ \frac{1408}{243} L_{ijij}^{S8,RR} - \frac{4160}{81} L_{ijij}^{S1,RR} \right] \\ &\quad + \alpha^2 \left[ \frac{6944}{729} L_{ijij}^{S1,RR} - \frac{22528}{2187} L_{ijij}^{S8,RR} \right]; \end{aligned}$$

$$\begin{aligned} \dot{L}_{ijij}^{S8,RR} &= g_s^2 \left[ \frac{8}{3} L_{ijij}^{S1,RR} + \frac{92}{9} L_{ijij}^{S8,RR} \right] + e^2 \left[ \frac{128}{9} L_{ijij}^{S1,RR} - \frac{112}{27} L_{ijij}^{S8,RR} \right] \\ &\quad + \alpha_s^2 \left[ \frac{6479}{81} L_{ijij}^{S8,RR} - \frac{112}{27} L_{ijij}^{S1,RR} \right] + \alpha_s \alpha \left[ -\frac{7360}{27} L_{ijij}^{S1,RR} - \frac{832}{81} L_{ijij}^{S8,RR} \right] \end{aligned}$$

$$+ \alpha^2 \left[ \frac{18208}{729} L_{ijij}^{S8,RR} - \frac{11264}{243} L_{ijij}^{S1,RR} \right];$$

### 1.1.3 $\Delta F = 2$ : $e$ -type ( $\bar{e}_i e_j \bar{e}_i e_j$ )

$$\dot{L}_{ijij}^{V,LL} = 12e^2 L_{ijij}^{V,LL} - \frac{866}{9} \alpha^2 L_{ijij}^{V,LL};$$

$$\dot{L}_{ijij}^{V,RR} = 12e^2 L_{ijij}^{V,RR} - \frac{866}{9} \alpha^2 L_{ijij}^{V,RR};$$

$$\dot{L}_{ijij}^{V,LR} = \frac{2030}{9} \alpha^2 L_{ijij}^{V,LR} - 12e^2 L_{ijij}^{V,LR};$$

$$\dot{L}_{ijij}^{S,RR} = 12e^2 L_{ijij}^{S,RR} - \frac{1058}{3} \alpha^2 L_{ijij}^{S,RR};$$

### 1.1.4 $\Delta F = 2$ : $\nu$ -type ( $\bar{\nu}_i \nu_j \bar{\nu}_i \nu_j$ )

$$\dot{L}_{ijij}^{V,LL} = 0;$$

## 1.2 $\Delta F = 1.5$ Transitions ( $\bar{f}_i f_j \bar{f}_k f_j$ )

### 1.2.1 $\Delta F = 1.5$ : $d$ -type ( $\bar{d}_i d_j \bar{d}_k d_j$ )

$$\begin{aligned} \dot{L}_{ijkj}^{V,LL} &= 4g_s^2 L_{ijkj}^{V,LL} + \frac{4}{3} e^2 L_{ijkj}^{V,LL} - \frac{43}{9} \alpha_s^2 L_{ijkj}^{V,LL} - \frac{148}{9} \alpha_s \alpha L_{ijkj}^{V,LL} \\ &\quad + \frac{46}{81} \alpha^2 L_{ijkj}^{V,LL}; \end{aligned}$$

$$\begin{aligned} \dot{L}_{ijkj}^{V,RR} &= 4g_s^2 L_{ijkj}^{V,RR} + \frac{4}{3} e^2 L_{ijkj}^{V,RR} - \frac{43}{9} \alpha_s^2 L_{ijkj}^{V,RR} - \frac{148}{9} \alpha_s \alpha L_{ijkj}^{V,RR} \\ &\quad + \frac{46}{81} \alpha^2 L_{ijkj}^{V,RR}; \end{aligned}$$

$$\begin{aligned} \dot{L}_{ijkj}^{V1,LR} &= -\frac{8}{3} g_s^2 L_{ijkj}^{V8,LR} - \frac{4}{3} e^2 L_{ijkj}^{V1,LR} + \alpha_s^2 \left[ -\frac{28}{3} L_{ijkj}^{V1,LR} - \frac{2044}{27} L_{ijkj}^{V8,LR} \right] \\ &\quad + \alpha_s \alpha \left[ \frac{32}{3} L_{ijkj}^{V1,LR} - \frac{8}{27} L_{ijkj}^{V8,LR} \right] + \frac{1790}{81} \alpha^2 L_{ijkj}^{V1,LR}; \end{aligned}$$

$$\dot{L}_{ijkj}^{V8,LR} = g_s^2 \left[ -12 L_{ijkj}^{V1,LR} - 14 L_{ijkj}^{V8,LR} \right] - \frac{4}{3} e^2 L_{ijkj}^{V8,LR} + \alpha_s^2 \left[ -\frac{374}{3} L_{ijkj}^{V1,LR} \right]$$

$$\begin{aligned}
& -\frac{2975}{18}L_{ijkj}^{V8,LR} \Big] + \alpha_s \alpha \left[ -\frac{4}{3}L_{ijkj}^{V1,LR} - \frac{26}{9}L_{ijkj}^{V8,LR} \right] + \frac{1790}{81}\alpha^2 L_{ijkj}^{V8,LR} ; \\
\dot{L}_{ijkj}^{S1,RR} &= g_s^2 \left[ \frac{160}{27}L_{ijkj}^{S8,RR} - \frac{80}{9}L_{ijkj}^{S1,RR} \right] + e^2 \left[ \frac{4}{27}L_{ijkj}^{S1,RR} + \frac{64}{81}L_{ijkj}^{S8,RR} \right] \\
& + \alpha_s^2 \left[ \frac{19360}{243}L_{ijkj}^{S8,RR} - \frac{9608}{81}L_{ijkj}^{S1,RR} \right] + \alpha_s \alpha \left[ \frac{352}{243}L_{ijkj}^{S8,RR} - \frac{1040}{81}L_{ijkj}^{S1,RR} \right] \\
& + \alpha^2 \left[ \frac{4634}{729}L_{ijkj}^{S1,RR} - \frac{3328}{2187}L_{ijkj}^{S8,RR} \right] ; \\
\dot{L}_{ijkj}^{S8,RR} &= g_s^2 \left[ \frac{8}{3}L_{ijkj}^{S1,RR} + \frac{92}{9}L_{ijkj}^{S8,RR} \right] + e^2 \left[ \frac{32}{9}L_{ijkj}^{S1,RR} - \frac{28}{27}L_{ijkj}^{S8,RR} \right] \\
& + \alpha_s^2 \left[ \frac{6479}{81}L_{ijkj}^{S8,RR} - \frac{112}{27}L_{ijkj}^{S1,RR} \right] + \alpha_s \alpha \left[ -\frac{1840}{27}L_{ijkj}^{S1,RR} - \frac{208}{81}L_{ijkj}^{S8,RR} \right] \\
& + \alpha^2 \left[ \frac{6298}{729}L_{ijkj}^{S8,RR} - \frac{1664}{243}L_{ijkj}^{S1,RR} \right] ; \\
\dot{L}_{jijk}^{V,LL} &= 4g_s^2 L_{jijk}^{V,LL} + \frac{4}{3}e^2 L_{jijk}^{V,LL} - \frac{43}{9}\alpha_s^2 L_{jijk}^{V,LL} - \frac{148}{9}\alpha_s \alpha L_{jijk}^{V,LL} \\
& + \frac{46}{81}\alpha^2 L_{jijk}^{V,LL} ; \\
\dot{L}_{jijk}^{V,RR} &= 4g_s^2 L_{jijk}^{V,RR} + \frac{4}{3}e^2 L_{jijk}^{V,RR} - \frac{43}{9}\alpha_s^2 L_{jijk}^{V,RR} - \frac{148}{9}\alpha_s \alpha L_{jijk}^{V,RR} \\
& + \frac{46}{81}\alpha^2 L_{jijk}^{V,RR} ; \\
\dot{L}_{jijk}^{V1,LR} &= -\frac{8}{3}g_s^2 L_{jijk}^{V8,LR} - \frac{4}{3}e^2 L_{jijk}^{V1,LR} + \alpha_s^2 \left[ -\frac{28}{3}L_{jijk}^{V1,LR} - \frac{2044}{27}L_{jijk}^{V8,LR} \right] \\
& + \alpha_s \alpha \left[ \frac{32}{3}L_{jijk}^{V1,LR} - \frac{8}{27}L_{jijk}^{V8,LR} \right] + \frac{1790}{81}\alpha^2 L_{jijk}^{V1,LR} ; \\
\dot{L}_{jijk}^{V8,LR} &= g_s^2 \left[ -12L_{jijk}^{V1,LR} - 14L_{jijk}^{V8,LR} \right] - \frac{4}{3}e^2 L_{jijk}^{V8,LR} + \alpha_s^2 \left[ -\frac{374}{3}L_{jijk}^{V1,LR} \right. \\
& \left. - \frac{2975}{18}L_{jijk}^{V8,LR} \right] + \alpha_s \alpha \left[ -\frac{4}{3}L_{jijk}^{V1,LR} - \frac{26}{9}L_{jijk}^{V8,LR} \right] + \frac{1790}{81}\alpha^2 L_{jijk}^{V8,LR} ;
\end{aligned}$$

$$\begin{aligned}
\dot{L}_{dd,jijk}^{S1,RR} &= g_s^2 \left[ \frac{160}{27} L_{dd,jijk}^{S8,RR} - \frac{80}{9} L_{dd,jijk}^{S1,RR} \right] + e^2 \left[ \frac{4}{27} L_{dd,jijk}^{S1,RR} + \frac{64}{81} L_{dd,jijk}^{S8,RR} \right] \\
&+ \alpha_s^2 \left[ \frac{19360}{243} L_{dd,jijk}^{S8,RR} - \frac{9608}{81} L_{dd,jijk}^{S1,RR} \right] + \alpha_s \alpha \left[ \frac{352}{243} L_{dd,jijk}^{S8,RR} - \frac{1040}{81} L_{dd,jijk}^{S1,RR} \right] \\
&+ \alpha^2 \left[ \frac{4634}{729} L_{dd,jijk}^{S1,RR} - \frac{3328}{2187} L_{dd,jijk}^{S8,RR} \right] ; \\
\dot{L}_{dd,jijk}^{S8,RR} &= g_s^2 \left[ \frac{8}{3} L_{dd,jijk}^{S1,RR} + \frac{92}{9} L_{dd,jijk}^{S8,RR} \right] + e^2 \left[ \frac{32}{9} L_{dd,jijk}^{S1,RR} - \frac{28}{27} L_{dd,jijk}^{S8,RR} \right] \\
&+ \alpha_s^2 \left[ \frac{6479}{81} L_{dd,jijk}^{S8,RR} - \frac{112}{27} L_{dd,jijk}^{S1,RR} \right] + \alpha_s \alpha \left[ -\frac{1840}{27} L_{dd,jijk}^{S1,RR} - \frac{208}{81} L_{dd,jijk}^{S8,RR} \right] \\
&+ \alpha^2 \left[ \frac{6298}{729} L_{dd,jijk}^{S8,RR} - \frac{1664}{243} L_{dd,jijk}^{S1,RR} \right] ;
\end{aligned}$$

### 1.2.2 $\Delta F = 1.5$ : $e$ -type ( $\bar{e}_i e_j \bar{e}_k e_j$ )

$$\begin{aligned}
\dot{L}_{ijkj}^{V,LL} &= 12e^2 L_{ijkj}^{V,LL} - \frac{866}{9} \alpha^2 L_{ijkj}^{V,LL} ; \\
\dot{L}_{ijkj}^{V,RR} &= 12e^2 L_{ijkj}^{V,RR} - \frac{866}{9} \alpha^2 L_{ijkj}^{V,RR} ; \\
\dot{L}_{ijkj}^{V,LR} &= \frac{2030}{9} \alpha^2 L_{ijkj}^{V,LR} - 12e^2 L_{ijkj}^{V,LR} ; \\
\dot{L}_{ijkj}^{S,RR} &= 12e^2 L_{ijkj}^{S,RR} - \frac{1058}{3} \alpha^2 L_{ijkj}^{S,RR} ; \\
\dot{L}_{jijk}^{V,LL} &= 12e^2 L_{jijk}^{V,LL} - \frac{866}{9} \alpha^2 L_{jijk}^{V,LL} ; \\
\dot{L}_{jijk}^{V,RR} &= 12e^2 L_{jijk}^{V,RR} - \frac{866}{9} \alpha^2 L_{jijk}^{V,RR} ; \\
\dot{L}_{jijk}^{V,LR} &= \frac{2030}{9} \alpha^2 L_{jijk}^{V,LR} - 12e^2 L_{jijk}^{V,LR} ; \\
\dot{L}_{jijk}^{S,RR} &= 12e^2 L_{jijk}^{S,RR} - \frac{1058}{3} \alpha^2 L_{jijk}^{S,RR} ;
\end{aligned}$$

### 1.2.3 $\Delta F = 2$ : $\nu$ -type ( $\bar{\nu}_i \nu_j \bar{\nu}_k \nu_j$ )

$$\dot{L}_{ijkj}^{V,LL} = 0 ;$$



$$\dot{L}_{j\bar{j}k}^{V,LL} = 0;$$

### 1.3 $\Delta F = 1$ Transitions ( $\bar{f}_i f_j \bar{f}'_k f'_l$ )

#### 1.3.1 $\Delta F = 1$ : $ud$ -type ( $\bar{u}_i u_j \bar{d}_k d_l$ )

$$\begin{aligned} \dot{L}_{j\bar{j}k}^{V1,LL} &= \frac{8}{3}g_s^2 L_{j\bar{j}k}^{V8,LL} - \frac{8}{3}e^2 L_{j\bar{j}k}^{V1,LL} + \alpha_s^2 \left[ \frac{82}{27} L_{j\bar{j}k}^{V8,LL} - \frac{28}{3} L_{j\bar{j}k}^{V1,LL} \right] \\ &\quad + \alpha_s \alpha \left[ \frac{64}{3} L_{j\bar{j}k}^{V1,LL} - \frac{8}{27} L_{j\bar{j}k}^{V8,LL} \right] - \frac{128}{81} \alpha^2 L_{j\bar{j}k}^{V1,LL}; \end{aligned}$$

$$\begin{aligned} \dot{L}_{j\bar{j}k}^{V8,LL} &= g_s^2 \left[ 12 L_{j\bar{j}k}^{V1,LL} - 4 L_{j\bar{j}k}^{V8,LL} \right] - \frac{8}{3}e^2 L_{j\bar{j}k}^{V8,LL} + \alpha_s^2 \left[ \frac{41}{3} L_{j\bar{j}k}^{V1,LL} \right. \\ &\quad \left. - \frac{125}{9} L_{j\bar{j}k}^{V8,LL} \right] + \alpha_s \alpha \left[ -\frac{4}{3} L_{j\bar{j}k}^{V1,LL} - \frac{47}{9} L_{j\bar{j}k}^{V8,LL} \right] - \frac{128}{81} \alpha^2 L_{j\bar{j}k}^{V8,LL}; \end{aligned}$$

$$\begin{aligned} \dot{L}_{j\bar{j}k}^{V1,RR} &= \frac{8}{3}g_s^2 L_{j\bar{j}k}^{V8,RR} - \frac{8}{3}e^2 L_{j\bar{j}k}^{V1,RR} + \alpha_s^2 \left[ \frac{82}{27} L_{j\bar{j}k}^{V8,RR} - \frac{28}{3} L_{j\bar{j}k}^{V1,RR} \right] \\ &\quad + \alpha_s \alpha \left[ \frac{64}{3} L_{j\bar{j}k}^{V1,RR} - \frac{8}{27} L_{j\bar{j}k}^{V8,RR} \right] - \frac{128}{81} \alpha^2 L_{j\bar{j}k}^{V1,RR}; \end{aligned}$$

$$\begin{aligned} \dot{L}_{j\bar{j}k}^{V8,RR} &= g_s^2 \left[ 12 L_{j\bar{j}k}^{V1,RR} - 4 L_{j\bar{j}k}^{V8,RR} \right] - \frac{8}{3}e^2 L_{j\bar{j}k}^{V8,RR} + \alpha_s^2 \left[ \frac{41}{3} L_{j\bar{j}k}^{V1,RR} \right. \\ &\quad \left. - \frac{125}{9} L_{j\bar{j}k}^{V8,RR} \right] + \alpha_s \alpha \left[ -\frac{4}{3} L_{j\bar{j}k}^{V1,RR} - \frac{47}{9} L_{j\bar{j}k}^{V8,RR} \right] - \frac{128}{81} \alpha^2 L_{j\bar{j}k}^{V8,RR}; \end{aligned}$$

$$\begin{aligned} \dot{L}_{j\bar{j}k}^{V1,LR} &= -\frac{8}{3}g_s^2 L_{j\bar{j}k}^{V8,LR} + \frac{8}{3}e^2 L_{j\bar{j}k}^{V1,LR} + \alpha_s^2 \left[ -\frac{28}{3} L_{j\bar{j}k}^{V1,LR} - \frac{2044}{27} L_{j\bar{j}k}^{V8,LR} \right] \\ &\quad + \alpha_s \alpha \left[ \frac{232}{27} L_{j\bar{j}k}^{V8,LR} - \frac{64}{3} L_{j\bar{j}k}^{V1,LR} \right] - \frac{4048}{81} \alpha^2 L_{j\bar{j}k}^{V1,LR}; \end{aligned}$$

$$\begin{aligned} \dot{L}_{j\bar{j}k}^{V8,LR} &= g_s^2 \left[ -12 L_{j\bar{j}k}^{V1,LR} - 14 L_{j\bar{j}k}^{V8,LR} \right] + \frac{8}{3}e^2 L_{j\bar{j}k}^{V8,LR} + \alpha_s^2 \left[ -\frac{374}{3} L_{j\bar{j}k}^{V1,LR} \right. \\ &\quad \left. - \frac{2975}{18} L_{j\bar{j}k}^{V8,LR} \right] + \alpha_s \alpha \left[ \frac{116}{3} L_{j\bar{j}k}^{V1,LR} + \frac{187}{9} L_{j\bar{j}k}^{V8,LR} \right] - \frac{4048}{81} \alpha^2 L_{j\bar{j}k}^{V8,LR}; \end{aligned}$$

$$\begin{aligned}
\dot{L}_{klij}^{V1,LR} &= -\frac{8}{3}g_s^2 L_{klij}^{V8,LR} + \frac{8}{3}e^2 L_{klij}^{V1,LR} + \alpha_s^2 \left[ -\frac{28}{3} L_{klij}^{V1,LR} - \frac{2044}{27} L_{klij}^{V8,LR} \right] \\
&\quad + \alpha_s \alpha \left[ \frac{232}{27} L_{klij}^{V8,LR} - \frac{64}{3} L_{klij}^{V1,LR} \right] - \frac{4048}{81} \alpha^2 L_{klij}^{V1,LR} ; \\
\dot{L}_{klij}^{V8,LR} &= g_s^2 \left[ -12 L_{klij}^{V1,LR} - 14 L_{klij}^{V8,LR} \right] + \frac{8}{3}e^2 L_{klij}^{V8,LR} + \alpha_s^2 \left[ -\frac{374}{3} L_{klij}^{V1,LR} \right. \\
&\quad \left. - \frac{2975}{18} L_{klij}^{V8,LR} \right] + \alpha_s \alpha \left[ \frac{116}{3} L_{klij}^{V1,LR} + \frac{187}{9} L_{klij}^{V8,LR} \right] - \frac{4048}{81} \alpha^2 L_{klij}^{V8,LR} ; \\
\dot{L}_{il kj}^{V1,LR} &= -\frac{8}{3}g_s^2 L_{il kj}^{V8,LR} - \frac{10}{3}e^2 L_{il kj}^{V1,LR} + \alpha_s^2 \left[ -\frac{28}{3} L_{il kj}^{V1,LR} - \frac{2044}{27} L_{il kj}^{V8,LR} \right] \\
&\quad + \alpha_s \alpha \left[ \frac{8}{3} L_{il kj}^{V1,LR} - \frac{128}{27} L_{il kj}^{V8,LR} \right] + \frac{173}{81} \alpha^2 L_{il kj}^{V1,LR} ; \\
\dot{L}_{il kj}^{V8,LR} &= g_s^2 \left[ -12 L_{il kj}^{V1,LR} - 14 L_{il kj}^{V8,LR} \right] - \frac{10}{3}e^2 L_{il kj}^{V8,LR} + \alpha_s^2 \left[ -\frac{374}{3} L_{il kj}^{V1,LR} \right. \\
&\quad \left. - \frac{2975}{18} L_{il kj}^{V8,LR} \right] + \alpha_s \alpha \left[ \frac{16}{9} L_{il kj}^{V8,LR} - \frac{64}{3} L_{il kj}^{V1,LR} \right] + \frac{173}{81} \alpha^2 L_{il kj}^{V8,LR} ; \\
\dot{L}_{ijkl}^{S1,RR} &= g_s^2 \left[ \frac{64}{9} L_{ijkl}^{S1,RR} + \frac{112}{27} L_{ijkl}^{S8,RR} - 16 L_{ijkl}^{S1,RR} + \frac{16}{9} L_{ijkl}^{S8,RR} \right] \\
&\quad + e^2 \left[ \frac{4}{27} L_{ijkl}^{S1,RR} + \frac{16}{81} L_{ijkl}^{S8,RR} - \frac{46}{9} L_{ijkl}^{S1,RR} \right] + \alpha_s^2 \left[ \frac{9472}{81} L_{ijkl}^{S1,RR} + \frac{16576}{243} L_{ijkl}^{S8,RR} \right. \\
&\quad \left. - \frac{2120}{9} L_{ijkl}^{S1,RR} + \frac{928}{81} L_{ijkl}^{S8,RR} \right] + \alpha_s \alpha \left[ \frac{1888}{81} L_{ijkl}^{S1,RR} + \frac{3808}{243} L_{ijkl}^{S8,RR} + \frac{136}{27} L_{ijkl}^{S1,RR} \right. \\
&\quad \left. + \frac{224}{81} L_{ijkl}^{S8,RR} \right] + \alpha^2 \left[ \frac{98}{729} L_{ijkl}^{S1,RR} + \frac{392}{2187} L_{ijkl}^{S8,RR} + \frac{6391}{243} L_{ijkl}^{S1,RR} \right] ; \\
\dot{L}_{ijkl}^{S8,RR} &= g_s^2 \left[ -\frac{16}{3} L_{ijkl}^{S1,RR} + \frac{44}{9} L_{ijkl}^{S8,RR} + 8 L_{ijkl}^{S1,RR} + \frac{16}{3} L_{ijkl}^{S8,RR} \right] \\
&\quad + e^2 \left[ \frac{8}{9} L_{ijkl}^{S1,RR} - \frac{4}{27} L_{ijkl}^{S8,RR} - \frac{46}{9} L_{ijkl}^{S8,RR} \right] + \alpha_s^2 \left[ -\frac{856}{27} L_{ijkl}^{S1,RR} - \frac{2506}{81} L_{ijkl}^{S8,RR} \right]
\end{aligned}$$

$$\begin{aligned}
& + \frac{248}{9} L_{ijkl}^{S1,RR} + \frac{2995}{27} L_{ijkl}^{S8,RR} \Big] + \alpha_s \alpha \Big[ - \frac{868}{27} L_{uddu}^{S1,RR} + \frac{1370}{81} L_{uddu}^{S8,RR} + \frac{112}{9} L_{ijkl}^{S1,RR} \\
& + \frac{224}{9} L_{ijkl}^{S8,RR} \Big] + \alpha^2 \Big[ \frac{196}{243} L_{uddu}^{S1,RR} - \frac{98}{729} L_{uddu}^{S8,RR} + \frac{6391}{243} L_{ijkl}^{S8,RR} \Big] ; \\
\dot{L}_{uddu}^{S1,RR} & = g_s^2 \Big[ -16 L_{uddu}^{S1,RR} + \frac{16}{9} L_{uddu}^{S8,RR} + \frac{64}{9} L_{ijkl}^{S1,RR} + \frac{112}{27} L_{ijkl}^{S8,RR} \Big] \\
& + e^2 \Big[ \frac{26}{9} L_{uddu}^{S1,RR} - \frac{32}{27} L_{ijkl}^{S1,RR} - \frac{128}{81} L_{ijkl}^{S8,RR} \Big] + \alpha_s^2 \Big[ - \frac{2120}{9} L_{uddu}^{S1,RR} + \frac{928}{81} L_{uddu}^{S8,RR} \\
& + \frac{9472}{81} L_{ijkl}^{S1,RR} + \frac{16576}{243} L_{ijkl}^{S8,RR} \Big] + \alpha_s \alpha \Big[ \frac{712}{27} L_{uddu}^{S1,RR} - \frac{64}{81} L_{uddu}^{S8,RR} - \frac{2144}{81} L_{ijkl}^{S1,RR} \\
& - \frac{7784}{243} L_{ijkl}^{S8,RR} \Big] + \alpha^2 \Big[ - \frac{13769}{243} L_{uddu}^{S1,RR} + \frac{5264}{729} L_{ijkl}^{S1,RR} + \frac{21056}{2187} L_{ijkl}^{S8,RR} \Big] ; \\
\dot{L}_{uddu}^{S8,RR} & = g_s^2 \Big[ 8 L_{uddu}^{S1,RR} + \frac{16}{3} L_{uddu}^{S8,RR} - \frac{16}{3} L_{ijkl}^{S1,RR} + \frac{44}{9} L_{ijkl}^{S8,RR} \Big] \\
& + e^2 \Big[ \frac{26}{9} L_{uddu}^{S8,RR} - \frac{64}{9} L_{ijkl}^{S1,RR} + \frac{32}{27} L_{ijkl}^{S8,RR} \Big] + \alpha_s^2 \Big[ \frac{248}{9} L_{uddu}^{S1,RR} + \frac{2995}{27} L_{uddu}^{S8,RR} \\
& - \frac{856}{27} L_{ijkl}^{S1,RR} - \frac{2506}{81} L_{ijkl}^{S8,RR} \Big] + \alpha_s \alpha \Big[ - \frac{32}{9} L_{uddu}^{S1,RR} - \frac{400}{9} L_{uddu}^{S8,RR} + \frac{3704}{27} L_{ijkl}^{S1,RR} \\
& - \frac{2050}{81} L_{ijkl}^{S8,RR} \Big] + \alpha^2 \Big[ - \frac{13769}{243} L_{uddu}^{S8,RR} + \frac{10528}{243} L_{ijkl}^{S1,RR} - \frac{5264}{729} L_{ijkl}^{S8,RR} \Big] ;
\end{aligned}$$

### 1.3.2 $\Delta F = 1 : ed\text{-type } (\bar{e}_i e_j \bar{d}_k d_l)$

$$\begin{aligned}
\dot{L}_{ijkl}^{V,LL} & = 4e^2 L_{ijkl}^{V,LL} - 16\alpha_s \alpha L_{ijkl}^{V,LL} - \frac{326}{27} \alpha^2 L_{ijkl}^{V,LL} ; \\
\dot{L}_{ijkl}^{V,RR} & = 4e^2 L_{ijkl}^{V,RR} - 16\alpha_s \alpha L_{ijkl}^{V,RR} - \frac{326}{27} \alpha^2 L_{ijkl}^{V,RR} ; \\
\dot{L}_{ijkl}^{V,LR} & = -4e^2 L_{ijkl}^{V,LR} + 16\alpha_s \alpha L_{ijkl}^{V,LR} + \frac{1994}{27} \alpha^2 L_{ijkl}^{V,LR} ; \\
\dot{L}_{kl ij}^{V,LR} & = -4e^2 L_{kl ij}^{V,LR} + 16\alpha_s \alpha L_{kl ij}^{V,LR} + \frac{1994}{27} \alpha^2 L_{kl ij}^{V,LR} ;
\end{aligned}$$

$$\begin{aligned}
\dot{L}_{ed\,ijkl}^{S,RL} &= -8g_s^2 L_{ed\,ijkl}^{S,RL} - \frac{20}{3} e^2 L_{ed\,ijkl}^{S,RL} - \frac{1012}{9} \alpha_s^2 L_{ed\,ijkl}^{S,RL} - \frac{8}{9} \alpha_s \alpha L_{ed\,ijkl}^{S,RL} \\
&\quad + \frac{6958}{81} \alpha^2 L_{ed\,ijkl}^{S,RL} ; \\
\dot{L}_{ed\,ijkl}^{S,RR} &= -8g_s^2 L_{ed\,ijkl}^{S,RR} + e^2 \left[ -\frac{20}{3} L_{ed\,ijkl}^{S,RR} - 32 L_{ed\,ijkl}^{T,RR} \right] - \frac{1012}{9} \alpha_s^2 L_{ed\,ijkl}^{S,RR} \\
&\quad + \alpha_s \alpha \left[ \frac{1792}{9} L_{ed\,ijkl}^{T,RR} - \frac{8}{9} L_{ed\,ijkl}^{S,RR} \right] + \alpha^2 \left[ \frac{1882}{81} L_{ed\,ijkl}^{S,RR} + \frac{19712}{27} L_{ed\,ijkl}^{T,RR} \right] ; \\
\dot{L}_{ed\,ijkl}^{T,RR} &= \frac{8}{3} g_s^2 L_{ed\,ijkl}^{T,RR} + e^2 \left[ \frac{20}{9} L_{ed\,ijkl}^{T,RR} - \frac{2}{3} L_{ed\,ijkl}^{S,RR} \right] + \frac{1652}{27} \alpha_s^2 L_{ed\,ijkl}^{T,RR} \\
&\quad + \alpha_s \alpha \left[ \frac{16}{3} L_{ed\,ijkl}^{S,RR} - \frac{152}{27} L_{ed\,ijkl}^{T,RR} \right] + \alpha^2 \left[ \frac{368}{81} L_{ed\,ijkl}^{S,RR} - \frac{7154}{243} L_{ed\,ijkl}^{T,RR} \right] ;
\end{aligned}$$

### 1.3.3 $\Delta F = 1$ : $eu$ -type ( $\bar{e}_i e_j \bar{u}_k u_l$ )

$$\begin{aligned}
\dot{L}_{eu\,ijkl}^{V,LL} &= -8e^2 L_{eu\,ijkl}^{V,LL} + 32\alpha_s \alpha L_{eu\,ijkl}^{V,LL} + \frac{112}{27} \alpha^2 L_{eu\,ijkl}^{V,LL} ; \\
\dot{L}_{eu\,ijkl}^{V,RR} &= -8e^2 L_{eu\,ijkl}^{V,RR} + 32\alpha_s \alpha L_{eu\,ijkl}^{V,RR} + \frac{112}{27} \alpha^2 L_{eu\,ijkl}^{V,RR} ; \\
\dot{L}_{eu\,ijkl}^{V,LR} &= 8e^2 L_{eu\,ijkl}^{V,LR} - 32\alpha_s \alpha L_{eu\,ijkl}^{V,LR} - \frac{4960}{27} \alpha^2 L_{eu\,ijkl}^{V,LR} ; \\
\dot{L}_{ue\,kl ij}^{V,LR} &= 8e^2 L_{ue\,kl ij}^{V,LR} - 32\alpha_s \alpha L_{ue\,kl ij}^{V,LR} - \frac{4960}{27} \alpha^2 L_{ue\,kl ij}^{V,LR} ; \\
\dot{L}_{eu\,ijkl}^{S,RL} &= -8g_s^2 L_{eu\,ijkl}^{S,RL} - \frac{26}{3} e^2 L_{eu\,ijkl}^{S,RL} - \frac{1012}{9} \alpha_s^2 L_{eu\,ijkl}^{S,RL} - \frac{32}{9} \alpha_s \alpha L_{eu\,ijkl}^{S,RL} \\
&\quad + \frac{445}{81} \alpha^2 L_{eu\,ijkl}^{S,RL} ; \\
\dot{L}_{eu\,ijkl}^{S,RR} &= -8g_s^2 L_{eu\,ijkl}^{S,RR} + e^2 \left[ 64 L_{eu\,ijkl}^{T,RR} - \frac{26}{3} L_{eu\,ijkl}^{S,RR} \right] - \frac{1012}{9} \alpha_s^2 L_{eu\,ijkl}^{S,RR} \\
&\quad + \alpha_s \alpha \left[ -\frac{32}{9} L_{eu\,ijkl}^{S,RR} - \frac{3584}{9} L_{eu\,ijkl}^{T,RR} \right] + \alpha^2 \left[ -\frac{2579}{81} L_{eu\,ijkl}^{S,RR} - \frac{35200}{27} L_{eu\,ijkl}^{T,RR} \right] ; \\
\dot{L}_{eu\,ijkl}^{T,RR} &= \frac{8}{3} g_s^2 L_{eu\,ijkl}^{T,RR} + e^2 \left[ \frac{4}{3} L_{eu\,ijkl}^{S,RR} + \frac{26}{9} L_{eu\,ijkl}^{T,RR} \right] + \frac{1652}{27} \alpha_s^2 L_{eu\,ijkl}^{T,RR}
\end{aligned}$$

$$+ \alpha_s \alpha \left[ -\frac{32}{3} L_{ijkl}^{S,RR} - \frac{608}{27} L_{ijkl}^{T,RR} \right] + \alpha^2 \left[ -\frac{1384}{81} L_{ijkl}^{S,RR} - \frac{21929}{243} L_{ijkl}^{T,RR} \right];$$

### 1.3.4 $\Delta F = 1 : \nu d\text{-type } (\bar{\nu}_i \nu_j \bar{d}_k d_l)$

$$\dot{L}_{\nu d,ijkl}^{V,LL} = 0;$$

$$\dot{L}_{\nu d,ijkl}^{V,LR} = 0;$$

### 1.3.5 $\Delta F = 1 : \nu u\text{-type } (\bar{\nu}_i \nu_j \bar{u}_k u_l)$

$$\dot{L}_{\nu u,ijkl}^{V,LL} = 0;$$

$$\dot{L}_{\nu u,ijkl}^{V,LR} = 0;$$

### 1.3.6 $\Delta F = 1 : \nu e\text{-type } (\bar{\nu}_i \nu_j \bar{e}_k e_l)$

$$\dot{L}_{\nu e,ijkl}^{V,LL} = 0;$$

$$\dot{L}_{\nu e,ijkl}^{V,LR} = 0;$$

### 1.3.7 $\Delta F = 1 : \nu edu\text{-type } (\bar{\nu}_i e_j \bar{d}_k u_l)$

$$\dot{L}_{\nu edu,ijkl}^{V,LL} = -4e^2 L_{\nu edu,ijkl}^{V,LL} + 4\alpha_s \alpha L_{\nu edu,ijkl}^{V,LL} - \frac{160}{27} \alpha^2 L_{\nu edu,ijkl}^{V,LL};$$

$$\dot{L}_{\nu edu,ijkl}^{V,LR} = -2e^2 L_{\nu edu,ijkl}^{V,LR} - 4\alpha_s \alpha L_{\nu edu,ijkl}^{V,LR} - \frac{497}{27} \alpha^2 L_{\nu edu,ijkl}^{V,LR};$$

$$\begin{aligned} \dot{L}_{\nu edu,ijkl}^{S,RL} = & -8g_s^2 L_{\nu edu,ijkl}^{S,RL} + \frac{4}{3} e^2 L_{\nu edu,ijkl}^{S,RL} - \frac{1012}{9} \alpha_s^2 L_{\nu edu,ijkl}^{S,RL} + 12\alpha_s \alpha L_{\nu edu,ijkl}^{S,RL} \\ & - \frac{4016}{81} \alpha^2 L_{\nu edu,ijkl}^{S,RL}; \end{aligned}$$

$$\begin{aligned} \dot{L}_{\nu edu,ijkl}^{S,RR} = & -8g_s^2 L_{\nu edu,ijkl}^{S,RR} + e^2 \left[ \frac{4}{3} L_{\nu edu,ijkl}^{S,RR} + 8 L_{\nu edu,ijkl}^{T,RR} \right] - \frac{1012}{9} \alpha_s^2 L_{\nu edu,ijkl}^{S,RR} \\ & + \alpha_s \alpha \left[ 12 L_{\nu edu,ijkl}^{S,RR} - \frac{448}{9} L_{\nu edu,ijkl}^{T,RR} \right] + \alpha^2 \left[ -\frac{3953}{81} L_{\nu edu,ijkl}^{S,RR} - \frac{3368}{27} L_{\nu edu,ijkl}^{T,RR} \right]; \end{aligned}$$

$$\begin{aligned}\dot{L}_{\nu edu}^{T,RR}{}_{ijkl} &= \frac{8}{3}g_s^2 L_{\nu edu}^{T,RR}{}_{ijkl} + e^2 \left[ \frac{1}{6} L_{\nu edu}^{S,RR}{}_{ijkl} - \frac{40}{9} L_{\nu edu}^{T,RR}{}_{ijkl} \right] + \frac{1652}{27} \alpha_s^2 L_{\nu edu}^{T,RR}{}_{ijkl} \\ &\quad + \alpha_s \alpha \left[ \frac{4}{3} L_{\nu edu}^{T,RR}{}_{ijkl} - \frac{4}{3} L_{\nu edu}^{S,RR}{}_{ijkl} \right] + \alpha^2 \left[ \frac{3985}{243} L_{\nu edu}^{T,RR}{}_{ijkl} - \frac{13}{162} L_{\nu edu}^{S,RR}{}_{ijkl} \right];\end{aligned}$$

#### 1.4 $\Delta F = 1^{\bar{f}f}$ Transitions ( $\bar{f}_i f_j \bar{f}'_k f'_k$ )

#### 1.5 $\Delta F = 1^{\bar{f}f} : d\text{-type}$ ( $\bar{d}_i d_j \bar{f}_k f_k$ )

$$\begin{aligned}\dot{L}_{ed}^{V,LL}{}_{11ij} &= e^2 \left[ \frac{4}{3} L_{dd}^{V1,LR}{}_{ijkk} + \frac{8}{3} L_{dd}^{V,LL}{}_{ijkk} + \frac{8}{9} L_{dd}^{V,LL}{}_{ikkj} + \frac{4}{3} L_{dd}^{V1,LR}{}_{ijii} + \frac{4}{3} L_{dd}^{V1,LR}{}_{ijjj} \right. \\ &\quad + \frac{32}{9} L_{dd}^{V,LL}{}_{ijii} + \frac{32}{9} L_{dd}^{V,LL}{}_{ijjj} + \frac{4}{3} L_{de}^{V,LR}{}_{ij11} + \frac{4}{3} L_{de}^{V,LR}{}_{ij22} + \frac{4}{3} L_{de}^{V,LR}{}_{ij33} - \frac{8}{3} L_{du}^{V1,LR}{}_{ij11} \\ &\quad - \frac{8}{3} L_{du}^{V1,LR}{}_{ij22} + \frac{16}{3} L_{ed}^{V,LL}{}_{11ij} + \frac{4}{3} L_{ed}^{V,LL}{}_{22ij} + \frac{4}{3} L_{ed}^{V,LL}{}_{33ij} - \frac{8}{3} L_{ud}^{V1,LL}{}_{11ij} - \frac{8}{3} L_{ud}^{V1,LL}{}_{22ij} \left. \right] \\ &\quad + \alpha_s \alpha \left[ \frac{16}{3} L_{dd}^{V1,LR}{}_{ijkk} - \frac{1010}{243} L_{dd}^{V8,LR}{}_{ijkk} + 8 L_{dd}^{V,LL}{}_{ijkk} + \frac{304}{243} L_{dd}^{V,LL}{}_{ikkj} + \frac{16}{3} L_{dd}^{V1,LR}{}_{ijii} \right. \\ &\quad + \frac{16}{3} L_{dd}^{V1,LR}{}_{ijjj} - \frac{1010}{243} L_{dd}^{V8,LR}{}_{ijii} - \frac{1010}{243} L_{dd}^{V8,LR}{}_{ijjj} + \frac{1096}{81} L_{dd}^{V,LL}{}_{ijii} + \frac{1096}{81} L_{dd}^{V,LL}{}_{ijjj} \\ &\quad - \frac{32}{3} L_{du}^{V1,LR}{}_{ij11} - \frac{32}{3} L_{du}^{V1,LR}{}_{ij22} + \frac{1366}{243} L_{du}^{V8,LR}{}_{ij11} + \frac{1366}{243} L_{du}^{V8,LR}{}_{ij22} - 16 L_{ed}^{V,LL}{}_{11ij} - \frac{32}{3} L_{ud}^{V1,LL}{}_{11ij} \\ &\quad - \frac{32}{3} L_{ud}^{V1,LL}{}_{22ij} - \frac{74}{243} L_{ud}^{V8,LL}{}_{11ij} - \frac{74}{243} L_{ud}^{V8,LL}{}_{22ij} \left. \right] + \alpha^2 \left[ -\frac{1288}{243} L_{dd}^{V1,LR}{}_{ijkk} + \frac{2032}{243} L_{dd}^{V,LL}{}_{ijkk} \right. \\ &\quad + \frac{2992}{729} L_{dd}^{V,LL}{}_{ikkj} - \frac{1288}{243} L_{dd}^{V1,LR}{}_{ijii} - \frac{1288}{243} L_{dd}^{V1,LR}{}_{ijjj} + \frac{4864}{243} L_{dd}^{V,LL}{}_{ijii} + \frac{4864}{243} L_{dd}^{V,LL}{}_{ijjj} \\ &\quad - \frac{3160}{243} L_{de}^{V,LR}{}_{ij11} - \frac{3160}{243} L_{de}^{V,LR}{}_{ij22} - \frac{3160}{243} L_{de}^{V,LR}{}_{ij33} - \frac{6280}{243} L_{du}^{V1,LR}{}_{ij11} - \frac{6280}{243} L_{du}^{V1,LR}{}_{ij22} \\ &\quad + \frac{818}{243} L_{ed}^{V,LL}{}_{11ij} + \frac{3752}{243} L_{ed}^{V,LL}{}_{22ij} + \frac{3752}{243} L_{ed}^{V,LL}{}_{33ij} + \frac{2936}{243} L_{ud}^{V1,LL}{}_{11ij} + \frac{2936}{243} L_{ud}^{V1,LL}{}_{22ij} \left. \right];\end{aligned}$$

$$\begin{aligned}\dot{L}_{ed}^{V,LL}{}_{22ij} &= e^2 \left[ \frac{4}{3} L_{dd}^{V1,LR}{}_{ijkk} + \frac{8}{3} L_{dd}^{V,LL}{}_{ijkk} + \frac{8}{9} L_{dd}^{V,LL}{}_{ikkj} + \frac{4}{3} L_{dd}^{V1,LR}{}_{ijii} + \frac{4}{3} L_{dd}^{V1,LR}{}_{ijjj} \right. \\ &\quad + \frac{32}{9} L_{dd}^{V,LL}{}_{ijii} + \frac{32}{9} L_{dd}^{V,LL}{}_{ijjj} + \frac{4}{3} L_{de}^{V,LR}{}_{ij11} + \frac{4}{3} L_{de}^{V,LR}{}_{ij22} + \frac{4}{3} L_{de}^{V,LR}{}_{ij33} - \frac{8}{3} L_{du}^{V1,LR}{}_{ij11} \\ &\quad - \frac{8}{3} L_{du}^{V1,LR}{}_{ij22} + \frac{16}{3} L_{ed}^{V,LL}{}_{11ij} + \frac{4}{3} L_{ed}^{V,LL}{}_{22ij} + \frac{4}{3} L_{ed}^{V,LL}{}_{33ij} - \frac{8}{3} L_{ud}^{V1,LL}{}_{11ij} - \frac{8}{3} L_{ud}^{V1,LL}{}_{22ij} \left. \right] \\ &\quad + \alpha_s \alpha \left[ \frac{16}{3} L_{dd}^{V1,LR}{}_{ijkk} - \frac{1010}{243} L_{dd}^{V8,LR}{}_{ijkk} + 8 L_{dd}^{V,LL}{}_{ijkk} + \frac{304}{243} L_{dd}^{V,LL}{}_{ikkj} + \frac{16}{3} L_{dd}^{V1,LR}{}_{ijii} \right. \\ &\quad + \frac{16}{3} L_{dd}^{V1,LR}{}_{ijjj} - \frac{1010}{243} L_{dd}^{V8,LR}{}_{ijii} - \frac{1010}{243} L_{dd}^{V8,LR}{}_{ijjj} + \frac{1096}{81} L_{dd}^{V,LL}{}_{ijii} + \frac{1096}{81} L_{dd}^{V,LL}{}_{ijjj} \\ &\quad - \frac{32}{3} L_{du}^{V1,LR}{}_{ij11} - \frac{32}{3} L_{du}^{V1,LR}{}_{ij22} + \frac{1366}{243} L_{du}^{V8,LR}{}_{ij11} + \frac{1366}{243} L_{du}^{V8,LR}{}_{ij22} - 16 L_{ed}^{V,LL}{}_{11ij} - \frac{32}{3} L_{ud}^{V1,LL}{}_{11ij} \\ &\quad - \frac{32}{3} L_{ud}^{V1,LL}{}_{22ij} - \frac{74}{243} L_{ud}^{V8,LL}{}_{11ij} - \frac{74}{243} L_{ud}^{V8,LL}{}_{22ij} \left. \right] + \alpha^2 \left[ -\frac{1288}{243} L_{dd}^{V1,LR}{}_{ijkk} + \frac{2032}{243} L_{dd}^{V,LL}{}_{ijkk} \right. \\ &\quad + \frac{2992}{729} L_{dd}^{V,LL}{}_{ikkj} - \frac{1288}{243} L_{dd}^{V1,LR}{}_{ijii} - \frac{1288}{243} L_{dd}^{V1,LR}{}_{ijjj} + \frac{4864}{243} L_{dd}^{V,LL}{}_{ijii} + \frac{4864}{243} L_{dd}^{V,LL}{}_{ijjj} \\ &\quad - \frac{3160}{243} L_{de}^{V,LR}{}_{ij11} - \frac{3160}{243} L_{de}^{V,LR}{}_{ij22} - \frac{3160}{243} L_{de}^{V,LR}{}_{ij33} - \frac{6280}{243} L_{du}^{V1,LR}{}_{ij11} - \frac{6280}{243} L_{du}^{V1,LR}{}_{ij22} \\ &\quad + \frac{818}{243} L_{ed}^{V,LL}{}_{11ij} + \frac{3752}{243} L_{ed}^{V,LL}{}_{22ij} + \frac{3752}{243} L_{ed}^{V,LL}{}_{33ij} + \frac{2936}{243} L_{ud}^{V1,LL}{}_{11ij} + \frac{2936}{243} L_{ud}^{V1,LL}{}_{22ij} \left. \right];\end{aligned}$$

$$\begin{aligned}
& -\frac{8}{3}L_{ij22}^{V1,LR} + \frac{4}{3}L_{11ij}^{V,LL} + \frac{16}{3}L_{22ij}^{V,LL} + \frac{4}{3}L_{33ij}^{V,LL} - \frac{8}{3}L_{11ij}^{V1,LL} - \frac{8}{3}L_{22ij}^{V1,LL} \Big] \\
& + \alpha_s \alpha \left[ \frac{16}{3}L_{ijkk}^{V1,LR} - \frac{1010}{243}L_{ijkk}^{V8,LR} + 8L_{ijkk}^{V,LL} + \frac{304}{243}L_{ikkj}^{V,LL} + \frac{16}{3}L_{ijii}^{V1,LR} \right. \\
& + \frac{16}{3}L_{ijjj}^{V1,LR} - \frac{1010}{243}L_{ijii}^{V8,LR} - \frac{1010}{243}L_{ijjj}^{V8,LR} + \frac{1096}{81}L_{ijii}^{V,LL} + \frac{1096}{81}L_{ijjj}^{V,LL} \\
& - \frac{32}{3}L_{ij11}^{V1,LR} - \frac{32}{3}L_{ij22}^{V1,LR} + \frac{1366}{243}L_{ij11}^{V8,LR} + \frac{1366}{243}L_{ij22}^{V8,LR} - 16L_{22ij}^{V,LL} - \frac{32}{3}L_{11ij}^{V1,LL} \\
& - \frac{32}{3}L_{22ij}^{V1,LL} - \frac{74}{243}L_{11ij}^{V8,LL} - \frac{74}{243}L_{22ij}^{V8,LL} \Big] + \alpha^2 \left[ -\frac{1288}{243}L_{ijkk}^{V1,LR} + \frac{2032}{243}L_{ijkk}^{V,LL} \right. \\
& + \frac{2992}{729}L_{ikkj}^{V,LL} - \frac{1288}{243}L_{ijii}^{V1,LR} - \frac{1288}{243}L_{ijjj}^{V1,LR} + \frac{4864}{243}L_{ijii}^{V,LL} + \frac{4864}{243}L_{ijjj}^{V,LL} \\
& - \frac{3160}{243}L_{ij11}^{V,LR} - \frac{3160}{243}L_{ij22}^{V,LR} - \frac{3160}{243}L_{ij33}^{V,LR} - \frac{6280}{243}L_{ij11}^{V1,LR} - \frac{6280}{243}L_{ij22}^{V1,LR} \\
& \left. + \frac{3752}{243}L_{11ij}^{V,LL} + \frac{818}{243}L_{22ij}^{V,LL} + \frac{3752}{243}L_{33ij}^{V,LL} + \frac{2936}{243}L_{11ij}^{V1,LL} + \frac{2936}{243}L_{22ij}^{V1,LL} \right] ;
\end{aligned}$$

$$\begin{aligned}
\dot{L}_{ed33ij}^{V,LL} & = e^2 \left[ \frac{4}{3}L_{ijkk}^{V1,LR} + \frac{8}{3}L_{ijkk}^{V,LL} + \frac{8}{9}L_{ikkj}^{V,LL} + \frac{4}{3}L_{ijii}^{V1,LR} + \frac{4}{3}L_{ijjj}^{V1,LR} \right. \\
& + \frac{32}{9}L_{ijii}^{V,LL} + \frac{32}{9}L_{ijjj}^{V,LL} + \frac{4}{3}L_{ij11}^{V,LR} + \frac{4}{3}L_{ij22}^{V,LR} + \frac{4}{3}L_{ij33}^{V,LR} - \frac{8}{3}L_{ij11}^{V1,LR} \\
& - \frac{8}{3}L_{ij22}^{V1,LR} + \frac{4}{3}L_{11ij}^{V,LL} + \frac{4}{3}L_{22ij}^{V,LL} + \frac{16}{3}L_{33ij}^{V,LL} - \frac{8}{3}L_{11ij}^{V1,LL} - \frac{8}{3}L_{22ij}^{V1,LL} \Big] \\
& + \alpha_s \alpha \left[ \frac{16}{3}L_{ijkk}^{V1,LR} - \frac{1010}{243}L_{ijkk}^{V8,LR} + 8L_{ijkk}^{V,LL} + \frac{304}{243}L_{ikkj}^{V,LL} + \frac{16}{3}L_{ijii}^{V1,LR} \right. \\
& + \frac{16}{3}L_{ijjj}^{V1,LR} - \frac{1010}{243}L_{ijii}^{V8,LR} - \frac{1010}{243}L_{ijjj}^{V8,LR} + \frac{1096}{81}L_{ijii}^{V,LL} + \frac{1096}{81}L_{ijjj}^{V,LL} \\
& - \frac{32}{3}L_{ij11}^{V1,LR} - \frac{32}{3}L_{ij22}^{V1,LR} + \frac{1366}{243}L_{ij11}^{V8,LR} + \frac{1366}{243}L_{ij22}^{V8,LR} - 16L_{33ij}^{V,LL} - \frac{32}{3}L_{11ij}^{V1,LL} \\
& - \frac{32}{3}L_{22ij}^{V1,LL} - \frac{74}{243}L_{11ij}^{V8,LL} - \frac{74}{243}L_{22ij}^{V8,LL} \Big] + \alpha^2 \left[ -\frac{1288}{243}L_{ijkk}^{V1,LR} + \frac{2032}{243}L_{ijkk}^{V,LL} \right. \\
& + \frac{2992}{729}L_{ikkj}^{V,LL} - \frac{1288}{243}L_{ijii}^{V1,LR} - \frac{1288}{243}L_{ijjj}^{V1,LR} + \frac{4864}{243}L_{ijii}^{V,LL} + \frac{4864}{243}L_{ijjj}^{V,LL}
\end{aligned}$$

$$\begin{aligned}
& -\frac{3160}{243}L_{ij11}^{V,LR} - \frac{3160}{243}L_{ij22}^{V,LR} - \frac{3160}{243}L_{ij33}^{V,LR} - \frac{6280}{243}L_{ij11}^{V1,LR} - \frac{6280}{243}L_{ij22}^{V1,LR} \\
& + \frac{3752}{243}L_{11ij}^{V,LL} + \frac{3752}{243}L_{22ij}^{V,LL} + \frac{818}{243}L_{33ij}^{V,LL} + \frac{2936}{243}L_{11ij}^{V1,LL} + \frac{2936}{243}L_{22ij}^{V1,LL} \Bigg]; \\
\dot{L}_{11ij}^{V1,LL} &= \frac{8}{3}g_s^2 L_{11ij}^{V8,LL} + e^2 \Bigg[ -\frac{8}{9}L_{ijkk}^{V1,LR} - \frac{16}{9}L_{ijkk}^{V,LL} - \frac{16}{27}L_{ikkj}^{V,LL} - \frac{8}{9}L_{ijii}^{V1,LR} \\
& - \frac{8}{9}L_{ijjj}^{V1,LR} - \frac{64}{27}L_{ijii}^{V,LL} - \frac{64}{27}L_{ijjj}^{V,LL} - \frac{8}{9}L_{ij11}^{V,LR} - \frac{8}{9}L_{ij22}^{V,LR} - \frac{8}{9}L_{ij33}^{V,LR} \\
& + \frac{16}{9}L_{ij11}^{V1,LR} + \frac{16}{9}L_{ij22}^{V1,LR} - \frac{8}{9}L_{11ij}^{V,LL} - \frac{8}{9}L_{22ij}^{V,LL} - \frac{8}{9}L_{33ij}^{V,LL} - \frac{8}{9}L_{11ij}^{V1,LL} \\
& + \frac{16}{9}L_{22ij}^{V1,LL} \Bigg] + \alpha_s^2 \Bigg[ -8L_{ijkk}^{V1,LR} + \frac{4}{27}L_{ijkk}^{V8,LR} + 16L_{ijkk}^{V,LL} + \frac{256}{27}L_{ikkj}^{V,LL} \\
& - 8L_{ijii}^{V1,LR} - 8L_{ijjj}^{V1,LR} + \frac{4}{27}L_{ijii}^{V8,LR} + \frac{4}{27}L_{ijjj}^{V8,LR} + \frac{328}{9}L_{ijii}^{V,LL} + \frac{328}{9}L_{ijjj}^{V,LL} \\
& - 8L_{ij11}^{V1,LR} - 8L_{ij22}^{V1,LR} + \frac{4}{27}L_{ij11}^{V8,LR} + \frac{4}{27}L_{ij22}^{V8,LR} - \frac{4}{3}L_{11ij}^{V1,LL} + 8L_{22ij}^{V1,LL} \\
& + \frac{86}{27}L_{11ij}^{V8,LL} + \frac{4}{27}L_{22ij}^{V8,LL} \Bigg] + \alpha_s \alpha \Bigg[ -\frac{32}{9}L_{ijkk}^{V1,LR} + \frac{2020}{729}L_{ijkk}^{V8,LR} - \frac{16}{3}L_{ijkk}^{V,LL} \\
& - \frac{608}{729}L_{ikkj}^{V,LL} - \frac{32}{9}L_{ijii}^{V1,LR} - \frac{32}{9}L_{ijjj}^{V1,LR} + \frac{2020}{729}L_{ijii}^{V8,LR} + \frac{2020}{729}L_{ijjj}^{V8,LR} - \frac{2192}{243}L_{ijii}^{V,LL} \\
& - \frac{2192}{243}L_{ijjj}^{V,LL} + \frac{64}{9}L_{ij11}^{V1,LR} + \frac{64}{9}L_{ij22}^{V1,LR} - \frac{2732}{729}L_{ij11}^{V8,LR} - \frac{2732}{729}L_{ij22}^{V8,LR} \\
& + \frac{256}{9}L_{11ij}^{V1,LL} + \frac{64}{9}L_{22ij}^{V1,LL} - \frac{68}{729}L_{11ij}^{V8,LL} + \frac{148}{729}L_{22ij}^{V8,LL} \Bigg] + \alpha^2 \Bigg[ -\frac{304}{729}L_{ijkk}^{V1,LR} \\
& + \frac{3136}{729}L_{ijkk}^{V,LL} + \frac{5536}{2187}L_{ikkj}^{V,LL} - \frac{304}{729}L_{ijii}^{V1,LR} - \frac{304}{729}L_{ijjj}^{V1,LR} + \frac{8272}{729}L_{ijii}^{V,LL} \\
& + \frac{8272}{729}L_{ijjj}^{V,LL} - \frac{3040}{729}L_{ij11}^{V,LR} - \frac{3040}{729}L_{ij22}^{V,LR} - \frac{3040}{729}L_{ij33}^{V,LR} - \frac{1120}{729}L_{ij11}^{V1,LR} \\
& - \frac{1120}{729}L_{ij22}^{V1,LR} + \frac{2576}{729}L_{11ij}^{V,LL} + \frac{2576}{729}L_{22ij}^{V,LL} + \frac{2576}{729}L_{33ij}^{V,LL} + \frac{5216}{729}L_{11ij}^{V1,LL} \\
& + \frac{6368}{729}L_{22ij}^{V1,LL} \Bigg];
\end{aligned}$$



$$\begin{aligned}
\dot{L}_{11ij}^{V8,LL} = & g_s^2 \left[ \frac{2}{3} L_{ijkk}^{V8,LR} + \frac{8}{3} L_{ikkj}^{V,LL} + \frac{2}{3} L_{ijii}^{V8,LR} + \frac{2}{3} L_{ijjj}^{V8,LR} + \frac{8}{3} L_{ijii}^{V,LL} \right. \\
& + \frac{8}{3} L_{ijjj}^{V,LL} + \frac{2}{3} L_{ij11}^{V8,LR} + \frac{2}{3} L_{ij22}^{V8,LR} + 12 L_{11ij}^{V1,LL} - \frac{10}{3} L_{11ij}^{V8,LL} + \frac{2}{3} L_{22ij}^{V8,LL} \Big] \\
& - \frac{8}{3} e^2 L_{11ij}^{V8,LL} + \alpha_s^2 \left[ -\frac{22}{3} L_{ijkk}^{V1,LR} + \frac{151}{81} L_{ijkk}^{V8,LR} - \frac{28}{3} L_{ijkk}^{V,LL} + \frac{5200}{81} L_{ikkj}^{V,LL} \right. \\
& - \frac{22}{3} L_{ijii}^{V1,LR} - \frac{22}{3} L_{ijjj}^{V1,LR} + \frac{151}{81} L_{ijii}^{V8,LR} + \frac{151}{81} L_{ijjj}^{V8,LR} + \frac{1906}{27} L_{ijii}^{V,LL} + \frac{1906}{27} L_{ijjj}^{V,LL} \\
& - \frac{22}{3} L_{ij11}^{V1,LR} - \frac{22}{3} L_{ij22}^{V1,LR} + \frac{151}{81} L_{ij11}^{V8,LR} + \frac{151}{81} L_{ij22}^{V8,LR} + 13 L_{11ij}^{V1,LL} - \frac{2}{3} L_{22ij}^{V1,LL} \\
& - \frac{344}{81} L_{11ij}^{V8,LL} + \frac{781}{81} L_{22ij}^{V8,LL} \Big] + \alpha_s \alpha \left[ -\frac{208}{81} L_{ijkk}^{V1,LR} + \frac{52}{27} L_{ijkk}^{V8,LR} - \frac{416}{81} L_{ijkk}^{V,LL} \right. \\
& - \frac{5072}{243} L_{ikkj}^{V,LL} - \frac{208}{81} L_{ijii}^{V1,LR} - \frac{208}{81} L_{ijjj}^{V1,LR} + \frac{52}{27} L_{ijii}^{V8,LR} + \frac{52}{27} L_{ijjj}^{V8,LR} - \frac{3200}{81} L_{ijii}^{V,LL} \\
& - \frac{3200}{81} L_{ijjj}^{V,LL} - \frac{208}{81} L_{ij11}^{V,LR} - \frac{208}{81} L_{ij22}^{V,LR} - \frac{208}{81} L_{ij33}^{V,LR} + \frac{416}{81} L_{ij11}^{V1,LR} + \frac{416}{81} L_{ij22}^{V1,LR} \\
& - \frac{80}{27} L_{ij11}^{V8,LR} - \frac{80}{27} L_{ij22}^{V8,LR} - \frac{208}{81} L_{11ij}^{V,LL} - \frac{208}{81} L_{22ij}^{V,LL} - \frac{208}{81} L_{33ij}^{V,LL} + \frac{308}{81} L_{11ij}^{V1,LL} \\
& + \frac{416}{81} L_{22ij}^{V1,LL} + L_{11ij}^{V8,LL} + \frac{56}{9} L_{22ij}^{V8,LL} \Big] - \frac{128}{81} \alpha^2 L_{11ij}^{V8,LL} ;
\end{aligned}$$

$$\begin{aligned}
\dot{L}_{22ij}^{V1,LL} = & \frac{8}{3} g_s^2 L_{22ij}^{V8,LL} + e^2 \left[ -\frac{8}{9} L_{ijkk}^{V1,LR} - \frac{16}{9} L_{ijkk}^{V,LL} - \frac{16}{27} L_{ikkj}^{V,LL} - \frac{8}{9} L_{ijii}^{V1,LR} \right. \\
& - \frac{8}{9} L_{ijjj}^{V1,LR} - \frac{64}{27} L_{ijii}^{V,LL} - \frac{64}{27} L_{ijjj}^{V,LL} - \frac{8}{9} L_{ij11}^{V,LR} - \frac{8}{9} L_{ij22}^{V,LR} - \frac{8}{9} L_{ij33}^{V,LR} \\
& + \frac{16}{9} L_{ij11}^{V1,LR} + \frac{16}{9} L_{ij22}^{V1,LR} - \frac{8}{9} L_{11ij}^{V,LL} - \frac{8}{9} L_{22ij}^{V,LL} - \frac{8}{9} L_{33ij}^{V,LL} + \frac{16}{9} L_{11ij}^{V1,LL} \\
& \left. - \frac{8}{9} L_{22ij}^{V1,LL} \right] + \alpha_s^2 \left[ -8 L_{ijkk}^{V1,LR} + \frac{4}{27} L_{ijkk}^{V8,LR} + 16 L_{ijkk}^{V,LL} + \frac{256}{27} L_{ikkj}^{V,LL} \right. \\
& - 8 L_{ijii}^{V1,LR} - 8 L_{ijjj}^{V1,LR} + \frac{4}{27} L_{ijii}^{V8,LR} + \frac{4}{27} L_{ijjj}^{V8,LR} + \frac{328}{9} L_{ijii}^{V,LL} + \frac{328}{9} L_{ijjj}^{V,LL} \\
& - 8 L_{ij11}^{V1,LR} - 8 L_{ij22}^{V1,LR} + \frac{4}{27} L_{ij11}^{V8,LR} + \frac{4}{27} L_{ij22}^{V8,LR} + 8 L_{11ij}^{V1,LL} - \frac{4}{3} L_{22ij}^{V1,LL}
\end{aligned}$$

$$\begin{aligned}
& + \frac{4}{27} L_{11ij}^{V8,LL} + \frac{86}{27} L_{22ij}^{V8,LL} \Big] + \alpha_s \alpha \Big[ - \frac{32}{9} L_{ijkk}^{V1,LR} + \frac{2020}{729} L_{ijkk}^{V8,LR} - \frac{16}{3} L_{ijkk}^{V,LL} \\
& - \frac{608}{729} L_{ikkj}^{V,LL} - \frac{32}{9} L_{ijii}^{V1,LR} - \frac{32}{9} L_{ijjj}^{V1,LR} + \frac{2020}{729} L_{ijii}^{V8,LR} + \frac{2020}{729} L_{ijjj}^{V8,LR} - \frac{2192}{243} L_{ijii}^{V,LL} \\
& - \frac{2192}{243} L_{ijjj}^{V,LL} + \frac{64}{9} L_{ij11}^{V1,LR} + \frac{64}{9} L_{ij22}^{V1,LR} - \frac{2732}{729} L_{ij11}^{V8,LR} - \frac{2732}{729} L_{ij22}^{V8,LR} \\
& + \frac{64}{9} L_{11ij}^{V1,LL} + \frac{256}{9} L_{22ij}^{V1,LL} + \frac{148}{729} L_{11ij}^{V8,LL} - \frac{68}{729} L_{22ij}^{V8,LL} \Big] + \alpha^2 \Big[ - \frac{304}{729} L_{ijkk}^{V1,LR} \\
& + \frac{3136}{729} L_{ijkk}^{V,LL} + \frac{5536}{2187} L_{ikkj}^{V,LL} - \frac{304}{729} L_{ijii}^{V1,LR} - \frac{304}{729} L_{ijjj}^{V1,LR} + \frac{8272}{729} L_{ijii}^{V,LL} \\
& + \frac{8272}{729} L_{ijjj}^{V,LL} - \frac{3040}{729} L_{ij11}^{V,LR} - \frac{3040}{729} L_{ij22}^{V,LR} - \frac{3040}{729} L_{ij33}^{V,LR} - \frac{1120}{729} L_{ij11}^{V1,LR} \\
& - \frac{1120}{729} L_{ij22}^{V1,LR} + \frac{2576}{729} L_{11ij}^{V,LL} + \frac{2576}{729} L_{22ij}^{V,LL} + \frac{2576}{729} L_{33ij}^{V,LL} + \frac{6368}{729} L_{11ij}^{V1,LL} \\
& + \frac{5216}{729} L_{22ij}^{V1,LL} \Big] ;
\end{aligned}$$

$$\begin{aligned}
\dot{L}_{22ij}^{V8,LL} & = g_s^2 \Big[ \frac{2}{3} L_{ijkk}^{V8,LR} + \frac{8}{3} L_{ikkj}^{V,LL} + \frac{2}{3} L_{ijii}^{V8,LR} + \frac{2}{3} L_{ijjj}^{V8,LR} + \frac{8}{3} L_{ijii}^{V,LL} \\
& + \frac{8}{3} L_{ijjj}^{V,LL} + \frac{2}{3} L_{ij11}^{V8,LR} + \frac{2}{3} L_{ij22}^{V8,LR} + 12 L_{22ij}^{V1,LL} + \frac{2}{3} L_{11ij}^{V8,LL} - \frac{10}{3} L_{22ij}^{V8,LL} \Big] \\
& - \frac{8}{3} e^2 L_{22ij}^{V8,LL} + \alpha_s^2 \Big[ - \frac{22}{3} L_{ijkk}^{V1,LR} + \frac{151}{81} L_{ijkk}^{V8,LR} - \frac{28}{3} L_{ijkk}^{V,LL} + \frac{5200}{81} L_{ikkj}^{V,LL} \\
& - \frac{22}{3} L_{ijii}^{V1,LR} - \frac{22}{3} L_{ijjj}^{V1,LR} + \frac{151}{81} L_{ijii}^{V8,LR} + \frac{151}{81} L_{ijjj}^{V8,LR} + \frac{1906}{27} L_{ijii}^{V,LL} + \frac{1906}{27} L_{ijjj}^{V,LL} \\
& - \frac{22}{3} L_{ij11}^{V1,LR} - \frac{22}{3} L_{ij22}^{V1,LR} + \frac{151}{81} L_{ij11}^{V8,LR} + \frac{151}{81} L_{ij22}^{V8,LR} - \frac{2}{3} L_{11ij}^{V1,LL} + 13 L_{22ij}^{V1,LL} \\
& + \frac{781}{81} L_{11ij}^{V8,LL} - \frac{344}{81} L_{22ij}^{V8,LL} \Big] + \alpha_s \alpha \Big[ - \frac{208}{81} L_{ijkk}^{V1,LR} + \frac{52}{27} L_{ijkk}^{V8,LR} - \frac{416}{81} L_{ijkk}^{V,LL} \\
& - \frac{5072}{243} L_{ikkj}^{V,LL} - \frac{208}{81} L_{ijii}^{V1,LR} - \frac{208}{81} L_{ijjj}^{V1,LR} + \frac{52}{27} L_{ijii}^{V8,LR} + \frac{52}{27} L_{ijjj}^{V8,LR} - \frac{3200}{81} L_{ijii}^{V,LL} \\
& - \frac{3200}{81} L_{ijjj}^{V,LL} - \frac{208}{81} L_{ij11}^{V,LR} - \frac{208}{81} L_{ij22}^{V,LR} - \frac{208}{81} L_{ij33}^{V,LR} + \frac{416}{81} L_{ij11}^{V1,LR} + \frac{416}{81} L_{ij22}^{V1,LR}
\end{aligned}$$

$$\begin{aligned}
& -\frac{80}{27}L_{ij11}^{V8,LR} - \frac{80}{27}L_{ij22}^{V8,LR} - \frac{208}{81}L_{11ij}^{V,LL} - \frac{208}{81}L_{22ij}^{V,LL} - \frac{208}{81}L_{33ij}^{V,LL} + \frac{416}{81}L_{11ij}^{V1,LL} \\
& + \frac{308}{81}L_{22ij}^{V1,LL} + \frac{56}{9}L_{11ij}^{V8,LL} + L_{22ij}^{V8,LL} \Big] - \frac{128}{81}\alpha^2 L_{22ij}^{V8,LL} ; \\
\dot{L}_{ijkk}^{V,LL} = & g_s^2 \Bigg[ -\frac{1}{18}L_{ijii}^{V8,LR} - \frac{1}{18}L_{ijjj}^{V8,LR} - \frac{1}{18}L_{ijkk}^{V8,LR} - \frac{2}{9}L_{ijii}^{V,LL} - \frac{2}{9}L_{ijjj}^{V,LL} \\
& - 2L_{ijkk}^{V,LL} + \frac{52}{9}L_{ikkj}^{V,LL} - \frac{1}{18}L_{ij11}^{V8,LR} - \frac{1}{18}L_{ij22}^{V8,LR} - \frac{1}{18}L_{11ij}^{V8,LL} - \frac{1}{18}L_{22ij}^{V8,LL} \Big] \\
& + e^2 \Bigg[ \frac{2}{9}L_{ijii}^{V1,LR} + \frac{2}{9}L_{ijjj}^{V1,LR} + \frac{2}{9}L_{ijkk}^{V1,LR} + \frac{16}{27}L_{ijii}^{V,LL} + \frac{16}{27}L_{ijjj}^{V,LL} + \frac{16}{9}L_{ijkk}^{V,LL} \\
& + \frac{4}{27}L_{ikkj}^{V,LL} + \frac{2}{9}L_{ij11}^{V,LR} + \frac{2}{9}L_{ij22}^{V,LR} + \frac{2}{9}L_{ij33}^{V,LR} - \frac{4}{9}L_{ij11}^{V1,LR} - \frac{4}{9}L_{ij22}^{V1,LR} \\
& + \frac{2}{9}L_{11ij}^{V,LL} + \frac{2}{9}L_{22ij}^{V,LL} + \frac{2}{9}L_{33ij}^{V,LL} - \frac{4}{9}L_{11ij}^{V1,LL} - \frac{4}{9}L_{22ij}^{V1,LL} \Big] + \alpha_s^2 \Bigg[ -\frac{61}{18}L_{ijii}^{V1,LR} \\
& - \frac{61}{18}L_{ijjj}^{V1,LR} - \frac{61}{18}L_{ijkk}^{V1,LR} - \frac{79}{972}L_{ijii}^{V8,LR} - \frac{79}{972}L_{ijjj}^{V8,LR} - \frac{79}{972}L_{ijkk}^{V8,LR} + \frac{1999}{162}L_{ijii}^{V,LL} \\
& + \frac{1999}{162}L_{ijjj}^{V,LL} - \frac{17}{6}L_{ijkk}^{V,LL} + \frac{3025}{486}L_{ikkj}^{V,LL} - \frac{61}{18}L_{ij11}^{V,LR} - \frac{61}{18}L_{ij22}^{V,LR} - \frac{79}{972}L_{ij11}^{V8,LR} \\
& - \frac{79}{972}L_{ij22}^{V8,LR} + \frac{73}{18}L_{11ij}^{V1,LL} + \frac{73}{18}L_{22ij}^{V1,LL} - \frac{709}{972}L_{11ij}^{V8,LL} - \frac{709}{972}L_{22ij}^{V8,LL} \Big] \\
& + \alpha_s \alpha \Bigg[ \frac{241}{243}L_{ijii}^{V1,LR} + \frac{241}{243}L_{ijjj}^{V1,LR} + \frac{241}{243}L_{ijkk}^{V1,LR} - \frac{785}{1458}L_{ijii}^{V8,LR} - \frac{785}{1458}L_{ijjj}^{V8,LR} \\
& - \frac{785}{1458}L_{ijkk}^{V8,LR} + \frac{349}{243}L_{ijii}^{V,LL} + \frac{349}{243}L_{ijjj}^{V,LL} - \frac{1516}{243}L_{ijkk}^{V,LL} - \frac{6626}{729}L_{ikkj}^{V,LL} \\
& + \frac{25}{243}L_{ij11}^{V,LR} + \frac{25}{243}L_{ij22}^{V,LR} + \frac{25}{243}L_{ij33}^{V,LR} - \frac{482}{243}L_{ij11}^{V1,LR} - \frac{482}{243}L_{ij22}^{V1,LR} + \frac{727}{1458}L_{ij11}^{V8,LR} \\
& + \frac{727}{1458}L_{ij22}^{V8,LR} + \frac{25}{243}L_{11ij}^{V,LL} + \frac{25}{243}L_{22ij}^{V,LL} + \frac{25}{243}L_{33ij}^{V,LL} - \frac{482}{243}L_{11ij}^{V1,LL} - \frac{482}{243}L_{22ij}^{V1,LL} \\
& + \frac{115}{1458}L_{11ij}^{V8,LL} + \frac{115}{1458}L_{22ij}^{V8,LL} \Big] + \alpha^2 \Bigg[ -\frac{356}{729}L_{ijii}^{V1,LR} - \frac{356}{729}L_{ijjj}^{V1,LR} - \frac{356}{729}L_{ijkk}^{V1,LR} \\
& + \frac{632}{729}L_{ijii}^{V,LL} + \frac{632}{729}L_{ijjj}^{V,LL} + \frac{710}{729}L_{ijkk}^{V,LL} + \frac{344}{2187}L_{ikkj}^{V,LL} - \frac{644}{729}L_{ij11}^{V,LR}
\end{aligned}$$

$$\begin{aligned}
& -\frac{644}{729}L_{ij22}^{V,LR} - \frac{644}{729}L_{ij33}^{V,LR} - \frac{1772}{729}L_{ij11}^{V1,LR} - \frac{1772}{729}L_{ij22}^{V1,LR} + \frac{868}{729}L_{11ij}^{V,LL} \\
& + \frac{868}{729}L_{22ij}^{V,LL} + \frac{868}{729}L_{33ij}^{V,LL} + \frac{244}{729}L_{11ij}^{V1,LL} + \frac{244}{729}L_{22ij}^{V1,LL} \Big] ; \\
\dot{L}_{ikkj}^{V,LL} = & g_s^2 \left[ \frac{1}{6}L_{ijkk}^{V8,LR} + 6L_{ijkk}^{V,LL} - \frac{4}{3}L_{ikkj}^{V,LL} + \frac{1}{6}L_{ijii}^{V8,LR} + \frac{1}{6}L_{ijjj}^{V8,LR} \right. \\
& + \frac{2}{3}L_{ijii}^{V,LL} + \frac{2}{3}L_{ijjj}^{V,LL} + \frac{1}{6}L_{ij11}^{V8,LR} + \frac{1}{6}L_{ij22}^{V8,LR} + \frac{1}{6}L_{11ij}^{V8,LL} + \frac{1}{6}L_{22ij}^{V8,LL} \Big] \\
& + \frac{4}{3}e^2L_{ikkj}^{V,LL} + \alpha_s^2 \left[ -\frac{11}{6}L_{ijkk}^{V1,LR} + \frac{151}{324}L_{ijkk}^{V8,LR} + \frac{9}{2}L_{ijkk}^{V,LL} + \frac{719}{162}L_{ikkj}^{V,LL} \right. \\
& - \frac{11}{6}L_{ijii}^{V1,LR} - \frac{11}{6}L_{ijjj}^{V1,LR} + \frac{151}{324}L_{ijii}^{V8,LR} + \frac{151}{324}L_{ijjj}^{V8,LR} + \frac{953}{54}L_{ijii}^{V,LL} + \frac{953}{54}L_{ijjj}^{V,LL} \\
& - \frac{11}{6}L_{ij11}^{V1,LR} - \frac{11}{6}L_{ij22}^{V1,LR} + \frac{151}{324}L_{ij11}^{V8,LR} + \frac{151}{324}L_{ij22}^{V8,LR} - \frac{1}{6}L_{11ij}^{V1,LL} - \frac{1}{6}L_{22ij}^{V1,LL} \\
& + \frac{781}{324}L_{11ij}^{V8,LL} + \frac{781}{324}L_{22ij}^{V8,LL} \Big] + \alpha_s \alpha \left[ -\frac{25}{81}L_{ijkk}^{V1,LR} - \frac{25}{54}L_{ijkk}^{V8,LR} - \frac{752}{81}L_{ijkk}^{V,LL} \right. \\
& - \frac{1430}{243}L_{ikkj}^{V,LL} - \frac{25}{81}L_{ijii}^{V1,LR} - \frac{25}{81}L_{ijjj}^{V1,LR} - \frac{25}{54}L_{ijii}^{V8,LR} - \frac{25}{54}L_{ijjj}^{V8,LR} + \frac{199}{81}L_{ijii}^{V,LL} \\
& + \frac{199}{81}L_{ijjj}^{V,LL} - \frac{25}{81}L_{ij11}^{V,LR} - \frac{25}{81}L_{ij22}^{V,LR} - \frac{25}{81}L_{ij33}^{V,LR} + \frac{50}{81}L_{ij11}^{V1,LR} + \frac{50}{81}L_{ij22}^{V1,LR} \\
& + \frac{71}{54}L_{ij11}^{V8,LR} + \frac{71}{54}L_{ij22}^{V8,LR} - \frac{25}{81}L_{11ij}^{V,LL} - \frac{25}{81}L_{22ij}^{V,LL} - \frac{25}{81}L_{33ij}^{V,LL} + \frac{50}{81}L_{11ij}^{V1,LL} \\
& + \frac{50}{81}L_{22ij}^{V1,LL} - \frac{7}{18}L_{11ij}^{V8,LL} - \frac{7}{18}L_{22ij}^{V8,LL} \Big] + \frac{46}{81}\alpha^2L_{ikkj}^{V,LL} ; \\
\dot{L}_{ijjj}^{V,LL} = & g_s^2 \left[ \frac{1}{9}L_{ijii}^{V8,LR} + \frac{1}{9}L_{ijjj}^{V8,LR} + \frac{1}{9}L_{ijkk}^{V8,LR} + \frac{4}{9}L_{ijii}^{V,LL} + \frac{40}{9}L_{ijjj}^{V,LL} \right. \\
& + \frac{4}{9}L_{ikkj}^{V,LL} + \frac{1}{9}L_{ij11}^{V8,LR} + \frac{1}{9}L_{ij22}^{V8,LR} + \frac{1}{9}L_{11ij}^{V8,LL} + \frac{1}{9}L_{22ij}^{V8,LL} \Big] + e^2 \left[ \frac{2}{9}L_{ijii}^{V1,LR} \right. \\
& + \frac{2}{9}L_{ijjj}^{V1,LR} + \frac{2}{9}L_{ijkk}^{V1,LR} + \frac{16}{27}L_{ijii}^{V,LL} + \frac{52}{27}L_{ijjj}^{V,LL} + \frac{4}{9}L_{ijkk}^{V,LL} + \frac{4}{27}L_{ikkj}^{V,LL} \\
& + \frac{2}{9}L_{ij11}^{V,LR} + \frac{2}{9}L_{ij22}^{V,LR} + \frac{2}{9}L_{ij33}^{V,LR} - \frac{4}{9}L_{ij11}^{V1,LR} - \frac{4}{9}L_{ij22}^{V1,LR} + \frac{2}{9}L_{11ij}^{V,LL}
\end{aligned}$$

$$\begin{aligned}
& + \frac{2}{9} L_{22ij}^{V,LL} + \frac{2}{9} L_{33ij}^{V,LL} - \frac{4}{9} L_{11ij}^{V1,LL} - \frac{4}{9} L_{22ij}^{V1,LL} \Big] + \alpha_s^2 \Bigg[ - \frac{47}{9} L_{ijii}^{V1,LR} \\
& - \frac{47}{9} L_{ijjj}^{V1,LR} - \frac{47}{9} L_{ijkk}^{V1,LR} + \frac{187}{486} L_{ijii}^{V8,LR} + \frac{187}{486} L_{ijjj}^{V8,LR} + \frac{187}{486} L_{ijkk}^{V8,LR} + \frac{2429}{81} L_{ijii}^{V,LL} \\
& + \frac{2042}{81} L_{ijjj}^{V,LL} + \frac{58}{9} L_{ijkk}^{V,LL} + \frac{3752}{243} L_{ikkj}^{V,LL} - \frac{47}{9} L_{ij11}^{V1,LR} - \frac{47}{9} L_{ij22}^{V1,LR} + \frac{187}{486} L_{ij11}^{V8,LR} \\
& + \frac{187}{486} L_{ij22}^{V8,LR} + \frac{35}{9} L_{11ij}^{V1,LL} + \frac{35}{9} L_{22ij}^{V1,LL} + \frac{817}{486} L_{11ij}^{V8,LL} + \frac{817}{486} L_{22ij}^{V8,LL} \Big] \\
& + \alpha_s \alpha \Bigg[ \frac{166}{243} L_{ijii}^{V1,LR} + \frac{166}{243} L_{ijjj}^{V1,LR} + \frac{166}{243} L_{ijkk}^{V1,LR} - \frac{730}{729} L_{ijii}^{V8,LR} - \frac{730}{729} L_{ijjj}^{V8,LR} \\
& - \frac{730}{729} L_{ijkk}^{V8,LR} + \frac{946}{243} L_{ijii}^{V,LL} - \frac{3050}{243} L_{ijjj}^{V,LL} + \frac{224}{243} L_{ijkk}^{V,LL} + \frac{1072}{729} L_{ikkj}^{V,LL} \\
& - \frac{50}{243} L_{ij11}^{V,LR} - \frac{50}{243} L_{ij22}^{V,LR} - \frac{50}{243} L_{ij33}^{V,LR} - \frac{332}{243} L_{ij11}^{V1,LR} - \frac{332}{243} L_{ij22}^{V1,LR} + \frac{1322}{729} L_{ij11}^{V8,LR} \\
& + \frac{1322}{729} L_{ij22}^{V8,LR} - \frac{50}{243} L_{ed11ij}^{V,LL} - \frac{50}{243} L_{ed22ij}^{V,LL} - \frac{50}{243} L_{ed33ij}^{V,LL} - \frac{332}{243} L_{11ij}^{V1,LL} - \frac{332}{243} L_{22ij}^{V1,LL} \\
& - \frac{226}{729} L_{11ij}^{V8,LL} - \frac{226}{729} L_{22ij}^{V8,LL} \Big] + \alpha^2 \Bigg[ - \frac{356}{729} L_{ijii}^{V1,LR} - \frac{356}{729} L_{ijjj}^{V1,LR} - \frac{356}{729} L_{ijkk}^{V1,LR} \\
& + \frac{632}{729} L_{ijii}^{V,LL} + \frac{1046}{729} L_{ijjj}^{V,LL} + \frac{296}{729} L_{ijkk}^{V,LL} + \frac{344}{2187} L_{ikkj}^{V,LL} - \frac{644}{729} L_{ij11}^{V,LR} \\
& - \frac{644}{729} L_{ij22}^{V,LR} - \frac{644}{729} L_{ij33}^{V,LR} - \frac{1772}{729} L_{ij11}^{V1,LR} - \frac{1772}{729} L_{ij22}^{V1,LR} + \frac{868}{729} L_{11ij}^{V,LL} \\
& + \frac{868}{729} L_{ed22ij}^{V,LL} + \frac{868}{729} L_{ed33ij}^{V,LL} + \frac{244}{729} L_{11ij}^{V1,LL} + \frac{244}{729} L_{22ij}^{V1,LL} \Big] ;
\end{aligned}$$

$$\begin{aligned}
\dot{L}_{ijii}^{V,LL} & = g_s^2 \Bigg[ \frac{1}{9} L_{ijii}^{V8,LR} + \frac{1}{9} L_{ijjj}^{V8,LR} + \frac{1}{9} L_{ijkk}^{V8,LR} + \frac{40}{9} L_{ijii}^{V,LL} + \frac{4}{9} L_{ijjj}^{V,LL} \\
& + \frac{4}{9} L_{ikkj}^{V,LL} + \frac{1}{9} L_{ij11}^{V8,LR} + \frac{1}{9} L_{ij22}^{V8,LR} + \frac{1}{9} L_{11ij}^{V8,LL} + \frac{1}{9} L_{22ij}^{V8,LL} \Big] + e^2 \Bigg[ \frac{2}{9} L_{ijii}^{V1,LR} \\
& + \frac{2}{9} L_{ijjj}^{V1,LR} + \frac{2}{9} L_{ijkk}^{V1,LR} + \frac{52}{27} L_{ijii}^{V,LL} + \frac{16}{27} L_{ijjj}^{V,LL} + \frac{4}{9} L_{ijkk}^{V,LL} + \frac{4}{27} L_{ikkj}^{V,LL} \\
& + \frac{2}{9} L_{ij11}^{V,LR} + \frac{2}{9} L_{ij22}^{V,LR} + \frac{2}{9} L_{ij33}^{V,LR} - \frac{4}{9} L_{ij11}^{V1,LR} - \frac{4}{9} L_{ij22}^{V1,LR} + \frac{2}{9} L_{11ij}^{V,LL}
\end{aligned}$$

$$\begin{aligned}
& + \frac{2}{9} L_{22ij}^{V,LL} + \frac{2}{9} L_{33ij}^{V,LL} - \frac{4}{9} L_{11ij}^{V1,LL} - \frac{4}{9} L_{22ij}^{V1,LL} \Big] + \alpha_s^2 \Bigg[ - \frac{47}{9} L_{ijii}^{V1,LR} \\
& - \frac{47}{9} L_{ijjj}^{V1,LR} - \frac{47}{9} L_{ijkk}^{V1,LR} + \frac{187}{486} L_{ijii}^{V8,LR} + \frac{187}{486} L_{ijjj}^{V8,LR} + \frac{187}{486} L_{ijkk}^{V8,LR} + \frac{2042}{81} L_{ijii}^{V,LL} \\
& + \frac{2429}{81} L_{ijjj}^{V,LL} + \frac{58}{9} L_{ijkk}^{V,LL} + \frac{3752}{243} L_{ikkj}^{V,LL} - \frac{47}{9} L_{ij11}^{V1,LR} - \frac{47}{9} L_{ij22}^{V1,LR} + \frac{187}{486} L_{ij11}^{V8,LR} \\
& + \frac{187}{486} L_{ij22}^{V8,LR} + \frac{35}{9} L_{11ij}^{V1,LL} + \frac{35}{9} L_{22ij}^{V1,LL} + \frac{817}{486} L_{11ij}^{V8,LL} + \frac{817}{486} L_{22ij}^{V8,LL} \Big] \\
& + \alpha_s \alpha \Bigg[ \frac{166}{243} L_{ijii}^{V1,LR} + \frac{166}{243} L_{ijjj}^{V1,LR} + \frac{166}{243} L_{ijkk}^{V1,LR} - \frac{730}{729} L_{ijii}^{V8,LR} - \frac{730}{729} L_{ijjj}^{V8,LR} \\
& - \frac{730}{729} L_{ijkk}^{V8,LR} - \frac{3050}{243} L_{ijii}^{V,LL} + \frac{946}{243} L_{ijjj}^{V,LL} + \frac{224}{243} L_{ijkk}^{V,LL} + \frac{1072}{729} L_{ikkj}^{V,LL} \\
& - \frac{50}{243} L_{ij11}^{V,LR} - \frac{50}{243} L_{ij22}^{V,LR} - \frac{50}{243} L_{ij33}^{V,LR} - \frac{332}{243} L_{ij11}^{V1,LR} - \frac{332}{243} L_{ij22}^{V1,LR} + \frac{1322}{729} L_{ij11}^{V8,LR} \\
& + \frac{1322}{729} L_{ij22}^{V8,LR} - \frac{50}{243} L_{11ij}^{V,LL} - \frac{50}{243} L_{22ij}^{V,LL} - \frac{50}{243} L_{33ij}^{V,LL} - \frac{332}{243} L_{11ij}^{V1,LL} - \frac{332}{243} L_{22ij}^{V1,LL} \\
& - \frac{226}{729} L_{11ij}^{V8,LL} - \frac{226}{729} L_{22ij}^{V8,LL} \Big] + \alpha^2 \Bigg[ - \frac{356}{729} L_{ijii}^{V1,LR} - \frac{356}{729} L_{ijjj}^{V1,LR} - \frac{356}{729} L_{ijkk}^{V1,LR} \\
& + \frac{1046}{729} L_{ijii}^{V,LL} + \frac{632}{729} L_{ijjj}^{V,LL} + \frac{296}{729} L_{ijkk}^{V,LL} + \frac{344}{2187} L_{ikkj}^{V,LL} - \frac{644}{729} L_{ij11}^{V,LR} \\
& - \frac{644}{729} L_{ij22}^{V,LR} - \frac{644}{729} L_{ij33}^{V,LR} - \frac{1772}{729} L_{ij11}^{V1,LR} - \frac{1772}{729} L_{ij22}^{V1,LR} + \frac{868}{729} L_{11ij}^{V,LL} \\
& + \frac{868}{729} L_{22ij}^{V,LL} + \frac{868}{729} L_{33ij}^{V,LL} + \frac{244}{729} L_{11ij}^{V1,LL} + \frac{244}{729} L_{22ij}^{V1,LL} \Big] ; \\
\end{aligned}$$

$$\begin{aligned}
\dot{L}_{de}^{V,LR}{}_{ij11} & = e^2 \Bigg[ \frac{4}{3} L_{ijkk}^{V1,LR} + \frac{8}{3} L_{ijkk}^{V,LL} + \frac{8}{9} L_{ikkj}^{V,LL} + \frac{4}{3} L_{ijii}^{V1,LR} + \frac{4}{3} L_{ijjj}^{V1,LR} \\
& + \frac{32}{9} L_{ijii}^{V,LL} + \frac{32}{9} L_{ijjj}^{V,LL} - \frac{8}{3} L_{ij11}^{V,LR} + \frac{4}{3} L_{ij22}^{V,LR} + \frac{4}{3} L_{ij33}^{V,LR} - \frac{8}{3} L_{ij11}^{V1,LR} \\
& - \frac{8}{3} L_{ij22}^{V1,LR} + \frac{4}{3} L_{11ij}^{V,LL} + \frac{4}{3} L_{22ij}^{V,LL} + \frac{4}{3} L_{33ij}^{V,LL} - \frac{8}{3} L_{11ij}^{V1,LL} - \frac{8}{3} L_{22ij}^{V1,LL} \Big] \\
& + \alpha_s \alpha \Bigg[ \frac{16}{3} L_{ijkk}^{V1,LR} - \frac{1010}{243} L_{ijkk}^{V8,LR} + 8 L_{ijkk}^{V,LL} + \frac{304}{243} L_{ikkj}^{V,LL} + \frac{16}{3} L_{ijii}^{V1,LR}
\end{aligned}$$

$$\begin{aligned}
& + \frac{16}{3} L_{ijjj}^{V1,LR} - \frac{1010}{243} L_{ijii}^{V8,LR} - \frac{1010}{243} L_{ijjj}^{V8,LR} + \frac{1096}{81} L_{ijii}^{V,LL} + \frac{1096}{81} L_{ijjj}^{V,LL} \\
& + 16 L_{ij11}^{V,LR} - \frac{32}{3} L_{ij11}^{V1,LR} - \frac{32}{3} L_{ij22}^{V1,LR} + \frac{1366}{243} L_{ij11}^{V8,LR} + \frac{1366}{243} L_{ij22}^{V8,LR} - \frac{32}{3} L_{11ij}^{V1,LL} \\
& - \frac{32}{3} L_{22ij}^{V1,LL} - \frac{74}{243} L_{11ij}^{V8,LL} - \frac{74}{243} L_{22ij}^{V8,LL} \Big] + \alpha^2 \Big[ \frac{1736}{243} L_{ijkk}^{V1,LR} + \frac{304}{243} L_{ijkk}^{V,LL} \\
& - \frac{1328}{729} L_{ikkj}^{V,LL} + \frac{1736}{243} L_{ijii}^{V1,LR} + \frac{1736}{243} L_{ijjj}^{V1,LR} - \frac{752}{243} L_{ijii}^{V,LL} - \frac{752}{243} L_{ijjj}^{V,LL} \\
& + \frac{21698}{243} L_{ij11}^{V,LR} + \frac{3752}{243} L_{ij22}^{V,LR} + \frac{3752}{243} L_{ij33}^{V,LR} - \frac{664}{243} L_{ij11}^{V1,LR} - \frac{664}{243} L_{ij22}^{V1,LR} \\
& - \frac{1000}{243} L_{11ij}^{V,LL} - \frac{1000}{243} L_{22ij}^{V,LL} - \frac{1000}{243} L_{33ij}^{V,LL} - \frac{7000}{243} L_{11ij}^{V1,LL} - \frac{7000}{243} L_{22ij}^{V1,LL} \Big] ; \\
\dot{L}_{ij22}^{V,LR} & = e^2 \Big[ \frac{4}{3} L_{ijkk}^{V1,LR} + \frac{8}{3} L_{ijkk}^{V,LL} + \frac{8}{9} L_{ikkj}^{V,LL} + \frac{4}{3} L_{ijii}^{V1,LR} + \frac{4}{3} L_{ijjj}^{V1,LR} \\
& + \frac{32}{9} L_{ijii}^{V,LL} + \frac{32}{9} L_{ijjj}^{V,LL} + \frac{4}{3} L_{ij11}^{V,LR} - \frac{8}{3} L_{ij22}^{V,LR} + \frac{4}{3} L_{ij33}^{V,LR} - \frac{8}{3} L_{ij11}^{V1,LR} \\
& - \frac{8}{3} L_{ij22}^{V1,LR} + \frac{4}{3} L_{11ij}^{V,LL} + \frac{4}{3} L_{22ij}^{V,LL} + \frac{4}{3} L_{33ij}^{V,LL} - \frac{8}{3} L_{11ij}^{V1,LL} - \frac{8}{3} L_{22ij}^{V1,LL} \Big] \\
& + \alpha_s \alpha \Big[ \frac{16}{3} L_{ijkk}^{V1,LR} - \frac{1010}{243} L_{ijkk}^{V8,LR} + 8 L_{ijkk}^{V,LL} + \frac{304}{243} L_{ikkj}^{V,LL} + \frac{16}{3} L_{ijii}^{V1,LR} \\
& + \frac{16}{3} L_{ijjj}^{V1,LR} - \frac{1010}{243} L_{ijii}^{V8,LR} - \frac{1010}{243} L_{ijjj}^{V8,LR} + \frac{1096}{81} L_{ijii}^{V,LL} + \frac{1096}{81} L_{ijjj}^{V,LL} \\
& + 16 L_{ij22}^{V,LR} - \frac{32}{3} L_{ij11}^{V1,LR} - \frac{32}{3} L_{ij22}^{V1,LR} + \frac{1366}{243} L_{ij11}^{V8,LR} + \frac{1366}{243} L_{ij22}^{V8,LR} - \frac{32}{3} L_{11ij}^{V1,LL} \\
& - \frac{32}{3} L_{22ij}^{V1,LL} - \frac{74}{243} L_{11ij}^{V8,LL} - \frac{74}{243} L_{22ij}^{V8,LL} \Big] + \alpha^2 \Big[ \frac{1736}{243} L_{ijkk}^{V1,LR} + \frac{304}{243} L_{ijkk}^{V,LL} \\
& - \frac{1328}{729} L_{ikkj}^{V,LL} + \frac{1736}{243} L_{ijii}^{V1,LR} + \frac{1736}{243} L_{ijjj}^{V1,LR} - \frac{752}{243} L_{ijii}^{V,LL} - \frac{752}{243} L_{ijjj}^{V,LL} \\
& + \frac{3752}{243} L_{ij11}^{V,LR} + \frac{21698}{243} L_{ij22}^{V,LR} + \frac{3752}{243} L_{ij33}^{V,LR} - \frac{664}{243} L_{ij11}^{V1,LR} - \frac{664}{243} L_{ij22}^{V1,LR} \\
& - \frac{1000}{243} L_{11ij}^{V,LL} - \frac{1000}{243} L_{22ij}^{V,LL} - \frac{1000}{243} L_{33ij}^{V,LL} - \frac{7000}{243} L_{11ij}^{V1,LL} - \frac{7000}{243} L_{22ij}^{V1,LL} \Big] ;
\end{aligned}$$

$$\begin{aligned}
\dot{L}_{ij33}^{V,LR} = & e^2 \left[ \frac{4}{3} L_{ijkk}^{V1,LR} + \frac{8}{3} L_{ijkk}^{V,LL} + \frac{8}{9} L_{ikkj}^{V,LL} + \frac{4}{3} L_{ijii}^{V1,LR} + \frac{4}{3} L_{ijjj}^{V1,LR} \right. \\
& + \frac{32}{9} L_{ijii}^{V,LL} + \frac{32}{9} L_{ijjj}^{V,LL} + \frac{4}{3} L_{ij11}^{V,LR} + \frac{4}{3} L_{ij22}^{V,LR} - \frac{8}{3} L_{ij33}^{V,LR} - \frac{8}{3} L_{ij11}^{V1,LR} \\
& - \frac{8}{3} L_{ij22}^{V1,LR} + \frac{4}{3} L_{11ij}^{V,LL} + \frac{4}{3} L_{22ij}^{V,LL} + \frac{4}{3} L_{33ij}^{V,LL} - \frac{8}{3} L_{11ij}^{V1,LL} - \frac{8}{3} L_{22ij}^{V1,LL} \left. \right] \\
& + \alpha_s \alpha \left[ \frac{16}{3} L_{ijkk}^{V1,LR} - \frac{1010}{243} L_{ijkk}^{V8,LR} + 8 L_{ijkk}^{V,LL} + \frac{304}{243} L_{ikkj}^{V,LL} + \frac{16}{3} L_{ijii}^{V1,LR} \right. \\
& + \frac{16}{3} L_{ijjj}^{V1,LR} - \frac{1010}{243} L_{ijii}^{V8,LR} - \frac{1010}{243} L_{ijjj}^{V8,LR} + \frac{1096}{81} L_{ijii}^{V,LL} + \frac{1096}{81} L_{ijjj}^{V,LL} \\
& + 16 L_{ij33}^{V,LR} - \frac{32}{3} L_{ij11}^{V1,LR} - \frac{32}{3} L_{ij22}^{V1,LR} + \frac{1366}{243} L_{ij11}^{V8,LR} + \frac{1366}{243} L_{ij22}^{V8,LR} - \frac{32}{3} L_{11ij}^{V1,LL} \\
& - \frac{32}{3} L_{22ij}^{V1,LL} - \frac{74}{243} L_{11ij}^{V8,LL} - \frac{74}{243} L_{22ij}^{V8,LL} \left. \right] + \alpha^2 \left[ \frac{1736}{243} L_{ijkk}^{V1,LR} + \frac{304}{243} L_{ijkk}^{V,LL} \right. \\
& - \frac{1328}{729} L_{ikkj}^{V,LL} + \frac{1736}{243} L_{ijii}^{V1,LR} + \frac{1736}{243} L_{ijjj}^{V1,LR} - \frac{752}{243} L_{ijii}^{V,LL} - \frac{752}{243} L_{ijjj}^{V,LL} \\
& + \frac{3752}{243} L_{ij11}^{V,LR} + \frac{3752}{243} L_{ij22}^{V,LR} + \frac{21698}{243} L_{ij33}^{V,LR} - \frac{664}{243} L_{ij11}^{V1,LR} - \frac{664}{243} L_{ij22}^{V1,LR} \\
& - \frac{1000}{243} L_{11ij}^{V,LL} - \frac{1000}{243} L_{22ij}^{V,LL} - \frac{1000}{243} L_{33ij}^{V,LL} - \frac{7000}{243} L_{11ij}^{V1,LL} - \frac{7000}{243} L_{22ij}^{V1,LL} \left. \right];
\end{aligned}$$

$$\begin{aligned}
\dot{L}_{ij11}^{V1,LR} = & -\frac{8}{3} g_s^2 L_{ij11}^{V8,LR} + e^2 \left[ -\frac{8}{9} L_{ijkk}^{V1,LR} - \frac{16}{9} L_{ijkk}^{V,LL} - \frac{16}{27} L_{ikkj}^{V,LL} - \frac{8}{9} L_{ijii}^{V1,LR} \right. \\
& - \frac{8}{9} L_{ijjj}^{V1,LR} - \frac{64}{27} L_{ijii}^{V,LL} - \frac{64}{27} L_{ijjj}^{V,LL} - \frac{8}{9} L_{ij11}^{V,LR} - \frac{8}{9} L_{ij22}^{V,LR} - \frac{8}{9} L_{ij33}^{V,LR} \\
& + \frac{40}{9} L_{ij11}^{V1,LR} + \frac{16}{9} L_{ij22}^{V1,LR} - \frac{8}{9} L_{11ij}^{V,LL} - \frac{8}{9} L_{22ij}^{V,LL} - \frac{8}{9} L_{33ij}^{V,LL} + \frac{16}{9} L_{11ij}^{V1,LL} \\
& + \frac{16}{9} L_{22ij}^{V1,LL} \left. \right] + \alpha_s^2 \left[ 8 L_{ijkk}^{V1,LR} + \frac{44}{27} L_{ijkk}^{V8,LR} - 16 L_{ijkk}^{V,LL} - \frac{64}{27} L_{ikkj}^{V,LL} \right. \\
& + 8 L_{ijii}^{V1,LR} + 8 L_{ijjj}^{V1,LR} + \frac{44}{27} L_{ijii}^{V8,LR} + \frac{44}{27} L_{ijjj}^{V8,LR} - \frac{232}{9} L_{ijii}^{V,LL} - \frac{232}{9} L_{ijjj}^{V,LL} \\
& - \frac{4}{3} L_{ij11}^{V1,LR} + 8 L_{ij22}^{V1,LR} - \frac{2000}{27} L_{ij11}^{V8,LR} + \frac{44}{27} L_{ij22}^{V8,LR} - 8 L_{11ij}^{V1,LL} - 8 L_{22ij}^{V1,LL}
\end{aligned}$$



$$\begin{aligned}
& + \frac{44}{27} L_{11ij}^{V8,LL} + \frac{44}{27} L_{22ij}^{V8,LL} \Big] + \alpha_s \alpha \Bigg[ - \frac{32}{9} L_{ijkk}^{V1,LR} + \frac{2020}{729} L_{ijkk}^{V8,LR} - \frac{16}{3} L_{ijkk}^{V,LL} \\
& - \frac{608}{729} L_{ikkj}^{V,LL} - \frac{32}{9} L_{ijii}^{V1,LR} - \frac{32}{9} L_{ijjj}^{V1,LR} + \frac{2020}{729} L_{ijii}^{V8,LR} + \frac{2020}{729} L_{ijjj}^{V8,LR} - \frac{2192}{243} L_{ijii}^{V,LL} \\
& - \frac{2192}{243} L_{ijjj}^{V,LL} - \frac{128}{9} L_{ij11}^{V1,LR} + \frac{64}{9} L_{ij22}^{V1,LR} + \frac{3532}{729} L_{ij11}^{V8,LR} - \frac{2732}{729} L_{ij22}^{V8,LR} \\
& + \frac{64}{9} L_{11ij}^{V1,LL} + \frac{64}{9} L_{22ij}^{V1,LL} + \frac{148}{729} L_{11ij}^{V8,LL} + \frac{148}{729} L_{22ij}^{V8,LL} \Big] + \alpha^2 \Bigg[ \frac{3728}{729} L_{ijkk}^{V1,LR} \\
& + \frac{832}{729} L_{ikkj}^{V,LL} - \frac{224}{2187} L_{ikkj}^{V,LL} + \frac{3728}{729} L_{ijii}^{V1,LR} + \frac{3728}{729} L_{ijjj}^{V1,LR} + \frac{784}{729} L_{ijii}^{V,LL} \\
& + \frac{784}{729} L_{ijjj}^{V,LL} + \frac{6176}{729} L_{ij11}^{V,LR} + \frac{6176}{729} L_{ij22}^{V,LR} + \frac{6176}{729} L_{ij33}^{V,LR} - \frac{30064}{729} L_{ij11}^{V1,LR} \\
& + \frac{6368}{729} L_{ij22}^{V1,LR} - \frac{3760}{729} L_{ij11}^{V,LL} - \frac{3760}{729} L_{ij22}^{V,LL} - \frac{3760}{729} L_{ij33}^{V,LL} - \frac{6880}{729} L_{ij11}^{V1,LL} \\
& - \frac{6880}{729} L_{ij22}^{V1,LL} \Big] ;
\end{aligned}$$

$$\begin{aligned}
\dot{L}_{ij11}^{V8,LR} &= g_s^2 \Bigg[ \frac{2}{3} L_{ijkk}^{V8,LR} + \frac{8}{3} L_{ikkj}^{V,LL} + \frac{2}{3} L_{ijii}^{V8,LR} + \frac{2}{3} L_{ijjj}^{V8,LR} + \frac{8}{3} L_{ijii}^{V,LL} \\
& + \frac{8}{3} L_{ijjj}^{V,LL} - 12 L_{ij11}^{V1,LR} - \frac{40}{3} L_{ij11}^{V8,LR} + \frac{2}{3} L_{ij22}^{V8,LR} + \frac{2}{3} L_{ij11}^{V8,LL} + \frac{2}{3} L_{ij22}^{V8,LL} \Big] \\
& + \frac{8}{3} e^2 L_{ij11}^{V8,LR} + \alpha_s^2 \Bigg[ - \frac{22}{3} L_{ijkk}^{V1,LR} + \frac{781}{81} L_{ijkk}^{V8,LR} - \frac{28}{3} L_{ikkj}^{V,LL} + \frac{3400}{81} L_{ikkj}^{V,LL} \\
& - \frac{22}{3} L_{ijii}^{V1,LR} - \frac{22}{3} L_{ijjj}^{V1,LR} + \frac{781}{81} L_{ijii}^{V8,LR} + \frac{781}{81} L_{ijjj}^{V8,LR} + \frac{1186}{27} L_{ijii}^{V,LL} + \frac{1186}{27} L_{ijjj}^{V,LL} \\
& - 132 L_{ij11}^{V1,LR} - \frac{22}{3} L_{ij22}^{V1,LR} - \frac{25213}{162} L_{ij11}^{V8,LR} + \frac{781}{81} L_{ij22}^{V8,LR} - \frac{2}{3} L_{ij11}^{V1,LL} - \frac{2}{3} L_{ij22}^{V1,LL} \\
& + \frac{601}{81} L_{ij11}^{V8,LL} + \frac{601}{81} L_{ij22}^{V8,LL} \Big] + \alpha_s \alpha \Bigg[ - \frac{928}{81} L_{ijkk}^{V1,LR} - \frac{44}{9} L_{ijkk}^{V8,LR} - \frac{1856}{81} L_{ijkk}^{V,LL} \\
& + \frac{688}{243} L_{ikkj}^{V,LL} - \frac{928}{81} L_{ijii}^{V1,LR} - \frac{928}{81} L_{ijjj}^{V1,LR} - \frac{44}{9} L_{ijii}^{V8,LR} - \frac{44}{9} L_{ijjj}^{V8,LR} - \frac{2192}{81} L_{ijii}^{V,LL} \\
& - \frac{2192}{81} L_{ijjj}^{V,LL} - \frac{928}{81} L_{ij11}^{V,LR} - \frac{928}{81} L_{ij22}^{V,LR} - \frac{928}{81} L_{ij33}^{V,LR} + \frac{4988}{81} L_{ij11}^{V1,LR} + \frac{1856}{81} L_{ij22}^{V1,LR}
\end{aligned}$$

$$\begin{aligned}
& + 27L_{ij11}^{V8,LR} + \frac{56}{9}L_{ij22}^{V8,LR} - \frac{928}{81}L_{11ij}^{V,LL} - \frac{928}{81}L_{22ij}^{V,LL} - \frac{928}{81}L_{33ij}^{V,LL} + \frac{1856}{81}L_{11ij}^{V1,LL} \\
& + \frac{1856}{81}L_{22ij}^{V1,LL} - \frac{160}{27}L_{11ij}^{V8,LL} - \frac{160}{27}L_{22ij}^{V8,LL} \Big] - \frac{4048}{81}\alpha^2 L_{ij11}^{V8,LR} ; \\
\dot{L}_{ij22}^{V1,LR} = & -\frac{8}{3}g_s^2 L_{ij22}^{V8,LR} + e^2 \Big[ -\frac{8}{9}L_{ijkk}^{V1,LR} - \frac{16}{9}L_{ijkk}^{V,LL} - \frac{16}{27}L_{ikkj}^{V,LL} - \frac{8}{9}L_{ijii}^{V1,LR} \\
& - \frac{8}{9}L_{ijjj}^{V1,LR} - \frac{64}{27}L_{ijii}^{V,LL} - \frac{64}{27}L_{ijjj}^{V,LL} - \frac{8}{9}L_{ij11}^{V,LR} - \frac{8}{9}L_{ij22}^{V,LR} - \frac{8}{9}L_{ij33}^{V,LR} \\
& + \frac{16}{9}L_{ij11}^{V1,LR} + \frac{40}{9}L_{ij22}^{V1,LR} - \frac{8}{9}L_{11ij}^{V,LL} - \frac{8}{9}L_{22ij}^{V,LL} - \frac{8}{9}L_{33ij}^{V,LL} + \frac{16}{9}L_{11ij}^{V1,LL} \\
& + \frac{16}{9}L_{22ij}^{V1,LL} \Big] + \alpha_s^2 \Big[ 8L_{ijkk}^{V1,LR} + \frac{44}{27}L_{ijkk}^{V8,LR} - 16L_{ijkk}^{V,LL} - \frac{64}{27}L_{ikkj}^{V,LL} \\
& + 8L_{ijii}^{V1,LR} + 8L_{ijjj}^{V1,LR} + \frac{44}{27}L_{ijii}^{V8,LR} + \frac{44}{27}L_{ijjj}^{V8,LR} - \frac{232}{9}L_{ijii}^{V,LL} - \frac{232}{9}L_{ijjj}^{V,LL} \\
& + 8L_{ij11}^{V1,LR} - \frac{4}{3}L_{ij22}^{V1,LR} + \frac{44}{27}L_{ij11}^{V8,LR} - \frac{2000}{27}L_{ij22}^{V8,LR} - 8L_{11ij}^{V1,LL} - 8L_{22ij}^{V1,LL} \\
& + \frac{44}{27}L_{11ij}^{V8,LL} + \frac{44}{27}L_{22ij}^{V8,LL} \Big] + \alpha_s \alpha \Big[ -\frac{32}{9}L_{ijkk}^{V1,LR} + \frac{2020}{729}L_{ijkk}^{V8,LR} - \frac{16}{3}L_{ijkk}^{V,LL} \\
& - \frac{608}{729}L_{ikkj}^{V,LL} - \frac{32}{9}L_{ijii}^{V1,LR} - \frac{32}{9}L_{ijjj}^{V1,LR} + \frac{2020}{729}L_{ijii}^{V8,LR} + \frac{2020}{729}L_{ijjj}^{V8,LR} - \frac{2192}{243}L_{ijii}^{V,LL} \\
& - \frac{2192}{243}L_{ijjj}^{V,LL} + \frac{64}{9}L_{ij11}^{V1,LR} - \frac{128}{9}L_{ij22}^{V1,LR} - \frac{2732}{729}L_{ij11}^{V8,LR} + \frac{3532}{729}L_{ij22}^{V8,LR} \\
& + \frac{64}{9}L_{11ij}^{V1,LL} + \frac{64}{9}L_{22ij}^{V1,LL} + \frac{148}{729}L_{11ij}^{V8,LL} + \frac{148}{729}L_{22ij}^{V8,LL} \Big] + \alpha^2 \Big[ \frac{3728}{729}L_{ijkk}^{V1,LR} \\
& + \frac{832}{729}L_{ijkk}^{V,LL} - \frac{224}{2187}L_{ikkj}^{V,LL} + \frac{3728}{729}L_{ijii}^{V1,LR} + \frac{3728}{729}L_{ijjj}^{V1,LR} + \frac{784}{729}L_{ijii}^{V,LL} \\
& + \frac{784}{729}L_{ijjj}^{V,LL} + \frac{6176}{729}L_{ij11}^{V,LR} + \frac{6176}{729}L_{ij22}^{V,LR} + \frac{6176}{729}L_{ij33}^{V,LR} + \frac{6368}{729}L_{ij11}^{V1,LR} \\
& - \frac{30064}{729}L_{ij22}^{V1,LR} - \frac{3760}{729}L_{11ij}^{V,LL} - \frac{3760}{729}L_{22ij}^{V,LL} - \frac{3760}{729}L_{33ij}^{V,LL} - \frac{6880}{729}L_{11ij}^{V1,LL} \\
& - \frac{6880}{729}L_{22ij}^{V1,LL} \Big] ;
\end{aligned}$$

$$\begin{aligned}
\dot{L}_{ij22}^{V8,LR} = & g_s^2 \left[ \frac{2}{3} L_{ijkk}^{V8,LR} + \frac{8}{3} L_{ikkj}^{V,LL} + \frac{2}{3} L_{ijii}^{V8,LR} + \frac{2}{3} L_{ijjj}^{V8,LR} + \frac{8}{3} L_{ijii}^{V,LL} \right. \\
& + \frac{8}{3} L_{ijjj}^{V,LL} - 12 L_{ij22}^{V1,LR} + \frac{2}{3} L_{ij11}^{V8,LR} - \frac{40}{3} L_{ij22}^{V8,LR} + \frac{2}{3} L_{11ij}^{V8,LL} + \left. \frac{2}{3} L_{22ij}^{V8,LL} \right] \\
& + \frac{8}{3} e^2 L_{ij22}^{V8,LR} + \alpha_s^2 \left[ -\frac{22}{3} L_{ijkk}^{V1,LR} + \frac{781}{81} L_{ijkk}^{V8,LR} - \frac{28}{3} L_{ijkk}^{V,LL} + \frac{3400}{81} L_{ikkj}^{V,LL} \right. \\
& - \frac{22}{3} L_{ijii}^{V1,LR} - \frac{22}{3} L_{ijjj}^{V1,LR} + \frac{781}{81} L_{ijii}^{V8,LR} + \frac{781}{81} L_{ijjj}^{V8,LR} + \frac{1186}{27} L_{ijii}^{V,LL} + \frac{1186}{27} L_{ijjj}^{V,LL} \\
& - \frac{22}{3} L_{ij11}^{V1,LR} - 132 L_{ij22}^{V1,LR} + \frac{781}{81} L_{ij11}^{V8,LR} - \frac{25213}{162} L_{ij22}^{V8,LR} - \frac{2}{3} L_{11ij}^{V1,LL} - \frac{2}{3} L_{22ij}^{V1,LL} \\
& + \left. \frac{601}{81} L_{11ij}^{V8,LL} + \frac{601}{81} L_{22ij}^{V8,LL} \right] + \alpha_s \alpha \left[ -\frac{928}{81} L_{ijkk}^{V1,LR} - \frac{44}{9} L_{ijkk}^{V8,LR} - \frac{1856}{81} L_{ijkk}^{V,LL} \right. \\
& + \frac{688}{243} L_{ikkj}^{V,LL} - \frac{928}{81} L_{ijii}^{V1,LR} - \frac{928}{81} L_{ijjj}^{V1,LR} - \frac{44}{9} L_{ijii}^{V8,LR} - \frac{44}{9} L_{ijjj}^{V8,LR} - \frac{2192}{81} L_{ijii}^{V,LL} \\
& - \frac{2192}{81} L_{ijjj}^{V,LL} - \frac{928}{81} L_{ij11}^{V,LR} - \frac{928}{81} L_{ij22}^{V,LR} - \frac{928}{81} L_{ij33}^{V,LR} + \frac{1856}{81} L_{ij11}^{V1,LR} + \frac{4988}{81} L_{ij22}^{V1,LR} \\
& + \frac{56}{9} L_{ij11}^{V8,LR} + 27 L_{ij22}^{V8,LR} - \frac{928}{81} L_{11ij}^{V,LL} - \frac{928}{81} L_{22ij}^{V,LL} - \frac{928}{81} L_{33ij}^{V,LL} + \frac{1856}{81} L_{11ij}^{V1,LL} \\
& + \left. \frac{1856}{81} L_{22ij}^{V1,LL} - \frac{160}{27} L_{11ij}^{V8,LL} - \frac{160}{27} L_{22ij}^{V8,LL} \right] - \frac{4048}{81} \alpha^2 L_{ij22}^{V8,LR} ;
\end{aligned}$$

$$\begin{aligned}
\dot{L}_{ijkk}^{V1,LR} = & -\frac{8}{3} g_s^2 L_{ijkk}^{V8,LR} + e^2 \left[ -\frac{8}{9} L_{ijkk}^{V1,LR} + \frac{8}{9} L_{ijkk}^{V,LL} + \frac{8}{27} L_{ikkj}^{V,LL} + \frac{4}{9} L_{ijii}^{V1,LR} \right. \\
& + \frac{4}{9} L_{ijjj}^{V1,LR} + \frac{32}{27} L_{ijii}^{V,LL} + \frac{32}{27} L_{ijjj}^{V,LL} + \frac{4}{9} L_{ij11}^{V,LR} + \frac{4}{9} L_{ij22}^{V,LR} + \frac{4}{9} L_{ij33}^{V,LR} \\
& - \frac{8}{9} L_{ij11}^{V1,LR} - \frac{8}{9} L_{ij22}^{V1,LR} + \frac{4}{9} L_{11ij}^{V,LL} + \frac{4}{9} L_{22ij}^{V,LL} + \frac{4}{9} L_{33ij}^{V,LL} - \frac{8}{9} L_{11ij}^{V1,LL} \\
& - \left. \frac{8}{9} L_{22ij}^{V1,LL} \right] + \alpha_s^2 \left[ -\frac{4}{3} L_{ijkk}^{V1,LR} - \frac{2000}{27} L_{ijkk}^{V8,LR} - 16 L_{ijkk}^{V,LL} - \frac{64}{27} L_{ikkj}^{V,LL} \right. \\
& + 8 L_{ijii}^{V1,LR} + 8 L_{ijjj}^{V1,LR} + \frac{44}{27} L_{ijii}^{V8,LR} + \frac{44}{27} L_{ijjj}^{V8,LR} - \frac{232}{9} L_{ijii}^{V,LL} - \frac{232}{9} L_{ijjj}^{V,LL} \\
& + 8 L_{ij11}^{V1,LR} + 8 L_{ij22}^{V1,LR} + \frac{44}{27} L_{ij11}^{V8,LR} + \frac{44}{27} L_{ij22}^{V8,LR} - 8 L_{11ij}^{V1,LL} - 8 L_{22ij}^{V1,LL}
\end{aligned}$$

$$\begin{aligned}
& + \frac{44}{27} L_{11ij}^{V8,LL} + \frac{44}{27} L_{22ij}^{V8,LL} \Big] + \alpha_s \alpha \Bigg[ \frac{112}{9} L_{ijkk}^{V1,LR} - \frac{1226}{729} L_{ijkk}^{V8,LR} + \frac{8}{3} L_{ijkk}^{V,LL} \\
& + \frac{304}{729} L_{ikkj}^{V,LL} + \frac{16}{9} L_{ijii}^{V1,LR} + \frac{16}{9} L_{ijjj}^{V1,LR} - \frac{1010}{729} L_{ijii}^{V8,LR} - \frac{1010}{729} L_{ijjj}^{V8,LR} + \frac{1096}{243} L_{ijii}^{V,LL} \\
& + \frac{1096}{243} L_{ijjj}^{V,LL} - \frac{32}{9} L_{ij11}^{V1,LR} - \frac{32}{9} L_{ij22}^{V1,LR} + \frac{1366}{729} L_{ij11}^{V8,LR} + \frac{1366}{729} L_{ij22}^{V8,LR} \\
& - \frac{32}{9} L_{11ij}^{V1,LL} - \frac{32}{9} L_{22ij}^{V1,LL} - \frac{74}{729} L_{11ij}^{V8,LL} - \frac{74}{729} L_{22ij}^{V8,LL} \Big] + \alpha^2 \Bigg[ \frac{16406}{729} L_{ijkk}^{V1,LR} \\
& + \frac{16}{729} L_{ijkk}^{V,LL} - \frac{752}{2187} L_{ikkj}^{V,LL} + \frac{296}{729} L_{ijii}^{V1,LR} + \frac{296}{729} L_{ijjj}^{V1,LR} - \frac{608}{729} L_{ijii}^{V,LL} \\
& - \frac{608}{729} L_{ijjj}^{V,LL} + \frac{1016}{729} L_{ij11}^{V,LR} + \frac{1016}{729} L_{ij22}^{V,LR} + \frac{1016}{729} L_{ij33}^{V,LR} - \frac{1672}{729} L_{ij11}^{V1,LR} \\
& - \frac{1672}{729} L_{ij22}^{V1,LR} + \frac{152}{729} L_{ij11}^{V,LL} + \frac{152}{729} L_{ij22}^{V,LL} + \frac{152}{729} L_{ij33}^{V,LL} - \frac{2824}{729} L_{11ij}^{V1,LL} \\
& - \frac{2824}{729} L_{22ij}^{V1,LL} \Big] ;
\end{aligned}$$

$$\begin{aligned}
\dot{L}_{ijkk}^{V8,LR} &= g_s^2 \Bigg[ -12 L_{ijkk}^{V1,LR} - \frac{40}{3} L_{ijkk}^{V8,LR} + \frac{8}{3} L_{ikkj}^{V,LL} + \frac{2}{3} L_{ijii}^{V8,LR} + \frac{2}{3} L_{ijjj}^{V8,LR} \\
& + \frac{8}{3} L_{ijii}^{V,LL} + \frac{8}{3} L_{ijjj}^{V,LL} + \frac{2}{3} L_{ij11}^{V8,LR} + \frac{2}{3} L_{ij22}^{V8,LR} + \frac{2}{3} L_{11ij}^{V8,LL} + \frac{2}{3} L_{22ij}^{V8,LL} \Big] \\
& - \frac{4}{3} e^2 L_{ijkk}^{V8,LR} + \alpha_s^2 \Bigg[ -132 L_{ijkk}^{V1,LR} - \frac{25213}{162} L_{ijkk}^{V8,LR} - \frac{28}{3} L_{ikkj}^{V,LL} + \frac{3400}{81} L_{ikkj}^{V,LL} \\
& - \frac{22}{3} L_{ijii}^{V1,LR} - \frac{22}{3} L_{ijjj}^{V1,LR} + \frac{781}{81} L_{ijii}^{V8,LR} + \frac{781}{81} L_{ijjj}^{V8,LR} + \frac{1186}{27} L_{ijii}^{V,LL} + \frac{1186}{27} L_{ijjj}^{V,LL} \\
& - \frac{22}{3} L_{ij11}^{V1,LR} - \frac{22}{3} L_{ij22}^{V1,LR} + \frac{781}{81} L_{ij11}^{V8,LR} + \frac{781}{81} L_{ij22}^{V8,LR} - \frac{2}{3} L_{11ij}^{V1,LL} - \frac{2}{3} L_{22ij}^{V1,LL} \\
& + \frac{601}{81} L_{11ij}^{V8,LL} + \frac{601}{81} L_{22ij}^{V8,LL} \Big] + \alpha_s \alpha \Bigg[ \frac{152}{81} L_{ijkk}^{V1,LR} - \frac{4}{3} L_{ijkk}^{V8,LR} + \frac{520}{81} L_{ijkk}^{V,LL} \\
& - \frac{1040}{243} L_{ikkj}^{V,LL} + \frac{260}{81} L_{ijii}^{V1,LR} + \frac{260}{81} L_{ijjj}^{V1,LR} + \frac{14}{9} L_{ijii}^{V8,LR} + \frac{14}{9} L_{ijjj}^{V8,LR} + \frac{292}{81} L_{ijii}^{V,LL} \\
& + \frac{292}{81} L_{ijjj}^{V,LL} + \frac{260}{81} L_{ij11}^{V,LR} + \frac{260}{81} L_{ij22}^{V,LR} + \frac{260}{81} L_{ij33}^{V,LR} - \frac{520}{81} L_{ij11}^{V1,LR} - \frac{520}{81} L_{ij22}^{V1,LR}
\end{aligned}$$

$$\begin{aligned}
& + \frac{2}{3} L_{ij11}^{V8,LR} + \frac{2}{3} L_{ij22}^{V8,LR} + \frac{260}{81} L_{11ij}^{V,LL} + \frac{260}{81} L_{22ij}^{V,LL} + \frac{260}{81} L_{33ij}^{V,LL} - \frac{520}{81} L_{11ij}^{V1,LL} \\
& - \frac{520}{81} L_{22ij}^{V1,LL} + \frac{122}{27} L_{11ij}^{V8,LL} + \frac{122}{27} L_{22ij}^{V8,LL} \Big] + \frac{1790}{81} \alpha^2 L_{ijkk}^{V8,LR} ; \\
\dot{L}_{ijjj}^{V1,LR} = & - \frac{8}{3} g_s^2 L_{ijjj}^{V8,LR} + e^2 \Bigg[ \frac{4}{9} L_{ijkk}^{V1,LR} + \frac{8}{9} L_{ijkk}^{V,LL} + \frac{8}{27} L_{ikkj}^{V,LL} + \frac{4}{9} L_{ijii}^{V1,LR} \\
& - \frac{8}{9} L_{ijjj}^{V1,LR} + \frac{32}{27} L_{ddii}^{V,LL} + \frac{32}{27} L_{ddjj}^{V,LL} + \frac{4}{9} L_{ij11}^{V,LR} + \frac{4}{9} L_{ij22}^{V,LR} + \frac{4}{9} L_{ij33}^{V,LR} \\
& - \frac{8}{9} L_{ij11}^{V1,LR} - \frac{8}{9} L_{ij22}^{V1,LR} + \frac{4}{9} L_{11ij}^{V,LL} + \frac{4}{9} L_{22ij}^{V,LL} + \frac{4}{9} L_{33ij}^{V,LL} - \frac{8}{9} L_{11ij}^{V1,LL} \\
& - \frac{8}{9} L_{22ij}^{V1,LL} \Big] + \alpha_s^2 \Bigg[ 8 L_{ijkk}^{V1,LR} + \frac{44}{27} L_{ijkk}^{V8,LR} - 16 L_{ijkk}^{V,LL} - \frac{64}{27} L_{ikkj}^{V,LL} \\
& + 8 L_{ijii}^{V1,LR} - \frac{4}{3} L_{ijjj}^{V1,LR} + \frac{44}{27} L_{ijii}^{V8,LR} - \frac{2000}{27} L_{ijjj}^{V8,LR} - \frac{232}{9} L_{ijii}^{V,LL} - \frac{232}{9} L_{ijjj}^{V,LL} \\
& + 8 L_{ij11}^{V1,LR} + 8 L_{ij22}^{V1,LR} + \frac{44}{27} L_{ij11}^{V8,LR} + \frac{44}{27} L_{ij22}^{V8,LR} - 8 L_{11ij}^{V1,LL} - 8 L_{22ij}^{V1,LL} \\
& + \frac{44}{27} L_{11ij}^{V8,LL} + \frac{44}{27} L_{22ij}^{V8,LL} \Big] + \alpha_s \alpha \Bigg[ \frac{16}{9} L_{ijkk}^{V1,LR} - \frac{1010}{729} L_{ijkk}^{V8,LR} + \frac{8}{3} L_{ijkk}^{V,LL} \\
& + \frac{304}{729} L_{ikkj}^{V,LL} + \frac{16}{9} L_{ijii}^{V1,LR} + \frac{112}{9} L_{ijjj}^{V1,LR} - \frac{1010}{729} L_{ijii}^{V8,LR} - \frac{1226}{729} L_{ijjj}^{V8,LR} \\
& + \frac{1096}{243} L_{ijii}^{V,LL} + \frac{1096}{243} L_{ijjj}^{V,LL} - \frac{32}{9} L_{ij11}^{V1,LR} - \frac{32}{9} L_{ij22}^{V1,LR} + \frac{1366}{729} L_{ij11}^{V8,LR} + \frac{1366}{729} L_{ij22}^{V8,LR} \\
& - \frac{32}{9} L_{11ij}^{V1,LL} - \frac{32}{9} L_{22ij}^{V1,LL} - \frac{74}{729} L_{11ij}^{V8,LL} - \frac{74}{729} L_{22ij}^{V8,LL} \Big] + \alpha^2 \Bigg[ \frac{296}{729} L_{ijkk}^{V1,LR} \\
& + \frac{16}{729} L_{ijkk}^{V,LL} - \frac{752}{2187} L_{ikkj}^{V,LL} + \frac{296}{729} L_{ijii}^{V1,LR} + \frac{16406}{729} L_{ijjj}^{V1,LR} - \frac{608}{729} L_{ijii}^{V,LL} \\
& - \frac{608}{729} L_{ijjj}^{V,LL} + \frac{1016}{729} L_{ij11}^{V,LR} + \frac{1016}{729} L_{ij22}^{V,LR} + \frac{1016}{729} L_{ij33}^{V,LR} - \frac{1672}{729} L_{ij11}^{V1,LR} \\
& - \frac{1672}{729} L_{ij22}^{V1,LR} + \frac{152}{729} L_{11ij}^{V,LL} + \frac{152}{729} L_{22ij}^{V,LL} + \frac{152}{729} L_{33ij}^{V,LL} - \frac{2824}{729} L_{11ij}^{V1,LL} \\
& - \frac{2824}{729} L_{22ij}^{V1,LL} \Big] ;
\end{aligned}$$

$$\begin{aligned}
\dot{L}_{ijj}^{V8,LR} = & g_s^2 \left[ \frac{2}{3} L_{ijk}^{V8,LR} + \frac{8}{3} L_{ikk}^{V,LL} - 12 L_{ijj}^{V1,LR} + \frac{2}{3} L_{jii}^{V8,LR} - \frac{40}{3} L_{ijj}^{V8,LR} \right. \\
& + \frac{8}{3} L_{jii}^{V,LL} + \frac{8}{3} L_{ijj}^{V,LL} + \frac{2}{3} L_{ij11}^{V8,LR} + \frac{2}{3} L_{ij22}^{V8,LR} + \frac{2}{3} L_{11ij}^{V8,LL} + \left. \frac{2}{3} L_{22ij}^{V8,LL} \right] \\
& - \frac{4}{3} e^2 L_{ijj}^{V8,LR} + \alpha_s^2 \left[ -\frac{22}{3} L_{ijk}^{V1,LR} + \frac{781}{81} L_{ijk}^{V8,LR} - \frac{28}{3} L_{ijk}^{V,LL} + \frac{3400}{81} L_{ikk}^{V,LL} \right. \\
& - \frac{22}{3} L_{jii}^{V1,LR} - 132 L_{ijj}^{V1,LR} + \frac{781}{81} L_{jii}^{V8,LR} - \frac{25213}{162} L_{ijj}^{V8,LR} + \frac{1186}{27} L_{jii}^{V,LL} + \frac{1186}{27} L_{ijj}^{V,LL} \\
& - \frac{22}{3} L_{ij11}^{V1,LR} - \frac{22}{3} L_{ij22}^{V1,LR} + \frac{781}{81} L_{ij11}^{V8,LR} + \frac{781}{81} L_{ij22}^{V8,LR} - \frac{2}{3} L_{11ij}^{V1,LL} - \frac{2}{3} L_{22ij}^{V1,LL} \\
& + \left. \frac{601}{81} L_{11ij}^{V8,LL} + \frac{601}{81} L_{22ij}^{V8,LL} \right] + \alpha_s \alpha \left[ \frac{260}{81} L_{ijk}^{V1,LR} + \frac{14}{9} L_{ijk}^{V8,LR} + \frac{520}{81} L_{ijk}^{V,LL} \right. \\
& - \frac{1040}{243} L_{ikk}^{V,LL} + \frac{260}{81} L_{jii}^{V1,LR} + \frac{152}{81} L_{ijj}^{V1,LR} + \frac{14}{9} L_{jii}^{V8,LR} - \frac{4}{3} L_{ijj}^{V8,LR} + \frac{292}{81} L_{jii}^{V,LL} \\
& + \frac{292}{81} L_{ijj}^{V,LL} + \frac{260}{81} L_{ij11}^{V,LR} + \frac{260}{81} L_{ij22}^{V,LR} + \frac{260}{81} L_{ij33}^{V,LR} - \frac{520}{81} L_{ij11}^{V1,LR} - \frac{520}{81} L_{ij22}^{V1,LR} \\
& + \frac{2}{3} L_{ij11}^{V8,LR} + \frac{2}{3} L_{ij22}^{V8,LR} + \frac{260}{81} L_{11ij}^{V,LL} + \frac{260}{81} L_{22ij}^{V,LL} + \frac{260}{81} L_{33ij}^{V,LL} - \frac{520}{81} L_{11ij}^{V1,LL} \\
& - \left. \frac{520}{81} L_{22ij}^{V1,LL} + \frac{122}{27} L_{11ij}^{V8,LL} + \frac{122}{27} L_{22ij}^{V8,LL} \right] + \frac{1790}{81} \alpha^2 L_{ijj}^{V8,LR} ;
\end{aligned}$$

$$\begin{aligned}
\dot{L}_{jii}^{V1,LR} = & -\frac{8}{3} g_s^2 L_{jii}^{V8,LR} + e^2 \left[ \frac{4}{9} L_{ijk}^{V1,LR} + \frac{8}{9} L_{ikk}^{V,LL} + \frac{8}{27} L_{ikk}^{V,LL} - \frac{8}{9} L_{ijj}^{V1,LR} \right. \\
& + \frac{4}{9} L_{ijj}^{V1,LR} + \frac{32}{27} L_{jii}^{V,LL} + \frac{32}{27} L_{ijj}^{V,LL} + \frac{4}{9} L_{ij11}^{V,LR} + \frac{4}{9} L_{ij22}^{V,LR} + \frac{4}{9} L_{ij33}^{V,LR} \\
& - \frac{8}{9} L_{ij11}^{V1,LR} - \frac{8}{9} L_{ij22}^{V1,LR} + \frac{4}{9} L_{11ij}^{V,LL} + \frac{4}{9} L_{22ij}^{V,LL} + \frac{4}{9} L_{33ij}^{V,LL} - \frac{8}{9} L_{11ij}^{V1,LL} \\
& - \left. \frac{8}{9} L_{22ij}^{V1,LL} \right] + \alpha_s^2 \left[ 8 L_{ijk}^{V1,LR} + \frac{44}{27} L_{ijk}^{V8,LR} - 16 L_{ijk}^{V,LL} - \frac{64}{27} L_{ikk}^{V,LL} \right. \\
& - \frac{4}{3} L_{jii}^{V1,LR} + 8 L_{ijj}^{V1,LR} - \frac{2000}{27} L_{jii}^{V8,LR} + \frac{44}{27} L_{ijj}^{V8,LR} - \frac{232}{9} L_{jii}^{V,LL} - \frac{232}{9} L_{ijj}^{V,LL} \\
& + 8 L_{ij11}^{V1,LR} + 8 L_{ij22}^{V1,LR} + \frac{44}{27} L_{ij11}^{V8,LR} + \frac{44}{27} L_{ij22}^{V8,LR} - 8 L_{11ij}^{V1,LL} - 8 L_{22ij}^{V1,LL} \\
& + \left. 8 L_{33ij}^{V1,LL} \right]
\end{aligned}$$

$$\begin{aligned}
& + \frac{44}{27} L_{11ij}^{V8,LL} + \frac{44}{27} L_{22ij}^{V8,LL} \Big] + \alpha_s \alpha \Big[ \frac{16}{9} L_{ijkk}^{V1,LR} - \frac{1010}{729} L_{ijkk}^{V8,LR} + \frac{8}{3} L_{ijkk}^{V,LL} \\
& + \frac{304}{729} L_{ikkj}^{V,LL} + \frac{112}{9} L_{ijii}^{V1,LR} + \frac{16}{9} L_{ijjj}^{V1,LR} - \frac{1226}{729} L_{ijii}^{V8,LR} - \frac{1010}{729} L_{ijjj}^{V8,LR} \\
& + \frac{1096}{243} L_{ijii}^{V,LL} + \frac{1096}{243} L_{ijjj}^{V,LL} - \frac{32}{9} L_{ij11}^{V1,LR} - \frac{32}{9} L_{ij22}^{V1,LR} + \frac{1366}{729} L_{ij11}^{V8,LR} + \frac{1366}{729} L_{ij22}^{V8,LR} \\
& - \frac{32}{9} L_{11ij}^{V1,LL} - \frac{32}{9} L_{22ij}^{V1,LL} - \frac{74}{729} L_{11ij}^{V8,LL} - \frac{74}{729} L_{22ij}^{V8,LL} \Big] + \alpha^2 \Big[ \frac{296}{729} L_{ijkk}^{V1,LR} \\
& + \frac{16}{729} L_{ijkk}^{V,LL} - \frac{752}{2187} L_{ikkj}^{V,LL} + \frac{16406}{729} L_{ijii}^{V1,LR} + \frac{296}{729} L_{ijjj}^{V1,LR} - \frac{608}{729} L_{ijii}^{V,LL} \\
& - \frac{608}{729} L_{ijjj}^{V,LL} + \frac{1016}{729} L_{ij11}^{V,LR} + \frac{1016}{729} L_{ij22}^{V,LR} + \frac{1016}{729} L_{ij33}^{V,LR} - \frac{1672}{729} L_{ij11}^{V1,LR} \\
& - \frac{1672}{729} L_{ij22}^{V1,LR} + \frac{152}{729} L_{ij11}^{V,LL} + \frac{152}{729} L_{ij22}^{V,LL} + \frac{152}{729} L_{ij33}^{V,LL} - \frac{2824}{729} L_{11ij}^{V1,LL} \\
& - \frac{2824}{729} L_{22ij}^{V1,LL} \Big] ;
\end{aligned}$$

$$\begin{aligned}
\dot{L}_{ijii}^{V8,LR} & = g_s^2 \Big[ \frac{2}{3} L_{ijkk}^{V8,LR} + \frac{8}{3} L_{ikkj}^{V,LL} - 12 L_{ijii}^{V1,LR} - \frac{40}{3} L_{ijii}^{V8,LR} + \frac{2}{3} L_{ijjj}^{V8,LR} \\
& + \frac{8}{3} L_{ijii}^{V,LL} + \frac{8}{3} L_{ijjj}^{V,LL} + \frac{2}{3} L_{ij11}^{V8,LR} + \frac{2}{3} L_{ij22}^{V8,LR} + \frac{2}{3} L_{11ij}^{V8,LL} + \frac{2}{3} L_{22ij}^{V8,LL} \Big] \\
& - \frac{4}{3} e^2 L_{ijii}^{V8,LR} + \alpha_s^2 \Big[ - \frac{22}{3} L_{ijkk}^{V1,LR} + \frac{781}{81} L_{ijkk}^{V8,LR} - \frac{28}{3} L_{ijkk}^{V,LL} + \frac{3400}{81} L_{ikkj}^{V,LL} \\
& - 132 L_{ijii}^{V1,LR} - \frac{22}{3} L_{ijjj}^{V1,LR} - \frac{25213}{162} L_{ijii}^{V8,LR} + \frac{781}{81} L_{ijjj}^{V8,LR} + \frac{1186}{27} L_{ijii}^{V,LL} + \frac{1186}{27} L_{ijjj}^{V,LL} \\
& - \frac{22}{3} L_{ij11}^{V1,LR} - \frac{22}{3} L_{ij22}^{V1,LR} + \frac{781}{81} L_{ij11}^{V8,LR} + \frac{781}{81} L_{ij22}^{V8,LR} - \frac{2}{3} L_{11ij}^{V1,LL} - \frac{2}{3} L_{22ij}^{V1,LL} \\
& + \frac{601}{81} L_{11ij}^{V8,LL} + \frac{601}{81} L_{22ij}^{V8,LL} \Big] + \alpha_s \alpha \Big[ \frac{260}{81} L_{ijkk}^{V1,LR} + \frac{14}{9} L_{ijkk}^{V8,LR} + \frac{520}{81} L_{ijkk}^{V,LL} \\
& - \frac{1040}{243} L_{ikkj}^{V,LL} + \frac{152}{81} L_{ijii}^{V1,LR} + \frac{260}{81} L_{ijjj}^{V1,LR} - \frac{4}{3} L_{ijii}^{V8,LR} + \frac{14}{9} L_{ijjj}^{V8,LR} + \frac{292}{81} L_{ijii}^{V,LL} \\
& + \frac{292}{81} L_{ijjj}^{V,LL} + \frac{260}{81} L_{ij11}^{V,LR} + \frac{260}{81} L_{ij22}^{V,LR} + \frac{260}{81} L_{ij33}^{V,LR} - \frac{520}{81} L_{ij11}^{V1,LR} - \frac{520}{81} L_{ij22}^{V1,LR}
\end{aligned}$$

$$\begin{aligned}
& + \frac{2}{3} L_{ij11}^{V8,LR} + \frac{2}{3} L_{ij22}^{V8,LR} + \frac{260}{81} L_{11ij}^{V,LL} + \frac{260}{81} L_{22ij}^{V,LL} + \frac{260}{81} L_{33ij}^{V,LL} - \frac{520}{81} L_{11ij}^{V1,LL} \\
& - \frac{520}{81} L_{22ij}^{V1,LL} + \frac{122}{27} L_{11ij}^{V8,LL} + \frac{122}{27} L_{22ij}^{V8,LL} \Big] + \frac{1790}{81} \alpha^2 L_{ijii}^{V8,LR} ; \\
\dot{L}_{ed11ij}^{S,RL} & = -8g_s^2 L_{ed11ij}^{S,RL} - \frac{20}{3} e^2 L_{ed11ij}^{S,RL} - \frac{1012}{9} \alpha_s^2 L_{ed11ij}^{S,RL} - \frac{8}{9} \alpha_s \alpha L_{ed11ij}^{S,RL} \\
& + \frac{6958}{81} \alpha^2 L_{ed11ij}^{S,RL} ; \\
\dot{L}_{ed22ij}^{S,RL} & = -8g_s^2 L_{ed22ij}^{S,RL} - \frac{20}{3} e^2 L_{ed22ij}^{S,RL} - \frac{1012}{9} \alpha_s^2 L_{ed22ij}^{S,RL} - \frac{8}{9} \alpha_s \alpha L_{ed22ij}^{S,RL} \\
& + \frac{6958}{81} \alpha^2 L_{ed22ij}^{S,RL} ; \\
\dot{L}_{ed33ij}^{S,RL} & = -8g_s^2 L_{ed33ij}^{S,RL} - \frac{20}{3} e^2 L_{ed33ij}^{S,RL} - \frac{1012}{9} \alpha_s^2 L_{ed33ij}^{S,RL} - \frac{8}{9} \alpha_s \alpha L_{ed33ij}^{S,RL} \\
& + \frac{6958}{81} \alpha^2 L_{ed33ij}^{S,RL} ; \\
\dot{L}_{uddu1ji1}^{V1,LR} & = -\frac{8}{3} g_s^2 L_{uddu1ji1}^{V8,LR} - \frac{10}{3} e^2 L_{uddu1ji1}^{V1,LR} + \alpha_s^2 \left[ -\frac{28}{3} L_{uddu1ji1}^{V1,LR} - \frac{2044}{27} L_{uddu1ji1}^{V8,LR} \right] \\
& + \alpha_s \alpha \left[ \frac{8}{3} L_{uddu1ji1}^{V1,LR} - \frac{128}{27} L_{uddu1ji1}^{V8,LR} \right] + \frac{173}{81} \alpha^2 L_{uddu1ji1}^{V1,LR} ; \\
\dot{L}_{uddu1ji1}^{V8,LR} & = g_s^2 \left[ -12 L_{uddu1ji1}^{V1,LR} - 14 L_{uddu1ji1}^{V8,LR} \right] - \frac{10}{3} e^2 L_{uddu1ji1}^{V8,LR} + \alpha_s^2 \left[ -\frac{374}{3} L_{uddu1ji1}^{V1,LR} \right. \\
& \left. - \frac{2975}{18} L_{uddu1ji1}^{V8,LR} \right] + \alpha_s \alpha \left[ \frac{16}{9} L_{uddu1ji1}^{V8,LR} - \frac{64}{3} L_{uddu1ji1}^{V1,LR} \right] + \frac{173}{81} \alpha^2 L_{uddu1ji1}^{V8,LR} ; \\
\dot{L}_{uddu2ji2}^{V1,LR} & = -\frac{8}{3} g_s^2 L_{uddu2ji2}^{V8,LR} - \frac{10}{3} e^2 L_{uddu2ji2}^{V1,LR} + \alpha_s^2 \left[ -\frac{28}{3} L_{uddu2ji2}^{V1,LR} - \frac{2044}{27} L_{uddu2ji2}^{V8,LR} \right] \\
& + \alpha_s \alpha \left[ \frac{8}{3} L_{uddu2ji2}^{V1,LR} - \frac{128}{27} L_{uddu2ji2}^{V8,LR} \right] + \frac{173}{81} \alpha^2 L_{uddu2ji2}^{V1,LR} ; \\
\dot{L}_{uddu2ji2}^{V8,LR} & = g_s^2 \left[ -12 L_{uddu2ji2}^{V1,LR} - 14 L_{uddu2ji2}^{V8,LR} \right] - \frac{10}{3} e^2 L_{uddu2ji2}^{V8,LR} + \alpha_s^2 \left[ -\frac{374}{3} L_{uddu2ji2}^{V1,LR} \right. \\
& \left. - \frac{2975}{18} L_{uddu2ji2}^{V8,LR} \right] + \alpha_s \alpha \left[ \frac{16}{9} L_{uddu2ji2}^{V8,LR} - \frac{64}{3} L_{uddu2ji2}^{V1,LR} \right] + \frac{173}{81} \alpha^2 L_{uddu2ji2}^{V8,LR} ;
\end{aligned}$$



$$\begin{aligned}
\dot{L}_{dd\,kjik}^{V1,LR} &= -\frac{8}{3}g_s^2 L_{dd\,kjik}^{V8,LR} - \frac{4}{3}e^2 L_{dd\,kjik}^{V1,LR} + \alpha_s^2 \left[ -\frac{28}{3} L_{dd\,kjik}^{V1,LR} - \frac{2044}{27} L_{dd\,kjik}^{V8,LR} \right] \\
&\quad + \alpha_s \alpha \left[ \frac{32}{3} L_{dd\,kjik}^{V1,LR} - \frac{8}{27} L_{dd\,kjik}^{V8,LR} \right] + \frac{1790}{81} \alpha^2 L_{dd\,kjik}^{V1,LR} ; \\
\dot{L}_{dd\,kjik}^{V8,LR} &= g_s^2 \left[ -12 L_{dd\,kjik}^{V1,LR} - 14 L_{dd\,kjik}^{V8,LR} \right] - \frac{4}{3}e^2 L_{dd\,kjik}^{V8,LR} + \alpha_s^2 \left[ -\frac{374}{3} L_{dd\,kjik}^{V1,LR} \right. \\
&\quad \left. - \frac{2975}{18} L_{dd\,kjik}^{V8,LR} \right] + \alpha_s \alpha \left[ -\frac{4}{3} L_{dd\,kjik}^{V1,LR} - \frac{26}{9} L_{dd\,kjik}^{V8,LR} \right] + \frac{1790}{81} \alpha^2 L_{dd\,kjik}^{V8,LR} ; \\
\dot{L}_{ed\,11ij}^{S,RR} &= -8g_s^2 L_{ed\,11ij}^{S,RR} + e^2 \left[ -\frac{20}{3} L_{ed\,11ij}^{S,RR} - 32 L_{ed\,11ij}^{T,RR} \right] - \frac{1012}{9} \alpha_s^2 L_{ed\,11ij}^{S,RR} \\
&\quad + \alpha_s \alpha \left[ \frac{1792}{9} L_{ed\,11ij}^{T,RR} - \frac{8}{9} L_{ed\,11ij}^{S,RR} \right] + \alpha^2 \left[ \frac{1882}{81} L_{ed\,11ij}^{S,RR} + \frac{19712}{27} L_{ed\,11ij}^{T,RR} \right] ; \\
\dot{L}_{ed\,11ij}^{T,RR} &= \frac{8}{3}g_s^2 L_{ed\,11ij}^{T,RR} + e^2 \left[ \frac{20}{9} L_{ed\,11ij}^{T,RR} - \frac{2}{3} L_{ed\,11ij}^{S,RR} \right] + \frac{1652}{27} \alpha_s^2 L_{ed\,11ij}^{T,RR} \\
&\quad + \alpha_s \alpha \left[ \frac{16}{3} L_{ed\,11ij}^{S,RR} - \frac{152}{27} L_{ed\,11ij}^{T,RR} \right] + \alpha^2 \left[ \frac{368}{81} L_{ed\,11ij}^{S,RR} - \frac{7154}{243} L_{ed\,11ij}^{T,RR} \right] ; \\
\dot{L}_{ed\,22ij}^{S,RR} &= -8g_s^2 L_{ed\,22ij}^{S,RR} + e^2 \left[ -\frac{20}{3} L_{ed\,22ij}^{S,RR} - 32 L_{ed\,22ij}^{T,RR} \right] - \frac{1012}{9} \alpha_s^2 L_{ed\,22ij}^{S,RR} \\
&\quad + \alpha_s \alpha \left[ \frac{1792}{9} L_{ed\,22ij}^{T,RR} - \frac{8}{9} L_{ed\,22ij}^{S,RR} \right] + \alpha^2 \left[ \frac{1882}{81} L_{ed\,22ij}^{S,RR} + \frac{19712}{27} L_{ed\,22ij}^{T,RR} \right] ; \\
\dot{L}_{ed\,22ij}^{T,RR} &= \frac{8}{3}g_s^2 L_{ed\,22ij}^{T,RR} + e^2 \left[ \frac{20}{9} L_{ed\,22ij}^{T,RR} - \frac{2}{3} L_{ed\,22ij}^{S,RR} \right] + \frac{1652}{27} \alpha_s^2 L_{ed\,22ij}^{T,RR} \\
&\quad + \alpha_s \alpha \left[ \frac{16}{3} L_{ed\,22ij}^{S,RR} - \frac{152}{27} L_{ed\,22ij}^{T,RR} \right] + \alpha^2 \left[ \frac{368}{81} L_{ed\,22ij}^{S,RR} - \frac{7154}{243} L_{ed\,22ij}^{T,RR} \right] ; \\
\dot{L}_{ed\,33ij}^{S,RR} &= -8g_s^2 L_{ed\,33ij}^{S,RR} + e^2 \left[ -\frac{20}{3} L_{ed\,33ij}^{S,RR} - 32 L_{ed\,33ij}^{T,RR} \right] - \frac{1012}{9} \alpha_s^2 L_{ed\,33ij}^{S,RR} \\
&\quad + \alpha_s \alpha \left[ \frac{1792}{9} L_{ed\,33ij}^{T,RR} - \frac{8}{9} L_{ed\,33ij}^{S,RR} \right] + \alpha^2 \left[ \frac{1882}{81} L_{ed\,33ij}^{S,RR} + \frac{19712}{27} L_{ed\,33ij}^{T,RR} \right] ;
\end{aligned}$$

$$\begin{aligned}\dot{L}_{33ij}^{T,RR} &= \frac{8}{3}g_s^2 L_{33ij}^{T,RR} + e^2 \left[ \frac{20}{9} L_{33ij}^{T,RR} - \frac{2}{3} L_{33ij}^{S,RR} \right] + \frac{1652}{27} \alpha_s^2 L_{33ij}^{T,RR} \\ &\quad + \alpha_s \alpha \left[ \frac{16}{3} L_{33ij}^{S,RR} - \frac{152}{27} L_{33ij}^{T,RR} \right] + \alpha^2 \left[ \frac{368}{81} L_{33ij}^{S,RR} - \frac{7154}{243} L_{33ij}^{T,RR} \right];\end{aligned}$$

$$\begin{aligned}\dot{L}_{11ij}^{S1,RR} &= g_s^2 \left[ \frac{64}{9} L_{1ji1}^{S1,RR} + \frac{112}{27} L_{1ji1}^{S8,RR} - 16 L_{11ij}^{S1,RR} + \frac{16}{9} L_{11ij}^{S8,RR} \right] \\ &\quad + e^2 \left[ \frac{4}{27} L_{1ji1}^{S1,RR} + \frac{16}{81} L_{1ji1}^{S8,RR} - \frac{46}{9} L_{11ij}^{S1,RR} \right] + \alpha_s^2 \left[ \frac{9472}{81} L_{1ji1}^{S1,RR} + \frac{16576}{243} L_{1ji1}^{S8,RR} \right. \\ &\quad \left. - \frac{2120}{9} L_{11ij}^{S1,RR} + \frac{928}{81} L_{11ij}^{S8,RR} \right] + \alpha_s \alpha \left[ \frac{1888}{81} L_{1ji1}^{S1,RR} + \frac{3808}{243} L_{1ji1}^{S8,RR} + \frac{136}{27} L_{11ij}^{S1,RR} \right. \\ &\quad \left. + \frac{224}{81} L_{11ij}^{S8,RR} \right] + \alpha^2 \left[ \frac{98}{729} L_{1ji1}^{S1,RR} + \frac{392}{2187} L_{1ji1}^{S8,RR} + \frac{6391}{243} L_{11ij}^{S1,RR} \right];\end{aligned}$$

$$\begin{aligned}\dot{L}_{11ij}^{S8,RR} &= g_s^2 \left[ -\frac{16}{3} L_{1ji1}^{S1,RR} + \frac{44}{9} L_{1ji1}^{S8,RR} + 8 L_{11ij}^{S1,RR} + \frac{16}{3} L_{11ij}^{S8,RR} \right] \\ &\quad + e^2 \left[ \frac{8}{9} L_{1ji1}^{S1,RR} - \frac{4}{27} L_{1ji1}^{S8,RR} - \frac{46}{9} L_{11ij}^{S8,RR} \right] + \alpha_s^2 \left[ -\frac{856}{27} L_{1ji1}^{S1,RR} - \frac{2506}{81} L_{1ji1}^{S8,RR} \right. \\ &\quad \left. + \frac{248}{9} L_{11ij}^{S1,RR} + \frac{2995}{27} L_{11ij}^{S8,RR} \right] + \alpha_s \alpha \left[ -\frac{868}{27} L_{1ji1}^{S1,RR} + \frac{1370}{81} L_{1ji1}^{S8,RR} + \frac{112}{9} L_{11ij}^{S1,RR} \right. \\ &\quad \left. + \frac{224}{9} L_{11ij}^{S8,RR} \right] + \alpha^2 \left[ \frac{196}{243} L_{1ji1}^{S1,RR} - \frac{98}{729} L_{1ji1}^{S8,RR} + \frac{6391}{243} L_{11ij}^{S8,RR} \right];\end{aligned}$$

$$\begin{aligned}\dot{L}_{1ji1}^{S1,RR} &= g_s^2 \left[ -16 L_{1ji1}^{S1,RR} + \frac{16}{9} L_{1ji1}^{S8,RR} + \frac{64}{9} L_{11ij}^{S1,RR} + \frac{112}{27} L_{11ij}^{S8,RR} \right] \\ &\quad + e^2 \left[ \frac{26}{9} L_{1ji1}^{S1,RR} - \frac{32}{27} L_{11ij}^{S1,RR} - \frac{128}{81} L_{11ij}^{S8,RR} \right] + \alpha_s^2 \left[ -\frac{2120}{9} L_{1ji1}^{S1,RR} + \frac{928}{81} L_{1ji1}^{S8,RR} \right. \\ &\quad \left. + \frac{9472}{81} L_{11ij}^{S1,RR} + \frac{16576}{243} L_{11ij}^{S8,RR} \right] + \alpha_s \alpha \left[ \frac{712}{27} L_{1ji1}^{S1,RR} - \frac{64}{81} L_{1ji1}^{S8,RR} - \frac{2144}{81} L_{11ij}^{S1,RR} \right. \\ &\quad \left. - \frac{7784}{243} L_{11ij}^{S8,RR} \right] + \alpha^2 \left[ -\frac{13769}{243} L_{1ji1}^{S1,RR} + \frac{5264}{729} L_{11ij}^{S1,RR} + \frac{21056}{2187} L_{11ij}^{S8,RR} \right];\end{aligned}$$

$$\begin{aligned}
\dot{L}_{1ji1}^{S8,RR} &= g_s^2 \left[ 8L_{1ji1}^{S1,RR} + \frac{16}{3}L_{1ji1}^{S8,RR} - \frac{16}{3}L_{11ij}^{S1,RR} + \frac{44}{9}L_{11ij}^{S8,RR} \right] \\
&+ e^2 \left[ \frac{26}{9}L_{1ji1}^{S8,RR} - \frac{64}{9}L_{11ij}^{S1,RR} + \frac{32}{27}L_{11ij}^{S8,RR} \right] + \alpha_s^2 \left[ \frac{248}{9}L_{1ji1}^{S1,RR} + \frac{2995}{27}L_{1ji1}^{S8,RR} \right. \\
&- \frac{856}{27}L_{11ij}^{S1,RR} - \frac{2506}{81}L_{11ij}^{S8,RR} \left. \right] + \alpha_s \alpha \left[ -\frac{32}{9}L_{1ji1}^{S1,RR} - \frac{400}{9}L_{1ji1}^{S8,RR} + \frac{3704}{27}L_{11ij}^{S1,RR} \right. \\
&- \frac{2050}{81}L_{11ij}^{S8,RR} \left. \right] + \alpha^2 \left[ -\frac{13769}{243}L_{1ji1}^{S8,RR} + \frac{10528}{243}L_{11ij}^{S1,RR} - \frac{5264}{729}L_{11ij}^{S8,RR} \right]; \\
\dot{L}_{2ji2}^{S1,RR} &= g_s^2 \left[ \frac{64}{9}L_{2ji2}^{S1,RR} + \frac{112}{27}L_{2ji2}^{S8,RR} - 16L_{22ij}^{S1,RR} + \frac{16}{9}L_{22ij}^{S8,RR} \right] \\
&+ e^2 \left[ \frac{4}{27}L_{2ji2}^{S1,RR} + \frac{16}{81}L_{2ji2}^{S8,RR} - \frac{46}{9}L_{22ij}^{S1,RR} \right] + \alpha_s^2 \left[ \frac{9472}{81}L_{2ji2}^{S1,RR} + \frac{16576}{243}L_{2ji2}^{S8,RR} \right. \\
&- \frac{2120}{9}L_{22ij}^{S1,RR} + \frac{928}{81}L_{22ij}^{S8,RR} \left. \right] + \alpha_s \alpha \left[ \frac{1888}{81}L_{2ji2}^{S1,RR} + \frac{3808}{243}L_{2ji2}^{S8,RR} + \frac{136}{27}L_{22ij}^{S1,RR} \right. \\
&+ \frac{224}{81}L_{22ij}^{S8,RR} \left. \right] + \alpha^2 \left[ \frac{98}{729}L_{2ji2}^{S1,RR} + \frac{392}{2187}L_{2ji2}^{S8,RR} + \frac{6391}{243}L_{22ij}^{S1,RR} \right]; \\
\dot{L}_{2ji2}^{S8,RR} &= g_s^2 \left[ -\frac{16}{3}L_{2ji2}^{S1,RR} + \frac{44}{9}L_{2ji2}^{S8,RR} + 8L_{22ij}^{S1,RR} + \frac{16}{3}L_{22ij}^{S8,RR} \right] \\
&+ e^2 \left[ \frac{8}{9}L_{2ji2}^{S1,RR} - \frac{4}{27}L_{2ji2}^{S8,RR} - \frac{46}{9}L_{22ij}^{S8,RR} \right] + \alpha_s^2 \left[ -\frac{856}{27}L_{2ji2}^{S1,RR} - \frac{2506}{81}L_{2ji2}^{S8,RR} \right. \\
&+ \frac{248}{9}L_{22ij}^{S1,RR} + \frac{2995}{27}L_{22ij}^{S8,RR} \left. \right] + \alpha_s \alpha \left[ -\frac{868}{27}L_{2ji2}^{S1,RR} + \frac{1370}{81}L_{2ji2}^{S8,RR} + \frac{112}{9}L_{22ij}^{S1,RR} \right. \\
&+ \frac{224}{9}L_{22ij}^{S8,RR} \left. \right] + \alpha^2 \left[ \frac{196}{243}L_{2ji2}^{S1,RR} - \frac{98}{729}L_{2ji2}^{S8,RR} + \frac{6391}{243}L_{22ij}^{S8,RR} \right]; \\
\dot{L}_{2ji2}^{S1,RR} &= g_s^2 \left[ -16L_{2ji2}^{S1,RR} + \frac{16}{9}L_{2ji2}^{S8,RR} + \frac{64}{9}L_{22ij}^{S1,RR} + \frac{112}{27}L_{22ij}^{S8,RR} \right] \\
&+ e^2 \left[ \frac{26}{9}L_{2ji2}^{S1,RR} - \frac{32}{27}L_{22ij}^{S1,RR} - \frac{128}{81}L_{22ij}^{S8,RR} \right] + \alpha_s^2 \left[ -\frac{2120}{9}L_{2ji2}^{S1,RR} + \frac{928}{81}L_{2ji2}^{S8,RR} \right.
\end{aligned}$$

$$\begin{aligned}
& + \frac{9472}{81} L_{ud,22ij}^{S1,RR} + \frac{16576}{243} L_{ud,22ij}^{S8,RR} \Big] + \alpha_s \alpha \left[ \frac{712}{27} L_{uddu,2ji2}^{S1,RR} - \frac{64}{81} L_{uddu,2ji2}^{S8,RR} - \frac{2144}{81} L_{ud,22ij}^{S1,RR} \right. \\
& \left. - \frac{7784}{243} L_{ud,22ij}^{S8,RR} \right] + \alpha^2 \left[ - \frac{13769}{243} L_{uddu,2ji2}^{S1,RR} + \frac{5264}{729} L_{ud,22ij}^{S1,RR} + \frac{21056}{2187} L_{ud,22ij}^{S8,RR} \right]; \\
\dot{L}_{uddu,2ji2}^{S8,RR} &= g_s^2 \left[ 8 L_{uddu,2ji2}^{S1,RR} + \frac{16}{3} L_{uddu,2ji2}^{S8,RR} - \frac{16}{3} L_{ud,22ij}^{S1,RR} + \frac{44}{9} L_{ud,22ij}^{S8,RR} \right] \\
& + e^2 \left[ \frac{26}{9} L_{uddu,2ji2}^{S8,RR} - \frac{64}{9} L_{ud,22ij}^{S1,RR} + \frac{32}{27} L_{ud,22ij}^{S8,RR} \right] + \alpha_s^2 \left[ \frac{248}{9} L_{uddu,2ji2}^{S1,RR} + \frac{2995}{27} L_{uddu,2ji2}^{S8,RR} \right. \\
& \left. - \frac{856}{27} L_{ud,22ij}^{S1,RR} - \frac{2506}{81} L_{ud,22ij}^{S8,RR} \right] + \alpha_s \alpha \left[ - \frac{32}{9} L_{uddu,2ji2}^{S1,RR} - \frac{400}{9} L_{uddu,2ji2}^{S8,RR} + \frac{3704}{27} L_{ud,22ij}^{S1,RR} \right. \\
& \left. - \frac{2050}{81} L_{ud,22ij}^{S8,RR} \right] + \alpha^2 \left[ - \frac{13769}{243} L_{uddu,2ji2}^{S8,RR} + \frac{10528}{243} L_{ud,22ij}^{S1,RR} - \frac{5264}{729} L_{ud,22ij}^{S8,RR} \right]; \\
\dot{L}_{dd,ijkk}^{S1,RR} &= g_s^2 \left[ -16 L_{dd,ijkk}^{S1,RR} + \frac{64}{9} L_{dd,ikkj}^{S1,RR} + \frac{16}{9} L_{dd,ijkk}^{S8,RR} + \frac{112}{27} L_{dd,ikkj}^{S8,RR} \right] \\
& + e^2 \left[ - \frac{4}{9} L_{dd,ijkk}^{S1,RR} + \frac{16}{27} L_{dd,ikkj}^{S1,RR} + \frac{64}{81} L_{dd,ikkj}^{S8,RR} \right] + \alpha_s^2 \left[ - \frac{2120}{9} L_{dd,ijkk}^{S1,RR} + \frac{9472}{81} L_{dd,ikkj}^{S1,RR} \right. \\
& + \frac{928}{81} L_{dd,ijkk}^{S8,RR} + \frac{16576}{243} L_{dd,ikkj}^{S8,RR} \Big] + \alpha_s \alpha \left[ - \frac{176}{27} L_{dd,ijkk}^{S1,RR} - \frac{512}{81} L_{dd,ikkj}^{S1,RR} - \frac{256}{81} L_{dd,ijkk}^{S8,RR} \right. \\
& \left. + \frac{1120}{243} L_{dd,ikkj}^{S8,RR} \right] + \alpha^2 \left[ \frac{1822}{243} L_{dd,ijkk}^{S1,RR} - \frac{832}{729} L_{dd,ikkj}^{S1,RR} - \frac{3328}{2187} L_{dd,ikkj}^{S8,RR} \right]; \\
\dot{L}_{dd,ijkk}^{S8,RR} &= g_s^2 \left[ 8 L_{dd,ijkk}^{S1,RR} - \frac{16}{3} L_{dd,ikkj}^{S1,RR} + \frac{16}{3} L_{dd,ijkk}^{S8,RR} + \frac{44}{9} L_{dd,ikkj}^{S8,RR} \right] + e^2 \left[ \frac{32}{9} L_{dd,ikkj}^{S1,RR} \right. \\
& \left. - \frac{4}{9} L_{dd,ijkk}^{S8,RR} - \frac{16}{27} L_{dd,ikkj}^{S8,RR} \right] + \alpha_s^2 \left[ \frac{248}{9} L_{dd,ijkk}^{S1,RR} - \frac{856}{27} L_{dd,ikkj}^{S1,RR} + \frac{2995}{27} L_{dd,ijkk}^{S8,RR} \right. \\
& \left. - \frac{2506}{81} L_{dd,ikkj}^{S8,RR} \right] + \alpha_s \alpha \left[ - \frac{128}{9} L_{dd,ijkk}^{S1,RR} - \frac{1456}{27} L_{dd,ikkj}^{S1,RR} - \frac{16}{9} L_{dd,ijkk}^{S8,RR} - \frac{64}{81} L_{dd,ikkj}^{S8,RR} \right] \\
& + \alpha^2 \left[ - \frac{1664}{243} L_{dd,ikkj}^{S1,RR} + \frac{1822}{243} L_{dd,ijkk}^{S8,RR} + \frac{832}{729} L_{dd,ikkj}^{S8,RR} \right];
\end{aligned}$$

$$\begin{aligned}
\dot{L}_{ikkj}^{S1,RR} = & g_s^2 \left[ \frac{64}{9} L_{ijkk}^{S1,RR} - 16 L_{ikkj}^{S1,RR} + \frac{112}{27} L_{ijkk}^{S8,RR} + \frac{16}{9} L_{ikkj}^{S8,RR} \right] \\
& + e^2 \left[ \frac{16}{27} L_{ijkk}^{S1,RR} - \frac{4}{9} L_{ikkj}^{S1,RR} + \frac{64}{81} L_{ijkk}^{S8,RR} \right] + \alpha_s^2 \left[ \frac{9472}{81} L_{ijkk}^{S1,RR} - \frac{2120}{9} L_{ikkj}^{S1,RR} \right. \\
& + \frac{16576}{243} L_{ijkk}^{S8,RR} + \frac{928}{81} L_{ikkj}^{S8,RR} \left. \right] + \alpha_s \alpha \left[ -\frac{512}{81} L_{ijkk}^{S1,RR} - \frac{176}{27} L_{ikkj}^{S1,RR} + \frac{1120}{243} L_{ijkk}^{S8,RR} \right. \\
& \left. - \frac{256}{81} L_{ikkj}^{S8,RR} \right] + \alpha^2 \left[ -\frac{832}{729} L_{ijkk}^{S1,RR} + \frac{1822}{243} L_{ikkj}^{S1,RR} - \frac{3328}{2187} L_{ijkk}^{S8,RR} \right];
\end{aligned}$$

$$\begin{aligned}
\dot{L}_{ikkj}^{S8,RR} = & g_s^2 \left[ -\frac{16}{3} L_{ijkk}^{S1,RR} + 8 L_{ikkj}^{S1,RR} + \frac{44}{9} L_{ijkk}^{S8,RR} + \frac{16}{3} L_{ikkj}^{S8,RR} \right] \\
& + e^2 \left[ \frac{32}{9} L_{ijkk}^{S1,RR} - \frac{16}{27} L_{ijkk}^{S8,RR} - \frac{4}{9} L_{ikkj}^{S8,RR} \right] + \alpha_s^2 \left[ -\frac{856}{27} L_{ijkk}^{S1,RR} + \frac{248}{9} L_{ikkj}^{S1,RR} \right. \\
& - \frac{2506}{81} L_{ijkk}^{S8,RR} + \frac{2995}{27} L_{ikkj}^{S8,RR} \left. \right] + \alpha_s \alpha \left[ -\frac{1456}{27} L_{ijkk}^{S1,RR} - \frac{128}{9} L_{ikkj}^{S1,RR} - \frac{64}{81} L_{ijkk}^{S8,RR} \right. \\
& \left. - \frac{16}{9} L_{ikkj}^{S8,RR} \right] + \alpha^2 \left[ -\frac{1664}{243} L_{ijkk}^{S1,RR} + \frac{832}{729} L_{ijkk}^{S8,RR} + \frac{1822}{243} L_{ikkj}^{S8,RR} \right];
\end{aligned}$$

$$\begin{aligned}
\dot{L}_{ijjj}^{S1,RR} = & g_s^2 \left[ \frac{160}{27} L_{ijjj}^{S8,RR} - \frac{80}{9} L_{ijjj}^{S1,RR} \right] + e^2 \left[ \frac{4}{27} L_{ijjj}^{S1,RR} + \frac{64}{81} L_{ijjj}^{S8,RR} \right] \\
& + \alpha_s^2 \left[ \frac{19360}{243} L_{ijjj}^{S8,RR} - \frac{9608}{81} L_{ijjj}^{S1,RR} \right] + \alpha_s \alpha \left[ \frac{352}{243} L_{ijjj}^{S8,RR} - \frac{1040}{81} L_{ijjj}^{S1,RR} \right] \\
& + \alpha^2 \left[ \frac{4634}{729} L_{ijjj}^{S1,RR} - \frac{3328}{2187} L_{ijjj}^{S8,RR} \right];
\end{aligned}$$

$$\begin{aligned}
\dot{L}_{ijjj}^{S8,RR} = & g_s^2 \left[ \frac{8}{3} L_{ijjj}^{S1,RR} + \frac{92}{9} L_{ijjj}^{S8,RR} \right] + e^2 \left[ \frac{32}{9} L_{ijjj}^{S1,RR} - \frac{28}{27} L_{ijjj}^{S8,RR} \right] \\
& + \alpha_s^2 \left[ \frac{6479}{81} L_{ijjj}^{S8,RR} - \frac{112}{27} L_{ijjj}^{S1,RR} \right] + \alpha_s \alpha \left[ -\frac{1840}{27} L_{ijjj}^{S1,RR} - \frac{208}{81} L_{ijjj}^{S8,RR} \right] \\
& + \alpha^2 \left[ \frac{6298}{729} L_{ijjj}^{S8,RR} - \frac{1664}{243} L_{ijjj}^{S1,RR} \right];
\end{aligned}$$

$$\begin{aligned}
\dot{L}_{dd\,ij\bar{i}\bar{j}}^{S1,RR} &= g_s^2 \left[ \frac{160}{27} L_{dd\,ij\bar{i}\bar{j}}^{S8,RR} - \frac{80}{9} L_{dd\,ij\bar{i}\bar{j}}^{S1,RR} \right] + e^2 \left[ \frac{4}{27} L_{dd\,ij\bar{i}\bar{j}}^{S1,RR} + \frac{64}{81} L_{dd\,ij\bar{i}\bar{j}}^{S8,RR} \right] \\
&+ \alpha_s^2 \left[ \frac{19360}{243} L_{dd\,ij\bar{i}\bar{j}}^{S8,RR} - \frac{9608}{81} L_{dd\,ij\bar{i}\bar{j}}^{S1,RR} \right] + \alpha_s \alpha \left[ \frac{352}{243} L_{dd\,ij\bar{i}\bar{j}}^{S8,RR} - \frac{1040}{81} L_{dd\,ij\bar{i}\bar{j}}^{S1,RR} \right] \\
&+ \alpha^2 \left[ \frac{4634}{729} L_{dd\,ij\bar{i}\bar{j}}^{S1,RR} - \frac{3328}{2187} L_{dd\,ij\bar{i}\bar{j}}^{S8,RR} \right]; \\
\dot{L}_{dd\,ij\bar{i}\bar{j}}^{S8,RR} &= g_s^2 \left[ \frac{8}{3} L_{dd\,ij\bar{i}\bar{j}}^{S1,RR} + \frac{92}{9} L_{dd\,ij\bar{i}\bar{j}}^{S8,RR} \right] + e^2 \left[ \frac{32}{9} L_{dd\,ij\bar{i}\bar{j}}^{S1,RR} - \frac{28}{27} L_{dd\,ij\bar{i}\bar{j}}^{S8,RR} \right] \\
&+ \alpha_s^2 \left[ \frac{6479}{81} L_{dd\,ij\bar{i}\bar{j}}^{S8,RR} - \frac{112}{27} L_{dd\,ij\bar{i}\bar{j}}^{S1,RR} \right] + \alpha_s \alpha \left[ -\frac{1840}{27} L_{dd\,ij\bar{i}\bar{j}}^{S1,RR} - \frac{208}{81} L_{dd\,ij\bar{i}\bar{j}}^{S8,RR} \right] \\
&+ \alpha^2 \left[ \frac{6298}{729} L_{dd\,ij\bar{i}\bar{j}}^{S8,RR} - \frac{1664}{243} L_{dd\,ij\bar{i}\bar{j}}^{S1,RR} \right]; \\
\dot{L}_{ed\,11ij}^{V,RR} &= e^2 \left[ \frac{4}{3} L_{dd\,kkij}^{V1,LR} + \frac{8}{3} L_{dd\,ijkk}^{V,RR} + \frac{8}{9} L_{dd\,ikkj}^{V,RR} + \frac{4}{3} L_{dd\,iijj}^{V1,LR} + \frac{4}{3} L_{dd\,jjij}^{V1,LR} \right. \\
&+ \frac{32}{9} L_{dd\,ij\bar{j}\bar{i}}^{V,RR} + \frac{32}{9} L_{dd\,ij\bar{j}\bar{j}}^{V,RR} + \frac{4}{3} L_{ed\,11ij}^{V,LR} + \frac{4}{3} L_{ed\,22ij}^{V,LR} + \frac{4}{3} L_{ed\,33ij}^{V,LR} + \frac{16}{3} L_{ed\,11ij}^{V,RR} \\
&+ \left. \frac{4}{3} L_{ed\,22ij}^{V,RR} + \frac{4}{3} L_{ed\,33ij}^{V,RR} - \frac{8}{3} L_{ud\,11ij}^{V1,LR} - \frac{8}{3} L_{ud\,22ij}^{V1,LR} - \frac{8}{3} L_{ud\,11ij}^{V1,RR} - \frac{8}{3} L_{ud\,22ij}^{V1,RR} \right] \\
&+ \alpha_s \alpha \left[ \frac{16}{3} L_{dd\,kkij}^{V1,LR} - \frac{1010}{243} L_{dd\,kkij}^{V8,LR} + 8 L_{dd\,ijkk}^{V,RR} + \frac{304}{243} L_{dd\,ikkj}^{V,RR} + \frac{16}{3} L_{dd\,iijj}^{V1,LR} \right. \\
&+ \frac{16}{3} L_{dd\,jjij}^{V1,LR} - \frac{1010}{243} L_{dd\,iijj}^{V8,LR} - \frac{1010}{243} L_{dd\,jjij}^{V8,LR} + \frac{1096}{81} L_{dd\,ij\bar{i}\bar{i}}^{V,RR} + \frac{1096}{81} L_{dd\,ij\bar{j}\bar{j}}^{V,RR} \\
&- 16 L_{ed\,11ij}^{V,RR} - \frac{32}{3} L_{ud\,11ij}^{V1,LR} - \frac{32}{3} L_{ud\,22ij}^{V1,LR} - \frac{32}{3} L_{ud\,11ij}^{V1,RR} - \frac{32}{3} L_{ud\,22ij}^{V1,RR} + \frac{1366}{243} L_{ud\,11ij}^{V8,LR} \\
&+ \left. \frac{1366}{243} L_{ud\,22ij}^{V8,LR} - \frac{74}{243} L_{ud\,11ij}^{V8,RR} - \frac{74}{243} L_{ud\,22ij}^{V8,RR} \right] + \alpha^2 \left[ -\frac{1288}{243} L_{dd\,kkij}^{V1,LR} + \frac{2032}{243} L_{ij\bar{k}\bar{k}}^{V,RR} \right. \\
&+ \frac{2992}{729} L_{dd\,ikkj}^{V,RR} - \frac{1288}{243} L_{dd\,iijj}^{V1,LR} - \frac{1288}{243} L_{dd\,jjij}^{V1,LR} + \frac{4864}{243} L_{dd\,ij\bar{i}\bar{i}}^{V,RR} + \frac{4864}{243} L_{dd\,ij\bar{j}\bar{j}}^{V,RR} \\
&- \left. \frac{3160}{243} L_{ed\,11ij}^{V,LR} - \frac{3160}{243} L_{ed\,22ij}^{V,LR} - \frac{3160}{243} L_{ed\,33ij}^{V,LR} + \frac{818}{243} L_{ed\,11ij}^{V,RR} + \frac{3752}{243} L_{ed\,22ij}^{V,RR} \right]
\end{aligned}$$

$$\begin{aligned}
& + \frac{3752}{243} L_{33ij}^{V,RR} - \frac{6280}{243} L_{11ij}^{V1,LR} - \frac{6280}{243} L_{22ij}^{V1,LR} + \frac{2936}{243} L_{11ij}^{V1,RR} + \frac{2936}{243} L_{22ij}^{V1,RR} \Bigg] ; \\
\dot{L}_{ed,22ij}^{V,RR} = & e^2 \left[ \frac{4}{3} L_{kkij}^{V1,LR} + \frac{8}{3} L_{ijkk}^{V,RR} + \frac{8}{9} L_{ikkj}^{V,RR} + \frac{4}{3} L_{iiij}^{V1,LR} + \frac{4}{3} L_{jjij}^{V1,LR} \right. \\
& + \frac{32}{9} L_{dd}^{V,RR} + \frac{32}{9} L_{ijjj}^{V,RR} + \frac{4}{3} L_{11ij}^{V,LR} + \frac{4}{3} L_{22ij}^{V,LR} + \frac{4}{3} L_{33ij}^{V,LR} + \frac{4}{3} L_{11ij}^{V,RR} \\
& + \frac{16}{3} L_{ed,22ij}^{V,RR} + \frac{4}{3} L_{ed,33ij}^{V,RR} - \frac{8}{3} L_{ud,11ij}^{V1,LR} - \frac{8}{3} L_{ud,22ij}^{V1,LR} - \frac{8}{3} L_{ud,11ij}^{V1,RR} - \frac{8}{3} L_{ud,22ij}^{V1,RR} \Bigg] \\
& + \alpha_s \alpha \left[ \frac{16}{3} L_{kkij}^{V1,LR} - \frac{1010}{243} L_{kkij}^{V8,LR} + 8 L_{ijkk}^{V,RR} + \frac{304}{243} L_{ikkj}^{V,RR} + \frac{16}{3} L_{iiij}^{V1,LR} \right. \\
& + \frac{16}{3} L_{jjij}^{V1,LR} - \frac{1010}{243} L_{iiij}^{V8,LR} - \frac{1010}{243} L_{jjij}^{V8,LR} + \frac{1096}{81} L_{ijii}^{V,RR} + \frac{1096}{81} L_{ijjj}^{V,RR} \\
& - 16 L_{ed,22ij}^{V,RR} - \frac{32}{3} L_{ud,11ij}^{V1,LR} - \frac{32}{3} L_{ud,22ij}^{V1,LR} - \frac{32}{3} L_{ud,11ij}^{V1,RR} - \frac{32}{3} L_{ud,22ij}^{V1,RR} + \frac{1366}{243} L_{ud,11ij}^{V8,LR} \\
& + \frac{1366}{243} L_{ud,22ij}^{V8,LR} - \frac{74}{243} L_{ud,11ij}^{V8,RR} - \frac{74}{243} L_{ud,22ij}^{V8,RR} \Bigg] + \alpha^2 \left[ - \frac{1288}{243} L_{kkij}^{V1,LR} + \frac{2032}{243} L_{ijkk}^{V,RR} \right. \\
& + \frac{2992}{729} L_{ikkj}^{V,RR} - \frac{1288}{243} L_{iiij}^{V1,LR} - \frac{1288}{243} L_{jjij}^{V1,LR} + \frac{4864}{243} L_{ijii}^{V,RR} + \frac{4864}{243} L_{ijjj}^{V,RR} \\
& - \frac{3160}{243} L_{11ij}^{V,LR} - \frac{3160}{243} L_{22ij}^{V,LR} - \frac{3160}{243} L_{33ij}^{V,LR} + \frac{3752}{243} L_{11ij}^{V,RR} + \frac{818}{243} L_{22ij}^{V,RR} \\
& + \frac{3752}{243} L_{ed,33ij}^{V,RR} - \frac{6280}{243} L_{ud,11ij}^{V1,LR} - \frac{6280}{243} L_{ud,22ij}^{V1,LR} + \frac{2936}{243} L_{ud,11ij}^{V1,RR} + \frac{2936}{243} L_{ud,22ij}^{V1,RR} \Bigg] ; \\
\dot{L}_{ed,33ij}^{V,RR} = & e^2 \left[ \frac{4}{3} L_{kkij}^{V1,LR} + \frac{8}{3} L_{ijkk}^{V,RR} + \frac{8}{9} L_{ikkj}^{V,RR} + \frac{4}{3} L_{iiij}^{V1,LR} + \frac{4}{3} L_{jjij}^{V1,LR} \right. \\
& + \frac{32}{9} L_{dd}^{V,RR} + \frac{32}{9} L_{ijjj}^{V,RR} + \frac{4}{3} L_{11ij}^{V,LR} + \frac{4}{3} L_{22ij}^{V,LR} + \frac{4}{3} L_{33ij}^{V,LR} + \frac{4}{3} L_{11ij}^{V,RR} \\
& + \frac{4}{3} L_{ed,22ij}^{V,RR} + \frac{16}{3} L_{ed,33ij}^{V,RR} - \frac{8}{3} L_{ud,11ij}^{V1,LR} - \frac{8}{3} L_{ud,22ij}^{V1,LR} - \frac{8}{3} L_{ud,11ij}^{V1,RR} - \frac{8}{3} L_{ud,22ij}^{V1,RR} \Bigg] \\
& + \alpha_s \alpha \left[ \frac{16}{3} L_{kkij}^{V1,LR} - \frac{1010}{243} L_{kkij}^{V8,LR} + 8 L_{ijkk}^{V,RR} + \frac{304}{243} L_{ikkj}^{V,RR} + \frac{16}{3} L_{iiij}^{V1,LR} \right. \\
& + \frac{16}{3} L_{jjij}^{V1,LR} - \frac{1010}{243} L_{iiij}^{V8,LR} - \frac{1010}{243} L_{jjij}^{V8,LR} + \frac{1096}{81} L_{ijii}^{V,RR} + \frac{1096}{81} L_{ijjj}^{V,RR}
\end{aligned}$$

$$\begin{aligned}
& -16L_{33ij}^{V,RR} - \frac{32}{3}L_{11ij}^{V1,LR} - \frac{32}{3}L_{22ij}^{V1,LR} - \frac{32}{3}L_{11ij}^{V1,RR} - \frac{32}{3}L_{22ij}^{V1,RR} + \frac{1366}{243}L_{11ij}^{V8,LR} \\
& + \frac{1366}{243}L_{22ij}^{V8,LR} - \frac{74}{243}L_{11ij}^{V8,RR} - \frac{74}{243}L_{22ij}^{V8,RR} \Big] + \alpha^2 \Big[ -\frac{1288}{243}L_{kkij}^{V1,LR} + \frac{2032}{243}L_{ijkk}^{V,RR} \\
& + \frac{2992}{729}L_{ikkj}^{V,RR} - \frac{1288}{243}L_{iii}^{V1,LR} - \frac{1288}{243}L_{jjj}^{V1,LR} + \frac{4864}{243}L_{ijii}^{V,RR} + \frac{4864}{243}L_{ijjj}^{V,RR} \\
& - \frac{3160}{243}L_{11ij}^{V,LR} - \frac{3160}{243}L_{22ij}^{V,LR} - \frac{3160}{243}L_{33ij}^{V,LR} + \frac{3752}{243}L_{11ij}^{V,RR} + \frac{3752}{243}L_{22ij}^{V,RR} \\
& + \frac{818}{243}L_{33ij}^{V,RR} - \frac{6280}{243}L_{11ij}^{V1,LR} - \frac{6280}{243}L_{22ij}^{V1,LR} + \frac{2936}{243}L_{11ij}^{V1,RR} + \frac{2936}{243}L_{22ij}^{V1,RR} \Big] ; \\
\dot{L}_{11ij}^{V1,RR} &= \frac{8}{3}g_s^2 L_{11ij}^{V8,RR} + e^2 \Big[ -\frac{8}{9}L_{kkij}^{V1,LR} - \frac{16}{9}L_{ijkk}^{V,RR} - \frac{16}{27}L_{ikkj}^{V,RR} - \frac{8}{9}L_{iii}^{V1,LR} \\
& - \frac{8}{9}L_{jjj}^{V1,LR} - \frac{64}{27}L_{ijii}^{V,RR} - \frac{64}{27}L_{ijjj}^{V,RR} - \frac{8}{9}L_{11ij}^{V,LR} - \frac{8}{9}L_{22ij}^{V,LR} - \frac{8}{9}L_{33ij}^{V,LR} \\
& - \frac{8}{9}L_{11ij}^{V,RR} - \frac{8}{9}L_{22ij}^{V,RR} - \frac{8}{9}L_{33ij}^{V,RR} + \frac{16}{9}L_{11ij}^{V1,LR} + \frac{16}{9}L_{22ij}^{V1,LR} - \frac{8}{9}L_{11ij}^{V1,RR} \\
& + \frac{16}{9}L_{22ij}^{V1,RR} \Big] + \alpha_s^2 \Big[ -8L_{kkij}^{V1,LR} + \frac{4}{27}L_{kkij}^{V8,LR} + 16L_{ijkk}^{V,RR} + \frac{256}{27}L_{ikkj}^{V,RR} \\
& - 8L_{iii}^{V1,LR} - 8L_{jjj}^{V1,LR} + \frac{4}{27}L_{iii}^{V8,LR} + \frac{4}{27}L_{jjj}^{V8,LR} + \frac{328}{9}L_{ijii}^{V,RR} + \frac{328}{9}L_{ijjj}^{V,RR} \\
& - 8L_{11ij}^{V1,LR} - 8L_{22ij}^{V1,LR} - \frac{4}{3}L_{11ij}^{V1,RR} + 8L_{22ij}^{V1,RR} + \frac{4}{27}L_{11ij}^{V8,LR} + \frac{4}{27}L_{22ij}^{V8,LR} \\
& + \frac{86}{27}L_{11ij}^{V8,RR} + \frac{4}{27}L_{22ij}^{V8,RR} \Big] + \alpha_s \alpha \Big[ -\frac{32}{9}L_{kkij}^{V1,LR} + \frac{2020}{729}L_{kkij}^{V8,LR} - \frac{16}{3}L_{ijkk}^{V,RR} \\
& - \frac{608}{729}L_{ikkj}^{V,RR} - \frac{32}{9}L_{iii}^{V1,LR} - \frac{32}{9}L_{jjj}^{V1,LR} + \frac{2020}{729}L_{iii}^{V8,LR} + \frac{2020}{729}L_{jjj}^{V8,LR} - \frac{2192}{243}L_{ijii}^{V,RR} \\
& - \frac{2192}{243}L_{ijjj}^{V,RR} + \frac{64}{9}L_{11ij}^{V1,LR} + \frac{64}{9}L_{22ij}^{V1,LR} + \frac{256}{9}L_{11ij}^{V1,RR} + \frac{64}{9}L_{22ij}^{V1,RR} - \frac{2732}{729}L_{11ij}^{V8,LR} \\
& - \frac{2732}{729}L_{22ij}^{V8,LR} - \frac{68}{729}L_{11ij}^{V8,RR} + \frac{148}{729}L_{22ij}^{V8,RR} \Big] + \alpha^2 \Big[ -\frac{304}{729}L_{kkij}^{V1,LR} + \frac{3136}{729}L_{ijkk}^{V,RR} \\
& + \frac{5536}{2187}L_{ikkj}^{V,RR} - \frac{304}{729}L_{iii}^{V1,LR} - \frac{304}{729}L_{jjj}^{V1,LR} + \frac{8272}{729}L_{ijii}^{V,RR} + \frac{8272}{729}L_{ijjj}^{V,RR}
\end{aligned}$$



$$\begin{aligned}
& -\frac{3040}{729}L_{11ij}^{V,LR} - \frac{3040}{729}L_{22ij}^{V,LR} - \frac{3040}{729}L_{33ij}^{V,LR} + \frac{2576}{729}L_{11ij}^{V,RR} + \frac{2576}{729}L_{22ij}^{V,RR} \\
& + \frac{2576}{729}L_{33ij}^{V,RR} - \frac{1120}{729}L_{11ij}^{V1,LR} - \frac{1120}{729}L_{22ij}^{V1,LR} + \frac{5216}{729}L_{11ij}^{V1,RR} + \frac{6368}{729}L_{22ij}^{V1,RR} \Big] ; \\
\dot{L}_{11ij}^{V8,RR} = & g_s^2 \left[ \frac{2}{3}L_{kkij}^{V8,LR} + \frac{8}{3}L_{ikkj}^{V,RR} + \frac{2}{3}L_{iiij}^{V8,LR} + \frac{2}{3}L_{jjij}^{V8,LR} + \frac{8}{3}L_{ijii}^{V,RR} \right. \\
& + \frac{8}{3}L_{ijjj}^{V,RR} + 12L_{11ij}^{V1,RR} + \frac{2}{3}L_{11ij}^{V8,LR} + \frac{2}{3}L_{22ij}^{V8,LR} - \frac{10}{3}L_{11ij}^{V8,RR} + \frac{2}{3}L_{22ij}^{V8,RR} \Big] \\
& - \frac{8}{3}e^2L_{11ij}^{V8,RR} + \alpha_s^2 \left[ -\frac{22}{3}L_{kkij}^{V1,LR} + \frac{151}{81}L_{kkij}^{V8,LR} - \frac{28}{3}L_{ijkk}^{V,RR} + \frac{5200}{81}L_{ikkj}^{V,RR} \right. \\
& - \frac{22}{3}L_{iiij}^{V1,LR} - \frac{22}{3}L_{jjij}^{V1,LR} + \frac{151}{81}L_{iiij}^{V8,LR} + \frac{151}{81}L_{jjij}^{V8,LR} + \frac{1906}{27}L_{ijii}^{V,RR} + \frac{1906}{27}L_{ijjj}^{V,RR} \\
& - \frac{22}{3}L_{11ij}^{V1,LR} - \frac{22}{3}L_{22ij}^{V1,LR} + 13L_{11ij}^{V1,RR} - \frac{2}{3}L_{22ij}^{V1,RR} + \frac{151}{81}L_{11ij}^{V8,LR} + \frac{151}{81}L_{22ij}^{V8,LR} \\
& - \frac{344}{81}L_{11ij}^{V8,RR} + \frac{781}{81}L_{22ij}^{V8,RR} \Big] + \alpha_s \alpha \left[ -\frac{208}{81}L_{kkij}^{V1,LR} + \frac{52}{27}L_{kkij}^{V8,LR} - \frac{416}{81}L_{ijkk}^{V,RR} \right. \\
& - \frac{5072}{243}L_{ikkj}^{V,RR} - \frac{208}{81}L_{iiij}^{V1,LR} - \frac{208}{81}L_{jjij}^{V1,LR} + \frac{52}{27}L_{iiij}^{V8,LR} + \frac{52}{27}L_{jjij}^{V8,LR} - \frac{3200}{81}L_{ijii}^{V,RR} \\
& - \frac{3200}{81}L_{ijjj}^{V,RR} - \frac{208}{81}L_{11ij}^{V,LR} - \frac{208}{81}L_{22ij}^{V,LR} - \frac{208}{81}L_{33ij}^{V,LR} - \frac{208}{81}L_{11ij}^{V,RR} - \frac{208}{81}L_{22ij}^{V,RR} \\
& - \frac{208}{81}L_{33ij}^{V,RR} + \frac{416}{81}L_{11ij}^{V1,LR} + \frac{416}{81}L_{22ij}^{V1,LR} + \frac{308}{81}L_{11ij}^{V1,RR} + \frac{416}{81}L_{22ij}^{V1,RR} - \frac{80}{27}L_{11ij}^{V8,LR} \\
& - \frac{80}{27}L_{22ij}^{V8,LR} + L_{11ij}^{V8,RR} + \frac{56}{9}L_{22ij}^{V8,RR} \Big] - \frac{128}{81}\alpha^2L_{11ij}^{V8,RR} ; \\
\dot{L}_{22ij}^{V1,RR} = & \frac{8}{3}g_s^2L_{22ij}^{V8,RR} + e^2 \left[ -\frac{8}{9}L_{kkij}^{V1,LR} - \frac{16}{9}L_{ijkk}^{V,RR} - \frac{16}{27}L_{ikkj}^{V,RR} - \frac{8}{9}L_{iiij}^{V1,LR} \right. \\
& - \frac{8}{9}L_{jjij}^{V1,LR} - \frac{64}{27}L_{ijii}^{V,RR} - \frac{64}{27}L_{ijjj}^{V,RR} - \frac{8}{9}L_{11ij}^{V,LR} - \frac{8}{9}L_{22ij}^{V,LR} - \frac{8}{9}L_{33ij}^{V,LR} \\
& - \frac{8}{9}L_{11ij}^{V,RR} - \frac{8}{9}L_{22ij}^{V,RR} - \frac{8}{9}L_{33ij}^{V,RR} + \frac{16}{9}L_{11ij}^{V1,LR} + \frac{16}{9}L_{22ij}^{V1,LR} + \frac{16}{9}L_{11ij}^{V1,RR} \\
& \left. - \frac{8}{9}L_{22ij}^{V1,RR} \right] + \alpha_s^2 \left[ -8L_{kkij}^{V1,LR} + \frac{4}{27}L_{kkij}^{V8,LR} + 16L_{ijkk}^{V,RR} + \frac{256}{27}L_{ikkj}^{V,RR} \right]
\end{aligned}$$

$$\begin{aligned}
& -8L_{\ddot{u}i\ddot{j}}^{V1,LR} - 8L_{\ddot{j}j\ddot{i}}^{V1,LR} + \frac{4}{27}L_{\ddot{u}i\ddot{j}}^{V8,LR} + \frac{4}{27}L_{\ddot{j}j\ddot{i}}^{V8,LR} + \frac{328}{9}L_{\ddot{i}j\ddot{u}}^{V,RR} + \frac{328}{9}L_{\ddot{i}j\ddot{j}}^{V,RR} \\
& -8L_{\ddot{u}11\ddot{i}j}^{V1,LR} - 8L_{\ddot{u}22\ddot{i}j}^{V1,LR} + 8L_{\ddot{u}11\ddot{i}j}^{V1,RR} - \frac{4}{3}L_{\ddot{u}22\ddot{i}j}^{V1,RR} + \frac{4}{27}L_{\ddot{u}11\ddot{i}j}^{V8,LR} + \frac{4}{27}L_{\ddot{u}22\ddot{i}j}^{V8,LR} \\
& + \frac{4}{27}L_{\ddot{u}11\ddot{i}j}^{V8,RR} + \frac{86}{27}L_{\ddot{u}22\ddot{i}j}^{V8,RR} \Big] + \alpha_s \alpha \Big[ -\frac{32}{9}L_{\ddot{k}k\ddot{i}j}^{V1,LR} + \frac{2020}{729}L_{\ddot{k}k\ddot{i}j}^{V8,LR} - \frac{16}{3}L_{\ddot{i}j\ddot{k}k}^{V,RR} \\
& -\frac{608}{729}L_{\ddot{i}k\ddot{k}j}^{V,RR} - \frac{32}{9}L_{\ddot{u}i\ddot{j}}^{V1,LR} - \frac{32}{9}L_{\ddot{j}j\ddot{i}}^{V1,LR} + \frac{2020}{729}L_{\ddot{u}i\ddot{j}}^{V8,LR} + \frac{2020}{729}L_{\ddot{j}j\ddot{i}}^{V8,LR} - \frac{2192}{243}L_{\ddot{i}j\ddot{u}}^{V,RR} \\
& -\frac{2192}{243}L_{\ddot{i}j\ddot{j}}^{V,RR} + \frac{64}{9}L_{\ddot{u}11\ddot{i}j}^{V1,LR} + \frac{64}{9}L_{\ddot{u}22\ddot{i}j}^{V1,LR} + \frac{64}{9}L_{\ddot{u}11\ddot{i}j}^{V1,RR} + \frac{256}{9}L_{\ddot{u}22\ddot{i}j}^{V1,RR} - \frac{2732}{729}L_{\ddot{u}11\ddot{i}j}^{V8,LR} \\
& -\frac{2732}{729}L_{\ddot{u}22\ddot{i}j}^{V8,LR} + \frac{148}{729}L_{\ddot{u}11\ddot{i}j}^{V8,RR} - \frac{68}{729}L_{\ddot{u}22\ddot{i}j}^{V8,RR} \Big] + \alpha^2 \Big[ -\frac{304}{729}L_{\ddot{k}k\ddot{i}j}^{V1,LR} + \frac{3136}{729}L_{\ddot{i}j\ddot{k}k}^{V,RR} \\
& + \frac{5536}{2187}L_{\ddot{i}k\ddot{k}j}^{V,RR} - \frac{304}{729}L_{\ddot{u}i\ddot{j}}^{V1,LR} - \frac{304}{729}L_{\ddot{j}j\ddot{i}}^{V1,LR} + \frac{8272}{729}L_{\ddot{i}j\ddot{u}}^{V,RR} + \frac{8272}{729}L_{\ddot{i}j\ddot{j}}^{V,RR} \\
& -\frac{3040}{729}L_{\ddot{e}d\ddot{u}11\ddot{i}j}^{V,LR} - \frac{3040}{729}L_{\ddot{e}d\ddot{u}22\ddot{i}j}^{V,LR} - \frac{3040}{729}L_{\ddot{e}d\ddot{u}33\ddot{i}j}^{V,LR} + \frac{2576}{729}L_{\ddot{e}d\ddot{u}11\ddot{i}j}^{V,RR} + \frac{2576}{729}L_{\ddot{e}d\ddot{u}22\ddot{i}j}^{V,RR} \\
& + \frac{2576}{729}L_{\ddot{e}d\ddot{u}33\ddot{i}j}^{V,RR} - \frac{1120}{729}L_{\ddot{u}11\ddot{i}j}^{V1,LR} - \frac{1120}{729}L_{\ddot{u}22\ddot{i}j}^{V1,LR} + \frac{6368}{729}L_{\ddot{u}11\ddot{i}j}^{V1,RR} + \frac{5216}{729}L_{\ddot{u}22\ddot{i}j}^{V1,RR} \Big] ;
\end{aligned}$$

$$\begin{aligned}
\dot{L}_{\ddot{u}d\ddot{u}22\ddot{i}j}^{V8,RR} &= g_s^2 \Big[ \frac{2}{3}L_{\ddot{k}k\ddot{i}j}^{V8,LR} + \frac{8}{3}L_{\ddot{i}k\ddot{k}j}^{V,RR} + \frac{2}{3}L_{\ddot{u}i\ddot{j}}^{V8,LR} + \frac{2}{3}L_{\ddot{j}j\ddot{i}}^{V8,LR} + \frac{8}{3}L_{\ddot{i}j\ddot{u}}^{V,RR} \\
& + \frac{8}{3}L_{\ddot{i}j\ddot{j}}^{V,RR} + 12L_{\ddot{u}22\ddot{i}j}^{V1,RR} + \frac{2}{3}L_{\ddot{u}11\ddot{i}j}^{V8,LR} + \frac{2}{3}L_{\ddot{u}22\ddot{i}j}^{V8,LR} + \frac{2}{3}L_{\ddot{u}11\ddot{i}j}^{V8,RR} - \frac{10}{3}L_{\ddot{u}22\ddot{i}j}^{V8,RR} \Big] \\
& -\frac{8}{3}e^2L_{\ddot{u}d\ddot{u}22\ddot{i}j}^{V8,RR} + \alpha_s^2 \Big[ -\frac{22}{3}L_{\ddot{k}k\ddot{i}j}^{V1,LR} + \frac{151}{81}L_{\ddot{k}k\ddot{i}j}^{V8,LR} - \frac{28}{3}L_{\ddot{i}j\ddot{k}k}^{V,RR} + \frac{5200}{81}L_{\ddot{i}k\ddot{k}j}^{V,RR} \\
& -\frac{22}{3}L_{\ddot{u}i\ddot{j}}^{V1,LR} - \frac{22}{3}L_{\ddot{j}j\ddot{i}}^{V1,LR} + \frac{151}{81}L_{\ddot{u}i\ddot{j}}^{V8,LR} + \frac{151}{81}L_{\ddot{j}j\ddot{i}}^{V8,LR} + \frac{1906}{27}L_{\ddot{i}j\ddot{u}}^{V,RR} + \frac{1906}{27}L_{\ddot{i}j\ddot{j}}^{V,RR} \\
& -\frac{22}{3}L_{\ddot{u}11\ddot{i}j}^{V1,LR} - \frac{22}{3}L_{\ddot{u}22\ddot{i}j}^{V1,LR} - \frac{2}{3}L_{\ddot{u}11\ddot{i}j}^{V1,RR} + 13L_{\ddot{u}22\ddot{i}j}^{V1,RR} + \frac{151}{81}L_{\ddot{u}11\ddot{i}j}^{V8,LR} + \frac{151}{81}L_{\ddot{u}22\ddot{i}j}^{V8,LR} \\
& + \frac{781}{81}L_{\ddot{u}11\ddot{i}j}^{V8,RR} - \frac{344}{81}L_{\ddot{u}22\ddot{i}j}^{V8,RR} \Big] + \alpha_s \alpha \Big[ -\frac{208}{81}L_{\ddot{k}k\ddot{i}j}^{V1,LR} + \frac{52}{27}L_{\ddot{k}k\ddot{i}j}^{V8,LR} - \frac{416}{81}L_{\ddot{i}j\ddot{k}k}^{V,RR} \\
& -\frac{5072}{243}L_{\ddot{i}k\ddot{k}j}^{V,RR} - \frac{208}{81}L_{\ddot{u}i\ddot{j}}^{V1,LR} - \frac{208}{81}L_{\ddot{j}j\ddot{i}}^{V1,LR} + \frac{52}{27}L_{\ddot{u}i\ddot{j}}^{V8,LR} + \frac{52}{27}L_{\ddot{j}j\ddot{i}}^{V8,LR} - \frac{3200}{81}L_{\ddot{i}j\ddot{u}}^{V,RR} \\
& -\frac{3200}{81}L_{\ddot{i}j\ddot{j}}^{V,RR} \Big] ;
\end{aligned}$$

$$\begin{aligned}
& -\frac{3200}{81}L_{ijj}^{V,RR} - \frac{208}{81}L_{11ij}^{V,LR} - \frac{208}{81}L_{22ij}^{V,LR} - \frac{208}{81}L_{33ij}^{V,LR} - \frac{208}{81}L_{11ij}^{V,RR} - \frac{208}{81}L_{22ij}^{V,RR} \\
& - \frac{208}{81}L_{33ij}^{V,RR} + \frac{416}{81}L_{11ij}^{V1,LR} + \frac{416}{81}L_{22ij}^{V1,LR} + \frac{416}{81}L_{11ij}^{V1,RR} + \frac{308}{81}L_{22ij}^{V1,RR} - \frac{80}{27}L_{11ij}^{V8,LR} \\
& - \frac{80}{27}L_{22ij}^{V8,LR} + \frac{56}{9}L_{11ij}^{V8,RR} + L_{22ij}^{V8,RR} \Big] - \frac{128}{81}\alpha^2 L_{22ij}^{V8,RR} ; \\
\dot{L}_{ijk}^{V,RR} &= g_s^2 \Big[ -\frac{1}{18}L_{iii}^{V8,LR} - \frac{1}{18}L_{jjj}^{V8,LR} - \frac{1}{18}L_{kkj}^{V8,LR} - \frac{2}{9}L_{ijj}^{V,RR} - \frac{2}{9}L_{ijj}^{V,RR} \\
& - 2L_{ijk}^{V,RR} + \frac{52}{9}L_{ikk}^{V,RR} - \frac{1}{18}L_{11ij}^{V8,LR} - \frac{1}{18}L_{22ij}^{V8,LR} - \frac{1}{18}L_{11ij}^{V8,RR} - \frac{1}{18}L_{22ij}^{V8,RR} \Big] \\
& + e^2 \Big[ \frac{2}{9}L_{iii}^{V1,LR} + \frac{2}{9}L_{jjj}^{V1,LR} + \frac{2}{9}L_{kkj}^{V1,LR} + \frac{16}{27}L_{ijj}^{V,RR} + \frac{16}{27}L_{ijj}^{V,RR} + \frac{16}{9}L_{ijk}^{V,RR} \\
& + \frac{4}{27}L_{ikk}^{V,RR} + \frac{2}{9}L_{11ij}^{V,LR} + \frac{2}{9}L_{22ij}^{V,LR} + \frac{2}{9}L_{33ij}^{V,LR} + \frac{2}{9}L_{11ij}^{V,RR} + \frac{2}{9}L_{22ij}^{V,RR} \\
& + \frac{2}{9}L_{33ij}^{V,RR} - \frac{4}{9}L_{11ij}^{V1,LR} - \frac{4}{9}L_{22ij}^{V1,LR} - \frac{4}{9}L_{11ij}^{V1,RR} - \frac{4}{9}L_{22ij}^{V1,RR} \Big] + \alpha_s^2 \Big[ -\frac{61}{18}L_{iii}^{V1,LR} \\
& - \frac{61}{18}L_{jjj}^{V1,LR} - \frac{61}{18}L_{kkj}^{V1,LR} - \frac{79}{972}L_{ijj}^{V8,LR} - \frac{79}{972}L_{jjj}^{V8,LR} - \frac{79}{972}L_{kkj}^{V8,LR} + \frac{1999}{162}L_{ijj}^{V,RR} \\
& + \frac{1999}{162}L_{jjj}^{V,RR} - \frac{17}{6}L_{ijk}^{V,RR} + \frac{3025}{486}L_{ikk}^{V,RR} - \frac{61}{18}L_{11ij}^{V1,LR} - \frac{61}{18}L_{22ij}^{V1,LR} + \frac{73}{18}L_{11ij}^{V1,RR} \\
& + \frac{73}{18}L_{22ij}^{V1,RR} - \frac{79}{972}L_{11ij}^{V8,LR} - \frac{79}{972}L_{22ij}^{V8,LR} - \frac{709}{972}L_{11ij}^{V8,RR} - \frac{709}{972}L_{22ij}^{V8,RR} \Big] \\
& + \alpha_s \alpha \Big[ \frac{241}{243}L_{iii}^{V1,LR} + \frac{241}{243}L_{jjj}^{V1,LR} + \frac{241}{243}L_{kkj}^{V1,LR} - \frac{785}{1458}L_{iii}^{V8,LR} - \frac{785}{1458}L_{jjj}^{V8,LR} \\
& - \frac{785}{1458}L_{kkj}^{V8,LR} + \frac{349}{243}L_{ijj}^{V,RR} + \frac{349}{243}L_{ijj}^{V,RR} - \frac{1516}{243}L_{ijk}^{V,RR} - \frac{6626}{729}L_{ikk}^{V,RR} \\
& + \frac{25}{243}L_{11ij}^{V,LR} + \frac{25}{243}L_{22ij}^{V,LR} + \frac{25}{243}L_{33ij}^{V,LR} + \frac{25}{243}L_{11ij}^{V,RR} + \frac{25}{243}L_{22ij}^{V,RR} + \frac{25}{243}L_{33ij}^{V,RR} \\
& - \frac{482}{243}L_{11ij}^{V1,LR} - \frac{482}{243}L_{22ij}^{V1,LR} - \frac{482}{243}L_{11ij}^{V1,RR} - \frac{482}{243}L_{22ij}^{V1,RR} + \frac{727}{1458}L_{11ij}^{V8,LR} \\
& + \frac{727}{1458}L_{22ij}^{V8,LR} + \frac{115}{1458}L_{11ij}^{V8,RR} + \frac{115}{1458}L_{22ij}^{V8,RR} \Big] + \alpha^2 \Big[ -\frac{356}{729}L_{iii}^{V1,LR} - \frac{356}{729}L_{jjj}^{V1,LR}
\end{aligned}$$

$$\begin{aligned}
& -\frac{356}{729}L_{\overline{kk}ij}^{V1,LR} + \frac{632}{729}L_{\overline{ij}ii}^{V,RR} + \frac{632}{729}L_{\overline{ij}jj}^{V,RR} + \frac{710}{729}L_{\overline{ij}kk}^{V,RR} + \frac{344}{2187}L_{\overline{ikk}j}^{V,RR} \\
& -\frac{644}{729}L_{\overline{11}ij}^{V,LR} - \frac{644}{729}L_{\overline{22}ij}^{V,LR} - \frac{644}{729}L_{\overline{33}ij}^{V,LR} + \frac{868}{729}L_{\overline{11}ij}^{V,RR} + \frac{868}{729}L_{\overline{22}ij}^{V,RR} + \frac{868}{729}L_{\overline{33}ij}^{V,RR} \\
& -\frac{1772}{729}L_{\overline{11}ij}^{V1,LR} - \frac{1772}{729}L_{\overline{22}ij}^{V1,LR} + \frac{244}{729}L_{\overline{11}ij}^{V1,RR} + \frac{244}{729}L_{\overline{22}ij}^{V1,RR} \Big] ;
\end{aligned}$$

$$\begin{aligned}
\dot{L}_{\overline{ikk}j}^{V,RR} = & g_s^2 \left[ \frac{1}{6}L_{\overline{kk}ij}^{V8,LR} + 6L_{\overline{ij}kk}^{V,RR} - \frac{4}{3}L_{\overline{ikk}j}^{V,RR} + \frac{1}{6}L_{\overline{ii}ij}^{V8,LR} + \frac{1}{6}L_{\overline{jj}ij}^{V8,LR} \right. \\
& + \frac{2}{3}L_{\overline{ij}ii}^{V,RR} + \frac{2}{3}L_{\overline{ij}jj}^{V,RR} + \frac{1}{6}L_{\overline{11}ij}^{V8,LR} + \frac{1}{6}L_{\overline{22}ij}^{V8,LR} + \frac{1}{6}L_{\overline{11}ij}^{V8,RR} + \left. \frac{1}{6}L_{\overline{22}ij}^{V8,RR} \right] \\
& + \frac{4}{3}e^2L_{\overline{ikk}j}^{V,RR} + \alpha_s^2 \left[ -\frac{11}{6}L_{\overline{kk}ij}^{V1,LR} + \frac{151}{324}L_{\overline{kk}ij}^{V8,LR} + \frac{9}{2}L_{\overline{ij}kk}^{V,RR} + \frac{719}{162}L_{\overline{ikk}j}^{V,RR} \right. \\
& - \frac{11}{6}L_{\overline{ii}ij}^{V1,LR} - \frac{11}{6}L_{\overline{jj}ij}^{V1,LR} + \frac{151}{324}L_{\overline{ii}ij}^{V8,LR} + \frac{151}{324}L_{\overline{jj}ij}^{V8,LR} + \frac{953}{54}L_{\overline{ij}ii}^{V,RR} + \frac{953}{54}L_{\overline{ij}jj}^{V,RR} \\
& - \frac{11}{6}L_{\overline{11}ij}^{V1,LR} - \frac{11}{6}L_{\overline{22}ij}^{V1,LR} - \frac{1}{6}L_{\overline{11}ij}^{V1,RR} - \frac{1}{6}L_{\overline{22}ij}^{V1,RR} + \frac{151}{324}L_{\overline{11}ij}^{V8,LR} + \frac{151}{324}L_{\overline{22}ij}^{V8,LR} \\
& + \frac{781}{324}L_{\overline{11}ij}^{V8,RR} + \left. \frac{781}{324}L_{\overline{22}ij}^{V8,RR} \right] + \alpha_s\alpha \left[ -\frac{25}{81}L_{\overline{kk}ij}^{V1,LR} - \frac{25}{54}L_{\overline{kk}ij}^{V8,LR} - \frac{752}{81}L_{\overline{ij}kk}^{V,RR} \right. \\
& - \frac{1430}{243}L_{\overline{ikk}j}^{V,RR} - \frac{25}{81}L_{\overline{ii}ij}^{V1,LR} - \frac{25}{81}L_{\overline{jj}ij}^{V1,LR} - \frac{25}{54}L_{\overline{ii}ij}^{V8,LR} - \frac{25}{54}L_{\overline{jj}ij}^{V8,LR} + \frac{199}{81}L_{\overline{ij}ii}^{V,RR} \\
& + \frac{199}{81}L_{\overline{ij}jj}^{V,RR} - \frac{25}{81}L_{\overline{11}ij}^{V,LR} - \frac{25}{81}L_{\overline{22}ij}^{V,LR} - \frac{25}{81}L_{\overline{33}ij}^{V,LR} - \frac{25}{81}L_{\overline{11}ij}^{V,RR} - \frac{25}{81}L_{\overline{22}ij}^{V,RR} \\
& - \frac{25}{81}L_{\overline{33}ij}^{V,RR} + \frac{50}{81}L_{\overline{11}ij}^{V1,LR} + \frac{50}{81}L_{\overline{22}ij}^{V1,LR} + \frac{50}{81}L_{\overline{11}ij}^{V1,RR} + \frac{50}{81}L_{\overline{22}ij}^{V1,RR} + \frac{71}{54}L_{\overline{11}ij}^{V8,LR} \\
& + \left. \frac{71}{54}L_{\overline{22}ij}^{V8,LR} - \frac{7}{18}L_{\overline{11}ij}^{V8,RR} - \frac{7}{18}L_{\overline{22}ij}^{V8,RR} \right] + \frac{46}{81}\alpha^2L_{\overline{ikk}j}^{V,RR} ;
\end{aligned}$$

$$\begin{aligned}
\dot{L}_{\overline{ij}jj}^{V,RR} = & g_s^2 \left[ \frac{1}{9}L_{\overline{ii}ij}^{V8,LR} + \frac{1}{9}L_{\overline{jj}ij}^{V8,LR} + \frac{1}{9}L_{\overline{kk}ij}^{V8,LR} + \frac{4}{9}L_{\overline{ij}ii}^{V,RR} + \frac{40}{9}L_{\overline{ij}jj}^{V,RR} \right. \\
& + \frac{4}{9}L_{\overline{ikk}j}^{V,RR} + \frac{1}{9}L_{\overline{11}ij}^{V8,LR} + \frac{1}{9}L_{\overline{22}ij}^{V8,LR} + \frac{1}{9}L_{\overline{11}ij}^{V8,RR} + \left. \frac{1}{9}L_{\overline{22}ij}^{V8,RR} \right] + e^2 \left[ \frac{2}{9}L_{\overline{ii}ij}^{V1,LR} \right. \\
& + \frac{2}{9}L_{\overline{jj}ij}^{V1,LR} + \frac{2}{9}L_{\overline{kk}ij}^{V1,LR} + \frac{16}{27}L_{\overline{ij}ii}^{V,RR} + \frac{52}{27}L_{\overline{ij}jj}^{V,RR} + \frac{4}{9}L_{\overline{ij}kk}^{V,RR} + \left. \frac{4}{27}L_{\overline{ikk}j}^{V,RR} \right]
\end{aligned}$$

$$\begin{aligned}
& + \frac{2}{9}L_{ed\ 11ij}^{V,LR} + \frac{2}{9}L_{ed\ 22ij}^{V,LR} + \frac{2}{9}L_{ed\ 33ij}^{V,LR} + \frac{2}{9}L_{ed\ 11ij}^{V,RR} + \frac{2}{9}L_{ed\ 22ij}^{V,RR} + \frac{2}{9}L_{ed\ 33ij}^{V,RR} \\
& - \frac{4}{9}L_{ud\ 11ij}^{V1,LR} - \frac{4}{9}L_{ud\ 22ij}^{V1,LR} - \frac{4}{9}L_{ud\ 11ij}^{V1,RR} - \frac{4}{9}L_{ud\ 22ij}^{V1,RR} \Big] + \alpha_s^2 \Big[ - \frac{47}{9}L_{dd\ iij}^{V1,LR} \\
& - \frac{47}{9}L_{dd\ jjj}^{V1,LR} - \frac{47}{9}L_{dd\ kki}^{V1,LR} + \frac{187}{486}L_{dd\ iij}^{V8,LR} + \frac{187}{486}L_{dd\ jjj}^{V8,LR} + \frac{187}{486}L_{dd\ kki}^{V8,LR} + \frac{2429}{81}L_{dd\ iij}^{V,RR} \\
& + \frac{2042}{81}L_{dd\ ijj}^{V,RR} + \frac{58}{9}L_{dd\ ijj}^{V,RR} + \frac{3752}{243}L_{dd\ ijj}^{V,RR} - \frac{47}{9}L_{ud\ 11ij}^{V1,LR} - \frac{47}{9}L_{ud\ 22ij}^{V1,LR} + \frac{35}{9}L_{ud\ 11ij}^{V1,RR} \\
& + \frac{35}{9}L_{ud\ 22ij}^{V1,RR} + \frac{187}{486}L_{ud\ 11ij}^{V8,LR} + \frac{187}{486}L_{ud\ 22ij}^{V8,LR} + \frac{817}{486}L_{ud\ 11ij}^{V8,RR} + \frac{817}{486}L_{ud\ 22ij}^{V8,RR} \Big] \\
& + \alpha_s \alpha \Big[ \frac{166}{243}L_{dd\ iij}^{V1,LR} + \frac{166}{243}L_{dd\ jjj}^{V1,LR} + \frac{166}{243}L_{dd\ kki}^{V1,LR} - \frac{730}{729}L_{dd\ iij}^{V8,LR} - \frac{730}{729}L_{dd\ jjj}^{V8,LR} \\
& - \frac{730}{729}L_{dd\ kki}^{V8,LR} + \frac{946}{243}L_{dd\ iij}^{V,RR} - \frac{3050}{243}L_{dd\ ijj}^{V,RR} + \frac{224}{243}L_{dd\ ijj}^{V,RR} + \frac{1072}{729}L_{dd\ ijj}^{V,RR} \\
& - \frac{50}{243}L_{ed\ 11ij}^{V,LR} - \frac{50}{243}L_{ed\ 22ij}^{V,LR} - \frac{50}{243}L_{ed\ 33ij}^{V,LR} - \frac{50}{243}L_{ed\ 11ij}^{V,RR} - \frac{50}{243}L_{ed\ 22ij}^{V,RR} - \frac{50}{243}L_{ed\ 33ij}^{V,RR} \\
& - \frac{332}{243}L_{ud\ 11ij}^{V1,LR} - \frac{332}{243}L_{ud\ 22ij}^{V1,LR} - \frac{332}{243}L_{ud\ 11ij}^{V1,RR} - \frac{332}{243}L_{ud\ 22ij}^{V1,RR} + \frac{1322}{729}L_{ud\ 11ij}^{V8,LR} \\
& + \frac{1322}{729}L_{ud\ 22ij}^{V8,LR} - \frac{226}{729}L_{ud\ 11ij}^{V8,RR} - \frac{226}{729}L_{ud\ 22ij}^{V8,RR} \Big] + \alpha^2 \Big[ - \frac{356}{729}L_{dd\ iij}^{V1,LR} - \frac{356}{729}L_{dd\ jjj}^{V1,LR} \\
& - \frac{356}{729}L_{dd\ kki}^{V1,LR} + \frac{632}{729}L_{dd\ iij}^{V,RR} + \frac{1046}{729}L_{dd\ ijj}^{V,RR} + \frac{296}{729}L_{dd\ ijj}^{V,RR} + \frac{344}{2187}L_{dd\ ijj}^{V,RR} \\
& - \frac{644}{729}L_{ed\ 11ij}^{V,LR} - \frac{644}{729}L_{ed\ 22ij}^{V,LR} - \frac{644}{729}L_{ed\ 33ij}^{V,LR} + \frac{868}{729}L_{ed\ 11ij}^{V,RR} + \frac{868}{729}L_{ed\ 22ij}^{V,RR} + \frac{868}{729}L_{ed\ 33ij}^{V,RR} \\
& - \frac{1772}{729}L_{ud\ 11ij}^{V1,LR} - \frac{1772}{729}L_{ud\ 22ij}^{V1,LR} + \frac{244}{729}L_{ud\ 11ij}^{V1,RR} + \frac{244}{729}L_{ud\ 22ij}^{V1,RR} \Big] ; \\
\dot{L}_{dd\ iij}^{V,RR} & = g_s^2 \Big[ \frac{1}{9}L_{dd\ iij}^{V8,LR} + \frac{1}{9}L_{dd\ jjj}^{V8,LR} + \frac{1}{9}L_{dd\ kki}^{V8,LR} + \frac{40}{9}L_{dd\ iij}^{V,RR} + \frac{4}{9}L_{dd\ ijj}^{V,RR} \\
& + \frac{4}{9}L_{dd\ ijj}^{V,RR} + \frac{1}{9}L_{dd\ 11ij}^{V8,LR} + \frac{1}{9}L_{dd\ 22ij}^{V8,LR} + \frac{1}{9}L_{dd\ 11ij}^{V8,RR} + \frac{1}{9}L_{dd\ 22ij}^{V8,RR} \Big] + e^2 \Big[ \frac{2}{9}L_{dd\ iij}^{V1,LR} \\
& + \frac{2}{9}L_{dd\ ijj}^{V1,LR} + \frac{2}{9}L_{dd\ kki}^{V1,LR} + \frac{52}{27}L_{dd\ iij}^{V,RR} + \frac{16}{27}L_{dd\ ijj}^{V,RR} + \frac{4}{9}L_{dd\ ijj}^{V,RR} + \frac{4}{27}L_{dd\ ijj}^{V,RR} \\
& + \frac{4}{27}L_{dd\ ijj}^{V,RR} + \frac{4}{27}L_{dd\ ijj}^{V,RR} \Big]
\end{aligned}$$

$$\begin{aligned}
& + \frac{2}{9}L_{11ij}^{V,LR} + \frac{2}{9}L_{22ij}^{V,LR} + \frac{2}{9}L_{33ij}^{V,LR} + \frac{2}{9}L_{11ij}^{V,RR} + \frac{2}{9}L_{22ij}^{V,RR} + \frac{2}{9}L_{33ij}^{V,RR} \\
& - \frac{4}{9}L_{11ij}^{V1,LR} - \frac{4}{9}L_{22ij}^{V1,LR} - \frac{4}{9}L_{11ij}^{V1,RR} - \frac{4}{9}L_{22ij}^{V1,RR} \Big] + \alpha_s^2 \Big[ - \frac{47}{9}L_{iiij}^{V1,LR} \\
& - \frac{47}{9}L_{jjij}^{V1,LR} - \frac{47}{9}L_{kkij}^{V1,LR} + \frac{187}{486}L_{iiij}^{V8,LR} + \frac{187}{486}L_{jjij}^{V8,LR} + \frac{187}{486}L_{kkij}^{V8,LR} + \frac{2042}{81}L_{ijii}^{V,RR} \\
& + \frac{2429}{81}L_{ijjj}^{V,RR} + \frac{58}{9}L_{ijkk}^{V,RR} + \frac{3752}{243}L_{ikkj}^{V,RR} - \frac{47}{9}L_{11ij}^{V1,LR} - \frac{47}{9}L_{22ij}^{V1,LR} + \frac{35}{9}L_{11ij}^{V1,RR} \\
& + \frac{35}{9}L_{22ij}^{V1,RR} + \frac{187}{486}L_{11ij}^{V8,LR} + \frac{187}{486}L_{22ij}^{V8,LR} + \frac{817}{486}L_{11ij}^{V8,RR} + \frac{817}{486}L_{22ij}^{V8,RR} \Big] \\
& + \alpha_s \alpha \Big[ \frac{166}{243}L_{iiij}^{V1,LR} + \frac{166}{243}L_{jjij}^{V1,LR} + \frac{166}{243}L_{kkij}^{V1,LR} - \frac{730}{729}L_{iiij}^{V8,LR} - \frac{730}{729}L_{jjij}^{V8,LR} \\
& - \frac{730}{729}L_{kkij}^{V8,LR} - \frac{3050}{243}L_{ijii}^{V,RR} + \frac{946}{243}L_{ijjj}^{V,RR} + \frac{224}{243}L_{ijkk}^{V,RR} + \frac{1072}{729}L_{ikkj}^{V,RR} \\
& - \frac{50}{243}L_{11ij}^{V,LR} - \frac{50}{243}L_{22ij}^{V,LR} - \frac{50}{243}L_{33ij}^{V,LR} - \frac{50}{243}L_{11ij}^{V,RR} - \frac{50}{243}L_{22ij}^{V,RR} - \frac{50}{243}L_{33ij}^{V,RR} \\
& - \frac{332}{243}L_{11ij}^{V1,LR} - \frac{332}{243}L_{22ij}^{V1,LR} - \frac{332}{243}L_{11ij}^{V1,RR} - \frac{332}{243}L_{22ij}^{V1,RR} + \frac{1322}{729}L_{11ij}^{V8,LR} \\
& + \frac{1322}{729}L_{22ij}^{V8,LR} - \frac{226}{729}L_{11ij}^{V8,RR} - \frac{226}{729}L_{22ij}^{V8,RR} \Big] + \alpha^2 \Big[ - \frac{356}{729}L_{iiij}^{V1,LR} - \frac{356}{729}L_{jjij}^{V1,LR} \\
& - \frac{356}{729}L_{kkij}^{V1,LR} + \frac{1046}{729}L_{ijii}^{V,RR} + \frac{632}{729}L_{ijjj}^{V,RR} + \frac{296}{729}L_{ijkk}^{V,RR} + \frac{344}{2187}L_{ikkj}^{V,RR} \\
& - \frac{644}{729}L_{11ij}^{V,LR} - \frac{644}{729}L_{22ij}^{V,LR} - \frac{644}{729}L_{33ij}^{V,LR} + \frac{868}{729}L_{11ij}^{V,RR} + \frac{868}{729}L_{22ij}^{V,RR} + \frac{868}{729}L_{33ij}^{V,RR} \\
& - \frac{1772}{729}L_{11ij}^{V1,LR} - \frac{1772}{729}L_{22ij}^{V1,LR} + \frac{244}{729}L_{11ij}^{V1,RR} + \frac{244}{729}L_{22ij}^{V1,RR} \Big] ; \\
\dot{L}_{11ij}^{V,LR} & = e^2 \Big[ \frac{4}{3}L_{kkij}^{V1,LR} + \frac{8}{3}L_{ijkk}^{V,RR} + \frac{8}{9}L_{ikkj}^{V,RR} + \frac{4}{3}L_{iiij}^{V1,LR} + \frac{4}{3}L_{jjij}^{V1,LR} \\
& + \frac{32}{9}L_{ijii}^{V,RR} + \frac{32}{9}L_{ijjj}^{V,RR} - \frac{8}{3}L_{11ij}^{V,LR} + \frac{4}{3}L_{22ij}^{V,LR} + \frac{4}{3}L_{33ij}^{V,LR} + \frac{4}{3}L_{11ij}^{V,RR} \\
& + \frac{4}{3}L_{22ij}^{V,RR} + \frac{4}{3}L_{33ij}^{V,RR} - \frac{8}{3}L_{11ij}^{V1,LR} - \frac{8}{3}L_{22ij}^{V1,LR} - \frac{8}{3}L_{11ij}^{V1,RR} - \frac{8}{3}L_{22ij}^{V1,RR} \Big]
\end{aligned}$$

$$\begin{aligned}
& + \alpha_s \alpha \left[ \frac{16}{3} L_{kkij}^{V1,LR} - \frac{1010}{243} L_{kkij}^{V8,LR} + 8 L_{ijkk}^{V,RR} + \frac{304}{243} L_{ikkj}^{V,RR} + \frac{16}{3} L_{iijj}^{V1,LR} \right. \\
& + \frac{16}{3} L_{jjij}^{V1,LR} - \frac{1010}{243} L_{iijj}^{V8,LR} - \frac{1010}{243} L_{jjij}^{V8,LR} + \frac{1096}{81} L_{ijii}^{V,RR} + \frac{1096}{81} L_{ijjj}^{V,RR} \\
& + 16 L_{11ij}^{V,LR} - \frac{32}{3} L_{11ij}^{V1,LR} - \frac{32}{3} L_{22ij}^{V1,LR} - \frac{32}{3} L_{11ij}^{V1,RR} - \frac{32}{3} L_{22ij}^{V1,RR} + \frac{1366}{243} L_{11ij}^{V8,LR} \\
& + \frac{1366}{243} L_{22ij}^{V8,LR} - \frac{74}{243} L_{11ij}^{V8,RR} - \frac{74}{243} L_{22ij}^{V8,RR} \left. \right] + \alpha^2 \left[ \frac{1736}{243} L_{kkij}^{V1,LR} + \frac{304}{243} L_{ijkk}^{V,RR} \right. \\
& - \frac{1328}{729} L_{ikkj}^{V,RR} + \frac{1736}{243} L_{iijj}^{V1,LR} + \frac{1736}{243} L_{jjij}^{V1,LR} - \frac{752}{243} L_{ijii}^{V,RR} - \frac{752}{243} L_{ijjj}^{V,RR} \\
& + \frac{21698}{243} L_{11ij}^{V,LR} + \frac{3752}{243} L_{22ij}^{V,LR} + \frac{3752}{243} L_{33ij}^{V,LR} - \frac{1000}{243} L_{11ij}^{V,RR} - \frac{1000}{243} L_{22ij}^{V,RR} \\
& \left. - \frac{1000}{243} L_{33ij}^{V,RR} - \frac{664}{243} L_{11ij}^{V1,LR} - \frac{664}{243} L_{22ij}^{V1,LR} - \frac{7000}{243} L_{11ij}^{V1,RR} - \frac{7000}{243} L_{22ij}^{V1,RR} \right] ;
\end{aligned}$$

$$\begin{aligned}
\dot{L}_{ed22ij}^{V,LR} & = e^2 \left[ \frac{4}{3} L_{kkij}^{V1,LR} + \frac{8}{3} L_{ijkk}^{V,RR} + \frac{8}{9} L_{ikkj}^{V,RR} + \frac{4}{3} L_{iijj}^{V1,LR} + \frac{4}{3} L_{jjij}^{V1,LR} \right. \\
& + \frac{32}{9} L_{ijii}^{V,RR} + \frac{32}{9} L_{ijjj}^{V,RR} + \frac{4}{3} L_{11ij}^{V,LR} - \frac{8}{3} L_{22ij}^{V,LR} + \frac{4}{3} L_{33ij}^{V,LR} + \frac{4}{3} L_{11ij}^{V,RR} \\
& + \frac{4}{3} L_{22ij}^{V,RR} + \frac{4}{3} L_{33ij}^{V,RR} - \frac{8}{3} L_{11ij}^{V1,LR} - \frac{8}{3} L_{22ij}^{V1,LR} - \frac{8}{3} L_{11ij}^{V1,RR} - \frac{8}{3} L_{22ij}^{V1,RR} \left. \right] \\
& + \alpha_s \alpha \left[ \frac{16}{3} L_{kkij}^{V1,LR} - \frac{1010}{243} L_{kkij}^{V8,LR} + 8 L_{ijkk}^{V,RR} + \frac{304}{243} L_{ikkj}^{V,RR} + \frac{16}{3} L_{iijj}^{V1,LR} \right. \\
& + \frac{16}{3} L_{jjij}^{V1,LR} - \frac{1010}{243} L_{iijj}^{V8,LR} - \frac{1010}{243} L_{jjij}^{V8,LR} + \frac{1096}{81} L_{ijii}^{V,RR} + \frac{1096}{81} L_{ijjj}^{V,RR} \\
& + 16 L_{22ij}^{V,LR} - \frac{32}{3} L_{11ij}^{V1,LR} - \frac{32}{3} L_{22ij}^{V1,LR} - \frac{32}{3} L_{11ij}^{V1,RR} - \frac{32}{3} L_{22ij}^{V1,RR} + \frac{1366}{243} L_{11ij}^{V8,LR} \\
& + \frac{1366}{243} L_{22ij}^{V8,LR} - \frac{74}{243} L_{11ij}^{V8,RR} - \frac{74}{243} L_{22ij}^{V8,RR} \left. \right] + \alpha^2 \left[ \frac{1736}{243} L_{kkij}^{V1,LR} + \frac{304}{243} L_{ijkk}^{V,RR} \right. \\
& - \frac{1328}{729} L_{ikkj}^{V,RR} + \frac{1736}{243} L_{iijj}^{V1,LR} + \frac{1736}{243} L_{jjij}^{V1,LR} - \frac{752}{243} L_{ijii}^{V,RR} - \frac{752}{243} L_{ijjj}^{V,RR} \\
& + \frac{3752}{243} L_{11ij}^{V,LR} + \frac{21698}{243} L_{22ij}^{V,LR} + \frac{3752}{243} L_{33ij}^{V,LR} - \frac{1000}{243} L_{11ij}^{V,RR} - \frac{1000}{243} L_{22ij}^{V,RR}
\end{aligned}$$

$$\begin{aligned}
& -\frac{1000}{243}L_{33ij}^{V,RR} - \frac{664}{243}L_{11ij}^{V1,LR} - \frac{664}{243}L_{22ij}^{V1,LR} - \frac{7000}{243}L_{11ij}^{V1,RR} - \frac{7000}{243}L_{22ij}^{V1,RR} \Bigg]; \\
\dot{L}_{33ij}^{V,LR} = & e^2 \left[ \frac{4}{3}L_{kkij}^{V1,LR} + \frac{8}{3}L_{ijkk}^{V,RR} + \frac{8}{9}L_{ikkj}^{V,RR} + \frac{4}{3}L_{iiij}^{V1,LR} + \frac{4}{3}L_{jjij}^{V1,LR} \right. \\
& + \frac{32}{9}L_{ddij}^{V,RR} + \frac{32}{9}L_{ijjj}^{V,RR} + \frac{4}{3}L_{11ij}^{V,LR} + \frac{4}{3}L_{22ij}^{V,LR} - \frac{8}{3}L_{33ij}^{V,LR} + \frac{4}{3}L_{11ij}^{V,RR} \\
& + \frac{4}{3}L_{22ij}^{V,RR} + \frac{4}{3}L_{33ij}^{V,RR} - \frac{8}{3}L_{11ij}^{V1,LR} - \frac{8}{3}L_{22ij}^{V1,LR} - \frac{8}{3}L_{11ij}^{V1,RR} - \frac{8}{3}L_{22ij}^{V1,RR} \Bigg] \\
& + \alpha_s \alpha \left[ \frac{16}{3}L_{kkij}^{V1,LR} - \frac{1010}{243}L_{kkij}^{V8,LR} + 8L_{ijkk}^{V,RR} + \frac{304}{243}L_{ikkj}^{V,RR} + \frac{16}{3}L_{iiij}^{V1,LR} \right. \\
& + \frac{16}{3}L_{jjij}^{V1,LR} - \frac{1010}{243}L_{iiij}^{V8,LR} - \frac{1010}{243}L_{jjij}^{V8,LR} + \frac{1096}{81}L_{ijii}^{V,RR} + \frac{1096}{81}L_{ijjj}^{V,RR} \\
& + 16L_{33ij}^{V,LR} - \frac{32}{3}L_{11ij}^{V1,LR} - \frac{32}{3}L_{22ij}^{V1,LR} - \frac{32}{3}L_{11ij}^{V1,RR} - \frac{32}{3}L_{22ij}^{V1,RR} + \frac{1366}{243}L_{11ij}^{V8,LR} \\
& + \frac{1366}{243}L_{22ij}^{V8,LR} - \frac{74}{243}L_{11ij}^{V8,RR} - \frac{74}{243}L_{22ij}^{V8,RR} \Bigg] + \alpha^2 \left[ \frac{1736}{243}L_{kkij}^{V1,LR} + \frac{304}{243}L_{ikkj}^{V,RR} \right. \\
& - \frac{1328}{729}L_{ikkj}^{V,RR} + \frac{1736}{243}L_{iiij}^{V1,LR} + \frac{1736}{243}L_{jjij}^{V1,LR} - \frac{752}{243}L_{ijii}^{V,RR} - \frac{752}{243}L_{ijjj}^{V,RR} \\
& + \frac{3752}{243}L_{11ij}^{V,LR} + \frac{3752}{243}L_{22ij}^{V,LR} + \frac{21698}{243}L_{33ij}^{V,LR} - \frac{1000}{243}L_{11ij}^{V,RR} - \frac{1000}{243}L_{22ij}^{V,RR} \\
& - \frac{1000}{243}L_{33ij}^{V,RR} - \frac{664}{243}L_{11ij}^{V1,LR} - \frac{664}{243}L_{22ij}^{V1,LR} - \frac{7000}{243}L_{11ij}^{V1,RR} - \frac{7000}{243}L_{22ij}^{V1,RR} \Bigg]; \\
\dot{L}_{11ij}^{V1,LR} = & -\frac{8}{3}g_s^2 L_{11ij}^{V8,LR} + e^2 \left[ -\frac{8}{9}L_{kkij}^{V1,LR} - \frac{16}{9}L_{ijkk}^{V,RR} - \frac{16}{27}L_{ikkj}^{V,RR} - \frac{8}{9}L_{iiij}^{V1,LR} \right. \\
& - \frac{8}{9}L_{jjij}^{V1,LR} - \frac{64}{27}L_{ijii}^{V,RR} - \frac{64}{27}L_{ijjj}^{V,RR} - \frac{8}{9}L_{11ij}^{V,LR} - \frac{8}{9}L_{22ij}^{V,LR} - \frac{8}{9}L_{33ij}^{V,LR} \\
& - \frac{8}{9}L_{11ij}^{V,RR} - \frac{8}{9}L_{22ij}^{V,RR} - \frac{8}{9}L_{33ij}^{V,RR} + \frac{40}{9}L_{11ij}^{V1,LR} + \frac{16}{9}L_{22ij}^{V1,LR} + \frac{16}{9}L_{11ij}^{V1,RR} \\
& + \frac{16}{9}L_{22ij}^{V1,RR} \Bigg] + \alpha_s^2 \left[ 8L_{kkij}^{V1,LR} + \frac{44}{27}L_{kkij}^{V8,LR} - 16L_{ijkk}^{V,RR} - \frac{64}{27}L_{ikkj}^{V,RR} \right. \\
& + 8L_{iiij}^{V1,LR} + 8L_{jjij}^{V1,LR} + \frac{44}{27}L_{iiij}^{V8,LR} + \frac{44}{27}L_{jjij}^{V8,LR} - \frac{232}{9}L_{ijii}^{V,RR} - \frac{232}{9}L_{ijjj}^{V,RR}
\end{aligned}$$



$$\begin{aligned}
& -\frac{4}{3}L_{11ij}^{V1,LR} + 8L_{22ij}^{V1,LR} - 8L_{11ij}^{V1,RR} - 8L_{22ij}^{V1,RR} - \frac{2000}{27}L_{11ij}^{V8,LR} + \frac{44}{27}L_{22ij}^{V8,LR} \\
& + \frac{44}{27}L_{11ij}^{V8,RR} + \frac{44}{27}L_{22ij}^{V8,RR} \Big] + \alpha_s \alpha \Big[ -\frac{32}{9}L_{kkij}^{V1,LR} + \frac{2020}{729}L_{kkij}^{V8,LR} - \frac{16}{3}L_{ijkk}^{V,RR} \\
& - \frac{608}{729}L_{ikkj}^{V,RR} - \frac{32}{9}L_{iiij}^{V1,LR} - \frac{32}{9}L_{jjij}^{V1,LR} + \frac{2020}{729}L_{iiij}^{V8,LR} + \frac{2020}{729}L_{jjij}^{V8,LR} - \frac{2192}{243}L_{ijji}^{V,RR} \\
& - \frac{2192}{243}L_{ijjj}^{V,RR} - \frac{128}{9}L_{11ij}^{V1,LR} + \frac{64}{9}L_{22ij}^{V1,LR} + \frac{64}{9}L_{11ij}^{V1,RR} + \frac{64}{9}L_{22ij}^{V1,RR} + \frac{3532}{729}L_{11ij}^{V8,LR} \\
& - \frac{2732}{729}L_{22ij}^{V8,LR} + \frac{148}{729}L_{11ij}^{V8,RR} + \frac{148}{729}L_{22ij}^{V8,RR} \Big] + \alpha^2 \Big[ \frac{3728}{729}L_{kkij}^{V1,LR} + \frac{832}{729}L_{ijkk}^{V,RR} \\
& - \frac{224}{2187}L_{ikkj}^{V,RR} + \frac{3728}{729}L_{iiij}^{V1,LR} + \frac{3728}{729}L_{jjij}^{V1,LR} + \frac{784}{729}L_{ijii}^{V,RR} + \frac{784}{729}L_{ijjj}^{V,RR} \\
& + \frac{6176}{729}L_{11ij}^{V,LR} + \frac{6176}{729}L_{22ij}^{V,LR} + \frac{6176}{729}L_{33ij}^{V,LR} - \frac{3760}{729}L_{11ij}^{V,RR} - \frac{3760}{729}L_{22ij}^{V,RR} \\
& - \frac{3760}{729}L_{33ij}^{V,RR} - \frac{30064}{729}L_{11ij}^{V1,LR} + \frac{6368}{729}L_{22ij}^{V1,LR} - \frac{6880}{729}L_{11ij}^{V1,RR} - \frac{6880}{729}L_{22ij}^{V1,RR} \Big] ;
\end{aligned}$$

$$\begin{aligned}
\dot{L}_{11ij}^{V8,LR} &= g_s^2 \Big[ \frac{2}{3}L_{kkij}^{V8,LR} + \frac{8}{3}L_{ikkj}^{V,RR} + \frac{2}{3}L_{iiij}^{V8,LR} + \frac{2}{3}L_{jjij}^{V8,LR} + \frac{8}{3}L_{ijii}^{V,RR} \\
& + \frac{8}{3}L_{ijjj}^{V,RR} - 12L_{11ij}^{V1,LR} - \frac{40}{3}L_{11ij}^{V8,LR} + \frac{2}{3}L_{22ij}^{V8,LR} + \frac{2}{3}L_{11ij}^{V8,RR} + \frac{2}{3}L_{22ij}^{V8,RR} \Big] \\
& + \frac{8}{3}e^2L_{11ij}^{V8,LR} + \alpha_s^2 \Big[ -\frac{22}{3}L_{kkij}^{V1,LR} + \frac{781}{81}L_{kkij}^{V8,LR} - \frac{28}{3}L_{ijkk}^{V,RR} + \frac{3400}{81}L_{ikkj}^{V,RR} \\
& - \frac{22}{3}L_{iiij}^{V1,LR} - \frac{22}{3}L_{jjij}^{V1,LR} + \frac{781}{81}L_{iiij}^{V8,LR} + \frac{781}{81}L_{jjij}^{V8,LR} + \frac{1186}{27}L_{ijii}^{V,RR} + \frac{1186}{27}L_{ijjj}^{V,RR} \\
& - 132L_{11ij}^{V1,LR} - \frac{22}{3}L_{22ij}^{V1,LR} - \frac{2}{3}L_{11ij}^{V1,RR} - \frac{2}{3}L_{22ij}^{V1,RR} - \frac{25213}{162}L_{11ij}^{V8,LR} + \frac{781}{81}L_{22ij}^{V8,LR} \\
& + \frac{601}{81}L_{11ij}^{V8,RR} + \frac{601}{81}L_{22ij}^{V8,RR} \Big] + \alpha_s \alpha \Big[ -\frac{928}{81}L_{kkij}^{V1,LR} - \frac{44}{9}L_{kkij}^{V8,LR} - \frac{1856}{81}L_{ijkk}^{V,RR} \\
& + \frac{688}{243}L_{ikkj}^{V,RR} - \frac{928}{81}L_{iiij}^{V1,LR} - \frac{928}{81}L_{jjij}^{V1,LR} - \frac{44}{9}L_{iiij}^{V8,LR} - \frac{44}{9}L_{jjij}^{V8,LR} - \frac{2192}{81}L_{ijii}^{V,RR} \\
& - \frac{2192}{81}L_{ijjj}^{V,RR} - \frac{928}{81}L_{11ij}^{V,LR} - \frac{928}{81}L_{22ij}^{V,LR} - \frac{928}{81}L_{33ij}^{V,LR} - \frac{928}{81}L_{11ij}^{V,RR} - \frac{928}{81}L_{22ij}^{V,RR}
\end{aligned}$$

$$\begin{aligned}
& -\frac{928}{81}L_{33ij}^{V,RR} + \frac{4988}{81}L_{11ij}^{V1,LR} + \frac{1856}{81}L_{22ij}^{V1,LR} + \frac{1856}{81}L_{11ij}^{V1,RR} + \frac{1856}{81}L_{22ij}^{V1,RR} \\
& + 27L_{11ij}^{V8,LR} + \frac{56}{9}L_{22ij}^{V8,LR} - \frac{160}{27}L_{11ij}^{V8,RR} - \frac{160}{27}L_{22ij}^{V8,RR} \Big] - \frac{4048}{81}\alpha^2 L_{11ij}^{V8,LR} ; \\
\dot{L}_{22ij}^{V1,LR} = & -\frac{8}{3}g_s^2 L_{22ij}^{V8,LR} + e^2 \Big[ -\frac{8}{9}L_{kkij}^{V1,LR} - \frac{16}{9}L_{ijkk}^{V,RR} - \frac{16}{27}L_{ikkj}^{V,RR} - \frac{8}{9}L_{iiij}^{V1,LR} \\
& - \frac{8}{9}L_{jjij}^{V1,LR} - \frac{64}{27}L_{ddii}^{V,RR} - \frac{64}{27}L_{ijjj}^{V,RR} - \frac{8}{9}L_{11ij}^{V,LR} - \frac{8}{9}L_{22ij}^{V,LR} - \frac{8}{9}L_{33ij}^{V,LR} \\
& - \frac{8}{9}L_{11ij}^{V,RR} - \frac{8}{9}L_{22ij}^{V,RR} - \frac{8}{9}L_{33ij}^{V,RR} + \frac{16}{9}L_{11ij}^{V1,LR} + \frac{40}{9}L_{22ij}^{V1,LR} + \frac{16}{9}L_{11ij}^{V1,RR} \\
& + \frac{16}{9}L_{22ij}^{V1,RR} \Big] + \alpha_s^2 \Big[ 8L_{kkij}^{V1,LR} + \frac{44}{27}L_{kkij}^{V8,LR} - 16L_{ijkk}^{V,RR} - \frac{64}{27}L_{ikkj}^{V,RR} \\
& + 8L_{iiij}^{V1,LR} + 8L_{jjij}^{V1,LR} + \frac{44}{27}L_{iiij}^{V8,LR} + \frac{44}{27}L_{jjij}^{V8,LR} - \frac{232}{9}L_{ijii}^{V,RR} - \frac{232}{9}L_{ijjj}^{V,RR} \\
& + 8L_{11ij}^{V1,LR} - \frac{4}{3}L_{22ij}^{V1,LR} - 8L_{11ij}^{V1,RR} - 8L_{22ij}^{V1,RR} + \frac{44}{27}L_{11ij}^{V8,LR} - \frac{2000}{27}L_{22ij}^{V8,LR} \\
& + \frac{44}{27}L_{11ij}^{V8,RR} + \frac{44}{27}L_{22ij}^{V8,RR} \Big] + \alpha_s \alpha \Big[ -\frac{32}{9}L_{kkij}^{V1,LR} + \frac{2020}{729}L_{kkij}^{V8,LR} - \frac{16}{3}L_{ijkk}^{V,RR} \\
& - \frac{608}{729}L_{ikkj}^{V,RR} - \frac{32}{9}L_{iiij}^{V1,LR} - \frac{32}{9}L_{jjij}^{V1,LR} + \frac{2020}{729}L_{iiij}^{V8,LR} + \frac{2020}{729}L_{jjij}^{V8,LR} - \frac{2192}{243}L_{ijii}^{V,RR} \\
& - \frac{2192}{243}L_{ijjj}^{V,RR} + \frac{64}{9}L_{11ij}^{V1,LR} - \frac{128}{9}L_{22ij}^{V1,LR} + \frac{64}{9}L_{11ij}^{V1,RR} + \frac{64}{9}L_{22ij}^{V1,RR} - \frac{2732}{729}L_{11ij}^{V8,LR} \\
& + \frac{3532}{729}L_{22ij}^{V8,LR} + \frac{148}{729}L_{11ij}^{V8,RR} + \frac{148}{729}L_{22ij}^{V8,RR} \Big] + \alpha^2 \Big[ \frac{3728}{729}L_{kkij}^{V1,LR} + \frac{832}{729}L_{ijkk}^{V,RR} \\
& - \frac{224}{2187}L_{ikkj}^{V,RR} + \frac{3728}{729}L_{iiij}^{V1,LR} + \frac{3728}{729}L_{jjij}^{V1,LR} + \frac{784}{729}L_{ijii}^{V,RR} + \frac{784}{729}L_{ijjj}^{V,RR} \\
& + \frac{6176}{729}L_{11ij}^{V,LR} + \frac{6176}{729}L_{22ij}^{V,LR} + \frac{6176}{729}L_{33ij}^{V,LR} - \frac{3760}{729}L_{11ij}^{V,RR} - \frac{3760}{729}L_{22ij}^{V,RR} \\
& - \frac{3760}{729}L_{33ij}^{V,RR} + \frac{6368}{729}L_{11ij}^{V1,LR} - \frac{30064}{729}L_{22ij}^{V1,LR} - \frac{6880}{729}L_{11ij}^{V1,RR} - \frac{6880}{729}L_{22ij}^{V1,RR} \Big] ; \\
\dot{L}_{22ij}^{V8,LR} = & g_s^2 \Big[ \frac{2}{3}L_{kkij}^{V8,LR} + \frac{8}{3}L_{ikkj}^{V,RR} + \frac{2}{3}L_{iiij}^{V8,LR} + \frac{2}{3}L_{jjij}^{V8,LR} + \frac{8}{3}L_{ijii}^{V,RR}
\end{aligned}$$

$$\begin{aligned}
& + \frac{8}{3} L_{ijjj}^{V,RR} - 12 L_{22ij}^{V1,LR} + \frac{2}{3} L_{11ij}^{V8,LR} - \frac{40}{3} L_{22ij}^{V8,LR} + \frac{2}{3} L_{11ij}^{V8,RR} + \frac{2}{3} L_{22ij}^{V8,RR} \Big] \\
& + \frac{8}{3} e^2 L_{22ij}^{V8,LR} + \alpha_s^2 \Bigg[ - \frac{22}{3} L_{kkij}^{V1,LR} + \frac{781}{81} L_{kkij}^{V8,LR} - \frac{28}{3} L_{ijkk}^{V,RR} + \frac{3400}{81} L_{ikkj}^{V,RR} \\
& - \frac{22}{3} L_{iiij}^{V1,LR} - \frac{22}{3} L_{jjij}^{V1,LR} + \frac{781}{81} L_{iiij}^{V8,LR} + \frac{781}{81} L_{jjij}^{V8,LR} + \frac{1186}{27} L_{ddii}^{V,RR} + \frac{1186}{27} L_{ijjj}^{V,RR} \\
& - \frac{22}{3} L_{11ij}^{V1,LR} - 132 L_{22ij}^{V1,LR} - \frac{2}{3} L_{11ij}^{V1,RR} - \frac{2}{3} L_{22ij}^{V1,RR} + \frac{781}{81} L_{11ij}^{V8,LR} - \frac{25213}{162} L_{22ij}^{V8,LR} \\
& + \frac{601}{81} L_{11ij}^{V8,RR} + \frac{601}{81} L_{22ij}^{V8,RR} \Bigg] + \alpha_s \alpha \Bigg[ - \frac{928}{81} L_{kkij}^{V1,LR} - \frac{44}{9} L_{kkij}^{V8,LR} - \frac{1856}{81} L_{ijkk}^{V,RR} \\
& + \frac{688}{243} L_{ikkj}^{V,RR} - \frac{928}{81} L_{iiij}^{V1,LR} - \frac{928}{81} L_{jjij}^{V1,LR} - \frac{44}{9} L_{iiij}^{V8,LR} - \frac{44}{9} L_{jjij}^{V8,LR} - \frac{2192}{81} L_{ijii}^{V,RR} \\
& - \frac{2192}{81} L_{ijjj}^{V,RR} - \frac{928}{81} L_{11ij}^{V,LR} - \frac{928}{81} L_{22ij}^{V,LR} - \frac{928}{81} L_{33ij}^{V,LR} - \frac{928}{81} L_{11ij}^{V,RR} - \frac{928}{81} L_{22ij}^{V,RR} \\
& - \frac{928}{81} L_{33ij}^{V,RR} + \frac{1856}{81} L_{11ij}^{V1,LR} + \frac{4988}{81} L_{22ij}^{V1,LR} + \frac{1856}{81} L_{11ij}^{V1,RR} + \frac{1856}{81} L_{22ij}^{V1,RR} \\
& + \frac{56}{9} L_{11ij}^{V8,LR} + 27 L_{22ij}^{V8,LR} - \frac{160}{27} L_{11ij}^{V8,RR} - \frac{160}{27} L_{22ij}^{V8,RR} \Bigg] - \frac{4048}{81} \alpha^2 L_{22ij}^{V8,LR} ;
\end{aligned}$$

$$\begin{aligned}
\dot{L}_{kkij}^{V1,LR} = & - \frac{8}{3} g_s^2 L_{kkij}^{V8,LR} + e^2 \Bigg[ - \frac{8}{9} L_{kkij}^{V1,LR} + \frac{8}{9} L_{ijkk}^{V,RR} + \frac{8}{27} L_{ikkj}^{V,RR} + \frac{4}{9} L_{iiij}^{V1,LR} \\
& + \frac{4}{9} L_{jjij}^{V1,LR} + \frac{32}{27} L_{ijii}^{V,RR} + \frac{32}{27} L_{ijjj}^{V,RR} + \frac{4}{9} L_{11ij}^{V,LR} + \frac{4}{9} L_{22ij}^{V,LR} + \frac{4}{9} L_{33ij}^{V,LR} \\
& + \frac{4}{9} L_{11ij}^{V,RR} + \frac{4}{9} L_{22ij}^{V,RR} + \frac{4}{9} L_{33ij}^{V,RR} - \frac{8}{9} L_{11ij}^{V1,LR} - \frac{8}{9} L_{22ij}^{V1,LR} - \frac{8}{9} L_{11ij}^{V1,RR} \\
& - \frac{8}{9} L_{22ij}^{V1,RR} \Bigg] + \alpha_s^2 \Bigg[ - \frac{4}{3} L_{kkij}^{V1,LR} - \frac{2000}{27} L_{kkij}^{V8,LR} - 16 L_{ijkk}^{V,RR} - \frac{64}{27} L_{ikkj}^{V,RR} \\
& + 8 L_{iiij}^{V1,LR} + 8 L_{jjij}^{V1,LR} + \frac{44}{27} L_{iiij}^{V8,LR} + \frac{44}{27} L_{jjij}^{V8,LR} - \frac{232}{9} L_{ijii}^{V,RR} - \frac{232}{9} L_{ijjj}^{V,RR} \\
& + 8 L_{11ij}^{V1,LR} + 8 L_{22ij}^{V1,LR} - 8 L_{11ij}^{V1,RR} - 8 L_{22ij}^{V1,RR} + \frac{44}{27} L_{11ij}^{V8,LR} + \frac{44}{27} L_{22ij}^{V8,LR} \\
& + \frac{44}{27} L_{11ij}^{V8,RR} + \frac{44}{27} L_{22ij}^{V8,RR} \Bigg] + \alpha_s \alpha \Bigg[ \frac{112}{9} L_{kkij}^{V1,LR} - \frac{1226}{729} L_{kkij}^{V8,LR} + \frac{8}{3} L_{ijkk}^{V,RR}
\end{aligned}$$

$$\begin{aligned}
& + \frac{304}{729} L_{ikkj}^{V,RR} + \frac{16}{9} L_{iiij}^{V1,LR} + \frac{16}{9} L_{jjij}^{V1,LR} - \frac{1010}{729} L_{iiij}^{V8,LR} - \frac{1010}{729} L_{jjij}^{V8,LR} + \frac{1096}{243} L_{ijji}^{V,RR} \\
& + \frac{1096}{243} L_{ijjj}^{V,RR} - \frac{32}{9} L_{11ij}^{V1,LR} - \frac{32}{9} L_{22ij}^{V1,LR} - \frac{32}{9} L_{11ij}^{V1,RR} - \frac{32}{9} L_{22ij}^{V1,RR} + \frac{1366}{729} L_{11ij}^{V8,LR} \\
& + \frac{1366}{729} L_{22ij}^{V8,LR} - \frac{74}{729} L_{11ij}^{V8,RR} - \frac{74}{729} L_{22ij}^{V8,RR} \Big] + \alpha^2 \Big[ \frac{16406}{729} L_{kkij}^{V1,LR} + \frac{16}{729} L_{ijkk}^{V,RR} \\
& - \frac{752}{2187} L_{ikkj}^{V,RR} + \frac{296}{729} L_{iiij}^{V1,LR} + \frac{296}{729} L_{jjij}^{V1,LR} - \frac{608}{729} L_{ijii}^{V,RR} - \frac{608}{729} L_{ijjj}^{V,RR} \\
& + \frac{1016}{729} L_{11ij}^{V,LR} + \frac{1016}{729} L_{22ij}^{V,LR} + \frac{1016}{729} L_{33ij}^{V,LR} + \frac{152}{729} L_{11ij}^{V,RR} + \frac{152}{729} L_{22ij}^{V,RR} \\
& + \frac{152}{729} L_{33ij}^{V,RR} - \frac{1672}{729} L_{11ij}^{V1,LR} - \frac{1672}{729} L_{22ij}^{V1,LR} - \frac{2824}{729} L_{11ij}^{V1,RR} - \frac{2824}{729} L_{22ij}^{V1,RR} \Big] ;
\end{aligned}$$

$$\begin{aligned}
\dot{L}_{kkij}^{V8,LR} &= g_s^2 \Big[ -12 L_{kkij}^{V1,LR} - \frac{40}{3} L_{kkij}^{V8,LR} + \frac{8}{3} L_{ikkj}^{V,RR} + \frac{2}{3} L_{iiij}^{V8,LR} + \frac{2}{3} L_{jjij}^{V8,LR} \\
& + \frac{8}{3} L_{ijii}^{V,RR} + \frac{8}{3} L_{ijjj}^{V,RR} + \frac{2}{3} L_{11ij}^{V8,LR} + \frac{2}{3} L_{22ij}^{V8,LR} + \frac{2}{3} L_{11ij}^{V8,RR} + \frac{2}{3} L_{22ij}^{V8,RR} \Big] \\
& - \frac{4}{3} e^2 L_{kkij}^{V8,LR} + \alpha_s^2 \Big[ -132 L_{kkij}^{V1,LR} - \frac{25213}{162} L_{kkij}^{V8,LR} - \frac{28}{3} L_{ijkk}^{V,RR} + \frac{3400}{81} L_{ikkj}^{V,RR} \\
& - \frac{22}{3} L_{iiij}^{V1,LR} - \frac{22}{3} L_{jjij}^{V1,LR} + \frac{781}{81} L_{iiij}^{V8,LR} + \frac{781}{81} L_{jjij}^{V8,LR} + \frac{1186}{27} L_{ijii}^{V,RR} + \frac{1186}{27} L_{ijjj}^{V,RR} \\
& - \frac{22}{3} L_{11ij}^{V1,LR} - \frac{22}{3} L_{22ij}^{V1,LR} - \frac{2}{3} L_{11ij}^{V1,RR} - \frac{2}{3} L_{22ij}^{V1,RR} + \frac{781}{81} L_{11ij}^{V8,LR} + \frac{781}{81} L_{22ij}^{V8,LR} \\
& + \frac{601}{81} L_{11ij}^{V8,RR} + \frac{601}{81} L_{22ij}^{V8,RR} \Big] + \alpha_s \alpha \Big[ \frac{152}{81} L_{kkij}^{V1,LR} - \frac{4}{3} L_{kkij}^{V8,LR} + \frac{520}{81} L_{ijkk}^{V,RR} \\
& - \frac{1040}{243} L_{ikkj}^{V,RR} + \frac{260}{81} L_{iiij}^{V1,LR} + \frac{260}{81} L_{jjij}^{V1,LR} + \frac{14}{9} L_{iiij}^{V8,LR} + \frac{14}{9} L_{jjij}^{V8,LR} + \frac{292}{81} L_{ijii}^{V,RR} \\
& + \frac{292}{81} L_{ijjj}^{V,RR} + \frac{260}{81} L_{11ij}^{V,LR} + \frac{260}{81} L_{22ij}^{V,LR} + \frac{260}{81} L_{33ij}^{V,LR} + \frac{260}{81} L_{11ij}^{V,RR} + \frac{260}{81} L_{22ij}^{V,RR} \\
& + \frac{260}{81} L_{33ij}^{V,RR} - \frac{520}{81} L_{11ij}^{V1,LR} - \frac{520}{81} L_{22ij}^{V1,LR} - \frac{520}{81} L_{11ij}^{V1,RR} - \frac{520}{81} L_{22ij}^{V1,RR} + \frac{2}{3} L_{11ij}^{V8,LR} \\
& + \frac{2}{3} L_{22ij}^{V8,LR} + \frac{122}{27} L_{11ij}^{V8,RR} + \frac{122}{27} L_{22ij}^{V8,RR} \Big] + \frac{1790}{81} \alpha^2 L_{kkij}^{V8,LR} ;
\end{aligned}$$

$$\begin{aligned}
\dot{L}_{dd,jjij}^{V1,LR} = & -\frac{8}{3}g_s^2 L_{jjij}^{V8,LR} + e^2 \left[ \frac{4}{9} L_{kkij}^{V1,LR} + \frac{8}{9} L_{ijkk}^{V,RR} + \frac{8}{27} L_{ikkj}^{V,RR} + \frac{4}{9} L_{iijj}^{V1,LR} \right. \\
& - \frac{8}{9} L_{jjij}^{V1,LR} + \frac{32}{27} L_{ijii}^{V,RR} + \frac{32}{27} L_{ijjj}^{V,RR} + \frac{4}{9} L_{11ij}^{V,LR} + \frac{4}{9} L_{22ij}^{V,LR} + \frac{4}{9} L_{33ij}^{V,LR} \\
& + \frac{4}{9} L_{11ij}^{V,RR} + \frac{4}{9} L_{22ij}^{V,RR} + \frac{4}{9} L_{33ij}^{V,RR} - \frac{8}{9} L_{ud,11ij}^{V1,LR} - \frac{8}{9} L_{ud,22ij}^{V1,LR} - \frac{8}{9} L_{ud,11ij}^{V1,RR} \\
& \left. - \frac{8}{9} L_{ud,22ij}^{V1,RR} \right] + \alpha_s^2 \left[ 8 L_{kkij}^{V1,LR} + \frac{44}{27} L_{kkij}^{V8,LR} - 16 L_{ijkk}^{V,RR} - \frac{64}{27} L_{ikkj}^{V,RR} \right. \\
& + 8 L_{iijj}^{V1,LR} - \frac{4}{3} L_{jjij}^{V1,LR} + \frac{44}{27} L_{iijj}^{V8,LR} - \frac{2000}{27} L_{jjij}^{V8,LR} - \frac{232}{9} L_{ijii}^{V,RR} - \frac{232}{9} L_{ijjj}^{V,RR} \\
& + 8 L_{ud,11ij}^{V1,LR} + 8 L_{ud,22ij}^{V1,LR} - 8 L_{ud,11ij}^{V1,RR} - 8 L_{ud,22ij}^{V1,RR} + \frac{44}{27} L_{ud,11ij}^{V8,LR} + \frac{44}{27} L_{ud,22ij}^{V8,LR} \\
& + \frac{44}{27} L_{ud,11ij}^{V8,RR} + \frac{44}{27} L_{ud,22ij}^{V8,RR} \left. \right] + \alpha_s \alpha \left[ \frac{16}{9} L_{kkij}^{V1,LR} - \frac{1010}{729} L_{kkij}^{V8,LR} + \frac{8}{3} L_{ijkk}^{V,RR} \right. \\
& + \frac{304}{729} L_{ikkj}^{V,RR} + \frac{16}{9} L_{iijj}^{V1,LR} + \frac{112}{9} L_{jjij}^{V1,LR} - \frac{1010}{729} L_{iijj}^{V8,LR} - \frac{1226}{729} L_{jjij}^{V8,LR} \\
& + \frac{1096}{243} L_{ijii}^{V,RR} + \frac{1096}{243} L_{ijjj}^{V,RR} - \frac{32}{9} L_{ud,11ij}^{V1,LR} - \frac{32}{9} L_{ud,22ij}^{V1,LR} - \frac{32}{9} L_{ud,11ij}^{V1,RR} - \frac{32}{9} L_{ud,22ij}^{V1,RR} \\
& + \frac{1366}{729} L_{ud,11ij}^{V8,LR} + \frac{1366}{729} L_{ud,22ij}^{V8,LR} - \frac{74}{729} L_{ud,11ij}^{V8,RR} - \frac{74}{729} L_{ud,22ij}^{V8,RR} \left. \right] + \alpha^2 \left[ \frac{296}{729} L_{kkij}^{V1,LR} \right. \\
& + \frac{16}{729} L_{ijkk}^{V,RR} - \frac{752}{2187} L_{ikkj}^{V,RR} + \frac{296}{729} L_{iijj}^{V1,LR} + \frac{16406}{729} L_{jjij}^{V1,LR} - \frac{608}{729} L_{ijii}^{V,RR} \\
& - \frac{608}{729} L_{ijjj}^{V,RR} + \frac{1016}{729} L_{11ij}^{V,LR} + \frac{1016}{729} L_{22ij}^{V,LR} + \frac{1016}{729} L_{33ij}^{V,LR} + \frac{152}{729} L_{11ij}^{V,RR} \\
& + \frac{152}{729} L_{22ij}^{V,RR} + \frac{152}{729} L_{33ij}^{V,RR} - \frac{1672}{729} L_{ud,11ij}^{V1,LR} - \frac{1672}{729} L_{ud,22ij}^{V1,LR} - \frac{2824}{729} L_{ud,11ij}^{V1,RR} \\
& \left. - \frac{2824}{729} L_{ud,22ij}^{V1,RR} \right];
\end{aligned}$$

$$\begin{aligned}
\dot{L}_{dd,jjij}^{V8,LR} = & g_s^2 \left[ \frac{2}{3} L_{kkij}^{V8,LR} + \frac{8}{3} L_{ikkj}^{V,RR} - 12 L_{jjij}^{V1,LR} + \frac{2}{3} L_{iijj}^{V8,LR} - \frac{40}{3} L_{jjij}^{V8,LR} \right. \\
& \left. + \frac{8}{3} L_{ijii}^{V,RR} + \frac{8}{3} L_{ijjj}^{V,RR} + \frac{2}{3} L_{11ij}^{V8,LR} + \frac{2}{3} L_{22ij}^{V8,LR} + \frac{2}{3} L_{11ij}^{V8,RR} + \frac{2}{3} L_{22ij}^{V8,RR} \right]
\end{aligned}$$

$$\begin{aligned}
& -\frac{4}{3}e^2 L_{jjij}^{V8,LR} + \alpha_s^2 \left[ -\frac{22}{3} L_{kkij}^{V1,LR} + \frac{781}{81} L_{kkij}^{V8,LR} - \frac{28}{3} L_{ijkk}^{V,RR} + \frac{3400}{81} L_{ikkj}^{V,RR} \right. \\
& -\frac{22}{3} L_{iiij}^{V1,LR} - 132 L_{jjij}^{V1,LR} + \frac{781}{81} L_{iiij}^{V8,LR} - \frac{25213}{162} L_{jjij}^{V8,LR} + \frac{1186}{27} L_{ijii}^{V,RR} + \frac{1186}{27} L_{ijjj}^{V,RR} \\
& -\frac{22}{3} L_{ud11ij}^{V1,LR} - \frac{22}{3} L_{ud22ij}^{V1,LR} - \frac{2}{3} L_{ud11ij}^{V1,RR} - \frac{2}{3} L_{ud22ij}^{V1,RR} + \frac{781}{81} L_{ud11ij}^{V8,LR} + \frac{781}{81} L_{ud22ij}^{V8,LR} \\
& \left. + \frac{601}{81} L_{ud11ij}^{V8,RR} + \frac{601}{81} L_{ud22ij}^{V8,RR} \right] + \alpha_s \alpha \left[ \frac{260}{81} L_{kkij}^{V1,LR} + \frac{14}{9} L_{kkij}^{V8,LR} + \frac{520}{81} L_{ijkk}^{V,RR} \right. \\
& -\frac{1040}{243} L_{ikkj}^{V,RR} + \frac{260}{81} L_{iiij}^{V1,LR} + \frac{152}{81} L_{jjij}^{V1,LR} + \frac{14}{9} L_{iiij}^{V8,LR} - \frac{4}{3} L_{jjij}^{V8,LR} + \frac{292}{81} L_{ijii}^{V,RR} \\
& + \frac{292}{81} L_{ijjj}^{V,RR} + \frac{260}{81} L_{ed11ij}^{V,LR} + \frac{260}{81} L_{ed22ij}^{V,LR} + \frac{260}{81} L_{ed33ij}^{V,LR} + \frac{260}{81} L_{ed11ij}^{V,RR} + \frac{260}{81} L_{ed22ij}^{V,RR} \\
& + \frac{260}{81} L_{ed33ij}^{V,RR} - \frac{520}{81} L_{ud11ij}^{V1,LR} - \frac{520}{81} L_{ud22ij}^{V1,LR} - \frac{520}{81} L_{ud11ij}^{V1,RR} - \frac{520}{81} L_{ud22ij}^{V1,RR} + \frac{2}{3} L_{ud11ij}^{V8,LR} \\
& \left. + \frac{2}{3} L_{ud22ij}^{V8,LR} + \frac{122}{27} L_{ud11ij}^{V8,RR} + \frac{122}{27} L_{ud22ij}^{V8,RR} \right] + \frac{1790}{81} \alpha^2 L_{jjij}^{V8,LR} ;
\end{aligned}$$

$$\begin{aligned}
\dot{L}_{iiij}^{V1,LR} = & -\frac{8}{3}g_s^2 L_{iiij}^{V8,LR} + e^2 \left[ \frac{4}{9} L_{kkij}^{V1,LR} + \frac{8}{9} L_{ijkk}^{V,RR} + \frac{8}{27} L_{ikkj}^{V,RR} - \frac{8}{9} L_{iiij}^{V1,LR} \right. \\
& + \frac{4}{9} L_{jjij}^{V1,LR} + \frac{32}{27} L_{ijii}^{V,RR} + \frac{32}{27} L_{ijjj}^{V,RR} + \frac{4}{9} L_{ed11ij}^{V,LR} + \frac{4}{9} L_{ed22ij}^{V,LR} + \frac{4}{9} L_{ed33ij}^{V,LR} \\
& + \frac{4}{9} L_{ed11ij}^{V,RR} + \frac{4}{9} L_{ed22ij}^{V,RR} + \frac{4}{9} L_{ed33ij}^{V,RR} - \frac{8}{9} L_{ud11ij}^{V1,LR} - \frac{8}{9} L_{ud22ij}^{V1,LR} - \frac{8}{9} L_{ud11ij}^{V1,RR} \\
& \left. - \frac{8}{9} L_{ud22ij}^{V1,RR} \right] + \alpha_s^2 \left[ 8 L_{kkij}^{V1,LR} + \frac{44}{27} L_{kkij}^{V8,LR} - 16 L_{ijkk}^{V,RR} - \frac{64}{27} L_{ikkj}^{V,RR} \right. \\
& - \frac{4}{3} L_{iiij}^{V1,LR} + 8 L_{jjij}^{V1,LR} - \frac{2000}{27} L_{iiij}^{V8,LR} + \frac{44}{27} L_{jjij}^{V8,LR} - \frac{232}{9} L_{ijii}^{V,RR} - \frac{232}{9} L_{ijjj}^{V,RR} \\
& + 8 L_{ud11ij}^{V1,LR} + 8 L_{ud22ij}^{V1,LR} - 8 L_{ud11ij}^{V1,RR} - 8 L_{ud22ij}^{V1,RR} + \frac{44}{27} L_{ud11ij}^{V8,LR} + \frac{44}{27} L_{ud22ij}^{V8,LR} \\
& \left. + \frac{44}{27} L_{ud11ij}^{V8,RR} + \frac{44}{27} L_{ud22ij}^{V8,RR} \right] + \alpha_s \alpha \left[ \frac{16}{9} L_{kkij}^{V1,LR} - \frac{1010}{729} L_{kkij}^{V8,LR} + \frac{8}{3} L_{ijkk}^{V,RR} \right. \\
& \left. + \frac{304}{729} L_{ikkj}^{V,RR} + \frac{112}{9} L_{iiij}^{V1,LR} + \frac{16}{9} L_{jjij}^{V1,LR} - \frac{1226}{729} L_{iiij}^{V8,LR} - \frac{1010}{729} L_{jjij}^{V8,LR} \right]
\end{aligned}$$

$$\begin{aligned}
& + \frac{1096}{243} L_{ijii}^{V,RR} + \frac{1096}{243} L_{ijjj}^{V,RR} - \frac{32}{9} L_{11ij}^{V1,LR} - \frac{32}{9} L_{22ij}^{V1,LR} - \frac{32}{9} L_{11ij}^{V1,RR} - \frac{32}{9} L_{22ij}^{V1,RR} \\
& + \frac{1366}{729} L_{11ij}^{V8,LR} + \frac{1366}{729} L_{22ij}^{V8,LR} - \frac{74}{729} L_{11ij}^{V8,RR} - \frac{74}{729} L_{22ij}^{V8,RR} \Big] + \alpha^2 \Big[ \frac{296}{729} L_{kkij}^{V1,LR} \\
& + \frac{16}{729} L_{ijkk}^{V,RR} - \frac{752}{2187} L_{ikkj}^{V,RR} + \frac{16406}{729} L_{iiij}^{V1,LR} + \frac{296}{729} L_{jjij}^{V1,LR} - \frac{608}{729} L_{ijii}^{V,RR} \\
& - \frac{608}{729} L_{ijjj}^{V,RR} + \frac{1016}{729} L_{11ij}^{V,LR} + \frac{1016}{729} L_{22ij}^{V,LR} + \frac{1016}{729} L_{33ij}^{V,LR} + \frac{152}{729} L_{11ij}^{V,RR} \\
& + \frac{152}{729} L_{22ij}^{V,RR} + \frac{152}{729} L_{33ij}^{V,RR} - \frac{1672}{729} L_{11ij}^{V1,LR} - \frac{1672}{729} L_{22ij}^{V1,LR} - \frac{2824}{729} L_{11ij}^{V1,RR} \\
& - \frac{2824}{729} L_{22ij}^{V1,RR} \Big] ;
\end{aligned}$$

$$\begin{aligned}
\dot{L}_{iiij}^{V8,LR} & = g_s^2 \Big[ \frac{2}{3} L_{kkij}^{V8,LR} + \frac{8}{3} L_{ikkj}^{V,RR} - 12 L_{iiij}^{V1,LR} - \frac{40}{3} L_{iiij}^{V8,LR} + \frac{2}{3} L_{jjij}^{V8,LR} \\
& + \frac{8}{3} L_{ijii}^{V,RR} + \frac{8}{3} L_{ijjj}^{V,RR} + \frac{2}{3} L_{11ij}^{V8,LR} + \frac{2}{3} L_{22ij}^{V8,LR} + \frac{2}{3} L_{11ij}^{V8,RR} + \frac{2}{3} L_{22ij}^{V8,RR} \Big] \\
& - \frac{4}{3} e^2 L_{iiij}^{V8,LR} + \alpha_s^2 \Big[ - \frac{22}{3} L_{kkij}^{V1,LR} + \frac{781}{81} L_{kkij}^{V8,LR} - \frac{28}{3} L_{ijkk}^{V,RR} + \frac{3400}{81} L_{ikkj}^{V,RR} \\
& - 132 L_{iiij}^{V1,LR} - \frac{22}{3} L_{jjij}^{V1,LR} - \frac{25213}{162} L_{iiij}^{V8,LR} + \frac{781}{81} L_{jjij}^{V8,LR} + \frac{1186}{27} L_{ijii}^{V,RR} + \frac{1186}{27} L_{ijjj}^{V,RR} \\
& - \frac{22}{3} L_{11ij}^{V1,LR} - \frac{22}{3} L_{22ij}^{V1,LR} - \frac{2}{3} L_{11ij}^{V1,RR} - \frac{2}{3} L_{22ij}^{V1,RR} + \frac{781}{81} L_{11ij}^{V8,LR} + \frac{781}{81} L_{22ij}^{V8,LR} \\
& + \frac{601}{81} L_{11ij}^{V8,RR} + \frac{601}{81} L_{22ij}^{V8,RR} \Big] + \alpha_s \alpha \Big[ \frac{260}{81} L_{kkij}^{V1,LR} + \frac{14}{9} L_{kkij}^{V8,LR} + \frac{520}{81} L_{ijkk}^{V,RR} \\
& - \frac{1040}{243} L_{ikkj}^{V,RR} + \frac{152}{81} L_{iiij}^{V1,LR} + \frac{260}{81} L_{jjij}^{V1,LR} - \frac{4}{3} L_{iiij}^{V8,LR} + \frac{14}{9} L_{jjij}^{V8,LR} + \frac{292}{81} L_{ijii}^{V,RR} \\
& + \frac{292}{81} L_{ijjj}^{V,RR} + \frac{260}{81} L_{11ij}^{V,LR} + \frac{260}{81} L_{22ij}^{V,LR} + \frac{260}{81} L_{33ij}^{V,LR} + \frac{260}{81} L_{11ij}^{V,RR} + \frac{260}{81} L_{22ij}^{V,RR} \\
& + \frac{260}{81} L_{33ij}^{V,RR} - \frac{520}{81} L_{11ij}^{V1,LR} - \frac{520}{81} L_{22ij}^{V1,LR} - \frac{520}{81} L_{11ij}^{V1,RR} - \frac{520}{81} L_{22ij}^{V1,RR} + \frac{2}{3} L_{11ij}^{V8,LR} \\
& + \frac{2}{3} L_{22ij}^{V8,LR} + \frac{122}{27} L_{11ij}^{V8,RR} + \frac{122}{27} L_{22ij}^{V8,RR} \Big] + \frac{1790}{81} \alpha^2 L_{iiij}^{V8,LR} ;
\end{aligned}$$

$$\begin{aligned}
\dot{L}_{jkk i}^{V1,LR} &= -\frac{8}{3}g_s^2 L_{jkk i}^{V8,LR} - \frac{4}{3}e^2 L_{jkk i}^{V1,LR} + \alpha_s^2 \left[ -\frac{28}{3} L_{jkk i}^{V1,LR} - \frac{2044}{27} L_{jkk i}^{V8,LR} \right] \\
&\quad + \alpha_s \alpha \left[ \frac{32}{3} L_{jkk i}^{V1,LR} - \frac{8}{27} L_{jkk i}^{V8,LR} \right] + \frac{1790}{81} \alpha^2 L_{jkk i}^{V1,LR} ; \\
\dot{L}_{jkk i}^{V8,LR} &= g_s^2 \left[ -12 L_{jkk i}^{V1,LR} - 14 L_{jkk i}^{V8,LR} \right] - \frac{4}{3}e^2 L_{jkk i}^{V8,LR} + \alpha_s^2 \left[ -\frac{374}{3} L_{jkk i}^{V1,LR} \right. \\
&\quad \left. - \frac{2975}{18} L_{jkk i}^{V8,LR} \right] + \alpha_s \alpha \left[ -\frac{4}{3} L_{jkk i}^{V1,LR} - \frac{26}{9} L_{jkk i}^{V8,LR} \right] + \frac{1790}{81} \alpha^2 L_{jkk i}^{V8,LR} ; \\
\dot{L}_{11ij}^{V,LL} &= 0 ; \\
\dot{L}_{22ij}^{V,LL} &= 0 ; \\
\dot{L}_{33ij}^{V,LL} &= 0 ; \\
\dot{L}_{11ij}^{V,LR} &= 0 ; \\
\dot{L}_{22ij}^{V,LR} &= 0 ; \\
\dot{L}_{33ij}^{V,LR} &= 0 ; \\
\dot{L}_{11ij}^{S,LR} &= -8g_s^2 L_{11ij}^{S,LR} - \frac{2}{3}e^2 L_{11ij}^{S,LR} - \frac{1012}{9} \alpha_s^2 L_{11ij}^{S,LR} - \frac{8}{9} \alpha_s \alpha L_{11ij}^{S,LR} \\
&\quad + \frac{397}{81} \alpha^2 L_{11ij}^{S,LR} ; \\
\dot{L}_{22ij}^{S,LR} &= -8g_s^2 L_{22ij}^{S,LR} - \frac{2}{3}e^2 L_{22ij}^{S,LR} - \frac{1012}{9} \alpha_s^2 L_{22ij}^{S,LR} - \frac{8}{9} \alpha_s \alpha L_{22ij}^{S,LR} \\
&\quad + \frac{397}{81} \alpha^2 L_{22ij}^{S,LR} ; \\
\dot{L}_{33ij}^{S,LR} &= -8g_s^2 L_{33ij}^{S,LR} - \frac{2}{3}e^2 L_{33ij}^{S,LR} - \frac{1012}{9} \alpha_s^2 L_{33ij}^{S,LR} - \frac{8}{9} \alpha_s \alpha L_{33ij}^{S,LR} \\
&\quad + \frac{397}{81} \alpha^2 L_{33ij}^{S,LR} ; \\
\dot{L}_{11ij}^{S,LL} &= -8g_s^2 L_{11ij}^{S,LL} - \frac{2}{3}e^2 L_{11ij}^{S,LL} - \frac{1012}{9} \alpha_s^2 L_{11ij}^{S,LL} - \frac{8}{9} \alpha_s \alpha L_{11ij}^{S,LL}
\end{aligned}$$



$$\begin{aligned}
& + \frac{397}{81} \alpha^2 L_{11ij}^{S,LL} ; \\
\dot{L}_{11ij}^{T,LL} & = \frac{8}{3} g_s^2 L_{11ij}^{T,LL} + \frac{2}{9} e^2 L_{11ij}^{T,LL} + \frac{1652}{27} \alpha_s^2 L_{11ij}^{T,LL} - \frac{152}{27} \alpha_s \alpha L_{11ij}^{T,LL} \\
& - \frac{1097}{243} \alpha^2 L_{11ij}^{T,LL} ; \\
\dot{L}_{22ij}^{S,LL} & = -8g_s^2 L_{22ij}^{S,LL} - \frac{2}{3} e^2 L_{22ij}^{S,LL} - \frac{1012}{9} \alpha_s^2 L_{22ij}^{S,LL} - \frac{8}{9} \alpha_s \alpha L_{22ij}^{S,LL} \\
& + \frac{397}{81} \alpha^2 L_{22ij}^{S,LL} ; \\
\dot{L}_{22ij}^{T,LL} & = \frac{8}{3} g_s^2 L_{22ij}^{T,LL} + \frac{2}{9} e^2 L_{22ij}^{T,LL} + \frac{1652}{27} \alpha_s^2 L_{22ij}^{T,LL} - \frac{152}{27} \alpha_s \alpha L_{22ij}^{T,LL} \\
& - \frac{1097}{243} \alpha^2 L_{22ij}^{T,LL} ; \\
\dot{L}_{33ij}^{S,LL} & = -8g_s^2 L_{33ij}^{S,LL} - \frac{2}{3} e^2 L_{33ij}^{S,LL} - \frac{1012}{9} \alpha_s^2 L_{33ij}^{S,LL} - \frac{8}{9} \alpha_s \alpha L_{33ij}^{S,LL} \\
& + \frac{397}{81} \alpha^2 L_{33ij}^{S,LL} ; \\
\dot{L}_{33ij}^{T,LL} & = \frac{8}{3} g_s^2 L_{33ij}^{T,LL} + \frac{2}{9} e^2 L_{33ij}^{T,LL} + \frac{1652}{27} \alpha_s^2 L_{33ij}^{T,LL} - \frac{152}{27} \alpha_s \alpha L_{33ij}^{T,LL} \\
& - \frac{1097}{243} \alpha^2 L_{33ij}^{T,LL} ;
\end{aligned}$$

## 1.6 $\Delta F = 1^{\bar{f}f}$ : $u$ -type ( $\bar{u}_i u_j \bar{f}_k f_k$ )

$$\begin{aligned}
\dot{L}_{11ij}^{V,LL} & = e^2 \left[ -\frac{20}{3} L_{11ij}^{V,LL} + \frac{4}{3} L_{22ij}^{V,LL} + \frac{4}{3} L_{33ij}^{V,LL} + \frac{4}{3} L_{ij11}^{V1,LL} + \frac{4}{3} L_{ij22}^{V1,LL} \right. \\
& + \frac{4}{3} L_{ij33}^{V1,LL} + \frac{4}{3} L_{ij11}^{V1,LR} + \frac{4}{3} L_{ij22}^{V1,LR} + \frac{4}{3} L_{ij33}^{V1,LR} + \frac{4}{3} L_{ij11}^{V,LR} + \frac{4}{3} L_{ij22}^{V,LR} \\
& + \frac{4}{3} L_{ij33}^{V,LR} - \frac{8}{3} L_{ijii}^{V1,LR} - \frac{8}{3} L_{ijjj}^{V1,LR} - \frac{64}{9} L_{ijii}^{V,LL} - \frac{64}{9} L_{ijjj}^{V,LL} \left. \right] + \alpha_s \alpha \left[ 32 L_{11ij}^{V,LL} \right. \\
& + \frac{16}{3} L_{ij11}^{V1,LL} + \frac{16}{3} L_{ij22}^{V1,LL} + \frac{16}{3} L_{ij33}^{V1,LL} + \frac{16}{3} L_{ij11}^{V1,LR} + \frac{16}{3} L_{ij22}^{V1,LR} + \frac{16}{3} L_{ij33}^{V1,LR} \\
& + \frac{328}{243} L_{ij11}^{V8,LL} + \frac{328}{243} L_{ij22}^{V8,LL} + \frac{328}{243} L_{ij33}^{V8,LL} - \frac{392}{243} L_{ij11}^{V8,LR} - \frac{392}{243} L_{ij22}^{V8,LR} \\
& \left. - \frac{392}{243} L_{ij33}^{V8,LR} \right]
\end{aligned}$$

$$\begin{aligned}
& -\frac{392}{243}L_{ij33}^{V8,LR} - \frac{32}{3}L_{ijii}^{V1,LR} - \frac{32}{3}L_{ijjj}^{V1,LR} + \frac{1984}{243}L_{ijii}^{V8,LR} + \frac{1984}{243}L_{ijjj}^{V8,LR} \\
& - \frac{2240}{81}L_{ijii}^{V,LL} - \frac{2240}{81}L_{ijjj}^{V,LL} \Big] + \alpha^2 \Big[ \frac{4352}{243}L_{11ij}^{V,LL} + \frac{3344}{243}L_{22ij}^{V,LL} + \frac{3344}{243}L_{33ij}^{V,LL} \\
& + \frac{392}{243}L_{ij11}^{V1,LL} + \frac{392}{243}L_{ij22}^{V1,LL} + \frac{392}{243}L_{ij33}^{V1,LL} - \frac{832}{243}L_{ij11}^{V1,LR} - \frac{832}{243}L_{ij22}^{V1,LR} \\
& - \frac{832}{243}L_{ij33}^{V1,LR} - \frac{328}{243}L_{ij11}^{V,LR} - \frac{328}{243}L_{ij22}^{V,LR} - \frac{328}{243}L_{ij33}^{V,LR} - \frac{64}{243}L_{ijii}^{V1,LR} \\
& - \frac{64}{243}L_{ijjj}^{V1,LR} + \frac{25888}{243}L_{ijii}^{V,LL} + \frac{25888}{243}L_{ijjj}^{V,LL} \Big] ;
\end{aligned}$$

$$\begin{aligned}
\dot{L}_{22ij}^{V,LL} &= e^2 \Big[ \frac{4}{3}L_{11ij}^{V,LL} - \frac{20}{3}L_{22ij}^{V,LL} + \frac{4}{3}L_{33ij}^{V,LL} + \frac{4}{3}L_{ij11}^{V1,LL} + \frac{4}{3}L_{ij22}^{V1,LL} \\
& + \frac{4}{3}L_{ij33}^{V1,LL} + \frac{4}{3}L_{ij11}^{V1,LR} + \frac{4}{3}L_{ij22}^{V1,LR} + \frac{4}{3}L_{ij33}^{V1,LR} + \frac{4}{3}L_{ij11}^{V,LR} + \frac{4}{3}L_{ij22}^{V,LR} \\
& + \frac{4}{3}L_{ij33}^{V,LR} - \frac{8}{3}L_{ijii}^{V1,LR} - \frac{8}{3}L_{ijjj}^{V1,LR} - \frac{64}{9}L_{ijii}^{V,LL} - \frac{64}{9}L_{ijjj}^{V,LL} \Big] + \alpha_s \alpha \Big[ 32L_{22ij}^{V,LL} \\
& + \frac{16}{3}L_{ij11}^{V1,LL} + \frac{16}{3}L_{ij22}^{V1,LL} + \frac{16}{3}L_{ij33}^{V1,LL} + \frac{16}{3}L_{ij11}^{V1,LR} + \frac{16}{3}L_{ij22}^{V1,LR} + \frac{16}{3}L_{ij33}^{V1,LR} \\
& + \frac{328}{243}L_{ij11}^{V8,LL} + \frac{328}{243}L_{ij22}^{V8,LL} + \frac{328}{243}L_{ij33}^{V8,LL} - \frac{392}{243}L_{ij11}^{V8,LR} - \frac{392}{243}L_{ij22}^{V8,LR} \\
& - \frac{392}{243}L_{ij33}^{V8,LR} - \frac{32}{3}L_{ijii}^{V1,LR} - \frac{32}{3}L_{ijjj}^{V1,LR} + \frac{1984}{243}L_{ijii}^{V8,LR} + \frac{1984}{243}L_{ijjj}^{V8,LR} \\
& - \frac{2240}{81}L_{ijii}^{V,LL} - \frac{2240}{81}L_{ijjj}^{V,LL} \Big] + \alpha^2 \Big[ \frac{3344}{243}L_{11ij}^{V,LL} + \frac{4352}{243}L_{22ij}^{V,LL} + \frac{3344}{243}L_{33ij}^{V,LL} \\
& + \frac{392}{243}L_{ij11}^{V1,LL} + \frac{392}{243}L_{ij22}^{V1,LL} + \frac{392}{243}L_{ij33}^{V1,LL} - \frac{832}{243}L_{ij11}^{V1,LR} - \frac{832}{243}L_{ij22}^{V1,LR} \\
& - \frac{832}{243}L_{ij33}^{V1,LR} - \frac{328}{243}L_{ij11}^{V,LR} - \frac{328}{243}L_{ij22}^{V,LR} - \frac{328}{243}L_{ij33}^{V,LR} - \frac{64}{243}L_{ijii}^{V1,LR} \\
& - \frac{64}{243}L_{ijjj}^{V1,LR} + \frac{25888}{243}L_{ijii}^{V,LL} + \frac{25888}{243}L_{ijjj}^{V,LL} \Big] ;
\end{aligned}$$

$$\dot{L}_{33ij}^{V,LL} = e^2 \Big[ \frac{4}{3}L_{11ij}^{V,LL} + \frac{4}{3}L_{22ij}^{V,LL} - \frac{20}{3}L_{33ij}^{V,LL} + \frac{4}{3}L_{ij11}^{V1,LL} + \frac{4}{3}L_{ij22}^{V1,LL}$$

$$\begin{aligned}
& + \frac{4}{3}L_{ij33}^{V1,LL} + \frac{4}{3}L_{ij11}^{V1,LR} + \frac{4}{3}L_{ij22}^{V1,LR} + \frac{4}{3}L_{ij33}^{V1,LR} + \frac{4}{3}L_{ij11}^{V,LR} + \frac{4}{3}L_{ij22}^{V,LR} \\
& + \frac{4}{3}L_{ij33}^{V,LR} - \frac{8}{3}L_{ijii}^{V1,LR} - \frac{8}{3}L_{ijjj}^{V1,LR} - \frac{64}{9}L_{ijii}^{V,LL} - \frac{64}{9}L_{ijjj}^{V,LL} \Big] + \alpha_s \alpha \Big[ 32L_{33ij}^{V,LL} \\
& + \frac{16}{3}L_{ij11}^{V1,LL} + \frac{16}{3}L_{ij22}^{V1,LL} + \frac{16}{3}L_{ij33}^{V1,LL} + \frac{16}{3}L_{ij11}^{V1,LR} + \frac{16}{3}L_{ij22}^{V1,LR} + \frac{16}{3}L_{ij33}^{V1,LR} \\
& + \frac{328}{243}L_{ij11}^{V8,LL} + \frac{328}{243}L_{ij22}^{V8,LL} + \frac{328}{243}L_{ij33}^{V8,LL} - \frac{392}{243}L_{ij11}^{V8,LR} - \frac{392}{243}L_{ij22}^{V8,LR} \\
& - \frac{392}{243}L_{ij33}^{V8,LR} - \frac{32}{3}L_{ijii}^{V1,LR} - \frac{32}{3}L_{ijjj}^{V1,LR} + \frac{1984}{243}L_{ijii}^{V8,LR} + \frac{1984}{243}L_{ijjj}^{V8,LR} \\
& - \frac{2240}{81}L_{ijii}^{V,LL} - \frac{2240}{81}L_{ijjj}^{V,LL} \Big] + \alpha^2 \Big[ \frac{3344}{243}L_{11ij}^{V,LL} + \frac{3344}{243}L_{22ij}^{V,LL} + \frac{4352}{243}L_{33ij}^{V,LL} \\
& + \frac{392}{243}L_{ij11}^{V1,LL} + \frac{392}{243}L_{ij22}^{V1,LL} + \frac{392}{243}L_{ij33}^{V1,LL} - \frac{832}{243}L_{ij11}^{V1,LR} - \frac{832}{243}L_{ij22}^{V1,LR} \\
& - \frac{832}{243}L_{ij33}^{V1,LR} - \frac{328}{243}L_{ij11}^{V,LR} - \frac{328}{243}L_{ij22}^{V,LR} - \frac{328}{243}L_{ij33}^{V,LR} - \frac{64}{243}L_{ijii}^{V1,LR} \\
& - \frac{64}{243}L_{ijjj}^{V1,LR} + \frac{25888}{243}L_{ijii}^{V,LL} + \frac{25888}{243}L_{ijjj}^{V,LL} \Big] ;
\end{aligned}$$

$$\begin{aligned}
\dot{L}_{ij11}^{V1,LL} &= \frac{8}{3}g_s^2 L_{ij11}^{V8,LL} + e^2 \Big[ \frac{4}{9}L_{11ij}^{V,LL} + \frac{4}{9}L_{22ij}^{V,LL} + \frac{4}{9}L_{33ij}^{V,LL} - \frac{20}{9}L_{ij11}^{V1,LL} \\
& + \frac{4}{9}L_{ij22}^{V1,LL} + \frac{4}{9}L_{ij33}^{V1,LL} + \frac{4}{9}L_{ij11}^{V1,LR} + \frac{4}{9}L_{ij22}^{V1,LR} + \frac{4}{9}L_{ij33}^{V1,LR} + \frac{4}{9}L_{ij11}^{V,LR} \\
& + \frac{4}{9}L_{ij22}^{V,LR} + \frac{4}{9}L_{ij33}^{V,LR} - \frac{8}{9}L_{ijii}^{V1,LR} - \frac{8}{9}L_{ijjj}^{V1,LR} - \frac{64}{27}L_{ijii}^{V,LL} - \frac{64}{27}L_{ijjj}^{V,LL} \Big] \\
& + \alpha_s^2 \Big[ -\frac{4}{3}L_{ij11}^{V1,LL} + 8L_{ij22}^{V1,LL} + 8L_{ij33}^{V1,LL} - 8L_{ij11}^{V1,LR} - 8L_{ij22}^{V1,LR} \\
& - 8L_{ij33}^{V1,LR} + \frac{86}{27}L_{ij11}^{V8,LL} + \frac{4}{27}L_{ij22}^{V8,LL} + \frac{4}{27}L_{ij33}^{V8,LL} + \frac{4}{27}L_{ij11}^{V8,LR} + \frac{4}{27}L_{ij22}^{V8,LR} \\
& + \frac{4}{27}L_{ij33}^{V8,LR} - 8L_{ijii}^{V1,LR} - 8L_{ijjj}^{V1,LR} + \frac{4}{27}L_{ijii}^{V8,LR} + \frac{4}{27}L_{ijjj}^{V8,LR} + \frac{328}{9}L_{ijii}^{V,LL} \\
& + \frac{328}{9}L_{ijjj}^{V,LL} \Big] + \alpha_s \alpha \Big[ \frac{208}{9}L_{ij11}^{V1,LL} + \frac{16}{9}L_{ij22}^{V1,LL} + \frac{16}{9}L_{ij33}^{V1,LL} + \frac{16}{9}L_{ij11}^{V1,LR}
\end{aligned}$$

$$\begin{aligned}
& + \frac{16}{9} L_{ud}^{V1,LR} + \frac{16}{9} L_{ij33}^{V1,LR} + \frac{112}{729} L_{ij11}^{V8,LL} + \frac{328}{729} L_{ij22}^{V8,LL} + \frac{328}{729} L_{ij33}^{V8,LL} - \frac{392}{729} L_{ij11}^{V8,LR} \\
& - \frac{392}{729} L_{ij22}^{V8,LR} - \frac{392}{729} L_{ij33}^{V8,LR} - \frac{32}{9} L_{ijii}^{V1,LR} - \frac{32}{9} L_{ijjj}^{V1,LR} + \frac{1984}{729} L_{ijii}^{V8,LR} + \frac{1984}{729} L_{ijjj}^{V8,LR} \\
& - \frac{2240}{243} L_{ijii}^{V,LL} - \frac{2240}{243} L_{ijjj}^{V,LL} \Big] + \alpha^2 \Big[ \frac{1544}{729} L_{11ij}^{V,LL} + \frac{1544}{729} L_{22ij}^{V,LL} + \frac{1544}{729} L_{33ij}^{V,LL} \\
& - \frac{1264}{729} L_{ij11}^{V1,LL} - \frac{112}{729} L_{ij22}^{V1,LL} - \frac{112}{729} L_{ij33}^{V1,LL} - \frac{40}{729} L_{ij11}^{V1,LR} - \frac{40}{729} L_{ij22}^{V1,LR} \\
& - \frac{40}{729} L_{ij33}^{V1,LR} + \frac{1760}{729} L_{ij11}^{V,LR} + \frac{1760}{729} L_{ij22}^{V,LR} + \frac{1760}{729} L_{ij33}^{V,LR} + \frac{2240}{729} L_{ijii}^{V1,LR} \\
& + \frac{2240}{729} L_{ijjj}^{V1,LR} + \frac{11488}{729} L_{ijii}^{V,LL} + \frac{11488}{729} L_{ijjj}^{V,LL} \Big] ;
\end{aligned}$$

$$\begin{aligned}
\dot{L}_{ud}^{V8,LL} &= g_s^2 \Big[ 12 L_{ij11}^{V1,LL} - \frac{10}{3} L_{ij11}^{V8,LL} + \frac{2}{3} L_{ij22}^{V8,LL} + \frac{2}{3} L_{ij33}^{V8,LL} + \frac{2}{3} L_{ij11}^{V8,LR} \\
& + \frac{2}{3} L_{ij22}^{V8,LR} + \frac{2}{3} L_{ij33}^{V8,LR} + \frac{2}{3} L_{ijii}^{V8,LR} + \frac{2}{3} L_{ijjj}^{V8,LR} + \frac{8}{3} L_{ijii}^{V,LL} + \frac{8}{3} L_{ijjj}^{V,LL} \Big] \\
& - \frac{8}{3} e^2 L_{ij11}^{V8,LL} + \alpha_s^2 \Big[ 13 L_{ij11}^{V1,LL} - \frac{2}{3} L_{ij22}^{V1,LL} - \frac{2}{3} L_{ij33}^{V1,LL} - \frac{22}{3} L_{ij11}^{V1,LR} \\
& - \frac{22}{3} L_{ij22}^{V1,LR} - \frac{22}{3} L_{ij33}^{V1,LR} - \frac{326}{81} L_{ij11}^{V8,LL} + \frac{799}{81} L_{ij22}^{V8,LL} + \frac{799}{81} L_{ij33}^{V8,LL} + \frac{169}{81} L_{ij11}^{V8,LR} \\
& + \frac{169}{81} L_{ij22}^{V8,LR} + \frac{169}{81} L_{ij33}^{V8,LR} - \frac{22}{3} L_{ijii}^{V1,LR} - \frac{22}{3} L_{ijjj}^{V1,LR} + \frac{169}{81} L_{ijii}^{V8,LR} + \frac{169}{81} L_{ijjj}^{V8,LR} \\
& + \frac{1930}{27} L_{ijii}^{V,LL} + \frac{1930}{27} L_{ijjj}^{V,LL} \Big] + \alpha_s \alpha \Big[ \frac{308}{81} L_{11ij}^{V,LL} + \frac{308}{81} L_{22ij}^{V,LL} + \frac{308}{81} L_{33ij}^{V,LL} \\
& + \frac{200}{81} L_{ij11}^{V1,LL} + \frac{308}{81} L_{ij22}^{V1,LL} + \frac{308}{81} L_{ij33}^{V1,LL} + \frac{308}{81} L_{ij11}^{V1,LR} + \frac{308}{81} L_{ij22}^{V1,LR} + \frac{308}{81} L_{ij33}^{V1,LR} \\
& - \frac{11}{3} L_{ij11}^{V8,LL} + \frac{14}{9} L_{ij22}^{V8,LL} + \frac{14}{9} L_{ij33}^{V8,LL} + \frac{10}{27} L_{ij11}^{V8,LR} + \frac{10}{27} L_{ij22}^{V8,LR} + \frac{10}{27} L_{ij33}^{V8,LR} \\
& + \frac{308}{81} L_{ij11}^{V,LR} + \frac{308}{81} L_{ij22}^{V,LR} + \frac{308}{81} L_{ij33}^{V,LR} - \frac{616}{81} L_{ijii}^{V1,LR} - \frac{616}{81} L_{ijjj}^{V1,LR} + \frac{4}{27} L_{ijii}^{V8,LR} \\
& + \frac{4}{27} L_{ijjj}^{V8,LR} - \frac{4808}{81} L_{ijii}^{V,LL} - \frac{4808}{81} L_{ijjj}^{V,LL} \Big] - \frac{128}{81} \alpha^2 L_{ij11}^{V8,LL} ;
\end{aligned}$$

$$\begin{aligned}
\dot{L}_{ij22}^{V1,LL} &= \frac{8}{3}g_s^2 L_{ij22}^{V8,LL} + e^2 \left[ \frac{4}{9}L_{11ij}^{V,LL} + \frac{4}{9}L_{22ij}^{V,LL} + \frac{4}{9}L_{33ij}^{V,LL} + \frac{4}{9}L_{ij11}^{V1,LL} \right. \\
&\quad - \frac{20}{9}L_{ij22}^{V1,LL} + \frac{4}{9}L_{ij33}^{V1,LL} + \frac{4}{9}L_{ij11}^{V1,LR} + \frac{4}{9}L_{ij22}^{V1,LR} + \frac{4}{9}L_{ij33}^{V1,LR} + \frac{4}{9}L_{ij11}^{V,LR} \\
&\quad + \frac{4}{9}L_{ij22}^{V,LR} + \frac{4}{9}L_{ij33}^{V,LR} - \frac{8}{9}L_{ijii}^{V1,LR} - \frac{8}{9}L_{ijjj}^{V1,LR} - \frac{64}{27}L_{ijii}^{V,LL} - \frac{64}{27}L_{ijjj}^{V,LL} \left. \right] \\
&\quad + \alpha_s^2 \left[ 8L_{ij11}^{V1,LL} - \frac{4}{3}L_{ij22}^{V1,LL} + 8L_{ij33}^{V1,LL} - 8L_{ij11}^{V1,LR} - 8L_{ij22}^{V1,LR} \right. \\
&\quad - 8L_{ij33}^{V1,LR} + \frac{4}{27}L_{ij11}^{V8,LL} + \frac{86}{27}L_{ij22}^{V8,LL} + \frac{4}{27}L_{ij33}^{V8,LL} + \frac{4}{27}L_{ij11}^{V8,LR} + \frac{4}{27}L_{ij22}^{V8,LR} \\
&\quad + \frac{4}{27}L_{ij33}^{V8,LR} - 8L_{ijii}^{V1,LR} - 8L_{ijjj}^{V1,LR} + \frac{4}{27}L_{ijii}^{V8,LR} + \frac{4}{27}L_{ijjj}^{V8,LR} + \frac{328}{9}L_{ijii}^{V,LL} \\
&\quad + \frac{328}{9}L_{ijjj}^{V,LL} \left. \right] + \alpha_s \alpha \left[ \frac{16}{9}L_{ij11}^{V1,LL} + \frac{208}{9}L_{ij22}^{V1,LL} + \frac{16}{9}L_{ij33}^{V1,LL} + \frac{16}{9}L_{ij11}^{V1,LR} \right. \\
&\quad + \frac{16}{9}L_{ij22}^{V1,LR} + \frac{16}{9}L_{ij33}^{V1,LR} + \frac{328}{729}L_{ij11}^{V8,LL} + \frac{112}{729}L_{ij22}^{V8,LL} + \frac{328}{729}L_{ij33}^{V8,LL} - \frac{392}{729}L_{ij11}^{V8,LR} \\
&\quad - \frac{392}{729}L_{ij22}^{V8,LR} - \frac{392}{729}L_{ij33}^{V8,LR} - \frac{32}{9}L_{ijii}^{V1,LR} - \frac{32}{9}L_{ijjj}^{V1,LR} + \frac{1984}{729}L_{ijii}^{V8,LR} + \frac{1984}{729}L_{ijjj}^{V8,LR} \\
&\quad - \frac{2240}{243}L_{ijii}^{V,LL} - \frac{2240}{243}L_{ijjj}^{V,LL} \left. \right] + \alpha^2 \left[ \frac{1544}{729}L_{11ij}^{V,LL} + \frac{1544}{729}L_{22ij}^{V,LL} + \frac{1544}{729}L_{33ij}^{V,LL} \right. \\
&\quad - \frac{112}{729}L_{ij11}^{V1,LL} - \frac{1264}{729}L_{ij22}^{V1,LL} - \frac{112}{729}L_{ij33}^{V1,LL} - \frac{40}{729}L_{ij11}^{V1,LR} - \frac{40}{729}L_{ij22}^{V1,LR} \\
&\quad - \frac{40}{729}L_{ij33}^{V1,LR} + \frac{1760}{729}L_{ij11}^{V,LR} + \frac{1760}{729}L_{ij22}^{V,LR} + \frac{1760}{729}L_{ij33}^{V,LR} + \frac{2240}{729}L_{ijii}^{V1,LR} \\
&\quad + \frac{2240}{729}L_{ijjj}^{V1,LR} + \frac{11488}{729}L_{ijii}^{V,LL} + \frac{11488}{729}L_{ijjj}^{V,LL} \left. \right] ; \\
\dot{L}_{ij22}^{V8,LL} &= g_s^2 \left[ 12L_{ij22}^{V1,LL} + \frac{2}{3}L_{ij11}^{V8,LL} - \frac{10}{3}L_{ij22}^{V8,LL} + \frac{2}{3}L_{ij33}^{V8,LL} + \frac{2}{3}L_{ij11}^{V8,LR} \right. \\
&\quad + \frac{2}{3}L_{ij22}^{V8,LR} + \frac{2}{3}L_{ij33}^{V8,LR} + \frac{2}{3}L_{ijii}^{V8,LR} + \frac{2}{3}L_{ijjj}^{V8,LR} + \frac{8}{3}L_{ijii}^{V,LL} + \frac{8}{3}L_{ijjj}^{V,LL} \left. \right] \\
&\quad - \frac{8}{3}e^2 L_{ij22}^{V8,LL} + \alpha_s^2 \left[ -\frac{2}{3}L_{ij11}^{V1,LL} + 13L_{ij22}^{V1,LL} - \frac{2}{3}L_{ij33}^{V1,LL} - \frac{22}{3}L_{ij11}^{V1,LR} \right.
\end{aligned}$$

$$\begin{aligned}
& -\frac{22}{3}L_{ud\ ij22}^{V1,LR} - \frac{22}{3}L_{ud\ ij33}^{V1,LR} + \frac{799}{81}L_{ud\ ij11}^{V8,LL} - \frac{326}{81}L_{ud\ ij22}^{V8,LL} + \frac{799}{81}L_{ud\ ij33}^{V8,LL} + \frac{169}{81}L_{ud\ ij11}^{V8,LR} \\
& + \frac{169}{81}L_{ud\ ij22}^{V8,LR} + \frac{169}{81}L_{ud\ ij33}^{V8,LR} - \frac{22}{3}L_{uu\ ijii}^{V1,LR} - \frac{22}{3}L_{uu\ ijjj}^{V1,LR} + \frac{169}{81}L_{uu\ ijii}^{V8,LR} + \frac{169}{81}L_{uu\ ijjj}^{V8,LR} \\
& + \frac{1930}{27}L_{uu\ ijii}^{V,LL} + \frac{1930}{27}L_{uu\ ijjj}^{V,LL} \Big] + \alpha_s \alpha \Big[ \frac{308}{81}L_{eu\ 11ij}^{V,LL} + \frac{308}{81}L_{eu\ 22ij}^{V,LL} + \frac{308}{81}L_{eu\ 33ij}^{V,LL} \\
& + \frac{308}{81}L_{ud\ ij11}^{V1,LL} + \frac{200}{81}L_{ud\ ij22}^{V1,LL} + \frac{308}{81}L_{ud\ ij33}^{V1,LL} + \frac{308}{81}L_{ud\ ij11}^{V1,LR} + \frac{308}{81}L_{ud\ ij22}^{V1,LR} + \frac{308}{81}L_{ud\ ij33}^{V1,LR} \\
& + \frac{14}{9}L_{ud\ ij11}^{V8,LL} - \frac{11}{3}L_{ud\ ij22}^{V8,LL} + \frac{14}{9}L_{ud\ ij33}^{V8,LL} + \frac{10}{27}L_{ud\ ij11}^{V8,LR} + \frac{10}{27}L_{ud\ ij22}^{V8,LR} + \frac{10}{27}L_{ud\ ij33}^{V8,LR} \\
& + \frac{308}{81}L_{ue\ ij11}^{V,LR} + \frac{308}{81}L_{ue\ ij22}^{V,LR} + \frac{308}{81}L_{ue\ ij33}^{V,LR} - \frac{616}{81}L_{uu\ ijii}^{V1,LR} - \frac{616}{81}L_{uu\ ijjj}^{V1,LR} + \frac{4}{27}L_{uu\ ijii}^{V8,LR} \\
& + \frac{4}{27}L_{uu\ ijjj}^{V8,LR} - \frac{4808}{81}L_{uu\ ijii}^{V,LL} - \frac{4808}{81}L_{uu\ ijjj}^{V,LL} \Big] - \frac{128}{81}\alpha^2 L_{ud\ ij22}^{V8,LL} ;
\end{aligned}$$

$$\begin{aligned}
\dot{L}_{ud\ ij33}^{V1,LL} &= \frac{8}{3}g_s^2 L_{ud\ ij33}^{V8,LL} + e^2 \Big[ \frac{4}{9}L_{eu\ 11ij}^{V,LL} + \frac{4}{9}L_{eu\ 22ij}^{V,LL} + \frac{4}{9}L_{eu\ 33ij}^{V,LL} + \frac{4}{9}L_{ud\ ij11}^{V1,LL} \\
& + \frac{4}{9}L_{ud\ ij22}^{V1,LL} - \frac{20}{9}L_{ud\ ij33}^{V1,LL} + \frac{4}{9}L_{ud\ ij11}^{V1,LR} + \frac{4}{9}L_{ud\ ij22}^{V1,LR} + \frac{4}{9}L_{ud\ ij33}^{V1,LR} + \frac{4}{9}L_{ue\ ij11}^{V,LR} \\
& + \frac{4}{9}L_{ue\ ij22}^{V,LR} + \frac{4}{9}L_{ue\ ij33}^{V,LR} - \frac{8}{9}L_{uu\ ijii}^{V1,LR} - \frac{8}{9}L_{uu\ ijjj}^{V1,LR} - \frac{64}{27}L_{uu\ ijii}^{V,LL} - \frac{64}{27}L_{uu\ ijjj}^{V,LL} \Big] \\
& + \alpha_s^2 \Big[ 8L_{ud\ ij11}^{V1,LL} + 8L_{ud\ ij22}^{V1,LL} - \frac{4}{3}L_{ud\ ij33}^{V1,LL} - 8L_{ud\ ij11}^{V1,LR} - 8L_{ud\ ij22}^{V1,LR} \\
& - 8L_{ud\ ij33}^{V1,LR} + \frac{4}{27}L_{ud\ ij11}^{V8,LL} + \frac{4}{27}L_{ud\ ij22}^{V8,LL} + \frac{86}{27}L_{ud\ ij33}^{V8,LL} + \frac{4}{27}L_{ud\ ij11}^{V8,LR} + \frac{4}{27}L_{ud\ ij22}^{V8,LR} \\
& + \frac{4}{27}L_{ud\ ij33}^{V8,LR} - 8L_{uu\ ijii}^{V1,LR} - 8L_{uu\ ijjj}^{V1,LR} + \frac{4}{27}L_{uu\ ijii}^{V8,LR} + \frac{4}{27}L_{uu\ ijjj}^{V8,LR} + \frac{328}{9}L_{uu\ ijii}^{V,LL} \\
& + \frac{328}{9}L_{uu\ ijjj}^{V,LL} \Big] + \alpha_s \alpha \Big[ \frac{16}{9}L_{ud\ ij11}^{V1,LL} + \frac{16}{9}L_{ud\ ij22}^{V1,LL} + \frac{208}{9}L_{ud\ ij33}^{V1,LL} + \frac{16}{9}L_{ud\ ij11}^{V1,LR} \\
& + \frac{16}{9}L_{ud\ ij22}^{V1,LR} + \frac{16}{9}L_{ud\ ij33}^{V1,LR} + \frac{328}{729}L_{ud\ ij11}^{V8,LL} + \frac{328}{729}L_{ud\ ij22}^{V8,LL} + \frac{112}{729}L_{ud\ ij33}^{V8,LL} - \frac{392}{729}L_{ud\ ij11}^{V8,LR} \\
& - \frac{392}{729}L_{ud\ ij22}^{V8,LR} - \frac{392}{729}L_{ud\ ij33}^{V8,LR} - \frac{32}{9}L_{uu\ ijii}^{V1,LR} - \frac{32}{9}L_{uu\ ijjj}^{V1,LR} + \frac{1984}{729}L_{uu\ ijii}^{V8,LR} + \frac{1984}{729}L_{uu\ ijjj}^{V8,LR}
\end{aligned}$$

$$\begin{aligned}
& -\frac{2240}{243}L_{ij\bar{i}\bar{j}}^{V,LL} - \frac{2240}{243}L_{ij\bar{j}\bar{i}}^{V,LL} \Big] + \alpha^2 \Big[ \frac{1544}{729}L_{11ij}^{V,LL} + \frac{1544}{729}L_{22ij}^{V,LL} + \frac{1544}{729}L_{33ij}^{V,LL} \\
& - \frac{112}{729}L_{ud}^{V1,LL} - \frac{112}{729}L_{ud}^{V1,LL} - \frac{1264}{729}L_{ij33}^{V1,LL} - \frac{40}{729}L_{ij11}^{V1,LR} - \frac{40}{729}L_{ij22}^{V1,LR} \\
& - \frac{40}{729}L_{ij33}^{V1,LR} + \frac{1760}{729}L_{ue}^{V,LR} + \frac{1760}{729}L_{ue}^{V,LR} + \frac{1760}{729}L_{ue}^{V,LR} + \frac{1760}{729}L_{ue}^{V,LR} + \frac{2240}{729}L_{uu}^{V1,LR} \\
& + \frac{2240}{729}L_{uu}^{V1,LR} + \frac{11488}{729}L_{ij\bar{i}\bar{j}}^{V,LL} + \frac{11488}{729}L_{ij\bar{j}\bar{i}}^{V,LL} \Big] ;
\end{aligned}$$

$$\begin{aligned}
\dot{L}_{ij33}^{V8,LL} = & g_s^2 \Big[ 12L_{ij33}^{V1,LL} + \frac{2}{3}L_{ij11}^{V8,LL} + \frac{2}{3}L_{ij22}^{V8,LL} - \frac{10}{3}L_{ij33}^{V8,LL} + \frac{2}{3}L_{ij11}^{V8,LR} \\
& + \frac{2}{3}L_{ij22}^{V8,LR} + \frac{2}{3}L_{ij33}^{V8,LR} + \frac{2}{3}L_{ij\bar{i}\bar{j}}^{V8,LR} + \frac{2}{3}L_{ij\bar{j}\bar{i}}^{V8,LR} + \frac{8}{3}L_{ij\bar{i}\bar{j}}^{V,LL} + \frac{8}{3}L_{ij\bar{j}\bar{i}}^{V,LL} \Big] \\
& - \frac{8}{3}e^2L_{ij33}^{V8,LL} + \alpha_s^2 \Big[ -\frac{2}{3}L_{ij11}^{V1,LL} - \frac{2}{3}L_{ij22}^{V1,LL} + 13L_{ij33}^{V1,LL} - \frac{22}{3}L_{ij11}^{V1,LR} \\
& - \frac{22}{3}L_{ij22}^{V1,LR} - \frac{22}{3}L_{ij33}^{V1,LR} + \frac{799}{81}L_{ij11}^{V8,LL} + \frac{799}{81}L_{ij22}^{V8,LL} - \frac{326}{81}L_{ij33}^{V8,LL} + \frac{169}{81}L_{ij11}^{V8,LR} \\
& + \frac{169}{81}L_{ij22}^{V8,LR} + \frac{169}{81}L_{ij33}^{V8,LR} - \frac{22}{3}L_{ij\bar{i}\bar{j}}^{V1,LR} - \frac{22}{3}L_{ij\bar{j}\bar{i}}^{V1,LR} + \frac{169}{81}L_{ij\bar{i}\bar{j}}^{V8,LR} + \frac{169}{81}L_{ij\bar{j}\bar{i}}^{V8,LR} \\
& + \frac{1930}{27}L_{ij\bar{i}\bar{j}}^{V,LL} + \frac{1930}{27}L_{ij\bar{j}\bar{i}}^{V,LL} \Big] + \alpha_s \alpha \Big[ \frac{308}{81}L_{11ij}^{V,LL} + \frac{308}{81}L_{22ij}^{V,LL} + \frac{308}{81}L_{33ij}^{V,LL} \\
& + \frac{308}{81}L_{ij11}^{V1,LL} + \frac{308}{81}L_{ij22}^{V1,LL} + \frac{200}{81}L_{ij33}^{V1,LL} + \frac{308}{81}L_{ij11}^{V1,LR} + \frac{308}{81}L_{ij22}^{V1,LR} + \frac{308}{81}L_{ij33}^{V1,LR} \\
& + \frac{14}{9}L_{ij11}^{V8,LL} + \frac{14}{9}L_{ij22}^{V8,LL} - \frac{11}{3}L_{ij33}^{V8,LL} + \frac{10}{27}L_{ij11}^{V8,LR} + \frac{10}{27}L_{ij22}^{V8,LR} + \frac{10}{27}L_{ij33}^{V8,LR} \\
& + \frac{308}{81}L_{ue}^{V,LR} + \frac{308}{81}L_{ue}^{V,LR} + \frac{308}{81}L_{ue}^{V,LR} - \frac{616}{81}L_{ij\bar{i}\bar{j}}^{V1,LR} - \frac{616}{81}L_{ij\bar{j}\bar{i}}^{V1,LR} + \frac{4}{27}L_{ij\bar{i}\bar{j}}^{V8,LR} \\
& + \frac{4}{27}L_{ij\bar{j}\bar{i}}^{V8,LR} - \frac{4808}{81}L_{ij\bar{i}\bar{j}}^{V,LL} - \frac{4808}{81}L_{ij\bar{j}\bar{i}}^{V,LL} \Big] - \frac{128}{81}\alpha^2L_{ij33}^{V8,LL} ;
\end{aligned}$$

$$\begin{aligned}
\dot{L}_{ij\bar{j}\bar{i}}^{V,LL} = & g_s^2 \Big[ \frac{1}{9}L_{ij11}^{V8,LL} + \frac{1}{9}L_{ij22}^{V8,LL} + \frac{1}{9}L_{ij33}^{V8,LL} + \frac{1}{9}L_{ij11}^{V8,LR} + \frac{1}{9}L_{ij22}^{V8,LR} \\
& + \frac{1}{9}L_{ij33}^{V8,LR} + \frac{1}{9}L_{ij\bar{i}\bar{j}}^{V8,LR} + \frac{1}{9}L_{ij\bar{j}\bar{i}}^{V8,LR} + \frac{4}{9}L_{ij\bar{i}\bar{j}}^{V,LL} + \frac{40}{9}L_{ij\bar{j}\bar{i}}^{V,LL} \Big] + e^2 \Big[ -\frac{4}{9}L_{11ij}^{V,LL}
\end{aligned}$$

$$\begin{aligned}
& -\frac{4}{9}L_{22ij}^{V,LL} - \frac{4}{9}L_{33ij}^{V,LL} - \frac{4}{9}L_{ij11}^{V1,LL} - \frac{4}{9}L_{ij22}^{V1,LL} - \frac{4}{9}L_{ij33}^{V1,LL} - \frac{4}{9}L_{ij11}^{V1,LR} \\
& - \frac{4}{9}L_{ij22}^{V1,LR} - \frac{4}{9}L_{ij33}^{V1,LR} - \frac{4}{9}L_{ij11}^{V,LR} - \frac{4}{9}L_{ij22}^{V,LR} - \frac{4}{9}L_{ij33}^{V,LR} + \frac{8}{9}L_{ijii}^{V1,LR} \\
& + \frac{8}{9}L_{ijjj}^{V1,LR} + \frac{64}{27}L_{ijii}^{V,LL} + \frac{208}{27}L_{ijjj}^{V,LL} \Big] + \alpha_s^2 \Big[ \frac{35}{9}L_{ij11}^{V1,LL} + \frac{35}{9}L_{ij22}^{V1,LL} \\
& + \frac{35}{9}L_{ij33}^{V1,LL} - \frac{47}{9}L_{ij11}^{V1,LR} - \frac{47}{9}L_{ij22}^{V1,LR} - \frac{47}{9}L_{ij33}^{V1,LR} + \frac{835}{486}L_{ij11}^{V8,LL} + \frac{835}{486}L_{ij22}^{V8,LL} \\
& + \frac{835}{486}L_{ij33}^{V8,LL} + \frac{205}{486}L_{ij11}^{V8,LR} + \frac{205}{486}L_{ij22}^{V8,LR} + \frac{205}{486}L_{ij33}^{V8,LR} - \frac{47}{9}L_{ijii}^{V1,LR} \\
& - \frac{47}{9}L_{ijjj}^{V1,LR} + \frac{205}{486}L_{ijii}^{V8,LR} + \frac{205}{486}L_{ijjj}^{V8,LR} + \frac{2441}{81}L_{ijii}^{V,LL} + \frac{2054}{81}L_{ijjj}^{V,LL} \Big] \\
& + \alpha_s \alpha \Big[ \frac{100}{243}L_{11ij}^{V,LL} + \frac{100}{243}L_{22ij}^{V,LL} + \frac{100}{243}L_{33ij}^{V,LL} - \frac{332}{243}L_{ij11}^{V1,LL} - \frac{332}{243}L_{ij22}^{V1,LL} \\
& - \frac{332}{243}L_{ij33}^{V1,LL} - \frac{332}{243}L_{ij11}^{V1,LR} - \frac{332}{243}L_{ij22}^{V1,LR} - \frac{332}{243}L_{ij33}^{V1,LR} - \frac{571}{729}L_{ij11}^{V8,LL} \\
& - \frac{571}{729}L_{ij22}^{V8,LL} - \frac{571}{729}L_{ij33}^{V8,LL} + \frac{977}{729}L_{ij11}^{V8,LR} + \frac{977}{729}L_{ij22}^{V8,LR} + \frac{977}{729}L_{ij33}^{V8,LR} \\
& + \frac{100}{243}L_{ij11}^{V,LR} + \frac{100}{243}L_{ij22}^{V,LR} + \frac{100}{243}L_{ij33}^{V,LR} + \frac{664}{243}L_{ijii}^{V1,LR} + \frac{664}{243}L_{ijjj}^{V1,LR} \\
& - \frac{2884}{729}L_{ijii}^{V8,LR} - \frac{2884}{729}L_{ijjj}^{V8,LR} + \frac{3832}{243}L_{ijii}^{V,LL} - \frac{12152}{243}L_{ijjj}^{V,LL} \Big] + \alpha^2 \Big[ \frac{1156}{729}L_{11ij}^{V,LL} \\
& + \frac{1156}{729}L_{22ij}^{V,LL} + \frac{1156}{729}L_{33ij}^{V,LL} + \frac{868}{729}L_{ij11}^{V1,LL} + \frac{868}{729}L_{ij22}^{V1,LL} + \frac{868}{729}L_{ij33}^{V1,LL} \\
& - \frac{1148}{729}L_{ij11}^{V1,LR} - \frac{1148}{729}L_{ij22}^{V1,LR} - \frac{1148}{729}L_{ij33}^{V1,LR} - \frac{4892}{729}L_{ij11}^{V,LR} - \frac{4892}{729}L_{ij22}^{V,LR} \\
& - \frac{4892}{729}L_{ij33}^{V,LR} - \frac{5696}{729}L_{ijii}^{V1,LR} - \frac{5696}{729}L_{ijjj}^{V1,LR} + \frac{10112}{729}L_{ijii}^{V,LL} - \frac{544}{729}L_{ijjj}^{V,LL} \Big] ; \\
\dot{L}_{ijii}^{V,LL} & = g_s^2 \Big[ \frac{1}{9}L_{ij11}^{V8,LL} + \frac{1}{9}L_{ij22}^{V8,LL} + \frac{1}{9}L_{ij33}^{V8,LL} + \frac{1}{9}L_{ij11}^{V8,LR} + \frac{1}{9}L_{ij22}^{V8,LR} \\
& + \frac{1}{9}L_{ij33}^{V8,LR} + \frac{1}{9}L_{ijii}^{V8,LR} + \frac{40}{9}L_{ijii}^{V,LL} + \frac{4}{9}L_{ijjj}^{V,LL} \Big] + e^2 \Big[ -\frac{4}{9}L_{11ij}^{V,LL}
\end{aligned}$$



$$\begin{aligned}
& -\frac{4}{9}L_{22ij}^{V,LL} - \frac{4}{9}L_{33ij}^{V,LL} - \frac{4}{9}L_{ij11}^{V1,LL} - \frac{4}{9}L_{ij22}^{V1,LL} - \frac{4}{9}L_{ij33}^{V1,LL} - \frac{4}{9}L_{ij11}^{V1,LR} \\
& - \frac{4}{9}L_{ij22}^{V1,LR} - \frac{4}{9}L_{ij33}^{V1,LR} - \frac{4}{9}L_{ij11}^{V,LR} - \frac{4}{9}L_{ij22}^{V,LR} - \frac{4}{9}L_{ij33}^{V,LR} + \frac{8}{9}L_{ijii}^{V1,LR} \\
& + \frac{8}{9}L_{ijjj}^{V1,LR} + \frac{208}{27}L_{ijii}^{V,LL} + \frac{64}{27}L_{ijjj}^{V,LL} \Big] + \alpha_s^2 \Big[ \frac{35}{9}L_{ij11}^{V1,LL} + \frac{35}{9}L_{ij22}^{V1,LL} \\
& + \frac{35}{9}L_{ij33}^{V1,LL} - \frac{47}{9}L_{ij11}^{V1,LR} - \frac{47}{9}L_{ij22}^{V1,LR} - \frac{47}{9}L_{ij33}^{V1,LR} + \frac{835}{486}L_{ij11}^{V8,LL} + \frac{835}{486}L_{ij22}^{V8,LL} \\
& + \frac{835}{486}L_{ij33}^{V8,LL} + \frac{205}{486}L_{ij11}^{V8,LR} + \frac{205}{486}L_{ij22}^{V8,LR} + \frac{205}{486}L_{ij33}^{V8,LR} - \frac{47}{9}L_{ijii}^{V1,LR} \\
& - \frac{47}{9}L_{ijjj}^{V1,LR} + \frac{205}{486}L_{ijii}^{V8,LR} + \frac{205}{486}L_{ijjj}^{V8,LR} + \frac{2054}{81}L_{ijii}^{V,LL} + \frac{2441}{81}L_{ijjj}^{V,LL} \Big] \\
& + \alpha_s \alpha \Big[ \frac{100}{243}L_{11ij}^{V,LL} + \frac{100}{243}L_{22ij}^{V,LL} + \frac{100}{243}L_{33ij}^{V,LL} - \frac{332}{243}L_{ij11}^{V1,LL} - \frac{332}{243}L_{ij22}^{V1,LL} \\
& - \frac{332}{243}L_{ij33}^{V1,LL} - \frac{332}{243}L_{ij11}^{V1,LR} - \frac{332}{243}L_{ij22}^{V1,LR} - \frac{332}{243}L_{ij33}^{V1,LR} - \frac{571}{729}L_{ij11}^{V8,LL} \\
& - \frac{571}{729}L_{ij22}^{V8,LL} - \frac{571}{729}L_{ij33}^{V8,LL} + \frac{977}{729}L_{ij11}^{V8,LR} + \frac{977}{729}L_{ij22}^{V8,LR} + \frac{977}{729}L_{ij33}^{V8,LR} \\
& + \frac{100}{243}L_{ij11}^{V,LR} + \frac{100}{243}L_{ij22}^{V,LR} + \frac{100}{243}L_{ij33}^{V,LR} + \frac{664}{243}L_{ijii}^{V1,LR} + \frac{664}{243}L_{ijjj}^{V1,LR} \\
& - \frac{2884}{729}L_{ijii}^{V8,LR} - \frac{2884}{729}L_{ijjj}^{V8,LR} - \frac{12152}{243}L_{ijii}^{V,LL} + \frac{3832}{243}L_{ijjj}^{V,LL} \Big] + \alpha^2 \Big[ \frac{1156}{729}L_{11ij}^{V,LL} \\
& + \frac{1156}{729}L_{22ij}^{V,LL} + \frac{1156}{729}L_{33ij}^{V,LL} + \frac{868}{729}L_{ij11}^{V1,LL} + \frac{868}{729}L_{ij22}^{V1,LL} + \frac{868}{729}L_{ij33}^{V1,LL} \\
& - \frac{1148}{729}L_{ij11}^{V1,LR} - \frac{1148}{729}L_{ij22}^{V1,LR} - \frac{1148}{729}L_{ij33}^{V1,LR} - \frac{4892}{729}L_{ij11}^{V,LR} - \frac{4892}{729}L_{ij22}^{V,LR} \\
& - \frac{4892}{729}L_{ij33}^{V,LR} - \frac{5696}{729}L_{ijii}^{V1,LR} - \frac{5696}{729}L_{ijjj}^{V1,LR} - \frac{544}{729}L_{ijii}^{V,LL} + \frac{10112}{729}L_{ijjj}^{V,LL} \Big] ;
\end{aligned}$$

$$\begin{aligned}
\dot{L}_{ij11}^{V,LR} &= e^2 \Big[ \frac{4}{3}L_{11ij}^{V,LL} + \frac{4}{3}L_{22ij}^{V,LL} + \frac{4}{3}L_{33ij}^{V,LL} + \frac{4}{3}L_{ij11}^{V1,LL} + \frac{4}{3}L_{ij22}^{V1,LL} \\
& + \frac{4}{3}L_{ij33}^{V1,LL} + \frac{4}{3}L_{ij11}^{V1,LR} + \frac{4}{3}L_{ij22}^{V1,LR} + \frac{4}{3}L_{ij33}^{V1,LR} + \frac{28}{3}L_{ij11}^{V,LR} + \frac{4}{3}L_{ij22}^{V,LR} \\
& + \frac{4}{3}L_{ij33}^{V,LR} \Big]
\end{aligned}$$

$$\begin{aligned}
& + \frac{4}{3} L_{ij33}^{V,LR} - \frac{8}{3} L_{ijii}^{V1,LR} - \frac{8}{3} L_{ijjj}^{V1,LR} - \frac{64}{9} L_{ijii}^{V,LL} - \frac{64}{9} L_{ijjj}^{V,LL} \Big] + \alpha_s \alpha \Big[ \frac{16}{3} L_{ij11}^{V1,LL} \\
& + \frac{16}{3} L_{ij22}^{V1,LL} + \frac{16}{3} L_{ij33}^{V1,LL} + \frac{16}{3} L_{ij11}^{V1,LR} + \frac{16}{3} L_{ij22}^{V1,LR} + \frac{16}{3} L_{ij33}^{V1,LR} + \frac{328}{243} L_{ij11}^{V8,LL} \\
& + \frac{328}{243} L_{ij22}^{V8,LL} + \frac{328}{243} L_{ij33}^{V8,LL} - \frac{392}{243} L_{ij11}^{V8,LR} - \frac{392}{243} L_{ij22}^{V8,LR} - \frac{392}{243} L_{ij33}^{V8,LR} \\
& - 32 L_{ij11}^{V,LR} - \frac{32}{3} L_{ijii}^{V1,LR} - \frac{32}{3} L_{ijjj}^{V1,LR} + \frac{1984}{243} L_{ijii}^{V8,LR} + \frac{1984}{243} L_{ijjj}^{V8,LR} - \frac{2240}{81} L_{ijii}^{V,LL} \\
& - \frac{2240}{81} L_{ijjj}^{V,LL} \Big] + \alpha^2 \Big[ - \frac{4648}{243} L_{11ij}^{V,LL} - \frac{4648}{243} L_{22ij}^{V,LL} - \frac{4648}{243} L_{33ij}^{V,LL} - \frac{3712}{243} L_{ij11}^{V1,LL} \\
& - \frac{3712}{243} L_{ij22}^{V1,LL} - \frac{3712}{243} L_{ij33}^{V1,LL} - \frac{1048}{243} L_{ij11}^{V1,LR} - \frac{1048}{243} L_{ij22}^{V1,LR} - \frac{1048}{243} L_{ij33}^{V1,LR} \\
& - \frac{41296}{243} L_{ij11}^{V,LR} + \frac{3344}{243} L_{ij22}^{V,LR} + \frac{3344}{243} L_{ij33}^{V,LR} + \frac{12032}{243} L_{ijii}^{V1,LR} + \frac{12032}{243} L_{ijjj}^{V1,LR} \\
& + \frac{3424}{243} L_{ijii}^{V,LL} + \frac{3424}{243} L_{ijjj}^{V,LL} \Big] ;
\end{aligned}$$

$$\begin{aligned}
\dot{L}_{ij22}^{V,LR} & = e^2 \Big[ \frac{4}{3} L_{11ij}^{V,LL} + \frac{4}{3} L_{22ij}^{V,LL} + \frac{4}{3} L_{33ij}^{V,LL} + \frac{4}{3} L_{ij11}^{V1,LL} + \frac{4}{3} L_{ij22}^{V1,LL} \\
& + \frac{4}{3} L_{ij33}^{V1,LL} + \frac{4}{3} L_{ij11}^{V1,LR} + \frac{4}{3} L_{ij22}^{V1,LR} + \frac{4}{3} L_{ij33}^{V1,LR} + \frac{4}{3} L_{ij11}^{V,LR} + \frac{28}{3} L_{ij22}^{V,LR} \\
& + \frac{4}{3} L_{ij33}^{V,LR} - \frac{8}{3} L_{ijii}^{V1,LR} - \frac{8}{3} L_{ijjj}^{V1,LR} - \frac{64}{9} L_{ijii}^{V,LL} - \frac{64}{9} L_{ijjj}^{V,LL} \Big] + \alpha_s \alpha \Big[ \frac{16}{3} L_{ij11}^{V1,LL} \\
& + \frac{16}{3} L_{ij22}^{V1,LL} + \frac{16}{3} L_{ij33}^{V1,LL} + \frac{16}{3} L_{ij11}^{V1,LR} + \frac{16}{3} L_{ij22}^{V1,LR} + \frac{16}{3} L_{ij33}^{V1,LR} + \frac{328}{243} L_{ij11}^{V8,LL} \\
& + \frac{328}{243} L_{ij22}^{V8,LL} + \frac{328}{243} L_{ij33}^{V8,LL} - \frac{392}{243} L_{ij11}^{V8,LR} - \frac{392}{243} L_{ij22}^{V8,LR} - \frac{392}{243} L_{ij33}^{V8,LR} \\
& - 32 L_{ij22}^{V,LR} - \frac{32}{3} L_{ijii}^{V1,LR} - \frac{32}{3} L_{ijjj}^{V1,LR} + \frac{1984}{243} L_{ijii}^{V8,LR} + \frac{1984}{243} L_{ijjj}^{V8,LR} - \frac{2240}{81} L_{ijii}^{V,LL} \\
& - \frac{2240}{81} L_{ijjj}^{V,LL} \Big] + \alpha^2 \Big[ - \frac{4648}{243} L_{11ij}^{V,LL} - \frac{4648}{243} L_{22ij}^{V,LL} - \frac{4648}{243} L_{33ij}^{V,LL} - \frac{3712}{243} L_{ij11}^{V1,LL} \\
& - \frac{3712}{243} L_{ij22}^{V1,LL} - \frac{3712}{243} L_{ij33}^{V1,LL} - \frac{1048}{243} L_{ij11}^{V1,LR} - \frac{1048}{243} L_{ij22}^{V1,LR} - \frac{1048}{243} L_{ij33}^{V1,LR} \\
& + \frac{3344}{243} L_{ij11}^{V,LR} - \frac{41296}{243} L_{ij22}^{V,LR} + \frac{3344}{243} L_{ij33}^{V,LR} + \frac{12032}{243} L_{ijii}^{V1,LR} + \frac{12032}{243} L_{ijjj}^{V1,LR}
\end{aligned}$$

$$\begin{aligned}
& + \frac{3424}{243} L_{ij\bar{i}\bar{i}}^{V,LL} + \frac{3424}{243} L_{ij\bar{j}\bar{j}}^{V,LL} \Big] ; \\
\dot{L}_{ue\bar{i}\bar{j}33}^{V,LR} = & e^2 \left[ \frac{4}{3} L_{11ij}^{V,LL} + \frac{4}{3} L_{22ij}^{V,LL} + \frac{4}{3} L_{33ij}^{V,LL} + \frac{4}{3} L_{ij11}^{V1,LL} + \frac{4}{3} L_{ij22}^{V1,LL} \right. \\
& + \frac{4}{3} L_{ij33}^{V1,LL} + \frac{4}{3} L_{ij11}^{V1,LR} + \frac{4}{3} L_{ij22}^{V1,LR} + \frac{4}{3} L_{ij33}^{V1,LR} + \frac{4}{3} L_{ij11}^{V,LR} + \frac{4}{3} L_{ij22}^{V,LR} \\
& + \frac{28}{3} L_{ij33}^{V,LR} - \frac{8}{3} L_{ij\bar{i}\bar{i}}^{V1,LR} - \frac{8}{3} L_{ij\bar{j}\bar{j}}^{V1,LR} - \frac{64}{9} L_{ij\bar{i}\bar{i}}^{V,LL} - \frac{64}{9} L_{ij\bar{j}\bar{j}}^{V,LL} \Big] + \alpha_s \alpha \left[ \frac{16}{3} L_{ij11}^{V1,LL} \right. \\
& + \frac{16}{3} L_{ij22}^{V1,LL} + \frac{16}{3} L_{ij33}^{V1,LL} + \frac{16}{3} L_{ij11}^{V1,LR} + \frac{16}{3} L_{ij22}^{V1,LR} + \frac{16}{3} L_{ij33}^{V1,LR} + \frac{328}{243} L_{ij11}^{V8,LL} \\
& + \frac{328}{243} L_{ij22}^{V8,LL} + \frac{328}{243} L_{ij33}^{V8,LL} - \frac{392}{243} L_{ij11}^{V8,LR} - \frac{392}{243} L_{ij22}^{V8,LR} - \frac{392}{243} L_{ij33}^{V8,LR} \\
& - 32 L_{ij33}^{V,LR} - \frac{32}{3} L_{ij\bar{i}\bar{i}}^{V1,LR} - \frac{32}{3} L_{ij\bar{j}\bar{j}}^{V1,LR} + \frac{1984}{243} L_{ij\bar{i}\bar{i}}^{V8,LR} + \frac{1984}{243} L_{ij\bar{j}\bar{j}}^{V8,LR} - \frac{2240}{81} L_{ij\bar{i}\bar{i}}^{V,LL} \\
& \left. - \frac{2240}{81} L_{ij\bar{j}\bar{j}}^{V,LL} \right] + \alpha^2 \left[ - \frac{4648}{243} L_{11ij}^{V,LL} - \frac{4648}{243} L_{22ij}^{V,LL} - \frac{4648}{243} L_{33ij}^{V,LL} - \frac{3712}{243} L_{ij11}^{V1,LL} \right. \\
& - \frac{3712}{243} L_{ij22}^{V1,LL} - \frac{3712}{243} L_{ij33}^{V1,LL} - \frac{1048}{243} L_{ij11}^{V1,LR} - \frac{1048}{243} L_{ij22}^{V1,LR} - \frac{1048}{243} L_{ij33}^{V1,LR} \\
& + \frac{3344}{243} L_{ij11}^{V,LR} + \frac{3344}{243} L_{ij22}^{V,LR} - \frac{41296}{243} L_{ij33}^{V,LR} + \frac{12032}{243} L_{ij\bar{i}\bar{i}}^{V1,LR} + \frac{12032}{243} L_{ij\bar{j}\bar{j}}^{V1,LR} \\
& \left. + \frac{3424}{243} L_{ij\bar{i}\bar{i}}^{V,LL} + \frac{3424}{243} L_{ij\bar{j}\bar{j}}^{V,LL} \right] ; \\
\dot{L}_{ud\bar{i}\bar{j}11}^{V1,LR} = & - \frac{8}{3} g_s^2 L_{ij11}^{V8,LR} + e^2 \left[ \frac{4}{9} L_{11ij}^{V,LL} + \frac{4}{9} L_{22ij}^{V,LL} + \frac{4}{9} L_{33ij}^{V,LL} + \frac{4}{9} L_{ij11}^{V1,LL} \right. \\
& + \frac{4}{9} L_{ij22}^{V1,LL} + \frac{4}{9} L_{ij33}^{V1,LL} + \frac{28}{9} L_{ij11}^{V1,LR} + \frac{4}{9} L_{ij22}^{V1,LR} + \frac{4}{9} L_{ij33}^{V1,LR} + \frac{4}{9} L_{ij11}^{V,LR} \\
& + \frac{4}{9} L_{ij22}^{V,LR} + \frac{4}{9} L_{ij33}^{V,LR} - \frac{8}{9} L_{ij\bar{i}\bar{i}}^{V1,LR} - \frac{8}{9} L_{ij\bar{j}\bar{j}}^{V1,LR} - \frac{64}{27} L_{ij\bar{i}\bar{i}}^{V,LL} - \frac{64}{27} L_{ij\bar{j}\bar{j}}^{V,LL} \Big] \\
& + \alpha_s^2 \left[ - 8 L_{ij11}^{V1,LL} - 8 L_{ij22}^{V1,LL} - 8 L_{ij33}^{V1,LL} - \frac{4}{3} L_{ij11}^{V1,LR} + 8 L_{ij22}^{V1,LR} \right. \\
& + 8 L_{ij33}^{V1,LR} + \frac{44}{27} L_{ij11}^{V8,LL} + \frac{44}{27} L_{ij22}^{V8,LL} + \frac{44}{27} L_{ij33}^{V8,LL} - \frac{2000}{27} L_{ij11}^{V8,LR} + \frac{44}{27} L_{ij22}^{V8,LR} \\
& \left. + \frac{44}{27} L_{ij33}^{V8,LR} \right]
\end{aligned}$$

$$\begin{aligned}
& + \frac{44}{27} L_{ij33}^{V8,LR} + 8 L_{ijii}^{V1,LR} + 8 L_{ijjj}^{V1,LR} + \frac{44}{27} L_{ijii}^{V8,LR} + \frac{44}{27} L_{ijjj}^{V8,LR} - \frac{232}{9} L_{ijii}^{V,LL} \\
& - \frac{232}{9} L_{ijjj}^{V,LL} \Big] + \alpha_s \alpha \left[ \frac{16}{9} L_{ij11}^{V1,LL} + \frac{16}{9} L_{ij22}^{V1,LL} + \frac{16}{9} L_{ij33}^{V1,LL} - \frac{176}{9} L_{ij11}^{V1,LR} \right. \\
& + \frac{16}{9} L_{ij22}^{V1,LR} + \frac{16}{9} L_{ij33}^{V1,LR} + \frac{328}{729} L_{ij11}^{V8,LL} + \frac{328}{729} L_{ij22}^{V8,LL} + \frac{328}{729} L_{ij33}^{V8,LL} + \frac{5872}{729} L_{ij11}^{V8,LR} \\
& - \frac{392}{729} L_{ij22}^{V8,LR} - \frac{392}{729} L_{ij33}^{V8,LR} - \frac{32}{9} L_{ijii}^{V1,LR} - \frac{32}{9} L_{ijjj}^{V1,LR} + \frac{1984}{729} L_{ijii}^{V8,LR} + \frac{1984}{729} L_{ijjj}^{V8,LR} \\
& - \frac{2240}{243} L_{ijii}^{V,LL} - \frac{2240}{243} L_{ijjj}^{V,LL} \Big] + \alpha^2 \left[ - \frac{1120}{729} L_{11ij}^{V,LL} - \frac{1120}{729} L_{22ij}^{V,LL} - \frac{1120}{729} L_{33ij}^{V,LL} \right. \\
& - \frac{1480}{729} L_{ij11}^{V1,LL} - \frac{1480}{729} L_{ij22}^{V1,LL} - \frac{1480}{729} L_{ij33}^{V1,LL} - \frac{36544}{729} L_{ij11}^{V1,LR} - \frac{112}{729} L_{ij22}^{V1,LR} \\
& - \frac{112}{729} L_{ij33}^{V1,LR} + \frac{2984}{729} L_{ij11}^{V,LR} + \frac{2984}{729} L_{ij22}^{V,LR} + \frac{2984}{729} L_{ij33}^{V,LR} + \frac{6272}{729} L_{ijii}^{V1,LR} \\
& \left. + \frac{6272}{729} L_{ijjj}^{V1,LR} + \frac{4000}{729} L_{ijii}^{V,LL} + \frac{4000}{729} L_{ijjj}^{V,LL} \right] ;
\end{aligned}$$

$$\begin{aligned}
\dot{L}_{ij11}^{V8,LR} &= g_s^2 \left[ -12 L_{ij11}^{V1,LR} + \frac{2}{3} L_{ij11}^{V8,LL} + \frac{2}{3} L_{ij22}^{V8,LL} + \frac{2}{3} L_{ij33}^{V8,LL} - \frac{40}{3} L_{ij11}^{V8,LR} \right. \\
& + \frac{2}{3} L_{ij22}^{V8,LR} + \frac{2}{3} L_{ij33}^{V8,LR} + \frac{2}{3} L_{ijii}^{V8,LR} + \frac{2}{3} L_{ijjj}^{V8,LR} + \frac{8}{3} L_{ijii}^{V,LL} + \frac{8}{3} L_{ijjj}^{V,LL} \Big] \\
& + \frac{8}{3} e^2 L_{ij11}^{V8,LR} + \alpha_s^2 \left[ - \frac{2}{3} L_{ij11}^{V1,LL} - \frac{2}{3} L_{ij22}^{V1,LL} - \frac{2}{3} L_{ij33}^{V1,LL} - 132 L_{ij11}^{V1,LR} \right. \\
& - \frac{22}{3} L_{ij22}^{V1,LR} - \frac{22}{3} L_{ij33}^{V1,LR} + \frac{619}{81} L_{ij11}^{V8,LL} + \frac{619}{81} L_{ij22}^{V8,LL} + \frac{619}{81} L_{ij33}^{V8,LL} - \frac{25177}{162} L_{ij11}^{V8,LR} \\
& + \frac{799}{81} L_{ij22}^{V8,LR} + \frac{799}{81} L_{ij33}^{V8,LR} - \frac{22}{3} L_{ijii}^{V1,LR} - \frac{22}{3} L_{ijjj}^{V1,LR} + \frac{799}{81} L_{ijii}^{V8,LR} + \frac{799}{81} L_{ijjj}^{V8,LR} \\
& \left. + \frac{1210}{27} L_{ijii}^{V,LL} + \frac{1210}{27} L_{ijjj}^{V,LL} \right] + \alpha_s \alpha \left[ \frac{668}{81} L_{11ij}^{V,LL} + \frac{668}{81} L_{22ij}^{V,LL} + \frac{668}{81} L_{33ij}^{V,LL} \right. \\
& + \frac{668}{81} L_{ij11}^{V1,LL} + \frac{668}{81} L_{ij22}^{V1,LL} + \frac{668}{81} L_{ij33}^{V1,LL} + \frac{3800}{81} L_{ij11}^{V1,LR} + \frac{668}{81} L_{ij22}^{V1,LR} \\
& \left. + \frac{668}{81} L_{ij33}^{V1,LR} - \frac{70}{27} L_{ij11}^{V8,LL} - \frac{70}{27} L_{ij22}^{V8,LL} - \frac{70}{27} L_{ij33}^{V8,LL} + \frac{67}{3} L_{ij11}^{V8,LR} + \frac{14}{9} L_{ij22}^{V8,LR} \right]
\end{aligned}$$

$$\begin{aligned}
& + \frac{14}{9} L_{ud}^{V8,LR} + \frac{668}{81} L_{ij11}^{V,LR} + \frac{668}{81} L_{ij22}^{V,LR} + \frac{668}{81} L_{ij33}^{V,LR} - \frac{1336}{81} L_{ijii}^{V1,LR} - \frac{1336}{81} L_{ijjj}^{V1,LR} \\
& - \frac{20}{3} L_{ijii}^{V8,LR} - \frac{20}{3} L_{ijjj}^{V8,LR} - \frac{3800}{81} L_{ijii}^{V,LL} - \frac{3800}{81} L_{ijjj}^{V,LL} \Big] - \frac{4048}{81} \alpha^2 L_{ij11}^{V8,LR} ; \\
\dot{L}_{ud}^{V1,LR} = & - \frac{8}{3} g_s^2 L_{ij22}^{V8,LR} + e^2 \Bigg[ \frac{4}{9} L_{11ij}^{V,LL} + \frac{4}{9} L_{22ij}^{V,LL} + \frac{4}{9} L_{33ij}^{V,LL} + \frac{4}{9} L_{ij11}^{V1,LL} \\
& + \frac{4}{9} L_{ij22}^{V1,LL} + \frac{4}{9} L_{ij33}^{V1,LL} + \frac{4}{9} L_{ij11}^{V1,LR} + \frac{28}{9} L_{ij22}^{V1,LR} + \frac{4}{9} L_{ij33}^{V1,LR} + \frac{4}{9} L_{ij11}^{V,LR} \\
& + \frac{4}{9} L_{ij22}^{V,LR} + \frac{4}{9} L_{ij33}^{V,LR} - \frac{8}{9} L_{ijii}^{V1,LR} - \frac{8}{9} L_{ijjj}^{V1,LR} - \frac{64}{27} L_{ijii}^{V,LL} - \frac{64}{27} L_{ijjj}^{V,LL} \Big] \\
& + \alpha_s^2 \Bigg[ -8 L_{ij11}^{V1,LL} - 8 L_{ij22}^{V1,LL} - 8 L_{ij33}^{V1,LL} + 8 L_{ij11}^{V1,LR} - \frac{4}{3} L_{ij22}^{V1,LR} \\
& + 8 L_{ij33}^{V1,LR} + \frac{44}{27} L_{ij11}^{V8,LL} + \frac{44}{27} L_{ij22}^{V8,LL} + \frac{44}{27} L_{ij33}^{V8,LL} + \frac{44}{27} L_{ij11}^{V8,LR} - \frac{2000}{27} L_{ij22}^{V8,LR} \\
& + \frac{44}{27} L_{ij33}^{V8,LR} + 8 L_{ijii}^{V1,LR} + 8 L_{ijjj}^{V1,LR} + \frac{44}{27} L_{ijii}^{V8,LR} + \frac{44}{27} L_{ijjj}^{V8,LR} - \frac{232}{9} L_{ijii}^{V,LL} \\
& - \frac{232}{9} L_{ijjj}^{V,LL} \Big] + \alpha_s \alpha \Bigg[ \frac{16}{9} L_{ij11}^{V1,LL} + \frac{16}{9} L_{ij22}^{V1,LL} + \frac{16}{9} L_{ij33}^{V1,LL} + \frac{16}{9} L_{ij11}^{V1,LR} \\
& - \frac{176}{9} L_{ij22}^{V1,LR} + \frac{16}{9} L_{ij33}^{V1,LR} + \frac{328}{729} L_{ij11}^{V8,LL} + \frac{328}{729} L_{ij22}^{V8,LL} + \frac{328}{729} L_{ij33}^{V8,LL} - \frac{392}{729} L_{ij11}^{V8,LR} \\
& + \frac{5872}{729} L_{ij22}^{V8,LR} - \frac{392}{729} L_{ij33}^{V8,LR} - \frac{32}{9} L_{ijii}^{V1,LR} - \frac{32}{9} L_{ijjj}^{V1,LR} + \frac{1984}{729} L_{ijii}^{V8,LR} \\
& + \frac{1984}{729} L_{ijjj}^{V8,LR} - \frac{2240}{243} L_{ijii}^{V,LL} - \frac{2240}{243} L_{ijjj}^{V,LL} \Big] + \alpha^2 \Bigg[ -\frac{1120}{729} L_{11ij}^{V,LL} - \frac{1120}{729} L_{22ij}^{V,LL} \\
& - \frac{1120}{729} L_{33ij}^{V,LL} - \frac{1480}{729} L_{ij11}^{V1,LL} - \frac{1480}{729} L_{ij22}^{V1,LL} - \frac{1480}{729} L_{ij33}^{V1,LL} - \frac{112}{729} L_{ij11}^{V1,LR} \\
& - \frac{36544}{729} L_{ij22}^{V1,LR} - \frac{112}{729} L_{ij33}^{V1,LR} + \frac{2984}{729} L_{ij11}^{V,LR} + \frac{2984}{729} L_{ij22}^{V,LR} + \frac{2984}{729} L_{ij33}^{V,LR} \\
& + \frac{6272}{729} L_{ijii}^{V1,LR} + \frac{6272}{729} L_{ijjj}^{V1,LR} + \frac{4000}{729} L_{ijii}^{V,LL} + \frac{4000}{729} L_{ijjj}^{V,LL} \Big] ; \\
\dot{L}_{ud}^{V8,LR} = & g_s^2 \Bigg[ -12 L_{ij22}^{V1,LR} + \frac{2}{3} L_{ij11}^{V8,LL} + \frac{2}{3} L_{ij22}^{V8,LL} + \frac{2}{3} L_{ij33}^{V8,LL} + \frac{2}{3} L_{ij11}^{V8,LR} \\
& + \frac{2}{3} L_{ij22}^{V8,LR} + \frac{2}{3} L_{ij33}^{V8,LR} \Big] ;
\end{aligned}$$

$$\begin{aligned}
& -\frac{40}{3}L_{ij22}^{V8,LR} + \frac{2}{3}L_{ij33}^{V8,LR} + \frac{2}{3}L_{ijii}^{V8,LR} + \frac{2}{3}L_{ijjj}^{V8,LR} + \frac{8}{3}L_{ijii}^{V,LL} + \frac{8}{3}L_{ijjj}^{V,LL} \Big] \\
& + \frac{8}{3}e^2L_{ij22}^{V8,LR} + \alpha_s^2 \left[ -\frac{2}{3}L_{ij11}^{V1,LL} - \frac{2}{3}L_{ij22}^{V1,LL} - \frac{2}{3}L_{ij33}^{V1,LL} - \frac{22}{3}L_{ij11}^{V1,LR} \right. \\
& - 132L_{ij22}^{V1,LR} - \frac{22}{3}L_{ij33}^{V1,LR} + \frac{619}{81}L_{ij11}^{V8,LL} + \frac{619}{81}L_{ij22}^{V8,LL} + \frac{619}{81}L_{ij33}^{V8,LL} + \frac{799}{81}L_{ij11}^{V8,LR} \\
& - \frac{25177}{162}L_{ij22}^{V8,LR} + \frac{799}{81}L_{ij33}^{V8,LR} - \frac{22}{3}L_{ijii}^{V1,LR} - \frac{22}{3}L_{ijjj}^{V1,LR} + \frac{799}{81}L_{ijii}^{V8,LR} + \frac{799}{81}L_{ijjj}^{V8,LR} \\
& \left. + \frac{1210}{27}L_{ijii}^{V,LL} + \frac{1210}{27}L_{ijjj}^{V,LL} \right] + \alpha_s \alpha \left[ \frac{668}{81}L_{11ij}^{V,LL} + \frac{668}{81}L_{22ij}^{V,LL} + \frac{668}{81}L_{33ij}^{V,LL} \right. \\
& + \frac{668}{81}L_{ij11}^{V1,LL} + \frac{668}{81}L_{ij22}^{V1,LL} + \frac{668}{81}L_{ij33}^{V1,LL} + \frac{668}{81}L_{ij11}^{V1,LR} + \frac{3800}{81}L_{ij22}^{V1,LR} \\
& + \frac{668}{81}L_{ij33}^{V1,LR} - \frac{70}{27}L_{ij11}^{V8,LL} - \frac{70}{27}L_{ij22}^{V8,LL} - \frac{70}{27}L_{ij33}^{V8,LL} + \frac{14}{9}L_{ij11}^{V8,LR} + \frac{67}{3}L_{ij22}^{V8,LR} \\
& + \frac{14}{9}L_{ij33}^{V8,LR} + \frac{668}{81}L_{ij11}^{V,LR} + \frac{668}{81}L_{ij22}^{V,LR} + \frac{668}{81}L_{ij33}^{V,LR} - \frac{1336}{81}L_{ijii}^{V1,LR} - \frac{1336}{81}L_{ijjj}^{V1,LR} \\
& \left. - \frac{20}{3}L_{ijii}^{V8,LR} - \frac{20}{3}L_{ijjj}^{V8,LR} - \frac{3800}{81}L_{ijii}^{V,LL} - \frac{3800}{81}L_{ijjj}^{V,LL} \right] - \frac{4048}{81}\alpha^2L_{ij22}^{V8,LR} ;
\end{aligned}$$

$$\begin{aligned}
\dot{L}_{ij33}^{V1,LR} = & -\frac{8}{3}g_s^2L_{ij33}^{V8,LR} + e^2 \left[ \frac{4}{9}L_{11ij}^{V,LL} + \frac{4}{9}L_{22ij}^{V,LL} + \frac{4}{9}L_{33ij}^{V,LL} + \frac{4}{9}L_{ij11}^{V1,LL} \right. \\
& + \frac{4}{9}L_{ij22}^{V1,LL} + \frac{4}{9}L_{ij33}^{V1,LL} + \frac{4}{9}L_{ij11}^{V1,LR} + \frac{4}{9}L_{ij22}^{V1,LR} + \frac{28}{9}L_{ij33}^{V1,LR} + \frac{4}{9}L_{ij11}^{V,LR} \\
& + \frac{4}{9}L_{ij22}^{V,LR} + \frac{4}{9}L_{ij33}^{V,LR} - \frac{8}{9}L_{ijii}^{V1,LR} - \frac{8}{9}L_{ijjj}^{V1,LR} - \frac{64}{27}L_{ijii}^{V,LL} - \frac{64}{27}L_{ijjj}^{V,LL} \Big] \\
& + \alpha_s^2 \left[ -8L_{ij11}^{V1,LL} - 8L_{ij22}^{V1,LL} - 8L_{ij33}^{V1,LL} + 8L_{ij11}^{V1,LR} + 8L_{ij22}^{V1,LR} \right. \\
& - \frac{4}{3}L_{ij33}^{V1,LR} + \frac{44}{27}L_{ij11}^{V8,LL} + \frac{44}{27}L_{ij22}^{V8,LL} + \frac{44}{27}L_{ij33}^{V8,LL} + \frac{44}{27}L_{ij11}^{V8,LR} + \frac{44}{27}L_{ij22}^{V8,LR} \\
& - \frac{2000}{27}L_{ij33}^{V8,LR} + 8L_{ijii}^{V1,LR} + 8L_{ijjj}^{V1,LR} + \frac{44}{27}L_{ijii}^{V8,LR} + \frac{44}{27}L_{ijjj}^{V8,LR} - \frac{232}{9}L_{ijii}^{V,LL} \\
& \left. - \frac{232}{9}L_{ijjj}^{V,LL} \right] + \alpha_s \alpha \left[ \frac{16}{9}L_{ij11}^{V1,LL} + \frac{16}{9}L_{ij22}^{V1,LL} + \frac{16}{9}L_{ij33}^{V1,LL} + \frac{16}{9}L_{ij11}^{V1,LR} \right.
\end{aligned}$$

$$\begin{aligned}
& + \frac{16}{9} L_{ij22}^{V1,LR} - \frac{176}{9} L_{ij33}^{V1,LR} + \frac{328}{729} L_{ij11}^{V8,LL} + \frac{328}{729} L_{ij22}^{V8,LL} + \frac{328}{729} L_{ij33}^{V8,LL} - \frac{392}{729} L_{ij11}^{V8,LR} \\
& - \frac{392}{729} L_{ij22}^{V8,LR} + \frac{5872}{729} L_{ij33}^{V8,LR} - \frac{32}{9} L_{ijii}^{V1,LR} - \frac{32}{9} L_{ijjj}^{V1,LR} + \frac{1984}{729} L_{ijii}^{V8,LR} \\
& + \frac{1984}{729} L_{ijjj}^{V8,LR} - \frac{2240}{243} L_{ijii}^{V,LL} - \frac{2240}{243} L_{ijjj}^{V,LL} \Big] + \alpha^2 \Big[ - \frac{1120}{729} L_{11ij}^{V,LL} - \frac{1120}{729} L_{22ij}^{V,LL} \\
& - \frac{1120}{729} L_{33ij}^{V,LL} - \frac{1480}{729} L_{ij11}^{V1,LL} - \frac{1480}{729} L_{ij22}^{V1,LL} - \frac{1480}{729} L_{ij33}^{V1,LL} - \frac{112}{729} L_{ij11}^{V1,LR} \\
& - \frac{112}{729} L_{ij22}^{V1,LR} - \frac{36544}{729} L_{ij33}^{V1,LR} + \frac{2984}{729} L_{ij11}^{V,LR} + \frac{2984}{729} L_{ij22}^{V,LR} + \frac{2984}{729} L_{ij33}^{V,LR} \\
& + \frac{6272}{729} L_{ijii}^{V1,LR} + \frac{6272}{729} L_{ijjj}^{V1,LR} + \frac{4000}{729} L_{ijii}^{V,LL} + \frac{4000}{729} L_{ijjj}^{V,LL} \Big] ;
\end{aligned}$$

$$\begin{aligned}
\dot{L}_{ij33}^{V8,LR} = & g_s^2 \Big[ -12 L_{ij33}^{V1,LR} + \frac{2}{3} L_{ij11}^{V8,LL} + \frac{2}{3} L_{ij22}^{V8,LL} + \frac{2}{3} L_{ij33}^{V8,LL} + \frac{2}{3} L_{ij11}^{V8,LR} \\
& + \frac{2}{3} L_{ij22}^{V8,LR} - \frac{40}{3} L_{ij33}^{V8,LR} + \frac{2}{3} L_{ijii}^{V8,LR} + \frac{2}{3} L_{ijjj}^{V8,LR} + \frac{8}{3} L_{ijii}^{V,LL} + \frac{8}{3} L_{ijjj}^{V,LL} \Big] \\
& + \frac{8}{3} e^2 L_{ij33}^{V8,LR} + \alpha_s^2 \Big[ - \frac{2}{3} L_{ij11}^{V1,LL} - \frac{2}{3} L_{ij22}^{V1,LL} - \frac{2}{3} L_{ij33}^{V1,LL} - \frac{22}{3} L_{ij11}^{V1,LR} \\
& - \frac{22}{3} L_{ij22}^{V1,LR} - 132 L_{ij33}^{V1,LR} + \frac{619}{81} L_{ij11}^{V8,LL} + \frac{619}{81} L_{ij22}^{V8,LL} + \frac{619}{81} L_{ij33}^{V8,LL} + \frac{799}{81} L_{ij11}^{V8,LR} \\
& + \frac{799}{81} L_{ij22}^{V8,LR} - \frac{25177}{162} L_{ij33}^{V8,LR} - \frac{22}{3} L_{ijii}^{V1,LR} - \frac{22}{3} L_{ijjj}^{V1,LR} + \frac{799}{81} L_{ijii}^{V8,LR} + \frac{799}{81} L_{ijjj}^{V8,LR} \\
& + \frac{1210}{27} L_{ijii}^{V,LL} + \frac{1210}{27} L_{ijjj}^{V,LL} \Big] + \alpha_s \alpha \Big[ \frac{668}{81} L_{11ij}^{V,LL} + \frac{668}{81} L_{22ij}^{V,LL} + \frac{668}{81} L_{33ij}^{V,LL} \\
& + \frac{668}{81} L_{ij11}^{V1,LL} + \frac{668}{81} L_{ij22}^{V1,LL} + \frac{668}{81} L_{ij33}^{V1,LL} + \frac{668}{81} L_{ij11}^{V1,LR} + \frac{668}{81} L_{ij22}^{V1,LR} + \frac{3800}{81} L_{ij33}^{V1,LR} \\
& - \frac{70}{27} L_{ij11}^{V8,LL} - \frac{70}{27} L_{ij22}^{V8,LL} - \frac{70}{27} L_{ij33}^{V8,LL} + \frac{14}{9} L_{ij11}^{V8,LR} + \frac{14}{9} L_{ij22}^{V8,LR} + \frac{67}{3} L_{ij33}^{V8,LR} \\
& + \frac{668}{81} L_{ij11}^{V,LR} + \frac{668}{81} L_{ij22}^{V,LR} + \frac{668}{81} L_{ij33}^{V,LR} - \frac{1336}{81} L_{ijii}^{V1,LR} - \frac{1336}{81} L_{ijjj}^{V1,LR} - \frac{20}{3} L_{ijii}^{V8,LR} \\
& - \frac{20}{3} L_{ijjj}^{V8,LR} - \frac{3800}{81} L_{ijii}^{V,LL} - \frac{3800}{81} L_{ijjj}^{V,LL} \Big] - \frac{4048}{81} \alpha^2 L_{ij33}^{V8,LR} ;
\end{aligned}$$

$$\begin{aligned}
\dot{L}_{ijjj}^{V1,LR} = & -\frac{8}{3}g_s^2 L_{ijjj}^{V8,LR} + e^2 \left[ -\frac{8}{9}L_{11ij}^{V,LL} - \frac{8}{9}L_{22ij}^{V,LL} - \frac{8}{9}L_{33ij}^{V,LL} - \frac{8}{9}L_{ij11}^{V1,LL} \right. \\
& - \frac{8}{9}L_{ij22}^{V1,LL} - \frac{8}{9}L_{ij33}^{V1,LL} - \frac{8}{9}L_{ij11}^{V1,LR} - \frac{8}{9}L_{ij22}^{V1,LR} - \frac{8}{9}L_{ij33}^{V1,LR} - \frac{8}{9}L_{ij11}^{V,LR} \\
& \left. - \frac{8}{9}L_{ij22}^{V,LR} - \frac{8}{9}L_{ij33}^{V,LR} + \frac{16}{9}L_{ijii}^{V1,LR} - \frac{32}{9}L_{ijjj}^{V1,LR} + \frac{128}{27}L_{ijii}^{V,LL} + \frac{128}{27}L_{ijjj}^{V,LL} \right] \\
& + \alpha_s^2 \left[ -8L_{ij11}^{V1,LL} - 8L_{ij22}^{V1,LL} - 8L_{ij33}^{V1,LL} + 8L_{ij11}^{V1,LR} + 8L_{ij22}^{V1,LR} \right. \\
& + 8L_{ij33}^{V1,LR} + \frac{44}{27}L_{ij11}^{V8,LL} + \frac{44}{27}L_{ij22}^{V8,LL} + \frac{44}{27}L_{ij33}^{V8,LL} + \frac{44}{27}L_{ij11}^{V8,LR} + \frac{44}{27}L_{ij22}^{V8,LR} \\
& + \frac{44}{27}L_{ij33}^{V8,LR} + 8L_{ijii}^{V1,LR} - \frac{4}{3}L_{ijjj}^{V1,LR} + \frac{44}{27}L_{ijii}^{V8,LR} - \frac{2000}{27}L_{ijjj}^{V8,LR} - \frac{232}{9}L_{ijii}^{V,LL} \\
& \left. - \frac{232}{9}L_{ijjj}^{V,LL} \right] + \alpha_s \alpha \left[ -\frac{32}{9}L_{ij11}^{V1,LL} - \frac{32}{9}L_{ij22}^{V1,LL} - \frac{32}{9}L_{ij33}^{V1,LL} - \frac{32}{9}L_{ij11}^{V1,LR} \right. \\
& - \frac{32}{9}L_{ij22}^{V1,LR} - \frac{32}{9}L_{ij33}^{V1,LR} - \frac{656}{729}L_{ij11}^{V8,LL} - \frac{656}{729}L_{ij22}^{V8,LL} - \frac{656}{729}L_{ij33}^{V8,LL} + \frac{784}{729}L_{ij11}^{V8,LR} \\
& + \frac{784}{729}L_{ij22}^{V8,LR} + \frac{784}{729}L_{ij33}^{V8,LR} + \frac{64}{9}L_{ijii}^{V1,LR} + \frac{448}{9}L_{ijjj}^{V1,LR} - \frac{3968}{729}L_{ijii}^{V8,LR} \\
& \left. - \frac{4832}{729}L_{ijjj}^{V8,LR} + \frac{4480}{243}L_{ijii}^{V,LL} + \frac{4480}{243}L_{ijjj}^{V,LL} \right] + \alpha^2 \left[ -\frac{8344}{729}L_{11ij}^{V,LL} - \frac{8344}{729}L_{22ij}^{V,LL} \right. \\
& - \frac{8344}{729}L_{33ij}^{V,LL} - \frac{3736}{729}L_{ij11}^{V1,LL} - \frac{3736}{729}L_{ij22}^{V1,LL} - \frac{3736}{729}L_{ij33}^{V1,LL} - \frac{2584}{729}L_{ij11}^{V1,LR} \\
& - \frac{2584}{729}L_{ij22}^{V1,LR} - \frac{2584}{729}L_{ij33}^{V1,LR} - \frac{4888}{729}L_{ij11}^{V,LR} - \frac{4888}{729}L_{ij22}^{V,LR} - \frac{4888}{729}L_{ij33}^{V,LR} \\
& \left. + \frac{4736}{729}L_{ijii}^{V1,LR} + \frac{72416}{729}L_{ijjj}^{V1,LR} - \frac{9728}{729}L_{ijii}^{V,LL} - \frac{9728}{729}L_{ijjj}^{V,LL} \right];
\end{aligned}$$

$$\begin{aligned}
\dot{L}_{ijjj}^{V8,LR} = & g_s^2 \left[ \frac{2}{3}L_{ij11}^{V8,LL} + \frac{2}{3}L_{ij22}^{V8,LL} + \frac{2}{3}L_{ij33}^{V8,LL} + \frac{2}{3}L_{ij11}^{V8,LR} + \frac{2}{3}L_{ij22}^{V8,LR} \right. \\
& \left. + \frac{2}{3}L_{ij33}^{V8,LR} - 12L_{ijjj}^{V1,LR} + \frac{2}{3}L_{ijii}^{V8,LR} - \frac{40}{3}L_{ijjj}^{V8,LR} + \frac{8}{3}L_{ijii}^{V,LL} + \frac{8}{3}L_{ijjj}^{V,LL} \right] \\
& - \frac{16}{3}e^2 L_{ijjj}^{V8,LR} + \alpha_s^2 \left[ -\frac{2}{3}L_{ij11}^{V1,LL} - \frac{2}{3}L_{ij22}^{V1,LL} - \frac{2}{3}L_{ij33}^{V1,LL} - \frac{22}{3}L_{ij11}^{V1,LR} \right.
\end{aligned}$$



$$\begin{aligned}
& -\frac{22}{3}L_{ud\ ij22}^{V1,LR} - \frac{22}{3}L_{ud\ ij33}^{V1,LR} + \frac{619}{81}L_{ud\ ij11}^{V8,LL} + \frac{619}{81}L_{ud\ ij22}^{V8,LL} + \frac{619}{81}L_{ud\ ij33}^{V8,LL} + \frac{799}{81}L_{ud\ ij11}^{V8,LR} \\
& + \frac{799}{81}L_{ud\ ij22}^{V8,LR} + \frac{799}{81}L_{ud\ ij33}^{V8,LR} - \frac{22}{3}L_{uu\ ijii}^{V1,LR} - 132L_{uu\ ijjj}^{V1,LR} + \frac{799}{81}L_{uu\ ijii}^{V8,LR} - \frac{25177}{162}L_{uu\ ijjj}^{V8,LR} \\
& + \frac{1210}{27}L_{uu\ ijii}^{V,LL} + \frac{1210}{27}L_{uu\ ijjj}^{V,LL} \Big] + \alpha_s \alpha \Bigg[ -\frac{520}{81}L_{11ij}^{V,LL} - \frac{520}{81}L_{22ij}^{V,LL} - \frac{520}{81}L_{33ij}^{V,LL} \\
& - \frac{520}{81}L_{ud\ ij11}^{V1,LL} - \frac{520}{81}L_{ud\ ij22}^{V1,LL} - \frac{520}{81}L_{ud\ ij33}^{V1,LL} - \frac{520}{81}L_{ud\ ij11}^{V1,LR} - \frac{520}{81}L_{ud\ ij22}^{V1,LR} - \frac{520}{81}L_{ud\ ij33}^{V1,LR} \\
& + \frac{170}{27}L_{ud\ ij11}^{V8,LL} + \frac{170}{27}L_{ud\ ij22}^{V8,LL} + \frac{170}{27}L_{ud\ ij33}^{V8,LL} + \frac{22}{9}L_{ud\ ij11}^{V8,LR} + \frac{22}{9}L_{ud\ ij22}^{V8,LR} + \frac{22}{9}L_{ud\ ij33}^{V8,LR} \\
& - \frac{520}{81}L_{ue\ ij11}^{V,LR} - \frac{520}{81}L_{ue\ ij22}^{V,LR} - \frac{520}{81}L_{ue\ ij33}^{V,LR} + \frac{1040}{81}L_{uu\ ijii}^{V1,LR} + \frac{608}{81}L_{uu\ ijjj}^{V1,LR} + \frac{56}{9}L_{uu\ ijii}^{V8,LR} \\
& - \frac{16}{3}L_{uu\ ijjj}^{V8,LR} + \frac{1168}{81}L_{uu\ ijii}^{V,LL} + \frac{1168}{81}L_{uu\ ijjj}^{V,LL} \Big] + \frac{7520}{81}\alpha^2 L_{uu\ ijjj}^{V8,LR} ;
\end{aligned}$$

$$\begin{aligned}
\dot{L}_{uu\ ijii}^{V1,LR} = & -\frac{8}{3}g_s^2 L_{uu\ ijii}^{V8,LR} + e^2 \Bigg[ -\frac{8}{9}L_{11ij}^{V,LL} - \frac{8}{9}L_{22ij}^{V,LL} - \frac{8}{9}L_{33ij}^{V,LL} - \frac{8}{9}L_{ud\ ij11}^{V1,LL} \\
& - \frac{8}{9}L_{ud\ ij22}^{V1,LL} - \frac{8}{9}L_{ud\ ij33}^{V1,LL} - \frac{8}{9}L_{ud\ ij11}^{V1,LR} - \frac{8}{9}L_{ud\ ij22}^{V1,LR} - \frac{8}{9}L_{ud\ ij33}^{V1,LR} - \frac{8}{9}L_{ue\ ij11}^{V,LR} \\
& - \frac{8}{9}L_{ue\ ij22}^{V,LR} - \frac{8}{9}L_{ue\ ij33}^{V,LR} - \frac{32}{9}L_{uu\ ijii}^{V1,LR} + \frac{16}{9}L_{uu\ ijjj}^{V1,LR} + \frac{128}{27}L_{uu\ ijii}^{V,LL} + \frac{128}{27}L_{uu\ ijjj}^{V,LL} \Big] \\
& + \alpha_s^2 \Bigg[ -8L_{ud\ ij11}^{V1,LL} - 8L_{ud\ ij22}^{V1,LL} - 8L_{ud\ ij33}^{V1,LL} + 8L_{ud\ ij11}^{V1,LR} + 8L_{ud\ ij22}^{V1,LR} \\
& + 8L_{ud\ ij33}^{V1,LR} + \frac{44}{27}L_{ud\ ij11}^{V8,LL} + \frac{44}{27}L_{ud\ ij22}^{V8,LL} + \frac{44}{27}L_{ud\ ij33}^{V8,LL} + \frac{44}{27}L_{ud\ ij11}^{V8,LR} + \frac{44}{27}L_{ud\ ij22}^{V8,LR} \\
& + \frac{44}{27}L_{ud\ ij33}^{V8,LR} - \frac{4}{3}L_{uu\ ijii}^{V1,LR} + 8L_{uu\ ijjj}^{V1,LR} - \frac{2000}{27}L_{uu\ ijii}^{V8,LR} + \frac{44}{27}L_{uu\ ijjj}^{V8,LR} - \frac{232}{9}L_{uu\ ijii}^{V,LL} \\
& - \frac{232}{9}L_{uu\ ijjj}^{V,LL} \Big] + \alpha_s \alpha \Bigg[ -\frac{32}{9}L_{ud\ ij11}^{V1,LL} - \frac{32}{9}L_{ud\ ij22}^{V1,LL} - \frac{32}{9}L_{ud\ ij33}^{V1,LL} - \frac{32}{9}L_{ud\ ij11}^{V1,LR} \\
& - \frac{32}{9}L_{ud\ ij22}^{V1,LR} - \frac{32}{9}L_{ud\ ij33}^{V1,LR} - \frac{656}{729}L_{ud\ ij11}^{V8,LL} - \frac{656}{729}L_{ud\ ij22}^{V8,LL} - \frac{656}{729}L_{ud\ ij33}^{V8,LL} + \frac{784}{729}L_{ud\ ij11}^{V8,LR} \\
& + \frac{784}{729}L_{ud\ ij22}^{V8,LR} + \frac{784}{729}L_{ud\ ij33}^{V8,LR} + \frac{448}{9}L_{uu\ ijii}^{V1,LR} + \frac{64}{9}L_{uu\ ijjj}^{V1,LR} - \frac{4832}{729}L_{uu\ ijii}^{V8,LR}
\end{aligned}$$

$$\begin{aligned}
& -\frac{3968}{729}L_{ijj}^{V8,LR} + \frac{4480}{243}L_{ijj}^{V,LL} + \frac{4480}{243}L_{ijj}^{V,LL} \Big] + \alpha^2 \Big[ -\frac{8344}{729}L_{11ij}^{V,LL} - \frac{8344}{729}L_{22ij}^{V,LL} \\
& -\frac{8344}{729}L_{33ij}^{V,LL} - \frac{3736}{729}L_{ij11}^{V1,LL} - \frac{3736}{729}L_{ij22}^{V1,LL} - \frac{3736}{729}L_{ij33}^{V1,LL} - \frac{2584}{729}L_{ij11}^{V1,LR} \\
& -\frac{2584}{729}L_{ij22}^{V1,LR} - \frac{2584}{729}L_{ij33}^{V1,LR} - \frac{4888}{729}L_{ij11}^{V,LR} - \frac{4888}{729}L_{ij22}^{V,LR} - \frac{4888}{729}L_{ij33}^{V,LR} \\
& + \frac{72416}{729}L_{ijj}^{V1,LR} + \frac{4736}{729}L_{ijj}^{V1,LR} - \frac{9728}{729}L_{ijj}^{V,LL} - \frac{9728}{729}L_{ijj}^{V,LL} \Big] ; \\
\dot{L}_{ijj}^{V8,LR} &= g_s^2 \Big[ \frac{2}{3}L_{ij11}^{V8,LL} + \frac{2}{3}L_{ij22}^{V8,LL} + \frac{2}{3}L_{ij33}^{V8,LL} + \frac{2}{3}L_{ij11}^{V8,LR} + \frac{2}{3}L_{ij22}^{V8,LR} \\
& + \frac{2}{3}L_{ij33}^{V8,LR} - 12L_{ijj}^{V1,LR} - \frac{40}{3}L_{ijj}^{V8,LR} + \frac{2}{3}L_{ijj}^{V8,LR} + \frac{8}{3}L_{ijj}^{V,LL} + \frac{8}{3}L_{ijj}^{V,LL} \Big] \\
& - \frac{16}{3}e^2L_{ijj}^{V8,LR} + \alpha_s^2 \Big[ -\frac{2}{3}L_{ij11}^{V1,LL} - \frac{2}{3}L_{ij22}^{V1,LL} - \frac{2}{3}L_{ij33}^{V1,LL} - \frac{22}{3}L_{ij11}^{V1,LR} \\
& - \frac{22}{3}L_{ij22}^{V1,LR} - \frac{22}{3}L_{ij33}^{V1,LR} + \frac{619}{81}L_{ij11}^{V8,LL} + \frac{619}{81}L_{ij22}^{V8,LL} + \frac{619}{81}L_{ij33}^{V8,LL} + \frac{799}{81}L_{ij11}^{V8,LR} \\
& + \frac{799}{81}L_{ij22}^{V8,LR} + \frac{799}{81}L_{ij33}^{V8,LR} - 132L_{ijj}^{V1,LR} - \frac{22}{3}L_{ijj}^{V1,LR} - \frac{25177}{162}L_{ijj}^{V8,LR} + \frac{799}{81}L_{ijj}^{V8,LR} \\
& + \frac{1210}{27}L_{ijj}^{V,LL} + \frac{1210}{27}L_{ijj}^{V,LL} \Big] + \alpha_s \alpha \Big[ -\frac{520}{81}L_{11ij}^{V,LL} - \frac{520}{81}L_{22ij}^{V,LL} - \frac{520}{81}L_{33ij}^{V,LL} \\
& - \frac{520}{81}L_{ij11}^{V1,LL} - \frac{520}{81}L_{ij22}^{V1,LL} - \frac{520}{81}L_{ij33}^{V1,LL} - \frac{520}{81}L_{ij11}^{V1,LR} - \frac{520}{81}L_{ij22}^{V1,LR} - \frac{520}{81}L_{ij33}^{V1,LR} \\
& + \frac{170}{27}L_{ij11}^{V8,LL} + \frac{170}{27}L_{ij22}^{V8,LL} + \frac{170}{27}L_{ij33}^{V8,LL} + \frac{22}{9}L_{ij11}^{V8,LR} + \frac{22}{9}L_{ij22}^{V8,LR} + \frac{22}{9}L_{ij33}^{V8,LR} \\
& - \frac{520}{81}L_{ij11}^{V,LR} - \frac{520}{81}L_{ij22}^{V,LR} - \frac{520}{81}L_{ij33}^{V,LR} + \frac{608}{81}L_{ijj}^{V1,LR} + \frac{1040}{81}L_{ijj}^{V1,LR} - \frac{16}{3}L_{ijj}^{V8,LR} \\
& + \frac{56}{9}L_{ijj}^{V8,LR} + \frac{1168}{81}L_{ijj}^{V,LL} + \frac{1168}{81}L_{ijj}^{V,LL} \Big] + \frac{7520}{81}\alpha^2L_{ijj}^{V8,LR} ; \\
\dot{L}_{11ij}^{S,RL} &= -8g_s^2L_{11ij}^{S,RL} - \frac{26}{3}e^2L_{11ij}^{S,RL} - \frac{1012}{9}\alpha_s^2L_{11ij}^{S,RL} - \frac{32}{9}\alpha_s\alpha L_{11ij}^{S,RL} \\
& + \frac{445}{81}\alpha^2L_{11ij}^{S,RL} ;
\end{aligned}$$

$$\begin{aligned}\dot{L}_{22ij}^{S,RL} &= -8g_s^2 L_{22ij}^{S,RL} - \frac{26}{3} e^2 L_{22ij}^{S,RL} - \frac{1012}{9} \alpha_s^2 L_{22ij}^{S,RL} - \frac{32}{9} \alpha_s \alpha L_{22ij}^{S,RL} \\ &\quad + \frac{445}{81} \alpha^2 L_{22ij}^{S,RL} ;\end{aligned}$$

$$\begin{aligned}\dot{L}_{33ij}^{S,RL} &= -8g_s^2 L_{33ij}^{S,RL} - \frac{26}{3} e^2 L_{33ij}^{S,RL} - \frac{1012}{9} \alpha_s^2 L_{33ij}^{S,RL} - \frac{32}{9} \alpha_s \alpha L_{33ij}^{S,RL} \\ &\quad + \frac{445}{81} \alpha^2 L_{33ij}^{S,RL} ;\end{aligned}$$

$$\begin{aligned}\dot{L}_{i11j}^{V1,LR} &= -\frac{8}{3} g_s^2 L_{i11j}^{V8,LR} - \frac{10}{3} e^2 L_{i11j}^{V1,LR} + \alpha_s^2 \left[ -\frac{28}{3} L_{i11j}^{V1,LR} - \frac{2044}{27} L_{i11j}^{V8,LR} \right] \\ &\quad + \alpha_s \alpha \left[ \frac{8}{3} L_{i11j}^{V1,LR} - \frac{128}{27} L_{i11j}^{V8,LR} \right] + \frac{173}{81} \alpha^2 L_{i11j}^{V1,LR} ;\end{aligned}$$

$$\begin{aligned}\dot{L}_{i11j}^{V8,LR} &= g_s^2 \left[ -12 L_{i11j}^{V1,LR} - 14 L_{i11j}^{V8,LR} \right] - \frac{10}{3} e^2 L_{i11j}^{V8,LR} + \alpha_s^2 \left[ -\frac{374}{3} L_{i11j}^{V1,LR} \right. \\ &\quad \left. - \frac{2975}{18} L_{i11j}^{V8,LR} \right] + \alpha_s \alpha \left[ \frac{16}{9} L_{i11j}^{V8,LR} - \frac{64}{3} L_{i11j}^{V1,LR} \right] + \frac{173}{81} \alpha^2 L_{i11j}^{V8,LR} ;\end{aligned}$$

$$\begin{aligned}\dot{L}_{i22j}^{V1,LR} &= -\frac{8}{3} g_s^2 L_{i22j}^{V8,LR} - \frac{10}{3} e^2 L_{i22j}^{V1,LR} + \alpha_s^2 \left[ -\frac{28}{3} L_{i22j}^{V1,LR} - \frac{2044}{27} L_{i22j}^{V8,LR} \right] \\ &\quad + \alpha_s \alpha \left[ \frac{8}{3} L_{i22j}^{V1,LR} - \frac{128}{27} L_{i22j}^{V8,LR} \right] + \frac{173}{81} \alpha^2 L_{i22j}^{V1,LR} ;\end{aligned}$$

$$\begin{aligned}\dot{L}_{i22j}^{V8,LR} &= g_s^2 \left[ -12 L_{i22j}^{V1,LR} - 14 L_{i22j}^{V8,LR} \right] - \frac{10}{3} e^2 L_{i22j}^{V8,LR} + \alpha_s^2 \left[ -\frac{374}{3} L_{i22j}^{V1,LR} \right. \\ &\quad \left. - \frac{2975}{18} L_{i22j}^{V8,LR} \right] + \alpha_s \alpha \left[ \frac{16}{9} L_{i22j}^{V8,LR} - \frac{64}{3} L_{i22j}^{V1,LR} \right] + \frac{173}{81} \alpha^2 L_{i22j}^{V8,LR} ;\end{aligned}$$

$$\begin{aligned}\dot{L}_{i33j}^{V1,LR} &= -\frac{8}{3} g_s^2 L_{i33j}^{V8,LR} - \frac{10}{3} e^2 L_{i33j}^{V1,LR} + \alpha_s^2 \left[ -\frac{28}{3} L_{i33j}^{V1,LR} - \frac{2044}{27} L_{i33j}^{V8,LR} \right] \\ &\quad + \alpha_s \alpha \left[ \frac{8}{3} L_{i33j}^{V1,LR} - \frac{128}{27} L_{i33j}^{V8,LR} \right] + \frac{173}{81} \alpha^2 L_{i33j}^{V1,LR} ;\end{aligned}$$

$$\begin{aligned}\dot{L}_{i33j}^{V8,LR} &= g_s^2 \left[ -12 L_{i33j}^{V1,LR} - 14 L_{i33j}^{V8,LR} \right] - \frac{10}{3} e^2 L_{i33j}^{V8,LR} + \alpha_s^2 \left[ -\frac{374}{3} L_{i33j}^{V1,LR} \right. \\ &\quad \left. - \frac{2975}{18} L_{i33j}^{V8,LR} \right] + \alpha_s \alpha \left[ \frac{16}{9} L_{i33j}^{V8,LR} - \frac{64}{3} L_{i33j}^{V1,LR} \right] + \frac{173}{81} \alpha^2 L_{i33j}^{V8,LR} ;\end{aligned}$$

$$\begin{aligned}
& -\frac{2975}{18}L_{i33j}^{V8,LR} \Big] + \alpha_s \alpha \left[ \frac{16}{9}L_{i33j}^{V8,LR} - \frac{64}{3}L_{i33j}^{V1,LR} \right] + \frac{173}{81}\alpha^2 L_{i33j}^{V8,LR} ; \\
\dot{L}_{11ij}^{S,RR} &= -8g_s^2 L_{11ij}^{S,RR} + e^2 \left[ 64L_{11ij}^{T,RR} - \frac{26}{3}L_{11ij}^{S,RR} \right] - \frac{1012}{9}\alpha_s^2 L_{11ij}^{S,RR} \\
&+ \alpha_s \alpha \left[ -\frac{32}{9}L_{11ij}^{S,RR} - \frac{3584}{9}L_{11ij}^{T,RR} \right] + \alpha^2 \left[ -\frac{2579}{81}L_{11ij}^{S,RR} - \frac{35200}{27}L_{11ij}^{T,RR} \right] ; \\
\dot{L}_{11ij}^{T,RR} &= \frac{8}{3}g_s^2 L_{11ij}^{T,RR} + e^2 \left[ \frac{4}{3}L_{11ij}^{S,RR} + \frac{26}{9}L_{11ij}^{T,RR} \right] + \frac{1652}{27}\alpha_s^2 L_{11ij}^{T,RR} \\
&+ \alpha_s \alpha \left[ -\frac{32}{3}L_{11ij}^{S,RR} - \frac{608}{27}L_{11ij}^{T,RR} \right] + \alpha^2 \left[ -\frac{1384}{81}L_{11ij}^{S,RR} - \frac{21929}{243}L_{11ij}^{T,RR} \right] ; \\
\dot{L}_{22ij}^{S,RR} &= -8g_s^2 L_{22ij}^{S,RR} + e^2 \left[ 64L_{22ij}^{T,RR} - \frac{26}{3}L_{22ij}^{S,RR} \right] - \frac{1012}{9}\alpha_s^2 L_{22ij}^{S,RR} \\
&+ \alpha_s \alpha \left[ -\frac{32}{9}L_{22ij}^{S,RR} - \frac{3584}{9}L_{22ij}^{T,RR} \right] + \alpha^2 \left[ -\frac{2579}{81}L_{22ij}^{S,RR} - \frac{35200}{27}L_{22ij}^{T,RR} \right] ; \\
\dot{L}_{22ij}^{T,RR} &= \frac{8}{3}g_s^2 L_{22ij}^{T,RR} + e^2 \left[ \frac{4}{3}L_{22ij}^{S,RR} + \frac{26}{9}L_{22ij}^{T,RR} \right] + \frac{1652}{27}\alpha_s^2 L_{22ij}^{T,RR} \\
&+ \alpha_s \alpha \left[ -\frac{32}{3}L_{22ij}^{S,RR} - \frac{608}{27}L_{22ij}^{T,RR} \right] + \alpha^2 \left[ -\frac{1384}{81}L_{22ij}^{S,RR} - \frac{21929}{243}L_{22ij}^{T,RR} \right] ; \\
\dot{L}_{33ij}^{S,RR} &= -8g_s^2 L_{33ij}^{S,RR} + e^2 \left[ 64L_{33ij}^{T,RR} - \frac{26}{3}L_{33ij}^{S,RR} \right] - \frac{1012}{9}\alpha_s^2 L_{33ij}^{S,RR} \\
&+ \alpha_s \alpha \left[ -\frac{32}{9}L_{33ij}^{S,RR} - \frac{3584}{9}L_{33ij}^{T,RR} \right] + \alpha^2 \left[ -\frac{2579}{81}L_{33ij}^{S,RR} - \frac{35200}{27}L_{33ij}^{T,RR} \right] ; \\
\dot{L}_{33ij}^{T,RR} &= \frac{8}{3}g_s^2 L_{33ij}^{T,RR} + e^2 \left[ \frac{4}{3}L_{33ij}^{S,RR} + \frac{26}{9}L_{33ij}^{T,RR} \right] + \frac{1652}{27}\alpha_s^2 L_{33ij}^{T,RR} \\
&+ \alpha_s \alpha \left[ -\frac{32}{3}L_{33ij}^{S,RR} - \frac{608}{27}L_{33ij}^{T,RR} \right] + \alpha^2 \left[ -\frac{1384}{81}L_{33ij}^{S,RR} - \frac{21929}{243}L_{33ij}^{T,RR} \right] ; \\
\dot{L}_{ij11}^{S1,RR} &= g_s^2 \left[ \frac{64}{9}L_{i11j}^{S1,RR} + \frac{112}{27}L_{i11j}^{S8,RR} - 16L_{ij11}^{S1,RR} + \frac{16}{9}L_{ij11}^{S8,RR} \right]
\end{aligned}$$

$$\begin{aligned}
& + e^2 \left[ \frac{4}{27} L_{i11j}^{S1,RR} + \frac{16}{81} L_{i11j}^{S8,RR} - \frac{46}{9} L_{ij11}^{S1,RR} \right] + \alpha_s^2 \left[ \frac{9472}{81} L_{i11j}^{S1,RR} + \frac{16576}{243} L_{i11j}^{S8,RR} \right. \\
& - \frac{2120}{9} L_{ij11}^{S1,RR} + \frac{928}{81} L_{ij11}^{S8,RR} \left. \right] + \alpha_s \alpha \left[ \frac{1888}{81} L_{i11j}^{S1,RR} + \frac{3808}{243} L_{i11j}^{S8,RR} + \frac{136}{27} L_{ij11}^{S1,RR} \right. \\
& + \frac{224}{81} L_{ij11}^{S8,RR} \left. \right] + \alpha^2 \left[ \frac{98}{729} L_{i11j}^{S1,RR} + \frac{392}{2187} L_{i11j}^{S8,RR} + \frac{6391}{243} L_{ij11}^{S1,RR} \right] ; \\
\dot{L}_{ij11}^{S8,RR} & = g_s^2 \left[ -\frac{16}{3} L_{i11j}^{S1,RR} + \frac{44}{9} L_{i11j}^{S8,RR} + 8 L_{ij11}^{S1,RR} + \frac{16}{3} L_{ij11}^{S8,RR} \right] \\
& + e^2 \left[ \frac{8}{9} L_{i11j}^{S1,RR} - \frac{4}{27} L_{i11j}^{S8,RR} - \frac{46}{9} L_{ij11}^{S8,RR} \right] + \alpha_s^2 \left[ -\frac{856}{27} L_{i11j}^{S1,RR} - \frac{2506}{81} L_{i11j}^{S8,RR} \right. \\
& + \frac{248}{9} L_{ij11}^{S1,RR} + \frac{2995}{27} L_{ij11}^{S8,RR} \left. \right] + \alpha_s \alpha \left[ -\frac{868}{27} L_{i11j}^{S1,RR} + \frac{1370}{81} L_{i11j}^{S8,RR} + \frac{112}{9} L_{ij11}^{S1,RR} \right. \\
& + \frac{224}{9} L_{ij11}^{S8,RR} \left. \right] + \alpha^2 \left[ \frac{196}{243} L_{i11j}^{S1,RR} - \frac{98}{729} L_{i11j}^{S8,RR} + \frac{6391}{243} L_{ij11}^{S8,RR} \right] ; \\
\dot{L}_{i11j}^{S1,RR} & = g_s^2 \left[ -16 L_{i11j}^{S1,RR} + \frac{16}{9} L_{i11j}^{S8,RR} + \frac{64}{9} L_{ij11}^{S1,RR} + \frac{112}{27} L_{ij11}^{S8,RR} \right] \\
& + e^2 \left[ \frac{26}{9} L_{i11j}^{S1,RR} - \frac{32}{27} L_{ij11}^{S1,RR} - \frac{128}{81} L_{ij11}^{S8,RR} \right] + \alpha_s^2 \left[ -\frac{2120}{9} L_{i11j}^{S1,RR} + \frac{928}{81} L_{i11j}^{S8,RR} \right. \\
& + \frac{9472}{81} L_{ij11}^{S1,RR} + \frac{16576}{243} L_{ij11}^{S8,RR} \left. \right] + \alpha_s \alpha \left[ \frac{712}{27} L_{i11j}^{S1,RR} - \frac{64}{81} L_{i11j}^{S8,RR} - \frac{2144}{81} L_{ij11}^{S1,RR} \right. \\
& - \frac{7784}{243} L_{ij11}^{S8,RR} \left. \right] + \alpha^2 \left[ -\frac{13769}{243} L_{i11j}^{S1,RR} + \frac{5264}{729} L_{ij11}^{S1,RR} + \frac{21056}{2187} L_{ij11}^{S8,RR} \right] ; \\
\dot{L}_{i11j}^{S8,RR} & = g_s^2 \left[ 8 L_{i11j}^{S1,RR} + \frac{16}{3} L_{i11j}^{S8,RR} - \frac{16}{3} L_{ij11}^{S1,RR} + \frac{44}{9} L_{ij11}^{S8,RR} \right] \\
& + e^2 \left[ \frac{26}{9} L_{i11j}^{S8,RR} - \frac{64}{9} L_{ij11}^{S1,RR} + \frac{32}{27} L_{ij11}^{S8,RR} \right] + \alpha_s^2 \left[ \frac{248}{9} L_{i11j}^{S1,RR} + \frac{2995}{27} L_{i11j}^{S8,RR} \right. \\
& - \frac{856}{27} L_{ij11}^{S1,RR} - \frac{2506}{81} L_{ij11}^{S8,RR} \left. \right] + \alpha_s \alpha \left[ -\frac{32}{9} L_{i11j}^{S1,RR} - \frac{400}{9} L_{i11j}^{S8,RR} + \frac{3704}{27} L_{ij11}^{S1,RR} \right.
\end{aligned}$$

$$\begin{aligned}
& -\frac{2050}{81}L_{ij11}^{S8,RR} \Big] + \alpha^2 \Big[ -\frac{13769}{243}L_{i11j}^{S8,RR} + \frac{10528}{243}L_{ij11}^{S1,RR} - \frac{5264}{729}L_{ij11}^{S8,RR} \Big] ; \\
\dot{L}_{ij22}^{S1,RR} &= g_s^2 \Big[ \frac{64}{9}L_{i22j}^{S1,RR} + \frac{112}{27}L_{i22j}^{S8,RR} - 16L_{ij22}^{S1,RR} + \frac{16}{9}L_{ij22}^{S8,RR} \Big] \\
&+ e^2 \Big[ \frac{4}{27}L_{i22j}^{S1,RR} + \frac{16}{81}L_{i22j}^{S8,RR} - \frac{46}{9}L_{ij22}^{S1,RR} \Big] + \alpha_s^2 \Big[ \frac{9472}{81}L_{i22j}^{S1,RR} + \frac{16576}{243}L_{i22j}^{S8,RR} \\
&- \frac{2120}{9}L_{ij22}^{S1,RR} + \frac{928}{81}L_{ij22}^{S8,RR} \Big] + \alpha_s \alpha \Big[ \frac{1888}{81}L_{i22j}^{S1,RR} + \frac{3808}{243}L_{i22j}^{S8,RR} + \frac{136}{27}L_{ij22}^{S1,RR} \\
&+ \frac{224}{81}L_{ij22}^{S8,RR} \Big] + \alpha^2 \Big[ \frac{98}{729}L_{i22j}^{S1,RR} + \frac{392}{2187}L_{i22j}^{S8,RR} + \frac{6391}{243}L_{ij22}^{S1,RR} \Big] ; \\
\dot{L}_{ij22}^{S8,RR} &= g_s^2 \Big[ -\frac{16}{3}L_{i22j}^{S1,RR} + \frac{44}{9}L_{i22j}^{S8,RR} + 8L_{ij22}^{S1,RR} + \frac{16}{3}L_{ij22}^{S8,RR} \Big] \\
&+ e^2 \Big[ \frac{8}{9}L_{i22j}^{S1,RR} - \frac{4}{27}L_{i22j}^{S8,RR} - \frac{46}{9}L_{ij22}^{S8,RR} \Big] + \alpha_s^2 \Big[ -\frac{856}{27}L_{i22j}^{S1,RR} - \frac{2506}{81}L_{i22j}^{S8,RR} \\
&+ \frac{248}{9}L_{ij22}^{S1,RR} + \frac{2995}{27}L_{ij22}^{S8,RR} \Big] + \alpha_s \alpha \Big[ -\frac{868}{27}L_{i22j}^{S1,RR} + \frac{1370}{81}L_{i22j}^{S8,RR} + \frac{112}{9}L_{ij22}^{S1,RR} \\
&+ \frac{224}{9}L_{ij22}^{S8,RR} \Big] + \alpha^2 \Big[ \frac{196}{243}L_{i22j}^{S1,RR} - \frac{98}{729}L_{i22j}^{S8,RR} + \frac{6391}{243}L_{ij22}^{S8,RR} \Big] ; \\
\dot{L}_{i22j}^{S1,RR} &= g_s^2 \Big[ -16L_{i22j}^{S1,RR} + \frac{16}{9}L_{i22j}^{S8,RR} + \frac{64}{9}L_{ij22}^{S1,RR} + \frac{112}{27}L_{ij22}^{S8,RR} \Big] \\
&+ e^2 \Big[ \frac{26}{9}L_{i22j}^{S1,RR} - \frac{32}{27}L_{ij22}^{S1,RR} - \frac{128}{81}L_{ij22}^{S8,RR} \Big] + \alpha_s^2 \Big[ -\frac{2120}{9}L_{i22j}^{S1,RR} + \frac{928}{81}L_{i22j}^{S8,RR} \\
&+ \frac{9472}{81}L_{ij22}^{S1,RR} + \frac{16576}{243}L_{ij22}^{S8,RR} \Big] + \alpha_s \alpha \Big[ \frac{712}{27}L_{i22j}^{S1,RR} - \frac{64}{81}L_{i22j}^{S8,RR} - \frac{2144}{81}L_{ij22}^{S1,RR} \\
&- \frac{7784}{243}L_{ij22}^{S8,RR} \Big] + \alpha^2 \Big[ -\frac{13769}{243}L_{i22j}^{S1,RR} + \frac{5264}{729}L_{ij22}^{S1,RR} + \frac{21056}{2187}L_{ij22}^{S8,RR} \Big] ; \\
\dot{L}_{i22j}^{S8,RR} &= g_s^2 \Big[ 8L_{i22j}^{S1,RR} + \frac{16}{3}L_{i22j}^{S8,RR} - \frac{16}{3}L_{ij22}^{S1,RR} + \frac{44}{9}L_{ij22}^{S8,RR} \Big]
\end{aligned}$$

$$\begin{aligned}
& + e^2 \left[ \frac{26}{9} L_{i22j}^{S8,RR} - \frac{64}{9} L_{ij22}^{S1,RR} + \frac{32}{27} L_{ij22}^{S8,RR} \right] + \alpha_s^2 \left[ \frac{248}{9} L_{i22j}^{S1,RR} + \frac{2995}{27} L_{i22j}^{S8,RR} \right. \\
& \quad \left. - \frac{856}{27} L_{ij22}^{S1,RR} - \frac{2506}{81} L_{ij22}^{S8,RR} \right] + \alpha_s \alpha \left[ - \frac{32}{9} L_{i22j}^{S1,RR} - \frac{400}{9} L_{i22j}^{S8,RR} + \frac{3704}{27} L_{ij22}^{S1,RR} \right. \\
& \quad \left. - \frac{2050}{81} L_{ij22}^{S8,RR} \right] + \alpha^2 \left[ - \frac{13769}{243} L_{i22j}^{S8,RR} + \frac{10528}{243} L_{ij22}^{S1,RR} - \frac{5264}{729} L_{ij22}^{S8,RR} \right] ; \\
\dot{L}_{ij33}^{S1,RR} & = g_s^2 \left[ \frac{64}{9} L_{i33j}^{S1,RR} + \frac{112}{27} L_{i33j}^{S8,RR} - 16 L_{ij33}^{S1,RR} + \frac{16}{9} L_{ij33}^{S8,RR} \right] \\
& + e^2 \left[ \frac{4}{27} L_{i33j}^{S1,RR} + \frac{16}{81} L_{i33j}^{S8,RR} - \frac{46}{9} L_{ij33}^{S1,RR} \right] + \alpha_s^2 \left[ \frac{9472}{81} L_{i33j}^{S1,RR} + \frac{16576}{243} L_{i33j}^{S8,RR} \right. \\
& \quad \left. - \frac{2120}{9} L_{ij33}^{S1,RR} + \frac{928}{81} L_{ij33}^{S8,RR} \right] + \alpha_s \alpha \left[ \frac{1888}{81} L_{i33j}^{S1,RR} + \frac{3808}{243} L_{i33j}^{S8,RR} + \frac{136}{27} L_{ij33}^{S1,RR} \right. \\
& \quad \left. + \frac{224}{81} L_{ij33}^{S8,RR} \right] + \alpha^2 \left[ \frac{98}{729} L_{i33j}^{S1,RR} + \frac{392}{2187} L_{i33j}^{S8,RR} + \frac{6391}{243} L_{ij33}^{S1,RR} \right] ; \\
\dot{L}_{ij33}^{S8,RR} & = g_s^2 \left[ - \frac{16}{3} L_{i33j}^{S1,RR} + \frac{44}{9} L_{i33j}^{S8,RR} + 8 L_{ij33}^{S1,RR} + \frac{16}{3} L_{ij33}^{S8,RR} \right] \\
& + e^2 \left[ \frac{8}{9} L_{i33j}^{S1,RR} - \frac{4}{27} L_{i33j}^{S8,RR} - \frac{46}{9} L_{ij33}^{S8,RR} \right] + \alpha_s^2 \left[ - \frac{856}{27} L_{i33j}^{S1,RR} - \frac{2506}{81} L_{i33j}^{S8,RR} \right. \\
& \quad \left. + \frac{248}{9} L_{ij33}^{S1,RR} + \frac{2995}{27} L_{ij33}^{S8,RR} \right] + \alpha_s \alpha \left[ - \frac{868}{27} L_{i33j}^{S1,RR} + \frac{1370}{81} L_{i33j}^{S8,RR} + \frac{112}{9} L_{ij33}^{S1,RR} \right. \\
& \quad \left. + \frac{224}{9} L_{ij33}^{S8,RR} \right] + \alpha^2 \left[ \frac{196}{243} L_{i33j}^{S1,RR} - \frac{98}{729} L_{i33j}^{S8,RR} + \frac{6391}{243} L_{ij33}^{S8,RR} \right] ; \\
\dot{L}_{i33j}^{S1,RR} & = g_s^2 \left[ - 16 L_{i33j}^{S1,RR} + \frac{16}{9} L_{i33j}^{S8,RR} + \frac{64}{9} L_{ij33}^{S1,RR} + \frac{112}{27} L_{ij33}^{S8,RR} \right] \\
& + e^2 \left[ \frac{26}{9} L_{i33j}^{S1,RR} - \frac{32}{27} L_{ij33}^{S1,RR} - \frac{128}{81} L_{ij33}^{S8,RR} \right] + \alpha_s^2 \left[ - \frac{2120}{9} L_{i33j}^{S1,RR} + \frac{928}{81} L_{i33j}^{S8,RR} \right. \\
& \quad \left. + \frac{9472}{81} L_{ij33}^{S1,RR} + \frac{16576}{243} L_{ij33}^{S8,RR} \right] + \alpha_s \alpha \left[ \frac{712}{27} L_{i33j}^{S1,RR} - \frac{64}{81} L_{i33j}^{S8,RR} - \frac{2144}{81} L_{ij33}^{S1,RR} \right.
\end{aligned}$$

$$\begin{aligned}
& -\frac{7784}{243}L_{ij33}^{S8,RR} \Big] + \alpha^2 \Big[ -\frac{13769}{243}L_{ij33}^{S1,RR} + \frac{5264}{729}L_{ij33}^{S1,RR} + \frac{21056}{2187}L_{ij33}^{S8,RR} \Big] ; \\
\dot{L}_{i33j}^{S8,RR} &= g_s^2 \Big[ 8L_{i33j}^{S1,RR} + \frac{16}{3}L_{i33j}^{S8,RR} - \frac{16}{3}L_{ij33}^{S1,RR} + \frac{44}{9}L_{ij33}^{S8,RR} \Big] \\
&+ e^2 \Big[ \frac{26}{9}L_{i33j}^{S8,RR} - \frac{64}{9}L_{ij33}^{S1,RR} + \frac{32}{27}L_{ij33}^{S8,RR} \Big] + \alpha_s^2 \Big[ \frac{248}{9}L_{i33j}^{S1,RR} + \frac{2995}{27}L_{i33j}^{S8,RR} \\
&- \frac{856}{27}L_{ij33}^{S1,RR} - \frac{2506}{81}L_{ij33}^{S8,RR} \Big] + \alpha_s \alpha \Big[ -\frac{32}{9}L_{i33j}^{S1,RR} - \frac{400}{9}L_{i33j}^{S8,RR} + \frac{3704}{27}L_{ij33}^{S1,RR} \\
&- \frac{2050}{81}L_{ij33}^{S8,RR} \Big] + \alpha^2 \Big[ -\frac{13769}{243}L_{i33j}^{S8,RR} + \frac{10528}{243}L_{ij33}^{S1,RR} - \frac{5264}{729}L_{ij33}^{S8,RR} \Big] ; \\
\dot{L}_{ijj}^{S1,RR} &= g_s^2 \Big[ \frac{160}{27}L_{ijj}^{S8,RR} - \frac{80}{9}L_{ijj}^{S1,RR} \Big] + e^2 \Big[ \frac{16}{27}L_{ijj}^{S1,RR} + \frac{256}{81}L_{ijj}^{S8,RR} \Big] \\
&+ \alpha_s^2 \Big[ \frac{19360}{243}L_{ijj}^{S8,RR} - \frac{9608}{81}L_{ijj}^{S1,RR} \Big] + \alpha_s \alpha \Big[ \frac{1408}{243}L_{ijj}^{S8,RR} - \frac{4160}{81}L_{ijj}^{S1,RR} \Big] \\
&+ \alpha^2 \Big[ \frac{6944}{729}L_{ijj}^{S1,RR} - \frac{22528}{2187}L_{ijj}^{S8,RR} \Big] ; \\
\dot{L}_{ijj}^{S8,RR} &= g_s^2 \Big[ \frac{8}{3}L_{ijj}^{S1,RR} + \frac{92}{9}L_{ijj}^{S8,RR} \Big] + e^2 \Big[ \frac{128}{9}L_{ijj}^{S1,RR} - \frac{112}{27}L_{ijj}^{S8,RR} \Big] \\
&+ \alpha_s^2 \Big[ \frac{6479}{81}L_{ijj}^{S8,RR} - \frac{112}{27}L_{ijj}^{S1,RR} \Big] + \alpha_s \alpha \Big[ -\frac{7360}{27}L_{ijj}^{S1,RR} - \frac{832}{81}L_{ijj}^{S8,RR} \Big] \\
&+ \alpha^2 \Big[ \frac{18208}{729}L_{ijj}^{S8,RR} - \frac{11264}{243}L_{ijj}^{S1,RR} \Big] ; \\
\dot{L}_{ijii}^{S1,RR} &= g_s^2 \Big[ \frac{160}{27}L_{ijii}^{S8,RR} - \frac{80}{9}L_{ijii}^{S1,RR} \Big] + e^2 \Big[ \frac{16}{27}L_{ijii}^{S1,RR} + \frac{256}{81}L_{ijii}^{S8,RR} \Big] \\
&+ \alpha_s^2 \Big[ \frac{19360}{243}L_{ijii}^{S8,RR} - \frac{9608}{81}L_{ijii}^{S1,RR} \Big] + \alpha_s \alpha \Big[ \frac{1408}{243}L_{ijii}^{S8,RR} - \frac{4160}{81}L_{ijii}^{S1,RR} \Big] \\
&+ \alpha^2 \Big[ \frac{6944}{729}L_{ijii}^{S1,RR} - \frac{22528}{2187}L_{ijii}^{S8,RR} \Big] ;
\end{aligned}$$



$$\begin{aligned}
\dot{L}_{uu}^{S8,RR}{}_{ij\bar{i}} &= g_s^2 \left[ \frac{8}{3} L_{uu}^{S1,RR}{}_{ij\bar{i}} + \frac{92}{9} L_{uu}^{S8,RR}{}_{ij\bar{i}} \right] + e^2 \left[ \frac{128}{9} L_{uu}^{S1,RR}{}_{ij\bar{i}} - \frac{112}{27} L_{uu}^{S8,RR}{}_{ij\bar{i}} \right] \\
&+ \alpha_s^2 \left[ \frac{6479}{81} L_{uu}^{S8,RR}{}_{ij\bar{i}} - \frac{112}{27} L_{uu}^{S1,RR}{}_{ij\bar{i}} \right] + \alpha_s \alpha \left[ -\frac{7360}{27} L_{uu}^{S1,RR}{}_{ij\bar{i}} - \frac{832}{81} L_{uu}^{S8,RR}{}_{ij\bar{i}} \right] \\
&+ \alpha^2 \left[ \frac{18208}{729} L_{uu}^{S8,RR}{}_{ij\bar{i}} - \frac{11264}{243} L_{uu}^{S1,RR}{}_{ij\bar{i}} \right] ; \\
\dot{L}_{eu}^{V,RR}{}_{11ij} &= e^2 \left[ \frac{4}{3} L_{du}^{V1,LR}{}_{11ij} + \frac{4}{3} L_{du}^{V1,LR}{}_{22ij} + \frac{4}{3} L_{du}^{V1,LR}{}_{33ij} + \frac{4}{3} L_{eu}^{V,LR}{}_{11ij} + \frac{4}{3} L_{eu}^{V,LR}{}_{22ij} \right. \\
&+ \frac{4}{3} L_{eu}^{V,LR}{}_{33ij} - \frac{20}{3} L_{eu}^{V,RR}{}_{11ij} + \frac{4}{3} L_{eu}^{V,RR}{}_{22ij} + \frac{4}{3} L_{eu}^{V,RR}{}_{33ij} + \frac{4}{3} L_{ud}^{V1,RR}{}_{ij11} + \frac{4}{3} L_{ud}^{V1,RR}{}_{ij22} \\
&+ \frac{4}{3} L_{ud}^{V1,RR}{}_{ij33} - \frac{8}{3} L_{uu}^{V1,LR}{}_{ii\bar{j}} - \frac{8}{3} L_{uu}^{V1,LR}{}_{jj\bar{i}} - \frac{64}{9} L_{uu}^{V,RR}{}_{ij\bar{i}} - \frac{64}{9} L_{uu}^{V,RR}{}_{ij\bar{j}} \left. \right] + \alpha_s \alpha \left[ \frac{16}{3} L_{du}^{V1,LR}{}_{11ij} \right. \\
&+ \frac{16}{3} L_{du}^{V1,LR}{}_{22ij} + \frac{16}{3} L_{du}^{V1,LR}{}_{33ij} - \frac{392}{243} L_{du}^{V8,LR}{}_{11ij} - \frac{392}{243} L_{du}^{V8,LR}{}_{22ij} - \frac{392}{243} L_{du}^{V8,LR}{}_{33ij} + 32 L_{eu}^{V,RR}{}_{11ij} \\
&+ \frac{16}{3} L_{ud}^{V1,RR}{}_{ij11} + \frac{16}{3} L_{ud}^{V1,RR}{}_{ij22} + \frac{16}{3} L_{ud}^{V1,RR}{}_{ij33} + \frac{328}{243} L_{ud}^{V8,RR}{}_{ij11} + \frac{328}{243} L_{ud}^{V8,RR}{}_{ij22} + \frac{328}{243} L_{ud}^{V8,RR}{}_{ij33} \\
&- \frac{32}{3} L_{uu}^{V1,LR}{}_{ii\bar{j}} - \frac{32}{3} L_{uu}^{V1,LR}{}_{jj\bar{i}} + \frac{1984}{243} L_{uu}^{V8,LR}{}_{iii} + \frac{1984}{243} L_{uu}^{V8,LR}{}_{jjj} - \frac{2240}{81} L_{uu}^{V,RR}{}_{ij\bar{i}} - \frac{2240}{81} L_{uu}^{V,RR}{}_{ij\bar{j}} \left. \right] \\
&+ \alpha^2 \left[ -\frac{832}{243} L_{du}^{V1,LR}{}_{11ij} - \frac{832}{243} L_{du}^{V1,LR}{}_{22ij} - \frac{832}{243} L_{du}^{V1,LR}{}_{33ij} - \frac{328}{243} L_{eu}^{V,LR}{}_{11ij} - \frac{328}{243} L_{eu}^{V,LR}{}_{22ij} \right. \\
&- \frac{328}{243} L_{eu}^{V,LR}{}_{33ij} + \frac{4352}{243} L_{eu}^{V,RR}{}_{11ij} + \frac{3344}{243} L_{eu}^{V,RR}{}_{22ij} + \frac{3344}{243} L_{eu}^{V,RR}{}_{33ij} + \frac{392}{243} L_{ud}^{V1,RR}{}_{ij11} \\
&+ \frac{392}{243} L_{ud}^{V1,RR}{}_{ij22} + \frac{392}{243} L_{ud}^{V1,RR}{}_{ij33} - \frac{64}{243} L_{uu}^{V1,LR}{}_{ii\bar{j}} - \frac{64}{243} L_{uu}^{V1,LR}{}_{jj\bar{i}} + \frac{25888}{243} L_{uu}^{V,RR}{}_{ij\bar{i}} \\
&\left. + \frac{25888}{243} L_{uu}^{V,RR}{}_{ij\bar{j}} \right] ; \\
\dot{L}_{eu}^{V,RR}{}_{22ij} &= e^2 \left[ \frac{4}{3} L_{du}^{V1,LR}{}_{11ij} + \frac{4}{3} L_{du}^{V1,LR}{}_{22ij} + \frac{4}{3} L_{du}^{V1,LR}{}_{33ij} + \frac{4}{3} L_{eu}^{V,LR}{}_{11ij} + \frac{4}{3} L_{eu}^{V,LR}{}_{22ij} \right. \\
&+ \frac{4}{3} L_{eu}^{V,LR}{}_{33ij} + \frac{4}{3} L_{eu}^{V,RR}{}_{11ij} - \frac{20}{3} L_{eu}^{V,RR}{}_{22ij} + \frac{4}{3} L_{eu}^{V,RR}{}_{33ij} + \frac{4}{3} L_{ud}^{V1,RR}{}_{ij11} + \frac{4}{3} L_{ud}^{V1,RR}{}_{ij22} \\
&\left. + \frac{4}{3} L_{ud}^{V1,RR}{}_{ij33} - \frac{64}{243} L_{uu}^{V1,LR}{}_{ii\bar{j}} - \frac{64}{243} L_{uu}^{V1,LR}{}_{jj\bar{i}} + \frac{25888}{243} L_{uu}^{V,RR}{}_{ij\bar{i}} + \frac{25888}{243} L_{uu}^{V,RR}{}_{ij\bar{j}} \right] ;
\end{aligned}$$

$$\begin{aligned}
& + \frac{4}{3} L_{ij33}^{V1,RR} - \frac{8}{3} L_{iii}^{V1,LR} - \frac{8}{3} L_{jjij}^{V1,LR} - \frac{64}{9} L_{ijii}^{V,RR} - \frac{64}{9} L_{ijjj}^{V,RR} \Big] + \alpha_s \alpha \Big[ \frac{16}{3} L_{11ij}^{V1,LR} \\
& + \frac{16}{3} L_{du22ij}^{V1,LR} + \frac{16}{3} L_{du33ij}^{V1,LR} - \frac{392}{243} L_{du11ij}^{V8,LR} - \frac{392}{243} L_{du22ij}^{V8,LR} - \frac{392}{243} L_{du33ij}^{V8,LR} + 32 L_{22ij}^{V,RR} \\
& + \frac{16}{3} L_{udij11}^{V1,RR} + \frac{16}{3} L_{udij22}^{V1,RR} + \frac{16}{3} L_{udij33}^{V1,RR} + \frac{328}{243} L_{ij11}^{V8,RR} + \frac{328}{243} L_{ij22}^{V8,RR} + \frac{328}{243} L_{ij33}^{V8,RR} \\
& - \frac{32}{3} L_{uu}^{V1,LR} - \frac{32}{3} L_{jjij}^{V1,LR} + \frac{1984}{243} L_{uu}^{V8,LR} + \frac{1984}{243} L_{jjij}^{V8,LR} - \frac{2240}{81} L_{ijii}^{V,RR} - \frac{2240}{81} L_{ijjj}^{V,RR} \Big] \\
& + \alpha^2 \Big[ - \frac{832}{243} L_{du11ij}^{V1,LR} - \frac{832}{243} L_{du22ij}^{V1,LR} - \frac{832}{243} L_{du33ij}^{V1,LR} - \frac{328}{243} L_{11ij}^{V,LR} - \frac{328}{243} L_{22ij}^{V,LR} \\
& - \frac{328}{243} L_{33ij}^{V,LR} + \frac{3344}{243} L_{11ij}^{V,RR} + \frac{4352}{243} L_{22ij}^{V,RR} + \frac{3344}{243} L_{33ij}^{V,RR} + \frac{392}{243} L_{ij11}^{V1,RR} \\
& + \frac{392}{243} L_{ij22}^{V1,RR} + \frac{392}{243} L_{ij33}^{V1,RR} - \frac{64}{243} L_{uu}^{V1,LR} - \frac{64}{243} L_{jjij}^{V1,LR} + \frac{25888}{243} L_{ijii}^{V,RR} \\
& + \frac{25888}{243} L_{ijjj}^{V,RR} \Big] ;
\end{aligned}$$

$$\begin{aligned}
\dot{L}_{33ij}^{V,RR} & = e^2 \Big[ \frac{4}{3} L_{du11ij}^{V1,LR} + \frac{4}{3} L_{du22ij}^{V1,LR} + \frac{4}{3} L_{du33ij}^{V1,LR} + \frac{4}{3} L_{11ij}^{V,LR} + \frac{4}{3} L_{22ij}^{V,LR} \\
& + \frac{4}{3} L_{33ij}^{V,LR} + \frac{4}{3} L_{11ij}^{V,RR} + \frac{4}{3} L_{22ij}^{V,RR} - \frac{20}{3} L_{33ij}^{V,RR} + \frac{4}{3} L_{ij11}^{V1,RR} + \frac{4}{3} L_{ij22}^{V1,RR} \\
& + \frac{4}{3} L_{ij33}^{V1,RR} - \frac{8}{3} L_{iii}^{V1,LR} - \frac{8}{3} L_{jjij}^{V1,LR} - \frac{64}{9} L_{ijii}^{V,RR} - \frac{64}{9} L_{ijjj}^{V,RR} \Big] + \alpha_s \alpha \Big[ \frac{16}{3} L_{du11ij}^{V1,LR} \\
& + \frac{16}{3} L_{du22ij}^{V1,LR} + \frac{16}{3} L_{du33ij}^{V1,LR} - \frac{392}{243} L_{du11ij}^{V8,LR} - \frac{392}{243} L_{du22ij}^{V8,LR} - \frac{392}{243} L_{du33ij}^{V8,LR} + 32 L_{33ij}^{V,RR} \\
& + \frac{16}{3} L_{udij11}^{V1,RR} + \frac{16}{3} L_{udij22}^{V1,RR} + \frac{16}{3} L_{udij33}^{V1,RR} + \frac{328}{243} L_{ij11}^{V8,RR} + \frac{328}{243} L_{ij22}^{V8,RR} + \frac{328}{243} L_{ij33}^{V8,RR} \\
& - \frac{32}{3} L_{uu}^{V1,LR} - \frac{32}{3} L_{jjij}^{V1,LR} + \frac{1984}{243} L_{uu}^{V8,LR} + \frac{1984}{243} L_{jjij}^{V8,LR} - \frac{2240}{81} L_{ijii}^{V,RR} - \frac{2240}{81} L_{ijjj}^{V,RR} \Big] \\
& + \alpha^2 \Big[ - \frac{832}{243} L_{du11ij}^{V1,LR} - \frac{832}{243} L_{du22ij}^{V1,LR} - \frac{832}{243} L_{du33ij}^{V1,LR} - \frac{328}{243} L_{11ij}^{V,LR} - \frac{328}{243} L_{22ij}^{V,LR} \\
& - \frac{328}{243} L_{33ij}^{V,LR} + \frac{3344}{243} L_{11ij}^{V,RR} + \frac{3344}{243} L_{22ij}^{V,RR} + \frac{4352}{243} L_{33ij}^{V,RR} + \frac{392}{243} L_{ij11}^{V1,RR} \\
& + \frac{392}{243} L_{ij22}^{V1,RR} + \frac{392}{243} L_{ij33}^{V1,RR} - \frac{64}{243} L_{uu}^{V1,LR} - \frac{64}{243} L_{jjij}^{V1,LR} + \frac{25888}{243} L_{ijii}^{V,RR} \\
& + \frac{25888}{243} L_{ijjj}^{V,RR} \Big] ;
\end{aligned}$$

$$\begin{aligned}
& + \frac{392}{243} L_{ij22}^{V1,RR} + \frac{392}{243} L_{ij33}^{V1,RR} - \frac{64}{243} L_{iij}^{V1,LR} - \frac{64}{243} L_{jjij}^{V1,LR} + \frac{25888}{243} L_{iij}^{V,RR} \\
& + \frac{25888}{243} L_{ijjj}^{V,RR} \Big] ; \\
\dot{L}_{ij11}^{V1,RR} = & \frac{8}{3} g_s^2 L_{ij11}^{V8,RR} + e^2 \Bigg[ \frac{4}{9} L_{11ij}^{V1,LR} + \frac{4}{9} L_{22ij}^{V1,LR} + \frac{4}{9} L_{33ij}^{V1,LR} + \frac{4}{9} L_{11ij}^{V,LR} \\
& + \frac{4}{9} L_{22ij}^{V,LR} + \frac{4}{9} L_{33ij}^{V,LR} + \frac{4}{9} L_{11ij}^{V,RR} + \frac{4}{9} L_{22ij}^{V,RR} + \frac{4}{9} L_{33ij}^{V,RR} - \frac{20}{9} L_{ij11}^{V1,RR} \\
& + \frac{4}{9} L_{ij22}^{V1,RR} + \frac{4}{9} L_{ij33}^{V1,RR} - \frac{8}{9} L_{iij}^{V1,LR} - \frac{8}{9} L_{jjij}^{V1,LR} - \frac{64}{27} L_{iij}^{V,RR} - \frac{64}{27} L_{ijjj}^{V,RR} \Big] \\
& + \alpha_s^2 \Bigg[ -8 L_{11ij}^{V1,LR} - 8 L_{22ij}^{V1,LR} - 8 L_{33ij}^{V1,LR} + \frac{4}{27} L_{11ij}^{V8,LR} + \frac{4}{27} L_{22ij}^{V8,LR} \\
& + \frac{4}{27} L_{33ij}^{V8,LR} - \frac{4}{3} L_{ij11}^{V1,RR} + 8 L_{ij22}^{V1,RR} + 8 L_{ij33}^{V1,RR} + \frac{86}{27} L_{ij11}^{V8,RR} + \frac{4}{27} L_{ij22}^{V8,RR} \\
& + \frac{4}{27} L_{ij33}^{V8,RR} - 8 L_{iij}^{V1,LR} - 8 L_{jjij}^{V1,LR} + \frac{4}{27} L_{iij}^{V8,LR} + \frac{4}{27} L_{jjij}^{V8,LR} + \frac{328}{9} L_{iij}^{V,RR} \\
& + \frac{328}{9} L_{ijjj}^{V,RR} \Big] + \alpha_s \alpha \Bigg[ \frac{16}{9} L_{11ij}^{V1,LR} + \frac{16}{9} L_{22ij}^{V1,LR} + \frac{16}{9} L_{33ij}^{V1,LR} - \frac{392}{729} L_{11ij}^{V8,LR} \\
& - \frac{392}{729} L_{22ij}^{V8,LR} - \frac{392}{729} L_{33ij}^{V8,LR} + \frac{208}{9} L_{ij11}^{V1,RR} + \frac{16}{9} L_{ij22}^{V1,RR} + \frac{16}{9} L_{ij33}^{V1,RR} + \frac{112}{729} L_{ij11}^{V8,RR} \\
& + \frac{328}{729} L_{ij22}^{V8,RR} + \frac{328}{729} L_{ij33}^{V8,RR} - \frac{32}{9} L_{iij}^{V1,LR} - \frac{32}{9} L_{jjij}^{V1,LR} + \frac{1984}{729} L_{iij}^{V8,LR} + \frac{1984}{729} L_{jjij}^{V8,LR} \\
& - \frac{2240}{243} L_{iij}^{V,RR} - \frac{2240}{243} L_{ijjj}^{V,RR} \Big] + \alpha^2 \Bigg[ -\frac{40}{729} L_{11ij}^{V1,LR} - \frac{40}{729} L_{22ij}^{V1,LR} - \frac{40}{729} L_{33ij}^{V1,LR} \\
& + \frac{1760}{729} L_{11ij}^{V,LR} + \frac{1760}{729} L_{22ij}^{V,LR} + \frac{1760}{729} L_{33ij}^{V,LR} + \frac{1544}{729} L_{11ij}^{V,RR} + \frac{1544}{729} L_{22ij}^{V,RR} \\
& + \frac{1544}{729} L_{33ij}^{V,RR} - \frac{1264}{729} L_{ij11}^{V1,RR} - \frac{112}{729} L_{ij22}^{V1,RR} - \frac{112}{729} L_{ij33}^{V1,RR} + \frac{2240}{729} L_{iij}^{V1,LR} \\
& + \frac{2240}{729} L_{jjij}^{V1,LR} + \frac{11488}{729} L_{iij}^{V,RR} + \frac{11488}{729} L_{ijjj}^{V,RR} \Big] ; \\
\dot{L}_{ij11}^{V8,RR} = & g_s^2 \Bigg[ \frac{2}{3} L_{11ij}^{V8,LR} + \frac{2}{3} L_{22ij}^{V8,LR} + \frac{2}{3} L_{33ij}^{V8,LR} + 12 L_{ij11}^{V1,RR} - \frac{10}{3} L_{ij11}^{V8,RR}
\end{aligned}$$

$$\begin{aligned}
& + \frac{2}{3} L_{ij22}^{V8,RR} + \frac{2}{3} L_{ij33}^{V8,RR} + \frac{2}{3} L_{iij}^{V8,LR} + \frac{2}{3} L_{jjij}^{V8,LR} + \frac{8}{3} L_{ijii}^{V,RR} + \frac{8}{3} L_{ijjj}^{V,RR} \Big] \\
& - \frac{8}{3} e^2 L_{ij11}^{V8,RR} + \alpha_s^2 \left[ - \frac{22}{3} L_{11ij}^{V1,LR} - \frac{22}{3} L_{22ij}^{V1,LR} - \frac{22}{3} L_{33ij}^{V1,LR} + \frac{169}{81} L_{11ij}^{V8,LR} \right. \\
& + \frac{169}{81} L_{22ij}^{V8,LR} + \frac{169}{81} L_{33ij}^{V8,LR} + 13 L_{ij11}^{V1,RR} - \frac{2}{3} L_{ij22}^{V1,RR} - \frac{2}{3} L_{ij33}^{V1,RR} - \frac{326}{81} L_{ij11}^{V8,RR} \\
& + \frac{799}{81} L_{ij22}^{V8,RR} + \frac{799}{81} L_{ij33}^{V8,RR} - \frac{22}{3} L_{iij}^{V1,LR} - \frac{22}{3} L_{jjij}^{V1,LR} + \frac{169}{81} L_{iij}^{V8,LR} + \frac{169}{81} L_{jjij}^{V8,LR} \\
& + \frac{1930}{27} L_{ijii}^{V,RR} + \frac{1930}{27} L_{ijjj}^{V,RR} \Big] + \alpha_s \alpha \left[ \frac{308}{81} L_{11ij}^{V1,LR} + \frac{308}{81} L_{22ij}^{V1,LR} + \frac{308}{81} L_{33ij}^{V1,LR} \right. \\
& + \frac{10}{27} L_{11ij}^{V8,LR} + \frac{10}{27} L_{22ij}^{V8,LR} + \frac{10}{27} L_{33ij}^{V8,LR} + \frac{308}{81} L_{11ij}^{V,LR} + \frac{308}{81} L_{22ij}^{V,LR} + \frac{308}{81} L_{33ij}^{V,LR} \\
& + \frac{308}{81} L_{11ij}^{V,RR} + \frac{308}{81} L_{22ij}^{V,RR} + \frac{308}{81} L_{33ij}^{V,RR} + \frac{200}{81} L_{ij11}^{V1,RR} + \frac{308}{81} L_{ij22}^{V1,RR} + \frac{308}{81} L_{ij33}^{V1,RR} \\
& - \frac{11}{3} L_{ij11}^{V8,RR} + \frac{14}{9} L_{ij22}^{V8,RR} + \frac{14}{9} L_{ij33}^{V8,RR} - \frac{616}{81} L_{iij}^{V1,LR} - \frac{616}{81} L_{jjij}^{V1,LR} + \frac{4}{27} L_{iij}^{V8,LR} \\
& + \frac{4}{27} L_{jjij}^{V8,LR} - \frac{4808}{81} L_{ijii}^{V,RR} - \frac{4808}{81} L_{ijjj}^{V,RR} \Big] - \frac{128}{81} \alpha^2 L_{ij11}^{V8,RR} ;
\end{aligned}$$

$$\begin{aligned}
\dot{L}_{ij22}^{V1,RR} &= \frac{8}{3} g_s^2 L_{ij22}^{V8,RR} + e^2 \left[ \frac{4}{9} L_{11ij}^{V1,LR} + \frac{4}{9} L_{22ij}^{V1,LR} + \frac{4}{9} L_{33ij}^{V1,LR} + \frac{4}{9} L_{11ij}^{V,LR} \right. \\
& + \frac{4}{9} L_{22ij}^{V,LR} + \frac{4}{9} L_{33ij}^{V,LR} + \frac{4}{9} L_{11ij}^{V,RR} + \frac{4}{9} L_{22ij}^{V,RR} + \frac{4}{9} L_{33ij}^{V,RR} + \frac{4}{9} L_{ij11}^{V1,RR} \\
& - \frac{20}{9} L_{ij22}^{V1,RR} + \frac{4}{9} L_{ij33}^{V1,RR} - \frac{8}{9} L_{iij}^{V1,LR} - \frac{8}{9} L_{jjij}^{V1,LR} - \frac{64}{27} L_{ijii}^{V,RR} - \frac{64}{27} L_{ijjj}^{V,RR} \Big] \\
& + \alpha_s^2 \left[ - 8 L_{11ij}^{V1,LR} - 8 L_{22ij}^{V1,LR} - 8 L_{33ij}^{V1,LR} + \frac{4}{27} L_{11ij}^{V8,LR} + \frac{4}{27} L_{22ij}^{V8,LR} \right. \\
& + \frac{4}{27} L_{33ij}^{V8,LR} + 8 L_{ij11}^{V1,RR} - \frac{4}{3} L_{ij22}^{V1,RR} + 8 L_{ij33}^{V1,RR} + \frac{4}{27} L_{ij11}^{V8,RR} + \frac{86}{27} L_{ij22}^{V8,RR} \\
& + \frac{4}{27} L_{ij33}^{V8,RR} - 8 L_{iij}^{V1,LR} - 8 L_{jjij}^{V1,LR} + \frac{4}{27} L_{iij}^{V8,LR} + \frac{4}{27} L_{jjij}^{V8,LR} + \frac{328}{9} L_{ijii}^{V,RR} \\
& + \frac{328}{9} L_{ijjj}^{V,RR} \Big] + \alpha_s \alpha \left[ \frac{16}{9} L_{11ij}^{V1,LR} + \frac{16}{9} L_{22ij}^{V1,LR} + \frac{16}{9} L_{33ij}^{V1,LR} - \frac{392}{729} L_{11ij}^{V8,LR} \right.
\end{aligned}$$

$$\begin{aligned}
& -\frac{392}{729}L_{22ij}^{V8,LR} - \frac{392}{729}L_{33ij}^{V8,LR} + \frac{16}{9}L_{ij11}^{V1,RR} + \frac{208}{9}L_{ij22}^{V1,RR} + \frac{16}{9}L_{ij33}^{V1,RR} + \frac{328}{729}L_{ij11}^{V8,RR} \\
& + \frac{112}{729}L_{ij22}^{V8,RR} + \frac{328}{729}L_{ij33}^{V8,RR} - \frac{32}{9}L_{iiij}^{V1,LR} - \frac{32}{9}L_{jjij}^{V1,LR} + \frac{1984}{729}L_{iiij}^{V8,LR} + \frac{1984}{729}L_{jjij}^{V8,LR} \\
& - \frac{2240}{243}L_{ijii}^{V,RR} - \frac{2240}{243}L_{ijjj}^{V,RR} \Big] + \alpha^2 \Big[ -\frac{40}{729}L_{11ij}^{V1,LR} - \frac{40}{729}L_{22ij}^{V1,LR} - \frac{40}{729}L_{33ij}^{V1,LR} \\
& + \frac{1760}{729}L_{11ij}^{V,LR} + \frac{1760}{729}L_{22ij}^{V,LR} + \frac{1760}{729}L_{33ij}^{V,LR} + \frac{1544}{729}L_{11ij}^{V,RR} + \frac{1544}{729}L_{22ij}^{V,RR} \\
& + \frac{1544}{729}L_{33ij}^{V,RR} - \frac{112}{729}L_{ij11}^{V1,RR} - \frac{1264}{729}L_{ij22}^{V1,RR} - \frac{112}{729}L_{ij33}^{V1,RR} + \frac{2240}{729}L_{iiij}^{V1,LR} \\
& + \frac{2240}{729}L_{jjij}^{V1,LR} + \frac{11488}{729}L_{ijii}^{V,RR} + \frac{11488}{729}L_{ijjj}^{V,RR} \Big] ;
\end{aligned}$$

$$\begin{aligned}
\dot{L}_{ij22}^{V8,RR} &= g_s^2 \Big[ \frac{2}{3}L_{11ij}^{V8,LR} + \frac{2}{3}L_{22ij}^{V8,LR} + \frac{2}{3}L_{33ij}^{V8,LR} + 12L_{ij22}^{V1,RR} + \frac{2}{3}L_{ij11}^{V8,RR} \\
& - \frac{10}{3}L_{ij22}^{V8,RR} + \frac{2}{3}L_{ij33}^{V8,RR} + \frac{2}{3}L_{iiij}^{V8,LR} + \frac{2}{3}L_{jjij}^{V8,LR} + \frac{8}{3}L_{ijii}^{V,RR} + \frac{8}{3}L_{ijjj}^{V,RR} \Big] \\
& - \frac{8}{3}e^2L_{ij22}^{V8,RR} + \alpha_s^2 \Big[ -\frac{22}{3}L_{11ij}^{V1,LR} - \frac{22}{3}L_{22ij}^{V1,LR} - \frac{22}{3}L_{33ij}^{V1,LR} + \frac{169}{81}L_{11ij}^{V8,LR} \\
& + \frac{169}{81}L_{22ij}^{V8,LR} + \frac{169}{81}L_{33ij}^{V8,LR} - \frac{2}{3}L_{ij11}^{V1,RR} + 13L_{ij22}^{V1,RR} - \frac{2}{3}L_{ij33}^{V1,RR} + \frac{799}{81}L_{ij11}^{V8,RR} \\
& - \frac{326}{81}L_{ij22}^{V8,RR} + \frac{799}{81}L_{ij33}^{V8,RR} - \frac{22}{3}L_{iiij}^{V1,LR} - \frac{22}{3}L_{jjij}^{V1,LR} + \frac{169}{81}L_{iiij}^{V8,LR} + \frac{169}{81}L_{jjij}^{V8,LR} \\
& + \frac{1930}{27}L_{ijii}^{V,RR} + \frac{1930}{27}L_{ijjj}^{V,RR} \Big] + \alpha_s \alpha \Big[ \frac{308}{81}L_{11ij}^{V1,LR} + \frac{308}{81}L_{22ij}^{V1,LR} + \frac{308}{81}L_{33ij}^{V1,LR} \\
& + \frac{10}{27}L_{11ij}^{V8,LR} + \frac{10}{27}L_{22ij}^{V8,LR} + \frac{10}{27}L_{33ij}^{V8,LR} + \frac{308}{81}L_{11ij}^{V,LR} + \frac{308}{81}L_{22ij}^{V,LR} + \frac{308}{81}L_{33ij}^{V,LR} \\
& + \frac{308}{81}L_{11ij}^{V,RR} + \frac{308}{81}L_{22ij}^{V,RR} + \frac{308}{81}L_{33ij}^{V,RR} + \frac{308}{81}L_{ij11}^{V1,RR} + \frac{200}{81}L_{ij22}^{V1,RR} + \frac{308}{81}L_{ij33}^{V1,RR} \\
& + \frac{14}{9}L_{ij11}^{V8,RR} - \frac{11}{3}L_{ij22}^{V8,RR} + \frac{14}{9}L_{ij33}^{V8,RR} - \frac{616}{81}L_{iiij}^{V1,LR} - \frac{616}{81}L_{jjij}^{V1,LR} + \frac{4}{27}L_{iiij}^{V8,LR} \\
& + \frac{4}{27}L_{jjij}^{V8,LR} - \frac{4808}{81}L_{ijii}^{V,RR} - \frac{4808}{81}L_{ijjj}^{V,RR} \Big] - \frac{128}{81}\alpha^2L_{ij22}^{V8,RR} ;
\end{aligned}$$

$$\begin{aligned}
\dot{L}_{ud,ij33}^{V1,RR} = & \frac{8}{3}g_s^2 L_{ij33}^{V8,RR} + e^2 \left[ \frac{4}{9}L_{11ij}^{V1,LR} + \frac{4}{9}L_{22ij}^{V1,LR} + \frac{4}{9}L_{33ij}^{V1,LR} + \frac{4}{9}L_{11ij}^{V,LR} \right. \\
& + \frac{4}{9}L_{22ij}^{V,LR} + \frac{4}{9}L_{33ij}^{V,LR} + \frac{4}{9}L_{11ij}^{V,RR} + \frac{4}{9}L_{22ij}^{V,RR} + \frac{4}{9}L_{33ij}^{V,RR} + \frac{4}{9}L_{ij11}^{V1,RR} \\
& + \frac{4}{9}L_{ij22}^{V1,RR} - \frac{20}{9}L_{ij33}^{V1,RR} - \frac{8}{9}L_{iiij}^{V1,LR} - \frac{8}{9}L_{jjij}^{V1,LR} - \frac{64}{27}L_{ijii}^{V,RR} - \frac{64}{27}L_{ijjj}^{V,RR} \Big] \\
& + \alpha_s^2 \left[ -8L_{11ij}^{V1,LR} - 8L_{22ij}^{V1,LR} - 8L_{33ij}^{V1,LR} + \frac{4}{27}L_{11ij}^{V8,LR} + \frac{4}{27}L_{22ij}^{V8,LR} \right. \\
& + \frac{4}{27}L_{33ij}^{V8,LR} + 8L_{ij11}^{V1,RR} + 8L_{ij22}^{V1,RR} - \frac{4}{3}L_{ij33}^{V1,RR} + \frac{4}{27}L_{ij11}^{V8,RR} + \frac{4}{27}L_{ij22}^{V8,RR} \\
& + \frac{86}{27}L_{ij33}^{V8,RR} - 8L_{iiij}^{V1,LR} - 8L_{jjij}^{V1,LR} + \frac{4}{27}L_{iiij}^{V8,LR} + \frac{4}{27}L_{jjij}^{V8,LR} + \frac{328}{9}L_{ijii}^{V,RR} \\
& + \frac{328}{9}L_{ijjj}^{V,RR} \Big] + \alpha_s \alpha \left[ \frac{16}{9}L_{11ij}^{V1,LR} + \frac{16}{9}L_{22ij}^{V1,LR} + \frac{16}{9}L_{33ij}^{V1,LR} - \frac{392}{729}L_{11ij}^{V8,LR} \right. \\
& - \frac{392}{729}L_{22ij}^{V8,LR} - \frac{392}{729}L_{33ij}^{V8,LR} + \frac{16}{9}L_{ij11}^{V1,RR} + \frac{16}{9}L_{ij22}^{V1,RR} + \frac{208}{9}L_{ij33}^{V1,RR} + \frac{328}{729}L_{ij11}^{V8,RR} \\
& + \frac{328}{729}L_{ij22}^{V8,RR} + \frac{112}{729}L_{ij33}^{V8,RR} - \frac{32}{9}L_{iiij}^{V1,LR} - \frac{32}{9}L_{jjij}^{V1,LR} + \frac{1984}{729}L_{iiij}^{V8,LR} + \frac{1984}{729}L_{jjij}^{V8,LR} \\
& - \frac{2240}{243}L_{ijii}^{V,RR} - \frac{2240}{243}L_{ijjj}^{V,RR} \Big] + \alpha^2 \left[ -\frac{40}{729}L_{11ij}^{V1,LR} - \frac{40}{729}L_{22ij}^{V1,LR} - \frac{40}{729}L_{33ij}^{V1,LR} \right. \\
& + \frac{1760}{729}L_{11ij}^{V,LR} + \frac{1760}{729}L_{22ij}^{V,LR} + \frac{1760}{729}L_{33ij}^{V,LR} + \frac{1544}{729}L_{11ij}^{V,RR} + \frac{1544}{729}L_{22ij}^{V,RR} \\
& + \frac{1544}{729}L_{33ij}^{V,RR} - \frac{112}{729}L_{ij11}^{V1,RR} - \frac{112}{729}L_{ij22}^{V1,RR} - \frac{1264}{729}L_{ij33}^{V1,RR} + \frac{2240}{729}L_{iiij}^{V1,LR} \\
& + \frac{2240}{729}L_{jjij}^{V1,LR} + \frac{11488}{729}L_{ijii}^{V,RR} + \frac{11488}{729}L_{ijjj}^{V,RR} \Big] ; \\
\dot{L}_{ud,ij33}^{V8,RR} = & g_s^2 \left[ \frac{2}{3}L_{11ij}^{V8,LR} + \frac{2}{3}L_{22ij}^{V8,LR} + \frac{2}{3}L_{33ij}^{V8,LR} + 12L_{ij33}^{V1,RR} + \frac{2}{3}L_{ij11}^{V8,RR} \right. \\
& + \frac{2}{3}L_{ij22}^{V8,RR} - \frac{10}{3}L_{ij33}^{V8,RR} + \frac{2}{3}L_{iiij}^{V8,LR} + \frac{2}{3}L_{jjij}^{V8,LR} + \frac{8}{3}L_{ijii}^{V,RR} + \frac{8}{3}L_{ijjj}^{V,RR} \Big] \\
& - \frac{8}{3}e^2 L_{ij33}^{V8,RR} + \alpha_s^2 \left[ -\frac{22}{3}L_{11ij}^{V1,LR} - \frac{22}{3}L_{22ij}^{V1,LR} - \frac{22}{3}L_{33ij}^{V1,LR} + \frac{169}{81}L_{11ij}^{V8,LR} \right.
\end{aligned}$$

$$\begin{aligned}
& + \frac{169}{81} L_{22ij}^{V8,LR} + \frac{169}{81} L_{33ij}^{V8,LR} - \frac{2}{3} L_{ij11}^{V1,RR} - \frac{2}{3} L_{ij22}^{V1,RR} + 13 L_{ij33}^{V1,RR} + \frac{799}{81} L_{ij11}^{V8,RR} \\
& + \frac{799}{81} L_{ij22}^{V8,RR} - \frac{326}{81} L_{ij33}^{V8,RR} - \frac{22}{3} L_{iijj}^{V1,LR} - \frac{22}{3} L_{jjij}^{V1,LR} + \frac{169}{81} L_{iijj}^{V8,LR} + \frac{169}{81} L_{jjij}^{V8,LR} \\
& + \frac{1930}{27} L_{iijj}^{V,RR} + \frac{1930}{27} L_{jjjj}^{V,RR} \Big] + \alpha_s \alpha \Big[ \frac{308}{81} L_{11ij}^{V1,LR} + \frac{308}{81} L_{22ij}^{V1,LR} + \frac{308}{81} L_{33ij}^{V1,LR} \\
& + \frac{10}{27} L_{11ij}^{V8,LR} + \frac{10}{27} L_{22ij}^{V8,LR} + \frac{10}{27} L_{33ij}^{V8,LR} + \frac{308}{81} L_{11ij}^{V,LR} + \frac{308}{81} L_{22ij}^{V,LR} + \frac{308}{81} L_{33ij}^{V,LR} \\
& + \frac{308}{81} L_{11ij}^{V,RR} + \frac{308}{81} L_{22ij}^{V,RR} + \frac{308}{81} L_{33ij}^{V,RR} + \frac{308}{81} L_{ij11}^{V1,RR} + \frac{308}{81} L_{ij22}^{V1,RR} + \frac{200}{81} L_{ij33}^{V1,RR} \\
& + \frac{14}{9} L_{ij11}^{V8,RR} + \frac{14}{9} L_{ij22}^{V8,RR} - \frac{11}{3} L_{ij33}^{V8,RR} - \frac{616}{81} L_{iijj}^{V1,LR} - \frac{616}{81} L_{jjij}^{V1,LR} + \frac{4}{27} L_{iijj}^{V8,LR} \\
& + \frac{4}{27} L_{jjij}^{V8,LR} - \frac{4808}{81} L_{iijj}^{V,RR} - \frac{4808}{81} L_{jjjj}^{V,RR} \Big] - \frac{128}{81} \alpha^2 L_{ij33}^{V8,RR} ;
\end{aligned}$$

$$\begin{aligned}
\dot{L}_{iijj}^{V,RR} &= g_s^2 \Big[ \frac{1}{9} L_{11ij}^{V8,LR} + \frac{1}{9} L_{22ij}^{V8,LR} + \frac{1}{9} L_{33ij}^{V8,LR} + \frac{1}{9} L_{ij11}^{V8,RR} + \frac{1}{9} L_{ij22}^{V8,RR} \\
& + \frac{1}{9} L_{ij33}^{V8,RR} + \frac{1}{9} L_{iijj}^{V8,LR} + \frac{1}{9} L_{jjij}^{V8,LR} + \frac{4}{9} L_{iijj}^{V,RR} + \frac{40}{9} L_{jjjj}^{V,RR} \Big] + e^2 \Big[ - \frac{4}{9} L_{11ij}^{V1,LR} \\
& - \frac{4}{9} L_{22ij}^{V1,LR} - \frac{4}{9} L_{33ij}^{V1,LR} - \frac{4}{9} L_{11ij}^{V,LR} - \frac{4}{9} L_{22ij}^{V,LR} - \frac{4}{9} L_{33ij}^{V,LR} - \frac{4}{9} L_{11ij}^{V,RR} \\
& - \frac{4}{9} L_{22ij}^{V,RR} - \frac{4}{9} L_{33ij}^{V,RR} - \frac{4}{9} L_{ij11}^{V1,RR} - \frac{4}{9} L_{ij22}^{V1,RR} - \frac{4}{9} L_{ij33}^{V1,RR} + \frac{8}{9} L_{iijj}^{V1,LR} \\
& + \frac{8}{9} L_{jjij}^{V1,LR} + \frac{64}{27} L_{iijj}^{V,RR} + \frac{208}{27} L_{jjjj}^{V,RR} \Big] + \alpha_s^2 \Big[ - \frac{47}{9} L_{11ij}^{V1,LR} - \frac{47}{9} L_{22ij}^{V1,LR} \\
& - \frac{47}{9} L_{33ij}^{V1,LR} + \frac{205}{486} L_{11ij}^{V8,LR} + \frac{205}{486} L_{22ij}^{V8,LR} + \frac{205}{486} L_{33ij}^{V8,LR} + \frac{35}{9} L_{ij11}^{V1,RR} + \frac{35}{9} L_{ij22}^{V1,RR} \\
& + \frac{35}{9} L_{ij33}^{V1,RR} + \frac{835}{486} L_{ij11}^{V8,RR} + \frac{835}{486} L_{ij22}^{V8,RR} + \frac{835}{486} L_{ij33}^{V8,RR} - \frac{47}{9} L_{iijj}^{V1,LR} - \frac{47}{9} L_{jjij}^{V1,LR} \\
& + \frac{205}{486} L_{iijj}^{V8,LR} + \frac{205}{486} L_{jjij}^{V8,LR} + \frac{2441}{81} L_{iijj}^{V,RR} + \frac{2054}{81} L_{jjjj}^{V,RR} \Big] + \alpha_s \alpha \Big[ - \frac{332}{243} L_{11ij}^{V1,LR} \\
& - \frac{332}{243} L_{22ij}^{V1,LR} - \frac{332}{243} L_{33ij}^{V1,LR} + \frac{977}{729} L_{11ij}^{V8,LR} + \frac{977}{729} L_{22ij}^{V8,LR} + \frac{977}{729} L_{33ij}^{V8,LR}
\end{aligned}$$

$$\begin{aligned}
& + \frac{100}{243} L_{11ij}^{V,LR} + \frac{100}{243} L_{22ij}^{V,LR} + \frac{100}{243} L_{33ij}^{V,LR} + \frac{100}{243} L_{11ij}^{V,RR} + \frac{100}{243} L_{22ij}^{V,RR} + \frac{100}{243} L_{33ij}^{V,RR} \\
& - \frac{332}{243} L_{ij11}^{V1,RR} - \frac{332}{243} L_{ij22}^{V1,RR} - \frac{332}{243} L_{ij33}^{V1,RR} - \frac{571}{729} L_{ij11}^{V8,RR} - \frac{571}{729} L_{ij22}^{V8,RR} \\
& - \frac{571}{729} L_{ij33}^{V8,RR} + \frac{664}{243} L_{iij}^{V1,LR} + \frac{664}{243} L_{jjj}^{V1,LR} - \frac{2884}{729} L_{iij}^{V8,LR} - \frac{2884}{729} L_{jjj}^{V8,LR} \\
& + \frac{3832}{243} L_{ijii}^{V,RR} - \frac{12152}{243} L_{ijjj}^{V,RR} \Big] + \alpha^2 \Big[ - \frac{1148}{729} L_{11ij}^{V1,LR} - \frac{1148}{729} L_{22ij}^{V1,LR} - \frac{1148}{729} L_{33ij}^{V1,LR} \\
& - \frac{4892}{729} L_{11ij}^{V,LR} - \frac{4892}{729} L_{22ij}^{V,LR} - \frac{4892}{729} L_{33ij}^{V,LR} + \frac{1156}{729} L_{11ij}^{V,RR} + \frac{1156}{729} L_{22ij}^{V,RR} \\
& + \frac{1156}{729} L_{33ij}^{V,RR} + \frac{868}{729} L_{ij11}^{V1,RR} + \frac{868}{729} L_{ij22}^{V1,RR} + \frac{868}{729} L_{ij33}^{V1,RR} - \frac{5696}{729} L_{iij}^{V1,LR} \\
& - \frac{5696}{729} L_{jjj}^{V1,LR} + \frac{10112}{729} L_{iij}^{V,RR} - \frac{544}{729} L_{ijjj}^{V,RR} \Big] ;
\end{aligned}$$

$$\begin{aligned}
\dot{L}_{ijii}^{V,RR} & = g_s^2 \Big[ \frac{1}{9} L_{11ij}^{V8,LR} + \frac{1}{9} L_{22ij}^{V8,LR} + \frac{1}{9} L_{33ij}^{V8,LR} + \frac{1}{9} L_{ij11}^{V8,RR} + \frac{1}{9} L_{ij22}^{V8,RR} \\
& + \frac{1}{9} L_{ij33}^{V8,RR} + \frac{1}{9} L_{iij}^{V8,LR} + \frac{1}{9} L_{jjj}^{V8,LR} + \frac{40}{9} L_{ijii}^{V,RR} + \frac{4}{9} L_{ijjj}^{V,RR} \Big] + e^2 \Big[ - \frac{4}{9} L_{11ij}^{V1,LR} \\
& - \frac{4}{9} L_{22ij}^{V1,LR} - \frac{4}{9} L_{33ij}^{V1,LR} - \frac{4}{9} L_{ij11}^{V,LR} - \frac{4}{9} L_{ij22}^{V,LR} - \frac{4}{9} L_{ij33}^{V,LR} - \frac{4}{9} L_{iij}^{V,RR} \\
& - \frac{4}{9} L_{jjj}^{V,RR} - \frac{4}{9} L_{ij11}^{V1,RR} - \frac{4}{9} L_{ij22}^{V1,RR} - \frac{4}{9} L_{ij33}^{V1,RR} + \frac{8}{9} L_{iij}^{V1,LR} \\
& + \frac{8}{9} L_{jjj}^{V1,LR} + \frac{208}{27} L_{ijii}^{V,RR} + \frac{64}{27} L_{ijjj}^{V,RR} \Big] + \alpha_s^2 \Big[ - \frac{47}{9} L_{11ij}^{V1,LR} - \frac{47}{9} L_{22ij}^{V1,LR} \\
& - \frac{47}{9} L_{33ij}^{V1,LR} + \frac{205}{486} L_{11ij}^{V8,LR} + \frac{205}{486} L_{22ij}^{V8,LR} + \frac{205}{486} L_{33ij}^{V8,LR} + \frac{35}{9} L_{ij11}^{V1,RR} + \frac{35}{9} L_{ij22}^{V1,RR} \\
& + \frac{35}{9} L_{ij33}^{V1,RR} + \frac{835}{486} L_{ij11}^{V8,RR} + \frac{835}{486} L_{ij22}^{V8,RR} + \frac{835}{486} L_{ij33}^{V8,RR} - \frac{47}{9} L_{iij}^{V1,LR} - \frac{47}{9} L_{jjj}^{V1,LR} \\
& + \frac{205}{486} L_{iij}^{V8,LR} + \frac{205}{486} L_{jjj}^{V8,LR} + \frac{2054}{81} L_{ijii}^{V,RR} + \frac{2441}{81} L_{ijjj}^{V,RR} \Big] + \alpha_s \alpha \Big[ - \frac{332}{243} L_{11ij}^{V1,LR} \\
& - \frac{332}{243} L_{22ij}^{V1,LR} - \frac{332}{243} L_{33ij}^{V1,LR} + \frac{977}{729} L_{11ij}^{V8,LR} + \frac{977}{729} L_{22ij}^{V8,LR} + \frac{977}{729} L_{33ij}^{V8,LR} \\
& + \frac{100}{243} L_{11ij}^{V,LR} + \frac{100}{243} L_{22ij}^{V,LR} + \frac{100}{243} L_{33ij}^{V,LR} + \frac{100}{243} L_{11ij}^{V,RR} + \frac{100}{243} L_{22ij}^{V,RR} + \frac{100}{243} L_{33ij}^{V,RR}
\end{aligned}$$



$$\begin{aligned}
& -\frac{332}{243}L_{ij11}^{V1,RR} - \frac{332}{243}L_{ij22}^{V1,RR} - \frac{332}{243}L_{ij33}^{V1,RR} - \frac{571}{729}L_{ij11}^{V8,RR} - \frac{571}{729}L_{ij22}^{V8,RR} \\
& - \frac{571}{729}L_{ij33}^{V8,RR} + \frac{664}{243}L_{iij}^{V1,LR} + \frac{664}{243}L_{jjj}^{V1,LR} - \frac{2884}{729}L_{iij}^{V8,LR} - \frac{2884}{729}L_{jjj}^{V8,LR} \\
& - \frac{12152}{243}L_{iij}^{V,RR} + \frac{3832}{243}L_{jjj}^{V,RR} \Big] + \alpha^2 \Big[ -\frac{1148}{729}L_{11ij}^{V1,LR} - \frac{1148}{729}L_{22ij}^{V1,LR} - \frac{1148}{729}L_{33ij}^{V1,LR} \\
& - \frac{4892}{729}L_{11ij}^{V,LR} - \frac{4892}{729}L_{22ij}^{V,LR} - \frac{4892}{729}L_{33ij}^{V,LR} + \frac{1156}{729}L_{11ij}^{V,RR} + \frac{1156}{729}L_{22ij}^{V,RR} \\
& + \frac{1156}{729}L_{33ij}^{V,RR} + \frac{868}{729}L_{ij11}^{V1,RR} + \frac{868}{729}L_{ij22}^{V1,RR} + \frac{868}{729}L_{ij33}^{V1,RR} - \frac{5696}{729}L_{iij}^{V1,LR} \\
& - \frac{5696}{729}L_{jjj}^{V1,LR} - \frac{544}{729}L_{iij}^{V,RR} + \frac{10112}{729}L_{jjj}^{V,RR} \Big] ; \\
\dot{L}_{11ij}^{V,LR} &= e^2 \Big[ \frac{4}{3}L_{11ij}^{V1,LR} + \frac{4}{3}L_{22ij}^{V1,LR} + \frac{4}{3}L_{33ij}^{V1,LR} + \frac{28}{3}L_{11ij}^{V,LR} + \frac{4}{3}L_{22ij}^{V,LR} \\
& + \frac{4}{3}L_{33ij}^{V,LR} + \frac{4}{3}L_{11ij}^{V,RR} + \frac{4}{3}L_{22ij}^{V,RR} + \frac{4}{3}L_{33ij}^{V,RR} + \frac{4}{3}L_{ij11}^{V1,RR} + \frac{4}{3}L_{ij22}^{V1,RR} \\
& + \frac{4}{3}L_{ij33}^{V1,RR} - \frac{8}{3}L_{iij}^{V1,LR} - \frac{8}{3}L_{jjj}^{V1,LR} - \frac{64}{9}L_{iij}^{V,RR} - \frac{64}{9}L_{jjj}^{V,RR} \Big] + \alpha_s \alpha \Big[ \frac{16}{3}L_{11ij}^{V1,LR} \\
& + \frac{16}{3}L_{22ij}^{V1,LR} + \frac{16}{3}L_{33ij}^{V1,LR} - \frac{392}{243}L_{11ij}^{V8,LR} - \frac{392}{243}L_{22ij}^{V8,LR} - \frac{392}{243}L_{33ij}^{V8,LR} - 32L_{11ij}^{V,LR} \\
& + \frac{16}{3}L_{ij11}^{V1,RR} + \frac{16}{3}L_{ij22}^{V1,RR} + \frac{16}{3}L_{ij33}^{V1,RR} + \frac{328}{243}L_{ij11}^{V8,RR} + \frac{328}{243}L_{ij22}^{V8,RR} + \frac{328}{243}L_{ij33}^{V8,RR} \\
& - \frac{32}{3}L_{iij}^{V1,LR} - \frac{32}{3}L_{jjj}^{V1,LR} + \frac{1984}{243}L_{iij}^{V8,LR} + \frac{1984}{243}L_{jjj}^{V8,LR} - \frac{2240}{81}L_{iij}^{V,RR} - \frac{2240}{81}L_{jjj}^{V,RR} \Big] \\
& + \alpha^2 \Big[ -\frac{1048}{243}L_{11ij}^{V1,LR} - \frac{1048}{243}L_{22ij}^{V1,LR} - \frac{1048}{243}L_{33ij}^{V1,LR} - \frac{41296}{243}L_{11ij}^{V,LR} + \frac{3344}{243}L_{22ij}^{V,LR} \\
& + \frac{3344}{243}L_{33ij}^{V,LR} - \frac{4648}{243}L_{11ij}^{V,RR} - \frac{4648}{243}L_{22ij}^{V,RR} - \frac{4648}{243}L_{33ij}^{V,RR} - \frac{3712}{243}L_{ij11}^{V1,RR} \\
& - \frac{3712}{243}L_{ij22}^{V1,RR} - \frac{3712}{243}L_{ij33}^{V1,RR} + \frac{12032}{243}L_{iij}^{V1,LR} + \frac{12032}{243}L_{jjj}^{V1,LR} + \frac{3424}{243}L_{iij}^{V,RR} \\
& + \frac{3424}{243}L_{jjj}^{V,RR} \Big] ;
\end{aligned}$$

$$\begin{aligned}
\dot{L}_{22ij}^{V,LR} &= e^2 \left[ \frac{4}{3} L_{11ij}^{V1,LR} + \frac{4}{3} L_{22ij}^{V1,LR} + \frac{4}{3} L_{33ij}^{V1,LR} + \frac{4}{3} L_{11ij}^{V,LR} + \frac{28}{3} L_{22ij}^{V,LR} \right. \\
&\quad + \frac{4}{3} L_{33ij}^{V,LR} + \frac{4}{3} L_{11ij}^{V,RR} + \frac{4}{3} L_{22ij}^{V,RR} + \frac{4}{3} L_{33ij}^{V,RR} + \frac{4}{3} L_{ij11}^{V1,RR} + \frac{4}{3} L_{ij22}^{V1,RR} \\
&\quad + \frac{4}{3} L_{ij33}^{V1,RR} - \frac{8}{3} L_{iiij}^{V1,LR} - \frac{8}{3} L_{jjij}^{V1,LR} - \frac{64}{9} L_{ijii}^{V,RR} - \frac{64}{9} L_{ijjj}^{V,RR} \left. \right] + \alpha_s \alpha \left[ \frac{16}{3} L_{11ij}^{V1,LR} \right. \\
&\quad + \frac{16}{3} L_{22ij}^{V1,LR} + \frac{16}{3} L_{33ij}^{V1,LR} - \frac{392}{243} L_{11ij}^{V8,LR} - \frac{392}{243} L_{22ij}^{V8,LR} - \frac{392}{243} L_{33ij}^{V8,LR} - 32 L_{22ij}^{V,LR} \\
&\quad + \frac{16}{3} L_{ij11}^{V1,RR} + \frac{16}{3} L_{ij22}^{V1,RR} + \frac{16}{3} L_{ij33}^{V1,RR} + \frac{328}{243} L_{ij11}^{V8,RR} + \frac{328}{243} L_{ij22}^{V8,RR} + \frac{328}{243} L_{ij33}^{V8,RR} \\
&\quad - \frac{32}{3} L_{iiij}^{V1,LR} - \frac{32}{3} L_{jjij}^{V1,LR} + \frac{1984}{243} L_{iiij}^{V8,LR} + \frac{1984}{243} L_{jjij}^{V8,LR} - \frac{2240}{81} L_{ijii}^{V,RR} - \frac{2240}{81} L_{ijjj}^{V,RR} \left. \right] \\
&\quad + \alpha^2 \left[ -\frac{1048}{243} L_{11ij}^{V1,LR} - \frac{1048}{243} L_{22ij}^{V1,LR} - \frac{1048}{243} L_{33ij}^{V1,LR} + \frac{3344}{243} L_{11ij}^{V,LR} - \frac{41296}{243} L_{22ij}^{V,LR} \right. \\
&\quad + \frac{3344}{243} L_{33ij}^{V,LR} - \frac{4648}{243} L_{11ij}^{V,RR} - \frac{4648}{243} L_{22ij}^{V,RR} - \frac{4648}{243} L_{33ij}^{V,RR} - \frac{3712}{243} L_{ij11}^{V1,RR} \\
&\quad - \frac{3712}{243} L_{ij22}^{V1,RR} - \frac{3712}{243} L_{ij33}^{V1,RR} + \frac{12032}{243} L_{iiij}^{V1,LR} + \frac{12032}{243} L_{jjij}^{V1,LR} + \frac{3424}{243} L_{ijii}^{V,RR} \\
&\quad \left. + \frac{3424}{243} L_{ijjj}^{V,RR} \right]; \\
\dot{L}_{33ij}^{V,LR} &= e^2 \left[ \frac{4}{3} L_{11ij}^{V1,LR} + \frac{4}{3} L_{22ij}^{V1,LR} + \frac{4}{3} L_{33ij}^{V1,LR} + \frac{4}{3} L_{11ij}^{V,LR} + \frac{4}{3} L_{22ij}^{V,LR} \right. \\
&\quad + \frac{28}{3} L_{33ij}^{V,LR} + \frac{4}{3} L_{11ij}^{V,RR} + \frac{4}{3} L_{22ij}^{V,RR} + \frac{4}{3} L_{33ij}^{V,RR} + \frac{4}{3} L_{ij11}^{V1,RR} + \frac{4}{3} L_{ij22}^{V1,RR} \\
&\quad + \frac{4}{3} L_{ij33}^{V1,RR} - \frac{8}{3} L_{iiij}^{V1,LR} - \frac{8}{3} L_{jjij}^{V1,LR} - \frac{64}{9} L_{ijii}^{V,RR} - \frac{64}{9} L_{ijjj}^{V,RR} \left. \right] + \alpha_s \alpha \left[ \frac{16}{3} L_{11ij}^{V1,LR} \right. \\
&\quad + \frac{16}{3} L_{22ij}^{V1,LR} + \frac{16}{3} L_{33ij}^{V1,LR} - \frac{392}{243} L_{11ij}^{V8,LR} - \frac{392}{243} L_{22ij}^{V8,LR} - \frac{392}{243} L_{33ij}^{V8,LR} - 32 L_{33ij}^{V,LR} \\
&\quad + \frac{16}{3} L_{ij11}^{V1,RR} + \frac{16}{3} L_{ij22}^{V1,RR} + \frac{16}{3} L_{ij33}^{V1,RR} + \frac{328}{243} L_{ij11}^{V8,RR} + \frac{328}{243} L_{ij22}^{V8,RR} + \frac{328}{243} L_{ij33}^{V8,RR} \\
&\quad - \frac{32}{3} L_{iiij}^{V1,LR} - \frac{32}{3} L_{jjij}^{V1,LR} + \frac{1984}{243} L_{iiij}^{V8,LR} + \frac{1984}{243} L_{jjij}^{V8,LR} - \frac{2240}{81} L_{ijii}^{V,RR} - \frac{2240}{81} L_{ijjj}^{V,RR} \left. \right]
\end{aligned}$$

$$\begin{aligned}
& + \alpha^2 \left[ -\frac{1048}{243} L_{11ij}^{V1,LR} - \frac{1048}{243} L_{22ij}^{V1,LR} - \frac{1048}{243} L_{33ij}^{V1,LR} + \frac{3344}{243} L_{11ij}^{V,LR} + \frac{3344}{243} L_{22ij}^{V,LR} \right. \\
& - \frac{41296}{243} L_{33ij}^{V,LR} - \frac{4648}{243} L_{11ij}^{V,RR} - \frac{4648}{243} L_{22ij}^{V,RR} - \frac{4648}{243} L_{33ij}^{V,RR} - \frac{3712}{243} L_{ij11}^{V1,RR} \\
& - \frac{3712}{243} L_{ij22}^{V1,RR} - \frac{3712}{243} L_{ij33}^{V1,RR} + \frac{12032}{243} L_{iiij}^{V1,LR} + \frac{12032}{243} L_{jjij}^{V1,LR} + \frac{3424}{243} L_{ijii}^{V,RR} \\
& \left. + \frac{3424}{243} L_{ijjj}^{V,RR} \right];
\end{aligned}$$

$$\begin{aligned}
\dot{L}_{11ij}^{V1,LR} = & -\frac{8}{3} g_s^2 L_{11ij}^{V8,LR} + e^2 \left[ \frac{28}{9} L_{11ij}^{V1,LR} + \frac{4}{9} L_{22ij}^{V1,LR} + \frac{4}{9} L_{33ij}^{V1,LR} + \frac{4}{9} L_{11ij}^{V,LR} \right. \\
& + \frac{4}{9} L_{22ij}^{V,LR} + \frac{4}{9} L_{33ij}^{V,LR} + \frac{4}{9} L_{11ij}^{V,RR} + \frac{4}{9} L_{22ij}^{V,RR} + \frac{4}{9} L_{33ij}^{V,RR} + \frac{4}{9} L_{ij11}^{V1,RR} \\
& + \frac{4}{9} L_{ij22}^{V1,RR} + \frac{4}{9} L_{ij33}^{V1,RR} - \frac{8}{9} L_{iiij}^{V1,LR} - \frac{8}{9} L_{jjij}^{V1,LR} - \frac{64}{27} L_{ijii}^{V,RR} - \frac{64}{27} L_{ijjj}^{V,RR} \left. \right] \\
& + \alpha_s^2 \left[ -\frac{4}{3} L_{11ij}^{V1,LR} + 8 L_{22ij}^{V1,LR} + 8 L_{33ij}^{V1,LR} - \frac{2000}{27} L_{11ij}^{V8,LR} + \frac{44}{27} L_{22ij}^{V8,LR} \right. \\
& + \frac{44}{27} L_{33ij}^{V8,LR} - 8 L_{ij11}^{V1,RR} - 8 L_{ij22}^{V1,RR} - 8 L_{ij33}^{V1,RR} + \frac{44}{27} L_{ij11}^{V8,RR} + \frac{44}{27} L_{ij22}^{V8,RR} \\
& + \frac{44}{27} L_{ij33}^{V8,RR} + 8 L_{iiij}^{V1,LR} + 8 L_{jjij}^{V1,LR} + \frac{44}{27} L_{iiij}^{V8,LR} + \frac{44}{27} L_{jjij}^{V8,LR} - \frac{232}{9} L_{ijii}^{V,RR} \\
& \left. - \frac{232}{9} L_{ijjj}^{V,RR} \right] + \alpha_s \alpha \left[ -\frac{176}{9} L_{11ij}^{V1,LR} + \frac{16}{9} L_{22ij}^{V1,LR} + \frac{16}{9} L_{33ij}^{V1,LR} + \frac{5872}{729} L_{11ij}^{V8,LR} \right. \\
& - \frac{392}{729} L_{22ij}^{V8,LR} - \frac{392}{729} L_{33ij}^{V8,LR} + \frac{16}{9} L_{ij11}^{V1,RR} + \frac{16}{9} L_{ij22}^{V1,RR} + \frac{16}{9} L_{ij33}^{V1,RR} + \frac{328}{729} L_{ij11}^{V8,RR} \\
& + \frac{328}{729} L_{ij22}^{V8,RR} + \frac{328}{729} L_{ij33}^{V8,RR} - \frac{32}{9} L_{iiij}^{V1,LR} - \frac{32}{9} L_{jjij}^{V1,LR} + \frac{1984}{729} L_{iiij}^{V8,LR} + \frac{1984}{729} L_{jjij}^{V8,LR} \\
& \left. - \frac{2240}{243} L_{ijii}^{V,RR} - \frac{2240}{243} L_{ijjj}^{V,RR} \right] + \alpha^2 \left[ -\frac{36544}{729} L_{11ij}^{V1,LR} - \frac{112}{729} L_{22ij}^{V1,LR} - \frac{112}{729} L_{33ij}^{V1,LR} \right. \\
& + \frac{2984}{729} L_{11ij}^{V,LR} + \frac{2984}{729} L_{22ij}^{V,LR} + \frac{2984}{729} L_{33ij}^{V,LR} - \frac{1120}{729} L_{11ij}^{V,RR} - \frac{1120}{729} L_{22ij}^{V,RR} \\
& - \frac{1120}{729} L_{33ij}^{V,RR} - \frac{1480}{729} L_{ij11}^{V1,RR} - \frac{1480}{729} L_{ij22}^{V1,RR} - \frac{1480}{729} L_{ij33}^{V1,RR} + \frac{6272}{729} L_{iiij}^{V1,LR}
\end{aligned}$$

$$\begin{aligned}
& + \frac{6272}{729} L_{jjj}^{V1,LR} + \frac{4000}{729} L_{ijii}^{V,RR} + \frac{4000}{729} L_{ijjj}^{V,RR} \Big] ; \\
\dot{L}_{11ij}^{V8,LR} &= g_s^2 \Bigg[ -12 L_{11ij}^{V1,LR} - \frac{40}{3} L_{11ij}^{V8,LR} + \frac{2}{3} L_{22ij}^{V8,LR} + \frac{2}{3} L_{33ij}^{V8,LR} + \frac{2}{3} L_{ij11}^{V8,RR} \\
& + \frac{2}{3} L_{ij22}^{V8,RR} + \frac{2}{3} L_{ij33}^{V8,RR} + \frac{2}{3} L_{iiij}^{V8,LR} + \frac{2}{3} L_{jjij}^{V8,LR} + \frac{8}{3} L_{ijii}^{V,RR} + \frac{8}{3} L_{ijjj}^{V,RR} \Bigg] \\
& + \frac{8}{3} e^2 L_{11ij}^{V8,LR} + \alpha_s^2 \Bigg[ -132 L_{11ij}^{V1,LR} - \frac{22}{3} L_{22ij}^{V1,LR} - \frac{22}{3} L_{33ij}^{V1,LR} - \frac{25177}{162} L_{11ij}^{V8,LR} \\
& + \frac{799}{81} L_{22ij}^{V8,LR} + \frac{799}{81} L_{33ij}^{V8,LR} - \frac{2}{3} L_{ij11}^{V1,RR} - \frac{2}{3} L_{ij22}^{V1,RR} - \frac{2}{3} L_{ij33}^{V1,RR} + \frac{619}{81} L_{ij11}^{V8,RR} \\
& + \frac{619}{81} L_{ij22}^{V8,RR} + \frac{619}{81} L_{ij33}^{V8,RR} - \frac{22}{3} L_{iiij}^{V1,LR} - \frac{22}{3} L_{jjij}^{V1,LR} + \frac{799}{81} L_{iiij}^{V8,LR} + \frac{799}{81} L_{jjij}^{V8,LR} \\
& + \frac{1210}{27} L_{ijii}^{V,RR} + \frac{1210}{27} L_{ijjj}^{V,RR} \Bigg] + \alpha_s \alpha \Bigg[ \frac{3800}{81} L_{11ij}^{V1,LR} + \frac{668}{81} L_{22ij}^{V1,LR} + \frac{668}{81} L_{33ij}^{V1,LR} \\
& + \frac{67}{3} L_{11ij}^{V8,LR} + \frac{14}{9} L_{22ij}^{V8,LR} + \frac{14}{9} L_{33ij}^{V8,LR} + \frac{668}{81} L_{11ij}^{V,LR} + \frac{668}{81} L_{22ij}^{V,LR} + \frac{668}{81} L_{33ij}^{V,LR} \\
& + \frac{668}{81} L_{11ij}^{V,RR} + \frac{668}{81} L_{22ij}^{V,RR} + \frac{668}{81} L_{33ij}^{V,RR} + \frac{668}{81} L_{ij11}^{V1,RR} + \frac{668}{81} L_{ij22}^{V1,RR} + \frac{668}{81} L_{ij33}^{V1,RR} \\
& - \frac{70}{27} L_{ij11}^{V8,RR} - \frac{70}{27} L_{ij22}^{V8,RR} - \frac{70}{27} L_{ij33}^{V8,RR} - \frac{1336}{81} L_{iiij}^{V1,LR} - \frac{1336}{81} L_{jjij}^{V1,LR} - \frac{20}{3} L_{iiij}^{V8,LR} \\
& - \frac{20}{3} L_{jjij}^{V8,LR} - \frac{3800}{81} L_{ijii}^{V,RR} - \frac{3800}{81} L_{ijjj}^{V,RR} \Bigg] - \frac{4048}{81} \alpha^2 L_{11ij}^{V8,LR} ; \\
\dot{L}_{22ij}^{V1,LR} &= -\frac{8}{3} g_s^2 L_{22ij}^{V8,LR} + e^2 \Bigg[ \frac{4}{9} L_{11ij}^{V1,LR} + \frac{28}{9} L_{22ij}^{V1,LR} + \frac{4}{9} L_{33ij}^{V1,LR} + \frac{4}{9} L_{11ij}^{V,LR} \\
& + \frac{4}{9} L_{22ij}^{V,LR} + \frac{4}{9} L_{33ij}^{V,LR} + \frac{4}{9} L_{11ij}^{V,RR} + \frac{4}{9} L_{22ij}^{V,RR} + \frac{4}{9} L_{33ij}^{V,RR} + \frac{4}{9} L_{ij11}^{V1,RR} \\
& + \frac{4}{9} L_{ij22}^{V1,RR} + \frac{4}{9} L_{ij33}^{V1,RR} - \frac{8}{9} L_{iiij}^{V1,LR} - \frac{8}{9} L_{jjij}^{V1,LR} - \frac{64}{27} L_{ijii}^{V,RR} - \frac{64}{27} L_{ijjj}^{V,RR} \Bigg] \\
& + \alpha_s^2 \Bigg[ 8 L_{11ij}^{V1,LR} - \frac{4}{3} L_{22ij}^{V1,LR} + 8 L_{33ij}^{V1,LR} + \frac{44}{27} L_{11ij}^{V8,LR} - \frac{2000}{27} L_{22ij}^{V8,LR} \\
& + \frac{44}{27} L_{33ij}^{V8,LR} - 8 L_{ij11}^{V1,RR} - 8 L_{ij22}^{V1,RR} - 8 L_{ij33}^{V1,RR} + \frac{44}{27} L_{ij11}^{V8,RR} + \frac{44}{27} L_{ij22}^{V8,RR}
\end{aligned}$$

$$\begin{aligned}
& + \frac{44}{27} L_{ij33}^{V8,RR} + 8 L_{iijj}^{V1,LR} + 8 L_{jjij}^{V1,LR} + \frac{44}{27} L_{iijj}^{V8,LR} + \frac{44}{27} L_{jjij}^{V8,LR} - \frac{232}{9} L_{ijii}^{V,RR} \\
& - \frac{232}{9} L_{ijjj}^{V,RR} \Big] + \alpha_s \alpha \Big[ \frac{16}{9} L_{11ij}^{V1,LR} - \frac{176}{9} L_{22ij}^{V1,LR} + \frac{16}{9} L_{33ij}^{V1,LR} - \frac{392}{729} L_{11ij}^{V8,LR} \\
& + \frac{5872}{729} L_{22ij}^{V8,LR} - \frac{392}{729} L_{33ij}^{V8,LR} + \frac{16}{9} L_{ij11}^{V1,RR} + \frac{16}{9} L_{ij22}^{V1,RR} + \frac{16}{9} L_{ij33}^{V1,RR} + \frac{328}{729} L_{ij11}^{V8,RR} \\
& + \frac{328}{729} L_{ij22}^{V8,RR} + \frac{328}{729} L_{ij33}^{V8,RR} - \frac{32}{9} L_{iijj}^{V1,LR} - \frac{32}{9} L_{jjij}^{V1,LR} + \frac{1984}{729} L_{iijj}^{V8,LR} + \frac{1984}{729} L_{jjij}^{V8,LR} \\
& - \frac{2240}{243} L_{ijii}^{V,RR} - \frac{2240}{243} L_{ijjj}^{V,RR} \Big] + \alpha^2 \Big[ - \frac{112}{729} L_{11ij}^{V1,LR} - \frac{36544}{729} L_{22ij}^{V1,LR} - \frac{112}{729} L_{33ij}^{V1,LR} \\
& + \frac{2984}{729} L_{11ij}^{V,LR} + \frac{2984}{729} L_{22ij}^{V,LR} + \frac{2984}{729} L_{33ij}^{V,LR} - \frac{1120}{729} L_{11ij}^{V,RR} - \frac{1120}{729} L_{22ij}^{V,RR} \\
& - \frac{1120}{729} L_{33ij}^{V,RR} - \frac{1480}{729} L_{ij11}^{V1,RR} - \frac{1480}{729} L_{ij22}^{V1,RR} - \frac{1480}{729} L_{ij33}^{V1,RR} + \frac{6272}{729} L_{iijj}^{V1,LR} \\
& + \frac{6272}{729} L_{jjij}^{V1,LR} + \frac{4000}{729} L_{iijj}^{V,RR} + \frac{4000}{729} L_{jjij}^{V,RR} \Big] ;
\end{aligned}$$

$$\begin{aligned}
\dot{L}_{22ij}^{V8,LR} & = g_s^2 \Big[ -12 L_{22ij}^{V1,LR} + \frac{2}{3} L_{11ij}^{V8,LR} - \frac{40}{3} L_{22ij}^{V8,LR} + \frac{2}{3} L_{33ij}^{V8,LR} + \frac{2}{3} L_{ij11}^{V8,RR} \\
& + \frac{2}{3} L_{ij22}^{V8,RR} + \frac{2}{3} L_{ij33}^{V8,RR} + \frac{2}{3} L_{iijj}^{V8,LR} + \frac{2}{3} L_{jjij}^{V8,LR} + \frac{8}{3} L_{ijii}^{V,RR} + \frac{8}{3} L_{ijjj}^{V,RR} \Big] \\
& + \frac{8}{3} e^2 L_{22ij}^{V8,LR} + \alpha_s^2 \Big[ - \frac{22}{3} L_{11ij}^{V1,LR} - 132 L_{22ij}^{V1,LR} - \frac{22}{3} L_{33ij}^{V1,LR} + \frac{799}{81} L_{11ij}^{V8,LR} \\
& - \frac{25177}{162} L_{22ij}^{V8,LR} + \frac{799}{81} L_{33ij}^{V8,LR} - \frac{2}{3} L_{ij11}^{V1,RR} - \frac{2}{3} L_{ij22}^{V1,RR} - \frac{2}{3} L_{ij33}^{V1,RR} + \frac{619}{81} L_{ij11}^{V8,RR} \\
& + \frac{619}{81} L_{ij22}^{V8,RR} + \frac{619}{81} L_{ij33}^{V8,RR} - \frac{22}{3} L_{iijj}^{V1,LR} - \frac{22}{3} L_{jjij}^{V1,LR} + \frac{799}{81} L_{iijj}^{V8,LR} + \frac{799}{81} L_{jjij}^{V8,LR} \\
& + \frac{1210}{27} L_{ijii}^{V,RR} + \frac{1210}{27} L_{ijjj}^{V,RR} \Big] + \alpha_s \alpha \Big[ \frac{668}{81} L_{11ij}^{V1,LR} + \frac{3800}{81} L_{22ij}^{V1,LR} + \frac{668}{81} L_{33ij}^{V1,LR} \\
& + \frac{14}{9} L_{11ij}^{V8,LR} + \frac{67}{3} L_{22ij}^{V8,LR} + \frac{14}{9} L_{33ij}^{V8,LR} + \frac{668}{81} L_{11ij}^{V,LR} + \frac{668}{81} L_{22ij}^{V,LR} + \frac{668}{81} L_{33ij}^{V,LR} \\
& + \frac{668}{81} L_{11ij}^{V,RR} + \frac{668}{81} L_{22ij}^{V,RR} + \frac{668}{81} L_{33ij}^{V,RR} + \frac{668}{81} L_{ij11}^{V1,RR} + \frac{668}{81} L_{ij22}^{V1,RR} + \frac{668}{81} L_{ij33}^{V1,RR}
\end{aligned}$$

$$\begin{aligned}
& -\frac{70}{27}L_{ud\,ij11}^{V8,RR} - \frac{70}{27}L_{ud\,ij22}^{V8,RR} - \frac{70}{27}L_{ud\,ij33}^{V8,RR} - \frac{1336}{81}L_{uu\,iiij}^{V1,LR} - \frac{1336}{81}L_{uu\,jjij}^{V1,LR} - \frac{20}{3}L_{uu\,iiij}^{V8,LR} \\
& - \frac{20}{3}L_{uu\,jjij}^{V8,LR} - \frac{3800}{81}L_{uu\,ijii}^{V,RR} - \frac{3800}{81}L_{uu\,ijjj}^{V,RR} \Big] - \frac{4048}{81}\alpha^2 L_{du\,22ij}^{V8,LR} ; \\
\dot{L}_{du\,33ij}^{V1,LR} = & -\frac{8}{3}g_s^2 L_{du\,33ij}^{V8,LR} + e^2 \Bigg[ \frac{4}{9}L_{du\,11ij}^{V1,LR} + \frac{4}{9}L_{du\,22ij}^{V1,LR} + \frac{28}{9}L_{du\,33ij}^{V1,LR} + \frac{4}{9}L_{eu\,11ij}^{V,LR} \\
& + \frac{4}{9}L_{eu\,22ij}^{V,LR} + \frac{4}{9}L_{eu\,33ij}^{V,LR} + \frac{4}{9}L_{eu\,11ij}^{V,RR} + \frac{4}{9}L_{eu\,22ij}^{V,RR} + \frac{4}{9}L_{eu\,33ij}^{V,RR} + \frac{4}{9}L_{ud\,ij11}^{V1,RR} \\
& + \frac{4}{9}L_{ud\,ij22}^{V1,RR} + \frac{4}{9}L_{ud\,ij33}^{V1,RR} - \frac{8}{9}L_{uu\,iiij}^{V1,LR} - \frac{8}{9}L_{uu\,jjij}^{V1,LR} - \frac{64}{27}L_{uu\,ijii}^{V,RR} - \frac{64}{27}L_{uu\,ijjj}^{V,RR} \Big] \\
& + \alpha_s^2 \Bigg[ 8L_{du\,11ij}^{V1,LR} + 8L_{du\,22ij}^{V1,LR} - \frac{4}{3}L_{du\,33ij}^{V1,LR} + \frac{44}{27}L_{du\,11ij}^{V8,LR} + \frac{44}{27}L_{du\,22ij}^{V8,LR} \\
& - \frac{2000}{27}L_{du\,33ij}^{V8,LR} - 8L_{ud\,ij11}^{V1,RR} - 8L_{ud\,ij22}^{V1,RR} - 8L_{ud\,ij33}^{V1,RR} + \frac{44}{27}L_{ud\,ij11}^{V8,RR} + \frac{44}{27}L_{ud\,ij22}^{V8,RR} \\
& + \frac{44}{27}L_{ud\,ij33}^{V8,RR} + 8L_{uu\,iiij}^{V1,LR} + 8L_{uu\,jjij}^{V1,LR} + \frac{44}{27}L_{uu\,iiij}^{V8,LR} + \frac{44}{27}L_{uu\,jjij}^{V8,LR} - \frac{232}{9}L_{uu\,ijii}^{V,RR} \\
& - \frac{232}{9}L_{uu\,ijjj}^{V,RR} \Big] + \alpha_s \alpha \Bigg[ \frac{16}{9}L_{du\,11ij}^{V1,LR} + \frac{16}{9}L_{du\,22ij}^{V1,LR} - \frac{176}{9}L_{du\,33ij}^{V1,LR} - \frac{392}{729}L_{du\,11ij}^{V8,LR} \\
& - \frac{392}{729}L_{du\,22ij}^{V8,LR} + \frac{5872}{729}L_{du\,33ij}^{V8,LR} + \frac{16}{9}L_{ud\,ij11}^{V1,RR} + \frac{16}{9}L_{ud\,ij22}^{V1,RR} + \frac{16}{9}L_{ud\,ij33}^{V1,RR} + \frac{328}{729}L_{ud\,ij11}^{V8,RR} \\
& + \frac{328}{729}L_{ud\,ij22}^{V8,RR} + \frac{328}{729}L_{ud\,ij33}^{V8,RR} - \frac{32}{9}L_{uu\,iiij}^{V1,LR} - \frac{32}{9}L_{uu\,jjij}^{V1,LR} + \frac{1984}{729}L_{uu\,iiij}^{V8,LR} + \frac{1984}{729}L_{uu\,jjij}^{V8,LR} \\
& - \frac{2240}{243}L_{uu\,ijii}^{V,RR} - \frac{2240}{243}L_{uu\,ijjj}^{V,RR} \Big] + \alpha^2 \Bigg[ -\frac{112}{729}L_{du\,11ij}^{V1,LR} - \frac{112}{729}L_{du\,22ij}^{V1,LR} - \frac{36544}{729}L_{du\,33ij}^{V1,LR} \\
& + \frac{2984}{729}L_{eu\,11ij}^{V,LR} + \frac{2984}{729}L_{eu\,22ij}^{V,LR} + \frac{2984}{729}L_{eu\,33ij}^{V,LR} - \frac{1120}{729}L_{eu\,11ij}^{V,RR} - \frac{1120}{729}L_{eu\,22ij}^{V,RR} \\
& - \frac{1120}{729}L_{eu\,33ij}^{V,RR} - \frac{1480}{729}L_{ud\,ij11}^{V1,RR} - \frac{1480}{729}L_{ud\,ij22}^{V1,RR} - \frac{1480}{729}L_{ud\,ij33}^{V1,RR} + \frac{6272}{729}L_{uu\,iiij}^{V1,LR} \\
& + \frac{6272}{729}L_{uu\,jjij}^{V1,LR} + \frac{4000}{729}L_{uu\,ijii}^{V,RR} + \frac{4000}{729}L_{uu\,ijjj}^{V,RR} \Big] ; \\
\dot{L}_{du\,33ij}^{V8,LR} = & g_s^2 \Bigg[ -12L_{du\,33ij}^{V1,LR} + \frac{2}{3}L_{du\,11ij}^{V8,LR} + \frac{2}{3}L_{du\,22ij}^{V8,LR} - \frac{40}{3}L_{du\,33ij}^{V8,LR} + \frac{2}{3}L_{ud\,ij11}^{V8,RR}
\end{aligned}$$

$$\begin{aligned}
& + \frac{2}{3} L_{ij22}^{V8,RR} + \frac{2}{3} L_{ij33}^{V8,RR} + \frac{2}{3} L_{iij}^{V8,LR} + \frac{2}{3} L_{jjij}^{V8,LR} + \frac{8}{3} L_{ijii}^{V,RR} + \frac{8}{3} L_{ijjj}^{V,RR} \Big] \\
& + \frac{8}{3} e^2 L_{33ij}^{V8,LR} + \alpha_s^2 \left[ -\frac{22}{3} L_{11ij}^{V1,LR} - \frac{22}{3} L_{22ij}^{V1,LR} - 132 L_{33ij}^{V1,LR} + \frac{799}{81} L_{11ij}^{V8,LR} \right. \\
& + \frac{799}{81} L_{22ij}^{V8,LR} - \frac{25177}{162} L_{33ij}^{V8,LR} - \frac{2}{3} L_{ij11}^{V1,RR} - \frac{2}{3} L_{ij22}^{V1,RR} - \frac{2}{3} L_{ij33}^{V1,RR} + \frac{619}{81} L_{ij11}^{V8,RR} \\
& + \frac{619}{81} L_{ij22}^{V8,RR} + \frac{619}{81} L_{ij33}^{V8,RR} - \frac{22}{3} L_{iij}^{V1,LR} - \frac{22}{3} L_{jjij}^{V1,LR} + \frac{799}{81} L_{iij}^{V8,LR} + \frac{799}{81} L_{jjij}^{V8,LR} \\
& \left. + \frac{1210}{27} L_{ijii}^{V,RR} + \frac{1210}{27} L_{ijjj}^{V,RR} \right] + \alpha_s \alpha \left[ \frac{668}{81} L_{11ij}^{V1,LR} + \frac{668}{81} L_{22ij}^{V1,LR} + \frac{3800}{81} L_{33ij}^{V1,LR} \right. \\
& + \frac{14}{9} L_{11ij}^{V8,LR} + \frac{14}{9} L_{22ij}^{V8,LR} + \frac{67}{3} L_{33ij}^{V8,LR} + \frac{668}{81} L_{11ij}^{V,LR} + \frac{668}{81} L_{22ij}^{V,LR} + \frac{668}{81} L_{33ij}^{V,LR} \\
& + \frac{668}{81} L_{11ij}^{V,RR} + \frac{668}{81} L_{22ij}^{V,RR} + \frac{668}{81} L_{33ij}^{V,RR} + \frac{668}{81} L_{ij11}^{V1,RR} + \frac{668}{81} L_{ij22}^{V1,RR} + \frac{668}{81} L_{ij33}^{V1,RR} \\
& - \frac{70}{27} L_{ij11}^{V8,RR} - \frac{70}{27} L_{ij22}^{V8,RR} - \frac{70}{27} L_{ij33}^{V8,RR} - \frac{1336}{81} L_{iij}^{V1,LR} - \frac{1336}{81} L_{jjij}^{V1,LR} - \frac{20}{3} L_{iij}^{V8,LR} \\
& \left. - \frac{20}{3} L_{jjij}^{V8,LR} - \frac{3800}{81} L_{ijii}^{V,RR} - \frac{3800}{81} L_{ijjj}^{V,RR} \right] - \frac{4048}{81} \alpha^2 L_{33ij}^{V8,LR} ;
\end{aligned}$$

$$\begin{aligned}
\dot{L}_{jjij}^{V1,LR} & = -\frac{8}{3} g_s^2 L_{jjij}^{V8,LR} + e^2 \left[ -\frac{8}{9} L_{11ij}^{V1,LR} - \frac{8}{9} L_{22ij}^{V1,LR} - \frac{8}{9} L_{33ij}^{V1,LR} - \frac{8}{9} L_{11ij}^{V,LR} \right. \\
& - \frac{8}{9} L_{22ij}^{V,LR} - \frac{8}{9} L_{33ij}^{V,LR} - \frac{8}{9} L_{11ij}^{V,RR} - \frac{8}{9} L_{22ij}^{V,RR} - \frac{8}{9} L_{33ij}^{V,RR} - \frac{8}{9} L_{ij11}^{V1,RR} \\
& \left. - \frac{8}{9} L_{ij22}^{V1,RR} - \frac{8}{9} L_{ij33}^{V1,RR} + \frac{16}{9} L_{iij}^{V1,LR} - \frac{32}{9} L_{jjij}^{V1,LR} + \frac{128}{27} L_{ijii}^{V,RR} + \frac{128}{27} L_{ijjj}^{V,RR} \right] \\
& + \alpha_s^2 \left[ 8 L_{11ij}^{V1,LR} + 8 L_{22ij}^{V1,LR} + 8 L_{33ij}^{V1,LR} + \frac{44}{27} L_{11ij}^{V8,LR} + \frac{44}{27} L_{22ij}^{V8,LR} \right. \\
& + \frac{44}{27} L_{33ij}^{V8,LR} - 8 L_{ij11}^{V1,RR} - 8 L_{ij22}^{V1,RR} - 8 L_{ij33}^{V1,RR} + \frac{44}{27} L_{ij11}^{V8,RR} + \frac{44}{27} L_{ij22}^{V8,RR} \\
& + \frac{44}{27} L_{ij33}^{V8,RR} + 8 L_{iij}^{V1,LR} - \frac{4}{3} L_{jjij}^{V1,LR} + \frac{44}{27} L_{iij}^{V8,LR} - \frac{2000}{27} L_{jjij}^{V8,LR} - \frac{232}{9} L_{ijii}^{V,RR} \\
& \left. - \frac{232}{9} L_{ijjj}^{V,RR} \right] + \alpha_s \alpha \left[ -\frac{32}{9} L_{11ij}^{V1,LR} - \frac{32}{9} L_{22ij}^{V1,LR} - \frac{32}{9} L_{33ij}^{V1,LR} + \frac{784}{729} L_{11ij}^{V8,LR} \right.
\end{aligned}$$

$$\begin{aligned}
& + \frac{784}{729} L_{22ij}^{V8,LR} + \frac{784}{729} L_{33ij}^{V8,LR} - \frac{32}{9} L_{ij11}^{V1,RR} - \frac{32}{9} L_{ij22}^{V1,RR} - \frac{32}{9} L_{ij33}^{V1,RR} - \frac{656}{729} L_{ij11}^{V8,RR} \\
& - \frac{656}{729} L_{ij22}^{V8,RR} - \frac{656}{729} L_{ij33}^{V8,RR} + \frac{64}{9} L_{iiij}^{V1,LR} + \frac{448}{9} L_{jjij}^{V1,LR} - \frac{3968}{729} L_{iiij}^{V8,LR} \\
& - \frac{4832}{729} L_{jjij}^{V8,LR} + \frac{4480}{243} L_{ijii}^{V,RR} + \frac{4480}{243} L_{ijjj}^{V,RR} \Big] + \alpha^2 \Big[ - \frac{2584}{729} L_{11ij}^{V1,LR} - \frac{2584}{729} L_{22ij}^{V1,LR} \\
& - \frac{2584}{729} L_{33ij}^{V1,LR} - \frac{4888}{729} L_{11ij}^{V,LR} - \frac{4888}{729} L_{22ij}^{V,LR} - \frac{4888}{729} L_{33ij}^{V,LR} - \frac{8344}{729} L_{11ij}^{V,RR} \\
& - \frac{8344}{729} L_{22ij}^{V,RR} - \frac{8344}{729} L_{33ij}^{V,RR} - \frac{3736}{729} L_{ij11}^{V1,RR} - \frac{3736}{729} L_{ij22}^{V1,RR} - \frac{3736}{729} L_{ij33}^{V1,RR} \\
& + \frac{4736}{729} L_{iiij}^{V1,LR} + \frac{72416}{729} L_{jjij}^{V1,LR} - \frac{9728}{729} L_{ijii}^{V,RR} - \frac{9728}{729} L_{ijjj}^{V,RR} \Big] ;
\end{aligned}$$

$$\begin{aligned}
\dot{L}_{jjij}^{V8,LR} & = g_s^2 \Big[ \frac{2}{3} L_{11ij}^{V8,LR} + \frac{2}{3} L_{22ij}^{V8,LR} + \frac{2}{3} L_{33ij}^{V8,LR} + \frac{2}{3} L_{ij11}^{V8,RR} + \frac{2}{3} L_{ij22}^{V8,RR} \\
& + \frac{2}{3} L_{ij33}^{V8,RR} - 12 L_{jjij}^{V1,LR} + \frac{2}{3} L_{iiij}^{V8,LR} - \frac{40}{3} L_{jjij}^{V8,LR} + \frac{8}{3} L_{ijii}^{V,RR} + \frac{8}{3} L_{ijjj}^{V,RR} \Big] \\
& - \frac{16}{3} e^2 L_{jjij}^{V8,LR} + \alpha_s^2 \Big[ - \frac{22}{3} L_{11ij}^{V1,LR} - \frac{22}{3} L_{22ij}^{V1,LR} - \frac{22}{3} L_{33ij}^{V1,LR} + \frac{799}{81} L_{11ij}^{V8,LR} \\
& + \frac{799}{81} L_{22ij}^{V8,LR} + \frac{799}{81} L_{33ij}^{V8,LR} - \frac{2}{3} L_{ij11}^{V1,RR} - \frac{2}{3} L_{ij22}^{V1,RR} - \frac{2}{3} L_{ij33}^{V1,RR} + \frac{619}{81} L_{ij11}^{V8,RR} \\
& + \frac{619}{81} L_{ij22}^{V8,RR} + \frac{619}{81} L_{ij33}^{V8,RR} - \frac{22}{3} L_{iiij}^{V1,LR} - 132 L_{jjij}^{V1,LR} + \frac{799}{81} L_{iiij}^{V8,LR} - \frac{25177}{162} L_{jjij}^{V8,LR} \\
& + \frac{1210}{27} L_{ijii}^{V,RR} + \frac{1210}{27} L_{ijjj}^{V,RR} \Big] + \alpha_s \alpha \Big[ - \frac{520}{81} L_{11ij}^{V1,LR} - \frac{520}{81} L_{22ij}^{V1,LR} - \frac{520}{81} L_{33ij}^{V1,LR} \\
& + \frac{22}{9} L_{11ij}^{V8,LR} + \frac{22}{9} L_{22ij}^{V8,LR} + \frac{22}{9} L_{33ij}^{V8,LR} - \frac{520}{81} L_{11ij}^{V,LR} - \frac{520}{81} L_{22ij}^{V,LR} - \frac{520}{81} L_{33ij}^{V,LR} \\
& - \frac{520}{81} L_{11ij}^{V,RR} - \frac{520}{81} L_{22ij}^{V,RR} - \frac{520}{81} L_{33ij}^{V,RR} - \frac{520}{81} L_{ij11}^{V1,RR} - \frac{520}{81} L_{ij22}^{V1,RR} - \frac{520}{81} L_{ij33}^{V1,RR} \\
& + \frac{170}{27} L_{ij11}^{V8,RR} + \frac{170}{27} L_{ij22}^{V8,RR} + \frac{170}{27} L_{ij33}^{V8,RR} + \frac{1040}{81} L_{iiij}^{V1,LR} + \frac{608}{81} L_{jjij}^{V1,LR} \\
& + \frac{56}{9} L_{iiij}^{V8,LR} - \frac{16}{3} L_{jjij}^{V8,LR} + \frac{1168}{81} L_{ijii}^{V,RR} + \frac{1168}{81} L_{ijjj}^{V,RR} \Big] + \frac{7520}{81} \alpha^2 L_{jjij}^{V8,LR} ;
\end{aligned}$$



$$\begin{aligned}
\dot{L}_{uu}^{V1,LR}{}_{iij} &= -\frac{8}{3}g_s^2 L_{iij}^{V8,LR} + e^2 \left[ -\frac{8}{9}L_{11ij}^{V1,LR} - \frac{8}{9}L_{22ij}^{V1,LR} - \frac{8}{9}L_{33ij}^{V1,LR} - \frac{8}{9}L_{11ij}^{V,LR} \right. \\
&\quad - \frac{8}{9}L_{22ij}^{V,LR} - \frac{8}{9}L_{33ij}^{V,LR} - \frac{8}{9}L_{11ij}^{V,RR} - \frac{8}{9}L_{22ij}^{V,RR} - \frac{8}{9}L_{33ij}^{V,RR} - \frac{8}{9}L_{ij11}^{V1,RR} \\
&\quad \left. - \frac{8}{9}L_{ij22}^{V1,RR} - \frac{8}{9}L_{ij33}^{V1,RR} - \frac{32}{9}L_{iij}^{V1,LR} + \frac{16}{9}L_{jjij}^{V1,LR} + \frac{128}{27}L_{iij}^{V,RR} + \frac{128}{27}L_{ijjj}^{V,RR} \right] \\
&\quad + \alpha_s^2 \left[ 8L_{11ij}^{V1,LR} + 8L_{22ij}^{V1,LR} + 8L_{33ij}^{V1,LR} + \frac{44}{27}L_{11ij}^{V8,LR} + \frac{44}{27}L_{22ij}^{V8,LR} \right. \\
&\quad + \frac{44}{27}L_{33ij}^{V8,LR} - 8L_{ij11}^{V1,RR} - 8L_{ij22}^{V1,RR} - 8L_{ij33}^{V1,RR} + \frac{44}{27}L_{ij11}^{V8,RR} + \frac{44}{27}L_{ij22}^{V8,RR} \\
&\quad + \frac{44}{27}L_{ij33}^{V8,RR} - \frac{4}{3}L_{iij}^{V1,LR} + 8L_{jjij}^{V1,LR} - \frac{2000}{27}L_{iij}^{V8,LR} + \frac{44}{27}L_{jjij}^{V8,LR} - \frac{232}{9}L_{iij}^{V,RR} \\
&\quad \left. - \frac{232}{9}L_{ijjj}^{V,RR} \right] + \alpha_s \alpha \left[ -\frac{32}{9}L_{11ij}^{V1,LR} - \frac{32}{9}L_{22ij}^{V1,LR} - \frac{32}{9}L_{33ij}^{V1,LR} + \frac{784}{729}L_{11ij}^{V8,LR} \right. \\
&\quad + \frac{784}{729}L_{22ij}^{V8,LR} + \frac{784}{729}L_{33ij}^{V8,LR} - \frac{32}{9}L_{ij11}^{V1,RR} - \frac{32}{9}L_{ij22}^{V1,RR} - \frac{32}{9}L_{ij33}^{V1,RR} - \frac{656}{729}L_{ij11}^{V8,RR} \\
&\quad - \frac{656}{729}L_{ij22}^{V8,RR} - \frac{656}{729}L_{ij33}^{V8,RR} + \frac{448}{9}L_{iij}^{V1,LR} + \frac{64}{9}L_{jjij}^{V1,LR} - \frac{4832}{729}L_{iij}^{V8,LR} \\
&\quad - \frac{3968}{729}L_{ijjj}^{V8,LR} + \frac{4480}{243}L_{iij}^{V,RR} + \frac{4480}{243}L_{ijjj}^{V,RR} \left. \right] + \alpha^2 \left[ -\frac{2584}{729}L_{11ij}^{V1,LR} - \frac{2584}{729}L_{22ij}^{V1,LR} \right. \\
&\quad - \frac{2584}{729}L_{33ij}^{V1,LR} - \frac{4888}{729}L_{11ij}^{V,LR} - \frac{4888}{729}L_{22ij}^{V,LR} - \frac{4888}{729}L_{33ij}^{V,LR} - \frac{8344}{729}L_{11ij}^{V,RR} \\
&\quad - \frac{8344}{729}L_{22ij}^{V,RR} - \frac{8344}{729}L_{33ij}^{V,RR} - \frac{3736}{729}L_{ij11}^{V1,RR} - \frac{3736}{729}L_{ij22}^{V1,RR} - \frac{3736}{729}L_{ij33}^{V1,RR} \\
&\quad \left. + \frac{72416}{729}L_{iij}^{V1,LR} + \frac{4736}{729}L_{jjij}^{V1,LR} - \frac{9728}{729}L_{iij}^{V,RR} - \frac{9728}{729}L_{ijjj}^{V,RR} \right];
\end{aligned}$$

$$\begin{aligned}
\dot{L}_{uu}^{V8,LR}{}_{iij} &= g_s^2 \left[ \frac{2}{3}L_{11ij}^{V8,LR} + \frac{2}{3}L_{22ij}^{V8,LR} + \frac{2}{3}L_{33ij}^{V8,LR} + \frac{2}{3}L_{ij11}^{V8,RR} + \frac{2}{3}L_{ij22}^{V8,RR} \right. \\
&\quad \left. + \frac{2}{3}L_{ij33}^{V8,RR} - 12L_{iij}^{V1,LR} - \frac{40}{3}L_{jjij}^{V8,LR} + \frac{2}{3}L_{jjij}^{V8,LR} + \frac{8}{3}L_{iij}^{V,RR} + \frac{8}{3}L_{ijjj}^{V,RR} \right] \\
&\quad - \frac{16}{3}e^2 L_{iij}^{V8,LR} + \alpha_s^2 \left[ -\frac{22}{3}L_{11ij}^{V1,LR} - \frac{22}{3}L_{22ij}^{V1,LR} - \frac{22}{3}L_{33ij}^{V1,LR} + \frac{799}{81}L_{11ij}^{V8,LR} \right.
\end{aligned}$$

$$\begin{aligned}
& + \frac{799}{81} L_{22ij}^{V8,LR} + \frac{799}{81} L_{33ij}^{V8,LR} - \frac{2}{3} L_{ij11}^{V1,RR} - \frac{2}{3} L_{ij22}^{V1,RR} - \frac{2}{3} L_{ij33}^{V1,RR} + \frac{619}{81} L_{ij11}^{V8,RR} \\
& + \frac{619}{81} L_{ij22}^{V8,RR} + \frac{619}{81} L_{ij33}^{V8,RR} - 132 L_{iiij}^{V1,LR} - \frac{22}{3} L_{jjij}^{V1,LR} - \frac{25177}{162} L_{iiij}^{V8,LR} + \frac{799}{81} L_{jjij}^{V8,LR} \\
& + \frac{1210}{27} L_{ijii}^{V,RR} + \frac{1210}{27} L_{ijjj}^{V,RR} \Big] + \alpha_s \alpha \Big[ - \frac{520}{81} L_{11ij}^{V1,LR} - \frac{520}{81} L_{22ij}^{V1,LR} - \frac{520}{81} L_{33ij}^{V1,LR} \\
& + \frac{22}{9} L_{11ij}^{V8,LR} + \frac{22}{9} L_{22ij}^{V8,LR} + \frac{22}{9} L_{33ij}^{V8,LR} - \frac{520}{81} L_{11ij}^{V,LR} - \frac{520}{81} L_{22ij}^{V,LR} - \frac{520}{81} L_{33ij}^{V,LR} \\
& - \frac{520}{81} L_{11ij}^{V,RR} - \frac{520}{81} L_{22ij}^{V,RR} - \frac{520}{81} L_{33ij}^{V,RR} - \frac{520}{81} L_{ij11}^{V1,RR} - \frac{520}{81} L_{ij22}^{V1,RR} - \frac{520}{81} L_{ij33}^{V1,RR} \\
& + \frac{170}{27} L_{ij11}^{V8,RR} + \frac{170}{27} L_{ij22}^{V8,RR} + \frac{170}{27} L_{ij33}^{V8,RR} + \frac{608}{81} L_{iiij}^{V1,LR} + \frac{1040}{81} L_{jjij}^{V1,LR} \\
& - \frac{16}{3} L_{iiij}^{V8,LR} + \frac{56}{9} L_{jjij}^{V8,LR} + \frac{1168}{81} L_{ijii}^{V,RR} + \frac{1168}{81} L_{ijjj}^{V,RR} \Big] + \frac{7520}{81} \alpha^2 L_{iiij}^{V8,LR} ;
\end{aligned}$$

$$\dot{L}_{11ij}^{V,LL} = 0 ;$$

$$\dot{L}_{22ij}^{V,LL} = 0 ;$$

$$\dot{L}_{33ij}^{V,LL} = 0 ;$$

$$\dot{L}_{11ij}^{V,LR} = 0 ;$$

$$\dot{L}_{22ij}^{V,LR} = 0 ;$$

$$\dot{L}_{33ij}^{V,LR} = 0 ;$$

$$\begin{aligned}
\dot{L}_{11ij}^{S,LR} &= -8g_s^2 L_{11ij}^{S,LR} - \frac{8}{3} e^2 L_{11ij}^{S,LR} - \frac{1012}{9} \alpha_s^2 L_{11ij}^{S,LR} - \frac{32}{9} \alpha_s \alpha L_{11ij}^{S,LR} \\
&+ \frac{1552}{81} \alpha^2 L_{11ij}^{S,LR} ;
\end{aligned}$$

$$\begin{aligned}
\dot{L}_{22ij}^{S,LR} &= -8g_s^2 L_{22ij}^{S,LR} - \frac{8}{3} e^2 L_{22ij}^{S,LR} - \frac{1012}{9} \alpha_s^2 L_{22ij}^{S,LR} - \frac{32}{9} \alpha_s \alpha L_{22ij}^{S,LR} \\
&+ \frac{1552}{81} \alpha^2 L_{22ij}^{S,LR} ;
\end{aligned}$$

$$\begin{aligned}
\dot{L}_{33ij}^{S,LR} &= -8g_s^2 L_{33ij}^{S,LR} - \frac{8}{3} e^2 L_{33ij}^{S,LR} - \frac{1012}{9} \alpha_s^2 L_{33ij}^{S,LR} - \frac{32}{9} \alpha_s \alpha L_{33ij}^{S,LR} \\
&+ \frac{1552}{81} \alpha^2 L_{33ij}^{S,LR} ;
\end{aligned}$$

$$\begin{aligned}
\dot{L}_{11ij}^{S,LL} &= -8g_s^2 L_{11ij}^{S,LL} - \frac{8}{3}e^2 L_{11ij}^{S,LL} - \frac{1012}{9}\alpha_s^2 L_{11ij}^{S,LL} - \frac{32}{9}\alpha_s \alpha L_{11ij}^{S,LL} \\
&\quad + \frac{1552}{81}\alpha^2 L_{11ij}^{S,LL} ; \\
\dot{L}_{11ij}^{T,LL} &= \frac{8}{3}g_s^2 L_{11ij}^{T,LL} + \frac{8}{9}e^2 L_{11ij}^{T,LL} + \frac{1652}{27}\alpha_s^2 L_{11ij}^{T,LL} - \frac{608}{27}\alpha_s \alpha L_{11ij}^{T,LL} \\
&\quad - \frac{5072}{243}\alpha^2 L_{11ij}^{T,LL} ; \\
\dot{L}_{22ij}^{S,LL} &= -8g_s^2 L_{22ij}^{S,LL} - \frac{8}{3}e^2 L_{22ij}^{S,LL} - \frac{1012}{9}\alpha_s^2 L_{22ij}^{S,LL} - \frac{32}{9}\alpha_s \alpha L_{22ij}^{S,LL} \\
&\quad + \frac{1552}{81}\alpha^2 L_{22ij}^{S,LL} ; \\
\dot{L}_{22ij}^{T,LL} &= \frac{8}{3}g_s^2 L_{22ij}^{T,LL} + \frac{8}{9}e^2 L_{22ij}^{T,LL} + \frac{1652}{27}\alpha_s^2 L_{22ij}^{T,LL} - \frac{608}{27}\alpha_s \alpha L_{22ij}^{T,LL} \\
&\quad - \frac{5072}{243}\alpha^2 L_{22ij}^{T,LL} ; \\
\dot{L}_{33ij}^{S,LL} &= -8g_s^2 L_{33ij}^{S,LL} - \frac{8}{3}e^2 L_{33ij}^{S,LL} - \frac{1012}{9}\alpha_s^2 L_{33ij}^{S,LL} - \frac{32}{9}\alpha_s \alpha L_{33ij}^{S,LL} \\
&\quad + \frac{1552}{81}\alpha^2 L_{33ij}^{S,LL} ; \\
\dot{L}_{33ij}^{T,LL} &= \frac{8}{3}g_s^2 L_{33ij}^{T,LL} + \frac{8}{9}e^2 L_{33ij}^{T,LL} + \frac{1652}{27}\alpha_s^2 L_{33ij}^{T,LL} - \frac{608}{27}\alpha_s \alpha L_{33ij}^{T,LL} \\
&\quad - \frac{5072}{243}\alpha^2 L_{33ij}^{T,LL} ;
\end{aligned}$$

### 1.7 $\Delta F = 1^{\bar{f}f} : e\text{-type } (\bar{e}_i e_j \bar{f}_k f_k)$

$$\begin{aligned}
\dot{L}_{ij11}^{V,LL} &= e^2 \left[ \frac{16}{9}L_{ijkk}^{V,LL} + \frac{4}{9}L_{ijkk}^{V,LR} + \frac{40}{9}L_{ij11}^{V,LL} + \frac{4}{9}L_{ij22}^{V,LL} + \frac{4}{9}L_{ij33}^{V,LL} \right. \\
&\quad + \frac{4}{9}L_{ij11}^{V,LR} + \frac{4}{9}L_{ij22}^{V,LR} + \frac{4}{9}L_{ij33}^{V,LR} + \frac{16}{9}L_{ijii}^{V,LL} + \frac{16}{9}L_{ijjj}^{V,LL} + \frac{4}{9}L_{ijii}^{V,LR} \\
&\quad + \frac{4}{9}L_{ijjj}^{V,LR} - \frac{8}{9}L_{ij11}^{V,LL} - \frac{8}{9}L_{ij22}^{V,LL} - \frac{8}{9}L_{ij11}^{V,LR} - \frac{8}{9}L_{ij22}^{V,LR} \left. \right] + \alpha_s^2 \left[ 8L_{ij11}^{V,LL} \right. \\
&\quad + 8L_{ij22}^{V,LL} + 8L_{ij33}^{V,LL} - 8L_{ij11}^{V,LR} - 8L_{ij22}^{V,LR} - 8L_{ij33}^{V,LR} + 8L_{ij11}^{V,LL} \\
&\quad + 8L_{ij22}^{V,LL} - 8L_{ij11}^{V,LR} - 8L_{ij22}^{V,LR} \left. \right] + \alpha_s \alpha \left[ -\frac{128}{9}L_{ij11}^{V,LL} + \frac{16}{9}L_{ij22}^{V,LL} \right.
\end{aligned}$$

$$\begin{aligned}
& + \frac{16}{9} L_{ij33}^{V,LL} + \frac{16}{9} L_{ij11}^{V,LR} + \frac{16}{9} L_{ij22}^{V,LR} + \frac{16}{9} L_{ij33}^{V,LR} - \frac{32}{9} L_{ij11}^{V,LL} - \frac{32}{9} L_{ij22}^{V,LL} \\
& - \frac{32}{9} L_{ij11}^{V,LR} - \frac{32}{9} L_{ij22}^{V,LR} \Big] + \alpha^2 \Big[ \frac{224}{81} L_{ijkk}^{V,LL} - \frac{520}{81} L_{ijkk}^{V,LR} - \frac{3038}{243} L_{ij11}^{V,LL} \\
& - \frac{104}{243} L_{ij22}^{V,LL} - \frac{104}{243} L_{ij33}^{V,LL} - \frac{200}{243} L_{ij11}^{V,LR} - \frac{200}{243} L_{ij22}^{V,LR} - \frac{200}{243} L_{ij33}^{V,LR} + \frac{32}{81} L_{ijii}^{V,LL} \\
& + \frac{32}{81} L_{ijjj}^{V,LL} - \frac{520}{81} L_{ijii}^{V,LR} - \frac{520}{81} L_{ijjj}^{V,LR} - \frac{1016}{243} L_{ij11}^{V,LL} - \frac{1016}{243} L_{ij22}^{V,LL} - \frac{1400}{243} L_{ij11}^{V,LR} \\
& - \frac{1400}{243} L_{ij22}^{V,LR} \Big] ;
\end{aligned}$$

$$\begin{aligned}
\dot{L}_{ed\ ij22}^{V,LL} &= e^2 \Big[ \frac{16}{9} L_{ijkk}^{V,LL} + \frac{4}{9} L_{ijkk}^{V,LR} + \frac{4}{9} L_{ij11}^{V,LL} + \frac{40}{9} L_{ed\ ij22}^{V,LL} + \frac{4}{9} L_{ij33}^{V,LL} \\
& + \frac{4}{9} L_{ed\ ij11}^{V,LR} + \frac{4}{9} L_{ed\ ij22}^{V,LR} + \frac{4}{9} L_{ed\ ij33}^{V,LR} + \frac{16}{9} L_{ijii}^{V,LL} + \frac{16}{9} L_{ijjj}^{V,LL} + \frac{4}{9} L_{ijii}^{V,LR} \\
& + \frac{4}{9} L_{ijjj}^{V,LR} - \frac{8}{9} L_{ij11}^{V,LL} - \frac{8}{9} L_{ij22}^{V,LL} - \frac{8}{9} L_{ij11}^{V,LR} - \frac{8}{9} L_{ij22}^{V,LR} \Big] + \alpha_s^2 \Big[ 8 L_{ed\ ij11}^{V,LL} \\
& + 8 L_{ed\ ij22}^{V,LL} + 8 L_{ed\ ij33}^{V,LL} - 8 L_{ed\ ij11}^{V,LR} - 8 L_{ed\ ij22}^{V,LR} - 8 L_{ed\ ij33}^{V,LR} + 8 L_{ij11}^{V,LL} \\
& + 8 L_{ij22}^{V,LL} - 8 L_{ij11}^{V,LR} - 8 L_{ij22}^{V,LR} \Big] + \alpha_s \alpha \Big[ \frac{16}{9} L_{ed\ ij11}^{V,LL} - \frac{128}{9} L_{ed\ ij22}^{V,LL} \\
& + \frac{16}{9} L_{ed\ ij33}^{V,LL} + \frac{16}{9} L_{ed\ ij11}^{V,LR} + \frac{16}{9} L_{ed\ ij22}^{V,LR} + \frac{16}{9} L_{ed\ ij33}^{V,LR} - \frac{32}{9} L_{ij11}^{V,LL} - \frac{32}{9} L_{ij22}^{V,LL} \\
& - \frac{32}{9} L_{ij11}^{V,LR} - \frac{32}{9} L_{ij22}^{V,LR} \Big] + \alpha^2 \Big[ \frac{224}{81} L_{ijkk}^{V,LL} - \frac{520}{81} L_{ijkk}^{V,LR} - \frac{104}{243} L_{ij11}^{V,LL} \\
& - \frac{3038}{243} L_{ij22}^{V,LL} - \frac{104}{243} L_{ij33}^{V,LL} - \frac{200}{243} L_{ij11}^{V,LR} - \frac{200}{243} L_{ij22}^{V,LR} - \frac{200}{243} L_{ij33}^{V,LR} \\
& + \frac{32}{81} L_{ijii}^{V,LL} + \frac{32}{81} L_{ijjj}^{V,LL} - \frac{520}{81} L_{ijii}^{V,LR} - \frac{520}{81} L_{ijjj}^{V,LR} - \frac{1016}{243} L_{ij11}^{V,LL} - \frac{1016}{243} L_{ij22}^{V,LL} \\
& - \frac{1400}{243} L_{ij11}^{V,LR} - \frac{1400}{243} L_{ij22}^{V,LR} \Big] ;
\end{aligned}$$

$$\dot{L}_{ij33}^{V,LL} = e^2 \Big[ \frac{16}{9} L_{ijkk}^{V,LL} + \frac{4}{9} L_{ijkk}^{V,LR} + \frac{4}{9} L_{ij11}^{V,LL} + \frac{4}{9} L_{ed\ ij22}^{V,LL} + \frac{40}{9} L_{ij33}^{V,LL}$$

$$\begin{aligned}
& + \frac{4}{9}L_{ed\,ij11}^{V,LR} + \frac{4}{9}L_{ed\,ij22}^{V,LR} + \frac{4}{9}L_{ed\,ij33}^{V,LR} + \frac{16}{9}L_{ee\,ijii}^{V,LL} + \frac{16}{9}L_{ee\,ijjj}^{V,LL} + \frac{4}{9}L_{ee\,ijii}^{V,LR} \\
& + \frac{4}{9}L_{ee\,ijjj}^{V,LR} - \frac{8}{9}L_{eu\,ij11}^{V,LL} - \frac{8}{9}L_{eu\,ij22}^{V,LL} - \frac{8}{9}L_{eu\,ij11}^{V,LR} - \frac{8}{9}L_{eu\,ij22}^{V,LR} \Big] + \alpha_s^2 \Big[ 8L_{ed\,ij11}^{V,LL} \\
& + 8L_{ed\,ij22}^{V,LL} + 8L_{ed\,ij33}^{V,LL} - 8L_{ed\,ij11}^{V,LR} - 8L_{ed\,ij22}^{V,LR} - 8L_{ed\,ij33}^{V,LR} + 8L_{eu\,ij11}^{V,LL} \\
& + 8L_{eu\,ij22}^{V,LL} - 8L_{eu\,ij11}^{V,LR} - 8L_{eu\,ij22}^{V,LR} \Big] + \alpha_s \alpha \Big[ \frac{16}{9}L_{ed\,ij11}^{V,LL} + \frac{16}{9}L_{ed\,ij22}^{V,LL} \\
& - \frac{128}{9}L_{ed\,ij33}^{V,LL} + \frac{16}{9}L_{ed\,ij11}^{V,LR} + \frac{16}{9}L_{ed\,ij22}^{V,LR} + \frac{16}{9}L_{ed\,ij33}^{V,LR} - \frac{32}{9}L_{eu\,ij11}^{V,LL} - \frac{32}{9}L_{eu\,ij22}^{V,LL} \\
& - \frac{32}{9}L_{eu\,ij11}^{V,LR} - \frac{32}{9}L_{eu\,ij22}^{V,LR} \Big] + \alpha^2 \Big[ \frac{224}{81}L_{ee\,ijkk}^{V,LL} - \frac{520}{81}L_{ee\,ijkk}^{V,LR} - \frac{104}{243}L_{ed\,ij11}^{V,LL} \\
& - \frac{104}{243}L_{ed\,ij22}^{V,LL} - \frac{3038}{243}L_{ed\,ij33}^{V,LL} - \frac{200}{243}L_{ed\,ij11}^{V,LR} - \frac{200}{243}L_{ed\,ij22}^{V,LR} - \frac{200}{243}L_{ed\,ij33}^{V,LR} \\
& + \frac{32}{81}L_{ee\,ijii}^{V,LL} + \frac{32}{81}L_{ee\,ijjj}^{V,LL} - \frac{520}{81}L_{ee\,ijii}^{V,LR} - \frac{520}{81}L_{ee\,ijjj}^{V,LR} - \frac{1016}{243}L_{eu\,ij11}^{V,LL} - \frac{1016}{243}L_{eu\,ij22}^{V,LL} \\
& - \frac{1400}{243}L_{eu\,ij11}^{V,LR} - \frac{1400}{243}L_{eu\,ij22}^{V,LR} \Big] ;
\end{aligned}$$

$$\begin{aligned}
\dot{L}_{eu\,ij11}^{V,LL} & = e^2 \Big[ -\frac{32}{9}L_{ee\,ijkk}^{V,LL} - \frac{8}{9}L_{ee\,ijkk}^{V,LR} - \frac{8}{9}L_{ed\,ij11}^{V,LL} - \frac{8}{9}L_{ed\,ij22}^{V,LL} - \frac{8}{9}L_{ed\,ij33}^{V,LL} \\
& - \frac{8}{9}L_{ed\,ij11}^{V,LR} - \frac{8}{9}L_{ed\,ij22}^{V,LR} - \frac{8}{9}L_{ed\,ij33}^{V,LR} - \frac{32}{9}L_{ee\,ijii}^{V,LL} - \frac{32}{9}L_{ee\,ijjj}^{V,LL} - \frac{8}{9}L_{ee\,ijii}^{V,LR} \\
& - \frac{8}{9}L_{ee\,ijjj}^{V,LR} - \frac{56}{9}L_{eu\,ij11}^{V,LL} + \frac{16}{9}L_{eu\,ij22}^{V,LL} + \frac{16}{9}L_{eu\,ij11}^{V,LR} + \frac{16}{9}L_{eu\,ij22}^{V,LR} \Big] + \alpha_s^2 \Big[ 8L_{ed\,ij11}^{V,LL} \\
& + 8L_{ed\,ij22}^{V,LL} + 8L_{ed\,ij33}^{V,LL} - 8L_{ed\,ij11}^{V,LR} - 8L_{ed\,ij22}^{V,LR} - 8L_{ed\,ij33}^{V,LR} + 8L_{eu\,ij11}^{V,LL} \\
& + 8L_{eu\,ij22}^{V,LL} - 8L_{eu\,ij11}^{V,LR} - 8L_{eu\,ij22}^{V,LR} \Big] + \alpha_s \alpha \Big[ -\frac{32}{9}L_{ed\,ij11}^{V,LL} - \frac{32}{9}L_{ed\,ij22}^{V,LL} \\
& - \frac{32}{9}L_{ed\,ij33}^{V,LL} - \frac{32}{9}L_{ed\,ij11}^{V,LR} - \frac{32}{9}L_{ed\,ij22}^{V,LR} - \frac{32}{9}L_{ed\,ij33}^{V,LR} + \frac{352}{9}L_{eu\,ij11}^{V,LL} + \frac{64}{9}L_{eu\,ij22}^{V,LL} \\
& + \frac{64}{9}L_{eu\,ij11}^{V,LR} + \frac{64}{9}L_{eu\,ij22}^{V,LR} \Big] + \alpha^2 \Big[ \frac{2432}{81}L_{ee\,ijkk}^{V,LL} + \frac{464}{81}L_{ee\,ijkk}^{V,LR} + \frac{2512}{243}L_{ed\,ij11}^{V,LL}
\end{aligned}$$

$$\begin{aligned}
& + \frac{2512}{243} L_{ij22}^{V,LL} + \frac{2512}{243} L_{ij33}^{V,LL} + \frac{1408}{243} L_{ij11}^{V,LR} + \frac{1408}{243} L_{ij22}^{V,LR} + \frac{1408}{243} L_{ij33}^{V,LR} \\
& + \frac{3680}{81} L_{ijii}^{V,LL} + \frac{3680}{81} L_{ijjj}^{V,LL} + \frac{464}{81} L_{ijii}^{V,LR} + \frac{464}{81} L_{ijjj}^{V,LR} + \frac{2320}{243} L_{ij11}^{V,LL} + \frac{1312}{243} L_{ij22}^{V,LL} \\
& - \frac{3104}{243} L_{ij11}^{V,LR} - \frac{3104}{243} L_{ij22}^{V,LR} \Big] ; \\
\dot{L}_{ij22}^{V,LL} & = e^2 \Bigg[ -\frac{32}{9} L_{ijkk}^{V,LL} - \frac{8}{9} L_{ijkk}^{V,LR} - \frac{8}{9} L_{ed11}^{V,LL} - \frac{8}{9} L_{ed22}^{V,LL} - \frac{8}{9} L_{ed33}^{V,LL} \\
& - \frac{8}{9} L_{ed11}^{V,LR} - \frac{8}{9} L_{ed22}^{V,LR} - \frac{8}{9} L_{ed33}^{V,LR} - \frac{32}{9} L_{ijii}^{V,LL} - \frac{32}{9} L_{ijjj}^{V,LL} - \frac{8}{9} L_{ijii}^{V,LR} \\
& - \frac{8}{9} L_{ijjj}^{V,LR} + \frac{16}{9} L_{ij11}^{V,LL} - \frac{56}{9} L_{ij22}^{V,LL} + \frac{16}{9} L_{ij11}^{V,LR} + \frac{16}{9} L_{ij22}^{V,LR} \Big] + \alpha_s^2 \Bigg[ 8 L_{ed11}^{V,LL} \\
& + 8 L_{ed22}^{V,LL} + 8 L_{ed33}^{V,LL} - 8 L_{ed11}^{V,LR} - 8 L_{ed22}^{V,LR} - 8 L_{ed33}^{V,LR} + 8 L_{ij11}^{V,LL} \\
& + 8 L_{ij22}^{V,LL} - 8 L_{ij11}^{V,LR} - 8 L_{ij22}^{V,LR} \Big] + \alpha_s \alpha \Bigg[ -\frac{32}{9} L_{ed11}^{V,LL} - \frac{32}{9} L_{ed22}^{V,LL} \\
& - \frac{32}{9} L_{ed33}^{V,LL} - \frac{32}{9} L_{ed11}^{V,LR} - \frac{32}{9} L_{ed22}^{V,LR} - \frac{32}{9} L_{ed33}^{V,LR} + \frac{64}{9} L_{ij11}^{V,LL} + \frac{352}{9} L_{ij22}^{V,LL} \\
& + \frac{64}{9} L_{ij11}^{V,LR} + \frac{64}{9} L_{ij22}^{V,LR} \Big] + \alpha^2 \Bigg[ \frac{2432}{81} L_{ijkk}^{V,LL} + \frac{464}{81} L_{ijkk}^{V,LR} + \frac{2512}{243} L_{ed11}^{V,LL} \\
& + \frac{2512}{243} L_{ed22}^{V,LL} + \frac{2512}{243} L_{ed33}^{V,LL} + \frac{1408}{243} L_{ed11}^{V,LR} + \frac{1408}{243} L_{ed22}^{V,LR} + \frac{1408}{243} L_{ed33}^{V,LR} \\
& + \frac{3680}{81} L_{ijii}^{V,LL} + \frac{3680}{81} L_{ijjj}^{V,LL} + \frac{464}{81} L_{ijii}^{V,LR} + \frac{464}{81} L_{ijjj}^{V,LR} + \frac{1312}{243} L_{ij11}^{V,LL} + \frac{2320}{243} L_{ij22}^{V,LL} \\
& - \frac{3104}{243} L_{ij11}^{V,LR} - \frac{3104}{243} L_{ij22}^{V,LR} \Big] ; \\
\dot{L}_{ijkk}^{V,LL} & = e^2 \Bigg[ \frac{40}{3} L_{ijkk}^{V,LL} + \frac{1}{3} L_{ijkk}^{V,LR} + \frac{1}{3} L_{ed11}^{V,LL} + \frac{1}{3} L_{ed22}^{V,LL} + \frac{1}{3} L_{ed33}^{V,LL} \\
& + \frac{1}{3} L_{ed11}^{V,LR} + \frac{1}{3} L_{ed22}^{V,LR} + \frac{1}{3} L_{ed33}^{V,LR} + \frac{4}{3} L_{ijii}^{V,LL} + \frac{4}{3} L_{ijjj}^{V,LL} + \frac{1}{3} L_{ijii}^{V,LR} \\
& + \frac{1}{3} L_{ijjj}^{V,LR} - \frac{2}{3} L_{ij11}^{V,LL} - \frac{2}{3} L_{ij22}^{V,LL} - \frac{2}{3} L_{ij11}^{V,LR} - \frac{2}{3} L_{ij22}^{V,LR} \Big] + \alpha_s \alpha \Bigg[ \frac{4}{3} L_{ed11}^{V,LL}
\end{aligned}$$

$$\begin{aligned}
& + \frac{4}{3}L_{ij22}^{V,LL} + \frac{4}{3}L_{ij33}^{V,LL} + \frac{4}{3}L_{ij11}^{V,LR} + \frac{4}{3}L_{ij22}^{V,LR} + \frac{4}{3}L_{ij33}^{V,LR} - \frac{8}{3}L_{ij11}^{V,LL} \\
& - \frac{8}{3}L_{ij22}^{V,LL} - \frac{8}{3}L_{ij11}^{V,LR} - \frac{8}{3}L_{ij22}^{V,LR} \Big] + \alpha^2 \Big[ -\frac{2302}{27}L_{ijkk}^{V,LL} - \frac{178}{27}L_{ijkk}^{V,LR} \\
& + \frac{166}{81}L_{ij11}^{V,LL} + \frac{166}{81}L_{ij22}^{V,LL} + \frac{166}{81}L_{ij33}^{V,LL} + \frac{34}{81}L_{ij11}^{V,LR} + \frac{34}{81}L_{ij22}^{V,LR} + \frac{34}{81}L_{ij33}^{V,LR} \\
& + \frac{320}{27}L_{ijii}^{V,LL} + \frac{320}{27}L_{ijjj}^{V,LL} - \frac{178}{27}L_{ijii}^{V,LR} - \frac{178}{27}L_{ijjj}^{V,LR} - \frac{314}{81}L_{ij11}^{V,LL} - \frac{314}{81}L_{ij22}^{V,LL} \\
& - \frac{842}{81}L_{ij11}^{V,LR} - \frac{842}{81}L_{ij22}^{V,LR} \Big] ;
\end{aligned}$$

$$\begin{aligned}
\dot{L}_{ijjj}^{V,LL} &= e^2 \Big[ \frac{8}{3}L_{ijkk}^{V,LL} + \frac{2}{3}L_{ijkk}^{V,LR} + \frac{2}{3}L_{ij11}^{V,LL} + \frac{2}{3}L_{ij22}^{V,LL} + \frac{2}{3}L_{ij33}^{V,LL} \\
& + \frac{2}{3}L_{ij11}^{V,LR} + \frac{2}{3}L_{ij22}^{V,LR} + \frac{2}{3}L_{ij33}^{V,LR} + \frac{8}{3}L_{ijii}^{V,LL} + \frac{44}{3}L_{ijjj}^{V,LL} + \frac{2}{3}L_{ijii}^{V,LR} \\
& + \frac{2}{3}L_{ijjj}^{V,LR} - \frac{4}{3}L_{ij11}^{V,LL} - \frac{4}{3}L_{ij22}^{V,LL} - \frac{4}{3}L_{ij11}^{V,LR} - \frac{4}{3}L_{ij22}^{V,LR} \Big] + \alpha_s \alpha \Big[ \frac{8}{3}L_{ij11}^{V,LL} \\
& + \frac{8}{3}L_{ij22}^{V,LL} + \frac{8}{3}L_{ij33}^{V,LL} + \frac{8}{3}L_{ij22}^{V,LR} + \frac{8}{3}L_{ij33}^{V,LR} - \frac{16}{3}L_{ij11}^{V,LL} \\
& - \frac{16}{3}L_{ij22}^{V,LL} - \frac{16}{3}L_{ij11}^{V,LR} - \frac{16}{3}L_{ij22}^{V,LR} \Big] + \alpha^2 \Big[ \frac{592}{27}L_{ijkk}^{V,LL} - \frac{356}{27}L_{ijkk}^{V,LR} \\
& + \frac{332}{81}L_{ij11}^{V,LL} + \frac{332}{81}L_{ij22}^{V,LL} + \frac{332}{81}L_{ij33}^{V,LL} + \frac{68}{81}L_{ij11}^{V,LR} + \frac{68}{81}L_{ij22}^{V,LR} + \frac{68}{81}L_{ij33}^{V,LR} \\
& + \frac{640}{27}L_{ijii}^{V,LL} - \frac{1958}{27}L_{ijjj}^{V,LL} - \frac{356}{27}L_{ijii}^{V,LR} - \frac{356}{27}L_{ijjj}^{V,LR} - \frac{628}{81}L_{ij11}^{V,LL} - \frac{628}{81}L_{ij22}^{V,LL} \\
& - \frac{1684}{81}L_{ij11}^{V,LR} - \frac{1684}{81}L_{ij22}^{V,LR} \Big] ;
\end{aligned}$$

$$\begin{aligned}
\dot{L}_{ijii}^{V,LL} &= e^2 \Big[ \frac{8}{3}L_{ijkk}^{V,LL} + \frac{2}{3}L_{ijkk}^{V,LR} + \frac{2}{3}L_{ij11}^{V,LL} + \frac{2}{3}L_{ij22}^{V,LL} + \frac{2}{3}L_{ij33}^{V,LL} \\
& + \frac{2}{3}L_{ij11}^{V,LR} + \frac{2}{3}L_{ij22}^{V,LR} + \frac{2}{3}L_{ij33}^{V,LR} + \frac{44}{3}L_{ijii}^{V,LL} + \frac{8}{3}L_{ijjj}^{V,LL} + \frac{2}{3}L_{ijii}^{V,LR} \\
& + \frac{2}{3}L_{ijjj}^{V,LR} - \frac{4}{3}L_{ij11}^{V,LL} - \frac{4}{3}L_{ij22}^{V,LL} - \frac{4}{3}L_{ij11}^{V,LR} - \frac{4}{3}L_{ij22}^{V,LR} \Big] + \alpha_s \alpha \Big[ \frac{8}{3}L_{ij11}^{V,LL}
\end{aligned}$$

$$\begin{aligned}
& + \frac{8}{3}L_{ij22}^{V,LL} + \frac{8}{3}L_{ij33}^{V,LL} + \frac{8}{3}L_{ij11}^{V,LR} + \frac{8}{3}L_{ij22}^{V,LR} + \frac{8}{3}L_{ij33}^{V,LR} - \frac{16}{3}L_{ij11}^{V,LL} \\
& - \frac{16}{3}L_{ij22}^{V,LL} - \frac{16}{3}L_{ij11}^{V,LR} - \frac{16}{3}L_{ij22}^{V,LR} \Big] + \alpha^2 \Big[ \frac{592}{27}L_{ijkk}^{V,LL} - \frac{356}{27}L_{ijkk}^{V,LR} \\
& + \frac{332}{81}L_{ij11}^{V,LL} + \frac{332}{81}L_{ij22}^{V,LL} + \frac{332}{81}L_{ij33}^{V,LL} + \frac{68}{81}L_{ij11}^{V,LR} + \frac{68}{81}L_{ij22}^{V,LR} + \frac{68}{81}L_{ij33}^{V,LR} \\
& - \frac{1958}{27}L_{ijii}^{V,LL} + \frac{640}{27}L_{ijjj}^{V,LL} - \frac{356}{27}L_{ijii}^{V,LR} - \frac{356}{27}L_{ijjj}^{V,LR} - \frac{628}{81}L_{ij11}^{V,LL} - \frac{628}{81}L_{ij22}^{V,LL} \\
& - \frac{1684}{81}L_{ij11}^{V,LR} - \frac{1684}{81}L_{ij22}^{V,LR} \Big] ;
\end{aligned}$$

$$\begin{aligned}
\dot{L}_{ij11}^{V,LR} &= e^2 \Big[ \frac{16}{9}L_{ijkk}^{V,LL} + \frac{4}{9}L_{ijkk}^{V,LR} + \frac{4}{9}L_{ij11}^{V,LL} + \frac{4}{9}L_{ij22}^{V,LL} + \frac{4}{9}L_{ij33}^{V,LL} \\
& - \frac{32}{9}L_{ij11}^{V,LR} + \frac{4}{9}L_{ij22}^{V,LR} + \frac{4}{9}L_{ij33}^{V,LR} + \frac{16}{9}L_{ijii}^{V,LL} + \frac{16}{9}L_{ijjj}^{V,LL} + \frac{4}{9}L_{ijii}^{V,LR} \\
& + \frac{4}{9}L_{ijjj}^{V,LR} - \frac{8}{9}L_{ij11}^{V,LL} - \frac{8}{9}L_{ij22}^{V,LL} - \frac{8}{9}L_{ij11}^{V,LR} - \frac{8}{9}L_{ij22}^{V,LR} \Big] + \alpha_s^2 \Big[ -8L_{ij11}^{V,LL} \\
& - 8L_{ij22}^{V,LL} - 8L_{ij33}^{V,LL} + 8L_{ij11}^{V,LR} + 8L_{ij22}^{V,LR} + 8L_{ij33}^{V,LR} - 8L_{ij11}^{V,LL} \\
& - 8L_{ij22}^{V,LL} + 8L_{ij11}^{V,LR} + 8L_{ij22}^{V,LR} \Big] + \alpha_s \alpha \Big[ \frac{16}{9}L_{ij11}^{V,LL} + \frac{16}{9}L_{ij22}^{V,LL} \\
& + \frac{16}{9}L_{ij33}^{V,LL} + \frac{160}{9}L_{ij11}^{V,LR} + \frac{16}{9}L_{ij22}^{V,LR} + \frac{16}{9}L_{ij33}^{V,LR} - \frac{32}{9}L_{ij11}^{V,LL} - \frac{32}{9}L_{ij22}^{V,LL} \\
& - \frac{32}{9}L_{ij11}^{V,LR} - \frac{32}{9}L_{ij22}^{V,LR} \Big] + \alpha^2 \Big[ -\frac{160}{81}L_{ijkk}^{V,LL} - \frac{184}{81}L_{ijkk}^{V,LR} - \frac{440}{243}L_{ij11}^{V,LL} \\
& - \frac{440}{243}L_{ij22}^{V,LL} - \frac{440}{243}L_{ij33}^{V,LL} + \frac{17842}{243}L_{ij11}^{V,LR} - \frac{104}{243}L_{ij22}^{V,LR} - \frac{104}{243}L_{ij33}^{V,LR} \\
& - \frac{640}{81}L_{ijii}^{V,LL} - \frac{640}{81}L_{ijjj}^{V,LL} - \frac{184}{81}L_{ijii}^{V,LR} - \frac{184}{81}L_{ijjj}^{V,LR} - \frac{1640}{243}L_{ij11}^{V,LL} - \frac{1640}{243}L_{ij22}^{V,LL} \\
& - \frac{296}{243}L_{ij11}^{V,LR} - \frac{296}{243}L_{ij22}^{V,LR} \Big] ;
\end{aligned}$$

$$\dot{L}_{ij22}^{V,LR} = e^2 \Big[ \frac{16}{9}L_{ijkk}^{V,LL} + \frac{4}{9}L_{ijkk}^{V,LR} + \frac{4}{9}L_{ij11}^{V,LL} + \frac{4}{9}L_{ij22}^{V,LL} + \frac{4}{9}L_{ij33}^{V,LL}$$



$$\begin{aligned}
& + \frac{4}{9}L_{ed\ ij11}^{V,LR} - \frac{32}{9}L_{ed\ ij22}^{V,LR} + \frac{4}{9}L_{ed\ ij33}^{V,LR} + \frac{16}{9}L_{ee\ ijii}^{V,LL} + \frac{16}{9}L_{ee\ ijjj}^{V,LL} + \frac{4}{9}L_{ee\ ijii}^{V,LR} \\
& + \frac{4}{9}L_{ee\ ijjj}^{V,LR} - \frac{8}{9}L_{eu\ ij11}^{V,LL} - \frac{8}{9}L_{eu\ ij22}^{V,LL} - \frac{8}{9}L_{eu\ ij11}^{V,LR} - \frac{8}{9}L_{eu\ ij22}^{V,LR} \Big] + \alpha_s^2 \Big[ -8L_{ed\ ij11}^{V,LL} \\
& - 8L_{ed\ ij22}^{V,LL} - 8L_{ed\ ij33}^{V,LL} + 8L_{ed\ ij11}^{V,LR} + 8L_{ed\ ij22}^{V,LR} + 8L_{ed\ ij33}^{V,LR} - 8L_{eu\ ij11}^{V,LL} \\
& - 8L_{eu\ ij22}^{V,LL} + 8L_{eu\ ij11}^{V,LR} + 8L_{eu\ ij22}^{V,LR} \Big] + \alpha_s \alpha \Big[ \frac{16}{9}L_{ed\ ij11}^{V,LL} + \frac{16}{9}L_{ed\ ij22}^{V,LL} \\
& + \frac{16}{9}L_{ed\ ij33}^{V,LL} + \frac{16}{9}L_{ed\ ij11}^{V,LR} + \frac{160}{9}L_{ed\ ij22}^{V,LR} + \frac{16}{9}L_{ed\ ij33}^{V,LR} - \frac{32}{9}L_{eu\ ij11}^{V,LL} - \frac{32}{9}L_{eu\ ij22}^{V,LL} \\
& - \frac{32}{9}L_{eu\ ij11}^{V,LR} - \frac{32}{9}L_{eu\ ij22}^{V,LR} \Big] + \alpha^2 \Big[ -\frac{160}{81}L_{ee\ ijkk}^{V,LL} - \frac{184}{81}L_{ee\ ijkk}^{V,LR} - \frac{440}{243}L_{ed\ ij11}^{V,LL} \\
& - \frac{440}{243}L_{ed\ ij22}^{V,LL} - \frac{440}{243}L_{ed\ ij33}^{V,LL} - \frac{104}{243}L_{ed\ ij11}^{V,LR} + \frac{17842}{243}L_{ed\ ij22}^{V,LR} - \frac{104}{243}L_{ed\ ij33}^{V,LR} \\
& - \frac{640}{81}L_{ee\ ijii}^{V,LL} - \frac{640}{81}L_{ee\ ijjj}^{V,LL} - \frac{184}{81}L_{ee\ ijii}^{V,LR} - \frac{184}{81}L_{ee\ ijjj}^{V,LR} - \frac{1640}{243}L_{eu\ ij11}^{V,LL} - \frac{1640}{243}L_{eu\ ij22}^{V,LL} \\
& - \frac{296}{243}L_{eu\ ij11}^{V,LR} - \frac{296}{243}L_{eu\ ij22}^{V,LR} \Big] ;
\end{aligned}$$

$$\begin{aligned}
\dot{L}_{ed\ ij33}^{V,LR} & = e^2 \Big[ \frac{16}{9}L_{ee\ ijkk}^{V,LL} + \frac{4}{9}L_{ee\ ijkk}^{V,LR} + \frac{4}{9}L_{ed\ ij11}^{V,LL} + \frac{4}{9}L_{ed\ ij22}^{V,LL} + \frac{4}{9}L_{ed\ ij33}^{V,LL} \\
& + \frac{4}{9}L_{ed\ ij11}^{V,LR} + \frac{4}{9}L_{ed\ ij22}^{V,LR} - \frac{32}{9}L_{ed\ ij33}^{V,LR} + \frac{16}{9}L_{ee\ ijii}^{V,LL} + \frac{16}{9}L_{ee\ ijjj}^{V,LL} + \frac{4}{9}L_{ee\ ijii}^{V,LR} \\
& + \frac{4}{9}L_{ee\ ijjj}^{V,LR} - \frac{8}{9}L_{eu\ ij11}^{V,LL} - \frac{8}{9}L_{eu\ ij22}^{V,LL} - \frac{8}{9}L_{eu\ ij11}^{V,LR} - \frac{8}{9}L_{eu\ ij22}^{V,LR} \Big] + \alpha_s^2 \Big[ -8L_{ed\ ij11}^{V,LL} \\
& - 8L_{ed\ ij22}^{V,LL} - 8L_{ed\ ij33}^{V,LL} + 8L_{ed\ ij11}^{V,LR} + 8L_{ed\ ij22}^{V,LR} + 8L_{ed\ ij33}^{V,LR} - 8L_{eu\ ij11}^{V,LL} \\
& - 8L_{eu\ ij22}^{V,LL} + 8L_{eu\ ij11}^{V,LR} + 8L_{eu\ ij22}^{V,LR} \Big] + \alpha_s \alpha \Big[ \frac{16}{9}L_{ed\ ij11}^{V,LL} + \frac{16}{9}L_{ed\ ij22}^{V,LL} \\
& + \frac{16}{9}L_{ed\ ij33}^{V,LL} + \frac{16}{9}L_{ed\ ij11}^{V,LR} + \frac{16}{9}L_{ed\ ij22}^{V,LR} + \frac{160}{9}L_{ed\ ij33}^{V,LR} - \frac{32}{9}L_{eu\ ij11}^{V,LL} - \frac{32}{9}L_{eu\ ij22}^{V,LL} \\
& - \frac{32}{9}L_{eu\ ij11}^{V,LR} - \frac{32}{9}L_{eu\ ij22}^{V,LR} \Big] + \alpha^2 \Big[ -\frac{160}{81}L_{ee\ ijkk}^{V,LL} - \frac{184}{81}L_{ee\ ijkk}^{V,LR} - \frac{440}{243}L_{ed\ ij11}^{V,LL}
\end{aligned}$$

$$\begin{aligned}
& -\frac{440}{243}L_{ij22}^{V,LL} - \frac{440}{243}L_{ij33}^{V,LL} - \frac{104}{243}L_{ij11}^{V,LR} - \frac{104}{243}L_{ij22}^{V,LR} + \frac{17842}{243}L_{ij33}^{V,LR} \\
& -\frac{640}{81}L_{ijii}^{V,LL} - \frac{640}{81}L_{ijjj}^{V,LL} - \frac{184}{81}L_{ijii}^{V,LR} - \frac{184}{81}L_{ijjj}^{V,LR} - \frac{1640}{243}L_{ij11}^{V,LL} - \frac{1640}{243}L_{ij22}^{V,LL} \\
& -\frac{296}{243}L_{ij11}^{V,LR} - \frac{296}{243}L_{ij22}^{V,LR} \Big] ;
\end{aligned}$$

$$\begin{aligned}
\dot{L}_{ij11}^{V,LR} = & e^2 \Bigg[ -\frac{32}{9}L_{ijkk}^{V,LL} - \frac{8}{9}L_{ijkk}^{V,LR} - \frac{8}{9}L_{ij11}^{V,LL} - \frac{8}{9}L_{ij22}^{V,LL} - \frac{8}{9}L_{ij33}^{V,LL} \\
& -\frac{8}{9}L_{ij11}^{V,LR} - \frac{8}{9}L_{ij22}^{V,LR} - \frac{8}{9}L_{ij33}^{V,LR} - \frac{32}{9}L_{ijii}^{V,LL} - \frac{32}{9}L_{ijjj}^{V,LL} - \frac{8}{9}L_{ijii}^{V,LR} \\
& -\frac{8}{9}L_{ijjj}^{V,LR} + \frac{16}{9}L_{ij11}^{V,LL} + \frac{16}{9}L_{ij22}^{V,LL} + \frac{88}{9}L_{ij11}^{V,LR} + \frac{16}{9}L_{ij22}^{V,LR} \Big] + \alpha_s^2 \Bigg[ -8L_{ij11}^{V,LL} \\
& -8L_{ij22}^{V,LL} -8L_{ij33}^{V,LL} +8L_{ij11}^{V,LR} +8L_{ij22}^{V,LR} +8L_{ij33}^{V,LR} -8L_{ij11}^{V,LL} \\
& -8L_{ij22}^{V,LL} +8L_{ij11}^{V,LR} +8L_{ij22}^{V,LR} \Big] + \alpha_s \alpha \Bigg[ -\frac{32}{9}L_{ij11}^{V,LL} - \frac{32}{9}L_{ij22}^{V,LL} \\
& -\frac{32}{9}L_{ij33}^{V,LL} - \frac{32}{9}L_{ij11}^{V,LR} - \frac{32}{9}L_{ij22}^{V,LR} - \frac{32}{9}L_{ij33}^{V,LR} + \frac{64}{9}L_{ij11}^{V,LL} + \frac{64}{9}L_{ij22}^{V,LL} \\
& -\frac{224}{9}L_{ij11}^{V,LR} + \frac{64}{9}L_{ij22}^{V,LR} \Big] + \alpha^2 \Bigg[ \frac{896}{81}L_{ijkk}^{V,LL} + \frac{1808}{81}L_{ijkk}^{V,LR} + \frac{1168}{243}L_{ij11}^{V,LL} \\
& + \frac{1168}{243}L_{ij22}^{V,LL} + \frac{1168}{243}L_{ij33}^{V,LL} + \frac{1792}{243}L_{ij11}^{V,LR} + \frac{1792}{243}L_{ij22}^{V,LR} + \frac{1792}{243}L_{ij33}^{V,LR} \\
& + \frac{992}{81}L_{ijii}^{V,LL} + \frac{992}{81}L_{ijjj}^{V,LL} + \frac{1808}{81}L_{ijii}^{V,LR} + \frac{1808}{81}L_{ijjj}^{V,LR} - \frac{1184}{243}L_{ij11}^{V,LL} - \frac{1184}{243}L_{ij22}^{V,LL} \\
& -\frac{43328}{243}L_{ij11}^{V,LR} + \frac{1312}{243}L_{ij22}^{V,LR} \Big] ;
\end{aligned}$$

$$\begin{aligned}
\dot{L}_{ij22}^{V,LR} = & e^2 \Bigg[ -\frac{32}{9}L_{ijkk}^{V,LL} - \frac{8}{9}L_{ijkk}^{V,LR} - \frac{8}{9}L_{ij11}^{V,LL} - \frac{8}{9}L_{ij22}^{V,LL} - \frac{8}{9}L_{ij33}^{V,LL} \\
& -\frac{8}{9}L_{ij11}^{V,LR} - \frac{8}{9}L_{ij22}^{V,LR} - \frac{8}{9}L_{ij33}^{V,LR} - \frac{32}{9}L_{ijii}^{V,LL} - \frac{32}{9}L_{ijjj}^{V,LL} - \frac{8}{9}L_{ijii}^{V,LR} \\
& -\frac{8}{9}L_{ijjj}^{V,LR} + \frac{16}{9}L_{ij11}^{V,LL} + \frac{16}{9}L_{ij22}^{V,LL} + \frac{16}{9}L_{ij11}^{V,LR} + \frac{88}{9}L_{ij22}^{V,LR} \Big] + \alpha_s^2 \Bigg[ -8L_{ij11}^{V,LL}
\end{aligned}$$

$$\begin{aligned}
& -8L_{ij22}^{V,LL} - 8L_{ij33}^{V,LL} + 8L_{ij11}^{V,LR} + 8L_{ij22}^{V,LR} + 8L_{ij33}^{V,LR} - 8L_{ij11}^{V,LL} \\
& - 8L_{ij22}^{V,LL} + 8L_{ij11}^{V,LR} + 8L_{ij22}^{V,LR} \Big] + \alpha_s \alpha \Bigg[ -\frac{32}{9}L_{ij11}^{V,LL} - \frac{32}{9}L_{ij22}^{V,LL} \\
& - \frac{32}{9}L_{ij33}^{V,LL} - \frac{32}{9}L_{ij11}^{V,LR} - \frac{32}{9}L_{ij22}^{V,LR} - \frac{32}{9}L_{ij33}^{V,LR} + \frac{64}{9}L_{ij11}^{V,LL} + \frac{64}{9}L_{ij22}^{V,LL} \\
& + \frac{64}{9}L_{ij11}^{V,LR} - \frac{224}{9}L_{ij22}^{V,LR} \Big] + \alpha^2 \Bigg[ \frac{896}{81}L_{ijkk}^{V,LL} + \frac{1808}{81}L_{ijkk}^{V,LR} + \frac{1168}{243}L_{ij11}^{V,LL} \\
& + \frac{1168}{243}L_{ij22}^{V,LL} + \frac{1168}{243}L_{ij33}^{V,LL} + \frac{1792}{243}L_{ij11}^{V,LR} + \frac{1792}{243}L_{ij22}^{V,LR} + \frac{1792}{243}L_{ij33}^{V,LR} \\
& + \frac{992}{81}L_{ijii}^{V,LL} + \frac{992}{81}L_{ijjj}^{V,LL} + \frac{1808}{81}L_{ijii}^{V,LR} + \frac{1808}{81}L_{ijjj}^{V,LR} - \frac{1184}{243}L_{ij11}^{V,LL} - \frac{1184}{243}L_{ij22}^{V,LL} \\
& + \frac{1312}{243}L_{ij11}^{V,LR} - \frac{43328}{243}L_{ij22}^{V,LR} \Big] ;
\end{aligned}$$

$$\begin{aligned}
\dot{L}_{ijkk}^{V,LR} &= e^2 \Bigg[ \frac{16}{3}L_{ijkk}^{V,LL} - \frac{32}{3}L_{ijkk}^{V,LR} + \frac{4}{3}L_{ij11}^{V,LL} + \frac{4}{3}L_{ij22}^{V,LL} + \frac{4}{3}L_{ij33}^{V,LL} \\
& + \frac{4}{3}L_{ij11}^{V,LR} + \frac{4}{3}L_{ij22}^{V,LR} + \frac{4}{3}L_{ij33}^{V,LR} + \frac{16}{3}L_{ijii}^{V,LL} + \frac{16}{3}L_{ijjj}^{V,LL} + \frac{4}{3}L_{ijii}^{V,LR} \\
& + \frac{4}{3}L_{ijjj}^{V,LR} - \frac{8}{3}L_{ij11}^{V,LL} - \frac{8}{3}L_{ij22}^{V,LL} - \frac{8}{3}L_{ij11}^{V,LR} - \frac{8}{3}L_{ij22}^{V,LR} \Big] + \alpha_s \alpha \Bigg[ \frac{16}{3}L_{ij11}^{V,LL} \\
& + \frac{16}{3}L_{ij22}^{V,LL} + \frac{16}{3}L_{ij33}^{V,LL} + \frac{16}{3}L_{ij11}^{V,LR} + \frac{16}{3}L_{ij22}^{V,LR} + \frac{16}{3}L_{ij33}^{V,LR} - \frac{32}{3}L_{ij11}^{V,LL} \\
& - \frac{32}{3}L_{ij22}^{V,LL} - \frac{32}{3}L_{ij11}^{V,LR} - \frac{32}{3}L_{ij22}^{V,LR} \Big] + \alpha^2 \Bigg[ \frac{32}{27}L_{ijkk}^{V,LL} + \frac{6386}{27}L_{ijkk}^{V,LR} \\
& - \frac{344}{81}L_{ij11}^{V,LL} - \frac{344}{81}L_{ij22}^{V,LL} - \frac{344}{81}L_{ij33}^{V,LL} + \frac{424}{81}L_{ij11}^{V,LR} + \frac{424}{81}L_{ij22}^{V,LR} + \frac{424}{81}L_{ij33}^{V,LR} \\
& - \frac{736}{27}L_{ijii}^{V,LL} - \frac{736}{27}L_{ijjj}^{V,LL} + \frac{296}{27}L_{ijii}^{V,LR} + \frac{296}{27}L_{ijjj}^{V,LR} - \frac{3128}{81}L_{ij11}^{V,LL} - \frac{3128}{81}L_{ij22}^{V,LL} \\
& - \frac{56}{81}L_{ij11}^{V,LR} - \frac{56}{81}L_{ij22}^{V,LR} \Big] ;
\end{aligned}$$

$$\dot{L}_{ijjj}^{V,LR} = e^2 \Bigg[ \frac{16}{3}L_{ijkk}^{V,LL} + \frac{4}{3}L_{ijkk}^{V,LR} + \frac{4}{3}L_{ij11}^{V,LL} + \frac{4}{3}L_{ij22}^{V,LL} + \frac{4}{3}L_{ij33}^{V,LL}$$

$$\begin{aligned}
& + \frac{4}{3}L_{ij11}^{V,LR} + \frac{4}{3}L_{ij22}^{V,LR} + \frac{4}{3}L_{ij33}^{V,LR} + \frac{16}{3}L_{ijii}^{V,LL} + \frac{16}{3}L_{ijjj}^{V,LL} + \frac{4}{3}L_{ijii}^{V,LR} \\
& - \frac{32}{3}L_{ijjj}^{V,LR} - \frac{8}{3}L_{ij11}^{V,LL} - \frac{8}{3}L_{ij22}^{V,LL} - \frac{8}{3}L_{ij11}^{V,LR} - \frac{8}{3}L_{ij22}^{V,LR} \Big] + \alpha_s \alpha \Big[ \frac{16}{3}L_{ij11}^{V,LL} \\
& + \frac{16}{3}L_{ij22}^{V,LL} + \frac{16}{3}L_{ij33}^{V,LL} + \frac{16}{3}L_{ij11}^{V,LR} + \frac{16}{3}L_{ij22}^{V,LR} + \frac{16}{3}L_{ij33}^{V,LR} - \frac{32}{3}L_{ij11}^{V,LL} \\
& - \frac{32}{3}L_{ij22}^{V,LL} - \frac{32}{3}L_{ij11}^{V,LR} - \frac{32}{3}L_{ij22}^{V,LR} \Big] + \alpha^2 \Big[ \frac{32}{27}L_{ijkk}^{V,LL} + \frac{296}{27}L_{ijkk}^{V,LR} \\
& - \frac{344}{81}L_{ij11}^{V,LL} - \frac{344}{81}L_{ij22}^{V,LL} - \frac{344}{81}L_{ij33}^{V,LL} + \frac{424}{81}L_{ij11}^{V,LR} + \frac{424}{81}L_{ij22}^{V,LR} + \frac{424}{81}L_{ij33}^{V,LR} \\
& - \frac{736}{27}L_{ijii}^{V,LL} - \frac{736}{27}L_{ijjj}^{V,LL} + \frac{296}{27}L_{ijii}^{V,LR} + \frac{6386}{27}L_{ijjj}^{V,LR} - \frac{3128}{81}L_{ij11}^{V,LL} - \frac{3128}{81}L_{ij22}^{V,LL} \\
& - \frac{56}{81}L_{ij11}^{V,LR} - \frac{56}{81}L_{ij22}^{V,LR} \Big] ;
\end{aligned}$$

$$\begin{aligned}
\dot{L}_{ijii}^{V,LR} & = e^2 \Big[ \frac{16}{3}L_{ijkk}^{V,LL} + \frac{4}{3}L_{ijkk}^{V,LR} + \frac{4}{3}L_{ij11}^{V,LL} + \frac{4}{3}L_{ij22}^{V,LL} + \frac{4}{3}L_{ij33}^{V,LL} \\
& + \frac{4}{3}L_{ij11}^{V,LR} + \frac{4}{3}L_{ij22}^{V,LR} + \frac{4}{3}L_{ij33}^{V,LR} + \frac{16}{3}L_{ijii}^{V,LL} + \frac{16}{3}L_{ijjj}^{V,LL} - \frac{32}{3}L_{ijii}^{V,LR} \\
& + \frac{4}{3}L_{ijjj}^{V,LR} - \frac{8}{3}L_{ij11}^{V,LL} - \frac{8}{3}L_{ij22}^{V,LL} - \frac{8}{3}L_{ij11}^{V,LR} - \frac{8}{3}L_{ij22}^{V,LR} \Big] + \alpha_s \alpha \Big[ \frac{16}{3}L_{ij11}^{V,LL} \\
& + \frac{16}{3}L_{ij22}^{V,LL} + \frac{16}{3}L_{ij33}^{V,LL} + \frac{16}{3}L_{ij11}^{V,LR} + \frac{16}{3}L_{ij22}^{V,LR} + \frac{16}{3}L_{ij33}^{V,LR} - \frac{32}{3}L_{ij11}^{V,LL} \\
& - \frac{32}{3}L_{ij22}^{V,LL} - \frac{32}{3}L_{ij11}^{V,LR} - \frac{32}{3}L_{ij22}^{V,LR} \Big] + \alpha^2 \Big[ \frac{32}{27}L_{ijkk}^{V,LL} + \frac{296}{27}L_{ijkk}^{V,LR} \\
& - \frac{344}{81}L_{ij11}^{V,LL} - \frac{344}{81}L_{ij22}^{V,LL} - \frac{344}{81}L_{ij33}^{V,LL} + \frac{424}{81}L_{ij11}^{V,LR} + \frac{424}{81}L_{ij22}^{V,LR} + \frac{424}{81}L_{ij33}^{V,LR} \\
& - \frac{736}{27}L_{ijii}^{V,LL} - \frac{736}{27}L_{ijjj}^{V,LL} + \frac{6386}{27}L_{ijii}^{V,LR} + \frac{296}{27}L_{ijjj}^{V,LR} - \frac{3128}{81}L_{ij11}^{V,LL} - \frac{3128}{81}L_{ij22}^{V,LL} \\
& - \frac{56}{81}L_{ij11}^{V,LR} - \frac{56}{81}L_{ij22}^{V,LR} \Big] ;
\end{aligned}$$

$$\dot{L}_{ij11}^{S,RL} = -8g_s^2 L_{ij11}^{S,RL} - \frac{20}{3}e^2 L_{ij11}^{S,RL} - \frac{1012}{9}\alpha_s^2 L_{ij11}^{S,RL} - \frac{8}{9}\alpha_s \alpha L_{ij11}^{S,RL}$$

$$\begin{aligned}
& + \frac{6958}{81} \alpha^2 L_{ij11}^{S,RL} ; \\
\dot{L}_{ij22}^{S,RL} &= -8g_s^2 L_{ij22}^{S,RL} - \frac{20}{3} e^2 L_{ij22}^{S,RL} - \frac{1012}{9} \alpha_s^2 L_{ij22}^{S,RL} - \frac{8}{9} \alpha_s \alpha L_{ij22}^{S,RL} \\
& + \frac{6958}{81} \alpha^2 L_{ij22}^{S,RL} ; \\
\dot{L}_{ij33}^{S,RL} &= -8g_s^2 L_{ij33}^{S,RL} - \frac{20}{3} e^2 L_{ij33}^{S,RL} - \frac{1012}{9} \alpha_s^2 L_{ij33}^{S,RL} - \frac{8}{9} \alpha_s \alpha L_{ij33}^{S,RL} \\
& + \frac{6958}{81} \alpha^2 L_{ij33}^{S,RL} ; \\
\dot{L}_{ij11}^{S,RL} &= -8g_s^2 L_{ij11}^{S,RL} - \frac{26}{3} e^2 L_{ij11}^{S,RL} - \frac{1012}{9} \alpha_s^2 L_{ij11}^{S,RL} - \frac{32}{9} \alpha_s \alpha L_{ij11}^{S,RL} \\
& + \frac{445}{81} \alpha^2 L_{ij11}^{S,RL} ; \\
\dot{L}_{ij22}^{S,RL} &= -8g_s^2 L_{ij22}^{S,RL} - \frac{26}{3} e^2 L_{ij22}^{S,RL} - \frac{1012}{9} \alpha_s^2 L_{ij22}^{S,RL} - \frac{32}{9} \alpha_s \alpha L_{ij22}^{S,RL} \\
& + \frac{445}{81} \alpha^2 L_{ij22}^{S,RL} ; \\
\dot{L}_{kjik}^{V,LR} &= \frac{2030}{9} \alpha^2 L_{kjik}^{V,LR} - 12e^2 L_{kjik}^{V,LR} ; \\
\dot{L}_{ij11}^{S,RR} &= -8g_s^2 L_{ij11}^{S,RR} + e^2 \left[ -\frac{20}{3} L_{ij11}^{S,RR} - 32 L_{ij11}^{T,RR} \right] - \frac{1012}{9} \alpha_s^2 L_{ij11}^{S,RR} \\
& + \alpha_s \alpha \left[ \frac{1792}{9} L_{ij11}^{T,RR} - \frac{8}{9} L_{ij11}^{S,RR} \right] + \alpha^2 \left[ \frac{1882}{81} L_{ij11}^{S,RR} + \frac{19712}{27} L_{ij11}^{T,RR} \right] ; \\
\dot{L}_{ij11}^{T,RR} &= \frac{8}{3} g_s^2 L_{ij11}^{T,RR} + e^2 \left[ \frac{20}{9} L_{ij11}^{T,RR} - \frac{2}{3} L_{ij11}^{S,RR} \right] + \frac{1652}{27} \alpha_s^2 L_{ij11}^{T,RR} \\
& + \alpha_s \alpha \left[ \frac{16}{3} L_{ij11}^{S,RR} - \frac{152}{27} L_{ij11}^{T,RR} \right] + \alpha^2 \left[ \frac{368}{81} L_{ij11}^{S,RR} - \frac{7154}{243} L_{ij11}^{T,RR} \right] ; \\
\dot{L}_{ij22}^{S,RR} &= -8g_s^2 L_{ij22}^{S,RR} + e^2 \left[ -\frac{20}{3} L_{ij22}^{S,RR} - 32 L_{ij22}^{T,RR} \right] - \frac{1012}{9} \alpha_s^2 L_{ij22}^{S,RR} \\
& + \alpha_s \alpha \left[ \frac{1792}{9} L_{ij22}^{T,RR} - \frac{8}{9} L_{ij22}^{S,RR} \right] + \alpha^2 \left[ \frac{1882}{81} L_{ij22}^{S,RR} + \frac{19712}{27} L_{ij22}^{T,RR} \right] ;
\end{aligned}$$

$$\begin{aligned}
\dot{L}_{ed\ ij22}^{T,RR} &= \frac{8}{3}g_s^2 L_{ed\ ij22}^{T,RR} + e^2 \left[ \frac{20}{9} L_{ed\ ij22}^{T,RR} - \frac{2}{3} L_{ed\ ij22}^{S,RR} \right] + \frac{1652}{27} \alpha_s^2 L_{ed\ ij22}^{T,RR} \\
&\quad + \alpha_s \alpha \left[ \frac{16}{3} L_{ed\ ij22}^{S,RR} - \frac{152}{27} L_{ed\ ij22}^{T,RR} \right] + \alpha^2 \left[ \frac{368}{81} L_{ed\ ij22}^{S,RR} - \frac{7154}{243} L_{ed\ ij22}^{T,RR} \right]; \\
\dot{L}_{ed\ ij33}^{S,RR} &= -8g_s^2 L_{ed\ ij33}^{S,RR} + e^2 \left[ -\frac{20}{3} L_{ed\ ij33}^{S,RR} - 32 L_{ed\ ij33}^{T,RR} \right] - \frac{1012}{9} \alpha_s^2 L_{ed\ ij33}^{S,RR} \\
&\quad + \alpha_s \alpha \left[ \frac{1792}{9} L_{ed\ ij33}^{T,RR} - \frac{8}{9} L_{ed\ ij33}^{S,RR} \right] + \alpha^2 \left[ \frac{1882}{81} L_{ed\ ij33}^{S,RR} + \frac{19712}{27} L_{ed\ ij33}^{T,RR} \right]; \\
\dot{L}_{ed\ ij33}^{T,RR} &= \frac{8}{3}g_s^2 L_{ed\ ij33}^{T,RR} + e^2 \left[ \frac{20}{9} L_{ed\ ij33}^{T,RR} - \frac{2}{3} L_{ed\ ij33}^{S,RR} \right] + \frac{1652}{27} \alpha_s^2 L_{ed\ ij33}^{T,RR} \\
&\quad + \alpha_s \alpha \left[ \frac{16}{3} L_{ed\ ij33}^{S,RR} - \frac{152}{27} L_{ed\ ij33}^{T,RR} \right] + \alpha^2 \left[ \frac{368}{81} L_{ed\ ij33}^{S,RR} - \frac{7154}{243} L_{ed\ ij33}^{T,RR} \right]; \\
\dot{L}_{eu\ ij11}^{S,RR} &= -8g_s^2 L_{eu\ ij11}^{S,RR} + e^2 \left[ 64 L_{eu\ ij11}^{T,RR} - \frac{26}{3} L_{eu\ ij11}^{S,RR} \right] - \frac{1012}{9} \alpha_s^2 L_{eu\ ij11}^{S,RR} \\
&\quad + \alpha_s \alpha \left[ -\frac{32}{9} L_{eu\ ij11}^{S,RR} - \frac{3584}{9} L_{eu\ ij11}^{T,RR} \right] + \alpha^2 \left[ -\frac{2579}{81} L_{eu\ ij11}^{S,RR} - \frac{35200}{27} L_{eu\ ij11}^{T,RR} \right]; \\
\dot{L}_{eu\ ij11}^{T,RR} &= \frac{8}{3}g_s^2 L_{eu\ ij11}^{T,RR} + e^2 \left[ \frac{4}{3} L_{eu\ ij11}^{S,RR} + \frac{26}{9} L_{eu\ ij11}^{T,RR} \right] + \frac{1652}{27} \alpha_s^2 L_{eu\ ij11}^{T,RR} \\
&\quad + \alpha_s \alpha \left[ -\frac{32}{3} L_{eu\ ij11}^{S,RR} - \frac{608}{27} L_{eu\ ij11}^{T,RR} \right] + \alpha^2 \left[ -\frac{1384}{81} L_{eu\ ij11}^{S,RR} - \frac{21929}{243} L_{eu\ ij11}^{T,RR} \right]; \\
\dot{L}_{eu\ ij22}^{S,RR} &= -8g_s^2 L_{eu\ ij22}^{S,RR} + e^2 \left[ 64 L_{eu\ ij22}^{T,RR} - \frac{26}{3} L_{eu\ ij22}^{S,RR} \right] - \frac{1012}{9} \alpha_s^2 L_{eu\ ij22}^{S,RR} \\
&\quad + \alpha_s \alpha \left[ -\frac{32}{9} L_{eu\ ij22}^{S,RR} - \frac{3584}{9} L_{eu\ ij22}^{T,RR} \right] + \alpha^2 \left[ -\frac{2579}{81} L_{eu\ ij22}^{S,RR} - \frac{35200}{27} L_{eu\ ij22}^{T,RR} \right]; \\
\dot{L}_{eu\ ij22}^{T,RR} &= \frac{8}{3}g_s^2 L_{eu\ ij22}^{T,RR} + e^2 \left[ \frac{4}{3} L_{eu\ ij22}^{S,RR} + \frac{26}{9} L_{eu\ ij22}^{T,RR} \right] + \frac{1652}{27} \alpha_s^2 L_{eu\ ij22}^{T,RR} \\
&\quad + \alpha_s \alpha \left[ -\frac{32}{3} L_{eu\ ij22}^{S,RR} - \frac{608}{27} L_{eu\ ij22}^{T,RR} \right] + \alpha^2 \left[ -\frac{1384}{81} L_{eu\ ij22}^{S,RR} - \frac{21929}{243} L_{eu\ ij22}^{T,RR} \right];
\end{aligned}$$

$$\begin{aligned}
\dot{L}_{ijkk}^{S,RR} &= e^2 \left[ 16L_{\substack{ee \\ ikkj}}^{S,RR} - 4L_{\substack{ee \\ ijkk}}^{S,RR} \right] - \frac{5426}{27} \alpha^2 L_{\substack{ee \\ ijkk}}^{S,RR} ; \\
\dot{L}_{ikkj}^{S,RR} &= e^2 \left[ 16L_{\substack{ee \\ ijkk}}^{S,RR} - 4L_{\substack{ee \\ ikkj}}^{S,RR} \right] + \frac{640}{9} \alpha^2 L_{\substack{ee \\ ikkj}}^{S,RR} ; \\
\dot{L}_{ijjj}^{S,RR} &= 12e^2 L_{\substack{ee \\ ijjj}}^{S,RR} - \frac{1753}{27} \alpha^2 L_{\substack{ee \\ ijjj}}^{S,RR} ; \\
\dot{L}_{ijii}^{S,RR} &= 12e^2 L_{\substack{ee \\ ijii}}^{S,RR} - \frac{1753}{27} \alpha^2 L_{\substack{ee \\ ijii}}^{S,RR} ; \\
\dot{L}_{edij11}^{V,RR} &= e^2 \left[ \frac{4}{9} L_{\substack{ee \\ kkij}}^{V,LR} + \frac{16}{9} L_{\substack{ee \\ ijkk}}^{V,RR} + \frac{4}{9} L_{\substack{de \\ 11ij}}^{V,LR} + \frac{4}{9} L_{\substack{de \\ 22ij}}^{V,LR} + \frac{4}{9} L_{\substack{de \\ 33ij}}^{V,LR} \right. \\
&\quad + \frac{40}{9} L_{\substack{ed \\ ij11}}^{V,RR} + \frac{4}{9} L_{\substack{ed \\ ij22}}^{V,RR} + \frac{4}{9} L_{\substack{ed \\ ij33}}^{V,RR} + \frac{4}{9} L_{\substack{ee \\ iijj}}^{V,LR} + \frac{4}{9} L_{\substack{ee \\ jjij}}^{V,LR} + \frac{16}{9} L_{\substack{ee \\ ijii}}^{V,RR} \\
&\quad + \frac{16}{9} L_{\substack{ee \\ ijjj}}^{V,RR} - \frac{8}{9} L_{\substack{eu \\ ij11}}^{V,RR} - \frac{8}{9} L_{\substack{eu \\ ij22}}^{V,RR} - \frac{8}{9} L_{\substack{ue \\ 11ij}}^{V,LR} - \frac{8}{9} L_{\substack{ue \\ 22ij}}^{V,LR} \left. \right] + \alpha_s^2 \left[ -8L_{\substack{de \\ 11ij}}^{V,LR} \right. \\
&\quad - 8L_{\substack{de \\ 22ij}}^{V,LR} - 8L_{\substack{de \\ 33ij}}^{V,LR} + 8L_{\substack{ed \\ ij11}}^{V,RR} + 8L_{\substack{ed \\ ij22}}^{V,RR} + 8L_{\substack{ed \\ ij33}}^{V,RR} + 8L_{\substack{eu \\ ij11}}^{V,RR} \\
&\quad + 8L_{\substack{eu \\ ij22}}^{V,RR} - 8L_{\substack{ue \\ 11ij}}^{V,LR} - 8L_{\substack{ue \\ 22ij}}^{V,LR} \left. \right] + \alpha_s \alpha \left[ \frac{16}{9} L_{\substack{de \\ 11ij}}^{V,LR} + \frac{16}{9} L_{\substack{de \\ 22ij}}^{V,LR} \right. \\
&\quad + \frac{16}{9} L_{\substack{de \\ 33ij}}^{V,LR} - \frac{128}{9} L_{\substack{ed \\ ij11}}^{V,RR} + \frac{16}{9} L_{\substack{ed \\ ij22}}^{V,RR} + \frac{16}{9} L_{\substack{ed \\ ij33}}^{V,RR} - \frac{32}{9} L_{\substack{eu \\ ij11}}^{V,RR} - \frac{32}{9} L_{\substack{eu \\ ij22}}^{V,RR} \\
&\quad - \frac{32}{9} L_{\substack{ue \\ 11ij}}^{V,LR} - \frac{32}{9} L_{\substack{ue \\ 22ij}}^{V,LR} \left. \right] + \alpha^2 \left[ -\frac{520}{81} L_{\substack{ee \\ kkij}}^{V,LR} + \frac{224}{81} L_{\substack{ee \\ ijkk}}^{V,RR} - \frac{200}{243} L_{\substack{de \\ 11ij}}^{V,LR} \right. \\
&\quad - \frac{200}{243} L_{\substack{de \\ 22ij}}^{V,LR} - \frac{200}{243} L_{\substack{de \\ 33ij}}^{V,LR} - \frac{3038}{243} L_{\substack{ed \\ ij11}}^{V,RR} - \frac{104}{243} L_{\substack{ed \\ ij22}}^{V,RR} - \frac{104}{243} L_{\substack{ed \\ ij33}}^{V,RR} \\
&\quad - \frac{520}{81} L_{\substack{ee \\ iijj}}^{V,LR} - \frac{520}{81} L_{\substack{ee \\ jjij}}^{V,LR} + \frac{32}{81} L_{\substack{ee \\ ijii}}^{V,RR} + \frac{32}{81} L_{\substack{ee \\ ijjj}}^{V,RR} - \frac{1016}{243} L_{\substack{eu \\ ij11}}^{V,RR} - \frac{1016}{243} L_{\substack{eu \\ ij22}}^{V,RR} \\
&\quad \left. - \frac{1400}{243} L_{\substack{ue \\ 11ij}}^{V,LR} - \frac{1400}{243} L_{\substack{ue \\ 22ij}}^{V,LR} \right] ; \\
\dot{L}_{edij22}^{V,RR} &= e^2 \left[ \frac{4}{9} L_{\substack{ee \\ kkij}}^{V,LR} + \frac{16}{9} L_{\substack{ee \\ ijkk}}^{V,RR} + \frac{4}{9} L_{\substack{de \\ 11ij}}^{V,LR} + \frac{4}{9} L_{\substack{de \\ 22ij}}^{V,LR} + \frac{4}{9} L_{\substack{de \\ 33ij}}^{V,LR} \right. \\
&\quad + \frac{4}{9} L_{\substack{ed \\ ij11}}^{V,RR} + \frac{40}{9} L_{\substack{ed \\ ij22}}^{V,RR} + \frac{4}{9} L_{\substack{ed \\ ij33}}^{V,RR} + \frac{4}{9} L_{\substack{ee \\ iijj}}^{V,LR} + \frac{4}{9} L_{\substack{ee \\ jjij}}^{V,LR} + \frac{16}{9} L_{\substack{ee \\ ijii}}^{V,RR} \\
&\quad \left. - \frac{1400}{243} L_{\substack{ue \\ 11ij}}^{V,LR} - \frac{1400}{243} L_{\substack{ue \\ 22ij}}^{V,LR} \right] ;
\end{aligned}$$

$$\begin{aligned}
& + \frac{16}{9} L_{ijjj}^{V,RR} - \frac{8}{9} L_{ij11}^{V,RR} - \frac{8}{9} L_{ij22}^{V,RR} - \frac{8}{9} L_{11ij}^{V,LR} - \frac{8}{9} L_{22ij}^{V,LR} \Big] + \alpha_s^2 \Big[ - 8 L_{11ij}^{V,LR} \\
& - 8 L_{22ij}^{V,LR} - 8 L_{33ij}^{V,LR} + 8 L_{ij11}^{V,RR} + 8 L_{ij22}^{V,RR} + 8 L_{ij33}^{V,RR} + 8 L_{ij11}^{V,RR} \\
& + 8 L_{ij22}^{V,RR} - 8 L_{11ij}^{V,LR} - 8 L_{22ij}^{V,LR} \Big] + \alpha_s \alpha \Big[ \frac{16}{9} L_{11ij}^{V,LR} + \frac{16}{9} L_{22ij}^{V,LR} \\
& + \frac{16}{9} L_{33ij}^{V,LR} + \frac{16}{9} L_{ij11}^{V,RR} - \frac{128}{9} L_{ij22}^{V,RR} + \frac{16}{9} L_{ij33}^{V,RR} - \frac{32}{9} L_{ij11}^{V,RR} - \frac{32}{9} L_{ij22}^{V,RR} \\
& - \frac{32}{9} L_{11ij}^{V,LR} - \frac{32}{9} L_{22ij}^{V,LR} \Big] + \alpha^2 \Big[ - \frac{520}{81} L_{kkij}^{V,LR} + \frac{224}{81} L_{ijkk}^{V,RR} - \frac{200}{243} L_{11ij}^{V,LR} \\
& - \frac{200}{243} L_{22ij}^{V,LR} - \frac{200}{243} L_{33ij}^{V,LR} - \frac{104}{243} L_{ij11}^{V,RR} - \frac{3038}{243} L_{ij22}^{V,RR} - \frac{104}{243} L_{ij33}^{V,RR} \\
& - \frac{520}{81} L_{iijj}^{V,LR} - \frac{520}{81} L_{jjij}^{V,LR} + \frac{32}{81} L_{ijii}^{V,RR} + \frac{32}{81} L_{ijjj}^{V,RR} - \frac{1016}{243} L_{ij11}^{V,RR} - \frac{1016}{243} L_{ij22}^{V,RR} \\
& - \frac{1400}{243} L_{11ij}^{V,LR} - \frac{1400}{243} L_{22ij}^{V,LR} \Big] ;
\end{aligned}$$

$$\begin{aligned}
\dot{L}_{ij33}^{V,RR} & = e^2 \Big[ \frac{4}{9} L_{kkij}^{V,LR} + \frac{16}{9} L_{ijkk}^{V,RR} + \frac{4}{9} L_{11ij}^{V,LR} + \frac{4}{9} L_{22ij}^{V,LR} + \frac{4}{9} L_{33ij}^{V,LR} \\
& + \frac{4}{9} L_{ij11}^{V,RR} + \frac{4}{9} L_{ij22}^{V,RR} + \frac{40}{9} L_{ij33}^{V,RR} + \frac{4}{9} L_{iijj}^{V,LR} + \frac{4}{9} L_{jjij}^{V,LR} + \frac{16}{9} L_{ijii}^{V,RR} \\
& + \frac{16}{9} L_{ijjj}^{V,RR} - \frac{8}{9} L_{ij11}^{V,RR} - \frac{8}{9} L_{ij22}^{V,RR} - \frac{8}{9} L_{11ij}^{V,LR} - \frac{8}{9} L_{22ij}^{V,LR} \Big] + \alpha_s^2 \Big[ - 8 L_{11ij}^{V,LR} \\
& - 8 L_{22ij}^{V,LR} - 8 L_{33ij}^{V,LR} + 8 L_{ij11}^{V,RR} + 8 L_{ij22}^{V,RR} + 8 L_{ij33}^{V,RR} + 8 L_{ij11}^{V,RR} \\
& + 8 L_{ij22}^{V,RR} - 8 L_{11ij}^{V,LR} - 8 L_{22ij}^{V,LR} \Big] + \alpha_s \alpha \Big[ \frac{16}{9} L_{11ij}^{V,LR} + \frac{16}{9} L_{22ij}^{V,LR} \\
& + \frac{16}{9} L_{33ij}^{V,LR} + \frac{16}{9} L_{ij11}^{V,RR} - \frac{128}{9} L_{ij22}^{V,RR} - \frac{32}{9} L_{ij33}^{V,RR} - \frac{32}{9} L_{ij11}^{V,RR} - \frac{32}{9} L_{ij22}^{V,RR} \\
& - \frac{32}{9} L_{11ij}^{V,LR} - \frac{32}{9} L_{22ij}^{V,LR} \Big] + \alpha^2 \Big[ - \frac{520}{81} L_{kkij}^{V,LR} + \frac{224}{81} L_{ijkk}^{V,RR} - \frac{200}{243} L_{11ij}^{V,LR} \\
& - \frac{200}{243} L_{22ij}^{V,LR} - \frac{200}{243} L_{33ij}^{V,LR} - \frac{104}{243} L_{ij11}^{V,RR} - \frac{3038}{243} L_{ij22}^{V,RR} - \frac{104}{243} L_{ij33}^{V,RR}
\end{aligned}$$



$$\begin{aligned}
& -\frac{520}{81}L_{iii}^{V,LR} - \frac{520}{81}L_{jjj}^{V,LR} + \frac{32}{81}L_{ijii}^{V,RR} + \frac{32}{81}L_{ijjj}^{V,RR} - \frac{1016}{243}L_{ij11}^{V,RR} - \frac{1016}{243}L_{ij22}^{V,RR} \\
& - \frac{1400}{243}L_{11ij}^{V,LR} - \frac{1400}{243}L_{22ij}^{V,LR} \Big] ; \\
\dot{L}_{ij11}^{V,RR} = & e^2 \Bigg[ -\frac{8}{9}L_{kki}^{V,LR} - \frac{32}{9}L_{jkk}^{V,RR} - \frac{8}{9}L_{11ij}^{V,LR} - \frac{8}{9}L_{22ij}^{V,LR} - \frac{8}{9}L_{33ij}^{V,LR} \\
& - \frac{8}{9}L_{ij11}^{V,RR} - \frac{8}{9}L_{ij22}^{V,RR} - \frac{8}{9}L_{ij33}^{V,RR} - \frac{8}{9}L_{iiij}^{V,LR} - \frac{8}{9}L_{jjij}^{V,LR} - \frac{32}{9}L_{ijii}^{V,RR} \\
& - \frac{32}{9}L_{ijjj}^{V,RR} - \frac{56}{9}L_{ij11}^{V,RR} + \frac{16}{9}L_{ij22}^{V,RR} + \frac{16}{9}L_{ij33}^{V,RR} + \frac{16}{9}L_{11ij}^{V,LR} + \frac{16}{9}L_{22ij}^{V,LR} \Big] + \alpha_s^2 \Bigg[ -8L_{11ij}^{V,LR} \\
& - 8L_{22ij}^{V,LR} - 8L_{33ij}^{V,LR} + 8L_{ij11}^{V,RR} + 8L_{ij22}^{V,RR} + 8L_{ij33}^{V,RR} + 8L_{ij11}^{V,RR} \\
& + 8L_{ij22}^{V,RR} - 8L_{11ij}^{V,LR} - 8L_{22ij}^{V,LR} \Big] + \alpha_s \alpha \Bigg[ -\frac{32}{9}L_{11ij}^{V,LR} - \frac{32}{9}L_{22ij}^{V,LR} \\
& - \frac{32}{9}L_{33ij}^{V,LR} - \frac{32}{9}L_{ij11}^{V,RR} - \frac{32}{9}L_{ij22}^{V,RR} - \frac{32}{9}L_{ij33}^{V,RR} + \frac{352}{9}L_{ij11}^{V,RR} + \frac{64}{9}L_{ij22}^{V,RR} \\
& + \frac{64}{9}L_{11ij}^{V,LR} + \frac{64}{9}L_{22ij}^{V,LR} \Big] + \alpha^2 \Bigg[ \frac{464}{81}L_{kki}^{V,LR} + \frac{2432}{81}L_{jkk}^{V,RR} + \frac{1408}{243}L_{11ij}^{V,LR} \\
& + \frac{1408}{243}L_{22ij}^{V,LR} + \frac{1408}{243}L_{33ij}^{V,LR} + \frac{2512}{243}L_{ij11}^{V,RR} + \frac{2512}{243}L_{ij22}^{V,RR} + \frac{2512}{243}L_{ij33}^{V,RR} \\
& + \frac{464}{81}L_{iiij}^{V,LR} + \frac{464}{81}L_{jjij}^{V,LR} + \frac{3680}{81}L_{ijii}^{V,RR} + \frac{3680}{81}L_{ijjj}^{V,RR} + \frac{2320}{243}L_{ij11}^{V,RR} + \frac{1312}{243}L_{ij22}^{V,RR} \\
& - \frac{3104}{243}L_{11ij}^{V,LR} - \frac{3104}{243}L_{22ij}^{V,LR} \Big] ; \\
\dot{L}_{ij22}^{V,RR} = & e^2 \Bigg[ -\frac{8}{9}L_{kki}^{V,LR} - \frac{32}{9}L_{jkk}^{V,RR} - \frac{8}{9}L_{11ij}^{V,LR} - \frac{8}{9}L_{22ij}^{V,LR} - \frac{8}{9}L_{33ij}^{V,LR} \\
& - \frac{8}{9}L_{ij11}^{V,RR} - \frac{8}{9}L_{ij22}^{V,RR} - \frac{8}{9}L_{ij33}^{V,RR} - \frac{8}{9}L_{iiij}^{V,LR} - \frac{8}{9}L_{jjij}^{V,LR} - \frac{32}{9}L_{ijii}^{V,RR} \\
& - \frac{32}{9}L_{ijjj}^{V,RR} + \frac{16}{9}L_{ij11}^{V,RR} - \frac{56}{9}L_{ij22}^{V,RR} + \frac{16}{9}L_{11ij}^{V,LR} + \frac{16}{9}L_{22ij}^{V,LR} \Big] + \alpha_s^2 \Bigg[ -8L_{11ij}^{V,LR} \\
& - 8L_{22ij}^{V,LR} - 8L_{33ij}^{V,LR} + 8L_{ij11}^{V,RR} + 8L_{ij22}^{V,RR} + 8L_{ij33}^{V,RR} + 8L_{ij11}^{V,RR} \\
& + 8L_{ij22}^{V,RR} - 8L_{11ij}^{V,LR} - 8L_{22ij}^{V,LR} \Big] + \alpha_s \alpha \Bigg[ -\frac{32}{9}L_{11ij}^{V,LR} - \frac{32}{9}L_{22ij}^{V,LR} \\
& - \frac{32}{9}L_{33ij}^{V,LR} - \frac{32}{9}L_{ij11}^{V,RR} - \frac{32}{9}L_{ij22}^{V,RR} - \frac{32}{9}L_{ij33}^{V,RR} + \frac{352}{9}L_{ij11}^{V,RR} + \frac{64}{9}L_{ij22}^{V,RR} \\
& + \frac{64}{9}L_{11ij}^{V,LR} + \frac{64}{9}L_{22ij}^{V,LR} \Big] + \alpha^2 \Bigg[ \frac{464}{81}L_{kki}^{V,LR} + \frac{2432}{81}L_{jkk}^{V,RR} + \frac{1408}{243}L_{11ij}^{V,LR} \\
& + \frac{1408}{243}L_{22ij}^{V,LR} + \frac{1408}{243}L_{33ij}^{V,LR} + \frac{2512}{243}L_{ij11}^{V,RR} + \frac{2512}{243}L_{ij22}^{V,RR} + \frac{2512}{243}L_{ij33}^{V,RR} \\
& + \frac{464}{81}L_{iiij}^{V,LR} + \frac{464}{81}L_{jjij}^{V,LR} + \frac{3680}{81}L_{ijii}^{V,RR} + \frac{3680}{81}L_{ijjj}^{V,RR} + \frac{2320}{243}L_{ij11}^{V,RR} + \frac{1312}{243}L_{ij22}^{V,RR} \\
& - \frac{3104}{243}L_{11ij}^{V,LR} - \frac{3104}{243}L_{22ij}^{V,LR} \Big] ;
\end{aligned}$$

$$\begin{aligned}
& + 8L_{ij22}^{V,RR} - 8L_{11ij}^{V,LR} - 8L_{22ij}^{V,LR} \Big] + \alpha_s \alpha \Bigg[ -\frac{32}{9}L_{11ij}^{V,LR} - \frac{32}{9}L_{22ij}^{V,LR} \\
& - \frac{32}{9}L_{33ij}^{V,LR} - \frac{32}{9}L_{ij11}^{V,RR} - \frac{32}{9}L_{ij22}^{V,RR} - \frac{32}{9}L_{ij33}^{V,RR} + \frac{64}{9}L_{ij11}^{V,RR} + \frac{352}{9}L_{ij22}^{V,RR} \\
& + \frac{64}{9}L_{11ij}^{V,LR} + \frac{64}{9}L_{22ij}^{V,LR} \Big] + \alpha^2 \Bigg[ \frac{464}{81}L_{kkij}^{V,LR} + \frac{2432}{81}L_{ijkk}^{V,RR} + \frac{1408}{243}L_{11ij}^{V,LR} \\
& + \frac{1408}{243}L_{22ij}^{V,LR} + \frac{1408}{243}L_{33ij}^{V,LR} + \frac{2512}{243}L_{ij11}^{V,RR} + \frac{2512}{243}L_{ij22}^{V,RR} + \frac{2512}{243}L_{ij33}^{V,RR} \\
& + \frac{464}{81}L_{iijj}^{V,LR} + \frac{464}{81}L_{jjij}^{V,LR} + \frac{3680}{81}L_{ijii}^{V,RR} + \frac{3680}{81}L_{ijjj}^{V,RR} + \frac{1312}{243}L_{ij11}^{V,RR} + \frac{2320}{243}L_{ij22}^{V,RR} \\
& - \frac{3104}{243}L_{11ij}^{V,LR} - \frac{3104}{243}L_{22ij}^{V,LR} \Big] ;
\end{aligned}$$

$$\begin{aligned}
\dot{L}_{ijkk}^{V,RR} &= e^2 \Bigg[ \frac{1}{3}L_{kkij}^{V,LR} + \frac{40}{3}L_{ijkk}^{V,RR} + \frac{1}{3}L_{11ij}^{V,LR} + \frac{1}{3}L_{22ij}^{V,LR} + \frac{1}{3}L_{33ij}^{V,LR} \\
& + \frac{1}{3}L_{ij11}^{V,RR} + \frac{1}{3}L_{ij22}^{V,RR} + \frac{1}{3}L_{ij33}^{V,RR} + \frac{1}{3}L_{iijj}^{V,LR} + \frac{1}{3}L_{jjij}^{V,LR} + \frac{4}{3}L_{ijii}^{V,RR} \\
& + \frac{4}{3}L_{ijjj}^{V,RR} - \frac{2}{3}L_{ij11}^{V,RR} - \frac{2}{3}L_{ij22}^{V,RR} - \frac{2}{3}L_{11ij}^{V,LR} - \frac{2}{3}L_{22ij}^{V,LR} \Big] + \alpha_s \alpha \Bigg[ \frac{4}{3}L_{11ij}^{V,LR} \\
& + \frac{4}{3}L_{22ij}^{V,LR} + \frac{4}{3}L_{33ij}^{V,LR} + \frac{4}{3}L_{ij11}^{V,RR} + \frac{4}{3}L_{ij22}^{V,RR} + \frac{4}{3}L_{ij33}^{V,RR} - \frac{8}{3}L_{ij11}^{V,RR} \\
& - \frac{8}{3}L_{ij22}^{V,RR} - \frac{8}{3}L_{11ij}^{V,LR} - \frac{8}{3}L_{22ij}^{V,LR} \Big] + \alpha^2 \Bigg[ -\frac{178}{27}L_{kkij}^{V,LR} - \frac{2302}{27}L_{ijkk}^{V,RR} \\
& + \frac{34}{81}L_{11ij}^{V,LR} + \frac{34}{81}L_{22ij}^{V,LR} + \frac{34}{81}L_{33ij}^{V,LR} + \frac{166}{81}L_{ij11}^{V,RR} + \frac{166}{81}L_{ij22}^{V,RR} + \frac{166}{81}L_{ij33}^{V,RR} \\
& - \frac{178}{27}L_{iijj}^{V,LR} - \frac{178}{27}L_{jjij}^{V,LR} + \frac{320}{27}L_{ijii}^{V,RR} + \frac{320}{27}L_{ijjj}^{V,RR} - \frac{314}{81}L_{ij11}^{V,RR} - \frac{314}{81}L_{ij22}^{V,RR} \\
& - \frac{842}{81}L_{11ij}^{V,LR} - \frac{842}{81}L_{22ij}^{V,LR} \Big] ;
\end{aligned}$$

$$\begin{aligned}
\dot{L}_{ijjj}^{V,RR} &= e^2 \Bigg[ \frac{2}{3}L_{kkij}^{V,LR} + \frac{8}{3}L_{ijkk}^{V,RR} + \frac{2}{3}L_{11ij}^{V,LR} + \frac{2}{3}L_{22ij}^{V,LR} + \frac{2}{3}L_{33ij}^{V,LR} \\
& + \frac{2}{3}L_{ij11}^{V,RR} + \frac{2}{3}L_{ij22}^{V,RR} + \frac{2}{3}L_{ij33}^{V,RR} + \frac{2}{3}L_{iijj}^{V,LR} + \frac{2}{3}L_{jjij}^{V,LR} + \frac{8}{3}L_{ijii}^{V,RR}
\end{aligned}$$

$$\begin{aligned}
& + \frac{44}{3} L_{ijjj}^{V,RR} - \frac{4}{3} L_{ij11}^{V,RR} - \frac{4}{3} L_{ij22}^{V,RR} - \frac{4}{3} L_{11ij}^{V,LR} - \frac{4}{3} L_{22ij}^{V,LR} \Big] + \alpha_s \alpha \Big[ \frac{8}{3} L_{11ij}^{V,LR} \\
& + \frac{8}{3} L_{22ij}^{V,LR} + \frac{8}{3} L_{33ij}^{V,LR} + \frac{8}{3} L_{ij11}^{V,RR} + \frac{8}{3} L_{ij22}^{V,RR} + \frac{8}{3} L_{ij33}^{V,RR} - \frac{16}{3} L_{ij11}^{V,RR} \\
& - \frac{16}{3} L_{ij22}^{V,RR} - \frac{16}{3} L_{11ij}^{V,LR} - \frac{16}{3} L_{22ij}^{V,LR} \Big] + \alpha^2 \Big[ - \frac{356}{27} L_{kkij}^{V,LR} + \frac{592}{27} L_{ijkk}^{V,RR} \\
& + \frac{68}{81} L_{11ij}^{V,LR} + \frac{68}{81} L_{22ij}^{V,LR} + \frac{68}{81} L_{33ij}^{V,LR} + \frac{332}{81} L_{ij11}^{V,RR} + \frac{332}{81} L_{ij22}^{V,RR} + \frac{332}{81} L_{ij33}^{V,RR} \\
& - \frac{356}{27} L_{iijj}^{V,LR} - \frac{356}{27} L_{jjij}^{V,LR} + \frac{640}{27} L_{ijii}^{V,RR} - \frac{1958}{27} L_{ijjj}^{V,RR} - \frac{628}{81} L_{ij11}^{V,RR} - \frac{628}{81} L_{ij22}^{V,RR} \\
& - \frac{1684}{81} L_{11ij}^{V,LR} - \frac{1684}{81} L_{22ij}^{V,LR} \Big] ;
\end{aligned}$$

$$\begin{aligned}
\dot{L}_{ijii}^{V,RR} &= e^2 \Big[ \frac{2}{3} L_{kkij}^{V,LR} + \frac{8}{3} L_{ijkk}^{V,RR} + \frac{2}{3} L_{11ij}^{V,LR} + \frac{2}{3} L_{22ij}^{V,LR} + \frac{2}{3} L_{33ij}^{V,LR} \\
& + \frac{2}{3} L_{ij11}^{V,RR} + \frac{2}{3} L_{ij22}^{V,RR} + \frac{2}{3} L_{ij33}^{V,RR} + \frac{2}{3} L_{iijj}^{V,LR} + \frac{2}{3} L_{jjij}^{V,LR} + \frac{44}{3} L_{ijii}^{V,RR} \\
& + \frac{8}{3} L_{ijjj}^{V,RR} - \frac{4}{3} L_{ij11}^{V,RR} - \frac{4}{3} L_{ij22}^{V,RR} - \frac{4}{3} L_{11ij}^{V,LR} - \frac{4}{3} L_{22ij}^{V,LR} \Big] + \alpha_s \alpha \Big[ \frac{8}{3} L_{11ij}^{V,LR} \\
& + \frac{8}{3} L_{22ij}^{V,LR} + \frac{8}{3} L_{33ij}^{V,LR} + \frac{8}{3} L_{ij11}^{V,RR} + \frac{8}{3} L_{ij22}^{V,RR} + \frac{8}{3} L_{ij33}^{V,RR} - \frac{16}{3} L_{ij11}^{V,RR} \\
& - \frac{16}{3} L_{ij22}^{V,RR} - \frac{16}{3} L_{11ij}^{V,LR} - \frac{16}{3} L_{22ij}^{V,LR} \Big] + \alpha^2 \Big[ - \frac{356}{27} L_{kkij}^{V,LR} + \frac{592}{27} L_{ijkk}^{V,RR} \\
& + \frac{68}{81} L_{11ij}^{V,LR} + \frac{68}{81} L_{22ij}^{V,LR} + \frac{68}{81} L_{33ij}^{V,LR} + \frac{332}{81} L_{ij11}^{V,RR} + \frac{332}{81} L_{ij22}^{V,RR} + \frac{332}{81} L_{ij33}^{V,RR} \\
& - \frac{356}{27} L_{iijj}^{V,LR} - \frac{356}{27} L_{jjij}^{V,LR} - \frac{1958}{27} L_{ijii}^{V,RR} + \frac{640}{27} L_{ijjj}^{V,RR} - \frac{628}{81} L_{ij11}^{V,RR} - \frac{628}{81} L_{ij22}^{V,RR} \\
& - \frac{1684}{81} L_{11ij}^{V,LR} - \frac{1684}{81} L_{22ij}^{V,LR} \Big] ;
\end{aligned}$$

$$\begin{aligned}
\dot{L}_{11ij}^{V,LR} &= e^2 \Big[ \frac{4}{9} L_{kkij}^{V,LR} + \frac{16}{9} L_{ijkk}^{V,RR} - \frac{32}{9} L_{11ij}^{V,LR} + \frac{4}{9} L_{22ij}^{V,LR} + \frac{4}{9} L_{33ij}^{V,LR} \\
& + \frac{4}{9} L_{ij11}^{V,RR} + \frac{4}{9} L_{ij22}^{V,RR} + \frac{4}{9} L_{ij33}^{V,RR} + \frac{4}{9} L_{iijj}^{V,LR} + \frac{4}{9} L_{jjij}^{V,LR} + \frac{16}{9} L_{ijii}^{V,RR} \\
& - \frac{4}{9} L_{ijjj}^{V,RR} - \frac{4}{9} L_{11ij}^{V,RR} - \frac{4}{9} L_{22ij}^{V,RR} - \frac{4}{9} L_{33ij}^{V,RR} \Big] ;
\end{aligned}$$

$$\begin{aligned}
& + \frac{16}{9} L_{ijjj}^{V,RR} - \frac{8}{9} L_{ij11}^{V,RR} - \frac{8}{9} L_{ij22}^{V,RR} - \frac{8}{9} L_{11ij}^{V,LR} - \frac{8}{9} L_{22ij}^{V,LR} \Big] + \alpha_s^2 \Big[ 8 L_{11ij}^{V,LR} \\
& + 8 L_{22ij}^{V,LR} + 8 L_{33ij}^{V,LR} - 8 L_{ij11}^{V,RR} - 8 L_{ij22}^{V,RR} - 8 L_{ij33}^{V,RR} - 8 L_{ij11}^{V,RR} \\
& - 8 L_{ij22}^{V,RR} + 8 L_{11ij}^{V,LR} + 8 L_{22ij}^{V,LR} \Big] + \alpha_s \alpha \Big[ \frac{160}{9} L_{11ij}^{V,LR} + \frac{16}{9} L_{22ij}^{V,LR} \\
& + \frac{16}{9} L_{33ij}^{V,LR} + \frac{16}{9} L_{ij11}^{V,RR} + \frac{16}{9} L_{ij22}^{V,RR} + \frac{16}{9} L_{ij33}^{V,RR} - \frac{32}{9} L_{ij11}^{V,RR} - \frac{32}{9} L_{ij22}^{V,RR} \\
& - \frac{32}{9} L_{11ij}^{V,LR} - \frac{32}{9} L_{22ij}^{V,LR} \Big] + \alpha^2 \Big[ - \frac{184}{81} L_{kkij}^{V,LR} - \frac{160}{81} L_{ijkk}^{V,RR} + \frac{17842}{243} L_{11ij}^{V,LR} \\
& - \frac{104}{243} L_{22ij}^{V,LR} - \frac{104}{243} L_{33ij}^{V,LR} - \frac{440}{243} L_{ij11}^{V,RR} - \frac{440}{243} L_{ij22}^{V,RR} - \frac{440}{243} L_{ij33}^{V,RR} - \frac{184}{81} L_{iij}^{V,LR} \\
& - \frac{184}{81} L_{jjij}^{V,LR} - \frac{640}{81} L_{ijii}^{V,RR} - \frac{640}{81} L_{ijjj}^{V,RR} - \frac{1640}{243} L_{ij11}^{V,RR} - \frac{1640}{243} L_{ij22}^{V,RR} - \frac{296}{243} L_{11ij}^{V,LR} \\
& - \frac{296}{243} L_{22ij}^{V,LR} \Big] ;
\end{aligned}$$

$$\begin{aligned}
\dot{L}_{de,22ij}^{V,LR} & = e^2 \Big[ \frac{4}{9} L_{kkij}^{V,LR} + \frac{16}{9} L_{ijkk}^{V,RR} + \frac{4}{9} L_{11ij}^{V,LR} - \frac{32}{9} L_{22ij}^{V,LR} + \frac{4}{9} L_{33ij}^{V,LR} \\
& + \frac{4}{9} L_{ij11}^{V,RR} + \frac{4}{9} L_{ij22}^{V,RR} + \frac{4}{9} L_{ij33}^{V,RR} + \frac{4}{9} L_{iij}^{V,LR} + \frac{4}{9} L_{jjij}^{V,LR} + \frac{16}{9} L_{ijii}^{V,RR} \\
& + \frac{16}{9} L_{ijjj}^{V,RR} - \frac{8}{9} L_{ij11}^{V,RR} - \frac{8}{9} L_{ij22}^{V,RR} - \frac{8}{9} L_{11ij}^{V,LR} - \frac{8}{9} L_{22ij}^{V,LR} \Big] + \alpha_s^2 \Big[ 8 L_{11ij}^{V,LR} \\
& + 8 L_{22ij}^{V,LR} + 8 L_{33ij}^{V,LR} - 8 L_{ij11}^{V,RR} - 8 L_{ij22}^{V,RR} - 8 L_{ij33}^{V,RR} - 8 L_{ij11}^{V,RR} \\
& - 8 L_{ij22}^{V,RR} + 8 L_{11ij}^{V,LR} + 8 L_{22ij}^{V,LR} \Big] + \alpha_s \alpha \Big[ \frac{16}{9} L_{11ij}^{V,LR} + \frac{160}{9} L_{22ij}^{V,LR} \\
& + \frac{16}{9} L_{33ij}^{V,LR} + \frac{16}{9} L_{ij11}^{V,RR} + \frac{16}{9} L_{ij22}^{V,RR} + \frac{16}{9} L_{ij33}^{V,RR} - \frac{32}{9} L_{ij11}^{V,RR} - \frac{32}{9} L_{ij22}^{V,RR} \\
& - \frac{32}{9} L_{11ij}^{V,LR} - \frac{32}{9} L_{22ij}^{V,LR} \Big] + \alpha^2 \Big[ - \frac{184}{81} L_{kkij}^{V,LR} - \frac{160}{81} L_{ijkk}^{V,RR} - \frac{104}{243} L_{11ij}^{V,LR} \\
& + \frac{17842}{243} L_{22ij}^{V,LR} - \frac{104}{243} L_{33ij}^{V,LR} - \frac{440}{243} L_{ij11}^{V,RR} - \frac{440}{243} L_{ij22}^{V,RR} - \frac{440}{243} L_{ij33}^{V,RR}
\end{aligned}$$



$$\begin{aligned}
& -8L_{ij22}^{V,RR} + 8L_{11ij}^{V,LR} + 8L_{22ij}^{V,LR} \Big] + \alpha_s \alpha \Big[ -\frac{32}{9}L_{11ij}^{V,LR} - \frac{32}{9}L_{22ij}^{V,LR} \\
& -\frac{32}{9}L_{33ij}^{V,LR} - \frac{32}{9}L_{ij11}^{V,RR} - \frac{32}{9}L_{ij22}^{V,RR} - \frac{32}{9}L_{ij33}^{V,RR} + \frac{64}{9}L_{ij11}^{V,RR} + \frac{64}{9}L_{ij22}^{V,RR} \\
& -\frac{224}{9}L_{11ij}^{V,LR} + \frac{64}{9}L_{22ij}^{V,LR} \Big] + \alpha^2 \Big[ \frac{1808}{81}L_{kkij}^{V,LR} + \frac{896}{81}L_{ijkk}^{V,RR} + \frac{1792}{243}L_{11ij}^{V,LR} \\
& + \frac{1792}{243}L_{22ij}^{V,LR} + \frac{1792}{243}L_{33ij}^{V,LR} + \frac{1168}{243}L_{ij11}^{V,RR} + \frac{1168}{243}L_{ij22}^{V,RR} + \frac{1168}{243}L_{ij33}^{V,RR} \\
& + \frac{1808}{81}L_{iijj}^{V,LR} + \frac{1808}{81}L_{jjij}^{V,LR} + \frac{992}{81}L_{ijii}^{V,RR} + \frac{992}{81}L_{ijjj}^{V,RR} - \frac{1184}{243}L_{ij11}^{V,RR} - \frac{1184}{243}L_{ij22}^{V,RR} \\
& -\frac{43328}{243}L_{11ij}^{V,LR} + \frac{1312}{243}L_{22ij}^{V,LR} \Big] ; \\
\dot{L}_{22ij}^{V,LR} = & e^2 \Big[ -\frac{8}{9}L_{kkij}^{V,LR} - \frac{32}{9}L_{ijkk}^{V,RR} - \frac{8}{9}L_{11ij}^{V,LR} - \frac{8}{9}L_{22ij}^{V,LR} - \frac{8}{9}L_{33ij}^{V,LR} \\
& -\frac{8}{9}L_{ij11}^{V,RR} - \frac{8}{9}L_{ij22}^{V,RR} - \frac{8}{9}L_{ij33}^{V,RR} - \frac{8}{9}L_{iijj}^{V,LR} - \frac{8}{9}L_{jjij}^{V,LR} - \frac{32}{9}L_{ijii}^{V,RR} \\
& -\frac{32}{9}L_{ijjj}^{V,RR} + \frac{16}{9}L_{ij11}^{V,RR} + \frac{16}{9}L_{ij22}^{V,RR} + \frac{16}{9}L_{11ij}^{V,LR} + \frac{88}{9}L_{22ij}^{V,LR} \Big] + \alpha_s^2 \Big[ 8L_{11ij}^{V,LR} \\
& + 8L_{22ij}^{V,LR} + 8L_{33ij}^{V,LR} - 8L_{ij11}^{V,RR} - 8L_{ij22}^{V,RR} - 8L_{ij33}^{V,RR} - 8L_{ij11}^{V,RR} \\
& - 8L_{ij22}^{V,RR} + 8L_{11ij}^{V,LR} + 8L_{22ij}^{V,LR} \Big] + \alpha_s \alpha \Big[ -\frac{32}{9}L_{11ij}^{V,LR} - \frac{32}{9}L_{22ij}^{V,LR} \\
& -\frac{32}{9}L_{33ij}^{V,LR} - \frac{32}{9}L_{ij11}^{V,RR} - \frac{32}{9}L_{ij22}^{V,RR} - \frac{32}{9}L_{ij33}^{V,RR} + \frac{64}{9}L_{ij11}^{V,RR} + \frac{64}{9}L_{ij22}^{V,RR} \\
& + \frac{64}{9}L_{ij33}^{V,RR} - \frac{224}{9}L_{11ij}^{V,LR} + \frac{64}{9}L_{22ij}^{V,LR} \Big] + \alpha^2 \Big[ \frac{1808}{81}L_{kkij}^{V,LR} + \frac{896}{81}L_{ijkk}^{V,RR} + \frac{1792}{243}L_{11ij}^{V,LR} \\
& + \frac{1792}{243}L_{22ij}^{V,LR} + \frac{1792}{243}L_{33ij}^{V,LR} + \frac{1168}{243}L_{ij11}^{V,RR} + \frac{1168}{243}L_{ij22}^{V,RR} + \frac{1168}{243}L_{ij33}^{V,RR} \\
& + \frac{1808}{81}L_{iijj}^{V,LR} + \frac{1808}{81}L_{jjij}^{V,LR} + \frac{992}{81}L_{ijii}^{V,RR} + \frac{992}{81}L_{ijjj}^{V,RR} - \frac{1184}{243}L_{ij11}^{V,RR} - \frac{1184}{243}L_{ij22}^{V,RR} \\
& + \frac{1312}{243}L_{11ij}^{V,LR} - \frac{43328}{243}L_{22ij}^{V,LR} \Big] ;
\end{aligned}$$

$$\begin{aligned}
\dot{L}_{kkij}^{V,LR} = & e^2 \left[ -\frac{32}{3} L_{kkij}^{V,LR} + \frac{16}{3} L_{ijkk}^{V,RR} + \frac{4}{3} L_{11ij}^{V,LR} + \frac{4}{3} L_{22ij}^{V,LR} + \frac{4}{3} L_{33ij}^{V,LR} \right. \\
& + \frac{4}{3} L_{ij11}^{V,RR} + \frac{4}{3} L_{ij22}^{V,RR} + \frac{4}{3} L_{ij33}^{V,RR} + \frac{4}{3} L_{iiij}^{V,LR} + \frac{4}{3} L_{jjij}^{V,LR} + \frac{16}{3} L_{ijii}^{V,RR} \\
& + \frac{16}{3} L_{ijjj}^{V,RR} - \frac{8}{3} L_{ij11}^{V,RR} - \frac{8}{3} L_{ij22}^{V,RR} - \frac{8}{3} L_{11ij}^{V,LR} - \frac{8}{3} L_{22ij}^{V,LR} \left. \right] + \alpha_s \alpha \left[ \frac{16}{3} L_{11ij}^{V,LR} \right. \\
& + \frac{16}{3} L_{22ij}^{V,LR} + \frac{16}{3} L_{33ij}^{V,LR} + \frac{16}{3} L_{ij11}^{V,RR} + \frac{16}{3} L_{ij22}^{V,RR} + \frac{16}{3} L_{ij33}^{V,RR} - \frac{32}{3} L_{ij11}^{V,RR} \\
& - \frac{32}{3} L_{ij22}^{V,RR} - \frac{32}{3} L_{11ij}^{V,LR} - \frac{32}{3} L_{22ij}^{V,LR} \left. \right] + \alpha^2 \left[ \frac{6386}{27} L_{kkij}^{V,LR} + \frac{32}{27} L_{ijkk}^{V,RR} \right. \\
& + \frac{424}{81} L_{11ij}^{V,LR} + \frac{424}{81} L_{22ij}^{V,LR} + \frac{424}{81} L_{33ij}^{V,LR} - \frac{344}{81} L_{ij11}^{V,RR} - \frac{344}{81} L_{ij22}^{V,RR} - \frac{344}{81} L_{ij33}^{V,RR} \\
& + \frac{296}{27} L_{iiij}^{V,LR} + \frac{296}{27} L_{jjij}^{V,LR} - \frac{736}{27} L_{ijii}^{V,RR} - \frac{736}{27} L_{ijjj}^{V,RR} - \frac{3128}{81} L_{ij11}^{V,RR} - \frac{3128}{81} L_{ij22}^{V,RR} \\
& \left. - \frac{56}{81} L_{11ij}^{V,LR} - \frac{56}{81} L_{22ij}^{V,LR} \right];
\end{aligned}$$

$$\begin{aligned}
\dot{L}_{jjij}^{V,LR} = & e^2 \left[ \frac{4}{3} L_{kkij}^{V,LR} + \frac{16}{3} L_{ijkk}^{V,RR} + \frac{4}{3} L_{11ij}^{V,LR} + \frac{4}{3} L_{22ij}^{V,LR} + \frac{4}{3} L_{33ij}^{V,LR} \right. \\
& + \frac{4}{3} L_{ij11}^{V,RR} + \frac{4}{3} L_{ij22}^{V,RR} + \frac{4}{3} L_{ij33}^{V,RR} + \frac{4}{3} L_{iiij}^{V,LR} - \frac{32}{3} L_{jjij}^{V,LR} + \frac{16}{3} L_{ijii}^{V,RR} \\
& + \frac{16}{3} L_{ijjj}^{V,RR} - \frac{8}{3} L_{ij11}^{V,RR} - \frac{8}{3} L_{ij22}^{V,RR} - \frac{8}{3} L_{11ij}^{V,LR} - \frac{8}{3} L_{22ij}^{V,LR} \left. \right] + \alpha_s \alpha \left[ \frac{16}{3} L_{11ij}^{V,LR} \right. \\
& + \frac{16}{3} L_{22ij}^{V,LR} + \frac{16}{3} L_{33ij}^{V,LR} + \frac{16}{3} L_{ij11}^{V,RR} + \frac{16}{3} L_{ij22}^{V,RR} + \frac{16}{3} L_{ij33}^{V,RR} - \frac{32}{3} L_{ij11}^{V,RR} \\
& - \frac{32}{3} L_{ij22}^{V,RR} - \frac{32}{3} L_{11ij}^{V,LR} - \frac{32}{3} L_{22ij}^{V,LR} \left. \right] + \alpha^2 \left[ \frac{296}{27} L_{kkij}^{V,LR} + \frac{32}{27} L_{ijkk}^{V,RR} \right. \\
& + \frac{424}{81} L_{11ij}^{V,LR} + \frac{424}{81} L_{22ij}^{V,LR} + \frac{424}{81} L_{33ij}^{V,LR} - \frac{344}{81} L_{ij11}^{V,RR} - \frac{344}{81} L_{ij22}^{V,RR} - \frac{344}{81} L_{ij33}^{V,RR} \\
& + \frac{296}{27} L_{iiij}^{V,LR} + \frac{6386}{27} L_{jjij}^{V,LR} - \frac{736}{27} L_{ijii}^{V,RR} - \frac{736}{27} L_{ijjj}^{V,RR} - \frac{3128}{81} L_{ij11}^{V,RR} - \frac{3128}{81} L_{ij22}^{V,RR} \\
& \left. - \frac{56}{81} L_{11ij}^{V,LR} - \frac{56}{81} L_{22ij}^{V,LR} \right];
\end{aligned}$$

$$\begin{aligned}
\dot{L}_{iiij}^{V,LR} = & e^2 \left[ \frac{4}{3} L_{kkij}^{V,LR} + \frac{16}{3} L_{ijkk}^{V,RR} + \frac{4}{3} L_{11ij}^{V,LR} + \frac{4}{3} L_{22ij}^{V,LR} + \frac{4}{3} L_{33ij}^{V,LR} \right. \\
& + \frac{4}{3} L_{ij11}^{V,RR} + \frac{4}{3} L_{ij22}^{V,RR} + \frac{4}{3} L_{ij33}^{V,RR} - \frac{32}{3} L_{iii}^{V,LR} + \frac{4}{3} L_{jjij}^{V,LR} + \frac{16}{3} L_{ijii}^{V,RR} \\
& + \frac{16}{3} L_{ijjj}^{V,RR} - \frac{8}{3} L_{ij11}^{V,RR} - \frac{8}{3} L_{ij22}^{V,RR} - \frac{8}{3} L_{ij11}^{V,LR} - \frac{8}{3} L_{22ij}^{V,LR} \left. \right] + \alpha_s \alpha \left[ \frac{16}{3} L_{11ij}^{V,LR} \right. \\
& + \frac{16}{3} L_{22ij}^{V,LR} + \frac{16}{3} L_{33ij}^{V,LR} + \frac{16}{3} L_{ij11}^{V,RR} + \frac{16}{3} L_{ij22}^{V,RR} + \frac{16}{3} L_{ij33}^{V,RR} - \frac{32}{3} L_{ij11}^{V,RR} \\
& - \frac{32}{3} L_{ij22}^{V,RR} - \frac{32}{3} L_{ij11}^{V,LR} - \frac{32}{3} L_{22ij}^{V,LR} \left. \right] + \alpha^2 \left[ \frac{296}{27} L_{kkij}^{V,LR} + \frac{32}{27} L_{ijkk}^{V,RR} \right. \\
& + \frac{424}{81} L_{11ij}^{V,LR} + \frac{424}{81} L_{22ij}^{V,LR} + \frac{424}{81} L_{33ij}^{V,LR} - \frac{344}{81} L_{ij11}^{V,RR} - \frac{344}{81} L_{ij22}^{V,RR} - \frac{344}{81} L_{ij33}^{V,RR} \\
& + \frac{6386}{27} L_{iii}^{V,LR} + \frac{296}{27} L_{jjij}^{V,LR} - \frac{736}{27} L_{ijii}^{V,RR} - \frac{736}{27} L_{ijjj}^{V,RR} - \frac{3128}{81} L_{ij11}^{V,RR} - \frac{3128}{81} L_{ij22}^{V,RR} \\
& \left. - \frac{56}{81} L_{ij11}^{V,LR} - \frac{56}{81} L_{22ij}^{V,LR} \right] ;
\end{aligned}$$

$$\dot{L}_{jkki}^{V,LR} = \frac{2030}{9} \alpha^2 L_{jkki}^{V,LR} - 12e^2 L_{jkki}^{V,LR} ;$$

$$\dot{L}_{11ij}^{V,LL} = 0 ;$$

$$\dot{L}_{22ij}^{V,LL} = 0 ;$$

$$\dot{L}_{33ij}^{V,LL} = 0 ;$$

$$\dot{L}_{ij11}^{V,LR} = 0 ;$$

$$\dot{L}_{ij22}^{V,LR} = 0 ;$$

$$\dot{L}_{ij33}^{V,LR} = 0 ;$$

$$\dot{L}_{ij11}^{S,LR} = \frac{373}{9} \alpha^2 L_{ij11}^{S,LR} - 6e^2 L_{ij11}^{S,LR} ;$$

$$\dot{L}_{ij22}^{S,LR} = \frac{373}{9} \alpha^2 L_{ij22}^{S,LR} - 6e^2 L_{ij22}^{S,LR} ;$$

$$\dot{L}_{ij33}^{S,LR} = \frac{373}{9} \alpha^2 L_{ij33}^{S,LR} - 6e^2 L_{ij33}^{S,LR} ;$$



$$\begin{aligned}
\dot{L}_{11ij}^{S,LL} &= \frac{373}{9}\alpha^2 L_{11ij}^{S,LL} - 6e^2 L_{11ij}^{S,LL} ; \\
\dot{L}_{11ij}^{T,LL} &= 2e^2 L_{11ij}^{T,LL} - \frac{1553}{27}\alpha^2 L_{11ij}^{T,LL} ; \\
\dot{L}_{22ij}^{S,LL} &= \frac{373}{9}\alpha^2 L_{22ij}^{S,LL} - 6e^2 L_{22ij}^{S,LL} ; \\
\dot{L}_{22ij}^{T,LL} &= 2e^2 L_{22ij}^{T,LL} - \frac{1553}{27}\alpha^2 L_{22ij}^{T,LL} ; \\
\dot{L}_{33ij}^{S,LL} &= \frac{373}{9}\alpha^2 L_{33ij}^{S,LL} - 6e^2 L_{33ij}^{S,LL} ; \\
\dot{L}_{33ij}^{T,LL} &= 2e^2 L_{33ij}^{T,LL} - \frac{1553}{27}\alpha^2 L_{33ij}^{T,LL} ;
\end{aligned}$$

## 1.8 $\Delta F = 1^{\bar{f}f} : \nu\text{-type } (\bar{\nu}_i \nu_j \bar{f}_k f_k)$

$$\begin{aligned}
\dot{L}_{ij11}^{V,LL} &= e^2 \left[ \frac{4}{3} L_{ij11}^{V,LL} + \frac{4}{3} L_{ij22}^{V,LL} + \frac{4}{3} L_{ij33}^{V,LL} + \frac{4}{3} L_{ij11}^{V,LR} + \frac{4}{3} L_{ij22}^{V,LR} \right. \\
&\quad + \frac{4}{3} L_{ij33}^{V,LR} + \frac{4}{3} L_{ij11}^{V,LL} + \frac{4}{3} L_{ij22}^{V,LL} + \frac{4}{3} L_{ij33}^{V,LL} + \frac{4}{3} L_{ij11}^{V,LR} + \frac{4}{3} L_{ij22}^{V,LR} + \frac{4}{3} L_{ij33}^{V,LR} \\
&\quad \left. + \frac{4}{3} L_{ij33}^{V,LR} - \frac{8}{3} L_{ij11}^{V,LL} - \frac{8}{3} L_{ij22}^{V,LL} - \frac{8}{3} L_{ij11}^{V,LR} - \frac{8}{3} L_{ij22}^{V,LR} \right] \\
&\quad + \alpha_s \alpha \left[ \frac{16}{3} L_{ij11}^{V,LL} + \frac{16}{3} L_{ij22}^{V,LL} + \frac{16}{3} L_{ij33}^{V,LL} + \frac{16}{3} L_{ij11}^{V,LR} + \frac{16}{3} L_{ij22}^{V,LR} \right. \\
&\quad \left. + \frac{16}{3} L_{ij33}^{V,LR} - \frac{32}{3} L_{ij11}^{V,LL} - \frac{32}{3} L_{ij22}^{V,LL} - \frac{32}{3} L_{ij11}^{V,LR} - \frac{32}{3} L_{ij22}^{V,LR} \right] \\
&\quad + \alpha^2 \left[ \frac{40}{9} L_{ij11}^{V,LL} + \frac{40}{9} L_{ij22}^{V,LL} + \frac{40}{9} L_{ij33}^{V,LL} - \frac{32}{9} L_{ij11}^{V,LR} - \frac{32}{9} L_{ij22}^{V,LR} \right. \\
&\quad - \frac{32}{9} L_{ij33}^{V,LR} + 16 L_{ij11}^{V,LL} + 16 L_{ij22}^{V,LL} + 16 L_{ij33}^{V,LL} - 8 L_{ij11}^{V,LR} - 8 L_{ij22}^{V,LR} \\
&\quad \left. - 8 L_{ij33}^{V,LR} + \frac{112}{9} L_{ij11}^{V,LL} + \frac{112}{9} L_{ij22}^{V,LL} - \frac{176}{9} L_{ij11}^{V,LR} - \frac{176}{9} L_{ij22}^{V,LR} \right] ; \\
\dot{L}_{ij22}^{V,LL} &= e^2 \left[ \frac{4}{3} L_{ij11}^{V,LL} + \frac{4}{3} L_{ij22}^{V,LL} + \frac{4}{3} L_{ij33}^{V,LL} + \frac{4}{3} L_{ij11}^{V,LR} + \frac{4}{3} L_{ij22}^{V,LR} \right.
\end{aligned}$$

$$\begin{aligned}
& + \frac{4}{3}L_{\nu d}^{V,LR} + \frac{4}{3}L_{ij11}^{V,LL} + \frac{4}{3}L_{ij22}^{V,LL} + \frac{4}{3}L_{ij33}^{V,LL} + \frac{4}{3}L_{ij11}^{V,LR} + \frac{4}{3}L_{ij22}^{V,LR} \\
& + \frac{4}{3}L_{ij33}^{V,LR} - \frac{8}{3}L_{ij11}^{V,LL} - \frac{8}{3}L_{ij22}^{V,LL} - \frac{8}{3}L_{ij11}^{V,LR} - \frac{8}{3}L_{ij22}^{V,LR} \Big] \\
& + \alpha_s \alpha \left[ \frac{16}{3}L_{ij11}^{V,LL} + \frac{16}{3}L_{ij22}^{V,LL} + \frac{16}{3}L_{ij33}^{V,LL} + \frac{16}{3}L_{ij11}^{V,LR} + \frac{16}{3}L_{ij22}^{V,LR} \right. \\
& + \left. \frac{16}{3}L_{ij33}^{V,LR} - \frac{32}{3}L_{ij11}^{V,LL} - \frac{32}{3}L_{ij22}^{V,LL} - \frac{32}{3}L_{ij11}^{V,LR} - \frac{32}{3}L_{ij22}^{V,LR} \right] \\
& + \alpha^2 \left[ \frac{40}{9}L_{ij11}^{V,LL} + \frac{40}{9}L_{ij22}^{V,LL} + \frac{40}{9}L_{ij33}^{V,LL} - \frac{32}{9}L_{ij11}^{V,LR} - \frac{32}{9}L_{ij22}^{V,LR} \right. \\
& - \frac{32}{9}L_{ij33}^{V,LR} + 16L_{ij11}^{V,LL} + 16L_{ij22}^{V,LL} + 16L_{ij33}^{V,LL} - 8L_{ij11}^{V,LR} - 8L_{ij22}^{V,LR} \\
& - 8L_{ij33}^{V,LR} + \frac{112}{9}L_{ij11}^{V,LL} + \frac{112}{9}L_{ij22}^{V,LL} - \frac{176}{9}L_{ij11}^{V,LR} - \frac{176}{9}L_{ij22}^{V,LR} \Big] ; \\
\dot{L}_{ij33}^{V,LL} & = e^2 \left[ \frac{4}{3}L_{ij11}^{V,LL} + \frac{4}{3}L_{ij22}^{V,LL} + \frac{4}{3}L_{ij33}^{V,LL} + \frac{4}{3}L_{ij11}^{V,LR} + \frac{4}{3}L_{ij22}^{V,LR} \right. \\
& + \frac{4}{3}L_{ij33}^{V,LR} + \frac{4}{3}L_{ij11}^{V,LL} + \frac{4}{3}L_{ij22}^{V,LL} + \frac{4}{3}L_{ij33}^{V,LL} + \frac{4}{3}L_{ij11}^{V,LR} + \frac{4}{3}L_{ij22}^{V,LR} \\
& + \frac{4}{3}L_{ij33}^{V,LR} - \frac{8}{3}L_{ij11}^{V,LL} - \frac{8}{3}L_{ij22}^{V,LL} - \frac{8}{3}L_{ij11}^{V,LR} - \frac{8}{3}L_{ij22}^{V,LR} \Big] \\
& + \alpha_s \alpha \left[ \frac{16}{3}L_{ij11}^{V,LL} + \frac{16}{3}L_{ij22}^{V,LL} + \frac{16}{3}L_{ij33}^{V,LL} + \frac{16}{3}L_{ij11}^{V,LR} + \frac{16}{3}L_{ij22}^{V,LR} \right. \\
& + \left. \frac{16}{3}L_{ij33}^{V,LR} - \frac{32}{3}L_{ij11}^{V,LL} - \frac{32}{3}L_{ij22}^{V,LL} - \frac{32}{3}L_{ij11}^{V,LR} - \frac{32}{3}L_{ij22}^{V,LR} \right] \\
& + \alpha^2 \left[ \frac{40}{9}L_{ij11}^{V,LL} + \frac{40}{9}L_{ij22}^{V,LL} + \frac{40}{9}L_{ij33}^{V,LL} - \frac{32}{9}L_{ij11}^{V,LR} - \frac{32}{9}L_{ij22}^{V,LR} \right. \\
& - \frac{32}{9}L_{ij33}^{V,LR} + 16L_{ij11}^{V,LL} + 16L_{ij22}^{V,LL} + 16L_{ij33}^{V,LL} - 8L_{ij11}^{V,LR} - 8L_{ij22}^{V,LR} \\
& - 8L_{ij33}^{V,LR} + \frac{112}{9}L_{ij11}^{V,LL} + \frac{112}{9}L_{ij22}^{V,LL} - \frac{176}{9}L_{ij11}^{V,LR} - \frac{176}{9}L_{ij22}^{V,LR} \Big] ;
\end{aligned}$$

$$\begin{aligned}
\dot{L}_{\nu d, ij11}^{V,LL} = & e^2 \left[ \frac{4}{9} L_{\nu d, ij11}^{V,LL} + \frac{4}{9} L_{\nu d, ij22}^{V,LL} + \frac{4}{9} L_{\nu d, ij33}^{V,LL} + \frac{4}{9} L_{\nu d, ij11}^{V,LR} + \frac{4}{9} L_{\nu d, ij22}^{V,LR} \right. \\
& + \frac{4}{9} L_{\nu d, ij33}^{V,LR} + \frac{4}{9} L_{\nu e, ij11}^{V,LL} + \frac{4}{9} L_{\nu e, ij22}^{V,LL} + \frac{4}{9} L_{\nu e, ij33}^{V,LL} + \frac{4}{9} L_{\nu e, ij11}^{V,LR} + \frac{4}{9} L_{\nu e, ij22}^{V,LR} \\
& \left. + \frac{4}{9} L_{\nu e, ij33}^{V,LR} - \frac{8}{9} L_{\nu u, ij11}^{V,LL} - \frac{8}{9} L_{\nu u, ij22}^{V,LL} - \frac{8}{9} L_{\nu u, ij33}^{V,LL} - \frac{8}{9} L_{\nu u, ij11}^{V,LR} - \frac{8}{9} L_{\nu u, ij22}^{V,LR} \right] \\
& + \alpha_s^2 \left[ 8 L_{\nu d, ij11}^{V,LL} + 8 L_{\nu d, ij22}^{V,LL} + 8 L_{\nu d, ij33}^{V,LL} - 8 L_{\nu d, ij11}^{V,LR} - 8 L_{\nu d, ij22}^{V,LR} \right. \\
& \left. - 8 L_{\nu d, ij33}^{V,LR} + 8 L_{\nu u, ij11}^{V,LL} + 8 L_{\nu u, ij22}^{V,LL} - 8 L_{\nu u, ij11}^{V,LR} - 8 L_{\nu u, ij22}^{V,LR} \right] \\
& + \alpha_s \alpha \left[ \frac{16}{9} L_{\nu d, ij11}^{V,LL} + \frac{16}{9} L_{\nu d, ij22}^{V,LL} + \frac{16}{9} L_{\nu d, ij33}^{V,LL} + \frac{16}{9} L_{\nu d, ij11}^{V,LR} + \frac{16}{9} L_{\nu d, ij22}^{V,LR} \right. \\
& \left. + \frac{16}{9} L_{\nu d, ij33}^{V,LR} - \frac{32}{9} L_{\nu u, ij11}^{V,LL} - \frac{32}{9} L_{\nu u, ij22}^{V,LL} - \frac{32}{9} L_{\nu u, ij11}^{V,LR} - \frac{32}{9} L_{\nu u, ij22}^{V,LR} \right] \\
& + \alpha^2 \left[ \frac{16}{27} L_{\nu d, ij11}^{V,LL} + \frac{16}{27} L_{\nu d, ij22}^{V,LL} + \frac{16}{27} L_{\nu d, ij33}^{V,LL} - \frac{8}{27} L_{\nu d, ij11}^{V,LR} - \frac{8}{27} L_{\nu d, ij22}^{V,LR} \right. \\
& - \frac{8}{27} L_{\nu d, ij33}^{V,LR} + \frac{8}{3} L_{\nu e, ij11}^{V,LL} + \frac{8}{3} L_{\nu e, ij22}^{V,LL} + \frac{8}{3} L_{\nu e, ij33}^{V,LL} + \frac{16}{27} L_{\nu u, ij11}^{V,LL} + \frac{16}{27} L_{\nu u, ij22}^{V,LL} \\
& \left. - \frac{80}{27} L_{\nu u, ij11}^{V,LR} - \frac{80}{27} L_{\nu u, ij22}^{V,LR} \right];
\end{aligned}$$

$$\begin{aligned}
\dot{L}_{\nu d, ij22}^{V,LL} = & e^2 \left[ \frac{4}{9} L_{\nu d, ij11}^{V,LL} + \frac{4}{9} L_{\nu d, ij22}^{V,LL} + \frac{4}{9} L_{\nu d, ij33}^{V,LL} + \frac{4}{9} L_{\nu d, ij11}^{V,LR} + \frac{4}{9} L_{\nu d, ij22}^{V,LR} \right. \\
& + \frac{4}{9} L_{\nu d, ij33}^{V,LR} + \frac{4}{9} L_{\nu e, ij11}^{V,LL} + \frac{4}{9} L_{\nu e, ij22}^{V,LL} + \frac{4}{9} L_{\nu e, ij33}^{V,LL} + \frac{4}{9} L_{\nu e, ij11}^{V,LR} + \frac{4}{9} L_{\nu e, ij22}^{V,LR} \\
& \left. + \frac{4}{9} L_{\nu e, ij33}^{V,LR} - \frac{8}{9} L_{\nu u, ij11}^{V,LL} - \frac{8}{9} L_{\nu u, ij22}^{V,LL} - \frac{8}{9} L_{\nu u, ij33}^{V,LL} - \frac{8}{9} L_{\nu u, ij11}^{V,LR} - \frac{8}{9} L_{\nu u, ij22}^{V,LR} \right] \\
& + \alpha_s^2 \left[ 8 L_{\nu d, ij11}^{V,LL} + 8 L_{\nu d, ij22}^{V,LL} + 8 L_{\nu d, ij33}^{V,LL} - 8 L_{\nu d, ij11}^{V,LR} - 8 L_{\nu d, ij22}^{V,LR} \right. \\
& \left. - 8 L_{\nu d, ij33}^{V,LR} + 8 L_{\nu u, ij11}^{V,LL} + 8 L_{\nu u, ij22}^{V,LL} - 8 L_{\nu u, ij11}^{V,LR} - 8 L_{\nu u, ij22}^{V,LR} \right]
\end{aligned}$$

$$\begin{aligned}
& + \alpha_s \alpha \left[ \frac{16}{9} L_{ij11}^{V,LL} + \frac{16}{9} L_{ij22}^{V,LL} + \frac{16}{9} L_{ij33}^{V,LL} + \frac{16}{9} L_{ij11}^{V,LR} + \frac{16}{9} L_{ij22}^{V,LR} \right. \\
& + \left. \frac{16}{9} L_{ij33}^{V,LR} - \frac{32}{9} L_{ij11}^{V,LL} - \frac{32}{9} L_{ij22}^{V,LL} - \frac{32}{9} L_{ij11}^{V,LR} - \frac{32}{9} L_{ij22}^{V,LR} \right] \\
& + \alpha^2 \left[ \frac{16}{27} L_{ij11}^{V,LL} + \frac{16}{27} L_{ij22}^{V,LL} + \frac{16}{27} L_{ij33}^{V,LL} - \frac{8}{27} L_{ij11}^{V,LR} - \frac{8}{27} L_{ij22}^{V,LR} \right. \\
& - \frac{8}{27} L_{ij33}^{V,LR} + \frac{8}{3} L_{ij11}^{V,LL} + \frac{8}{3} L_{ij22}^{V,LL} + \frac{8}{3} L_{ij33}^{V,LL} + \frac{16}{27} L_{ij11}^{V,LL} + \frac{16}{27} L_{ij22}^{V,LL} \\
& \left. - \frac{80}{27} L_{ij11}^{V,LR} - \frac{80}{27} L_{ij22}^{V,LR} \right]; \\
\dot{L}_{ij33}^{V,LL} & = e^2 \left[ \frac{4}{9} L_{ij11}^{V,LL} + \frac{4}{9} L_{ij22}^{V,LL} + \frac{4}{9} L_{ij33}^{V,LL} + \frac{4}{9} L_{ij11}^{V,LR} + \frac{4}{9} L_{ij22}^{V,LR} \right. \\
& + \frac{4}{9} L_{ij33}^{V,LR} + \frac{4}{9} L_{ij11}^{V,LL} + \frac{4}{9} L_{ij22}^{V,LL} + \frac{4}{9} L_{ij33}^{V,LL} + \frac{4}{9} L_{ij11}^{V,LR} + \frac{4}{9} L_{ij22}^{V,LR} \\
& \left. + \frac{4}{9} L_{ij33}^{V,LR} - \frac{8}{9} L_{ij11}^{V,LL} - \frac{8}{9} L_{ij22}^{V,LL} - \frac{8}{9} L_{ij11}^{V,LR} - \frac{8}{9} L_{ij22}^{V,LR} \right] \\
& + \alpha_s^2 \left[ 8 L_{ij11}^{V,LL} + 8 L_{ij22}^{V,LL} + 8 L_{ij33}^{V,LL} - 8 L_{ij11}^{V,LR} - 8 L_{ij22}^{V,LR} \right. \\
& \left. - 8 L_{ij33}^{V,LR} + 8 L_{ij11}^{V,LL} + 8 L_{ij22}^{V,LL} - 8 L_{ij11}^{V,LR} - 8 L_{ij22}^{V,LR} \right] \\
& + \alpha_s \alpha \left[ \frac{16}{9} L_{ij11}^{V,LL} + \frac{16}{9} L_{ij22}^{V,LL} + \frac{16}{9} L_{ij33}^{V,LL} + \frac{16}{9} L_{ij11}^{V,LR} + \frac{16}{9} L_{ij22}^{V,LR} \right. \\
& + \left. \frac{16}{9} L_{ij33}^{V,LR} - \frac{32}{9} L_{ij11}^{V,LL} - \frac{32}{9} L_{ij22}^{V,LL} - \frac{32}{9} L_{ij11}^{V,LR} - \frac{32}{9} L_{ij22}^{V,LR} \right] \\
& + \alpha^2 \left[ \frac{16}{27} L_{ij11}^{V,LL} + \frac{16}{27} L_{ij22}^{V,LL} + \frac{16}{27} L_{ij33}^{V,LL} - \frac{8}{27} L_{ij11}^{V,LR} - \frac{8}{27} L_{ij22}^{V,LR} \right. \\
& - \frac{8}{27} L_{ij33}^{V,LR} + \frac{8}{3} L_{ij11}^{V,LL} + \frac{8}{3} L_{ij22}^{V,LL} + \frac{8}{3} L_{ij33}^{V,LL} + \frac{16}{27} L_{ij11}^{V,LL} + \frac{16}{27} L_{ij22}^{V,LL} \\
& \left. - \frac{80}{27} L_{ij11}^{V,LR} - \frac{80}{27} L_{ij22}^{V,LR} \right];
\end{aligned}$$

$$\begin{aligned}
\dot{L}_{ij11}^{V,LL} &= e^2 \left[ -\frac{8}{9}L_{ij11}^{V,LL} - \frac{8}{9}L_{ij22}^{V,LL} - \frac{8}{9}L_{ij33}^{V,LL} - \frac{8}{9}L_{ij11}^{V,LR} - \frac{8}{9}L_{ij22}^{V,LR} \right. \\
&\quad - \frac{8}{9}L_{ij33}^{V,LR} - \frac{8}{9}L_{ij11}^{V,LL} - \frac{8}{9}L_{ij22}^{V,LL} - \frac{8}{9}L_{ij33}^{V,LL} - \frac{8}{9}L_{ij11}^{V,LR} - \frac{8}{9}L_{ij22}^{V,LR} \\
&\quad \left. - \frac{8}{9}L_{ij33}^{V,LR} + \frac{16}{9}L_{ij11}^{V,LL} + \frac{16}{9}L_{ij22}^{V,LL} + \frac{16}{9}L_{ij33}^{V,LL} + \frac{16}{9}L_{ij11}^{V,LR} + \frac{16}{9}L_{ij22}^{V,LR} \right] \\
&\quad + \alpha_s^2 \left[ 8L_{ij11}^{V,LL} + 8L_{ij22}^{V,LL} + 8L_{ij33}^{V,LL} - 8L_{ij11}^{V,LR} - 8L_{ij22}^{V,LR} \right. \\
&\quad \left. - 8L_{ij33}^{V,LR} + 8L_{ij11}^{V,LL} + 8L_{ij22}^{V,LL} - 8L_{ij11}^{V,LR} - 8L_{ij22}^{V,LR} \right] \\
&\quad + \alpha_s \alpha \left[ -\frac{32}{9}L_{ij11}^{V,LL} - \frac{32}{9}L_{ij22}^{V,LL} - \frac{32}{9}L_{ij33}^{V,LL} - \frac{32}{9}L_{ij11}^{V,LR} - \frac{32}{9}L_{ij22}^{V,LR} \right. \\
&\quad \left. - \frac{32}{9}L_{ij33}^{V,LR} + \frac{64}{9}L_{ij11}^{V,LL} + \frac{64}{9}L_{ij22}^{V,LL} + \frac{64}{9}L_{ij33}^{V,LL} + \frac{64}{9}L_{ij11}^{V,LR} + \frac{64}{9}L_{ij22}^{V,LR} \right] \\
&\quad + \alpha^2 \left[ \frac{40}{27}L_{ij11}^{V,LL} + \frac{40}{27}L_{ij22}^{V,LL} + \frac{40}{27}L_{ij33}^{V,LL} - \frac{56}{27}L_{ij11}^{V,LR} - \frac{56}{27}L_{ij22}^{V,LR} \right. \\
&\quad - \frac{56}{27}L_{ij33}^{V,LR} + \frac{8}{3}L_{ij11}^{V,LL} + \frac{8}{3}L_{ij22}^{V,LL} + \frac{8}{3}L_{ij33}^{V,LL} - 8L_{ij11}^{V,LR} - 8L_{ij22}^{V,LR} \\
&\quad \left. - 8L_{ij33}^{V,LR} + \frac{256}{27}L_{ij11}^{V,LL} + \frac{256}{27}L_{ij22}^{V,LL} - \frac{128}{27}L_{ij11}^{V,LR} - \frac{128}{27}L_{ij22}^{V,LR} \right];
\end{aligned}$$

$$\begin{aligned}
\dot{L}_{ij22}^{V,LL} &= e^2 \left[ -\frac{8}{9}L_{ij11}^{V,LL} - \frac{8}{9}L_{ij22}^{V,LL} - \frac{8}{9}L_{ij33}^{V,LL} - \frac{8}{9}L_{ij11}^{V,LR} - \frac{8}{9}L_{ij22}^{V,LR} \right. \\
&\quad - \frac{8}{9}L_{ij33}^{V,LR} - \frac{8}{9}L_{ij11}^{V,LL} - \frac{8}{9}L_{ij22}^{V,LL} - \frac{8}{9}L_{ij33}^{V,LL} - \frac{8}{9}L_{ij11}^{V,LR} - \frac{8}{9}L_{ij22}^{V,LR} \\
&\quad \left. - \frac{8}{9}L_{ij33}^{V,LR} + \frac{16}{9}L_{ij11}^{V,LL} + \frac{16}{9}L_{ij22}^{V,LL} + \frac{16}{9}L_{ij33}^{V,LL} + \frac{16}{9}L_{ij11}^{V,LR} + \frac{16}{9}L_{ij22}^{V,LR} \right] \\
&\quad + \alpha_s^2 \left[ 8L_{ij11}^{V,LL} + 8L_{ij22}^{V,LL} + 8L_{ij33}^{V,LL} - 8L_{ij11}^{V,LR} - 8L_{ij22}^{V,LR} \right. \\
&\quad \left. - 8L_{ij33}^{V,LR} + 8L_{ij11}^{V,LL} + 8L_{ij22}^{V,LL} - 8L_{ij11}^{V,LR} - 8L_{ij22}^{V,LR} \right]
\end{aligned}$$

$$\begin{aligned}
& + \alpha_s \alpha \left[ -\frac{32}{9} L_{ij11}^{V,LL} - \frac{32}{9} L_{ij22}^{V,LL} - \frac{32}{9} L_{ij33}^{V,LL} - \frac{32}{9} L_{ij11}^{V,LR} - \frac{32}{9} L_{ij22}^{V,LR} \right. \\
& \quad \left. - \frac{32}{9} L_{ij33}^{V,LR} + \frac{64}{9} L_{ij11}^{V,LL} + \frac{64}{9} L_{ij22}^{V,LL} + \frac{64}{9} L_{ij33}^{V,LL} + \frac{64}{9} L_{ij11}^{V,LR} + \frac{64}{9} L_{ij22}^{V,LR} \right] \\
& + \alpha^2 \left[ \frac{40}{27} L_{ij11}^{V,LL} + \frac{40}{27} L_{ij22}^{V,LL} + \frac{40}{27} L_{ij33}^{V,LL} - \frac{56}{27} L_{ij11}^{V,LR} - \frac{56}{27} L_{ij22}^{V,LR} \right. \\
& \quad - \frac{56}{27} L_{ij33}^{V,LR} + \frac{8}{3} L_{ij11}^{V,LL} + \frac{8}{3} L_{ij22}^{V,LL} + \frac{8}{3} L_{ij33}^{V,LL} - 8 L_{ij11}^{V,LR} - 8 L_{ij22}^{V,LR} \\
& \quad \left. - 8 L_{ij33}^{V,LR} + \frac{256}{27} L_{ij11}^{V,LL} + \frac{256}{27} L_{ij22}^{V,LL} - \frac{128}{27} L_{ij11}^{V,LR} - \frac{128}{27} L_{ij22}^{V,LR} \right]; \\
\dot{L}_{ij11}^{V,LR} & = e^2 \left[ \frac{4}{3} L_{ij11}^{V,LL} + \frac{4}{3} L_{ij22}^{V,LL} + \frac{4}{3} L_{ij33}^{V,LL} + \frac{4}{3} L_{ij11}^{V,LR} + \frac{4}{3} L_{ij22}^{V,LR} \right. \\
& \quad + \frac{4}{3} L_{ij33}^{V,LR} + \frac{4}{3} L_{ij11}^{V,LL} + \frac{4}{3} L_{ij22}^{V,LL} + \frac{4}{3} L_{ij33}^{V,LL} + \frac{4}{3} L_{ij11}^{V,LR} + \frac{4}{3} L_{ij22}^{V,LR} \\
& \quad \left. + \frac{4}{3} L_{ij33}^{V,LR} - \frac{8}{3} L_{ij11}^{V,LL} - \frac{8}{3} L_{ij22}^{V,LL} - \frac{8}{3} L_{ij33}^{V,LL} - \frac{8}{3} L_{ij11}^{V,LR} - \frac{8}{3} L_{ij22}^{V,LR} \right] \\
& + \alpha_s \alpha \left[ \frac{16}{3} L_{ij11}^{V,LL} + \frac{16}{3} L_{ij22}^{V,LL} + \frac{16}{3} L_{ij33}^{V,LL} + \frac{16}{3} L_{ij11}^{V,LR} + \frac{16}{3} L_{ij22}^{V,LR} \right. \\
& \quad \left. + \frac{16}{3} L_{ij33}^{V,LR} - \frac{32}{3} L_{ij11}^{V,LL} - \frac{32}{3} L_{ij22}^{V,LL} - \frac{32}{3} L_{ij33}^{V,LL} - \frac{32}{3} L_{ij11}^{V,LR} - \frac{32}{3} L_{ij22}^{V,LR} \right] \\
& + \alpha^2 \left[ -\frac{32}{9} L_{ij11}^{V,LL} - \frac{32}{9} L_{ij22}^{V,LL} - \frac{32}{9} L_{ij33}^{V,LL} + \frac{40}{9} L_{ij11}^{V,LR} + \frac{40}{9} L_{ij22}^{V,LR} \right. \\
& \quad + \frac{40}{9} L_{ij33}^{V,LR} - 8 L_{ij11}^{V,LL} - 8 L_{ij22}^{V,LL} - 8 L_{ij33}^{V,LL} + 16 L_{ij11}^{V,LR} + 16 L_{ij22}^{V,LR} \\
& \quad \left. + 16 L_{ij33}^{V,LR} - \frac{176}{9} L_{ij11}^{V,LL} - \frac{176}{9} L_{ij22}^{V,LL} + \frac{112}{9} L_{ij11}^{V,LR} + \frac{112}{9} L_{ij22}^{V,LR} \right]; \\
\dot{L}_{ij22}^{V,LR} & = e^2 \left[ \frac{4}{3} L_{ij11}^{V,LL} + \frac{4}{3} L_{ij22}^{V,LL} + \frac{4}{3} L_{ij33}^{V,LL} + \frac{4}{3} L_{ij11}^{V,LR} + \frac{4}{3} L_{ij22}^{V,LR} \right. \\
& \quad + \frac{4}{3} L_{ij33}^{V,LR} + \frac{4}{3} L_{ij11}^{V,LL} + \frac{4}{3} L_{ij22}^{V,LL} + \frac{4}{3} L_{ij33}^{V,LL} + \frac{4}{3} L_{ij11}^{V,LR} + \frac{4}{3} L_{ij22}^{V,LR} \\
& \quad \left. + \frac{4}{3} L_{ij33}^{V,LR} - \frac{8}{3} L_{ij11}^{V,LL} - \frac{8}{3} L_{ij22}^{V,LL} - \frac{8}{3} L_{ij33}^{V,LL} - \frac{8}{3} L_{ij11}^{V,LR} - \frac{8}{3} L_{ij22}^{V,LR} \right]
\end{aligned}$$

$$\begin{aligned}
& + \frac{4}{3} L_{ij33}^{V,LR} - \frac{8}{3} L_{ij11}^{V,LL} - \frac{8}{3} L_{ij22}^{V,LL} - \frac{8}{3} L_{ij11}^{V,LR} - \frac{8}{3} L_{ij22}^{V,LR} \Big] \\
& + \alpha_s \alpha \left[ \frac{16}{3} L_{ij11}^{V,LL} + \frac{16}{3} L_{ij22}^{V,LL} + \frac{16}{3} L_{ij33}^{V,LL} + \frac{16}{3} L_{ij11}^{V,LR} + \frac{16}{3} L_{ij22}^{V,LR} \right. \\
& + \frac{16}{3} L_{ij33}^{V,LR} - \frac{32}{3} L_{ij11}^{V,LL} - \frac{32}{3} L_{ij22}^{V,LL} - \frac{32}{3} L_{ij11}^{V,LR} - \frac{32}{3} L_{ij22}^{V,LR} \Big] \\
& + \alpha^2 \left[ -\frac{32}{9} L_{ij11}^{V,LL} - \frac{32}{9} L_{ij22}^{V,LL} - \frac{32}{9} L_{ij33}^{V,LL} + \frac{40}{9} L_{ij11}^{V,LR} + \frac{40}{9} L_{ij22}^{V,LR} \right. \\
& + \frac{40}{9} L_{ij33}^{V,LR} - 8 L_{ij11}^{V,LL} - 8 L_{ij22}^{V,LL} - 8 L_{ij33}^{V,LL} + 16 L_{ij11}^{V,LR} + 16 L_{ij22}^{V,LR} \\
& + 16 L_{ij33}^{V,LR} - \frac{176}{9} L_{ij11}^{V,LL} - \frac{176}{9} L_{ij22}^{V,LL} + \frac{112}{9} L_{ij11}^{V,LR} + \frac{112}{9} L_{ij22}^{V,LR} \Big] ; \\
\dot{L}_{ij33}^{V,LR} & = e^2 \left[ \frac{4}{3} L_{ij11}^{V,LL} + \frac{4}{3} L_{ij22}^{V,LL} + \frac{4}{3} L_{ij33}^{V,LL} + \frac{4}{3} L_{ij11}^{V,LR} + \frac{4}{3} L_{ij22}^{V,LR} \right. \\
& + \frac{4}{3} L_{ij33}^{V,LR} + \frac{4}{3} L_{ij11}^{V,LL} + \frac{4}{3} L_{ij22}^{V,LL} + \frac{4}{3} L_{ij33}^{V,LL} + \frac{4}{3} L_{ij11}^{V,LR} + \frac{4}{3} L_{ij22}^{V,LR} \\
& + \frac{4}{3} L_{ij33}^{V,LR} - \frac{8}{3} L_{ij11}^{V,LL} - \frac{8}{3} L_{ij22}^{V,LL} - \frac{8}{3} L_{ij11}^{V,LR} - \frac{8}{3} L_{ij22}^{V,LR} \Big] \\
& + \alpha_s \alpha \left[ \frac{16}{3} L_{ij11}^{V,LL} + \frac{16}{3} L_{ij22}^{V,LL} + \frac{16}{3} L_{ij33}^{V,LL} + \frac{16}{3} L_{ij11}^{V,LR} + \frac{16}{3} L_{ij22}^{V,LR} \right. \\
& + \frac{16}{3} L_{ij33}^{V,LR} - \frac{32}{3} L_{ij11}^{V,LL} - \frac{32}{3} L_{ij22}^{V,LL} - \frac{32}{3} L_{ij11}^{V,LR} - \frac{32}{3} L_{ij22}^{V,LR} \Big] \\
& + \alpha^2 \left[ -\frac{32}{9} L_{ij11}^{V,LL} - \frac{32}{9} L_{ij22}^{V,LL} - \frac{32}{9} L_{ij33}^{V,LL} + \frac{40}{9} L_{ij11}^{V,LR} + \frac{40}{9} L_{ij22}^{V,LR} \right. \\
& + \frac{40}{9} L_{ij33}^{V,LR} - 8 L_{ij11}^{V,LL} - 8 L_{ij22}^{V,LL} - 8 L_{ij33}^{V,LL} + 16 L_{ij11}^{V,LR} + 16 L_{ij22}^{V,LR} \\
& + 16 L_{ij33}^{V,LR} - \frac{176}{9} L_{ij11}^{V,LL} - \frac{176}{9} L_{ij22}^{V,LL} + \frac{112}{9} L_{ij11}^{V,LR} + \frac{112}{9} L_{ij22}^{V,LR} \Big] ; \\
\dot{L}_{ij11}^{V,LR} & = e^2 \left[ \frac{4}{9} L_{ij11}^{V,LL} + \frac{4}{9} L_{ij22}^{V,LL} + \frac{4}{9} L_{ij33}^{V,LL} + \frac{4}{9} L_{ij11}^{V,LR} + \frac{4}{9} L_{ij22}^{V,LR} \right.
\end{aligned}$$

$$\begin{aligned}
& + \frac{4}{9}L_{\nu d, ij33}^{V,LR} + \frac{4}{9}L_{\nu e, ij11}^{V,LL} + \frac{4}{9}L_{\nu e, ij22}^{V,LL} + \frac{4}{9}L_{\nu e, ij33}^{V,LL} + \frac{4}{9}L_{\nu e, ij11}^{V,LR} + \frac{4}{9}L_{\nu e, ij22}^{V,LR} \\
& + \frac{4}{9}L_{\nu e, ij33}^{V,LR} - \frac{8}{9}L_{\nu u, ij11}^{V,LL} - \frac{8}{9}L_{\nu u, ij22}^{V,LL} - \frac{8}{9}L_{\nu u, ij11}^{V,LR} - \frac{8}{9}L_{\nu u, ij22}^{V,LR} \Big] \\
& + \alpha_s^2 \Big[ -8L_{\nu d, ij11}^{V,LL} - 8L_{\nu d, ij22}^{V,LL} - 8L_{\nu d, ij33}^{V,LL} + 8L_{\nu d, ij11}^{V,LR} + 8L_{\nu d, ij22}^{V,LR} \\
& + 8L_{\nu d, ij33}^{V,LR} - 8L_{\nu u, ij11}^{V,LL} - 8L_{\nu u, ij22}^{V,LL} + 8L_{\nu u, ij11}^{V,LR} + 8L_{\nu u, ij22}^{V,LR} \Big] \\
& + \alpha_s \alpha \Big[ \frac{16}{9}L_{\nu d, ij11}^{V,LL} + \frac{16}{9}L_{\nu d, ij22}^{V,LL} + \frac{16}{9}L_{\nu d, ij33}^{V,LL} + \frac{16}{9}L_{\nu d, ij11}^{V,LR} + \frac{16}{9}L_{\nu d, ij22}^{V,LR} \\
& + \frac{16}{9}L_{\nu d, ij33}^{V,LR} - \frac{32}{9}L_{\nu u, ij11}^{V,LL} - \frac{32}{9}L_{\nu u, ij22}^{V,LL} - \frac{32}{9}L_{\nu u, ij11}^{V,LR} - \frac{32}{9}L_{\nu u, ij22}^{V,LR} \Big] \\
& + \alpha^2 \Big[ -\frac{8}{27}L_{\nu d, ij11}^{V,LL} - \frac{8}{27}L_{\nu d, ij22}^{V,LL} - \frac{8}{27}L_{\nu d, ij33}^{V,LL} + \frac{16}{27}L_{\nu d, ij11}^{V,LR} + \frac{16}{27}L_{\nu d, ij22}^{V,LR} \\
& + \frac{16}{27}L_{\nu d, ij33}^{V,LR} + \frac{8}{3}L_{\nu e, ij11}^{V,LR} + \frac{8}{3}L_{\nu e, ij22}^{V,LR} + \frac{8}{3}L_{\nu e, ij33}^{V,LR} - \frac{80}{27}L_{\nu u, ij11}^{V,LL} - \frac{80}{27}L_{\nu u, ij22}^{V,LL} \\
& + \frac{16}{27}L_{\nu u, ij11}^{V,LR} + \frac{16}{27}L_{\nu u, ij22}^{V,LR} \Big] ; \\
\dot{L}_{\nu d, ij22}^{V,LR} & = e^2 \Big[ \frac{4}{9}L_{\nu d, ij11}^{V,LL} + \frac{4}{9}L_{\nu d, ij22}^{V,LL} + \frac{4}{9}L_{\nu d, ij33}^{V,LL} + \frac{4}{9}L_{\nu d, ij11}^{V,LR} + \frac{4}{9}L_{\nu d, ij22}^{V,LR} \\
& + \frac{4}{9}L_{\nu e, ij33}^{V,LR} + \frac{4}{9}L_{\nu e, ij11}^{V,LL} + \frac{4}{9}L_{\nu e, ij22}^{V,LL} + \frac{4}{9}L_{\nu e, ij33}^{V,LL} + \frac{4}{9}L_{\nu e, ij11}^{V,LR} + \frac{4}{9}L_{\nu e, ij22}^{V,LR} \\
& + \frac{4}{9}L_{\nu e, ij33}^{V,LR} - \frac{8}{9}L_{\nu u, ij11}^{V,LL} - \frac{8}{9}L_{\nu u, ij22}^{V,LL} - \frac{8}{9}L_{\nu u, ij11}^{V,LR} - \frac{8}{9}L_{\nu u, ij22}^{V,LR} \Big] \\
& + \alpha_s^2 \Big[ -8L_{\nu d, ij11}^{V,LL} - 8L_{\nu d, ij22}^{V,LL} - 8L_{\nu d, ij33}^{V,LL} + 8L_{\nu d, ij11}^{V,LR} + 8L_{\nu d, ij22}^{V,LR} \\
& + 8L_{\nu d, ij33}^{V,LR} - 8L_{\nu u, ij11}^{V,LL} - 8L_{\nu u, ij22}^{V,LL} + 8L_{\nu u, ij11}^{V,LR} + 8L_{\nu u, ij22}^{V,LR} \Big] \\
& + \alpha_s \alpha \Big[ \frac{16}{9}L_{\nu d, ij11}^{V,LL} + \frac{16}{9}L_{\nu d, ij22}^{V,LL} + \frac{16}{9}L_{\nu d, ij33}^{V,LL} + \frac{16}{9}L_{\nu d, ij11}^{V,LR} + \frac{16}{9}L_{\nu d, ij22}^{V,LR}
\end{aligned}$$



$$\begin{aligned}
& + \frac{16}{9} L_{\nu d, ij33}^{V,LR} - \frac{32}{9} L_{\nu u, ij11}^{V,LL} - \frac{32}{9} L_{\nu u, ij22}^{V,LL} - \frac{32}{9} L_{\nu u, ij11}^{V,LR} - \frac{32}{9} L_{\nu u, ij22}^{V,LR} \Big] \\
& + \alpha^2 \Bigg[ -\frac{8}{27} L_{\nu d, ij11}^{V,LL} - \frac{8}{27} L_{\nu d, ij22}^{V,LL} - \frac{8}{27} L_{\nu d, ij33}^{V,LL} + \frac{16}{27} L_{\nu d, ij11}^{V,LR} + \frac{16}{27} L_{\nu d, ij22}^{V,LR} \\
& + \frac{16}{27} L_{\nu d, ij33}^{V,LR} + \frac{8}{3} L_{\nu e, ij11}^{V,LR} + \frac{8}{3} L_{\nu e, ij22}^{V,LR} + \frac{8}{3} L_{\nu e, ij33}^{V,LR} - \frac{80}{27} L_{\nu u, ij11}^{V,LL} - \frac{80}{27} L_{\nu u, ij22}^{V,LL} \\
& + \frac{16}{27} L_{\nu u, ij11}^{V,LR} + \frac{16}{27} L_{\nu u, ij22}^{V,LR} \Bigg] ; \\
\dot{L}_{\nu d, ij33}^{V,LR} & = e^2 \Bigg[ \frac{4}{9} L_{\nu d, ij11}^{V,LL} + \frac{4}{9} L_{\nu d, ij22}^{V,LL} + \frac{4}{9} L_{\nu d, ij33}^{V,LL} + \frac{4}{9} L_{\nu d, ij11}^{V,LR} + \frac{4}{9} L_{\nu d, ij22}^{V,LR} \\
& + \frac{4}{9} L_{\nu d, ij33}^{V,LR} + \frac{4}{9} L_{\nu e, ij11}^{V,LL} + \frac{4}{9} L_{\nu e, ij22}^{V,LL} + \frac{4}{9} L_{\nu e, ij33}^{V,LL} + \frac{4}{9} L_{\nu e, ij11}^{V,LR} + \frac{4}{9} L_{\nu e, ij22}^{V,LR} + \frac{4}{9} L_{\nu e, ij33}^{V,LR} \\
& + \frac{4}{9} L_{\nu e, ij33}^{V,LR} - \frac{8}{9} L_{\nu u, ij11}^{V,LL} - \frac{8}{9} L_{\nu u, ij22}^{V,LL} - \frac{8}{9} L_{\nu u, ij11}^{V,LR} - \frac{8}{9} L_{\nu u, ij22}^{V,LR} \Bigg] \\
& + \alpha_s^2 \Bigg[ -8 L_{\nu d, ij11}^{V,LL} - 8 L_{\nu d, ij22}^{V,LL} - 8 L_{\nu d, ij33}^{V,LL} + 8 L_{\nu d, ij11}^{V,LR} + 8 L_{\nu d, ij22}^{V,LR} \\
& + 8 L_{\nu d, ij33}^{V,LR} - 8 L_{\nu u, ij11}^{V,LL} - 8 L_{\nu u, ij22}^{V,LL} + 8 L_{\nu u, ij11}^{V,LR} + 8 L_{\nu u, ij22}^{V,LR} \Bigg] \\
& + \alpha_s \alpha \Bigg[ \frac{16}{9} L_{\nu d, ij11}^{V,LL} + \frac{16}{9} L_{\nu d, ij22}^{V,LL} + \frac{16}{9} L_{\nu d, ij33}^{V,LL} + \frac{16}{9} L_{\nu d, ij11}^{V,LR} + \frac{16}{9} L_{\nu d, ij22}^{V,LR} \\
& + \frac{16}{9} L_{\nu d, ij33}^{V,LR} - \frac{32}{9} L_{\nu u, ij11}^{V,LL} - \frac{32}{9} L_{\nu u, ij22}^{V,LL} - \frac{32}{9} L_{\nu u, ij11}^{V,LR} - \frac{32}{9} L_{\nu u, ij22}^{V,LR} \Bigg] \\
& + \alpha^2 \Bigg[ -\frac{8}{27} L_{\nu d, ij11}^{V,LL} - \frac{8}{27} L_{\nu d, ij22}^{V,LL} - \frac{8}{27} L_{\nu d, ij33}^{V,LL} + \frac{16}{27} L_{\nu d, ij11}^{V,LR} + \frac{16}{27} L_{\nu d, ij22}^{V,LR} \\
& + \frac{16}{27} L_{\nu d, ij33}^{V,LR} + \frac{8}{3} L_{\nu e, ij11}^{V,LR} + \frac{8}{3} L_{\nu e, ij22}^{V,LR} + \frac{8}{3} L_{\nu e, ij33}^{V,LR} - \frac{80}{27} L_{\nu u, ij11}^{V,LL} - \frac{80}{27} L_{\nu u, ij22}^{V,LL} \\
& + \frac{16}{27} L_{\nu u, ij11}^{V,LR} + \frac{16}{27} L_{\nu u, ij22}^{V,LR} \Bigg] ; \\
\dot{L}_{\nu u, ij11}^{V,LR} & = e^2 \Bigg[ -\frac{8}{9} L_{\nu d, ij11}^{V,LL} - \frac{8}{9} L_{\nu d, ij22}^{V,LL} - \frac{8}{9} L_{\nu d, ij33}^{V,LL} - \frac{8}{9} L_{\nu d, ij11}^{V,LR} - \frac{8}{9} L_{\nu d, ij22}^{V,LR}
\end{aligned}$$

$$\begin{aligned}
& -\frac{8}{9}L_{ij33}^{V,LR} - \frac{8}{9}L_{ij11}^{V,LL} - \frac{8}{9}L_{ij22}^{V,LL} - \frac{8}{9}L_{ij33}^{V,LL} - \frac{8}{9}L_{ij11}^{V,LR} - \frac{8}{9}L_{ij22}^{V,LR} \\
& - \frac{8}{9}L_{ij33}^{V,LR} + \frac{16}{9}L_{ij11}^{V,LL} + \frac{16}{9}L_{ij22}^{V,LL} + \frac{16}{9}L_{ij11}^{V,LR} + \frac{16}{9}L_{ij22}^{V,LR} \Big] \\
& + \alpha_s^2 \Big[ -8L_{ij11}^{V,LL} - 8L_{ij22}^{V,LL} - 8L_{ij33}^{V,LL} + 8L_{ij11}^{V,LR} + 8L_{ij22}^{V,LR} \\
& + 8L_{ij33}^{V,LR} - 8L_{ij11}^{V,LL} - 8L_{ij22}^{V,LL} + 8L_{ij11}^{V,LR} + 8L_{ij22}^{V,LR} \Big] \\
& + \alpha_s \alpha \Big[ -\frac{32}{9}L_{ij11}^{V,LL} - \frac{32}{9}L_{ij22}^{V,LL} - \frac{32}{9}L_{ij33}^{V,LL} - \frac{32}{9}L_{ij11}^{V,LR} - \frac{32}{9}L_{ij22}^{V,LR} \\
& - \frac{32}{9}L_{ij33}^{V,LR} + \frac{64}{9}L_{ij11}^{V,LL} + \frac{64}{9}L_{ij22}^{V,LL} + \frac{64}{9}L_{ij11}^{V,LR} + \frac{64}{9}L_{ij22}^{V,LR} \Big] \\
& + \alpha^2 \Big[ -\frac{56}{27}L_{ij11}^{V,LL} - \frac{56}{27}L_{ij22}^{V,LL} - \frac{56}{27}L_{ij33}^{V,LL} + \frac{40}{27}L_{ij11}^{V,LR} + \frac{40}{27}L_{ij22}^{V,LR} \\
& + \frac{40}{27}L_{ij33}^{V,LR} - 8L_{ij11}^{V,LL} - 8L_{ij22}^{V,LL} - 8L_{ij33}^{V,LL} + \frac{8}{3}L_{ij11}^{V,LR} + \frac{8}{3}L_{ij22}^{V,LR} \\
& + \frac{8}{3}L_{ij33}^{V,LR} - \frac{128}{27}L_{ij11}^{V,LL} - \frac{128}{27}L_{ij22}^{V,LL} + \frac{256}{27}L_{ij11}^{V,LR} + \frac{256}{27}L_{ij22}^{V,LR} \Big] ; \\
\dot{L}_{ij22}^{V,LR} & = e^2 \Big[ -\frac{8}{9}L_{ij11}^{V,LL} - \frac{8}{9}L_{ij22}^{V,LL} - \frac{8}{9}L_{ij33}^{V,LL} - \frac{8}{9}L_{ij11}^{V,LR} - \frac{8}{9}L_{ij22}^{V,LR} \\
& - \frac{8}{9}L_{ij33}^{V,LR} - \frac{8}{9}L_{ij11}^{V,LL} - \frac{8}{9}L_{ij22}^{V,LL} - \frac{8}{9}L_{ij33}^{V,LL} - \frac{8}{9}L_{ij11}^{V,LR} - \frac{8}{9}L_{ij22}^{V,LR} \\
& - \frac{8}{9}L_{ij33}^{V,LR} + \frac{16}{9}L_{ij11}^{V,LL} + \frac{16}{9}L_{ij22}^{V,LL} + \frac{16}{9}L_{ij11}^{V,LR} + \frac{16}{9}L_{ij22}^{V,LR} \Big] \\
& + \alpha_s^2 \Big[ -8L_{ij11}^{V,LL} - 8L_{ij22}^{V,LL} - 8L_{ij33}^{V,LL} + 8L_{ij11}^{V,LR} + 8L_{ij22}^{V,LR} \\
& + 8L_{ij33}^{V,LR} - 8L_{ij11}^{V,LL} - 8L_{ij22}^{V,LL} + 8L_{ij11}^{V,LR} + 8L_{ij22}^{V,LR} \Big] \\
& + \alpha_s \alpha \Big[ -\frac{32}{9}L_{ij11}^{V,LL} - \frac{32}{9}L_{ij22}^{V,LL} - \frac{32}{9}L_{ij33}^{V,LL} - \frac{32}{9}L_{ij11}^{V,LR} - \frac{32}{9}L_{ij22}^{V,LR}
\end{aligned}$$

$$\begin{aligned}
& -\frac{32}{9}L_{ij33}^{V,LR} + \frac{64}{9}L_{ij11}^{V,LL} + \frac{64}{9}L_{ij22}^{V,LL} + \frac{64}{9}L_{ij11}^{V,LR} + \frac{64}{9}L_{ij22}^{V,LR} \Big] \\
& + \alpha^2 \Big[ -\frac{56}{27}L_{ij11}^{V,LL} - \frac{56}{27}L_{ij22}^{V,LL} - \frac{56}{27}L_{ij33}^{V,LL} + \frac{40}{27}L_{ij11}^{V,LR} + \frac{40}{27}L_{ij22}^{V,LR} \\
& + \frac{40}{27}L_{ij33}^{V,LR} - 8L_{ij11}^{V,LL} - 8L_{ij22}^{V,LL} - 8L_{ij33}^{V,LL} + \frac{8}{3}L_{ij11}^{V,LR} + \frac{8}{3}L_{ij22}^{V,LR} \\
& + \frac{8}{3}L_{ij33}^{V,LR} - \frac{128}{27}L_{ij11}^{V,LL} - \frac{128}{27}L_{ij22}^{V,LL} + \frac{256}{27}L_{ij11}^{V,LR} + \frac{256}{27}L_{ij22}^{V,LR} \Big] ;
\end{aligned}$$

$$\dot{L}_{ij11}^{S,LR} = \frac{373}{9}\alpha^2 L_{ij11}^{S,LR} - 6e^2 L_{ij11}^{S,LR} ;$$

$$\dot{L}_{ij22}^{S,LR} = \frac{373}{9}\alpha^2 L_{ij22}^{S,LR} - 6e^2 L_{ij22}^{S,LR} ;$$

$$\dot{L}_{ij33}^{S,LR} = \frac{373}{9}\alpha^2 L_{ij33}^{S,LR} - 6e^2 L_{ij33}^{S,LR} ;$$

$$\begin{aligned}
\dot{L}_{ij11}^{S,LR} &= -8g_s^2 L_{ij11}^{S,LR} - \frac{2}{3}e^2 L_{ij11}^{S,LR} - \frac{1012}{9}\alpha_s^2 L_{ij11}^{S,LR} - \frac{8}{9}\alpha_s \alpha L_{ij11}^{S,LR} \\
&+ \frac{397}{81}\alpha^2 L_{ij11}^{S,LR} ;
\end{aligned}$$

$$\begin{aligned}
\dot{L}_{ij22}^{S,LR} &= -8g_s^2 L_{ij22}^{S,LR} - \frac{2}{3}e^2 L_{ij22}^{S,LR} - \frac{1012}{9}\alpha_s^2 L_{ij22}^{S,LR} - \frac{8}{9}\alpha_s \alpha L_{ij22}^{S,LR} \\
&+ \frac{397}{81}\alpha^2 L_{ij22}^{S,LR} ;
\end{aligned}$$

$$\begin{aligned}
\dot{L}_{ij33}^{S,LR} &= -8g_s^2 L_{ij33}^{S,LR} - \frac{2}{3}e^2 L_{ij33}^{S,LR} - \frac{1012}{9}\alpha_s^2 L_{ij33}^{S,LR} - \frac{8}{9}\alpha_s \alpha L_{ij33}^{S,LR} \\
&+ \frac{397}{81}\alpha^2 L_{ij33}^{S,LR} ;
\end{aligned}$$

$$\begin{aligned}
\dot{L}_{ij11}^{S,LR} &= -8g_s^2 L_{ij11}^{S,LR} - \frac{8}{3}e^2 L_{ij11}^{S,LR} - \frac{1012}{9}\alpha_s^2 L_{ij11}^{S,LR} - \frac{32}{9}\alpha_s \alpha L_{ij11}^{S,LR} \\
&+ \frac{1552}{81}\alpha^2 L_{ij11}^{S,LR} ;
\end{aligned}$$

$$\begin{aligned}
\dot{L}_{ij22}^{S,LR} &= -8g_s^2 L_{ij22}^{S,LR} - \frac{8}{3}e^2 L_{ij22}^{S,LR} - \frac{1012}{9}\alpha_s^2 L_{ij22}^{S,LR} - \frac{32}{9}\alpha_s \alpha L_{ij22}^{S,LR} \\
&+ \frac{1552}{81}\alpha^2 L_{ij22}^{S,LR} ;
\end{aligned}$$

$$\dot{L}_{ij11}^{S,LL} = \frac{373}{9}\alpha^2 L_{ij11}^{S,LL} - 6e^2 L_{ij11}^{S,LL} ;$$

$$\begin{aligned}
\dot{L}_{ij11}^{T,LL} &= 2e^2 L_{ij11}^{T,LL} - \frac{1553}{27} \alpha^2 L_{ij11}^{T,LL} ; \\
\dot{L}_{ij22}^{S,LL} &= \frac{373}{9} \alpha^2 L_{ij22}^{S,LL} - 6e^2 L_{ij22}^{S,LL} ; \\
\dot{L}_{ij22}^{T,LL} &= 2e^2 L_{ij22}^{T,LL} - \frac{1553}{27} \alpha^2 L_{ij22}^{T,LL} ; \\
\dot{L}_{ij33}^{S,LL} &= \frac{373}{9} \alpha^2 L_{ij33}^{S,LL} - 6e^2 L_{ij33}^{S,LL} ; \\
\dot{L}_{ij33}^{T,LL} &= 2e^2 L_{ij33}^{T,LL} - \frac{1553}{27} \alpha^2 L_{ij33}^{T,LL} ; \\
\dot{L}_{ij11}^{S,LL} &= -8g_s^2 L_{ij11}^{S,LL} - \frac{2}{3} e^2 L_{ij11}^{S,LL} - \frac{1012}{9} \alpha_s^2 L_{ij11}^{S,LL} - \frac{8}{9} \alpha_s \alpha L_{ij11}^{S,LL} \\
&\quad + \frac{397}{81} \alpha^2 L_{ij11}^{S,LL} ; \\
\dot{L}_{ij11}^{T,LL} &= \frac{8}{3} g_s^2 L_{ij11}^{T,LL} + \frac{2}{9} e^2 L_{ij11}^{T,LL} + \frac{1652}{27} \alpha_s^2 L_{ij11}^{T,LL} - \frac{152}{27} \alpha_s \alpha L_{ij11}^{T,LL} \\
&\quad - \frac{1097}{243} \alpha^2 L_{ij11}^{T,LL} ; \\
\dot{L}_{ij22}^{S,LL} &= -8g_s^2 L_{ij22}^{S,LL} - \frac{2}{3} e^2 L_{ij22}^{S,LL} - \frac{1012}{9} \alpha_s^2 L_{ij22}^{S,LL} - \frac{8}{9} \alpha_s \alpha L_{ij22}^{S,LL} \\
&\quad + \frac{397}{81} \alpha^2 L_{ij22}^{S,LL} ; \\
\dot{L}_{ij22}^{T,LL} &= \frac{8}{3} g_s^2 L_{ij22}^{T,LL} + \frac{2}{9} e^2 L_{ij22}^{T,LL} + \frac{1652}{27} \alpha_s^2 L_{ij22}^{T,LL} - \frac{152}{27} \alpha_s \alpha L_{ij22}^{T,LL} \\
&\quad - \frac{1097}{243} \alpha^2 L_{ij22}^{T,LL} ; \\
\dot{L}_{ij33}^{S,LL} &= -8g_s^2 L_{ij33}^{S,LL} - \frac{2}{3} e^2 L_{ij33}^{S,LL} - \frac{1012}{9} \alpha_s^2 L_{ij33}^{S,LL} - \frac{8}{9} \alpha_s \alpha L_{ij33}^{S,LL} \\
&\quad + \frac{397}{81} \alpha^2 L_{ij33}^{S,LL} ; \\
\dot{L}_{ij33}^{T,LL} &= \frac{8}{3} g_s^2 L_{ij33}^{T,LL} + \frac{2}{9} e^2 L_{ij33}^{T,LL} + \frac{1652}{27} \alpha_s^2 L_{ij33}^{T,LL} - \frac{152}{27} \alpha_s \alpha L_{ij33}^{T,LL} \\
&\quad - \frac{1097}{243} \alpha^2 L_{ij33}^{T,LL} ; \\
\dot{L}_{ij11}^{S,LL} &= -8g_s^2 L_{ij11}^{S,LL} - \frac{8}{3} e^2 L_{ij11}^{S,LL} - \frac{1012}{9} \alpha_s^2 L_{ij11}^{S,LL} - \frac{32}{9} \alpha_s \alpha L_{ij11}^{S,LL}
\end{aligned}$$

$$\begin{aligned}
& + \frac{1552}{81} \alpha^2 L_{ij11}^{S,LL} ; \\
\dot{L}_{ij11}^{T,LL} &= \frac{8}{3} g_s^2 L_{ij11}^{T,LL} + \frac{8}{9} e^2 L_{ij11}^{T,LL} + \frac{1652}{27} \alpha_s^2 L_{ij11}^{T,LL} - \frac{608}{27} \alpha_s \alpha L_{ij11}^{T,LL} \\
& - \frac{5072}{243} \alpha^2 L_{ij11}^{T,LL} ; \\
\dot{L}_{ij22}^{S,LL} &= -8g_s^2 L_{ij22}^{S,LL} - \frac{8}{3} e^2 L_{ij22}^{S,LL} - \frac{1012}{9} \alpha_s^2 L_{ij22}^{S,LL} - \frac{32}{9} \alpha_s \alpha L_{ij22}^{S,LL} \\
& + \frac{1552}{81} \alpha^2 L_{ij22}^{S,LL} ; \\
\dot{L}_{ij22}^{T,LL} &= \frac{8}{3} g_s^2 L_{ij22}^{T,LL} + \frac{8}{9} e^2 L_{ij22}^{T,LL} + \frac{1652}{27} \alpha_s^2 L_{ij22}^{T,LL} - \frac{608}{27} \alpha_s \alpha L_{ij22}^{T,LL} \\
& - \frac{5072}{243} \alpha^2 L_{ij22}^{T,LL} ; \\
\dot{L}_{ijkk}^{V,LL} &= 0 ; \\
\dot{L}_{ijjj}^{V,LL} &= 0 ; \\
\dot{L}_{ijii}^{V,LL} &= 0 ; \\
\dot{L}_{ijkk}^{S,LL} &= 0 ; \\
\dot{L}_{ikkj}^{S,LL} &= 0 ; \\
\dot{L}_{ijjj}^{S,LL} &= 0 ; \\
\dot{L}_{ijii}^{S,LL} &= 0 ;
\end{aligned}$$

### 1.9 $\Delta F = 0$ Transitions ( $\bar{f}_i f_i \bar{f}_j f_j$ )

$$\begin{aligned}
\dot{L}_{ijj}^{S,RL} &= -8g_s^2 L_{ijj}^{S,RL} - \frac{20}{3} e^2 L_{ijj}^{S,RL} - \frac{1012}{9} \alpha_s^2 L_{ijj}^{S,RL} - \frac{8}{9} \alpha_s \alpha L_{ijj}^{S,RL} \\
& + \frac{6958}{81} \alpha^2 L_{ijj}^{S,RL} ; \\
\dot{L}_{iij}^{S,RL} &= -8g_s^2 L_{iij}^{S,RL} - \frac{26}{3} e^2 L_{iij}^{S,RL} - \frac{1012}{9} \alpha_s^2 L_{iij}^{S,RL} - \frac{32}{9} \alpha_s \alpha L_{iij}^{S,RL} \\
& + \frac{445}{81} \alpha^2 L_{iij}^{S,RL} ;
\end{aligned}$$

$$\begin{aligned}
\dot{L}_{\nu e ij}^{S,LR} &= -6e^2 L_{\nu e ij}^{S,LR} ; \\
\dot{L}_{\nu d ij}^{S,LR} &= -8g_s^2 L_{\nu d ij}^{S,LR} - \frac{2}{3}e^2 L_{\nu d ij}^{S,LR} - \frac{1012}{9}\alpha_s^2 L_{\nu d ij}^{S,LR} - \frac{8}{9}\alpha_s \alpha L_{\nu d ij}^{S,LR} \\
&\quad + \frac{397}{81}\alpha^2 L_{\nu d ij}^{S,LR} ; \\
\dot{L}_{\nu u ij}^{S,LR} &= -8g_s^2 L_{\nu u ij}^{S,LR} - \frac{8}{3}e^2 L_{\nu u ij}^{S,LR} - \frac{1012}{9}\alpha_s^2 L_{\nu u ij}^{S,LR} - \frac{32}{9}\alpha_s \alpha L_{\nu u ij}^{S,LR} \\
&\quad + \frac{1552}{81}\alpha^2 L_{\nu u ij}^{S,LR} ; \\
\dot{L}_{uddu ij}^{V1,LR} &= -\frac{8}{3}g_s^2 L_{uddu ij}^{V8,LR} - \frac{10}{3}e^2 L_{uddu ij}^{V1,LR} + \alpha_s^2 \left[ -\frac{28}{3}L_{uddu ij}^{V1,LR} - \frac{2044}{27}L_{uddu ij}^{V8,LR} \right] \\
&\quad + \alpha_s \alpha \left[ \frac{8}{3}L_{uddu ij}^{V1,LR} - \frac{128}{27}L_{uddu ij}^{V8,LR} \right] + \frac{173}{81}\alpha^2 L_{uddu ij}^{V1,LR} ; \\
\dot{L}_{uddu ij}^{V8,LR} &= g_s^2 \left[ -12L_{uddu ij}^{V1,LR} - 14L_{uddu ij}^{V8,LR} \right] - \frac{10}{3}e^2 L_{uddu ij}^{V8,LR} + \alpha_s^2 \left[ -\frac{374}{3}L_{uddu ij}^{V1,LR} \right. \\
&\quad \left. - \frac{2975}{18}L_{uddu ij}^{V8,LR} \right] + \alpha_s \alpha \left[ \frac{16}{9}L_{uddu ij}^{V8,LR} - \frac{64}{3}L_{uddu ij}^{V1,LR} \right] + \frac{173}{81}\alpha^2 L_{uddu ij}^{V8,LR} ; \\
\dot{L}_{dd ij}^{V1,LR} &= -\frac{8}{3}g_s^2 L_{dd ij}^{V8,LR} - \frac{4}{3}e^2 L_{dd ij}^{V1,LR} + \alpha_s^2 \left[ -\frac{28}{3}L_{dd ij}^{V1,LR} - \frac{2044}{27}L_{dd ij}^{V8,LR} \right] \\
&\quad + \alpha_s \alpha \left[ \frac{32}{3}L_{dd ij}^{V1,LR} - \frac{8}{27}L_{dd ij}^{V8,LR} \right] + \frac{1790}{81}\alpha^2 L_{dd ij}^{V1,LR} ; \\
\dot{L}_{dd ij}^{V8,LR} &= g_s^2 \left[ -12L_{dd ij}^{V1,LR} - 14L_{dd ij}^{V8,LR} \right] - \frac{4}{3}e^2 L_{dd ij}^{V8,LR} + \alpha_s^2 \left[ -\frac{374}{3}L_{dd ij}^{V1,LR} \right. \\
&\quad \left. - \frac{2975}{18}L_{dd ij}^{V8,LR} \right] + \alpha_s \alpha \left[ -\frac{4}{3}L_{dd ij}^{V1,LR} - \frac{26}{9}L_{dd ij}^{V8,LR} \right] + \frac{1790}{81}\alpha^2 L_{dd ij}^{V8,LR} ; \\
\dot{L}_{uu ij}^{V1,LR} &= -\frac{8}{3}g_s^2 L_{uu ij}^{V8,LR} - \frac{16}{3}e^2 L_{uu ij}^{V1,LR} + \alpha_s^2 \left[ -\frac{28}{3}L_{uu ij}^{V1,LR} - \frac{2044}{27}L_{uu ij}^{V8,LR} \right] \\
&\quad + \alpha_s \alpha \left[ \frac{128}{3}L_{uu ij}^{V1,LR} - \frac{32}{27}L_{uu ij}^{V8,LR} \right] + \frac{7520}{81}\alpha^2 L_{uu ij}^{V1,LR} ;
\end{aligned}$$

$$\begin{aligned}
\dot{L}_{ijji}^{V8,LR} &= g_s^2 \left[ -12L_{ijji}^{V1,LR} - 14L_{ijji}^{V8,LR} \right] - \frac{16}{3}e^2 L_{ijji}^{V8,LR} + \alpha_s^2 \left[ -\frac{374}{3}L_{ijji}^{V1,LR} \right. \\
&\quad \left. - \frac{2975}{18}L_{ijji}^{V8,LR} \right] + \alpha_s \alpha \left[ -\frac{16}{3}L_{ijji}^{V1,LR} - \frac{104}{9}L_{ijji}^{V8,LR} \right] + \frac{7520}{81}\alpha^2 L_{ijji}^{V8,LR} ; \\
\dot{L}_{ijji}^{V,LR} &= \frac{2030}{9}\alpha^2 L_{ijji}^{V,LR} - 12e^2 L_{ijji}^{V,LR} ; \\
\dot{L}_{jjii}^{S,RL} &= -8g_s^2 L_{jjii}^{S,RL} - \frac{20}{3}e^2 L_{jjii}^{S,RL} - \frac{1012}{9}\alpha_s^2 L_{jjii}^{S,RL} - \frac{8}{9}\alpha_s \alpha L_{jjii}^{S,RL} \\
&\quad + \frac{6958}{81}\alpha^2 L_{jjii}^{S,RL} ; \\
\dot{L}_{jjii}^{S,RL} &= -8g_s^2 L_{jjii}^{S,RL} - \frac{26}{3}e^2 L_{jjii}^{S,RL} - \frac{1012}{9}\alpha_s^2 L_{jjii}^{S,RL} - \frac{32}{9}\alpha_s \alpha L_{jjii}^{S,RL} \\
&\quad + \frac{445}{81}\alpha^2 L_{jjii}^{S,RL} ; \\
\dot{L}_{jjii}^{S,LR} &= -6e^2 L_{jjii}^{S,LR} ; \\
\dot{L}_{jjii}^{S,LR} &= -8g_s^2 L_{jjii}^{S,LR} - \frac{2}{3}e^2 L_{jjii}^{S,LR} - \frac{1012}{9}\alpha_s^2 L_{jjii}^{S,LR} - \frac{8}{9}\alpha_s \alpha L_{jjii}^{S,LR} \\
&\quad + \frac{397}{81}\alpha^2 L_{jjii}^{S,LR} ; \\
\dot{L}_{jjii}^{S,LR} &= -8g_s^2 L_{jjii}^{S,LR} - \frac{8}{3}e^2 L_{jjii}^{S,LR} - \frac{1012}{9}\alpha_s^2 L_{jjii}^{S,LR} - \frac{32}{9}\alpha_s \alpha L_{jjii}^{S,LR} \\
&\quad + \frac{1552}{81}\alpha^2 L_{jjii}^{S,LR} ; \\
\dot{L}_{jijj}^{V1,LR} &= -\frac{8}{3}g_s^2 L_{jijj}^{V8,LR} - \frac{10}{3}e^2 L_{jijj}^{V1,LR} + \alpha_s^2 \left[ -\frac{28}{3}L_{jijj}^{V1,LR} - \frac{2044}{27}L_{jijj}^{V8,LR} \right] \\
&\quad + \alpha_s \alpha \left[ \frac{8}{3}L_{jijj}^{V1,LR} - \frac{128}{27}L_{jijj}^{V8,LR} \right] + \frac{173}{81}\alpha^2 L_{jijj}^{V1,LR} ; \\
\dot{L}_{jijj}^{V8,LR} &= g_s^2 \left[ -12L_{jijj}^{V1,LR} - 14L_{jijj}^{V8,LR} \right] - \frac{10}{3}e^2 L_{jijj}^{V8,LR} + \alpha_s^2 \left[ -\frac{374}{3}L_{jijj}^{V1,LR} \right. \\
&\quad \left. - \frac{2975}{18}L_{jijj}^{V8,LR} \right] + \alpha_s \alpha \left[ \frac{16}{9}L_{jijj}^{V8,LR} - \frac{64}{3}L_{jijj}^{V1,LR} \right] + \frac{173}{81}\alpha^2 L_{jijj}^{V8,LR} ; \\
\dot{L}_{jijj}^{V1,LR} &= -\frac{8}{3}g_s^2 L_{jijj}^{V8,LR} - \frac{4}{3}e^2 L_{jijj}^{V1,LR} + \alpha_s^2 \left[ -\frac{28}{3}L_{jijj}^{V1,LR} - \frac{2044}{27}L_{jijj}^{V8,LR} \right]
\end{aligned}$$

$$\begin{aligned}
& + \alpha_s \alpha \left[ \frac{32}{3} L_{j\bar{i}i}^{V1,LR} - \frac{8}{27} L_{j\bar{i}i}^{V8,LR} \right] + \frac{1790}{81} \alpha^2 L_{j\bar{i}i}^{V1,LR} ; \\
\dot{L}_{j\bar{i}i}^{V8,LR} & = g_s^2 \left[ -12 L_{j\bar{i}i}^{V1,LR} - 14 L_{j\bar{i}i}^{V8,LR} \right] - \frac{4}{3} e^2 L_{j\bar{i}i}^{V8,LR} + \alpha_s^2 \left[ -\frac{374}{3} L_{j\bar{i}i}^{V1,LR} \right. \\
& \quad \left. - \frac{2975}{18} L_{j\bar{i}i}^{V8,LR} \right] + \alpha_s \alpha \left[ -\frac{4}{3} L_{j\bar{i}i}^{V1,LR} - \frac{26}{9} L_{j\bar{i}i}^{V8,LR} \right] + \frac{1790}{81} \alpha^2 L_{j\bar{i}i}^{V8,LR} ; \\
\dot{L}_{j\bar{i}i}^{V1,LR} & = -\frac{8}{3} g_s^2 L_{j\bar{i}i}^{V8,LR} - \frac{16}{3} e^2 L_{j\bar{i}i}^{V1,LR} + \alpha_s^2 \left[ -\frac{28}{3} L_{j\bar{i}i}^{V1,LR} - \frac{2044}{27} L_{j\bar{i}i}^{V8,LR} \right] \\
& \quad + \alpha_s \alpha \left[ \frac{128}{3} L_{j\bar{i}i}^{V1,LR} - \frac{32}{27} L_{j\bar{i}i}^{V8,LR} \right] + \frac{7520}{81} \alpha^2 L_{j\bar{i}i}^{V1,LR} ; \\
\dot{L}_{j\bar{i}i}^{V8,LR} & = g_s^2 \left[ -12 L_{j\bar{i}i}^{V1,LR} - 14 L_{j\bar{i}i}^{V8,LR} \right] - \frac{16}{3} e^2 L_{j\bar{i}i}^{V8,LR} + \alpha_s^2 \left[ -\frac{374}{3} L_{j\bar{i}i}^{V1,LR} \right. \\
& \quad \left. - \frac{2975}{18} L_{j\bar{i}i}^{V8,LR} \right] + \alpha_s \alpha \left[ -\frac{16}{3} L_{j\bar{i}i}^{V1,LR} - \frac{104}{9} L_{j\bar{i}i}^{V8,LR} \right] + \frac{7520}{81} \alpha^2 L_{j\bar{i}i}^{V8,LR} ; \\
\dot{L}_{j\bar{i}i}^{V,LR} & = \frac{2030}{9} \alpha^2 L_{j\bar{i}i}^{V,LR} - 12 e^2 L_{j\bar{i}i}^{V,LR} ; \\
\dot{L}_{i\bar{j}j}^{S,RR} & = -8 g_s^2 L_{i\bar{j}j}^{S,RR} + e^2 \left[ -\frac{20}{3} L_{i\bar{j}j}^{S,RR} - 32 L_{i\bar{j}j}^{T,RR} \right] - \frac{1012}{9} \alpha_s^2 L_{i\bar{j}j}^{S,RR} \\
& \quad + \alpha_s \alpha \left[ \frac{1792}{9} L_{i\bar{j}j}^{T,RR} - \frac{8}{9} L_{i\bar{j}j}^{S,RR} \right] + \alpha^2 \left[ \frac{1882}{81} L_{i\bar{j}j}^{S,RR} + \frac{19712}{27} L_{i\bar{j}j}^{T,RR} \right] ; \\
\dot{L}_{i\bar{j}j}^{T,RR} & = \frac{8}{3} g_s^2 L_{i\bar{j}j}^{T,RR} + e^2 \left[ \frac{20}{9} L_{i\bar{j}j}^{T,RR} - \frac{2}{3} L_{i\bar{j}j}^{S,RR} \right] + \frac{1652}{27} \alpha_s^2 L_{i\bar{j}j}^{T,RR} \\
& \quad + \alpha_s \alpha \left[ \frac{16}{3} L_{i\bar{j}j}^{S,RR} - \frac{152}{27} L_{i\bar{j}j}^{T,RR} \right] + \alpha^2 \left[ \frac{368}{81} L_{i\bar{j}j}^{S,RR} - \frac{7154}{243} L_{i\bar{j}j}^{T,RR} \right] ; \\
\dot{L}_{i\bar{j}j}^{S,RR} & = -8 g_s^2 L_{i\bar{j}j}^{S,RR} + e^2 \left[ 64 L_{i\bar{j}j}^{T,RR} - \frac{26}{3} L_{i\bar{j}j}^{S,RR} \right] - \frac{1012}{9} \alpha_s^2 L_{i\bar{j}j}^{S,RR} \\
& \quad + \alpha_s \alpha \left[ -\frac{32}{9} L_{i\bar{j}j}^{S,RR} - \frac{3584}{9} L_{i\bar{j}j}^{T,RR} \right] + \alpha^2 \left[ -\frac{2579}{81} L_{i\bar{j}j}^{S,RR} - \frac{35200}{27} L_{i\bar{j}j}^{T,RR} \right] ;
\end{aligned}$$



$$\begin{aligned}
\dot{L}_{\substack{eu \\ ij\bar{j}}}^{T,RR} &= \frac{8}{3}g_s^2 L_{\substack{eu \\ ij\bar{j}}}^{T,RR} + e^2 \left[ \frac{4}{3} L_{\substack{eu \\ ij\bar{j}}}^{S,RR} + \frac{26}{9} L_{\substack{eu \\ ij\bar{j}}}^{T,RR} \right] + \frac{1652}{27} \alpha_s^2 L_{\substack{eu \\ ij\bar{j}}}^{T,RR} \\
&\quad + \alpha_s \alpha \left[ -\frac{32}{3} L_{\substack{eu \\ ij\bar{j}}}^{S,RR} - \frac{608}{27} L_{\substack{eu \\ ij\bar{j}}}^{T,RR} \right] + \alpha^2 \left[ -\frac{1384}{81} L_{\substack{eu \\ ij\bar{j}}}^{S,RR} - \frac{21929}{243} L_{\substack{eu \\ ij\bar{j}}}^{T,RR} \right]; \\
\dot{L}_{\substack{\nu e \\ ij\bar{j}}}^{S,LL} &= \frac{373}{9} \alpha^2 L_{\substack{\nu e \\ ij\bar{j}}}^{S,LL} - 6e^2 L_{\substack{\nu e \\ ij\bar{j}}}^{S,LL}; \\
\dot{L}_{\substack{\nu e \\ ij\bar{j}}}^{T,LL} &= 2e^2 L_{\substack{\nu e \\ ij\bar{j}}}^{T,LL} - \frac{1553}{27} \alpha^2 L_{\substack{\nu e \\ ij\bar{j}}}^{T,LL}; \\
\dot{L}_{\substack{\nu d \\ ij\bar{j}}}^{S,LL} &= -8g_s^2 L_{\substack{\nu d \\ ij\bar{j}}}^{S,LL} - \frac{2}{3} e^2 L_{\substack{\nu d \\ ij\bar{j}}}^{S,LL} - \frac{1012}{9} \alpha_s^2 L_{\substack{\nu d \\ ij\bar{j}}}^{S,LL} - \frac{8}{9} \alpha_s \alpha L_{\substack{\nu d \\ ij\bar{j}}}^{S,LL} \\
&\quad + \frac{397}{81} \alpha^2 L_{\substack{\nu d \\ ij\bar{j}}}^{S,LL}; \\
\dot{L}_{\substack{\nu d \\ ij\bar{j}}}^{T,LL} &= \frac{8}{3} g_s^2 L_{\substack{\nu d \\ ij\bar{j}}}^{T,LL} + \frac{2}{9} e^2 L_{\substack{\nu d \\ ij\bar{j}}}^{T,LL} + \frac{1652}{27} \alpha_s^2 L_{\substack{\nu d \\ ij\bar{j}}}^{T,LL} - \frac{152}{27} \alpha_s \alpha L_{\substack{\nu d \\ ij\bar{j}}}^{T,LL} \\
&\quad - \frac{1097}{243} \alpha^2 L_{\substack{\nu d \\ ij\bar{j}}}^{T,LL}; \\
\dot{L}_{\substack{\nu u \\ ij\bar{j}}}^{S,LL} &= -8g_s^2 L_{\substack{\nu u \\ ij\bar{j}}}^{S,LL} - \frac{8}{3} e^2 L_{\substack{\nu u \\ ij\bar{j}}}^{S,LL} - \frac{1012}{9} \alpha_s^2 L_{\substack{\nu u \\ ij\bar{j}}}^{S,LL} - \frac{32}{9} \alpha_s \alpha L_{\substack{\nu u \\ ij\bar{j}}}^{S,LL} \\
&\quad + \frac{1552}{81} \alpha^2 L_{\substack{\nu u \\ ij\bar{j}}}^{S,LL}; \\
\dot{L}_{\substack{\nu u \\ ij\bar{j}}}^{T,LL} &= \frac{8}{3} g_s^2 L_{\substack{\nu u \\ ij\bar{j}}}^{T,LL} + \frac{8}{9} e^2 L_{\substack{\nu u \\ ij\bar{j}}}^{T,LL} + \frac{1652}{27} \alpha_s^2 L_{\substack{\nu u \\ ij\bar{j}}}^{T,LL} - \frac{608}{27} \alpha_s \alpha L_{\substack{\nu u \\ ij\bar{j}}}^{T,LL} \\
&\quad - \frac{5072}{243} \alpha^2 L_{\substack{\nu u \\ ij\bar{j}}}^{T,LL}; \\
\dot{L}_{\substack{ud \\ ij\bar{j}}}^{S1,RR} &= g_s^2 \left[ \frac{64}{9} L_{\substack{uddu \\ ij\bar{j}i}}^{S1,RR} + \frac{112}{27} L_{\substack{uddu \\ ij\bar{j}i}}^{S8,RR} - 16 L_{\substack{ud \\ ij\bar{j}}}^{S1,RR} + \frac{16}{9} L_{\substack{ud \\ ij\bar{j}}}^{S8,RR} \right] \\
&\quad + e^2 \left[ \frac{4}{27} L_{\substack{uddu \\ ij\bar{j}i}}^{S1,RR} + \frac{16}{81} L_{\substack{uddu \\ ij\bar{j}i}}^{S8,RR} - \frac{46}{9} L_{\substack{ud \\ ij\bar{j}}}^{S1,RR} \right] + \alpha_s^2 \left[ \frac{9472}{81} L_{\substack{uddu \\ ij\bar{j}i}}^{S1,RR} + \frac{16576}{243} L_{\substack{uddu \\ ij\bar{j}i}}^{S8,RR} \right. \\
&\quad \left. - \frac{2120}{9} L_{\substack{ud \\ ij\bar{j}}}^{S1,RR} + \frac{928}{81} L_{\substack{ud \\ ij\bar{j}}}^{S8,RR} \right] + \alpha_s \alpha \left[ \frac{1888}{81} L_{\substack{uddu \\ ij\bar{j}i}}^{S1,RR} + \frac{3808}{243} L_{\substack{uddu \\ ij\bar{j}i}}^{S8,RR} + \frac{136}{27} L_{\substack{ud \\ ij\bar{j}}}^{S1,RR} \right. \\
&\quad \left. + \frac{224}{81} L_{\substack{ud \\ ij\bar{j}}}^{S8,RR} \right] + \alpha^2 \left[ \frac{98}{729} L_{\substack{uddu \\ ij\bar{j}i}}^{S1,RR} + \frac{392}{2187} L_{\substack{uddu \\ ij\bar{j}i}}^{S8,RR} + \frac{6391}{243} L_{\substack{ud \\ ij\bar{j}}}^{S1,RR} \right];
\end{aligned}$$

$$\begin{aligned}
\dot{L}_{ijj}^{S8,RR} = & g_s^2 \left[ -\frac{16}{3} L_{ijji}^{S1,RR} + \frac{44}{9} L_{ijji}^{S8,RR} + 8 L_{ijj}^{S1,RR} + \frac{16}{3} L_{ijj}^{S8,RR} \right] \\
& + e^2 \left[ \frac{8}{9} L_{ijji}^{S1,RR} - \frac{4}{27} L_{ijji}^{S8,RR} - \frac{46}{9} L_{ijj}^{S8,RR} \right] + \alpha_s^2 \left[ -\frac{856}{27} L_{ijji}^{S1,RR} - \frac{2506}{81} L_{ijji}^{S8,RR} \right. \\
& + \frac{248}{9} L_{ijj}^{S1,RR} + \frac{2995}{27} L_{ijj}^{S8,RR} \left. \right] + \alpha_s \alpha \left[ -\frac{868}{27} L_{ijji}^{S1,RR} + \frac{1370}{81} L_{ijji}^{S8,RR} + \frac{112}{9} L_{ijj}^{S1,RR} \right. \\
& + \frac{224}{9} L_{ijj}^{S8,RR} \left. \right] + \alpha^2 \left[ \frac{196}{243} L_{ijji}^{S1,RR} - \frac{98}{729} L_{ijji}^{S8,RR} + \frac{6391}{243} L_{ijj}^{S8,RR} \right];
\end{aligned}$$

$$\begin{aligned}
\dot{L}_{ijji}^{S1,RR} = & g_s^2 \left[ -16 L_{ijji}^{S1,RR} + \frac{16}{9} L_{ijji}^{S8,RR} + \frac{64}{9} L_{ijj}^{S1,RR} + \frac{112}{27} L_{ijj}^{S8,RR} \right] \\
& + e^2 \left[ \frac{26}{9} L_{ijji}^{S1,RR} - \frac{32}{27} L_{ijji}^{S8,RR} - \frac{128}{81} L_{ijj}^{S8,RR} \right] + \alpha_s^2 \left[ -\frac{2120}{9} L_{ijji}^{S1,RR} + \frac{928}{81} L_{ijji}^{S8,RR} \right. \\
& + \frac{9472}{81} L_{ijj}^{S1,RR} + \frac{16576}{243} L_{ijj}^{S8,RR} \left. \right] + \alpha_s \alpha \left[ \frac{712}{27} L_{ijji}^{S1,RR} - \frac{64}{81} L_{ijji}^{S8,RR} - \frac{2144}{81} L_{ijj}^{S1,RR} \right. \\
& - \frac{7784}{243} L_{ijj}^{S8,RR} \left. \right] + \alpha^2 \left[ -\frac{13769}{243} L_{ijji}^{S1,RR} + \frac{5264}{729} L_{ijji}^{S8,RR} + \frac{21056}{2187} L_{ijj}^{S8,RR} \right];
\end{aligned}$$

$$\begin{aligned}
\dot{L}_{ijji}^{S8,RR} = & g_s^2 \left[ 8 L_{ijji}^{S1,RR} + \frac{16}{3} L_{ijji}^{S8,RR} - \frac{16}{3} L_{ijj}^{S1,RR} + \frac{44}{9} L_{ijj}^{S8,RR} \right] \\
& + e^2 \left[ \frac{26}{9} L_{ijji}^{S8,RR} - \frac{64}{9} L_{ijj}^{S1,RR} + \frac{32}{27} L_{ijj}^{S8,RR} \right] + \alpha_s^2 \left[ \frac{248}{9} L_{ijji}^{S1,RR} + \frac{2995}{27} L_{ijji}^{S8,RR} \right. \\
& - \frac{856}{27} L_{ijj}^{S1,RR} - \frac{2506}{81} L_{ijj}^{S8,RR} \left. \right] + \alpha_s \alpha \left[ -\frac{32}{9} L_{ijji}^{S1,RR} - \frac{400}{9} L_{ijji}^{S8,RR} + \frac{3704}{27} L_{ijj}^{S1,RR} \right. \\
& - \frac{2050}{81} L_{ijj}^{S8,RR} \left. \right] + \alpha^2 \left[ -\frac{13769}{243} L_{ijji}^{S8,RR} + \frac{10528}{243} L_{ijj}^{S1,RR} - \frac{5264}{729} L_{ijj}^{S8,RR} \right];
\end{aligned}$$

$$\begin{aligned}
\dot{L}_{jji}^{S,RR} = & -8g_s^2 L_{jji}^{S,RR} + e^2 \left[ -\frac{20}{3} L_{jji}^{S,RR} - 32 L_{jji}^{T,RR} \right] - \frac{1012}{9} \alpha_s^2 L_{jji}^{S,RR} \\
& + \alpha_s \alpha \left[ \frac{1792}{9} L_{jji}^{T,RR} - \frac{8}{9} L_{jji}^{S,RR} \right] + \alpha^2 \left[ \frac{1882}{81} L_{jji}^{S,RR} + \frac{19712}{27} L_{jji}^{T,RR} \right];
\end{aligned}$$

$$\begin{aligned}
\dot{L}_{ed,jji}^{T,RR} &= \frac{8}{3}g_s^2 L_{ed,jji}^{T,RR} + e^2 \left[ \frac{20}{9} L_{ed,jji}^{T,RR} - \frac{2}{3} L_{ed,jji}^{S,RR} \right] + \frac{1652}{27} \alpha_s^2 L_{ed,jji}^{T,RR} \\
&\quad + \alpha_s \alpha \left[ \frac{16}{3} L_{ed,jji}^{S,RR} - \frac{152}{27} L_{ed,jji}^{T,RR} \right] + \alpha^2 \left[ \frac{368}{81} L_{ed,jji}^{S,RR} - \frac{7154}{243} L_{ed,jji}^{T,RR} \right]; \\
\dot{L}_{eu,jji}^{S,RR} &= -8g_s^2 L_{eu,jji}^{S,RR} + e^2 \left[ 64 L_{eu,jji}^{T,RR} - \frac{26}{3} L_{eu,jji}^{S,RR} \right] - \frac{1012}{9} \alpha_s^2 L_{eu,jji}^{S,RR} \\
&\quad + \alpha_s \alpha \left[ -\frac{32}{9} L_{eu,jji}^{S,RR} - \frac{3584}{9} L_{eu,jji}^{T,RR} \right] + \alpha^2 \left[ -\frac{2579}{81} L_{eu,jji}^{S,RR} - \frac{35200}{27} L_{eu,jji}^{T,RR} \right]; \\
\dot{L}_{eu,jji}^{T,RR} &= \frac{8}{3}g_s^2 L_{eu,jji}^{T,RR} + e^2 \left[ \frac{4}{3} L_{eu,jji}^{S,RR} + \frac{26}{9} L_{eu,jji}^{T,RR} \right] + \frac{1652}{27} \alpha_s^2 L_{eu,jji}^{T,RR} \\
&\quad + \alpha_s \alpha \left[ -\frac{32}{3} L_{eu,jji}^{S,RR} - \frac{608}{27} L_{eu,jji}^{T,RR} \right] + \alpha^2 \left[ -\frac{1384}{81} L_{eu,jji}^{S,RR} - \frac{21929}{243} L_{eu,jji}^{T,RR} \right]; \\
\dot{L}_{\nu e,jji}^{S,LL} &= \frac{373}{9} \alpha^2 L_{\nu e,jji}^{S,LL} - 6e^2 L_{\nu e,jji}^{S,LL}; \\
\dot{L}_{\nu e,jji}^{T,LL} &= 2e^2 L_{\nu e,jji}^{T,LL} - \frac{1553}{27} \alpha^2 L_{\nu e,jji}^{T,LL}; \\
\dot{L}_{\nu d,jji}^{S,LL} &= -8g_s^2 L_{\nu d,jji}^{S,LL} - \frac{2}{3} e^2 L_{\nu d,jji}^{S,LL} - \frac{1012}{9} \alpha_s^2 L_{\nu d,jji}^{S,LL} - \frac{8}{9} \alpha_s \alpha L_{\nu d,jji}^{S,LL} \\
&\quad + \frac{397}{81} \alpha^2 L_{\nu d,jji}^{S,LL}; \\
\dot{L}_{\nu d,jji}^{T,LL} &= \frac{8}{3} g_s^2 L_{\nu d,jji}^{T,LL} + \frac{2}{9} e^2 L_{\nu d,jji}^{T,LL} + \frac{1652}{27} \alpha_s^2 L_{\nu d,jji}^{T,LL} - \frac{152}{27} \alpha_s \alpha L_{\nu d,jji}^{T,LL} \\
&\quad - \frac{1097}{243} \alpha^2 L_{\nu d,jji}^{T,LL}; \\
\dot{L}_{\nu u,jji}^{S,LL} &= -8g_s^2 L_{\nu u,jji}^{S,LL} - \frac{8}{3} e^2 L_{\nu u,jji}^{S,LL} - \frac{1012}{9} \alpha_s^2 L_{\nu u,jji}^{S,LL} - \frac{32}{9} \alpha_s \alpha L_{\nu u,jji}^{S,LL} \\
&\quad + \frac{1552}{81} \alpha^2 L_{\nu u,jji}^{S,LL}; \\
\dot{L}_{\nu u,jji}^{T,LL} &= \frac{8}{3} g_s^2 L_{\nu u,jji}^{T,LL} + \frac{8}{9} e^2 L_{\nu u,jji}^{T,LL} + \frac{1652}{27} \alpha_s^2 L_{\nu u,jji}^{T,LL} - \frac{608}{27} \alpha_s \alpha L_{\nu u,jji}^{T,LL} \\
&\quad - \frac{5072}{243} \alpha^2 L_{\nu u,jji}^{T,LL};
\end{aligned}$$

$$\begin{aligned}
\dot{L}_{\substack{ud \\ jj\bar{i}}}^{S1,RR} = & g_s^2 \left[ \frac{64}{9} L_{\substack{uddu \\ j\bar{i}j}}^{S1,RR} + \frac{112}{27} L_{\substack{uddu \\ j\bar{i}j}}^{S8,RR} - 16 L_{\substack{ud \\ j\bar{j}i}}^{S1,RR} + \frac{16}{9} L_{\substack{ud \\ j\bar{j}i}}^{S8,RR} \right] \\
& + e^2 \left[ \frac{4}{27} L_{\substack{uddu \\ j\bar{i}j}}^{S1,RR} + \frac{16}{81} L_{\substack{uddu \\ j\bar{i}j}}^{S8,RR} - \frac{46}{9} L_{\substack{ud \\ j\bar{j}i}}^{S1,RR} \right] + \alpha_s^2 \left[ \frac{9472}{81} L_{\substack{uddu \\ j\bar{i}j}}^{S1,RR} + \frac{16576}{243} L_{\substack{uddu \\ j\bar{i}j}}^{S8,RR} \right. \\
& - \frac{2120}{9} L_{\substack{ud \\ j\bar{j}i}}^{S1,RR} + \frac{928}{81} L_{\substack{ud \\ j\bar{j}i}}^{S8,RR} \left. \right] + \alpha_s \alpha \left[ \frac{1888}{81} L_{\substack{uddu \\ j\bar{i}j}}^{S1,RR} + \frac{3808}{243} L_{\substack{uddu \\ j\bar{i}j}}^{S8,RR} + \frac{136}{27} L_{\substack{ud \\ j\bar{j}i}}^{S1,RR} \right. \\
& + \frac{224}{81} L_{\substack{ud \\ j\bar{j}i}}^{S8,RR} \left. \right] + \alpha^2 \left[ \frac{98}{729} L_{\substack{uddu \\ j\bar{i}j}}^{S1,RR} + \frac{392}{2187} L_{\substack{uddu \\ j\bar{i}j}}^{S8,RR} + \frac{6391}{243} L_{\substack{ud \\ j\bar{j}i}}^{S1,RR} \right];
\end{aligned}$$

$$\begin{aligned}
\dot{L}_{\substack{ud \\ jj\bar{i}}}^{S8,RR} = & g_s^2 \left[ -\frac{16}{3} L_{\substack{uddu \\ j\bar{i}j}}^{S1,RR} + \frac{44}{9} L_{\substack{uddu \\ j\bar{i}j}}^{S8,RR} + 8 L_{\substack{ud \\ j\bar{j}i}}^{S1,RR} + \frac{16}{3} L_{\substack{ud \\ j\bar{j}i}}^{S8,RR} \right] \\
& + e^2 \left[ \frac{8}{9} L_{\substack{uddu \\ j\bar{i}j}}^{S1,RR} - \frac{4}{27} L_{\substack{uddu \\ j\bar{i}j}}^{S8,RR} - \frac{46}{9} L_{\substack{ud \\ j\bar{j}i}}^{S8,RR} \right] + \alpha_s^2 \left[ -\frac{856}{27} L_{\substack{uddu \\ j\bar{i}j}}^{S1,RR} - \frac{2506}{81} L_{\substack{uddu \\ j\bar{i}j}}^{S8,RR} \right. \\
& + \frac{248}{9} L_{\substack{ud \\ j\bar{j}i}}^{S1,RR} + \frac{2995}{27} L_{\substack{ud \\ j\bar{j}i}}^{S8,RR} \left. \right] + \alpha_s \alpha \left[ -\frac{868}{27} L_{\substack{uddu \\ j\bar{i}j}}^{S1,RR} + \frac{1370}{81} L_{\substack{uddu \\ j\bar{i}j}}^{S8,RR} + \frac{112}{9} L_{\substack{ud \\ j\bar{j}i}}^{S1,RR} \right. \\
& + \frac{224}{9} L_{\substack{ud \\ j\bar{j}i}}^{S8,RR} \left. \right] + \alpha^2 \left[ \frac{196}{243} L_{\substack{uddu \\ j\bar{i}j}}^{S1,RR} - \frac{98}{729} L_{\substack{uddu \\ j\bar{i}j}}^{S8,RR} + \frac{6391}{243} L_{\substack{ud \\ j\bar{j}i}}^{S8,RR} \right];
\end{aligned}$$

$$\begin{aligned}
\dot{L}_{\substack{uddu \\ j\bar{i}j}}^{S1,RR} = & g_s^2 \left[ -16 L_{\substack{uddu \\ j\bar{i}j}}^{S1,RR} + \frac{16}{9} L_{\substack{uddu \\ j\bar{i}j}}^{S8,RR} + \frac{64}{9} L_{\substack{ud \\ j\bar{j}i}}^{S1,RR} + \frac{112}{27} L_{\substack{ud \\ j\bar{j}i}}^{S8,RR} \right] \\
& + e^2 \left[ \frac{26}{9} L_{\substack{uddu \\ j\bar{i}j}}^{S1,RR} - \frac{32}{27} L_{\substack{ud \\ j\bar{j}i}}^{S1,RR} - \frac{128}{81} L_{\substack{ud \\ j\bar{j}i}}^{S8,RR} \right] + \alpha_s^2 \left[ -\frac{2120}{9} L_{\substack{uddu \\ j\bar{i}j}}^{S1,RR} + \frac{928}{81} L_{\substack{uddu \\ j\bar{i}j}}^{S8,RR} \right. \\
& + \frac{9472}{81} L_{\substack{ud \\ j\bar{j}i}}^{S1,RR} + \frac{16576}{243} L_{\substack{ud \\ j\bar{j}i}}^{S8,RR} \left. \right] + \alpha_s \alpha \left[ \frac{712}{27} L_{\substack{uddu \\ j\bar{i}j}}^{S1,RR} - \frac{64}{81} L_{\substack{uddu \\ j\bar{i}j}}^{S8,RR} - \frac{2144}{81} L_{\substack{ud \\ j\bar{j}i}}^{S1,RR} \right. \\
& - \frac{7784}{243} L_{\substack{ud \\ j\bar{j}i}}^{S8,RR} \left. \right] + \alpha^2 \left[ -\frac{13769}{243} L_{\substack{uddu \\ j\bar{i}j}}^{S1,RR} + \frac{5264}{729} L_{\substack{ud \\ j\bar{j}i}}^{S1,RR} + \frac{21056}{2187} L_{\substack{ud \\ j\bar{j}i}}^{S8,RR} \right];
\end{aligned}$$

$$\begin{aligned}
\dot{L}_{\substack{uddu \\ j\bar{i}j}}^{S8,RR} = & g_s^2 \left[ 8 L_{\substack{uddu \\ j\bar{i}j}}^{S1,RR} + \frac{16}{3} L_{\substack{uddu \\ j\bar{i}j}}^{S8,RR} - \frac{16}{3} L_{\substack{ud \\ j\bar{j}i}}^{S1,RR} + \frac{44}{9} L_{\substack{ud \\ j\bar{j}i}}^{S8,RR} \right] \\
& + e^2 \left[ \frac{26}{9} L_{\substack{uddu \\ j\bar{i}j}}^{S8,RR} - \frac{64}{9} L_{\substack{ud \\ j\bar{j}i}}^{S1,RR} + \frac{32}{27} L_{\substack{ud \\ j\bar{j}i}}^{S8,RR} \right] + \alpha_s^2 \left[ \frac{248}{9} L_{\substack{uddu \\ j\bar{i}j}}^{S1,RR} + \frac{2995}{27} L_{\substack{uddu \\ j\bar{i}j}}^{S8,RR} \right.
\end{aligned}$$

$$\begin{aligned}
& -\frac{856}{27}L_{jji}^{S1,RR} - \frac{2506}{81}L_{jji}^{S8,RR} \Big] + \alpha_s \alpha \Big[ -\frac{32}{9}L_{jij}^{S1,RR} - \frac{400}{9}L_{jij}^{S8,RR} + \frac{3704}{27}L_{jji}^{S1,RR} \\
& - \frac{2050}{81}L_{jji}^{S8,RR} \Big] + \alpha^2 \Big[ -\frac{13769}{243}L_{jij}^{S8,RR} + \frac{10528}{243}L_{jji}^{S1,RR} - \frac{5264}{729}L_{jji}^{S8,RR} \Big] ; \\
\dot{L}_{iij}^{S1,RR} &= g_s^2 \Big[ -16L_{iij}^{S1,RR} + \frac{64}{9}L_{iij}^{S1,RR} + \frac{16}{9}L_{iij}^{S8,RR} + \frac{112}{27}L_{iij}^{S8,RR} \Big] \\
& + e^2 \Big[ -\frac{4}{9}L_{iij}^{S1,RR} + \frac{16}{27}L_{iij}^{S1,RR} + \frac{64}{81}L_{iij}^{S8,RR} \Big] + \alpha_s^2 \Big[ -\frac{2120}{9}L_{iij}^{S1,RR} + \frac{9472}{81}L_{iij}^{S1,RR} \\
& + \frac{928}{81}L_{iij}^{S8,RR} + \frac{16576}{243}L_{iij}^{S8,RR} \Big] + \alpha_s \alpha \Big[ -\frac{176}{27}L_{iij}^{S1,RR} - \frac{512}{81}L_{iij}^{S1,RR} - \frac{256}{81}L_{iij}^{S8,RR} \\
& + \frac{1120}{243}L_{iij}^{S8,RR} \Big] + \alpha^2 \Big[ \frac{1822}{243}L_{iij}^{S1,RR} - \frac{832}{729}L_{iij}^{S1,RR} - \frac{3328}{2187}L_{iij}^{S8,RR} \Big] ; \\
\dot{L}_{iij}^{S8,RR} &= g_s^2 \Big[ 8L_{iij}^{S1,RR} - \frac{16}{3}L_{iij}^{S1,RR} + \frac{16}{3}L_{iij}^{S8,RR} + \frac{44}{9}L_{iij}^{S8,RR} \Big] + e^2 \Big[ \frac{32}{9}L_{iij}^{S1,RR} \\
& - \frac{4}{9}L_{iij}^{S8,RR} - \frac{16}{27}L_{iij}^{S8,RR} \Big] + \alpha_s^2 \Big[ \frac{248}{9}L_{iij}^{S1,RR} - \frac{856}{27}L_{iij}^{S1,RR} + \frac{2995}{27}L_{iij}^{S8,RR} \\
& - \frac{2506}{81}L_{iij}^{S8,RR} \Big] + \alpha_s \alpha \Big[ -\frac{128}{9}L_{iij}^{S1,RR} - \frac{1456}{27}L_{iij}^{S1,RR} - \frac{16}{9}L_{iij}^{S8,RR} - \frac{64}{81}L_{iij}^{S8,RR} \Big] \\
& + \alpha^2 \Big[ -\frac{1664}{243}L_{iij}^{S1,RR} + \frac{1822}{243}L_{iij}^{S8,RR} + \frac{832}{729}L_{iij}^{S8,RR} \Big] ; \\
\dot{L}_{iij}^{S1,RR} &= g_s^2 \Big[ \frac{64}{9}L_{iij}^{S1,RR} - 16L_{iij}^{S1,RR} + \frac{112}{27}L_{iij}^{S8,RR} + \frac{16}{9}L_{iij}^{S8,RR} \Big] \\
& + e^2 \Big[ \frac{16}{27}L_{iij}^{S1,RR} - \frac{4}{9}L_{iij}^{S1,RR} + \frac{64}{81}L_{iij}^{S8,RR} \Big] + \alpha_s^2 \Big[ \frac{9472}{81}L_{iij}^{S1,RR} - \frac{2120}{9}L_{iij}^{S1,RR} \\
& + \frac{16576}{243}L_{iij}^{S8,RR} + \frac{928}{81}L_{iij}^{S8,RR} \Big] + \alpha_s \alpha \Big[ -\frac{512}{81}L_{iij}^{S1,RR} - \frac{176}{27}L_{iij}^{S1,RR} + \frac{1120}{243}L_{iij}^{S8,RR} \\
& - \frac{256}{81}L_{iij}^{S8,RR} \Big] + \alpha^2 \Big[ -\frac{832}{729}L_{iij}^{S1,RR} + \frac{1822}{243}L_{iij}^{S1,RR} - \frac{3328}{2187}L_{iij}^{S8,RR} \Big] ;
\end{aligned}$$

$$\begin{aligned}
\dot{L}_{dd\ ijj}^{S8,RR} = & g_s^2 \left[ -\frac{16}{3} L_{dd\ ijj}^{S1,RR} + 8 L_{dd\ ijj}^{S1,RR} + \frac{44}{9} L_{dd\ ijj}^{S8,RR} + \frac{16}{3} L_{dd\ ijj}^{S8,RR} \right] \\
& + e^2 \left[ \frac{32}{9} L_{dd\ ijj}^{S1,RR} - \frac{16}{27} L_{dd\ ijj}^{S8,RR} - \frac{4}{9} L_{dd\ ijj}^{S8,RR} \right] + \alpha_s^2 \left[ -\frac{856}{27} L_{dd\ ijj}^{S1,RR} + \frac{248}{9} L_{dd\ ijj}^{S1,RR} \right. \\
& - \frac{2506}{81} L_{dd\ ijj}^{S8,RR} + \frac{2995}{27} L_{dd\ ijj}^{S8,RR} \left. \right] + \alpha_s \alpha \left[ -\frac{1456}{27} L_{dd\ ijj}^{S1,RR} - \frac{128}{9} L_{dd\ ijj}^{S1,RR} - \frac{64}{81} L_{dd\ ijj}^{S8,RR} \right. \\
& \left. - \frac{16}{9} L_{dd\ ijj}^{S8,RR} \right] + \alpha^2 \left[ -\frac{1664}{243} L_{dd\ ijj}^{S1,RR} + \frac{832}{729} L_{dd\ ijj}^{S8,RR} + \frac{1822}{243} L_{dd\ ijj}^{S8,RR} \right];
\end{aligned}$$

$$\begin{aligned}
\dot{L}_{dd\ iii}^{S1,RR} = & g_s^2 \left[ \frac{160}{27} L_{dd\ iii}^{S8,RR} - \frac{80}{9} L_{dd\ iii}^{S1,RR} \right] + e^2 \left[ \frac{4}{27} L_{dd\ iii}^{S1,RR} + \frac{64}{81} L_{dd\ iii}^{S8,RR} \right] \\
& + \alpha_s^2 \left[ \frac{19360}{243} L_{dd\ iii}^{S8,RR} - \frac{9608}{81} L_{dd\ iii}^{S1,RR} \right] + \alpha_s \alpha \left[ \frac{352}{243} L_{dd\ iii}^{S8,RR} - \frac{1040}{81} L_{dd\ iii}^{S1,RR} \right] \\
& + \alpha^2 \left[ \frac{4634}{729} L_{dd\ iii}^{S1,RR} - \frac{3328}{2187} L_{dd\ iii}^{S8,RR} \right];
\end{aligned}$$

$$\begin{aligned}
\dot{L}_{dd\ iii}^{S8,RR} = & g_s^2 \left[ \frac{8}{3} L_{dd\ iii}^{S1,RR} + \frac{92}{9} L_{dd\ iii}^{S8,RR} \right] + e^2 \left[ \frac{32}{9} L_{dd\ iii}^{S1,RR} - \frac{28}{27} L_{dd\ iii}^{S8,RR} \right] \\
& + \alpha_s^2 \left[ \frac{6479}{81} L_{dd\ iii}^{S8,RR} - \frac{112}{27} L_{dd\ iii}^{S1,RR} \right] + \alpha_s \alpha \left[ -\frac{1840}{27} L_{dd\ iii}^{S1,RR} - \frac{208}{81} L_{dd\ iii}^{S8,RR} \right] \\
& + \alpha^2 \left[ \frac{6298}{729} L_{dd\ iii}^{S8,RR} - \frac{1664}{243} L_{dd\ iii}^{S1,RR} \right];
\end{aligned}$$

$$\begin{aligned}
\dot{L}_{uu\ ijj}^{S1,RR} = & g_s^2 \left[ -16 L_{uu\ ijj}^{S1,RR} + \frac{64}{9} L_{uu\ ijj}^{S1,RR} + \frac{16}{9} L_{uu\ ijj}^{S8,RR} + \frac{112}{27} L_{uu\ ijj}^{S8,RR} \right] \\
& + e^2 \left[ -\frac{16}{9} L_{uu\ ijj}^{S1,RR} + \frac{64}{27} L_{uu\ ijj}^{S1,RR} + \frac{256}{81} L_{uu\ ijj}^{S8,RR} \right] + \alpha_s^2 \left[ -\frac{2120}{9} L_{uu\ ijj}^{S1,RR} + \frac{9472}{81} L_{uu\ ijj}^{S1,RR} \right. \\
& + \frac{928}{81} L_{uu\ ijj}^{S8,RR} + \frac{16576}{243} L_{uu\ ijj}^{S8,RR} \left. \right] + \alpha_s \alpha \left[ -\frac{704}{27} L_{uu\ ijj}^{S1,RR} - \frac{2048}{81} L_{uu\ ijj}^{S1,RR} - \frac{1024}{81} L_{uu\ ijj}^{S8,RR} \right. \\
& \left. + \frac{4480}{243} L_{uu\ ijj}^{S8,RR} \right] + \alpha^2 \left[ \frac{4192}{243} L_{uu\ ijj}^{S1,RR} - \frac{5632}{729} L_{uu\ ijj}^{S1,RR} - \frac{22528}{2187} L_{uu\ ijj}^{S8,RR} \right];
\end{aligned}$$

$$\begin{aligned}
\dot{L}_{ijj}^{S8,RR} &= g_s^2 \left[ 8L_{ijj}^{S1,RR} - \frac{16}{3}L_{ijji}^{S1,RR} + \frac{16}{3}L_{ijj}^{S8,RR} + \frac{44}{9}L_{ijji}^{S8,RR} \right] + e^2 \left[ \frac{128}{9}L_{ijji}^{S1,RR} \right. \\
&\quad \left. - \frac{16}{9}L_{ijj}^{S8,RR} - \frac{64}{27}L_{ijji}^{S8,RR} \right] + \alpha_s^2 \left[ \frac{248}{9}L_{ijj}^{S1,RR} - \frac{856}{27}L_{ijji}^{S1,RR} + \frac{2995}{27}L_{ijj}^{S8,RR} \right. \\
&\quad \left. - \frac{2506}{81}L_{ijji}^{S8,RR} \right] + \alpha_s \alpha \left[ -\frac{512}{9}L_{ijj}^{S1,RR} - \frac{5824}{27}L_{ijji}^{S1,RR} - \frac{64}{9}L_{ijj}^{S8,RR} - \frac{256}{81}L_{ijji}^{S8,RR} \right] \\
&\quad + \alpha^2 \left[ -\frac{11264}{243}L_{ijji}^{S1,RR} + \frac{4192}{243}L_{ijj}^{S8,RR} + \frac{5632}{729}L_{ijji}^{S8,RR} \right]; \\
\dot{L}_{ijji}^{S1,RR} &= g_s^2 \left[ \frac{64}{9}L_{ijj}^{S1,RR} - 16L_{ijji}^{S1,RR} + \frac{112}{27}L_{ijj}^{S8,RR} + \frac{16}{9}L_{ijji}^{S8,RR} \right] \\
&\quad + e^2 \left[ \frac{64}{27}L_{ijj}^{S1,RR} - \frac{16}{9}L_{ijji}^{S1,RR} + \frac{256}{81}L_{ijj}^{S8,RR} \right] + \alpha_s^2 \left[ \frac{9472}{81}L_{ijj}^{S1,RR} - \frac{2120}{9}L_{ijji}^{S1,RR} \right. \\
&\quad \left. + \frac{16576}{243}L_{ijj}^{S8,RR} + \frac{928}{81}L_{ijji}^{S8,RR} \right] + \alpha_s \alpha \left[ -\frac{2048}{81}L_{ijj}^{S1,RR} - \frac{704}{27}L_{ijji}^{S1,RR} + \frac{4480}{243}L_{ijj}^{S8,RR} \right. \\
&\quad \left. - \frac{1024}{81}L_{ijji}^{S8,RR} \right] + \alpha^2 \left[ -\frac{5632}{729}L_{ijj}^{S1,RR} + \frac{4192}{243}L_{ijji}^{S1,RR} - \frac{22528}{2187}L_{ijj}^{S8,RR} \right]; \\
\dot{L}_{ijji}^{S8,RR} &= g_s^2 \left[ -\frac{16}{3}L_{ijj}^{S1,RR} + 8L_{ijji}^{S1,RR} + \frac{44}{9}L_{ijj}^{S8,RR} + \frac{16}{3}L_{ijji}^{S8,RR} \right] \\
&\quad + e^2 \left[ \frac{128}{9}L_{ijj}^{S1,RR} - \frac{64}{27}L_{ijj}^{S8,RR} - \frac{16}{9}L_{ijji}^{S8,RR} \right] + \alpha_s^2 \left[ -\frac{856}{27}L_{ijj}^{S1,RR} + \frac{248}{9}L_{ijji}^{S1,RR} \right. \\
&\quad \left. - \frac{2506}{81}L_{ijj}^{S8,RR} + \frac{2995}{27}L_{ijji}^{S8,RR} \right] + \alpha_s \alpha \left[ -\frac{5824}{27}L_{ijj}^{S1,RR} - \frac{512}{9}L_{ijji}^{S1,RR} - \frac{256}{81}L_{ijj}^{S8,RR} \right. \\
&\quad \left. - \frac{64}{9}L_{ijji}^{S8,RR} \right] + \alpha^2 \left[ -\frac{11264}{243}L_{ijj}^{S1,RR} + \frac{5632}{729}L_{ijj}^{S8,RR} + \frac{4192}{243}L_{ijji}^{S8,RR} \right]; \\
\dot{L}_{iii}^{S1,RR} &= g_s^2 \left[ \frac{160}{27}L_{iii}^{S8,RR} - \frac{80}{9}L_{iii}^{S1,RR} \right] + e^2 \left[ \frac{16}{27}L_{iii}^{S1,RR} + \frac{256}{81}L_{iii}^{S8,RR} \right] \\
&\quad + \alpha_s^2 \left[ \frac{19360}{243}L_{iii}^{S8,RR} - \frac{9608}{81}L_{iii}^{S1,RR} \right] + \alpha_s \alpha \left[ \frac{1408}{243}L_{iii}^{S8,RR} - \frac{4160}{81}L_{iii}^{S1,RR} \right]
\end{aligned}$$

$$\begin{aligned}
& + \alpha^2 \left[ \frac{6944}{729} L_{uu\bar{iii}}^{S1,RR} - \frac{22528}{2187} L_{uu\bar{iii}}^{S8,RR} \right] ; \\
\dot{L}_{uu\bar{iii}}^{S8,RR} & = g_s^2 \left[ \frac{8}{3} L_{uu\bar{iii}}^{S1,RR} + \frac{92}{9} L_{uu\bar{iii}}^{S8,RR} \right] + e^2 \left[ \frac{128}{9} L_{uu\bar{iii}}^{S1,RR} - \frac{112}{27} L_{uu\bar{iii}}^{S8,RR} \right] \\
& + \alpha_s^2 \left[ \frac{6479}{81} L_{uu\bar{iii}}^{S8,RR} - \frac{112}{27} L_{uu\bar{iii}}^{S1,RR} \right] + \alpha_s \alpha \left[ -\frac{7360}{27} L_{uu\bar{iii}}^{S1,RR} - \frac{832}{81} L_{uu\bar{iii}}^{S8,RR} \right] \\
& + \alpha^2 \left[ \frac{18208}{729} L_{uu\bar{iii}}^{S8,RR} - \frac{11264}{243} L_{uu\bar{iii}}^{S1,RR} \right] ; \\
\dot{L}_{ij\bar{j}}^{S,RR} & = e^2 \left[ 16 L_{ij\bar{j}}^{S,RR} - 4 L_{ij\bar{j}}^{S,RR} \right] - \frac{5426}{27} \alpha^2 L_{ij\bar{j}}^{S,RR} ; \\
\dot{L}_{ij\bar{j}}^{S,RR} & = e^2 \left[ 16 L_{ij\bar{j}}^{S,RR} - 4 L_{ij\bar{j}}^{S,RR} \right] + \frac{640}{9} \alpha^2 L_{ij\bar{j}}^{S,RR} ; \\
\dot{L}_{ii\bar{iii}}^{S,RR} & = 12 e^2 L_{ii\bar{iii}}^{S,RR} - \frac{1753}{27} \alpha^2 L_{ii\bar{iii}}^{S,RR} ; \\
\dot{L}_{ij\bar{j}}^{S,LL} & = 0 ; \\
\dot{L}_{ij\bar{j}}^{S,LL} & = 0 ; \\
\dot{L}_{ii\bar{iii}}^{S,LL} & = 0 ;
\end{aligned}$$

$$\begin{aligned}
\dot{L}_{ij\bar{j}}^{V,LL} & = e^2 \left[ \frac{8}{3} L_{jj\bar{j}}^{V1,LR} + \frac{4}{3} L_{jj\bar{k}}^{V1,LR} + \frac{64}{9} L_{jj\bar{j}}^{V,LL} + \frac{8}{3} L_{jj\bar{k}}^{V,LL} + \frac{8}{9} L_{jj\bar{k}}^{V,LL} \right. \\
& + \frac{4}{3} L_{de\bar{j}}^{V,LR} + \frac{4}{3} L_{de\bar{j}}^{V,LR} + \frac{4}{3} L_{de\bar{j}}^{V,LR} - \frac{8}{3} L_{du\bar{j}}^{V1,LR} - \frac{8}{3} L_{du\bar{j}}^{V1,LR} + \frac{4}{3} L_{11\bar{j}}^{V,LL} \\
& + \frac{4}{3} L_{ed\bar{j}}^{V,LL} + \frac{4}{3} L_{ed\bar{j}}^{V,LL} + \frac{4}{9} L_{ed\bar{i}}^{V,LL} + \frac{4}{9} L_{ed\bar{i}}^{V,LL} + \frac{4}{9} L_{ed\bar{i}}^{V,LL} + 4 L_{ed\bar{i}}^{V,LL} \\
& + \frac{4}{9} L_{ed\bar{i}}^{V,LR} + \frac{4}{9} L_{ed\bar{i}}^{V,LR} + \frac{4}{9} L_{ed\bar{i}}^{V,LR} + \frac{16}{9} L_{ee\bar{iii}}^{V,LL} + \frac{16}{9} L_{ee\bar{ijj}}^{V,LL} + \frac{16}{9} L_{ee\bar{ikk}}^{V,LL} \\
& \left. + \frac{4}{9} L_{ee\bar{iii}}^{V,LR} + \frac{4}{9} L_{ee\bar{ijj}}^{V,LR} + \frac{4}{9} L_{ee\bar{ikk}}^{V,LR} - \frac{8}{9} L_{eu\bar{ii1}}^{V,LL} - \frac{8}{9} L_{eu\bar{ii2}}^{V,LL} - \frac{8}{9} L_{eu\bar{ii1}}^{V,LR} \right]
\end{aligned}$$



$$\begin{aligned}
& -\frac{8}{9}L_{ii22}^{V,LR} - \frac{8}{3}L_{11jj}^{V1,LL} - \frac{8}{3}L_{22jj}^{V1,LL} \Big] + \alpha_s^2 \Big[ 8L_{ii11}^{V,LL} + 8L_{ii22}^{V,LL} \\
& + 8L_{ii33}^{V,LL} - 8L_{ii11}^{V,LR} - 8L_{ii22}^{V,LR} - 8L_{ii33}^{V,LR} + 8L_{ii11}^{V,LL} + 8L_{ii22}^{V,LL} \\
& - 8L_{ii11}^{V,LR} - 8L_{ii22}^{V,LR} \Big] + \alpha_s \alpha \Big[ \frac{32}{3}L_{jjjj}^{V1,LR} + \frac{16}{3}L_{jjkk}^{V1,LR} - \frac{2080}{243}L_{jjjj}^{V8,LR} \\
& - \frac{1040}{243}L_{jjkk}^{V8,LR} + \frac{5008}{243}L_{jjjj}^{V,LL} + 8L_{jjkk}^{V,LL} - \frac{8}{243}L_{jjkk}^{V,LL} - \frac{32}{3}L_{jj11}^{V1,LR} - \frac{32}{3}L_{jj22}^{V1,LR} \\
& + \frac{1336}{243}L_{jj11}^{V8,LR} + \frac{1336}{243}L_{jj22}^{V8,LR} + \frac{16}{9}L_{ii11}^{V,LL} + \frac{16}{9}L_{ii22}^{V,LL} + \frac{16}{9}L_{ii33}^{V,LL} - 16L_{iijj}^{V,LL} \\
& + \frac{16}{9}L_{ii11}^{V,LR} + \frac{16}{9}L_{ii22}^{V,LR} + \frac{16}{9}L_{ii33}^{V,LR} - \frac{32}{9}L_{ii11}^{V,LL} - \frac{32}{9}L_{ii22}^{V,LL} - \frac{32}{9}L_{ii11}^{V,LR} \\
& - \frac{32}{9}L_{ii22}^{V,LR} - \frac{32}{3}L_{11jj}^{V1,LL} - \frac{32}{3}L_{22jj}^{V1,LL} - \frac{104}{243}L_{11jj}^{V8,LL} - \frac{104}{243}L_{22jj}^{V8,LL} \Big] \\
& + \alpha^2 \Big[ -\frac{2624}{243}L_{jjjj}^{V1,LR} - \frac{1312}{243}L_{jjkk}^{V1,LR} + \frac{23296}{729}L_{jjjj}^{V,LL} + \frac{1984}{243}L_{jjkk}^{V,LL} + \frac{2896}{729}L_{jjkk}^{V,LL} \\
& - \frac{3184}{243}L_{jj11}^{V,LR} - \frac{3184}{243}L_{jj22}^{V,LR} - \frac{3184}{243}L_{jj33}^{V,LR} - \frac{6232}{243}L_{jj11}^{V1,LR} - \frac{6232}{243}L_{jj22}^{V1,LR} \\
& + \frac{3728}{243}L_{jj11}^{V,LL} + \frac{3728}{243}L_{jj22}^{V,LL} + \frac{3728}{243}L_{jj33}^{V,LL} - \frac{104}{243}L_{ii11}^{V,LL} - \frac{104}{243}L_{ii22}^{V,LL} \\
& - \frac{104}{243}L_{ii33}^{V,LL} - \frac{326}{27}L_{iijj}^{V,LL} - \frac{200}{243}L_{ii11}^{V,LR} - \frac{200}{243}L_{ii22}^{V,LR} - \frac{200}{243}L_{ii33}^{V,LR} + \frac{32}{81}L_{iii}^{V,LL} \\
& + \frac{224}{81}L_{iijj}^{V,LL} + \frac{224}{81}L_{iikk}^{V,LL} - \frac{520}{81}L_{iii}^{V,LR} - \frac{520}{81}L_{iijj}^{V,LR} - \frac{520}{81}L_{iikk}^{V,LR} - \frac{1016}{243}L_{ii11}^{V,LL} \\
& - \frac{1016}{243}L_{ii22}^{V,LL} - \frac{1400}{243}L_{ii11}^{V,LR} - \frac{1400}{243}L_{ii22}^{V,LR} + \frac{2984}{243}L_{11jj}^{V1,LL} + \frac{2984}{243}L_{22jj}^{V1,LL} \Big] ;
\end{aligned}$$

$$\begin{aligned}
\dot{L}_{iijj}^{V,LL} &= e^2 \Big[ -\frac{8}{9}L_{ii11}^{V,LL} - \frac{8}{9}L_{ii22}^{V,LL} - \frac{8}{9}L_{ii33}^{V,LL} - \frac{8}{9}L_{ii11}^{V,LR} - \frac{8}{9}L_{ii22}^{V,LR} \\
& - \frac{8}{9}L_{ii33}^{V,LR} - \frac{32}{9}L_{iii}^{V,LL} - \frac{32}{9}L_{iijj}^{V,LL} - \frac{32}{9}L_{iikk}^{V,LL} - \frac{8}{9}L_{iii}^{V,LR} - \frac{8}{9}L_{iijj}^{V,LR} \\
& - \frac{8}{9}L_{iikk}^{V,LR} + \frac{4}{3}L_{11jj}^{V,LL} + \frac{4}{3}L_{22jj}^{V,LL} + \frac{4}{3}L_{33jj}^{V,LL} + \frac{16}{9}L_{ii11}^{V,LL} + \frac{16}{9}L_{ii22}^{V,LL} \\
& - 8L_{iijj}^{V,LL} + \frac{16}{9}L_{ii11}^{V,LR} + \frac{16}{9}L_{ii22}^{V,LR} + \frac{4}{3}L_{11jj}^{V1,LL} + \frac{4}{3}L_{22jj}^{V1,LL} + \frac{4}{3}L_{33jj}^{V1,LL}
\end{aligned}$$

$$\begin{aligned}
& + \frac{4}{3}L_{ud,jj11}^{V1,LR} + \frac{4}{3}L_{ud,jj22}^{V1,LR} + \frac{4}{3}L_{ud,jj33}^{V1,LR} + \frac{4}{3}L_{ue,jj11}^{V,LR} + \frac{4}{3}L_{ue,jj22}^{V,LR} + \frac{4}{3}L_{ue,jj33}^{V,LR} \\
& - \frac{8}{3}L_{uu,jjjj}^{V1,LR} - \frac{8}{3}L_{uu,jjkk}^{V1,LR} - \frac{64}{9}L_{uu,jjjj}^{V,LL} - \frac{16}{3}L_{uu,jjkk}^{V,LL} - \frac{16}{9}L_{uu,jkkj}^{V,LL} \Big] + \alpha_s^2 \Big[ 8L_{ii11}^{V,LL} \\
& + 8L_{ed,ii22}^{V,LL} + 8L_{ed,ii33}^{V,LL} - 8L_{ed,ii11}^{V,LR} - 8L_{ed,ii22}^{V,LR} - 8L_{ed,ii33}^{V,LR} + 8L_{eu,ii11}^{V,LL} \\
& + 8L_{eu,ii22}^{V,LL} - 8L_{eu,ii11}^{V,LR} - 8L_{eu,ii22}^{V,LR} \Big] + \alpha_s \alpha \Big[ -\frac{32}{9}L_{ed,ii11}^{V,LL} - \frac{32}{9}L_{ed,ii22}^{V,LL} \\
& - \frac{32}{9}L_{ed,ii33}^{V,LL} - \frac{32}{9}L_{ed,ii11}^{V,LR} - \frac{32}{9}L_{ed,ii22}^{V,LR} - \frac{32}{9}L_{ed,ii33}^{V,LR} + \frac{64}{9}L_{eu,ii11}^{V,LL} + \frac{64}{9}L_{eu,ii22}^{V,LL} \\
& + 32L_{eu,iijj}^{V,LL} + \frac{64}{9}L_{eu,ii11}^{V,LR} + \frac{64}{9}L_{eu,ii22}^{V,LR} + \frac{16}{3}L_{ud,jj11}^{V1,LL} + \frac{16}{3}L_{ud,jj22}^{V1,LL} + \frac{16}{3}L_{ud,jj33}^{V1,LL} \\
& + \frac{16}{3}L_{ud,jj11}^{V1,LR} + \frac{16}{3}L_{ud,jj22}^{V1,LR} - \frac{32}{3}L_{ud,jj33}^{V1,LR} + \frac{388}{243}L_{ud,jj11}^{V8,LL} + \frac{388}{243}L_{ud,jj22}^{V8,LL} + \frac{388}{243}L_{ud,jj33}^{V8,LL} \\
& - \frac{332}{243}L_{ud,jj11}^{V8,LR} - \frac{332}{243}L_{ud,jj22}^{V8,LR} + \frac{2044}{243}L_{ud,jj33}^{V8,LR} - \frac{32}{3}L_{uu,jjjj}^{V1,LR} - \frac{32}{3}L_{uu,jjkk}^{V1,LR} + \frac{2044}{243}L_{uu,jjjj}^{V8,LR} \\
& + \frac{2044}{243}L_{uu,jjkk}^{V8,LR} - \frac{2096}{81}L_{uu,jjjj}^{V,LL} - 16L_{uu,jjkk}^{V,LL} - \frac{128}{243}L_{uu,jkkj}^{V,LL} \Big] + \alpha^2 \Big[ \frac{2512}{243}L_{ed,ii11}^{V,LL} \\
& + \frac{2512}{243}L_{ed,ii22}^{V,LL} + \frac{2512}{243}L_{ed,ii33}^{V,LL} + \frac{1408}{243}L_{ed,ii11}^{V,LR} + \frac{1408}{243}L_{ed,ii22}^{V,LR} + \frac{1408}{243}L_{ed,ii33}^{V,LR} \\
& + \frac{3680}{81}L_{ee,iiii}^{V,LL} + \frac{2432}{81}L_{ee,iijj}^{V,LL} + \frac{2432}{81}L_{ee,ii kk}^{V,LL} + \frac{464}{81}L_{ee,iiii}^{V,LR} + \frac{464}{81}L_{ee,iijj}^{V,LR} + \frac{464}{81}L_{ee,ii kk}^{V,LR} \\
& + \frac{3248}{243}L_{eu,11jj}^{V,LL} + \frac{3248}{243}L_{eu,22jj}^{V,LL} + \frac{3248}{243}L_{eu,33jj}^{V,LL} + \frac{1312}{243}L_{eu,ii11}^{V,LL} + \frac{1312}{243}L_{eu,ii22}^{V,LL} \\
& + \frac{112}{27}L_{eu,iijj}^{V,LL} - \frac{3104}{243}L_{eu,ii11}^{V,LR} - \frac{3104}{243}L_{eu,ii22}^{V,LR} + \frac{296}{243}L_{ud,jj11}^{V1,LL} + \frac{296}{243}L_{ud,jj22}^{V1,LL} \\
& + \frac{296}{243}L_{ud,jj33}^{V1,LL} - \frac{928}{243}L_{ud,jj11}^{V1,LR} - \frac{928}{243}L_{ud,jj22}^{V1,LR} + \frac{416}{243}L_{ud,jj33}^{V1,LR} - \frac{424}{243}L_{ue,jj11}^{V,LL} \\
& - \frac{424}{243}L_{ue,jj22}^{V,LR} - \frac{424}{243}L_{ue,jj33}^{V,LR} + \frac{128}{243}L_{uu,jjjj}^{V1,LR} + \frac{128}{243}L_{uu,jjkk}^{V1,LR} + \frac{26272}{243}L_{uu,jjjj}^{V,LL} \\
& + \frac{10048}{243}L_{uu,jjkk}^{V,LL} + \frac{18304}{729}L_{uu,jkkj}^{V,LL} \Big] ;
\end{aligned}$$

$$\dot{L}_{ve,ii jj}^{V,LL} = e^2 \Big[ \frac{4}{3}L_{\nu d,ii11}^{V,LL} + \frac{4}{3}L_{\nu d,ii22}^{V,LL} + \frac{4}{3}L_{\nu d,ii33}^{V,LL} + \frac{4}{3}L_{\nu d,ii11}^{V,LR} + \frac{4}{3}L_{\nu d,ii22}^{V,LR}$$

$$\begin{aligned}
& + \frac{4}{3}L_{\nu d, i33}^{V,LR} + \frac{4}{3}L_{\nu e, i11}^{V,LL} + \frac{4}{3}L_{\nu e, i22}^{V,LL} + \frac{4}{3}L_{\nu e, i33}^{V,LL} + \frac{4}{3}L_{\nu e, i11}^{V,LR} + \frac{4}{3}L_{\nu e, i22}^{V,LR} \\
& + \frac{4}{3}L_{\nu e, i33}^{V,LR} - \frac{8}{3}L_{\nu u, i11}^{V,LL} - \frac{8}{3}L_{\nu u, i22}^{V,LL} - \frac{8}{3}L_{\nu u, i11}^{V,LR} - \frac{8}{3}L_{\nu u, i22}^{V,LR} \Big] \\
& + \alpha_s \alpha \left[ \frac{16}{3}L_{\nu d, i11}^{V,LL} + \frac{16}{3}L_{\nu d, i22}^{V,LL} + \frac{16}{3}L_{\nu d, i33}^{V,LL} + \frac{16}{3}L_{\nu d, i11}^{V,LR} + \frac{16}{3}L_{\nu d, i22}^{V,LR} \right. \\
& + \left. \frac{16}{3}L_{\nu d, i33}^{V,LR} - \frac{32}{3}L_{\nu u, i11}^{V,LL} - \frac{32}{3}L_{\nu u, i22}^{V,LL} - \frac{32}{3}L_{\nu u, i11}^{V,LR} - \frac{32}{3}L_{\nu u, i22}^{V,LR} \right] \\
& + \alpha^2 \left[ \frac{40}{9}L_{\nu d, i11}^{V,LL} + \frac{40}{9}L_{\nu d, i22}^{V,LL} + \frac{40}{9}L_{\nu d, i33}^{V,LL} - \frac{32}{9}L_{\nu d, i11}^{V,LR} - \frac{32}{9}L_{\nu d, i22}^{V,LR} \right. \\
& - \frac{32}{9}L_{\nu d, i33}^{V,LR} + 16L_{\nu e, i11}^{V,LL} + 16L_{\nu e, i22}^{V,LL} + 16L_{\nu e, i33}^{V,LL} - 8L_{\nu e, i11}^{V,LR} - 8L_{\nu e, i22}^{V,LR} \\
& - 8L_{\nu e, i33}^{V,LR} + \frac{112}{9}L_{\nu u, i11}^{V,LL} + \frac{112}{9}L_{\nu u, i22}^{V,LL} - \frac{176}{9}L_{\nu u, i11}^{V,LR} - \frac{176}{9}L_{\nu u, i22}^{V,LR} \Big] ; \\
\dot{L}_{\nu d, ij}^{V,LL} & = e^2 \left[ \frac{4}{9}L_{\nu d, i11}^{V,LL} + \frac{4}{9}L_{\nu d, i22}^{V,LL} + \frac{4}{9}L_{\nu d, i33}^{V,LL} + \frac{4}{9}L_{\nu d, i11}^{V,LR} + \frac{4}{9}L_{\nu d, i22}^{V,LR} \right. \\
& + \frac{4}{9}L_{\nu d, i33}^{V,LR} + \frac{4}{9}L_{\nu e, i11}^{V,LL} + \frac{4}{9}L_{\nu e, i22}^{V,LL} + \frac{4}{9}L_{\nu e, i33}^{V,LL} + \frac{4}{9}L_{\nu e, i11}^{V,LR} + \frac{4}{9}L_{\nu e, i22}^{V,LR} \\
& + \frac{4}{9}L_{\nu e, i33}^{V,LR} - \frac{8}{9}L_{\nu u, i11}^{V,LL} - \frac{8}{9}L_{\nu u, i22}^{V,LL} - \frac{8}{9}L_{\nu u, i11}^{V,LR} - \frac{8}{9}L_{\nu u, i22}^{V,LR} \Big] \\
& + \alpha_s^2 \left[ 8L_{\nu d, i11}^{V,LL} + 8L_{\nu d, i22}^{V,LL} + 8L_{\nu d, i33}^{V,LL} - 8L_{\nu d, i11}^{V,LR} - 8L_{\nu d, i22}^{V,LR} \right. \\
& - 8L_{\nu d, i33}^{V,LR} + 8L_{\nu u, i11}^{V,LL} + 8L_{\nu u, i22}^{V,LL} - 8L_{\nu u, i11}^{V,LR} - 8L_{\nu u, i22}^{V,LR} \Big] \\
& + \alpha_s \alpha \left[ \frac{16}{9}L_{\nu d, i11}^{V,LL} + \frac{16}{9}L_{\nu d, i22}^{V,LL} + \frac{16}{9}L_{\nu d, i33}^{V,LL} + \frac{16}{9}L_{\nu d, i11}^{V,LR} + \frac{16}{9}L_{\nu d, i22}^{V,LR} \right. \\
& + \left. \frac{16}{9}L_{\nu d, i33}^{V,LR} - \frac{32}{9}L_{\nu u, i11}^{V,LL} - \frac{32}{9}L_{\nu u, i22}^{V,LL} - \frac{32}{9}L_{\nu u, i11}^{V,LR} - \frac{32}{9}L_{\nu u, i22}^{V,LR} \right] \\
& + \alpha^2 \left[ \frac{16}{27}L_{\nu d, i11}^{V,LL} + \frac{16}{27}L_{\nu d, i22}^{V,LL} + \frac{16}{27}L_{\nu d, i33}^{V,LL} - \frac{8}{27}L_{\nu d, i11}^{V,LR} - \frac{8}{27}L_{\nu d, i22}^{V,LR} \right.
\end{aligned}$$

$$\begin{aligned}
& -\frac{8}{27}L_{\nu d, i33}^{V,LR} + \frac{8}{3}L_{\nu e, i11}^{V,LL} + \frac{8}{3}L_{\nu e, i22}^{V,LL} + \frac{8}{3}L_{\nu e, i33}^{V,LL} + \frac{16}{27}L_{\nu u, i11}^{V,LL} + \frac{16}{27}L_{\nu u, i22}^{V,LL} \\
& -\frac{80}{27}L_{\nu u, i11}^{V,LR} - \frac{80}{27}L_{\nu u, i22}^{V,LR} \Big] ; \\
\dot{L}_{\nu u, ij}^{V,LL} = & e^2 \Big[ -\frac{8}{9}L_{\nu d, i11}^{V,LL} - \frac{8}{9}L_{\nu d, i22}^{V,LL} - \frac{8}{9}L_{\nu d, i33}^{V,LL} - \frac{8}{9}L_{\nu d, i11}^{V,LR} - \frac{8}{9}L_{\nu d, i22}^{V,LR} \\
& -\frac{8}{9}L_{\nu e, i33}^{V,LR} - \frac{8}{9}L_{\nu e, i11}^{V,LL} - \frac{8}{9}L_{\nu e, i22}^{V,LL} - \frac{8}{9}L_{\nu e, i33}^{V,LL} - \frac{8}{9}L_{\nu e, i11}^{V,LR} - \frac{8}{9}L_{\nu e, i22}^{V,LR} \\
& -\frac{8}{9}L_{\nu e, i33}^{V,LR} + \frac{16}{9}L_{\nu u, i11}^{V,LL} + \frac{16}{9}L_{\nu u, i22}^{V,LL} + \frac{16}{9}L_{\nu u, i33}^{V,LL} + \frac{16}{9}L_{\nu u, i11}^{V,LR} + \frac{16}{9}L_{\nu u, i22}^{V,LR} \Big] \\
& + \alpha_s^2 \Big[ 8L_{\nu d, i11}^{V,LL} + 8L_{\nu d, i22}^{V,LL} + 8L_{\nu d, i33}^{V,LL} - 8L_{\nu d, i11}^{V,LR} - 8L_{\nu d, i22}^{V,LR} \\
& - 8L_{\nu d, i33}^{V,LR} + 8L_{\nu u, i11}^{V,LL} + 8L_{\nu u, i22}^{V,LL} - 8L_{\nu u, i11}^{V,LR} - 8L_{\nu u, i22}^{V,LR} \Big] \\
& + \alpha_s \alpha \Big[ -\frac{32}{9}L_{\nu d, i11}^{V,LL} - \frac{32}{9}L_{\nu d, i22}^{V,LL} - \frac{32}{9}L_{\nu d, i33}^{V,LL} - \frac{32}{9}L_{\nu d, i11}^{V,LR} - \frac{32}{9}L_{\nu d, i22}^{V,LR} \\
& - \frac{32}{9}L_{\nu d, i33}^{V,LR} + \frac{64}{9}L_{\nu u, i11}^{V,LL} + \frac{64}{9}L_{\nu u, i22}^{V,LL} + \frac{64}{9}L_{\nu u, i33}^{V,LL} + \frac{64}{9}L_{\nu u, i11}^{V,LR} + \frac{64}{9}L_{\nu u, i22}^{V,LR} \Big] \\
& + \alpha^2 \Big[ \frac{40}{27}L_{\nu d, i11}^{V,LL} + \frac{40}{27}L_{\nu d, i22}^{V,LL} + \frac{40}{27}L_{\nu d, i33}^{V,LL} - \frac{56}{27}L_{\nu d, i11}^{V,LR} - \frac{56}{27}L_{\nu d, i22}^{V,LR} \\
& - \frac{56}{27}L_{\nu d, i33}^{V,LR} + \frac{8}{3}L_{\nu e, i11}^{V,LL} + \frac{8}{3}L_{\nu e, i22}^{V,LL} + \frac{8}{3}L_{\nu e, i33}^{V,LL} - 8L_{\nu e, i11}^{V,LR} - 8L_{\nu e, i22}^{V,LR} \\
& - 8L_{\nu e, i33}^{V,LR} + \frac{256}{27}L_{\nu u, i11}^{V,LL} + \frac{256}{27}L_{\nu u, i22}^{V,LL} - \frac{128}{27}L_{\nu u, i11}^{V,LR} - \frac{128}{27}L_{\nu u, i22}^{V,LR} \Big] ; \\
\dot{L}_{\nu d, ij}^{V1,LL} = & \frac{8}{3}L_{\nu d, ij}^{V8,LL} g_s^2 + e^2 \Big[ -\frac{16}{9}L_{dd, jjjj}^{V1,LR} - \frac{8}{9}L_{dd, jjkk}^{V1,LR} - \frac{128}{27}L_{dd, jjjj}^{V,LL} - \frac{16}{9}L_{dd, jjkk}^{V,LL} \\
& - \frac{16}{27}L_{dd, jjkk}^{V,LL} - \frac{8}{9}L_{de, jj11}^{V,LR} - \frac{8}{9}L_{de, jj22}^{V,LR} - \frac{8}{9}L_{de, jj33}^{V,LR} + \frac{16}{9}L_{du, jj11}^{V1,LR} + \frac{16}{9}L_{du, jj22}^{V1,LR} \\
& - \frac{8}{9}L_{ed, 11jj}^{V,LL} - \frac{8}{9}L_{ed, 22jj}^{V,LL} - \frac{8}{9}L_{ed, 33jj}^{V,LL} + \frac{4}{9}L_{eu, 11ii}^{V,LL} + \frac{4}{9}L_{eu, 22ii}^{V,LL} + \frac{4}{9}L_{eu, 33ii}^{V,LL}
\end{aligned}$$

$$\begin{aligned}
& + \frac{16}{9}L_{11jj}^{V1,LL} + \frac{16}{9}L_{22jj}^{V1,LL} + \frac{4}{9}L_{ii11}^{V1,LL} + \frac{4}{9}L_{ii22}^{V1,LL} + \frac{4}{9}L_{ii33}^{V1,LL} - \frac{8}{3}L_{ijjj}^{V1,LL} \\
& + \frac{4}{9}L_{ii11}^{V1,LR} + \frac{4}{9}L_{ii22}^{V1,LR} + \frac{4}{9}L_{ii33}^{V1,LR} + \frac{4}{9}L_{ii11}^{V,LR} + \frac{4}{9}L_{ii22}^{V,LR} + \frac{4}{9}L_{ii33}^{V,LR} \\
& - \frac{8}{9}L_{iii}^{V1,LR} - \frac{8}{9}L_{ikk}^{V1,LR} - \frac{64}{27}L_{iii}^{V,LL} - \frac{16}{9}L_{ikk}^{V,LL} - \frac{16}{27}L_{ikki}^{V,LL} \Big] + \alpha_s^2 \Big[ -16L_{jjjj}^{V1,LR} \\
& - 8L_{jjkk}^{V1,LR} + \frac{8}{27}L_{jjjj}^{V8,LR} + \frac{4}{27}L_{jjkk}^{V8,LR} + \frac{1672}{27}L_{jjjj}^{V,LL} + 16L_{jjkk}^{V,LL} + \frac{256}{27}L_{jjkj}^{V,LL} \\
& - 8L_{jj11}^{V1,LR} - 8L_{jj22}^{V1,LR} + \frac{4}{27}L_{jj11}^{V8,LR} + \frac{4}{27}L_{jj22}^{V8,LR} + 8L_{11jj}^{V1,LL} + 8L_{22jj}^{V1,LL} \\
& + 8L_{ii11}^{V1,LL} + 8L_{ii22}^{V1,LL} + 8L_{ii33}^{V1,LL} - \frac{28}{3}L_{ijjj}^{V1,LL} - 8L_{ii11}^{V1,LR} - 8L_{ii22}^{V1,LR} \\
& - 8L_{ii33}^{V1,LR} + \frac{4}{27}L_{11jj}^{V8,LL} + \frac{4}{27}L_{22jj}^{V8,LL} + \frac{4}{27}L_{ii11}^{V8,LL} + \frac{4}{27}L_{ii22}^{V8,LL} + \frac{4}{27}L_{ii33}^{V8,LL} \\
& + \frac{82}{27}L_{ijjj}^{V8,LL} + \frac{4}{27}L_{ii11}^{V8,LR} + \frac{4}{27}L_{ii22}^{V8,LR} + \frac{4}{27}L_{ii33}^{V8,LR} - 8L_{iii}^{V1,LR} - 8L_{ikk}^{V1,LR} \\
& + \frac{4}{27}L_{iii}^{V8,LR} + \frac{4}{27}L_{ikk}^{V8,LR} + \frac{328}{9}L_{iii}^{V,LL} + 16L_{ikk}^{V,LL} + \frac{256}{27}L_{ikki}^{V,LL} \Big] + \alpha_s \alpha \Big[ -\frac{64}{9}L_{jjjj}^{V1,LR} \\
& - \frac{32}{9}L_{jjkk}^{V1,LR} + \frac{4160}{729}L_{jjjj}^{V8,LR} + \frac{2080}{729}L_{jjkk}^{V8,LR} - \frac{10016}{729}L_{jjjj}^{V,LL} - \frac{16}{3}L_{jjkk}^{V,LL} \\
& + \frac{16}{729}L_{jjkj}^{V,LL} + \frac{64}{9}L_{jj11}^{V1,LR} + \frac{64}{9}L_{jj22}^{V1,LR} - \frac{2672}{729}L_{jj11}^{V8,LR} - \frac{2672}{729}L_{jj22}^{V8,LR} + \frac{64}{9}L_{11jj}^{V1,LL} \\
& + \frac{64}{9}L_{22jj}^{V1,LL} + \frac{16}{9}L_{ii11}^{V1,LL} + \frac{16}{9}L_{ii22}^{V1,LL} + \frac{16}{9}L_{ii33}^{V1,LL} + \frac{64}{3}L_{ijjj}^{V1,LL} + \frac{16}{9}L_{ii11}^{V1,LR} \\
& + \frac{16}{9}L_{ii22}^{V1,LR} - \frac{32}{9}L_{ii33}^{V1,LR} + \frac{208}{729}L_{11jj}^{V8,LL} + \frac{208}{729}L_{22jj}^{V8,LL} + \frac{388}{729}L_{ii11}^{V8,LL} + \frac{388}{729}L_{ii22}^{V8,LL} \\
& + \frac{388}{729}L_{ii33}^{V8,LL} - \frac{8}{27}L_{ijjj}^{V8,LL} - \frac{332}{729}L_{ii11}^{V8,LR} - \frac{332}{729}L_{ii22}^{V8,LR} + \frac{2044}{729}L_{ii33}^{V8,LR} \\
& - \frac{32}{9}L_{iii}^{V1,LR} - \frac{32}{9}L_{ikk}^{V1,LR} + \frac{2044}{729}L_{iii}^{V8,LR} + \frac{2044}{729}L_{ikk}^{V8,LR} - \frac{2096}{243}L_{iii}^{V,LL} \\
& - \frac{16}{3}L_{ikk}^{V,LL} - \frac{128}{729}L_{ikki}^{V,LL} \Big] + \alpha^2 \Big[ -\frac{512}{729}L_{jjjj}^{V1,LR} - \frac{256}{729}L_{jjkk}^{V1,LR} + \frac{40528}{2187}L_{jjjj}^{V,LL} \\
& + \frac{3232}{729}L_{jjkk}^{V,LL} + \frac{5728}{2187}L_{jjkj}^{V,LL} - \frac{2992}{729}L_{jj11}^{V,LR} - \frac{2992}{729}L_{jj22}^{V,LR} - \frac{2992}{729}L_{jj33}^{V,LR}
\end{aligned}$$

$$\begin{aligned}
& -\frac{1216}{729}L_{jj11}^{V1,LR} - \frac{1216}{729}L_{jj22}^{V1,LR} + \frac{2624}{729}L_{11jj}^{V,LL} + \frac{2624}{729}L_{22jj}^{V,LL} + \frac{2624}{729}L_{33jj}^{V,LL} \\
& + \frac{1448}{729}L_{11ii}^{V,LL} + \frac{1448}{729}L_{22ii}^{V,LL} + \frac{1448}{729}L_{33ii}^{V,LL} + \frac{6272}{729}L_{11jj}^{V1,LL} + \frac{6272}{729}L_{22jj}^{V1,LL} \\
& - \frac{208}{729}L_{ii11}^{V1,LL} - \frac{208}{729}L_{ii22}^{V1,LL} - \frac{208}{729}L_{ii33}^{V1,LL} - \frac{128}{81}L_{ijjj}^{V1,LL} - \frac{136}{729}L_{ii11}^{V1,LR} \\
& - \frac{136}{729}L_{ii22}^{V1,LR} + \frac{2720}{729}L_{ii33}^{V1,LR} + \frac{1664}{729}L_{ii11}^{V,LR} + \frac{1664}{729}L_{ii22}^{V,LR} + \frac{1664}{729}L_{ii33}^{V,LR} \\
& + \frac{2432}{729}L_{iii}^{V1,LR} + \frac{2432}{729}L_{ikk}^{V1,LR} + \frac{11872}{729}L_{iii}^{V,LL} + \frac{4288}{729}L_{ikk}^{V,LL} + \frac{9088}{2187}L_{ikki}^{V,LL} \Big] ;
\end{aligned}$$

$$\begin{aligned}
\dot{L}_{ijj}^{V8,LL} &= g_s^2 \left[ \frac{4}{3}L_{jjjj}^{V8,LR} + \frac{2}{3}L_{jjkk}^{V8,LR} + \frac{16}{3}L_{jjjj}^{V,LL} + \frac{8}{3}L_{jjkj}^{V,LL} + \frac{2}{3}L_{jj11}^{V8,LR} \right. \\
& + \frac{2}{3}L_{jj22}^{V8,LR} + 12L_{ijjj}^{V1,LL} + \frac{2}{3}L_{11jj}^{V8,LL} + \frac{2}{3}L_{22jj}^{V8,LL} + \frac{2}{3}L_{ii11}^{V8,LL} + \frac{2}{3}L_{ii22}^{V8,LL} \\
& + \frac{2}{3}L_{ii33}^{V8,LL} - 4L_{ijjj}^{V8,LL} + \frac{2}{3}L_{ii11}^{V8,LR} + \frac{2}{3}L_{ii22}^{V8,LR} + \frac{2}{3}L_{ii33}^{V8,LR} + \frac{2}{3}L_{iii}^{V8,LR} \\
& + \frac{2}{3}L_{ikk}^{V8,LR} + \frac{8}{3}L_{iii}^{V,LL} + \frac{8}{3}L_{ikki}^{V,LL} \Big] - \frac{8}{3}L_{ijjj}^{V8,LL}e^2 + \alpha_s^2 \left[ -\frac{44}{3}L_{jjjj}^{V1,LR} \right. \\
& - \frac{22}{3}L_{jjkk}^{V1,LR} + \frac{278}{81}L_{jjjj}^{V8,LR} + \frac{139}{81}L_{jjkk}^{V8,LR} + \frac{10102}{81}L_{jjjj}^{V,LL} - \frac{28}{3}L_{jjkk}^{V,LL} + \frac{5176}{81}L_{jjkj}^{V,LL} \\
& - \frac{22}{3}L_{jj11}^{V1,LR} - \frac{22}{3}L_{jj22}^{V1,LR} + \frac{139}{81}L_{jj11}^{V8,LR} + \frac{139}{81}L_{jj22}^{V8,LR} - \frac{2}{3}L_{11jj}^{V1,LL} - \frac{2}{3}L_{22jj}^{V1,LL} \\
& - \frac{2}{3}L_{ii11}^{V1,LL} - \frac{2}{3}L_{ii22}^{V1,LL} - \frac{2}{3}L_{ii33}^{V1,LL} + \frac{41}{3}L_{ijjj}^{V1,LL} - \frac{22}{3}L_{ii11}^{V1,LR} - \frac{22}{3}L_{ii22}^{V1,LR} \\
& - \frac{22}{3}L_{ii33}^{V1,LR} + \frac{769}{81}L_{11jj}^{V8,LL} + \frac{769}{81}L_{22jj}^{V8,LL} + \frac{787}{81}L_{ii11}^{V8,LL} + \frac{787}{81}L_{ii22}^{V8,LL} + \frac{787}{81}L_{ii33}^{V8,LL} \\
& - \frac{125}{9}L_{ijjj}^{V8,LL} + \frac{157}{81}L_{ii11}^{V8,LR} + \frac{157}{81}L_{ii22}^{V8,LR} + \frac{157}{81}L_{ii33}^{V8,LR} - \frac{22}{3}L_{iii}^{V1,LR} - \frac{22}{3}L_{ikk}^{V1,LR} \\
& + \frac{157}{81}L_{iii}^{V8,LR} + \frac{157}{81}L_{ikk}^{V8,LR} + \frac{1918}{27}L_{iii}^{V,LL} - \frac{28}{3}L_{ikk}^{V,LL} + \frac{5248}{81}L_{ikki}^{V,LL} \Big] \\
& + \alpha_s \alpha \left[ -\frac{392}{81}L_{jjjj}^{V1,LR} - \frac{196}{81}L_{jjkk}^{V1,LR} + \frac{104}{27}L_{jjjj}^{V8,LR} + \frac{52}{27}L_{jjkk}^{V8,LR} - \frac{15728}{243}L_{jjjj}^{V,LL} \right. \\
& - \frac{392}{81}L_{jjkk}^{V,LL} - \frac{5096}{243}L_{jjkj}^{V,LL} - \frac{196}{81}L_{jj11}^{V,LR} - \frac{196}{81}L_{jj22}^{V,LR} - \frac{196}{81}L_{jj33}^{V,LR} + \frac{392}{81}L_{jj11}^{V1,LR}
\end{aligned}$$

$$\begin{aligned}
& + \frac{392}{81} L_{jj22}^{V1,LR} - \frac{80}{27} L_{jj11}^{V8,LR} - \frac{80}{27} L_{jj22}^{V8,LR} - \frac{196}{81} L_{11jj}^{V,LL} - \frac{196}{81} L_{22jj}^{V,LL} - \frac{196}{81} L_{33jj}^{V,LL} \\
& + \frac{284}{81} L_{11ii}^{V,LL} + \frac{284}{81} L_{22ii}^{V,LL} + \frac{284}{81} L_{33ii}^{V,LL} + \frac{392}{81} L_{11jj}^{V1,LL} + \frac{392}{81} L_{22jj}^{V1,LL} + \frac{284}{81} L_{ii11}^{V1,LL} \\
& + \frac{284}{81} L_{ii22}^{V1,LL} + \frac{284}{81} L_{ii33}^{V1,LL} - \frac{4}{3} L_{iijj}^{V1,LL} + \frac{284}{81} L_{ii11}^{V1,LR} + \frac{284}{81} L_{ii22}^{V1,LR} - \frac{496}{81} L_{ii33}^{V1,LR} \\
& + \frac{56}{9} L_{11jj}^{V8,LL} + \frac{56}{9} L_{22jj}^{V8,LL} + \frac{14}{9} L_{ii11}^{V8,LL} + \frac{14}{9} L_{ii22}^{V8,LL} + \frac{14}{9} L_{ii33}^{V8,LL} - \frac{47}{9} L_{iijj}^{V8,LL} \\
& + \frac{10}{27} L_{ii11}^{V8,LR} + \frac{10}{27} L_{ii22}^{V8,LR} + \frac{4}{27} L_{ii33}^{V8,LR} + \frac{284}{81} L_{ii11}^{V,LR} + \frac{284}{81} L_{ii22}^{V,LR} + \frac{284}{81} L_{ii33}^{V,LR} \\
& - \frac{568}{81} L_{iii}^{V1,LR} - \frac{568}{81} L_{iikk}^{V1,LR} + \frac{4}{27} L_{iii}^{V8,LR} + \frac{4}{27} L_{iikk}^{V8,LR} - \frac{4616}{81} L_{iii}^{V,LL} - \frac{1136}{81} L_{iikk}^{V,LL} \\
& - \frac{6560}{243} L_{iikki}^{V,LL} \Big] - \frac{128}{81} L_{iijj}^{V8,LL} \alpha^2 ;
\end{aligned}$$

$$\begin{aligned}
\dot{L}_{ed,jji}^{V,LL} & = e^2 \left[ \frac{4}{3} L_{iii}^{V1,LR} + \frac{4}{3} L_{ijj}^{V1,LR} + \frac{4}{3} L_{ikk}^{V1,LR} + \frac{32}{9} L_{iii}^{V,LL} + \frac{8}{3} L_{ijj}^{V,LL} \right. \\
& + \frac{8}{3} L_{ikk}^{V,LL} + \frac{8}{9} L_{ijji}^{V,LL} + \frac{8}{9} L_{ikki}^{V,LL} + \frac{4}{3} L_{ii11}^{V,LR} + \frac{4}{3} L_{ii22}^{V,LR} + \frac{4}{3} L_{ii33}^{V,LR} \\
& - \frac{8}{3} L_{ii11}^{V1,LR} - \frac{8}{3} L_{ii22}^{V1,LR} + \frac{4}{3} L_{11ii}^{V,LL} + \frac{4}{3} L_{22ii}^{V,LL} + \frac{4}{3} L_{33ii}^{V,LL} + \frac{4}{9} L_{jj11}^{V,LL} \\
& + \frac{4}{9} L_{jj22}^{V,LL} + \frac{4}{9} L_{jj33}^{V,LL} + 4 L_{jjii}^{V,LL} + \frac{4}{9} L_{jj11}^{V,LR} + \frac{4}{9} L_{jj22}^{V,LR} + \frac{4}{9} L_{jj33}^{V,LR} \\
& + \frac{8}{3} L_{jjjj}^{V,LL} + \frac{16}{9} L_{jjkk}^{V,LL} + \frac{8}{9} L_{jjjj}^{V,LR} + \frac{4}{9} L_{jjkk}^{V,LR} - \frac{8}{9} L_{jj11}^{V,LL} - \frac{8}{9} L_{jj22}^{V,LL} \\
& \left. - \frac{8}{9} L_{jj11}^{V,LR} - \frac{8}{9} L_{jj22}^{V,LR} - \frac{8}{3} L_{11ii}^{V1,LL} - \frac{8}{3} L_{22ii}^{V1,LL} \right] + \alpha_s^2 \left[ 8 L_{jj11}^{V,LL} \right. \\
& + 8 L_{jj22}^{V,LL} + 8 L_{jj33}^{V,LL} - 8 L_{jj11}^{V,LR} - 8 L_{jj22}^{V,LR} - 8 L_{jj33}^{V,LR} + 8 L_{jj11}^{V,LL} \\
& + 8 L_{jj22}^{V,LL} - 8 L_{jj11}^{V,LR} - 8 L_{jj22}^{V,LR} \Big] + \alpha_s \alpha \left[ \frac{16}{3} L_{iii}^{V1,LR} + \frac{16}{3} L_{ijj}^{V1,LR} \right. \\
& + \frac{16}{3} L_{ikk}^{V1,LR} - \frac{1040}{243} L_{iii}^{V8,LR} - \frac{1040}{243} L_{ijj}^{V8,LR} - \frac{1040}{243} L_{ikk}^{V8,LR} + \frac{1024}{81} L_{iii}^{V,LL} \\
& + 8 L_{ijj}^{V,LL} + 8 L_{ikk}^{V,LL} - \frac{8}{243} L_{ijji}^{V,LL} - \frac{8}{243} L_{ikki}^{V,LL} - \frac{32}{3} L_{ii11}^{V1,LR} - \frac{32}{3} L_{ii22}^{V1,LR}
\end{aligned}$$

$$\begin{aligned}
& + \frac{1336}{243} L_{ii11}^{V8,LR} + \frac{1336}{243} L_{ii22}^{V8,LR} + \frac{16}{9} L_{jj11}^{V,LL} + \frac{16}{9} L_{jj22}^{V,LL} + \frac{16}{9} L_{jj33}^{V,LL} - 16 L_{jjii}^{V,LL} \\
& + \frac{16}{9} L_{jj11}^{V,LR} + \frac{16}{9} L_{jj22}^{V,LR} + \frac{16}{9} L_{jj33}^{V,LR} - \frac{32}{9} L_{jj11}^{V,LL} - \frac{32}{9} L_{jj22}^{V,LL} - \frac{32}{9} L_{jj11}^{V,LR} \\
& - \frac{32}{9} L_{jj22}^{V,LR} - \frac{32}{3} L_{11ii}^{V1,LL} - \frac{32}{3} L_{22ii}^{V1,LL} - \frac{104}{243} L_{11ii}^{V8,LL} - \frac{104}{243} L_{22ii}^{V8,LL} \Big] \\
& + \alpha^2 \Bigg[ - \frac{1312}{243} L_{iiii}^{V1,LR} - \frac{1312}{243} L_{iijj}^{V1,LR} - \frac{1312}{243} L_{iikk}^{V1,LR} + \frac{4816}{243} L_{iiii}^{V,LL} + \frac{1984}{243} L_{iijj}^{V,LL} \\
& + \frac{1984}{243} L_{iikk}^{V,LL} + \frac{2896}{729} L_{ijji}^{V,LL} + \frac{2896}{729} L_{ikki}^{V,LL} - \frac{3184}{243} L_{ii11}^{V,LR} - \frac{3184}{243} L_{ii22}^{V,LR} \\
& - \frac{3184}{243} L_{ii33}^{V,LR} - \frac{6232}{243} L_{ii11}^{V1,LR} - \frac{6232}{243} L_{ii22}^{V1,LR} + \frac{3728}{243} L_{11ii}^{V,LL} + \frac{3728}{243} L_{22ii}^{V,LL} \\
& + \frac{3728}{243} L_{33ii}^{V,LL} - \frac{104}{243} L_{jj11}^{V,LL} - \frac{104}{243} L_{jj22}^{V,LL} - \frac{104}{243} L_{jj33}^{V,LL} - \frac{326}{27} L_{jjii}^{V,LL} - \frac{200}{243} L_{jj11}^{V,LR} \\
& - \frac{200}{243} L_{jj22}^{V,LR} - \frac{200}{243} L_{jj33}^{V,LR} + \frac{16}{9} L_{jjjj}^{V,LL} + \frac{224}{81} L_{jjkk}^{V,LL} - \frac{1040}{81} L_{jjjj}^{V,LR} - \frac{520}{81} L_{jjkk}^{V,LR} \\
& - \frac{1016}{243} L_{jj11}^{V,LL} - \frac{1016}{243} L_{jj22}^{V,LL} - \frac{1400}{243} L_{jj11}^{V,LR} - \frac{1400}{243} L_{jj22}^{V,LR} + \frac{2984}{243} L_{11ii}^{V1,LL} \\
& + \frac{2984}{243} L_{22ii}^{V1,LL} \Bigg] ;
\end{aligned}$$

$$\begin{aligned}
\dot{L}_{jjii}^{V,LL} & = e^2 \Bigg[ - \frac{8}{9} L_{jj11}^{V,LL} - \frac{8}{9} L_{jj22}^{V,LL} - \frac{8}{9} L_{jj33}^{V,LL} - \frac{8}{9} L_{jj11}^{V,LR} - \frac{8}{9} L_{jj22}^{V,LR} \\
& - \frac{8}{9} L_{jj33}^{V,LR} - \frac{16}{3} L_{jjjj}^{V,LL} - \frac{32}{9} L_{jjkk}^{V,LL} - \frac{16}{9} L_{jjjj}^{V,LR} - \frac{8}{9} L_{jjkk}^{V,LR} + \frac{4}{3} L_{11ii}^{V,LL} \\
& + \frac{4}{3} L_{22ii}^{V,LL} + \frac{4}{3} L_{33ii}^{V,LL} + \frac{16}{9} L_{jj11}^{V,LL} + \frac{16}{9} L_{jj22}^{V,LL} - 8 L_{jjii}^{V,LL} + \frac{16}{9} L_{jj11}^{V,LR} \\
& + \frac{16}{9} L_{jj22}^{V,LR} + \frac{4}{3} L_{11ii}^{V1,LL} + \frac{4}{3} L_{ii22}^{V1,LL} + \frac{4}{3} L_{ii33}^{V1,LL} + \frac{4}{3} L_{ii11}^{V1,LR} + \frac{4}{3} L_{ii22}^{V1,LR} \\
& + \frac{4}{3} L_{ii33}^{V1,LR} + \frac{4}{3} L_{ii11}^{V,LR} + \frac{4}{3} L_{ii22}^{V,LR} + \frac{4}{3} L_{ii33}^{V,LR} - \frac{8}{3} L_{ii11}^{V1,LR} - \frac{8}{3} L_{ii22}^{V1,LR} \\
& - \frac{64}{9} L_{ii11}^{V,LL} - \frac{16}{3} L_{ii22}^{V,LL} - \frac{16}{9} L_{ii33}^{V,LL} \Bigg] + \alpha_s^2 \Bigg[ 8 L_{jj11}^{V,LL} + 8 L_{jj22}^{V,LL} \\
& + 8 L_{jj33}^{V,LL} - 8 L_{jj11}^{V,LR} - 8 L_{jj22}^{V,LR} - 8 L_{jj33}^{V,LR} + 8 L_{jj11}^{V,LL} + 8 L_{jj22}^{V,LL}
\end{aligned}$$



$$\begin{aligned}
& -8L_{jj11}^{V,LR} - 8L_{jj22}^{V,LR} \Big] + \alpha_s \alpha \Bigg[ -\frac{32}{9}L_{jj11}^{V,LL} - \frac{32}{9}L_{jj22}^{V,LL} - \frac{32}{9}L_{jj33}^{V,LL} \\
& -\frac{32}{9}L_{jj11}^{V,LR} - \frac{32}{9}L_{jj22}^{V,LR} - \frac{32}{9}L_{jj33}^{V,LR} + \frac{64}{9}L_{jj11}^{V,LL} + \frac{64}{9}L_{jj22}^{V,LL} + 32L_{jjii}^{V,LL} \\
& + \frac{64}{9}L_{jj11}^{V,LR} + \frac{64}{9}L_{jj22}^{V,LR} + \frac{16}{3}L_{ud11}^{V1,LL} + \frac{16}{3}L_{ud22}^{V1,LL} + \frac{16}{3}L_{ud33}^{V1,LL} + \frac{16}{3}L_{ud11}^{V1,LR} \\
& + \frac{16}{3}L_{ud22}^{V1,LR} - \frac{32}{3}L_{ud33}^{V1,LR} + \frac{388}{243}L_{ud11}^{V8,LL} + \frac{388}{243}L_{ud22}^{V8,LL} + \frac{388}{243}L_{ud33}^{V8,LL} - \frac{332}{243}L_{ud11}^{V8,LR} \\
& - \frac{332}{243}L_{ud22}^{V8,LR} + \frac{2044}{243}L_{ud33}^{V8,LR} - \frac{32}{3}L_{uu11}^{V1,LR} - \frac{32}{3}L_{uu22}^{V1,LR} + \frac{2044}{243}L_{uu33}^{V8,LR} \\
& + \frac{2044}{243}L_{uu11}^{V8,LR} - \frac{2096}{81}L_{uu33}^{V,LL} - 16L_{uukk}^{V,LL} - \frac{128}{243}L_{ikki}^{V,LL} \Big] + \alpha^2 \Bigg[ \frac{2512}{243}L_{jj11}^{V,LL} \\
& + \frac{2512}{243}L_{jj22}^{V,LL} + \frac{2512}{243}L_{jj33}^{V,LL} + \frac{1408}{243}L_{jj11}^{V,LR} + \frac{1408}{243}L_{jj22}^{V,LR} + \frac{1408}{243}L_{jj33}^{V,LR} \\
& + \frac{544}{9}L_{jjjj}^{V,LL} + \frac{2432}{81}L_{jjkk}^{V,LL} + \frac{928}{81}L_{jjjj}^{V,LR} + \frac{464}{81}L_{jjkk}^{V,LR} + \frac{3248}{243}L_{11ii}^{V,LL} + \frac{3248}{243}L_{22ii}^{V,LL} \\
& + \frac{3248}{243}L_{33ii}^{V,LL} + \frac{1312}{243}L_{jj11}^{V,LL} + \frac{1312}{243}L_{jj22}^{V,LL} + \frac{112}{27}L_{jjii}^{V,LL} - \frac{3104}{243}L_{jj11}^{V,LR} \\
& - \frac{3104}{243}L_{jj22}^{V,LR} + \frac{296}{243}L_{ud11}^{V1,LL} + \frac{296}{243}L_{ud22}^{V1,LL} + \frac{296}{243}L_{ud33}^{V1,LL} - \frac{928}{243}L_{ud11}^{V1,LR} \\
& - \frac{928}{243}L_{ud22}^{V1,LR} + \frac{416}{243}L_{ud33}^{V1,LR} - \frac{424}{243}L_{ue11}^{V,LR} - \frac{424}{243}L_{ue22}^{V,LR} - \frac{424}{243}L_{ue33}^{V,LR} \\
& + \frac{128}{243}L_{uu11}^{V1,LR} + \frac{128}{243}L_{uu22}^{V1,LR} + \frac{26272}{243}L_{uu33}^{V,LL} + \frac{10048}{243}L_{uukk}^{V,LL} + \frac{18304}{729}L_{ikki}^{V,LL} \Big] ;
\end{aligned}$$

$$\begin{aligned}
\dot{L}_{jjii}^{V,LL} &= e^2 \Bigg[ \frac{4}{3}L_{jj11}^{V,LL} + \frac{4}{3}L_{jj22}^{V,LL} + \frac{4}{3}L_{jj33}^{V,LL} + \frac{4}{3}L_{jj11}^{V,LR} + \frac{4}{3}L_{jj22}^{V,LR} \\
& + \frac{4}{3}L_{jj33}^{V,LR} + \frac{4}{3}L_{jj11}^{V,LL} + \frac{4}{3}L_{jj22}^{V,LL} + \frac{4}{3}L_{jj33}^{V,LL} + \frac{4}{3}L_{jj11}^{V,LR} + \frac{4}{3}L_{jj22}^{V,LR} \\
& + \frac{4}{3}L_{jj33}^{V,LR} - \frac{8}{3}L_{jj11}^{V,LL} - \frac{8}{3}L_{jj22}^{V,LL} - \frac{8}{3}L_{jj11}^{V,LR} - \frac{8}{3}L_{jj22}^{V,LR} \Big] \\
& + \alpha_s \alpha \Bigg[ \frac{16}{3}L_{jj11}^{V,LL} + \frac{16}{3}L_{jj22}^{V,LL} + \frac{16}{3}L_{jj33}^{V,LL} + \frac{16}{3}L_{jj11}^{V,LR} + \frac{16}{3}L_{jj22}^{V,LR}
\end{aligned}$$

$$\begin{aligned}
& + \frac{16}{3} L_{jj33}^{V,LR} - \frac{32}{3} L_{jj11}^{V,LL} - \frac{32}{3} L_{jj22}^{V,LL} - \frac{32}{3} L_{jj11}^{V,LR} - \frac{32}{3} L_{jj22}^{V,LR} \Big] \\
& + \alpha^2 \left[ \frac{40}{9} L_{jj11}^{V,LL} + \frac{40}{9} L_{jj22}^{V,LL} + \frac{40}{9} L_{jj33}^{V,LL} - \frac{32}{9} L_{jj11}^{V,LR} - \frac{32}{9} L_{jj22}^{V,LR} \right. \\
& - \frac{32}{9} L_{jj33}^{V,LR} + 16 L_{jj11}^{V,LL} + 16 L_{jj22}^{V,LL} + 16 L_{jj33}^{V,LL} - 8 L_{jj11}^{V,LR} - 8 L_{jj22}^{V,LR} \\
& \left. - 8 L_{jj33}^{V,LR} + \frac{112}{9} L_{jj11}^{V,LL} + \frac{112}{9} L_{jj22}^{V,LL} - \frac{176}{9} L_{jj11}^{V,LR} - \frac{176}{9} L_{jj22}^{V,LR} \right] ; \\
\dot{L}_{jj\ddot{i}}^{V,LL} & = e^2 \left[ \frac{4}{9} L_{jj11}^{V,LL} + \frac{4}{9} L_{jj22}^{V,LL} + \frac{4}{9} L_{jj33}^{V,LL} + \frac{4}{9} L_{jj11}^{V,LR} + \frac{4}{9} L_{jj22}^{V,LR} \right. \\
& + \frac{4}{9} L_{jj33}^{V,LR} + \frac{4}{9} L_{jj11}^{V,LL} + \frac{4}{9} L_{jj22}^{V,LL} + \frac{4}{9} L_{jj33}^{V,LL} + \frac{4}{9} L_{jj11}^{V,LR} + \frac{4}{9} L_{jj22}^{V,LR} \\
& \left. + \frac{4}{9} L_{jj33}^{V,LR} - \frac{8}{9} L_{jj11}^{V,LL} - \frac{8}{9} L_{jj22}^{V,LL} - \frac{8}{9} L_{jj11}^{V,LR} - \frac{8}{9} L_{jj22}^{V,LR} \right] \\
& + \alpha_s^2 \left[ 8 L_{jj11}^{V,LL} + 8 L_{jj22}^{V,LL} + 8 L_{jj33}^{V,LL} - 8 L_{jj11}^{V,LR} - 8 L_{jj22}^{V,LR} \right. \\
& \left. - 8 L_{jj33}^{V,LR} + 8 L_{jj11}^{V,LL} + 8 L_{jj22}^{V,LL} - 8 L_{jj11}^{V,LR} - 8 L_{jj22}^{V,LR} \right] \\
& + \alpha_s \alpha \left[ \frac{16}{9} L_{jj11}^{V,LL} + \frac{16}{9} L_{jj22}^{V,LL} + \frac{16}{9} L_{jj33}^{V,LL} + \frac{16}{9} L_{jj11}^{V,LR} + \frac{16}{9} L_{jj22}^{V,LR} \right. \\
& \left. + \frac{16}{9} L_{jj33}^{V,LR} - \frac{32}{9} L_{jj11}^{V,LL} - \frac{32}{9} L_{jj22}^{V,LL} - \frac{32}{9} L_{jj11}^{V,LR} - \frac{32}{9} L_{jj22}^{V,LR} \right] \\
& + \alpha^2 \left[ \frac{16}{27} L_{jj11}^{V,LL} + \frac{16}{27} L_{jj22}^{V,LL} + \frac{16}{27} L_{jj33}^{V,LL} - \frac{8}{27} L_{jj11}^{V,LR} - \frac{8}{27} L_{jj22}^{V,LR} \right. \\
& - \frac{8}{27} L_{jj33}^{V,LR} + \frac{8}{3} L_{jj11}^{V,LL} + \frac{8}{3} L_{jj22}^{V,LL} + \frac{8}{3} L_{jj33}^{V,LL} + \frac{16}{27} L_{jj11}^{V,LL} + \frac{16}{27} L_{jj22}^{V,LL} \\
& \left. - \frac{80}{27} L_{jj11}^{V,LR} - \frac{80}{27} L_{jj22}^{V,LR} \right] ; \\
\dot{L}_{jj\ddot{u}}^{V,LL} & = e^2 \left[ -\frac{8}{9} L_{jj11}^{V,LL} - \frac{8}{9} L_{jj22}^{V,LL} - \frac{8}{9} L_{jj33}^{V,LL} - \frac{8}{9} L_{jj11}^{V,LR} - \frac{8}{9} L_{jj22}^{V,LR} \right.
\end{aligned}$$

$$\begin{aligned}
& -\frac{8}{9}L_{jj33}^{V,LR} - \frac{8}{9}L_{jj11}^{V,LL} - \frac{8}{9}L_{jj22}^{V,LL} - \frac{8}{9}L_{jj33}^{V,LL} - \frac{8}{9}L_{jj11}^{V,LR} - \frac{8}{9}L_{jj22}^{V,LR} \\
& - \frac{8}{9}L_{jj33}^{V,LR} + \frac{16}{9}L_{jj11}^{V,LL} + \frac{16}{9}L_{jj22}^{V,LL} + \frac{16}{9}L_{jj11}^{V,LR} + \frac{16}{9}L_{jj22}^{V,LR} \Big] \\
& + \alpha_s^2 \Big[ 8L_{jj11}^{V,LL} + 8L_{jj22}^{V,LL} + 8L_{jj33}^{V,LL} - 8L_{jj11}^{V,LR} - 8L_{jj22}^{V,LR} \\
& - 8L_{jj33}^{V,LR} + 8L_{jj11}^{V,LL} + 8L_{jj22}^{V,LL} - 8L_{jj11}^{V,LR} - 8L_{jj22}^{V,LR} \Big] \\
& + \alpha_s \alpha \Big[ -\frac{32}{9}L_{jj11}^{V,LL} - \frac{32}{9}L_{jj22}^{V,LL} - \frac{32}{9}L_{jj33}^{V,LL} - \frac{32}{9}L_{jj11}^{V,LR} - \frac{32}{9}L_{jj22}^{V,LR} \\
& - \frac{32}{9}L_{jj33}^{V,LR} + \frac{64}{9}L_{jj11}^{V,LL} + \frac{64}{9}L_{jj22}^{V,LL} + \frac{64}{9}L_{jj11}^{V,LR} + \frac{64}{9}L_{jj22}^{V,LR} \Big] \\
& + \alpha^2 \Big[ \frac{40}{27}L_{jj11}^{V,LL} + \frac{40}{27}L_{jj22}^{V,LL} + \frac{40}{27}L_{jj33}^{V,LL} - \frac{56}{27}L_{jj11}^{V,LR} - \frac{56}{27}L_{jj22}^{V,LR} \\
& - \frac{56}{27}L_{jj33}^{V,LR} + \frac{8}{3}L_{jj11}^{V,LL} + \frac{8}{3}L_{jj22}^{V,LL} + \frac{8}{3}L_{jj33}^{V,LL} - 8L_{jj11}^{V,LR} - 8L_{jj22}^{V,LR} \\
& - 8L_{jj33}^{V,LR} + \frac{256}{27}L_{jj11}^{V,LL} + \frac{256}{27}L_{jj22}^{V,LL} - \frac{128}{27}L_{jj11}^{V,LR} - \frac{128}{27}L_{jj22}^{V,LR} \Big] ;
\end{aligned}$$

$$\begin{aligned}
\dot{L}_{jj\dot{ii}}^{V1,LL} &= \frac{8}{3}L_{jj\dot{ii}}^{V8,LL}g_s^2 + e^2 \Big[ -\frac{8}{9}L_{\dot{iii}}^{V1,LR} - \frac{8}{9}L_{\dot{ij}j}^{V1,LR} - \frac{8}{9}L_{\dot{ikk}}^{V1,LR} - \frac{64}{27}L_{\dot{iii}}^{V,LL} \\
& - \frac{16}{9}L_{\dot{ij}j}^{V,LL} - \frac{16}{9}L_{\dot{ikk}}^{V,LL} - \frac{16}{27}L_{\dot{ij}ji}^{V,LL} - \frac{16}{27}L_{\dot{ikki}}^{V,LL} - \frac{8}{9}L_{\dot{ii}11}^{V,LR} - \frac{8}{9}L_{\dot{ii}22}^{V,LR} \\
& - \frac{8}{9}L_{\dot{ii}33}^{V,LR} + \frac{16}{9}L_{\dot{ii}11}^{V1,LR} + \frac{16}{9}L_{\dot{ii}22}^{V1,LR} - \frac{8}{9}L_{\dot{ii}11}^{V,LL} - \frac{8}{9}L_{\dot{ii}22}^{V,LL} - \frac{8}{9}L_{\dot{ii}33}^{V,LL} \\
& + \frac{4}{9}L_{\dot{ii}jj}^{V,LL} + \frac{4}{9}L_{\dot{ii}jj}^{V,LL} + \frac{4}{9}L_{\dot{ii}jj}^{V,LL} + \frac{16}{9}L_{\dot{ii}jj}^{V1,LL} + \frac{16}{9}L_{\dot{ii}jj}^{V1,LL} + \frac{4}{9}L_{\dot{ii}jj}^{V1,LL} \\
& + \frac{4}{9}L_{\dot{ii}jj}^{V1,LL} + \frac{4}{9}L_{\dot{ii}jj}^{V1,LL} - \frac{8}{3}L_{\dot{ii}jj}^{V1,LL} + \frac{4}{9}L_{\dot{ii}jj}^{V1,LR} + \frac{4}{9}L_{\dot{ii}jj}^{V1,LR} + \frac{4}{9}L_{\dot{ii}jj}^{V1,LR} \\
& + \frac{4}{9}L_{\dot{ii}jj}^{V,LR} + \frac{4}{9}L_{\dot{ii}jj}^{V,LR} + \frac{4}{9}L_{\dot{ii}jj}^{V,LR} - \frac{8}{9}L_{\dot{ii}jj}^{V1,LR} - \frac{8}{9}L_{\dot{ii}jj}^{V1,LR} - \frac{64}{27}L_{\dot{ii}jj}^{V,LL} \\
& - \frac{16}{9}L_{\dot{ii}jj}^{V,LL} - \frac{16}{27}L_{\dot{ii}jj}^{V,LL} \Big] + \alpha_s^2 \Big[ -8L_{\dot{iii}}^{V1,LR} - 8L_{\dot{ij}j}^{V1,LR} - 8L_{\dot{ikk}}^{V1,LR}
\end{aligned}$$

$$\begin{aligned}
& + \frac{4}{27} L_{\ddot{iii}}^{V8,LR} + \frac{4}{27} L_{\ddot{ijj}}^{V8,LR} + \frac{4}{27} L_{\ddot{ikk}}^{V8,LR} + \frac{328}{9} L_{\ddot{iii}}^{V,LL} + 16 L_{\ddot{ijj}}^{V,LL} + 16 L_{\ddot{ikk}}^{V,LL} \\
& + \frac{256}{27} L_{\ddot{ijji}}^{V,LL} + \frac{256}{27} L_{\ddot{ikki}}^{V,LL} - 8 L_{\ddot{ii11}}^{V1,LR} - 8 L_{\ddot{ii22}}^{V1,LR} + \frac{4}{27} L_{\ddot{ii11}}^{V8,LR} + \frac{4}{27} L_{\ddot{ii22}}^{V8,LR} \\
& + 8 L_{\ddot{11ii}}^{V1,LL} + 8 L_{\ddot{22ii}}^{V1,LL} + 8 L_{\ddot{jj11}}^{V1,LL} + 8 L_{\ddot{jj22}}^{V1,LL} + 8 L_{\ddot{jj33}}^{V1,LL} - \frac{28}{3} L_{\ddot{jjii}}^{V1,LL} \\
& - 8 L_{\ddot{jj11}}^{V1,LR} - 8 L_{\ddot{jj22}}^{V1,LR} - 8 L_{\ddot{jj33}}^{V1,LR} + \frac{4}{27} L_{\ddot{11ii}}^{V8,LL} + \frac{4}{27} L_{\ddot{22ii}}^{V8,LL} + \frac{4}{27} L_{\ddot{jj11}}^{V8,LL} \\
& + \frac{4}{27} L_{\ddot{jj22}}^{V8,LL} + \frac{4}{27} L_{\ddot{jj33}}^{V8,LL} + \frac{82}{27} L_{\ddot{jjii}}^{V8,LL} + \frac{4}{27} L_{\ddot{jj11}}^{V8,LR} + \frac{4}{27} L_{\ddot{jj22}}^{V8,LR} + \frac{4}{27} L_{\ddot{jj33}}^{V8,LR} \\
& - 8 L_{\ddot{jjjj}}^{V1,LR} - 8 L_{\ddot{jjkk}}^{V1,LR} + \frac{4}{27} L_{\ddot{jjjj}}^{V8,LR} + \frac{4}{27} L_{\ddot{jjkk}}^{V8,LR} + \frac{328}{9} L_{\ddot{jjjj}}^{V,LL} + 16 L_{\ddot{jjkk}}^{V,LL} \\
& + \frac{256}{27} L_{\ddot{jjkj}}^{V,LL} \Big] + \alpha_s \alpha \Bigg[ - \frac{32}{9} L_{\ddot{iii}}^{V1,LR} - \frac{32}{9} L_{\ddot{ijj}}^{V1,LR} - \frac{32}{9} L_{\ddot{ikk}}^{V1,LR} + \frac{2080}{729} L_{\ddot{dd}}^{V8,LR} \\
& + \frac{2080}{729} L_{\ddot{ijj}}^{V8,LR} + \frac{2080}{729} L_{\ddot{ikk}}^{V8,LR} - \frac{2048}{243} L_{\ddot{iii}}^{V,LL} - \frac{16}{3} L_{\ddot{ijj}}^{V,LL} - \frac{16}{3} L_{\ddot{ikk}}^{V,LL} + \frac{16}{729} L_{\ddot{ijji}}^{V,LL} \\
& + \frac{16}{729} L_{\ddot{ikki}}^{V,LL} + \frac{64}{9} L_{\ddot{ii11}}^{V1,LR} + \frac{64}{9} L_{\ddot{ii22}}^{V1,LR} - \frac{2672}{729} L_{\ddot{ii11}}^{V8,LR} - \frac{2672}{729} L_{\ddot{ii22}}^{V8,LR} + \frac{64}{9} L_{\ddot{11ii}}^{V1,LL} \\
& + \frac{64}{9} L_{\ddot{22ii}}^{V1,LL} + \frac{16}{9} L_{\ddot{jj11}}^{V1,LL} + \frac{16}{9} L_{\ddot{jj22}}^{V1,LL} + \frac{16}{9} L_{\ddot{jj33}}^{V1,LL} + \frac{64}{3} L_{\ddot{jjii}}^{V1,LL} + \frac{16}{9} L_{\ddot{jj11}}^{V1,LR} \\
& + \frac{16}{9} L_{\ddot{jj22}}^{V1,LR} - \frac{32}{9} L_{\ddot{jj33}}^{V1,LR} + \frac{208}{729} L_{\ddot{11ii}}^{V8,LL} + \frac{208}{729} L_{\ddot{22ii}}^{V8,LL} + \frac{388}{729} L_{\ddot{jj11}}^{V8,LL} + \frac{388}{729} L_{\ddot{jj22}}^{V8,LL} \\
& + \frac{388}{729} L_{\ddot{jj33}}^{V8,LL} - \frac{8}{27} L_{\ddot{jjii}}^{V8,LL} - \frac{332}{729} L_{\ddot{jj11}}^{V8,LR} - \frac{332}{729} L_{\ddot{jj22}}^{V8,LR} + \frac{2044}{729} L_{\ddot{jj33}}^{V8,LR} \\
& - \frac{32}{9} L_{\ddot{jjjj}}^{V1,LR} - \frac{32}{9} L_{\ddot{jjkk}}^{V1,LR} + \frac{2044}{729} L_{\ddot{jjjj}}^{V8,LR} + \frac{2044}{729} L_{\ddot{jjkk}}^{V8,LR} - \frac{2096}{243} L_{\ddot{jjjj}}^{V,LL} \\
& - \frac{16}{3} L_{\ddot{jjkk}}^{V,LL} - \frac{128}{729} L_{\ddot{jjkj}}^{V,LL} \Big] + \alpha^2 \Bigg[ - \frac{256}{729} L_{\ddot{iii}}^{V1,LR} - \frac{256}{729} L_{\ddot{ijj}}^{V1,LR} - \frac{256}{729} L_{\ddot{ikk}}^{V1,LR} \\
& + \frac{8368}{729} L_{\ddot{iii}}^{V,LL} + \frac{3232}{729} L_{\ddot{ijj}}^{V,LL} + \frac{3232}{729} L_{\ddot{ikk}}^{V,LL} + \frac{5728}{2187} L_{\ddot{ijji}}^{V,LL} + \frac{5728}{2187} L_{\ddot{ikki}}^{V,LL} \\
& - \frac{2992}{729} L_{\ddot{ii11}}^{V,LR} - \frac{2992}{729} L_{\ddot{ii22}}^{V,LR} - \frac{2992}{729} L_{\ddot{ii33}}^{V,LR} - \frac{1216}{729} L_{\ddot{ii11}}^{V1,LR} - \frac{1216}{729} L_{\ddot{ii22}}^{V1,LR} \\
& + \frac{2624}{729} L_{\ddot{11ii}}^{V,LL} + \frac{2624}{729} L_{\ddot{22ii}}^{V,LL} + \frac{2624}{729} L_{\ddot{33ii}}^{V,LL} + \frac{1448}{729} L_{\ddot{11jj}}^{V,LL} + \frac{1448}{729} L_{\ddot{22jj}}^{V,LL} \\
& + \frac{1448}{729} L_{\ddot{33jj}}^{V,LL} + \frac{6272}{729} L_{\ddot{11ii}}^{V1,LL} + \frac{6272}{729} L_{\ddot{22ii}}^{V1,LL} - \frac{208}{729} L_{\ddot{jj11}}^{V1,LL} - \frac{208}{729} L_{\ddot{jj22}}^{V1,LL}
\end{aligned}$$

$$\begin{aligned}
& -\frac{208}{729}L_{jj33}^{V1,LL} - \frac{128}{81}L_{jji}^{V1,LL} - \frac{136}{729}L_{jj11}^{V1,LR} - \frac{136}{729}L_{jj22}^{V1,LR} + \frac{2720}{729}L_{jj33}^{V1,LR} \\
& + \frac{1664}{729}L_{jj11}^{V,LR} + \frac{1664}{729}L_{jj22}^{V,LR} + \frac{1664}{729}L_{jj33}^{V,LR} + \frac{2432}{729}L_{jjjj}^{V1,LR} + \frac{2432}{729}L_{jjkk}^{V1,LR} \\
& + \frac{11872}{729}L_{jjjj}^{V,LL} + \frac{4288}{729}L_{jjkk}^{V,LL} + \frac{9088}{2187}L_{jjkj}^{V,LL} \Big] ;
\end{aligned}$$

$$\begin{aligned}
\dot{L}_{jj\dot{u}}^{V8,LL} &= g_s^2 \left[ \frac{2}{3}L_{iii}^{V8,LR} + \frac{2}{3}L_{ijj}^{V8,LR} + \frac{2}{3}L_{ikk}^{V8,LR} + \frac{8}{3}L_{iii}^{V,LL} + \frac{8}{3}L_{ijj}^{V,LL} \right. \\
& + \frac{8}{3}L_{ikki}^{V,LL} + \frac{2}{3}L_{ii11}^{V8,LR} + \frac{2}{3}L_{ii22}^{V8,LR} + 12L_{jjii}^{V1,LL} + \frac{2}{3}L_{11ii}^{V8,LL} + \frac{2}{3}L_{22ii}^{V8,LL} \\
& + \frac{2}{3}L_{jj11}^{V8,LL} + \frac{2}{3}L_{jj22}^{V8,LL} + \frac{2}{3}L_{jj33}^{V8,LL} - 4L_{jjii}^{V8,LL} + \frac{2}{3}L_{jj11}^{V8,LR} + \frac{2}{3}L_{jj22}^{V8,LR} \\
& \left. + \frac{2}{3}L_{jj33}^{V8,LR} + \frac{2}{3}L_{jjjj}^{V8,LR} + \frac{2}{3}L_{jjkk}^{V8,LR} + \frac{8}{3}L_{jjjj}^{V,LL} + \frac{8}{3}L_{jjkj}^{V,LL} \right] - \frac{8}{3}L_{jjii}^{V8,LL} \\
& e^2 + \alpha_s^2 \left[ -\frac{22}{3}L_{iii}^{V1,LR} - \frac{22}{3}L_{ijj}^{V1,LR} - \frac{22}{3}L_{ikk}^{V1,LR} + \frac{139}{81}L_{iii}^{V8,LR} + \frac{139}{81}L_{ijj}^{V8,LR} \right. \\
& + \frac{139}{81}L_{ikk}^{V8,LR} + \frac{1894}{27}L_{iii}^{V,LL} - \frac{28}{3}L_{ijj}^{V,LL} - \frac{28}{3}L_{ikk}^{V,LL} + \frac{5176}{81}L_{ijji}^{V,LL} + \frac{5176}{81}L_{ikki}^{V,LL} \\
& - \frac{22}{3}L_{ii11}^{V1,LR} - \frac{22}{3}L_{ii22}^{V1,LR} + \frac{139}{81}L_{ii11}^{V8,LR} + \frac{139}{81}L_{ii22}^{V8,LR} - \frac{2}{3}L_{11ii}^{V1,LL} - \frac{2}{3}L_{22ii}^{V1,LL} \\
& - \frac{2}{3}L_{jj11}^{V1,LL} - \frac{2}{3}L_{jj22}^{V1,LL} - \frac{2}{3}L_{jj33}^{V1,LL} + \frac{41}{3}L_{jjii}^{V1,LL} - \frac{22}{3}L_{jj11}^{V1,LR} - \frac{22}{3}L_{jj22}^{V1,LR} \\
& - \frac{22}{3}L_{jj33}^{V1,LR} + \frac{769}{81}L_{11ii}^{V8,LL} + \frac{769}{81}L_{22ii}^{V8,LL} + \frac{787}{81}L_{jj11}^{V8,LL} + \frac{787}{81}L_{jj22}^{V8,LL} + \frac{787}{81}L_{jj33}^{V8,LL} \\
& - \frac{125}{9}L_{jjii}^{V8,LL} + \frac{157}{81}L_{jj11}^{V8,LR} + \frac{157}{81}L_{jj22}^{V8,LR} + \frac{157}{81}L_{jj33}^{V8,LR} - \frac{22}{3}L_{jjjj}^{V1,LR} - \frac{22}{3}L_{jjkk}^{V1,LR} \\
& \left. + \frac{157}{81}L_{jjjj}^{V8,LR} + \frac{157}{81}L_{jjkk}^{V8,LR} + \frac{1918}{27}L_{jjjj}^{V,LL} - \frac{28}{3}L_{jjkk}^{V,LL} + \frac{5248}{81}L_{jjkj}^{V,LL} \right] \\
& + \alpha_s \alpha \left[ -\frac{196}{81}L_{iii}^{V1,LR} - \frac{196}{81}L_{ijj}^{V1,LR} - \frac{196}{81}L_{ikk}^{V1,LR} + \frac{52}{27}L_{iii}^{V8,LR} + \frac{52}{27}L_{ijj}^{V8,LR} \right. \\
& \left. + \frac{52}{27}L_{ikk}^{V8,LR} - \frac{3152}{81}L_{iii}^{V,LL} - \frac{392}{81}L_{ijj}^{V,LL} - \frac{392}{81}L_{ikk}^{V,LL} - \frac{5096}{243}L_{ijji}^{V,LL} - \frac{5096}{243}L_{ikki}^{V,LL} \right]
\end{aligned}$$

$$\begin{aligned}
& -\frac{196}{81}L_{ii11}^{V,LR} - \frac{196}{81}L_{ii22}^{V,LR} - \frac{196}{81}L_{ii33}^{V,LR} + \frac{392}{81}L_{ii11}^{V1,LR} + \frac{392}{81}L_{ii22}^{V1,LR} - \frac{80}{27}L_{ii11}^{V8,LR} \\
& - \frac{80}{27}L_{ii22}^{V8,LR} - \frac{196}{81}L_{11ii}^{V,LL} - \frac{196}{81}L_{22ii}^{V,LL} - \frac{196}{81}L_{33ii}^{V,LL} + \frac{284}{81}L_{11jj}^{V,LL} + \frac{284}{81}L_{22jj}^{V,LL} \\
& + \frac{284}{81}L_{33jj}^{V,LL} + \frac{392}{81}L_{11ii}^{V1,LL} + \frac{392}{81}L_{22ii}^{V1,LL} + \frac{284}{81}L_{jj11}^{V1,LL} + \frac{284}{81}L_{jj22}^{V1,LL} + \frac{284}{81}L_{jj33}^{V1,LL} \\
& - \frac{4}{3}L_{jjii}^{V1,LL} + \frac{284}{81}L_{jj11}^{V1,LR} + \frac{284}{81}L_{jj22}^{V1,LR} - \frac{496}{81}L_{jj33}^{V1,LR} + \frac{56}{9}L_{11ii}^{V8,LL} + \frac{56}{9}L_{22ii}^{V8,LL} \\
& + \frac{14}{9}L_{jj11}^{V8,LL} + \frac{14}{9}L_{jj22}^{V8,LL} + \frac{14}{9}L_{jj33}^{V8,LL} - \frac{47}{9}L_{jjii}^{V8,LL} + \frac{10}{27}L_{jj11}^{V8,LR} + \frac{10}{27}L_{jj22}^{V8,LR} \\
& + \frac{4}{27}L_{jj33}^{V8,LR} + \frac{284}{81}L_{jj11}^{V,LR} + \frac{284}{81}L_{jj22}^{V,LR} + \frac{284}{81}L_{jj33}^{V,LR} - \frac{568}{81}L_{jjjj}^{V1,LR} - \frac{568}{81}L_{jjkk}^{V1,LR} \\
& + \frac{4}{27}L_{jjjj}^{V8,LR} + \frac{4}{27}L_{jjkk}^{V8,LR} - \frac{4616}{81}L_{jjjj}^{V,LL} - \frac{1136}{81}L_{jjkk}^{V,LL} - \frac{6560}{243}L_{jjkk}^{V,LL} \Big] \\
& - \frac{128}{81}L_{jjii}^{V8,LL}\alpha^2;
\end{aligned}$$

$$\begin{aligned}
\dot{L}_{dd\,ijj}^{V,LL} &= g_s^2 \left[ -\frac{1}{18}L_{iii}^{V8,LR} - \frac{1}{18}L_{ijj}^{V8,LR} - \frac{1}{18}L_{ikk}^{V8,LR} - \frac{1}{9}L_{jjjj}^{V8,LR} - \frac{1}{18}L_{jjkk}^{V8,LR} \right. \\
& - \frac{2}{9}L_{iii}^{V,LL} - 2L_{ijj}^{V,LL} + \frac{52}{9}L_{ijji}^{V,LL} - \frac{2}{9}L_{ikki}^{V,LL} - \frac{4}{9}L_{jjjj}^{V,LL} - \frac{2}{9}L_{jjkk}^{V,LL} \\
& - \frac{1}{18}L_{ii11}^{V8,LR} - \frac{1}{18}L_{ii22}^{V8,LR} - \frac{1}{18}L_{jj11}^{V8,LR} - \frac{1}{18}L_{jj22}^{V8,LR} - \frac{1}{18}L_{11ii}^{V8,LL} - \frac{1}{18}L_{11jj}^{V8,LL} \\
& \left. - \frac{1}{18}L_{22ii}^{V8,LL} - \frac{1}{18}L_{22jj}^{V8,LL} \right] + e^2 \left[ \frac{2}{9}L_{iii}^{V1,LR} + \frac{2}{9}L_{ijj}^{V1,LR} + \frac{2}{9}L_{ikk}^{V1,LR} \right. \\
& + \frac{4}{9}L_{jjjj}^{V1,LR} + \frac{2}{9}L_{jjkk}^{V1,LR} + \frac{16}{27}L_{iii}^{V,LL} + \frac{16}{9}L_{ijj}^{V,LL} + \frac{4}{9}L_{ikk}^{V,LL} + \frac{4}{27}L_{ijji}^{V,LL} \\
& + \frac{4}{27}L_{ikki}^{V,LL} + \frac{32}{27}L_{jjjj}^{V,LL} + \frac{4}{9}L_{jjkk}^{V,LL} + \frac{4}{27}L_{jjkk}^{V,LL} + \frac{2}{9}L_{ii11}^{V,LR} + \frac{2}{9}L_{ii22}^{V,LR} \\
& + \frac{2}{9}L_{ii33}^{V,LR} + \frac{2}{9}L_{jj11}^{V,LR} + \frac{2}{9}L_{jj22}^{V,LR} + \frac{2}{9}L_{jj33}^{V,LR} - \frac{4}{9}L_{ii11}^{V1,LR} - \frac{4}{9}L_{ii22}^{V1,LR} \\
& - \frac{4}{9}L_{jj11}^{V1,LR} - \frac{4}{9}L_{jj22}^{V1,LR} + \frac{2}{9}L_{11ii}^{V,LL} + \frac{2}{9}L_{11jj}^{V,LL} + \frac{2}{9}L_{22ii}^{V,LL} + \frac{2}{9}L_{22jj}^{V,LL} \\
& \left. + \frac{2}{9}L_{33ii}^{V,LL} + \frac{2}{9}L_{33jj}^{V,LL} - \frac{4}{9}L_{11ii}^{V1,LL} - \frac{4}{9}L_{11jj}^{V1,LL} - \frac{4}{9}L_{22ii}^{V1,LL} - \frac{4}{9}L_{22jj}^{V1,LL} \right]
\end{aligned}$$

$$\begin{aligned}
& + \alpha_s^2 \left[ -\frac{61}{18} L_{\overline{iii}}^{V1,LR} - \frac{61}{18} L_{\overline{ijj}}^{V1,LR} - \frac{61}{18} L_{\overline{ikk}}^{V1,LR} - \frac{61}{9} L_{\overline{jjjj}}^{V1,LR} - \frac{61}{18} L_{\overline{jjkk}}^{V1,LR} \right. \\
& - \frac{67}{972} L_{\overline{iii}}^{V8,LR} - \frac{67}{972} L_{\overline{ijj}}^{V8,LR} - \frac{67}{972} L_{\overline{ikk}}^{V8,LR} - \frac{67}{486} L_{\overline{jjjj}}^{V8,LR} - \frac{67}{972} L_{\overline{jjkk}}^{V8,LR} + \frac{2005}{162} L_{\overline{iii}}^{V,LL} \\
& - \frac{17}{6} L_{\overline{ijj}}^{V,LL} + \frac{79}{9} L_{\overline{ikk}}^{V,LL} + \frac{3037}{486} L_{\overline{ijji}}^{V,LL} - \frac{142}{243} L_{\overline{ikki}}^{V,LL} + \frac{9997}{486} L_{\overline{jjjj}}^{V,LL} + \frac{79}{9} L_{\overline{jjkk}}^{V,LL} \\
& - \frac{142}{243} L_{\overline{jjkj}}^{V,LL} - \frac{61}{18} L_{\overline{ii11}}^{V1,LR} - \frac{61}{18} L_{\overline{ii22}}^{V1,LR} - \frac{61}{18} L_{\overline{jj11}}^{V1,LR} - \frac{61}{18} L_{\overline{jj22}}^{V1,LR} - \frac{67}{972} L_{\overline{ii11}}^{V8,LR} \\
& - \frac{67}{972} L_{\overline{ii22}}^{V8,LR} - \frac{67}{972} L_{\overline{jj11}}^{V8,LR} - \frac{67}{972} L_{\overline{jj22}}^{V8,LR} + \frac{73}{18} L_{\overline{11ii}}^{V1,LL} + \frac{73}{18} L_{\overline{11jj}}^{V1,LL} + \frac{73}{18} L_{\overline{22ii}}^{V1,LL} \\
& \left. + \frac{73}{18} L_{\overline{22jj}}^{V1,LL} - \frac{697}{972} L_{\overline{11ii}}^{V8,LL} - \frac{697}{972} L_{\overline{11jj}}^{V8,LL} - \frac{697}{972} L_{\overline{22ii}}^{V8,LL} - \frac{697}{972} L_{\overline{22jj}}^{V8,LL} \right] \\
& + \alpha_s \alpha \left[ \frac{238}{243} L_{\overline{iii}}^{V1,LR} + \frac{238}{243} L_{\overline{ijj}}^{V1,LR} + \frac{238}{243} L_{\overline{ikk}}^{V1,LR} + \frac{476}{243} L_{\overline{jjjj}}^{V1,LR} + \frac{238}{243} L_{\overline{jjkk}}^{V1,LR} \right. \\
& - \frac{815}{1458} L_{\overline{iii}}^{V8,LR} - \frac{815}{1458} L_{\overline{ijj}}^{V8,LR} - \frac{815}{1458} L_{\overline{ikk}}^{V8,LR} - \frac{815}{729} L_{\overline{jjjj}}^{V8,LR} - \frac{815}{1458} L_{\overline{jjkk}}^{V8,LR} \\
& + \frac{301}{243} L_{\overline{iii}}^{V,LL} - \frac{1522}{243} L_{\overline{ijj}}^{V,LL} + \frac{368}{243} L_{\overline{ikk}}^{V,LL} - \frac{6776}{729} L_{\overline{ijji}}^{V,LL} - \frac{458}{729} L_{\overline{ikki}}^{V,LL} \\
& + \frac{1549}{729} L_{\overline{jjjj}}^{V,LL} + \frac{368}{243} L_{\overline{jjkk}}^{V,LL} - \frac{458}{729} L_{\overline{jjkj}}^{V,LL} + \frac{22}{243} L_{\overline{ii11}}^{V,LR} + \frac{22}{243} L_{\overline{de ii22}}^{V,LR} + \frac{22}{243} L_{\overline{de ii33}}^{V,LR} \\
& + \frac{22}{243} L_{\overline{jj11}}^{V,LR} + \frac{22}{243} L_{\overline{de jj22}}^{V,LR} + \frac{22}{243} L_{\overline{de jj33}}^{V,LR} - \frac{476}{243} L_{\overline{ii11}}^{V1,LR} - \frac{476}{243} L_{\overline{ii22}}^{V1,LR} - \frac{476}{243} L_{\overline{ii11}}^{V1,LR} \\
& - \frac{476}{243} L_{\overline{ii22}}^{V1,LR} + \frac{697}{1458} L_{\overline{ii11}}^{V8,LR} + \frac{697}{1458} L_{\overline{ii22}}^{V8,LR} + \frac{697}{1458} L_{\overline{jj11}}^{V8,LR} + \frac{697}{1458} L_{\overline{jj22}}^{V8,LR} \\
& + \frac{22}{243} L_{\overline{ed 11ii}}^{V,LL} + \frac{22}{243} L_{\overline{ed 11jj}}^{V,LL} + \frac{22}{243} L_{\overline{ed 22ii}}^{V,LL} + \frac{22}{243} L_{\overline{ed 22jj}}^{V,LL} + \frac{22}{243} L_{\overline{ed 33ii}}^{V,LL} + \frac{22}{243} L_{\overline{ed 33jj}}^{V,LL} \\
& - \frac{476}{243} L_{\overline{11ii}}^{V1,LL} - \frac{476}{243} L_{\overline{11jj}}^{V1,LL} - \frac{476}{243} L_{\overline{22ii}}^{V1,LL} - \frac{476}{243} L_{\overline{22jj}}^{V1,LL} + \frac{85}{1458} L_{\overline{11ii}}^{V8,LL} \\
& \left. + \frac{85}{1458} L_{\overline{11jj}}^{V8,LL} + \frac{85}{1458} L_{\overline{22ii}}^{V8,LL} + \frac{85}{1458} L_{\overline{22jj}}^{V8,LL} \right] + \alpha^2 \left[ -\frac{368}{729} L_{\overline{iii}}^{V1,LR} - \frac{368}{729} L_{\overline{ijj}}^{V1,LR} \right. \\
& - \frac{368}{729} L_{\overline{ikk}}^{V1,LR} - \frac{736}{729} L_{\overline{jjjj}}^{V1,LR} - \frac{368}{729} L_{\overline{jjkk}}^{V1,LR} + \frac{608}{729} L_{\overline{iii}}^{V,LL} + \frac{686}{729} L_{\overline{ijj}}^{V,LL} \\
& \left. + \frac{272}{729} L_{\overline{ikk}}^{V,LL} + \frac{296}{2187} L_{\overline{ijji}}^{V,LL} + \frac{296}{2187} L_{\overline{ikki}}^{V,LL} + \frac{2936}{2187} L_{\overline{jjjj}}^{V,LL} + \frac{272}{729} L_{\overline{jjkk}}^{V,LL} \right]
\end{aligned}$$

$$\begin{aligned}
& + \frac{296}{2187} L_{jkkj}^{V,LL} - \frac{656}{729} L_{ii11}^{V,LR} - \frac{656}{729} L_{ii22}^{V,LR} - \frac{656}{729} L_{ii33}^{V,LR} - \frac{656}{729} L_{jj11}^{V,LR} \\
& - \frac{656}{729} L_{jj22}^{V,LR} - \frac{656}{729} L_{jj33}^{V,LR} - \frac{1748}{729} L_{ii11}^{V1,LR} - \frac{1748}{729} L_{ii22}^{V1,LR} - \frac{1748}{729} L_{jj11}^{V1,LR} \\
& - \frac{1748}{729} L_{jj22}^{V1,LR} + \frac{856}{729} L_{11ii}^{V,LL} + \frac{856}{729} L_{11jj}^{V,LL} + \frac{856}{729} L_{22ii}^{V,LL} + \frac{856}{729} L_{22jj}^{V,LL} \\
& + \frac{856}{729} L_{33ii}^{V,LL} + \frac{856}{729} L_{33jj}^{V,LL} + \frac{268}{729} L_{11ii}^{V1,LL} + \frac{268}{729} L_{11jj}^{V1,LL} + \frac{268}{729} L_{22ii}^{V1,LL} \\
& + \frac{268}{729} L_{22jj}^{V1,LL} \Bigg];
\end{aligned}$$

$$\begin{aligned}
\dot{L}_{ijji}^{V,LL} &= g_s^2 \left[ \frac{1}{6} L_{iii}^{V8,LR} + \frac{1}{6} L_{ijj}^{V8,LR} + \frac{1}{6} L_{ikk}^{V8,LR} + \frac{1}{3} L_{jjj}^{V8,LR} + \frac{1}{6} L_{jjkk}^{V8,LR} \right. \\
& + \frac{2}{3} L_{iii}^{V,LL} + 6 L_{ijj}^{V,LL} - \frac{4}{3} L_{ijji}^{V,LL} + \frac{2}{3} L_{ikki}^{V,LL} + \frac{4}{3} L_{jjjj}^{V,LL} + \frac{2}{3} L_{jjkk}^{V,LL} \\
& + \frac{1}{6} L_{ii11}^{V8,LR} + \frac{1}{6} L_{ii22}^{V8,LR} + \frac{1}{6} L_{jj11}^{V8,LR} + \frac{1}{6} L_{jj22}^{V8,LR} + \frac{1}{6} L_{11ii}^{V8,LL} + \frac{1}{6} L_{11jj}^{V8,LL} \\
& + \frac{1}{6} L_{22ii}^{V8,LL} + \frac{1}{6} L_{22jj}^{V8,LL} \Bigg] + \frac{4}{3} L_{ijji}^{V,LL} e^2 + \alpha_s^2 \left[ -\frac{11}{6} L_{iii}^{V1,LR} - \frac{11}{6} L_{ijj}^{V1,LR} \right. \\
& - \frac{11}{6} L_{ikk}^{V1,LR} - \frac{11}{3} L_{jjj}^{V1,LR} - \frac{11}{6} L_{jjkk}^{V1,LR} + \frac{139}{324} L_{iii}^{V8,LR} + \frac{139}{324} L_{ijj}^{V8,LR} + \frac{139}{324} L_{ikk}^{V8,LR} \\
& + \frac{139}{162} L_{jjjj}^{V8,LR} + \frac{139}{324} L_{jjkk}^{V8,LR} + \frac{947}{54} L_{iii}^{V,LL} + \frac{9}{2} L_{ijj}^{V,LL} - \frac{7}{3} L_{ikk}^{V,LL} + \frac{707}{162} L_{ijji}^{V,LL} \\
& + \frac{1294}{81} L_{ikki}^{V,LL} + \frac{5051}{162} L_{jjjj}^{V,LL} - \frac{7}{3} L_{jjkk}^{V,LL} + \frac{1294}{81} L_{jjkj}^{V,LL} - \frac{11}{6} L_{ii11}^{V1,LR} - \frac{11}{6} L_{ii22}^{V1,LR} \\
& - \frac{11}{6} L_{jj11}^{V1,LR} - \frac{11}{6} L_{jj22}^{V1,LR} + \frac{139}{324} L_{ii11}^{V8,LR} + \frac{139}{324} L_{ii22}^{V8,LR} + \frac{139}{324} L_{jj11}^{V8,LR} + \frac{139}{324} L_{jj22}^{V8,LR} \\
& - \frac{1}{6} L_{11ii}^{V1,LL} - \frac{1}{6} L_{11jj}^{V1,LL} - \frac{1}{6} L_{22ii}^{V1,LL} - \frac{1}{6} L_{22jj}^{V1,LL} + \frac{769}{324} L_{11ii}^{V8,LL} + \frac{769}{324} L_{11jj}^{V8,LL} \\
& + \frac{769}{324} L_{22ii}^{V8,LL} + \frac{769}{324} L_{22jj}^{V8,LL} \Bigg] + \alpha_s \alpha \left[ -\frac{22}{81} L_{iii}^{V1,LR} - \frac{22}{81} L_{ijj}^{V1,LR} - \frac{22}{81} L_{ikk}^{V1,LR} \right. \\
& - \frac{44}{81} L_{jjj}^{V1,LR} - \frac{22}{81} L_{jjkk}^{V1,LR} - \frac{25}{54} L_{iii}^{V8,LR} - \frac{25}{54} L_{ijj}^{V8,LR} - \frac{25}{54} L_{ikk}^{V8,LR} - \frac{25}{27} L_{jjjj}^{V8,LR} \\
& - \frac{25}{54} L_{jjkk}^{V8,LR} + \frac{211}{81} L_{iii}^{V,LL} - \frac{746}{81} L_{ijj}^{V,LL} - \frac{44}{81} L_{ikk}^{V,LL} - \frac{1436}{243} L_{ijji}^{V,LL} + \frac{454}{243} L_{ikki}^{V,LL}
\end{aligned}$$



$$\begin{aligned}
& + \frac{955}{243} L_{jjjj}^{V,LL} - \frac{44}{81} L_{jjkk}^{V,LL} + \frac{454}{243} L_{jjkj}^{V,LL} - \frac{22}{81} L_{ii11}^{V,LR} - \frac{22}{81} L_{ii22}^{V,LR} - \frac{22}{81} L_{ii33}^{V,LR} \\
& - \frac{22}{81} L_{jj11}^{V,LR} - \frac{22}{81} L_{jj22}^{V,LR} - \frac{22}{81} L_{jj33}^{V,LR} + \frac{44}{81} L_{ii11}^{V1,LR} + \frac{44}{81} L_{ii22}^{V1,LR} + \frac{44}{81} L_{jj11}^{V1,LR} \\
& + \frac{44}{81} L_{jj22}^{V1,LR} + \frac{71}{54} L_{ii11}^{V8,LR} + \frac{71}{54} L_{ii22}^{V8,LR} + \frac{71}{54} L_{jj11}^{V8,LR} + \frac{71}{54} L_{jj22}^{V8,LR} - \frac{22}{81} L_{11ii}^{V,LL} \\
& - \frac{22}{81} L_{11jj}^{V,LL} - \frac{22}{81} L_{22ii}^{V,LL} - \frac{22}{81} L_{22jj}^{V,LL} - \frac{22}{81} L_{33ii}^{V,LL} - \frac{22}{81} L_{33jj}^{V,LL} + \frac{44}{81} L_{11ii}^{V1,LL} \\
& + \frac{44}{81} L_{11jj}^{V1,LL} + \frac{44}{81} L_{22ii}^{V1,LL} + \frac{44}{81} L_{22jj}^{V1,LL} - \frac{7}{18} L_{11ii}^{V8,LL} - \frac{7}{18} L_{11jj}^{V8,LL} - \frac{7}{18} L_{22ii}^{V8,LL} \\
& - \frac{7}{18} L_{22jj}^{V8,LL} \Big] + \frac{46}{81} L_{ijji}^{V,LL} \alpha^2 ;
\end{aligned}$$

$$\begin{aligned}
\dot{L}_{iii}^{V,LL} &= g_s^2 \left[ \frac{2}{9} L_{iii}^{V8,LR} + \frac{2}{9} L_{ijj}^{V8,LR} + \frac{2}{9} L_{ikk}^{V8,LR} + \frac{44}{9} L_{iii}^{V,LL} + \frac{8}{9} L_{ijji}^{V,LL} \right. \\
& + \frac{8}{9} L_{ikki}^{V,LL} + \frac{2}{9} L_{ii11}^{V8,LR} + \frac{2}{9} L_{ii22}^{V8,LR} + \frac{2}{9} L_{ii33}^{V8,LR} + \frac{2}{9} L_{11ii}^{V8,LL} + \frac{2}{9} L_{22ii}^{V8,LL} \Big] + e^2 \left[ \frac{4}{9} L_{iii}^{V1,LR} \right. \\
& + \frac{4}{9} L_{ijj}^{V1,LR} + \frac{4}{9} L_{ikk}^{V1,LR} + \frac{68}{27} L_{iii}^{V,LL} + \frac{8}{9} L_{ijj}^{V,LL} + \frac{8}{9} L_{ikk}^{V,LL} + \frac{8}{27} L_{ijji}^{V,LL} \\
& + \frac{8}{27} L_{ikki}^{V,LL} + \frac{4}{9} L_{ii11}^{V,LR} + \frac{4}{9} L_{ii22}^{V,LR} + \frac{4}{9} L_{ii33}^{V,LR} - \frac{8}{9} L_{11ii}^{V1,LR} - \frac{8}{9} L_{22ii}^{V1,LR} \\
& + \frac{4}{9} L_{11ii}^{V,LL} + \frac{4}{9} L_{22ii}^{V,LL} + \frac{4}{9} L_{33ii}^{V,LL} - \frac{8}{9} L_{11ii}^{V1,LL} - \frac{8}{9} L_{22ii}^{V1,LL} \Big] + \alpha_s^2 \left[ -\frac{94}{9} L_{iii}^{V1,LR} \right. \\
& - \frac{94}{9} L_{ijj}^{V1,LR} - \frac{94}{9} L_{ikk}^{V1,LR} + \frac{175}{243} L_{iii}^{V8,LR} + \frac{175}{243} L_{ijj}^{V8,LR} + \frac{175}{243} L_{ikk}^{V8,LR} + \frac{4459}{81} L_{iii}^{V,LL} \\
& + \frac{116}{9} L_{ijj}^{V,LL} + \frac{116}{9} L_{ikk}^{V,LL} + \frac{7480}{243} L_{ijji}^{V,LL} + \frac{7480}{243} L_{ikki}^{V,LL} - \frac{94}{9} L_{ii11}^{V1,LR} - \frac{94}{9} L_{ii22}^{V1,LR} \\
& + \frac{175}{243} L_{ii11}^{V8,LR} + \frac{175}{243} L_{ii22}^{V8,LR} + \frac{70}{9} L_{11ii}^{V1,LL} + \frac{70}{9} L_{22ii}^{V1,LL} + \frac{805}{243} L_{11ii}^{V8,LL} + \frac{805}{243} L_{22ii}^{V8,LL} \Big] \\
& + \alpha_s \alpha \left[ \frac{344}{243} L_{iii}^{V1,LR} + \frac{344}{243} L_{ijj}^{V1,LR} + \frac{344}{243} L_{ikk}^{V1,LR} - \frac{1490}{729} L_{iii}^{V8,LR} - \frac{1490}{729} L_{ijj}^{V8,LR} \right. \\
& - \frac{1490}{729} L_{ikk}^{V8,LR} - \frac{2128}{243} L_{iii}^{V,LL} + \frac{472}{243} L_{ijj}^{V,LL} + \frac{472}{243} L_{ikk}^{V,LL} + \frac{1808}{729} L_{ijji}^{V,LL} \\
& \left. - \frac{1808}{729} L_{ikki}^{V,LL} \right]
\end{aligned}$$

$$\begin{aligned}
& + \frac{1808}{729} L_{dd}^{V,LL} - \frac{88}{243} L_{de}^{V,LR} - \frac{88}{243} L_{de}^{V,LR} - \frac{88}{243} L_{de}^{V,LR} - \frac{688}{243} L_{du}^{V1,LR} - \frac{688}{243} L_{du}^{V1,LR} \\
& + \frac{2614}{729} L_{du}^{V8,LR} + \frac{2614}{729} L_{du}^{V8,LR} - \frac{88}{243} L_{ed}^{V,LL} - \frac{88}{243} L_{ed}^{V,LL} - \frac{88}{243} L_{ed}^{V,LL} \\
& - \frac{688}{243} L_{ud}^{V1,LL} - \frac{688}{243} L_{ud}^{V1,LL} - \frac{482}{729} L_{ud}^{V8,LL} - \frac{482}{729} L_{ud}^{V8,LL} \Big] + \alpha^2 \Big[ - \frac{736}{729} L_{dd}^{V1,LR} \\
& - \frac{736}{729} L_{ij}^{V1,LR} - \frac{736}{729} L_{dd}^{V1,LR} + \frac{1630}{729} L_{dd}^{V,LL} + \frac{544}{729} L_{ij}^{V,LL} + \frac{544}{729} L_{dd}^{V,LL} \\
& + \frac{592}{2187} L_{dd}^{V,LL} + \frac{592}{2187} L_{dd}^{V,LL} - \frac{1312}{729} L_{de}^{V,LR} - \frac{1312}{729} L_{de}^{V,LR} - \frac{1312}{729} L_{de}^{V,LR} \\
& - \frac{3496}{729} L_{du}^{V1,LR} - \frac{3496}{729} L_{du}^{V1,LR} + \frac{1712}{729} L_{ed}^{V,LL} + \frac{1712}{729} L_{ed}^{V,LL} + \frac{1712}{729} L_{ed}^{V,LL} \\
& + \frac{536}{729} L_{ud}^{V1,LL} + \frac{536}{729} L_{ud}^{V1,LL} \Big] ;
\end{aligned}$$

$$\begin{aligned}
\dot{L}_{uu}^{V,LL} = & g_s^2 \Big[ - \frac{1}{18} L_{ud}^{V8,LL} - \frac{1}{18} L_{ud}^{V8,LL} - \frac{1}{18} L_{ud}^{V8,LL} - \frac{1}{18} L_{ud}^{V8,LL} - \frac{1}{18} L_{ud}^{V8,LL} \\
& - \frac{1}{18} L_{ud}^{V8,LL} - \frac{1}{18} L_{ud}^{V8,LR} - \frac{1}{18} L_{ud}^{V8,LR} - \frac{1}{18} L_{ud}^{V8,LR} - \frac{1}{18} L_{ud}^{V8,LR} - \frac{1}{18} L_{ud}^{V8,LR} - \frac{1}{18} L_{ud}^{V8,LR} \\
& - \frac{1}{18} L_{ud}^{V8,LR} - \frac{1}{18} L_{uu}^{V8,LR} - \frac{1}{18} L_{uu}^{V8,LR} - \frac{1}{18} L_{uu}^{V8,LR} - \frac{1}{18} L_{uu}^{V8,LR} - \frac{1}{18} L_{uu}^{V8,LR} - \frac{2}{9} L_{uu}^{V8,LL} \\
& - 2L_{uu}^{V,LL} + 6L_{uu}^{V,LL} - \frac{2}{9} L_{uu}^{V,LL} - \frac{2}{9} L_{uu}^{V,LL} - \frac{2}{9} L_{uu}^{V,LL} \Big] + e^2 \Big[ - \frac{4}{9} L_{eu}^{V,LL} \\
& - \frac{4}{9} L_{eu}^{V,LL} - \frac{4}{9} L_{eu}^{V,LL} - \frac{4}{9} L_{eu}^{V,LL} - \frac{4}{9} L_{eu}^{V,LL} - \frac{4}{9} L_{eu}^{V1,LL} \\
& - \frac{4}{9} L_{ud}^{V1,LL} - \frac{4}{9} L_{ud}^{V1,LL} - \frac{4}{9} L_{ud}^{V1,LL} - \frac{4}{9} L_{ud}^{V1,LL} - \frac{4}{9} L_{ud}^{V1,LL} - \frac{4}{9} L_{ud}^{V1,LL} \\
& - \frac{4}{9} L_{ud}^{V1,LR} - \frac{4}{9} L_{ud}^{V1,LR} - \frac{4}{9} L_{ud}^{V1,LR} - \frac{4}{9} L_{ud}^{V1,LR} - \frac{4}{9} L_{ud}^{V1,LR} - \frac{4}{9} L_{ud}^{V1,LR} \\
& - \frac{4}{9} L_{ue}^{V,LR} - \frac{4}{9} L_{ue}^{V,LR} - \frac{4}{9} L_{ue}^{V,LR} - \frac{4}{9} L_{ue}^{V,LR} - \frac{4}{9} L_{ue}^{V,LR} + \frac{8}{9} L_{uu}^{V1,LR} \\
& + \frac{8}{9} L_{uu}^{V1,LR} + \frac{8}{9} L_{uu}^{V1,LR} + \frac{8}{9} L_{uu}^{V1,LR} + \frac{64}{27} L_{uu}^{V,LL} + \frac{16}{3} L_{uu}^{V,LL} + \frac{16}{9} L_{uu}^{V,LL} \\
& + \frac{16}{27} L_{uu}^{V,LL} + \frac{64}{27} L_{uu}^{V,LL} + \frac{16}{9} L_{uu}^{V,LL} + \frac{16}{27} L_{uu}^{V,LL} \Big] + \alpha_s^2 \Big[ \frac{73}{18} L_{ud}^{V1,LL}
\end{aligned}$$

$$\begin{aligned}
& + \frac{73}{18} L_{ud\,ii22}^{V1,LL} + \frac{73}{18} L_{ud\,ii33}^{V1,LL} + \frac{73}{18} L_{ud\,jj11}^{V1,LL} + \frac{73}{18} L_{ud\,jj22}^{V1,LL} + \frac{73}{18} L_{ud\,jj33}^{V1,LL} - \frac{61}{18} L_{ud\,ii11}^{V1,LR} \\
& - \frac{61}{18} L_{ud\,ii22}^{V1,LR} - \frac{61}{18} L_{ud\,ii33}^{V1,LR} - \frac{61}{18} L_{ud\,jj11}^{V1,LR} - \frac{61}{18} L_{ud\,jj22}^{V1,LR} - \frac{61}{18} L_{ud\,jj33}^{V1,LR} - \frac{715}{972} L_{ud\,ii11}^{V8,LL} \\
& - \frac{715}{972} L_{ud\,ii22}^{V8,LL} - \frac{715}{972} L_{ud\,ii33}^{V8,LL} - \frac{715}{972} L_{ud\,jj11}^{V8,LL} - \frac{715}{972} L_{ud\,jj22}^{V8,LL} - \frac{715}{972} L_{ud\,jj33}^{V8,LL} \\
& - \frac{85}{972} L_{ud\,ii11}^{V8,LR} - \frac{85}{972} L_{ud\,ii22}^{V8,LR} - \frac{85}{972} L_{ud\,ii33}^{V8,LR} - \frac{85}{972} L_{ud\,jj11}^{V8,LR} - \frac{85}{972} L_{ud\,jj22}^{V8,LR} - \frac{85}{972} L_{ud\,jj33}^{V8,LR} \\
& - \frac{61}{18} L_{uu\,iii}^{V1,LR} - \frac{61}{18} L_{uu\,ikk}^{V1,LR} - \frac{61}{18} L_{uu\,jjjj}^{V1,LR} - \frac{61}{18} L_{uu\,jjkk}^{V1,LR} - \frac{85}{972} L_{uu\,iii}^{V8,LR} - \frac{85}{972} L_{uu\,ikk}^{V8,LR} \\
& - \frac{85}{972} L_{uu\,jjjj}^{V8,LR} - \frac{85}{972} L_{uu\,jjkk}^{V8,LR} + \frac{1993}{162} L_{uu\,iii}^{V,LL} - \frac{209}{18} L_{uu\,ijj}^{V,LL} + \frac{79}{9} L_{uu\,ikk}^{V,LL} + \frac{41}{6} L_{uu\,ijji}^{V,LL} \\
& - \frac{160}{243} L_{uu\,ikki}^{V,LL} + \frac{1993}{162} L_{uu\,jjjj}^{V,LL} + \frac{79}{9} L_{uu\,jjkk}^{V,LL} - \frac{160}{243} L_{uu\,jjkj}^{V,LL} \Big] + \alpha_s \alpha \Bigg[ - \frac{44}{243} L_{eu\,11ii}^{V,LL} \\
& - \frac{44}{243} L_{eu\,11jj}^{V,LL} - \frac{44}{243} L_{eu\,22ii}^{V,LL} - \frac{44}{243} L_{eu\,22jj}^{V,LL} - \frac{44}{243} L_{eu\,33ii}^{V,LL} - \frac{44}{243} L_{eu\,33jj}^{V,LL} - \frac{476}{243} L_{ud\,ii11}^{V1,LL} \\
& - \frac{476}{243} L_{ud\,ii22}^{V1,LL} - \frac{476}{243} L_{ud\,ii33}^{V1,LL} - \frac{476}{243} L_{ud\,jj11}^{V1,LL} - \frac{476}{243} L_{ud\,jj22}^{V1,LL} - \frac{476}{243} L_{ud\,jj33}^{V1,LL} \\
& - \frac{476}{243} L_{ud\,ii11}^{V1,LR} - \frac{476}{243} L_{ud\,ii22}^{V1,LR} + \frac{934}{243} L_{ud\,ii33}^{V1,LR} - \frac{476}{243} L_{ud\,jj11}^{V1,LR} - \frac{476}{243} L_{ud\,jj22}^{V1,LR} \\
& + \frac{934}{243} L_{ud\,jj33}^{V1,LR} - \frac{533}{1458} L_{ud\,ii11}^{V8,LL} - \frac{533}{1458} L_{ud\,ii22}^{V8,LL} - \frac{533}{1458} L_{ud\,ii33}^{V8,LL} - \frac{533}{1458} L_{ud\,jj11}^{V8,LL} \\
& - \frac{533}{1458} L_{ud\,jj22}^{V8,LL} - \frac{533}{1458} L_{ud\,jj33}^{V8,LL} + \frac{79}{1458} L_{ud\,ii11}^{V8,LR} + \frac{79}{1458} L_{ud\,ii22}^{V8,LR} - \frac{1594}{729} L_{ud\,ii33}^{V8,LR} \\
& + \frac{79}{1458} L_{ud\,jj11}^{V8,LR} + \frac{79}{1458} L_{ud\,jj22}^{V8,LR} - \frac{1594}{729} L_{ud\,jj33}^{V8,LR} - \frac{44}{243} L_{ue\,ii11}^{V,LR} - \frac{44}{243} L_{ue\,ii22}^{V,LR} \\
& - \frac{44}{243} L_{ue\,ii33}^{V,LR} - \frac{44}{243} L_{ue\,jj11}^{V,LR} - \frac{44}{243} L_{ue\,jj22}^{V,LR} - \frac{44}{243} L_{ue\,jj33}^{V,LR} + \frac{952}{243} L_{uu\,iii}^{V1,LR} + \frac{952}{243} L_{uu\,ikk}^{V1,LR} \\
& + \frac{952}{243} L_{uu\,jjjj}^{V1,LR} + \frac{952}{243} L_{uu\,jjkk}^{V1,LR} - \frac{1594}{729} L_{uu\,iii}^{V8,LR} - \frac{1594}{729} L_{uu\,ikk}^{V8,LR} - \frac{1594}{729} L_{uu\,jjjj}^{V8,LR} \\
& - \frac{1594}{729} L_{uu\,jjkk}^{V8,LR} + \frac{1252}{243} L_{uu\,iii}^{V,LL} - \frac{280}{9} L_{uu\,ijj}^{V,LL} + \frac{1472}{243} L_{uu\,ikk}^{V,LL} - \frac{104}{3} L_{uu\,ijji}^{V,LL} - \frac{1688}{729} L_{uu\,ikki}^{V,LL} \\
& + \frac{1252}{243} L_{uu\,jjjj}^{V,LL} + \frac{1472}{243} L_{uu\,jjkk}^{V,LL} - \frac{1688}{729} L_{uu\,jjkj}^{V,LL} \Big] + \alpha^2 \Bigg[ \frac{1252}{729} L_{eu\,11ii}^{V,LL} + \frac{1252}{729} L_{eu\,11jj}^{V,LL} \\
& + \frac{1252}{729} L_{eu\,22ii}^{V,LL} + \frac{1252}{729} L_{eu\,22jj}^{V,LL} + \frac{1252}{729} L_{eu\,33ii}^{V,LL} + \frac{1252}{729} L_{eu\,33jj}^{V,LL} + \frac{964}{729} L_{ud\,ii11}^{V1,LL}
\end{aligned}$$

$$\begin{aligned}
& + \frac{964}{729} L_{ii22}^{V1,LL} + \frac{964}{729} L_{ii33}^{V1,LL} + \frac{964}{729} L_{jj11}^{V1,LL} + \frac{964}{729} L_{jj22}^{V1,LL} + \frac{964}{729} L_{jj33}^{V1,LL} \\
& - \frac{1052}{729} L_{ii11}^{V1,LR} - \frac{1052}{729} L_{ii22}^{V1,LR} - \frac{6176}{729} L_{ii33}^{V1,LR} - \frac{1052}{729} L_{jj11}^{V1,LR} - \frac{1052}{729} L_{jj22}^{V1,LR} \\
& - \frac{6176}{729} L_{jj33}^{V1,LR} - \frac{4796}{729} L_{ii11}^{V,LR} - \frac{4796}{729} L_{ii22}^{V,LR} - \frac{4796}{729} L_{ii33}^{V,LR} - \frac{4796}{729} L_{jj11}^{V,LR} - \frac{4796}{729} L_{jj22}^{V,LR} \\
& - \frac{4796}{729} L_{jj33}^{V,LR} - \frac{4796}{729} L_{jj33}^{V,LR} - \frac{5888}{729} L_{iii}^{V1,LR} - \frac{5888}{729} L_{ikk}^{V1,LR} - \frac{5888}{729} L_{jjj}^{V1,LR} \\
& - \frac{5888}{729} L_{jjk}^{V1,LR} + \frac{9728}{729} L_{uu}^{V,LL} - \frac{1184}{81} L_{ijj}^{V,LL} + \frac{4352}{729} L_{ikk}^{V,LL} + \frac{4736}{2187} L_{ikki}^{V,LL} \\
& + \frac{9728}{729} L_{jjj}^{V,LL} + \frac{4352}{729} L_{jjk}^{V,LL} + \frac{4736}{2187} L_{kkj}^{V,LL} \Big] ;
\end{aligned}$$

$$\begin{aligned}
\dot{L}_{ijji}^{V,LL} &= g_s^2 \left[ \frac{1}{6} L_{ii11}^{V8,LL} + \frac{1}{6} L_{ii22}^{V8,LL} + \frac{1}{6} L_{ii33}^{V8,LL} + \frac{1}{6} L_{jj11}^{V8,LL} + \frac{1}{6} L_{jj22}^{V8,LL} \right. \\
& + \frac{1}{6} L_{jj33}^{V8,LL} + \frac{1}{6} L_{ii11}^{V8,LR} + \frac{1}{6} L_{ii22}^{V8,LR} + \frac{1}{6} L_{ii33}^{V8,LR} + \frac{1}{6} L_{jj11}^{V8,LR} + \frac{1}{6} L_{jj22}^{V8,LR} \\
& + \frac{1}{6} L_{jj33}^{V8,LR} + \frac{1}{6} L_{iii}^{V8,LR} + \frac{1}{6} L_{ikk}^{V8,LR} + \frac{1}{6} L_{jjj}^{V8,LR} + \frac{1}{6} L_{jjk}^{V8,LR} + \frac{2}{3} L_{iii}^{V,LL} \\
& \left. + 6 L_{ijj}^{V,LL} - 2 L_{ijji}^{V,LL} + \frac{2}{3} L_{ikki}^{V,LL} + \frac{2}{3} L_{jjjj}^{V,LL} + \frac{2}{3} L_{jjkj}^{V,LL} \right] + \frac{16}{3} L_{ijji}^{V,LL} \\
& e^2 + \alpha_s^2 \left[ -\frac{1}{6} L_{ii11}^{V1,LL} - \frac{1}{6} L_{ii22}^{V1,LL} - \frac{1}{6} L_{ii33}^{V1,LL} - \frac{1}{6} L_{jj11}^{V1,LL} - \frac{1}{6} L_{jj22}^{V1,LL} \right. \\
& - \frac{1}{6} L_{jj33}^{V1,LL} - \frac{11}{6} L_{ii11}^{V1,LR} - \frac{11}{6} L_{ii22}^{V1,LR} - \frac{11}{6} L_{ii33}^{V1,LR} - \frac{11}{6} L_{jj11}^{V1,LR} - \frac{11}{6} L_{jj22}^{V1,LR} \\
& - \frac{11}{6} L_{jj33}^{V1,LR} + \frac{787}{324} L_{ii11}^{V8,LL} + \frac{787}{324} L_{ii22}^{V8,LL} + \frac{787}{324} L_{ii33}^{V8,LL} + \frac{787}{324} L_{jj11}^{V8,LL} \\
& + \frac{787}{324} L_{jj22}^{V8,LL} + \frac{787}{324} L_{jj33}^{V8,LL} + \frac{157}{324} L_{ii11}^{V8,LR} + \frac{157}{324} L_{ii22}^{V8,LR} + \frac{157}{324} L_{ii33}^{V8,LR} \\
& + \frac{157}{324} L_{jj11}^{V8,LR} + \frac{157}{324} L_{jj22}^{V8,LR} + \frac{157}{324} L_{jj33}^{V8,LR} - \frac{11}{6} L_{iii}^{V1,LR} - \frac{11}{6} L_{ikk}^{V1,LR} - \frac{11}{6} L_{jjj}^{V1,LR} \\
& - \frac{11}{6} L_{jjk}^{V1,LR} + \frac{157}{324} L_{iii}^{V8,LR} + \frac{157}{324} L_{ikk}^{V8,LR} + \frac{157}{324} L_{jjj}^{V8,LR} + \frac{157}{324} L_{jjk}^{V8,LR} \\
& \left. + \frac{959}{54} L_{iii}^{V,LL} + \frac{41}{6} L_{ijj}^{V,LL} - \frac{7}{3} L_{ikk}^{V,LL} - \frac{209}{18} L_{ijji}^{V,LL} + \frac{1312}{81} L_{ikki}^{V,LL} + \frac{959}{54} L_{jjjj}^{V,LL} \right]
\end{aligned}$$

$$\begin{aligned}
& -\frac{7}{3}L_{jjkk}^{V,LL} + \frac{1312}{81}L_{jkkj}^{V,LL} \Big] + \alpha_s \alpha \Big[ \frac{44}{81}L_{11ii}^{V,LL} + \frac{44}{81}L_{11jj}^{V,LL} + \frac{44}{81}L_{22ii}^{V,LL} \\
& + \frac{44}{81}L_{22jj}^{V,LL} + \frac{44}{81}L_{33ii}^{V,LL} + \frac{44}{81}L_{33jj}^{V,LL} + \frac{44}{81}L_{ii11}^{V1,LL} + \frac{44}{81}L_{ii22}^{V1,LL} + \frac{44}{81}L_{ii33}^{V1,LL} \\
& + \frac{44}{81}L_{jj11}^{V1,LL} + \frac{44}{81}L_{jj22}^{V1,LL} + \frac{44}{81}L_{jj33}^{V1,LL} + \frac{44}{81}L_{ii11}^{V1,LR} + \frac{44}{81}L_{ii22}^{V1,LR} - \frac{70}{81}L_{ii33}^{V1,LR} \\
& + \frac{44}{81}L_{jj11}^{V1,LR} + \frac{44}{81}L_{jj22}^{V1,LR} - \frac{70}{81}L_{jj33}^{V1,LR} - \frac{1}{2}L_{ii11}^{V8,LL} - \frac{1}{2}L_{ii22}^{V8,LL} - \frac{1}{2}L_{ii33}^{V8,LL} \\
& - \frac{1}{2}L_{jj11}^{V8,LL} - \frac{1}{2}L_{jj22}^{V8,LL} - \frac{1}{2}L_{jj33}^{V8,LL} + \frac{65}{54}L_{ii11}^{V8,LR} + \frac{65}{54}L_{ii22}^{V8,LR} - \frac{50}{27}L_{ii33}^{V8,LR} \\
& + \frac{65}{54}L_{jj11}^{V8,LR} + \frac{65}{54}L_{jj22}^{V8,LR} - \frac{50}{27}L_{jj33}^{V8,LR} + \frac{44}{81}L_{ii11}^{V,LR} + \frac{44}{81}L_{ii22}^{V,LR} + \frac{44}{81}L_{ii33}^{V,LR} \\
& + \frac{44}{81}L_{jj11}^{V,LR} + \frac{44}{81}L_{jj22}^{V,LR} + \frac{44}{81}L_{jj33}^{V,LR} - \frac{88}{81}L_{iii}^{V1,LR} - \frac{88}{81}L_{iikk}^{V1,LR} - \frac{88}{81}L_{jjj}^{V1,LR} \\
& - \frac{88}{81}L_{jjkk}^{V1,LR} - \frac{50}{27}L_{iii}^{V8,LR} - \frac{50}{27}L_{iikk}^{V8,LR} - \frac{50}{27}L_{jjj}^{V8,LR} - \frac{50}{27}L_{jjkk}^{V8,LR} + \frac{844}{81}L_{iii}^{V,LL} \\
& - \frac{104}{3}L_{iijj}^{V,LL} - \frac{176}{81}L_{iikk}^{V,LL} - \frac{280}{9}L_{ijji}^{V,LL} + \frac{1816}{243}L_{ikki}^{V,LL} + \frac{844}{81}L_{jjjj}^{V,LL} - \frac{176}{81}L_{jjkk}^{V,LL} \\
& + \frac{1816}{243}L_{jkkj}^{V,LL} \Big] - \frac{1184}{81}L_{ijji}^{V,LL} \alpha^2 ;
\end{aligned}$$

$$\begin{aligned}
\dot{L}_{iii}^{V,LL} & = g_s^2 \Big[ \frac{2}{9}L_{ii11}^{V8,LL} + \frac{2}{9}L_{ii22}^{V8,LL} + \frac{2}{9}L_{ii33}^{V8,LL} + \frac{2}{9}L_{ii11}^{V8,LR} + \frac{2}{9}L_{ii22}^{V8,LR} \\
& + \frac{2}{9}L_{ii33}^{V8,LR} + \frac{2}{9}L_{iii}^{V8,LR} + \frac{2}{9}L_{iikk}^{V8,LR} + \frac{44}{9}L_{iii}^{V,LL} + \frac{8}{9}L_{ikki}^{V,LL} \Big] + e^2 \Big[ -\frac{8}{9}L_{11ii}^{V,LL} \\
& - \frac{8}{9}L_{22ii}^{V,LL} - \frac{8}{9}L_{33ii}^{V,LL} - \frac{8}{9}L_{ii11}^{V1,LL} - \frac{8}{9}L_{ii22}^{V1,LL} - \frac{8}{9}L_{ii33}^{V1,LL} - \frac{8}{9}L_{ii11}^{V1,LR} \\
& - \frac{8}{9}L_{ii22}^{V1,LR} - \frac{8}{9}L_{ii33}^{V1,LR} - \frac{8}{9}L_{ii11}^{V,LR} - \frac{8}{9}L_{ii22}^{V,LR} - \frac{8}{9}L_{ii33}^{V,LR} + \frac{16}{9}L_{iii}^{V1,LR} \\
& + \frac{16}{9}L_{iikk}^{V1,LR} + \frac{272}{27}L_{iii}^{V,LL} + \frac{32}{9}L_{iikk}^{V,LL} + \frac{32}{27}L_{ikki}^{V,LL} \Big] + \alpha_s^2 \Big[ \frac{70}{9}L_{ii11}^{V1,LL} \\
& + \frac{70}{9}L_{ii22}^{V1,LL} + \frac{70}{9}L_{ii33}^{V1,LL} - \frac{94}{9}L_{ii11}^{V1,LR} - \frac{94}{9}L_{ii22}^{V1,LR} - \frac{94}{9}L_{ii33}^{V1,LR} + \frac{823}{243}L_{ii11}^{V8,LL} \\
& + \frac{823}{243}L_{ii22}^{V8,LL} + \frac{823}{243}L_{ii33}^{V8,LL} + \frac{193}{243}L_{ii11}^{V8,LR} + \frac{193}{243}L_{ii22}^{V8,LR} + \frac{193}{243}L_{ii33}^{V8,LR}
\end{aligned}$$

$$\begin{aligned}
& -\frac{94}{9}L_{uu}^{V1,LR} - \frac{94}{9}L_{iikk}^{V1,LR} + \frac{193}{243}L_{iii}^{V8,LR} + \frac{193}{243}L_{iikk}^{V8,LR} + \frac{4483}{81}L_{iii}^{V,LL} + \frac{116}{9}L_{iikk}^{V,LL} \\
& + \frac{7552}{243}L_{iikki}^{V,LL} \Big] + \alpha_s \alpha \Big[ \frac{176}{243}L_{11ii}^{V,LL} + \frac{176}{243}L_{22ii}^{V,LL} + \frac{176}{243}L_{33ii}^{V,LL} - \frac{688}{243}L_{ii11}^{V1,LL} \\
& - \frac{688}{243}L_{ii22}^{V1,LL} - \frac{688}{243}L_{ii33}^{V1,LL} - \frac{688}{243}L_{ii11}^{V1,LR} - \frac{688}{243}L_{ii22}^{V1,LR} + \frac{1448}{243}L_{ii33}^{V1,LR} \\
& - \frac{1262}{729}L_{ii11}^{V8,LL} - \frac{1262}{729}L_{ii22}^{V8,LL} - \frac{1262}{729}L_{ii33}^{V8,LL} + \frac{1834}{729}L_{ii11}^{V8,LR} + \frac{1834}{729}L_{ii22}^{V8,LR} \\
& - \frac{5888}{729}L_{ii33}^{V8,LR} + \frac{176}{243}L_{ii11}^{V,LR} + \frac{176}{243}L_{ii22}^{V,LR} + \frac{176}{243}L_{ii33}^{V,LR} + \frac{1376}{243}L_{iii}^{V1,LR} \\
& + \frac{1376}{243}L_{iikk}^{V1,LR} - \frac{5888}{729}L_{iii}^{V8,LR} - \frac{5888}{729}L_{iikk}^{V8,LR} - \frac{8416}{243}L_{iii}^{V,LL} + \frac{1888}{243}L_{iikk}^{V,LL} \\
& + \frac{7520}{729}L_{iikki}^{V,LL} \Big] + \alpha^2 \Big[ \frac{2504}{729}L_{11ii}^{V,LL} + \frac{2504}{729}L_{22ii}^{V,LL} + \frac{2504}{729}L_{33ii}^{V,LL} + \frac{1928}{729}L_{ii11}^{V1,LL} \\
& + \frac{1928}{729}L_{ii22}^{V1,LL} + \frac{1928}{729}L_{ii33}^{V1,LL} - \frac{2104}{729}L_{ii11}^{V1,LR} - \frac{2104}{729}L_{ii22}^{V1,LR} - \frac{12352}{729}L_{ii33}^{V1,LR} \\
& - \frac{9592}{729}L_{ii11}^{V,LR} - \frac{9592}{729}L_{ii22}^{V,LR} - \frac{9592}{729}L_{ii33}^{V,LR} - \frac{11776}{729}L_{iii}^{V1,LR} - \frac{11776}{729}L_{iikk}^{V1,LR} \\
& + \frac{8800}{729}L_{iii}^{V,LL} + \frac{8704}{729}L_{iikk}^{V,LL} + \frac{9472}{2187}L_{iikki}^{V,LL} \Big] ;
\end{aligned}$$

$$\begin{aligned}
\dot{L}_{ee}^{V,LL}{}_{ijj} &= e^2 \Big[ \frac{40}{3}L_{ee}^{V,LL}{}_{ijj} + \frac{1}{3}L_{ee}^{V,LR}{}_{ijj} + \frac{4}{3}L_{ee}^{V,LL}{}_{iikk} + \frac{1}{3}L_{ee}^{V,LR}{}_{iikk} + \frac{1}{3}L_{ed}^{V,LL}{}_{ii11} \\
& + \frac{1}{3}L_{ed}^{V,LL}{}_{ii22} + \frac{1}{3}L_{ed}^{V,LL}{}_{ii33} + \frac{1}{3}L_{ed}^{V,LR}{}_{ii11} + \frac{1}{3}L_{ed}^{V,LR}{}_{ii22} + \frac{1}{3}L_{ed}^{V,LR}{}_{ii33} + \frac{4}{3}L_{ee}^{V,LL}{}_{iii} \\
& + \frac{1}{3}L_{ee}^{V,LR}{}_{iii} - \frac{2}{3}L_{eu}^{V,LL}{}_{ii11} - \frac{2}{3}L_{eu}^{V,LL}{}_{ii22} - \frac{2}{3}L_{eu}^{V,LR}{}_{ii11} - \frac{2}{3}L_{eu}^{V,LR}{}_{ii22} + \frac{4}{3}L_{ee}^{V,LL}{}_{jjkk} \\
& + \frac{1}{3}L_{ee}^{V,LR}{}_{jjkk} + \frac{1}{3}L_{ed}^{V,LL}{}_{jj11} + \frac{1}{3}L_{ed}^{V,LL}{}_{jj22} + \frac{1}{3}L_{ed}^{V,LL}{}_{jj33} + \frac{1}{3}L_{ed}^{V,LR}{}_{jj11} + \frac{1}{3}L_{ed}^{V,LR}{}_{jj22} \\
& + \frac{1}{3}L_{ed}^{V,LR}{}_{jj33} + 2L_{ee}^{V,LL}{}_{jjjj} + \frac{2}{3}L_{ee}^{V,LR}{}_{jjjj} - \frac{2}{3}L_{eu}^{V,LL}{}_{jj11} - \frac{2}{3}L_{eu}^{V,LL}{}_{jj22} - \frac{2}{3}L_{eu}^{V,LR}{}_{jj11} \\
& - \frac{2}{3}L_{eu}^{V,LR}{}_{jj22} \Big] + \alpha_s \alpha \Big[ \frac{4}{3}L_{ed}^{V,LL}{}_{ii11} + \frac{4}{3}L_{ed}^{V,LL}{}_{ii22} + \frac{4}{3}L_{ed}^{V,LL}{}_{ii33} + \frac{4}{3}L_{ed}^{V,LR}{}_{ii11} \\
& + \frac{4}{3}L_{ed}^{V,LR}{}_{ii22} + \frac{4}{3}L_{ed}^{V,LR}{}_{ii33} - \frac{8}{3}L_{eu}^{V,LL}{}_{ii11} - \frac{8}{3}L_{eu}^{V,LL}{}_{ii22} - \frac{8}{3}L_{eu}^{V,LR}{}_{ii11} - \frac{8}{3}L_{eu}^{V,LR}{}_{ii22}
\end{aligned}$$

$$\begin{aligned}
& + \frac{4}{3}L_{jj11}^{V,LL} + \frac{4}{3}L_{jj22}^{V,LL} + \frac{4}{3}L_{jj33}^{V,LL} + \frac{4}{3}L_{jj11}^{V,LR} + \frac{4}{3}L_{jj22}^{V,LR} + \frac{4}{3}L_{jj33}^{V,LR} \\
& - \frac{8}{3}L_{jj11}^{V,LL} - \frac{8}{3}L_{jj22}^{V,LL} - \frac{8}{3}L_{jj11}^{V,LR} - \frac{8}{3}L_{jj22}^{V,LR} \Big] + \alpha^2 \Big[ - \frac{2302}{27}L_{ijj}^{ee,LL} \\
& - \frac{178}{27}L_{ijj}^{ee,LR} + \frac{296}{27}L_{iik}^{ee,LL} - \frac{178}{27}L_{iik}^{ee,LR} + \frac{166}{81}L_{ii11}^{V,LL} + \frac{166}{81}L_{ii22}^{V,LL} + \frac{166}{81}L_{ii33}^{V,LL} \\
& + \frac{34}{81}L_{ii11}^{V,LR} + \frac{34}{81}L_{ii22}^{V,LR} + \frac{34}{81}L_{ii33}^{V,LR} + \frac{320}{27}L_{iii}^{ee,LL} - \frac{178}{27}L_{iii}^{ee,LR} - \frac{314}{81}L_{ii11}^{V,LL} \\
& - \frac{314}{81}L_{ii22}^{V,LL} - \frac{842}{81}L_{ii11}^{V,LR} - \frac{842}{81}L_{ii22}^{V,LR} + \frac{296}{27}L_{jjkk}^{V,LL} - \frac{178}{27}L_{jjkk}^{V,LR} + \frac{166}{81}L_{ed}^{V,LL} \\
& + \frac{166}{81}L_{ed}^{V,LL} + \frac{166}{81}L_{ed}^{V,LL} + \frac{34}{81}L_{jj11}^{V,LR} + \frac{34}{81}L_{jj22}^{V,LR} + \frac{34}{81}L_{jj33}^{V,LR} + \frac{52}{3}L_{jjj}^{ee,LL} \\
& - \frac{356}{27}L_{jjj}^{ee,LR} - \frac{314}{81}L_{jj11}^{V,LL} - \frac{314}{81}L_{jj22}^{V,LL} - \frac{842}{81}L_{jj11}^{V,LR} - \frac{842}{81}L_{jj22}^{V,LR} \Big] ;
\end{aligned}$$

$$\begin{aligned}
\dot{L}_{iii}^{V,LL} &= e^2 \Big[ \frac{16}{3}L_{ijj}^{ee,LL} + \frac{4}{3}L_{ijj}^{ee,LR} + \frac{16}{3}L_{iik}^{ee,LL} + \frac{4}{3}L_{iik}^{ee,LR} + \frac{4}{3}L_{ii11}^{V,LL} \\
& + \frac{4}{3}L_{ii22}^{V,LL} + \frac{4}{3}L_{ii33}^{V,LL} + \frac{4}{3}L_{ii11}^{V,LR} + \frac{4}{3}L_{ii22}^{V,LR} + \frac{4}{3}L_{ii33}^{V,LR} + \frac{52}{3}L_{iii}^{ee,LL} \\
& + \frac{4}{3}L_{iii}^{ee,LR} - \frac{8}{3}L_{ii11}^{V,LL} - \frac{8}{3}L_{ii22}^{V,LL} - \frac{8}{3}L_{ii11}^{V,LR} - \frac{8}{3}L_{ii22}^{V,LR} \Big] + \alpha_s \alpha \Big[ \frac{16}{3}L_{ii11}^{V,LL} \\
& + \frac{16}{3}L_{ii22}^{V,LL} + \frac{16}{3}L_{ii33}^{V,LL} + \frac{16}{3}L_{ii11}^{V,LR} + \frac{16}{3}L_{ii22}^{V,LR} + \frac{16}{3}L_{ii33}^{V,LR} - \frac{32}{3}L_{ii11}^{V,LL} \\
& - \frac{32}{3}L_{ii22}^{V,LL} - \frac{32}{3}L_{ii11}^{V,LR} - \frac{32}{3}L_{ii22}^{V,LR} \Big] + \alpha^2 \Big[ \frac{1184}{27}L_{ijj}^{ee,LL} - \frac{712}{27}L_{ijj}^{ee,LR} \\
& + \frac{1184}{27}L_{iik}^{ee,LL} - \frac{712}{27}L_{iik}^{ee,LR} + \frac{664}{81}L_{ii11}^{V,LL} + \frac{664}{81}L_{ii22}^{V,LL} + \frac{664}{81}L_{ii33}^{V,LL} + \frac{136}{81}L_{ii11}^{V,LR} \\
& + \frac{136}{81}L_{ii22}^{V,LR} + \frac{136}{81}L_{ii33}^{V,LR} - \frac{1318}{27}L_{iii}^{ee,LL} - \frac{712}{27}L_{iii}^{ee,LR} - \frac{1256}{81}L_{ii11}^{V,LL} - \frac{1256}{81}L_{ii22}^{V,LL} \\
& - \frac{3368}{81}L_{ii11}^{V,LR} - \frac{3368}{81}L_{ii22}^{V,LR} \Big] ;
\end{aligned}$$

$$\dot{L}_{ijj}^{V,LL} = 0 ;$$

$$\dot{L}_{iii}^{V,LL} = 0 ;$$

$$\begin{aligned}
\dot{L}_{de}^{V,LR}{}_{ijj} &= e^2 \left[ \frac{4}{3} L_{iii}^{V1,LR} + \frac{4}{3} L_{ijj}^{V1,LR} + \frac{4}{3} L_{ikk}^{V1,LR} + \frac{32}{9} L_{iii}^{V,LL} + \frac{8}{3} L_{ijj}^{V,LL} \right. \\
&\quad + \frac{8}{3} L_{ikk}^{V,LL} + \frac{8}{9} L_{ijj}^{V,LL} + \frac{8}{9} L_{ikk}^{V,LL} + \frac{4}{9} L_{11jj}^{V,LR} + \frac{4}{9} L_{22jj}^{V,LR} + \frac{4}{9} L_{33jj}^{V,LR} \\
&\quad + \frac{4}{3} L_{ii11}^{V,LR} + \frac{4}{3} L_{ii22}^{V,LR} + \frac{4}{3} L_{ii33}^{V,LR} - 4 L_{ijj}^{V,LR} - \frac{8}{3} L_{ii11}^{V1,LR} - \frac{8}{3} L_{ii22}^{V1,LR} \\
&\quad + \frac{4}{3} L_{11ii}^{V,LL} + \frac{4}{3} L_{22ii}^{V,LL} + \frac{4}{3} L_{33ii}^{V,LL} + \frac{4}{9} L_{jj11}^{V,RR} + \frac{4}{9} L_{jj22}^{V,RR} + \frac{4}{9} L_{jj33}^{V,RR} \\
&\quad + \frac{8}{9} L_{jjj}^{V,LR} + \frac{4}{9} L_{kkjj}^{V,LR} + \frac{8}{3} L_{jjj}^{V,RR} + \frac{16}{9} L_{jjkk}^{V,RR} - \frac{8}{9} L_{jj11}^{V,RR} - \frac{8}{9} L_{jj22}^{V,RR} \\
&\quad - \frac{8}{3} L_{11ii}^{V1,LL} - \frac{8}{3} L_{22ii}^{V1,LL} - \frac{8}{9} L_{11jj}^{V,LR} - \frac{8}{9} L_{22jj}^{V,LR} \left. \right] + \alpha_s^2 \left[ 8 L_{11jj}^{V,LR} \right. \\
&\quad + 8 L_{22jj}^{V,LR} + 8 L_{33jj}^{V,LR} - 8 L_{jj11}^{V,RR} - 8 L_{jj22}^{V,RR} - 8 L_{jj33}^{V,RR} - 8 L_{jj11}^{V,RR} \\
&\quad - 8 L_{jj22}^{V,RR} + 8 L_{jj11}^{V,LR} + 8 L_{jj22}^{V,LR} \left. \right] + \alpha_s \alpha \left[ \frac{16}{3} L_{iii}^{V1,LR} + \frac{16}{3} L_{ijj}^{V1,LR} \right. \\
&\quad + \frac{16}{3} L_{ikk}^{V1,LR} - \frac{1040}{243} L_{iii}^{V8,LR} - \frac{1040}{243} L_{ijj}^{V8,LR} - \frac{1040}{243} L_{ikk}^{V8,LR} + \frac{1024}{81} L_{iii}^{V,LL} \\
&\quad + 8 L_{ijj}^{V,LL} + 8 L_{ikk}^{V,LL} - \frac{8}{243} L_{ijj}^{V,LL} - \frac{8}{243} L_{ikk}^{V,LL} + \frac{16}{9} L_{11jj}^{V,LR} + \frac{16}{9} L_{22jj}^{V,LR} \\
&\quad + \frac{16}{9} L_{33jj}^{V,LR} + 16 L_{ijj}^{V,LR} - \frac{32}{3} L_{ii11}^{V1,LR} - \frac{32}{3} L_{ii22}^{V1,LR} + \frac{1336}{243} L_{ii11}^{V8,LR} + \frac{1336}{243} L_{ii22}^{V8,LR} \\
&\quad + \frac{16}{9} L_{jj11}^{V,RR} + \frac{16}{9} L_{jj22}^{V,RR} + \frac{16}{9} L_{jj33}^{V,RR} - \frac{32}{9} L_{jj11}^{V,RR} - \frac{32}{9} L_{jj22}^{V,RR} - \frac{32}{3} L_{11ii}^{V1,LL} \\
&\quad - \frac{32}{3} L_{22ii}^{V1,LL} - \frac{104}{243} L_{11ii}^{V8,LL} - \frac{104}{243} L_{22ii}^{V8,LL} - \frac{32}{9} L_{11jj}^{V,LR} - \frac{32}{9} L_{22jj}^{V,LR} \left. \right] \\
&\quad + \alpha^2 \left[ \frac{1712}{243} L_{iii}^{V1,LR} + \frac{1712}{243} L_{ijj}^{V1,LR} + \frac{1712}{243} L_{ikk}^{V1,LR} - \frac{800}{243} L_{iii}^{V,LL} + \frac{256}{243} L_{ijj}^{V,LL} \right. \\
&\quad + \frac{256}{243} L_{ikk}^{V,LL} - \frac{1424}{729} L_{ijj}^{V,LL} - \frac{1424}{729} L_{ikk}^{V,LL} - \frac{104}{243} L_{11jj}^{V,LR} - \frac{104}{243} L_{22jj}^{V,LR} \\
&\quad - \frac{104}{243} L_{33jj}^{V,LR} + \frac{3728}{243} L_{ii11}^{V,LR} + \frac{3728}{243} L_{ii22}^{V,LR} + \frac{3728}{243} L_{ii33}^{V,LR} + \frac{1994}{27} L_{ijj}^{V,LR} \\
&\quad - \frac{616}{243} L_{ii11}^{V1,LR} - \frac{616}{243} L_{ii22}^{V1,LR} - \frac{1024}{243} L_{11ii}^{V,LL} - \frac{1024}{243} L_{22ii}^{V,LL} - \frac{1024}{243} L_{33ii}^{V,LL} \left. \right]
\end{aligned}$$



$$\begin{aligned}
& -\frac{440}{243}L_{jj11}^{V,RR} - \frac{440}{243}L_{jj22}^{V,RR} - \frac{440}{243}L_{jj33}^{V,RR} - \frac{368}{81}L_{jjjj}^{V,LR} - \frac{184}{81}L_{kkjj}^{V,LR} - \frac{80}{9}L_{jjjj}^{V,RR} \\
& - \frac{160}{81}L_{jjkk}^{V,RR} - \frac{1640}{243}L_{jj11}^{V,RR} - \frac{1640}{243}L_{jj22}^{V,RR} - \frac{6952}{243}L_{11ii}^{V1,LL} - \frac{6952}{243}L_{22ii}^{V1,LL} \\
& - \frac{296}{243}L_{11jj}^{V,LR} - \frac{296}{243}L_{22jj}^{V,LR} \Big] ;
\end{aligned}$$

$$\begin{aligned}
\dot{L}_{ue}^{V,LR}{}_{ijj} &= e^2 \Bigg[ -\frac{8}{9}L_{11jj}^{V,LR} - \frac{8}{9}L_{22jj}^{V,LR} - \frac{8}{9}L_{33jj}^{V,LR} - \frac{8}{9}L_{jj11}^{V,RR} - \frac{8}{9}L_{jj22}^{V,RR} \\
& - \frac{8}{9}L_{jj33}^{V,RR} - \frac{16}{9}L_{jjjj}^{V,LR} - \frac{8}{9}L_{kkjj}^{V,LR} - \frac{16}{3}L_{jjjj}^{V,RR} - \frac{32}{9}L_{jjkk}^{V,RR} + \frac{4}{3}L_{11ii}^{V,LL} \\
& + \frac{4}{3}L_{22ii}^{V,LL} + \frac{4}{3}L_{33ii}^{V,LL} + \frac{16}{9}L_{jj11}^{V,RR} + \frac{16}{9}L_{jj22}^{V,RR} + \frac{4}{3}L_{ii11}^{V1,LL} + \frac{4}{3}L_{ii22}^{V1,LL} \\
& + \frac{4}{3}L_{ii33}^{V1,LL} + \frac{4}{3}L_{ii11}^{V1,LR} + \frac{4}{3}L_{ii22}^{V1,LR} + \frac{4}{3}L_{ii33}^{V1,LR} + \frac{16}{9}L_{11jj}^{V,LR} + \frac{16}{9}L_{22jj}^{V,LR} \\
& + \frac{4}{3}L_{ii11}^{V,LR} + \frac{4}{3}L_{ii22}^{V,LR} + \frac{4}{3}L_{ii33}^{V,LR} + 8L_{ijjj}^{V,LR} - \frac{8}{3}L_{iii}^{V1,LR} - \frac{8}{3}L_{ikk}^{V1,LR} \\
& - \frac{64}{9}L_{iii}^{V,LL} - \frac{16}{3}L_{iik}^{V,LL} - \frac{16}{9}L_{ikk}^{V,LL} \Big] + \alpha_s^2 \Bigg[ 8L_{11jj}^{V,LR} + 8L_{22jj}^{V,LR} \\
& + 8L_{33jj}^{V,LR} - 8L_{jj11}^{V,RR} - 8L_{jj22}^{V,RR} - 8L_{jj33}^{V,RR} - 8L_{jj11}^{V,RR} - 8L_{jj22}^{V,RR} - 8L_{jj33}^{V,RR} \\
& + 8L_{11jj}^{V,LR} + 8L_{22jj}^{V,LR} \Big] + \alpha_s \alpha \Bigg[ -\frac{32}{9}L_{11jj}^{V,LR} - \frac{32}{9}L_{22jj}^{V,LR} - \frac{32}{9}L_{33jj}^{V,LR} \\
& - \frac{32}{9}L_{jj11}^{V,RR} - \frac{32}{9}L_{jj22}^{V,RR} - \frac{32}{9}L_{jj33}^{V,RR} + \frac{64}{9}L_{jj11}^{V,RR} + \frac{64}{9}L_{jj22}^{V,RR} + \frac{16}{3}L_{ii11}^{V1,LL} \\
& + \frac{16}{3}L_{ii22}^{V1,LL} + \frac{16}{3}L_{ii33}^{V1,LL} + \frac{16}{3}L_{ii11}^{V1,LR} + \frac{16}{3}L_{ii22}^{V1,LR} - \frac{32}{3}L_{ii33}^{V1,LR} + \frac{388}{243}L_{ii11}^{V8,LL} \\
& + \frac{388}{243}L_{ii22}^{V8,LL} + \frac{388}{243}L_{ii33}^{V8,LL} - \frac{332}{243}L_{ii11}^{V8,LR} - \frac{332}{243}L_{ii22}^{V8,LR} + \frac{2044}{243}L_{ii33}^{V8,LR} \\
& + \frac{64}{9}L_{11jj}^{V,LR} + \frac{64}{9}L_{22jj}^{V,LR} - 32L_{ijjj}^{V,LR} - \frac{32}{3}L_{iii}^{V1,LR} - \frac{32}{3}L_{iik}^{V1,LR} + \frac{2044}{243}L_{iii}^{V8,LR} \\
& + \frac{2044}{243}L_{iik}^{V8,LR} - \frac{2096}{81}L_{iii}^{V,LL} - 16L_{iik}^{V,LL} - \frac{128}{243}L_{ikk}^{V,LL} \Big] + \alpha^2 \Bigg[ \frac{1792}{243}L_{11jj}^{V,LR} \\
& + \frac{1792}{243}L_{22jj}^{V,LR} + \frac{1792}{243}L_{33jj}^{V,LR} + \frac{1168}{243}L_{jj11}^{V,RR} + \frac{1168}{243}L_{jj22}^{V,RR} + \frac{1168}{243}L_{jj33}^{V,RR}
\end{aligned}$$

$$\begin{aligned}
& + \frac{3616}{81} L_{jjjj}^{V,LR} + \frac{1808}{81} L_{kkjj}^{V,LR} + \frac{160}{9} L_{jjjj}^{V,RR} + \frac{896}{81} L_{jjkk}^{V,RR} - \frac{4744}{243} L_{11ii}^{V,LL} - \frac{4744}{243} L_{22ii}^{V,LL} \\
& - \frac{4744}{243} L_{33ii}^{V,LL} - \frac{1184}{243} L_{jj11}^{V,RR} - \frac{1184}{243} L_{jj22}^{V,RR} - \frac{3808}{243} L_{ii11}^{V1,LL} - \frac{3808}{243} L_{ii22}^{V1,LL} \\
& - \frac{3808}{243} L_{ii33}^{V1,LL} - \frac{1144}{243} L_{ii11}^{V1,LR} - \frac{1144}{243} L_{ii22}^{V1,LR} + \frac{12512}{243} L_{ii33}^{V1,LR} + \frac{1312}{243} L_{11jj}^{V,LR} \\
& + \frac{1312}{243} L_{22jj}^{V,LR} + \frac{3248}{243} L_{ii11}^{V,LR} + \frac{3248}{243} L_{ii22}^{V,LR} + \frac{3248}{243} L_{ii33}^{V,LR} - \frac{4960}{27} L_{iijj}^{V,LR} \\
& + \frac{12224}{243} L_{uu}^{V1,LR} + \frac{12224}{243} L_{ii}^{V1,LR} + \frac{3808}{243} L_{uu}^{V,LL} + \frac{3136}{243} L_{ii}^{V,LL} + \frac{1024}{729} L_{ikki}^{V,LL} \Bigg] ;
\end{aligned}$$

$$\begin{aligned}
\dot{L}_{\nu e}^{V,LR} = & e^2 \left[ \frac{4}{3} L_{ii11}^{V,LL} + \frac{4}{3} L_{ii22}^{V,LL} + \frac{4}{3} L_{ii33}^{V,LL} + \frac{4}{3} L_{ii11}^{V,LR} + \frac{4}{3} L_{ii22}^{V,LR} \right. \\
& + \frac{4}{3} L_{ii33}^{V,LR} + \frac{4}{3} L_{ii11}^{V,LL} + \frac{4}{3} L_{ii22}^{V,LL} + \frac{4}{3} L_{ii33}^{V,LL} + \frac{4}{3} L_{ii11}^{V,LR} + \frac{4}{3} L_{ii22}^{V,LR} + \frac{4}{3} L_{ii33}^{V,LR} \\
& \left. + \frac{4}{3} L_{ii33}^{V,LR} - \frac{8}{3} L_{ii11}^{V,LL} - \frac{8}{3} L_{ii22}^{V,LL} - \frac{8}{3} L_{ii11}^{V,LR} - \frac{8}{3} L_{ii22}^{V,LR} \right] \\
& + \alpha_s \alpha \left[ \frac{16}{3} L_{ii11}^{V,LL} + \frac{16}{3} L_{ii22}^{V,LL} + \frac{16}{3} L_{ii33}^{V,LL} + \frac{16}{3} L_{ii11}^{V,LR} + \frac{16}{3} L_{ii22}^{V,LR} \right. \\
& \left. + \frac{16}{3} L_{ii33}^{V,LR} - \frac{32}{3} L_{ii11}^{V,LL} - \frac{32}{3} L_{ii22}^{V,LL} - \frac{32}{3} L_{ii11}^{V,LR} - \frac{32}{3} L_{ii22}^{V,LR} \right] \\
& + \alpha^2 \left[ -\frac{32}{9} L_{ii11}^{V,LL} - \frac{32}{9} L_{ii22}^{V,LL} - \frac{32}{9} L_{ii33}^{V,LL} + \frac{40}{9} L_{ii11}^{V,LR} + \frac{40}{9} L_{ii22}^{V,LR} \right. \\
& + \frac{40}{9} L_{ii33}^{V,LR} - 8 L_{ii11}^{V,LL} - 8 L_{ii22}^{V,LL} - 8 L_{ii33}^{V,LL} + 16 L_{ii11}^{V,LR} + 16 L_{ii22}^{V,LR} \\
& \left. + 16 L_{ii33}^{V,LR} - \frac{176}{9} L_{ii11}^{V,LL} - \frac{176}{9} L_{ii22}^{V,LL} + \frac{112}{9} L_{ii11}^{V,LR} + \frac{112}{9} L_{ii22}^{V,LR} \right] ;
\end{aligned}$$

$$\begin{aligned}
\dot{L}_{\nu d}^{V,LR} = & e^2 \left[ \frac{4}{9} L_{ii11}^{V,LL} + \frac{4}{9} L_{ii22}^{V,LL} + \frac{4}{9} L_{ii33}^{V,LL} + \frac{4}{9} L_{ii11}^{V,LR} + \frac{4}{9} L_{ii22}^{V,LR} \right. \\
& + \frac{4}{9} L_{ii33}^{V,LR} + \frac{4}{9} L_{ii11}^{V,LL} + \frac{4}{9} L_{ii22}^{V,LL} + \frac{4}{9} L_{ii33}^{V,LL} + \frac{4}{9} L_{ii11}^{V,LR} + \frac{4}{9} L_{ii22}^{V,LR} + \frac{4}{9} L_{ii33}^{V,LR} \\
& \left. + \frac{4}{9} L_{ii33}^{V,LR} - \frac{8}{9} L_{ii11}^{V,LL} - \frac{8}{9} L_{ii22}^{V,LL} - \frac{8}{9} L_{ii11}^{V,LR} - \frac{8}{9} L_{ii22}^{V,LR} \right]
\end{aligned}$$

$$\begin{aligned}
& + \alpha_s^2 \left[ -8L_{\nu d, ii11}^{V,LL} - 8L_{\nu d, ii22}^{V,LL} - 8L_{\nu d, ii33}^{V,LL} + 8L_{\nu d, ii11}^{V,LR} + 8L_{\nu d, ii22}^{V,LR} \right. \\
& \left. + 8L_{\nu d, ii33}^{V,LR} - 8L_{\nu u, ii11}^{V,LL} - 8L_{\nu u, ii22}^{V,LL} + 8L_{\nu u, ii11}^{V,LR} + 8L_{\nu u, ii22}^{V,LR} \right] \\
& + \alpha_s \alpha \left[ \frac{16}{9}L_{\nu d, ii11}^{V,LL} + \frac{16}{9}L_{\nu d, ii22}^{V,LL} + \frac{16}{9}L_{\nu d, ii33}^{V,LL} + \frac{16}{9}L_{\nu d, ii11}^{V,LR} + \frac{16}{9}L_{\nu d, ii22}^{V,LR} \right. \\
& \left. + \frac{16}{9}L_{\nu d, ii33}^{V,LR} - \frac{32}{9}L_{\nu u, ii11}^{V,LL} - \frac{32}{9}L_{\nu u, ii22}^{V,LL} - \frac{32}{9}L_{\nu u, ii11}^{V,LR} - \frac{32}{9}L_{\nu u, ii22}^{V,LR} \right] \\
& + \alpha^2 \left[ -\frac{8}{27}L_{\nu d, ii11}^{V,LL} - \frac{8}{27}L_{\nu d, ii22}^{V,LL} - \frac{8}{27}L_{\nu d, ii33}^{V,LL} + \frac{16}{27}L_{\nu d, ii11}^{V,LR} + \frac{16}{27}L_{\nu d, ii22}^{V,LR} \right. \\
& + \frac{16}{27}L_{\nu d, ii33}^{V,LR} + \frac{8}{3}L_{\nu e, ii11}^{V,LR} + \frac{8}{3}L_{\nu e, ii22}^{V,LR} + \frac{8}{3}L_{\nu e, ii33}^{V,LR} - \frac{80}{27}L_{\nu u, ii11}^{V,LL} - \frac{80}{27}L_{\nu u, ii22}^{V,LL} \\
& \left. + \frac{16}{27}L_{\nu u, ii11}^{V,LR} + \frac{16}{27}L_{\nu u, ii22}^{V,LR} \right];
\end{aligned}$$

$$\begin{aligned}
\dot{L}_{\nu u, ij j}^{V,LR} &= e^2 \left[ -\frac{8}{9}L_{\nu d, ii11}^{V,LL} - \frac{8}{9}L_{\nu d, ii22}^{V,LL} - \frac{8}{9}L_{\nu d, ii33}^{V,LL} - \frac{8}{9}L_{\nu d, ii11}^{V,LR} - \frac{8}{9}L_{\nu d, ii22}^{V,LR} \right. \\
& - \frac{8}{9}L_{\nu d, ii33}^{V,LR} - \frac{8}{9}L_{\nu e, ii11}^{V,LL} - \frac{8}{9}L_{\nu e, ii22}^{V,LL} - \frac{8}{9}L_{\nu e, ii33}^{V,LL} - \frac{8}{9}L_{\nu e, ii11}^{V,LR} - \frac{8}{9}L_{\nu e, ii22}^{V,LR} \\
& \left. - \frac{8}{9}L_{\nu e, ii33}^{V,LR} + \frac{16}{9}L_{\nu u, ii11}^{V,LL} + \frac{16}{9}L_{\nu u, ii22}^{V,LL} + \frac{16}{9}L_{\nu u, ii11}^{V,LR} + \frac{16}{9}L_{\nu u, ii22}^{V,LR} \right] \\
& + \alpha_s^2 \left[ -8L_{\nu d, ii11}^{V,LL} - 8L_{\nu d, ii22}^{V,LL} - 8L_{\nu d, ii33}^{V,LL} + 8L_{\nu d, ii11}^{V,LR} + 8L_{\nu d, ii22}^{V,LR} \right. \\
& \left. + 8L_{\nu d, ii33}^{V,LR} - 8L_{\nu u, ii11}^{V,LL} - 8L_{\nu u, ii22}^{V,LL} + 8L_{\nu u, ii11}^{V,LR} + 8L_{\nu u, ii22}^{V,LR} \right] \\
& + \alpha_s \alpha \left[ -\frac{32}{9}L_{\nu d, ii11}^{V,LL} - \frac{32}{9}L_{\nu d, ii22}^{V,LL} - \frac{32}{9}L_{\nu d, ii33}^{V,LL} - \frac{32}{9}L_{\nu d, ii11}^{V,LR} - \frac{32}{9}L_{\nu d, ii22}^{V,LR} \right. \\
& \left. - \frac{32}{9}L_{\nu d, ii33}^{V,LR} + \frac{64}{9}L_{\nu u, ii11}^{V,LL} + \frac{64}{9}L_{\nu u, ii22}^{V,LL} + \frac{64}{9}L_{\nu u, ii11}^{V,LR} + \frac{64}{9}L_{\nu u, ii22}^{V,LR} \right] \\
& + \alpha^2 \left[ -\frac{56}{27}L_{\nu d, ii11}^{V,LL} - \frac{56}{27}L_{\nu d, ii22}^{V,LL} - \frac{56}{27}L_{\nu d, ii33}^{V,LL} + \frac{40}{27}L_{\nu d, ii11}^{V,LR} + \frac{40}{27}L_{\nu d, ii22}^{V,LR} \right.
\end{aligned}$$

$$\begin{aligned}
& + \frac{40}{27} L_{\nu d, i33}^{V,LR} - 8 L_{\nu e, i11}^{V,LL} - 8 L_{\nu e, i22}^{V,LL} - 8 L_{\nu e, i33}^{V,LL} + \frac{8}{3} L_{\nu e, i11}^{V,LR} + \frac{8}{3} L_{\nu e, i22}^{V,LR} \\
& + \frac{8}{3} L_{\nu e, i33}^{V,LR} - \frac{128}{27} L_{\nu u, i11}^{V,LL} - \frac{128}{27} L_{\nu u, i22}^{V,LL} + \frac{256}{27} L_{\nu u, i11}^{V,LR} + \frac{256}{27} L_{\nu u, i22}^{V,LR} \Big] ; \\
\dot{L}_{du, ij}^{V1,LR} = & - \frac{8}{3} L_{du, ij}^{V8,LR} g_s^2 + e^2 \Bigg[ - \frac{8}{9} L_{dd, iii}^{V1,LR} - \frac{8}{9} L_{dd, ijj}^{V1,LR} - \frac{8}{9} L_{dd, ikk}^{V1,LR} - \frac{64}{27} L_{dd, iii}^{V,LL} \\
& - \frac{16}{9} L_{dd, ijj}^{V,LL} - \frac{16}{9} L_{dd, ikk}^{V,LL} - \frac{16}{27} L_{dd, ijj}^{V,LL} - \frac{16}{27} L_{dd, ikk}^{V,LL} - \frac{8}{9} L_{de, i11}^{V,LR} - \frac{8}{9} L_{de, i22}^{V,LR} \\
& - \frac{8}{9} L_{de, i33}^{V,LR} + \frac{4}{9} L_{11jj}^{V1,LR} + \frac{4}{9} L_{22jj}^{V1,LR} + \frac{4}{9} L_{33jj}^{V1,LR} + \frac{16}{9} L_{du, i11}^{V1,LR} + \frac{16}{9} L_{du, i22}^{V1,LR} \\
& + \frac{8}{3} L_{du, ijj}^{V1,LR} - \frac{8}{9} L_{ed, 11ii}^{V,LL} - \frac{8}{9} L_{ed, 22ii}^{V,LL} - \frac{8}{9} L_{ed, 33ii}^{V,LL} + \frac{4}{9} L_{eu, 11jj}^{V,LR} + \frac{4}{9} L_{eu, 22jj}^{V,LR} \\
& + \frac{4}{9} L_{eu, 33jj}^{V,LR} + \frac{4}{9} L_{eu, 11jj}^{V,RR} + \frac{4}{9} L_{eu, 22jj}^{V,RR} + \frac{4}{9} L_{eu, 33jj}^{V,RR} + \frac{16}{9} L_{ud, 11ii}^{V1,LL} + \frac{16}{9} L_{ud, 22ii}^{V1,LL} \\
& + \frac{4}{9} L_{ud, jj11}^{V1,RR} + \frac{4}{9} L_{ud, jj22}^{V1,RR} + \frac{4}{9} L_{ud, jj33}^{V1,RR} - \frac{8}{9} L_{jjjj}^{V1,LR} - \frac{8}{9} L_{kkjj}^{V1,LR} - \frac{64}{27} L_{jjjj}^{V,RR} \\
& - \frac{16}{9} L_{uu, jjkk}^{V,RR} - \frac{16}{27} L_{uu, jjkk}^{V,RR} \Big] + \alpha_s^2 \Bigg[ 8 L_{dd, iii}^{V1,LR} + 8 L_{dd, ijj}^{V1,LR} + 8 L_{dd, ikk}^{V1,LR} \\
& + \frac{44}{27} L_{dd, iii}^{V8,LR} + \frac{44}{27} L_{dd, ijj}^{V8,LR} + \frac{44}{27} L_{dd, ikk}^{V8,LR} - \frac{232}{9} L_{dd, iii}^{V,LL} - 16 L_{dd, ijj}^{V,LL} - 16 L_{dd, ikk}^{V,LL} \\
& - \frac{64}{27} L_{dd, ijj}^{V,LL} - \frac{64}{27} L_{dd, ikk}^{V,LL} + 8 L_{du, 11jj}^{V1,LR} + 8 L_{du, 22jj}^{V1,LR} + 8 L_{du, 33jj}^{V1,LR} + 8 L_{du, i11}^{V1,LR} \\
& + 8 L_{du, i22}^{V1,LR} - \frac{28}{3} L_{du, ijj}^{V1,LR} + \frac{44}{27} L_{du, 11jj}^{V8,LR} + \frac{44}{27} L_{du, 22jj}^{V8,LR} + \frac{44}{27} L_{du, 33jj}^{V8,LR} + \frac{44}{27} L_{du, i11}^{V8,LR} \\
& + \frac{44}{27} L_{du, i22}^{V8,LR} - \frac{2044}{27} L_{du, ijj}^{V8,LR} - 8 L_{ud, 11ii}^{V1,LL} - 8 L_{ud, 22ii}^{V1,LL} - 8 L_{ud, jj11}^{V1,RR} - 8 L_{ud, jj22}^{V1,RR} \\
& - 8 L_{ud, jj33}^{V1,RR} + \frac{44}{27} L_{ud, 11ii}^{V8,LL} + \frac{44}{27} L_{ud, 22ii}^{V8,LL} + \frac{44}{27} L_{ud, jj11}^{V8,RR} + \frac{44}{27} L_{ud, jj22}^{V8,RR} + \frac{44}{27} L_{ud, jj33}^{V8,RR} \\
& + 8 L_{uu, jjjj}^{V1,LR} + 8 L_{uu, kkjj}^{V1,LR} + \frac{44}{27} L_{uu, jjjj}^{V8,LR} + \frac{44}{27} L_{uu, kkjj}^{V8,LR} - \frac{232}{9} L_{uu, jjjj}^{V,RR} - 16 L_{uu, jjkk}^{V,RR} \\
& - \frac{64}{27} L_{uu, jjkk}^{V,RR} \Big] + \alpha_s \alpha \Bigg[ - \frac{32}{9} L_{dd, iii}^{V1,LR} - \frac{32}{9} L_{dd, ijj}^{V1,LR} - \frac{32}{9} L_{dd, ikk}^{V1,LR} + \frac{2080}{729} L_{dd, iii}^{V8,LR} \\
& + \frac{2080}{729} L_{dd, ijj}^{V8,LR} + \frac{2080}{729} L_{dd, ikk}^{V8,LR} - \frac{2048}{243} L_{dd, iii}^{V,LL} - \frac{16}{3} L_{dd, ijj}^{V,LL} - \frac{16}{3} L_{dd, ikk}^{V,LL} + \frac{16}{729} L_{dd, ijj}^{V,LL} \\
& + \frac{16}{729} L_{dd, ikk}^{V,LL} + \frac{16}{729} L_{dd, ijj}^{V,LL} + \frac{16}{729} L_{dd, ikk}^{V,LL} \Big]
\end{aligned}$$

$$\begin{aligned}
& + \frac{16}{729} L_{ikki}^{V,LL} + \frac{16}{9} L_{11jj}^{V1,LR} + \frac{16}{9} L_{22jj}^{V1,LR} - \frac{32}{9} L_{33jj}^{V1,LR} + \frac{64}{9} L_{ii11}^{V1,LR} + \frac{64}{9} L_{ii22}^{V1,LR} \\
& - \frac{64}{3} L_{iijj}^{V1,LR} - \frac{332}{729} L_{11jj}^{V8,LR} - \frac{332}{729} L_{22jj}^{V8,LR} + \frac{2044}{729} L_{33jj}^{V8,LR} - \frac{2672}{729} L_{ii11}^{V8,LR} \\
& - \frac{2672}{729} L_{ii22}^{V8,LR} + \frac{232}{27} L_{iijj}^{V8,LR} + \frac{64}{9} L_{11ii}^{V1,LL} + \frac{64}{9} L_{22ii}^{V1,LL} + \frac{16}{9} L_{jj11}^{V1,RR} + \frac{16}{9} L_{jj22}^{V1,RR} \\
& + \frac{16}{9} L_{jj33}^{V1,RR} + \frac{208}{729} L_{11ii}^{V8,LL} + \frac{208}{729} L_{22ii}^{V8,LL} + \frac{388}{729} L_{jj11}^{V8,RR} + \frac{388}{729} L_{jj22}^{V8,RR} \\
& + \frac{388}{729} L_{jj33}^{V8,RR} - \frac{32}{9} L_{jjjj}^{V1,LR} - \frac{32}{9} L_{kkjj}^{V1,LR} + \frac{2044}{729} L_{jjjj}^{V8,LR} + \frac{2044}{729} L_{kkjj}^{V8,LR} \\
& - \frac{2096}{243} L_{jjjj}^{V,RR} - \frac{16}{3} L_{jjkk}^{V,RR} - \frac{128}{729} L_{jkkj}^{V,RR} \Big] + \alpha^2 \Big[ \frac{3776}{729} L_{ddii}^{V1,LR} + \frac{3776}{729} L_{iijj}^{V1,LR} \\
& + \frac{3776}{729} L_{ddkk}^{V1,LR} + \frac{880}{729} L_{ddii}^{V,LL} + \frac{928}{729} L_{ddij}^{V,LL} + \frac{928}{729} L_{ddkk}^{V,LL} - \frac{32}{2187} L_{ijji}^{V,LL} \\
& - \frac{32}{2187} L_{ddkk}^{V,LL} + \frac{6224}{729} L_{de11}^{V,LR} + \frac{6224}{729} L_{de22}^{V,LR} + \frac{6224}{729} L_{de33}^{V,LR} - \frac{208}{729} L_{11jj}^{V1,LR} \\
& - \frac{208}{729} L_{22jj}^{V1,LR} + \frac{6752}{729} L_{33jj}^{V1,LR} + \frac{6272}{729} L_{ii11}^{V1,LR} + \frac{6272}{729} L_{ii22}^{V1,LR} - \frac{4048}{81} L_{iijj}^{V1,LR} \\
& - \frac{3712}{729} L_{11ii}^{V,LL} - \frac{3712}{729} L_{22ii}^{V,LL} - \frac{3712}{729} L_{33ii}^{V,LL} + \frac{2888}{729} L_{11jj}^{V,LR} + \frac{2888}{729} L_{22jj}^{V,LR} \\
& + \frac{2888}{729} L_{33jj}^{V,LR} - \frac{1216}{729} L_{11jj}^{V,RR} - \frac{1216}{729} L_{22jj}^{V,RR} - \frac{1216}{729} L_{33jj}^{V,RR} - \frac{6976}{729} L_{11ii}^{V1,LL} \\
& - \frac{6976}{729} L_{22ii}^{V1,LL} - \frac{1576}{729} L_{jj11}^{V1,RR} - \frac{1576}{729} L_{jj22}^{V1,RR} - \frac{1576}{729} L_{jj33}^{V1,RR} + \frac{6464}{729} L_{jjjj}^{V1,LR} \\
& + \frac{6464}{729} L_{kkjj}^{V1,LR} + \frac{4384}{729} L_{jjjj}^{V,RR} + \frac{1984}{729} L_{jkkk}^{V,RR} + \frac{3328}{2187} L_{jkkj}^{V,RR} \Big] ;
\end{aligned}$$

$$\begin{aligned}
\dot{L}_{iijj}^{V8,LR} &= g_s^2 \Big[ \frac{2}{3} L_{iii}^{V8,LR} + \frac{2}{3} L_{iijj}^{V8,LR} + \frac{2}{3} L_{iikk}^{V8,LR} + \frac{8}{3} L_{iii}^{V,LL} + \frac{8}{3} L_{iijj}^{V,LL} \\
& + \frac{8}{3} L_{ikki}^{V,LL} - 12 L_{iijj}^{V1,LR} + \frac{2}{3} L_{11jj}^{V8,LR} + \frac{2}{3} L_{22jj}^{V8,LR} + \frac{2}{3} L_{33jj}^{V8,LR} + \frac{2}{3} L_{ii11}^{V8,LR} \\
& + \frac{2}{3} L_{ii22}^{V8,LR} - 14 L_{iijj}^{V8,LR} + \frac{2}{3} L_{11ii}^{V8,LL} + \frac{2}{3} L_{22ii}^{V8,LL} + \frac{2}{3} L_{jj11}^{V8,RR} + \frac{2}{3} L_{jj22}^{V8,RR} \\
& + \frac{2}{3} L_{jj33}^{V8,RR} + \frac{2}{3} L_{jjjj}^{V8,LR} + \frac{2}{3} L_{kkjj}^{V8,LR} + \frac{8}{3} L_{jjjj}^{V,RR} + \frac{8}{3} L_{jkkj}^{V,RR} \Big] + \frac{8}{3} L_{iijj}^{V8,LR}
\end{aligned}$$

$$\begin{aligned}
& e^2 + \alpha_s^2 \left[ -\frac{22}{3} L_{\overline{iii}}^{V1,LR} - \frac{22}{3} L_{\overline{ijj}}^{V1,LR} - \frac{22}{3} L_{\overline{ikk}}^{V1,LR} + \frac{769}{81} L_{\overline{iii}}^{V8,LR} + \frac{769}{81} L_{\overline{ijj}}^{V8,LR} \right. \\
& + \frac{769}{81} L_{\overline{ikk}}^{V8,LR} + \frac{1174}{27} L_{\overline{iii}}^{V,LL} - \frac{28}{3} L_{\overline{ijj}}^{V,LL} - \frac{28}{3} L_{\overline{ikk}}^{V,LL} + \frac{3376}{81} L_{\overline{ijji}}^{V,LL} + \frac{3376}{81} L_{\overline{ikki}}^{V,LL} \\
& - \frac{22}{3} L_{\overline{11jj}}^{V1,LR} - \frac{22}{3} L_{\overline{22jj}}^{V1,LR} - \frac{22}{3} L_{\overline{33jj}}^{V1,LR} - \frac{22}{3} L_{\overline{ii11}}^{V1,LR} - \frac{22}{3} L_{\overline{ii22}}^{V1,LR} - \frac{374}{3} L_{\overline{ijjj}}^{V1,LR} \\
& + \frac{787}{81} L_{\overline{11jj}}^{V8,LR} + \frac{787}{81} L_{\overline{22jj}}^{V8,LR} + \frac{787}{81} L_{\overline{33jj}}^{V8,LR} + \frac{769}{81} L_{\overline{ii11}}^{V8,LR} + \frac{769}{81} L_{\overline{ii22}}^{V8,LR} - \frac{2975}{18} L_{\overline{ijjj}}^{V8,LR} \\
& - \frac{2}{3} L_{\overline{11ii}}^{V1,LL} - \frac{2}{3} L_{\overline{22ii}}^{V1,LL} - \frac{2}{3} L_{\overline{jj11}}^{V1,RR} - \frac{2}{3} L_{\overline{jj22}}^{V1,RR} - \frac{2}{3} L_{\overline{jj33}}^{V1,RR} + \frac{589}{81} L_{\overline{11ii}}^{V8,LL} \\
& + \frac{589}{81} L_{\overline{22ii}}^{V8,LL} + \frac{607}{81} L_{\overline{jj11}}^{V8,RR} + \frac{607}{81} L_{\overline{jj22}}^{V8,RR} + \frac{607}{81} L_{\overline{jj33}}^{V8,RR} - \frac{22}{3} L_{\overline{jjjj}}^{V1,LR} - \frac{22}{3} L_{\overline{kkjj}}^{V1,LR} \\
& + \left. \frac{787}{81} L_{\overline{jjjj}}^{V8,LR} + \frac{787}{81} L_{\overline{kkjj}}^{V8,LR} + \frac{1198}{27} L_{\overline{jjjj}}^{V,RR} - \frac{28}{3} L_{\overline{jjkk}}^{V,RR} + \frac{3448}{81} L_{\overline{jjkk}}^{V,RR} \right] \\
& + \alpha_s \alpha \left[ -\frac{916}{81} L_{\overline{iii}}^{V1,LR} - \frac{916}{81} L_{\overline{ijj}}^{V1,LR} - \frac{916}{81} L_{\overline{ikk}}^{V1,LR} - \frac{44}{9} L_{\overline{iii}}^{V8,LR} - \frac{44}{9} L_{\overline{ijj}}^{V8,LR} \right. \\
& - \frac{44}{9} L_{\overline{ikk}}^{V8,LR} - \frac{2144}{81} L_{\overline{iii}}^{V,LL} - \frac{1832}{81} L_{\overline{ijj}}^{V,LL} - \frac{1832}{81} L_{\overline{ikk}}^{V,LL} + \frac{664}{243} L_{\overline{ijji}}^{V,LL} + \frac{664}{243} L_{\overline{ikki}}^{V,LL} \\
& - \frac{916}{81} L_{\overline{ii11}}^{V,LR} - \frac{916}{81} L_{\overline{de22}}^{V,LR} - \frac{916}{81} L_{\overline{ii33}}^{V,LR} + \frac{644}{81} L_{\overline{11jj}}^{V1,LR} + \frac{644}{81} L_{\overline{22jj}}^{V1,LR} - \frac{1216}{81} L_{\overline{33jj}}^{V1,LR} \\
& + \frac{1832}{81} L_{\overline{ii11}}^{V1,LR} + \frac{1832}{81} L_{\overline{ii22}}^{V1,LR} + \frac{116}{3} L_{\overline{iijj}}^{V1,LR} + \frac{14}{9} L_{\overline{11jj}}^{V8,LR} + \frac{14}{9} L_{\overline{22jj}}^{V8,LR} - \frac{20}{3} L_{\overline{33jj}}^{V8,LR} \\
& + \frac{56}{9} L_{\overline{ii11}}^{V8,LR} + \frac{56}{9} L_{\overline{ii22}}^{V8,LR} + \frac{187}{9} L_{\overline{iijj}}^{V8,LR} - \frac{916}{81} L_{\overline{11ii}}^{V,LL} - \frac{916}{81} L_{\overline{22ii}}^{V,LL} - \frac{916}{81} L_{\overline{33ii}}^{V,LL} \\
& + \frac{644}{81} L_{\overline{11jj}}^{V,LR} + \frac{644}{81} L_{\overline{22jj}}^{V,LR} + \frac{644}{81} L_{\overline{33jj}}^{V,LR} + \frac{644}{81} L_{\overline{11jj}}^{V,RR} + \frac{644}{81} L_{\overline{22jj}}^{V,RR} + \frac{644}{81} L_{\overline{33jj}}^{V,RR} \\
& + \frac{1832}{81} L_{\overline{11ii}}^{V1,LL} + \frac{1832}{81} L_{\overline{22ii}}^{V1,LL} + \frac{644}{81} L_{\overline{jj11}}^{V1,RR} + \frac{644}{81} L_{\overline{jj22}}^{V1,RR} + \frac{644}{81} L_{\overline{jj33}}^{V1,RR} \\
& - \frac{160}{27} L_{\overline{11ii}}^{V8,LL} - \frac{160}{27} L_{\overline{22ii}}^{V8,LL} - \frac{70}{27} L_{\overline{jj11}}^{V8,RR} - \frac{70}{27} L_{\overline{jj22}}^{V8,RR} - \frac{70}{27} L_{\overline{jj33}}^{V8,RR} - \frac{1288}{81} L_{\overline{jjjj}}^{V1,LR} \\
& - \frac{1288}{81} L_{\overline{kkjj}}^{V1,LR} - \frac{20}{3} L_{\overline{jjjj}}^{V8,LR} - \frac{20}{3} L_{\overline{kkjj}}^{V8,LR} - \frac{3608}{81} L_{\overline{jjjj}}^{V,RR} - \frac{2576}{81} L_{\overline{jjkk}}^{V,RR} - \frac{800}{243} L_{\overline{jjkk}}^{V,RR} \left. \right] \\
& - \frac{4048}{81} L_{\overline{ijjj}}^{V8,LR} \alpha^2 ;
\end{aligned}$$

$$\begin{aligned}
\dot{L}_{de}^{V,LR}{}_{jji} &= e^2 \left[ \frac{8}{3} L_{dd}^{V1,LR}{}_{jjj} + \frac{4}{3} L_{jjkk}^{V1,LR} + \frac{64}{9} L_{jjjj}^{V,LL} + \frac{8}{3} L_{jjkk}^{V,LL} + \frac{8}{9} L_{jjkk}^{V,LL} \right. \\
&\quad + \frac{4}{9} L_{11ii}^{V,LR} + \frac{4}{9} L_{22ii}^{V,LR} + \frac{4}{9} L_{33ii}^{V,LR} + \frac{4}{3} L_{jj11}^{V,LR} + \frac{4}{3} L_{jj22}^{V,LR} + \frac{4}{3} L_{jj33}^{V,LR} \\
&\quad - 4 L_{jjii}^{V,LR} - \frac{8}{3} L_{jj11}^{V1,LR} - \frac{8}{3} L_{jj22}^{V1,LR} + \frac{4}{3} L_{11jj}^{V,LL} + \frac{4}{3} L_{22jj}^{V,LL} + \frac{4}{3} L_{33jj}^{V,LL} \\
&\quad + \frac{4}{9} L_{ii11}^{V,RR} + \frac{4}{9} L_{ii22}^{V,RR} + \frac{4}{9} L_{ii33}^{V,RR} + \frac{4}{9} L_{jjii}^{V,RR} + \frac{4}{9} L_{jjii}^{V,RR} + \frac{4}{9} L_{kkii}^{V,RR} \\
&\quad + \frac{16}{9} L_{iii}^{V,RR} + \frac{16}{9} L_{jjj}^{V,RR} + \frac{16}{9} L_{kkk}^{V,RR} - \frac{8}{9} L_{ii11}^{V,RR} - \frac{8}{9} L_{ii22}^{V,RR} - \frac{8}{3} L_{11jj}^{V1,LL} \\
&\quad - \frac{8}{3} L_{22jj}^{V1,LL} - \frac{8}{9} L_{11ii}^{V,LR} - \frac{8}{9} L_{22ii}^{V,LR} \left. \right] + \alpha_s^2 \left[ 8 L_{11ii}^{V,LR} + 8 L_{22ii}^{V,LR} \right. \\
&\quad + 8 L_{33ii}^{V,LR} - 8 L_{ii11}^{V,RR} - 8 L_{ii22}^{V,RR} - 8 L_{ii33}^{V,RR} - 8 L_{ii11}^{V,RR} - 8 L_{ii22}^{V,RR} \\
&\quad + 8 L_{11ii}^{V,LR} + 8 L_{22ii}^{V,LR} \left. \right] + \alpha_s \alpha \left[ \frac{32}{3} L_{jjj}^{V1,LR} + \frac{16}{3} L_{jjkk}^{V1,LR} - \frac{2080}{243} L_{jjj}^{V8,LR} \right. \\
&\quad - \frac{1040}{243} L_{jjkk}^{V8,LR} + \frac{5008}{243} L_{jjjj}^{V,LL} + 8 L_{jjkk}^{V,LL} - \frac{8}{243} L_{jjkk}^{V,LL} + \frac{16}{9} L_{11ii}^{V,LR} + \frac{16}{9} L_{22ii}^{V,LR} \\
&\quad + \frac{16}{9} L_{33ii}^{V,LR} + 16 L_{jjii}^{V,LR} - \frac{32}{3} L_{jj11}^{V1,LR} - \frac{32}{3} L_{jj22}^{V1,LR} + \frac{1336}{243} L_{jj11}^{V8,LR} + \frac{1336}{243} L_{jj22}^{V8,LR} \\
&\quad + \frac{16}{9} L_{ii11}^{V,RR} + \frac{16}{9} L_{ii22}^{V,RR} + \frac{16}{9} L_{ii33}^{V,RR} - \frac{32}{9} L_{ii11}^{V,RR} - \frac{32}{9} L_{ii22}^{V,RR} - \frac{32}{3} L_{11jj}^{V1,LL} \\
&\quad - \frac{32}{3} L_{22jj}^{V1,LL} - \frac{104}{243} L_{11jj}^{V8,LL} - \frac{104}{243} L_{22jj}^{V8,LL} - \frac{32}{9} L_{11ii}^{V,LR} - \frac{32}{9} L_{22ii}^{V,LR} \left. \right] \\
&\quad + \alpha^2 \left[ \frac{3424}{243} L_{jjj}^{V1,LR} + \frac{1712}{243} L_{jjkk}^{V1,LR} - \frac{3056}{729} L_{jjjj}^{V,LL} + \frac{256}{243} L_{jjkk}^{V,LL} - \frac{1424}{729} L_{jjkk}^{V,LL} \right. \\
&\quad - \frac{104}{243} L_{11ii}^{V,LR} - \frac{104}{243} L_{22ii}^{V,LR} - \frac{104}{243} L_{33ii}^{V,LR} + \frac{3728}{243} L_{jj11}^{V,LR} + \frac{3728}{243} L_{jj22}^{V,LR} \\
&\quad + \frac{3728}{243} L_{jj33}^{V,LR} + \frac{1994}{27} L_{jjii}^{V,LR} - \frac{616}{243} L_{jj11}^{V1,LR} - \frac{616}{243} L_{jj22}^{V1,LR} - \frac{1024}{243} L_{11jj}^{V,LL} \\
&\quad - \frac{1024}{243} L_{22jj}^{V,LL} - \frac{1024}{243} L_{33jj}^{V,LL} - \frac{440}{243} L_{ii11}^{V,RR} - \frac{440}{243} L_{ii22}^{V,RR} - \frac{440}{243} L_{ii33}^{V,RR} \\
&\quad - \frac{184}{81} L_{iii}^{V,LR} - \frac{184}{81} L_{jjj}^{V,LR} - \frac{184}{81} L_{kkk}^{V,LR} - \frac{640}{81} L_{iii}^{V,RR} - \frac{160}{81} L_{jjj}^{V,RR} - \frac{160}{81} L_{kkk}^{V,RR} \left. \right]
\end{aligned}$$

$$\begin{aligned}
& -\frac{1640}{243}L_{\substack{eu \\ ii11}}^{V,RR} - \frac{1640}{243}L_{\substack{eu \\ ii22}}^{V,RR} - \frac{6952}{243}L_{\substack{ud \\ 11jj}}^{V1,LL} - \frac{6952}{243}L_{\substack{ud \\ 22jj}}^{V1,LL} - \frac{296}{243}L_{\substack{ue \\ 11ii}}^{V,LR} \\
& - \frac{296}{243}L_{\substack{ue \\ 22ii}}^{V,LR} \Big] ; \\
\dot{L}_{\substack{ue \\ jjii}}^{V,LR} = & e^2 \Bigg[ -\frac{8}{9}L_{\substack{de \\ 11ii}}^{V,LR} - \frac{8}{9}L_{\substack{de \\ 22ii}}^{V,LR} - \frac{8}{9}L_{\substack{de \\ 33ii}}^{V,LR} - \frac{8}{9}L_{\substack{ed \\ ii11}}^{V,RR} - \frac{8}{9}L_{\substack{ed \\ ii22}}^{V,RR} \\
& - \frac{8}{9}L_{\substack{ed \\ ii33}}^{V,RR} - \frac{8}{9}L_{\substack{ee \\ iii}}^{V,LR} - \frac{8}{9}L_{\substack{ee \\ jjii}}^{V,LR} - \frac{8}{9}L_{\substack{ee \\ kkii}}^{V,LR} - \frac{32}{9}L_{\substack{ee \\ iii}}^{V,RR} - \frac{32}{9}L_{\substack{ee \\ iijj}}^{V,RR} \\
& - \frac{32}{9}L_{\substack{ee \\ iikk}}^{V,RR} + \frac{4}{3}L_{\substack{eu \\ 11jj}}^{V,LL} + \frac{4}{3}L_{\substack{eu \\ 22jj}}^{V,LL} + \frac{4}{3}L_{\substack{eu \\ 33jj}}^{V,LL} + \frac{16}{9}L_{\substack{eu \\ ii11}}^{V,RR} + \frac{16}{9}L_{\substack{eu \\ ii22}}^{V,RR} \\
& + \frac{4}{3}L_{\substack{ud \\ jj11}}^{V1,LL} + \frac{4}{3}L_{\substack{ud \\ jj22}}^{V1,LL} + \frac{4}{3}L_{\substack{ud \\ jj33}}^{V1,LL} + \frac{4}{3}L_{\substack{ud \\ jj11}}^{V1,LR} + \frac{4}{3}L_{\substack{ud \\ jj22}}^{V1,LR} + \frac{4}{3}L_{\substack{ud \\ jj33}}^{V1,LR} \\
& + \frac{16}{9}L_{\substack{ue \\ 11ii}}^{V,LR} + \frac{16}{9}L_{\substack{ue \\ 22ii}}^{V,LR} + \frac{4}{3}L_{\substack{ue \\ jj11}}^{V,LR} + \frac{4}{3}L_{\substack{ue \\ jj22}}^{V,LR} + \frac{4}{3}L_{\substack{ue \\ jj33}}^{V,LR} + 8L_{\substack{ue \\ jjii}}^{V,LR} \\
& - \frac{8}{3}L_{\substack{uu \\ jjjj}}^{V1,LR} - \frac{8}{3}L_{\substack{uu \\ jjkk}}^{V1,LR} - \frac{64}{9}L_{\substack{uu \\ jjjj}}^{V,LL} - \frac{16}{3}L_{\substack{uu \\ jjkk}}^{V,LL} - \frac{16}{9}L_{\substack{uu \\ jkkj}}^{V,LL} \Big] + \alpha_s^2 \Bigg[ 8L_{\substack{de \\ 11ii}}^{V,LR} \\
& + 8L_{\substack{de \\ 22ii}}^{V,LR} + 8L_{\substack{de \\ 33ii}}^{V,LR} - 8L_{\substack{ed \\ ii11}}^{V,RR} - 8L_{\substack{ed \\ ii22}}^{V,RR} - 8L_{\substack{ed \\ ii33}}^{V,RR} - 8L_{\substack{eu \\ ii11}}^{V,RR} \\
& - 8L_{\substack{eu \\ ii22}}^{V,RR} + 8L_{\substack{ue \\ 11ii}}^{V,LR} + 8L_{\substack{ue \\ 22ii}}^{V,LR} \Big] + \alpha_s \alpha \Bigg[ -\frac{32}{9}L_{\substack{de \\ 11ii}}^{V,LR} - \frac{32}{9}L_{\substack{de \\ 22ii}}^{V,LR} \\
& - \frac{32}{9}L_{\substack{de \\ 33ii}}^{V,LR} - \frac{32}{9}L_{\substack{ed \\ ii11}}^{V,RR} - \frac{32}{9}L_{\substack{ed \\ ii22}}^{V,RR} - \frac{32}{9}L_{\substack{ed \\ ii33}}^{V,RR} + \frac{64}{9}L_{\substack{eu \\ ii11}}^{V,RR} + \frac{64}{9}L_{\substack{eu \\ ii22}}^{V,RR} \\
& + \frac{16}{3}L_{\substack{ud \\ jj11}}^{V1,LL} + \frac{16}{3}L_{\substack{ud \\ jj22}}^{V1,LL} + \frac{16}{3}L_{\substack{ud \\ jj33}}^{V1,LL} + \frac{16}{3}L_{\substack{ud \\ jj11}}^{V1,LR} + \frac{16}{3}L_{\substack{ud \\ jj22}}^{V1,LR} - \frac{32}{3}L_{\substack{ud \\ jj33}}^{V1,LR} \\
& + \frac{388}{243}L_{\substack{ud \\ jj11}}^{V8,LL} + \frac{388}{243}L_{\substack{ud \\ jj22}}^{V8,LL} + \frac{388}{243}L_{\substack{ud \\ jj33}}^{V8,LL} - \frac{332}{243}L_{\substack{ud \\ jj11}}^{V8,LR} - \frac{332}{243}L_{\substack{ud \\ jj22}}^{V8,LR} \\
& + \frac{2044}{243}L_{\substack{ud \\ jj33}}^{V8,LR} + \frac{64}{9}L_{\substack{ue \\ 11ii}}^{V,LR} + \frac{64}{9}L_{\substack{ue \\ 22ii}}^{V,LR} - 32L_{\substack{ue \\ jjii}}^{V,LR} - \frac{32}{3}L_{\substack{uu \\ jjjj}}^{V1,LR} - \frac{32}{3}L_{\substack{uu \\ jkkk}}^{V1,LR} \\
& + \frac{2044}{243}L_{\substack{uu \\ jjjj}}^{V8,LR} + \frac{2044}{243}L_{\substack{uu \\ jjkk}}^{V8,LR} - \frac{2096}{81}L_{\substack{uu \\ jjjj}}^{V,LL} - 16L_{\substack{uu \\ jjkk}}^{V,LL} - \frac{128}{243}L_{\substack{uu \\ jkkj}}^{V,LL} \Big] \\
& + \alpha^2 \Bigg[ \frac{1792}{243}L_{\substack{de \\ 11ii}}^{V,LR} + \frac{1792}{243}L_{\substack{de \\ 22ii}}^{V,LR} + \frac{1792}{243}L_{\substack{de \\ 33ii}}^{V,LR} + \frac{1168}{243}L_{\substack{ed \\ ii11}}^{V,RR} + \frac{1168}{243}L_{\substack{ed \\ ii22}}^{V,RR} \\
& + \frac{1168}{243}L_{\substack{ed \\ ii33}}^{V,RR} + \frac{1808}{81}L_{\substack{ee \\ iii}}^{V,LR} + \frac{1808}{81}L_{\substack{ee \\ jjii}}^{V,LR} + \frac{1808}{81}L_{\substack{ee \\ kkii}}^{V,LR} + \frac{992}{81}L_{\substack{ee \\ iii}}^{V,RR} + \frac{896}{81}L_{\substack{ee \\ iijj}}^{V,RR}
\end{aligned}$$



$$\begin{aligned}
& + \frac{896}{81} L_{ikk}^{V,RR} - \frac{4744}{243} L_{11jj}^{V,LL} - \frac{4744}{243} L_{22jj}^{V,LL} - \frac{4744}{243} L_{33jj}^{V,LL} - \frac{1184}{243} L_{ii11}^{V,RR} \\
& - \frac{1184}{243} L_{ii22}^{V,RR} - \frac{3808}{243} L_{jj11}^{V1,LL} - \frac{3808}{243} L_{jj22}^{V1,LL} - \frac{3808}{243} L_{jj33}^{V1,LL} - \frac{1144}{243} L_{jj11}^{V1,LR} \\
& - \frac{1144}{243} L_{jj22}^{V1,LR} + \frac{12512}{243} L_{jj33}^{V1,LR} + \frac{1312}{243} L_{11ii}^{V,LR} + \frac{1312}{243} L_{22ii}^{V,LR} + \frac{3248}{243} L_{jj11}^{V,LR} \\
& + \frac{3248}{243} L_{jj22}^{V,LR} + \frac{3248}{243} L_{jj33}^{V,LR} - \frac{4960}{27} L_{jjii}^{V,LR} + \frac{12224}{243} L_{jjjj}^{V1,LR} + \frac{12224}{243} L_{jjkk}^{V1,LR} \\
& + \frac{3808}{243} L_{jjjj}^{V,LL} + \frac{3136}{243} L_{jjkk}^{V,LL} + \frac{1024}{729} L_{jjkk}^{V,LL} \Bigg] ;
\end{aligned}$$

$$\begin{aligned}
\dot{L}_{jjii}^{V,LR} &= e^2 \left[ \frac{4}{3} L_{jj11}^{V,LL} + \frac{4}{3} L_{jj22}^{V,LL} + \frac{4}{3} L_{jj33}^{V,LL} + \frac{4}{3} L_{jj11}^{V,LR} + \frac{4}{3} L_{jj22}^{V,LR} \right. \\
& + \frac{4}{3} L_{jj33}^{V,LR} + \frac{4}{3} L_{jj11}^{V,LL} + \frac{4}{3} L_{jj22}^{V,LL} + \frac{4}{3} L_{jj33}^{V,LL} + \frac{4}{3} L_{jj11}^{V,LR} + \frac{4}{3} L_{jj22}^{V,LR} \\
& \left. + \frac{4}{3} L_{jj33}^{V,LR} - \frac{8}{3} L_{jj11}^{V,LL} - \frac{8}{3} L_{jj22}^{V,LL} - \frac{8}{3} L_{jj11}^{V,LR} - \frac{8}{3} L_{jj22}^{V,LR} \right] \\
& + \alpha_s \alpha \left[ \frac{16}{3} L_{jj11}^{V,LL} + \frac{16}{3} L_{jj22}^{V,LL} + \frac{16}{3} L_{jj33}^{V,LL} + \frac{16}{3} L_{jj11}^{V,LR} + \frac{16}{3} L_{jj22}^{V,LR} \right. \\
& \left. + \frac{16}{3} L_{jj33}^{V,LR} - \frac{32}{3} L_{jj11}^{V,LL} - \frac{32}{3} L_{jj22}^{V,LL} - \frac{32}{3} L_{jj11}^{V,LR} - \frac{32}{3} L_{jj22}^{V,LR} \right] \\
& + \alpha^2 \left[ -\frac{32}{9} L_{jj11}^{V,LL} - \frac{32}{9} L_{jj22}^{V,LL} - \frac{32}{9} L_{jj33}^{V,LL} + \frac{40}{9} L_{jj11}^{V,LR} + \frac{40}{9} L_{jj22}^{V,LR} \right. \\
& + \frac{40}{9} L_{jj33}^{V,LR} - 8 L_{jj11}^{V,LL} - 8 L_{jj22}^{V,LL} - 8 L_{jj33}^{V,LL} + 16 L_{jj11}^{V,LR} + 16 L_{jj22}^{V,LR} \\
& \left. + 16 L_{jj33}^{V,LR} - \frac{176}{9} L_{jj11}^{V,LL} - \frac{176}{9} L_{jj22}^{V,LL} + \frac{112}{9} L_{jj11}^{V,LR} + \frac{112}{9} L_{jj22}^{V,LR} \right] ;
\end{aligned}$$

$$\begin{aligned}
\dot{L}_{jjii}^{V,LR} &= e^2 \left[ \frac{4}{9} L_{jj11}^{V,LL} + \frac{4}{9} L_{jj22}^{V,LL} + \frac{4}{9} L_{jj33}^{V,LL} + \frac{4}{9} L_{jj11}^{V,LR} + \frac{4}{9} L_{jj22}^{V,LR} \right. \\
& + \frac{4}{9} L_{jj33}^{V,LR} + \frac{4}{9} L_{jj11}^{V,LL} + \frac{4}{9} L_{jj22}^{V,LL} + \frac{4}{9} L_{jj33}^{V,LL} + \frac{4}{9} L_{jj11}^{V,LR} + \frac{4}{9} L_{jj22}^{V,LR} \\
& \left. + \frac{4}{9} L_{jj33}^{V,LR} - \frac{8}{9} L_{jj11}^{V,LL} - \frac{8}{9} L_{jj22}^{V,LL} - \frac{8}{9} L_{jj11}^{V,LR} - \frac{8}{9} L_{jj22}^{V,LR} \right]
\end{aligned}$$

$$\begin{aligned}
& + \alpha_s^2 \left[ -8L_{jj11}^{V,LL} - 8L_{jj22}^{V,LL} - 8L_{jj33}^{V,LL} + 8L_{jj11}^{V,LR} + 8L_{jj22}^{V,LR} \right. \\
& \left. + 8L_{jj33}^{V,LR} - 8L_{jj11}^{V,LL} - 8L_{jj22}^{V,LL} + 8L_{jj11}^{V,LR} + 8L_{jj22}^{V,LR} \right] \\
& + \alpha_s \alpha \left[ \frac{16}{9}L_{jj11}^{V,LL} + \frac{16}{9}L_{jj22}^{V,LL} + \frac{16}{9}L_{jj33}^{V,LL} + \frac{16}{9}L_{jj11}^{V,LR} + \frac{16}{9}L_{jj22}^{V,LR} \right. \\
& \left. + \frac{16}{9}L_{jj33}^{V,LR} - \frac{32}{9}L_{jj11}^{V,LL} - \frac{32}{9}L_{jj22}^{V,LL} - \frac{32}{9}L_{jj11}^{V,LR} - \frac{32}{9}L_{jj22}^{V,LR} \right] \\
& + \alpha^2 \left[ -\frac{8}{27}L_{jj11}^{V,LL} - \frac{8}{27}L_{jj22}^{V,LL} - \frac{8}{27}L_{jj33}^{V,LL} + \frac{16}{27}L_{jj11}^{V,LR} + \frac{16}{27}L_{jj22}^{V,LR} \right. \\
& + \frac{16}{27}L_{jj33}^{V,LR} + \frac{8}{3}L_{jj11}^{V,LR} + \frac{8}{3}L_{jj22}^{V,LR} + \frac{8}{3}L_{jj33}^{V,LR} - \frac{80}{27}L_{jj11}^{V,LL} - \frac{80}{27}L_{jj22}^{V,LL} \\
& \left. + \frac{16}{27}L_{jj11}^{V,LR} + \frac{16}{27}L_{jj22}^{V,LR} \right]; \\
\dot{L}_{jj\bar{i}}^{V,LR} & = e^2 \left[ -\frac{8}{9}L_{jj11}^{V,LL} - \frac{8}{9}L_{jj22}^{V,LL} - \frac{8}{9}L_{jj33}^{V,LL} - \frac{8}{9}L_{jj11}^{V,LR} - \frac{8}{9}L_{jj22}^{V,LR} \right. \\
& - \frac{8}{9}L_{jj33}^{V,LR} - \frac{8}{9}L_{jj11}^{V,LL} - \frac{8}{9}L_{jj22}^{V,LL} - \frac{8}{9}L_{jj33}^{V,LL} - \frac{8}{9}L_{jj11}^{V,LR} - \frac{8}{9}L_{jj22}^{V,LR} \\
& \left. - \frac{8}{9}L_{jj33}^{V,LR} + \frac{16}{9}L_{jj11}^{V,LL} + \frac{16}{9}L_{jj22}^{V,LL} + \frac{16}{9}L_{jj11}^{V,LR} + \frac{16}{9}L_{jj22}^{V,LR} \right] \\
& + \alpha_s^2 \left[ -8L_{jj11}^{V,LL} - 8L_{jj22}^{V,LL} - 8L_{jj33}^{V,LL} + 8L_{jj11}^{V,LR} + 8L_{jj22}^{V,LR} \right. \\
& \left. + 8L_{jj33}^{V,LR} - 8L_{jj11}^{V,LL} - 8L_{jj22}^{V,LL} + 8L_{jj11}^{V,LR} + 8L_{jj22}^{V,LR} \right] \\
& + \alpha_s \alpha \left[ -\frac{32}{9}L_{jj11}^{V,LL} - \frac{32}{9}L_{jj22}^{V,LL} - \frac{32}{9}L_{jj33}^{V,LL} - \frac{32}{9}L_{jj11}^{V,LR} - \frac{32}{9}L_{jj22}^{V,LR} \right. \\
& \left. - \frac{32}{9}L_{jj33}^{V,LR} + \frac{64}{9}L_{jj11}^{V,LL} + \frac{64}{9}L_{jj22}^{V,LL} + \frac{64}{9}L_{jj11}^{V,LR} + \frac{64}{9}L_{jj22}^{V,LR} \right] \\
& + \alpha^2 \left[ -\frac{56}{27}L_{jj11}^{V,LL} - \frac{56}{27}L_{jj22}^{V,LL} - \frac{56}{27}L_{jj33}^{V,LL} + \frac{40}{27}L_{jj11}^{V,LR} + \frac{40}{27}L_{jj22}^{V,LR} \right.
\end{aligned}$$

$$\begin{aligned}
& + \frac{40}{27} L_{\nu d, jj33}^{V,LR} - 8 L_{\nu e, jj11}^{V,LL} - 8 L_{\nu e, jj22}^{V,LL} - 8 L_{\nu e, jj33}^{V,LL} + \frac{8}{3} L_{\nu e, jj11}^{V,LR} + \frac{8}{3} L_{\nu e, jj22}^{V,LR} \\
& + \frac{8}{3} L_{\nu e, jj33}^{V,LR} - \frac{128}{27} L_{\nu u, jj11}^{V,LL} - \frac{128}{27} L_{\nu u, jj22}^{V,LL} + \frac{256}{27} L_{\nu u, jj11}^{V,LR} + \frac{256}{27} L_{\nu u, jj22}^{V,LR} \Bigg]; \\
\dot{L}_{\frac{du}{jjii}}^{V1,LR} = & - \frac{8}{3} L_{\frac{du}{jjii}}^{V8,LR} g_s^2 + e^2 \Bigg[ - \frac{16}{9} L_{\frac{dd}{jjjj}}^{V1,LR} - \frac{8}{9} L_{\frac{dd}{jjkk}}^{V1,LR} - \frac{128}{27} L_{\frac{dd}{jjjj}}^{V,LL} - \frac{16}{9} L_{\frac{dd}{jjkk}}^{V,LL} \\
& - \frac{16}{27} L_{\frac{dd}{jjkj}}^{V,LL} - \frac{8}{9} L_{\frac{de}{jj11}}^{V,LR} - \frac{8}{9} L_{\frac{de}{jj22}}^{V,LR} - \frac{8}{9} L_{\frac{de}{jj33}}^{V,LR} + \frac{4}{9} L_{\frac{du}{11ii}}^{V1,LR} + \frac{4}{9} L_{\frac{du}{22ii}}^{V1,LR} \\
& + \frac{4}{9} L_{\frac{du}{33ii}}^{V1,LR} + \frac{16}{9} L_{\frac{du}{jj11}}^{V1,LR} + \frac{16}{9} L_{\frac{du}{jj22}}^{V1,LR} + \frac{8}{3} L_{\frac{du}{jjii}}^{V1,LR} - \frac{8}{9} L_{\frac{ed}{11jj}}^{V,LL} - \frac{8}{9} L_{\frac{ed}{22jj}}^{V,LL} \\
& - \frac{8}{9} L_{\frac{ed}{33jj}}^{V,LL} + \frac{4}{9} L_{\frac{eu}{11ii}}^{V,LR} + \frac{4}{9} L_{\frac{eu}{22ii}}^{V,LR} + \frac{4}{9} L_{\frac{eu}{33ii}}^{V,LR} + \frac{4}{9} L_{\frac{eu}{11ii}}^{V,RR} + \frac{4}{9} L_{\frac{eu}{22ii}}^{V,RR} \\
& + \frac{4}{9} L_{\frac{eu}{33ii}}^{V,RR} + \frac{16}{9} L_{\frac{ud}{11jj}}^{V1,LL} + \frac{16}{9} L_{\frac{ud}{22jj}}^{V1,LL} + \frac{4}{9} L_{\frac{ud}{ii11}}^{V1,RR} + \frac{4}{9} L_{\frac{ud}{ii22}}^{V1,RR} + \frac{4}{9} L_{\frac{ud}{ii33}}^{V1,RR} \\
& - \frac{8}{9} L_{\frac{uu}{iii}}^{V1,LR} - \frac{8}{9} L_{\frac{uu}{kkii}}^{V1,LR} - \frac{64}{27} L_{\frac{uu}{iii}}^{V,RR} - \frac{16}{9} L_{\frac{uu}{ikk}}^{V,RR} - \frac{16}{27} L_{\frac{uu}{ikki}}^{V,RR} \Bigg] + \alpha_s^2 \Bigg[ 16 L_{\frac{dd}{jjjj}}^{V1,LR} \\
& + 8 L_{\frac{dd}{jjkk}}^{V1,LR} + \frac{88}{27} L_{\frac{dd}{jjjj}}^{V8,LR} + \frac{44}{27} L_{\frac{dd}{jjkk}}^{V8,LR} - \frac{1192}{27} L_{\frac{dd}{jjjj}}^{V,LL} - 16 L_{\frac{dd}{jjkk}}^{V,LL} - \frac{64}{27} L_{\frac{dd}{jjkj}}^{V,LL} \\
& + 8 L_{\frac{du}{11ii}}^{V1,LR} + 8 L_{\frac{du}{22ii}}^{V1,LR} + 8 L_{\frac{du}{33ii}}^{V1,LR} + 8 L_{\frac{du}{jj11}}^{V1,LR} + 8 L_{\frac{du}{jj22}}^{V1,LR} - \frac{28}{3} L_{\frac{du}{jjii}}^{V1,LR} \\
& + \frac{44}{27} L_{\frac{du}{11ii}}^{V8,LR} + \frac{44}{27} L_{\frac{du}{22ii}}^{V8,LR} + \frac{44}{27} L_{\frac{du}{33ii}}^{V8,LR} + \frac{44}{27} L_{\frac{du}{jj11}}^{V8,LR} + \frac{44}{27} L_{\frac{du}{jj22}}^{V8,LR} - \frac{2044}{27} L_{\frac{du}{jjii}}^{V8,LR} \\
& - 8 L_{\frac{ud}{11jj}}^{V1,LL} - 8 L_{\frac{ud}{22jj}}^{V1,LL} - 8 L_{\frac{ud}{ii11}}^{V1,RR} - 8 L_{\frac{ud}{ii22}}^{V1,RR} - 8 L_{\frac{ud}{ii33}}^{V1,RR} + \frac{44}{27} L_{\frac{ud}{11jj}}^{V8,LL} \\
& + \frac{44}{27} L_{\frac{ud}{22jj}}^{V8,LL} + \frac{44}{27} L_{\frac{ud}{ii11}}^{V8,RR} + \frac{44}{27} L_{\frac{ud}{ii22}}^{V8,RR} + \frac{44}{27} L_{\frac{ud}{ii33}}^{V8,RR} + 8 L_{\frac{uu}{iii}}^{V1,LR} + 8 L_{\frac{uu}{kkii}}^{V1,LR} \\
& + \frac{44}{27} L_{\frac{uu}{iii}}^{V8,LR} + \frac{44}{27} L_{\frac{uu}{kkii}}^{V8,LR} - \frac{232}{9} L_{\frac{uu}{iii}}^{V,RR} - 16 L_{\frac{uu}{ikk}}^{V,RR} - \frac{64}{27} L_{\frac{uu}{ikki}}^{V,RR} \Bigg] + \alpha_s \alpha \Bigg[ - \frac{64}{9} L_{\frac{dd}{jjjj}}^{V1,LR} \\
& - \frac{32}{9} L_{\frac{dd}{jjkk}}^{V1,LR} + \frac{4160}{729} L_{\frac{dd}{jjjj}}^{V8,LR} + \frac{2080}{729} L_{\frac{dd}{jjkk}}^{V8,LR} - \frac{10016}{729} L_{\frac{dd}{jjjj}}^{V,LL} - \frac{16}{3} L_{\frac{dd}{jjkk}}^{V,LL} \\
& + \frac{16}{729} L_{\frac{dd}{jjkj}}^{V,LL} + \frac{16}{9} L_{\frac{du}{11ii}}^{V1,LR} + \frac{16}{9} L_{\frac{du}{22ii}}^{V1,LR} - \frac{32}{9} L_{\frac{du}{33ii}}^{V1,LR} + \frac{64}{9} L_{\frac{du}{jj11}}^{V1,LR} + \frac{64}{9} L_{\frac{du}{jj22}}^{V1,LR} \\
& - \frac{64}{3} L_{\frac{du}{jjii}}^{V1,LR} - \frac{332}{729} L_{\frac{du}{11ii}}^{V8,LR} - \frac{332}{729} L_{\frac{du}{22ii}}^{V8,LR} + \frac{2044}{729} L_{\frac{du}{33ii}}^{V8,LR} - \frac{2672}{729} L_{\frac{du}{jj11}}^{V8,LR}
\end{aligned}$$

$$\begin{aligned}
& -\frac{2672}{729}L_{jj22}^{V8,LR} + \frac{232}{27}L_{jjii}^{V8,LR} + \frac{64}{9}L_{11jj}^{V1,LL} + \frac{64}{9}L_{22jj}^{V1,LL} + \frac{16}{9}L_{ii11}^{V1,RR} + \frac{16}{9}L_{ii22}^{V1,RR} \\
& + \frac{16}{9}L_{ii33}^{V1,RR} + \frac{208}{729}L_{11jj}^{V8,LL} + \frac{208}{729}L_{22jj}^{V8,LL} + \frac{388}{729}L_{ii11}^{V8,RR} + \frac{388}{729}L_{ii22}^{V8,RR} \\
& + \frac{388}{729}L_{ii33}^{V8,RR} - \frac{32}{9}L_{iiii}^{V1,LR} - \frac{32}{9}L_{kkii}^{V1,LR} + \frac{2044}{729}L_{iiii}^{V8,LR} + \frac{2044}{729}L_{kkii}^{V8,LR} \\
& - \frac{2096}{243}L_{iiii}^{V,RR} - \frac{16}{3}L_{iikk}^{V,RR} - \frac{128}{729}L_{ikki}^{V,RR} \Big] + \alpha^2 \Big[ \frac{7552}{729}L_{jjjj}^{V1,LR} + \frac{3776}{729}L_{jjkk}^{V1,LR} \\
& + \frac{5392}{2187}L_{jjjj}^{V,LL} + \frac{928}{729}L_{jjkk}^{V,LL} - \frac{32}{2187}L_{jjkk}^{V,LL} + \frac{6224}{729}L_{jj11}^{V,LR} + \frac{6224}{729}L_{jj22}^{V,LR} \\
& + \frac{6224}{729}L_{jj33}^{V,LR} - \frac{208}{729}L_{11ii}^{V1,LR} - \frac{208}{729}L_{22ii}^{V1,LR} + \frac{6752}{729}L_{33ii}^{V1,LR} + \frac{6272}{729}L_{jj11}^{V1,LR} \\
& + \frac{6272}{729}L_{jj22}^{V1,LR} - \frac{4048}{81}L_{jjii}^{V1,LR} - \frac{3712}{729}L_{11jj}^{V,LL} - \frac{3712}{729}L_{22jj}^{V,LL} - \frac{3712}{729}L_{33jj}^{V,LL} \\
& + \frac{2888}{729}L_{11ii}^{V,LR} + \frac{2888}{729}L_{22ii}^{V,LR} + \frac{2888}{729}L_{33ii}^{V,LR} - \frac{1216}{729}L_{11ii}^{V,RR} - \frac{1216}{729}L_{22ii}^{V,RR} \\
& - \frac{1216}{729}L_{33ii}^{V,RR} - \frac{6976}{729}L_{11jj}^{V1,LL} - \frac{6976}{729}L_{22jj}^{V1,LL} - \frac{1576}{729}L_{ii11}^{V1,RR} - \frac{1576}{729}L_{ii22}^{V1,RR} \\
& - \frac{1576}{729}L_{ii33}^{V1,RR} + \frac{6464}{729}L_{iiii}^{V1,LR} + \frac{6464}{729}L_{kkii}^{V1,LR} + \frac{4384}{729}L_{iiii}^{V,RR} + \frac{1984}{729}L_{iikk}^{V,RR} \\
& + \frac{3328}{2187}L_{iikk}^{V,RR} \Big] ;
\end{aligned}$$

$$\begin{aligned}
\dot{L}_{jjii}^{V8,LR} &= g_s^2 \Big[ \frac{4}{3}L_{jjjj}^{V8,LR} + \frac{2}{3}L_{jjkk}^{V8,LR} + \frac{16}{3}L_{jjjj}^{V,LL} + \frac{8}{3}L_{jjkk}^{V,LL} - 12L_{jjii}^{V1,LR} \\
& + \frac{2}{3}L_{11ii}^{V8,LR} + \frac{2}{3}L_{22ii}^{V8,LR} + \frac{2}{3}L_{33ii}^{V8,LR} + \frac{2}{3}L_{jj11}^{V8,LR} + \frac{2}{3}L_{jj22}^{V8,LR} - 14L_{jjii}^{V8,LR} \\
& + \frac{2}{3}L_{11jj}^{V8,LL} + \frac{2}{3}L_{22jj}^{V8,LL} + \frac{2}{3}L_{ii11}^{V8,RR} + \frac{2}{3}L_{ii22}^{V8,RR} + \frac{2}{3}L_{ii33}^{V8,RR} + \frac{2}{3}L_{uu}^{V8,LR} \\
& + \frac{2}{3}L_{kkii}^{V8,LR} + \frac{8}{3}L_{iiii}^{V,RR} + \frac{8}{3}L_{ikki}^{V,RR} \Big] + \frac{8}{3}L_{jjii}^{V8,LR}e^2 + \alpha_s^2 \Big[ -\frac{44}{3}L_{jjjj}^{V1,LR} \\
& - \frac{22}{3}L_{jjkk}^{V1,LR} + \frac{1538}{81}L_{jjjj}^{V8,LR} + \frac{769}{81}L_{jjkk}^{V8,LR} + \frac{6142}{81}L_{jjjj}^{V,LL} - \frac{28}{3}L_{jjkk}^{V,LL} + \frac{3376}{81}L_{jjkk}^{V,LL} \\
& - \frac{22}{3}L_{11ii}^{V1,LR} - \frac{22}{3}L_{22ii}^{V1,LR} - \frac{22}{3}L_{33ii}^{V1,LR} - \frac{22}{3}L_{jj11}^{V1,LR} - \frac{22}{3}L_{jj22}^{V1,LR} - \frac{374}{3}L_{jjii}^{V1,LR}
\end{aligned}$$

$$\begin{aligned}
& + \frac{787}{81} L_{11ii}^{V8,LR} + \frac{787}{81} L_{22ii}^{V8,LR} + \frac{787}{81} L_{33ii}^{V8,LR} + \frac{769}{81} L_{jj11}^{V8,LR} + \frac{769}{81} L_{jj22}^{V8,LR} - \frac{2975}{18} L_{jjii}^{V8,LR} \\
& - \frac{2}{3} L_{11jj}^{V1,LL} - \frac{2}{3} L_{22jj}^{V1,LL} - \frac{2}{3} L_{ii11}^{V1,RR} - \frac{2}{3} L_{ii22}^{V1,RR} - \frac{2}{3} L_{ii33}^{V1,RR} + \frac{589}{81} L_{11jj}^{V8,LL} \\
& + \frac{589}{81} L_{22jj}^{V8,LL} + \frac{607}{81} L_{ii11}^{V8,RR} + \frac{607}{81} L_{ii22}^{V8,RR} + \frac{607}{81} L_{ii33}^{V8,RR} - \frac{22}{3} L_{iiii}^{V1,LR} - \frac{22}{3} L_{kkii}^{V1,LR} \\
& + \frac{787}{81} L_{iiii}^{V8,LR} + \frac{787}{81} L_{kkii}^{V8,LR} + \frac{1198}{27} L_{iiii}^{V,RR} - \frac{28}{3} L_{iikk}^{V,RR} + \frac{3448}{81} L_{ikki}^{V,RR} \Big] \\
& + \alpha_s \alpha \Bigg[ - \frac{1832}{81} L_{jjjj}^{V1,LR} - \frac{916}{81} L_{jjkk}^{V1,LR} - \frac{88}{9} L_{jjjj}^{V8,LR} - \frac{44}{9} L_{jjkk}^{V8,LR} - \frac{11264}{243} L_{jjjj}^{V,LL} \\
& - \frac{1832}{81} L_{jjkk}^{V,LL} + \frac{664}{243} L_{jjkk}^{V,LL} - \frac{916}{81} L_{jj11}^{V,LR} - \frac{916}{81} L_{jj22}^{V,LR} - \frac{916}{81} L_{jj33}^{V,LR} + \frac{644}{81} L_{11ii}^{V1,LR} \\
& + \frac{644}{81} L_{22ii}^{V1,LR} - \frac{1216}{81} L_{33ii}^{V1,LR} + \frac{1832}{81} L_{jj11}^{V1,LR} + \frac{1832}{81} L_{jj22}^{V1,LR} + \frac{116}{3} L_{jjii}^{V1,LR} \\
& + \frac{14}{9} L_{11ii}^{V8,LR} + \frac{14}{9} L_{22ii}^{V8,LR} - \frac{20}{3} L_{33ii}^{V8,LR} + \frac{56}{9} L_{jj11}^{V8,LR} + \frac{56}{9} L_{jj22}^{V8,LR} + \frac{187}{9} L_{jjii}^{V8,LR} \\
& - \frac{916}{81} L_{11jj}^{V,LL} - \frac{916}{81} L_{22jj}^{V,LL} - \frac{916}{81} L_{33jj}^{V,LL} + \frac{644}{81} L_{11ii}^{V,LR} + \frac{644}{81} L_{22ii}^{V,LR} + \frac{644}{81} L_{33ii}^{V,LR} \\
& + \frac{644}{81} L_{11ii}^{V,RR} + \frac{644}{81} L_{22ii}^{V,RR} + \frac{644}{81} L_{33ii}^{V,RR} + \frac{1832}{81} L_{11jj}^{V1,LL} + \frac{1832}{81} L_{22jj}^{V1,LL} + \frac{644}{81} L_{ii11}^{V1,RR} \\
& + \frac{644}{81} L_{ii22}^{V1,RR} + \frac{644}{81} L_{ii33}^{V1,RR} - \frac{160}{27} L_{11jj}^{V8,LL} - \frac{160}{27} L_{22jj}^{V8,LL} - \frac{70}{27} L_{ii11}^{V8,RR} - \frac{70}{27} L_{ii22}^{V8,RR} \\
& - \frac{70}{27} L_{ii33}^{V8,RR} - \frac{1288}{81} L_{iiii}^{V1,LR} - \frac{1288}{81} L_{kkii}^{V1,LR} - \frac{20}{3} L_{iiii}^{V8,LR} - \frac{20}{3} L_{kkii}^{V8,LR} - \frac{3608}{81} L_{iiii}^{V,RR} \\
& - \frac{2576}{81} L_{iikk}^{V,RR} - \frac{800}{243} L_{ikki}^{V,RR} \Big] - \frac{4048}{81} L_{jjii}^{V8,LR} \alpha^2 ;
\end{aligned}$$

$$\begin{aligned}
\dot{L}_{ijj}^{V1,LR} & = - \frac{8}{3} L_{ijj}^{V8,LR} g_s^2 + e^2 \Bigg[ \frac{4}{9} L_{iii}^{V1,LR} - \frac{8}{9} L_{ijj}^{V1,LR} + \frac{4}{9} L_{ikk}^{V1,LR} + \frac{8}{9} L_{jjj}^{V1,LR} \\
& + \frac{4}{9} L_{kkjj}^{V1,LR} + \frac{32}{27} L_{iii}^{V,LL} + \frac{8}{9} L_{ijj}^{V,LL} + \frac{8}{9} L_{ikk}^{V,LL} + \frac{8}{27} L_{ijji}^{V,LL} + \frac{8}{27} L_{ikki}^{V,LL} \\
& + \frac{64}{27} L_{jjjj}^{V,RR} + \frac{8}{9} L_{jjkk}^{V,RR} + \frac{8}{27} L_{jjkk}^{V,RR} + \frac{4}{9} L_{ii11}^{V,LR} + \frac{4}{9} L_{ii22}^{V,LR} + \frac{4}{9} L_{ii33}^{V,LR} \\
& - \frac{8}{9} L_{ii11}^{V1,LR} - \frac{8}{9} L_{ii22}^{V1,LR} + \frac{4}{9} L_{11ii}^{V,LL} + \frac{4}{9} L_{22ii}^{V,LL} + \frac{4}{9} L_{33ii}^{V,LL} + \frac{4}{9} L_{11jj}^{V,LR}
\end{aligned}$$

$$\begin{aligned}
& + \frac{4}{9}L_{22jj}^{V,LR} + \frac{4}{9}L_{33jj}^{V,LR} + \frac{4}{9}L_{11jj}^{V,RR} + \frac{4}{9}L_{22jj}^{V,RR} + \frac{4}{9}L_{33jj}^{V,RR} - \frac{8}{9}L_{11ii}^{V1,LL} \\
& - \frac{8}{9}L_{22ii}^{V1,LL} - \frac{8}{9}L_{11jj}^{V1,LR} - \frac{8}{9}L_{22jj}^{V1,LR} - \frac{8}{9}L_{11jj}^{V1,RR} - \frac{8}{9}L_{22jj}^{V1,RR} \Big] + \alpha_s^2 \Big[ 8L_{iii}^{V1,LR} \\
& - \frac{4}{3}L_{ijj}^{V1,LR} + 8L_{ikk}^{V1,LR} + 16L_{jjj}^{V1,LR} + 8L_{kkj}^{V1,LR} + \frac{44}{27}L_{iii}^{V8,LR} - \frac{2000}{27}L_{ijj}^{V8,LR} \\
& + \frac{44}{27}L_{ikk}^{V8,LR} + \frac{88}{27}L_{jjj}^{V8,LR} + \frac{44}{27}L_{kkj}^{V8,LR} - \frac{232}{9}L_{iii}^{V,LL} - 16L_{ijj}^{V,LL} - 16L_{ikk}^{V,LL} \\
& - \frac{64}{27}L_{ijj}^{V,LL} - \frac{64}{27}L_{ikk}^{V,LL} - \frac{1192}{27}L_{jjj}^{V,RR} - 16L_{jjk}^{V,RR} - \frac{64}{27}L_{jkk}^{V,RR} + 8L_{ii1}^{V1,LR} \\
& + 8L_{ii2}^{V1,LR} + \frac{44}{27}L_{ii1}^{V8,LR} + \frac{44}{27}L_{ii2}^{V8,LR} - 8L_{11ii}^{V1,LL} - 8L_{22ii}^{V1,LL} + 8L_{11jj}^{V1,LR} \\
& + 8L_{22jj}^{V1,LR} - 8L_{11jj}^{V1,RR} - 8L_{22jj}^{V1,RR} + \frac{44}{27}L_{11ii}^{V8,LL} + \frac{44}{27}L_{22ii}^{V8,LL} + \frac{44}{27}L_{11jj}^{V8,LR} \\
& + \frac{44}{27}L_{22jj}^{V8,LR} + \frac{44}{27}L_{11jj}^{V8,RR} + \frac{44}{27}L_{22jj}^{V8,RR} \Big] + \alpha_s \alpha \Big[ \frac{16}{9}L_{iii}^{V1,LR} + \frac{112}{9}L_{ijj}^{V1,LR} \\
& + \frac{16}{9}L_{ikk}^{V1,LR} + \frac{32}{9}L_{jjj}^{V1,LR} + \frac{16}{9}L_{kkj}^{V1,LR} - \frac{1040}{729}L_{iii}^{V8,LR} - \frac{1256}{729}L_{ijj}^{V8,LR} - \frac{1040}{729}L_{ikk}^{V8,LR} \\
& - \frac{2080}{729}L_{jjj}^{V8,LR} - \frac{1040}{729}L_{kkj}^{V8,LR} + \frac{1024}{243}L_{iii}^{V,LL} + \frac{8}{3}L_{ijj}^{V,LL} + \frac{8}{3}L_{ikk}^{V,LL} - \frac{8}{729}L_{ijj}^{V,LL} \\
& - \frac{8}{729}L_{ikk}^{V,LL} + \frac{5008}{729}L_{jjj}^{V,RR} + \frac{8}{3}L_{jkk}^{V,RR} - \frac{8}{729}L_{jkk}^{V,RR} - \frac{32}{9}L_{ii1}^{V1,LR} - \frac{32}{9}L_{ii2}^{V1,LR} \\
& + \frac{1336}{729}L_{ii1}^{V8,LR} + \frac{1336}{729}L_{ii2}^{V8,LR} - \frac{32}{9}L_{11ii}^{V1,LL} - \frac{32}{9}L_{22ii}^{V1,LL} - \frac{32}{9}L_{11jj}^{V1,LR} - \frac{32}{9}L_{22jj}^{V1,LR} \\
& - \frac{32}{9}L_{11jj}^{V1,RR} - \frac{32}{9}L_{22jj}^{V1,RR} - \frac{104}{729}L_{11ii}^{V8,LL} - \frac{104}{729}L_{22ii}^{V8,LL} + \frac{1336}{729}L_{11jj}^{V8,LR} + \frac{1336}{729}L_{22jj}^{V8,LR} \\
& - \frac{104}{729}L_{11jj}^{V8,RR} - \frac{104}{729}L_{22jj}^{V8,RR} \Big] + \alpha^2 \Big[ \frac{272}{729}L_{iii}^{V1,LR} + \frac{16382}{729}L_{ijj}^{V1,LR} + \frac{272}{729}L_{ikk}^{V1,LR} \\
& + \frac{544}{729}L_{jjj}^{V1,LR} + \frac{272}{729}L_{kkj}^{V1,LR} - \frac{656}{729}L_{iii}^{V,LL} - \frac{32}{729}L_{ijj}^{V,LL} - \frac{32}{729}L_{ikk}^{V,LL} - \frac{848}{2187}L_{ijj}^{V,LL} \\
& - \frac{848}{2187}L_{ikk}^{V,LL} - \frac{2912}{2187}L_{jjj}^{V,RR} - \frac{32}{729}L_{jkk}^{V,RR} - \frac{848}{2187}L_{jkk}^{V,RR} + \frac{992}{729}L_{ii1}^{V,LR} \\
& + \frac{992}{729}L_{ii2}^{V,LR} + \frac{992}{729}L_{ii3}^{V,LR} - \frac{1624}{729}L_{ii1}^{V1,LR} - \frac{1624}{729}L_{ii2}^{V1,LR} + \frac{128}{729}L_{11ii}^{V,LL}
\end{aligned}$$

$$\begin{aligned}
& + \frac{128}{729} L_{22ii}^{V,LL} + \frac{128}{729} L_{33ii}^{V,LL} + \frac{992}{729} L_{11jj}^{V,LR} + \frac{992}{729} L_{22jj}^{V,LR} + \frac{992}{729} L_{33jj}^{V,LR} + \frac{128}{729} L_{11jj}^{V,RR} \\
& + \frac{128}{729} L_{22jj}^{V,RR} + \frac{128}{729} L_{33jj}^{V,RR} - \frac{2776}{729} L_{11ii}^{V1,LL} - \frac{2776}{729} L_{22ii}^{V1,LL} - \frac{1624}{729} L_{11jj}^{V1,LR} \\
& - \frac{1624}{729} L_{22jj}^{V1,LR} - \frac{2776}{729} L_{11jj}^{V1,RR} - \frac{2776}{729} L_{22jj}^{V1,RR} \Big] ;
\end{aligned}$$

$$\begin{aligned}
\dot{L}_{ijj}^{V8,LR} = & g_s^2 \Bigg[ -12 L_{ijj}^{V1,LR} + \frac{2}{3} L_{iii}^{V8,LR} - \frac{40}{3} L_{ijj}^{V8,LR} + \frac{2}{3} L_{ikk}^{V8,LR} + \frac{4}{3} L_{jjj}^{V8,LR} \\
& + \frac{2}{3} L_{kkjj}^{V8,LR} + \frac{8}{3} L_{dd}^{V,LL} + \frac{8}{3} L_{dd}^{V,LL} + \frac{8}{3} L_{dd}^{V,LL} + \frac{16}{3} L_{jjj}^{V,RR} + \frac{8}{3} L_{jjj}^{V,RR} \\
& + \frac{2}{3} L_{du}^{V8,LR} + \frac{2}{3} L_{du}^{V8,LR} + \frac{2}{3} L_{ud}^{V8,LL} + \frac{2}{3} L_{ud}^{V8,LL} + \frac{2}{3} L_{ud}^{V8,LR} + \frac{2}{3} L_{ud}^{V8,LR} \\
& + \frac{2}{3} L_{ud}^{V8,RR} + \frac{2}{3} L_{ud}^{V8,RR} \Bigg] - \frac{4}{3} L_{ijj}^{V8,LR} e^2 + \alpha_s^2 \Bigg[ -\frac{22}{3} L_{iii}^{V1,LR} - 132 L_{ijj}^{V1,LR} \\
& - \frac{22}{3} L_{ikk}^{V1,LR} - \frac{44}{3} L_{jjj}^{V1,LR} - \frac{22}{3} L_{kkjj}^{V1,LR} + \frac{769}{81} L_{iii}^{V8,LR} - \frac{25237}{162} L_{ijj}^{V8,LR} + \frac{769}{81} L_{ikk}^{V8,LR} \\
& + \frac{1538}{81} L_{jjj}^{V8,LR} + \frac{769}{81} L_{kkjj}^{V8,LR} + \frac{1174}{27} L_{iii}^{V,LL} - \frac{28}{3} L_{ijj}^{V,LL} - \frac{28}{3} L_{ikk}^{V,LL} + \frac{3376}{81} L_{ijj}^{V,LL} \\
& + \frac{3376}{81} L_{ikk}^{V,LL} + \frac{6142}{81} L_{jjj}^{V,RR} - \frac{28}{3} L_{jjkk}^{V,RR} + \frac{3376}{81} L_{jjkk}^{V,RR} - \frac{22}{3} L_{du}^{V1,LR} - \frac{22}{3} L_{du}^{V1,LR} \\
& + \frac{769}{81} L_{du}^{V8,LR} + \frac{769}{81} L_{du}^{V8,LR} - \frac{2}{3} L_{ud}^{V1,LL} - \frac{2}{3} L_{ud}^{V1,LL} - \frac{22}{3} L_{ud}^{V1,LR} - \frac{22}{3} L_{ud}^{V1,LR} \\
& - \frac{2}{3} L_{ud}^{V1,RR} - \frac{2}{3} L_{ud}^{V1,RR} + \frac{589}{81} L_{ud}^{V8,LL} + \frac{589}{81} L_{ud}^{V8,LL} + \frac{769}{81} L_{ud}^{V8,LR} + \frac{769}{81} L_{ud}^{V8,LR} \\
& + \frac{589}{81} L_{ud}^{V8,RR} + \frac{589}{81} L_{ud}^{V8,RR} \Bigg] + \alpha_s \alpha \Bigg[ \frac{272}{81} L_{iii}^{V1,LR} + \frac{164}{81} L_{ijj}^{V1,LR} + \frac{272}{81} L_{ikk}^{V1,LR} \\
& + \frac{544}{81} L_{jjjj}^{V1,LR} + \frac{272}{81} L_{kkjj}^{V1,LR} + \frac{14}{9} L_{iii}^{V8,LR} - \frac{4}{3} L_{ijj}^{V8,LR} + \frac{14}{9} L_{ikk}^{V8,LR} + \frac{28}{9} L_{jjjj}^{V8,LR} \\
& + \frac{14}{9} L_{kkjj}^{V8,LR} + \frac{340}{81} L_{iii}^{V,LL} + \frac{544}{81} L_{ijj}^{V,LL} + \frac{544}{81} L_{ikk}^{V,LL} - \frac{1064}{243} L_{ijji}^{V,LL} - \frac{1064}{243} L_{ikki}^{V,LL} \\
& + \frac{1588}{243} L_{jjjj}^{V,RR} + \frac{544}{81} L_{jjkk}^{V,RR} - \frac{1064}{243} L_{jjkk}^{V,RR} + \frac{272}{81} L_{du}^{V,LR} + \frac{272}{81} L_{du}^{V,LR} + \frac{272}{81} L_{du}^{V,LR} \\
& - \frac{544}{81} L_{du}^{V1,LR} - \frac{544}{81} L_{du}^{V1,LR} + \frac{2}{3} L_{du}^{V8,LR} + \frac{2}{3} L_{du}^{V8,LR} + \frac{272}{81} L_{ed}^{V,LL} + \frac{272}{81} L_{ed}^{V,LL}
\end{aligned}$$

$$\begin{aligned}
& + \frac{272}{81} L_{33ii}^{V,LL} + \frac{272}{81} L_{11jj}^{V,LR} + \frac{272}{81} L_{22jj}^{V,LR} + \frac{272}{81} L_{33jj}^{V,LR} + \frac{272}{81} L_{11jj}^{V,RR} + \frac{272}{81} L_{22jj}^{V,RR} \\
& + \frac{272}{81} L_{33jj}^{V,RR} - \frac{544}{81} L_{11ii}^{V1,LL} - \frac{544}{81} L_{22ii}^{V1,LL} - \frac{544}{81} L_{11jj}^{V1,LR} - \frac{544}{81} L_{22jj}^{V1,LR} - \frac{544}{81} L_{11jj}^{V1,RR} \\
& - \frac{544}{81} L_{22jj}^{V1,RR} + \frac{122}{27} L_{11ii}^{V8,LL} + \frac{122}{27} L_{22ii}^{V8,LL} + \frac{2}{3} L_{11jj}^{V8,LR} + \frac{2}{3} L_{22jj}^{V8,LR} + \frac{122}{27} L_{11jj}^{V8,RR} \\
& + \frac{122}{27} L_{22jj}^{V8,RR} \Big] + \frac{1790}{81} L_{ii jj}^{V8,LR} \alpha^2 ;
\end{aligned}$$

$$\begin{aligned}
\dot{L}_{dd}^{V1,LR} = & - \frac{8}{3} L_{iii}^{V8,LR} g_s^2 + e^2 \Bigg[ - \frac{4}{9} L_{iii}^{V1,LR} + \frac{4}{9} L_{ijjj}^{V1,LR} + \frac{4}{9} L_{iikk}^{V1,LR} + \frac{4}{9} L_{jjii}^{V1,LR} \\
& + \frac{4}{9} L_{kkii}^{V1,LR} + \frac{32}{27} L_{iii}^{V,LL} + \frac{8}{9} L_{jjjj}^{V,LL} + \frac{8}{9} L_{iikk}^{V,LL} + \frac{8}{27} L_{ijji}^{V,LL} + \frac{8}{27} L_{dd}^{V,LL} + \frac{8}{27} L_{kkii}^{V,LL} \\
& + \frac{32}{27} L_{iii}^{V,RR} + \frac{8}{9} L_{jjjj}^{V,RR} + \frac{8}{9} L_{iikk}^{V,RR} + \frac{8}{27} L_{ijji}^{V,RR} + \frac{8}{27} L_{dd}^{V,RR} + \frac{4}{9} L_{de}^{V,LR} + \frac{4}{9} L_{ii11}^{V,LR} \\
& + \frac{4}{9} L_{de}^{V,LR} + \frac{4}{9} L_{ii33}^{V,LR} - \frac{8}{9} L_{du}^{V1,LR} - \frac{8}{9} L_{ii22}^{V1,LR} + \frac{4}{9} L_{ed}^{V,LL} + \frac{4}{9} L_{22ii}^{V,LL} \\
& + \frac{4}{9} L_{33ii}^{V,LL} + \frac{4}{9} L_{ed}^{V,LR} + \frac{4}{9} L_{22ii}^{V,LR} + \frac{4}{9} L_{ed}^{V,RR} + \frac{4}{9} L_{11ii}^{V,RR} + \frac{4}{9} L_{22ii}^{V,RR} \\
& + \frac{4}{9} L_{ed}^{V,RR} - \frac{8}{9} L_{11ii}^{V1,LL} - \frac{8}{9} L_{22ii}^{V1,LL} - \frac{8}{9} L_{11ii}^{V1,LR} - \frac{8}{9} L_{22ii}^{V1,LR} - \frac{8}{9} L_{11ii}^{V1,RR} \\
& - \frac{8}{9} L_{22ii}^{V1,RR} \Big] + \alpha_s^2 \Bigg[ \frac{20}{3} L_{iii}^{V1,LR} + 8 L_{ijjj}^{V1,LR} + 8 L_{iikk}^{V1,LR} + 8 L_{jjii}^{V1,LR} \\
& + 8 L_{kkii}^{V1,LR} - \frac{652}{9} L_{iii}^{V8,LR} + \frac{44}{27} L_{ijjj}^{V8,LR} + \frac{44}{27} L_{iikk}^{V8,LR} + \frac{44}{27} L_{jjii}^{V8,LR} + \frac{44}{27} L_{kkii}^{V8,LR} \\
& - \frac{232}{9} L_{iii}^{V,LL} - 16 L_{ijjj}^{V,LL} - 16 L_{iikk}^{V,LL} - \frac{64}{27} L_{ijji}^{V,LL} - \frac{64}{27} L_{kkii}^{V,LL} - \frac{232}{9} L_{iii}^{V,RR} \\
& - 16 L_{ijjj}^{V,RR} - 16 L_{iikk}^{V,RR} - \frac{64}{27} L_{ijji}^{V,RR} - \frac{64}{27} L_{kkii}^{V,RR} + 8 L_{du}^{V1,LR} + 8 L_{ii22}^{V1,LR} \\
& + \frac{44}{27} L_{du}^{V8,LR} + \frac{44}{27} L_{ii22}^{V8,LR} - 8 L_{11ii}^{V1,LL} - 8 L_{22ii}^{V1,LL} + 8 L_{11ii}^{V1,LR} + 8 L_{22ii}^{V1,LR} \\
& - 8 L_{11ii}^{V1,RR} - 8 L_{22ii}^{V1,RR} + \frac{44}{27} L_{11ii}^{V8,LL} + \frac{44}{27} L_{22ii}^{V8,LL} + \frac{44}{27} L_{11ii}^{V8,LR} + \frac{44}{27} L_{22ii}^{V8,LR} \\
& + \frac{44}{27} L_{11ii}^{V8,RR} + \frac{44}{27} L_{22ii}^{V8,RR} \Big] + \alpha_s \alpha \Bigg[ \frac{128}{9} L_{iii}^{V1,LR} + \frac{16}{9} L_{ijjj}^{V1,LR} + \frac{16}{9} L_{iikk}^{V1,LR}
\end{aligned}$$



$$\begin{aligned}
& + \frac{16}{9} L_{jjii}^{V1,LR} + \frac{16}{9} L_{kkii}^{V1,LR} - \frac{2296}{729} L_{iii}^{V8,LR} - \frac{1040}{729} L_{ijj}^{V8,LR} - \frac{1040}{729} L_{ikk}^{V8,LR} \\
& - \frac{1040}{729} L_{jjii}^{V8,LR} - \frac{1040}{729} L_{kkii}^{V8,LR} + \frac{1024}{243} L_{iii}^{V,LL} + \frac{8}{3} L_{ijj}^{V,LL} + \frac{8}{3} L_{ikk}^{V,LL} - \frac{8}{729} L_{ijji}^{V,LL} \\
& - \frac{8}{729} L_{ikki}^{V,LL} + \frac{1024}{243} L_{iii}^{V,RR} + \frac{8}{3} L_{ijj}^{V,RR} + \frac{8}{3} L_{ikk}^{V,RR} - \frac{8}{729} L_{ijji}^{V,RR} - \frac{8}{729} L_{ikki}^{V,RR} \\
& - \frac{32}{9} L_{ii11}^{V1,LR} - \frac{32}{9} L_{ii22}^{V1,LR} + \frac{1336}{729} L_{ii11}^{V8,LR} + \frac{1336}{729} L_{ii22}^{V8,LR} - \frac{32}{9} L_{11ii}^{V1,LL} - \frac{32}{9} L_{22ii}^{V1,LL} \\
& - \frac{32}{9} L_{11ii}^{V1,LR} - \frac{32}{9} L_{22ii}^{V1,LR} - \frac{32}{9} L_{11ii}^{V1,RR} - \frac{32}{9} L_{22ii}^{V1,RR} - \frac{104}{729} L_{11ii}^{V8,LL} - \frac{104}{729} L_{22ii}^{V8,LL} \\
& + \frac{1336}{729} L_{11ii}^{V8,LR} + \frac{1336}{729} L_{22ii}^{V8,LR} - \frac{104}{729} L_{11ii}^{V8,RR} - \frac{104}{729} L_{22ii}^{V8,RR} \Big] + \alpha^2 \Big[ \frac{16654}{729} L_{iii}^{V1,LR} \\
& + \frac{272}{729} L_{ijj}^{V1,LR} + \frac{272}{729} L_{ikk}^{V1,LR} + \frac{272}{729} L_{jjii}^{V1,LR} + \frac{272}{729} L_{kkii}^{V1,LR} - \frac{656}{729} L_{iii}^{V,LL} \\
& - \frac{32}{729} L_{ijj}^{V,LL} - \frac{32}{729} L_{ikk}^{V,LL} - \frac{848}{2187} L_{ijji}^{V,LL} - \frac{848}{2187} L_{ikki}^{V,LL} - \frac{656}{729} L_{iii}^{V,RR} - \frac{32}{729} L_{ijj}^{V,RR} \\
& - \frac{32}{729} L_{ikk}^{V,RR} - \frac{848}{2187} L_{ijji}^{V,RR} - \frac{848}{2187} L_{ikki}^{V,RR} + \frac{992}{729} L_{ii11}^{V,LR} + \frac{992}{729} L_{ii22}^{V,LR} \\
& + \frac{992}{729} L_{ii33}^{V,LR} - \frac{1624}{729} L_{ii11}^{V1,LR} - \frac{1624}{729} L_{ii22}^{V1,LR} + \frac{128}{729} L_{11ii}^{V,LL} + \frac{128}{729} L_{22ii}^{V,LL} \\
& + \frac{128}{729} L_{33ii}^{V,LL} + \frac{992}{729} L_{11ii}^{V,LR} + \frac{992}{729} L_{22ii}^{V,LR} + \frac{992}{729} L_{33ii}^{V,LR} + \frac{128}{729} L_{11ii}^{V,RR} + \frac{128}{729} L_{22ii}^{V,RR} \\
& + \frac{128}{729} L_{33ii}^{V,RR} - \frac{2776}{729} L_{11ii}^{V1,LL} - \frac{2776}{729} L_{22ii}^{V1,LL} - \frac{1624}{729} L_{11ii}^{V1,LR} - \frac{1624}{729} L_{22ii}^{V1,LR} \\
& - \frac{2776}{729} L_{11ii}^{V1,RR} - \frac{2776}{729} L_{22ii}^{V1,RR} \Big] ;
\end{aligned}$$

$$\begin{aligned}
\dot{L}_{iii}^{V8,LR} &= g_s^2 \Big[ -12 L_{iii}^{V1,LR} - \frac{38}{3} L_{iii}^{V8,LR} + \frac{2}{3} L_{ijj}^{V8,LR} + \frac{2}{3} L_{ikk}^{V8,LR} + \frac{2}{3} L_{jjii}^{V8,LR} \\
& + \frac{2}{3} L_{kkii}^{V8,LR} + \frac{8}{3} L_{iii}^{V,LL} + \frac{8}{3} L_{ijji}^{V,LL} + \frac{8}{3} L_{ikki}^{V,LL} + \frac{8}{3} L_{iii}^{V,RR} + \frac{8}{3} L_{ijji}^{V,RR} \\
& + \frac{8}{3} L_{ikki}^{V,RR} + \frac{2}{3} L_{ii11}^{V8,LR} + \frac{2}{3} L_{ii22}^{V8,LR} + \frac{2}{3} L_{11ii}^{V8,LL} + \frac{2}{3} L_{22ii}^{V8,LL} + \frac{2}{3} L_{11ii}^{V8,LR} \\
& + \frac{2}{3} L_{22ii}^{V8,LR} + \frac{2}{3} L_{11ii}^{V8,RR} + \frac{2}{3} L_{22ii}^{V8,RR} \Big] - \frac{4}{3} L_{iii}^{V8,LR} e^2 + \alpha_s^2 \Big[ -\frac{418}{3} L_{iii}^{V1,LR}
\end{aligned}$$

$$\begin{aligned}
& -\frac{22}{3}L_{dd\ ijj}^{V1,LR} - \frac{22}{3}L_{dd\ iikk}^{V1,LR} - \frac{22}{3}L_{dd\ jjii}^{V1,LR} - \frac{22}{3}L_{dd\ kkii}^{V1,LR} - \frac{23699}{162}L_{dd\ iii}^{V8,LR} + \frac{769}{81}L_{dd\ ijj}^{V8,LR} \\
& + \frac{769}{81}L_{dd\ iikk}^{V8,LR} + \frac{769}{81}L_{dd\ jjii}^{V8,LR} + \frac{769}{81}L_{dd\ kkii}^{V8,LR} + \frac{1174}{27}L_{dd\ iii}^{V,LL} - \frac{28}{3}L_{dd\ ijj}^{V,LL} - \frac{28}{3}L_{dd\ iikk}^{V,LL} \\
& + \frac{3376}{81}L_{dd\ ijj}^{V,LL} + \frac{3376}{81}L_{dd\ iikk}^{V,LL} + \frac{1174}{27}L_{dd\ iii}^{V,RR} - \frac{28}{3}L_{dd\ ijj}^{V,RR} - \frac{28}{3}L_{dd\ iikk}^{V,RR} + \frac{3376}{81}L_{dd\ ijj}^{V,RR} \\
& + \frac{3376}{81}L_{dd\ iikk}^{V,RR} - \frac{22}{3}L_{du\ ii11}^{V1,LR} - \frac{22}{3}L_{du\ ii22}^{V1,LR} + \frac{769}{81}L_{du\ ii11}^{V8,LR} + \frac{769}{81}L_{du\ ii22}^{V8,LR} - \frac{2}{3}L_{ud\ 11ii}^{V1,LL} \\
& - \frac{2}{3}L_{ud\ 22ii}^{V1,LL} - \frac{22}{3}L_{ud\ 11ii}^{V1,LR} - \frac{22}{3}L_{ud\ 22ii}^{V1,LR} - \frac{2}{3}L_{ud\ 11ii}^{V1,RR} - \frac{2}{3}L_{ud\ 22ii}^{V1,RR} + \frac{589}{81}L_{ud\ 11ii}^{V8,LL} \\
& + \frac{589}{81}L_{ud\ 22ii}^{V8,LL} + \frac{769}{81}L_{ud\ 11ii}^{V8,LR} + \frac{769}{81}L_{ud\ 22ii}^{V8,LR} + \frac{589}{81}L_{ud\ 11ii}^{V8,RR} + \frac{589}{81}L_{ud\ 22ii}^{V8,RR} \Big] \\
& + \alpha_s \alpha \left[ \frac{436}{81}L_{dd\ iii}^{V1,LR} + \frac{272}{81}L_{dd\ ijj}^{V1,LR} + \frac{272}{81}L_{dd\ iikk}^{V1,LR} + \frac{272}{81}L_{dd\ jjii}^{V1,LR} + \frac{272}{81}L_{dd\ kkii}^{V1,LR} \right. \\
& + \frac{2}{9}L_{dd\ iii}^{V8,LR} + \frac{14}{9}L_{dd\ ijj}^{V8,LR} + \frac{14}{9}L_{dd\ iikk}^{V8,LR} + \frac{14}{9}L_{dd\ jjii}^{V8,LR} + \frac{14}{9}L_{dd\ kkii}^{V8,LR} + \frac{340}{81}L_{dd\ iii}^{V,LL} \\
& + \frac{544}{81}L_{dd\ ijj}^{V,LL} + \frac{544}{81}L_{dd\ iikk}^{V,LL} - \frac{1064}{243}L_{dd\ ijj}^{V,LL} - \frac{1064}{243}L_{dd\ iikk}^{V,LL} + \frac{340}{81}L_{dd\ iii}^{V,RR} + \frac{544}{81}L_{dd\ ijj}^{V,RR} \\
& + \frac{544}{81}L_{dd\ iikk}^{V,RR} - \frac{1064}{243}L_{dd\ ijj}^{V,RR} - \frac{1064}{243}L_{dd\ iikk}^{V,RR} + \frac{272}{81}L_{de\ ii11}^{V,LR} + \frac{272}{81}L_{de\ ii22}^{V,LR} + \frac{272}{81}L_{de\ ii33}^{V,LR} \\
& - \frac{544}{81}L_{du\ ii11}^{V1,LR} - \frac{544}{81}L_{du\ ii22}^{V1,LR} + \frac{2}{3}L_{du\ ii11}^{V8,LR} + \frac{2}{3}L_{du\ ii22}^{V8,LR} + \frac{272}{81}L_{ed\ 11ii}^{V,LL} + \frac{272}{81}L_{ed\ 22ii}^{V,LL} \\
& + \frac{272}{81}L_{ed\ 33ii}^{V,LL} + \frac{272}{81}L_{ed\ 11ii}^{V,LR} + \frac{272}{81}L_{ed\ 22ii}^{V,LR} + \frac{272}{81}L_{ed\ 33ii}^{V,LR} + \frac{272}{81}L_{ed\ 11ii}^{V,RR} + \frac{272}{81}L_{ed\ 22ii}^{V,RR} \\
& + \frac{272}{81}L_{ed\ 33ii}^{V,RR} - \frac{544}{81}L_{ud\ 11ii}^{V1,LL} - \frac{544}{81}L_{ud\ 22ii}^{V1,LL} - \frac{544}{81}L_{ud\ 11ii}^{V1,LR} - \frac{544}{81}L_{ud\ 22ii}^{V1,LR} - \frac{544}{81}L_{ud\ 11ii}^{V1,RR} \\
& - \frac{544}{81}L_{ud\ 22ii}^{V1,RR} + \frac{122}{27}L_{ud\ 11ii}^{V8,LL} + \frac{122}{27}L_{ud\ 22ii}^{V8,LL} + \frac{2}{3}L_{ud\ 11ii}^{V8,LR} + \frac{2}{3}L_{ud\ 22ii}^{V8,LR} + \frac{122}{27}L_{ud\ 11ii}^{V8,RR} \\
& \left. + \frac{122}{27}L_{ud\ 22ii}^{V8,RR} \right] + \frac{1790}{81}L_{dd\ iii}^{V8,LR}\alpha^2 ;
\end{aligned}$$

$$\begin{aligned}
\dot{L}_{uu\ ijj}^{V1,LR} & = -\frac{8}{3}L_{uu\ ijj}^{V8,LR}g_s^2 + e^2 \left[ -\frac{8}{9}L_{du\ 11jj}^{V1,LR} - \frac{8}{9}L_{du\ 22jj}^{V1,LR} - \frac{8}{9}L_{du\ 33jj}^{V1,LR} - \frac{8}{9}L_{eu\ 11ii}^{V,LL} \right. \\
& \quad \left. - \frac{8}{9}L_{eu\ 22ii}^{V,LL} - \frac{8}{9}L_{eu\ 33ii}^{V,LL} - \frac{8}{9}L_{eu\ 11jj}^{V,LR} - \frac{8}{9}L_{eu\ 22jj}^{V,LR} - \frac{8}{9}L_{eu\ 33jj}^{V,LR} - \frac{8}{9}L_{eu\ 11jj}^{V,RR} \right]
\end{aligned}$$

$$\begin{aligned}
& -\frac{8}{9}L_{22jj}^{V,RR} - \frac{8}{9}L_{33jj}^{V,RR} - \frac{8}{9}L_{ii11}^{V1,LL} - \frac{8}{9}L_{ii22}^{V1,LL} - \frac{8}{9}L_{ii33}^{V1,LL} - \frac{8}{9}L_{ii11}^{V1,LR} \\
& - \frac{8}{9}L_{ii22}^{V1,LR} - \frac{8}{9}L_{ii33}^{V1,LR} - \frac{8}{9}L_{jj11}^{V1,RR} - \frac{8}{9}L_{jj22}^{V1,RR} - \frac{8}{9}L_{jj33}^{V1,RR} - \frac{8}{9}L_{ii11}^{V,LR} \\
& - \frac{8}{9}L_{ii22}^{V,LR} - \frac{8}{9}L_{ii33}^{V,LR} + \frac{16}{9}L_{uu}^{V1,LR} - \frac{16}{3}L_{uu}^{V1,LR} + \frac{16}{9}L_{iikk}^{V1,LR} + \frac{16}{9}L_{jjjj}^{V1,LR} \\
& + \frac{16}{9}L_{kkjj}^{V1,LR} + \frac{128}{27}L_{uu}^{V,LL} + \frac{32}{9}L_{iikk}^{V,LL} + \frac{32}{27}L_{iikk}^{V,LL} + \frac{128}{27}L_{jjjj}^{V,RR} + \frac{32}{9}L_{jjkk}^{V,RR} \\
& + \frac{32}{27}L_{jjkk}^{V,RR} \Big] + \alpha_s^2 \Big[ 8L_{11jj}^{V1,LR} + 8L_{22jj}^{V1,LR} + 8L_{33jj}^{V1,LR} + \frac{44}{27}L_{11jj}^{V8,LR} \\
& + \frac{44}{27}L_{22jj}^{V8,LR} + \frac{44}{27}L_{33jj}^{V8,LR} - 8L_{ii11}^{V1,LL} - 8L_{ii22}^{V1,LL} - 8L_{ii33}^{V1,LL} + 8L_{ii11}^{V1,LR} \\
& + 8L_{ii22}^{V1,LR} + 8L_{ii33}^{V1,LR} - 8L_{jj11}^{V1,RR} - 8L_{jj22}^{V1,RR} - 8L_{jj33}^{V1,RR} + \frac{44}{27}L_{ii11}^{V8,LL} \\
& + \frac{44}{27}L_{ii22}^{V8,LL} + \frac{44}{27}L_{ii33}^{V8,LL} + \frac{44}{27}L_{ii11}^{V8,LR} + \frac{44}{27}L_{ii22}^{V8,LR} + \frac{44}{27}L_{ii33}^{V8,LR} + \frac{44}{27}L_{jj11}^{V8,RR} \\
& + \frac{44}{27}L_{jj22}^{V8,RR} + \frac{44}{27}L_{jj33}^{V8,RR} + 8L_{uu}^{V1,LR} - \frac{28}{3}L_{iijj}^{V1,LR} + 8L_{iikk}^{V1,LR} + 8L_{jjjj}^{V1,LR} \\
& + 8L_{kkjj}^{V1,LR} + \frac{44}{27}L_{uu}^{V8,LR} - \frac{2044}{27}L_{iijj}^{V8,LR} + \frac{44}{27}L_{iikk}^{V8,LR} + \frac{44}{27}L_{jjjj}^{V8,LR} + \frac{44}{27}L_{kkjj}^{V8,LR} \\
& - \frac{232}{9}L_{uu}^{V,LL} - 16L_{iikk}^{V,LL} - \frac{64}{27}L_{iikk}^{V,LL} - \frac{232}{9}L_{jjjj}^{V,RR} - 16L_{jjkk}^{V,RR} - \frac{64}{27}L_{jjkk}^{V,RR} \Big] \\
& + \alpha_s \alpha \Big[ -\frac{32}{9}L_{11jj}^{V1,LR} - \frac{32}{9}L_{22jj}^{V1,LR} + \frac{64}{9}L_{33jj}^{V1,LR} + \frac{664}{729}L_{11jj}^{V8,LR} + \frac{664}{729}L_{22jj}^{V8,LR} \\
& - \frac{4088}{729}L_{33jj}^{V8,LR} - \frac{32}{9}L_{ii11}^{V1,LL} - \frac{32}{9}L_{ii22}^{V1,LL} - \frac{32}{9}L_{ii33}^{V1,LL} - \frac{32}{9}L_{ii11}^{V1,LR} - \frac{32}{9}L_{ii22}^{V1,LR} \\
& + \frac{64}{9}L_{ii33}^{V1,LR} - \frac{32}{9}L_{jj11}^{V1,RR} - \frac{32}{9}L_{jj22}^{V1,RR} - \frac{32}{9}L_{jj33}^{V1,RR} - \frac{776}{729}L_{ii11}^{V8,LL} - \frac{776}{729}L_{ii22}^{V8,LL} \\
& - \frac{776}{729}L_{ii33}^{V8,LL} + \frac{664}{729}L_{ii11}^{V8,LR} + \frac{664}{729}L_{ii22}^{V8,LR} - \frac{4088}{729}L_{ii33}^{V8,LR} - \frac{776}{729}L_{jj11}^{V8,RR} \\
& - \frac{776}{729}L_{jj22}^{V8,RR} - \frac{776}{729}L_{jj33}^{V8,RR} + \frac{64}{9}L_{uu}^{V1,LR} + \frac{128}{3}L_{iijj}^{V1,LR} + \frac{64}{9}L_{iikk}^{V1,LR} + \frac{64}{9}L_{jjjj}^{V1,LR} \\
& + \frac{64}{9}L_{kkjj}^{V1,LR} - \frac{4088}{729}L_{uu}^{V8,LR} - \frac{32}{27}L_{iijj}^{V8,LR} - \frac{4088}{729}L_{iikk}^{V8,LR} - \frac{4088}{729}L_{jjjj}^{V8,LR}
\end{aligned}$$

$$\begin{aligned}
& -\frac{4088}{729}L_{\overline{u}\overline{u}kkjj}^{V8,LR} + \frac{4192}{243}L_{\overline{u}\overline{u}iii}^{V,LL} + \frac{32}{3}L_{\overline{u}\overline{u}ikk}^{V,LL} + \frac{256}{729}L_{\overline{u}\overline{u}ikki}^{V,LL} + \frac{4192}{243}L_{\overline{u}\overline{u}jjj}^{V,RR} \\
& + \frac{32}{3}L_{\overline{u}\overline{u}jjkk}^{V,RR} + \frac{256}{729}L_{\overline{u}\overline{u}jjkk}^{V,RR} \Big] + \alpha^2 \Big[ -\frac{2392}{729}L_{\overline{d}\overline{u}11jj}^{V1,LR} - \frac{2392}{729}L_{\overline{d}\overline{u}22jj}^{V1,LR} + \frac{3776}{729}L_{\overline{d}\overline{u}33jj}^{V1,LR} \\
& - \frac{8152}{729}L_{\overline{e}\overline{u}11ii}^{V,LL} - \frac{8152}{729}L_{\overline{e}\overline{u}22ii}^{V,LL} - \frac{8152}{729}L_{\overline{e}\overline{u}33ii}^{V,LL} - \frac{4696}{729}L_{\overline{e}\overline{u}11jj}^{V,LR} - \frac{4696}{729}L_{\overline{e}\overline{u}22jj}^{V,LR} \\
& - \frac{4696}{729}L_{\overline{e}\overline{u}33jj}^{V,LR} - \frac{8152}{729}L_{\overline{e}\overline{u}11jj}^{V,RR} - \frac{8152}{729}L_{\overline{e}\overline{u}22jj}^{V,RR} - \frac{8152}{729}L_{\overline{e}\overline{u}33jj}^{V,RR} - \frac{3544}{729}L_{\overline{u}\overline{d}ii11}^{V1,LL} \\
& - \frac{3544}{729}L_{\overline{u}\overline{d}ii22}^{V1,LL} - \frac{3544}{729}L_{\overline{u}\overline{d}ii33}^{V1,LL} - \frac{2392}{729}L_{\overline{u}\overline{d}ii11}^{V1,LR} - \frac{2392}{729}L_{\overline{u}\overline{d}ii22}^{V1,LR} + \frac{3776}{729}L_{\overline{u}\overline{d}ii33}^{V1,LR} \\
& - \frac{3544}{729}L_{\overline{u}\overline{d}jj11}^{V1,RR} - \frac{3544}{729}L_{\overline{u}\overline{d}jj22}^{V1,RR} - \frac{3544}{729}L_{\overline{u}\overline{d}jj33}^{V1,RR} - \frac{4696}{729}L_{\overline{u}\overline{e}ii11}^{V,LR} - \frac{4696}{729}L_{\overline{u}\overline{e}ii22}^{V,LR} \\
& - \frac{4696}{729}L_{\overline{u}\overline{e}ii33}^{V,LR} + \frac{4352}{729}L_{\overline{u}\overline{u}iii}^{V1,LR} + \frac{7520}{81}L_{\overline{u}\overline{u}ijj}^{V1,LR} + \frac{4352}{729}L_{\overline{u}\overline{u}ikk}^{V1,LR} + \frac{4352}{729}L_{\overline{u}\overline{u}jjj}^{V1,LR} \\
& + \frac{4352}{729}L_{\overline{u}\overline{u}kkjj}^{V1,LR} - \frac{10496}{729}L_{\overline{u}\overline{u}iii}^{V,LL} - \frac{512}{729}L_{\overline{u}\overline{u}ikk}^{V,LL} - \frac{13568}{2187}L_{\overline{u}\overline{u}ikki}^{V,LL} - \frac{10496}{729}L_{\overline{u}\overline{u}jjj}^{V,RR} \\
& - \frac{512}{729}L_{\overline{u}\overline{u}jjkk}^{V,RR} - \frac{13568}{2187}L_{\overline{u}\overline{u}jjkk}^{V,RR} \Big] ;
\end{aligned}$$

$$\begin{aligned}
\dot{L}_{\overline{u}\overline{u}ijj}^{V8,LR} &= g_s^2 \Big[ \frac{2}{3}L_{\overline{d}\overline{u}11jj}^{V8,LR} + \frac{2}{3}L_{\overline{d}\overline{u}22jj}^{V8,LR} + \frac{2}{3}L_{\overline{d}\overline{u}33jj}^{V8,LR} + \frac{2}{3}L_{\overline{u}\overline{d}ii11}^{V8,LL} + \frac{2}{3}L_{\overline{u}\overline{d}ii22}^{V8,LL} \\
& + \frac{2}{3}L_{\overline{u}\overline{d}ii33}^{V8,LL} + \frac{2}{3}L_{\overline{u}\overline{d}ii11}^{V8,LR} + \frac{2}{3}L_{\overline{u}\overline{d}ii22}^{V8,LR} + \frac{2}{3}L_{\overline{u}\overline{d}ii33}^{V8,LR} + \frac{2}{3}L_{\overline{u}\overline{d}jj11}^{V8,RR} + \frac{2}{3}L_{\overline{u}\overline{d}jj22}^{V8,RR} \\
& + \frac{2}{3}L_{\overline{u}\overline{d}jj33}^{V8,RR} - 12L_{\overline{u}\overline{u}ijj}^{V1,LR} + \frac{2}{3}L_{\overline{u}\overline{u}iii}^{V8,LR} - 14L_{\overline{u}\overline{u}ijj}^{V8,LR} + \frac{2}{3}L_{\overline{u}\overline{u}ikk}^{V8,LR} + \frac{2}{3}L_{\overline{u}\overline{u}jjj}^{V8,LR} \\
& + \frac{2}{3}L_{\overline{u}\overline{u}kkjj}^{V8,LR} + \frac{8}{3}L_{\overline{u}\overline{u}iii}^{V,LL} + \frac{8}{3}L_{\overline{u}\overline{u}ikki}^{V,LL} + \frac{8}{3}L_{\overline{u}\overline{u}jjjj}^{V,RR} + \frac{8}{3}L_{\overline{u}\overline{u}jjkk}^{V,RR} \Big] - \frac{16}{3}L_{\overline{u}\overline{u}ijj}^{V8,LR} \\
& e^2 + \alpha_s^2 \Big[ -\frac{22}{3}L_{\overline{d}\overline{u}11jj}^{V1,LR} - \frac{22}{3}L_{\overline{d}\overline{u}22jj}^{V1,LR} - \frac{22}{3}L_{\overline{d}\overline{u}33jj}^{V1,LR} + \frac{787}{81}L_{\overline{d}\overline{u}11jj}^{V8,LR} + \frac{787}{81}L_{\overline{d}\overline{u}22jj}^{V8,LR} \\
& + \frac{787}{81}L_{\overline{d}\overline{u}33jj}^{V8,LR} - \frac{2}{3}L_{\overline{u}\overline{d}ii11}^{V1,LL} - \frac{2}{3}L_{\overline{u}\overline{d}ii22}^{V1,LL} - \frac{2}{3}L_{\overline{u}\overline{d}ii33}^{V1,LL} - \frac{22}{3}L_{\overline{u}\overline{d}ii11}^{V1,LR} - \frac{22}{3}L_{\overline{u}\overline{d}ii22}^{V1,LR} \\
& - \frac{22}{3}L_{\overline{u}\overline{d}ii33}^{V1,LR} - \frac{2}{3}L_{\overline{u}\overline{d}jj11}^{V1,RR} - \frac{2}{3}L_{\overline{u}\overline{d}jj22}^{V1,RR} - \frac{2}{3}L_{\overline{u}\overline{d}jj33}^{V1,RR} + \frac{607}{81}L_{\overline{u}\overline{d}ii11}^{V8,LL} + \frac{607}{81}L_{\overline{u}\overline{d}ii22}^{V8,LL} \\
& + \frac{607}{81}L_{\overline{u}\overline{d}ii33}^{V8,LL} + \frac{787}{81}L_{\overline{u}\overline{d}ii11}^{V8,LR} + \frac{787}{81}L_{\overline{u}\overline{d}ii22}^{V8,LR} + \frac{787}{81}L_{\overline{u}\overline{d}ii33}^{V8,LR} + \frac{607}{81}L_{\overline{u}\overline{d}jj11}^{V8,RR} + \frac{607}{81}L_{\overline{u}\overline{d}jj22}^{V8,RR} \\
& + \frac{607}{81}L_{\overline{u}\overline{d}jj33}^{V8,RR} \Big]
\end{aligned}$$

$$\begin{aligned}
& + \frac{607}{81} L_{ud,jj33}^{V8,RR} - \frac{22}{3} L_{uu,iii}^{V1,LR} - \frac{374}{3} L_{uu,ijj}^{V1,LR} - \frac{22}{3} L_{uu,ikk}^{V1,LR} - \frac{22}{3} L_{uu,jjj}^{V1,LR} - \frac{22}{3} L_{uu,kkj}^{V1,LR} \\
& + \frac{787}{81} L_{uu,iii}^{V8,LR} - \frac{2975}{18} L_{uu,ijj}^{V8,LR} + \frac{787}{81} L_{uu,ikk}^{V8,LR} + \frac{787}{81} L_{uu,jjj}^{V8,LR} + \frac{787}{81} L_{uu,kkj}^{V8,LR} \\
& + \frac{1198}{27} L_{uu,iii}^{V,LL} - \frac{28}{3} L_{uu,ikk}^{V,LL} + \frac{3448}{81} L_{uu,ikk}^{V,LL} + \frac{1198}{27} L_{uu,jjj}^{V,RR} - \frac{28}{3} L_{uu,jjk}^{V,RR} + \frac{3448}{81} L_{uu,jkk}^{V,RR} \Big] \\
& + \alpha_s \alpha \Bigg[ - \frac{544}{81} L_{du,11jj}^{V1,LR} - \frac{544}{81} L_{du,22jj}^{V1,LR} + \frac{1160}{81} L_{du,33jj}^{V1,LR} + \frac{22}{9} L_{du,11jj}^{V8,LR} + \frac{22}{9} L_{du,22jj}^{V8,LR} \\
& + \frac{56}{9} L_{du,33jj}^{V8,LR} - \frac{544}{81} L_{eu,11ii}^{V,LL} - \frac{544}{81} L_{eu,22ii}^{V,LL} - \frac{544}{81} L_{eu,33ii}^{V,LL} - \frac{544}{81} L_{eu,11jj}^{V,LR} - \frac{544}{81} L_{eu,22jj}^{V,LR} \\
& - \frac{544}{81} L_{eu,33jj}^{V,LR} - \frac{544}{81} L_{eu,11jj}^{V,RR} - \frac{544}{81} L_{eu,22jj}^{V,RR} - \frac{544}{81} L_{eu,33jj}^{V,RR} - \frac{544}{81} L_{ud,ii11}^{V1,LL} - \frac{544}{81} L_{ud,ii22}^{V1,LL} \\
& - \frac{544}{81} L_{ud,ii33}^{V1,LL} - \frac{544}{81} L_{ud,ii11}^{V1,LR} - \frac{544}{81} L_{ud,ii22}^{V1,LR} + \frac{1160}{81} L_{ud,ii33}^{V1,LR} - \frac{544}{81} L_{ud,jj11}^{V1,RR} \\
& - \frac{544}{81} L_{ud,jj22}^{V1,RR} - \frac{544}{81} L_{ud,jj33}^{V1,RR} + \frac{170}{27} L_{ud,ii11}^{V8,LL} + \frac{170}{27} L_{ud,ii22}^{V8,LL} + \frac{170}{27} L_{ud,ii33}^{V8,LL} + \frac{22}{9} L_{ud,ii11}^{V8,LR} \\
& + \frac{22}{9} L_{ud,ii22}^{V8,LR} + \frac{56}{9} L_{ud,ii33}^{V8,LR} + \frac{170}{27} L_{ud,jj11}^{V8,RR} + \frac{170}{27} L_{ud,jj22}^{V8,RR} + \frac{170}{27} L_{ud,jj33}^{V8,RR} - \frac{544}{81} L_{ue,ii11}^{V,LR} \\
& - \frac{544}{81} L_{ue,ii22}^{V,LR} - \frac{544}{81} L_{ue,ii33}^{V,LR} + \frac{1088}{81} L_{uu,iii}^{V1,LR} - \frac{16}{3} L_{uu,ijj}^{V1,LR} + \frac{1088}{81} L_{uu,ikk}^{V1,LR} + \frac{1088}{81} L_{uu,jjj}^{V1,LR} \\
& + \frac{1088}{81} L_{uu,kkj}^{V1,LR} + \frac{56}{9} L_{uu,iii}^{V8,LR} - \frac{104}{9} L_{uu,ijj}^{V8,LR} + \frac{56}{9} L_{uu,ikk}^{V8,LR} + \frac{56}{9} L_{uu,jjj}^{V8,LR} + \frac{56}{9} L_{uu,kkj}^{V8,LR} \\
& + \frac{1360}{81} L_{uu,iii}^{V,LL} + \frac{2176}{81} L_{uu,ikk}^{V,LL} - \frac{4256}{243} L_{uu,ikk}^{V,LL} + \frac{1360}{81} L_{uu,jjj}^{V,RR} + \frac{2176}{81} L_{uu,jjk}^{V,RR} \\
& - \frac{4256}{243} L_{uu,jkk}^{V,RR} \Big] + \frac{7520}{81} L_{uu,ijj}^{V8,LR} \alpha^2 ;
\end{aligned}$$

$$\begin{aligned}
\dot{L}_{uu,iii}^{V1,LR} = & - \frac{8}{3} L_{uu,iii}^{V8,LR} g_s^2 + e^2 \Bigg[ - \frac{8}{9} L_{du,11ii}^{V1,LR} - \frac{8}{9} L_{du,22ii}^{V1,LR} - \frac{8}{9} L_{du,33ii}^{V1,LR} - \frac{8}{9} L_{eu,11ii}^{V,LL} \\
& - \frac{8}{9} L_{eu,22ii}^{V,LL} - \frac{8}{9} L_{eu,33ii}^{V,LL} - \frac{8}{9} L_{eu,11ii}^{V,LR} - \frac{8}{9} L_{eu,22ii}^{V,LR} - \frac{8}{9} L_{eu,33ii}^{V,LR} - \frac{8}{9} L_{eu,11ii}^{V,RR} \\
& - \frac{8}{9} L_{eu,22ii}^{V,RR} - \frac{8}{9} L_{eu,33ii}^{V,RR} - \frac{8}{9} L_{ud,ii11}^{V1,LL} - \frac{8}{9} L_{ud,ii22}^{V1,LL} - \frac{8}{9} L_{ud,ii33}^{V1,LL} - \frac{8}{9} L_{ud,ii11}^{V1,LR} \\
& - \frac{8}{9} L_{ud,ii22}^{V1,LR} - \frac{8}{9} L_{ud,ii33}^{V1,LR} - \frac{8}{9} L_{ud,ii11}^{V1,RR} - \frac{8}{9} L_{ud,ii22}^{V1,RR} - \frac{8}{9} L_{ud,ii33}^{V1,RR} - \frac{8}{9} L_{ue,ii11}^{V,LR}
\end{aligned}$$

$$\begin{aligned}
& -\frac{8}{9}L_{ue,ii22}^{V,LR} - \frac{8}{9}L_{ue,ii33}^{V,LR} - \frac{16}{9}L_{uu,iii}^{V1,LR} + \frac{16}{9}L_{uu,ikk}^{V1,LR} + \frac{16}{9}L_{uu,kki}^{V1,LR} + \frac{128}{27}L_{uu,iii}^{V,LL} \\
& + \frac{32}{9}L_{uu,ikk}^{V,LL} + \frac{32}{27}L_{uu,ikki}^{V,LL} + \frac{128}{27}L_{uu,iii}^{V,RR} + \frac{32}{9}L_{uu,ikk}^{V,RR} + \frac{32}{27}L_{uu,ikki}^{V,RR} \Big] + \alpha_s^2 \Big[ 8L_{du,11ii}^{V1,LR} \\
& + 8L_{du,22ii}^{V1,LR} + 8L_{du,33ii}^{V1,LR} + \frac{44}{27}L_{du,11ii}^{V8,LR} + \frac{44}{27}L_{du,22ii}^{V8,LR} + \frac{44}{27}L_{du,33ii}^{V8,LR} - 8L_{ud,i11}^{V1,LL} \\
& - 8L_{ud,i22}^{V1,LL} - 8L_{ud,i33}^{V1,LL} + 8L_{ud,i11}^{V1,LR} + 8L_{ud,i22}^{V1,LR} + 8L_{ud,i33}^{V1,LR} - 8L_{ud,i11}^{V1,RR} \\
& - 8L_{ud,i22}^{V1,RR} - 8L_{ud,i33}^{V1,RR} + \frac{44}{27}L_{ud,i11}^{V8,LL} + \frac{44}{27}L_{ud,i22}^{V8,LL} + \frac{44}{27}L_{ud,i33}^{V8,LL} + \frac{44}{27}L_{ud,i11}^{V8,LR} \\
& + \frac{44}{27}L_{ud,i22}^{V8,LR} + \frac{44}{27}L_{ud,i33}^{V8,LR} + \frac{44}{27}L_{ud,i11}^{V8,RR} + \frac{44}{27}L_{ud,i22}^{V8,RR} + \frac{44}{27}L_{ud,i33}^{V8,RR} + \frac{20}{3}L_{uu,iii}^{V1,LR} \\
& + 8L_{uu,ikk}^{V1,LR} + 8L_{uu,kki}^{V1,LR} - \frac{652}{9}L_{uu,iii}^{V8,LR} + \frac{44}{27}L_{uu,ikk}^{V8,LR} + \frac{44}{27}L_{uu,kki}^{V8,LR} - \frac{232}{9}L_{uu,iii}^{V,LL} \\
& - 16L_{uu,ikk}^{V,LL} - \frac{64}{27}L_{uu,ikki}^{V,LL} - \frac{232}{9}L_{uu,iii}^{V,RR} - 16L_{uu,ikk}^{V,RR} - \frac{64}{27}L_{uu,ikki}^{V,RR} \Big] + \alpha_s \alpha \Big[ -\frac{32}{9}L_{du,11ii}^{V1,LR} \\
& - \frac{32}{9}L_{du,22ii}^{V1,LR} + \frac{64}{9}L_{du,33ii}^{V1,LR} + \frac{664}{729}L_{du,11ii}^{V8,LR} + \frac{664}{729}L_{du,22ii}^{V8,LR} - \frac{4088}{729}L_{du,33ii}^{V8,LR} - \frac{32}{9}L_{ud,i11}^{V1,LL} \\
& - \frac{32}{9}L_{ud,i22}^{V1,LL} - \frac{32}{9}L_{ud,i33}^{V1,LL} - \frac{32}{9}L_{ud,i11}^{V1,LR} - \frac{32}{9}L_{ud,i22}^{V1,LR} + \frac{64}{9}L_{ud,i33}^{V1,LR} - \frac{32}{9}L_{ud,i11}^{V1,RR} \\
& - \frac{32}{9}L_{ud,i22}^{V1,RR} - \frac{32}{9}L_{ud,i33}^{V1,RR} - \frac{776}{729}L_{ud,i11}^{V8,LL} - \frac{776}{729}L_{ud,i22}^{V8,LL} - \frac{776}{729}L_{ud,i33}^{V8,LL} + \frac{664}{729}L_{ud,i11}^{V8,LR} \\
& + \frac{664}{729}L_{ud,i22}^{V8,LR} - \frac{4088}{729}L_{ud,i33}^{V8,LR} - \frac{776}{729}L_{ud,i11}^{V8,RR} - \frac{776}{729}L_{ud,i22}^{V8,RR} - \frac{776}{729}L_{ud,i33}^{V8,RR} \\
& + \frac{512}{9}L_{uu,iii}^{V1,LR} + \frac{64}{9}L_{uu,ikk}^{V1,LR} + \frac{64}{9}L_{uu,kki}^{V1,LR} - \frac{9040}{729}L_{uu,iii}^{V8,LR} - \frac{4088}{729}L_{uu,ikk}^{V8,LR} - \frac{4088}{729}L_{uu,kki}^{V8,LR} \\
& + \frac{4192}{243}L_{uu,iii}^{V,LL} + \frac{32}{3}L_{uu,ikk}^{V,LL} + \frac{256}{729}L_{uu,ikki}^{V,LL} + \frac{4192}{243}L_{uu,iii}^{V,RR} + \frac{32}{3}L_{uu,ikk}^{V,RR} + \frac{256}{729}L_{uu,ikki}^{V,RR} \Big] \\
& + \alpha^2 \Big[ -\frac{2392}{729}L_{du,11ii}^{V1,LR} - \frac{2392}{729}L_{du,22ii}^{V1,LR} + \frac{3776}{729}L_{du,33ii}^{V1,LR} - \frac{8152}{729}L_{du,11ii}^{V,LL} - \frac{8152}{729}L_{du,22ii}^{V,LL} \\
& - \frac{8152}{729}L_{du,33ii}^{V,LL} - \frac{4696}{729}L_{du,11ii}^{V,LR} - \frac{4696}{729}L_{du,22ii}^{V,LR} - \frac{4696}{729}L_{du,33ii}^{V,LR} - \frac{8152}{729}L_{du,11ii}^{V,RR} \\
& - \frac{8152}{729}L_{du,22ii}^{V,RR} - \frac{8152}{729}L_{du,33ii}^{V,RR} - \frac{3544}{729}L_{ud,i11}^{V1,LL} - \frac{3544}{729}L_{ud,i22}^{V1,LL} - \frac{3544}{729}L_{ud,i33}^{V1,LL} \\
& - \frac{2392}{729}L_{ud,i11}^{V1,LR} - \frac{2392}{729}L_{ud,i22}^{V1,LR} + \frac{3776}{729}L_{ud,i33}^{V1,LR} - \frac{3544}{729}L_{ud,i11}^{V1,RR} - \frac{3544}{729}L_{ud,i22}^{V1,RR} \\
& - \frac{3544}{729}L_{ud,i33}^{V1,RR} \Big]
\end{aligned}$$

$$\begin{aligned}
& -\frac{3544}{729}L_{ud\ i33}^{V1,RR} - \frac{4696}{729}L_{ue\ ii1}^{V,LR} - \frac{4696}{729}L_{ue\ ii2}^{V,LR} - \frac{4696}{729}L_{ue\ i33}^{V,LR} + \frac{76384}{729}L_{uu\ iii}^{V1,LR} \\
& + \frac{4352}{729}L_{uu\ iikk}^{V1,LR} + \frac{4352}{729}L_{uu\ kkii}^{V1,LR} - \frac{10496}{729}L_{uu\ iii}^{V,LL} - \frac{512}{729}L_{uu\ iikk}^{V,LL} - \frac{13568}{2187}L_{uu\ ikki}^{V,LL} \\
& - \frac{10496}{729}L_{uu\ iii}^{V,RR} - \frac{512}{729}L_{uu\ iikk}^{V,RR} - \frac{13568}{2187}L_{uu\ ikki}^{V,RR} \Big] ;
\end{aligned}$$

$$\begin{aligned}
\dot{L}_{uu\ iii}^{V8,LR} = & g_s^2 \Bigg[ \frac{2}{3}L_{du\ 11ii}^{V8,LR} + \frac{2}{3}L_{du\ 22ii}^{V8,LR} + \frac{2}{3}L_{du\ 33ii}^{V8,LR} + \frac{2}{3}L_{ud\ ii1}^{V8,LL} + \frac{2}{3}L_{ud\ ii2}^{V8,LL} \\
& + \frac{2}{3}L_{ud\ i33}^{V8,LL} + \frac{2}{3}L_{ud\ ii1}^{V8,LR} + \frac{2}{3}L_{ud\ ii2}^{V8,LR} + \frac{2}{3}L_{ud\ i33}^{V8,LR} + \frac{2}{3}L_{ud\ ii1}^{V8,RR} + \frac{2}{3}L_{ud\ ii2}^{V8,RR} \\
& + \frac{2}{3}L_{ud\ i33}^{V8,RR} - 12L_{uu\ iii}^{V1,LR} - \frac{38}{3}L_{uu\ iii}^{V8,LR} + \frac{2}{3}L_{uu\ iikk}^{V8,LR} + \frac{2}{3}L_{uu\ kkii}^{V8,LR} + \frac{8}{3}L_{uu\ iii}^{V,LL} \\
& + \frac{8}{3}L_{uu\ ikki}^{V,LL} + \frac{8}{3}L_{uu\ iii}^{V,RR} + \frac{8}{3}L_{uu\ ikki}^{V,RR} \Bigg] - \frac{16}{3}L_{uu\ iii}^{V8,LR}e^2 + \alpha_s^2 \Bigg[ -\frac{22}{3}L_{du\ 11ii}^{V1,LR} \\
& - \frac{22}{3}L_{du\ 22ii}^{V1,LR} - \frac{22}{3}L_{du\ 33ii}^{V1,LR} + \frac{787}{81}L_{du\ 11ii}^{V8,LR} + \frac{787}{81}L_{du\ 22ii}^{V8,LR} + \frac{787}{81}L_{du\ 33ii}^{V8,LR} - \frac{2}{3}L_{ud\ ii1}^{V1,LL} \\
& - \frac{2}{3}L_{ud\ ii2}^{V1,LL} - \frac{2}{3}L_{ud\ i33}^{V1,LL} - \frac{22}{3}L_{ud\ ii1}^{V1,LR} - \frac{22}{3}L_{ud\ ii2}^{V1,LR} - \frac{22}{3}L_{ud\ i33}^{V1,LR} - \frac{2}{3}L_{ud\ ii1}^{V1,RR} \\
& - \frac{2}{3}L_{ud\ ii2}^{V1,RR} - \frac{2}{3}L_{ud\ i33}^{V1,RR} + \frac{607}{81}L_{ud\ ii1}^{V8,LL} + \frac{607}{81}L_{ud\ ii2}^{V8,LL} + \frac{607}{81}L_{ud\ i33}^{V8,LL} + \frac{787}{81}L_{ud\ ii1}^{V8,LR} \\
& + \frac{787}{81}L_{ud\ ii2}^{V8,LR} + \frac{787}{81}L_{ud\ i33}^{V8,LR} + \frac{607}{81}L_{ud\ ii1}^{V8,RR} + \frac{607}{81}L_{ud\ ii2}^{V8,RR} + \frac{607}{81}L_{ud\ i33}^{V8,RR} - \frac{418}{3}L_{uu\ iii}^{V1,LR} \\
& - \frac{22}{3}L_{uu\ iikk}^{V1,LR} - \frac{22}{3}L_{uu\ kkii}^{V1,LR} - \frac{23627}{162}L_{uu\ iii}^{V8,LR} + \frac{787}{81}L_{uu\ iikk}^{V8,LR} + \frac{787}{81}L_{uu\ kkii}^{V8,LR} + \frac{1198}{27}L_{uu\ iii}^{V,LL} \\
& - \frac{28}{3}L_{uu\ iikk}^{V,LL} + \frac{3448}{81}L_{uu\ ikki}^{V,LL} + \frac{1198}{27}L_{uu\ iii}^{V,RR} - \frac{28}{3}L_{uu\ iikk}^{V,RR} + \frac{3448}{81}L_{uu\ ikki}^{V,RR} \Bigg] \\
& + \alpha_s \alpha \Bigg[ -\frac{544}{81}L_{du\ 11ii}^{V1,LR} - \frac{544}{81}L_{du\ 22ii}^{V1,LR} + \frac{1160}{81}L_{du\ 33ii}^{V1,LR} + \frac{22}{9}L_{du\ 11ii}^{V8,LR} + \frac{22}{9}L_{du\ 22ii}^{V8,LR} \\
& + \frac{56}{9}L_{du\ 33ii}^{V8,LR} - \frac{544}{81}L_{eu\ 11ii}^{V,LL} - \frac{544}{81}L_{eu\ 22ii}^{V,LL} - \frac{544}{81}L_{eu\ 33ii}^{V,LL} - \frac{544}{81}L_{eu\ 11ii}^{V,LR} - \frac{544}{81}L_{eu\ 22ii}^{V,LR} \\
& - \frac{544}{81}L_{eu\ 33ii}^{V,LR} - \frac{544}{81}L_{eu\ 11ii}^{V,RR} - \frac{544}{81}L_{eu\ 22ii}^{V,RR} - \frac{544}{81}L_{eu\ 33ii}^{V,RR} - \frac{544}{81}L_{ud\ ii1}^{V1,LL} - \frac{544}{81}L_{ud\ ii2}^{V1,LL} \\
& - \frac{544}{81}L_{ud\ i33}^{V1,LL} - \frac{544}{81}L_{ud\ ii1}^{V1,LR} - \frac{544}{81}L_{ud\ ii2}^{V1,LR} + \frac{1160}{81}L_{ud\ i33}^{V1,LR} - \frac{544}{81}L_{ud\ ii1}^{V1,RR}
\end{aligned}$$

$$\begin{aligned}
& -\frac{544}{81}L_{ud\ i22}^{V1,RR} - \frac{544}{81}L_{ud\ i33}^{V1,RR} + \frac{170}{27}L_{ud\ i11}^{V8,LL} + \frac{170}{27}L_{ud\ i22}^{V8,LL} + \frac{170}{27}L_{ud\ i33}^{V8,LL} + \frac{22}{9}L_{ud\ i11}^{V8,LR} \\
& + \frac{22}{9}L_{ud\ i22}^{V8,LR} + \frac{56}{9}L_{ud\ i33}^{V8,LR} + \frac{170}{27}L_{ud\ i11}^{V8,RR} + \frac{170}{27}L_{ud\ i22}^{V8,RR} + \frac{170}{27}L_{ud\ i33}^{V8,RR} - \frac{544}{81}L_{ue\ i11}^{V,LR} \\
& - \frac{544}{81}L_{ue\ i22}^{V,LR} - \frac{544}{81}L_{ue\ i33}^{V,LR} + \frac{1744}{81}L_{uu\ i11}^{V1,LR} + \frac{1088}{81}L_{uu\ i22}^{V1,LR} + \frac{1088}{81}L_{uu\ i33}^{V1,LR} \\
& + \frac{8}{9}L_{uu\ i11}^{V8,LR} + \frac{56}{9}L_{uu\ i22}^{V8,LR} + \frac{56}{9}L_{uu\ i33}^{V8,LR} + \frac{1360}{81}L_{uu\ i11}^{V,LL} + \frac{2176}{81}L_{uu\ i22}^{V,LL} - \frac{4256}{243}L_{uu\ i33}^{V,LL} \\
& + \frac{1360}{81}L_{uu\ i11}^{V,RR} + \frac{2176}{81}L_{uu\ i22}^{V,RR} - \frac{4256}{243}L_{uu\ i33}^{V,RR} \Big] + \frac{7520}{81}L_{uu\ i11}^{V8,LR}\alpha^2;
\end{aligned}$$

$$\begin{aligned}
\dot{L}_{ee\ ij}^{V,LR} &= e^2 \Bigg[ \frac{16}{3}L_{ee\ ij}^{V,LL} - \frac{32}{3}L_{ee\ ij}^{V,LR} + \frac{16}{3}L_{ee\ ijk}^{V,LL} + \frac{4}{3}L_{ee\ ijk}^{V,LR} + \frac{4}{3}L_{ed\ i11}^{V,LL} \\
& + \frac{4}{3}L_{ed\ i22}^{V,LL} + \frac{4}{3}L_{ed\ i33}^{V,LL} + \frac{4}{3}L_{ed\ i11}^{V,LR} + \frac{4}{3}L_{ed\ i22}^{V,LR} + \frac{4}{3}L_{ed\ i33}^{V,LR} + \frac{16}{3}L_{ee\ i11}^{V,LL} \\
& + \frac{4}{3}L_{ee\ i22}^{V,LR} - \frac{8}{3}L_{eu\ i11}^{V,LL} - \frac{8}{3}L_{eu\ i22}^{V,LL} - \frac{8}{3}L_{eu\ i11}^{V,LR} - \frac{8}{3}L_{eu\ i22}^{V,LR} + \frac{4}{3}L_{ee\ i33}^{V,LR} \\
& + \frac{16}{3}L_{ee\ j11}^{V,RR} + \frac{4}{3}L_{de\ i11}^{V,LR} + \frac{4}{3}L_{de\ i22}^{V,LR} + \frac{4}{3}L_{de\ i33}^{V,LR} + \frac{4}{3}L_{ed\ j11}^{V,RR} + \frac{4}{3}L_{ed\ j22}^{V,RR} \\
& + \frac{4}{3}L_{ed\ j33}^{V,RR} + \frac{8}{3}L_{ee\ j11}^{V,LR} + 8L_{ee\ j22}^{V,RR} - \frac{8}{3}L_{eu\ j11}^{V,RR} - \frac{8}{3}L_{eu\ j22}^{V,RR} - \frac{8}{3}L_{eu\ j33}^{V,LR} \\
& - \frac{8}{3}L_{ue\ j11}^{V,LR} \Big] + \alpha_s \alpha \Bigg[ \frac{16}{3}L_{ed\ i11}^{V,LL} + \frac{16}{3}L_{ed\ i22}^{V,LL} + \frac{16}{3}L_{ed\ i33}^{V,LL} + \frac{16}{3}L_{ed\ i11}^{V,LR} \\
& + \frac{16}{3}L_{ed\ i22}^{V,LR} + \frac{16}{3}L_{ed\ i33}^{V,LR} - \frac{32}{3}L_{eu\ i11}^{V,LL} - \frac{32}{3}L_{eu\ i22}^{V,LL} - \frac{32}{3}L_{eu\ i11}^{V,LR} - \frac{32}{3}L_{eu\ i22}^{V,LR} \\
& + \frac{16}{3}L_{de\ i11}^{V,LR} + \frac{16}{3}L_{de\ i22}^{V,LR} + \frac{16}{3}L_{de\ i33}^{V,LR} + \frac{16}{3}L_{ed\ j11}^{V,RR} + \frac{16}{3}L_{ed\ j22}^{V,RR} + \frac{16}{3}L_{ed\ j33}^{V,RR} \\
& - \frac{32}{3}L_{eu\ j11}^{V,RR} - \frac{32}{3}L_{eu\ j22}^{V,RR} - \frac{32}{3}L_{ue\ i11}^{V,LR} - \frac{32}{3}L_{ue\ i22}^{V,LR} \Big] + \alpha^2 \Bigg[ \frac{32}{27}L_{ee\ ij}^{V,LL} \\
& + \frac{6386}{27}L_{ee\ ij}^{V,LR} + \frac{32}{27}L_{ee\ ijk}^{V,LL} + \frac{296}{27}L_{ee\ ijk}^{V,LR} - \frac{344}{81}L_{ed\ i11}^{V,LL} - \frac{344}{81}L_{ed\ i22}^{V,LL} - \frac{344}{81}L_{ed\ i33}^{V,LL} \\
& + \frac{424}{81}L_{ed\ i11}^{V,LR} + \frac{424}{81}L_{ed\ i22}^{V,LR} + \frac{424}{81}L_{ed\ i33}^{V,LR} - \frac{736}{27}L_{ee\ i11}^{V,LL} + \frac{296}{27}L_{ee\ i22}^{V,LR} - \frac{3128}{81}L_{eu\ i11}^{V,LL} \\
& - \frac{3128}{81}L_{eu\ i22}^{V,LL} - \frac{56}{81}L_{eu\ i11}^{V,LR} - \frac{56}{81}L_{eu\ i22}^{V,LR} + \frac{296}{27}L_{ee\ ijk}^{V,LR} + \frac{32}{27}L_{ee\ j11}^{V,RR} + \frac{424}{81}L_{de\ i11}^{V,LR}
\end{aligned}$$



$$\begin{aligned}
& + \frac{424}{81} L_{22jj}^{V,LR} + \frac{424}{81} L_{33jj}^{V,LR} - \frac{344}{81} L_{jj11}^{V,RR} - \frac{344}{81} L_{jj22}^{V,RR} - \frac{344}{81} L_{jj33}^{V,RR} + \frac{592}{27} L_{jjj}^{V,LR} \\
& - \frac{80}{3} L_{jjjj}^{V,RR} - \frac{3128}{81} L_{jj11}^{V,RR} - \frac{3128}{81} L_{jj22}^{V,RR} - \frac{56}{81} L_{11jj}^{V,LR} - \frac{56}{81} L_{22jj}^{V,LR} \Bigg] ;
\end{aligned}$$

$$\begin{aligned}
\dot{L}_{iii}^{V,LR} = & e^2 \left[ \frac{16}{3} L_{ijj}^{V,LL} + \frac{4}{3} L_{ijj}^{V,LR} + \frac{4}{3} L_{jji}^{V,LR} + \frac{16}{3} L_{ijj}^{V,RR} + \frac{16}{3} L_{iik}^{V,LL} \right. \\
& + \frac{4}{3} L_{iik}^{V,LR} + \frac{4}{3} L_{kkii}^{V,LR} + \frac{16}{3} L_{iik}^{V,RR} + \frac{4}{3} L_{de11ii}^{V,LR} + \frac{4}{3} L_{de22ii}^{V,LR} + \frac{4}{3} L_{de33ii}^{V,LR} \\
& + \frac{4}{3} L_{edii11}^{V,LL} + \frac{4}{3} L_{edii22}^{V,LL} + \frac{4}{3} L_{edii33}^{V,LL} + \frac{4}{3} L_{edii11}^{V,LR} + \frac{4}{3} L_{edii22}^{V,LR} + \frac{4}{3} L_{edii33}^{V,LR} \\
& + \frac{4}{3} L_{edii11}^{V,RR} + \frac{4}{3} L_{edii22}^{V,RR} + \frac{4}{3} L_{edii33}^{V,RR} + \frac{16}{3} L_{iii}^{V,LL} - \frac{28}{3} L_{iii}^{V,LR} + \frac{16}{3} L_{iii}^{V,RR} \\
& - \frac{8}{3} L_{ii11}^{V,LL} - \frac{8}{3} L_{ii22}^{V,LL} - \frac{8}{3} L_{ii11}^{V,LR} - \frac{8}{3} L_{ii22}^{V,LR} - \frac{8}{3} L_{ii11}^{V,RR} - \frac{8}{3} L_{ii22}^{V,RR} \\
& \left. - \frac{8}{3} L_{11ii}^{V,LR} - \frac{8}{3} L_{22ii}^{V,LR} \right] + \alpha_s \alpha \left[ \frac{16}{3} L_{de11ii}^{V,LR} + \frac{16}{3} L_{de22ii}^{V,LR} + \frac{16}{3} L_{de33ii}^{V,LR} \right. \\
& + \frac{16}{3} L_{edii11}^{V,LL} + \frac{16}{3} L_{edii22}^{V,LL} + \frac{16}{3} L_{edii33}^{V,LL} + \frac{16}{3} L_{edii11}^{V,LR} + \frac{16}{3} L_{edii22}^{V,LR} + \frac{16}{3} L_{edii33}^{V,LR} \\
& + \frac{16}{3} L_{edii11}^{V,RR} + \frac{16}{3} L_{edii22}^{V,RR} + \frac{16}{3} L_{edii33}^{V,RR} - \frac{32}{3} L_{ii11}^{V,LL} - \frac{32}{3} L_{ii22}^{V,LL} - \frac{32}{3} L_{ii11}^{V,LR} \\
& - \frac{32}{3} L_{ii22}^{V,LR} - \frac{32}{3} L_{ii11}^{V,RR} - \frac{32}{3} L_{ii22}^{V,RR} - \frac{32}{3} L_{11ii}^{V,LR} - \frac{32}{3} L_{22ii}^{V,LR} \Bigg] + \alpha^2 \left[ \frac{32}{27} L_{ijj}^{V,LL} \right. \\
& + \frac{296}{27} L_{ijj}^{V,LR} + \frac{296}{27} L_{jji}^{V,LR} + \frac{32}{27} L_{ijj}^{V,RR} + \frac{32}{27} L_{iik}^{V,LL} + \frac{296}{27} L_{iik}^{V,LR} + \frac{296}{27} L_{kkii}^{V,LR} \\
& + \frac{32}{27} L_{iik}^{V,RR} + \frac{424}{81} L_{de11ii}^{V,LR} + \frac{424}{81} L_{de22ii}^{V,LR} + \frac{424}{81} L_{de33ii}^{V,LR} - \frac{344}{81} L_{edii11}^{V,LL} - \frac{344}{81} L_{edii22}^{V,LL} \\
& - \frac{344}{81} L_{edii33}^{V,LL} + \frac{424}{81} L_{edii11}^{V,LR} + \frac{424}{81} L_{edii22}^{V,LR} + \frac{424}{81} L_{edii33}^{V,LR} - \frac{344}{81} L_{edii11}^{V,RR} - \frac{344}{81} L_{edii22}^{V,RR} \\
& - \frac{344}{81} L_{edii33}^{V,RR} - \frac{736}{27} L_{iii}^{V,LL} + \frac{6682}{27} L_{iii}^{V,LR} - \frac{736}{27} L_{iii}^{V,RR} - \frac{3128}{81} L_{ii11}^{V,LL} - \frac{3128}{81} L_{ii22}^{V,LL} \\
& \left. - \frac{56}{81} L_{ii11}^{V,LR} - \frac{56}{81} L_{ii22}^{V,LR} - \frac{3128}{81} L_{ii11}^{V,RR} - \frac{3128}{81} L_{ii22}^{V,RR} - \frac{56}{81} L_{11ii}^{V,LR} - \frac{56}{81} L_{22ii}^{V,LR} \right] ;
\end{aligned}$$

$$\dot{L}_{ijj}^{V,RR} = e^2 \left[ \frac{8}{3} L_{jjjj}^{V1,LR} + \frac{4}{3} L_{kkjj}^{V1,LR} + \frac{64}{9} L_{jjjj}^{V,RR} + \frac{8}{3} L_{jjkk}^{V,RR} + \frac{8}{9} L_{jkkj}^{V,RR} \right]$$

$$\begin{aligned}
& + \frac{4}{9}L_{11ii}^{V,LR} + \frac{4}{9}L_{22ii}^{V,LR} + \frac{4}{9}L_{33ii}^{V,LR} + \frac{4}{3}L_{11jj}^{V,LR} + \frac{4}{3}L_{22jj}^{V,LR} + \frac{4}{3}L_{33jj}^{V,LR} \\
& + \frac{4}{3}L_{11jj}^{V,RR} + \frac{4}{3}L_{22jj}^{V,RR} + \frac{4}{3}L_{33jj}^{V,RR} + \frac{4}{9}L_{ii11}^{V,RR} + \frac{4}{9}L_{ii22}^{V,RR} + \frac{4}{9}L_{ii33}^{V,RR} \\
& + 4L_{ijjj}^{V,RR} + \frac{4}{9}L_{iiii}^{V,LR} + \frac{4}{9}L_{jjii}^{V,LR} + \frac{4}{9}L_{kkii}^{V,LR} + \frac{16}{9}L_{iiii}^{V,RR} + \frac{16}{9}L_{ijjj}^{V,RR} \\
& + \frac{16}{9}L_{iikk}^{V,RR} - \frac{8}{9}L_{ii11}^{V,RR} - \frac{8}{9}L_{ii22}^{V,RR} - \frac{8}{3}L_{11jj}^{V1,LR} - \frac{8}{3}L_{22jj}^{V1,LR} - \frac{8}{3}L_{11jj}^{V1,RR} \\
& - \frac{8}{3}L_{22jj}^{V1,RR} - \frac{8}{9}L_{11ii}^{V,LR} - \frac{8}{9}L_{22ii}^{V,LR} \Big] + \alpha_s^2 \Bigg[ -8L_{11ii}^{V,LR} - 8L_{22ii}^{V,LR} \\
& - 8L_{33ii}^{V,LR} + 8L_{ii11}^{V,RR} + 8L_{ii22}^{V,RR} + 8L_{ii33}^{V,RR} + 8L_{ii11}^{V,RR} + 8L_{ii22}^{V,RR} \\
& - 8L_{11ii}^{V,LR} - 8L_{22ii}^{V,LR} \Big] + \alpha_s \alpha \Bigg[ \frac{32}{3}L_{jjjj}^{V1,LR} + \frac{16}{3}L_{kkjj}^{V1,LR} - \frac{2080}{243}L_{jjjj}^{V8,LR} \\
& - \frac{1040}{243}L_{kkjj}^{V8,LR} + \frac{5008}{243}L_{jjjj}^{V,RR} + 8L_{jjkk}^{V,RR} - \frac{8}{243}L_{jjkk}^{V,RR} + \frac{16}{9}L_{11ii}^{V,LR} + \frac{16}{9}L_{22ii}^{V,LR} \\
& + \frac{16}{9}L_{33ii}^{V,LR} + \frac{16}{9}L_{ii11}^{V,RR} + \frac{16}{9}L_{ii22}^{V,RR} + \frac{16}{9}L_{ii33}^{V,RR} - 16L_{ijjj}^{V,RR} - \frac{32}{9}L_{ii11}^{V,RR} \\
& - \frac{32}{9}L_{ii22}^{V,RR} - \frac{32}{3}L_{11jj}^{V1,LR} - \frac{32}{3}L_{22jj}^{V1,LR} - \frac{32}{3}L_{11jj}^{V1,RR} - \frac{32}{3}L_{22jj}^{V1,RR} + \frac{1336}{243}L_{11jj}^{V8,LR} \\
& + \frac{1336}{243}L_{22jj}^{V8,LR} - \frac{104}{243}L_{11jj}^{V8,RR} - \frac{104}{243}L_{22jj}^{V8,RR} - \frac{32}{9}L_{11ii}^{V,LR} - \frac{32}{9}L_{22ii}^{V,LR} \Big] \\
& + \alpha^2 \Bigg[ -\frac{2624}{243}L_{jjjj}^{V1,LR} - \frac{1312}{243}L_{kkjj}^{V1,LR} + \frac{23296}{729}L_{jjjj}^{V,RR} + \frac{1984}{243}L_{jjkk}^{V,RR} + \frac{2896}{729}L_{jjkk}^{V,RR} \\
& - \frac{200}{243}L_{11ii}^{V,LR} - \frac{200}{243}L_{22ii}^{V,LR} - \frac{200}{243}L_{33ii}^{V,LR} - \frac{3184}{243}L_{11jj}^{V,LR} - \frac{3184}{243}L_{22jj}^{V,LR} \\
& - \frac{3184}{243}L_{33jj}^{V,LR} + \frac{3728}{243}L_{11jj}^{V,RR} + \frac{3728}{243}L_{22jj}^{V,RR} + \frac{3728}{243}L_{33jj}^{V,RR} - \frac{104}{243}L_{ii11}^{V,RR} \\
& - \frac{104}{243}L_{ii22}^{V,RR} - \frac{104}{243}L_{ii33}^{V,RR} - \frac{326}{27}L_{ijjj}^{V,RR} - \frac{520}{81}L_{iiii}^{V,LR} - \frac{520}{81}L_{jjii}^{V,LR} - \frac{520}{81}L_{kkii}^{V,LR} \\
& + \frac{32}{81}L_{iiii}^{V,RR} + \frac{224}{81}L_{ijjj}^{V,RR} + \frac{224}{81}L_{iikk}^{V,RR} - \frac{1016}{243}L_{ii11}^{V,RR} - \frac{1016}{243}L_{ii22}^{V,RR} - \frac{6232}{243}L_{11jj}^{V1,LR} \\
& - \frac{6232}{243}L_{22jj}^{V1,LR} + \frac{2984}{243}L_{11jj}^{V1,RR} + \frac{2984}{243}L_{22jj}^{V1,RR} - \frac{1400}{243}L_{11ii}^{V,LR} - \frac{1400}{243}L_{22ii}^{V,LR} \Big] ;
\end{aligned}$$

$$\begin{aligned}
\dot{L}_{ijj}^{V,RR} = & e^2 \left[ -\frac{8}{9}L_{11ii}^{V,LR} - \frac{8}{9}L_{22ii}^{V,LR} - \frac{8}{9}L_{33ii}^{V,LR} + \frac{4}{3}L_{11jj}^{V1,LR} + \frac{4}{3}L_{22jj}^{V1,LR} \right. \\
& + \frac{4}{3}L_{33jj}^{V1,LR} - \frac{8}{9}L_{ii11}^{V,RR} - \frac{8}{9}L_{ii22}^{V,RR} - \frac{8}{9}L_{ii33}^{V,RR} - \frac{8}{9}L_{iii}^{V,RR} - \frac{8}{9}L_{jjii}^{V,RR} \\
& - \frac{8}{9}L_{kkii}^{V,RR} - \frac{32}{9}L_{iii}^{V,RR} - \frac{32}{9}L_{ijj}^{V,RR} - \frac{32}{9}L_{iik}^{V,RR} + \frac{4}{3}L_{11jj}^{V,LR} + \frac{4}{3}L_{22jj}^{V,LR} \\
& + \frac{4}{3}L_{33jj}^{V,LR} + \frac{4}{3}L_{11jj}^{V,RR} + \frac{4}{3}L_{22jj}^{V,RR} + \frac{4}{3}L_{33jj}^{V,RR} + \frac{16}{9}L_{ii11}^{V,RR} + \frac{16}{9}L_{ii22}^{V,RR} \\
& - 8L_{ijj}^{V,RR} + \frac{4}{3}L_{jj11}^{V1,RR} + \frac{4}{3}L_{jj22}^{V1,RR} + \frac{4}{3}L_{jj33}^{V1,RR} + \frac{16}{9}L_{11ii}^{V,LR} + \frac{16}{9}L_{22ii}^{V,LR} \\
& \left. - \frac{8}{3}L_{jjjj}^{V1,LR} - \frac{8}{3}L_{kkjj}^{V1,LR} - \frac{64}{9}L_{jjjj}^{V,RR} - \frac{16}{3}L_{jjkk}^{V,RR} - \frac{16}{9}L_{jjkk}^{V,RR} \right] + \alpha_s^2 \left[ -8L_{11ii}^{V,LR} \right. \\
& - 8L_{22ii}^{V,LR} - 8L_{33ii}^{V,LR} + 8L_{ii11}^{V,RR} + 8L_{ii22}^{V,RR} + 8L_{ii33}^{V,RR} + 8L_{ii11}^{V,RR} \\
& \left. + 8L_{ii22}^{V,RR} - 8L_{11ii}^{V,LR} - 8L_{22ii}^{V,LR} \right] + \alpha_s \alpha \left[ -\frac{32}{9}L_{11ii}^{V,LR} - \frac{32}{9}L_{22ii}^{V,LR} \right. \\
& - \frac{32}{9}L_{33ii}^{V,LR} + \frac{16}{3}L_{11jj}^{V1,LR} + \frac{16}{3}L_{22jj}^{V1,LR} - \frac{32}{3}L_{33jj}^{V1,LR} - \frac{332}{243}L_{11jj}^{V8,LR} - \frac{332}{243}L_{22jj}^{V8,LR} \\
& + \frac{2044}{243}L_{33jj}^{V8,LR} - \frac{32}{9}L_{ii11}^{V,RR} - \frac{32}{9}L_{ii22}^{V,RR} - \frac{32}{9}L_{ii33}^{V,RR} + \frac{64}{9}L_{ii11}^{V,RR} + \frac{64}{9}L_{ii22}^{V,RR} \\
& + 32L_{ijj}^{V,RR} + \frac{16}{3}L_{jj11}^{V1,RR} + \frac{16}{3}L_{jj22}^{V1,RR} + \frac{16}{3}L_{jj33}^{V1,RR} + \frac{388}{243}L_{jj11}^{V8,RR} + \frac{388}{243}L_{jj22}^{V8,RR} \\
& + \frac{388}{243}L_{jj33}^{V8,RR} + \frac{64}{9}L_{11ii}^{V,LR} + \frac{64}{9}L_{22ii}^{V,LR} - \frac{32}{3}L_{jjjj}^{V1,LR} - \frac{32}{3}L_{kkjj}^{V1,LR} + \frac{2044}{243}L_{jjjj}^{V8,LR} \\
& + \frac{2044}{243}L_{kkjj}^{V8,LR} - \frac{2096}{81}L_{jjjj}^{V,RR} - 16L_{jjkk}^{V,RR} - \frac{128}{243}L_{jjkk}^{V,RR} \left. \right] + \alpha^2 \left[ \frac{1408}{243}L_{11ii}^{V,LR} \right. \\
& + \frac{1408}{243}L_{22ii}^{V,LR} + \frac{1408}{243}L_{33ii}^{V,LR} - \frac{928}{243}L_{11jj}^{V1,LR} - \frac{928}{243}L_{22jj}^{V1,LR} + \frac{416}{243}L_{33jj}^{V1,LR} \\
& + \frac{2512}{243}L_{ii11}^{V,RR} + \frac{2512}{243}L_{ii22}^{V,RR} + \frac{2512}{243}L_{ii33}^{V,RR} + \frac{464}{81}L_{iii}^{V,RR} + \frac{464}{81}L_{jjii}^{V,RR} \\
& + \frac{464}{81}L_{kkii}^{V,RR} + \frac{3680}{81}L_{iii}^{V,RR} + \frac{2432}{81}L_{ijj}^{V,RR} + \frac{2432}{81}L_{iik}^{V,RR} - \frac{424}{243}L_{11jj}^{V,LR} - \frac{424}{243}L_{22jj}^{V,LR} \\
& \left. - \frac{424}{243}L_{33jj}^{V,LR} + \frac{3248}{243}L_{11jj}^{V,RR} + \frac{3248}{243}L_{22jj}^{V,RR} + \frac{3248}{243}L_{33jj}^{V,RR} + \frac{1312}{243}L_{ii11}^{V,RR} \right]
\end{aligned}$$

$$\begin{aligned}
& + \frac{1312}{243} L_{ii22}^{V,RR} + \frac{112}{27} L_{iijj}^{V,RR} + \frac{296}{243} L_{jj11}^{V1,RR} + \frac{296}{243} L_{jj22}^{V1,RR} + \frac{296}{243} L_{jj33}^{V1,RR} \\
& - \frac{3104}{243} L_{11ii}^{V,LR} - \frac{3104}{243} L_{22ii}^{V,LR} + \frac{128}{243} L_{jjjj}^{V1,LR} + \frac{128}{243} L_{kkjj}^{V1,LR} + \frac{26272}{243} L_{jjjj}^{V,RR} \\
& + \frac{10048}{243} L_{jjkk}^{V,RR} + \frac{18304}{729} L_{jjkk}^{V,RR} \Bigg];
\end{aligned}$$

$$\begin{aligned}
\dot{L}_{iijj}^{V1,RR} &= \frac{8}{3} L_{iijj}^{V8,RR} g_s^2 + e^2 \Bigg[ -\frac{16}{9} L_{jjjj}^{V1,LR} - \frac{8}{9} L_{kkjj}^{V1,LR} - \frac{128}{27} L_{jjjj}^{V,RR} - \frac{16}{9} L_{jjkk}^{V,RR} \\
& - \frac{16}{27} L_{jjkk}^{V,RR} + \frac{4}{9} L_{11ii}^{V1,LR} + \frac{4}{9} L_{22ii}^{V1,LR} + \frac{4}{9} L_{33ii}^{V1,LR} - \frac{8}{9} L_{11jj}^{V,LR} - \frac{8}{9} L_{22jj}^{V,LR} \\
& - \frac{8}{9} L_{33jj}^{V,LR} - \frac{8}{9} L_{11jj}^{V,RR} - \frac{8}{9} L_{22jj}^{V,RR} - \frac{8}{9} L_{33jj}^{V,RR} + \frac{4}{9} L_{11ii}^{V,LR} + \frac{4}{9} L_{22ii}^{V,LR} \\
& + \frac{4}{9} L_{33ii}^{V,LR} + \frac{4}{9} L_{11ii}^{V,RR} + \frac{4}{9} L_{22ii}^{V,RR} + \frac{4}{9} L_{33ii}^{V,RR} + \frac{16}{9} L_{11jj}^{V1,LR} + \frac{16}{9} L_{22jj}^{V1,LR} \\
& + \frac{16}{9} L_{11jj}^{V1,RR} + \frac{16}{9} L_{22jj}^{V1,RR} + \frac{4}{9} L_{ii11}^{V1,RR} + \frac{4}{9} L_{ii22}^{V1,RR} + \frac{4}{9} L_{ii33}^{V1,RR} - \frac{8}{3} L_{iijj}^{V1,RR} \\
& - \frac{8}{9} L_{iiii}^{V1,LR} - \frac{8}{9} L_{kkii}^{V1,LR} - \frac{64}{27} L_{iiii}^{V,RR} - \frac{16}{9} L_{iikk}^{V,RR} - \frac{16}{27} L_{ikki}^{V,RR} \Bigg] + \alpha_s^2 \Bigg[ -16 L_{jjjj}^{V1,LR} \\
& - 8 L_{kkjj}^{V1,LR} + \frac{8}{27} L_{jjjj}^{V8,LR} + \frac{4}{27} L_{kkjj}^{V8,LR} + \frac{1672}{27} L_{jjjj}^{V,RR} + 16 L_{jjkk}^{V,RR} + \frac{256}{27} L_{jjkk}^{V,RR} \\
& - 8 L_{11ii}^{V1,LR} - 8 L_{22ii}^{V1,LR} - 8 L_{33ii}^{V1,LR} + \frac{4}{27} L_{11ii}^{V8,LR} + \frac{4}{27} L_{22ii}^{V8,LR} + \frac{4}{27} L_{33ii}^{V8,LR} \\
& - 8 L_{11jj}^{V1,LR} - 8 L_{22jj}^{V1,LR} + 8 L_{11jj}^{V1,RR} + 8 L_{22jj}^{V1,RR} + 8 L_{ii11}^{V1,RR} + 8 L_{ii22}^{V1,RR} \\
& + 8 L_{ii33}^{V1,RR} - \frac{28}{3} L_{iijj}^{V1,RR} + \frac{4}{27} L_{11jj}^{V8,LR} + \frac{4}{27} L_{22jj}^{V8,LR} + \frac{4}{27} L_{11jj}^{V8,RR} + \frac{4}{27} L_{22jj}^{V8,RR} \\
& + \frac{4}{27} L_{ii11}^{V8,RR} + \frac{4}{27} L_{ii22}^{V8,RR} + \frac{4}{27} L_{ii33}^{V8,RR} + \frac{82}{27} L_{iijj}^{V8,RR} - 8 L_{iiii}^{V1,LR} - 8 L_{kkii}^{V1,LR} \\
& + \frac{4}{27} L_{iiii}^{V8,LR} + \frac{4}{27} L_{kkii}^{V8,LR} + \frac{328}{9} L_{iiii}^{V,RR} + 16 L_{iikk}^{V,RR} + \frac{256}{27} L_{ikki}^{V,RR} \Bigg] + \alpha_s \alpha \Bigg[ -\frac{64}{9} L_{jjjj}^{V1,LR} \\
& - \frac{32}{9} L_{kkjj}^{V1,LR} + \frac{4160}{729} L_{jjjj}^{V8,LR} + \frac{2080}{729} L_{kkjj}^{V8,LR} - \frac{10016}{729} L_{jjjj}^{V,RR} - \frac{16}{3} L_{jjkk}^{V,RR} \\
& + \frac{16}{729} L_{jjkk}^{V,RR} + \frac{16}{9} L_{11ii}^{V1,LR} + \frac{16}{9} L_{22ii}^{V1,LR} - \frac{32}{9} L_{33ii}^{V1,LR} - \frac{332}{729} L_{11ii}^{V8,LR} - \frac{332}{729} L_{22ii}^{V8,LR}
\end{aligned}$$

$$\begin{aligned}
& + \frac{2044}{729} L_{33ii}^{V8,LR} + \frac{64}{9} L_{11jj}^{V1,LR} + \frac{64}{9} L_{22jj}^{V1,LR} + \frac{64}{9} L_{11jj}^{V1,RR} + \frac{64}{9} L_{22jj}^{V1,RR} + \frac{16}{9} L_{ii11}^{V1,RR} \\
& + \frac{16}{9} L_{ii22}^{V1,RR} + \frac{16}{9} L_{ii33}^{V1,RR} + \frac{64}{3} L_{ijjj}^{V1,RR} - \frac{2672}{729} L_{11jj}^{V8,LR} - \frac{2672}{729} L_{22jj}^{V8,LR} + \frac{208}{729} L_{11jj}^{V8,RR} \\
& + \frac{208}{729} L_{22jj}^{V8,RR} + \frac{388}{729} L_{ii11}^{V8,RR} + \frac{388}{729} L_{ii22}^{V8,RR} + \frac{388}{729} L_{ii33}^{V8,RR} - \frac{8}{27} L_{ijjj}^{V8,RR} \\
& - \frac{32}{9} L_{iii}^{V1,LR} - \frac{32}{9} L_{kkii}^{V1,LR} + \frac{2044}{729} L_{iii}^{V8,LR} + \frac{2044}{729} L_{kkii}^{V8,LR} - \frac{2096}{243} L_{iii}^{V,RR} \\
& - \frac{16}{3} L_{ikk}^{V,RR} - \frac{128}{729} L_{ikki}^{V,RR} \Big] + \alpha^2 \Big[ - \frac{512}{729} L_{jjjj}^{V1,LR} - \frac{256}{729} L_{kkjj}^{V1,LR} + \frac{40528}{2187} L_{jjjj}^{V,RR} \\
& + \frac{3232}{729} L_{jjkk}^{V,RR} + \frac{5728}{2187} L_{jjkk}^{V,RR} - \frac{136}{729} L_{11ii}^{V1,LR} - \frac{136}{729} L_{22ii}^{V1,LR} + \frac{2720}{729} L_{33ii}^{V1,LR} \\
& - \frac{2992}{729} L_{11jj}^{V,LR} - \frac{2992}{729} L_{22jj}^{V,LR} - \frac{2992}{729} L_{33jj}^{V,LR} + \frac{2624}{729} L_{11jj}^{V,RR} + \frac{2624}{729} L_{22jj}^{V,RR} \\
& + \frac{2624}{729} L_{33jj}^{V,RR} + \frac{1664}{729} L_{11ii}^{V,LR} + \frac{1664}{729} L_{22ii}^{V,LR} + \frac{1664}{729} L_{33ii}^{V,LR} + \frac{1448}{729} L_{11ii}^{V,RR} \\
& + \frac{1448}{729} L_{22ii}^{V,RR} + \frac{1448}{729} L_{33ii}^{V,RR} - \frac{1216}{729} L_{11jj}^{V1,LR} - \frac{1216}{729} L_{22jj}^{V1,LR} + \frac{6272}{729} L_{11jj}^{V1,RR} \\
& + \frac{6272}{729} L_{22jj}^{V1,RR} - \frac{208}{729} L_{ii11}^{V1,RR} - \frac{208}{729} L_{ii22}^{V1,RR} - \frac{208}{729} L_{ii33}^{V1,RR} - \frac{128}{81} L_{ijjj}^{V1,RR} \\
& + \frac{2432}{729} L_{iii}^{V1,LR} + \frac{2432}{729} L_{kkii}^{V1,LR} + \frac{11872}{729} L_{iii}^{V,RR} + \frac{4288}{729} L_{ikk}^{V,RR} + \frac{9088}{2187} L_{ikki}^{V,RR} \Big] ;
\end{aligned}$$

$$\begin{aligned}
\dot{L}_{ijj}^{V8,RR} & = g_s^2 \Big[ \frac{4}{3} L_{jjjj}^{V8,LR} + \frac{2}{3} L_{kkjj}^{V8,LR} + \frac{16}{3} L_{jjjj}^{V,RR} + \frac{8}{3} L_{jjkk}^{V,RR} + \frac{2}{3} L_{11ii}^{V8,LR} \\
& + \frac{2}{3} L_{22ii}^{V8,LR} + \frac{2}{3} L_{33ii}^{V8,LR} + 12 L_{ijjj}^{V1,RR} + \frac{2}{3} L_{11jj}^{V8,LR} + \frac{2}{3} L_{22jj}^{V8,LR} + \frac{2}{3} L_{11jj}^{V8,RR} \\
& + \frac{2}{3} L_{22jj}^{V8,RR} + \frac{2}{3} L_{ii11}^{V8,RR} + \frac{2}{3} L_{ii22}^{V8,RR} + \frac{2}{3} L_{ii33}^{V8,RR} - 4 L_{ijjj}^{V8,RR} + \frac{2}{3} L_{iii}^{V8,LR} \\
& + \frac{2}{3} L_{kkii}^{V8,LR} + \frac{8}{3} L_{iii}^{V,RR} + \frac{8}{3} L_{ikki}^{V,RR} \Big] - \frac{8}{3} L_{ijj}^{V8,RR} e^2 + \alpha_s^2 \Big[ - \frac{44}{3} L_{jjjj}^{V1,LR} \\
& - \frac{22}{3} L_{kkjj}^{V1,LR} + \frac{278}{81} L_{jjjj}^{V8,LR} + \frac{139}{81} L_{kkjj}^{V8,LR} + \frac{10102}{81} L_{jjjj}^{V,RR} - \frac{28}{3} L_{jjkk}^{V,RR} + \frac{5176}{81} L_{jjkk}^{V,RR} \\
& - \frac{22}{3} L_{11ii}^{V1,LR} - \frac{22}{3} L_{22ii}^{V1,LR} - \frac{22}{3} L_{33ii}^{V1,LR} + \frac{157}{81} L_{11ii}^{V8,LR} + \frac{157}{81} L_{22ii}^{V8,LR} + \frac{157}{81} L_{33ii}^{V8,LR}
\end{aligned}$$

$$\begin{aligned}
& -\frac{22}{3}L_{11jj}^{V1,LR} - \frac{22}{3}L_{22jj}^{V1,LR} - \frac{2}{3}L_{11jj}^{V1,RR} - \frac{2}{3}L_{22jj}^{V1,RR} - \frac{2}{3}L_{ii11}^{V1,RR} - \frac{2}{3}L_{ii22}^{V1,RR} \\
& - \frac{2}{3}L_{ii33}^{V1,RR} + \frac{41}{3}L_{iijj}^{V1,RR} + \frac{139}{81}L_{11jj}^{V8,LR} + \frac{139}{81}L_{22jj}^{V8,LR} + \frac{769}{81}L_{11jj}^{V8,RR} + \frac{769}{81}L_{22jj}^{V8,RR} \\
& + \frac{787}{81}L_{ii11}^{V8,RR} + \frac{787}{81}L_{ii22}^{V8,RR} + \frac{787}{81}L_{ii33}^{V8,RR} - \frac{125}{9}L_{iijj}^{V8,RR} - \frac{22}{3}L_{iii}^{V1,LR} - \frac{22}{3}L_{kkii}^{V1,LR} \\
& + \frac{157}{81}L_{iii}^{V8,LR} + \frac{157}{81}L_{kkii}^{V8,LR} + \frac{1918}{27}L_{iii}^{V,RR} - \frac{28}{3}L_{ikk}^{V,RR} + \frac{5248}{81}L_{ikki}^{V,RR} \Big] \\
& + \alpha_s \alpha \Bigg[ -\frac{392}{81}L_{jjjj}^{V1,LR} - \frac{196}{81}L_{kkjj}^{V1,LR} + \frac{104}{27}L_{jjjj}^{V8,LR} + \frac{52}{27}L_{kkjj}^{V8,LR} - \frac{15728}{243}L_{jjjj}^{V,RR} \\
& - \frac{392}{81}L_{jjkk}^{V,RR} - \frac{5096}{243}L_{jjkj}^{V,RR} + \frac{284}{81}L_{11ii}^{V1,LR} + \frac{284}{81}L_{22ii}^{V1,LR} - \frac{496}{81}L_{33ii}^{V1,LR} + \frac{10}{27}L_{11ii}^{V8,LR} \\
& + \frac{10}{27}L_{22ii}^{V8,LR} + \frac{4}{27}L_{33ii}^{V8,LR} - \frac{196}{81}L_{11jj}^{V,LR} - \frac{196}{81}L_{22jj}^{V,LR} - \frac{196}{81}L_{33jj}^{V,LR} - \frac{196}{81}L_{11jj}^{V,RR} \\
& - \frac{196}{81}L_{22jj}^{V,RR} - \frac{196}{81}L_{33jj}^{V,RR} + \frac{284}{81}L_{11ii}^{V,LR} + \frac{284}{81}L_{22ii}^{V,LR} + \frac{284}{81}L_{33ii}^{V,LR} + \frac{284}{81}L_{11ii}^{V,RR} \\
& + \frac{284}{81}L_{22ii}^{V,RR} + \frac{284}{81}L_{33ii}^{V,RR} + \frac{392}{81}L_{11jj}^{V1,LR} + \frac{392}{81}L_{22jj}^{V1,LR} + \frac{392}{81}L_{11jj}^{V1,RR} + \frac{392}{81}L_{22jj}^{V1,RR} \\
& + \frac{284}{81}L_{ii11}^{V1,RR} + \frac{284}{81}L_{ii22}^{V1,RR} + \frac{284}{81}L_{ii33}^{V1,RR} - \frac{4}{3}L_{iijj}^{V1,RR} - \frac{80}{27}L_{11jj}^{V8,LR} - \frac{80}{27}L_{22jj}^{V8,LR} \\
& + \frac{56}{9}L_{11jj}^{V8,RR} + \frac{56}{9}L_{22jj}^{V8,RR} + \frac{14}{9}L_{ii11}^{V8,RR} + \frac{14}{9}L_{ii22}^{V8,RR} + \frac{14}{9}L_{ii33}^{V8,RR} - \frac{47}{9}L_{iijj}^{V8,RR} \\
& - \frac{568}{81}L_{iii}^{V1,LR} - \frac{568}{81}L_{kkii}^{V1,LR} + \frac{4}{27}L_{iii}^{V8,LR} + \frac{4}{27}L_{kkii}^{V8,LR} - \frac{4616}{81}L_{iii}^{V,RR} - \frac{1136}{81}L_{kkii}^{V,RR} \\
& - \frac{6560}{243}L_{ikki}^{V,RR} \Big] - \frac{128}{81}L_{iijj}^{V8,RR}\alpha^2 ;
\end{aligned}$$

$$\begin{aligned}
\dot{L}_{jjii}^{V,RR} &= e^2 \Bigg[ \frac{4}{3}L_{iii}^{V1,LR} + \frac{4}{3}L_{jjii}^{V1,LR} + \frac{4}{3}L_{kkii}^{V1,LR} + \frac{32}{9}L_{iii}^{V,RR} + \frac{8}{3}L_{iijj}^{V,RR} \\
& + \frac{8}{3}L_{ikk}^{V,RR} + \frac{8}{9}L_{ijji}^{V,RR} + \frac{8}{9}L_{ikki}^{V,RR} + \frac{4}{9}L_{11jj}^{V,LR} + \frac{4}{9}L_{22jj}^{V,LR} + \frac{4}{9}L_{33jj}^{V,LR} \\
& + \frac{4}{3}L_{11ii}^{V,LR} + \frac{4}{3}L_{22ii}^{V,LR} + \frac{4}{3}L_{33ii}^{V,LR} + \frac{4}{3}L_{11ii}^{V,RR} + \frac{4}{3}L_{22ii}^{V,RR} + \frac{4}{3}L_{33ii}^{V,RR} \\
& + \frac{4}{9}L_{jj11}^{V,RR} + \frac{4}{9}L_{jj22}^{V,RR} + \frac{4}{9}L_{jj33}^{V,RR} + 4L_{jjii}^{V,RR} + \frac{8}{9}L_{jjjj}^{V,LR} + \frac{4}{9}L_{kkjj}^{V,LR} \Big]
\end{aligned}$$

$$\begin{aligned}
& + \frac{8}{3} L_{jjj}^{V,RR} + \frac{16}{9} L_{jjkk}^{V,RR} - \frac{8}{9} L_{jj11}^{V,RR} - \frac{8}{9} L_{jj22}^{V,RR} - \frac{8}{3} L_{11ii}^{V1,LR} - \frac{8}{3} L_{22ii}^{V1,LR} \\
& - \frac{8}{3} L_{11ii}^{V1,RR} - \frac{8}{3} L_{22ii}^{V1,RR} - \frac{8}{9} L_{11jj}^{V,LR} - \frac{8}{9} L_{22jj}^{V,LR} \Big] + \alpha_s^2 \Big[ - 8 L_{11jj}^{V,LR} \\
& - 8 L_{22jj}^{V,LR} - 8 L_{33jj}^{V,LR} + 8 L_{jj11}^{V,RR} + 8 L_{jj22}^{V,RR} + 8 L_{jj33}^{V,RR} + 8 L_{jj11}^{V,RR} \\
& + 8 L_{jj22}^{V,RR} - 8 L_{11jj}^{V,LR} - 8 L_{22jj}^{V,LR} \Big] + \alpha_s \alpha \Big[ \frac{16}{3} L_{iii}^{V1,LR} + \frac{16}{3} L_{jji}^{V1,LR} \\
& + \frac{16}{3} L_{dd}^{V1,LR} - \frac{1040}{243} L_{iii}^{V8,LR} - \frac{1040}{243} L_{jji}^{V8,LR} - \frac{1040}{243} L_{dd}^{V8,LR} + \frac{1024}{81} L_{iii}^{V,RR} \\
& + 8 L_{ijj}^{V,RR} + 8 L_{ikk}^{V,RR} - \frac{8}{243} L_{ijji}^{V,RR} - \frac{8}{243} L_{ikki}^{V,RR} + \frac{16}{9} L_{11jj}^{V,LR} + \frac{16}{9} L_{22jj}^{V,LR} \\
& + \frac{16}{9} L_{33jj}^{V,LR} + \frac{16}{9} L_{jj11}^{V,RR} + \frac{16}{9} L_{jj22}^{V,RR} + \frac{16}{9} L_{jj33}^{V,RR} - 16 L_{jji}^{V,RR} - \frac{32}{9} L_{jj11}^{V,RR} \\
& - \frac{32}{9} L_{jj22}^{V,RR} - \frac{32}{3} L_{11ii}^{V1,LR} - \frac{32}{3} L_{22ii}^{V1,LR} - \frac{32}{3} L_{11ii}^{V1,RR} - \frac{32}{3} L_{22ii}^{V1,RR} + \frac{1336}{243} L_{11ii}^{V8,LR} \\
& + \frac{1336}{243} L_{22ii}^{V8,LR} - \frac{104}{243} L_{11ii}^{V8,RR} - \frac{104}{243} L_{22ii}^{V8,RR} - \frac{32}{9} L_{11jj}^{V,LR} - \frac{32}{9} L_{22jj}^{V,LR} \Big] \\
& + \alpha^2 \Big[ - \frac{1312}{243} L_{iii}^{V1,LR} - \frac{1312}{243} L_{jji}^{V1,LR} - \frac{1312}{243} L_{kkii}^{V1,LR} + \frac{4816}{243} L_{iii}^{V,RR} + \frac{1984}{243} L_{ijj}^{V,RR} \\
& + \frac{1984}{243} L_{dd}^{V,RR} + \frac{2896}{729} L_{ijji}^{V,RR} + \frac{2896}{729} L_{ikki}^{V,RR} - \frac{200}{243} L_{11jj}^{V,LR} - \frac{200}{243} L_{22jj}^{V,LR} \\
& - \frac{200}{243} L_{33jj}^{V,LR} - \frac{3184}{243} L_{11ii}^{V,LR} - \frac{3184}{243} L_{22ii}^{V,LR} - \frac{3184}{243} L_{33ii}^{V,LR} + \frac{3728}{243} L_{11ii}^{V,RR} \\
& + \frac{3728}{243} L_{22ii}^{V,RR} + \frac{3728}{243} L_{33ii}^{V,RR} - \frac{104}{243} L_{jj11}^{V,RR} - \frac{104}{243} L_{jj22}^{V,RR} - \frac{104}{243} L_{jj33}^{V,RR} \\
& - \frac{326}{27} L_{jji}^{V,RR} - \frac{1040}{81} L_{jjj}^{V,LR} - \frac{520}{81} L_{kkjj}^{V,LR} + \frac{16}{9} L_{jjj}^{V,RR} + \frac{224}{81} L_{jjkk}^{V,RR} - \frac{1016}{243} L_{jj11}^{V,RR} \\
& - \frac{1016}{243} L_{jj22}^{V,RR} - \frac{6232}{243} L_{11ii}^{V1,LR} - \frac{6232}{243} L_{22ii}^{V1,LR} + \frac{2984}{243} L_{11ii}^{V1,RR} + \frac{2984}{243} L_{22ii}^{V1,RR} \\
& - \frac{1400}{243} L_{11jj}^{V,LR} - \frac{1400}{243} L_{22jj}^{V,LR} \Big] ;
\end{aligned}$$

$$\dot{L}_{jji}^{V,RR} = e^2 \Big[ - \frac{8}{9} L_{11jj}^{V,LR} - \frac{8}{9} L_{22jj}^{V,LR} - \frac{8}{9} L_{33jj}^{V,LR} + \frac{4}{3} L_{11ii}^{V1,LR} + \frac{4}{3} L_{22ii}^{V1,LR}$$

$$\begin{aligned}
& + \frac{4}{3}L_{33ii}^{V1,LR} - \frac{8}{9}L_{jj11}^{V,RR} - \frac{8}{9}L_{jj22}^{V,RR} - \frac{8}{9}L_{jj33}^{V,RR} - \frac{16}{9}L_{jjjj}^{V,LR} - \frac{8}{9}L_{kkjj}^{V,LR} \\
& - \frac{16}{3}L_{jjjj}^{V,RR} - \frac{32}{9}L_{jjkk}^{V,RR} + \frac{4}{3}L_{11ii}^{V,LR} + \frac{4}{3}L_{22ii}^{V,LR} + \frac{4}{3}L_{33ii}^{V,LR} + \frac{4}{3}L_{11ii}^{V,RR} \\
& + \frac{4}{3}L_{22ii}^{V,RR} + \frac{4}{3}L_{33ii}^{V,RR} + \frac{16}{9}L_{jj11}^{V,RR} + \frac{16}{9}L_{jj22}^{V,RR} - 8L_{jjii}^{V,RR} + \frac{4}{3}L_{ii11}^{V1,RR} \\
& + \frac{4}{3}L_{ii22}^{V1,RR} + \frac{4}{3}L_{ii33}^{V1,RR} + \frac{16}{9}L_{11jj}^{V,LR} + \frac{16}{9}L_{22jj}^{V,LR} - \frac{8}{3}L_{iii}^{V1,LR} - \frac{8}{3}L_{kkii}^{V1,LR} \\
& - \frac{64}{9}L_{iii}^{V,RR} - \frac{16}{3}L_{ikk}^{V,RR} - \frac{16}{9}L_{ikki}^{V,RR} \Big] + \alpha_s^2 \Big[ -8L_{11jj}^{V,LR} - 8L_{22jj}^{V,LR} \\
& - 8L_{33jj}^{V,LR} + 8L_{jj11}^{V,RR} + 8L_{jj22}^{V,RR} + 8L_{jj33}^{V,RR} + 8L_{jj11}^{V,RR} + 8L_{jj22}^{V,RR} \\
& - 8L_{11jj}^{V,LR} - 8L_{22jj}^{V,LR} \Big] + \alpha_s \alpha \Big[ -\frac{32}{9}L_{11jj}^{V,LR} - \frac{32}{9}L_{22jj}^{V,LR} - \frac{32}{9}L_{33jj}^{V,LR} \\
& + \frac{16}{3}L_{11ii}^{V1,LR} + \frac{16}{3}L_{22ii}^{V1,LR} - \frac{32}{3}L_{33ii}^{V1,LR} - \frac{332}{243}L_{11ii}^{V8,LR} - \frac{332}{243}L_{22ii}^{V8,LR} + \frac{2044}{243}L_{33ii}^{V8,LR} \\
& - \frac{32}{9}L_{jj11}^{V,RR} - \frac{32}{9}L_{jj22}^{V,RR} - \frac{32}{9}L_{jj33}^{V,RR} + \frac{64}{9}L_{jj11}^{V,RR} + \frac{64}{9}L_{jj22}^{V,RR} + 32L_{jjii}^{V,RR} \\
& + \frac{16}{3}L_{ii11}^{V1,RR} + \frac{16}{3}L_{ii22}^{V1,RR} + \frac{16}{3}L_{ii33}^{V1,RR} + \frac{388}{243}L_{ii11}^{V8,RR} + \frac{388}{243}L_{ii22}^{V8,RR} + \frac{388}{243}L_{ii33}^{V8,RR} \\
& + \frac{64}{9}L_{11jj}^{V,LR} + \frac{64}{9}L_{22jj}^{V,LR} - \frac{32}{3}L_{iii}^{V1,LR} - \frac{32}{3}L_{kkii}^{V1,LR} + \frac{2044}{243}L_{iii}^{V8,LR} + \frac{2044}{243}L_{kkii}^{V8,LR} \\
& - \frac{2096}{81}L_{iii}^{V,RR} - 16L_{ikk}^{V,RR} - \frac{128}{243}L_{ikki}^{V,RR} \Big] + \alpha^2 \Big[ \frac{1408}{243}L_{11jj}^{V,LR} + \frac{1408}{243}L_{22jj}^{V,LR} \\
& + \frac{1408}{243}L_{33jj}^{V,LR} - \frac{928}{243}L_{11ii}^{V1,LR} - \frac{928}{243}L_{22ii}^{V1,LR} + \frac{416}{243}L_{33ii}^{V1,LR} + \frac{2512}{243}L_{jj11}^{V,RR} \\
& + \frac{2512}{243}L_{jj22}^{V,RR} + \frac{2512}{243}L_{jj33}^{V,RR} + \frac{928}{81}L_{jjjj}^{V,LR} + \frac{464}{81}L_{kkjj}^{V,LR} + \frac{544}{9}L_{jjjj}^{V,RR} + \frac{2432}{81}L_{jjkk}^{V,RR} \\
& - \frac{424}{243}L_{11ii}^{V,LR} - \frac{424}{243}L_{22ii}^{V,LR} - \frac{424}{243}L_{33ii}^{V,LR} + \frac{3248}{243}L_{11ii}^{V,RR} + \frac{3248}{243}L_{22ii}^{V,RR} \\
& + \frac{3248}{243}L_{33ii}^{V,RR} + \frac{1312}{243}L_{jj11}^{V,RR} + \frac{1312}{243}L_{jj22}^{V,RR} + \frac{112}{27}L_{jjii}^{V,RR} + \frac{296}{243}L_{ii11}^{V1,RR} \\
& + \frac{296}{243}L_{ii22}^{V1,RR} + \frac{296}{243}L_{ii33}^{V1,RR} - \frac{3104}{243}L_{11jj}^{V,LR} - \frac{3104}{243}L_{22jj}^{V,LR} + \frac{128}{243}L_{iii}^{V1,LR}
\end{aligned}$$



$$\begin{aligned}
& + \frac{128}{243} L_{\overline{kk}ii}^{V1,LR} + \frac{26272}{243} L_{\overline{iii}}^{V,RR} + \frac{10048}{243} L_{\overline{ikk}}^{V,RR} + \frac{18304}{729} L_{\overline{ikki}}^{V,RR} \Bigg] ; \\
\dot{L}_{\overline{jj}i}^{V1,RR} &= \frac{8}{3} L_{\overline{jj}i}^{V8,RR} g_s^2 + e^2 \Bigg[ -\frac{8}{9} L_{\overline{dd}iii}^{V1,LR} - \frac{8}{9} L_{\overline{jj}i}^{V1,LR} - \frac{8}{9} L_{\overline{kki}}^{V1,LR} - \frac{64}{27} L_{\overline{iii}}^{V,RR} \\
& - \frac{16}{9} L_{\overline{ijj}}^{V,RR} - \frac{16}{9} L_{\overline{ikk}}^{V,RR} - \frac{16}{27} L_{\overline{ijj}}^{V,RR} - \frac{16}{27} L_{\overline{ikki}}^{V,RR} + \frac{4}{9} L_{\overline{11jj}}^{V1,LR} + \frac{4}{9} L_{\overline{22jj}}^{V1,LR} \\
& + \frac{4}{9} L_{\overline{33jj}}^{V1,LR} - \frac{8}{9} L_{\overline{11ii}}^{V,LR} - \frac{8}{9} L_{\overline{22ii}}^{V,LR} - \frac{8}{9} L_{\overline{33ii}}^{V,LR} - \frac{8}{9} L_{\overline{11ii}}^{V,RR} - \frac{8}{9} L_{\overline{22ii}}^{V,RR} \\
& - \frac{8}{9} L_{\overline{33ii}}^{V,RR} + \frac{4}{9} L_{\overline{11jj}}^{V,LR} + \frac{4}{9} L_{\overline{22jj}}^{V,LR} + \frac{4}{9} L_{\overline{33jj}}^{V,LR} + \frac{4}{9} L_{\overline{11jj}}^{V,RR} + \frac{4}{9} L_{\overline{22jj}}^{V,RR} \\
& + \frac{4}{9} L_{\overline{33jj}}^{V,RR} + \frac{16}{9} L_{\overline{11ii}}^{V1,LR} + \frac{16}{9} L_{\overline{22ii}}^{V1,LR} + \frac{16}{9} L_{\overline{33ii}}^{V1,LR} + \frac{16}{9} L_{\overline{11ii}}^{V1,RR} + \frac{16}{9} L_{\overline{22ii}}^{V1,RR} + \frac{4}{9} L_{\overline{33ii}}^{V1,RR} \\
& + \frac{4}{9} L_{\overline{jj22}}^{V1,RR} + \frac{4}{9} L_{\overline{jj33}}^{V1,RR} - \frac{8}{3} L_{\overline{jjii}}^{V1,RR} - \frac{8}{9} L_{\overline{jjjj}}^{V1,LR} - \frac{8}{9} L_{\overline{kkjj}}^{V1,LR} - \frac{64}{27} L_{\overline{jjjj}}^{V,RR} \\
& - \frac{16}{9} L_{\overline{jjkk}}^{V,RR} - \frac{16}{27} L_{\overline{jjkk}}^{V,RR} \Bigg] + \alpha_s^2 \Bigg[ -8 L_{\overline{dd}iii}^{V1,LR} - 8 L_{\overline{jj}i}^{V1,LR} - 8 L_{\overline{kki}}^{V1,LR} \\
& + \frac{4}{27} L_{\overline{iii}}^{V8,LR} + \frac{4}{27} L_{\overline{jj}i}^{V8,LR} + \frac{4}{27} L_{\overline{kki}}^{V8,LR} + \frac{328}{9} L_{\overline{iii}}^{V,RR} + 16 L_{\overline{ijj}}^{V,RR} + 16 L_{\overline{ikk}}^{V,RR} \\
& + \frac{256}{27} L_{\overline{ijji}}^{V,RR} + \frac{256}{27} L_{\overline{ikki}}^{V,RR} - 8 L_{\overline{11jj}}^{V1,LR} - 8 L_{\overline{22jj}}^{V1,LR} - 8 L_{\overline{33jj}}^{V1,LR} + \frac{4}{27} L_{\overline{11jj}}^{V8,LR} \\
& + \frac{4}{27} L_{\overline{22jj}}^{V8,LR} + \frac{4}{27} L_{\overline{33jj}}^{V8,LR} - 8 L_{\overline{11ii}}^{V1,LR} - 8 L_{\overline{22ii}}^{V1,LR} + 8 L_{\overline{11ii}}^{V1,RR} + 8 L_{\overline{22ii}}^{V1,RR} \\
& + 8 L_{\overline{33ii}}^{V1,RR} + 8 L_{\overline{jj11}}^{V1,RR} + 8 L_{\overline{jj22}}^{V1,RR} + 8 L_{\overline{jj33}}^{V1,RR} - \frac{28}{3} L_{\overline{jjii}}^{V1,RR} + \frac{4}{27} L_{\overline{11ii}}^{V8,LR} + \frac{4}{27} L_{\overline{22ii}}^{V8,LR} \\
& + \frac{4}{27} L_{\overline{33ii}}^{V8,RR} + \frac{4}{27} L_{\overline{11ii}}^{V8,RR} + \frac{4}{27} L_{\overline{22ii}}^{V8,RR} + \frac{4}{27} L_{\overline{33ii}}^{V8,RR} + \frac{82}{27} L_{\overline{jjii}}^{V8,RR} \\
& - 8 L_{\overline{jjjj}}^{V1,LR} - 8 L_{\overline{kkjj}}^{V1,LR} + \frac{4}{27} L_{\overline{jjjj}}^{V8,LR} + \frac{4}{27} L_{\overline{kkjj}}^{V8,LR} + \frac{328}{9} L_{\overline{jjjj}}^{V,RR} + 16 L_{\overline{jjkk}}^{V,RR} \\
& + \frac{256}{27} L_{\overline{jjkk}}^{V,RR} \Bigg] + \alpha_s \alpha \Bigg[ -\frac{32}{9} L_{\overline{dd}iii}^{V1,LR} - \frac{32}{9} L_{\overline{jj}i}^{V1,LR} - \frac{32}{9} L_{\overline{kki}}^{V1,LR} + \frac{2080}{729} L_{\overline{iii}}^{V8,LR} \\
& + \frac{2080}{729} L_{\overline{jj}i}^{V8,LR} + \frac{2080}{729} L_{\overline{kki}}^{V8,LR} - \frac{2048}{243} L_{\overline{iii}}^{V,RR} - \frac{16}{3} L_{\overline{ijj}}^{V,RR} - \frac{16}{3} L_{\overline{ikk}}^{V,RR} + \frac{16}{729} L_{\overline{ijji}}^{V,RR} \\
& + \frac{16}{729} L_{\overline{ikk}i}^{V,RR} + \frac{16}{9} L_{\overline{11jj}}^{V1,LR} + \frac{16}{9} L_{\overline{22jj}}^{V1,LR} - \frac{32}{9} L_{\overline{33jj}}^{V1,LR} - \frac{332}{729} L_{\overline{11jj}}^{V8,LR} - \frac{332}{729} L_{\overline{22jj}}^{V8,LR}
\end{aligned}$$

$$\begin{aligned}
& + \frac{2044}{729} L_{33jj}^{V8,LR} + \frac{64}{9} L_{11ii}^{V1,LR} + \frac{64}{9} L_{22ii}^{V1,LR} + \frac{64}{9} L_{11ii}^{V1,RR} + \frac{64}{9} L_{22ii}^{V1,RR} + \frac{16}{9} L_{jj11}^{V1,RR} \\
& + \frac{16}{9} L_{jj22}^{V1,RR} + \frac{16}{9} L_{jj33}^{V1,RR} + \frac{64}{3} L_{jjii}^{V1,RR} - \frac{2672}{729} L_{11ii}^{V8,LR} - \frac{2672}{729} L_{22ii}^{V8,LR} + \frac{208}{729} L_{11ii}^{V8,RR} \\
& + \frac{208}{729} L_{22ii}^{V8,RR} + \frac{388}{729} L_{jj11}^{V8,RR} + \frac{388}{729} L_{jj22}^{V8,RR} + \frac{388}{729} L_{jj33}^{V8,RR} - \frac{8}{27} L_{jjii}^{V8,RR} \\
& - \frac{32}{9} L_{jjjj}^{V1,LR} - \frac{32}{9} L_{kkjj}^{V1,LR} + \frac{2044}{729} L_{jjjj}^{V8,LR} + \frac{2044}{729} L_{kkjj}^{V8,LR} - \frac{2096}{243} L_{jjjj}^{V,RR} \\
& - \frac{16}{3} L_{jjkk}^{V,RR} - \frac{128}{729} L_{jjkk}^{V,RR} \Big] + \alpha^2 \Big[ - \frac{256}{729} L_{iiii}^{V1,LR} - \frac{256}{729} L_{jjii}^{V1,LR} - \frac{256}{729} L_{kkii}^{V1,LR} \\
& + \frac{8368}{729} L_{iiii}^{V,RR} + \frac{3232}{729} L_{iijj}^{V,RR} + \frac{3232}{729} L_{ddkk}^{V,RR} + \frac{5728}{2187} L_{ijji}^{V,RR} + \frac{5728}{2187} L_{ddki}^{V,RR} \\
& - \frac{136}{729} L_{11jj}^{V1,LR} - \frac{136}{729} L_{22jj}^{V1,LR} + \frac{2720}{729} L_{33jj}^{V1,LR} - \frac{2992}{729} L_{11ii}^{V,LR} - \frac{2992}{729} L_{22ii}^{V,LR} \\
& - \frac{2992}{729} L_{33ii}^{V,LR} + \frac{2624}{729} L_{11ii}^{V,RR} + \frac{2624}{729} L_{22ii}^{V,RR} + \frac{2624}{729} L_{33ii}^{V,RR} + \frac{1664}{729} L_{11jj}^{V,LR} \\
& + \frac{1664}{729} L_{22jj}^{V,LR} + \frac{1664}{729} L_{33jj}^{V,LR} + \frac{1448}{729} L_{11jj}^{V,RR} + \frac{1448}{729} L_{22jj}^{V,RR} + \frac{1448}{729} L_{33jj}^{V,RR} \\
& - \frac{1216}{729} L_{11ii}^{V1,LR} - \frac{1216}{729} L_{22ii}^{V1,LR} + \frac{6272}{729} L_{11ii}^{V1,RR} + \frac{6272}{729} L_{22ii}^{V1,RR} - \frac{208}{729} L_{jj11}^{V1,RR} \\
& - \frac{208}{729} L_{jj22}^{V1,RR} - \frac{208}{729} L_{jj33}^{V1,RR} - \frac{128}{81} L_{jjii}^{V1,RR} + \frac{2432}{729} L_{jjjj}^{V1,LR} + \frac{2432}{729} L_{kkjj}^{V1,LR} \\
& + \frac{11872}{729} L_{jjjj}^{V,RR} + \frac{4288}{729} L_{jjkk}^{V,RR} + \frac{9088}{2187} L_{jjkk}^{V,RR} \Big] ;
\end{aligned}$$

$$\begin{aligned}
\dot{L}_{jjii}^{V8,RR} & = g_s^2 \Big[ \frac{2}{3} L_{iiii}^{V8,LR} + \frac{2}{3} L_{jjii}^{V8,LR} + \frac{2}{3} L_{kkii}^{V8,LR} + \frac{8}{3} L_{iiii}^{V,RR} + \frac{8}{3} L_{ijji}^{V,RR} \\
& + \frac{8}{3} L_{ddki}^{V,RR} + \frac{2}{3} L_{11jj}^{V8,LR} + \frac{2}{3} L_{22jj}^{V8,LR} + \frac{2}{3} L_{33jj}^{V8,LR} + 12 L_{jjii}^{V1,RR} + \frac{2}{3} L_{11ii}^{V8,LR} \\
& + \frac{2}{3} L_{22ii}^{V8,LR} + \frac{2}{3} L_{11ii}^{V8,RR} + \frac{2}{3} L_{22ii}^{V8,RR} + \frac{2}{3} L_{jj11}^{V8,RR} + \frac{2}{3} L_{jj22}^{V8,RR} + \frac{2}{3} L_{jj33}^{V8,RR} \\
& - 4 L_{jjii}^{V8,RR} + \frac{2}{3} L_{jjjj}^{V8,LR} + \frac{2}{3} L_{kkjj}^{V8,LR} + \frac{8}{3} L_{jjjj}^{V,RR} + \frac{8}{3} L_{jjkk}^{V,RR} \Big] - \frac{8}{3} L_{jjii}^{V8,RR} \\
& e^2 + \alpha_s^2 \Big[ - \frac{22}{3} L_{iiii}^{V1,LR} - \frac{22}{3} L_{jjii}^{V1,LR} - \frac{22}{3} L_{kkii}^{V1,LR} + \frac{139}{81} L_{iiii}^{V8,LR} + \frac{139}{81} L_{jjii}^{V8,LR}
\end{aligned}$$

$$\begin{aligned}
& + \frac{139}{81} L_{\ddot{k}k\ddot{i}i}^{V8,LR} + \frac{1894}{27} L_{\ddot{u}i\ddot{i}i}^{V,RR} - \frac{28}{3} L_{\ddot{i}i\ddot{j}j}^{V,RR} - \frac{28}{3} L_{\ddot{i}i\ddot{k}k}^{V,RR} + \frac{5176}{81} L_{\ddot{i}j\ddot{j}i}^{V,RR} + \frac{5176}{81} L_{\ddot{i}k\ddot{k}i}^{V,RR} \\
& - \frac{22}{3} L_{\ddot{u}i\ddot{j}j}^{V1,LR} - \frac{22}{3} L_{\ddot{u}i\ddot{j}j}^{V1,LR} - \frac{22}{3} L_{\ddot{u}i\ddot{j}j}^{V1,LR} + \frac{157}{81} L_{\ddot{u}i\ddot{j}j}^{V8,LR} + \frac{157}{81} L_{\ddot{u}i\ddot{j}j}^{V8,LR} + \frac{157}{81} L_{\ddot{u}i\ddot{j}j}^{V8,LR} \\
& - \frac{22}{3} L_{\ddot{u}i\ddot{j}j}^{V1,LR} - \frac{22}{3} L_{\ddot{u}i\ddot{j}j}^{V1,LR} - \frac{2}{3} L_{\ddot{u}i\ddot{j}j}^{V1,RR} - \frac{2}{3} L_{\ddot{u}i\ddot{j}j}^{V1,RR} - \frac{2}{3} L_{\ddot{u}i\ddot{j}j}^{V1,RR} - \frac{2}{3} L_{\ddot{u}i\ddot{j}j}^{V1,RR} \\
& - \frac{2}{3} L_{\ddot{u}i\ddot{j}j}^{V1,RR} + \frac{41}{3} L_{\ddot{u}i\ddot{j}j}^{V1,RR} + \frac{139}{81} L_{\ddot{u}i\ddot{j}j}^{V8,LR} + \frac{139}{81} L_{\ddot{u}i\ddot{j}j}^{V8,LR} + \frac{769}{81} L_{\ddot{u}i\ddot{j}j}^{V8,RR} + \frac{769}{81} L_{\ddot{u}i\ddot{j}j}^{V8,RR} \\
& + \frac{787}{81} L_{\ddot{u}i\ddot{j}j}^{V8,RR} + \frac{787}{81} L_{\ddot{u}i\ddot{j}j}^{V8,RR} + \frac{787}{81} L_{\ddot{u}i\ddot{j}j}^{V8,RR} - \frac{125}{9} L_{\ddot{u}i\ddot{j}j}^{V8,RR} - \frac{22}{3} L_{\ddot{u}i\ddot{j}j}^{V1,LR} - \frac{22}{3} L_{\ddot{u}i\ddot{j}j}^{V1,LR} \\
& + \frac{157}{81} L_{\ddot{u}i\ddot{j}j}^{V8,LR} + \frac{157}{81} L_{\ddot{u}i\ddot{j}j}^{V8,LR} + \frac{1918}{27} L_{\ddot{u}i\ddot{j}j}^{V,RR} - \frac{28}{3} L_{\ddot{u}i\ddot{j}j}^{V,RR} + \frac{5248}{81} L_{\ddot{u}i\ddot{j}j}^{V,RR} \Big] \\
& + \alpha_s \alpha \Bigg[ - \frac{196}{81} L_{\ddot{u}i\ddot{i}i}^{V1,LR} - \frac{196}{81} L_{\ddot{u}i\ddot{j}j}^{V1,LR} - \frac{196}{81} L_{\ddot{u}i\ddot{k}k}^{V1,LR} + \frac{52}{27} L_{\ddot{u}i\ddot{i}i}^{V8,LR} + \frac{52}{27} L_{\ddot{u}i\ddot{j}j}^{V8,LR} \\
& + \frac{52}{27} L_{\ddot{u}i\ddot{k}k}^{V8,LR} - \frac{3152}{81} L_{\ddot{u}i\ddot{i}i}^{V,RR} - \frac{392}{81} L_{\ddot{u}i\ddot{j}j}^{V,RR} - \frac{392}{81} L_{\ddot{u}i\ddot{k}k}^{V,RR} - \frac{5096}{243} L_{\ddot{u}i\ddot{j}j}^{V,RR} - \frac{5096}{243} L_{\ddot{u}i\ddot{k}k}^{V,RR} \\
& + \frac{284}{81} L_{\ddot{u}i\ddot{j}j}^{V1,LR} + \frac{284}{81} L_{\ddot{u}i\ddot{j}j}^{V1,LR} - \frac{496}{81} L_{\ddot{u}i\ddot{j}j}^{V1,LR} + \frac{10}{27} L_{\ddot{u}i\ddot{j}j}^{V8,LR} + \frac{10}{27} L_{\ddot{u}i\ddot{j}j}^{V8,LR} + \frac{4}{27} L_{\ddot{u}i\ddot{j}j}^{V8,LR} \\
& - \frac{196}{81} L_{\ddot{u}i\ddot{j}j}^{V,LR} - \frac{196}{81} L_{\ddot{u}i\ddot{j}j}^{V,LR} - \frac{196}{81} L_{\ddot{u}i\ddot{j}j}^{V,LR} - \frac{196}{81} L_{\ddot{u}i\ddot{j}j}^{V,RR} - \frac{196}{81} L_{\ddot{u}i\ddot{j}j}^{V,RR} - \frac{196}{81} L_{\ddot{u}i\ddot{j}j}^{V,RR} \\
& + \frac{284}{81} L_{\ddot{u}i\ddot{j}j}^{V,LR} + \frac{284}{81} L_{\ddot{u}i\ddot{j}j}^{V,LR} + \frac{284}{81} L_{\ddot{u}i\ddot{j}j}^{V,LR} + \frac{284}{81} L_{\ddot{u}i\ddot{j}j}^{V,RR} + \frac{284}{81} L_{\ddot{u}i\ddot{j}j}^{V,RR} + \frac{284}{81} L_{\ddot{u}i\ddot{j}j}^{V,RR} \\
& + \frac{392}{81} L_{\ddot{u}i\ddot{j}j}^{V1,LR} + \frac{392}{81} L_{\ddot{u}i\ddot{j}j}^{V1,LR} + \frac{392}{81} L_{\ddot{u}i\ddot{j}j}^{V1,RR} + \frac{392}{81} L_{\ddot{u}i\ddot{j}j}^{V1,RR} + \frac{284}{81} L_{\ddot{u}i\ddot{j}j}^{V1,RR} + \frac{284}{81} L_{\ddot{u}i\ddot{j}j}^{V1,RR} \\
& + \frac{284}{81} L_{\ddot{u}i\ddot{j}j}^{V1,RR} - \frac{4}{3} L_{\ddot{u}i\ddot{j}j}^{V1,RR} - \frac{80}{27} L_{\ddot{u}i\ddot{j}j}^{V8,LR} - \frac{80}{27} L_{\ddot{u}i\ddot{j}j}^{V8,LR} + \frac{56}{9} L_{\ddot{u}i\ddot{j}j}^{V8,RR} + \frac{56}{9} L_{\ddot{u}i\ddot{j}j}^{V8,RR} \\
& + \frac{14}{9} L_{\ddot{u}i\ddot{j}j}^{V8,RR} + \frac{14}{9} L_{\ddot{u}i\ddot{j}j}^{V8,RR} + \frac{14}{9} L_{\ddot{u}i\ddot{j}j}^{V8,RR} - \frac{47}{9} L_{\ddot{u}i\ddot{j}j}^{V8,RR} - \frac{568}{81} L_{\ddot{u}i\ddot{j}j}^{V1,LR} - \frac{568}{81} L_{\ddot{u}i\ddot{j}j}^{V1,LR} \\
& + \frac{4}{27} L_{\ddot{u}i\ddot{j}j}^{V8,LR} + \frac{4}{27} L_{\ddot{u}i\ddot{j}j}^{V8,LR} - \frac{4616}{81} L_{\ddot{u}i\ddot{j}j}^{V,RR} - \frac{1136}{81} L_{\ddot{u}i\ddot{j}j}^{V,RR} - \frac{6560}{243} L_{\ddot{u}i\ddot{j}j}^{V,RR} \Big] \\
& - \frac{128}{81} L_{\ddot{u}i\ddot{j}j}^{V8,RR} \alpha^2 ;
\end{aligned}$$

$$\dot{L}_{\ddot{u}i\ddot{j}j}^{V,RR} = g_s^2 \Bigg[ - \frac{1}{18} L_{\ddot{u}i\ddot{i}i}^{V8,LR} - \frac{1}{18} L_{\ddot{u}i\ddot{j}j}^{V8,LR} - \frac{1}{9} L_{\ddot{u}i\ddot{j}j}^{V8,LR} - \frac{1}{18} L_{\ddot{u}i\ddot{k}k}^{V8,LR} - \frac{1}{18} L_{\ddot{u}i\ddot{k}k}^{V8,LR}$$

$$\begin{aligned}
& -\frac{2}{9}L_{\overline{ii}ii}^{V,RR} - 2L_{\overline{ij}jj}^{V,RR} + \frac{52}{9}L_{\overline{ij}ji}^{V,RR} - \frac{2}{9}L_{\overline{ik}ki}^{V,RR} - \frac{4}{9}L_{\overline{jj}jj}^{V,RR} - \frac{2}{9}L_{\overline{jk}kj}^{V,RR} \\
& -\frac{1}{18}L_{\overline{ud}11\overline{ii}}^{V8,LR} - \frac{1}{18}L_{\overline{ud}11\overline{jj}}^{V8,LR} - \frac{1}{18}L_{\overline{ud}22\overline{ii}}^{V8,LR} - \frac{1}{18}L_{\overline{ud}22\overline{jj}}^{V8,LR} - \frac{1}{18}L_{\overline{ud}11\overline{ii}}^{V8,RR} - \frac{1}{18}L_{\overline{ud}11\overline{jj}}^{V8,RR} \\
& -\frac{1}{18}L_{\overline{ud}22\overline{ii}}^{V8,RR} - \frac{1}{18}L_{\overline{ud}22\overline{jj}}^{V8,RR} \Big] + e^2 \Big[ \frac{2}{9}L_{\overline{dd}iii}^{V1,LR} + \frac{2}{9}L_{\overline{dd}jj\overline{ii}}^{V1,LR} + \frac{4}{9}L_{\overline{jj}jj}^{V1,LR} \\
& + \frac{2}{9}L_{\overline{dd}kk\overline{ii}}^{V1,LR} + \frac{2}{9}L_{\overline{dd}kk\overline{jj}}^{V1,LR} + \frac{16}{27}L_{\overline{dd}iii}^{V,RR} + \frac{16}{9}L_{\overline{dd}ij\overline{jj}}^{V,RR} + \frac{4}{9}L_{\overline{dd}ikk}^{V,RR} + \frac{4}{27}L_{\overline{dd}ij\overline{ji}}^{V,RR} \\
& + \frac{4}{27}L_{\overline{dd}ik\overline{ki}}^{V,RR} + \frac{32}{27}L_{\overline{dd}jj\overline{jj}}^{V,RR} + \frac{4}{9}L_{\overline{dd}jj\overline{kk}}^{V,RR} + \frac{4}{27}L_{\overline{dd}jj\overline{kk}}^{V,RR} + \frac{2}{9}L_{\overline{ed}11\overline{ii}}^{V,LR} + \frac{2}{9}L_{\overline{ed}11\overline{jj}}^{V,LR} \\
& + \frac{2}{9}L_{\overline{ed}22\overline{ii}}^{V,LR} + \frac{2}{9}L_{\overline{ed}22\overline{jj}}^{V,LR} + \frac{2}{9}L_{\overline{ed}33\overline{ii}}^{V,LR} + \frac{2}{9}L_{\overline{ed}33\overline{jj}}^{V,LR} + \frac{2}{9}L_{\overline{ed}11\overline{ii}}^{V,RR} + \frac{2}{9}L_{\overline{ed}11\overline{jj}}^{V,RR} \\
& + \frac{2}{9}L_{\overline{ed}22\overline{ii}}^{V,RR} + \frac{2}{9}L_{\overline{ed}22\overline{jj}}^{V,RR} + \frac{2}{9}L_{\overline{ed}33\overline{ii}}^{V,RR} + \frac{2}{9}L_{\overline{ed}33\overline{jj}}^{V,RR} - \frac{4}{9}L_{\overline{ud}11\overline{ii}}^{V1,LR} - \frac{4}{9}L_{\overline{ud}11\overline{jj}}^{V1,LR} \\
& - \frac{4}{9}L_{\overline{ud}22\overline{ii}}^{V1,LR} - \frac{4}{9}L_{\overline{ud}22\overline{jj}}^{V1,LR} - \frac{4}{9}L_{\overline{ud}11\overline{ii}}^{V1,RR} - \frac{4}{9}L_{\overline{ud}11\overline{jj}}^{V1,RR} - \frac{4}{9}L_{\overline{ud}22\overline{ii}}^{V1,RR} - \frac{4}{9}L_{\overline{ud}22\overline{jj}}^{V1,RR} \Big] \\
& + \alpha_s^2 \Big[ -\frac{61}{18}L_{\overline{dd}iii}^{V1,LR} - \frac{61}{18}L_{\overline{dd}jj\overline{ii}}^{V1,LR} - \frac{61}{9}L_{\overline{dd}jj\overline{jj}}^{V1,LR} - \frac{61}{18}L_{\overline{dd}kk\overline{ii}}^{V1,LR} - \frac{61}{18}L_{\overline{dd}kk\overline{jj}}^{V1,LR} \\
& - \frac{67}{972}L_{\overline{dd}iii}^{V8,LR} - \frac{67}{972}L_{\overline{dd}jj\overline{ii}}^{V8,LR} - \frac{67}{486}L_{\overline{dd}jj\overline{jj}}^{V8,LR} - \frac{67}{972}L_{\overline{dd}kk\overline{ii}}^{V8,LR} - \frac{67}{972}L_{\overline{dd}kk\overline{jj}}^{V8,LR} + \frac{2005}{162}L_{\overline{dd}iii}^{V,RR} \\
& - \frac{17}{6}L_{\overline{dd}ij\overline{jj}}^{V,RR} + \frac{79}{9}L_{\overline{dd}ik\overline{kk}}^{V,RR} + \frac{3037}{486}L_{\overline{dd}ij\overline{ji}}^{V,RR} - \frac{142}{243}L_{\overline{dd}ik\overline{ki}}^{V,RR} + \frac{9997}{486}L_{\overline{dd}jj\overline{jj}}^{V,RR} + \frac{79}{9}L_{\overline{dd}jj\overline{kk}}^{V,RR} \\
& - \frac{142}{243}L_{\overline{dd}jk\overline{kj}}^{V,RR} - \frac{61}{18}L_{\overline{ud}11\overline{ii}}^{V1,LR} - \frac{61}{18}L_{\overline{ud}11\overline{jj}}^{V1,LR} - \frac{61}{18}L_{\overline{ud}22\overline{ii}}^{V1,LR} - \frac{61}{18}L_{\overline{ud}22\overline{jj}}^{V1,LR} + \frac{73}{18}L_{\overline{ud}11\overline{ii}}^{V1,RR} \\
& + \frac{73}{18}L_{\overline{ud}11\overline{jj}}^{V1,RR} + \frac{73}{18}L_{\overline{ud}22\overline{ii}}^{V1,RR} + \frac{73}{18}L_{\overline{ud}22\overline{jj}}^{V1,RR} - \frac{67}{972}L_{\overline{ud}11\overline{ii}}^{V8,LR} - \frac{67}{972}L_{\overline{ud}11\overline{jj}}^{V8,LR} - \frac{67}{972}L_{\overline{ud}22\overline{ii}}^{V8,LR} \\
& - \frac{67}{972}L_{\overline{ud}22\overline{jj}}^{V8,LR} - \frac{697}{972}L_{\overline{ud}11\overline{ii}}^{V8,RR} - \frac{697}{972}L_{\overline{ud}11\overline{jj}}^{V8,RR} - \frac{697}{972}L_{\overline{ud}22\overline{ii}}^{V8,RR} - \frac{697}{972}L_{\overline{ud}22\overline{jj}}^{V8,RR} \Big] \\
& + \alpha_s \alpha \Big[ \frac{238}{243}L_{\overline{dd}iii}^{V1,LR} + \frac{238}{243}L_{\overline{dd}jj\overline{ii}}^{V1,LR} + \frac{476}{243}L_{\overline{dd}jj\overline{jj}}^{V1,LR} + \frac{238}{243}L_{\overline{dd}kk\overline{ii}}^{V1,LR} + \frac{238}{243}L_{\overline{dd}kk\overline{jj}}^{V1,LR} \\
& - \frac{815}{1458}L_{\overline{dd}iii}^{V8,LR} - \frac{815}{1458}L_{\overline{dd}jj\overline{ii}}^{V8,LR} - \frac{815}{729}L_{\overline{dd}jj\overline{jj}}^{V8,LR} - \frac{815}{1458}L_{\overline{dd}kk\overline{ii}}^{V8,LR} - \frac{815}{1458}L_{\overline{dd}kk\overline{jj}}^{V8,LR} \\
& + \frac{301}{243}L_{\overline{dd}iii}^{V,RR} - \frac{1522}{243}L_{\overline{dd}ij\overline{jj}}^{V,RR} + \frac{368}{243}L_{\overline{dd}ik\overline{kk}}^{V,RR} - \frac{6776}{729}L_{\overline{dd}ij\overline{ji}}^{V,RR} - \frac{458}{729}L_{\overline{dd}ik\overline{ki}}^{V,RR}
\end{aligned}$$

$$\begin{aligned}
& + \frac{1549}{729} L_{jjj}^{V,RR} + \frac{368}{243} L_{jjk}^{V,RR} - \frac{458}{729} L_{jkk}^{V,RR} + \frac{22}{243} L_{11i}^{V,LR} + \frac{22}{243} L_{11j}^{V,LR} + \frac{22}{243} L_{22i}^{V,LR} \\
& + \frac{22}{243} L_{22j}^{V,LR} + \frac{22}{243} L_{33i}^{V,LR} + \frac{22}{243} L_{33j}^{V,LR} + \frac{22}{243} L_{11i}^{V,RR} + \frac{22}{243} L_{11j}^{V,RR} + \frac{22}{243} L_{22i}^{V,RR} \\
& + \frac{22}{243} L_{22j}^{V,RR} + \frac{22}{243} L_{33i}^{V,RR} + \frac{22}{243} L_{33j}^{V,RR} - \frac{476}{243} L_{11i}^{V1,LR} - \frac{476}{243} L_{11j}^{V1,LR} - \frac{476}{243} L_{22i}^{V1,LR} \\
& - \frac{476}{243} L_{22j}^{V1,LR} - \frac{476}{243} L_{11i}^{V1,RR} - \frac{476}{243} L_{11j}^{V1,RR} - \frac{476}{243} L_{22i}^{V1,RR} - \frac{476}{243} L_{22j}^{V1,RR} \\
& + \frac{697}{1458} L_{11i}^{V8,LR} + \frac{697}{1458} L_{11j}^{V8,LR} + \frac{697}{1458} L_{22i}^{V8,LR} + \frac{697}{1458} L_{22j}^{V8,LR} + \frac{85}{1458} L_{11i}^{V8,RR} \\
& + \frac{85}{1458} L_{11j}^{V8,RR} + \frac{85}{1458} L_{22i}^{V8,RR} + \frac{85}{1458} L_{22j}^{V8,RR} \Big] + \alpha^2 \Big[ - \frac{368}{729} L_{iii}^{V1,LR} - \frac{368}{729} L_{jji}^{V1,LR} \\
& - \frac{736}{729} L_{jjj}^{V1,LR} - \frac{368}{729} L_{kkii}^{V1,LR} - \frac{368}{729} L_{kkjj}^{V1,LR} + \frac{608}{729} L_{iii}^{V,RR} + \frac{686}{729} L_{iij}^{V,RR} \\
& + \frac{272}{729} L_{ikk}^{V,RR} + \frac{296}{2187} L_{ijji}^{V,RR} + \frac{296}{2187} L_{ikki}^{V,RR} + \frac{2936}{2187} L_{jjjj}^{V,RR} + \frac{272}{729} L_{jjk}^{V,RR} \\
& + \frac{296}{2187} L_{jkk}^{V,RR} - \frac{656}{729} L_{11i}^{V,LR} - \frac{656}{729} L_{11j}^{V,LR} - \frac{656}{729} L_{22i}^{V,LR} - \frac{656}{729} L_{22j}^{V,LR} \\
& - \frac{656}{729} L_{33i}^{V,LR} - \frac{656}{729} L_{33j}^{V,LR} + \frac{856}{729} L_{11i}^{V,RR} + \frac{856}{729} L_{11j}^{V,RR} + \frac{856}{729} L_{22i}^{V,RR} + \frac{856}{729} L_{22j}^{V,RR} \\
& + \frac{856}{729} L_{33i}^{V,RR} + \frac{856}{729} L_{33j}^{V,RR} - \frac{1748}{729} L_{11i}^{V1,LR} - \frac{1748}{729} L_{11j}^{V1,LR} - \frac{1748}{729} L_{22i}^{V1,LR} \\
& - \frac{1748}{729} L_{22j}^{V1,LR} + \frac{268}{729} L_{11i}^{V1,RR} + \frac{268}{729} L_{11j}^{V1,RR} + \frac{268}{729} L_{22i}^{V1,RR} + \frac{268}{729} L_{22j}^{V1,RR} \Big] ;
\end{aligned}$$

$$\begin{aligned}
\dot{L}_{ijji}^{V,RR} & = g_s^2 \Big[ \frac{1}{6} L_{iii}^{V8,LR} + \frac{1}{6} L_{jji}^{V8,LR} + \frac{1}{3} L_{jjj}^{V8,LR} + \frac{1}{6} L_{kkii}^{V8,LR} + \frac{1}{6} L_{kkjj}^{V8,LR} \\
& + \frac{2}{3} L_{iii}^{V,RR} + 6 L_{iij}^{V,RR} - \frac{4}{3} L_{ijji}^{V,RR} + \frac{2}{3} L_{ikki}^{V,RR} + \frac{4}{3} L_{jjjj}^{V,RR} + \frac{2}{3} L_{jkk}^{V,RR} \\
& + \frac{1}{6} L_{11i}^{V8,LR} + \frac{1}{6} L_{11j}^{V8,LR} + \frac{1}{6} L_{22i}^{V8,LR} + \frac{1}{6} L_{22j}^{V8,LR} + \frac{1}{6} L_{11i}^{V8,RR} + \frac{1}{6} L_{11j}^{V8,RR} \\
& + \frac{1}{6} L_{22i}^{V8,RR} + \frac{1}{6} L_{22j}^{V8,RR} \Big] + \frac{4}{3} L_{ijji}^{V,RR} e^2 + \alpha_s^2 \Big[ - \frac{11}{6} L_{iii}^{V1,LR} - \frac{11}{6} L_{jji}^{V1,LR} \\
& - \frac{11}{3} L_{jjj}^{V1,LR} - \frac{11}{6} L_{kkii}^{V1,LR} - \frac{11}{6} L_{kkjj}^{V1,LR} + \frac{139}{324} L_{iii}^{V8,LR} + \frac{139}{324} L_{jji}^{V8,LR} + \frac{139}{162} L_{jjj}^{V8,LR}
\end{aligned}$$

$$\begin{aligned}
& + \frac{139}{324} L_{kkii}^{V8,LR} + \frac{139}{324} L_{kkjj}^{V8,LR} + \frac{947}{54} L_{iii}^{V,RR} + \frac{9}{2} L_{ijj}^{V,RR} - \frac{7}{3} L_{ikk}^{V,RR} + \frac{707}{162} L_{ijji}^{V,RR} \\
& + \frac{1294}{81} L_{ikki}^{V,RR} + \frac{5051}{162} L_{jjjj}^{V,RR} - \frac{7}{3} L_{jjkk}^{V,RR} + \frac{1294}{81} L_{jkkj}^{V,RR} - \frac{11}{6} L_{11ii}^{V1,LR} - \frac{11}{6} L_{11jj}^{V1,LR} \\
& - \frac{11}{6} L_{22ii}^{V1,LR} - \frac{11}{6} L_{22jj}^{V1,LR} - \frac{1}{6} L_{11ii}^{V1,RR} - \frac{1}{6} L_{11jj}^{V1,RR} - \frac{1}{6} L_{22ii}^{V1,RR} - \frac{1}{6} L_{22jj}^{V1,RR} \\
& + \frac{139}{324} L_{11ii}^{V8,LR} + \frac{139}{324} L_{11jj}^{V8,LR} + \frac{139}{324} L_{22ii}^{V8,LR} + \frac{139}{324} L_{22jj}^{V8,LR} + \frac{769}{324} L_{11ii}^{V8,RR} \\
& + \frac{769}{324} L_{11jj}^{V8,RR} + \frac{769}{324} L_{22ii}^{V8,RR} + \frac{769}{324} L_{22jj}^{V8,RR} \Big] + \alpha_s \alpha \Bigg[ - \frac{22}{81} L_{iii}^{V1,LR} - \frac{22}{81} L_{jji}^{V1,LR} \\
& - \frac{44}{81} L_{jjjj}^{V1,LR} - \frac{22}{81} L_{kkii}^{V1,LR} - \frac{22}{81} L_{kkjj}^{V1,LR} - \frac{25}{54} L_{iii}^{V8,LR} - \frac{25}{54} L_{jjii}^{V8,LR} - \frac{25}{27} L_{jjjj}^{V8,LR} \\
& - \frac{25}{54} L_{kkii}^{V8,LR} - \frac{25}{54} L_{kkjj}^{V8,LR} + \frac{211}{81} L_{iii}^{V,RR} - \frac{746}{81} L_{ijj}^{V,RR} - \frac{44}{81} L_{ikk}^{V,RR} - \frac{1436}{243} L_{ijji}^{V,RR} \\
& + \frac{454}{243} L_{ikki}^{V,RR} + \frac{955}{243} L_{jjjj}^{V,RR} - \frac{44}{81} L_{jjkk}^{V,RR} + \frac{454}{243} L_{jkkj}^{V,RR} - \frac{22}{81} L_{11ii}^{V,LR} - \frac{22}{81} L_{11jj}^{V,LR} \\
& - \frac{22}{81} L_{22ii}^{V,LR} - \frac{22}{81} L_{22jj}^{V,LR} - \frac{22}{81} L_{33ii}^{V,LR} - \frac{22}{81} L_{33jj}^{V,LR} - \frac{22}{81} L_{11ii}^{V,RR} - \frac{22}{81} L_{11jj}^{V,RR} \\
& - \frac{22}{81} L_{22ii}^{V,RR} - \frac{22}{81} L_{22jj}^{V,RR} - \frac{22}{81} L_{33ii}^{V,RR} - \frac{22}{81} L_{33jj}^{V,RR} + \frac{44}{81} L_{11ii}^{V1,LR} + \frac{44}{81} L_{11jj}^{V1,LR} \\
& + \frac{44}{81} L_{22ii}^{V1,LR} + \frac{44}{81} L_{22jj}^{V1,LR} + \frac{44}{81} L_{11ii}^{V1,RR} + \frac{44}{81} L_{11jj}^{V1,RR} + \frac{44}{81} L_{22ii}^{V1,RR} + \frac{44}{81} L_{22jj}^{V1,RR} \\
& + \frac{71}{54} L_{11ii}^{V8,LR} + \frac{71}{54} L_{11jj}^{V8,LR} + \frac{71}{54} L_{22ii}^{V8,LR} + \frac{71}{54} L_{22jj}^{V8,LR} - \frac{7}{18} L_{11ii}^{V8,RR} - \frac{7}{18} L_{11jj}^{V8,RR} \\
& - \frac{7}{18} L_{22ii}^{V8,RR} - \frac{7}{18} L_{22jj}^{V8,RR} \Big] + \frac{46}{81} L_{ijji}^{V,RR} \alpha^2 ;
\end{aligned}$$

$$\begin{aligned}
\dot{L}_{iii}^{V,RR} &= g_s^2 \Bigg[ \frac{2}{9} L_{iii}^{V8,LR} + \frac{2}{9} L_{jji}^{V8,LR} + \frac{2}{9} L_{kkii}^{V8,LR} + \frac{44}{9} L_{iii}^{V,RR} + \frac{8}{9} L_{ijji}^{V,RR} \\
& + \frac{8}{9} L_{ikki}^{V,RR} + \frac{2}{9} L_{11ii}^{V8,LR} + \frac{2}{9} L_{22ii}^{V8,LR} + \frac{2}{9} L_{11ii}^{V8,RR} + \frac{2}{9} L_{22ii}^{V8,RR} \Big] + e^2 \Bigg[ \frac{4}{9} L_{iii}^{V1,LR} \\
& + \frac{4}{9} L_{jji}^{V1,LR} + \frac{4}{9} L_{kkii}^{V1,LR} + \frac{68}{27} L_{iii}^{V,RR} + \frac{8}{9} L_{ijj}^{V,RR} + \frac{8}{9} L_{ikk}^{V,RR} + \frac{8}{27} L_{ijji}^{V,RR} \\
& + \frac{8}{27} L_{ikki}^{V,RR} + \frac{4}{9} L_{11ii}^{V,LR} + \frac{4}{9} L_{22ii}^{V,LR} + \frac{4}{9} L_{33ii}^{V,LR} + \frac{4}{9} L_{11ii}^{V,RR} + \frac{4}{9} L_{22ii}^{V,RR}
\end{aligned}$$

$$\begin{aligned}
& + \frac{4}{9} L_{33ii}^{V,RR} - \frac{8}{9} L_{11ii}^{V1,LR} - \frac{8}{9} L_{22ii}^{V1,LR} - \frac{8}{9} L_{11ii}^{V1,RR} - \frac{8}{9} L_{22ii}^{V1,RR} \Big] + \alpha_s^2 \Big[ - \frac{94}{9} L_{iii}^{V1,LR} \\
& - \frac{94}{9} L_{jjii}^{V1,LR} - \frac{94}{9} L_{kkii}^{V1,LR} + \frac{175}{243} L_{iii}^{V8,LR} + \frac{175}{243} L_{jjii}^{V8,LR} + \frac{175}{243} L_{kkii}^{V8,LR} + \frac{4459}{81} L_{iii}^{V,RR} \\
& + \frac{116}{9} L_{ijjj}^{V,RR} + \frac{116}{9} L_{iikk}^{V,RR} + \frac{7480}{243} L_{ijji}^{V,RR} + \frac{7480}{243} L_{ikki}^{V,RR} - \frac{94}{9} L_{11ii}^{V1,LR} - \frac{94}{9} L_{22ii}^{V1,LR} \\
& + \frac{70}{9} L_{11ii}^{V1,RR} + \frac{70}{9} L_{22ii}^{V1,RR} + \frac{175}{243} L_{11ii}^{V8,LR} + \frac{175}{243} L_{22ii}^{V8,LR} + \frac{805}{243} L_{11ii}^{V8,RR} + \frac{805}{243} L_{22ii}^{V8,RR} \Big] \\
& + \alpha_s \alpha \Big[ \frac{344}{243} L_{iii}^{V1,LR} + \frac{344}{243} L_{jjii}^{V1,LR} + \frac{344}{243} L_{kkii}^{V1,LR} - \frac{1490}{729} L_{iii}^{V8,LR} - \frac{1490}{729} L_{jjii}^{V8,LR} \\
& - \frac{1490}{729} L_{kkii}^{V8,LR} - \frac{2128}{243} L_{iii}^{V,RR} + \frac{472}{243} L_{ijji}^{V,RR} + \frac{472}{243} L_{iikk}^{V,RR} + \frac{1808}{729} L_{ijji}^{V,RR} \\
& + \frac{1808}{729} L_{iikk}^{V,RR} - \frac{88}{243} L_{11ii}^{V,LR} - \frac{88}{243} L_{22ii}^{V,LR} - \frac{88}{243} L_{33ii}^{V,LR} - \frac{88}{243} L_{11ii}^{V,RR} - \frac{88}{243} L_{22ii}^{V,RR} \\
& - \frac{88}{243} L_{33ii}^{V,RR} - \frac{688}{243} L_{11ii}^{V1,LR} - \frac{688}{243} L_{22ii}^{V1,LR} - \frac{688}{243} L_{11ii}^{V1,RR} - \frac{688}{243} L_{22ii}^{V1,RR} \\
& + \frac{2614}{729} L_{11ii}^{V8,LR} + \frac{2614}{729} L_{22ii}^{V8,LR} - \frac{482}{729} L_{11ii}^{V8,RR} - \frac{482}{729} L_{22ii}^{V8,RR} \Big] + \alpha^2 \Big[ - \frac{736}{729} L_{iii}^{V1,LR} \\
& - \frac{736}{729} L_{jjii}^{V1,LR} - \frac{736}{729} L_{kkii}^{V1,LR} + \frac{1630}{729} L_{iii}^{V,RR} + \frac{544}{729} L_{ijji}^{V,RR} + \frac{544}{729} L_{iikk}^{V,RR} \\
& + \frac{592}{2187} L_{ijji}^{V,RR} + \frac{592}{2187} L_{iikk}^{V,RR} - \frac{1312}{729} L_{11ii}^{V,LR} - \frac{1312}{729} L_{22ii}^{V,LR} - \frac{1312}{729} L_{33ii}^{V,LR} \\
& + \frac{1712}{729} L_{11ii}^{V,RR} + \frac{1712}{729} L_{22ii}^{V,RR} + \frac{1712}{729} L_{33ii}^{V,RR} - \frac{3496}{729} L_{11ii}^{V1,LR} - \frac{3496}{729} L_{22ii}^{V1,LR} \\
& + \frac{536}{729} L_{11ii}^{V1,RR} + \frac{536}{729} L_{22ii}^{V1,RR} \Big] ;
\end{aligned}$$

$$\begin{aligned}
\dot{L}_{ijjj}^{V,RR} &= g_s^2 \Big[ - \frac{1}{18} L_{11ii}^{V8,LR} - \frac{1}{18} L_{11jj}^{V8,LR} - \frac{1}{18} L_{22ii}^{V8,LR} - \frac{1}{18} L_{22jj}^{V8,LR} - \frac{1}{18} L_{33ii}^{V8,LR} \\
& - \frac{1}{18} L_{33jj}^{V8,LR} - \frac{1}{18} L_{ii11}^{V8,RR} - \frac{1}{18} L_{ii22}^{V8,RR} - \frac{1}{18} L_{ii33}^{V8,RR} - \frac{1}{18} L_{jj11}^{V8,RR} - \frac{1}{18} L_{jj22}^{V8,RR} \\
& - \frac{1}{18} L_{jj33}^{V8,RR} - \frac{1}{18} L_{iiii}^{V8,LR} - \frac{1}{18} L_{jjjj}^{V8,LR} - \frac{1}{18} L_{kkii}^{V8,LR} - \frac{1}{18} L_{kkjj}^{V8,LR} - \frac{2}{9} L_{iii}^{V,RR} \Big]
\end{aligned}$$

$$\begin{aligned}
& -2L_{ii jj}^{V,RR} + 6L_{ij ji}^{V,RR} - \frac{2}{9}L_{ik ki}^{V,RR} - \frac{2}{9}L_{jj jj}^{V,RR} - \frac{2}{9}L_{jk kj}^{V,RR} \Big] + e^2 \Big[ -\frac{4}{9}L_{11 ii}^{V1,LR} \\
& -\frac{4}{9}L_{du}^{V1,LR} - \frac{4}{9}L_{du}^{V1,LR} - \frac{4}{9}L_{du}^{V1,LR} - \frac{4}{9}L_{du}^{V1,LR} - \frac{4}{9}L_{du}^{V1,LR} - \frac{4}{9}L_{eu}^{V,LR} \\
& -\frac{4}{9}L_{eu}^{V,LR} - \frac{4}{9}L_{eu}^{V,LR} - \frac{4}{9}L_{eu}^{V,LR} - \frac{4}{9}L_{eu}^{V,LR} - \frac{4}{9}L_{eu}^{V,LR} - \frac{4}{9}L_{eu}^{V,RR} \\
& -\frac{4}{9}L_{11 jj}^{V,RR} - \frac{4}{9}L_{22 ii}^{V,RR} - \frac{4}{9}L_{22 jj}^{V,RR} - \frac{4}{9}L_{33 ii}^{V,RR} - \frac{4}{9}L_{33 jj}^{V,RR} - \frac{4}{9}L_{ii 11}^{V,RR} \\
& -\frac{4}{9}L_{11 jj}^{V,RR} - \frac{4}{9}L_{22 ii}^{V,RR} - \frac{4}{9}L_{22 jj}^{V,RR} - \frac{4}{9}L_{33 ii}^{V,RR} - \frac{4}{9}L_{33 jj}^{V,RR} - \frac{4}{9}L_{ii 11}^{V,RR} \\
& -\frac{4}{9}L_{ud}^{V1,RR} - \frac{4}{9}L_{ud}^{V1,RR} - \frac{4}{9}L_{ud}^{V1,RR} - \frac{4}{9}L_{ud}^{V1,RR} - \frac{4}{9}L_{ud}^{V1,RR} + \frac{8}{9}L_{iii}^{V1,LR} \\
& + \frac{8}{9}L_{jj jj}^{V1,LR} + \frac{8}{9}L_{kk ii}^{V1,LR} + \frac{8}{9}L_{kk jj}^{V1,LR} + \frac{64}{27}L_{iii}^{V,RR} + \frac{16}{3}L_{ii jj}^{V,RR} + \frac{16}{9}L_{ikk}^{V,RR} \\
& + \frac{16}{27}L_{uu}^{V,RR} + \frac{64}{27}L_{jj jj}^{V,RR} + \frac{16}{9}L_{jj kk}^{V,RR} + \frac{16}{27}L_{jj kk}^{V,RR} \Big] + \alpha_s^2 \Big[ -\frac{61}{18}L_{11 ii}^{V1,LR} \\
& -\frac{61}{18}L_{du}^{V1,LR} - \frac{61}{18}L_{du}^{V1,LR} - \frac{61}{18}L_{du}^{V1,LR} - \frac{61}{18}L_{du}^{V1,LR} - \frac{61}{18}L_{du}^{V1,LR} - \frac{85}{972}L_{11 ii}^{V8,LR} \\
& -\frac{85}{972}L_{11 jj}^{V8,LR} - \frac{85}{972}L_{22 ii}^{V8,LR} - \frac{85}{972}L_{22 jj}^{V8,LR} - \frac{85}{972}L_{33 ii}^{V8,LR} - \frac{85}{972}L_{33 jj}^{V8,LR} + \frac{73}{18}L_{ii 11}^{V1,RR} \\
& + \frac{73}{18}L_{ii 22}^{V1,RR} + \frac{73}{18}L_{ii 33}^{V1,RR} + \frac{73}{18}L_{jj 11}^{V1,RR} + \frac{73}{18}L_{jj 22}^{V1,RR} + \frac{73}{18}L_{jj 33}^{V1,RR} - \frac{715}{972}L_{ii 11}^{V8,RR} \\
& -\frac{715}{972}L_{ii 22}^{V8,RR} - \frac{715}{972}L_{ii 33}^{V8,RR} - \frac{715}{972}L_{jj 11}^{V8,RR} - \frac{715}{972}L_{jj 22}^{V8,RR} - \frac{715}{972}L_{jj 33}^{V8,RR} \\
& -\frac{61}{18}L_{uu}^{V1,LR} - \frac{61}{18}L_{uu}^{V1,LR} - \frac{61}{18}L_{uu}^{V1,LR} - \frac{61}{18}L_{uu}^{V1,LR} - \frac{85}{972}L_{uu}^{V8,LR} - \frac{85}{972}L_{uu}^{V8,LR} \\
& -\frac{85}{972}L_{uu}^{V8,LR} - \frac{85}{972}L_{uu}^{V8,LR} + \frac{1993}{162}L_{uu}^{V,RR} - \frac{209}{18}L_{ii jj}^{V,RR} + \frac{79}{9}L_{ikk}^{V,RR} + \frac{41}{6}L_{ij ji}^{V,RR} \\
& -\frac{160}{243}L_{ikk}^{V,RR} + \frac{1993}{162}L_{jj jj}^{V,RR} + \frac{79}{9}L_{jj kk}^{V,RR} - \frac{160}{243}L_{jj kk}^{V,RR} \Big] + \alpha_s \alpha \Big[ -\frac{476}{243}L_{11 ii}^{V1,LR} \\
& -\frac{476}{243}L_{du}^{V1,LR} - \frac{476}{243}L_{du}^{V1,LR} - \frac{476}{243}L_{du}^{V1,LR} + \frac{934}{243}L_{33 ii}^{V1,LR} + \frac{934}{243}L_{33 jj}^{V1,LR} \\
& + \frac{79}{1458}L_{11 ii}^{V8,LR} + \frac{79}{1458}L_{11 jj}^{V8,LR} + \frac{79}{1458}L_{22 ii}^{V8,LR} + \frac{79}{1458}L_{22 jj}^{V8,LR} - \frac{1594}{729}L_{33 ii}^{V8,LR} \\
& -\frac{1594}{729}L_{33 jj}^{V8,LR} - \frac{44}{243}L_{11 ii}^{V,LR} - \frac{44}{243}L_{11 jj}^{V,LR} - \frac{44}{243}L_{22 ii}^{V,LR} - \frac{44}{243}L_{22 jj}^{V,LR} - \frac{44}{243}L_{33 ii}^{V,LR}
\end{aligned}$$



$$\begin{aligned}
& -\frac{44}{243}L_{33jj}^{V,LR} - \frac{44}{243}L_{11ii}^{V,RR} - \frac{44}{243}L_{11jj}^{V,RR} - \frac{44}{243}L_{22ii}^{V,RR} - \frac{44}{243}L_{22jj}^{V,RR} - \frac{44}{243}L_{33ii}^{V,RR} \\
& -\frac{44}{243}L_{33jj}^{V,RR} - \frac{476}{243}L_{ii11}^{V1,RR} - \frac{476}{243}L_{ii22}^{V1,RR} - \frac{476}{243}L_{ii33}^{V1,RR} - \frac{476}{243}L_{jj11}^{V1,RR} \\
& -\frac{476}{243}L_{jj22}^{V1,RR} - \frac{476}{243}L_{jj33}^{V1,RR} - \frac{533}{1458}L_{ii11}^{V8,RR} - \frac{533}{1458}L_{ii22}^{V8,RR} - \frac{533}{1458}L_{ii33}^{V8,RR} \\
& -\frac{533}{1458}L_{jj11}^{V8,RR} - \frac{533}{1458}L_{jj22}^{V8,RR} - \frac{533}{1458}L_{jj33}^{V8,RR} + \frac{952}{243}L_{iii}^{V1,LR} + \frac{952}{243}L_{jjj}^{V1,LR} \\
& + \frac{952}{243}L_{kii}^{V1,LR} + \frac{952}{243}L_{kkj}^{V1,LR} - \frac{1594}{729}L_{iii}^{V8,LR} - \frac{1594}{729}L_{jjj}^{V8,LR} - \frac{1594}{729}L_{kii}^{V8,LR} \\
& - \frac{1594}{729}L_{kkj}^{V8,LR} + \frac{1252}{243}L_{iii}^{V,RR} - \frac{280}{9}L_{ijj}^{V,RR} + \frac{1472}{243}L_{iik}^{V,RR} - \frac{104}{3}L_{ijji}^{V,RR} - \frac{1688}{729}L_{ikki}^{V,RR} \\
& + \frac{1252}{243}L_{jjj}^{V,RR} + \frac{1472}{243}L_{jjkk}^{V,RR} - \frac{1688}{729}L_{jjkj}^{V,RR} \Big] + \alpha^2 \Big[ -\frac{1052}{729}L_{11ii}^{V1,LR} - \frac{1052}{729}L_{11jj}^{V1,LR} \\
& - \frac{1052}{729}L_{22ii}^{V1,LR} - \frac{1052}{729}L_{22jj}^{V1,LR} - \frac{6176}{729}L_{33ii}^{V1,LR} - \frac{6176}{729}L_{33jj}^{V1,LR} - \frac{4796}{729}L_{11ii}^{V,LR} \\
& - \frac{4796}{729}L_{11jj}^{V,LR} - \frac{4796}{729}L_{22ii}^{V,LR} - \frac{4796}{729}L_{22jj}^{V,LR} - \frac{4796}{729}L_{33ii}^{V,LR} - \frac{4796}{729}L_{33jj}^{V,LR} \\
& + \frac{1252}{729}L_{11ii}^{V,RR} + \frac{1252}{729}L_{11jj}^{V,RR} + \frac{1252}{729}L_{22ii}^{V,RR} + \frac{1252}{729}L_{22jj}^{V,RR} + \frac{1252}{729}L_{33ii}^{V,RR} \\
& + \frac{1252}{729}L_{33jj}^{V,RR} + \frac{964}{729}L_{ii11}^{V1,RR} + \frac{964}{729}L_{ii22}^{V1,RR} + \frac{964}{729}L_{ii33}^{V1,RR} + \frac{964}{729}L_{jj11}^{V1,RR} \\
& + \frac{964}{729}L_{jj22}^{V1,RR} + \frac{964}{729}L_{jj33}^{V1,RR} - \frac{5888}{729}L_{iii}^{V1,LR} - \frac{5888}{729}L_{jjj}^{V1,LR} - \frac{5888}{729}L_{kii}^{V1,LR} \\
& - \frac{5888}{729}L_{kkj}^{V1,LR} + \frac{9728}{729}L_{iii}^{V,RR} - \frac{1184}{81}L_{ijj}^{V,RR} + \frac{4352}{729}L_{iik}^{V,RR} + \frac{4736}{2187}L_{ikki}^{V,RR} \\
& + \frac{9728}{729}L_{jjj}^{V,RR} + \frac{4352}{729}L_{jjkk}^{V,RR} + \frac{4736}{2187}L_{jjkj}^{V,RR} \Big] ;
\end{aligned}$$

$$\begin{aligned}
\dot{L}_{ijji}^{V,RR} &= g_s^2 \Big[ \frac{1}{6}L_{11ii}^{V8,LR} + \frac{1}{6}L_{11jj}^{V8,LR} + \frac{1}{6}L_{22ii}^{V8,LR} + \frac{1}{6}L_{22jj}^{V8,LR} + \frac{1}{6}L_{33ii}^{V8,LR} \\
& + \frac{1}{6}L_{33jj}^{V8,LR} + \frac{1}{6}L_{ii11}^{V8,RR} + \frac{1}{6}L_{ii22}^{V8,RR} + \frac{1}{6}L_{ii33}^{V8,RR} + \frac{1}{6}L_{jj11}^{V8,RR} + \frac{1}{6}L_{jj22}^{V8,RR} \\
& + \frac{1}{6}L_{jj33}^{V8,RR} + \frac{1}{6}L_{iii}^{V8,LR} + \frac{1}{6}L_{jjj}^{V8,LR} + \frac{1}{6}L_{kii}^{V8,LR} + \frac{1}{6}L_{kkj}^{V8,LR} + \frac{2}{3}L_{iii}^{V,RR} \Big]
\end{aligned}$$

$$\begin{aligned}
& + 6L_{ijj}^{V,RR} - 2L_{ijji}^{V,RR} + \frac{2}{3}L_{ikki}^{V,RR} + \frac{2}{3}L_{jjjj}^{V,RR} + \frac{2}{3}L_{jkkj}^{V,RR} \Big] + \frac{16}{3}L_{ijji}^{V,RR} \\
e^2 + \alpha_s^2 & \left[ -\frac{11}{6}L_{11ii}^{V1,LR} - \frac{11}{6}L_{11jj}^{V1,LR} - \frac{11}{6}L_{22ii}^{V1,LR} - \frac{11}{6}L_{22jj}^{V1,LR} - \frac{11}{6}L_{33ii}^{V1,LR} \right. \\
& - \frac{11}{6}L_{33jj}^{V1,LR} + \frac{157}{324}L_{11ii}^{V8,LR} + \frac{157}{324}L_{11jj}^{V8,LR} + \frac{157}{324}L_{22ii}^{V8,LR} + \frac{157}{324}L_{22jj}^{V8,LR} \\
& + \frac{157}{324}L_{33ii}^{V8,LR} + \frac{157}{324}L_{33jj}^{V8,LR} - \frac{1}{6}L_{ii11}^{V1,RR} - \frac{1}{6}L_{ii22}^{V1,RR} - \frac{1}{6}L_{ii33}^{V1,RR} - \frac{1}{6}L_{jj11}^{V1,RR} \\
& - \frac{1}{6}L_{jj22}^{V1,RR} - \frac{1}{6}L_{jj33}^{V1,RR} + \frac{787}{324}L_{ii11}^{V8,RR} + \frac{787}{324}L_{ii22}^{V8,RR} + \frac{787}{324}L_{ii33}^{V8,RR} + \frac{787}{324}L_{jj11}^{V8,RR} \\
& + \frac{787}{324}L_{jj22}^{V8,RR} + \frac{787}{324}L_{jj33}^{V8,RR} - \frac{11}{6}L_{iii}^{V1,LR} - \frac{11}{6}L_{jjj}^{V1,LR} - \frac{11}{6}L_{kkj}^{V1,LR} - \frac{11}{6}L_{kkj}^{V1,LR} \\
& + \frac{157}{324}L_{iii}^{V8,LR} + \frac{157}{324}L_{jjj}^{V8,LR} + \frac{157}{324}L_{kkj}^{V8,LR} + \frac{157}{324}L_{kkj}^{V8,LR} + \frac{959}{54}L_{iii}^{V,RR} \\
& + \frac{41}{6}L_{ijj}^{V,RR} - \frac{7}{3}L_{ikk}^{V,RR} - \frac{209}{18}L_{ijji}^{V,RR} + \frac{1312}{81}L_{ikki}^{V,RR} + \frac{959}{54}L_{jjjj}^{V,RR} - \frac{7}{3}L_{jjkk}^{V,RR} \\
& + \frac{1312}{81}L_{jkkj}^{V,RR} \Big] + \alpha_s \alpha \left[ \frac{44}{81}L_{11ii}^{V1,LR} + \frac{44}{81}L_{11jj}^{V1,LR} + \frac{44}{81}L_{22ii}^{V1,LR} + \frac{44}{81}L_{22jj}^{V1,LR} \right. \\
& - \frac{70}{81}L_{33ii}^{V1,LR} - \frac{70}{81}L_{33jj}^{V1,LR} + \frac{65}{54}L_{11ii}^{V8,LR} + \frac{65}{54}L_{11jj}^{V8,LR} + \frac{65}{54}L_{22ii}^{V8,LR} + \frac{65}{54}L_{22jj}^{V8,LR} \\
& - \frac{50}{27}L_{33ii}^{V8,LR} - \frac{50}{27}L_{33jj}^{V8,LR} + \frac{44}{81}L_{11ii}^{V,LR} + \frac{44}{81}L_{11jj}^{V,LR} + \frac{44}{81}L_{22ii}^{V,LR} + \frac{44}{81}L_{22jj}^{V,LR} \\
& + \frac{44}{81}L_{33ii}^{V,LR} + \frac{44}{81}L_{33jj}^{V,LR} + \frac{44}{81}L_{11ii}^{V,RR} + \frac{44}{81}L_{11jj}^{V,RR} + \frac{44}{81}L_{22ii}^{V,RR} + \frac{44}{81}L_{22jj}^{V,RR} \\
& + \frac{44}{81}L_{33ii}^{V,RR} + \frac{44}{81}L_{33jj}^{V,RR} + \frac{44}{81}L_{ii11}^{V1,RR} + \frac{44}{81}L_{ii22}^{V1,RR} + \frac{44}{81}L_{ii33}^{V1,RR} + \frac{44}{81}L_{jj11}^{V1,RR} \\
& + \frac{44}{81}L_{jj22}^{V1,RR} + \frac{44}{81}L_{jj33}^{V1,RR} - \frac{1}{2}L_{ii11}^{V8,RR} - \frac{1}{2}L_{ii22}^{V8,RR} - \frac{1}{2}L_{ii33}^{V8,RR} - \frac{1}{2}L_{jj11}^{V8,RR} \\
& - \frac{1}{2}L_{jj22}^{V8,RR} - \frac{1}{2}L_{jj33}^{V8,RR} - \frac{88}{81}L_{iii}^{V1,LR} - \frac{88}{81}L_{jjj}^{V1,LR} - \frac{88}{81}L_{kkj}^{V1,LR} - \frac{88}{81}L_{kkj}^{V1,LR} \\
& - \frac{50}{27}L_{iii}^{V8,LR} - \frac{50}{27}L_{jjj}^{V8,LR} - \frac{50}{27}L_{kkj}^{V8,LR} - \frac{50}{27}L_{kkj}^{V8,LR} + \frac{844}{81}L_{iii}^{V,RR} - \frac{104}{3}L_{ijj}^{V,RR} \\
& \left. - \frac{176}{81}L_{ikk}^{V,RR} - \frac{280}{9}L_{ijji}^{V,RR} + \frac{1816}{243}L_{ikki}^{V,RR} + \frac{844}{81}L_{jjjj}^{V,RR} - \frac{176}{81}L_{jjkk}^{V,RR} + \frac{1816}{243}L_{jkkj}^{V,RR} \right]
\end{aligned}$$

$$\begin{aligned}
& -\frac{1184}{81}L_{ijji}^{V,RR}\alpha^2; \\
\dot{L}_{uu\bar{iii}}^{V,RR} = & g_s^2 \left[ \frac{2}{9}L_{11\bar{ii}}^{V8,LR} + \frac{2}{9}L_{22\bar{ii}}^{V8,LR} + \frac{2}{9}L_{33\bar{ii}}^{V8,LR} + \frac{2}{9}L_{\bar{ii}11}^{V8,RR} + \frac{2}{9}L_{\bar{ii}22}^{V8,RR} \right. \\
& + \frac{2}{9}L_{\bar{ii}33}^{V8,RR} + \frac{2}{9}L_{\bar{iii}i}^{V8,LR} + \frac{2}{9}L_{\bar{kk}ii}^{V8,LR} + \frac{44}{9}L_{\bar{iii}i}^{V,RR} + \frac{8}{9}L_{\bar{ikk}i}^{V,RR} \left. \right] + e^2 \left[ -\frac{8}{9}L_{11\bar{ii}}^{V1,LR} \right. \\
& - \frac{8}{9}L_{22\bar{ii}}^{V1,LR} - \frac{8}{9}L_{33\bar{ii}}^{V1,LR} - \frac{8}{9}L_{11\bar{ii}}^{V,LR} - \frac{8}{9}L_{22\bar{ii}}^{V,LR} - \frac{8}{9}L_{33\bar{ii}}^{V,LR} - \frac{8}{9}L_{11\bar{ii}}^{V,RR} \\
& - \frac{8}{9}L_{22\bar{ii}}^{V,RR} - \frac{8}{9}L_{33\bar{ii}}^{V,RR} - \frac{8}{9}L_{\bar{ii}11}^{V1,RR} - \frac{8}{9}L_{\bar{ii}22}^{V1,RR} - \frac{8}{9}L_{\bar{ii}33}^{V1,RR} + \frac{16}{9}L_{\bar{iii}i}^{V1,LR} \\
& + \frac{16}{9}L_{\bar{kk}ii}^{V1,LR} + \frac{272}{27}L_{\bar{iii}i}^{V,RR} + \frac{32}{9}L_{\bar{uu}i}^{V,RR} + \frac{32}{27}L_{\bar{ikk}i}^{V,RR} \left. \right] + \alpha_s^2 \left[ -\frac{94}{9}L_{11\bar{ii}}^{V1,LR} \right. \\
& - \frac{94}{9}L_{22\bar{ii}}^{V1,LR} - \frac{94}{9}L_{33\bar{ii}}^{V1,LR} + \frac{193}{243}L_{11\bar{ii}}^{V8,LR} + \frac{193}{243}L_{22\bar{ii}}^{V8,LR} + \frac{193}{243}L_{33\bar{ii}}^{V8,LR} + \frac{70}{9}L_{\bar{ii}11}^{V1,RR} \\
& + \frac{70}{9}L_{\bar{ii}22}^{V1,RR} + \frac{70}{9}L_{\bar{ii}33}^{V1,RR} + \frac{823}{243}L_{\bar{ii}11}^{V8,RR} + \frac{823}{243}L_{\bar{ii}22}^{V8,RR} + \frac{823}{243}L_{\bar{ii}33}^{V8,RR} - \frac{94}{9}L_{\bar{iii}i}^{V1,LR} \\
& - \frac{94}{9}L_{\bar{kk}ii}^{V1,LR} + \frac{193}{243}L_{\bar{iii}i}^{V8,LR} + \frac{193}{243}L_{\bar{kk}ii}^{V8,LR} + \frac{4483}{81}L_{\bar{iii}i}^{V,RR} + \frac{116}{9}L_{\bar{ikk}i}^{V,RR} + \frac{7552}{243}L_{\bar{ikk}i}^{V,RR} \left. \right] \\
& + \alpha_s \alpha \left[ -\frac{688}{243}L_{11\bar{ii}}^{V1,LR} - \frac{688}{243}L_{22\bar{ii}}^{V1,LR} + \frac{1448}{243}L_{33\bar{ii}}^{V1,LR} + \frac{1834}{729}L_{11\bar{ii}}^{V8,LR} + \frac{1834}{729}L_{22\bar{ii}}^{V8,LR} \right. \\
& - \frac{5888}{729}L_{33\bar{ii}}^{V8,LR} + \frac{176}{243}L_{11\bar{ii}}^{V,LR} + \frac{176}{243}L_{22\bar{ii}}^{V,LR} + \frac{176}{243}L_{33\bar{ii}}^{V,LR} + \frac{176}{243}L_{11\bar{ii}}^{V,RR} \\
& + \frac{176}{243}L_{22\bar{ii}}^{V,RR} + \frac{176}{243}L_{33\bar{ii}}^{V,RR} - \frac{688}{243}L_{\bar{ii}11}^{V1,RR} - \frac{688}{243}L_{\bar{ii}22}^{V1,RR} - \frac{688}{243}L_{\bar{ii}33}^{V1,RR} \\
& - \frac{1262}{729}L_{\bar{ii}11}^{V8,RR} - \frac{1262}{729}L_{\bar{ii}22}^{V8,RR} - \frac{1262}{729}L_{\bar{ii}33}^{V8,RR} + \frac{1376}{243}L_{\bar{iii}i}^{V1,LR} + \frac{1376}{243}L_{\bar{kk}ii}^{V1,LR} \\
& - \frac{5888}{729}L_{\bar{iii}i}^{V8,LR} - \frac{5888}{729}L_{\bar{kk}ii}^{V8,LR} - \frac{8416}{243}L_{\bar{iii}i}^{V,RR} + \frac{1888}{243}L_{\bar{ikk}i}^{V,RR} + \frac{7520}{729}L_{\bar{ikk}i}^{V,RR} \left. \right] \\
& + \alpha^2 \left[ -\frac{2104}{729}L_{11\bar{ii}}^{V1,LR} - \frac{2104}{729}L_{22\bar{ii}}^{V1,LR} - \frac{12352}{729}L_{33\bar{ii}}^{V1,LR} - \frac{9592}{729}L_{11\bar{ii}}^{V,LR} - \frac{9592}{729}L_{22\bar{ii}}^{V,LR} \right. \\
& - \frac{9592}{729}L_{33\bar{ii}}^{V,LR} + \frac{2504}{729}L_{11\bar{ii}}^{V,RR} + \frac{2504}{729}L_{22\bar{ii}}^{V,RR} + \frac{2504}{729}L_{33\bar{ii}}^{V,RR} + \frac{1928}{729}L_{\bar{ii}11}^{V1,RR} \\
& + \frac{1928}{729}L_{\bar{ii}22}^{V1,RR} + \frac{1928}{729}L_{\bar{ii}33}^{V1,RR} - \frac{11776}{729}L_{\bar{iii}i}^{V1,LR} - \frac{11776}{729}L_{\bar{kk}ii}^{V1,LR} + \frac{8800}{729}L_{\bar{iii}i}^{V,RR} \left. \right]
\end{aligned}$$

$$\begin{aligned}
& + \frac{8704}{729} L_{uu}^{V,RR} + \frac{9472}{2187} L_{ikk}^{V,RR} \Big] ; \\
\dot{L}_{ijj}^{V,RR} = & e^2 \left[ \frac{1}{3} L_{jjii}^{V,LR} + \frac{40}{3} L_{ijj}^{V,RR} + \frac{1}{3} L_{kkii}^{V,LR} + \frac{4}{3} L_{ikk}^{V,RR} + \frac{1}{3} L_{11ii}^{V,LR} \right. \\
& + \frac{1}{3} L_{22ii}^{V,LR} + \frac{1}{3} L_{33ii}^{V,LR} + \frac{1}{3} L_{ii11}^{V,RR} + \frac{1}{3} L_{ii22}^{V,RR} + \frac{1}{3} L_{ii33}^{V,RR} + \frac{1}{3} L_{iii}^{V,LR} \\
& + \frac{4}{3} L_{iii}^{V,RR} - \frac{2}{3} L_{ii11}^{V,RR} - \frac{2}{3} L_{ii22}^{V,RR} - \frac{2}{3} L_{ii33}^{V,RR} - \frac{2}{3} L_{11ii}^{V,LR} - \frac{2}{3} L_{22ii}^{V,LR} + \frac{1}{3} L_{kkjj}^{V,RR} \\
& + \frac{4}{3} L_{jjkk}^{V,RR} + \frac{1}{3} L_{11jj}^{V,LR} + \frac{1}{3} L_{22jj}^{V,LR} + \frac{1}{3} L_{33jj}^{V,LR} + \frac{1}{3} L_{jj11}^{V,RR} + \frac{1}{3} L_{jj22}^{V,RR} \\
& + \frac{1}{3} L_{jj33}^{V,RR} + \frac{2}{3} L_{jjjj}^{V,LR} + 2 L_{jjjj}^{V,RR} - \frac{2}{3} L_{jj11}^{V,RR} - \frac{2}{3} L_{jj22}^{V,RR} - \frac{2}{3} L_{jj33}^{V,RR} \\
& \left. - \frac{2}{3} L_{ue}^{V,LR} \right] + \alpha_s \alpha \left[ \frac{4}{3} L_{11ii}^{V,LR} + \frac{4}{3} L_{22ii}^{V,LR} + \frac{4}{3} L_{33ii}^{V,LR} + \frac{4}{3} L_{ii11}^{V,RR} \right. \\
& + \frac{4}{3} L_{ii22}^{V,RR} + \frac{4}{3} L_{ii33}^{V,RR} - \frac{8}{3} L_{ii11}^{V,RR} - \frac{8}{3} L_{ii22}^{V,RR} - \frac{8}{3} L_{ii33}^{V,RR} - \frac{8}{3} L_{11ii}^{V,LR} - \frac{8}{3} L_{22ii}^{V,LR} \\
& + \frac{4}{3} L_{11jj}^{V,LR} + \frac{4}{3} L_{22jj}^{V,LR} + \frac{4}{3} L_{33jj}^{V,LR} + \frac{4}{3} L_{jj11}^{V,RR} + \frac{4}{3} L_{jj22}^{V,RR} + \frac{4}{3} L_{jj33}^{V,RR} \\
& \left. - \frac{8}{3} L_{jj11}^{V,RR} - \frac{8}{3} L_{jj22}^{V,RR} - \frac{8}{3} L_{jj33}^{V,RR} - \frac{8}{3} L_{11jj}^{V,LR} - \frac{8}{3} L_{22jj}^{V,LR} \right] + \alpha^2 \left[ - \frac{178}{27} L_{jjii}^{V,LR} \right. \\
& - \frac{2302}{27} L_{ijj}^{V,RR} - \frac{178}{27} L_{kkii}^{V,LR} + \frac{296}{27} L_{ikk}^{V,RR} + \frac{34}{81} L_{11ii}^{V,LR} + \frac{34}{81} L_{22ii}^{V,LR} + \frac{34}{81} L_{33ii}^{V,LR} \\
& + \frac{166}{81} L_{ii11}^{V,RR} + \frac{166}{81} L_{ii22}^{V,RR} + \frac{166}{81} L_{ii33}^{V,RR} - \frac{178}{27} L_{iii}^{V,LR} + \frac{320}{27} L_{iii}^{V,RR} - \frac{314}{81} L_{ii11}^{V,RR} \\
& - \frac{314}{81} L_{ii22}^{V,RR} - \frac{842}{81} L_{ii33}^{V,RR} - \frac{842}{81} L_{11ii}^{V,LR} - \frac{178}{27} L_{kkjj}^{V,LR} + \frac{296}{27} L_{jjkk}^{V,RR} + \frac{34}{81} L_{11jj}^{V,LR} \\
& + \frac{34}{81} L_{22jj}^{V,LR} + \frac{34}{81} L_{33jj}^{V,LR} + \frac{166}{81} L_{jj11}^{V,RR} + \frac{166}{81} L_{jj22}^{V,RR} + \frac{166}{81} L_{jj33}^{V,RR} - \frac{356}{27} L_{jjjj}^{V,LR} \\
& \left. + \frac{52}{3} L_{jjjj}^{V,RR} - \frac{314}{81} L_{jj11}^{V,RR} - \frac{314}{81} L_{jj22}^{V,RR} - \frac{842}{81} L_{jj33}^{V,RR} - \frac{842}{81} L_{11jj}^{V,LR} - \frac{842}{81} L_{22jj}^{V,LR} \right] ; \\
\dot{L}_{iii}^{V,RR} = & e^2 \left[ \frac{4}{3} L_{jjii}^{V,LR} + \frac{16}{3} L_{ijj}^{V,RR} + \frac{4}{3} L_{kkii}^{V,LR} + \frac{16}{3} L_{ikk}^{V,RR} + \frac{4}{3} L_{11ii}^{V,LR} \right. \\
& + \frac{4}{3} L_{22ii}^{V,LR} + \frac{4}{3} L_{33ii}^{V,LR} + \frac{4}{3} L_{ii11}^{V,RR} + \frac{4}{3} L_{ii22}^{V,RR} + \frac{4}{3} L_{ii33}^{V,RR} + \frac{4}{3} L_{iii}^{V,LR} \\
& + \frac{4}{3} L_{iii}^{V,RR} - \frac{2}{3} L_{ii11}^{V,RR} - \frac{2}{3} L_{ii22}^{V,RR} - \frac{2}{3} L_{ii33}^{V,RR} - \frac{2}{3} L_{11ii}^{V,LR} - \frac{2}{3} L_{22ii}^{V,LR} + \frac{1}{3} L_{kkjj}^{V,RR} \\
& + \frac{4}{3} L_{jjkk}^{V,RR} + \frac{1}{3} L_{11jj}^{V,LR} + \frac{1}{3} L_{22jj}^{V,LR} + \frac{1}{3} L_{33jj}^{V,LR} + \frac{1}{3} L_{jj11}^{V,RR} + \frac{1}{3} L_{jj22}^{V,RR} \\
& + \frac{1}{3} L_{jj33}^{V,RR} + \frac{2}{3} L_{jjjj}^{V,LR} + 2 L_{jjjj}^{V,RR} - \frac{2}{3} L_{jj11}^{V,RR} - \frac{2}{3} L_{jj22}^{V,RR} - \frac{2}{3} L_{jj33}^{V,RR} \\
& \left. - \frac{2}{3} L_{ue}^{V,LR} \right] + \alpha_s \alpha \left[ \frac{4}{3} L_{11ii}^{V,LR} + \frac{4}{3} L_{22ii}^{V,LR} + \frac{4}{3} L_{33ii}^{V,LR} + \frac{4}{3} L_{ii11}^{V,RR} \right. \\
& + \frac{4}{3} L_{ii22}^{V,RR} + \frac{4}{3} L_{ii33}^{V,RR} - \frac{8}{3} L_{ii11}^{V,RR} - \frac{8}{3} L_{ii22}^{V,RR} - \frac{8}{3} L_{ii33}^{V,RR} - \frac{8}{3} L_{11ii}^{V,LR} - \frac{8}{3} L_{22ii}^{V,LR} \\
& + \frac{4}{3} L_{11jj}^{V,LR} + \frac{4}{3} L_{22jj}^{V,LR} + \frac{4}{3} L_{33jj}^{V,LR} + \frac{4}{3} L_{jj11}^{V,RR} + \frac{4}{3} L_{jj22}^{V,RR} + \frac{4}{3} L_{jj33}^{V,RR} \\
& \left. - \frac{8}{3} L_{jj11}^{V,RR} - \frac{8}{3} L_{jj22}^{V,RR} - \frac{8}{3} L_{jj33}^{V,RR} - \frac{8}{3} L_{11jj}^{V,LR} - \frac{8}{3} L_{22jj}^{V,LR} \right] + \alpha^2 \left[ - \frac{178}{27} L_{jjii}^{V,LR} \right. \\
& - \frac{2302}{27} L_{ijj}^{V,RR} - \frac{178}{27} L_{kkii}^{V,LR} + \frac{296}{27} L_{ikk}^{V,RR} + \frac{34}{81} L_{11ii}^{V,LR} + \frac{34}{81} L_{22ii}^{V,LR} + \frac{34}{81} L_{33ii}^{V,LR} \\
& + \frac{166}{81} L_{ii11}^{V,RR} + \frac{166}{81} L_{ii22}^{V,RR} + \frac{166}{81} L_{ii33}^{V,RR} - \frac{178}{27} L_{iii}^{V,LR} + \frac{320}{27} L_{iii}^{V,RR} - \frac{314}{81} L_{ii11}^{V,RR} \\
& - \frac{314}{81} L_{ii22}^{V,RR} - \frac{842}{81} L_{ii33}^{V,RR} - \frac{842}{81} L_{11ii}^{V,LR} - \frac{178}{27} L_{kkjj}^{V,LR} + \frac{296}{27} L_{jjkk}^{V,RR} + \frac{34}{81} L_{11jj}^{V,LR} \\
& + \frac{34}{81} L_{22jj}^{V,LR} + \frac{34}{81} L_{33jj}^{V,LR} + \frac{166}{81} L_{jj11}^{V,RR} + \frac{166}{81} L_{jj22}^{V,RR} + \frac{166}{81} L_{jj33}^{V,RR} - \frac{356}{27} L_{jjjj}^{V,LR} \\
& \left. + \frac{52}{3} L_{jjjj}^{V,RR} - \frac{314}{81} L_{jj11}^{V,RR} - \frac{314}{81} L_{jj22}^{V,RR} - \frac{842}{81} L_{jj33}^{V,RR} - \frac{842}{81} L_{11jj}^{V,LR} - \frac{842}{81} L_{22jj}^{V,LR} \right] ;
\end{aligned}$$

$$\begin{aligned}
& + \frac{52}{3} L_{\bar{u}\bar{u}\bar{u}}^{V,RR} - \frac{8}{3} L_{\bar{u}\bar{u}11}^{V,RR} - \frac{8}{3} L_{\bar{u}\bar{u}22}^{V,RR} - \frac{8}{3} L_{11\bar{u}\bar{u}}^{V,LR} - \frac{8}{3} L_{22\bar{u}\bar{u}}^{V,LR} \Big] + \alpha_s \alpha \Big[ \frac{16}{3} L_{11\bar{u}\bar{u}}^{V,LR} \\
& + \frac{16}{3} L_{22\bar{u}\bar{u}}^{V,LR} + \frac{16}{3} L_{33\bar{u}\bar{u}}^{V,LR} + \frac{16}{3} L_{\bar{u}\bar{u}11}^{V,RR} + \frac{16}{3} L_{\bar{u}\bar{u}22}^{V,RR} + \frac{16}{3} L_{\bar{u}\bar{u}33}^{V,RR} - \frac{32}{3} L_{\bar{u}\bar{u}11}^{V,RR} \\
& - \frac{32}{3} L_{\bar{u}\bar{u}22}^{V,RR} - \frac{32}{3} L_{11\bar{u}\bar{u}}^{V,LR} - \frac{32}{3} L_{22\bar{u}\bar{u}}^{V,LR} \Big] + \alpha^2 \Big[ -\frac{712}{27} L_{\bar{u}\bar{u}\bar{u}}^{V,LR} + \frac{1184}{27} L_{\bar{u}\bar{u}\bar{u}}^{V,RR} \\
& - \frac{712}{27} L_{\bar{u}\bar{u}\bar{u}}^{V,LR} + \frac{1184}{27} L_{\bar{u}\bar{u}\bar{u}}^{V,RR} + \frac{136}{81} L_{11\bar{u}\bar{u}}^{V,LR} + \frac{136}{81} L_{22\bar{u}\bar{u}}^{V,LR} + \frac{136}{81} L_{33\bar{u}\bar{u}}^{V,LR} + \frac{664}{81} L_{\bar{u}\bar{u}11}^{V,RR} \\
& + \frac{664}{81} L_{\bar{u}\bar{u}22}^{V,RR} + \frac{664}{81} L_{\bar{u}\bar{u}33}^{V,RR} - \frac{712}{27} L_{\bar{u}\bar{u}\bar{u}}^{V,LR} - \frac{1318}{27} L_{\bar{u}\bar{u}\bar{u}}^{V,RR} - \frac{1256}{81} L_{\bar{u}\bar{u}11}^{V,RR} - \frac{1256}{81} L_{\bar{u}\bar{u}22}^{V,RR} \\
& - \frac{3368}{81} L_{11\bar{u}\bar{u}}^{V,LR} - \frac{3368}{81} L_{22\bar{u}\bar{u}}^{V,LR} \Big] ;
\end{aligned}$$

$$\begin{aligned}
\dot{L}_{\bar{u}\bar{u}\bar{u}}^{V,LR} & = e^2 \Big[ \frac{8}{3} L_{\bar{u}\bar{u}\bar{u}}^{V1,LR} + \frac{4}{3} L_{\bar{u}\bar{u}\bar{u}}^{V1,LR} + \frac{64}{9} L_{\bar{u}\bar{u}\bar{u}}^{V,RR} + \frac{8}{3} L_{\bar{u}\bar{u}\bar{u}}^{V,RR} + \frac{8}{9} L_{\bar{u}\bar{u}\bar{u}}^{V,RR} \\
& + \frac{4}{9} L_{\bar{u}\bar{u}11}^{V,LL} + \frac{4}{9} L_{\bar{u}\bar{u}22}^{V,LL} + \frac{4}{9} L_{\bar{u}\bar{u}33}^{V,LL} + \frac{4}{3} L_{11\bar{u}\bar{u}}^{V,LR} + \frac{4}{3} L_{22\bar{u}\bar{u}}^{V,LR} + \frac{4}{3} L_{33\bar{u}\bar{u}}^{V,LR} \\
& + \frac{4}{9} L_{\bar{u}\bar{u}11}^{V,LR} + \frac{4}{9} L_{\bar{u}\bar{u}22}^{V,LR} + \frac{4}{9} L_{\bar{u}\bar{u}33}^{V,LR} - 4 L_{\bar{u}\bar{u}\bar{u}}^{V,LR} + \frac{4}{3} L_{11\bar{u}\bar{u}}^{V,RR} + \frac{4}{3} L_{22\bar{u}\bar{u}}^{V,RR} \\
& + \frac{4}{3} L_{\bar{u}\bar{u}33}^{V,RR} + \frac{16}{9} L_{\bar{u}\bar{u}\bar{u}}^{V,LL} + \frac{16}{9} L_{\bar{u}\bar{u}\bar{u}}^{V,LL} + \frac{16}{9} L_{\bar{u}\bar{u}\bar{u}}^{V,LL} + \frac{4}{9} L_{\bar{u}\bar{u}\bar{u}}^{V,LR} + \frac{4}{9} L_{\bar{u}\bar{u}\bar{u}}^{V,LR} \\
& + \frac{4}{9} L_{\bar{u}\bar{u}\bar{u}}^{V,LR} - \frac{8}{9} L_{\bar{u}\bar{u}11}^{V,LL} - \frac{8}{9} L_{\bar{u}\bar{u}22}^{V,LL} - \frac{8}{9} L_{\bar{u}\bar{u}33}^{V,LL} - \frac{8}{9} L_{11\bar{u}\bar{u}}^{V,LR} - \frac{8}{9} L_{22\bar{u}\bar{u}}^{V,LR} - \frac{8}{3} L_{11\bar{u}\bar{u}}^{V1,LR} \\
& - \frac{8}{3} L_{22\bar{u}\bar{u}}^{V1,LR} - \frac{8}{3} L_{11\bar{u}\bar{u}}^{V1,RR} - \frac{8}{3} L_{22\bar{u}\bar{u}}^{V1,RR} \Big] + \alpha_s^2 \Big[ -8 L_{\bar{u}\bar{u}11}^{V,LL} - 8 L_{\bar{u}\bar{u}22}^{V,LL} \\
& - 8 L_{\bar{u}\bar{u}33}^{V,LL} + 8 L_{\bar{u}\bar{u}11}^{V,LR} + 8 L_{\bar{u}\bar{u}22}^{V,LR} + 8 L_{\bar{u}\bar{u}33}^{V,LR} - 8 L_{\bar{u}\bar{u}11}^{V,LL} - 8 L_{\bar{u}\bar{u}22}^{V,LL} \\
& + 8 L_{\bar{u}\bar{u}11}^{V,LR} + 8 L_{\bar{u}\bar{u}22}^{V,LR} \Big] + \alpha_s \alpha \Big[ \frac{32}{3} L_{\bar{u}\bar{u}\bar{u}}^{V1,LR} + \frac{16}{3} L_{\bar{u}\bar{u}\bar{u}}^{V1,LR} - \frac{2080}{243} L_{\bar{u}\bar{u}\bar{u}}^{V8,LR} \\
& - \frac{1040}{243} L_{\bar{u}\bar{u}\bar{u}}^{V8,LR} + \frac{5008}{243} L_{\bar{u}\bar{u}\bar{u}}^{V,RR} + 8 L_{\bar{u}\bar{u}\bar{u}}^{V,RR} - \frac{8}{243} L_{\bar{u}\bar{u}\bar{u}}^{V,RR} + \frac{16}{9} L_{\bar{u}\bar{u}11}^{V,LL} + \frac{16}{9} L_{\bar{u}\bar{u}22}^{V,LL} \\
& + \frac{16}{9} L_{\bar{u}\bar{u}33}^{V,LL} + \frac{16}{9} L_{\bar{u}\bar{u}11}^{V,LR} + \frac{16}{9} L_{\bar{u}\bar{u}22}^{V,LR} + \frac{16}{9} L_{\bar{u}\bar{u}33}^{V,LR} + 16 L_{\bar{u}\bar{u}\bar{u}}^{V,LR} - \frac{32}{9} L_{\bar{u}\bar{u}11}^{V,LL} \\
& - \frac{32}{9} L_{\bar{u}\bar{u}22}^{V,LL} - \frac{32}{9} L_{\bar{u}\bar{u}33}^{V,LL} - \frac{32}{9} L_{\bar{u}\bar{u}\bar{u}}^{V,LR} - \frac{32}{3} L_{11\bar{u}\bar{u}}^{V1,LR} - \frac{32}{3} L_{22\bar{u}\bar{u}}^{V1,LR} - \frac{32}{3} L_{11\bar{u}\bar{u}}^{V1,RR} \\
& - \frac{32}{3} L_{22\bar{u}\bar{u}}^{V1,RR} \Big] ;
\end{aligned}$$

$$\begin{aligned}
& -\frac{32}{3}L_{22jj}^{V1,RR} + \frac{1336}{243}L_{11jj}^{V8,LR} + \frac{1336}{243}L_{22jj}^{V8,LR} - \frac{104}{243}L_{11jj}^{V8,RR} - \frac{104}{243}L_{22jj}^{V8,RR} \Big] \\
& + \alpha^2 \Big[ \frac{3424}{243}L_{jjjj}^{V1,LR} + \frac{1712}{243}L_{kkjj}^{V1,LR} - \frac{3056}{729}L_{jjjj}^{V,RR} + \frac{256}{243}L_{jjkk}^{V,RR} - \frac{1424}{729}L_{jjkk}^{V,RR} \\
& - \frac{440}{243}L_{ii11}^{V,LL} - \frac{440}{243}L_{ii22}^{V,LL} - \frac{440}{243}L_{ii33}^{V,LL} + \frac{3728}{243}L_{11jj}^{V,LR} + \frac{3728}{243}L_{22jj}^{V,LR} \\
& + \frac{3728}{243}L_{33jj}^{V,LR} - \frac{104}{243}L_{ii11}^{V,LR} - \frac{104}{243}L_{ii22}^{V,LR} - \frac{104}{243}L_{ii33}^{V,LR} + \frac{1994}{27}L_{ijjj}^{V,LR} \\
& - \frac{1024}{243}L_{11jj}^{V,RR} - \frac{1024}{243}L_{22jj}^{V,RR} - \frac{1024}{243}L_{33jj}^{V,RR} - \frac{640}{81}L_{iii}^{V,LL} - \frac{160}{81}L_{ijjj}^{V,LL} \\
& - \frac{160}{81}L_{iikk}^{V,LL} - \frac{184}{81}L_{iii}^{V,LR} - \frac{184}{81}L_{ijjj}^{V,LR} - \frac{184}{81}L_{iikk}^{V,LR} - \frac{1640}{243}L_{ii11}^{V,LL} - \frac{1640}{243}L_{ii22}^{V,LL} \\
& - \frac{296}{243}L_{ii11}^{V,LR} - \frac{296}{243}L_{ii22}^{V,LR} - \frac{616}{243}L_{11jj}^{V1,LR} - \frac{616}{243}L_{22jj}^{V1,LR} - \frac{6952}{243}L_{11jj}^{V1,RR} \\
& - \frac{6952}{243}L_{22jj}^{V1,RR} \Big] ;
\end{aligned}$$

$$\begin{aligned}
\dot{L}_{ijj}^{V,LR} &= e^2 \Big[ \frac{4}{3}L_{11jj}^{V1,LR} + \frac{4}{3}L_{22jj}^{V1,LR} + \frac{4}{3}L_{33jj}^{V1,LR} - \frac{8}{9}L_{ii11}^{V,LL} - \frac{8}{9}L_{ii22}^{V,LL} \\
& - \frac{8}{9}L_{ii33}^{V,LL} - \frac{8}{9}L_{ii11}^{V,LR} - \frac{8}{9}L_{ii22}^{V,LR} - \frac{8}{9}L_{ii33}^{V,LR} - \frac{32}{9}L_{iii}^{V,LL} - \frac{32}{9}L_{ijjj}^{V,LL} \\
& - \frac{32}{9}L_{iikk}^{V,LL} - \frac{8}{9}L_{iii}^{V,LR} - \frac{8}{9}L_{ijjj}^{V,LR} - \frac{8}{9}L_{iikk}^{V,LR} + \frac{16}{9}L_{ii11}^{V,LL} + \frac{16}{9}L_{ii22}^{V,LL} \\
& + \frac{4}{3}L_{11jj}^{V,LR} + \frac{4}{3}L_{22jj}^{V,LR} + \frac{4}{3}L_{33jj}^{V,LR} + \frac{16}{9}L_{ii11}^{V,LR} + \frac{16}{9}L_{ii22}^{V,LR} + 8L_{ijjj}^{V,LR} \\
& + \frac{4}{3}L_{11jj}^{V,RR} + \frac{4}{3}L_{22jj}^{V,RR} + \frac{4}{3}L_{33jj}^{V,RR} + \frac{4}{3}L_{ud}^{V1,RR} + \frac{4}{3}L_{jj22}^{V1,RR} + \frac{4}{3}L_{jj33}^{V1,RR} \\
& - \frac{8}{3}L_{jjjj}^{V1,LR} - \frac{8}{3}L_{kkjj}^{V1,LR} - \frac{64}{9}L_{jjjj}^{V,RR} - \frac{16}{3}L_{jjkk}^{V,RR} - \frac{16}{9}L_{jjkk}^{V,RR} \Big] + \alpha_s^2 \Big[ -8L_{ii11}^{V,LL} \\
& - 8L_{ii22}^{V,LL} - 8L_{ii33}^{V,LL} + 8L_{ii11}^{V,LR} + 8L_{ii22}^{V,LR} + 8L_{ii33}^{V,LR} - 8L_{ii11}^{V,LL} \\
& - 8L_{ii22}^{V,LL} + 8L_{ii11}^{V,LR} + 8L_{ii22}^{V,LR} \Big] + \alpha_s \alpha \Big[ \frac{16}{3}L_{11jj}^{V1,LR} + \frac{16}{3}L_{22jj}^{V1,LR} \\
& - \frac{32}{3}L_{33jj}^{V1,LR} - \frac{332}{243}L_{11jj}^{V8,LR} - \frac{332}{243}L_{22jj}^{V8,LR} + \frac{2044}{243}L_{33jj}^{V8,LR} - \frac{32}{9}L_{ii11}^{V,LL} - \frac{32}{9}L_{ii22}^{V,LL}
\end{aligned}$$

$$\begin{aligned}
& -\frac{32}{9}L_{ed\ i33}^{V,LL} - \frac{32}{9}L_{ed\ ii11}^{V,LR} - \frac{32}{9}L_{ed\ ii22}^{V,LR} - \frac{32}{9}L_{ed\ i33}^{V,LR} + \frac{64}{9}L_{eu\ ii11}^{V,LL} + \frac{64}{9}L_{eu\ ii22}^{V,LL} \\
& + \frac{64}{9}L_{eu\ ii11}^{V,LR} + \frac{64}{9}L_{eu\ ii22}^{V,LR} - 32L_{eu\ ijj}^{V,LR} + \frac{16}{3}L_{ud\ jj11}^{V1,RR} + \frac{16}{3}L_{ud\ jj22}^{V1,RR} + \frac{16}{3}L_{ud\ jj33}^{V1,RR} \\
& + \frac{388}{243}L_{ud\ jj11}^{V8,RR} + \frac{388}{243}L_{ud\ jj22}^{V8,RR} + \frac{388}{243}L_{ud\ jj33}^{V8,RR} - \frac{32}{3}L_{uu\ jjjj}^{V1,LR} - \frac{32}{3}L_{uu\ kkjj}^{V1,LR} + \frac{2044}{243}L_{uu\ jjjj}^{V8,LR} \\
& + \frac{2044}{243}L_{uu\ kkjj}^{V8,LR} - \frac{2096}{81}L_{uu\ jjjj}^{V,RR} - 16L_{uu\ jjkk}^{V,RR} - \frac{128}{243}L_{jjkk}^{V,RR} \Big] + \alpha^2 \Big[ -\frac{1144}{243}L_{11jj}^{V1,LR} \\
& - \frac{1144}{243}L_{22jj}^{V1,LR} + \frac{12512}{243}L_{33jj}^{V1,LR} + \frac{1168}{243}L_{ed\ ii11}^{V,LL} + \frac{1168}{243}L_{ed\ ii22}^{V,LL} + \frac{1168}{243}L_{ed\ ii33}^{V,LL} \\
& + \frac{1792}{243}L_{ed\ ii11}^{V,LR} + \frac{1792}{243}L_{ed\ ii22}^{V,LR} + \frac{1792}{243}L_{ed\ ii33}^{V,LR} + \frac{992}{81}L_{ee\ iii}^{V,LL} + \frac{896}{81}L_{ee\ ijj}^{V,LL} \\
& + \frac{896}{81}L_{ee\ iikk}^{V,LL} + \frac{1808}{81}L_{ee\ iii}^{V,LR} + \frac{1808}{81}L_{ee\ ijj}^{V,LR} + \frac{1808}{81}L_{ee\ iikk}^{V,LR} - \frac{1184}{243}L_{eu\ ii11}^{V,LL} - \frac{1184}{243}L_{eu\ ii22}^{V,LL} \\
& + \frac{3248}{243}L_{eu\ 11jj}^{V,LR} + \frac{3248}{243}L_{eu\ 22jj}^{V,LR} + \frac{3248}{243}L_{eu\ 33jj}^{V,LR} + \frac{1312}{243}L_{eu\ ii11}^{V,LR} + \frac{1312}{243}L_{eu\ ii22}^{V,LR} \\
& - \frac{4960}{27}L_{eu\ ijj}^{V,LR} - \frac{4744}{243}L_{11jj}^{V,RR} - \frac{4744}{243}L_{22jj}^{V,RR} - \frac{4744}{243}L_{33jj}^{V,RR} - \frac{3808}{243}L_{ud\ jj11}^{V1,RR} \\
& - \frac{3808}{243}L_{ud\ jj22}^{V1,RR} - \frac{3808}{243}L_{ud\ jj33}^{V1,RR} + \frac{12224}{243}L_{uu\ jjjj}^{V1,LR} + \frac{12224}{243}L_{uu\ kkjj}^{V1,LR} + \frac{3808}{243}L_{uu\ jjjj}^{V,RR} \\
& + \frac{3136}{243}L_{uu\ jjkk}^{V,RR} + \frac{1024}{729}L_{jjkk}^{V,RR} \Big] ;
\end{aligned}$$

$$\begin{aligned}
\dot{L}_{ud\ ijj}^{V1,LR} = & -\frac{8}{3}L_{ud\ ijj}^{V8,LR}g_s^2 + e^2 \Big[ -\frac{16}{9}L_{dd\ jjjj}^{V1,LR} - \frac{8}{9}L_{dd\ kkjj}^{V1,LR} - \frac{128}{27}L_{dd\ jjjj}^{V,RR} - \frac{16}{9}L_{dd\ jjkk}^{V,RR} \\
& - \frac{16}{27}L_{dd\ jjkk}^{V,RR} - \frac{8}{9}L_{ed\ 11jj}^{V,LR} - \frac{8}{9}L_{ed\ 22jj}^{V,LR} - \frac{8}{9}L_{ed\ 33jj}^{V,LR} - \frac{8}{9}L_{ed\ 11jj}^{V,RR} - \frac{8}{9}L_{ed\ 22jj}^{V,RR} \\
& - \frac{8}{9}L_{ed\ 33jj}^{V,RR} + \frac{4}{9}L_{eu\ 11ii}^{V,LL} + \frac{4}{9}L_{eu\ 22ii}^{V,LL} + \frac{4}{9}L_{eu\ 33ii}^{V,LL} + \frac{4}{9}L_{ud\ ii11}^{V1,LL} + \frac{4}{9}L_{ud\ ii22}^{V1,LL} \\
& + \frac{4}{9}L_{ud\ ii33}^{V1,LL} + \frac{16}{9}L_{ud\ 11jj}^{V1,LR} + \frac{16}{9}L_{ud\ 22jj}^{V1,LR} + \frac{4}{9}L_{ud\ ii11}^{V1,LR} + \frac{4}{9}L_{ud\ ii22}^{V1,LR} + \frac{4}{9}L_{ud\ ii33}^{V1,LR} \\
& + \frac{8}{3}L_{ud\ ijj}^{V1,LR} + \frac{16}{9}L_{ud\ 11jj}^{V1,RR} + \frac{16}{9}L_{ud\ 22jj}^{V1,RR} + \frac{4}{9}L_{ue\ ii11}^{V,LR} + \frac{4}{9}L_{ue\ ii22}^{V,LR} + \frac{4}{9}L_{ue\ ii33}^{V,LR} \\
& - \frac{8}{9}L_{uu\ iii}^{V1,LR} - \frac{8}{9}L_{uu\ iikk}^{V1,LR} - \frac{64}{27}L_{uu\ iii}^{V,LL} - \frac{16}{9}L_{uu\ iikk}^{V,LL} - \frac{16}{27}L_{ikki}^{V,LL} \Big] + \alpha_s^2 \Big[ 16L_{dd\ jjjj}^{V1,LR}
\end{aligned}$$

$$\begin{aligned}
& + 8L_{\substack{dd \\ kkjj}}^{V1,LR} + \frac{88}{27}L_{\substack{dd \\ jjjj}}^{V8,LR} + \frac{44}{27}L_{\substack{dd \\ kkjj}}^{V8,LR} - \frac{1192}{27}L_{\substack{dd \\ jjjj}}^{V,RR} - 16L_{\substack{dd \\ jjkk}}^{V,RR} - \frac{64}{27}L_{\substack{dd \\ jkkj}}^{V,RR} \\
& - 8L_{\substack{ud \\ ii11}}^{V1,LL} - 8L_{\substack{ud \\ ii22}}^{V1,LL} - 8L_{\substack{ud \\ ii33}}^{V1,LL} + 8L_{\substack{ud \\ 11jj}}^{V1,LR} + 8L_{\substack{ud \\ 22jj}}^{V1,LR} + 8L_{\substack{ud \\ ii11}}^{V1,LR} \\
& + 8L_{\substack{ud \\ ii22}}^{V1,LR} + 8L_{\substack{ud \\ ii33}}^{V1,LR} - \frac{28}{3}L_{\substack{ud \\ 11jj}}^{V1,LR} - 8L_{\substack{ud \\ 11jj}}^{V1,RR} - 8L_{\substack{ud \\ 22jj}}^{V1,RR} + \frac{44}{27}L_{\substack{ud \\ ii11}}^{V8,LL} \\
& + \frac{44}{27}L_{\substack{ud \\ ii22}}^{V8,LL} + \frac{44}{27}L_{\substack{ud \\ ii33}}^{V8,LL} + \frac{44}{27}L_{\substack{ud \\ 11jj}}^{V8,LR} + \frac{44}{27}L_{\substack{ud \\ 22jj}}^{V8,LR} + \frac{44}{27}L_{\substack{ud \\ ii11}}^{V8,LR} + \frac{44}{27}L_{\substack{ud \\ ii22}}^{V8,LR} \\
& + \frac{44}{27}L_{\substack{ud \\ ii33}}^{V8,LR} - \frac{2044}{27}L_{\substack{ud \\ iijj}}^{V8,LR} + \frac{44}{27}L_{\substack{ud \\ 11jj}}^{V8,RR} + \frac{44}{27}L_{\substack{ud \\ 22jj}}^{V8,RR} + 8L_{\substack{uu \\ iii}}^{V1,LR} + 8L_{\substack{uu \\ iikk}}^{V1,LR} \\
& + \frac{44}{27}L_{\substack{uu \\ iii}}^{V8,LR} + \frac{44}{27}L_{\substack{uu \\ iikk}}^{V8,LR} - \frac{232}{9}L_{\substack{uu \\ iii}}^{V,LL} - 16L_{\substack{uu \\ iikk}}^{V,LL} - \frac{64}{27}L_{\substack{uu \\ ikki}}^{V,LL} \Big] + \alpha_s \alpha \Big[ - \frac{64}{9}L_{\substack{dd \\ jjjj}}^{V1,LR} \\
& - \frac{32}{9}L_{\substack{dd \\ kkjj}}^{V1,LR} + \frac{4160}{729}L_{\substack{dd \\ jjjj}}^{V8,LR} + \frac{2080}{729}L_{\substack{dd \\ kkjj}}^{V8,LR} - \frac{10016}{729}L_{\substack{dd \\ jjjj}}^{V,RR} - \frac{16}{3}L_{\substack{dd \\ jjkk}}^{V,RR} \\
& + \frac{16}{729}L_{\substack{dd \\ jkkj}}^{V,RR} + \frac{16}{9}L_{\substack{ud \\ ii11}}^{V1,LL} + \frac{16}{9}L_{\substack{ud \\ ii22}}^{V1,LL} + \frac{16}{9}L_{\substack{ud \\ ii33}}^{V1,LL} + \frac{64}{9}L_{\substack{ud \\ 11jj}}^{V1,LR} + \frac{64}{9}L_{\substack{ud \\ 22jj}}^{V1,LR} \\
& + \frac{16}{9}L_{\substack{ud \\ ii11}}^{V1,LR} + \frac{16}{9}L_{\substack{ud \\ ii22}}^{V1,LR} - \frac{32}{9}L_{\substack{ud \\ ii33}}^{V1,LR} - \frac{64}{3}L_{\substack{ud \\ iijj}}^{V1,LR} + \frac{64}{9}L_{\substack{ud \\ 11jj}}^{V1,RR} + \frac{64}{9}L_{\substack{ud \\ 22jj}}^{V1,RR} \\
& + \frac{388}{729}L_{\substack{ud \\ ii11}}^{V8,LL} + \frac{388}{729}L_{\substack{ud \\ ii22}}^{V8,LL} + \frac{388}{729}L_{\substack{ud \\ ii33}}^{V8,LL} - \frac{2672}{729}L_{\substack{ud \\ 11jj}}^{V8,LR} - \frac{2672}{729}L_{\substack{ud \\ 22jj}}^{V8,LR} \\
& - \frac{332}{729}L_{\substack{ud \\ ii11}}^{V8,LR} - \frac{332}{729}L_{\substack{ud \\ ii22}}^{V8,LR} + \frac{2044}{729}L_{\substack{ud \\ ii33}}^{V8,LR} + \frac{232}{27}L_{\substack{ud \\ iijj}}^{V8,LR} + \frac{208}{729}L_{\substack{ud \\ 11jj}}^{V8,RR} \\
& + \frac{208}{729}L_{\substack{ud \\ 22jj}}^{V8,RR} - \frac{32}{9}L_{\substack{uu \\ iii}}^{V1,LR} - \frac{32}{9}L_{\substack{uu \\ iikk}}^{V1,LR} + \frac{2044}{729}L_{\substack{uu \\ iii}}^{V8,LR} + \frac{2044}{729}L_{\substack{uu \\ iikk}}^{V8,LR} \\
& - \frac{2096}{243}L_{\substack{uu \\ iii}}^{V,LL} - \frac{16}{3}L_{\substack{uu \\ iikk}}^{V,LL} - \frac{128}{729}L_{\substack{uu \\ ikki}}^{V,LL} \Big] + \alpha^2 \Big[ \frac{7552}{729}L_{\substack{dd \\ jjjj}}^{V1,LR} + \frac{3776}{729}L_{\substack{dd \\ kkjj}}^{V1,LR} \\
& + \frac{5392}{2187}L_{\substack{dd \\ jjjj}}^{V,RR} + \frac{928}{729}L_{\substack{dd \\ jjkk}}^{V,RR} - \frac{32}{2187}L_{\substack{dd \\ jkkj}}^{V,RR} + \frac{6224}{729}L_{\substack{ed \\ 11jj}}^{V,LR} + \frac{6224}{729}L_{\substack{ed \\ 22jj}}^{V,LR} \\
& + \frac{6224}{729}L_{\substack{ed \\ 33jj}}^{V,LR} - \frac{3712}{729}L_{\substack{ed \\ 11jj}}^{V,RR} - \frac{3712}{729}L_{\substack{ed \\ 22jj}}^{V,RR} - \frac{3712}{729}L_{\substack{ed \\ 33jj}}^{V,RR} - \frac{1216}{729}L_{\substack{eu \\ 11ii}}^{V,LL} \\
& - \frac{1216}{729}L_{\substack{eu \\ 22ii}}^{V,LL} - \frac{1216}{729}L_{\substack{eu \\ 33ii}}^{V,LL} - \frac{1576}{729}L_{\substack{ud \\ ii11}}^{V1,LL} - \frac{1576}{729}L_{\substack{ud \\ ii22}}^{V1,LL} - \frac{1576}{729}L_{\substack{ud \\ ii33}}^{V1,LL} \\
& + \frac{6272}{729}L_{\substack{ud \\ 11jj}}^{V1,LR} + \frac{6272}{729}L_{\substack{ud \\ 22jj}}^{V1,LR} - \frac{208}{729}L_{\substack{ud \\ ii11}}^{V1,LR} - \frac{208}{729}L_{\substack{ud \\ ii22}}^{V1,LR} + \frac{6752}{729}L_{\substack{ud \\ ii33}}^{V1,LR}
\end{aligned}$$



$$\begin{aligned}
& -\frac{4048}{81}L_{ud\,ijj}^{V1,LR} - \frac{6976}{729}L_{11jj}^{V1,RR} - \frac{6976}{729}L_{22jj}^{V1,RR} + \frac{2888}{729}L_{ue\,ii11}^{V,LR} + \frac{2888}{729}L_{ue\,ii22}^{V,LR} \\
& + \frac{2888}{729}L_{ue\,ii33}^{V,LR} + \frac{6464}{729}L_{uu\,iii}^{V1,LR} + \frac{6464}{729}L_{uu\,ikk}^{V1,LR} + \frac{4384}{729}L_{uu\,iii}^{V,LL} + \frac{1984}{729}L_{uu\,ikk}^{V,LL} \\
& + \frac{3328}{2187}L_{uu\,ikki}^{V,LL} \Bigg] ; \\
\dot{L}_{ud\,ijj}^{V8,LR} = & g_s^2 \Bigg[ \frac{4}{3}L_{dd\,jjjj}^{V8,LR} + \frac{2}{3}L_{kkjj}^{V8,LR} + \frac{16}{3}L_{dd\,jjjj}^{V,RR} + \frac{8}{3}L_{jkkj}^{V,RR} - 12L_{ud\,ijj}^{V1,LR} \\
& + \frac{2}{3}L_{ud\,ii11}^{V8,LL} + \frac{2}{3}L_{ud\,ii22}^{V8,LL} + \frac{2}{3}L_{ud\,ii33}^{V8,LL} + \frac{2}{3}L_{11jj}^{V8,LR} + \frac{2}{3}L_{22jj}^{V8,LR} + \frac{2}{3}L_{ud\,ii11}^{V8,LR} \\
& + \frac{2}{3}L_{ud\,ii22}^{V8,LR} + \frac{2}{3}L_{ud\,ii33}^{V8,LR} - 14L_{ud\,ijj}^{V8,LR} + \frac{2}{3}L_{11jj}^{V8,RR} + \frac{2}{3}L_{22jj}^{V8,RR} + \frac{2}{3}L_{uu\,iii}^{V8,LR} \\
& + \frac{2}{3}L_{uu\,ikk}^{V8,LR} + \frac{8}{3}L_{uu\,iii}^{V,LL} + \frac{8}{3}L_{uu\,ikki}^{V,LL} \Bigg] + \frac{8}{3}L_{ud\,ijj}^{V8,LR}e^2 + \alpha_s^2 \Bigg[ -\frac{44}{3}L_{dd\,jjjj}^{V1,LR} \\
& - \frac{22}{3}L_{kkjj}^{V1,LR} + \frac{1538}{81}L_{dd\,jjjj}^{V8,LR} + \frac{769}{81}L_{kkjj}^{V8,LR} + \frac{6142}{81}L_{jjjj}^{V,RR} - \frac{28}{3}L_{jjkk}^{V,RR} + \frac{3376}{81}L_{jjkk}^{V,RR} \\
& - \frac{2}{3}L_{ud\,ii11}^{V1,LL} - \frac{2}{3}L_{ud\,ii22}^{V1,LL} - \frac{2}{3}L_{ud\,ii33}^{V1,LL} - \frac{22}{3}L_{11jj}^{V1,LR} - \frac{22}{3}L_{22jj}^{V1,LR} - \frac{22}{3}L_{ud\,ii11}^{V1,LR} \\
& - \frac{22}{3}L_{ud\,ii22}^{V1,LR} - \frac{22}{3}L_{ud\,ii33}^{V1,LR} - \frac{374}{3}L_{ud\,ijj}^{V1,LR} - \frac{2}{3}L_{11jj}^{V1,RR} - \frac{2}{3}L_{22jj}^{V1,RR} + \frac{607}{81}L_{ud\,ii11}^{V8,LL} \\
& + \frac{607}{81}L_{ud\,ii22}^{V8,LL} + \frac{607}{81}L_{ud\,ii33}^{V8,LL} + \frac{769}{81}L_{11jj}^{V8,LR} + \frac{769}{81}L_{22jj}^{V8,LR} + \frac{787}{81}L_{ud\,ii11}^{V8,LR} + \frac{787}{81}L_{ud\,ii22}^{V8,LR} \\
& + \frac{787}{81}L_{ud\,ii33}^{V8,LR} - \frac{2975}{18}L_{ud\,ijj}^{V8,LR} + \frac{589}{81}L_{11jj}^{V8,RR} + \frac{589}{81}L_{22jj}^{V8,RR} - \frac{22}{3}L_{uu\,iii}^{V1,LR} - \frac{22}{3}L_{uu\,ikk}^{V1,LR} \\
& + \frac{787}{81}L_{uu\,iii}^{V8,LR} + \frac{787}{81}L_{uu\,ikk}^{V8,LR} + \frac{1198}{27}L_{uu\,iii}^{V,LL} - \frac{28}{3}L_{uu\,ikk}^{V,LL} + \frac{3448}{81}L_{uu\,ikki}^{V,LL} \Bigg] \\
& + \alpha_s \alpha \Bigg[ -\frac{1832}{81}L_{dd\,jjjj}^{V1,LR} - \frac{916}{81}L_{kkjj}^{V1,LR} - \frac{88}{9}L_{dd\,jjjj}^{V8,LR} - \frac{44}{9}L_{kkjj}^{V8,LR} - \frac{11264}{243}L_{jjjj}^{V,RR} \\
& - \frac{1832}{81}L_{jjkk}^{V,RR} + \frac{664}{243}L_{jjkk}^{V,RR} - \frac{916}{81}L_{11jj}^{V,LR} - \frac{916}{81}L_{22jj}^{V,LR} - \frac{916}{81}L_{33jj}^{V,LR} - \frac{916}{81}L_{11jj}^{V,RR} \\
& - \frac{916}{81}L_{22jj}^{V,RR} - \frac{916}{81}L_{33jj}^{V,RR} + \frac{644}{81}L_{11ii}^{V,LL} + \frac{644}{81}L_{22ii}^{V,LL} + \frac{644}{81}L_{33ii}^{V,LL} + \frac{644}{81}L_{ud\,ii11}^{V1,LL} \\
& + \frac{644}{81}L_{ud\,ii22}^{V1,LL} + \frac{644}{81}L_{ud\,ii33}^{V1,LL} + \frac{1832}{81}L_{11jj}^{V1,LR} + \frac{1832}{81}L_{22jj}^{V1,LR} + \frac{644}{81}L_{ud\,ii11}^{V1,LR}
\end{aligned}$$

$$\begin{aligned}
& + \frac{644}{81} L_{ud,ii22}^{V1,LR} - \frac{1216}{81} L_{ud,ii33}^{V1,LR} + \frac{116}{3} L_{ud,ijj}^{V1,LR} + \frac{1832}{81} L_{ud,11jj}^{V1,RR} + \frac{1832}{81} L_{ud,22jj}^{V1,RR} \\
& - \frac{70}{27} L_{ud,ii11}^{V8,LL} - \frac{70}{27} L_{ud,ii22}^{V8,LL} - \frac{70}{27} L_{ud,ii33}^{V8,LL} + \frac{56}{9} L_{ud,11jj}^{V8,LR} + \frac{56}{9} L_{ud,22jj}^{V8,LR} + \frac{14}{9} L_{ud,ii11}^{V8,LR} \\
& + \frac{14}{9} L_{ud,ii22}^{V8,LR} - \frac{20}{3} L_{ud,ii33}^{V8,LR} + \frac{187}{9} L_{ud,ijj}^{V8,LR} - \frac{160}{27} L_{ud,11jj}^{V8,RR} - \frac{160}{27} L_{ud,22jj}^{V8,RR} + \frac{644}{81} L_{ue,ii11}^{V,LR} \\
& + \frac{644}{81} L_{ue,ii22}^{V,LR} + \frac{644}{81} L_{ue,ii33}^{V,LR} - \frac{1288}{81} L_{uu,iii}^{V1,LR} - \frac{1288}{81} L_{uu,iikk}^{V1,LR} - \frac{20}{3} L_{uu,iii}^{V8,LR} - \frac{20}{3} L_{uu,iikk}^{V8,LR} \\
& - \frac{3608}{81} L_{uu,iii}^{V,LL} - \frac{2576}{81} L_{uu,iikk}^{V,LL} - \frac{800}{243} L_{ikki}^{V,LL} \Big] - \frac{4048}{81} L_{ud,ijj}^{V8,LR} \alpha^2 ;
\end{aligned}$$

$$\begin{aligned}
\dot{L}_{ed,jji}^{V,LR} &= e^2 \Big[ \frac{4}{3} L_{dd,iii}^{V1,LR} + \frac{4}{3} L_{dd,jji}^{V1,LR} + \frac{4}{3} L_{dd,kkii}^{V1,LR} + \frac{32}{9} L_{dd,iii}^{V,RR} + \frac{8}{3} L_{dd,ijj}^{V,RR} \\
& + \frac{8}{3} L_{dd,iikk}^{V,RR} + \frac{8}{9} L_{dd,ijji}^{V,RR} + \frac{8}{9} L_{dd,ikki}^{V,RR} + \frac{4}{9} L_{ed,jj11}^{V,LL} + \frac{4}{9} L_{ed,jj22}^{V,LL} + \frac{4}{9} L_{ed,jj33}^{V,LL} \\
& + \frac{4}{3} L_{ed,11ii}^{V,LR} + \frac{4}{3} L_{ed,22ii}^{V,LR} + \frac{4}{3} L_{ed,33ii}^{V,LR} + \frac{4}{9} L_{ed,jj11}^{V,LR} + \frac{4}{9} L_{ed,jj22}^{V,LR} + \frac{4}{9} L_{ed,jj33}^{V,LR} \\
& - 4 L_{ed,jji}^{V,LR} + \frac{4}{3} L_{ed,11ii}^{V,RR} + \frac{4}{3} L_{ed,22ii}^{V,RR} + \frac{4}{3} L_{ed,33ii}^{V,RR} + \frac{8}{3} L_{ee,jjjj}^{V,LL} + \frac{16}{9} L_{ee,jjkk}^{V,LL} \\
& + \frac{8}{9} L_{ee,jjjj}^{V,LR} + \frac{4}{9} L_{ee,jjkk}^{V,LR} - \frac{8}{9} L_{ee,jj11}^{V,LL} - \frac{8}{9} L_{ee,jj22}^{V,LL} - \frac{8}{9} L_{ee,jj11}^{V,LR} - \frac{8}{9} L_{ee,jj22}^{V,LR} \\
& - \frac{8}{3} L_{ud,11ii}^{V1,LR} - \frac{8}{3} L_{ud,22ii}^{V1,LR} - \frac{8}{3} L_{ud,11ii}^{V1,RR} - \frac{8}{3} L_{ud,22ii}^{V1,RR} \Big] + \alpha_s^2 \Big[ - 8 L_{ed,jj11}^{V,LL} \\
& - 8 L_{ed,jj22}^{V,LL} - 8 L_{ed,jj33}^{V,LL} + 8 L_{ed,jj11}^{V,LR} + 8 L_{ed,jj22}^{V,LR} + 8 L_{ed,jj33}^{V,LR} - 8 L_{eu,jj11}^{V,LL} \\
& - 8 L_{eu,jj22}^{V,LL} + 8 L_{eu,jj11}^{V,LR} + 8 L_{eu,jj22}^{V,LR} \Big] + \alpha_s \alpha \Big[ \frac{16}{3} L_{dd,iii}^{V1,LR} + \frac{16}{3} L_{dd,jji}^{V1,LR} \\
& + \frac{16}{3} L_{dd,kkii}^{V1,LR} - \frac{1040}{243} L_{dd,iii}^{V8,LR} - \frac{1040}{243} L_{dd,jji}^{V8,LR} - \frac{1040}{243} L_{dd,kkii}^{V8,LR} + \frac{1024}{81} L_{dd,iii}^{V,RR} \\
& + 8 L_{dd,ijj}^{V,RR} + 8 L_{dd,iikk}^{V,RR} - \frac{8}{243} L_{dd,ijji}^{V,RR} - \frac{8}{243} L_{dd,ikki}^{V,RR} + \frac{16}{9} L_{ed,jj11}^{V,LL} + \frac{16}{9} L_{ed,jj22}^{V,LL} \\
& + \frac{16}{9} L_{ed,jj33}^{V,LL} + \frac{16}{9} L_{ed,jj11}^{V,LR} + \frac{16}{9} L_{ed,jj22}^{V,LR} + \frac{16}{9} L_{ed,jj33}^{V,LR} + 16 L_{ed,jji}^{V,LR} - \frac{32}{9} L_{eu,jj11}^{V,LL} \\
& - \frac{32}{9} L_{eu,jj22}^{V,LL} - \frac{32}{9} L_{eu,jj11}^{V,LR} - \frac{32}{9} L_{eu,jj22}^{V,LR} - \frac{32}{3} L_{ud,11ii}^{V1,LR} - \frac{32}{3} L_{ud,22ii}^{V1,LR} - \frac{32}{3} L_{ud,11ii}^{V1,RR}
\end{aligned}$$

$$\begin{aligned}
& -\frac{32}{3}L_{22ii}^{V1,RR} + \frac{1336}{243}L_{11ii}^{V8,LR} + \frac{1336}{243}L_{22ii}^{V8,LR} - \frac{104}{243}L_{11ii}^{V8,RR} - \frac{104}{243}L_{22ii}^{V8,RR} \Bigg] \\
& + \alpha^2 \Bigg[ \frac{1712}{243}L_{dd\bar{iii}}^{V1,LR} + \frac{1712}{243}L_{jj\bar{ii}}^{V1,LR} + \frac{1712}{243}L_{kk\bar{ii}}^{V1,LR} - \frac{800}{243}L_{dd\bar{iii}}^{V,RR} + \frac{256}{243}L_{ij\bar{j}}^{V,RR} \\
& + \frac{256}{243}L_{ikk}^{V,RR} - \frac{1424}{729}L_{ij\bar{j}}^{V,RR} - \frac{1424}{729}L_{ikk}^{V,RR} - \frac{440}{243}L_{jj11}^{V,LL} - \frac{440}{243}L_{jj22}^{V,LL} \\
& - \frac{440}{243}L_{jj33}^{V,LL} + \frac{3728}{243}L_{11ii}^{V,LR} + \frac{3728}{243}L_{22ii}^{V,LR} + \frac{3728}{243}L_{33ii}^{V,LR} - \frac{104}{243}L_{jj11}^{V,LR} \\
& - \frac{104}{243}L_{jj22}^{V,LR} - \frac{104}{243}L_{jj33}^{V,LR} + \frac{1994}{27}L_{jj\bar{ii}}^{V,LR} - \frac{1024}{243}L_{11ii}^{V,RR} - \frac{1024}{243}L_{22ii}^{V,RR} \\
& - \frac{1024}{243}L_{33ii}^{V,RR} - \frac{80}{9}L_{jjjj}^{V,LL} - \frac{160}{81}L_{jjkk}^{V,LL} - \frac{368}{81}L_{jjjj}^{V,LR} - \frac{184}{81}L_{jjkk}^{V,LR} - \frac{1640}{243}L_{jj11}^{V,LL} \\
& - \frac{1640}{243}L_{jj22}^{V,LL} - \frac{296}{243}L_{jj11}^{V,LR} - \frac{296}{243}L_{jj22}^{V,LR} - \frac{616}{243}L_{ud\bar{11ii}}^{V1,LR} - \frac{616}{243}L_{22ii}^{V1,LR} \\
& - \frac{6952}{243}L_{ud\bar{11ii}}^{V1,RR} - \frac{6952}{243}L_{22ii}^{V1,RR} \Bigg] ;
\end{aligned}$$

$$\begin{aligned}
\dot{L}_{jj\bar{ii}}^{V,LR} & = e^2 \Bigg[ \frac{4}{3}L_{du\bar{11ii}}^{V1,LR} + \frac{4}{3}L_{du\bar{22ii}}^{V1,LR} + \frac{4}{3}L_{du\bar{33ii}}^{V1,LR} - \frac{8}{9}L_{jj11}^{V,LL} - \frac{8}{9}L_{jj22}^{V,LL} \\
& - \frac{8}{9}L_{jj33}^{V,LL} - \frac{8}{9}L_{jj11}^{V,LR} - \frac{8}{9}L_{jj22}^{V,LR} - \frac{8}{9}L_{jj33}^{V,LR} - \frac{16}{3}L_{jjjj}^{V,LL} - \frac{32}{9}L_{jjkk}^{V,LL} \\
& - \frac{16}{9}L_{jjjj}^{V,LR} - \frac{8}{9}L_{jjkk}^{V,LR} + \frac{16}{9}L_{jj11}^{V,LL} + \frac{16}{9}L_{jj22}^{V,LL} + \frac{4}{3}L_{11ii}^{V,LR} + \frac{4}{3}L_{22ii}^{V,LR} \\
& + \frac{4}{3}L_{33ii}^{V,LR} + \frac{16}{9}L_{jj11}^{V,LR} + \frac{16}{9}L_{jj22}^{V,LR} + 8L_{jj\bar{ii}}^{V,LR} + \frac{4}{3}L_{11ii}^{V,RR} + \frac{4}{3}L_{22ii}^{V,RR} \\
& + \frac{4}{3}L_{33ii}^{V,RR} + \frac{4}{3}L_{ii11}^{V1,RR} + \frac{4}{3}L_{ii22}^{V1,RR} + \frac{4}{3}L_{ii33}^{V1,RR} - \frac{8}{3}L_{uu\bar{iii}}^{V1,LR} - \frac{8}{3}L_{kk\bar{ii}}^{V1,LR} \\
& - \frac{64}{9}L_{uu\bar{iii}}^{V,RR} - \frac{16}{3}L_{iikk}^{V,RR} - \frac{16}{9}L_{ikki}^{V,RR} \Bigg] + \alpha_s^2 \Bigg[ -8L_{jj11}^{V,LL} - 8L_{jj22}^{V,LL} \\
& - 8L_{jj33}^{V,LL} + 8L_{jj11}^{V,LR} + 8L_{jj22}^{V,LR} + 8L_{jj33}^{V,LR} - 8L_{jj11}^{V,LL} - 8L_{jj22}^{V,LL} \\
& + 8L_{jj11}^{V,LR} + 8L_{jj22}^{V,LR} \Bigg] + \alpha_s \alpha \Bigg[ \frac{16}{3}L_{du\bar{11ii}}^{V1,LR} + \frac{16}{3}L_{du\bar{22ii}}^{V1,LR} - \frac{32}{3}L_{du\bar{33ii}}^{V1,LR} \\
& - \frac{332}{243}L_{du\bar{11ii}}^{V8,LR} - \frac{332}{243}L_{du\bar{22ii}}^{V8,LR} + \frac{2044}{243}L_{du\bar{33ii}}^{V8,LR} - \frac{32}{9}L_{jj11}^{V,LL} - \frac{32}{9}L_{jj22}^{V,LL} - \frac{32}{9}L_{jj33}^{V,LL}
\end{aligned}$$

$$\begin{aligned}
& -\frac{32}{9}L_{jj11}^{V,LR} - \frac{32}{9}L_{jj22}^{V,LR} - \frac{32}{9}L_{jj33}^{V,LR} + \frac{64}{9}L_{jj11}^{V,LL} + \frac{64}{9}L_{jj22}^{V,LL} + \frac{64}{9}L_{jj11}^{V,LR} \\
& + \frac{64}{9}L_{jj22}^{V,LR} - 32L_{jjii}^{V,LR} + \frac{16}{3}L_{ii11}^{V1,RR} + \frac{16}{3}L_{ii22}^{V1,RR} + \frac{16}{3}L_{ii33}^{V1,RR} + \frac{388}{243}L_{ii11}^{V8,RR} \\
& + \frac{388}{243}L_{ii22}^{V8,RR} + \frac{388}{243}L_{ii33}^{V8,RR} - \frac{32}{3}L_{iii}^{V1,LR} - \frac{32}{3}L_{kkii}^{V1,LR} + \frac{2044}{243}L_{iii}^{V8,LR} + \frac{2044}{243}L_{kkii}^{V8,LR} \\
& - \frac{2096}{81}L_{iii}^{V,RR} - 16L_{ikk}^{V,RR} - \frac{128}{243}L_{ikki}^{V,RR} \Big] + \alpha^2 \Big[ -\frac{1144}{243}L_{11ii}^{V1,LR} - \frac{1144}{243}L_{22ii}^{V1,LR} \\
& + \frac{12512}{243}L_{33ii}^{V1,LR} + \frac{1168}{243}L_{jj11}^{V,LL} + \frac{1168}{243}L_{jj22}^{V,LL} + \frac{1168}{243}L_{jj33}^{V,LL} + \frac{1792}{243}L_{jj11}^{V,LR} \\
& + \frac{1792}{243}L_{jj22}^{V,LR} + \frac{1792}{243}L_{jj33}^{V,LR} + \frac{160}{9}L_{jjj}^{V,ee} + \frac{896}{81}L_{jjkk}^{V,LL} + \frac{3616}{81}L_{jjj}^{V,LR} + \frac{1808}{81}L_{jjkk}^{V,LR} \\
& - \frac{1184}{243}L_{jj11}^{V,LL} - \frac{1184}{243}L_{jj22}^{V,LL} + \frac{3248}{243}L_{jjii}^{V,LR} + \frac{3248}{243}L_{22ii}^{V,LR} + \frac{3248}{243}L_{33ii}^{V,LR} \\
& + \frac{1312}{243}L_{jj11}^{V,LR} + \frac{1312}{243}L_{jj22}^{V,LR} - \frac{4960}{27}L_{jjii}^{V,LR} - \frac{4744}{243}L_{11ii}^{V,RR} - \frac{4744}{243}L_{22ii}^{V,RR} \\
& - \frac{4744}{243}L_{33ii}^{V,RR} - \frac{3808}{243}L_{ii11}^{V1,RR} - \frac{3808}{243}L_{ii22}^{V1,RR} - \frac{3808}{243}L_{ii33}^{V1,RR} + \frac{12224}{243}L_{iii}^{V1,LR} \\
& + \frac{12224}{243}L_{kkii}^{V1,LR} + \frac{3808}{243}L_{iii}^{V,RR} + \frac{3136}{243}L_{ikk}^{V,RR} + \frac{1024}{729}L_{ikki}^{V,RR} \Big] ;
\end{aligned}$$

$$\begin{aligned}
\dot{L}_{jjii}^{V1,LR} = & -\frac{8}{3}L_{jjii}^{V8,LR}g_s^2 + e^2 \Big[ -\frac{8}{9}L_{dd}^{V1,LR} - \frac{8}{9}L_{jjii}^{V1,LR} - \frac{8}{9}L_{kkii}^{V1,LR} - \frac{64}{27}L_{iii}^{V,RR} \\
& - \frac{16}{9}L_{dd}^{V,RR} - \frac{16}{9}L_{ikk}^{V,RR} - \frac{16}{27}L_{ijji}^{V,RR} - \frac{16}{27}L_{ikki}^{V,RR} - \frac{8}{9}L_{11ii}^{V,LR} - \frac{8}{9}L_{22ii}^{V,LR} \\
& - \frac{8}{9}L_{33ii}^{V,LR} - \frac{8}{9}L_{11ii}^{V,RR} - \frac{8}{9}L_{22ii}^{V,RR} - \frac{8}{9}L_{33ii}^{V,RR} + \frac{4}{9}L_{11jj}^{V,LL} + \frac{4}{9}L_{22jj}^{V,LL} \\
& + \frac{4}{9}L_{33jj}^{V,LL} + \frac{4}{9}L_{jj11}^{V1,LL} + \frac{4}{9}L_{jj22}^{V1,LL} + \frac{4}{9}L_{jj33}^{V1,LL} + \frac{16}{9}L_{11ii}^{V1,LR} + \frac{16}{9}L_{22ii}^{V1,LR} \\
& + \frac{4}{9}L_{jj11}^{V1,LR} + \frac{4}{9}L_{jj22}^{V1,LR} + \frac{4}{9}L_{jj33}^{V1,LR} + \frac{8}{3}L_{jjii}^{V1,LR} + \frac{16}{9}L_{11ii}^{V1,RR} + \frac{16}{9}L_{22ii}^{V1,RR} \\
& + \frac{4}{9}L_{jj11}^{V,LR} + \frac{4}{9}L_{jj22}^{V,LR} + \frac{4}{9}L_{jj33}^{V,LR} - \frac{8}{9}L_{jjj}^{V1,LR} - \frac{8}{9}L_{jjkk}^{V1,LR} - \frac{64}{27}L_{jjj}^{V,LL} \\
& - \frac{16}{9}L_{jjkk}^{V,LL} - \frac{16}{27}L_{jjkj}^{V,LL} \Big] + \alpha_s^2 \Big[ 8L_{iii}^{V1,LR} + 8L_{jjii}^{V1,LR} + 8L_{kkii}^{V1,LR}
\end{aligned}$$

$$\begin{aligned}
& + \frac{44}{27} L_{\bar{u}\bar{u}\bar{u}}^{V8,LR} + \frac{44}{27} L_{\bar{u}\bar{u}\bar{u}}^{V8,LR} + \frac{44}{27} L_{\bar{u}\bar{u}\bar{u}}^{V8,LR} - \frac{232}{9} L_{\bar{u}\bar{u}\bar{u}}^{V,RR} - 16 L_{\bar{u}\bar{u}\bar{u}}^{V,RR} - 16 L_{\bar{u}\bar{u}\bar{u}}^{V,RR} \\
& - \frac{64}{27} L_{\bar{u}\bar{u}\bar{u}}^{V,RR} - \frac{64}{27} L_{\bar{u}\bar{u}\bar{u}}^{V,RR} - 8 L_{\bar{u}\bar{u}\bar{u}}^{V1,LL} - 8 L_{\bar{u}\bar{u}\bar{u}}^{V1,LL} - 8 L_{\bar{u}\bar{u}\bar{u}}^{V1,LL} + 8 L_{\bar{u}\bar{u}\bar{u}}^{V1,LR} \\
& + 8 L_{\bar{u}\bar{u}\bar{u}}^{V1,LR} + 8 L_{\bar{u}\bar{u}\bar{u}}^{V1,LR} + 8 L_{\bar{u}\bar{u}\bar{u}}^{V1,LR} + 8 L_{\bar{u}\bar{u}\bar{u}}^{V1,LR} - \frac{28}{3} L_{\bar{u}\bar{u}\bar{u}}^{V1,LR} - 8 L_{\bar{u}\bar{u}\bar{u}}^{V1,RR} \\
& - 8 L_{\bar{u}\bar{u}\bar{u}}^{V1,RR} + \frac{44}{27} L_{\bar{u}\bar{u}\bar{u}}^{V8,LL} + \frac{44}{27} L_{\bar{u}\bar{u}\bar{u}}^{V8,LL} + \frac{44}{27} L_{\bar{u}\bar{u}\bar{u}}^{V8,LL} + \frac{44}{27} L_{\bar{u}\bar{u}\bar{u}}^{V8,LL} + \frac{44}{27} L_{\bar{u}\bar{u}\bar{u}}^{V8,LR} + \frac{44}{27} L_{\bar{u}\bar{u}\bar{u}}^{V8,LR} \\
& + \frac{44}{27} L_{\bar{u}\bar{u}\bar{u}}^{V8,LR} + \frac{44}{27} L_{\bar{u}\bar{u}\bar{u}}^{V8,LR} + \frac{44}{27} L_{\bar{u}\bar{u}\bar{u}}^{V8,LR} - \frac{2044}{27} L_{\bar{u}\bar{u}\bar{u}}^{V8,LR} + \frac{44}{27} L_{\bar{u}\bar{u}\bar{u}}^{V8,RR} + \frac{44}{27} L_{\bar{u}\bar{u}\bar{u}}^{V8,RR} \\
& + 8 L_{\bar{u}\bar{u}\bar{u}}^{V1,LR} + 8 L_{\bar{u}\bar{u}\bar{u}}^{V1,LR} + \frac{44}{27} L_{\bar{u}\bar{u}\bar{u}}^{V8,LR} + \frac{44}{27} L_{\bar{u}\bar{u}\bar{u}}^{V8,LR} - \frac{232}{9} L_{\bar{u}\bar{u}\bar{u}}^{V,LL} - 16 L_{\bar{u}\bar{u}\bar{u}}^{V,LL} \\
& - \frac{64}{27} L_{\bar{u}\bar{u}\bar{u}}^{V,LL} \Big] + \alpha_s \alpha \Big[ - \frac{32}{9} L_{\bar{u}\bar{u}\bar{u}}^{V1,LR} - \frac{32}{9} L_{\bar{u}\bar{u}\bar{u}}^{V1,LR} - \frac{32}{9} L_{\bar{u}\bar{u}\bar{u}}^{V1,LR} + \frac{2080}{729} L_{\bar{u}\bar{u}\bar{u}}^{V8,LR} \\
& + \frac{2080}{729} L_{\bar{u}\bar{u}\bar{u}}^{V8,LR} + \frac{2080}{729} L_{\bar{u}\bar{u}\bar{u}}^{V8,LR} - \frac{2048}{243} L_{\bar{u}\bar{u}\bar{u}}^{V,RR} - \frac{16}{3} L_{\bar{u}\bar{u}\bar{u}}^{V,RR} - \frac{16}{3} L_{\bar{u}\bar{u}\bar{u}}^{V,RR} + \frac{16}{729} L_{\bar{u}\bar{u}\bar{u}}^{V,RR} \\
& + \frac{16}{729} L_{\bar{u}\bar{u}\bar{u}}^{V,RR} + \frac{16}{9} L_{\bar{u}\bar{u}\bar{u}}^{V1,LL} + \frac{16}{9} L_{\bar{u}\bar{u}\bar{u}}^{V1,LL} + \frac{16}{9} L_{\bar{u}\bar{u}\bar{u}}^{V1,LL} + \frac{16}{9} L_{\bar{u}\bar{u}\bar{u}}^{V1,LL} + \frac{64}{9} L_{\bar{u}\bar{u}\bar{u}}^{V1,LR} + \frac{64}{9} L_{\bar{u}\bar{u}\bar{u}}^{V1,LR} \\
& + \frac{16}{9} L_{\bar{u}\bar{u}\bar{u}}^{V1,LR} + \frac{16}{9} L_{\bar{u}\bar{u}\bar{u}}^{V1,LR} - \frac{32}{9} L_{\bar{u}\bar{u}\bar{u}}^{V1,LR} - \frac{64}{3} L_{\bar{u}\bar{u}\bar{u}}^{V1,LR} + \frac{64}{9} L_{\bar{u}\bar{u}\bar{u}}^{V1,RR} + \frac{64}{9} L_{\bar{u}\bar{u}\bar{u}}^{V1,RR} \\
& + \frac{388}{729} L_{\bar{u}\bar{u}\bar{u}}^{V8,LL} + \frac{388}{729} L_{\bar{u}\bar{u}\bar{u}}^{V8,LL} + \frac{388}{729} L_{\bar{u}\bar{u}\bar{u}}^{V8,LL} - \frac{2672}{729} L_{\bar{u}\bar{u}\bar{u}}^{V8,LR} - \frac{2672}{729} L_{\bar{u}\bar{u}\bar{u}}^{V8,LR} \\
& - \frac{332}{729} L_{\bar{u}\bar{u}\bar{u}}^{V8,LR} - \frac{332}{729} L_{\bar{u}\bar{u}\bar{u}}^{V8,LR} + \frac{2044}{729} L_{\bar{u}\bar{u}\bar{u}}^{V8,LR} + \frac{232}{27} L_{\bar{u}\bar{u}\bar{u}}^{V8,LR} + \frac{208}{729} L_{\bar{u}\bar{u}\bar{u}}^{V8,RR} \\
& + \frac{208}{729} L_{\bar{u}\bar{u}\bar{u}}^{V8,RR} - \frac{32}{9} L_{\bar{u}\bar{u}\bar{u}}^{V1,LR} - \frac{32}{9} L_{\bar{u}\bar{u}\bar{u}}^{V1,LR} + \frac{2044}{729} L_{\bar{u}\bar{u}\bar{u}}^{V8,LR} + \frac{2044}{729} L_{\bar{u}\bar{u}\bar{u}}^{V8,LR} \\
& - \frac{2096}{243} L_{\bar{u}\bar{u}\bar{u}}^{V,LL} - \frac{16}{3} L_{\bar{u}\bar{u}\bar{u}}^{V,LL} - \frac{128}{729} L_{\bar{u}\bar{u}\bar{u}}^{V,LL} \Big] + \alpha^2 \Big[ \frac{3776}{729} L_{\bar{u}\bar{u}\bar{u}}^{V1,LR} + \frac{3776}{729} L_{\bar{u}\bar{u}\bar{u}}^{V1,LR} \\
& + \frac{3776}{729} L_{\bar{u}\bar{u}\bar{u}}^{V1,LR} + \frac{880}{729} L_{\bar{u}\bar{u}\bar{u}}^{V,RR} + \frac{928}{729} L_{\bar{u}\bar{u}\bar{u}}^{V,RR} + \frac{928}{729} L_{\bar{u}\bar{u}\bar{u}}^{V,RR} - \frac{32}{2187} L_{\bar{u}\bar{u}\bar{u}}^{V,RR} \\
& - \frac{32}{2187} L_{\bar{u}\bar{u}\bar{u}}^{V,RR} + \frac{6224}{729} L_{\bar{u}\bar{u}\bar{u}}^{V,LR} + \frac{6224}{729} L_{\bar{u}\bar{u}\bar{u}}^{V,LR} + \frac{6224}{729} L_{\bar{u}\bar{u}\bar{u}}^{V,LR} - \frac{3712}{729} L_{\bar{u}\bar{u}\bar{u}}^{V,RR} \\
& - \frac{3712}{729} L_{\bar{u}\bar{u}\bar{u}}^{V,RR} - \frac{3712}{729} L_{\bar{u}\bar{u}\bar{u}}^{V,RR} - \frac{1216}{729} L_{\bar{u}\bar{u}\bar{u}}^{V,LL} - \frac{1216}{729} L_{\bar{u}\bar{u}\bar{u}}^{V,LL} - \frac{1216}{729} L_{\bar{u}\bar{u}\bar{u}}^{V,LL} \\
& - \frac{1576}{729} L_{\bar{u}\bar{u}\bar{u}}^{V1,LL} - \frac{1576}{729} L_{\bar{u}\bar{u}\bar{u}}^{V1,LL} - \frac{1576}{729} L_{\bar{u}\bar{u}\bar{u}}^{V1,LL} + \frac{6272}{729} L_{\bar{u}\bar{u}\bar{u}}^{V1,LR} + \frac{6272}{729} L_{\bar{u}\bar{u}\bar{u}}^{V1,LR}
\end{aligned}$$

$$\begin{aligned}
& -\frac{208}{729}L_{\frac{ud}{jj11}}^{V1,LR} - \frac{208}{729}L_{\frac{ud}{jj22}}^{V1,LR} + \frac{6752}{729}L_{\frac{ud}{jj33}}^{V1,LR} - \frac{4048}{81}L_{\frac{ud}{jjii}}^{V1,LR} - \frac{6976}{729}L_{\frac{ud}{11ii}}^{V1,RR} \\
& - \frac{6976}{729}L_{\frac{ud}{22ii}}^{V1,RR} + \frac{2888}{729}L_{\frac{ue}{jj11}}^{V,LR} + \frac{2888}{729}L_{\frac{ue}{jj22}}^{V,LR} + \frac{2888}{729}L_{\frac{ue}{jj33}}^{V,LR} + \frac{6464}{729}L_{\frac{uu}{jjjj}}^{V1,LR} \\
& + \frac{6464}{729}L_{\frac{uu}{jjkk}}^{V1,LR} + \frac{4384}{729}L_{\frac{uu}{jjjj}}^{V,LL} + \frac{1984}{729}L_{\frac{uu}{jjkk}}^{V,LL} + \frac{3328}{2187}L_{\frac{uu}{jjkk}}^{V,LL} \Bigg];
\end{aligned}$$

$$\begin{aligned}
\dot{L}_{\frac{ud}{jjii}}^{V8,LR} &= g_s^2 \left[ \frac{2}{3}L_{\frac{dd}{iii}}^{V8,LR} + \frac{2}{3}L_{\frac{dd}{jjii}}^{V8,LR} + \frac{2}{3}L_{\frac{dd}{kkii}}^{V8,LR} + \frac{8}{3}L_{\frac{dd}{iii}}^{V,RR} + \frac{8}{3}L_{\frac{dd}{ijji}}^{V,RR} \right. \\
& + \frac{8}{3}L_{\frac{dd}{ikkii}}^{V,RR} - 12L_{\frac{ud}{jjii}}^{V1,LR} + \frac{2}{3}L_{\frac{ud}{jj11}}^{V8,LL} + \frac{2}{3}L_{\frac{ud}{jj22}}^{V8,LL} + \frac{2}{3}L_{\frac{ud}{jj33}}^{V8,LL} + \frac{2}{3}L_{\frac{ud}{11ii}}^{V8,LR} \\
& + \frac{2}{3}L_{\frac{ud}{22ii}}^{V8,LR} + \frac{2}{3}L_{\frac{ud}{jj11}}^{V8,LR} + \frac{2}{3}L_{\frac{ud}{jj22}}^{V8,LR} + \frac{2}{3}L_{\frac{ud}{jj33}}^{V8,LR} - 14L_{\frac{ud}{jjii}}^{V8,LR} + \frac{2}{3}L_{\frac{ud}{11ii}}^{V8,RR} \\
& \left. + \frac{2}{3}L_{\frac{ud}{22ii}}^{V8,RR} + \frac{2}{3}L_{\frac{uu}{jjjj}}^{V8,LR} + \frac{2}{3}L_{\frac{uu}{jjkk}}^{V8,LR} + \frac{8}{3}L_{\frac{uu}{jjjj}}^{V,LL} + \frac{8}{3}L_{\frac{uu}{jjkk}}^{V,LL} \right] + \frac{8}{3}L_{\frac{ud}{jjii}}^{V8,LR} \\
& e^2 + \alpha_s^2 \left[ -\frac{22}{3}L_{\frac{dd}{iii}}^{V1,LR} - \frac{22}{3}L_{\frac{dd}{jjii}}^{V1,LR} - \frac{22}{3}L_{\frac{dd}{kkii}}^{V1,LR} + \frac{769}{81}L_{\frac{dd}{iii}}^{V8,LR} + \frac{769}{81}L_{\frac{dd}{jjii}}^{V8,LR} \right. \\
& + \frac{769}{81}L_{\frac{dd}{kkii}}^{V8,LR} + \frac{1174}{27}L_{\frac{dd}{iii}}^{V,RR} - \frac{28}{3}L_{\frac{dd}{ijji}}^{V,RR} - \frac{28}{3}L_{\frac{dd}{iikk}}^{V,RR} + \frac{3376}{81}L_{\frac{dd}{ijji}}^{V,RR} + \frac{3376}{81}L_{\frac{dd}{ikkii}}^{V,RR} \\
& - \frac{2}{3}L_{\frac{ud}{jj11}}^{V1,LL} - \frac{2}{3}L_{\frac{ud}{jj22}}^{V1,LL} - \frac{2}{3}L_{\frac{ud}{jj33}}^{V1,LL} - \frac{22}{3}L_{\frac{ud}{11ii}}^{V1,LR} - \frac{22}{3}L_{\frac{ud}{22ii}}^{V1,LR} - \frac{22}{3}L_{\frac{ud}{jj11}}^{V1,LR} \\
& - \frac{22}{3}L_{\frac{ud}{jj22}}^{V1,LR} - \frac{22}{3}L_{\frac{ud}{jj33}}^{V1,LR} - \frac{374}{3}L_{\frac{ud}{jjii}}^{V1,LR} - \frac{2}{3}L_{\frac{ud}{11ii}}^{V1,RR} - \frac{2}{3}L_{\frac{ud}{22ii}}^{V1,RR} + \frac{607}{81}L_{\frac{ud}{jj11}}^{V8,LL} \\
& + \frac{607}{81}L_{\frac{ud}{jj22}}^{V8,LL} + \frac{607}{81}L_{\frac{ud}{jj33}}^{V8,LL} + \frac{769}{81}L_{\frac{ud}{11ii}}^{V8,LR} + \frac{769}{81}L_{\frac{ud}{22ii}}^{V8,LR} + \frac{787}{81}L_{\frac{ud}{jj11}}^{V8,LR} + \frac{787}{81}L_{\frac{ud}{jj22}}^{V8,LR} \\
& + \frac{787}{81}L_{\frac{ud}{jj33}}^{V8,LR} - \frac{2975}{18}L_{\frac{ud}{jjii}}^{V8,LR} + \frac{589}{81}L_{\frac{ud}{11ii}}^{V8,RR} + \frac{589}{81}L_{\frac{ud}{22ii}}^{V8,RR} - \frac{22}{3}L_{\frac{uu}{jjjj}}^{V1,LR} - \frac{22}{3}L_{\frac{uu}{jjkk}}^{V1,LR} \\
& \left. + \frac{787}{81}L_{\frac{uu}{jjjj}}^{V8,LR} + \frac{787}{81}L_{\frac{uu}{jjkk}}^{V8,LR} + \frac{1198}{27}L_{\frac{uu}{jjjj}}^{V,LL} - \frac{28}{3}L_{\frac{uu}{jjkk}}^{V,LL} + \frac{3448}{81}L_{\frac{uu}{jjkk}}^{V,LL} \right] \\
& + \alpha_s \alpha \left[ -\frac{916}{81}L_{\frac{dd}{iii}}^{V1,LR} - \frac{916}{81}L_{\frac{dd}{jjii}}^{V1,LR} - \frac{916}{81}L_{\frac{dd}{kkii}}^{V1,LR} - \frac{44}{9}L_{\frac{dd}{iii}}^{V8,LR} - \frac{44}{9}L_{\frac{dd}{jjii}}^{V8,LR} \right. \\
& - \frac{44}{9}L_{\frac{dd}{kkii}}^{V8,LR} - \frac{2144}{81}L_{\frac{dd}{iii}}^{V,RR} - \frac{1832}{81}L_{\frac{dd}{ijji}}^{V,RR} - \frac{1832}{81}L_{\frac{dd}{iikk}}^{V,RR} + \frac{664}{243}L_{\frac{dd}{ijji}}^{V,RR} + \frac{664}{243}L_{\frac{dd}{ikkii}}^{V,RR}
\end{aligned}$$

$$\begin{aligned}
& -\frac{916}{81}L_{11ii}^{V,LR} - \frac{916}{81}L_{22ii}^{V,LR} - \frac{916}{81}L_{33ii}^{V,LR} - \frac{916}{81}L_{11ii}^{V,RR} - \frac{916}{81}L_{22ii}^{V,RR} - \frac{916}{81}L_{33ii}^{V,RR} \\
& + \frac{644}{81}L_{11jj}^{V,LL} + \frac{644}{81}L_{22jj}^{V,LL} + \frac{644}{81}L_{33jj}^{V,LL} + \frac{644}{81}L_{jj11}^{V1,LL} + \frac{644}{81}L_{jj22}^{V1,LL} + \frac{644}{81}L_{jj33}^{V1,LL} \\
& + \frac{1832}{81}L_{11ii}^{V1,LR} + \frac{1832}{81}L_{22ii}^{V1,LR} + \frac{644}{81}L_{jj11}^{V1,LR} + \frac{644}{81}L_{jj22}^{V1,LR} - \frac{1216}{81}L_{jj33}^{V1,LR} \\
& + \frac{116}{3}L_{jjii}^{V1,LR} + \frac{1832}{81}L_{11ii}^{V1,RR} + \frac{1832}{81}L_{22ii}^{V1,RR} - \frac{70}{27}L_{jj11}^{V8,LL} - \frac{70}{27}L_{jj22}^{V8,LL} - \frac{70}{27}L_{jj33}^{V8,LL} \\
& + \frac{56}{9}L_{11ii}^{V8,LR} + \frac{56}{9}L_{22ii}^{V8,LR} + \frac{14}{9}L_{jj11}^{V8,LR} + \frac{14}{9}L_{jj22}^{V8,LR} - \frac{20}{3}L_{jj33}^{V8,LR} + \frac{187}{9}L_{jjii}^{V8,LR} \\
& - \frac{160}{27}L_{11ii}^{V8,RR} - \frac{160}{27}L_{22ii}^{V8,RR} + \frac{644}{81}L_{jj11}^{V,LR} + \frac{644}{81}L_{jj22}^{V,LR} + \frac{644}{81}L_{jj33}^{V,LR} - \frac{1288}{81}L_{jjjj}^{V1,LR} \\
& - \frac{1288}{81}L_{jjkk}^{V1,LR} - \frac{20}{3}L_{jjjj}^{V8,LR} - \frac{20}{3}L_{jjkk}^{V8,LR} - \frac{3608}{81}L_{jjjj}^{V,LL} - \frac{2576}{81}L_{jjkk}^{V,LL} - \frac{800}{243}L_{jjkk}^{V,LL} \Big] \\
& - \frac{4048}{81}L_{jjii}^{V8,LR}\alpha^2;
\end{aligned}$$

$$\begin{aligned}
\dot{L}_{jjii}^{V1,LR} = & -\frac{8}{3}L_{jjii}^{V8,LR}g_s^2 + e^2 \Big[ \frac{4}{9}L_{iii}^{V1,LR} - \frac{8}{9}L_{jjii}^{V1,LR} + \frac{8}{9}L_{jjjj}^{V1,LR} + \frac{4}{9}L_{jjkk}^{V1,LR} \\
& + \frac{4}{9}L_{kkii}^{V1,LR} + \frac{64}{27}L_{jjjj}^{V,LL} + \frac{8}{9}L_{jjkk}^{V,LL} + \frac{8}{27}L_{jjkk}^{V,LL} + \frac{32}{27}L_{iii}^{V,RR} + \frac{8}{9}L_{jjj}^{V,RR} \\
& + \frac{8}{9}L_{iikk}^{V,RR} + \frac{8}{27}L_{jjji}^{V,RR} + \frac{8}{27}L_{ikki}^{V,RR} + \frac{4}{9}L_{jj11}^{V,LR} + \frac{4}{9}L_{jj22}^{V,LR} + \frac{4}{9}L_{jj33}^{V,LR} \\
& - \frac{8}{9}L_{jj11}^{V1,LR} - \frac{8}{9}L_{jj22}^{V1,LR} + \frac{4}{9}L_{11jj}^{V,LL} + \frac{4}{9}L_{22jj}^{V,LL} + \frac{4}{9}L_{33jj}^{V,LL} + \frac{4}{9}L_{11ii}^{V,LR} \\
& + \frac{4}{9}L_{22ii}^{V,LR} + \frac{4}{9}L_{33ii}^{V,LR} + \frac{4}{9}L_{11ii}^{V,RR} + \frac{4}{9}L_{22ii}^{V,RR} + \frac{4}{9}L_{33ii}^{V,RR} - \frac{8}{9}L_{11jj}^{V1,LL} \\
& - \frac{8}{9}L_{22jj}^{V1,LL} - \frac{8}{9}L_{11ii}^{V1,LR} - \frac{8}{9}L_{22ii}^{V1,LR} - \frac{8}{9}L_{11ii}^{V1,RR} - \frac{8}{9}L_{22ii}^{V1,RR} \Big] + \alpha_s^2 \Big[ 8L_{iii}^{V1,LR} \\
& - \frac{4}{3}L_{jjii}^{V1,LR} + 16L_{jjjj}^{V1,LR} + 8L_{jjkk}^{V1,LR} + 8L_{kkii}^{V1,LR} + \frac{44}{27}L_{iii}^{V8,LR} - \frac{2000}{27}L_{jjii}^{V8,LR} \\
& + \frac{88}{27}L_{jjjj}^{V8,LR} + \frac{44}{27}L_{jjkk}^{V8,LR} + \frac{44}{27}L_{kkii}^{V8,LR} - \frac{1192}{27}L_{jjjj}^{V,LL} - 16L_{jjkk}^{V,LL} - \frac{64}{27}L_{jjkk}^{V,LL} \\
& - \frac{232}{9}L_{iii}^{V,RR} - 16L_{jjj}^{V,RR} - 16L_{iikk}^{V,RR} - \frac{64}{27}L_{jjji}^{V,RR} - \frac{64}{27}L_{ikki}^{V,RR} + 8L_{jj11}^{V1,LR}
\end{aligned}$$

$$\begin{aligned}
& + 8L_{jj22}^{V1,LR} + \frac{44}{27}L_{jj11}^{V8,LR} + \frac{44}{27}L_{jj22}^{V8,LR} - 8L_{11jj}^{V1,LL} - 8L_{22jj}^{V1,LL} + 8L_{11ii}^{V1,LR} \\
& + 8L_{22ii}^{V1,LR} - 8L_{11ii}^{V1,RR} - 8L_{22ii}^{V1,RR} + \frac{44}{27}L_{11jj}^{V8,LL} + \frac{44}{27}L_{22jj}^{V8,LL} + \frac{44}{27}L_{11ii}^{V8,LR} \\
& + \frac{44}{27}L_{22ii}^{V8,LR} + \frac{44}{27}L_{11ii}^{V8,RR} + \frac{44}{27}L_{22ii}^{V8,RR} \Big] + \alpha_s \alpha \Big[ \frac{16}{9}L_{iii}^{V1,LR} + \frac{112}{9}L_{jji}^{V1,LR} \\
& + \frac{32}{9}L_{jjj}^{V1,LR} + \frac{16}{9}L_{jjk}^{V1,LR} + \frac{16}{9}L_{kji}^{V1,LR} - \frac{1040}{729}L_{iii}^{V8,LR} - \frac{1256}{729}L_{jji}^{V8,LR} - \frac{2080}{729}L_{jjj}^{V8,LR} \\
& - \frac{1040}{729}L_{jjk}^{V8,LR} - \frac{1040}{729}L_{kji}^{V8,LR} + \frac{5008}{729}L_{jjj}^{V,LL} + \frac{8}{3}L_{jjk}^{V,LL} - \frac{8}{729}L_{jjk}^{V,LL} + \frac{1024}{243}L_{iii}^{V,RR} \\
& + \frac{8}{3}L_{iij}^{V,RR} + \frac{8}{3}L_{ikk}^{V,RR} - \frac{8}{729}L_{iij}^{V,RR} - \frac{8}{729}L_{ikk}^{V,RR} - \frac{32}{9}L_{jj11}^{V1,LR} - \frac{32}{9}L_{jj22}^{V1,LR} \\
& + \frac{1336}{729}L_{jj11}^{V8,LR} + \frac{1336}{729}L_{jj22}^{V8,LR} - \frac{32}{9}L_{11jj}^{V1,LL} - \frac{32}{9}L_{22jj}^{V1,LL} - \frac{32}{9}L_{11ii}^{V1,LR} - \frac{32}{9}L_{22ii}^{V1,LR} \\
& - \frac{32}{9}L_{11ii}^{V1,RR} - \frac{32}{9}L_{22ii}^{V1,RR} - \frac{104}{729}L_{11jj}^{V8,LL} - \frac{104}{729}L_{22jj}^{V8,LL} + \frac{1336}{729}L_{11ii}^{V8,LR} + \frac{1336}{729}L_{22ii}^{V8,LR} \\
& - \frac{104}{729}L_{11ii}^{V8,RR} - \frac{104}{729}L_{22ii}^{V8,RR} \Big] + \alpha^2 \Big[ \frac{272}{729}L_{iii}^{V1,LR} + \frac{16382}{729}L_{jji}^{V1,LR} + \frac{544}{729}L_{jjj}^{V1,LR} \\
& + \frac{272}{729}L_{jjk}^{V1,LR} + \frac{272}{729}L_{kji}^{V1,LR} - \frac{2912}{2187}L_{jjj}^{V,LL} - \frac{32}{729}L_{jjk}^{V,LL} - \frac{848}{2187}L_{jjk}^{V,LL} \\
& - \frac{656}{729}L_{iii}^{V,RR} - \frac{32}{729}L_{iij}^{V,RR} - \frac{32}{729}L_{ikk}^{V,RR} - \frac{848}{2187}L_{iij}^{V,RR} - \frac{848}{2187}L_{ikk}^{V,RR} + \frac{992}{729}L_{jj11}^{V,LR} \\
& + \frac{992}{729}L_{jj22}^{V,LR} + \frac{992}{729}L_{jj33}^{V,LR} - \frac{1624}{729}L_{jj11}^{V1,LR} - \frac{1624}{729}L_{jj22}^{V1,LR} + \frac{128}{729}L_{11jj}^{V,LL} \\
& + \frac{128}{729}L_{22jj}^{V,LL} + \frac{128}{729}L_{33jj}^{V,LL} + \frac{992}{729}L_{11ii}^{V,LR} + \frac{992}{729}L_{22ii}^{V,LR} + \frac{992}{729}L_{33ii}^{V,LR} + \frac{128}{729}L_{11ii}^{V,RR} \\
& + \frac{128}{729}L_{22ii}^{V,RR} + \frac{128}{729}L_{33ii}^{V,RR} - \frac{2776}{729}L_{11jj}^{V1,LL} - \frac{2776}{729}L_{22jj}^{V1,LL} - \frac{1624}{729}L_{11ii}^{V1,LR} \\
& - \frac{1624}{729}L_{22ii}^{V1,LR} - \frac{2776}{729}L_{11ii}^{V1,RR} - \frac{2776}{729}L_{22ii}^{V1,RR} \Big] ;
\end{aligned}$$

$$\begin{aligned}
\dot{L}_{jjii}^{V8,LR} &= g_s^2 \Big[ -12L_{jjii}^{V1,LR} + \frac{2}{3}L_{iii}^{V8,LR} - \frac{40}{3}L_{jjii}^{V8,LR} + \frac{4}{3}L_{jjjj}^{V8,LR} + \frac{2}{3}L_{jjkk}^{V8,LR} \\
& + \frac{2}{3}L_{kkii}^{V8,LR} + \frac{16}{3}L_{jjjj}^{V,LL} + \frac{8}{3}L_{jjk}^{V,LL} + \frac{8}{3}L_{iij}^{V,RR} + \frac{8}{3}L_{jjj}^{V,RR} + \frac{8}{3}L_{ikk}^{V,RR}
\end{aligned}$$



$$\begin{aligned}
& + \frac{2}{3}L_{\frac{du}{jj11}}^{V8,LR} + \frac{2}{3}L_{\frac{du}{jj22}}^{V8,LR} + \frac{2}{3}L_{\frac{ud}{11jj}}^{V8,LL} + \frac{2}{3}L_{\frac{ud}{22jj}}^{V8,LL} + \frac{2}{3}L_{\frac{ud}{11ii}}^{V8,LR} + \frac{2}{3}L_{\frac{ud}{22ii}}^{V8,LR} \\
& + \frac{2}{3}L_{\frac{ud}{11ii}}^{V8,RR} + \frac{2}{3}L_{\frac{ud}{22ii}}^{V8,RR} \Big] - \frac{4}{3}L_{\frac{dd}{jjii}}^{V8,LR}e^2 + \alpha_s^2 \Big[ -\frac{22}{3}L_{\frac{dd}{iii}}^{V1,LR} - 132L_{\frac{dd}{jjii}}^{V1,LR} \\
& - \frac{44}{3}L_{\frac{dd}{jjjj}}^{V1,LR} - \frac{22}{3}L_{\frac{dd}{jjkk}}^{V1,LR} - \frac{22}{3}L_{\frac{dd}{kkii}}^{V1,LR} + \frac{769}{81}L_{\frac{dd}{iii}}^{V8,LR} - \frac{25237}{162}L_{\frac{dd}{jjii}}^{V8,LR} + \frac{1538}{81}L_{\frac{dd}{jjjj}}^{V8,LR} \\
& + \frac{769}{81}L_{\frac{dd}{jjkk}}^{V8,LR} + \frac{769}{81}L_{\frac{dd}{kkii}}^{V8,LR} + \frac{6142}{81}L_{\frac{dd}{jjjj}}^{V,LL} - \frac{28}{3}L_{\frac{dd}{jjkk}}^{V,LL} + \frac{3376}{81}L_{\frac{dd}{jjkk}}^{V,LL} + \frac{1174}{27}L_{\frac{dd}{iii}}^{V,RR} \\
& - \frac{28}{3}L_{\frac{dd}{iijj}}^{V,RR} - \frac{28}{3}L_{\frac{dd}{iikk}}^{V,RR} + \frac{3376}{81}L_{\frac{dd}{ijji}}^{V,RR} + \frac{3376}{81}L_{\frac{dd}{ikki}}^{V,RR} - \frac{22}{3}L_{\frac{du}{jj11}}^{V1,LR} - \frac{22}{3}L_{\frac{du}{jj22}}^{V1,LR} \\
& + \frac{769}{81}L_{\frac{du}{jj11}}^{V8,LR} + \frac{769}{81}L_{\frac{du}{jj22}}^{V8,LR} - \frac{2}{3}L_{\frac{ud}{11jj}}^{V1,LL} - \frac{2}{3}L_{\frac{ud}{22jj}}^{V1,LL} - \frac{22}{3}L_{\frac{ud}{11ii}}^{V1,LR} - \frac{22}{3}L_{\frac{ud}{22ii}}^{V1,LR} \\
& - \frac{2}{3}L_{\frac{ud}{11ii}}^{V1,RR} - \frac{2}{3}L_{\frac{ud}{22ii}}^{V1,RR} + \frac{589}{81}L_{\frac{ud}{11jj}}^{V8,LL} + \frac{589}{81}L_{\frac{ud}{22jj}}^{V8,LL} + \frac{769}{81}L_{\frac{ud}{11ii}}^{V8,LR} + \frac{769}{81}L_{\frac{ud}{22ii}}^{V8,LR} \\
& + \frac{589}{81}L_{\frac{ud}{11ii}}^{V8,RR} + \frac{589}{81}L_{\frac{ud}{22ii}}^{V8,RR} \Big] + \alpha_s\alpha \Big[ \frac{272}{81}L_{\frac{dd}{iii}}^{V1,LR} + \frac{164}{81}L_{\frac{dd}{jjii}}^{V1,LR} + \frac{544}{81}L_{\frac{dd}{jjjj}}^{V1,LR} \\
& + \frac{272}{81}L_{\frac{dd}{jjkk}}^{V1,LR} + \frac{272}{81}L_{\frac{dd}{kkii}}^{V1,LR} + \frac{14}{9}L_{\frac{dd}{iii}}^{V8,LR} - \frac{4}{3}L_{\frac{dd}{jjii}}^{V8,LR} + \frac{28}{9}L_{\frac{dd}{jjjj}}^{V8,LR} + \frac{14}{9}L_{\frac{dd}{jjkk}}^{V8,LR} \\
& + \frac{14}{9}L_{\frac{dd}{kkii}}^{V8,LR} + \frac{1588}{243}L_{\frac{dd}{jjjj}}^{V,LL} + \frac{544}{81}L_{\frac{dd}{jjkk}}^{V,LL} - \frac{1064}{243}L_{\frac{dd}{jjkk}}^{V,LL} + \frac{340}{81}L_{\frac{dd}{iii}}^{V,RR} + \frac{544}{81}L_{\frac{dd}{iijj}}^{V,RR} \\
& + \frac{544}{81}L_{\frac{dd}{iikk}}^{V,RR} - \frac{1064}{243}L_{\frac{dd}{ijji}}^{V,RR} - \frac{1064}{243}L_{\frac{dd}{ikki}}^{V,RR} + \frac{272}{81}L_{\frac{de}{jj11}}^{V,LR} + \frac{272}{81}L_{\frac{de}{jj22}}^{V,LR} + \frac{272}{81}L_{\frac{de}{jj33}}^{V,LR} \\
& - \frac{544}{81}L_{\frac{du}{jj11}}^{V1,LR} - \frac{544}{81}L_{\frac{du}{jj22}}^{V1,LR} + \frac{2}{3}L_{\frac{du}{jj11}}^{V8,LR} + \frac{2}{3}L_{\frac{du}{jj22}}^{V8,LR} + \frac{272}{81}L_{\frac{ed}{11jj}}^{V,LL} + \frac{272}{81}L_{\frac{ed}{22jj}}^{V,LL} \\
& + \frac{272}{81}L_{\frac{ed}{33jj}}^{V,LL} + \frac{272}{81}L_{\frac{ed}{11ii}}^{V,LR} + \frac{272}{81}L_{\frac{ed}{22ii}}^{V,LR} + \frac{272}{81}L_{\frac{ed}{33ii}}^{V,LR} + \frac{272}{81}L_{\frac{ed}{11ii}}^{V,RR} + \frac{272}{81}L_{\frac{ed}{22ii}}^{V,RR} \\
& + \frac{272}{81}L_{\frac{ed}{33ii}}^{V,RR} - \frac{544}{81}L_{\frac{ud}{11jj}}^{V1,LL} - \frac{544}{81}L_{\frac{ud}{22jj}}^{V1,LL} - \frac{544}{81}L_{\frac{ud}{11ii}}^{V1,LR} - \frac{544}{81}L_{\frac{ud}{22ii}}^{V1,LR} - \frac{544}{81}L_{\frac{ud}{11ii}}^{V1,RR} \\
& - \frac{544}{81}L_{\frac{ud}{22ii}}^{V1,RR} + \frac{122}{27}L_{\frac{ud}{11jj}}^{V8,LL} + \frac{122}{27}L_{\frac{ud}{22jj}}^{V8,LL} + \frac{2}{3}L_{\frac{ud}{11ii}}^{V8,LR} + \frac{2}{3}L_{\frac{ud}{22ii}}^{V8,LR} + \frac{122}{27}L_{\frac{ud}{11ii}}^{V8,RR} \\
& + \frac{122}{27}L_{\frac{ud}{22ii}}^{V8,RR} \Big] + \frac{1790}{81}L_{\frac{dd}{jjii}}^{V8,LR}\alpha^2 ;
\end{aligned}$$

$$\dot{L}_{\frac{uu}{jjii}}^{V1,LR} = -\frac{8}{3}L_{\frac{uu}{jjii}}^{V8,LR}g_s^2 + e^2 \Big[ -\frac{8}{9}L_{\frac{du}{11ii}}^{V1,LR} - \frac{8}{9}L_{\frac{du}{22ii}}^{V1,LR} - \frac{8}{9}L_{\frac{du}{33ii}}^{V1,LR} - \frac{8}{9}L_{\frac{eu}{11jj}}^{V,LL}$$

$$\begin{aligned}
& -\frac{8}{9}L_{22jj}^{V,LL} - \frac{8}{9}L_{33jj}^{V,LL} - \frac{8}{9}L_{11ii}^{V,LR} - \frac{8}{9}L_{22ii}^{V,LR} - \frac{8}{9}L_{33ii}^{V,LR} - \frac{8}{9}L_{11ii}^{V,RR} \\
& -\frac{8}{9}L_{22ii}^{V,RR} - \frac{8}{9}L_{33ii}^{V,RR} - \frac{8}{9}L_{jj11}^{V1,LL} - \frac{8}{9}L_{jj22}^{V1,LL} - \frac{8}{9}L_{jj33}^{V1,LL} - \frac{8}{9}L_{jj11}^{V1,LR} \\
& -\frac{8}{9}L_{jj22}^{V1,LR} - \frac{8}{9}L_{jj33}^{V1,LR} - \frac{8}{9}L_{ii11}^{V1,RR} - \frac{8}{9}L_{ii22}^{V1,RR} - \frac{8}{9}L_{ii33}^{V1,RR} - \frac{8}{9}L_{jj11}^{V,LR} \\
& -\frac{8}{9}L_{jj22}^{V,LR} - \frac{8}{9}L_{jj33}^{V,LR} + \frac{16}{9}L_{uu}^{V1,LR} - \frac{16}{3}L_{jjii}^{V1,LR} + \frac{16}{9}L_{jjjj}^{V1,LR} + \frac{16}{9}L_{jjkk}^{V1,LR} \\
& + \frac{16}{9}L_{kkii}^{V1,LR} + \frac{128}{27}L_{uu}^{V,LL} + \frac{32}{9}L_{jjkk}^{V,LL} + \frac{32}{27}L_{jjkj}^{V,LL} + \frac{128}{27}L_{uu}^{V,RR} + \frac{32}{9}L_{uu}^{V,RR} \\
& + \frac{32}{27}L_{kkii}^{V,RR} \Big] + \alpha_s^2 \Bigg[ 8L_{11ii}^{V1,LR} + 8L_{22ii}^{V1,LR} + 8L_{33ii}^{V1,LR} + \frac{44}{27}L_{11ii}^{V8,LR} \\
& + \frac{44}{27}L_{22ii}^{V8,LR} + \frac{44}{27}L_{33ii}^{V8,LR} - 8L_{jj11}^{V1,LL} - 8L_{jj22}^{V1,LL} - 8L_{jj33}^{V1,LL} + 8L_{jj11}^{V1,LR} \\
& + 8L_{jj22}^{V1,LR} + 8L_{jj33}^{V1,LR} - 8L_{ii11}^{V1,RR} - 8L_{ii22}^{V1,RR} - 8L_{ii33}^{V1,RR} + \frac{44}{27}L_{jj11}^{V8,LL} \\
& + \frac{44}{27}L_{jj22}^{V8,LL} + \frac{44}{27}L_{jj33}^{V8,LL} + \frac{44}{27}L_{jj11}^{V8,LR} + \frac{44}{27}L_{jj22}^{V8,LR} + \frac{44}{27}L_{jj33}^{V8,LR} + \frac{44}{27}L_{ii11}^{V8,RR} \\
& + \frac{44}{27}L_{ii22}^{V8,RR} + \frac{44}{27}L_{ii33}^{V8,RR} + 8L_{iii}^{V1,LR} - \frac{28}{3}L_{jjii}^{V1,LR} + 8L_{jjjj}^{V1,LR} + 8L_{jjkk}^{V1,LR} \\
& + 8L_{kkii}^{V1,LR} + \frac{44}{27}L_{uu}^{V8,LR} - \frac{2044}{27}L_{jjii}^{V8,LR} + \frac{44}{27}L_{jjjj}^{V8,LR} + \frac{44}{27}L_{jjkk}^{V8,LR} + \frac{44}{27}L_{kkii}^{V8,LR} \\
& - \frac{232}{9}L_{jjjj}^{V,LL} - 16L_{jjkk}^{V,LL} - \frac{64}{27}L_{jjkj}^{V,LL} - \frac{232}{9}L_{iii}^{V,RR} - 16L_{iikk}^{V,RR} - \frac{64}{27}L_{kkii}^{V,RR} \Big] \\
& + \alpha_s \alpha \Bigg[ -\frac{32}{9}L_{11ii}^{V1,LR} - \frac{32}{9}L_{22ii}^{V1,LR} + \frac{64}{9}L_{33ii}^{V1,LR} + \frac{664}{729}L_{11ii}^{V8,LR} + \frac{664}{729}L_{22ii}^{V8,LR} \\
& - \frac{4088}{729}L_{33ii}^{V8,LR} - \frac{32}{9}L_{jj11}^{V1,LL} - \frac{32}{9}L_{jj22}^{V1,LL} - \frac{32}{9}L_{jj33}^{V1,LL} - \frac{32}{9}L_{jj11}^{V1,LR} - \frac{32}{9}L_{jj22}^{V1,LR} \\
& + \frac{64}{9}L_{jj33}^{V1,LR} - \frac{32}{9}L_{ii11}^{V1,RR} - \frac{32}{9}L_{ii22}^{V1,RR} - \frac{32}{9}L_{ii33}^{V1,RR} - \frac{776}{729}L_{jj11}^{V8,LL} - \frac{776}{729}L_{jj22}^{V8,LL} \\
& - \frac{776}{729}L_{jj33}^{V8,LL} + \frac{664}{729}L_{jj11}^{V8,LR} + \frac{664}{729}L_{jj22}^{V8,LR} - \frac{4088}{729}L_{jj33}^{V8,LR} - \frac{776}{729}L_{ii11}^{V8,RR} \\
& - \frac{776}{729}L_{ii22}^{V8,RR} - \frac{776}{729}L_{ii33}^{V8,RR} + \frac{64}{9}L_{iii}^{V1,LR} + \frac{128}{3}L_{jjii}^{V1,LR} + \frac{64}{9}L_{jjjj}^{V1,LR} + \frac{64}{9}L_{jjkk}^{V1,LR}
\end{aligned}$$

$$\begin{aligned}
& + \frac{64}{9} L_{\overline{uu} \overline{kkii}}^{V1,LR} - \frac{4088}{729} L_{\overline{uu} \overline{iii}}^{V8,LR} - \frac{32}{27} L_{\overline{uu} \overline{jjii}}^{V8,LR} - \frac{4088}{729} L_{\overline{uu} \overline{jjjj}}^{V8,LR} - \frac{4088}{729} L_{\overline{uu} \overline{jjkk}}^{V8,LR} \\
& - \frac{4088}{729} L_{\overline{uu} \overline{kkii}}^{V8,LR} + \frac{4192}{243} L_{\overline{uu} \overline{jjjj}}^{V,LL} + \frac{32}{3} L_{\overline{uu} \overline{jjkk}}^{V,LL} + \frac{256}{729} L_{\overline{uu} \overline{jjkj}}^{V,LL} + \frac{4192}{243} L_{\overline{uu} \overline{iii}}^{V,RR} \\
& + \frac{32}{3} L_{\overline{uu} \overline{ikk}}^{V,RR} + \frac{256}{729} L_{\overline{uu} \overline{ikki}}^{V,RR} \Big] + \alpha^2 \Big[ - \frac{2392}{729} L_{\overline{du} \overline{11ii}}^{V1,LR} - \frac{2392}{729} L_{\overline{du} \overline{22ii}}^{V1,LR} + \frac{3776}{729} L_{\overline{du} \overline{33ii}}^{V1,LR} \\
& - \frac{8152}{729} L_{\overline{eu} \overline{11jj}}^{V,LL} - \frac{8152}{729} L_{\overline{eu} \overline{22jj}}^{V,LL} - \frac{8152}{729} L_{\overline{eu} \overline{33jj}}^{V,LL} - \frac{4696}{729} L_{\overline{eu} \overline{11ii}}^{V,LR} - \frac{4696}{729} L_{\overline{eu} \overline{22ii}}^{V,LR} \\
& - \frac{4696}{729} L_{\overline{eu} \overline{33ii}}^{V,LR} - \frac{8152}{729} L_{\overline{eu} \overline{11ii}}^{V,RR} - \frac{8152}{729} L_{\overline{eu} \overline{22ii}}^{V,RR} - \frac{8152}{729} L_{\overline{eu} \overline{33ii}}^{V,RR} - \frac{3544}{729} L_{\overline{ud} \overline{jj11}}^{V1,LL} \\
& - \frac{3544}{729} L_{\overline{ud} \overline{jj22}}^{V1,LL} - \frac{3544}{729} L_{\overline{ud} \overline{jj33}}^{V1,LL} - \frac{2392}{729} L_{\overline{ud} \overline{jj11}}^{V1,LR} - \frac{2392}{729} L_{\overline{ud} \overline{jj22}}^{V1,LR} + \frac{3776}{729} L_{\overline{ud} \overline{jj33}}^{V1,LR} \\
& - \frac{3544}{729} L_{\overline{ud} \overline{ii11}}^{V1,RR} - \frac{3544}{729} L_{\overline{ud} \overline{ii22}}^{V1,RR} - \frac{3544}{729} L_{\overline{ud} \overline{ii33}}^{V1,RR} - \frac{4696}{729} L_{\overline{ue} \overline{jj11}}^{V,LR} - \frac{4696}{729} L_{\overline{ue} \overline{jj22}}^{V,LR} \\
& - \frac{4696}{729} L_{\overline{ue} \overline{jj33}}^{V,LR} + \frac{4352}{729} L_{\overline{uu} \overline{iii}}^{V1,LR} + \frac{7520}{81} L_{\overline{uu} \overline{jjii}}^{V1,LR} + \frac{4352}{729} L_{\overline{uu} \overline{jjjj}}^{V1,LR} + \frac{4352}{729} L_{\overline{uu} \overline{jjkk}}^{V1,LR} \\
& + \frac{4352}{729} L_{\overline{uu} \overline{kkii}}^{V1,LR} - \frac{10496}{729} L_{\overline{uu} \overline{jjjj}}^{V,LL} - \frac{512}{729} L_{\overline{uu} \overline{jjkk}}^{V,LL} - \frac{13568}{2187} L_{\overline{uu} \overline{jjkj}}^{V,LL} - \frac{10496}{729} L_{\overline{uu} \overline{iii}}^{V,RR} \\
& - \frac{512}{729} L_{\overline{uu} \overline{ikk}}^{V,RR} - \frac{13568}{2187} L_{\overline{uu} \overline{ikki}}^{V,RR} \Big] ;
\end{aligned}$$

$$\begin{aligned}
\dot{L}_{\overline{uu} \overline{jjii}}^{V8,LR} & = g_s^2 \Big[ \frac{2}{3} L_{\overline{du} \overline{11ii}}^{V8,LR} + \frac{2}{3} L_{\overline{du} \overline{22ii}}^{V8,LR} + \frac{2}{3} L_{\overline{du} \overline{33ii}}^{V8,LR} + \frac{2}{3} L_{\overline{ud} \overline{jj11}}^{V8,LL} + \frac{2}{3} L_{\overline{ud} \overline{jj22}}^{V8,LL} \\
& + \frac{2}{3} L_{\overline{ud} \overline{jj33}}^{V8,LL} + \frac{2}{3} L_{\overline{ud} \overline{jj11}}^{V8,LR} + \frac{2}{3} L_{\overline{ud} \overline{jj22}}^{V8,LR} + \frac{2}{3} L_{\overline{ud} \overline{jj33}}^{V8,LR} + \frac{2}{3} L_{\overline{ud} \overline{ii11}}^{V8,RR} + \frac{2}{3} L_{\overline{ud} \overline{ii22}}^{V8,RR} \\
& + \frac{2}{3} L_{\overline{ud} \overline{ii33}}^{V8,RR} - 12 L_{\overline{uu} \overline{jjii}}^{V1,LR} + \frac{2}{3} L_{\overline{uu} \overline{iii}}^{V8,LR} - 14 L_{\overline{uu} \overline{jjii}}^{V8,LR} + \frac{2}{3} L_{\overline{uu} \overline{jjjj}}^{V8,LR} + \frac{2}{3} L_{\overline{uu} \overline{jjkk}}^{V8,LR} \\
& + \frac{2}{3} L_{\overline{uu} \overline{kkii}}^{V8,LR} + \frac{8}{3} L_{\overline{uu} \overline{jjjj}}^{V,LL} + \frac{8}{3} L_{\overline{uu} \overline{jjkk}}^{V,LL} + \frac{8}{3} L_{\overline{uu} \overline{iii}}^{V,RR} + \frac{8}{3} L_{\overline{uu} \overline{ikki}}^{V,RR} \Big] - \frac{16}{3} L_{\overline{uu} \overline{jjii}}^{V8,LR} \\
& e^2 + \alpha_s^2 \Big[ - \frac{22}{3} L_{\overline{du} \overline{11ii}}^{V1,LR} - \frac{22}{3} L_{\overline{du} \overline{22ii}}^{V1,LR} - \frac{22}{3} L_{\overline{du} \overline{33ii}}^{V1,LR} + \frac{787}{81} L_{\overline{du} \overline{11ii}}^{V8,LR} + \frac{787}{81} L_{\overline{du} \overline{22ii}}^{V8,LR} \\
& + \frac{787}{81} L_{\overline{du} \overline{33ii}}^{V8,LR} - \frac{2}{3} L_{\overline{ud} \overline{jj11}}^{V1,LL} - \frac{2}{3} L_{\overline{ud} \overline{jj22}}^{V1,LL} - \frac{2}{3} L_{\overline{ud} \overline{jj33}}^{V1,LL} - \frac{22}{3} L_{\overline{ud} \overline{jj11}}^{V1,LR} - \frac{22}{3} L_{\overline{ud} \overline{jj22}}^{V1,LR} \\
& - \frac{22}{3} L_{\overline{ud} \overline{jj33}}^{V1,LR} - \frac{2}{3} L_{\overline{ud} \overline{ii11}}^{V1,RR} - \frac{2}{3} L_{\overline{ud} \overline{ii22}}^{V1,RR} - \frac{2}{3} L_{\overline{ud} \overline{ii33}}^{V1,RR} + \frac{607}{81} L_{\overline{ud} \overline{jj11}}^{V8,LL} + \frac{607}{81} L_{\overline{ud} \overline{jj22}}^{V8,LL}
\end{aligned}$$

$$\begin{aligned}
& + \frac{607}{81} L_{ud,jj33}^{V8,LL} + \frac{787}{81} L_{ud,jj11}^{V8,LR} + \frac{787}{81} L_{ud,jj22}^{V8,LR} + \frac{787}{81} L_{ud,jj33}^{V8,LR} + \frac{607}{81} L_{ud,ii11}^{V8,RR} + \frac{607}{81} L_{ud,ii22}^{V8,RR} \\
& + \frac{607}{81} L_{ud,ii33}^{V8,RR} - \frac{22}{3} L_{uu,iii}^{V1,LR} - \frac{374}{3} L_{uu,jji}^{V1,LR} - \frac{22}{3} L_{uu,jjj}^{V1,LR} - \frac{22}{3} L_{uu,jkk}^{V1,LR} - \frac{22}{3} L_{uu,kki}^{V1,LR} \\
& + \frac{787}{81} L_{uu,iii}^{V8,LR} - \frac{2975}{18} L_{uu,jji}^{V8,LR} + \frac{787}{81} L_{uu,jjj}^{V8,LR} + \frac{787}{81} L_{uu,jkk}^{V8,LR} + \frac{787}{81} L_{uu,kki}^{V8,LR} \\
& + \frac{1198}{27} L_{uu,jjj}^{V,LL} - \frac{28}{3} L_{uu,jjk}^{V,LL} + \frac{3448}{81} L_{uu,jkj}^{V,LL} + \frac{1198}{27} L_{uu,iii}^{V,RR} - \frac{28}{3} L_{uu,iik}^{V,RR} + \frac{3448}{81} L_{uu,iki}^{V,RR} \Big] \\
& + \alpha_s \alpha \Bigg[ - \frac{544}{81} L_{du,11ii}^{V1,LR} - \frac{544}{81} L_{du,22ii}^{V1,LR} + \frac{1160}{81} L_{du,33ii}^{V1,LR} + \frac{22}{9} L_{du,11ii}^{V8,LR} + \frac{22}{9} L_{du,22ii}^{V8,LR} \\
& + \frac{56}{9} L_{du,33ii}^{V8,LR} - \frac{544}{81} L_{eu,11jj}^{V,LL} - \frac{544}{81} L_{eu,22jj}^{V,LL} - \frac{544}{81} L_{eu,33jj}^{V,LL} - \frac{544}{81} L_{eu,11ii}^{V,LR} - \frac{544}{81} L_{eu,22ii}^{V,LR} \\
& - \frac{544}{81} L_{eu,33ii}^{V,LR} - \frac{544}{81} L_{eu,11ii}^{V,RR} - \frac{544}{81} L_{eu,22ii}^{V,RR} - \frac{544}{81} L_{eu,33ii}^{V,RR} - \frac{544}{81} L_{ud,jj11}^{V1,LL} - \frac{544}{81} L_{ud,jj22}^{V1,LL} \\
& - \frac{544}{81} L_{ud,jj33}^{V1,LL} - \frac{544}{81} L_{ud,jj11}^{V1,LR} - \frac{544}{81} L_{ud,jj22}^{V1,LR} + \frac{1160}{81} L_{ud,jj33}^{V1,LR} - \frac{544}{81} L_{ud,ii11}^{V1,RR} \\
& - \frac{544}{81} L_{ud,ii22}^{V1,RR} - \frac{544}{81} L_{ud,ii33}^{V1,RR} + \frac{170}{27} L_{ud,jj11}^{V8,LL} + \frac{170}{27} L_{ud,jj22}^{V8,LL} + \frac{170}{27} L_{ud,jj33}^{V8,LL} + \frac{22}{9} L_{ud,jj11}^{V8,LR} \\
& + \frac{22}{9} L_{ud,jj22}^{V8,LR} + \frac{56}{9} L_{ud,jj33}^{V8,LR} + \frac{170}{27} L_{ud,ii11}^{V8,RR} + \frac{170}{27} L_{ud,ii22}^{V8,RR} + \frac{170}{27} L_{ud,ii33}^{V8,RR} - \frac{544}{81} L_{ue,jj11}^{V,LR} \\
& - \frac{544}{81} L_{ue,jj22}^{V,LR} - \frac{544}{81} L_{ue,jj33}^{V,LR} + \frac{1088}{81} L_{uu,iii}^{V1,LR} - \frac{16}{3} L_{uu,jji}^{V1,LR} + \frac{1088}{81} L_{uu,jjj}^{V1,LR} + \frac{1088}{81} L_{uu,jkk}^{V1,LR} \\
& + \frac{1088}{81} L_{uu,kki}^{V1,LR} + \frac{56}{9} L_{uu,iii}^{V8,LR} - \frac{104}{9} L_{uu,jji}^{V8,LR} + \frac{56}{9} L_{uu,jjj}^{V8,LR} + \frac{56}{9} L_{uu,jkk}^{V8,LR} + \frac{56}{9} L_{uu,kki}^{V8,LR} \\
& + \frac{1360}{81} L_{uu,jjj}^{V,LL} + \frac{2176}{81} L_{uu,jkk}^{V,LL} - \frac{4256}{243} L_{uu,jkj}^{V,LL} + \frac{1360}{81} L_{uu,iii}^{V,RR} + \frac{2176}{81} L_{uu,iik}^{V,RR} \\
& - \frac{4256}{243} L_{uu,iki}^{V,RR} \Big] + \frac{7520}{81} L_{uu,jji}^{V8,LR} \alpha^2 ;
\end{aligned}$$

$$\begin{aligned}
\dot{L}_{ee,jji}^{V,LR} & = e^2 \Bigg[ - \frac{32}{3} L_{ee,jji}^{V,LR} + \frac{16}{3} L_{ee,ijj}^{V,RR} + \frac{4}{3} L_{ee,kki}^{V,LR} + \frac{16}{3} L_{ee,iik}^{V,RR} + \frac{4}{3} L_{de,11ii}^{V,LR} \\
& + \frac{4}{3} L_{de,22ii}^{V,LR} + \frac{4}{3} L_{de,33ii}^{V,LR} + \frac{4}{3} L_{ed,ii11}^{V,RR} + \frac{4}{3} L_{ed,ii22}^{V,RR} + \frac{4}{3} L_{ed,ii33}^{V,RR} + \frac{4}{3} L_{ee,iii}^{V,LR} \\
& + \frac{16}{3} L_{ee,iii}^{V,RR} - \frac{8}{3} L_{ee,ii11}^{V,RR} - \frac{8}{3} L_{ee,ii22}^{V,RR} - \frac{8}{3} L_{ue,11ii}^{V,LR} - \frac{8}{3} L_{ue,22ii}^{V,LR} + \frac{16}{3} L_{ue,jkk}^{V,LL} \Big]
\end{aligned}$$

$$\begin{aligned}
& + \frac{4}{3}L_{jjkk}^{V,LR} + \frac{4}{3}L_{jj11}^{V,LL} + \frac{4}{3}L_{jj22}^{V,LL} + \frac{4}{3}L_{jj33}^{V,LL} + \frac{4}{3}L_{jj11}^{V,LR} + \frac{4}{3}L_{jj22}^{V,LR} \\
& + \frac{4}{3}L_{jj33}^{V,LR} + 8L_{jjjj}^{V,LL} + \frac{8}{3}L_{jjjj}^{V,LR} - \frac{8}{3}L_{jj11}^{V,LL} - \frac{8}{3}L_{jj22}^{V,LL} - \frac{8}{3}L_{jj11}^{V,LR} \\
& - \frac{8}{3}L_{jj22}^{V,LR} \Big] + \alpha_s \alpha \left[ \frac{16}{3}L_{11ii}^{V,LR} + \frac{16}{3}L_{22ii}^{V,LR} + \frac{16}{3}L_{33ii}^{V,LR} + \frac{16}{3}L_{ii11}^{V,RR} \right. \\
& + \frac{16}{3}L_{ii22}^{V,RR} + \frac{16}{3}L_{ii33}^{V,RR} - \frac{32}{3}L_{ii11}^{V,RR} - \frac{32}{3}L_{ii22}^{V,RR} - \frac{32}{3}L_{11ii}^{V,LR} - \frac{32}{3}L_{22ii}^{V,LR} \\
& + \frac{16}{3}L_{jj11}^{V,LL} + \frac{16}{3}L_{jj22}^{V,LL} + \frac{16}{3}L_{jj33}^{V,LL} + \frac{16}{3}L_{jj11}^{V,LR} + \frac{16}{3}L_{jj22}^{V,LR} + \frac{16}{3}L_{jj33}^{V,LR} \\
& \left. - \frac{32}{3}L_{jj11}^{V,LL} - \frac{32}{3}L_{jj22}^{V,LL} - \frac{32}{3}L_{jj11}^{V,LR} - \frac{32}{3}L_{jj22}^{V,LR} \right] + \alpha^2 \left[ \frac{6386}{27}L_{jjii}^{V,LR} \right. \\
& + \frac{32}{27}L_{iijj}^{V,RR} + \frac{296}{27}L_{kkii}^{V,LR} + \frac{32}{27}L_{iikk}^{V,RR} + \frac{424}{81}L_{11ii}^{V,LR} + \frac{424}{81}L_{22ii}^{V,LR} + \frac{424}{81}L_{33ii}^{V,LR} \\
& - \frac{344}{81}L_{ii11}^{V,RR} - \frac{344}{81}L_{ii22}^{V,RR} - \frac{344}{81}L_{ii33}^{V,RR} + \frac{296}{27}L_{iii}^{V,LR} - \frac{736}{27}L_{iii}^{V,RR} - \frac{3128}{81}L_{ii11}^{V,RR} \\
& - \frac{3128}{81}L_{ii22}^{V,RR} - \frac{56}{81}L_{11ii}^{V,LR} - \frac{56}{81}L_{22ii}^{V,LR} + \frac{32}{27}L_{jjkk}^{V,LL} + \frac{296}{27}L_{jjkk}^{V,LR} - \frac{344}{81}L_{jj11}^{V,LL} \\
& - \frac{344}{81}L_{jj22}^{V,LL} - \frac{344}{81}L_{jj33}^{V,LL} + \frac{424}{81}L_{jj11}^{V,LR} + \frac{424}{81}L_{jj22}^{V,LR} + \frac{424}{81}L_{jj33}^{V,LR} - \frac{80}{3}L_{jjjj}^{V,LL} \\
& \left. + \frac{592}{27}L_{jjjj}^{V,LR} - \frac{3128}{81}L_{jj11}^{V,LL} - \frac{3128}{81}L_{jj22}^{V,LL} - \frac{56}{81}L_{jj11}^{V,LR} - \frac{56}{81}L_{jj22}^{V,LR} \right] ;
\end{aligned}$$

### 1.10 $\Delta L = 2$ Transitions ( $\bar{\nu}_i^c \nu_j \bar{f}_k f_l$ or $\bar{\nu}_i^c e_j \bar{d}_k u_l$ )

$$\begin{aligned}
\dot{L}_{\nu d}^{S,LR}{}_{ijkl} &= -8g_s^2 L_{\nu d}^{S,LR}{}_{ijkl} - \frac{2}{3}e^2 L_{\nu d}^{S,LR}{}_{ijkl} - \frac{1012}{9}\alpha_s^2 L_{\nu d}^{S,LR}{}_{ijkl} - \frac{8}{9}\alpha_s \alpha L_{\nu d}^{S,LR}{}_{ijkl} \\
&+ \frac{397}{81}\alpha^2 L_{\nu d}^{S,LR}{}_{ijkl} ; \\
\dot{L}_{\nu d}^{S,LL}{}_{ijkl} &= -8g_s^2 L_{\nu d}^{S,LL}{}_{ijkl} - \frac{2}{3}e^2 L_{\nu d}^{S,LL}{}_{ijkl} - \frac{1012}{9}\alpha_s^2 L_{\nu d}^{S,LL}{}_{ijkl} - \frac{8}{9}\alpha_s \alpha L_{\nu d}^{S,LL}{}_{ijkl} \\
&+ \frac{397}{81}\alpha^2 L_{\nu d}^{S,LL}{}_{ijkl} ;
\end{aligned}$$

$$\begin{aligned}
\dot{L}_{ijkl}^{T,LL} &= \frac{8}{3}g_s^2 L_{ijkl}^{T,LL} + \frac{2}{9}e^2 L_{ijkl}^{T,LL} + \frac{1652}{27}\alpha_s^2 L_{ijkl}^{T,LL} - \frac{152}{27}\alpha_s \alpha L_{ijkl}^{T,LL} \\
&\quad - \frac{1097}{243}\alpha^2 L_{ijkl}^{T,LL} ; \\
\dot{L}_{ijkl}^{S,LR} &= -8g_s^2 L_{ijkl}^{S,LR} - \frac{8}{3}e^2 L_{ijkl}^{S,LR} - \frac{1012}{9}\alpha_s^2 L_{ijkl}^{S,LR} - \frac{32}{9}\alpha_s \alpha L_{ijkl}^{S,LR} \\
&\quad + \frac{1552}{81}\alpha^2 L_{ijkl}^{S,LR} ; \\
\dot{L}_{ijkl}^{S,LL} &= -8g_s^2 L_{ijkl}^{S,LL} - \frac{8}{3}e^2 L_{ijkl}^{S,LL} - \frac{1012}{9}\alpha_s^2 L_{ijkl}^{S,LL} - \frac{32}{9}\alpha_s \alpha L_{ijkl}^{S,LL} \\
&\quad + \frac{1552}{81}\alpha^2 L_{ijkl}^{S,LL} ; \\
\dot{L}_{ijkl}^{T,LL} &= \frac{8}{3}g_s^2 L_{ijkl}^{T,LL} + \frac{8}{9}e^2 L_{ijkl}^{T,LL} + \frac{1652}{27}\alpha_s^2 L_{ijkl}^{T,LL} - \frac{608}{27}\alpha_s \alpha L_{ijkl}^{T,LL} \\
&\quad - \frac{5072}{243}\alpha^2 L_{ijkl}^{T,LL} ; \\
\dot{L}_{ijkl}^{S,LR} &= \frac{373}{9}\alpha^2 L_{ijkl}^{S,LR} - 6e^2 L_{ijkl}^{S,LR} ; \\
\dot{L}_{ijkl}^{S,LL} &= \frac{373}{9}\alpha^2 L_{ijkl}^{S,LL} - 6e^2 L_{ijkl}^{S,LL} ; \\
\dot{L}_{ijkl}^{T,LL} &= 2e^2 L_{ijkl}^{T,LL} - \frac{1553}{27}\alpha^2 L_{ijkl}^{T,LL} ; \\
\dot{L}_{vedu}^{V,RR} &= -4e^2 L_{vedu}^{V,RR} + 4\alpha_s \alpha L_{vedu}^{V,RR} - \frac{160}{27}\alpha^2 L_{vedu}^{V,RR} ; \\
\dot{L}_{vedu}^{V,RL} &= -2e^2 L_{vedu}^{V,RL} - 4\alpha_s \alpha L_{vedu}^{V,RL} - \frac{497}{27}\alpha^2 L_{vedu}^{V,RL} ; \\
\dot{L}_{vedu}^{S,LR} &= -8g_s^2 L_{vedu}^{S,LR} + \frac{4}{3}e^2 L_{vedu}^{S,LR} - \frac{1012}{9}\alpha_s^2 L_{vedu}^{S,LR} + 12\alpha_s \alpha L_{vedu}^{S,LR} \\
&\quad - \frac{4016}{81}\alpha^2 L_{vedu}^{S,LR} ; \\
\dot{L}_{vedu}^{S,LL} &= -8g_s^2 L_{vedu}^{S,LL} + e^2 \left[ \frac{4}{3}L_{vedu}^{S,LL} + 8L_{vedu}^{T,LL} \right] - \frac{1012}{9}\alpha_s^2 L_{vedu}^{S,LL}
\end{aligned}$$

$$\begin{aligned}
& + \alpha_s \alpha \left[ 12 L_{\nu edu}^{S,LL} - \frac{448}{9} L_{ijkl}^{T,LL} \right] + \alpha^2 \left[ -\frac{3953}{81} L_{\nu edu}^{S,LL} - \frac{3368}{27} L_{ijkl}^{T,LL} \right]; \\
\dot{L}_{\nu edu}^{T,LL} &= \frac{8}{3} g_s^2 L_{\nu edu}^{T,LL} + e^2 \left[ \frac{1}{6} L_{\nu edu}^{S,LL} - \frac{40}{9} L_{ijkl}^{T,LL} \right] + \frac{1652}{27} \alpha_s^2 L_{\nu edu}^{T,LL} \\
& + \alpha_s \alpha \left[ \frac{4}{3} L_{\nu edu}^{T,LL} - \frac{4}{3} L_{\nu edu}^{S,LL} \right] + \alpha^2 \left[ \frac{3985}{243} L_{\nu edu}^{T,LL} - \frac{13}{162} L_{\nu edu}^{S,LL} \right];
\end{aligned}$$

### 1.11 $\Delta L = 4$ Transitions ( $\bar{\nu}_i^c \nu_j \bar{\nu}_k^c \nu_l$ )

$$\dot{L}_{\nu\nu}^{S,LL} = 0;$$

### 1.12 $|\Delta B| = |\Delta L| = 1$ Transitions: Baryon Number Violation

$$\begin{aligned}
\dot{L}_{ijkl}^{S,LL} &= -4g_s^2 L_{ijkl}^{S,LL} - \frac{4}{3} e^2 L_{ijkl}^{S,LL} + \frac{370}{9} \alpha_s^2 L_{ijkl}^{S,LL} + \alpha_s \alpha \left[ -\frac{260}{27} L_{ijkl}^{S,LL} \right. \\
& \quad \left. - \frac{256}{27} L_{il kj}^{S,LL} \right] + \alpha^2 \left[ -\frac{10570}{243} L_{ijkl}^{S,LL} - \frac{7936}{243} L_{il kj}^{S,LL} \right]; \\
\dot{L}_{ijkl}^{S,RR} &= -4g_s^2 L_{ijkl}^{S,RR} - \frac{4}{3} e^2 L_{ijkl}^{S,RR} + \frac{370}{9} \alpha_s^2 L_{ijkl}^{S,RR} + \alpha_s \alpha \left[ -\frac{260}{27} L_{ijkl}^{S,RR} \right. \\
& \quad \left. - \frac{256}{27} L_{il kj}^{S,RR} \right] + \alpha^2 \left[ -\frac{10570}{243} L_{ijkl}^{S,RR} - \frac{7936}{243} L_{il kj}^{S,RR} \right]; \\
\dot{L}_{ijkl}^{S,LR} &= -4g_s^2 L_{ijkl}^{S,LR} - \frac{4}{3} e^2 L_{ijkl}^{S,LR} + \frac{250}{9} \alpha_s^2 L_{ijkl}^{S,LR} - \frac{4}{9} \alpha_s \alpha L_{ijkl}^{S,LR} \\
& \quad - \frac{4298}{81} \alpha^2 L_{ijkl}^{S,LR}; \\
\dot{L}_{ijkl}^{S,RL} &= -4g_s^2 L_{ijkl}^{S,RL} - \frac{4}{3} e^2 L_{ijkl}^{S,RL} + \frac{250}{9} \alpha_s^2 L_{ijkl}^{S,RL} - \frac{4}{9} \alpha_s \alpha L_{ijkl}^{S,RL} \\
& \quad - \frac{4298}{81} \alpha^2 L_{ijkl}^{S,RL}; \\
\dot{L}_{ijkl}^{S,LL} &= -4g_s^2 L_{ijkl}^{S,LL} + e^2 \left[ -\frac{2}{3} L_{ijkl}^{S,LL} - \frac{4}{3} L_{ikjl}^{S,LL} \right] + \frac{370}{9} \alpha_s^2 L_{ijkl}^{S,LL}
\end{aligned}$$

$$\begin{aligned}
& + \alpha_s \alpha \left[ \frac{16}{3} L_{ikjl}^{S,LL} - \frac{8}{3} L_{ijkl}^{S,LL} \right] + \alpha^2 \left[ \frac{127}{27} L_{ijkl}^{S,LL} + \frac{1672}{81} L_{ikjl}^{S,LL} \right] ; \\
\dot{L}_{ijkl}^{S,RR} & = -4g_s^2 L_{ijkl}^{S,RR} + e^2 \left[ -\frac{2}{3} L_{ijkl}^{S,RR} - \frac{4}{3} L_{ilkj}^{S,RR} \right] + \frac{370}{9} \alpha_s^2 L_{ijkl}^{S,RR} \\
& + \alpha_s \alpha \left[ -\frac{584}{27} L_{ijkl}^{S,RR} - \frac{304}{27} L_{ilkj}^{S,RR} \right] + \alpha^2 \left[ -\frac{6409}{243} L_{ijkl}^{S,RR} - \frac{1768}{243} L_{ilkj}^{S,RR} \right] ; \\
\dot{L}_{ijkl}^{S,LR} & = -4g_s^2 L_{ijkl}^{S,LR} - \frac{4}{3} e^2 L_{ijkl}^{S,LR} + \frac{250}{9} \alpha_s^2 L_{ijkl}^{S,LR} - \frac{184}{9} \alpha_s \alpha L_{ijkl}^{S,LR} \\
& - \frac{2480}{81} \alpha^2 L_{ijkl}^{S,LR} ; \\
\dot{L}_{ijkl}^{S,RL} & = -4g_s^2 L_{ijkl}^{S,RL} - \frac{4}{3} e^2 L_{ijkl}^{S,RL} + \frac{250}{9} \alpha_s^2 L_{ijkl}^{S,RL} + \frac{16}{9} \alpha_s \alpha L_{ijkl}^{S,RL} \\
& + \frac{1304}{81} \alpha^2 L_{ijkl}^{S,RL} ; \\
\dot{L}_{ijkl}^{S,LR} & = -4g_s^2 L_{ijkl}^{S,LR} + \frac{2}{3} e^2 L_{ijkl}^{S,LR} + \frac{250}{9} \alpha_s^2 L_{ijkl}^{S,LR} - \frac{8}{9} \alpha_s \alpha L_{ijkl}^{S,LR} \\
& - \frac{1435}{81} \alpha^2 L_{ijkl}^{S,LR} ; \\
\dot{L}_{ijkl}^{S,RL} & = -4g_s^2 L_{ijkl}^{S,RL} + \frac{2}{3} e^2 L_{ijkl}^{S,RL} + \frac{250}{9} \alpha_s^2 L_{ijkl}^{S,RL} - \frac{8}{9} \alpha_s \alpha L_{ijkl}^{S,RL} \\
& - \frac{1435}{81} \alpha^2 L_{ijkl}^{S,RL} ; \\
\dot{L}_{ijkl}^{S,LR} & = -4g_s^2 L_{ijkl}^{S,LR} + \frac{14}{3} e^2 L_{ijkl}^{S,LR} + \frac{250}{9} \alpha_s^2 L_{ijkl}^{S,LR} - \frac{68}{9} \alpha_s \alpha L_{ijkl}^{S,LR} \\
& - \frac{8299}{81} \alpha^2 L_{ijkl}^{S,LR} ; \\
\dot{L}_{ijkl}^{S,RL} & = -4g_s^2 L_{ijkl}^{S,RL} + \frac{14}{3} e^2 L_{ijkl}^{S,RL} + \frac{250}{9} \alpha_s^2 L_{ijkl}^{S,RL} - \frac{68}{9} \alpha_s \alpha L_{ijkl}^{S,RL} \\
& - \frac{8299}{81} \alpha^2 L_{ijkl}^{S,RL} ;
\end{aligned}$$



$$\begin{aligned}
\dot{L}_{duu}^{S,LL}{}_{ijkl} &= -4g_s^2 L_{duu}^{S,LL}{}_{ijkl} + e^2 \left[ -2L_{duu}^{S,LL}{}_{ijkl} - \frac{20}{3} L_{duu}^{S,LL}{}_{ikjl} \right] + \frac{370}{9} \alpha_s^2 L_{duu}^{S,LL}{}_{ijkl} \\
&\quad + \alpha_s \alpha \left[ \frac{20}{3} L_{duu}^{S,LL}{}_{ijkl} + 16L_{duu}^{S,LL}{}_{ikjl} \right] + \alpha^2 \left[ \frac{1165}{81} L_{duu}^{S,LL}{}_{ijkl} + \frac{9080}{81} L_{duu}^{S,LL}{}_{ikjl} \right] ; \\
\dot{L}_{duu}^{S,RR}{}_{ijkl} &= -4g_s^2 L_{duu}^{S,RR}{}_{ijkl} + e^2 \left[ -2L_{duu}^{S,RR}{}_{ijkl} - \frac{20}{3} L_{duu}^{S,RR}{}_{ikjl} \right] + \frac{370}{9} \alpha_s^2 L_{duu}^{S,RR}{}_{ijkl} \\
&\quad + \alpha_s \alpha \left[ \frac{20}{3} L_{duu}^{S,RR}{}_{ijkl} + 16L_{duu}^{S,RR}{}_{ikjl} \right] + \alpha^2 \left[ \frac{1165}{81} L_{duu}^{S,RR}{}_{ijkl} + \frac{9080}{81} L_{duu}^{S,RR}{}_{ikjl} \right] ; \\
\dot{L}_{duu}^{S,LR}{}_{ijkl} &= -4g_s^2 L_{duu}^{S,LR}{}_{ijkl} - \frac{16}{3} e^2 L_{duu}^{S,LR}{}_{ijkl} + \frac{250}{9} \alpha_s^2 L_{duu}^{S,LR}{}_{ijkl} + \frac{88}{9} \alpha_s \alpha L_{duu}^{S,LR}{}_{ijkl} \\
&\quad - \frac{184}{81} \alpha^2 L_{duu}^{S,LR}{}_{ijkl} ; \\
\dot{L}_{duu}^{S,RL}{}_{ijkl} &= -4g_s^2 L_{duu}^{S,RL}{}_{ijkl} - \frac{16}{3} e^2 L_{duu}^{S,RL}{}_{ijkl} + \frac{250}{9} \alpha_s^2 L_{duu}^{S,RL}{}_{ijkl} + \frac{88}{9} \alpha_s \alpha L_{duu}^{S,RL}{}_{ijkl} \\
&\quad - \frac{184}{81} \alpha^2 L_{duu}^{S,RL}{}_{ijkl} ;
\end{aligned}$$

## 2 Four Flavor LEFT

### 2.1 $\Delta F = 2$ Transitions ( $\bar{f}_i f_j \bar{f}_i f_j$ )

#### 2.1.1 $\Delta F = 2$ : $d$ -type ( $\bar{d}_i d_j \bar{d}_i d_j$ )

$$\begin{aligned}
\dot{L}_{dd,ijij}^{V,LL} &= 4g_s^2 L_{dd,ijij}^{V,LL} + \frac{4}{3}e^2 L_{dd,ijij}^{V,LL} - \frac{43}{9}\alpha_s^2 L_{dd,ijij}^{V,LL} - \frac{148}{9}\alpha_s\alpha L_{dd,ijij}^{V,LL} \\
&\quad + \frac{38}{81}\alpha^2 L_{dd,ijij}^{V,LL} ; \\
\dot{L}_{dd,ijij}^{V,RR} &= 4g_s^2 L_{dd,ijij}^{V,RR} + \frac{4}{3}e^2 L_{dd,ijij}^{V,RR} - \frac{43}{9}\alpha_s^2 L_{dd,ijij}^{V,RR} - \frac{148}{9}\alpha_s\alpha L_{dd,ijij}^{V,RR} \\
&\quad + \frac{38}{81}\alpha^2 L_{dd,ijij}^{V,RR} ; \\
\dot{L}_{dd,ijij}^{V1,LR} &= -\frac{8}{3}g_s^2 L_{dd,ijij}^{V8,LR} - \frac{4}{3}e^2 L_{dd,ijij}^{V1,LR} + \alpha_s^2 \left[ -\frac{28}{3}L_{dd,ijij}^{V1,LR} - \frac{2044}{27}L_{dd,ijij}^{V8,LR} \right] \\
&\quad + \alpha_s\alpha \left[ \frac{32}{3}L_{dd,ijij}^{V1,LR} - \frac{8}{27}L_{dd,ijij}^{V8,LR} \right] + \frac{1702}{81}\alpha^2 L_{dd,ijij}^{V1,LR} ; \\
\dot{L}_{dd,ijij}^{V8,LR} &= g_s^2 \left[ -12L_{dd,ijij}^{V1,LR} - 14L_{dd,ijij}^{V8,LR} \right] - \frac{4}{3}e^2 L_{dd,ijij}^{V8,LR} + \alpha_s^2 \left[ -\frac{374}{3}L_{dd,ijij}^{V1,LR} \right. \\
&\quad \left. - \frac{2975}{18}L_{dd,ijij}^{V8,LR} \right] + \alpha_s\alpha \left[ -\frac{4}{3}L_{dd,ijij}^{V1,LR} - \frac{26}{9}L_{dd,ijij}^{V8,LR} \right] + \frac{1702}{81}\alpha^2 L_{dd,ijij}^{V8,LR} ; \\
\dot{L}_{dd,ijij}^{S1,RR} &= g_s^2 \left[ \frac{160}{27}L_{dd,ijij}^{S8,RR} - \frac{80}{9}L_{dd,ijij}^{S1,RR} \right] + e^2 \left[ \frac{4}{27}L_{dd,ijij}^{S1,RR} + \frac{64}{81}L_{dd,ijij}^{S8,RR} \right] \\
&\quad + \alpha_s^2 \left[ \frac{19360}{243}L_{dd,ijij}^{S8,RR} - \frac{9608}{81}L_{dd,ijij}^{S1,RR} \right] + \alpha_s\alpha \left[ \frac{352}{243}L_{dd,ijij}^{S8,RR} - \frac{1040}{81}L_{dd,ijij}^{S1,RR} \right] \\
&\quad + \alpha^2 \left[ \frac{4354}{729}L_{dd,ijij}^{S1,RR} - \frac{3200}{2187}L_{dd,ijij}^{S8,RR} \right] ; \\
\dot{L}_{dd,ijij}^{S8,RR} &= g_s^2 \left[ \frac{8}{3}L_{dd,ijij}^{S1,RR} + \frac{92}{9}L_{dd,ijij}^{S8,RR} \right] + e^2 \left[ \frac{32}{9}L_{dd,ijij}^{S1,RR} - \frac{28}{27}L_{dd,ijij}^{S8,RR} \right] \\
&\quad + \alpha_s^2 \left[ \frac{6479}{81}L_{dd,ijij}^{S8,RR} - \frac{112}{27}L_{dd,ijij}^{S1,RR} \right] + \alpha_s\alpha \left[ -\frac{1840}{27}L_{dd,ijij}^{S1,RR} - \frac{208}{81}L_{dd,ijij}^{S8,RR} \right]
\end{aligned}$$

$$+ \alpha^2 \left[ \frac{5954}{729} L_{ijij}^{S8,RR} - \frac{1600}{243} L_{ijij}^{S1,RR} \right];$$

### 2.1.2 $\Delta F = 2$ : $u$ -type ( $\bar{u}_i u_j \bar{u}_i u_j$ )

$$\begin{aligned} \dot{L}_{ijij}^{V,LL} &= 4g_s^2 L_{ijij}^{V,LL} + \frac{16}{3} e^2 L_{ijij}^{V,LL} - \frac{43}{9} \alpha_s^2 L_{ijij}^{V,LL} - \frac{592}{9} \alpha_s \alpha L_{ijij}^{V,LL} \\ &\quad - \frac{1216}{81} \alpha^2 L_{ijij}^{V,LL}; \end{aligned}$$

$$\begin{aligned} \dot{L}_{ijij}^{V,RR} &= 4g_s^2 L_{ijij}^{V,RR} + \frac{16}{3} e^2 L_{ijij}^{V,RR} - \frac{43}{9} \alpha_s^2 L_{ijij}^{V,RR} - \frac{592}{9} \alpha_s \alpha L_{ijij}^{V,RR} \\ &\quad - \frac{1216}{81} \alpha^2 L_{ijij}^{V,RR}; \end{aligned}$$

$$\begin{aligned} \dot{L}_{ijij}^{V1,LR} &= -\frac{8}{3} g_s^2 L_{ijij}^{V8,LR} - \frac{16}{3} e^2 L_{ijij}^{V1,LR} + \alpha_s^2 \left[ -\frac{28}{3} L_{ijij}^{V1,LR} - \frac{2044}{27} L_{ijij}^{V8,LR} \right] \\ &\quad + \alpha_s \alpha \left[ \frac{128}{3} L_{ijij}^{V1,LR} - \frac{32}{27} L_{ijij}^{V8,LR} \right] + \frac{7168}{81} \alpha^2 L_{ijij}^{V1,LR}; \end{aligned}$$

$$\begin{aligned} \dot{L}_{ijij}^{V8,LR} &= g_s^2 \left[ -12 L_{ijij}^{V1,LR} - 14 L_{ijij}^{V8,LR} \right] - \frac{16}{3} e^2 L_{ijij}^{V8,LR} + \alpha_s^2 \left[ -\frac{374}{3} L_{ijij}^{V1,LR} \right. \\ &\quad \left. - \frac{2975}{18} L_{ijij}^{V8,LR} \right] + \alpha_s \alpha \left[ -\frac{16}{3} L_{ijij}^{V1,LR} - \frac{104}{9} L_{ijij}^{V8,LR} \right] + \frac{7168}{81} \alpha^2 L_{ijij}^{V8,LR}; \end{aligned}$$

$$\begin{aligned} \dot{L}_{ijij}^{S1,RR} &= g_s^2 \left[ \frac{160}{27} L_{ijij}^{S8,RR} - \frac{80}{9} L_{ijij}^{S1,RR} \right] + e^2 \left[ \frac{16}{27} L_{ijij}^{S1,RR} + \frac{256}{81} L_{ijij}^{S8,RR} \right] \\ &\quad + \alpha_s^2 \left[ \frac{19360}{243} L_{ijij}^{S8,RR} - \frac{9608}{81} L_{ijij}^{S1,RR} \right] + \alpha_s \alpha \left[ \frac{1408}{243} L_{ijij}^{S8,RR} - \frac{4160}{81} L_{ijij}^{S1,RR} \right] \\ &\quad + \alpha^2 \left[ \frac{5824}{729} L_{ijij}^{S1,RR} - \frac{22016}{2187} L_{ijij}^{S8,RR} \right]; \end{aligned}$$

$$\begin{aligned} \dot{L}_{ijij}^{S8,RR} &= g_s^2 \left[ \frac{8}{3} L_{ijij}^{S1,RR} + \frac{92}{9} L_{ijij}^{S8,RR} \right] + e^2 \left[ \frac{128}{9} L_{ijij}^{S1,RR} - \frac{112}{27} L_{ijij}^{S8,RR} \right] \\ &\quad + \alpha_s^2 \left[ \frac{6479}{81} L_{ijij}^{S8,RR} - \frac{112}{27} L_{ijij}^{S1,RR} \right] + \alpha_s \alpha \left[ -\frac{7360}{27} L_{ijij}^{S1,RR} - \frac{832}{81} L_{ijij}^{S8,RR} \right] \end{aligned}$$

$$+ \alpha^2 \left[ \frac{16832}{729} L_{ijij}^{S8,RR} - \frac{11008}{243} L_{ijij}^{S1,RR} \right];$$

### 2.1.3 $\Delta F = 2$ : $e$ -type ( $\bar{e}_i e_j \bar{e}_i e_j$ )

$$\dot{L}_{ijij}^{V,LL} = 12e^2 L_{ijij}^{V,LL} - \frac{874}{9} \alpha^2 L_{ijij}^{V,LL};$$

$$\dot{L}_{ijij}^{V,RR} = 12e^2 L_{ijij}^{V,RR} - \frac{874}{9} \alpha^2 L_{ijij}^{V,RR};$$

$$\dot{L}_{ijij}^{V,LR} = \frac{1942}{9} \alpha^2 L_{ijij}^{V,LR} - 12e^2 L_{ijij}^{V,LR};$$

$$\dot{L}_{ijij}^{S,RR} = 12e^2 L_{ijij}^{S,RR} - \frac{1066}{3} \alpha^2 L_{ijij}^{S,RR};$$

### 2.1.4 $\Delta F = 2$ : $\nu$ -type ( $\bar{\nu}_i \nu_j \bar{\nu}_i \nu_j$ )

$$\dot{L}_{ijij}^{V,LL} = 0;$$

## 2.2 $\Delta F = 1.5$ Transitions ( $\bar{f}_i f_j \bar{f}_k f_j$ )

### 2.2.1 $\Delta F = 1.5$ : $e$ -type ( $\bar{e}_i e_j \bar{e}_k e_j$ )

$$\dot{L}_{ijkj}^{V,LL} = 12e^2 L_{ijkj}^{V,LL} - \frac{874}{9} \alpha^2 L_{ijkj}^{V,LL};$$

$$\dot{L}_{ijkj}^{V,RR} = 12e^2 L_{ijkj}^{V,RR} - \frac{874}{9} \alpha^2 L_{ijkj}^{V,RR};$$

$$\dot{L}_{ijkj}^{V,LR} = \frac{1942}{9} \alpha^2 L_{ijkj}^{V,LR} - 12e^2 L_{ijkj}^{V,LR};$$

$$\dot{L}_{ijkj}^{S,RR} = 12e^2 L_{ijkj}^{S,RR} - \frac{1066}{3} \alpha^2 L_{ijkj}^{S,RR};$$

$$\dot{L}_{jijk}^{V,LL} = 12e^2 L_{jijk}^{V,LL} - \frac{874}{9} \alpha^2 L_{jijk}^{V,LL};$$

$$\dot{L}_{jijk}^{V,RR} = 12e^2 L_{jijk}^{V,RR} - \frac{874}{9} \alpha^2 L_{jijk}^{V,RR};$$

$$\dot{L}_{jijk}^{V,LR} = \frac{1942}{9} \alpha^2 L_{jijk}^{V,LR} - 12e^2 L_{jijk}^{V,LR};$$

$$\dot{L}_{jijk}^{S,RR} = 12e^2 L_{jijk}^{S,RR} - \frac{1066}{3} \alpha^2 L_{jijk}^{S,RR};$$

### 2.2.2 $\Delta F = 2$ : $\nu$ -type ( $\bar{\nu}_i \nu_j \bar{\nu}_k \nu_l$ )

$$\dot{L}_{\nu\nu}^{V,LL} = 0 ;$$

$$\dot{L}_{jj}^{V,LL} = 0 ;$$

## 2.3 $\Delta F = 1$ Transitions ( $\bar{f}_i f_j \bar{f}'_k f'_l$ )

### 2.3.1 $\Delta F = 1$ : $ud$ -type ( $\bar{u}_i u_j \bar{d}_k d_l$ )

$$\begin{aligned} \dot{L}_{ijkl}^{V1,LL} &= \frac{8}{3} g_s^2 L_{ijkl}^{V8,LL} - \frac{8}{3} e^2 L_{ijkl}^{V1,LL} + \alpha_s^2 \left[ \frac{82}{27} L_{ijkl}^{V8,LL} - \frac{28}{3} L_{ijkl}^{V1,LL} \right] \\ &\quad + \alpha_s \alpha \left[ \frac{64}{3} L_{ijkl}^{V1,LL} - \frac{8}{27} L_{ijkl}^{V8,LL} \right] - \frac{112}{81} \alpha^2 L_{ijkl}^{V1,LL} ; \\ \dot{L}_{ijkl}^{V8,LL} &= g_s^2 \left[ 12 L_{ijkl}^{V1,LL} - 4 L_{ijkl}^{V8,LL} \right] - \frac{8}{3} e^2 L_{ijkl}^{V8,LL} + \alpha_s^2 \left[ \frac{41}{3} L_{ijkl}^{V1,LL} \right. \\ &\quad \left. - \frac{125}{9} L_{ijkl}^{V8,LL} \right] + \alpha_s \alpha \left[ -\frac{4}{3} L_{ijkl}^{V1,LL} - \frac{47}{9} L_{ijkl}^{V8,LL} \right] - \frac{112}{81} \alpha^2 L_{ijkl}^{V8,LL} ; \\ \dot{L}_{ijkl}^{V1,RR} &= \frac{8}{3} g_s^2 L_{ijkl}^{V8,RR} - \frac{8}{3} e^2 L_{ijkl}^{V1,RR} + \alpha_s^2 \left[ \frac{82}{27} L_{ijkl}^{V8,RR} - \frac{28}{3} L_{ijkl}^{V1,RR} \right] \\ &\quad + \alpha_s \alpha \left[ \frac{64}{3} L_{ijkl}^{V1,RR} - \frac{8}{27} L_{ijkl}^{V8,RR} \right] - \frac{112}{81} \alpha^2 L_{ijkl}^{V1,RR} ; \\ \dot{L}_{ijkl}^{V8,RR} &= g_s^2 \left[ 12 L_{ijkl}^{V1,RR} - 4 L_{ijkl}^{V8,RR} \right] - \frac{8}{3} e^2 L_{ijkl}^{V8,RR} + \alpha_s^2 \left[ \frac{41}{3} L_{ijkl}^{V1,RR} \right. \\ &\quad \left. - \frac{125}{9} L_{ijkl}^{V8,RR} \right] + \alpha_s \alpha \left[ -\frac{4}{3} L_{ijkl}^{V1,RR} - \frac{47}{9} L_{ijkl}^{V8,RR} \right] - \frac{112}{81} \alpha^2 L_{ijkl}^{V8,RR} ; \\ \dot{L}_{ijkl}^{V1,LR} &= -\frac{8}{3} g_s^2 L_{ijkl}^{V8,LR} + \frac{8}{3} e^2 L_{ijkl}^{V1,LR} + \alpha_s^2 \left[ -\frac{28}{3} L_{ijkl}^{V1,LR} - \frac{2044}{27} L_{ijkl}^{V8,LR} \right] \\ &\quad + \alpha_s \alpha \left[ \frac{232}{27} L_{ijkl}^{V8,LR} - \frac{64}{3} L_{ijkl}^{V1,LR} \right] - \frac{3872}{81} \alpha^2 L_{ijkl}^{V1,LR} ; \end{aligned}$$

$$\begin{aligned}
\dot{L}_{ijkl}^{V8,LR} &= g_s^2 \left[ -12L_{ijkl}^{V1,LR} - 14L_{ijkl}^{V8,LR} \right] + \frac{8}{3}e^2 L_{ijkl}^{V8,LR} + \alpha_s^2 \left[ -\frac{374}{3}L_{ijkl}^{V1,LR} \right. \\
&\quad \left. - \frac{2975}{18}L_{ijkl}^{V8,LR} \right] + \alpha_s \alpha \left[ \frac{116}{3}L_{ijkl}^{V1,LR} + \frac{187}{9}L_{ijkl}^{V8,LR} \right] - \frac{3872}{81}\alpha^2 L_{ijkl}^{V8,LR} ; \\
\dot{L}_{klij}^{V1,LR} &= -\frac{8}{3}g_s^2 L_{klij}^{V8,LR} + \frac{8}{3}e^2 L_{klij}^{V1,LR} + \alpha_s^2 \left[ -\frac{28}{3}L_{klij}^{V1,LR} - \frac{2044}{27}L_{klij}^{V8,LR} \right] \\
&\quad + \alpha_s \alpha \left[ \frac{232}{27}L_{klij}^{V8,LR} - \frac{64}{3}L_{klij}^{V1,LR} \right] - \frac{3872}{81}\alpha^2 L_{klij}^{V1,LR} ; \\
\dot{L}_{klij}^{V8,LR} &= g_s^2 \left[ -12L_{klij}^{V1,LR} - 14L_{klij}^{V8,LR} \right] + \frac{8}{3}e^2 L_{klij}^{V8,LR} + \alpha_s^2 \left[ -\frac{374}{3}L_{klij}^{V1,LR} \right. \\
&\quad \left. - \frac{2975}{18}L_{klij}^{V8,LR} \right] + \alpha_s \alpha \left[ \frac{116}{3}L_{klij}^{V1,LR} + \frac{187}{9}L_{klij}^{V8,LR} \right] - \frac{3872}{81}\alpha^2 L_{klij}^{V8,LR} ; \\
\dot{L}_{ilkj}^{V1,LR} &= -\frac{8}{3}g_s^2 L_{ilkj}^{V8,LR} - \frac{10}{3}e^2 L_{ilkj}^{V1,LR} + \alpha_s^2 \left[ -\frac{28}{3}L_{ilkj}^{V1,LR} - \frac{2044}{27}L_{ilkj}^{V8,LR} \right] \\
&\quad + \alpha_s \alpha \left[ \frac{8}{3}L_{ilkj}^{V1,LR} - \frac{128}{27}L_{ilkj}^{V8,LR} \right] + \frac{169}{81}\alpha^2 L_{ilkj}^{V1,LR} ; \\
\dot{L}_{ilkj}^{V8,LR} &= g_s^2 \left[ -12L_{ilkj}^{V1,LR} - 14L_{ilkj}^{V8,LR} \right] - \frac{10}{3}e^2 L_{ilkj}^{V8,LR} + \alpha_s^2 \left[ -\frac{374}{3}L_{ilkj}^{V1,LR} \right. \\
&\quad \left. - \frac{2975}{18}L_{ilkj}^{V8,LR} \right] + \alpha_s \alpha \left[ \frac{16}{9}L_{ilkj}^{V8,LR} - \frac{64}{3}L_{ilkj}^{V1,LR} \right] + \frac{169}{81}\alpha^2 L_{ilkj}^{V8,LR} ; \\
\dot{L}_{ijkl}^{S1,RR} &= g_s^2 \left[ \frac{64}{9}L_{ilkj}^{S1,RR} + \frac{112}{27}L_{ilkj}^{S8,RR} - 16L_{ijkl}^{S1,RR} + \frac{16}{9}L_{ijkl}^{S8,RR} \right] \\
&\quad + e^2 \left[ \frac{4}{27}L_{ilkj}^{S1,RR} + \frac{16}{81}L_{ilkj}^{S8,RR} - \frac{46}{9}L_{ijkl}^{S1,RR} \right] + \alpha_s^2 \left[ \frac{9472}{81}L_{ilkj}^{S1,RR} + \frac{16576}{243}L_{ilkj}^{S8,RR} \right. \\
&\quad \left. - \frac{2120}{9}L_{ijkl}^{S1,RR} + \frac{928}{81}L_{ijkl}^{S8,RR} \right] + \alpha_s \alpha \left[ \frac{1888}{81}L_{ilkj}^{S1,RR} + \frac{3808}{243}L_{ilkj}^{S8,RR} + \frac{136}{27}L_{ijkl}^{S1,RR} \right. \\
&\quad \left. + \frac{224}{81}L_{ijkl}^{S8,RR} \right] + \alpha^2 \left[ \frac{106}{729}L_{ilkj}^{S1,RR} + \frac{424}{2187}L_{ilkj}^{S8,RR} + \frac{6059}{243}L_{ijkl}^{S1,RR} \right] ;
\end{aligned}$$

$$\begin{aligned}
\dot{L}_{ud}^{S8,RR}{}_{ijkl} &= g_s^2 \left[ -\frac{16}{3} L_{uddu}^{S1,RR}{}_{ilkj} + \frac{44}{9} L_{uddu}^{S8,RR}{}_{ilkj} + 8 L_{ud}^{S1,RR}{}_{ijkl} + \frac{16}{3} L_{ud}^{S8,RR}{}_{ijkl} \right] \\
&+ e^2 \left[ \frac{8}{9} L_{uddu}^{S1,RR}{}_{ilkj} - \frac{4}{27} L_{uddu}^{S8,RR}{}_{ilkj} - \frac{46}{9} L_{ud}^{S8,RR}{}_{ijkl} \right] + \alpha_s^2 \left[ -\frac{856}{27} L_{uddu}^{S1,RR}{}_{ilkj} - \frac{2506}{81} L_{uddu}^{S8,RR}{}_{ilkj} \right. \\
&+ \frac{248}{9} L_{ud}^{S1,RR}{}_{ijkl} + \frac{2995}{27} L_{ud}^{S8,RR}{}_{ijkl} \left. \right] + \alpha_s \alpha \left[ -\frac{868}{27} L_{uddu}^{S1,RR}{}_{ilkj} + \frac{1370}{81} L_{uddu}^{S8,RR}{}_{ilkj} + \frac{112}{9} L_{ud}^{S1,RR}{}_{ijkl} \right. \\
&+ \left. \frac{224}{9} L_{ud}^{S8,RR}{}_{ijkl} \right] + \alpha^2 \left[ \frac{212}{243} L_{uddu}^{S1,RR}{}_{ilkj} - \frac{106}{729} L_{uddu}^{S8,RR}{}_{ilkj} + \frac{6059}{243} L_{ud}^{S8,RR}{}_{ijkl} \right];
\end{aligned}$$

$$\begin{aligned}
\dot{L}_{uddu}^{S1,RR}{}_{ilkj} &= g_s^2 \left[ -16 L_{uddu}^{S1,RR}{}_{ilkj} + \frac{16}{9} L_{uddu}^{S8,RR}{}_{ilkj} + \frac{64}{9} L_{ud}^{S1,RR}{}_{ijkl} + \frac{112}{27} L_{ud}^{S8,RR}{}_{ijkl} \right] \\
&+ e^2 \left[ \frac{26}{9} L_{uddu}^{S1,RR}{}_{ilkj} - \frac{32}{27} L_{ud}^{S1,RR}{}_{ijkl} - \frac{128}{81} L_{ud}^{S8,RR}{}_{ijkl} \right] + \alpha_s^2 \left[ -\frac{2120}{9} L_{uddu}^{S1,RR}{}_{ilkj} + \frac{928}{81} L_{uddu}^{S8,RR}{}_{ilkj} \right. \\
&+ \frac{9472}{81} L_{ud}^{S1,RR}{}_{ijkl} + \frac{16576}{243} L_{ud}^{S8,RR}{}_{ijkl} \left. \right] + \alpha_s \alpha \left[ \frac{712}{27} L_{uddu}^{S1,RR}{}_{ilkj} - \frac{64}{81} L_{uddu}^{S8,RR}{}_{ilkj} - \frac{2144}{81} L_{ud}^{S1,RR}{}_{ijkl} \right. \\
&- \left. \frac{7784}{243} L_{ud}^{S8,RR}{}_{ijkl} \right] + \alpha^2 \left[ -\frac{13201}{243} L_{uddu}^{S1,RR}{}_{ilkj} + \frac{5200}{729} L_{ud}^{S1,RR}{}_{ijkl} + \frac{20800}{2187} L_{ud}^{S8,RR}{}_{ijkl} \right];
\end{aligned}$$

$$\begin{aligned}
\dot{L}_{uddu}^{S8,RR}{}_{ilkj} &= g_s^2 \left[ 8 L_{uddu}^{S1,RR}{}_{ilkj} + \frac{16}{3} L_{uddu}^{S8,RR}{}_{ilkj} - \frac{16}{3} L_{ud}^{S1,RR}{}_{ijkl} + \frac{44}{9} L_{ud}^{S8,RR}{}_{ijkl} \right] \\
&+ e^2 \left[ \frac{26}{9} L_{uddu}^{S8,RR}{}_{ilkj} - \frac{64}{9} L_{ud}^{S1,RR}{}_{ijkl} + \frac{32}{27} L_{ud}^{S8,RR}{}_{ijkl} \right] + \alpha_s^2 \left[ \frac{248}{9} L_{uddu}^{S1,RR}{}_{ilkj} + \frac{2995}{27} L_{uddu}^{S8,RR}{}_{ilkj} \right. \\
&- \frac{856}{27} L_{ud}^{S1,RR}{}_{ijkl} - \frac{2506}{81} L_{ud}^{S8,RR}{}_{ijkl} \left. \right] + \alpha_s \alpha \left[ -\frac{32}{9} L_{uddu}^{S1,RR}{}_{ilkj} - \frac{400}{9} L_{uddu}^{S8,RR}{}_{ilkj} + \frac{3704}{27} L_{ud}^{S1,RR}{}_{ijkl} \right. \\
&- \left. \frac{2050}{81} L_{ud}^{S8,RR}{}_{ijkl} \right] + \alpha^2 \left[ -\frac{13201}{243} L_{uddu}^{S8,RR}{}_{ilkj} + \frac{10400}{243} L_{ud}^{S1,RR}{}_{ijkl} - \frac{5200}{729} L_{ud}^{S8,RR}{}_{ijkl} \right];
\end{aligned}$$

### 2.3.2 $\Delta F = 1$ : *ed*-type ( $\bar{e}_i e_j \bar{d}_k d_l$ )

$$\dot{L}_{ed}^{V,LL}{}_{ijkl} = 4e^2 L_{ed}^{V,LL}{}_{ijkl} - 16\alpha_s \alpha L_{ed}^{V,LL}{}_{ijkl} - \frac{334}{27} \alpha^2 L_{ed}^{V,LL}{}_{ijkl};$$

$$\dot{L}_{ed}^{V,RR}{}_{ijkl} = 4e^2 L_{ed}^{V,RR}{}_{ijkl} - 16\alpha_s \alpha L_{ed}^{V,RR}{}_{ijkl} - \frac{334}{27} \alpha^2 L_{ed}^{V,RR}{}_{ijkl};$$

$$\begin{aligned}
\dot{L}_{ed\,ijkl}^{V,LR} &= -4e^2 L_{ed\,ijkl}^{V,LR} + 16\alpha_s \alpha L_{ed\,ijkl}^{V,LR} + \frac{1906}{27} \alpha^2 L_{ed\,ijkl}^{V,LR} ; \\
\dot{L}_{de\,klij}^{V,LR} &= -4e^2 L_{de\,klij}^{V,LR} + 16\alpha_s \alpha L_{de\,klij}^{V,LR} + \frac{1906}{27} \alpha^2 L_{de\,klij}^{V,LR} ; \\
\dot{L}_{ed\,ijkl}^{S,RL} &= -8g_s^2 L_{ed\,ijkl}^{S,RL} - \frac{20}{3} e^2 L_{ed\,ijkl}^{S,RL} - \frac{1012}{9} \alpha_s^2 L_{ed\,ijkl}^{S,RL} - \frac{8}{9} \alpha_s \alpha L_{ed\,ijkl}^{S,RL} \\
&\quad + \frac{6614}{81} \alpha^2 L_{ed\,ijkl}^{S,RL} ; \\
\dot{L}_{ed\,ijkl}^{S,RR} &= -8g_s^2 L_{ed\,ijkl}^{S,RR} + e^2 \left[ -\frac{20}{3} L_{ed\,ijkl}^{S,RR} - 32 L_{ed\,ijkl}^{T,RR} \right] - \frac{1012}{9} \alpha_s^2 L_{ed\,ijkl}^{S,RR} \\
&\quad + \alpha_s \alpha \left[ \frac{1792}{9} L_{ed\,ijkl}^{T,RR} - \frac{8}{9} L_{ed\,ijkl}^{S,RR} \right] + \alpha^2 \left[ \frac{1682}{81} L_{ed\,ijkl}^{S,RR} + 704 L_{ed\,ijkl}^{T,RR} \right] ; \\
\dot{L}_{ed\,ijkl}^{T,RR} &= \frac{8}{3} g_s^2 L_{ed\,ijkl}^{T,RR} + e^2 \left[ \frac{20}{9} L_{ed\,ijkl}^{T,RR} - \frac{2}{3} L_{ed\,ijkl}^{S,RR} \right] + \frac{1652}{27} \alpha_s^2 L_{ed\,ijkl}^{T,RR} \\
&\quad + \alpha_s \alpha \left[ \frac{16}{3} L_{ed\,ijkl}^{S,RR} - \frac{152}{27} L_{ed\,ijkl}^{T,RR} \right] + \alpha^2 \left[ \frac{364}{81} L_{ed\,ijkl}^{S,RR} - \frac{6922}{243} L_{ed\,ijkl}^{T,RR} \right] ;
\end{aligned}$$

### 2.3.3 $\Delta F = 1$ : $eu$ -type ( $\bar{e}_i e_j \bar{u}_k u_l$ )

$$\begin{aligned}
\dot{L}_{eu\,ijkl}^{V,LL} &= -8e^2 L_{eu\,ijkl}^{V,LL} + 32\alpha_s \alpha L_{eu\,ijkl}^{V,LL} + \frac{128}{27} \alpha^2 L_{eu\,ijkl}^{V,LL} ; \\
\dot{L}_{eu\,ijkl}^{V,RR} &= -8e^2 L_{eu\,ijkl}^{V,RR} + 32\alpha_s \alpha L_{eu\,ijkl}^{V,RR} + \frac{128}{27} \alpha^2 L_{eu\,ijkl}^{V,RR} ; \\
\dot{L}_{eu\,ijkl}^{V,LR} &= 8e^2 L_{eu\,ijkl}^{V,LR} - 32\alpha_s \alpha L_{eu\,ijkl}^{V,LR} - \frac{4784}{27} \alpha^2 L_{eu\,ijkl}^{V,LR} ; \\
\dot{L}_{ue\,klij}^{V,LR} &= 8e^2 L_{ue\,klij}^{V,LR} - 32\alpha_s \alpha L_{ue\,klij}^{V,LR} - \frac{4784}{27} \alpha^2 L_{ue\,klij}^{V,LR} ; \\
\dot{L}_{eu\,ijkl}^{S,RL} &= -8g_s^2 L_{eu\,ijkl}^{S,RL} - \frac{26}{3} e^2 L_{eu\,ijkl}^{S,RL} - \frac{1012}{9} \alpha_s^2 L_{eu\,ijkl}^{S,RL} - \frac{32}{9} \alpha_s \alpha L_{eu\,ijkl}^{S,RL} \\
&\quad + \frac{473}{81} \alpha^2 L_{eu\,ijkl}^{S,RL} ; \\
\dot{L}_{eu\,ijkl}^{S,RR} &= -8g_s^2 L_{eu\,ijkl}^{S,RR} + e^2 \left[ 64 L_{eu\,ijkl}^{T,RR} - \frac{26}{3} L_{eu\,ijkl}^{S,RR} \right] - \frac{1012}{9} \alpha_s^2 L_{eu\,ijkl}^{S,RR}
\end{aligned}$$



$$\begin{aligned}
& + \alpha_s \alpha \left[ -\frac{32}{9} L_{ijkl}^{S,RR} - \frac{3584}{9} L_{ijkl}^{T,RR} \right] + \alpha^2 \left[ -\frac{2839}{81} L_{ijkl}^{S,RR} - \frac{11264}{9} L_{ijkl}^{T,RR} \right] ; \\
\dot{L}_{ijkl}^{T,RR} &= \frac{8}{3} g_s^2 L_{ijkl}^{T,RR} + e^2 \left[ \frac{4}{3} L_{ijkl}^{S,RR} + \frac{26}{9} L_{ijkl}^{T,RR} \right] + \frac{1652}{27} \alpha_s^2 L_{ijkl}^{T,RR} \\
& + \alpha_s \alpha \left[ -\frac{32}{3} L_{ijkl}^{S,RR} - \frac{608}{27} L_{ijkl}^{T,RR} \right] + \alpha^2 \left[ -\frac{1376}{81} L_{ijkl}^{S,RR} - \frac{20677}{243} L_{ijkl}^{T,RR} \right] ;
\end{aligned}$$

### 2.3.4 $\Delta F = 1$ : $\nu d$ -type ( $\bar{\nu}_i \nu_j \bar{d}_k d_l$ )

$$\dot{L}_{ijkl}^{V,LL} = 0 ;$$

$$\dot{L}_{ijkl}^{V,LR} = 0 ;$$

### 2.3.5 $\Delta F = 1$ : $\nu u$ -type ( $\bar{\nu}_i \nu_j \bar{u}_k u_l$ )

$$\dot{L}_{ijkl}^{V,LL} = 0 ;$$

$$\dot{L}_{ijkl}^{V,LR} = 0 ;$$

### 2.3.6 $\Delta F = 1$ : $\nu e$ -type ( $\bar{\nu}_i \nu_j \bar{e}_k e_l$ )

$$\dot{L}_{ijkl}^{V,LL} = 0 ;$$

$$\dot{L}_{ijkl}^{V,LR} = 0 ;$$

### 2.3.7 $\Delta F = 1$ : $\nu edu$ -type ( $\bar{\nu}_i e_j \bar{d}_k u_l$ )

$$\dot{L}_{ijkl}^{V,LL} = -4e^2 L_{ijkl}^{V,LL} + 4\alpha_s \alpha L_{ijkl}^{V,LL} - \frac{152}{27} \alpha^2 L_{ijkl}^{V,LL} ;$$

$$\dot{L}_{ijkl}^{V,LR} = -2e^2 L_{ijkl}^{V,LR} - 4\alpha_s \alpha L_{ijkl}^{V,LR} - \frac{469}{27} \alpha^2 L_{ijkl}^{V,LR} ;$$

$$\begin{aligned}
\dot{L}_{ijkl}^{S,RL} &= -8g_s^2 L_{ijkl}^{S,RL} + \frac{4}{3} e^2 L_{ijkl}^{S,RL} - \frac{1012}{9} \alpha_s^2 L_{ijkl}^{S,RL} + 12\alpha_s \alpha L_{ijkl}^{S,RL} \\
& - \frac{3832}{81} \alpha^2 L_{ijkl}^{S,RL} ;
\end{aligned}$$

$$\begin{aligned}
\dot{L}_{ijkl}^{S,RR} &= -8g_s^2 L_{ijkl}^{S,RR} + e^2 \left[ \frac{4}{3} L_{ijkl}^{S,RR} + 8 L_{ijkl}^{T,RR} \right] - \frac{1012}{9} \alpha_s^2 L_{ijkl}^{S,RR} \\
&\quad + \alpha_s \alpha \left[ 12 L_{ijkl}^{S,RR} - \frac{448}{9} L_{ijkl}^{T,RR} \right] + \alpha^2 \left[ -\frac{3805}{81} L_{ijkl}^{S,RR} - \frac{1064}{9} L_{ijkl}^{T,RR} \right]; \\
\dot{L}_{\nu edu}^{T,RR} &= \frac{8}{3} g_s^2 L_{\nu edu}^{T,RR} + e^2 \left[ \frac{1}{6} L_{\nu edu}^{S,RR} - \frac{40}{9} L_{\nu edu}^{T,RR} \right] + \frac{1652}{27} \alpha_s^2 L_{\nu edu}^{T,RR} \\
&\quad + \alpha_s \alpha \left[ \frac{4}{3} L_{\nu edu}^{T,RR} - \frac{4}{3} L_{\nu edu}^{S,RR} \right] + \alpha^2 \left[ \frac{3773}{243} L_{\nu edu}^{T,RR} - \frac{11}{162} L_{\nu edu}^{S,RR} \right];
\end{aligned}$$

## 2.4 $\Delta F = 1^{\bar{f}f}$ Transitions ( $\bar{f}_i f_j \bar{f}'_k f'_k$ )

## 2.5 $\Delta F = 1^{\bar{f}f}$ : $d$ -type ( $\bar{d}_i d_j \bar{f}_k f_k$ )

$$\begin{aligned}
\dot{L}_{11ij}^{V,LL} &= e^2 \left[ \frac{4}{3} L_{ijii}^{V1,LR} + \frac{4}{3} L_{ijjj}^{V1,LR} + \frac{32}{9} L_{ijii}^{V,LL} + \frac{32}{9} L_{ijjj}^{V,LL} + \frac{4}{3} L_{ij11}^{V,LR} \right. \\
&\quad + \frac{4}{3} L_{ij22}^{V,LR} + \frac{4}{3} L_{ij33}^{V,LR} - \frac{8}{3} L_{ij11}^{V1,LR} - \frac{8}{3} L_{ij22}^{V1,LR} + \frac{16}{3} L_{11ij}^{V,LL} + \frac{4}{3} L_{22ij}^{V,LL} \\
&\quad + \frac{4}{3} L_{33ij}^{V,LL} - \frac{8}{3} L_{11ij}^{V1,LL} - \frac{8}{3} L_{22ij}^{V1,LL} \left. \right] + \alpha_s \alpha \left[ \frac{16}{3} L_{ijii}^{V1,LR} + \frac{16}{3} L_{ijjj}^{V1,LR} \right. \\
&\quad - \frac{992}{243} L_{ijii}^{V8,LR} - \frac{992}{243} L_{ijjj}^{V8,LR} + \frac{1120}{81} L_{ijii}^{V,LL} + \frac{1120}{81} L_{ijjj}^{V,LL} - \frac{32}{3} L_{ij11}^{V1,LR} - \frac{32}{3} L_{ij22}^{V1,LR} \\
&\quad + \frac{1384}{243} L_{ij11}^{V8,LR} + \frac{1384}{243} L_{ij22}^{V8,LR} - 16 L_{11ij}^{V,LL} - \frac{32}{3} L_{11ij}^{V1,LL} - \frac{32}{3} L_{22ij}^{V1,LL} - \frac{56}{243} L_{11ij}^{V8,LL} \\
&\quad - \frac{56}{243} L_{22ij}^{V8,LL} \left. \right] + \alpha^2 \left[ -\frac{1288}{243} L_{ijii}^{V1,LR} - \frac{1288}{243} L_{ijjj}^{V1,LR} + \frac{4864}{243} L_{ijii}^{V,LL} + \frac{4864}{243} L_{ijjj}^{V,LL} \right. \\
&\quad - \frac{3160}{243} L_{ij11}^{V,LR} - \frac{3160}{243} L_{ij22}^{V,LR} - \frac{3160}{243} L_{ij33}^{V,LR} - \frac{6280}{243} L_{ij11}^{V1,LR} - \frac{6280}{243} L_{ij22}^{V1,LR} \\
&\quad + \frac{746}{243} L_{11ij}^{V,LL} + \frac{3752}{243} L_{22ij}^{V,LL} + \frac{3752}{243} L_{33ij}^{V,LL} + \frac{2936}{243} L_{11ij}^{V1,LL} + \frac{2936}{243} L_{22ij}^{V1,LL} \left. \right]; \\
\dot{L}_{22ij}^{V,LL} &= e^2 \left[ \frac{4}{3} L_{ijii}^{V1,LR} + \frac{4}{3} L_{ijjj}^{V1,LR} + \frac{32}{9} L_{ijii}^{V,LL} + \frac{32}{9} L_{ijjj}^{V,LL} + \frac{4}{3} L_{ij11}^{V,LR} \right.
\end{aligned}$$

$$\begin{aligned}
& + \frac{4}{3}L_{ij22}^{V,LR} + \frac{4}{3}L_{ij33}^{V,LR} - \frac{8}{3}L_{ij11}^{V1,LR} - \frac{8}{3}L_{ij22}^{V1,LR} + \frac{4}{3}L_{11ij}^{V,LL} + \frac{16}{3}L_{22ij}^{V,LL} \\
& + \frac{4}{3}L_{33ij}^{V,LL} - \frac{8}{3}L_{11ij}^{V1,LL} - \frac{8}{3}L_{22ij}^{V1,LL} \Big] + \alpha_s \alpha \Big[ \frac{16}{3}L_{ijii}^{V1,LR} + \frac{16}{3}L_{ijjj}^{V1,LR} \\
& - \frac{992}{243}L_{ijii}^{V8,LR} - \frac{992}{243}L_{ijjj}^{V8,LR} + \frac{1120}{81}L_{ijii}^{V,LL} + \frac{1120}{81}L_{ijjj}^{V,LL} - \frac{32}{3}L_{ij11}^{V1,LR} - \frac{32}{3}L_{ij22}^{V1,LR} \\
& + \frac{1384}{243}L_{ij11}^{V8,LR} + \frac{1384}{243}L_{ij22}^{V8,LR} - 16L_{22ij}^{V,LL} - \frac{32}{3}L_{11ij}^{V1,LL} - \frac{32}{3}L_{22ij}^{V1,LL} - \frac{56}{243}L_{11ij}^{V8,LL} \\
& - \frac{56}{243}L_{22ij}^{V8,LL} \Big] + \alpha^2 \Big[ -\frac{1288}{243}L_{ijii}^{V1,LR} - \frac{1288}{243}L_{ijjj}^{V1,LR} + \frac{4864}{243}L_{ijii}^{V,LL} + \frac{4864}{243}L_{ijjj}^{V,LL} \\
& - \frac{3160}{243}L_{ij11}^{V,LR} - \frac{3160}{243}L_{ij22}^{V,LR} - \frac{3160}{243}L_{ij33}^{V,LR} - \frac{6280}{243}L_{ij11}^{V1,LR} - \frac{6280}{243}L_{ij22}^{V1,LR} \\
& + \frac{3752}{243}L_{11ij}^{V,LL} + \frac{746}{243}L_{22ij}^{V,LL} + \frac{3752}{243}L_{33ij}^{V,LL} + \frac{2936}{243}L_{11ij}^{V1,LL} + \frac{2936}{243}L_{22ij}^{V1,LL} \Big] ;
\end{aligned}$$

$$\begin{aligned}
\dot{L}_{33ij}^{V,LL} &= e^2 \Big[ \frac{4}{3}L_{ijii}^{V1,LR} + \frac{4}{3}L_{ijjj}^{V1,LR} + \frac{32}{9}L_{ijii}^{V,LL} + \frac{32}{9}L_{ijjj}^{V,LL} + \frac{4}{3}L_{ij11}^{V,LR} \\
& + \frac{4}{3}L_{ij22}^{V,LR} + \frac{4}{3}L_{ij33}^{V,LR} - \frac{8}{3}L_{ij11}^{V1,LR} - \frac{8}{3}L_{ij22}^{V1,LR} + \frac{4}{3}L_{11ij}^{V,LL} + \frac{4}{3}L_{22ij}^{V,LL} \\
& + \frac{16}{3}L_{33ij}^{V,LL} - \frac{8}{3}L_{11ij}^{V1,LL} - \frac{8}{3}L_{22ij}^{V1,LL} \Big] + \alpha_s \alpha \Big[ \frac{16}{3}L_{ijii}^{V1,LR} + \frac{16}{3}L_{ijjj}^{V1,LR} \\
& - \frac{992}{243}L_{ijii}^{V8,LR} - \frac{992}{243}L_{ijjj}^{V8,LR} + \frac{1120}{81}L_{ijii}^{V,LL} + \frac{1120}{81}L_{ijjj}^{V,LL} - \frac{32}{3}L_{ij11}^{V1,LR} - \frac{32}{3}L_{ij22}^{V1,LR} \\
& + \frac{1384}{243}L_{ij11}^{V8,LR} + \frac{1384}{243}L_{ij22}^{V8,LR} - 16L_{33ij}^{V,LL} - \frac{32}{3}L_{11ij}^{V1,LL} - \frac{32}{3}L_{22ij}^{V1,LL} - \frac{56}{243}L_{11ij}^{V8,LL} \\
& - \frac{56}{243}L_{22ij}^{V8,LL} \Big] + \alpha^2 \Big[ -\frac{1288}{243}L_{ijii}^{V1,LR} - \frac{1288}{243}L_{ijjj}^{V1,LR} + \frac{4864}{243}L_{ijii}^{V,LL} + \frac{4864}{243}L_{ijjj}^{V,LL} \\
& - \frac{3160}{243}L_{ij11}^{V,LR} - \frac{3160}{243}L_{ij22}^{V,LR} - \frac{3160}{243}L_{ij33}^{V,LR} - \frac{6280}{243}L_{ij11}^{V1,LR} - \frac{6280}{243}L_{ij22}^{V1,LR} \\
& + \frac{3752}{243}L_{11ij}^{V,LL} + \frac{3752}{243}L_{22ij}^{V,LL} + \frac{746}{243}L_{33ij}^{V,LL} + \frac{2936}{243}L_{11ij}^{V1,LL} + \frac{2936}{243}L_{22ij}^{V1,LL} \Big] ;
\end{aligned}$$

$$\dot{L}_{11ij}^{V1,LL} = \frac{8}{3}g_s^2 L_{11ij}^{V8,LL} + e^2 \Big[ -\frac{8}{9}L_{ijii}^{V1,LR} - \frac{8}{9}L_{ijjj}^{V1,LR} - \frac{64}{27}L_{ijii}^{V,LL} - \frac{64}{27}L_{ijjj}^{V,LL}$$

$$\begin{aligned}
& -\frac{8}{9}L_{ij11}^{V,LR} - \frac{8}{9}L_{ij22}^{V,LR} - \frac{8}{9}L_{ij33}^{V,LR} + \frac{16}{9}L_{ij11}^{V1,LR} + \frac{16}{9}L_{ij22}^{V1,LR} - \frac{8}{9}L_{11ij}^{V,LL} \\
& - \frac{8}{9}L_{22ij}^{V,LL} - \frac{8}{9}L_{33ij}^{V,LL} - \frac{8}{9}L_{11ij}^{V1,LL} + \frac{16}{9}L_{22ij}^{V1,LL} \Big] + \alpha_s^2 \Big[ -8L_{ijii}^{V1,LR} \\
& - 8L_{ijjj}^{V1,LR} + \frac{4}{27}L_{ijii}^{V8,LR} + \frac{4}{27}L_{ijjj}^{V8,LR} + \frac{328}{9}L_{ijii}^{V,LL} + \frac{328}{9}L_{ijjj}^{V,LL} - 8L_{ij11}^{V1,LR} \\
& - 8L_{ij22}^{V1,LR} + \frac{4}{27}L_{ij11}^{V8,LR} + \frac{4}{27}L_{ij22}^{V8,LR} - \frac{4}{3}L_{11ij}^{V1,LL} + 8L_{22ij}^{V1,LL} + \frac{86}{27}L_{11ij}^{V8,LL} \\
& + \frac{4}{27}L_{22ij}^{V8,LL} \Big] + \alpha_s \alpha \Big[ -\frac{32}{9}L_{ijii}^{V1,LR} - \frac{32}{9}L_{ijjj}^{V1,LR} + \frac{1984}{729}L_{ijii}^{V8,LR} + \frac{1984}{729}L_{ijjj}^{V8,LR} \\
& - \frac{2240}{243}L_{ijii}^{V,LL} - \frac{2240}{243}L_{ijjj}^{V,LL} + \frac{64}{9}L_{ij11}^{V1,LR} + \frac{64}{9}L_{ij22}^{V1,LR} - \frac{2768}{729}L_{ij11}^{V8,LR} - \frac{2768}{729}L_{ij22}^{V8,LR} \\
& + \frac{256}{9}L_{11ij}^{V1,LL} + \frac{64}{9}L_{22ij}^{V1,LL} - \frac{104}{729}L_{11ij}^{V8,LL} + \frac{112}{729}L_{22ij}^{V8,LL} \Big] + \alpha^2 \Big[ -\frac{304}{729}L_{ijii}^{V1,LR} \\
& - \frac{304}{729}L_{ijjj}^{V1,LR} + \frac{8272}{729}L_{ijii}^{V,LL} + \frac{8272}{729}L_{ijjj}^{V,LL} - \frac{3040}{729}L_{ij11}^{V,LR} - \frac{3040}{729}L_{ij22}^{V,LR} \\
& - \frac{3040}{729}L_{ij33}^{V,LR} - \frac{1120}{729}L_{ij11}^{V1,LR} - \frac{1120}{729}L_{ij22}^{V1,LR} + \frac{2576}{729}L_{11ij}^{V,LL} + \frac{2576}{729}L_{22ij}^{V,LL} \\
& + \frac{2576}{729}L_{33ij}^{V,LL} + \frac{5360}{729}L_{11ij}^{V1,LL} + \frac{6368}{729}L_{22ij}^{V1,LL} \Big] ;
\end{aligned}$$

$$\begin{aligned}
\dot{L}_{11ij}^{V8,LL} &= g_s^2 \Big[ \frac{2}{3}L_{ijii}^{V8,LR} + \frac{2}{3}L_{ijjj}^{V8,LR} + \frac{8}{3}L_{ijii}^{V,LL} + \frac{8}{3}L_{ijjj}^{V,LL} + \frac{2}{3}L_{ij11}^{V8,LR} \\
& + \frac{2}{3}L_{ij22}^{V8,LR} + 12L_{11ij}^{V1,LL} - \frac{10}{3}L_{11ij}^{V8,LL} + \frac{2}{3}L_{22ij}^{V8,LL} \Big] - \frac{8}{3}e^2L_{11ij}^{V8,LL} + \alpha_s^2 \Big[ -\frac{22}{3}L_{ijii}^{V1,LR} \\
& - \frac{22}{3}L_{ijjj}^{V1,LR} + \frac{169}{81}L_{ijii}^{V8,LR} + \frac{169}{81}L_{ijjj}^{V8,LR} + \frac{1930}{27}L_{ijii}^{V,LL} + \frac{1930}{27}L_{ijjj}^{V,LL} - \frac{22}{3}L_{ij11}^{V1,LR} \\
& - \frac{22}{3}L_{ij22}^{V1,LR} + \frac{169}{81}L_{ij11}^{V8,LR} + \frac{169}{81}L_{ij22}^{V8,LR} + 13L_{11ij}^{V1,LL} - \frac{2}{3}L_{22ij}^{V1,LL} - \frac{326}{81}L_{11ij}^{V8,LL} \\
& + \frac{799}{81}L_{22ij}^{V8,LL} \Big] + \alpha_s \alpha \Big[ -\frac{208}{81}L_{ijii}^{V1,LR} - \frac{208}{81}L_{ijjj}^{V1,LR} + \frac{52}{27}L_{ijii}^{V8,LR} + \frac{52}{27}L_{ijjj}^{V8,LR} \\
& - \frac{3200}{81}L_{ijii}^{V,LL} - \frac{3200}{81}L_{ijjj}^{V,LL} - \frac{208}{81}L_{ij11}^{V,LR} - \frac{208}{81}L_{ij22}^{V,LR} - \frac{208}{81}L_{ij33}^{V,LR} + \frac{416}{81}L_{ij11}^{V1,LR}
\end{aligned}$$

$$\begin{aligned}
& + \frac{416}{81} L_{ij22}^{V1,LR} - \frac{80}{27} L_{ij11}^{V8,LR} - \frac{80}{27} L_{ij22}^{V8,LR} - \frac{208}{81} L_{11ij}^{V,LL} - \frac{208}{81} L_{22ij}^{V,LL} - \frac{208}{81} L_{33ij}^{V,LL} \\
& + \frac{308}{81} L_{11ij}^{V1,LL} + \frac{416}{81} L_{22ij}^{V1,LL} + L_{11ij}^{V8,LL} + \frac{56}{9} L_{22ij}^{V8,LL} \Big] - \frac{112}{81} \alpha^2 L_{11ij}^{V8,LL} ; \\
\dot{L}_{ud,22ij}^{V1,LL} = & \frac{8}{3} g_s^2 L_{ud,22ij}^{V8,LL} + e^2 \Bigg[ -\frac{8}{9} L_{ijii}^{V1,LR} - \frac{8}{9} L_{ijjj}^{V1,LR} - \frac{64}{27} L_{ijii}^{V,LL} - \frac{64}{27} L_{ijjj}^{V,LL} \\
& - \frac{8}{9} L_{ij11}^{V,LR} - \frac{8}{9} L_{ij22}^{V,LR} - \frac{8}{9} L_{ij33}^{V,LR} + \frac{16}{9} L_{ij11}^{V1,LR} + \frac{16}{9} L_{ij22}^{V1,LR} - \frac{8}{9} L_{11ij}^{V,LL} \\
& - \frac{8}{9} L_{22ij}^{V,LL} - \frac{8}{9} L_{33ij}^{V,LL} + \frac{16}{9} L_{11ij}^{V1,LL} - \frac{8}{9} L_{22ij}^{V1,LL} \Big] + \alpha_s^2 \Bigg[ -8 L_{ijii}^{V1,LR} \\
& - 8 L_{ijjj}^{V1,LR} + \frac{4}{27} L_{ijii}^{V8,LR} + \frac{4}{27} L_{ijjj}^{V8,LR} + \frac{328}{9} L_{ijii}^{V,LL} + \frac{328}{9} L_{ijjj}^{V,LL} - 8 L_{ij11}^{V1,LR} \\
& - 8 L_{ij22}^{V1,LR} + \frac{4}{27} L_{ij11}^{V8,LR} + \frac{4}{27} L_{ij22}^{V8,LR} + 8 L_{11ij}^{V1,LL} - \frac{4}{3} L_{22ij}^{V1,LL} + \frac{4}{27} L_{11ij}^{V8,LL} \\
& + \frac{86}{27} L_{22ij}^{V8,LL} \Big] + \alpha_s \alpha \Bigg[ -\frac{32}{9} L_{ijii}^{V1,LR} - \frac{32}{9} L_{ijjj}^{V1,LR} + \frac{1984}{729} L_{ijii}^{V8,LR} + \frac{1984}{729} L_{ijjj}^{V8,LR} \\
& - \frac{2240}{243} L_{ijii}^{V,LL} - \frac{2240}{243} L_{ijjj}^{V,LL} + \frac{64}{9} L_{ij11}^{V1,LR} + \frac{64}{9} L_{ij22}^{V1,LR} - \frac{2768}{729} L_{ij11}^{V8,LR} - \frac{2768}{729} L_{ij22}^{V8,LR} \\
& + \frac{64}{9} L_{11ij}^{V1,LL} + \frac{256}{9} L_{22ij}^{V1,LL} + \frac{112}{729} L_{11ij}^{V8,LL} - \frac{104}{729} L_{22ij}^{V8,LL} \Big] + \alpha^2 \Bigg[ -\frac{304}{729} L_{ijii}^{V1,LR} \\
& - \frac{304}{729} L_{ijjj}^{V1,LR} + \frac{8272}{729} L_{ijii}^{V,LL} + \frac{8272}{729} L_{ijjj}^{V,LL} - \frac{3040}{729} L_{ij11}^{V,LR} - \frac{3040}{729} L_{ij22}^{V,LR} \\
& - \frac{3040}{729} L_{ij33}^{V,LR} - \frac{1120}{729} L_{ij11}^{V1,LR} - \frac{1120}{729} L_{ij22}^{V1,LR} + \frac{2576}{729} L_{11ij}^{V,LL} + \frac{2576}{729} L_{22ij}^{V,LL} \\
& + \frac{2576}{729} L_{33ij}^{V,LL} + \frac{6368}{729} L_{11ij}^{V1,LL} + \frac{5360}{729} L_{22ij}^{V1,LL} \Big] ; \\
\dot{L}_{ud,22ij}^{V8,LL} = & g_s^2 \Bigg[ \frac{2}{3} L_{ijii}^{V8,LR} + \frac{2}{3} L_{ijjj}^{V8,LR} + \frac{8}{3} L_{ijii}^{V,LL} + \frac{8}{3} L_{ijjj}^{V,LL} + \frac{2}{3} L_{ij11}^{V8,LR} \\
& + \frac{2}{3} L_{ij22}^{V8,LR} + 12 L_{ud,22ij}^{V1,LL} + \frac{2}{3} L_{11ij}^{V8,LL} - \frac{10}{3} L_{22ij}^{V8,LL} \Big] - \frac{8}{3} e^2 L_{ud,22ij}^{V8,LL} + \alpha_s^2 \Bigg[ -\frac{22}{3} L_{ijii}^{V1,LR} \\
& - \frac{22}{3} L_{ijjj}^{V1,LR} + \frac{169}{81} L_{ijii}^{V8,LR} + \frac{169}{81} L_{ijjj}^{V8,LR} + \frac{1930}{27} L_{ijii}^{V,LL} + \frac{1930}{27} L_{ijjj}^{V,LL} - \frac{22}{3} L_{ij11}^{V1,LR}
\end{aligned}$$

$$\begin{aligned}
& -\frac{22}{3}L_{ij22}^{V1,LR} + \frac{169}{81}L_{ij11}^{V8,LR} + \frac{169}{81}L_{ij22}^{V8,LR} - \frac{2}{3}L_{11ij}^{V1,LL} + 13L_{22ij}^{V1,LL} + \frac{799}{81}L_{11ij}^{V8,LL} \\
& - \frac{326}{81}L_{22ij}^{V8,LL} \Big] + \alpha_s \alpha \Big[ -\frac{208}{81}L_{ijii}^{V1,LR} - \frac{208}{81}L_{ijjj}^{V1,LR} + \frac{52}{27}L_{ijii}^{V8,LR} + \frac{52}{27}L_{ijjj}^{V8,LR} \\
& - \frac{3200}{81}L_{ijii}^{V,LL} - \frac{3200}{81}L_{ijjj}^{V,LL} - \frac{208}{81}L_{ij11}^{V,LR} - \frac{208}{81}L_{ij22}^{V,LR} - \frac{208}{81}L_{ij33}^{V,LR} + \frac{416}{81}L_{ij11}^{V1,LR} \\
& + \frac{416}{81}L_{ij22}^{V1,LR} - \frac{80}{27}L_{ij11}^{V8,LR} - \frac{80}{27}L_{ij22}^{V8,LR} - \frac{208}{81}L_{11ij}^{V,LL} - \frac{208}{81}L_{22ij}^{V,LL} - \frac{208}{81}L_{33ij}^{V,LL} \\
& + \frac{416}{81}L_{11ij}^{V1,LL} + \frac{308}{81}L_{22ij}^{V1,LL} + \frac{56}{9}L_{11ij}^{V8,LL} + L_{22ij}^{V8,LL} \Big] - \frac{112}{81}\alpha^2 L_{22ij}^{V8,LL} ; \\
\dot{L}_{ijjj}^{V,LL} = & g_s^2 \Big[ \frac{1}{9}L_{ijii}^{V8,LR} + \frac{1}{9}L_{ijjj}^{V8,LR} + \frac{4}{9}L_{ijii}^{V,LL} + \frac{40}{9}L_{ijjj}^{V,LL} + \frac{1}{9}L_{ij11}^{V8,LR} \\
& + \frac{1}{9}L_{ij22}^{V8,LR} + \frac{1}{9}L_{11ij}^{V8,LL} + \frac{1}{9}L_{22ij}^{V8,LL} \Big] + e^2 \Big[ \frac{2}{9}L_{ijii}^{V1,LR} + \frac{2}{9}L_{ijjj}^{V1,LR} \\
& + \frac{16}{27}L_{ijii}^{V,LL} + \frac{52}{27}L_{ijjj}^{V,LL} + \frac{2}{9}L_{ij11}^{V,LR} + \frac{2}{9}L_{ij22}^{V,LR} + \frac{2}{9}L_{ij33}^{V,LR} - \frac{4}{9}L_{ij11}^{V1,LR} \\
& - \frac{4}{9}L_{ij22}^{V1,LR} + \frac{2}{9}L_{11ij}^{V,LL} + \frac{2}{9}L_{22ij}^{V,LL} + \frac{2}{9}L_{33ij}^{V,LL} - \frac{4}{9}L_{11ij}^{V1,LL} - \frac{4}{9}L_{22ij}^{V1,LL} \Big] \\
& + \alpha_s^2 \Big[ -\frac{47}{9}L_{ijii}^{V1,LR} - \frac{47}{9}L_{ijjj}^{V1,LR} + \frac{205}{486}L_{ijii}^{V8,LR} + \frac{205}{486}L_{ijjj}^{V8,LR} + \frac{2441}{81}L_{ijii}^{V,LL} \\
& + \frac{2054}{81}L_{ijjj}^{V,LL} - \frac{47}{9}L_{ij11}^{V1,LR} - \frac{47}{9}L_{ij22}^{V1,LR} + \frac{205}{486}L_{ij11}^{V8,LR} + \frac{205}{486}L_{ij22}^{V8,LR} + \frac{35}{9}L_{11ij}^{V1,LL} \\
& + \frac{35}{9}L_{22ij}^{V1,LL} + \frac{835}{486}L_{11ij}^{V8,LL} + \frac{835}{486}L_{22ij}^{V8,LL} \Big] + \alpha_s \alpha \Big[ \frac{166}{243}L_{ijii}^{V1,LR} + \frac{166}{243}L_{ijjj}^{V1,LR} \\
& - \frac{721}{729}L_{ijii}^{V8,LR} - \frac{721}{729}L_{ijjj}^{V8,LR} + \frac{958}{243}L_{ijii}^{V,LL} - \frac{3038}{243}L_{ijjj}^{V,LL} - \frac{50}{243}L_{ij11}^{V,LR} \\
& - \frac{50}{243}L_{ij22}^{V,LR} - \frac{50}{243}L_{ij33}^{V,LR} - \frac{332}{243}L_{ij11}^{V1,LR} - \frac{332}{243}L_{ij22}^{V1,LR} + \frac{1331}{729}L_{ij11}^{V8,LR} \\
& + \frac{1331}{729}L_{ij22}^{V8,LR} - \frac{50}{243}L_{11ij}^{V,LL} - \frac{50}{243}L_{22ij}^{V,LL} - \frac{50}{243}L_{33ij}^{V,LL} - \frac{332}{243}L_{11ij}^{V1,LL} - \frac{332}{243}L_{22ij}^{V1,LL} \\
& - \frac{217}{729}L_{11ij}^{V8,LL} - \frac{217}{729}L_{22ij}^{V8,LL} \Big] + \alpha^2 \Big[ -\frac{356}{729}L_{ijii}^{V1,LR} - \frac{356}{729}L_{ijjj}^{V1,LR} + \frac{632}{729}L_{ijii}^{V,LL}
\end{aligned}$$

$$\begin{aligned}
& + \frac{974}{729} L_{ijj}^{V,LL} - \frac{644}{729} L_{ij11}^{V,LR} - \frac{644}{729} L_{ij22}^{V,LR} - \frac{644}{729} L_{ij33}^{V,LR} - \frac{1772}{729} L_{ij11}^{V1,LR} \\
& - \frac{1772}{729} L_{ij22}^{V1,LR} + \frac{868}{729} L_{11ij}^{V,LL} + \frac{868}{729} L_{22ij}^{V,LL} + \frac{868}{729} L_{33ij}^{V,LL} + \frac{244}{729} L_{11ij}^{V1,LL} \\
& + \frac{244}{729} L_{22ij}^{V1,LL} \Big] ;
\end{aligned}$$

$$\begin{aligned}
\dot{L}_{ij\bar{i}\bar{i}}^{V,LL} = & g_s^2 \left[ \frac{1}{9} L_{ij\bar{i}\bar{i}}^{V8,LR} + \frac{1}{9} L_{ijjj}^{V8,LR} + \frac{40}{9} L_{ij\bar{i}\bar{i}}^{V,LL} + \frac{4}{9} L_{ijjj}^{V,LL} + \frac{1}{9} L_{ij11}^{V8,LR} \right. \\
& + \frac{1}{9} L_{ij22}^{V8,LR} + \frac{1}{9} L_{11ij}^{V8,LL} + \left. \frac{1}{9} L_{22ij}^{V8,LL} \right] + e^2 \left[ \frac{2}{9} L_{ij\bar{i}\bar{i}}^{V1,LR} + \frac{2}{9} L_{ijjj}^{V1,LR} \right. \\
& + \frac{52}{27} L_{ij\bar{i}\bar{i}}^{V,LL} + \frac{16}{27} L_{ijjj}^{V,LL} + \frac{2}{9} L_{ij11}^{V,LR} + \frac{2}{9} L_{ij22}^{V,LR} + \frac{2}{9} L_{ij33}^{V,LR} - \frac{4}{9} L_{ij11}^{V1,LR} \\
& - \frac{4}{9} L_{ij22}^{V1,LR} + \frac{2}{9} L_{11ij}^{V,LL} + \frac{2}{9} L_{22ij}^{V,LL} + \frac{2}{9} L_{33ij}^{V,LL} - \frac{4}{9} L_{11ij}^{V1,LL} - \left. \frac{4}{9} L_{22ij}^{V1,LL} \right] \\
& + \alpha_s^2 \left[ -\frac{47}{9} L_{ij\bar{i}\bar{i}}^{V1,LR} - \frac{47}{9} L_{ijjj}^{V1,LR} + \frac{205}{486} L_{ij\bar{i}\bar{i}}^{V8,LR} + \frac{205}{486} L_{ijjj}^{V8,LR} + \frac{2054}{81} L_{ij\bar{i}\bar{i}}^{V,LL} \right. \\
& + \frac{2441}{81} L_{ijjj}^{V,LL} - \frac{47}{9} L_{ij11}^{V1,LR} - \frac{47}{9} L_{ij22}^{V1,LR} + \frac{205}{486} L_{ij11}^{V8,LR} + \frac{205}{486} L_{ij22}^{V8,LR} + \frac{35}{9} L_{11ij}^{V1,LL} \\
& + \frac{35}{9} L_{22ij}^{V1,LL} + \frac{835}{486} L_{11ij}^{V8,LL} + \left. \frac{835}{486} L_{22ij}^{V8,LL} \right] + \alpha_s \alpha \left[ \frac{166}{243} L_{ij\bar{i}\bar{i}}^{V1,LR} + \frac{166}{243} L_{ijjj}^{V1,LR} \right. \\
& - \frac{721}{729} L_{ij\bar{i}\bar{i}}^{V8,LR} - \frac{721}{729} L_{ijjj}^{V8,LR} - \frac{3038}{243} L_{ij\bar{i}\bar{i}}^{V,LL} + \frac{958}{243} L_{ijjj}^{V,LL} - \frac{50}{243} L_{ij11}^{V,LR} \\
& - \frac{50}{243} L_{ij22}^{V,LR} - \frac{50}{243} L_{ij33}^{V,LR} - \frac{332}{243} L_{ij11}^{V1,LR} - \frac{332}{243} L_{ij22}^{V1,LR} + \frac{1331}{729} L_{ij11}^{V8,LR} \\
& + \frac{1331}{729} L_{ij22}^{V8,LR} - \frac{50}{243} L_{11ij}^{V,LL} - \frac{50}{243} L_{22ij}^{V,LL} - \frac{50}{243} L_{33ij}^{V,LL} - \frac{332}{243} L_{11ij}^{V1,LL} - \frac{332}{243} L_{22ij}^{V1,LL} \\
& - \left. \frac{217}{729} L_{11ij}^{V8,LL} - \frac{217}{729} L_{22ij}^{V8,LL} \right] + \alpha^2 \left[ -\frac{356}{729} L_{ij\bar{i}\bar{i}}^{V1,LR} - \frac{356}{729} L_{ijjj}^{V1,LR} + \frac{974}{729} L_{ij\bar{i}\bar{i}}^{V,LL} \right. \\
& + \frac{632}{729} L_{ijjj}^{V,LL} - \frac{644}{729} L_{ij11}^{V,LR} - \frac{644}{729} L_{ij22}^{V,LR} - \frac{644}{729} L_{ij33}^{V,LR} - \frac{1772}{729} L_{ij11}^{V1,LR} \\
& - \frac{1772}{729} L_{ij22}^{V1,LR} + \frac{868}{729} L_{11ij}^{V,LL} + \frac{868}{729} L_{22ij}^{V,LL} + \frac{868}{729} L_{33ij}^{V,LL} + \frac{244}{729} L_{11ij}^{V1,LL} \\
& \left. - \frac{244}{729} L_{22ij}^{V1,LL} \right]
\end{aligned}$$

$$\begin{aligned}
& + \frac{244}{729} L_{22ij}^{V1,LL} \Big] ; \\
\dot{L}_{ij11}^{V,LR} = & e^2 \left[ \frac{4}{3} L_{ijii}^{V1,LR} + \frac{4}{3} L_{ijjj}^{V1,LR} + \frac{32}{9} L_{ijii}^{V,LL} + \frac{32}{9} L_{ijjj}^{V,LL} - \frac{8}{3} L_{ij11}^{V,LR} \right. \\
& + \frac{4}{3} L_{ij22}^{V,LR} + \frac{4}{3} L_{ij33}^{V,LR} - \frac{8}{3} L_{ij11}^{V1,LR} - \frac{8}{3} L_{ij22}^{V1,LR} + \frac{4}{3} L_{11ij}^{V,LL} + \frac{4}{3} L_{22ij}^{V,LL} \\
& + \left. \frac{4}{3} L_{33ij}^{V,LL} - \frac{8}{3} L_{11ij}^{V1,LL} - \frac{8}{3} L_{22ij}^{V1,LL} \right] + \alpha_s \alpha \left[ \frac{16}{3} L_{ijii}^{V1,LR} + \frac{16}{3} L_{ijjj}^{V1,LR} \right. \\
& - \frac{992}{243} L_{ijii}^{V8,LR} - \frac{992}{243} L_{ijjj}^{V8,LR} + \frac{1120}{81} L_{ijii}^{V,LL} + \frac{1120}{81} L_{ijjj}^{V,LL} + 16 L_{ij11}^{V,LR} - \frac{32}{3} L_{ij11}^{V1,LR} \\
& - \frac{32}{3} L_{ij22}^{V1,LR} + \frac{1384}{243} L_{ij11}^{V8,LR} + \frac{1384}{243} L_{ij22}^{V8,LR} - \frac{32}{3} L_{11ij}^{V1,LL} - \frac{32}{3} L_{22ij}^{V1,LL} - \frac{56}{243} L_{11ij}^{V8,LL} \\
& - \left. \frac{56}{243} L_{22ij}^{V8,LL} \right] + \alpha^2 \left[ \frac{1736}{243} L_{ijii}^{V1,LR} + \frac{1736}{243} L_{ijjj}^{V1,LR} - \frac{752}{243} L_{ijii}^{V,LL} - \frac{752}{243} L_{ijjj}^{V,LL} \right. \\
& + \frac{20906}{243} L_{ij11}^{V,LR} + \frac{3752}{243} L_{ij22}^{V,LR} + \frac{3752}{243} L_{ij33}^{V,LR} - \frac{664}{243} L_{ij11}^{V1,LR} - \frac{664}{243} L_{ij22}^{V1,LR} \\
& - \frac{1000}{243} L_{11ij}^{V,LL} - \frac{1000}{243} L_{22ij}^{V,LL} - \frac{1000}{243} L_{33ij}^{V,LL} - \frac{7000}{243} L_{11ij}^{V1,LL} - \frac{7000}{243} L_{22ij}^{V1,LL} \Big] ; \\
\dot{L}_{ij22}^{V,LR} = & e^2 \left[ \frac{4}{3} L_{ijii}^{V1,LR} + \frac{4}{3} L_{ijjj}^{V1,LR} + \frac{32}{9} L_{ijii}^{V,LL} + \frac{32}{9} L_{ijjj}^{V,LL} + \frac{4}{3} L_{ij11}^{V,LR} \right. \\
& - \frac{8}{3} L_{ij22}^{V,LR} + \frac{4}{3} L_{ij33}^{V,LR} - \frac{8}{3} L_{ij11}^{V1,LR} - \frac{8}{3} L_{ij22}^{V1,LR} + \frac{4}{3} L_{11ij}^{V,LL} + \frac{4}{3} L_{22ij}^{V,LL} \\
& + \left. \frac{4}{3} L_{33ij}^{V,LL} - \frac{8}{3} L_{11ij}^{V1,LL} - \frac{8}{3} L_{22ij}^{V1,LL} \right] + \alpha_s \alpha \left[ \frac{16}{3} L_{ijii}^{V1,LR} + \frac{16}{3} L_{ijjj}^{V1,LR} \right. \\
& - \frac{992}{243} L_{ijii}^{V8,LR} - \frac{992}{243} L_{ijjj}^{V8,LR} + \frac{1120}{81} L_{ijii}^{V,LL} + \frac{1120}{81} L_{ijjj}^{V,LL} + 16 L_{ij22}^{V,LR} - \frac{32}{3} L_{ij11}^{V1,LR} \\
& - \frac{32}{3} L_{ij22}^{V1,LR} + \frac{1384}{243} L_{ij11}^{V8,LR} + \frac{1384}{243} L_{ij22}^{V8,LR} - \frac{32}{3} L_{11ij}^{V1,LL} - \frac{32}{3} L_{22ij}^{V1,LL} - \frac{56}{243} L_{11ij}^{V8,LL} \\
& - \left. \frac{56}{243} L_{22ij}^{V8,LL} \right] + \alpha^2 \left[ \frac{1736}{243} L_{ijii}^{V1,LR} + \frac{1736}{243} L_{ijjj}^{V1,LR} - \frac{752}{243} L_{ijii}^{V,LL} - \frac{752}{243} L_{ijjj}^{V,LL} \right. \\
& + \frac{3752}{243} L_{ij11}^{V,LR} + \frac{20906}{243} L_{ij22}^{V,LR} + \frac{3752}{243} L_{ij33}^{V,LR} - \frac{664}{243} L_{ij11}^{V1,LR} - \frac{664}{243} L_{ij22}^{V1,LR}
\end{aligned}$$



$$\begin{aligned}
& -\frac{1000}{243}L_{11ij}^{V,LL} - \frac{1000}{243}L_{22ij}^{V,LL} - \frac{1000}{243}L_{33ij}^{V,LL} - \frac{7000}{243}L_{11ij}^{V1,LL} - \frac{7000}{243}L_{22ij}^{V1,LL} \Big] ; \\
\dot{L}_{ij33}^{V,LR} = & e^2 \left[ \frac{4}{3}L_{ijii}^{V1,LR} + \frac{4}{3}L_{ijjj}^{V1,LR} + \frac{32}{9}L_{ijii}^{V,LL} + \frac{32}{9}L_{ijjj}^{V,LL} + \frac{4}{3}L_{ij11}^{V,LR} \right. \\
& + \frac{4}{3}L_{ij22}^{V,LR} - \frac{8}{3}L_{ij33}^{V,LR} - \frac{8}{3}L_{ij11}^{V1,LR} - \frac{8}{3}L_{ij22}^{V1,LR} + \frac{4}{3}L_{11ij}^{V,LL} + \frac{4}{3}L_{22ij}^{V,LL} \\
& + \left. \frac{4}{3}L_{33ij}^{V,LL} - \frac{8}{3}L_{11ij}^{V1,LL} - \frac{8}{3}L_{22ij}^{V1,LL} \right] + \alpha_s \alpha \left[ \frac{16}{3}L_{ijii}^{V1,LR} + \frac{16}{3}L_{ijjj}^{V1,LR} \right. \\
& - \frac{992}{243}L_{ijii}^{V8,LR} - \frac{992}{243}L_{ijjj}^{V8,LR} + \frac{1120}{81}L_{ijii}^{V,LL} + \frac{1120}{81}L_{ijjj}^{V,LL} + 16L_{ij33}^{V,LR} - \frac{32}{3}L_{ij11}^{V1,LR} \\
& - \frac{32}{3}L_{ij22}^{V1,LR} + \frac{1384}{243}L_{ij11}^{V8,LR} + \frac{1384}{243}L_{ij22}^{V8,LR} - \frac{32}{3}L_{11ij}^{V1,LL} - \frac{32}{3}L_{22ij}^{V1,LL} - \frac{56}{243}L_{11ij}^{V8,LL} \\
& - \left. \frac{56}{243}L_{22ij}^{V8,LL} \right] + \alpha^2 \left[ \frac{1736}{243}L_{ijii}^{V1,LR} + \frac{1736}{243}L_{ijjj}^{V1,LR} - \frac{752}{243}L_{ijii}^{V,LL} - \frac{752}{243}L_{ijjj}^{V,LL} \right. \\
& + \frac{3752}{243}L_{ij11}^{V,LR} + \frac{3752}{243}L_{ij22}^{V,LR} + \frac{20906}{243}L_{ij33}^{V,LR} - \frac{664}{243}L_{ij11}^{V1,LR} - \frac{664}{243}L_{ij22}^{V1,LR} \\
& - \frac{1000}{243}L_{11ij}^{V,LL} - \frac{1000}{243}L_{22ij}^{V,LL} - \frac{1000}{243}L_{33ij}^{V,LL} - \frac{7000}{243}L_{11ij}^{V1,LL} - \frac{7000}{243}L_{22ij}^{V1,LL} \Big] ; \\
\dot{L}_{ij11}^{V1,LR} = & -\frac{8}{3}g_s^2 L_{ij11}^{V8,LR} + e^2 \left[ -\frac{8}{9}L_{ijii}^{V1,LR} - \frac{8}{9}L_{ijjj}^{V1,LR} - \frac{64}{27}L_{ijii}^{V,LL} - \frac{64}{27}L_{ijjj}^{V,LL} \right. \\
& - \frac{8}{9}L_{ij11}^{V,LR} - \frac{8}{9}L_{ij22}^{V,LR} - \frac{8}{9}L_{ij33}^{V,LR} + \frac{40}{9}L_{ij11}^{V1,LR} + \frac{16}{9}L_{ij22}^{V1,LR} - \frac{8}{9}L_{11ij}^{V,LL} \\
& - \frac{8}{9}L_{22ij}^{V,LL} - \frac{8}{9}L_{33ij}^{V,LL} + \frac{16}{9}L_{11ij}^{V1,LL} + \frac{16}{9}L_{22ij}^{V1,LL} \Big] + \alpha_s^2 \left[ 8L_{ijii}^{V1,LR} \right. \\
& + 8L_{ijjj}^{V1,LR} + \frac{44}{27}L_{ijii}^{V8,LR} + \frac{44}{27}L_{ijjj}^{V8,LR} - \frac{232}{9}L_{ijii}^{V,LL} - \frac{232}{9}L_{ijjj}^{V,LL} - \frac{4}{3}L_{ij11}^{V1,LR} \\
& + 8L_{ij22}^{V1,LR} - \frac{2000}{27}L_{ij11}^{V8,LR} + \frac{44}{27}L_{ij22}^{V8,LR} - 8L_{11ij}^{V1,LL} - 8L_{22ij}^{V1,LL} + \frac{44}{27}L_{11ij}^{V8,LL} \\
& + \left. \frac{44}{27}L_{22ij}^{V8,LL} \right] + \alpha_s \alpha \left[ -\frac{32}{9}L_{ijii}^{V1,LR} - \frac{32}{9}L_{ijjj}^{V1,LR} + \frac{1984}{729}L_{ijii}^{V8,LR} + \frac{1984}{729}L_{ijjj}^{V8,LR} \right. \\
& - \frac{2240}{243}L_{ijii}^{V,LL} - \frac{2240}{243}L_{ijjj}^{V,LL} - \frac{128}{9}L_{ij11}^{V1,LR} + \frac{64}{9}L_{ij22}^{V1,LR} + \frac{3496}{729}L_{ij11}^{V8,LR} \\
& + \frac{3496}{729}L_{ij22}^{V8,LR} \Big] ;
\end{aligned}$$

$$\begin{aligned}
& -\frac{2768}{729}L_{ij22}^{V8,LR} + \frac{64}{9}L_{11ij}^{V1,LL} + \frac{64}{9}L_{22ij}^{V1,LL} + \frac{112}{729}L_{11ij}^{V8,LL} + \frac{112}{729}L_{22ij}^{V8,LL} \Big] \\
& + \alpha^2 \Big[ \frac{3728}{729}L_{ijii}^{V1,LR} + \frac{3728}{729}L_{ijjj}^{V1,LR} + \frac{784}{729}L_{ijii}^{V,LL} + \frac{784}{729}L_{ijjj}^{V,LL} + \frac{6176}{729}L_{ij11}^{V,LR} \\
& + \frac{6176}{729}L_{ij22}^{V,LR} + \frac{6176}{729}L_{ij33}^{V,LR} - \frac{28480}{729}L_{ij11}^{V1,LR} + \frac{6368}{729}L_{ij22}^{V1,LR} - \frac{3760}{729}L_{11ij}^{V,LL} \\
& - \frac{3760}{729}L_{22ij}^{V,LL} - \frac{3760}{729}L_{33ij}^{V,LL} - \frac{6880}{729}L_{11ij}^{V1,LL} - \frac{6880}{729}L_{22ij}^{V1,LL} \Big] ;
\end{aligned}$$

$$\begin{aligned}
\dot{L}_{ij11}^{V8,LR} = & g_s^2 \Big[ \frac{2}{3}L_{ijii}^{V8,LR} + \frac{2}{3}L_{ijjj}^{V8,LR} + \frac{8}{3}L_{ijii}^{V,LL} + \frac{8}{3}L_{ijjj}^{V,LL} - 12L_{ij11}^{V1,LR} \\
& - \frac{40}{3}L_{ij11}^{V8,LR} + \frac{2}{3}L_{ij22}^{V8,LR} + \frac{2}{3}L_{11ij}^{V8,LL} + \frac{2}{3}L_{22ij}^{V8,LL} \Big] + \frac{8}{3}e^2L_{ij11}^{V8,LR} + \alpha_s^2 \Big[ -\frac{22}{3}L_{ijii}^{V1,LR} \\
& - \frac{22}{3}L_{ijjj}^{V1,LR} + \frac{799}{81}L_{ijii}^{V8,LR} + \frac{799}{81}L_{ijjj}^{V8,LR} + \frac{1210}{27}L_{ijii}^{V,LL} + \frac{1210}{27}L_{ijjj}^{V,LL} - 132L_{ij11}^{V1,LR} \\
& - \frac{22}{3}L_{ij22}^{V1,LR} - \frac{25177}{162}L_{ij11}^{V8,LR} + \frac{799}{81}L_{ij22}^{V8,LR} - \frac{2}{3}L_{11ij}^{V1,LL} - \frac{2}{3}L_{22ij}^{V1,LL} + \frac{619}{81}L_{11ij}^{V8,LL} \\
& + \frac{619}{81}L_{22ij}^{V8,LL} \Big] + \alpha_s \alpha \Big[ -\frac{928}{81}L_{ijii}^{V1,LR} - \frac{928}{81}L_{ijjj}^{V1,LR} - \frac{44}{9}L_{ijii}^{V8,LR} - \frac{44}{9}L_{ijjj}^{V8,LR} \\
& - \frac{2192}{81}L_{ijii}^{V,LL} - \frac{2192}{81}L_{ijjj}^{V,LL} - \frac{928}{81}L_{ij11}^{V,LR} - \frac{928}{81}L_{ij22}^{V,LR} - \frac{928}{81}L_{ij33}^{V,LR} + \frac{4988}{81}L_{ij11}^{V1,LR} \\
& + \frac{1856}{81}L_{ij22}^{V1,LR} + 27L_{ij11}^{V8,LR} + \frac{56}{9}L_{ij22}^{V8,LR} - \frac{928}{81}L_{11ij}^{V,LL} - \frac{928}{81}L_{22ij}^{V,LL} - \frac{928}{81}L_{33ij}^{V,LL} \\
& + \frac{1856}{81}L_{11ij}^{V1,LL} + \frac{1856}{81}L_{22ij}^{V1,LL} - \frac{160}{27}L_{11ij}^{V8,LL} - \frac{160}{27}L_{22ij}^{V8,LL} \Big] - \frac{3872}{81}\alpha^2L_{ij11}^{V8,LR} ;
\end{aligned}$$

$$\begin{aligned}
\dot{L}_{ij22}^{V1,LR} = & -\frac{8}{3}g_s^2L_{ij22}^{V8,LR} + e^2 \Big[ -\frac{8}{9}L_{ijii}^{V1,LR} - \frac{8}{9}L_{ijjj}^{V1,LR} - \frac{64}{27}L_{ijii}^{V,LL} - \frac{64}{27}L_{ijjj}^{V,LL} \\
& - \frac{8}{9}L_{ij11}^{V,LR} - \frac{8}{9}L_{ij22}^{V,LR} - \frac{8}{9}L_{ij33}^{V,LR} + \frac{16}{9}L_{ij11}^{V1,LR} + \frac{40}{9}L_{ij22}^{V1,LR} - \frac{8}{9}L_{11ij}^{V,LL} \\
& - \frac{8}{9}L_{22ij}^{V,LL} - \frac{8}{9}L_{33ij}^{V,LL} + \frac{16}{9}L_{11ij}^{V1,LL} + \frac{16}{9}L_{22ij}^{V1,LL} \Big] + \alpha_s^2 \Big[ 8L_{ijii}^{V1,LR} \\
& + 8L_{ijjj}^{V1,LR} + \frac{44}{27}L_{ijii}^{V8,LR} + \frac{44}{27}L_{ijjj}^{V8,LR} - \frac{232}{9}L_{ijii}^{V,LL} - \frac{232}{9}L_{ijjj}^{V,LL} + 8L_{ij11}^{V1,LR}
\end{aligned}$$

$$\begin{aligned}
& -\frac{4}{3}L_{ij22}^{V1,LR} + \frac{44}{27}L_{ij11}^{V8,LR} - \frac{2000}{27}L_{ij22}^{V8,LR} - 8L_{11ij}^{V1,LL} - 8L_{22ij}^{V1,LL} + \frac{44}{27}L_{11ij}^{V8,LL} \\
& + \frac{44}{27}L_{22ij}^{V8,LL} \Big] + \alpha_s \alpha \Big[ -\frac{32}{9}L_{ijii}^{V1,LR} - \frac{32}{9}L_{ijjj}^{V1,LR} + \frac{1984}{729}L_{ijii}^{V8,LR} + \frac{1984}{729}L_{ijjj}^{V8,LR} \\
& - \frac{2240}{243}L_{ijii}^{V,LL} - \frac{2240}{243}L_{ijjj}^{V,LL} + \frac{64}{9}L_{ij11}^{V1,LR} - \frac{128}{9}L_{ij22}^{V1,LR} - \frac{2768}{729}L_{ij11}^{V8,LR} \\
& + \frac{3496}{729}L_{ij22}^{V8,LR} + \frac{64}{9}L_{11ij}^{V1,LL} + \frac{64}{9}L_{22ij}^{V1,LL} + \frac{112}{729}L_{11ij}^{V8,LL} + \frac{112}{729}L_{22ij}^{V8,LL} \Big] \\
& + \alpha^2 \Big[ \frac{3728}{729}L_{ijii}^{V1,LR} + \frac{3728}{729}L_{ijjj}^{V1,LR} + \frac{784}{729}L_{ijii}^{V,LL} + \frac{784}{729}L_{ijjj}^{V,LL} + \frac{6176}{729}L_{ij11}^{V,LR} \\
& + \frac{6176}{729}L_{ij22}^{V,LR} + \frac{6176}{729}L_{ij33}^{V,LR} + \frac{6368}{729}L_{ij11}^{V1,LR} - \frac{28480}{729}L_{ij22}^{V1,LR} - \frac{3760}{729}L_{11ij}^{V,LL} \\
& - \frac{3760}{729}L_{22ij}^{V,LL} - \frac{3760}{729}L_{33ij}^{V,LL} - \frac{6880}{729}L_{11ij}^{V1,LL} - \frac{6880}{729}L_{22ij}^{V1,LL} \Big] ;
\end{aligned}$$

$$\begin{aligned}
\dot{L}_{ij22}^{V8,LR} &= g_s^2 \Big[ \frac{2}{3}L_{ijii}^{V8,LR} + \frac{2}{3}L_{ijjj}^{V8,LR} + \frac{8}{3}L_{ijii}^{V,LL} + \frac{8}{3}L_{ijjj}^{V,LL} - 12L_{ij22}^{V1,LR} \\
& + \frac{2}{3}L_{ij11}^{V8,LR} - \frac{40}{3}L_{ij22}^{V8,LR} + \frac{2}{3}L_{11ij}^{V8,LL} + \frac{2}{3}L_{22ij}^{V8,LL} \Big] + \frac{8}{3}e^2L_{ij22}^{V8,LR} + \alpha_s^2 \Big[ -\frac{22}{3}L_{ijii}^{V1,LR} \\
& - \frac{22}{3}L_{ijjj}^{V1,LR} + \frac{799}{81}L_{ijii}^{V8,LR} + \frac{799}{81}L_{ijjj}^{V8,LR} + \frac{1210}{27}L_{ijii}^{V,LL} + \frac{1210}{27}L_{ijjj}^{V,LL} - \frac{22}{3}L_{ij11}^{V1,LR} \\
& - 132L_{ij22}^{V1,LR} + \frac{799}{81}L_{ij11}^{V8,LR} - \frac{25177}{162}L_{ij22}^{V8,LR} - \frac{2}{3}L_{11ij}^{V1,LL} - \frac{2}{3}L_{22ij}^{V1,LL} + \frac{619}{81}L_{11ij}^{V8,LL} \\
& + \frac{619}{81}L_{22ij}^{V8,LL} \Big] + \alpha_s \alpha \Big[ -\frac{928}{81}L_{ijii}^{V1,LR} - \frac{928}{81}L_{ijjj}^{V1,LR} - \frac{44}{9}L_{ijii}^{V8,LR} - \frac{44}{9}L_{ijjj}^{V8,LR} \\
& - \frac{2192}{81}L_{ijii}^{V,LL} - \frac{2192}{81}L_{ijjj}^{V,LL} - \frac{928}{81}L_{ij11}^{V,LR} - \frac{928}{81}L_{ij22}^{V,LR} - \frac{928}{81}L_{ij33}^{V,LR} + \frac{1856}{81}L_{ij11}^{V1,LR} \\
& + \frac{4988}{81}L_{ij22}^{V1,LR} + \frac{56}{9}L_{ij11}^{V8,LR} + 27L_{ij22}^{V8,LR} - \frac{928}{81}L_{11ij}^{V,LL} - \frac{928}{81}L_{22ij}^{V,LL} - \frac{928}{81}L_{33ij}^{V,LL} \\
& + \frac{1856}{81}L_{11ij}^{V1,LL} + \frac{1856}{81}L_{22ij}^{V1,LL} - \frac{160}{27}L_{11ij}^{V8,LL} - \frac{160}{27}L_{22ij}^{V8,LL} \Big] - \frac{3872}{81}\alpha^2L_{ij22}^{V8,LR} ;
\end{aligned}$$

$$\dot{L}_{ijjj}^{V1,LR} = -\frac{8}{3}g_s^2L_{ijjj}^{V8,LR} + e^2 \Big[ \frac{4}{9}L_{ijii}^{V1,LR} - \frac{8}{9}L_{ijjj}^{V1,LR} + \frac{32}{27}L_{ijii}^{V,LL} + \frac{32}{27}L_{ijjj}^{V,LL}$$

$$\begin{aligned}
& + \frac{4}{9}L_{ij11}^{V,LR} + \frac{4}{9}L_{ij22}^{V,LR} + \frac{4}{9}L_{ij33}^{V,LR} - \frac{8}{9}L_{ij11}^{V1,LR} - \frac{8}{9}L_{ij22}^{V1,LR} + \frac{4}{9}L_{11ij}^{V,LL} \\
& + \frac{4}{9}L_{22ij}^{V,LL} + \frac{4}{9}L_{33ij}^{V,LL} - \frac{8}{9}L_{11ij}^{V1,LL} - \frac{8}{9}L_{22ij}^{V1,LL} \Big] + \alpha_s^2 \Big[ 8L_{ijii}^{V1,LR} \\
& - \frac{4}{3}L_{ijjj}^{V1,LR} + \frac{44}{27}L_{ijii}^{V8,LR} - \frac{2000}{27}L_{ijjj}^{V8,LR} - \frac{232}{9}L_{ijii}^{V,LL} - \frac{232}{9}L_{ijjj}^{V,LL} + 8L_{ij11}^{V1,LR} \\
& + 8L_{ij22}^{V1,LR} + \frac{44}{27}L_{ij11}^{V8,LR} + \frac{44}{27}L_{ij22}^{V8,LR} - 8L_{11ij}^{V1,LL} - 8L_{22ij}^{V1,LL} + \frac{44}{27}L_{11ij}^{V8,LL} \\
& + \frac{44}{27}L_{22ij}^{V8,LL} \Big] + \alpha_s \alpha \Big[ \frac{16}{9}L_{ijii}^{V1,LR} + \frac{112}{9}L_{ijjj}^{V1,LR} - \frac{992}{729}L_{ijii}^{V8,LR} - \frac{1208}{729}L_{ijjj}^{V8,LR} \\
& + \frac{1120}{243}L_{ijii}^{V,LL} + \frac{1120}{243}L_{ijjj}^{V,LL} - \frac{32}{9}L_{ij11}^{V1,LR} - \frac{32}{9}L_{ij22}^{V1,LR} + \frac{1384}{729}L_{ij11}^{V8,LR} + \frac{1384}{729}L_{ij22}^{V8,LR} \\
& - \frac{32}{9}L_{11ij}^{V1,LL} - \frac{32}{9}L_{22ij}^{V1,LL} - \frac{56}{729}L_{11ij}^{V8,LL} - \frac{56}{729}L_{22ij}^{V8,LL} \Big] + \alpha^2 \Big[ \frac{296}{729}L_{ijii}^{V1,LR} \\
& + \frac{15614}{729}L_{ijjj}^{V1,LR} - \frac{608}{729}L_{ijii}^{V,LL} - \frac{608}{729}L_{ijjj}^{V,LL} + \frac{1016}{729}L_{ij11}^{V,LR} + \frac{1016}{729}L_{ij22}^{V,LR} \\
& + \frac{1016}{729}L_{ij33}^{V,LR} - \frac{1672}{729}L_{ij11}^{V1,LR} - \frac{1672}{729}L_{ij22}^{V1,LR} + \frac{152}{729}L_{11ij}^{V,LL} + \frac{152}{729}L_{22ij}^{V,LL} \\
& + \frac{152}{729}L_{33ij}^{V,LL} - \frac{2824}{729}L_{11ij}^{V1,LL} - \frac{2824}{729}L_{22ij}^{V1,LL} \Big] ;
\end{aligned}$$

$$\begin{aligned}
\dot{L}_{ijjj}^{V8,LR} &= g_s^2 \Big[ -12L_{ijjj}^{V1,LR} + \frac{2}{3}L_{ijii}^{V8,LR} - \frac{40}{3}L_{ijjj}^{V8,LR} + \frac{8}{3}L_{ijii}^{V,LL} + \frac{8}{3}L_{ijjj}^{V,LL} \\
& + \frac{2}{3}L_{ij11}^{V8,LR} + \frac{2}{3}L_{ij22}^{V8,LR} + \frac{2}{3}L_{11ij}^{V8,LL} + \frac{2}{3}L_{22ij}^{V8,LL} \Big] - \frac{4}{3}e^2L_{ijjj}^{V8,LR} + \alpha_s^2 \Big[ -\frac{22}{3}L_{ijii}^{V1,LR} \\
& - 132L_{ijjj}^{V1,LR} + \frac{799}{81}L_{ijii}^{V8,LR} - \frac{25177}{162}L_{ijjj}^{V8,LR} + \frac{1210}{27}L_{ijii}^{V,LL} + \frac{1210}{27}L_{ijjj}^{V,LL} \\
& - \frac{22}{3}L_{ij11}^{V1,LR} - \frac{22}{3}L_{ij22}^{V1,LR} + \frac{799}{81}L_{ij11}^{V8,LR} + \frac{799}{81}L_{ij22}^{V8,LR} - \frac{2}{3}L_{11ij}^{V1,LL} - \frac{2}{3}L_{22ij}^{V1,LL} \\
& + \frac{619}{81}L_{11ij}^{V8,LL} + \frac{619}{81}L_{22ij}^{V8,LL} \Big] + \alpha_s \alpha \Big[ \frac{260}{81}L_{ijii}^{V1,LR} + \frac{152}{81}L_{ijjj}^{V1,LR} + \frac{14}{9}L_{ijii}^{V8,LR} \\
& - \frac{4}{3}L_{ijjj}^{V8,LR} + \frac{292}{81}L_{ijii}^{V,LL} + \frac{292}{81}L_{ijjj}^{V,LL} + \frac{260}{81}L_{ij11}^{V,LR} + \frac{260}{81}L_{ij22}^{V,LR} + \frac{260}{81}L_{ij33}^{V,LR}
\end{aligned}$$

$$\begin{aligned}
& -\frac{520}{81}L_{ij11}^{V1,LR} - \frac{520}{81}L_{ij22}^{V1,LR} + \frac{2}{3}L_{ij11}^{V8,LR} + \frac{2}{3}L_{ij22}^{V8,LR} + \frac{260}{81}L_{11ij}^{V,LL} + \frac{260}{81}L_{22ij}^{V,LL} \\
& + \frac{260}{81}L_{33ij}^{V,LL} - \frac{520}{81}L_{11ij}^{V1,LL} - \frac{520}{81}L_{22ij}^{V1,LL} + \frac{122}{27}L_{11ij}^{V8,LL} + \frac{122}{27}L_{22ij}^{V8,LL} \Big] \\
& + \frac{1702}{81}\alpha^2 L_{ijjj}^{V8,LR} ; \\
\dot{L}_{ijii}^{V1,LR} = & -\frac{8}{3}g_s^2 L_{ijii}^{V8,LR} + e^2 \Big[ -\frac{8}{9}L_{ijii}^{V1,LR} + \frac{4}{9}L_{ijjj}^{V1,LR} + \frac{32}{27}L_{ijii}^{V,LL} + \frac{32}{27}L_{ijjj}^{V,LL} \\
& + \frac{4}{9}L_{ij11}^{V,LR} + \frac{4}{9}L_{ij22}^{V,LR} + \frac{4}{9}L_{ij33}^{V,LR} - \frac{8}{9}L_{ij11}^{V1,LR} - \frac{8}{9}L_{ij22}^{V1,LR} + \frac{4}{9}L_{11ij}^{V,LL} \\
& + \frac{4}{9}L_{22ij}^{V,LL} + \frac{4}{9}L_{33ij}^{V,LL} - \frac{8}{9}L_{11ij}^{V1,LL} - \frac{8}{9}L_{22ij}^{V1,LL} \Big] + \alpha_s^2 \Big[ -\frac{4}{3}L_{ijii}^{V1,LR} \\
& + 8L_{ijjj}^{V1,LR} - \frac{2000}{27}L_{ijii}^{V8,LR} + \frac{44}{27}L_{ijjj}^{V8,LR} - \frac{232}{9}L_{ijii}^{V,LL} - \frac{232}{9}L_{ijjj}^{V,LL} + 8L_{ij11}^{V1,LR} \\
& + 8L_{ij22}^{V1,LR} + \frac{44}{27}L_{ij11}^{V8,LR} + \frac{44}{27}L_{ij22}^{V8,LR} - 8L_{11ij}^{V1,LL} - 8L_{22ij}^{V1,LL} + \frac{44}{27}L_{11ij}^{V8,LL} \\
& + \frac{44}{27}L_{22ij}^{V8,LL} \Big] + \alpha_s \alpha \Big[ \frac{112}{9}L_{ijii}^{V1,LR} + \frac{16}{9}L_{ijjj}^{V1,LR} - \frac{1208}{729}L_{ijii}^{V8,LR} - \frac{992}{729}L_{ijjj}^{V8,LR} \\
& + \frac{1120}{243}L_{ijii}^{V,LL} + \frac{1120}{243}L_{ijjj}^{V,LL} - \frac{32}{9}L_{ij11}^{V1,LR} - \frac{32}{9}L_{ij22}^{V1,LR} + \frac{1384}{729}L_{ij11}^{V8,LR} + \frac{1384}{729}L_{ij22}^{V8,LR} \\
& - \frac{32}{9}L_{11ij}^{V1,LL} - \frac{32}{9}L_{22ij}^{V1,LL} - \frac{56}{729}L_{11ij}^{V8,LL} - \frac{56}{729}L_{22ij}^{V8,LL} \Big] + \alpha^2 \Big[ \frac{15614}{729}L_{ijii}^{V1,LR} \\
& + \frac{296}{729}L_{ijjj}^{V1,LR} - \frac{608}{729}L_{ijii}^{V,LL} - \frac{608}{729}L_{ijjj}^{V,LL} + \frac{1016}{729}L_{ij11}^{V,LR} + \frac{1016}{729}L_{ij22}^{V,LR} \\
& + \frac{1016}{729}L_{ij33}^{V,LR} - \frac{1672}{729}L_{ij11}^{V1,LR} - \frac{1672}{729}L_{ij22}^{V1,LR} + \frac{152}{729}L_{11ij}^{V,LL} + \frac{152}{729}L_{22ij}^{V,LL} \\
& + \frac{152}{729}L_{33ij}^{V,LL} - \frac{2824}{729}L_{11ij}^{V1,LL} - \frac{2824}{729}L_{22ij}^{V1,LL} \Big] ; \\
\dot{L}_{ijii}^{V8,LR} = & g_s^2 \Big[ -12L_{ijii}^{V1,LR} - \frac{40}{3}L_{ijii}^{V8,LR} + \frac{2}{3}L_{ijjj}^{V8,LR} + \frac{8}{3}L_{ijii}^{V,LL} + \frac{8}{3}L_{ijjj}^{V,LL} \\
& + \frac{2}{3}L_{ij11}^{V8,LR} + \frac{2}{3}L_{ij22}^{V8,LR} + \frac{2}{3}L_{11ij}^{V8,LL} + \frac{2}{3}L_{22ij}^{V8,LL} \Big] - \frac{4}{3}e^2 L_{ijii}^{V8,LR} + \alpha_s^2 \Big[ -132L_{ijii}^{V1,LR}
\end{aligned}$$

$$\begin{aligned}
& -\frac{22}{3}L_{ijj}^{V1,LR} - \frac{25177}{162}L_{ijii}^{V8,LR} + \frac{799}{81}L_{ijjj}^{V8,LR} + \frac{1210}{27}L_{ijii}^{V,LL} + \frac{1210}{27}L_{ijjj}^{V,LL} \\
& -\frac{22}{3}L_{ij11}^{V1,LR} - \frac{22}{3}L_{ij22}^{V1,LR} + \frac{799}{81}L_{ij11}^{V8,LR} + \frac{799}{81}L_{ij22}^{V8,LR} - \frac{2}{3}L_{11ij}^{V1,LL} - \frac{2}{3}L_{22ij}^{V1,LL} \\
& + \frac{619}{81}L_{11ij}^{V8,LL} + \frac{619}{81}L_{22ij}^{V8,LL} \Big] + \alpha_s \alpha \Big[ \frac{152}{81}L_{ijii}^{V1,LR} + \frac{260}{81}L_{ijjj}^{V1,LR} - \frac{4}{3}L_{ijii}^{V8,LR} \\
& + \frac{14}{9}L_{ijjj}^{V8,LR} + \frac{292}{81}L_{ijii}^{V,LL} + \frac{292}{81}L_{ijjj}^{V,LL} + \frac{260}{81}L_{ij11}^{V,LR} + \frac{260}{81}L_{ij22}^{V,LR} + \frac{260}{81}L_{ij33}^{V,LR} \\
& - \frac{520}{81}L_{ij11}^{V1,LR} - \frac{520}{81}L_{ij22}^{V1,LR} + \frac{2}{3}L_{ij11}^{V8,LR} + \frac{2}{3}L_{ij22}^{V8,LR} + \frac{260}{81}L_{11ij}^{V,LL} + \frac{260}{81}L_{22ij}^{V,LL} \\
& + \frac{260}{81}L_{33ij}^{V,LL} - \frac{520}{81}L_{11ij}^{V1,LL} - \frac{520}{81}L_{22ij}^{V1,LL} + \frac{122}{27}L_{11ij}^{V8,LL} + \frac{122}{27}L_{22ij}^{V8,LL} \Big] \\
& + \frac{1702}{81}\alpha^2 L_{ijii}^{V8,LR} ;
\end{aligned}$$

$$\begin{aligned}
\dot{L}_{ed11ij}^{S,RL} = & -8g_s^2 L_{ed11ij}^{S,RL} - \frac{20}{3}e^2 L_{ed11ij}^{S,RL} - \frac{1012}{9}\alpha_s^2 L_{ed11ij}^{S,RL} - \frac{8}{9}\alpha_s \alpha L_{ed11ij}^{S,RL} \\
& + \frac{6614}{81}\alpha^2 L_{ed11ij}^{S,RL} ;
\end{aligned}$$

$$\begin{aligned}
\dot{L}_{ed22ij}^{S,RL} = & -8g_s^2 L_{ed22ij}^{S,RL} - \frac{20}{3}e^2 L_{ed22ij}^{S,RL} - \frac{1012}{9}\alpha_s^2 L_{ed22ij}^{S,RL} - \frac{8}{9}\alpha_s \alpha L_{ed22ij}^{S,RL} \\
& + \frac{6614}{81}\alpha^2 L_{ed22ij}^{S,RL} ;
\end{aligned}$$

$$\begin{aligned}
\dot{L}_{ed33ij}^{S,RL} = & -8g_s^2 L_{ed33ij}^{S,RL} - \frac{20}{3}e^2 L_{ed33ij}^{S,RL} - \frac{1012}{9}\alpha_s^2 L_{ed33ij}^{S,RL} - \frac{8}{9}\alpha_s \alpha L_{ed33ij}^{S,RL} \\
& + \frac{6614}{81}\alpha^2 L_{ed33ij}^{S,RL} ;
\end{aligned}$$

$$\begin{aligned}
\dot{L}_{uddu1ji1}^{V1,LR} = & -\frac{8}{3}g_s^2 L_{uddu1ji1}^{V8,LR} - \frac{10}{3}e^2 L_{uddu1ji1}^{V1,LR} + \alpha_s^2 \left[ -\frac{28}{3}L_{uddu1ji1}^{V1,LR} - \frac{2044}{27}L_{uddu1ji1}^{V8,LR} \right] \\
& + \alpha_s \alpha \left[ \frac{8}{3}L_{uddu1ji1}^{V1,LR} - \frac{128}{27}L_{uddu1ji1}^{V8,LR} \right] + \frac{169}{81}\alpha^2 L_{uddu1ji1}^{V1,LR} ;
\end{aligned}$$

$$\begin{aligned}
\dot{L}_{uddu1ji1}^{V8,LR} = & g_s^2 \left[ -12L_{uddu1ji1}^{V1,LR} - 14L_{uddu1ji1}^{V8,LR} \right] - \frac{10}{3}e^2 L_{uddu1ji1}^{V8,LR} + \alpha_s^2 \left[ -\frac{374}{3}L_{uddu1ji1}^{V1,LR} \right.
\end{aligned}$$

$$\begin{aligned}
& -\frac{2975}{18}L_{1ji1}^{V8,LR} \Big] + \alpha_s \alpha \left[ \frac{16}{9}L_{1ji1}^{V8,LR} - \frac{64}{3}L_{1ji1}^{V1,LR} \right] + \frac{169}{81}\alpha^2 L_{1ji1}^{V8,LR} ; \\
\dot{L}_{2ji2}^{V1,LR} &= -\frac{8}{3}g_s^2 L_{2ji2}^{V8,LR} - \frac{10}{3}e^2 L_{2ji2}^{V1,LR} + \alpha_s^2 \left[ -\frac{28}{3}L_{2ji2}^{V1,LR} - \frac{2044}{27}L_{2ji2}^{V8,LR} \right] \\
& + \alpha_s \alpha \left[ \frac{8}{3}L_{2ji2}^{V1,LR} - \frac{128}{27}L_{2ji2}^{V8,LR} \right] + \frac{169}{81}\alpha^2 L_{2ji2}^{V1,LR} ; \\
\dot{L}_{2ji2}^{V8,LR} &= g_s^2 \left[ -12L_{2ji2}^{V1,LR} - 14L_{2ji2}^{V8,LR} \right] - \frac{10}{3}e^2 L_{2ji2}^{V8,LR} + \alpha_s^2 \left[ -\frac{374}{3}L_{2ji2}^{V1,LR} \right. \\
& \left. - \frac{2975}{18}L_{2ji2}^{V8,LR} \right] + \alpha_s \alpha \left[ \frac{16}{9}L_{2ji2}^{V8,LR} - \frac{64}{3}L_{2ji2}^{V1,LR} \right] + \frac{169}{81}\alpha^2 L_{2ji2}^{V8,LR} ; \\
\dot{L}_{11ij}^{S,RR} &= -8g_s^2 L_{11ij}^{S,RR} + e^2 \left[ -\frac{20}{3}L_{11ij}^{S,RR} - 32L_{11ij}^{T,RR} \right] - \frac{1012}{9}\alpha_s^2 L_{11ij}^{S,RR} \\
& + \alpha_s \alpha \left[ \frac{1792}{9}L_{11ij}^{T,RR} - \frac{8}{9}L_{11ij}^{S,RR} \right] + \alpha^2 \left[ \frac{1682}{81}L_{11ij}^{S,RR} + 704L_{11ij}^{T,RR} \right] ; \\
\dot{L}_{11ij}^{T,RR} &= \frac{8}{3}g_s^2 L_{11ij}^{T,RR} + e^2 \left[ \frac{20}{9}L_{11ij}^{T,RR} - \frac{2}{3}L_{11ij}^{S,RR} \right] + \frac{1652}{27}\alpha_s^2 L_{11ij}^{T,RR} \\
& + \alpha_s \alpha \left[ \frac{16}{3}L_{11ij}^{S,RR} - \frac{152}{27}L_{11ij}^{T,RR} \right] + \alpha^2 \left[ \frac{364}{81}L_{11ij}^{S,RR} - \frac{6922}{243}L_{11ij}^{T,RR} \right] ; \\
\dot{L}_{22ij}^{S,RR} &= -8g_s^2 L_{22ij}^{S,RR} + e^2 \left[ -\frac{20}{3}L_{22ij}^{S,RR} - 32L_{22ij}^{T,RR} \right] - \frac{1012}{9}\alpha_s^2 L_{22ij}^{S,RR} \\
& + \alpha_s \alpha \left[ \frac{1792}{9}L_{22ij}^{T,RR} - \frac{8}{9}L_{22ij}^{S,RR} \right] + \alpha^2 \left[ \frac{1682}{81}L_{22ij}^{S,RR} + 704L_{22ij}^{T,RR} \right] ; \\
\dot{L}_{22ij}^{T,RR} &= \frac{8}{3}g_s^2 L_{22ij}^{T,RR} + e^2 \left[ \frac{20}{9}L_{22ij}^{T,RR} - \frac{2}{3}L_{22ij}^{S,RR} \right] + \frac{1652}{27}\alpha_s^2 L_{22ij}^{T,RR} \\
& + \alpha_s \alpha \left[ \frac{16}{3}L_{22ij}^{S,RR} - \frac{152}{27}L_{22ij}^{T,RR} \right] + \alpha^2 \left[ \frac{364}{81}L_{22ij}^{S,RR} - \frac{6922}{243}L_{22ij}^{T,RR} \right] ; \\
\dot{L}_{33ij}^{S,RR} &= -8g_s^2 L_{33ij}^{S,RR} + e^2 \left[ -\frac{20}{3}L_{33ij}^{S,RR} - 32L_{33ij}^{T,RR} \right] - \frac{1012}{9}\alpha_s^2 L_{33ij}^{S,RR}
\end{aligned}$$

$$\begin{aligned}
& + \alpha_s \alpha \left[ \frac{1792}{9} L_{33ij}^{T,RR} - \frac{8}{9} L_{33ij}^{S,RR} \right] + \alpha^2 \left[ \frac{1682}{81} L_{33ij}^{S,RR} + 704 L_{33ij}^{T,RR} \right] ; \\
\dot{L}_{33ij}^{T,RR} & = \frac{8}{3} g_s^2 L_{33ij}^{T,RR} + e^2 \left[ \frac{20}{9} L_{33ij}^{T,RR} - \frac{2}{3} L_{33ij}^{S,RR} \right] + \frac{1652}{27} \alpha_s^2 L_{33ij}^{T,RR} \\
& + \alpha_s \alpha \left[ \frac{16}{3} L_{33ij}^{S,RR} - \frac{152}{27} L_{33ij}^{T,RR} \right] + \alpha^2 \left[ \frac{364}{81} L_{33ij}^{S,RR} - \frac{6922}{243} L_{33ij}^{T,RR} \right] ; \\
\dot{L}_{11ij}^{S1,RR} & = g_s^2 \left[ \frac{64}{9} L_{1ji1}^{S1,RR} + \frac{112}{27} L_{1ji1}^{S8,RR} - 16 L_{11ij}^{S1,RR} + \frac{16}{9} L_{11ij}^{S8,RR} \right] \\
& + e^2 \left[ \frac{4}{27} L_{1ji1}^{S1,RR} + \frac{16}{81} L_{1ji1}^{S8,RR} - \frac{46}{9} L_{11ij}^{S1,RR} \right] + \alpha_s^2 \left[ \frac{9472}{81} L_{1ji1}^{S1,RR} + \frac{16576}{243} L_{1ji1}^{S8,RR} \right. \\
& \left. - \frac{2120}{9} L_{11ij}^{S1,RR} + \frac{928}{81} L_{11ij}^{S8,RR} \right] + \alpha_s \alpha \left[ \frac{1888}{81} L_{1ji1}^{S1,RR} + \frac{3808}{243} L_{1ji1}^{S8,RR} + \frac{136}{27} L_{11ij}^{S1,RR} \right. \\
& \left. + \frac{224}{81} L_{11ij}^{S8,RR} \right] + \alpha^2 \left[ \frac{106}{729} L_{1ji1}^{S1,RR} + \frac{424}{2187} L_{1ji1}^{S8,RR} + \frac{6059}{243} L_{11ij}^{S1,RR} \right] ; \\
\dot{L}_{11ij}^{S8,RR} & = g_s^2 \left[ -\frac{16}{3} L_{1ji1}^{S1,RR} + \frac{44}{9} L_{1ji1}^{S8,RR} + 8 L_{11ij}^{S1,RR} + \frac{16}{3} L_{11ij}^{S8,RR} \right] \\
& + e^2 \left[ \frac{8}{9} L_{1ji1}^{S1,RR} - \frac{4}{27} L_{1ji1}^{S8,RR} - \frac{46}{9} L_{11ij}^{S8,RR} \right] + \alpha_s^2 \left[ -\frac{856}{27} L_{1ji1}^{S1,RR} - \frac{2506}{81} L_{1ji1}^{S8,RR} \right. \\
& \left. + \frac{248}{9} L_{11ij}^{S1,RR} + \frac{2995}{27} L_{11ij}^{S8,RR} \right] + \alpha_s \alpha \left[ -\frac{868}{27} L_{1ji1}^{S1,RR} + \frac{1370}{81} L_{1ji1}^{S8,RR} + \frac{112}{9} L_{11ij}^{S1,RR} \right. \\
& \left. + \frac{224}{9} L_{11ij}^{S8,RR} \right] + \alpha^2 \left[ \frac{212}{243} L_{1ji1}^{S1,RR} - \frac{106}{729} L_{1ji1}^{S8,RR} + \frac{6059}{243} L_{11ij}^{S8,RR} \right] ; \\
\dot{L}_{1ji1}^{S1,RR} & = g_s^2 \left[ -16 L_{1ji1}^{S1,RR} + \frac{16}{9} L_{1ji1}^{S8,RR} + \frac{64}{9} L_{11ij}^{S1,RR} + \frac{112}{27} L_{11ij}^{S8,RR} \right] \\
& + e^2 \left[ \frac{26}{9} L_{1ji1}^{S1,RR} - \frac{32}{27} L_{11ij}^{S1,RR} - \frac{128}{81} L_{11ij}^{S8,RR} \right] + \alpha_s^2 \left[ -\frac{2120}{9} L_{1ji1}^{S1,RR} + \frac{928}{81} L_{1ji1}^{S8,RR} \right. \\
& \left. + \frac{9472}{81} L_{11ij}^{S1,RR} + \frac{16576}{243} L_{11ij}^{S8,RR} \right] + \alpha_s \alpha \left[ \frac{712}{27} L_{1ji1}^{S1,RR} - \frac{64}{81} L_{1ji1}^{S8,RR} - \frac{2144}{81} L_{11ij}^{S1,RR} \right.
\end{aligned}$$



$$\begin{aligned}
& -\frac{7784}{243}L_{11ij}^{S8,RR} \Big] + \alpha^2 \Big[ -\frac{13201}{243}L_{1ji1}^{S1,RR} + \frac{5200}{729}L_{11ij}^{S1,RR} + \frac{20800}{2187}L_{11ij}^{S8,RR} \Big] ; \\
\dot{L}_{1ji1}^{S8,RR} &= g_s^2 \Big[ 8L_{1ji1}^{S1,RR} + \frac{16}{3}L_{1ji1}^{S8,RR} - \frac{16}{3}L_{11ij}^{S1,RR} + \frac{44}{9}L_{11ij}^{S8,RR} \Big] \\
& + e^2 \Big[ \frac{26}{9}L_{1ji1}^{S8,RR} - \frac{64}{9}L_{11ij}^{S1,RR} + \frac{32}{27}L_{11ij}^{S8,RR} \Big] + \alpha_s^2 \Big[ \frac{248}{9}L_{1ji1}^{S1,RR} + \frac{2995}{27}L_{1ji1}^{S8,RR} \\
& - \frac{856}{27}L_{11ij}^{S1,RR} - \frac{2506}{81}L_{11ij}^{S8,RR} \Big] + \alpha_s \alpha \Big[ -\frac{32}{9}L_{1ji1}^{S1,RR} - \frac{400}{9}L_{1ji1}^{S8,RR} + \frac{3704}{27}L_{11ij}^{S1,RR} \\
& - \frac{2050}{81}L_{11ij}^{S8,RR} \Big] + \alpha^2 \Big[ -\frac{13201}{243}L_{1ji1}^{S8,RR} + \frac{10400}{243}L_{11ij}^{S1,RR} - \frac{5200}{729}L_{11ij}^{S8,RR} \Big] ; \\
\dot{L}_{22ij}^{S1,RR} &= g_s^2 \Big[ \frac{64}{9}L_{2ji2}^{S1,RR} + \frac{112}{27}L_{2ji2}^{S8,RR} - 16L_{22ij}^{S1,RR} + \frac{16}{9}L_{22ij}^{S8,RR} \Big] \\
& + e^2 \Big[ \frac{4}{27}L_{2ji2}^{S1,RR} + \frac{16}{81}L_{2ji2}^{S8,RR} - \frac{46}{9}L_{22ij}^{S1,RR} \Big] + \alpha_s^2 \Big[ \frac{9472}{81}L_{2ji2}^{S1,RR} + \frac{16576}{243}L_{2ji2}^{S8,RR} \\
& - \frac{2120}{9}L_{22ij}^{S1,RR} + \frac{928}{81}L_{22ij}^{S8,RR} \Big] + \alpha_s \alpha \Big[ \frac{1888}{81}L_{2ji2}^{S1,RR} + \frac{3808}{243}L_{2ji2}^{S8,RR} + \frac{136}{27}L_{22ij}^{S1,RR} \\
& + \frac{224}{81}L_{22ij}^{S8,RR} \Big] + \alpha^2 \Big[ \frac{106}{729}L_{2ji2}^{S1,RR} + \frac{424}{2187}L_{2ji2}^{S8,RR} + \frac{6059}{243}L_{22ij}^{S1,RR} \Big] ; \\
\dot{L}_{22ij}^{S8,RR} &= g_s^2 \Big[ -\frac{16}{3}L_{2ji2}^{S1,RR} + \frac{44}{9}L_{2ji2}^{S8,RR} + 8L_{22ij}^{S1,RR} + \frac{16}{3}L_{22ij}^{S8,RR} \Big] \\
& + e^2 \Big[ \frac{8}{9}L_{2ji2}^{S1,RR} - \frac{4}{27}L_{2ji2}^{S8,RR} - \frac{46}{9}L_{22ij}^{S8,RR} \Big] + \alpha_s^2 \Big[ -\frac{856}{27}L_{2ji2}^{S1,RR} - \frac{2506}{81}L_{2ji2}^{S8,RR} \\
& + \frac{248}{9}L_{22ij}^{S1,RR} + \frac{2995}{27}L_{22ij}^{S8,RR} \Big] + \alpha_s \alpha \Big[ -\frac{868}{27}L_{2ji2}^{S1,RR} + \frac{1370}{81}L_{2ji2}^{S8,RR} + \frac{112}{9}L_{22ij}^{S1,RR} \\
& + \frac{224}{9}L_{22ij}^{S8,RR} \Big] + \alpha^2 \Big[ \frac{212}{243}L_{2ji2}^{S1,RR} - \frac{106}{729}L_{2ji2}^{S8,RR} + \frac{6059}{243}L_{22ij}^{S8,RR} \Big] ; \\
\dot{L}_{2ji2}^{S1,RR} &= g_s^2 \Big[ -16L_{2ji2}^{S1,RR} + \frac{16}{9}L_{2ji2}^{S8,RR} + \frac{64}{9}L_{22ij}^{S1,RR} + \frac{112}{27}L_{22ij}^{S8,RR} \Big]
\end{aligned}$$

$$\begin{aligned}
& + e^2 \left[ \frac{26}{9} L_{2ji2}^{S1,RR} - \frac{32}{27} L_{22ij}^{S1,RR} - \frac{128}{81} L_{22ij}^{S8,RR} \right] + \alpha_s^2 \left[ -\frac{2120}{9} L_{2ji2}^{S1,RR} + \frac{928}{81} L_{2ji2}^{S8,RR} \right. \\
& + \frac{9472}{81} L_{22ij}^{S1,RR} + \frac{16576}{243} L_{22ij}^{S8,RR} \left. \right] + \alpha_s \alpha \left[ \frac{712}{27} L_{2ji2}^{S1,RR} - \frac{64}{81} L_{2ji2}^{S8,RR} - \frac{2144}{81} L_{22ij}^{S1,RR} \right. \\
& - \frac{7784}{243} L_{22ij}^{S8,RR} \left. \right] + \alpha^2 \left[ -\frac{13201}{243} L_{2ji2}^{S1,RR} + \frac{5200}{729} L_{22ij}^{S1,RR} + \frac{20800}{2187} L_{22ij}^{S8,RR} \right]; \\
\dot{L}_{2ji2}^{S8,RR} & = g_s^2 \left[ 8 L_{2ji2}^{S1,RR} + \frac{16}{3} L_{2ji2}^{S8,RR} - \frac{16}{3} L_{22ij}^{S1,RR} + \frac{44}{9} L_{22ij}^{S8,RR} \right] \\
& + e^2 \left[ \frac{26}{9} L_{2ji2}^{S8,RR} - \frac{64}{9} L_{22ij}^{S1,RR} + \frac{32}{27} L_{22ij}^{S8,RR} \right] + \alpha_s^2 \left[ \frac{248}{9} L_{2ji2}^{S1,RR} + \frac{2995}{27} L_{2ji2}^{S8,RR} \right. \\
& - \frac{856}{27} L_{22ij}^{S1,RR} - \frac{2506}{81} L_{22ij}^{S8,RR} \left. \right] + \alpha_s \alpha \left[ -\frac{32}{9} L_{2ji2}^{S1,RR} - \frac{400}{9} L_{2ji2}^{S8,RR} + \frac{3704}{27} L_{22ij}^{S1,RR} \right. \\
& - \frac{2050}{81} L_{22ij}^{S8,RR} \left. \right] + \alpha^2 \left[ -\frac{13201}{243} L_{2ji2}^{S8,RR} + \frac{10400}{243} L_{22ij}^{S1,RR} - \frac{5200}{729} L_{22ij}^{S8,RR} \right]; \\
\dot{L}_{ijj}^{S1,RR} & = g_s^2 \left[ \frac{160}{27} L_{ijj}^{S8,RR} - \frac{80}{9} L_{ijj}^{S1,RR} \right] + e^2 \left[ \frac{4}{27} L_{ijj}^{S1,RR} + \frac{64}{81} L_{ijj}^{S8,RR} \right] \\
& + \alpha_s^2 \left[ \frac{19360}{243} L_{ijj}^{S8,RR} - \frac{9608}{81} L_{ijj}^{S1,RR} \right] + \alpha_s \alpha \left[ \frac{352}{243} L_{ijj}^{S8,RR} - \frac{1040}{81} L_{ijj}^{S1,RR} \right] \\
& + \alpha^2 \left[ \frac{4354}{729} L_{ijj}^{S1,RR} - \frac{3200}{2187} L_{ijj}^{S8,RR} \right]; \\
\dot{L}_{ijj}^{S8,RR} & = g_s^2 \left[ \frac{8}{3} L_{ijj}^{S1,RR} + \frac{92}{9} L_{ijj}^{S8,RR} \right] + e^2 \left[ \frac{32}{9} L_{ijj}^{S1,RR} - \frac{28}{27} L_{ijj}^{S8,RR} \right] \\
& + \alpha_s^2 \left[ \frac{6479}{81} L_{ijj}^{S8,RR} - \frac{112}{27} L_{ijj}^{S1,RR} \right] + \alpha_s \alpha \left[ -\frac{1840}{27} L_{ijj}^{S1,RR} - \frac{208}{81} L_{ijj}^{S8,RR} \right] \\
& + \alpha^2 \left[ \frac{5954}{729} L_{ijj}^{S8,RR} - \frac{1600}{243} L_{ijj}^{S1,RR} \right]; \\
\dot{L}_{iji}^{S1,RR} & = g_s^2 \left[ \frac{160}{27} L_{iji}^{S8,RR} - \frac{80}{9} L_{iji}^{S1,RR} \right] + e^2 \left[ \frac{4}{27} L_{iji}^{S1,RR} + \frac{64}{81} L_{iji}^{S8,RR} \right]
\end{aligned}$$

$$\begin{aligned}
& + \alpha_s^2 \left[ \frac{19360}{243} L_{ij\bar{i}\bar{i}}^{S8,RR} - \frac{9608}{81} L_{ij\bar{i}\bar{i}}^{S1,RR} \right] + \alpha_s \alpha \left[ \frac{352}{243} L_{ij\bar{i}\bar{i}}^{S8,RR} - \frac{1040}{81} L_{ij\bar{i}\bar{i}}^{S1,RR} \right] \\
& + \alpha^2 \left[ \frac{4354}{729} L_{ij\bar{i}\bar{i}}^{S1,RR} - \frac{3200}{2187} L_{ij\bar{i}\bar{i}}^{S8,RR} \right]; \\
\dot{L}_{ij\bar{i}\bar{i}}^{S8,RR} & = g_s^2 \left[ \frac{8}{3} L_{ij\bar{i}\bar{i}}^{S1,RR} + \frac{92}{9} L_{ij\bar{i}\bar{i}}^{S8,RR} \right] + e^2 \left[ \frac{32}{9} L_{ij\bar{i}\bar{i}}^{S1,RR} - \frac{28}{27} L_{ij\bar{i}\bar{i}}^{S8,RR} \right] \\
& + \alpha_s^2 \left[ \frac{6479}{81} L_{ij\bar{i}\bar{i}}^{S8,RR} - \frac{112}{27} L_{ij\bar{i}\bar{i}}^{S1,RR} \right] + \alpha_s \alpha \left[ -\frac{1840}{27} L_{ij\bar{i}\bar{i}}^{S1,RR} - \frac{208}{81} L_{ij\bar{i}\bar{i}}^{S8,RR} \right] \\
& + \alpha^2 \left[ \frac{5954}{729} L_{ij\bar{i}\bar{i}}^{S8,RR} - \frac{1600}{243} L_{ij\bar{i}\bar{i}}^{S1,RR} \right]; \\
\dot{L}_{11ij}^{V,RR} & = e^2 \left[ \frac{4}{3} L_{i\bar{i}j}^{V1,LR} + \frac{4}{3} L_{j\bar{j}i}^{V1,LR} + \frac{32}{9} L_{ij\bar{i}\bar{i}}^{V,RR} + \frac{32}{9} L_{ij\bar{j}\bar{j}}^{V,RR} + \frac{4}{3} L_{11ij}^{V,LR} \right. \\
& + \frac{4}{3} L_{22ij}^{V,LR} + \frac{4}{3} L_{33ij}^{V,LR} + \frac{16}{3} L_{11ij}^{V,RR} + \frac{4}{3} L_{22ij}^{V,RR} + \frac{4}{3} L_{33ij}^{V,RR} - \frac{8}{3} L_{11ij}^{V1,LR} \\
& - \frac{8}{3} L_{22ij}^{V1,LR} - \frac{8}{3} L_{11ij}^{V1,RR} - \frac{8}{3} L_{22ij}^{V1,RR} \left. \right] + \alpha_s \alpha \left[ \frac{16}{3} L_{i\bar{i}j}^{V1,LR} + \frac{16}{3} L_{j\bar{j}i}^{V1,LR} \right. \\
& - \frac{992}{243} L_{i\bar{i}j}^{V8,LR} - \frac{992}{243} L_{j\bar{j}i}^{V8,LR} + \frac{1120}{81} L_{ij\bar{i}\bar{i}}^{V,RR} + \frac{1120}{81} L_{ij\bar{j}\bar{j}}^{V,RR} - 16 L_{11ij}^{V,RR} - \frac{32}{3} L_{11ij}^{V1,LR} \\
& - \frac{32}{3} L_{22ij}^{V1,LR} - \frac{32}{3} L_{11ij}^{V1,RR} - \frac{32}{3} L_{22ij}^{V1,RR} + \frac{1384}{243} L_{11ij}^{V8,LR} + \frac{1384}{243} L_{22ij}^{V8,LR} - \frac{56}{243} L_{11ij}^{V8,RR} \\
& - \frac{56}{243} L_{22ij}^{V8,RR} \left. \right] + \alpha^2 \left[ -\frac{1288}{243} L_{i\bar{i}j}^{V1,LR} - \frac{1288}{243} L_{j\bar{j}i}^{V1,LR} + \frac{4864}{243} L_{ij\bar{i}\bar{i}}^{V,RR} + \frac{4864}{243} L_{ij\bar{j}\bar{j}}^{V,RR} \right. \\
& - \frac{3160}{243} L_{11ij}^{V,LR} - \frac{3160}{243} L_{22ij}^{V,LR} - \frac{3160}{243} L_{33ij}^{V,LR} + \frac{746}{243} L_{11ij}^{V,RR} + \frac{3752}{243} L_{22ij}^{V,RR} \\
& + \frac{3752}{243} L_{33ij}^{V,RR} - \frac{6280}{243} L_{11ij}^{V1,LR} - \frac{6280}{243} L_{22ij}^{V1,LR} + \frac{2936}{243} L_{11ij}^{V1,RR} + \frac{2936}{243} L_{22ij}^{V1,RR} \left. \right]; \\
\dot{L}_{22ij}^{V,RR} & = e^2 \left[ \frac{4}{3} L_{i\bar{i}j}^{V1,LR} + \frac{4}{3} L_{j\bar{j}i}^{V1,LR} + \frac{32}{9} L_{ij\bar{i}\bar{i}}^{V,RR} + \frac{32}{9} L_{ij\bar{j}\bar{j}}^{V,RR} + \frac{4}{3} L_{11ij}^{V,LR} \right. \\
& + \frac{4}{3} L_{22ij}^{V,LR} + \frac{4}{3} L_{33ij}^{V,LR} + \frac{4}{3} L_{11ij}^{V,RR} + \frac{16}{3} L_{22ij}^{V,RR} + \frac{4}{3} L_{33ij}^{V,RR} - \frac{8}{3} L_{11ij}^{V1,LR} \\
& - \frac{8}{3} L_{22ij}^{V1,LR} - \frac{8}{3} L_{11ij}^{V1,RR} - \frac{8}{3} L_{22ij}^{V1,RR} \left. \right] + \alpha_s \alpha \left[ \frac{16}{3} L_{i\bar{i}j}^{V1,LR} + \frac{16}{3} L_{j\bar{j}i}^{V1,LR} \right. \\
& - \frac{992}{243} L_{i\bar{i}j}^{V8,LR} - \frac{992}{243} L_{j\bar{j}i}^{V8,LR} + \frac{1120}{81} L_{ij\bar{i}\bar{i}}^{V,RR} + \frac{1120}{81} L_{ij\bar{j}\bar{j}}^{V,RR} - 16 L_{11ij}^{V,RR} - \frac{32}{3} L_{11ij}^{V1,LR} \\
& - \frac{32}{3} L_{22ij}^{V1,LR} - \frac{32}{3} L_{11ij}^{V1,RR} - \frac{32}{3} L_{22ij}^{V1,RR} + \frac{1384}{243} L_{11ij}^{V8,LR} + \frac{1384}{243} L_{22ij}^{V8,LR} - \frac{56}{243} L_{11ij}^{V8,RR} \\
& - \frac{56}{243} L_{22ij}^{V8,RR} \left. \right] + \alpha^2 \left[ -\frac{1288}{243} L_{i\bar{i}j}^{V1,LR} - \frac{1288}{243} L_{j\bar{j}i}^{V1,LR} + \frac{4864}{243} L_{ij\bar{i}\bar{i}}^{V,RR} + \frac{4864}{243} L_{ij\bar{j}\bar{j}}^{V,RR} \right. \\
& - \frac{3160}{243} L_{11ij}^{V,LR} - \frac{3160}{243} L_{22ij}^{V,LR} - \frac{3160}{243} L_{33ij}^{V,LR} + \frac{746}{243} L_{11ij}^{V,RR} + \frac{3752}{243} L_{22ij}^{V,RR} \\
& + \frac{3752}{243} L_{33ij}^{V,RR} - \frac{6280}{243} L_{11ij}^{V1,LR} - \frac{6280}{243} L_{22ij}^{V1,LR} + \frac{2936}{243} L_{11ij}^{V1,RR} + \frac{2936}{243} L_{22ij}^{V1,RR} \left. \right];
\end{aligned}$$

$$\begin{aligned}
& -\frac{8}{3}L_{22ij}^{V1,LR} - \frac{8}{3}L_{11ij}^{V1,RR} - \frac{8}{3}L_{22ij}^{V1,RR} \Big] + \alpha_s \alpha \Big[ \frac{16}{3}L_{\bar{ii}j}^{V1,LR} + \frac{16}{3}L_{jjj}^{V1,LR} \\
& - \frac{992}{243}L_{\bar{ii}j}^{V8,LR} - \frac{992}{243}L_{jjj}^{V8,LR} + \frac{1120}{81}L_{\bar{ii}i}^{V,RR} + \frac{1120}{81}L_{ijj}^{V,RR} - 16L_{22ij}^{V,RR} - \frac{32}{3}L_{11ij}^{V1,LR} \\
& - \frac{32}{3}L_{22ij}^{V1,LR} - \frac{32}{3}L_{11ij}^{V1,RR} - \frac{32}{3}L_{22ij}^{V1,RR} + \frac{1384}{243}L_{11ij}^{V8,LR} + \frac{1384}{243}L_{22ij}^{V8,LR} - \frac{56}{243}L_{11ij}^{V8,RR} \\
& - \frac{56}{243}L_{22ij}^{V8,RR} \Big] + \alpha^2 \Big[ -\frac{1288}{243}L_{\bar{ii}j}^{V1,LR} - \frac{1288}{243}L_{jjj}^{V1,LR} + \frac{4864}{243}L_{\bar{ii}i}^{V,RR} + \frac{4864}{243}L_{ijj}^{V,RR} \\
& - \frac{3160}{243}L_{11ij}^{V,LR} - \frac{3160}{243}L_{22ij}^{V,LR} - \frac{3160}{243}L_{33ij}^{V,LR} + \frac{3752}{243}L_{11ij}^{V,RR} + \frac{746}{243}L_{22ij}^{V,RR} \\
& + \frac{3752}{243}L_{33ij}^{V,RR} - \frac{6280}{243}L_{11ij}^{V1,LR} - \frac{6280}{243}L_{22ij}^{V1,LR} + \frac{2936}{243}L_{11ij}^{V1,RR} + \frac{2936}{243}L_{22ij}^{V1,RR} \Big] ;
\end{aligned}$$

$$\begin{aligned}
\dot{L}_{33ij}^{V,RR} &= e^2 \Big[ \frac{4}{3}L_{\bar{ii}j}^{V1,LR} + \frac{4}{3}L_{jjj}^{V1,LR} + \frac{32}{9}L_{\bar{ii}i}^{V,RR} + \frac{32}{9}L_{ijj}^{V,RR} + \frac{4}{3}L_{11ij}^{V,LR} \\
& + \frac{4}{3}L_{22ij}^{V,LR} + \frac{4}{3}L_{33ij}^{V,LR} + \frac{4}{3}L_{11ij}^{V,RR} + \frac{4}{3}L_{22ij}^{V,RR} + \frac{16}{3}L_{33ij}^{V,RR} - \frac{8}{3}L_{11ij}^{V1,LR} \\
& - \frac{8}{3}L_{22ij}^{V1,LR} - \frac{8}{3}L_{11ij}^{V1,RR} - \frac{8}{3}L_{22ij}^{V1,RR} \Big] + \alpha_s \alpha \Big[ \frac{16}{3}L_{\bar{ii}j}^{V1,LR} + \frac{16}{3}L_{jjj}^{V1,LR} \\
& - \frac{992}{243}L_{\bar{ii}j}^{V8,LR} - \frac{992}{243}L_{jjj}^{V8,LR} + \frac{1120}{81}L_{\bar{ii}i}^{V,RR} + \frac{1120}{81}L_{ijj}^{V,RR} - 16L_{33ij}^{V,RR} - \frac{32}{3}L_{11ij}^{V1,LR} \\
& - \frac{32}{3}L_{22ij}^{V1,LR} - \frac{32}{3}L_{11ij}^{V1,RR} - \frac{32}{3}L_{22ij}^{V1,RR} + \frac{1384}{243}L_{11ij}^{V8,LR} + \frac{1384}{243}L_{22ij}^{V8,LR} - \frac{56}{243}L_{11ij}^{V8,RR} \\
& - \frac{56}{243}L_{22ij}^{V8,RR} \Big] + \alpha^2 \Big[ -\frac{1288}{243}L_{\bar{ii}j}^{V1,LR} - \frac{1288}{243}L_{jjj}^{V1,LR} + \frac{4864}{243}L_{\bar{ii}i}^{V,RR} + \frac{4864}{243}L_{ijj}^{V,RR} \\
& - \frac{3160}{243}L_{11ij}^{V,LR} - \frac{3160}{243}L_{22ij}^{V,LR} - \frac{3160}{243}L_{33ij}^{V,LR} + \frac{3752}{243}L_{11ij}^{V,RR} + \frac{3752}{243}L_{22ij}^{V,RR} \\
& + \frac{746}{243}L_{33ij}^{V,RR} - \frac{6280}{243}L_{11ij}^{V1,LR} - \frac{6280}{243}L_{22ij}^{V1,LR} + \frac{2936}{243}L_{11ij}^{V1,RR} + \frac{2936}{243}L_{22ij}^{V1,RR} \Big] ;
\end{aligned}$$

$$\begin{aligned}
\dot{L}_{11ij}^{V1,RR} &= \frac{8}{3}g_s^2 L_{11ij}^{V8,RR} + e^2 \Big[ -\frac{8}{9}L_{\bar{ii}j}^{V1,LR} - \frac{8}{9}L_{jjj}^{V1,LR} - \frac{64}{27}L_{\bar{ii}i}^{V,RR} - \frac{64}{27}L_{ijj}^{V,RR} \\
& - \frac{8}{9}L_{11ij}^{V,LR} - \frac{8}{9}L_{22ij}^{V,LR} - \frac{8}{9}L_{33ij}^{V,LR} - \frac{8}{9}L_{11ij}^{V,RR} - \frac{8}{9}L_{22ij}^{V,RR} - \frac{8}{9}L_{33ij}^{V,RR}
\end{aligned}$$

$$\begin{aligned}
& + \frac{16}{9} L_{11ij}^{V1,LR} + \frac{16}{9} L_{22ij}^{V1,LR} - \frac{8}{9} L_{11ij}^{V1,RR} + \frac{16}{9} L_{22ij}^{V1,RR} \Big] + \alpha_s^2 \Big[ - 8 L_{iii}^{V1,LR} \\
& - 8 L_{jjj}^{V1,LR} + \frac{4}{27} L_{iii}^{V8,LR} + \frac{4}{27} L_{jjj}^{V8,LR} + \frac{328}{9} L_{ijii}^{V,RR} + \frac{328}{9} L_{ijjj}^{V,RR} - 8 L_{11ij}^{V1,LR} \\
& - 8 L_{22ij}^{V1,LR} - \frac{4}{3} L_{11ij}^{V1,RR} + 8 L_{22ij}^{V1,RR} + \frac{4}{27} L_{11ij}^{V8,LR} + \frac{4}{27} L_{22ij}^{V8,LR} + \frac{86}{27} L_{11ij}^{V8,RR} \\
& + \frac{4}{27} L_{22ij}^{V8,RR} \Big] + \alpha_s \alpha \Big[ - \frac{32}{9} L_{iii}^{V1,LR} - \frac{32}{9} L_{jjj}^{V1,LR} + \frac{1984}{729} L_{iii}^{V8,LR} + \frac{1984}{729} L_{jjj}^{V8,LR} \\
& - \frac{2240}{243} L_{ijii}^{V,RR} - \frac{2240}{243} L_{ijjj}^{V,RR} + \frac{64}{9} L_{11ij}^{V1,LR} + \frac{64}{9} L_{22ij}^{V1,LR} + \frac{256}{9} L_{11ij}^{V1,RR} + \frac{64}{9} L_{22ij}^{V1,RR} \\
& - \frac{2768}{729} L_{11ij}^{V8,LR} - \frac{2768}{729} L_{22ij}^{V8,LR} - \frac{104}{729} L_{11ij}^{V8,RR} + \frac{112}{729} L_{22ij}^{V8,RR} \Big] + \alpha^2 \Big[ - \frac{304}{729} L_{iii}^{V1,LR} \\
& - \frac{304}{729} L_{jjj}^{V1,LR} + \frac{8272}{729} L_{ijii}^{V,RR} + \frac{8272}{729} L_{ijjj}^{V,RR} - \frac{3040}{729} L_{11ij}^{V,LR} - \frac{3040}{729} L_{22ij}^{V,LR} \\
& - \frac{3040}{729} L_{33ij}^{V,LR} + \frac{2576}{729} L_{11ij}^{V,RR} + \frac{2576}{729} L_{22ij}^{V,RR} + \frac{2576}{729} L_{33ij}^{V,RR} - \frac{1120}{729} L_{11ij}^{V1,RR} \\
& - \frac{1120}{729} L_{22ij}^{V1,RR} + \frac{5360}{729} L_{11ij}^{V1,RR} + \frac{6368}{729} L_{22ij}^{V1,RR} \Big] ;
\end{aligned}$$

$$\begin{aligned}
\dot{L}_{11ij}^{V8,RR} & = g_s^2 \Big[ \frac{2}{3} L_{iii}^{V8,LR} + \frac{2}{3} L_{jjj}^{V8,LR} + \frac{8}{3} L_{ijii}^{V,RR} + \frac{8}{3} L_{ijjj}^{V,RR} + 12 L_{11ij}^{V1,RR} \\
& + \frac{2}{3} L_{11ij}^{V8,LR} + \frac{2}{3} L_{22ij}^{V8,LR} - \frac{10}{3} L_{11ij}^{V8,RR} + \frac{2}{3} L_{22ij}^{V8,RR} \Big] - \frac{8}{3} e^2 L_{11ij}^{V8,RR} + \alpha_s^2 \Big[ - \frac{22}{3} L_{iii}^{V1,LR} \\
& - \frac{22}{3} L_{jjj}^{V1,LR} + \frac{169}{81} L_{iii}^{V8,LR} + \frac{169}{81} L_{jjj}^{V8,LR} + \frac{1930}{27} L_{ijii}^{V,RR} + \frac{1930}{27} L_{ijjj}^{V,RR} - \frac{22}{3} L_{11ij}^{V1,LR} \\
& - \frac{22}{3} L_{22ij}^{V1,LR} + 13 L_{11ij}^{V1,RR} - \frac{2}{3} L_{22ij}^{V1,RR} + \frac{169}{81} L_{11ij}^{V8,LR} + \frac{169}{81} L_{22ij}^{V8,LR} - \frac{326}{81} L_{11ij}^{V8,RR} \\
& + \frac{799}{81} L_{22ij}^{V8,RR} \Big] + \alpha_s \alpha \Big[ - \frac{208}{81} L_{iii}^{V1,LR} - \frac{208}{81} L_{jjj}^{V1,LR} + \frac{52}{27} L_{iii}^{V8,LR} + \frac{52}{27} L_{jjj}^{V8,LR} \\
& - \frac{3200}{81} L_{ijii}^{V,RR} - \frac{3200}{81} L_{ijjj}^{V,RR} - \frac{208}{81} L_{11ij}^{V,LR} - \frac{208}{81} L_{22ij}^{V,LR} - \frac{208}{81} L_{33ij}^{V,LR} - \frac{208}{81} L_{11ij}^{V,RR} \\
& - \frac{208}{81} L_{22ij}^{V,RR} - \frac{208}{81} L_{33ij}^{V,RR} + \frac{416}{81} L_{11ij}^{V1,LR} + \frac{416}{81} L_{22ij}^{V1,LR} + \frac{308}{81} L_{11ij}^{V1,RR} + \frac{416}{81} L_{22ij}^{V1,RR}
\end{aligned}$$

$$\begin{aligned}
& -\frac{80}{27}L_{11ij}^{V8,LR} - \frac{80}{27}L_{22ij}^{V8,LR} + L_{11ij}^{V8,RR} + \frac{56}{9}L_{22ij}^{V8,RR} \Big] - \frac{112}{81}\alpha^2 L_{11ij}^{V8,RR} ; \\
\dot{L}_{22ij}^{V1,RR} = & \frac{8}{3}g_s^2 L_{22ij}^{V8,RR} + e^2 \Bigg[ -\frac{8}{9}L_{iiij}^{V1,LR} - \frac{8}{9}L_{jjij}^{V1,LR} - \frac{64}{27}L_{ijii}^{V,RR} - \frac{64}{27}L_{ijjj}^{V,RR} \\
& -\frac{8}{9}L_{11ij}^{V,LR} - \frac{8}{9}L_{22ij}^{V,LR} - \frac{8}{9}L_{33ij}^{V,LR} - \frac{8}{9}L_{11ij}^{V,RR} - \frac{8}{9}L_{22ij}^{V,RR} - \frac{8}{9}L_{33ij}^{V,RR} \\
& + \frac{16}{9}L_{11ij}^{V1,LR} + \frac{16}{9}L_{22ij}^{V1,LR} + \frac{16}{9}L_{11ij}^{V1,RR} - \frac{8}{9}L_{22ij}^{V1,RR} \Big] + \alpha_s^2 \Bigg[ -8L_{iiij}^{V1,LR} \\
& -8L_{jjij}^{V1,LR} + \frac{4}{27}L_{iiij}^{V8,LR} + \frac{4}{27}L_{jjij}^{V8,LR} + \frac{328}{9}L_{ijii}^{V,RR} + \frac{328}{9}L_{ijjj}^{V,RR} - 8L_{11ij}^{V1,LR} \\
& -8L_{22ij}^{V1,LR} + 8L_{11ij}^{V1,RR} - \frac{4}{3}L_{22ij}^{V1,RR} + \frac{4}{27}L_{11ij}^{V8,LR} + \frac{4}{27}L_{22ij}^{V8,LR} + \frac{4}{27}L_{11ij}^{V8,RR} \\
& + \frac{86}{27}L_{22ij}^{V8,RR} \Big] + \alpha_s \alpha \Bigg[ -\frac{32}{9}L_{iiij}^{V1,LR} - \frac{32}{9}L_{jjij}^{V1,LR} + \frac{1984}{729}L_{iiij}^{V8,LR} + \frac{1984}{729}L_{jjij}^{V8,LR} \\
& -\frac{2240}{243}L_{ijii}^{V,RR} - \frac{2240}{243}L_{ijjj}^{V,RR} + \frac{64}{9}L_{11ij}^{V1,LR} + \frac{64}{9}L_{22ij}^{V1,LR} + \frac{64}{9}L_{11ij}^{V1,RR} + \frac{256}{9}L_{22ij}^{V1,RR} \\
& -\frac{2768}{729}L_{11ij}^{V8,LR} - \frac{2768}{729}L_{22ij}^{V8,LR} + \frac{112}{729}L_{11ij}^{V8,RR} - \frac{104}{729}L_{22ij}^{V8,RR} \Big] + \alpha^2 \Bigg[ -\frac{304}{729}L_{iiij}^{V1,LR} \\
& -\frac{304}{729}L_{jjij}^{V1,LR} + \frac{8272}{729}L_{ijii}^{V,RR} + \frac{8272}{729}L_{ijjj}^{V,RR} - \frac{3040}{729}L_{11ij}^{V,LR} - \frac{3040}{729}L_{22ij}^{V,LR} \\
& -\frac{3040}{729}L_{33ij}^{V,LR} + \frac{2576}{729}L_{11ij}^{V,RR} + \frac{2576}{729}L_{22ij}^{V,RR} + \frac{2576}{729}L_{33ij}^{V,RR} - \frac{1120}{729}L_{11ij}^{V1,LR} \\
& -\frac{1120}{729}L_{22ij}^{V1,LR} + \frac{6368}{729}L_{11ij}^{V1,RR} + \frac{5360}{729}L_{22ij}^{V1,RR} \Big] ; \\
\dot{L}_{22ij}^{V8,RR} = & g_s^2 \Bigg[ \frac{2}{3}L_{iiij}^{V8,LR} + \frac{2}{3}L_{jjij}^{V8,LR} + \frac{8}{3}L_{ijii}^{V,RR} + \frac{8}{3}L_{ijjj}^{V,RR} + 12L_{22ij}^{V1,RR} \\
& + \frac{2}{3}L_{11ij}^{V8,LR} + \frac{2}{3}L_{22ij}^{V8,LR} + \frac{2}{3}L_{11ij}^{V8,RR} - \frac{10}{3}L_{22ij}^{V8,RR} \Big] - \frac{8}{3}e^2 L_{22ij}^{V8,RR} + \alpha_s^2 \Bigg[ -\frac{22}{3}L_{iiij}^{V1,LR} \\
& -\frac{22}{3}L_{jjij}^{V1,LR} + \frac{169}{81}L_{iiij}^{V8,LR} + \frac{169}{81}L_{jjij}^{V8,LR} + \frac{1930}{27}L_{ijii}^{V,RR} + \frac{1930}{27}L_{ijjj}^{V,RR} - \frac{22}{3}L_{11ij}^{V1,LR} \\
& -\frac{22}{3}L_{22ij}^{V1,LR} - \frac{2}{3}L_{11ij}^{V1,RR} + 13L_{22ij}^{V1,RR} + \frac{169}{81}L_{11ij}^{V8,LR} + \frac{169}{81}L_{22ij}^{V8,LR} + \frac{799}{81}L_{11ij}^{V8,RR}
\end{aligned}$$

$$\begin{aligned}
& -\frac{326}{81}L_{22ij}^{V8,RR} \Big] + \alpha_s \alpha \Big[ -\frac{208}{81}L_{iiij}^{V1,LR} - \frac{208}{81}L_{jjij}^{V1,LR} + \frac{52}{27}L_{iiij}^{V8,LR} + \frac{52}{27}L_{jjij}^{V8,LR} \\
& -\frac{3200}{81}L_{ijji}^{V,RR} - \frac{3200}{81}L_{ijjj}^{V,RR} - \frac{208}{81}L_{11ij}^{V,LR} - \frac{208}{81}L_{22ij}^{V,LR} - \frac{208}{81}L_{33ij}^{V,LR} - \frac{208}{81}L_{11ij}^{V,RR} \\
& -\frac{208}{81}L_{22ij}^{V,RR} - \frac{208}{81}L_{33ij}^{V,RR} + \frac{416}{81}L_{11ij}^{V1,LR} + \frac{416}{81}L_{22ij}^{V1,LR} + \frac{416}{81}L_{11ij}^{V1,RR} + \frac{308}{81}L_{22ij}^{V1,RR} \\
& -\frac{80}{27}L_{11ij}^{V8,LR} - \frac{80}{27}L_{22ij}^{V8,LR} + \frac{56}{9}L_{11ij}^{V8,RR} + L_{22ij}^{V8,RR} \Big] - \frac{112}{81}\alpha^2 L_{22ij}^{V8,RR} ; \\
\dot{L}_{ijjj}^{V,RR} &= g_s^2 \Big[ \frac{1}{9}L_{iiij}^{V8,LR} + \frac{1}{9}L_{jjij}^{V8,LR} + \frac{4}{9}L_{ijji}^{V,RR} + \frac{40}{9}L_{ijjj}^{V,RR} + \frac{1}{9}L_{11ij}^{V8,LR} \\
& + \frac{1}{9}L_{22ij}^{V8,LR} + \frac{1}{9}L_{11ij}^{V8,RR} + \frac{1}{9}L_{22ij}^{V8,RR} \Big] + e^2 \Big[ \frac{2}{9}L_{iiij}^{V1,LR} + \frac{2}{9}L_{jjij}^{V1,LR} \\
& + \frac{16}{27}L_{ijji}^{V,RR} + \frac{52}{27}L_{ijjj}^{V,RR} + \frac{2}{9}L_{11ij}^{V,LR} + \frac{2}{9}L_{22ij}^{V,LR} + \frac{2}{9}L_{33ij}^{V,LR} + \frac{2}{9}L_{11ij}^{V,RR} \\
& + \frac{2}{9}L_{22ij}^{V,RR} + \frac{2}{9}L_{33ij}^{V,RR} - \frac{4}{9}L_{11ij}^{V1,LR} - \frac{4}{9}L_{22ij}^{V1,LR} - \frac{4}{9}L_{11ij}^{V1,RR} - \frac{4}{9}L_{22ij}^{V1,RR} \Big] \\
& + \alpha_s^2 \Big[ -\frac{47}{9}L_{iiij}^{V1,LR} - \frac{47}{9}L_{jjij}^{V1,LR} + \frac{205}{486}L_{iiij}^{V8,LR} + \frac{205}{486}L_{jjij}^{V8,LR} + \frac{2441}{81}L_{ijji}^{V,RR} \\
& + \frac{2054}{81}L_{ijjj}^{V,RR} - \frac{47}{9}L_{11ij}^{V1,LR} - \frac{47}{9}L_{22ij}^{V1,LR} + \frac{35}{9}L_{11ij}^{V1,RR} + \frac{35}{9}L_{22ij}^{V1,RR} + \frac{205}{486}L_{11ij}^{V8,LR} \\
& + \frac{205}{486}L_{22ij}^{V8,LR} + \frac{835}{486}L_{11ij}^{V8,RR} + \frac{835}{486}L_{22ij}^{V8,RR} \Big] + \alpha_s \alpha \Big[ \frac{166}{243}L_{iiij}^{V1,LR} + \frac{166}{243}L_{jjij}^{V1,LR} \\
& -\frac{721}{729}L_{iiij}^{V8,LR} - \frac{721}{729}L_{jjij}^{V8,LR} + \frac{958}{243}L_{ijji}^{V,RR} - \frac{3038}{243}L_{ijjj}^{V,RR} - \frac{50}{243}L_{11ij}^{V,LR} \\
& -\frac{50}{243}L_{22ij}^{V,LR} - \frac{50}{243}L_{33ij}^{V,LR} - \frac{50}{243}L_{11ij}^{V,RR} - \frac{50}{243}L_{22ij}^{V,RR} - \frac{50}{243}L_{33ij}^{V,RR} - \frac{332}{243}L_{11ij}^{V1,LR} \\
& -\frac{332}{243}L_{22ij}^{V1,LR} - \frac{332}{243}L_{11ij}^{V1,RR} - \frac{332}{243}L_{22ij}^{V1,RR} + \frac{1331}{729}L_{11ij}^{V8,LR} + \frac{1331}{729}L_{22ij}^{V8,LR} \\
& -\frac{217}{729}L_{11ij}^{V8,RR} - \frac{217}{729}L_{22ij}^{V8,RR} \Big] + \alpha^2 \Big[ -\frac{356}{729}L_{iiij}^{V1,LR} - \frac{356}{729}L_{jjij}^{V1,LR} + \frac{632}{729}L_{ijji}^{V,RR} \\
& + \frac{974}{729}L_{ijjj}^{V,RR} - \frac{644}{729}L_{11ij}^{V,LR} - \frac{644}{729}L_{22ij}^{V,LR} - \frac{644}{729}L_{33ij}^{V,LR} + \frac{868}{729}L_{11ij}^{V,RR} + \frac{868}{729}L_{22ij}^{V,RR}
\end{aligned}$$

$$\begin{aligned}
& + \frac{868}{729} L_{33ij}^{V,RR} - \frac{1772}{729} L_{11ij}^{V1,LR} - \frac{1772}{729} L_{22ij}^{V1,LR} + \frac{244}{729} L_{11ij}^{V1,RR} + \frac{244}{729} L_{22ij}^{V1,RR} \Big] ; \\
\dot{L}_{dd\ ij\ ii}^{V,RR} = & g_s^2 \left[ \frac{1}{9} L_{iiij}^{V8,LR} + \frac{1}{9} L_{jjij}^{V8,LR} + \frac{40}{9} L_{ijii}^{V,RR} + \frac{4}{9} L_{ijjj}^{V,RR} + \frac{1}{9} L_{11ij}^{V8,LR} \right. \\
& + \frac{1}{9} L_{22ij}^{V8,LR} + \frac{1}{9} L_{11ij}^{V8,RR} + \frac{1}{9} L_{22ij}^{V8,RR} \Big] + e^2 \left[ \frac{2}{9} L_{iiij}^{V1,LR} + \frac{2}{9} L_{jjij}^{V1,LR} \right. \\
& + \frac{52}{27} L_{ijii}^{V,RR} + \frac{16}{27} L_{ijjj}^{V,RR} + \frac{2}{9} L_{11ij}^{V,LR} + \frac{2}{9} L_{22ij}^{V,LR} + \frac{2}{9} L_{33ij}^{V,LR} + \frac{2}{9} L_{11ij}^{V,RR} \\
& + \frac{2}{9} L_{22ij}^{V,RR} + \frac{2}{9} L_{33ij}^{V,RR} - \frac{4}{9} L_{11ij}^{V1,LR} - \frac{4}{9} L_{22ij}^{V1,LR} - \frac{4}{9} L_{11ij}^{V1,RR} - \frac{4}{9} L_{22ij}^{V1,RR} \Big] \\
& + \alpha_s^2 \left[ -\frac{47}{9} L_{iiij}^{V1,LR} - \frac{47}{9} L_{jjij}^{V1,LR} + \frac{205}{486} L_{iiij}^{V8,LR} + \frac{205}{486} L_{jjij}^{V8,LR} + \frac{2054}{81} L_{ijii}^{V,RR} \right. \\
& + \frac{2441}{81} L_{ijjj}^{V,RR} - \frac{47}{9} L_{11ij}^{V1,LR} - \frac{47}{9} L_{22ij}^{V1,LR} + \frac{35}{9} L_{11ij}^{V1,RR} + \frac{35}{9} L_{22ij}^{V1,RR} + \frac{205}{486} L_{11ij}^{V8,LR} \\
& + \frac{205}{486} L_{22ij}^{V8,LR} + \frac{835}{486} L_{11ij}^{V8,RR} + \frac{835}{486} L_{22ij}^{V8,RR} \Big] + \alpha_s \alpha \left[ \frac{166}{243} L_{iiij}^{V1,LR} + \frac{166}{243} L_{jjij}^{V1,LR} \right. \\
& - \frac{721}{729} L_{iiij}^{V8,LR} - \frac{721}{729} L_{jjij}^{V8,LR} - \frac{3038}{243} L_{ijii}^{V,RR} + \frac{958}{243} L_{ijjj}^{V,RR} - \frac{50}{243} L_{11ij}^{V,LR} \\
& - \frac{50}{243} L_{22ij}^{V,LR} - \frac{50}{243} L_{33ij}^{V,LR} - \frac{50}{243} L_{11ij}^{V,RR} - \frac{50}{243} L_{22ij}^{V,RR} - \frac{50}{243} L_{33ij}^{V,RR} - \frac{332}{243} L_{11ij}^{V1,LR} \\
& - \frac{332}{243} L_{22ij}^{V1,LR} - \frac{332}{243} L_{11ij}^{V1,RR} - \frac{332}{243} L_{22ij}^{V1,RR} + \frac{1331}{729} L_{11ij}^{V8,LR} + \frac{1331}{729} L_{22ij}^{V8,LR} \\
& - \frac{217}{729} L_{11ij}^{V8,RR} - \frac{217}{729} L_{22ij}^{V8,RR} \Big] + \alpha^2 \left[ -\frac{356}{729} L_{iiij}^{V1,LR} - \frac{356}{729} L_{jjij}^{V1,LR} + \frac{974}{729} L_{ijii}^{V,RR} \right. \\
& + \frac{632}{729} L_{ijjj}^{V,RR} - \frac{644}{729} L_{11ij}^{V,LR} - \frac{644}{729} L_{22ij}^{V,LR} - \frac{644}{729} L_{33ij}^{V,LR} + \frac{868}{729} L_{11ij}^{V,RR} + \frac{868}{729} L_{22ij}^{V,RR} \\
& + \frac{868}{729} L_{33ij}^{V,RR} - \frac{1772}{729} L_{11ij}^{V1,LR} - \frac{1772}{729} L_{22ij}^{V1,LR} + \frac{244}{729} L_{11ij}^{V1,RR} + \frac{244}{729} L_{22ij}^{V1,RR} \Big] ; \\
\dot{L}_{ed\ 11ij}^{V,LR} = & e^2 \left[ \frac{4}{3} L_{iiij}^{V1,LR} + \frac{4}{3} L_{jjij}^{V1,LR} + \frac{32}{9} L_{ijii}^{V,RR} + \frac{32}{9} L_{ijjj}^{V,RR} - \frac{8}{3} L_{11ij}^{V,LR} \right. \\
& + \frac{4}{3} L_{22ij}^{V,LR} + \frac{4}{3} L_{33ij}^{V,LR} + \frac{4}{3} L_{11ij}^{V,RR} + \frac{4}{3} L_{22ij}^{V,RR} + \frac{4}{3} L_{33ij}^{V,RR} - \frac{8}{3} L_{11ij}^{V1,LR} \\
& + \frac{8}{3} L_{22ij}^{V1,LR} + \frac{8}{3} L_{33ij}^{V1,LR} \Big] ;
\end{aligned}$$



$$\begin{aligned}
& -\frac{8}{3}L_{22ij}^{V1,LR} - \frac{8}{3}L_{11ij}^{V1,RR} - \frac{8}{3}L_{22ij}^{V1,RR} \Big] + \alpha_s \alpha \Big[ \frac{16}{3}L_{iiij}^{V1,LR} + \frac{16}{3}L_{jjij}^{V1,LR} \\
& - \frac{992}{243}L_{iiij}^{V8,LR} - \frac{992}{243}L_{jjij}^{V8,LR} + \frac{1120}{81}L_{ijii}^{V,RR} + \frac{1120}{81}L_{ijjj}^{V,RR} + 16L_{11ij}^{V,LR} - \frac{32}{3}L_{11ij}^{V1,LR} \\
& - \frac{32}{3}L_{22ij}^{V1,LR} - \frac{32}{3}L_{11ij}^{V1,RR} - \frac{32}{3}L_{22ij}^{V1,RR} + \frac{1384}{243}L_{11ij}^{V8,LR} + \frac{1384}{243}L_{22ij}^{V8,LR} - \frac{56}{243}L_{11ij}^{V8,RR} \\
& - \frac{56}{243}L_{22ij}^{V8,RR} \Big] + \alpha^2 \Big[ \frac{1736}{243}L_{iiij}^{V1,LR} + \frac{1736}{243}L_{jjij}^{V1,LR} - \frac{752}{243}L_{ijii}^{V,RR} - \frac{752}{243}L_{ijjj}^{V,RR} \\
& + \frac{20906}{243}L_{11ij}^{V,LR} + \frac{3752}{243}L_{22ij}^{V,LR} + \frac{3752}{243}L_{33ij}^{V,LR} - \frac{1000}{243}L_{11ij}^{V,RR} - \frac{1000}{243}L_{22ij}^{V,RR} \\
& - \frac{1000}{243}L_{33ij}^{V,RR} - \frac{664}{243}L_{11ij}^{V1,LR} - \frac{664}{243}L_{22ij}^{V1,LR} - \frac{7000}{243}L_{11ij}^{V1,RR} - \frac{7000}{243}L_{22ij}^{V1,RR} \Big] ; \\
\dot{L}_{22ij}^{V,LR} &= e^2 \Big[ \frac{4}{3}L_{iiij}^{V1,LR} + \frac{4}{3}L_{jjij}^{V1,LR} + \frac{32}{9}L_{ijii}^{V,RR} + \frac{32}{9}L_{ijjj}^{V,RR} + \frac{4}{3}L_{11ij}^{V,LR} \\
& - \frac{8}{3}L_{22ij}^{V,LR} + \frac{4}{3}L_{33ij}^{V,LR} + \frac{4}{3}L_{11ij}^{V,RR} + \frac{4}{3}L_{22ij}^{V,RR} + \frac{4}{3}L_{33ij}^{V,RR} - \frac{8}{3}L_{11ij}^{V1,LR} \\
& - \frac{8}{3}L_{22ij}^{V1,LR} - \frac{8}{3}L_{11ij}^{V1,RR} - \frac{8}{3}L_{22ij}^{V1,RR} \Big] + \alpha_s \alpha \Big[ \frac{16}{3}L_{iiij}^{V1,LR} + \frac{16}{3}L_{jjij}^{V1,LR} \\
& - \frac{992}{243}L_{iiij}^{V8,LR} - \frac{992}{243}L_{jjij}^{V8,LR} + \frac{1120}{81}L_{ijii}^{V,RR} + \frac{1120}{81}L_{ijjj}^{V,RR} + 16L_{22ij}^{V,LR} - \frac{32}{3}L_{11ij}^{V1,LR} \\
& - \frac{32}{3}L_{22ij}^{V1,LR} - \frac{32}{3}L_{11ij}^{V1,RR} - \frac{32}{3}L_{22ij}^{V1,RR} + \frac{1384}{243}L_{11ij}^{V8,LR} + \frac{1384}{243}L_{22ij}^{V8,LR} - \frac{56}{243}L_{11ij}^{V8,RR} \\
& - \frac{56}{243}L_{22ij}^{V8,RR} \Big] + \alpha^2 \Big[ \frac{1736}{243}L_{iiij}^{V1,LR} + \frac{1736}{243}L_{jjij}^{V1,LR} - \frac{752}{243}L_{ijii}^{V,RR} - \frac{752}{243}L_{ijjj}^{V,RR} \\
& + \frac{3752}{243}L_{11ij}^{V,LR} + \frac{20906}{243}L_{22ij}^{V,LR} + \frac{3752}{243}L_{33ij}^{V,LR} - \frac{1000}{243}L_{11ij}^{V,RR} - \frac{1000}{243}L_{22ij}^{V,RR} \\
& - \frac{1000}{243}L_{33ij}^{V,RR} - \frac{664}{243}L_{11ij}^{V1,LR} - \frac{664}{243}L_{22ij}^{V1,LR} - \frac{7000}{243}L_{11ij}^{V1,RR} - \frac{7000}{243}L_{22ij}^{V1,RR} \Big] ; \\
\dot{L}_{33ij}^{V,LR} &= e^2 \Big[ \frac{4}{3}L_{iiij}^{V1,LR} + \frac{4}{3}L_{jjij}^{V1,LR} + \frac{32}{9}L_{ijii}^{V,RR} + \frac{32}{9}L_{ijjj}^{V,RR} + \frac{4}{3}L_{11ij}^{V,LR} \\
& + \frac{4}{3}L_{22ij}^{V,LR} - \frac{8}{3}L_{33ij}^{V,LR} + \frac{4}{3}L_{11ij}^{V,RR} + \frac{4}{3}L_{22ij}^{V,RR} + \frac{4}{3}L_{33ij}^{V,RR} - \frac{8}{3}L_{11ij}^{V1,LR} \\
& + \frac{4}{3}L_{22ij}^{V1,LR} - \frac{8}{3}L_{33ij}^{V1,LR} + \frac{4}{3}L_{11ij}^{V1,RR} + \frac{4}{3}L_{22ij}^{V1,RR} + \frac{4}{3}L_{33ij}^{V1,RR} - \frac{8}{3}L_{11ij}^{V1,RR} \\
& - \frac{8}{3}L_{22ij}^{V1,RR} - \frac{8}{3}L_{33ij}^{V1,RR} \Big] + \alpha_s \alpha \Big[ \frac{16}{3}L_{iiij}^{V1,LR} + \frac{16}{3}L_{jjij}^{V1,LR} \\
& - \frac{992}{243}L_{iiij}^{V8,LR} - \frac{992}{243}L_{jjij}^{V8,LR} + \frac{1120}{81}L_{ijii}^{V,RR} + \frac{1120}{81}L_{ijjj}^{V,RR} + 16L_{33ij}^{V,LR} - \frac{32}{3}L_{11ij}^{V1,LR} \\
& - \frac{32}{3}L_{22ij}^{V1,LR} - \frac{32}{3}L_{33ij}^{V1,LR} - \frac{32}{3}L_{11ij}^{V1,RR} - \frac{32}{3}L_{22ij}^{V1,RR} - \frac{32}{3}L_{33ij}^{V1,RR} + \frac{1384}{243}L_{11ij}^{V8,LR} \\
& + \frac{1384}{243}L_{22ij}^{V8,LR} + \frac{1384}{243}L_{33ij}^{V8,LR} - \frac{56}{243}L_{11ij}^{V8,RR} - \frac{56}{243}L_{22ij}^{V8,RR} - \frac{56}{243}L_{33ij}^{V8,RR} \Big] + \alpha^2 \Big[ \frac{1736}{243}L_{iiij}^{V1,LR} \\
& + \frac{1736}{243}L_{jjij}^{V1,LR} - \frac{752}{243}L_{ijii}^{V,RR} - \frac{752}{243}L_{ijjj}^{V,RR} + \frac{3752}{243}L_{11ij}^{V,LR} + \frac{20906}{243}L_{22ij}^{V,LR} \\
& + \frac{3752}{243}L_{33ij}^{V,LR} - \frac{1000}{243}L_{11ij}^{V,RR} - \frac{1000}{243}L_{22ij}^{V,RR} - \frac{1000}{243}L_{33ij}^{V,RR} - \frac{664}{243}L_{11ij}^{V1,LR} \\
& - \frac{664}{243}L_{22ij}^{V1,LR} - \frac{664}{243}L_{33ij}^{V1,LR} - \frac{7000}{243}L_{11ij}^{V1,RR} - \frac{7000}{243}L_{22ij}^{V1,RR} - \frac{7000}{243}L_{33ij}^{V1,RR} \Big] ;
\end{aligned}$$

$$\begin{aligned}
& -\frac{8}{3}L_{22ij}^{V1,LR} - \frac{8}{3}L_{11ij}^{V1,RR} - \frac{8}{3}L_{22ij}^{V1,RR} \Big] + \alpha_s \alpha \Big[ \frac{16}{3}L_{\bar{ii}j}^{V1,LR} + \frac{16}{3}L_{jj\bar{i}}^{V1,LR} \\
& - \frac{992}{243}L_{\bar{ii}j}^{V8,LR} - \frac{992}{243}L_{jj\bar{i}}^{V8,LR} + \frac{1120}{81}L_{\bar{ii}j}^{V,RR} + \frac{1120}{81}L_{jj\bar{i}}^{V,RR} + 16L_{33ij}^{V,LR} - \frac{32}{3}L_{11ij}^{V1,LR} \\
& - \frac{32}{3}L_{22ij}^{V1,LR} - \frac{32}{3}L_{11ij}^{V1,RR} - \frac{32}{3}L_{22ij}^{V1,RR} + \frac{1384}{243}L_{11ij}^{V8,LR} + \frac{1384}{243}L_{22ij}^{V8,LR} - \frac{56}{243}L_{11ij}^{V8,RR} \\
& - \frac{56}{243}L_{22ij}^{V8,RR} \Big] + \alpha^2 \Big[ \frac{1736}{243}L_{\bar{ii}j}^{V1,LR} + \frac{1736}{243}L_{jj\bar{i}}^{V1,LR} - \frac{752}{243}L_{\bar{ii}j}^{V,RR} - \frac{752}{243}L_{jj\bar{i}}^{V,RR} \\
& + \frac{3752}{243}L_{11ij}^{V,LR} + \frac{3752}{243}L_{22ij}^{V,LR} + \frac{20906}{243}L_{33ij}^{V,LR} - \frac{1000}{243}L_{11ij}^{V,RR} - \frac{1000}{243}L_{22ij}^{V,RR} \\
& - \frac{1000}{243}L_{33ij}^{V,RR} - \frac{664}{243}L_{11ij}^{V1,LR} - \frac{664}{243}L_{22ij}^{V1,LR} - \frac{7000}{243}L_{11ij}^{V1,RR} - \frac{7000}{243}L_{22ij}^{V1,RR} \Big] ; \\
\dot{L}_{11ij}^{V1,LR} = & -\frac{8}{3}g_s^2 L_{11ij}^{V8,LR} + e^2 \Big[ -\frac{8}{9}L_{\bar{ii}j}^{V1,LR} - \frac{8}{9}L_{jj\bar{i}}^{V1,LR} - \frac{64}{27}L_{\bar{ii}j}^{V,RR} - \frac{64}{27}L_{jj\bar{i}}^{V,RR} \\
& - \frac{8}{9}L_{11ij}^{V,LR} - \frac{8}{9}L_{22ij}^{V,LR} - \frac{8}{9}L_{33ij}^{V,LR} - \frac{8}{9}L_{11ij}^{V,RR} - \frac{8}{9}L_{22ij}^{V,RR} - \frac{8}{9}L_{33ij}^{V,RR} \\
& + \frac{40}{9}L_{11ij}^{V1,LR} + \frac{16}{9}L_{22ij}^{V1,LR} + \frac{16}{9}L_{11ij}^{V1,RR} + \frac{16}{9}L_{22ij}^{V1,RR} \Big] + \alpha_s^2 \Big[ 8L_{\bar{ii}j}^{V1,LR} \\
& + 8L_{jj\bar{i}}^{V1,LR} + \frac{44}{27}L_{\bar{ii}j}^{V8,LR} + \frac{44}{27}L_{jj\bar{i}}^{V8,LR} - \frac{232}{9}L_{\bar{ii}j}^{V,RR} - \frac{232}{9}L_{jj\bar{i}}^{V,RR} - \frac{4}{3}L_{11ij}^{V1,LR} \\
& + 8L_{22ij}^{V1,LR} - 8L_{11ij}^{V1,RR} - 8L_{22ij}^{V1,RR} - \frac{2000}{27}L_{11ij}^{V8,LR} + \frac{44}{27}L_{22ij}^{V8,LR} + \frac{44}{27}L_{11ij}^{V8,RR} \\
& + \frac{44}{27}L_{22ij}^{V8,RR} \Big] + \alpha_s \alpha \Big[ -\frac{32}{9}L_{\bar{ii}j}^{V1,LR} - \frac{32}{9}L_{jj\bar{i}}^{V1,LR} + \frac{1984}{729}L_{\bar{ii}j}^{V8,LR} + \frac{1984}{729}L_{jj\bar{i}}^{V8,LR} \\
& - \frac{2240}{243}L_{\bar{ii}j}^{V,RR} - \frac{2240}{243}L_{jj\bar{i}}^{V,RR} - \frac{128}{9}L_{11ij}^{V1,LR} + \frac{64}{9}L_{22ij}^{V1,LR} + \frac{64}{9}L_{11ij}^{V1,RR} + \frac{64}{9}L_{22ij}^{V1,RR} \\
& + \frac{3496}{729}L_{11ij}^{V8,LR} - \frac{2768}{729}L_{22ij}^{V8,LR} + \frac{112}{729}L_{11ij}^{V8,RR} + \frac{112}{729}L_{22ij}^{V8,RR} \Big] + \alpha^2 \Big[ \frac{3728}{729}L_{\bar{ii}j}^{V1,LR} \\
& + \frac{3728}{729}L_{jj\bar{i}}^{V1,LR} + \frac{784}{729}L_{\bar{ii}j}^{V,RR} + \frac{784}{729}L_{jj\bar{i}}^{V,RR} + \frac{6176}{729}L_{11ij}^{V,LR} + \frac{6176}{729}L_{22ij}^{V,LR} \\
& + \frac{6176}{729}L_{33ij}^{V,LR} - \frac{3760}{729}L_{11ij}^{V,RR} - \frac{3760}{729}L_{22ij}^{V,RR} - \frac{3760}{729}L_{33ij}^{V,RR} - \frac{28480}{729}L_{11ij}^{V1,LR}
\end{aligned}$$

$$\begin{aligned}
& + \frac{6368}{729} L_{22ij}^{V1,LR} - \frac{6880}{729} L_{11ij}^{V1,RR} - \frac{6880}{729} L_{22ij}^{V1,RR} \Big] ; \\
\dot{L}_{11ij}^{V8,LR} = & g_s^2 \left[ \frac{2}{3} L_{iiij}^{V8,LR} + \frac{2}{3} L_{jjij}^{V8,LR} + \frac{8}{3} L_{ijii}^{V,RR} + \frac{8}{3} L_{ijjj}^{V,RR} - 12 L_{11ij}^{V1,LR} \right. \\
& - \frac{40}{3} L_{11ij}^{V8,LR} + \frac{2}{3} L_{22ij}^{V8,LR} + \frac{2}{3} L_{11ij}^{V8,RR} + \frac{2}{3} L_{22ij}^{V8,RR} \Big] + \frac{8}{3} e^2 L_{11ij}^{V8,LR} + \alpha_s^2 \left[ - \frac{22}{3} L_{iiij}^{V1,LR} \right. \\
& - \frac{22}{3} L_{jjij}^{V1,LR} + \frac{799}{81} L_{iiij}^{V8,LR} + \frac{799}{81} L_{jjij}^{V8,LR} + \frac{1210}{27} L_{ijii}^{V,RR} + \frac{1210}{27} L_{ijjj}^{V,RR} - 132 L_{11ij}^{V1,LR} \\
& - \frac{22}{3} L_{22ij}^{V1,LR} - \frac{2}{3} L_{11ij}^{V1,RR} - \frac{2}{3} L_{22ij}^{V1,RR} - \frac{25177}{162} L_{11ij}^{V8,LR} + \frac{799}{81} L_{22ij}^{V8,LR} + \frac{619}{81} L_{11ij}^{V8,RR} \\
& + \frac{619}{81} L_{22ij}^{V8,RR} \Big] + \alpha_s \alpha \left[ - \frac{928}{81} L_{iiij}^{V1,LR} - \frac{928}{81} L_{jjij}^{V1,LR} - \frac{44}{9} L_{iiij}^{V8,LR} - \frac{44}{9} L_{jjij}^{V8,LR} \right. \\
& - \frac{2192}{81} L_{ijii}^{V,RR} - \frac{2192}{81} L_{ijjj}^{V,RR} - \frac{928}{81} L_{11ij}^{V,LR} - \frac{928}{81} L_{22ij}^{V,LR} - \frac{928}{81} L_{33ij}^{V,LR} - \frac{928}{81} L_{11ij}^{V,RR} \\
& - \frac{928}{81} L_{22ij}^{V,RR} - \frac{928}{81} L_{33ij}^{V,RR} + \frac{4988}{81} L_{11ij}^{V1,LR} + \frac{1856}{81} L_{22ij}^{V1,LR} + \frac{1856}{81} L_{11ij}^{V1,RR} \\
& + \frac{1856}{81} L_{22ij}^{V1,RR} + 27 L_{11ij}^{V8,LR} + \frac{56}{9} L_{22ij}^{V8,LR} - \frac{160}{27} L_{11ij}^{V8,RR} - \frac{160}{27} L_{22ij}^{V8,RR} \Big] \\
& - \frac{3872}{81} \alpha^2 L_{11ij}^{V8,LR} ; \\
\dot{L}_{22ij}^{V1,LR} = & - \frac{8}{3} g_s^2 L_{22ij}^{V8,LR} + e^2 \left[ - \frac{8}{9} L_{iiij}^{V1,LR} - \frac{8}{9} L_{jjij}^{V1,LR} - \frac{64}{27} L_{ijii}^{V,RR} - \frac{64}{27} L_{ijjj}^{V,RR} \right. \\
& - \frac{8}{9} L_{11ij}^{V,LR} - \frac{8}{9} L_{22ij}^{V,LR} - \frac{8}{9} L_{33ij}^{V,LR} - \frac{8}{9} L_{11ij}^{V,RR} - \frac{8}{9} L_{22ij}^{V,RR} - \frac{8}{9} L_{33ij}^{V,RR} \\
& + \frac{16}{9} L_{11ij}^{V1,LR} + \frac{40}{9} L_{22ij}^{V1,LR} + \frac{16}{9} L_{11ij}^{V1,RR} + \frac{16}{9} L_{22ij}^{V1,RR} \Big] + \alpha_s^2 \left[ 8 L_{iiij}^{V1,LR} \right. \\
& + 8 L_{jjij}^{V1,LR} + \frac{44}{27} L_{iiij}^{V8,LR} + \frac{44}{27} L_{jjij}^{V8,LR} - \frac{232}{9} L_{ijii}^{V,RR} - \frac{232}{9} L_{ijjj}^{V,RR} + 8 L_{11ij}^{V1,LR} \\
& - \frac{4}{3} L_{22ij}^{V1,LR} - 8 L_{11ij}^{V1,RR} - 8 L_{22ij}^{V1,RR} + \frac{44}{27} L_{11ij}^{V8,LR} - \frac{2000}{27} L_{22ij}^{V8,LR} + \frac{44}{27} L_{11ij}^{V8,RR} \\
& + \frac{44}{27} L_{22ij}^{V8,RR} \Big] + \alpha_s \alpha \left[ - \frac{32}{9} L_{iiij}^{V1,LR} - \frac{32}{9} L_{jjij}^{V1,LR} + \frac{1984}{729} L_{iiij}^{V8,LR} + \frac{1984}{729} L_{jjij}^{V8,LR} \right.
\end{aligned}$$

$$\begin{aligned}
& -\frac{2240}{243}L_{dd\,ij\bar{i}}^{V,RR} - \frac{2240}{243}L_{dd\,ij\bar{j}}^{V,RR} + \frac{64}{9}L_{ud\,11\bar{i}j}^{V1,LR} - \frac{128}{9}L_{ud\,22\bar{i}j}^{V1,LR} + \frac{64}{9}L_{ud\,11\bar{i}j}^{V1,RR} + \frac{64}{9}L_{ud\,22\bar{i}j}^{V1,RR} \\
& - \frac{2768}{729}L_{ud\,11\bar{i}j}^{V8,LR} + \frac{3496}{729}L_{ud\,22\bar{i}j}^{V8,LR} + \frac{112}{729}L_{ud\,11\bar{i}j}^{V8,RR} + \frac{112}{729}L_{ud\,22\bar{i}j}^{V8,RR} \Big] + \alpha^2 \Big[ \frac{3728}{729}L_{dd\,iii\bar{j}}^{V1,LR} \\
& + \frac{3728}{729}L_{dd\,jj\bar{i}i}^{V1,LR} + \frac{784}{729}L_{dd\,ij\bar{j}i}^{V,RR} + \frac{784}{729}L_{dd\,ij\bar{j}j}^{V,RR} + \frac{6176}{729}L_{ed\,11\bar{i}j}^{V,LR} + \frac{6176}{729}L_{ed\,22\bar{i}j}^{V,LR} \\
& + \frac{6176}{729}L_{ed\,33\bar{i}j}^{V,LR} - \frac{3760}{729}L_{ed\,11\bar{i}j}^{V,RR} - \frac{3760}{729}L_{ed\,22\bar{i}j}^{V,RR} - \frac{3760}{729}L_{ed\,33\bar{i}j}^{V,RR} + \frac{6368}{729}L_{ud\,11\bar{i}j}^{V1,LR} \\
& - \frac{28480}{729}L_{ud\,22\bar{i}j}^{V1,LR} - \frac{6880}{729}L_{ud\,11\bar{i}j}^{V1,RR} - \frac{6880}{729}L_{ud\,22\bar{i}j}^{V1,RR} \Big] ;
\end{aligned}$$

$$\begin{aligned}
\dot{L}_{ud\,22\bar{i}j}^{V8,LR} &= g_s^2 \Big[ \frac{2}{3}L_{dd\,iii\bar{j}}^{V8,LR} + \frac{2}{3}L_{dd\,jj\bar{i}i}^{V8,LR} + \frac{8}{3}L_{dd\,ij\bar{i}i}^{V,RR} + \frac{8}{3}L_{dd\,ij\bar{j}j}^{V,RR} - 12L_{ud\,22\bar{i}j}^{V1,LR} \\
& + \frac{2}{3}L_{ud\,11\bar{i}j}^{V8,LR} - \frac{40}{3}L_{ud\,22\bar{i}j}^{V8,LR} + \frac{2}{3}L_{ud\,11\bar{i}j}^{V8,RR} + \frac{2}{3}L_{ud\,22\bar{i}j}^{V8,RR} \Big] + \frac{8}{3}e^2L_{ud\,22\bar{i}j}^{V8,LR} + \alpha_s^2 \Big[ -\frac{22}{3}L_{dd\,iii\bar{j}}^{V1,LR} \\
& - \frac{22}{3}L_{dd\,jj\bar{i}i}^{V1,LR} + \frac{799}{81}L_{dd\,iii\bar{j}}^{V8,LR} + \frac{799}{81}L_{dd\,jj\bar{i}i}^{V8,LR} + \frac{1210}{27}L_{dd\,ij\bar{i}i}^{V,RR} + \frac{1210}{27}L_{dd\,ij\bar{j}j}^{V,RR} - \frac{22}{3}L_{ud\,11\bar{i}j}^{V1,LR} \\
& - 132L_{ud\,22\bar{i}j}^{V1,LR} - \frac{2}{3}L_{ud\,11\bar{i}j}^{V1,RR} - \frac{2}{3}L_{ud\,22\bar{i}j}^{V1,RR} + \frac{799}{81}L_{ud\,11\bar{i}j}^{V8,LR} - \frac{25177}{162}L_{ud\,22\bar{i}j}^{V8,LR} + \frac{619}{81}L_{ud\,11\bar{i}j}^{V8,RR} \\
& + \frac{619}{81}L_{ud\,22\bar{i}j}^{V8,RR} \Big] + \alpha_s\alpha \Big[ -\frac{928}{81}L_{dd\,iii\bar{j}}^{V1,LR} - \frac{928}{81}L_{dd\,jj\bar{i}i}^{V1,LR} - \frac{44}{9}L_{dd\,iii\bar{j}}^{V8,LR} - \frac{44}{9}L_{dd\,jj\bar{i}i}^{V8,LR} \\
& - \frac{2192}{81}L_{dd\,ij\bar{i}i}^{V,RR} - \frac{2192}{81}L_{dd\,ij\bar{j}j}^{V,RR} - \frac{928}{81}L_{ed\,11\bar{i}j}^{V,LR} - \frac{928}{81}L_{ed\,22\bar{i}j}^{V,LR} - \frac{928}{81}L_{ed\,33\bar{i}j}^{V,LR} - \frac{928}{81}L_{ed\,11\bar{i}j}^{V,RR} \\
& - \frac{928}{81}L_{ed\,22\bar{i}j}^{V,RR} - \frac{928}{81}L_{ed\,33\bar{i}j}^{V,RR} + \frac{1856}{81}L_{ud\,11\bar{i}j}^{V1,LR} + \frac{4988}{81}L_{ud\,22\bar{i}j}^{V1,LR} + \frac{1856}{81}L_{ud\,11\bar{i}j}^{V1,RR} \\
& + \frac{1856}{81}L_{ud\,22\bar{i}j}^{V1,RR} + \frac{56}{9}L_{ud\,11\bar{i}j}^{V8,LR} + 27L_{ud\,22\bar{i}j}^{V8,LR} - \frac{160}{27}L_{ud\,11\bar{i}j}^{V8,RR} - \frac{160}{27}L_{ud\,22\bar{i}j}^{V8,RR} \Big] \\
& - \frac{3872}{81}\alpha^2L_{ud\,22\bar{i}j}^{V8,LR} ;
\end{aligned}$$

$$\begin{aligned}
\dot{L}_{dd\,jj\bar{i}i}^{V1,LR} &= -\frac{8}{3}g_s^2L_{dd\,jj\bar{i}i}^{V8,LR} + e^2 \Big[ \frac{4}{9}L_{dd\,iii\bar{j}}^{V1,LR} - \frac{8}{9}L_{dd\,jj\bar{i}i}^{V1,LR} + \frac{32}{27}L_{dd\,ij\bar{i}i}^{V,RR} + \frac{32}{27}L_{dd\,ij\bar{j}j}^{V,RR} \\
& + \frac{4}{9}L_{ed\,11\bar{i}j}^{V,LR} + \frac{4}{9}L_{ed\,22\bar{i}j}^{V,LR} + \frac{4}{9}L_{ed\,33\bar{i}j}^{V,LR} + \frac{4}{9}L_{ed\,11\bar{i}j}^{V,RR} + \frac{4}{9}L_{ed\,22\bar{i}j}^{V,RR} + \frac{4}{9}L_{ed\,33\bar{i}j}^{V,RR} \Big]
\end{aligned}$$

$$\begin{aligned}
& -\frac{8}{9}L_{11ij}^{V1,LR} - \frac{8}{9}L_{22ij}^{V1,LR} - \frac{8}{9}L_{11ij}^{V1,RR} - \frac{8}{9}L_{22ij}^{V1,RR} \Big] + \alpha_s^2 \Big[ 8L_{iii}^{V1,LR} \\
& - \frac{4}{3}L_{jjj}^{V1,LR} + \frac{44}{27}L_{iii}^{V8,LR} - \frac{2000}{27}L_{jjj}^{V8,LR} - \frac{232}{9}L_{ijii}^{V,RR} - \frac{232}{9}L_{ijjj}^{V,RR} + 8L_{11ij}^{V1,LR} \\
& + 8L_{22ij}^{V1,LR} - 8L_{11ij}^{V1,RR} - 8L_{22ij}^{V1,RR} + \frac{44}{27}L_{11ij}^{V8,LR} + \frac{44}{27}L_{22ij}^{V8,LR} + \frac{44}{27}L_{11ij}^{V8,RR} \\
& + \frac{44}{27}L_{22ij}^{V8,RR} \Big] + \alpha_s \alpha \Big[ \frac{16}{9}L_{iii}^{V1,LR} + \frac{112}{9}L_{jjj}^{V1,LR} - \frac{992}{729}L_{iii}^{V8,LR} - \frac{1208}{729}L_{jjj}^{V8,LR} \\
& + \frac{1120}{243}L_{ijii}^{V,RR} + \frac{1120}{243}L_{ijjj}^{V,RR} - \frac{32}{9}L_{11ij}^{V1,LR} - \frac{32}{9}L_{22ij}^{V1,LR} - \frac{32}{9}L_{11ij}^{V1,RR} - \frac{32}{9}L_{22ij}^{V1,RR} \\
& + \frac{1384}{729}L_{11ij}^{V8,LR} + \frac{1384}{729}L_{22ij}^{V8,LR} - \frac{56}{729}L_{11ij}^{V8,RR} - \frac{56}{729}L_{22ij}^{V8,RR} \Big] + \alpha^2 \Big[ \frac{296}{729}L_{iii}^{V1,LR} \\
& + \frac{15614}{729}L_{jjj}^{V1,LR} - \frac{608}{729}L_{ijii}^{V,RR} - \frac{608}{729}L_{ijjj}^{V,RR} + \frac{1016}{729}L_{11ij}^{V,LR} + \frac{1016}{729}L_{22ij}^{V,LR} \\
& + \frac{1016}{729}L_{33ij}^{V,LR} + \frac{152}{729}L_{11ij}^{V,RR} + \frac{152}{729}L_{22ij}^{V,RR} + \frac{152}{729}L_{33ij}^{V,RR} - \frac{1672}{729}L_{11ij}^{V1,LR} \\
& - \frac{1672}{729}L_{22ij}^{V1,LR} - \frac{2824}{729}L_{11ij}^{V1,RR} - \frac{2824}{729}L_{22ij}^{V1,RR} \Big] ;
\end{aligned}$$

$$\begin{aligned}
\dot{L}_{jjj}^{V8,LR} &= g_s^2 \Big[ -12L_{jjj}^{V1,LR} + \frac{2}{3}L_{iii}^{V8,LR} - \frac{40}{3}L_{jjj}^{V8,LR} + \frac{8}{3}L_{ijii}^{V,RR} + \frac{8}{3}L_{ijjj}^{V,RR} \\
& + \frac{2}{3}L_{11ij}^{V8,LR} + \frac{2}{3}L_{22ij}^{V8,LR} + \frac{2}{3}L_{11ij}^{V8,RR} + \frac{2}{3}L_{22ij}^{V8,RR} \Big] - \frac{4}{3}e^2L_{jjj}^{V8,LR} + \alpha_s^2 \Big[ -\frac{22}{3}L_{iii}^{V1,LR} \\
& - 132L_{jjj}^{V1,LR} + \frac{799}{81}L_{iii}^{V8,LR} - \frac{25177}{162}L_{jjj}^{V8,LR} + \frac{1210}{27}L_{ijii}^{V,RR} + \frac{1210}{27}L_{ijjj}^{V,RR} \\
& - \frac{22}{3}L_{11ij}^{V1,LR} - \frac{22}{3}L_{22ij}^{V1,LR} - \frac{2}{3}L_{11ij}^{V1,RR} - \frac{2}{3}L_{22ij}^{V1,RR} + \frac{799}{81}L_{11ij}^{V8,LR} + \frac{799}{81}L_{22ij}^{V8,LR} \\
& + \frac{619}{81}L_{11ij}^{V8,RR} + \frac{619}{81}L_{22ij}^{V8,RR} \Big] + \alpha_s \alpha \Big[ \frac{260}{81}L_{iii}^{V1,LR} + \frac{152}{81}L_{jjj}^{V1,LR} + \frac{14}{9}L_{iii}^{V8,LR} \\
& - \frac{4}{3}L_{jjj}^{V8,LR} + \frac{292}{81}L_{ijii}^{V,RR} + \frac{292}{81}L_{ijjj}^{V,RR} + \frac{260}{81}L_{11ij}^{V,LR} + \frac{260}{81}L_{22ij}^{V,LR} + \frac{260}{81}L_{33ij}^{V,LR} \\
& + \frac{260}{81}L_{11ij}^{V,RR} + \frac{260}{81}L_{22ij}^{V,RR} + \frac{260}{81}L_{33ij}^{V,RR} - \frac{520}{81}L_{11ij}^{V1,LR} - \frac{520}{81}L_{22ij}^{V1,LR} - \frac{520}{81}L_{11ij}^{V1,RR}
\end{aligned}$$

$$\begin{aligned}
& -\frac{520}{81}L_{22ij}^{V1,RR} + \frac{2}{3}L_{11ij}^{V8,LR} + \frac{2}{3}L_{22ij}^{V8,LR} + \frac{122}{27}L_{11ij}^{V8,RR} + \frac{122}{27}L_{22ij}^{V8,RR} \Big] \\
& + \frac{1702}{81}\alpha^2 L_{jjij}^{V8,LR} ; \\
\dot{L}_{dd\, iij}^{V1,LR} = & -\frac{8}{3}g_s^2 L_{iij}^{V8,LR} + e^2 \Big[ -\frac{8}{9}L_{iij}^{V1,LR} + \frac{4}{9}L_{jjij}^{V1,LR} + \frac{32}{27}L_{ijii}^{V,RR} + \frac{32}{27}L_{ijjj}^{V,RR} \\
& + \frac{4}{9}L_{11ij}^{V,LR} + \frac{4}{9}L_{22ij}^{V,LR} + \frac{4}{9}L_{33ij}^{V,LR} + \frac{4}{9}L_{11ij}^{V,RR} + \frac{4}{9}L_{22ij}^{V,RR} + \frac{4}{9}L_{33ij}^{V,RR} \\
& - \frac{8}{9}L_{11ij}^{V1,LR} - \frac{8}{9}L_{22ij}^{V1,LR} - \frac{8}{9}L_{11ij}^{V1,RR} - \frac{8}{9}L_{22ij}^{V1,RR} \Big] + \alpha_s^2 \Big[ -\frac{4}{3}L_{iij}^{V1,LR} \\
& + 8L_{jjij}^{V1,LR} - \frac{2000}{27}L_{iij}^{V8,LR} + \frac{44}{27}L_{jjij}^{V8,LR} - \frac{232}{9}L_{ijii}^{V,RR} - \frac{232}{9}L_{ijjj}^{V,RR} + 8L_{11ij}^{V1,LR} \\
& + 8L_{22ij}^{V1,LR} - 8L_{11ij}^{V1,RR} - 8L_{22ij}^{V1,RR} + \frac{44}{27}L_{11ij}^{V8,LR} + \frac{44}{27}L_{22ij}^{V8,LR} + \frac{44}{27}L_{11ij}^{V8,RR} \\
& + \frac{44}{27}L_{22ij}^{V8,RR} \Big] + \alpha_s \alpha \Big[ \frac{112}{9}L_{iij}^{V1,LR} + \frac{16}{9}L_{jjij}^{V1,LR} - \frac{1208}{729}L_{iij}^{V8,LR} - \frac{992}{729}L_{jjij}^{V8,LR} \\
& + \frac{1120}{243}L_{ijii}^{V,RR} + \frac{1120}{243}L_{ijjj}^{V,RR} - \frac{32}{9}L_{11ij}^{V1,LR} - \frac{32}{9}L_{22ij}^{V1,LR} - \frac{32}{9}L_{11ij}^{V1,RR} - \frac{32}{9}L_{22ij}^{V1,RR} \\
& + \frac{1384}{729}L_{11ij}^{V8,LR} + \frac{1384}{729}L_{22ij}^{V8,LR} - \frac{56}{729}L_{11ij}^{V8,RR} - \frac{56}{729}L_{22ij}^{V8,RR} \Big] + \alpha^2 \Big[ \frac{15614}{729}L_{iij}^{V1,LR} \\
& + \frac{296}{729}L_{jjij}^{V1,LR} - \frac{608}{729}L_{ijii}^{V,RR} - \frac{608}{729}L_{ijjj}^{V,RR} + \frac{1016}{729}L_{11ij}^{V,LR} + \frac{1016}{729}L_{22ij}^{V,LR} \\
& + \frac{1016}{729}L_{33ij}^{V,LR} + \frac{152}{729}L_{11ij}^{V,RR} + \frac{152}{729}L_{22ij}^{V,RR} + \frac{152}{729}L_{33ij}^{V,RR} - \frac{1672}{729}L_{11ij}^{V1,LR} \\
& - \frac{1672}{729}L_{22ij}^{V1,LR} - \frac{2824}{729}L_{11ij}^{V1,RR} - \frac{2824}{729}L_{22ij}^{V1,RR} \Big] ; \\
\dot{L}_{dd\, iij}^{V8,LR} = & g_s^2 \Big[ -12L_{iij}^{V1,LR} - \frac{40}{3}L_{iij}^{V8,LR} + \frac{2}{3}L_{jjij}^{V8,LR} + \frac{8}{3}L_{ijii}^{V,RR} + \frac{8}{3}L_{ijjj}^{V,RR} \\
& + \frac{2}{3}L_{11ij}^{V8,LR} + \frac{2}{3}L_{22ij}^{V8,LR} + \frac{2}{3}L_{11ij}^{V8,RR} + \frac{2}{3}L_{22ij}^{V8,RR} \Big] - \frac{4}{3}e^2 L_{iij}^{V8,LR} + \alpha_s^2 \Big[ -132L_{iij}^{V1,LR} \\
& - \frac{22}{3}L_{jjij}^{V1,LR} - \frac{25177}{162}L_{iij}^{V8,LR} + \frac{799}{81}L_{jjij}^{V8,LR} + \frac{1210}{27}L_{ijii}^{V,RR} + \frac{1210}{27}L_{ijjj}^{V,RR}
\end{aligned}$$

$$\begin{aligned}
& -\frac{22}{3}L_{11ij}^{V1,LR} - \frac{22}{3}L_{22ij}^{V1,LR} - \frac{2}{3}L_{11ij}^{V1,RR} - \frac{2}{3}L_{22ij}^{V1,RR} + \frac{799}{81}L_{11ij}^{V8,LR} + \frac{799}{81}L_{22ij}^{V8,LR} \\
& + \frac{619}{81}L_{11ij}^{V8,RR} + \frac{619}{81}L_{22ij}^{V8,RR} \Big] + \alpha_s \alpha \Big[ \frac{152}{81}L_{iiij}^{V1,LR} + \frac{260}{81}L_{jjij}^{V1,LR} - \frac{4}{3}L_{iiij}^{V8,LR} \\
& + \frac{14}{9}L_{jjij}^{V8,LR} + \frac{292}{81}L_{ijii}^{V,RR} + \frac{292}{81}L_{ijjj}^{V,RR} + \frac{260}{81}L_{11ij}^{V,LR} + \frac{260}{81}L_{22ij}^{V,LR} + \frac{260}{81}L_{33ij}^{V,LR} \\
& + \frac{260}{81}L_{11ij}^{V,RR} + \frac{260}{81}L_{22ij}^{V,RR} + \frac{260}{81}L_{33ij}^{V,RR} - \frac{520}{81}L_{11ij}^{V1,LR} - \frac{520}{81}L_{22ij}^{V1,LR} - \frac{520}{81}L_{11ij}^{V1,RR} \\
& - \frac{520}{81}L_{22ij}^{V1,RR} + \frac{2}{3}L_{11ij}^{V8,LR} + \frac{2}{3}L_{22ij}^{V8,LR} + \frac{122}{27}L_{11ij}^{V8,RR} + \frac{122}{27}L_{22ij}^{V8,RR} \Big] \\
& + \frac{1702}{81}\alpha^2 L_{iiij}^{V8,LR} ;
\end{aligned}$$

$$\dot{L}_{11ij}^{V,LL} = 0 ;$$

$$\dot{L}_{22ij}^{V,LL} = 0 ;$$

$$\dot{L}_{33ij}^{V,LL} = 0 ;$$

$$\dot{L}_{11ij}^{V,LR} = 0 ;$$

$$\dot{L}_{22ij}^{V,LR} = 0 ;$$

$$\dot{L}_{33ij}^{V,LR} = 0 ;$$

$$\begin{aligned}
\dot{L}_{11ij}^{S,LR} &= -8g_s^2 L_{11ij}^{S,LR} - \frac{2}{3}e^2 L_{11ij}^{S,LR} - \frac{1012}{9}\alpha_s^2 L_{11ij}^{S,LR} - \frac{8}{9}\alpha_s \alpha L_{11ij}^{S,LR} \\
& + \frac{377}{81}\alpha^2 L_{11ij}^{S,LR} ;
\end{aligned}$$

$$\begin{aligned}
\dot{L}_{22ij}^{S,LR} &= -8g_s^2 L_{22ij}^{S,LR} - \frac{2}{3}e^2 L_{22ij}^{S,LR} - \frac{1012}{9}\alpha_s^2 L_{22ij}^{S,LR} - \frac{8}{9}\alpha_s \alpha L_{22ij}^{S,LR} \\
& + \frac{377}{81}\alpha^2 L_{22ij}^{S,LR} ;
\end{aligned}$$

$$\begin{aligned}
\dot{L}_{33ij}^{S,LR} &= -8g_s^2 L_{33ij}^{S,LR} - \frac{2}{3}e^2 L_{33ij}^{S,LR} - \frac{1012}{9}\alpha_s^2 L_{33ij}^{S,LR} - \frac{8}{9}\alpha_s \alpha L_{33ij}^{S,LR} \\
& + \frac{377}{81}\alpha^2 L_{33ij}^{S,LR} ;
\end{aligned}$$

$$\begin{aligned}
\dot{L}_{11ij}^{S,LL} &= -8g_s^2 L_{11ij}^{S,LL} - \frac{2}{3}e^2 L_{11ij}^{S,LL} - \frac{1012}{9}\alpha_s^2 L_{11ij}^{S,LL} - \frac{8}{9}\alpha_s\alpha L_{11ij}^{S,LL} \\
&\quad + \frac{377}{81}\alpha^2 L_{11ij}^{S,LL} ; \\
\dot{L}_{11ij}^{T,LL} &= \frac{8}{3}g_s^2 L_{11ij}^{T,LL} + \frac{2}{9}e^2 L_{11ij}^{T,LL} + \frac{1652}{27}\alpha_s^2 L_{11ij}^{T,LL} - \frac{152}{27}\alpha_s\alpha L_{11ij}^{T,LL} \\
&\quad - \frac{1045}{243}\alpha^2 L_{11ij}^{T,LL} ; \\
\dot{L}_{22ij}^{S,LL} &= -8g_s^2 L_{22ij}^{S,LL} - \frac{2}{3}e^2 L_{22ij}^{S,LL} - \frac{1012}{9}\alpha_s^2 L_{22ij}^{S,LL} - \frac{8}{9}\alpha_s\alpha L_{22ij}^{S,LL} \\
&\quad + \frac{377}{81}\alpha^2 L_{22ij}^{S,LL} ; \\
\dot{L}_{22ij}^{T,LL} &= \frac{8}{3}g_s^2 L_{22ij}^{T,LL} + \frac{2}{9}e^2 L_{22ij}^{T,LL} + \frac{1652}{27}\alpha_s^2 L_{22ij}^{T,LL} - \frac{152}{27}\alpha_s\alpha L_{22ij}^{T,LL} \\
&\quad - \frac{1045}{243}\alpha^2 L_{22ij}^{T,LL} ; \\
\dot{L}_{33ij}^{S,LL} &= -8g_s^2 L_{33ij}^{S,LL} - \frac{2}{3}e^2 L_{33ij}^{S,LL} - \frac{1012}{9}\alpha_s^2 L_{33ij}^{S,LL} - \frac{8}{9}\alpha_s\alpha L_{33ij}^{S,LL} \\
&\quad + \frac{377}{81}\alpha^2 L_{33ij}^{S,LL} ; \\
\dot{L}_{33ij}^{T,LL} &= \frac{8}{3}g_s^2 L_{33ij}^{T,LL} + \frac{2}{9}e^2 L_{33ij}^{T,LL} + \frac{1652}{27}\alpha_s^2 L_{33ij}^{T,LL} - \frac{152}{27}\alpha_s\alpha L_{33ij}^{T,LL} \\
&\quad - \frac{1045}{243}\alpha^2 L_{33ij}^{T,LL} ;
\end{aligned}$$

## 2.6 $\Delta F = 1^{\bar{f}f}$ : $u$ -type ( $\bar{u}_i u_j \bar{f}_k f_k$ )

$$\begin{aligned}
\dot{L}_{11ij}^{V,LL} &= e^2 \left[ -\frac{20}{3}L_{11ij}^{V,LL} + \frac{4}{3}L_{22ij}^{V,LL} + \frac{4}{3}L_{33ij}^{V,LL} + \frac{4}{3}L_{ij11}^{V1,LL} + \frac{4}{3}L_{ij22}^{V1,LL} \right. \\
&\quad + \frac{4}{3}L_{ij11}^{V1,LR} + \frac{4}{3}L_{ij22}^{V1,LR} + \frac{4}{3}L_{ij11}^{V,LR} + \frac{4}{3}L_{ij22}^{V,LR} + \frac{4}{3}L_{ij33}^{V,LR} - \frac{8}{3}L_{ijii}^{V1,LR} \\
&\quad \left. - \frac{8}{3}L_{ijjj}^{V1,LR} - \frac{64}{9}L_{ijii}^{V,LL} - \frac{64}{9}L_{ijjj}^{V,LL} \right] + \alpha_s\alpha \left[ 32L_{11ij}^{V,LL} + \frac{16}{3}L_{ij11}^{V1,LL} \right. \\
&\quad \left. + \frac{16}{3}L_{ij22}^{V1,LL} + \frac{16}{3}L_{ij11}^{V1,LR} + \frac{16}{3}L_{ij22}^{V1,LR} + \frac{328}{243}L_{ij11}^{V8,LL} + \frac{328}{243}L_{ij22}^{V8,LL} - \frac{392}{243}L_{ij11}^{V8,LR} \right]
\end{aligned}$$



$$\begin{aligned}
& -\frac{392}{243}L_{ij22}^{V8,LR} - \frac{32}{3}L_{ijii}^{V1,LR} - \frac{32}{3}L_{ijjj}^{V1,LR} + \frac{1984}{243}L_{ijii}^{V8,LR} + \frac{1984}{243}L_{ijjj}^{V8,LR} \\
& - \frac{2240}{81}L_{ijii}^{V,LL} - \frac{2240}{81}L_{ijjj}^{V,LL} \Big] + \alpha^2 \Big[ \frac{4496}{243}L_{11ij}^{V,LL} + \frac{3344}{243}L_{22ij}^{V,LL} + \frac{3344}{243}L_{33ij}^{V,LL} \\
& + \frac{392}{243}L_{ij11}^{V1,LL} + \frac{392}{243}L_{ij22}^{V1,LL} - \frac{832}{243}L_{ij11}^{V1,LR} - \frac{832}{243}L_{ij22}^{V1,LR} - \frac{328}{243}L_{ij11}^{V,LR} \\
& - \frac{328}{243}L_{ij22}^{V,LR} - \frac{328}{243}L_{ij33}^{V,LR} - \frac{64}{243}L_{ijii}^{V1,LR} - \frac{64}{243}L_{ijjj}^{V1,LR} + \frac{25888}{243}L_{ijii}^{V,LL} \\
& + \frac{25888}{243}L_{ijjj}^{V,LL} \Big] ;
\end{aligned}$$

$$\begin{aligned}
\dot{L}_{22ij}^{V,LL} &= e^2 \Big[ \frac{4}{3}L_{11ij}^{V,LL} - \frac{20}{3}L_{22ij}^{V,LL} + \frac{4}{3}L_{33ij}^{V,LL} + \frac{4}{3}L_{ij11}^{V1,LL} + \frac{4}{3}L_{ij22}^{V1,LL} \\
& + \frac{4}{3}L_{ij11}^{V1,LR} + \frac{4}{3}L_{ij22}^{V1,LR} + \frac{4}{3}L_{ij11}^{V,LR} + \frac{4}{3}L_{ij22}^{V,LR} + \frac{4}{3}L_{ij33}^{V,LR} - \frac{8}{3}L_{ijii}^{V1,LR} \\
& - \frac{8}{3}L_{ijjj}^{V1,LR} - \frac{64}{9}L_{ijii}^{V,LL} - \frac{64}{9}L_{ijjj}^{V,LL} \Big] + \alpha_s \alpha \Big[ 32L_{22ij}^{V,LL} + \frac{16}{3}L_{ij11}^{V1,LL} \\
& + \frac{16}{3}L_{ij22}^{V1,LL} + \frac{16}{3}L_{ij11}^{V1,LR} + \frac{16}{3}L_{ij22}^{V1,LR} + \frac{328}{243}L_{ij11}^{V8,LL} + \frac{328}{243}L_{ij22}^{V8,LL} - \frac{392}{243}L_{ij11}^{V8,LR} \\
& - \frac{392}{243}L_{ij22}^{V8,LR} - \frac{32}{3}L_{ijii}^{V1,LR} - \frac{32}{3}L_{ijjj}^{V1,LR} + \frac{1984}{243}L_{ijii}^{V8,LR} + \frac{1984}{243}L_{ijjj}^{V8,LR} \\
& - \frac{2240}{81}L_{ijii}^{V,LL} - \frac{2240}{81}L_{ijjj}^{V,LL} \Big] + \alpha^2 \Big[ \frac{3344}{243}L_{11ij}^{V,LL} + \frac{4496}{243}L_{22ij}^{V,LL} + \frac{3344}{243}L_{33ij}^{V,LL} \\
& + \frac{392}{243}L_{ij11}^{V1,LL} + \frac{392}{243}L_{ij22}^{V1,LL} - \frac{832}{243}L_{ij11}^{V1,LR} - \frac{832}{243}L_{ij22}^{V1,LR} - \frac{328}{243}L_{ij11}^{V,LR} \\
& - \frac{328}{243}L_{ij22}^{V,LR} - \frac{328}{243}L_{ij33}^{V,LR} - \frac{64}{243}L_{ijii}^{V1,LR} - \frac{64}{243}L_{ijjj}^{V1,LR} + \frac{25888}{243}L_{ijii}^{V,LL} \\
& + \frac{25888}{243}L_{ijjj}^{V,LL} \Big] ;
\end{aligned}$$

$$\begin{aligned}
\dot{L}_{33ij}^{V,LL} &= e^2 \Big[ \frac{4}{3}L_{11ij}^{V,LL} + \frac{4}{3}L_{22ij}^{V,LL} - \frac{20}{3}L_{33ij}^{V,LL} + \frac{4}{3}L_{ij11}^{V1,LL} + \frac{4}{3}L_{ij22}^{V1,LL} \\
& + \frac{4}{3}L_{ij11}^{V1,LR} + \frac{4}{3}L_{ij22}^{V1,LR} + \frac{4}{3}L_{ij11}^{V,LR} + \frac{4}{3}L_{ij22}^{V,LR} + \frac{4}{3}L_{ij33}^{V,LR} - \frac{8}{3}L_{ijii}^{V1,LR} \\
& - \frac{8}{3}L_{ijjj}^{V1,LR} - \frac{64}{9}L_{ijii}^{V,LL} - \frac{64}{9}L_{ijjj}^{V,LL} \Big] + \alpha_s \alpha \Big[ 32L_{33ij}^{V,LL} + \frac{16}{3}L_{ij11}^{V1,LL} \\
& + \frac{16}{3}L_{ij22}^{V1,LL} + \frac{16}{3}L_{ij11}^{V1,LR} + \frac{16}{3}L_{ij22}^{V1,LR} + \frac{328}{243}L_{ij11}^{V8,LL} + \frac{328}{243}L_{ij22}^{V8,LL} - \frac{392}{243}L_{ij11}^{V8,LR} \\
& - \frac{392}{243}L_{ij22}^{V8,LR} - \frac{32}{3}L_{ijii}^{V1,LR} - \frac{32}{3}L_{ijjj}^{V1,LR} + \frac{1984}{243}L_{ijii}^{V8,LR} + \frac{1984}{243}L_{ijjj}^{V8,LR} \\
& - \frac{2240}{81}L_{ijii}^{V,LL} - \frac{2240}{81}L_{ijjj}^{V,LL} \Big] + \alpha^2 \Big[ \frac{3344}{243}L_{11ij}^{V,LL} + \frac{4496}{243}L_{22ij}^{V,LL} + \frac{3344}{243}L_{33ij}^{V,LL} \\
& + \frac{392}{243}L_{ij11}^{V1,LL} + \frac{392}{243}L_{ij22}^{V1,LL} - \frac{832}{243}L_{ij11}^{V1,LR} - \frac{832}{243}L_{ij22}^{V1,LR} - \frac{328}{243}L_{ij11}^{V,LR} \\
& - \frac{328}{243}L_{ij22}^{V,LR} - \frac{328}{243}L_{ij33}^{V,LR} - \frac{64}{243}L_{ijii}^{V1,LR} - \frac{64}{243}L_{ijjj}^{V1,LR} + \frac{25888}{243}L_{ijii}^{V,LL} \\
& + \frac{25888}{243}L_{ijjj}^{V,LL} \Big] ;
\end{aligned}$$

$$\begin{aligned}
& -\frac{8}{3}L_{ijjj}^{V1,LR} - \frac{64}{9}L_{ijii}^{V,LL} - \frac{64}{9}L_{ijjj}^{V,LL} \Big] + \alpha_s \alpha \Big[ 32L_{33ij}^{V,LL} + \frac{16}{3}L_{ij11}^{V1,LL} \\
& + \frac{16}{3}L_{ud22}^{V1,LL} + \frac{16}{3}L_{ij11}^{V1,LR} + \frac{16}{3}L_{ud22}^{V1,LR} + \frac{328}{243}L_{ij11}^{V8,LL} + \frac{328}{243}L_{ud22}^{V8,LL} - \frac{392}{243}L_{ij11}^{V8,LR} \\
& - \frac{392}{243}L_{ud22}^{V8,LR} - \frac{32}{3}L_{ijii}^{V1,LR} - \frac{32}{3}L_{ijjj}^{V1,LR} + \frac{1984}{243}L_{ijii}^{V8,LR} + \frac{1984}{243}L_{ijjj}^{V8,LR} \\
& - \frac{2240}{81}L_{ijii}^{V,LL} - \frac{2240}{81}L_{ijjj}^{V,LL} \Big] + \alpha^2 \Big[ \frac{3344}{243}L_{11ij}^{V,LL} + \frac{3344}{243}L_{22ij}^{V,LL} + \frac{4496}{243}L_{33ij}^{V,LL} \\
& + \frac{392}{243}L_{ud11}^{V1,LL} + \frac{392}{243}L_{ud22}^{V1,LL} - \frac{832}{243}L_{ud11}^{V1,LR} - \frac{832}{243}L_{ud22}^{V1,LR} - \frac{328}{243}L_{ij11}^{V,LR} \\
& - \frac{328}{243}L_{ij22}^{V,LR} - \frac{328}{243}L_{ij33}^{V,LR} - \frac{64}{243}L_{ijii}^{V1,LR} - \frac{64}{243}L_{ijjj}^{V1,LR} + \frac{25888}{243}L_{ijii}^{V,LL} \\
& + \frac{25888}{243}L_{ijjj}^{V,LL} \Big] ;
\end{aligned}$$

$$\begin{aligned}
\dot{L}_{ij11}^{V1,LL} &= \frac{8}{3}g_s^2 L_{ij11}^{V8,LL} + e^2 \Big[ \frac{4}{9}L_{11ij}^{V,LL} + \frac{4}{9}L_{22ij}^{V,LL} + \frac{4}{9}L_{33ij}^{V,LL} - \frac{20}{9}L_{ij11}^{V1,LL} \\
& + \frac{4}{9}L_{ud22}^{V1,LL} + \frac{4}{9}L_{ij11}^{V1,LR} + \frac{4}{9}L_{ud22}^{V1,LR} + \frac{4}{9}L_{ij11}^{V,LR} + \frac{4}{9}L_{ij22}^{V,LR} + \frac{4}{9}L_{ij33}^{V,LR} \\
& - \frac{8}{9}L_{ijii}^{V1,LR} - \frac{8}{9}L_{ijjj}^{V1,LR} - \frac{64}{27}L_{ijii}^{V,LL} - \frac{64}{27}L_{ijjj}^{V,LL} \Big] + \alpha_s^2 \Big[ -\frac{4}{3}L_{ij11}^{V1,LL} \\
& + 8L_{ij22}^{V1,LL} - 8L_{ij11}^{V1,LR} - 8L_{ij22}^{V1,LR} + \frac{86}{27}L_{ij11}^{V8,LL} + \frac{4}{27}L_{ij22}^{V8,LL} + \frac{4}{27}L_{ij11}^{V8,LR} \\
& + \frac{4}{27}L_{ij22}^{V8,LR} - 8L_{ijii}^{V1,LR} - 8L_{ijjj}^{V1,LR} + \frac{4}{27}L_{ijii}^{V8,LR} + \frac{4}{27}L_{ijjj}^{V8,LR} + \frac{328}{9}L_{ijii}^{V,LL} \\
& + \frac{328}{9}L_{ijjj}^{V,LL} \Big] + \alpha_s \alpha \Big[ \frac{208}{9}L_{ij11}^{V1,LL} + \frac{16}{9}L_{ij22}^{V1,LL} + \frac{16}{9}L_{ij11}^{V1,LR} + \frac{16}{9}L_{ij22}^{V1,LR} \\
& + \frac{112}{729}L_{ij11}^{V8,LL} + \frac{328}{729}L_{ij22}^{V8,LL} - \frac{392}{729}L_{ij11}^{V8,LR} - \frac{392}{729}L_{ij22}^{V8,LR} - \frac{32}{9}L_{ijii}^{V1,LR} \\
& - \frac{32}{9}L_{ijjj}^{V1,LR} + \frac{1984}{729}L_{ijii}^{V8,LR} + \frac{1984}{729}L_{ijjj}^{V8,LR} - \frac{2240}{243}L_{ijii}^{V,LL} - \frac{2240}{243}L_{ijjj}^{V,LL} \Big] \\
& + \alpha^2 \Big[ \frac{1544}{729}L_{11ij}^{V,LL} + \frac{1544}{729}L_{22ij}^{V,LL} + \frac{1544}{729}L_{33ij}^{V,LL} - \frac{1120}{729}L_{ij11}^{V1,LL} - \frac{112}{729}L_{ij22}^{V1,LL}
\end{aligned}$$

$$\begin{aligned}
& -\frac{40}{729}L_{ud\ ij11}^{V1,LR} - \frac{40}{729}L_{ud\ ij22}^{V1,LR} + \frac{1760}{729}L_{ij11}^{V,LR} + \frac{1760}{729}L_{ij22}^{V,LR} + \frac{1760}{729}L_{ij33}^{V,LR} \\
& + \frac{2240}{729}L_{ijii}^{V1,LR} + \frac{2240}{729}L_{ijjj}^{V1,LR} + \frac{11488}{729}L_{ijii}^{V,LL} + \frac{11488}{729}L_{ijjj}^{V,LL} \Bigg] ; \\
\dot{L}_{ud\ ij11}^{V8,LL} = & g_s^2 \Bigg[ 12L_{ud\ ij11}^{V1,LL} - \frac{10}{3}L_{ud\ ij11}^{V8,LL} + \frac{2}{3}L_{ud\ ij22}^{V8,LL} + \frac{2}{3}L_{ud\ ij11}^{V8,LR} + \frac{2}{3}L_{ud\ ij22}^{V8,LR} \\
& + \frac{2}{3}L_{ijii}^{V8,LR} + \frac{2}{3}L_{ijjj}^{V8,LR} + \frac{8}{3}L_{ijii}^{V,LL} + \frac{8}{3}L_{ijjj}^{V,LL} \Bigg] - \frac{8}{3}e^2L_{ud\ ij11}^{V8,LL} + \alpha_s^2 \Bigg[ 13L_{ud\ ij11}^{V1,LL} \\
& - \frac{2}{3}L_{ud\ ij22}^{V1,LL} - \frac{22}{3}L_{ud\ ij11}^{V1,LR} - \frac{22}{3}L_{ud\ ij22}^{V1,LR} - \frac{326}{81}L_{ud\ ij11}^{V8,LL} + \frac{799}{81}L_{ud\ ij22}^{V8,LL} + \frac{169}{81}L_{ud\ ij11}^{V8,LR} \\
& + \frac{169}{81}L_{ud\ ij22}^{V8,LR} - \frac{22}{3}L_{ijii}^{V1,LR} - \frac{22}{3}L_{ijjj}^{V1,LR} + \frac{169}{81}L_{ijii}^{V8,LR} + \frac{169}{81}L_{ijjj}^{V8,LR} + \frac{1930}{27}L_{ijii}^{V,LL} \\
& + \frac{1930}{27}L_{ijjj}^{V,LL} \Bigg] + \alpha_s \alpha \Bigg[ \frac{308}{81}L_{11ij}^{V,LL} + \frac{308}{81}L_{22ij}^{V,LL} + \frac{308}{81}L_{33ij}^{V,LL} + \frac{200}{81}L_{ud\ ij11}^{V1,LL} \\
& + \frac{308}{81}L_{ud\ ij22}^{V1,LL} + \frac{308}{81}L_{ud\ ij11}^{V1,LR} + \frac{308}{81}L_{ud\ ij22}^{V1,LR} - \frac{11}{3}L_{ud\ ij11}^{V8,LL} + \frac{14}{9}L_{ud\ ij22}^{V8,LL} + \frac{10}{27}L_{ud\ ij11}^{V8,LR} \\
& + \frac{10}{27}L_{ud\ ij22}^{V8,LR} + \frac{308}{81}L_{ij11}^{V,LR} + \frac{308}{81}L_{ij22}^{V,LR} + \frac{308}{81}L_{ij33}^{V,LR} - \frac{616}{81}L_{ijii}^{V1,LR} - \frac{616}{81}L_{ijjj}^{V1,LR} \\
& + \frac{4}{27}L_{ijii}^{V8,LR} + \frac{4}{27}L_{ijjj}^{V8,LR} - \frac{4808}{81}L_{ijii}^{V,LL} - \frac{4808}{81}L_{ijjj}^{V,LL} \Bigg] - \frac{112}{81}\alpha^2L_{ud\ ij11}^{V8,LL} ; \\
\dot{L}_{ud\ ij22}^{V1,LL} = & \frac{8}{3}g_s^2L_{ud\ ij22}^{V8,LL} + e^2 \Bigg[ \frac{4}{9}L_{11ij}^{V,LL} + \frac{4}{9}L_{22ij}^{V,LL} + \frac{4}{9}L_{33ij}^{V,LL} + \frac{4}{9}L_{ud\ ij11}^{V1,LL} \\
& - \frac{20}{9}L_{ud\ ij22}^{V1,LL} + \frac{4}{9}L_{ud\ ij11}^{V1,LR} + \frac{4}{9}L_{ud\ ij22}^{V1,LR} + \frac{4}{9}L_{ij11}^{V,LR} + \frac{4}{9}L_{ij22}^{V,LR} + \frac{4}{9}L_{ij33}^{V,LR} \\
& - \frac{8}{9}L_{ijii}^{V1,LR} - \frac{8}{9}L_{ijjj}^{V1,LR} - \frac{64}{27}L_{ijii}^{V,LL} - \frac{64}{27}L_{ijjj}^{V,LL} \Bigg] + \alpha_s^2 \Bigg[ 8L_{ud\ ij11}^{V1,LL} \\
& - \frac{4}{3}L_{ud\ ij22}^{V1,LL} - 8L_{ud\ ij11}^{V1,LR} - 8L_{ud\ ij22}^{V1,LR} + \frac{4}{27}L_{ud\ ij11}^{V8,LL} + \frac{86}{27}L_{ud\ ij22}^{V8,LL} + \frac{4}{27}L_{ud\ ij11}^{V8,LR} \\
& + \frac{4}{27}L_{ud\ ij22}^{V8,LR} - 8L_{ijii}^{V1,LR} - 8L_{ijjj}^{V1,LR} + \frac{4}{27}L_{ijii}^{V8,LR} + \frac{4}{27}L_{ijjj}^{V8,LR} + \frac{328}{9}L_{ijii}^{V,LL} \\
& + \frac{328}{9}L_{ijjj}^{V,LL} \Bigg] + \alpha_s \alpha \Bigg[ \frac{16}{9}L_{ud\ ij11}^{V1,LL} + \frac{208}{9}L_{ud\ ij22}^{V1,LL} + \frac{16}{9}L_{ud\ ij11}^{V1,LR} + \frac{16}{9}L_{ud\ ij22}^{V1,LR}
\end{aligned}$$

$$\begin{aligned}
& + \frac{328}{729} L_{ud,ij11}^{V8,LL} + \frac{112}{729} L_{ud,ij22}^{V8,LL} - \frac{392}{729} L_{ud,ij11}^{V8,LR} - \frac{392}{729} L_{ud,ij22}^{V8,LR} - \frac{32}{9} L_{uu,ijii}^{V1,LR} \\
& - \frac{32}{9} L_{uu,ijjj}^{V1,LR} + \frac{1984}{729} L_{uu,ijii}^{V8,LR} + \frac{1984}{729} L_{uu,ijjj}^{V8,LR} - \frac{2240}{243} L_{uu,ijii}^{V,LL} - \frac{2240}{243} L_{uu,ijjj}^{V,LL} \Big] \\
& + \alpha^2 \Big[ \frac{1544}{729} L_{eu,11ij}^{V,LL} + \frac{1544}{729} L_{eu,22ij}^{V,LL} + \frac{1544}{729} L_{eu,33ij}^{V,LL} - \frac{112}{729} L_{ud,ij11}^{V1,LL} - \frac{1120}{729} L_{ud,ij22}^{V1,LL} \\
& - \frac{40}{729} L_{ud,ij11}^{V1,LR} - \frac{40}{729} L_{ud,ij22}^{V1,LR} + \frac{1760}{729} L_{ue,ij11}^{V,LR} + \frac{1760}{729} L_{ue,ij22}^{V,LR} + \frac{1760}{729} L_{ue,ij33}^{V,LR} \\
& + \frac{2240}{729} L_{uu,ijii}^{V1,LR} + \frac{2240}{729} L_{uu,ijjj}^{V1,LR} + \frac{11488}{729} L_{uu,ijii}^{V,LL} + \frac{11488}{729} L_{uu,ijjj}^{V,LL} \Big] ; \\
\dot{L}_{ud,ij22}^{V8,LL} & = g_s^2 \Big[ 12 L_{ud,ij22}^{V1,LL} + \frac{2}{3} L_{ud,ij11}^{V8,LL} - \frac{10}{3} L_{ud,ij22}^{V8,LL} + \frac{2}{3} L_{ud,ij11}^{V8,LR} + \frac{2}{3} L_{ud,ij22}^{V8,LR} \\
& + \frac{2}{3} L_{uu,ijii}^{V8,LR} + \frac{2}{3} L_{uu,ijjj}^{V8,LR} + \frac{8}{3} L_{uu,ijii}^{V,LL} + \frac{8}{3} L_{uu,ijjj}^{V,LL} \Big] - \frac{8}{3} e^2 L_{ud,ij22}^{V8,LL} + \alpha_s^2 \Big[ - \frac{2}{3} L_{ud,ij11}^{V1,LL} \\
& + 13 L_{ud,ij22}^{V1,LL} - \frac{22}{3} L_{ud,ij11}^{V1,LR} - \frac{22}{3} L_{ud,ij22}^{V1,LR} + \frac{799}{81} L_{ud,ij11}^{V8,LL} - \frac{326}{81} L_{ud,ij22}^{V8,LL} + \frac{169}{81} L_{ud,ij11}^{V8,LR} \\
& + \frac{169}{81} L_{ud,ij22}^{V8,LR} - \frac{22}{3} L_{uu,ijii}^{V1,LR} - \frac{22}{3} L_{uu,ijjj}^{V1,LR} + \frac{169}{81} L_{uu,ijii}^{V8,LR} + \frac{169}{81} L_{uu,ijjj}^{V8,LR} + \frac{1930}{27} L_{uu,ijii}^{V,LL} \\
& + \frac{1930}{27} L_{uu,ijjj}^{V,LL} \Big] + \alpha_s \alpha \Big[ \frac{308}{81} L_{eu,11ij}^{V,LL} + \frac{308}{81} L_{eu,22ij}^{V,LL} + \frac{308}{81} L_{eu,33ij}^{V,LL} + \frac{308}{81} L_{ud,ij11}^{V1,LL} \\
& + \frac{200}{81} L_{ud,ij22}^{V1,LL} + \frac{308}{81} L_{ud,ij11}^{V1,LR} + \frac{308}{81} L_{ud,ij22}^{V1,LR} + \frac{14}{9} L_{ud,ij11}^{V8,LL} - \frac{11}{3} L_{ud,ij22}^{V8,LL} + \frac{10}{27} L_{ud,ij11}^{V8,LR} \\
& + \frac{10}{27} L_{ud,ij22}^{V8,LR} + \frac{308}{81} L_{ue,ij11}^{V,LR} + \frac{308}{81} L_{ue,ij22}^{V,LR} + \frac{308}{81} L_{ue,ij33}^{V,LR} - \frac{616}{81} L_{uu,ijii}^{V1,LR} - \frac{616}{81} L_{uu,ijjj}^{V1,LR} \\
& + \frac{4}{27} L_{uu,ijii}^{V8,LR} + \frac{4}{27} L_{uu,ijjj}^{V8,LR} - \frac{4808}{81} L_{uu,ijii}^{V,LL} - \frac{4808}{81} L_{uu,ijjj}^{V,LL} \Big] - \frac{112}{81} \alpha^2 L_{ud,ij22}^{V8,LL} ; \\
\dot{L}_{uu,ijjj}^{V,LL} & = g_s^2 \Big[ \frac{1}{9} L_{ud,ij11}^{V8,LL} + \frac{1}{9} L_{ud,ij22}^{V8,LL} + \frac{1}{9} L_{ud,ij11}^{V8,LR} + \frac{1}{9} L_{ud,ij22}^{V8,LR} + \frac{1}{9} L_{uu,ijii}^{V8,LR} \\
& + \frac{1}{9} L_{uu,ijjj}^{V8,LR} + \frac{4}{9} L_{uu,ijii}^{V,LL} + \frac{40}{9} L_{uu,ijjj}^{V,LL} \Big] + e^2 \Big[ - \frac{4}{9} L_{eu,11ij}^{V,LL} - \frac{4}{9} L_{eu,22ij}^{V,LL} - \frac{4}{9} L_{eu,33ij}^{V,LL} \\
& - \frac{4}{9} L_{ud,ij11}^{V1,LL} - \frac{4}{9} L_{ud,ij22}^{V1,LL} - \frac{4}{9} L_{ud,ij11}^{V1,LR} - \frac{4}{9} L_{ud,ij22}^{V1,LR} - \frac{4}{9} L_{ue,ij11}^{V,LR} - \frac{4}{9} L_{ue,ij22}^{V,LR}
\end{aligned}$$

$$\begin{aligned}
& -\frac{4}{9}L_{ue,ij33}^{V,LR} + \frac{8}{9}L_{uu,ijii}^{V1,LR} + \frac{8}{9}L_{uu,ijjj}^{V1,LR} + \frac{64}{27}L_{uu,ijii}^{V,LL} + \frac{208}{27}L_{uu,ijjj}^{V,LL} \Big] + \alpha_s^2 \Big[ \frac{35}{9}L_{ud,ij11}^{V1,LL} \\
& + \frac{35}{9}L_{ud,ij22}^{V1,LL} - \frac{47}{9}L_{ud,ij11}^{V1,LR} - \frac{47}{9}L_{ud,ij22}^{V1,LR} + \frac{835}{486}L_{ud,ij11}^{V8,LL} + \frac{835}{486}L_{ud,ij22}^{V8,LL} + \frac{205}{486}L_{ud,ij11}^{V8,LR} \\
& + \frac{205}{486}L_{ud,ij22}^{V8,LR} - \frac{47}{9}L_{uu,ijii}^{V1,LR} - \frac{47}{9}L_{uu,ijjj}^{V1,LR} + \frac{205}{486}L_{uu,ijii}^{V8,LR} + \frac{205}{486}L_{uu,ijjj}^{V8,LR} + \frac{2441}{81}L_{uu,ijii}^{V,LL} \\
& + \frac{2054}{81}L_{uu,ijjj}^{V,LL} \Big] + \alpha_s \alpha \Big[ \frac{100}{243}L_{eu,11ij}^{V,LL} + \frac{100}{243}L_{eu,22ij}^{V,LL} + \frac{100}{243}L_{eu,33ij}^{V,LL} - \frac{332}{243}L_{ud,ij11}^{V1,LL} \\
& - \frac{332}{243}L_{ud,ij22}^{V1,LL} - \frac{332}{243}L_{ud,ij11}^{V1,LR} - \frac{332}{243}L_{ud,ij22}^{V1,LR} - \frac{571}{729}L_{ud,ij11}^{V8,LL} - \frac{571}{729}L_{ud,ij22}^{V8,LL} \\
& + \frac{977}{729}L_{ud,ij11}^{V8,LR} + \frac{977}{729}L_{ud,ij22}^{V8,LR} + \frac{100}{243}L_{ue,ij11}^{V,LR} + \frac{100}{243}L_{ue,ij22}^{V,LR} + \frac{100}{243}L_{ue,ij33}^{V,LR} \\
& + \frac{664}{243}L_{uu,ijii}^{V1,LR} + \frac{664}{243}L_{uu,ijjj}^{V1,LR} - \frac{2884}{729}L_{uu,ijii}^{V8,LR} - \frac{2884}{729}L_{uu,ijjj}^{V8,LR} + \frac{3832}{243}L_{uu,ijii}^{V,LL} \\
& - \frac{12152}{243}L_{uu,ijjj}^{V,LL} \Big] + \alpha^2 \Big[ \frac{1156}{729}L_{eu,11ij}^{V,LL} + \frac{1156}{729}L_{eu,22ij}^{V,LL} + \frac{1156}{729}L_{eu,33ij}^{V,LL} + \frac{868}{729}L_{ud,ij11}^{V1,LL} \\
& + \frac{868}{729}L_{ud,ij22}^{V1,LL} - \frac{1148}{729}L_{ud,ij11}^{V1,LR} - \frac{1148}{729}L_{ud,ij22}^{V1,LR} - \frac{4892}{729}L_{ue,ij11}^{V,LR} - \frac{4892}{729}L_{ue,ij22}^{V,LR} \\
& - \frac{4892}{729}L_{ue,ij33}^{V,LR} - \frac{5696}{729}L_{uu,ijii}^{V1,LR} - \frac{5696}{729}L_{uu,ijjj}^{V1,LR} + \frac{10112}{729}L_{uu,ijii}^{V,LL} - \frac{832}{729}L_{uu,ijjj}^{V,LL} \Big] ;
\end{aligned}$$

$$\begin{aligned}
\dot{L}_{uu,ijii}^{V,LL} & = g_s^2 \Big[ \frac{1}{9}L_{ud,ij11}^{V8,LL} + \frac{1}{9}L_{ud,ij22}^{V8,LL} + \frac{1}{9}L_{ud,ij11}^{V8,LR} + \frac{1}{9}L_{ud,ij22}^{V8,LR} + \frac{1}{9}L_{uu,ijii}^{V8,LR} \\
& + \frac{1}{9}L_{uu,ijjj}^{V8,LR} + \frac{40}{9}L_{uu,ijii}^{V,LL} + \frac{4}{9}L_{uu,ijjj}^{V,LL} \Big] + e^2 \Big[ -\frac{4}{9}L_{eu,11ij}^{V,LL} - \frac{4}{9}L_{eu,22ij}^{V,LL} - \frac{4}{9}L_{eu,33ij}^{V,LL} \\
& - \frac{4}{9}L_{ud,ij11}^{V1,LL} - \frac{4}{9}L_{ud,ij22}^{V1,LL} - \frac{4}{9}L_{ud,ij11}^{V1,LR} - \frac{4}{9}L_{ud,ij22}^{V1,LR} - \frac{4}{9}L_{ue,ij11}^{V,LR} - \frac{4}{9}L_{ue,ij22}^{V,LR} \\
& - \frac{4}{9}L_{ue,ij33}^{V,LR} + \frac{8}{9}L_{uu,ijii}^{V1,LR} + \frac{8}{9}L_{uu,ijjj}^{V1,LR} + \frac{208}{27}L_{uu,ijii}^{V,LL} + \frac{64}{27}L_{uu,ijjj}^{V,LL} \Big] + \alpha_s^2 \Big[ \frac{35}{9}L_{ud,ij11}^{V1,LL} \\
& + \frac{35}{9}L_{ud,ij22}^{V1,LL} - \frac{47}{9}L_{ud,ij11}^{V1,LR} - \frac{47}{9}L_{ud,ij22}^{V1,LR} + \frac{835}{486}L_{ud,ij11}^{V8,LL} + \frac{835}{486}L_{ud,ij22}^{V8,LL} + \frac{205}{486}L_{ud,ij11}^{V8,LR} \\
& + \frac{205}{486}L_{ud,ij22}^{V8,LR} - \frac{47}{9}L_{uu,ijii}^{V1,LR} - \frac{47}{9}L_{uu,ijjj}^{V1,LR} + \frac{205}{486}L_{uu,ijii}^{V8,LR} + \frac{205}{486}L_{uu,ijjj}^{V8,LR} + \frac{2054}{81}L_{uu,ijii}^{V,LL} \\
& + \frac{2054}{81}L_{uu,ijjj}^{V,LL} \Big]
\end{aligned}$$

$$\begin{aligned}
& + \frac{2441}{81} L_{ijjj}^{V,LL} \Big] + \alpha_s \alpha \Big[ \frac{100}{243} L_{11ij}^{V,LL} + \frac{100}{243} L_{22ij}^{V,LL} + \frac{100}{243} L_{33ij}^{V,LL} - \frac{332}{243} L_{ij11}^{V1,LL} \\
& - \frac{332}{243} L_{ij22}^{V1,LL} - \frac{332}{243} L_{ij11}^{V1,LR} - \frac{332}{243} L_{ij22}^{V1,LR} - \frac{571}{729} L_{ij11}^{V8,LL} - \frac{571}{729} L_{ij22}^{V8,LL} \\
& + \frac{977}{729} L_{ij11}^{V8,LR} + \frac{977}{729} L_{ij22}^{V8,LR} + \frac{100}{243} L_{ij11}^{V,LR} + \frac{100}{243} L_{ij22}^{V,LR} + \frac{100}{243} L_{ij33}^{V,LR} \\
& + \frac{664}{243} L_{ijii}^{V1,LR} + \frac{664}{243} L_{ijjj}^{V1,LR} - \frac{2884}{729} L_{ijii}^{V8,LR} - \frac{2884}{729} L_{ijjj}^{V8,LR} - \frac{12152}{243} L_{ijii}^{V,LL} \\
& + \frac{3832}{243} L_{ijjj}^{V,LL} \Big] + \alpha^2 \Big[ \frac{1156}{729} L_{11ij}^{V,LL} + \frac{1156}{729} L_{22ij}^{V,LL} + \frac{1156}{729} L_{33ij}^{V,LL} + \frac{868}{729} L_{ij11}^{V1,LL} \\
& + \frac{868}{729} L_{ij22}^{V1,LL} - \frac{1148}{729} L_{ij11}^{V1,LR} - \frac{1148}{729} L_{ij22}^{V1,LR} - \frac{4892}{729} L_{ij11}^{V,LR} - \frac{4892}{729} L_{ij22}^{V,LR} \\
& - \frac{4892}{729} L_{ij33}^{V,LR} - \frac{5696}{729} L_{ijii}^{V1,LR} - \frac{5696}{729} L_{ijjj}^{V1,LR} - \frac{832}{729} L_{ijii}^{V,LL} + \frac{10112}{729} L_{ijjj}^{V,LL} \Big] ;
\end{aligned}$$

$$\begin{aligned}
\dot{L}_{ij11}^{V,LR} = & e^2 \Big[ \frac{4}{3} L_{11ij}^{V,LL} + \frac{4}{3} L_{22ij}^{V,LL} + \frac{4}{3} L_{33ij}^{V,LL} + \frac{4}{3} L_{ij11}^{V1,LL} + \frac{4}{3} L_{ij22}^{V1,LL} \\
& + \frac{4}{3} L_{ij11}^{V1,LR} + \frac{4}{3} L_{ij22}^{V1,LR} + \frac{28}{3} L_{ij11}^{V,LR} + \frac{4}{3} L_{ij22}^{V,LR} + \frac{4}{3} L_{ij33}^{V,LR} - \frac{8}{3} L_{ijii}^{V1,LR} \\
& - \frac{8}{3} L_{ijjj}^{V1,LR} - \frac{64}{9} L_{ijii}^{V,LL} - \frac{64}{9} L_{ijjj}^{V,LL} \Big] + \alpha_s \alpha \Big[ \frac{16}{3} L_{ij11}^{V1,LL} + \frac{16}{3} L_{ij22}^{V1,LL} \\
& + \frac{16}{3} L_{ij11}^{V1,LR} + \frac{16}{3} L_{ij22}^{V1,LR} + \frac{328}{243} L_{ij11}^{V8,LL} + \frac{328}{243} L_{ij22}^{V8,LL} - \frac{392}{243} L_{ij11}^{V8,LR} - \frac{392}{243} L_{ij22}^{V8,LR} \\
& - 32 L_{ij11}^{V,LR} - \frac{32}{3} L_{ijii}^{V1,LR} - \frac{32}{3} L_{ijjj}^{V1,LR} + \frac{1984}{243} L_{ijii}^{V8,LR} + \frac{1984}{243} L_{ijjj}^{V8,LR} - \frac{2240}{81} L_{ijii}^{V,LL} \\
& - \frac{2240}{81} L_{ijjj}^{V,LL} \Big] + \alpha^2 \Big[ - \frac{4648}{243} L_{11ij}^{V,LL} - \frac{4648}{243} L_{22ij}^{V,LL} - \frac{4648}{243} L_{33ij}^{V,LL} - \frac{3712}{243} L_{ij11}^{V1,LL} \\
& - \frac{3712}{243} L_{ij22}^{V1,LL} - \frac{1048}{243} L_{ij11}^{V1,LR} - \frac{1048}{243} L_{ij22}^{V1,LR} - \frac{39712}{243} L_{ij11}^{V,LR} + \frac{3344}{243} L_{ij22}^{V,LR} \\
& + \frac{3344}{243} L_{ij33}^{V,LR} + \frac{12032}{243} L_{ijii}^{V1,LR} + \frac{12032}{243} L_{ijjj}^{V1,LR} + \frac{3424}{243} L_{ijii}^{V,LL} + \frac{3424}{243} L_{ijjj}^{V,LL} \Big] ;
\end{aligned}$$

$$\dot{L}_{ij22}^{V,LR} = e^2 \Big[ \frac{4}{3} L_{11ij}^{V,LL} + \frac{4}{3} L_{22ij}^{V,LL} + \frac{4}{3} L_{33ij}^{V,LL} + \frac{4}{3} L_{ij11}^{V1,LL} + \frac{4}{3} L_{ij22}^{V1,LL}$$

$$\begin{aligned}
& + \frac{4}{3}L_{ud\ ij11}^{V1,LR} + \frac{4}{3}L_{ud\ ij22}^{V1,LR} + \frac{4}{3}L_{ue\ ij11}^{V,LR} + \frac{28}{3}L_{ue\ ij22}^{V,LR} + \frac{4}{3}L_{ue\ ij33}^{V,LR} - \frac{8}{3}L_{uu\ ijii}^{V1,LR} \\
& - \frac{8}{3}L_{uu\ ijjj}^{V1,LR} - \frac{64}{9}L_{uu\ ijii}^{V,LL} - \frac{64}{9}L_{uu\ ijjj}^{V,LL} \Big] + \alpha_s \alpha \Big[ \frac{16}{3}L_{ud\ ij11}^{V1,LL} + \frac{16}{3}L_{ud\ ij22}^{V1,LL} \\
& + \frac{16}{3}L_{ud\ ij11}^{V1,LR} + \frac{16}{3}L_{ud\ ij22}^{V1,LR} + \frac{328}{243}L_{ud\ ij11}^{V8,LL} + \frac{328}{243}L_{ud\ ij22}^{V8,LL} - \frac{392}{243}L_{ud\ ij11}^{V8,LR} - \frac{392}{243}L_{ud\ ij22}^{V8,LR} \\
& - 32L_{ue\ ij22}^{V,LR} - \frac{32}{3}L_{uu\ ijii}^{V1,LR} - \frac{32}{3}L_{uu\ ijjj}^{V1,LR} + \frac{1984}{243}L_{uu\ ijii}^{V8,LR} + \frac{1984}{243}L_{uu\ ijjj}^{V8,LR} - \frac{2240}{81}L_{uu\ ijii}^{V,LL} \\
& - \frac{2240}{81}L_{uu\ ijjj}^{V,LL} \Big] + \alpha^2 \Big[ - \frac{4648}{243}L_{eu\ 11ij}^{V,LL} - \frac{4648}{243}L_{eu\ 22ij}^{V,LL} - \frac{4648}{243}L_{eu\ 33ij}^{V,LL} - \frac{3712}{243}L_{ud\ ij11}^{V1,LL} \\
& - \frac{3712}{243}L_{ud\ ij22}^{V1,LL} - \frac{1048}{243}L_{ud\ ij11}^{V1,LR} - \frac{1048}{243}L_{ud\ ij22}^{V1,LR} + \frac{3344}{243}L_{ue\ ij11}^{V,LR} - \frac{39712}{243}L_{ue\ ij22}^{V,LR} \\
& + \frac{3344}{243}L_{ue\ ij33}^{V,LR} + \frac{12032}{243}L_{uu\ ijii}^{V1,LR} + \frac{12032}{243}L_{uu\ ijjj}^{V1,LR} + \frac{3424}{243}L_{uu\ ijii}^{V,LL} + \frac{3424}{243}L_{uu\ ijjj}^{V,LL} \Big] ; \\
\dot{L}_{ue\ ij33}^{V,LR} & = e^2 \Big[ \frac{4}{3}L_{eu\ 11ij}^{V,LL} + \frac{4}{3}L_{eu\ 22ij}^{V,LL} + \frac{4}{3}L_{eu\ 33ij}^{V,LL} + \frac{4}{3}L_{ud\ ij11}^{V1,LL} + \frac{4}{3}L_{ud\ ij22}^{V1,LL} \\
& + \frac{4}{3}L_{ud\ ij11}^{V1,LR} + \frac{4}{3}L_{ud\ ij22}^{V1,LR} + \frac{4}{3}L_{ue\ ij11}^{V,LR} + \frac{4}{3}L_{ue\ ij22}^{V,LR} + \frac{28}{3}L_{ue\ ij33}^{V,LR} - \frac{8}{3}L_{uu\ ijii}^{V1,LR} \\
& - \frac{8}{3}L_{uu\ ijjj}^{V1,LR} - \frac{64}{9}L_{uu\ ijii}^{V,LL} - \frac{64}{9}L_{uu\ ijjj}^{V,LL} \Big] + \alpha_s \alpha \Big[ \frac{16}{3}L_{ud\ ij11}^{V1,LL} + \frac{16}{3}L_{ud\ ij22}^{V1,LL} \\
& + \frac{16}{3}L_{ud\ ij11}^{V1,LR} + \frac{16}{3}L_{ud\ ij22}^{V1,LR} + \frac{328}{243}L_{ud\ ij11}^{V8,LL} + \frac{328}{243}L_{ud\ ij22}^{V8,LL} - \frac{392}{243}L_{ud\ ij11}^{V8,LR} - \frac{392}{243}L_{ud\ ij22}^{V8,LR} \\
& - 32L_{ue\ ij33}^{V,LR} - \frac{32}{3}L_{uu\ ijii}^{V1,LR} - \frac{32}{3}L_{uu\ ijjj}^{V1,LR} + \frac{1984}{243}L_{uu\ ijii}^{V8,LR} + \frac{1984}{243}L_{uu\ ijjj}^{V8,LR} - \frac{2240}{81}L_{uu\ ijii}^{V,LL} \\
& - \frac{2240}{81}L_{uu\ ijjj}^{V,LL} \Big] + \alpha^2 \Big[ - \frac{4648}{243}L_{eu\ 11ij}^{V,LL} - \frac{4648}{243}L_{eu\ 22ij}^{V,LL} - \frac{4648}{243}L_{eu\ 33ij}^{V,LL} - \frac{3712}{243}L_{ud\ ij11}^{V1,LL} \\
& - \frac{3712}{243}L_{ud\ ij22}^{V1,LL} - \frac{1048}{243}L_{ud\ ij11}^{V1,LR} - \frac{1048}{243}L_{ud\ ij22}^{V1,LR} + \frac{3344}{243}L_{ue\ ij11}^{V,LR} + \frac{3344}{243}L_{ue\ ij22}^{V,LR} \\
& - \frac{39712}{243}L_{ue\ ij33}^{V,LR} + \frac{12032}{243}L_{uu\ ijii}^{V1,LR} + \frac{12032}{243}L_{uu\ ijjj}^{V1,LR} + \frac{3424}{243}L_{uu\ ijii}^{V,LL} + \frac{3424}{243}L_{uu\ ijjj}^{V,LL} \Big] ; \\
\dot{L}_{ud\ ij11}^{V1,LR} & = -\frac{8}{3}g_s^2L_{ud\ ij11}^{V8,LR} + e^2 \Big[ \frac{4}{9}L_{eu\ 11ij}^{V,LL} + \frac{4}{9}L_{eu\ 22ij}^{V,LL} + \frac{4}{9}L_{eu\ 33ij}^{V,LL} + \frac{4}{9}L_{ud\ ij11}^{V1,LL} \\
& + \frac{4}{9}L_{ud\ ij22}^{V1,LL} + \frac{4}{9}L_{ue\ ij11}^{V,LL} + \frac{4}{9}L_{ue\ ij22}^{V,LL} + \frac{28}{9}L_{ue\ ij33}^{V,LL} - \frac{8}{9}L_{uu\ ijii}^{V1,LL} \\
& - \frac{8}{9}L_{uu\ ijjj}^{V1,LL} - \frac{64}{9}L_{uu\ ijii}^{V,LL} - \frac{64}{9}L_{uu\ ijjj}^{V,LL} \Big] + \alpha_s \alpha \Big[ \frac{16}{3}L_{ud\ ij11}^{V1,LL} + \frac{16}{3}L_{ud\ ij22}^{V1,LL} \\
& + \frac{16}{3}L_{ud\ ij11}^{V1,LR} + \frac{16}{3}L_{ud\ ij22}^{V1,LR} + \frac{328}{243}L_{ud\ ij11}^{V8,LL} + \frac{328}{243}L_{ud\ ij22}^{V8,LL} - \frac{392}{243}L_{ud\ ij11}^{V8,LR} - \frac{392}{243}L_{ud\ ij22}^{V8,LR} \\
& - 32L_{ue\ ij33}^{V,LR} - \frac{32}{3}L_{uu\ ijii}^{V1,LR} - \frac{32}{3}L_{uu\ ijjj}^{V1,LR} + \frac{1984}{243}L_{uu\ ijii}^{V8,LR} + \frac{1984}{243}L_{uu\ ijjj}^{V8,LR} - \frac{2240}{81}L_{uu\ ijii}^{V,LL} \\
& - \frac{2240}{81}L_{uu\ ijjj}^{V,LL} \Big] + \alpha^2 \Big[ - \frac{4648}{243}L_{eu\ 11ij}^{V,LL} - \frac{4648}{243}L_{eu\ 22ij}^{V,LL} - \frac{4648}{243}L_{eu\ 33ij}^{V,LL} - \frac{3712}{243}L_{ud\ ij11}^{V1,LL} \\
& - \frac{3712}{243}L_{ud\ ij22}^{V1,LL} - \frac{1048}{243}L_{ud\ ij11}^{V1,LR} - \frac{1048}{243}L_{ud\ ij22}^{V1,LR} + \frac{3344}{243}L_{ue\ ij11}^{V,LR} + \frac{3344}{243}L_{ue\ ij22}^{V,LR} \\
& - \frac{39712}{243}L_{ue\ ij33}^{V,LR} + \frac{12032}{243}L_{uu\ ijii}^{V1,LR} + \frac{12032}{243}L_{uu\ ijjj}^{V1,LR} + \frac{3424}{243}L_{uu\ ijii}^{V,LL} + \frac{3424}{243}L_{uu\ ijjj}^{V,LL} \Big] ;
\end{aligned}$$

$$\begin{aligned}
& + \frac{4}{9} L_{ud}^{V1,LL} + \frac{28}{9} L_{ij11}^{V1,LR} + \frac{4}{9} L_{ij22}^{V1,LR} + \frac{4}{9} L_{ij11}^{V,LR} + \frac{4}{9} L_{ij22}^{V,LR} + \frac{4}{9} L_{ij33}^{V,LR} \\
& - \frac{8}{9} L_{ijii}^{V1,LR} - \frac{8}{9} L_{ijjj}^{V1,LR} - \frac{64}{27} L_{ijii}^{V,LL} - \frac{64}{27} L_{ijjj}^{V,LL} \Big] + \alpha_s^2 \Big[ -8 L_{ij11}^{V1,LL} \\
& - 8 L_{ud}^{V1,LL} - \frac{4}{3} L_{ij11}^{V1,LR} + 8 L_{ij22}^{V1,LR} + \frac{44}{27} L_{ij11}^{V8,LL} + \frac{44}{27} L_{ij22}^{V8,LL} - \frac{2000}{27} L_{ij11}^{V8,LR} \\
& + \frac{44}{27} L_{ij22}^{V8,LR} + 8 L_{ijii}^{V1,LR} + 8 L_{ijjj}^{V1,LR} + \frac{44}{27} L_{ijii}^{V8,LR} + \frac{44}{27} L_{ijjj}^{V8,LR} - \frac{232}{9} L_{ijii}^{V,LL} \\
& - \frac{232}{9} L_{ijjj}^{V,LL} \Big] + \alpha_s \alpha \Big[ \frac{16}{9} L_{ij11}^{V1,LL} + \frac{16}{9} L_{ij22}^{V1,LL} - \frac{176}{9} L_{ij11}^{V1,LR} + \frac{16}{9} L_{ij22}^{V1,LR} \\
& + \frac{328}{729} L_{ij11}^{V8,LL} + \frac{328}{729} L_{ij22}^{V8,LL} + \frac{5872}{729} L_{ij11}^{V8,LR} - \frac{392}{729} L_{ij22}^{V8,LR} - \frac{32}{9} L_{ijii}^{V1,LR} \\
& - \frac{32}{9} L_{ijjj}^{V1,LR} + \frac{1984}{729} L_{ijii}^{V8,LR} + \frac{1984}{729} L_{ijjj}^{V8,LR} - \frac{2240}{243} L_{ijii}^{V,LL} - \frac{2240}{243} L_{ijjj}^{V,LL} \Big] \\
& + \alpha^2 \Big[ -\frac{1120}{729} L_{11ij}^{V,LL} - \frac{1120}{729} L_{22ij}^{V,LL} - \frac{1120}{729} L_{33ij}^{V,LL} - \frac{1480}{729} L_{ij11}^{V1,LL} - \frac{1480}{729} L_{ij22}^{V1,LL} \\
& - \frac{34960}{729} L_{ij11}^{V1,LR} - \frac{112}{729} L_{ij22}^{V1,LR} + \frac{2984}{729} L_{ij11}^{V,LR} + \frac{2984}{729} L_{ij22}^{V,LR} + \frac{2984}{729} L_{ij33}^{V,LR} \\
& + \frac{6272}{729} L_{ijii}^{V1,LR} + \frac{6272}{729} L_{ijjj}^{V1,LR} + \frac{4000}{729} L_{ijii}^{V,LL} + \frac{4000}{729} L_{ijjj}^{V,LL} \Big] ;
\end{aligned}$$

$$\begin{aligned}
\dot{L}_{ij11}^{V8,LR} & = g_s^2 \Big[ -12 L_{ij11}^{V1,LR} + \frac{2}{3} L_{ij11}^{V8,LL} + \frac{2}{3} L_{ij22}^{V8,LL} - \frac{40}{3} L_{ij11}^{V8,LR} + \frac{2}{3} L_{ij22}^{V8,LR} \\
& + \frac{2}{3} L_{ijii}^{V8,LR} + \frac{2}{3} L_{ijjj}^{V8,LR} + \frac{8}{3} L_{ijii}^{V,LL} + \frac{8}{3} L_{ijjj}^{V,LL} \Big] + \frac{8}{3} e^2 L_{ij11}^{V8,LR} + \alpha_s^2 \Big[ -\frac{2}{3} L_{ij11}^{V1,LL} \\
& - \frac{2}{3} L_{ij22}^{V1,LL} - 132 L_{ij11}^{V1,LR} - \frac{22}{3} L_{ij22}^{V1,LR} + \frac{619}{81} L_{ij11}^{V8,LL} + \frac{619}{81} L_{ij22}^{V8,LL} - \frac{25177}{162} L_{ij11}^{V8,LR} \\
& + \frac{799}{81} L_{ij22}^{V8,LR} - \frac{22}{3} L_{ijii}^{V1,LR} - \frac{22}{3} L_{ijjj}^{V1,LR} + \frac{799}{81} L_{ijii}^{V8,LR} + \frac{799}{81} L_{ijjj}^{V8,LR} + \frac{1210}{27} L_{ijii}^{V,LL} \\
& + \frac{1210}{27} L_{ijjj}^{V,LL} \Big] + \alpha_s \alpha \Big[ \frac{668}{81} L_{11ij}^{V,LL} + \frac{668}{81} L_{22ij}^{V,LL} + \frac{668}{81} L_{33ij}^{V,LL} + \frac{668}{81} L_{ij11}^{V1,LL} \\
& + \frac{668}{81} L_{ij22}^{V1,LL} + \frac{3800}{81} L_{ij11}^{V1,LR} + \frac{668}{81} L_{ij22}^{V1,LR} - \frac{70}{27} L_{ij11}^{V8,LL} - \frac{70}{27} L_{ij22}^{V8,LL} + \frac{67}{3} L_{ij11}^{V8,LR}
\end{aligned}$$



$$\begin{aligned}
& + \frac{14}{9} L_{ud}^{V8,LR} + \frac{668}{81} L_{ij11}^{V,LR} + \frac{668}{81} L_{ij22}^{V,LR} + \frac{668}{81} L_{ij33}^{V,LR} - \frac{1336}{81} L_{ijii}^{V1,LR} - \frac{1336}{81} L_{ijjj}^{V1,LR} \\
& - \frac{20}{3} L_{ijii}^{V8,LR} - \frac{20}{3} L_{ijjj}^{V8,LR} - \frac{3800}{81} L_{ijii}^{V,LL} - \frac{3800}{81} L_{ijjj}^{V,LL} \Big] - \frac{3872}{81} \alpha^2 L_{ij11}^{V8,LR} ; \\
\dot{L}_{ud}^{V1,LR} = & - \frac{8}{3} g_s^2 L_{ij22}^{V8,LR} + e^2 \Big[ \frac{4}{9} L_{11ij}^{V,LL} + \frac{4}{9} L_{22ij}^{V,LL} + \frac{4}{9} L_{33ij}^{V,LL} + \frac{4}{9} L_{ij11}^{V1,LL} \\
& + \frac{4}{9} L_{ij22}^{V1,LL} + \frac{4}{9} L_{ij11}^{V1,LR} + \frac{28}{9} L_{ij22}^{V1,LR} + \frac{4}{9} L_{ij11}^{V,LR} + \frac{4}{9} L_{ij22}^{V,LR} + \frac{4}{9} L_{ij33}^{V,LR} \\
& - \frac{8}{9} L_{ijii}^{V1,LR} - \frac{8}{9} L_{ijjj}^{V1,LR} - \frac{64}{27} L_{ijii}^{V,LL} - \frac{64}{27} L_{ijjj}^{V,LL} \Big] + \alpha_s^2 \Big[ - 8 L_{ij11}^{V1,LL} \\
& - 8 L_{ij22}^{V1,LL} + 8 L_{ij11}^{V1,LR} - \frac{4}{3} L_{ij22}^{V1,LR} + \frac{44}{27} L_{ij11}^{V8,LL} + \frac{44}{27} L_{ij22}^{V8,LL} + \frac{44}{27} L_{ij11}^{V8,LR} \\
& - \frac{2000}{27} L_{ij22}^{V8,LR} + 8 L_{ijii}^{V1,LR} + 8 L_{ijjj}^{V1,LR} + \frac{44}{27} L_{ijii}^{V8,LR} + \frac{44}{27} L_{ijjj}^{V8,LR} - \frac{232}{9} L_{ijii}^{V,LL} \\
& - \frac{232}{9} L_{ijjj}^{V,LL} \Big] + \alpha_s \alpha \Big[ \frac{16}{9} L_{ij11}^{V1,LL} + \frac{16}{9} L_{ij22}^{V1,LL} + \frac{16}{9} L_{ij11}^{V1,LR} - \frac{176}{9} L_{ij22}^{V1,LR} \\
& + \frac{328}{729} L_{ij11}^{V8,LL} + \frac{328}{729} L_{ij22}^{V8,LL} - \frac{392}{729} L_{ij11}^{V8,LR} + \frac{5872}{729} L_{ij22}^{V8,LR} - \frac{32}{9} L_{ijii}^{V1,LR} \\
& - \frac{32}{9} L_{ijjj}^{V1,LR} + \frac{1984}{729} L_{ijii}^{V8,LR} + \frac{1984}{729} L_{ijjj}^{V8,LR} - \frac{2240}{243} L_{ijii}^{V,LL} - \frac{2240}{243} L_{ijjj}^{V,LL} \Big] \\
& + \alpha^2 \Big[ - \frac{1120}{729} L_{11ij}^{V,LL} - \frac{1120}{729} L_{22ij}^{V,LL} - \frac{1120}{729} L_{33ij}^{V,LL} - \frac{1480}{729} L_{ij11}^{V1,LL} - \frac{1480}{729} L_{ij22}^{V1,LL} \\
& - \frac{112}{729} L_{ij11}^{V1,LR} - \frac{34960}{729} L_{ij22}^{V1,LR} + \frac{2984}{729} L_{ij11}^{V,LR} + \frac{2984}{729} L_{ij22}^{V,LR} + \frac{2984}{729} L_{ij33}^{V,LR} \\
& + \frac{6272}{729} L_{ijii}^{V1,LR} + \frac{6272}{729} L_{ijjj}^{V1,LR} + \frac{4000}{729} L_{ijii}^{V,LL} + \frac{4000}{729} L_{ijjj}^{V,LL} \Big] ; \\
\dot{L}_{ud}^{V8,LR} = & g_s^2 \Big[ - 12 L_{ij22}^{V1,LR} + \frac{2}{3} L_{ij11}^{V8,LL} + \frac{2}{3} L_{ij22}^{V8,LL} + \frac{2}{3} L_{ij11}^{V8,LR} - \frac{40}{3} L_{ij22}^{V8,LR} \\
& + \frac{2}{3} L_{ijii}^{V8,LR} + \frac{2}{3} L_{ijjj}^{V8,LR} + \frac{8}{3} L_{ijii}^{V,LL} + \frac{8}{3} L_{ijjj}^{V,LL} \Big] + \frac{8}{3} e^2 L_{ij22}^{V8,LR} + \alpha_s^2 \Big[ - \frac{2}{3} L_{ij11}^{V1,LL} \\
& - \frac{2}{3} L_{ij22}^{V1,LL} - \frac{22}{3} L_{ij11}^{V1,LR} - 132 L_{ij22}^{V1,LR} + \frac{619}{81} L_{ij11}^{V8,LL} + \frac{619}{81} L_{ij22}^{V8,LL} + \frac{799}{81} L_{ij11}^{V8,LR} \\
& + \frac{799}{81} L_{ij22}^{V8,LR} \Big]
\end{aligned}$$

$$\begin{aligned}
& -\frac{25177}{162}L_{ud\ ij22}^{V8,LR} - \frac{22}{3}L_{uu\ ijii}^{V1,LR} - \frac{22}{3}L_{uu\ ijjj}^{V1,LR} + \frac{799}{81}L_{uu\ ijii}^{V8,LR} + \frac{799}{81}L_{uu\ ijjj}^{V8,LR} + \frac{1210}{27}L_{uu\ ijii}^{V,LL} \\
& + \frac{1210}{27}L_{uu\ ijjj}^{V,LL} \Big] + \alpha_s \alpha \Bigg[ \frac{668}{81}L_{eu\ 11ij}^{V,LL} + \frac{668}{81}L_{eu\ 22ij}^{V,LL} + \frac{668}{81}L_{eu\ 33ij}^{V,LL} + \frac{668}{81}L_{ud\ ij11}^{V1,LL} \\
& + \frac{668}{81}L_{ud\ ij22}^{V1,LL} + \frac{668}{81}L_{ud\ ij11}^{V1,LR} + \frac{3800}{81}L_{ud\ ij22}^{V1,LR} - \frac{70}{27}L_{ud\ ij11}^{V8,LL} - \frac{70}{27}L_{ud\ ij22}^{V8,LL} + \frac{14}{9}L_{ud\ ij11}^{V8,LR} \\
& + \frac{67}{3}L_{ud\ ij22}^{V8,LR} + \frac{668}{81}L_{ue\ ij11}^{V,LR} + \frac{668}{81}L_{ue\ ij22}^{V,LR} + \frac{668}{81}L_{ue\ ij33}^{V,LR} - \frac{1336}{81}L_{uu\ ijii}^{V1,LR} - \frac{1336}{81}L_{uu\ ijjj}^{V1,LR} \\
& - \frac{20}{3}L_{uu\ ijii}^{V8,LR} - \frac{20}{3}L_{uu\ ijjj}^{V8,LR} - \frac{3800}{81}L_{uu\ ijii}^{V,LL} - \frac{3800}{81}L_{uu\ ijjj}^{V,LL} \Big] - \frac{3872}{81}\alpha^2 L_{ud\ ij22}^{V8,LR} ; \\
\dot{L}_{uu\ ijjj}^{V1,LR} = & -\frac{8}{3}g_s^2 L_{uu\ ijjj}^{V8,LR} + e^2 \Bigg[ -\frac{8}{9}L_{eu\ 11ij}^{V,LL} - \frac{8}{9}L_{eu\ 22ij}^{V,LL} - \frac{8}{9}L_{eu\ 33ij}^{V,LL} - \frac{8}{9}L_{ud\ ij11}^{V1,LL} \\
& - \frac{8}{9}L_{ud\ ij22}^{V1,LL} - \frac{8}{9}L_{ud\ ij11}^{V1,LR} - \frac{8}{9}L_{ud\ ij22}^{V1,LR} - \frac{8}{9}L_{ue\ ij11}^{V,LR} - \frac{8}{9}L_{ue\ ij22}^{V,LR} - \frac{8}{9}L_{ue\ ij33}^{V,LR} \\
& + \frac{16}{9}L_{uu\ ijii}^{V1,LR} - \frac{32}{9}L_{uu\ ijjj}^{V1,LR} + \frac{128}{27}L_{uu\ ijii}^{V,LL} + \frac{128}{27}L_{uu\ ijjj}^{V,LL} \Big] + \alpha_s^2 \Bigg[ -8L_{ud\ ij11}^{V1,LL} \\
& - 8L_{ud\ ij22}^{V1,LL} + 8L_{ud\ ij11}^{V1,LR} + 8L_{ud\ ij22}^{V1,LR} + \frac{44}{27}L_{ud\ ij11}^{V8,LL} + \frac{44}{27}L_{ud\ ij22}^{V8,LL} + \frac{44}{27}L_{ud\ ij11}^{V8,LR} \\
& + \frac{44}{27}L_{ud\ ij22}^{V8,LR} + 8L_{uu\ ijii}^{V1,LR} - \frac{4}{3}L_{uu\ ijjj}^{V1,LR} + \frac{44}{27}L_{uu\ ijii}^{V8,LR} - \frac{2000}{27}L_{uu\ ijjj}^{V8,LR} - \frac{232}{9}L_{uu\ ijii}^{V,LL} \\
& - \frac{232}{9}L_{uu\ ijjj}^{V,LL} \Big] + \alpha_s \alpha \Bigg[ -\frac{32}{9}L_{ud\ ij11}^{V1,LL} - \frac{32}{9}L_{ud\ ij22}^{V1,LL} - \frac{32}{9}L_{ud\ ij11}^{V1,LR} - \frac{32}{9}L_{ud\ ij22}^{V1,LR} \\
& - \frac{656}{729}L_{ud\ ij11}^{V8,LL} - \frac{656}{729}L_{ud\ ij22}^{V8,LL} + \frac{784}{729}L_{ud\ ij11}^{V8,LR} + \frac{784}{729}L_{ud\ ij22}^{V8,LR} + \frac{64}{9}L_{uu\ ijii}^{V1,LR} \\
& + \frac{448}{9}L_{uu\ ijjj}^{V1,LR} - \frac{3968}{729}L_{uu\ ijii}^{V8,LR} - \frac{4832}{729}L_{uu\ ijjj}^{V8,LR} + \frac{4480}{243}L_{uu\ ijii}^{V,LL} + \frac{4480}{243}L_{uu\ ijjj}^{V,LL} \Big] \\
& + \alpha^2 \Bigg[ -\frac{8344}{729}L_{eu\ 11ij}^{V,LL} - \frac{8344}{729}L_{eu\ 22ij}^{V,LL} - \frac{8344}{729}L_{eu\ 33ij}^{V,LL} - \frac{3736}{729}L_{ud\ ij11}^{V1,LL} - \frac{3736}{729}L_{ud\ ij22}^{V1,LL} \\
& - \frac{2584}{729}L_{ud\ ij11}^{V1,LR} - \frac{2584}{729}L_{ud\ ij22}^{V1,LR} - \frac{4888}{729}L_{ue\ ij11}^{V,LR} - \frac{4888}{729}L_{ue\ ij22}^{V,LR} - \frac{4888}{729}L_{ue\ ij33}^{V,LR} \\
& + \frac{4736}{729}L_{uu\ ijii}^{V1,LR} + \frac{69248}{729}L_{uu\ ijjj}^{V1,LR} - \frac{9728}{729}L_{uu\ ijii}^{V,LL} - \frac{9728}{729}L_{uu\ ijjj}^{V,LL} \Big] ;
\end{aligned}$$

$$\begin{aligned}
\dot{L}_{ijjj}^{V8,LR} = & g_s^2 \left[ \frac{2}{3} L_{ij11}^{V8,LL} + \frac{2}{3} L_{ij22}^{V8,LL} + \frac{2}{3} L_{ij11}^{V8,LR} + \frac{2}{3} L_{ij22}^{V8,LR} - 12 L_{ijjj}^{V1,LR} \right. \\
& + \frac{2}{3} L_{ijii}^{V8,LR} - \frac{40}{3} L_{ijjj}^{V8,LR} + \frac{8}{3} L_{ijii}^{V,LL} + \frac{8}{3} L_{ijjj}^{V,LL} \left. \right] - \frac{16}{3} e^2 L_{ijjj}^{V8,LR} + \alpha_s^2 \left[ -\frac{2}{3} L_{ij11}^{V1,LL} \right. \\
& - \frac{2}{3} L_{ij22}^{V1,LL} - \frac{22}{3} L_{ij11}^{V1,LR} - \frac{22}{3} L_{ij22}^{V1,LR} + \frac{619}{81} L_{ij11}^{V8,LL} + \frac{619}{81} L_{ij22}^{V8,LL} + \frac{799}{81} L_{ij11}^{V8,LR} \\
& + \frac{799}{81} L_{ij22}^{V8,LR} - \frac{22}{3} L_{ijii}^{V1,LR} - 132 L_{ijjj}^{V1,LR} + \frac{799}{81} L_{ijii}^{V8,LR} - \frac{25177}{162} L_{ijjj}^{V8,LR} + \frac{1210}{27} L_{ijii}^{V,LL} \\
& + \frac{1210}{27} L_{ijjj}^{V,LL} \left. \right] + \alpha_s \alpha \left[ -\frac{520}{81} L_{11ij}^{V,LL} - \frac{520}{81} L_{22ij}^{V,LL} - \frac{520}{81} L_{33ij}^{V,LL} - \frac{520}{81} L_{ij11}^{V1,LL} \right. \\
& - \frac{520}{81} L_{ij22}^{V1,LL} - \frac{520}{81} L_{ij11}^{V1,LR} - \frac{520}{81} L_{ij22}^{V1,LR} + \frac{170}{27} L_{ij11}^{V8,LL} + \frac{170}{27} L_{ij22}^{V8,LL} + \frac{22}{9} L_{ij11}^{V8,LR} \\
& + \frac{22}{9} L_{ij22}^{V8,LR} - \frac{520}{81} L_{ij11}^{V,LR} - \frac{520}{81} L_{ij22}^{V,LR} - \frac{520}{81} L_{ij33}^{V,LR} + \frac{1040}{81} L_{ijii}^{V1,LR} + \frac{608}{81} L_{ijjj}^{V1,LR} \\
& + \frac{56}{9} L_{ijii}^{V8,LR} - \frac{16}{3} L_{ijjj}^{V8,LR} + \frac{1168}{81} L_{ijii}^{V,LL} + \frac{1168}{81} L_{ijjj}^{V,LL} \left. \right] + \frac{7168}{81} \alpha^2 L_{ijjj}^{V8,LR} ;
\end{aligned}$$

$$\begin{aligned}
\dot{L}_{ijii}^{V1,LR} = & -\frac{8}{3} g_s^2 L_{ijii}^{V8,LR} + e^2 \left[ -\frac{8}{9} L_{11ij}^{V,LL} - \frac{8}{9} L_{22ij}^{V,LL} - \frac{8}{9} L_{33ij}^{V,LL} - \frac{8}{9} L_{ij11}^{V1,LL} \right. \\
& - \frac{8}{9} L_{ij22}^{V1,LL} - \frac{8}{9} L_{ij11}^{V1,LR} - \frac{8}{9} L_{ij22}^{V1,LR} - \frac{8}{9} L_{ij11}^{V,LR} - \frac{8}{9} L_{ij22}^{V,LR} - \frac{8}{9} L_{ij33}^{V,LR} \\
& - \frac{32}{9} L_{ijii}^{V1,LR} + \frac{16}{9} L_{ijjj}^{V1,LR} + \frac{128}{27} L_{ijii}^{V,LL} + \frac{128}{27} L_{ijjj}^{V,LL} \left. \right] + \alpha_s^2 \left[ -8 L_{ij11}^{V1,LL} \right. \\
& - 8 L_{ij22}^{V1,LL} + 8 L_{ij11}^{V1,LR} + 8 L_{ij22}^{V1,LR} + \frac{44}{27} L_{ij11}^{V8,LL} + \frac{44}{27} L_{ij22}^{V8,LL} + \frac{44}{27} L_{ij11}^{V8,LR} \\
& + \frac{44}{27} L_{ij22}^{V8,LR} - \frac{4}{3} L_{ijii}^{V1,LR} + 8 L_{ijjj}^{V1,LR} - \frac{2000}{27} L_{ijii}^{V8,LR} + \frac{44}{27} L_{ijjj}^{V8,LR} - \frac{232}{9} L_{ijii}^{V,LL} \\
& - \frac{232}{9} L_{ijjj}^{V,LL} \left. \right] + \alpha_s \alpha \left[ -\frac{32}{9} L_{ij11}^{V1,LL} - \frac{32}{9} L_{ij22}^{V1,LL} - \frac{32}{9} L_{ij11}^{V1,LR} - \frac{32}{9} L_{ij22}^{V1,LR} \right. \\
& - \frac{656}{729} L_{ij11}^{V8,LL} - \frac{656}{729} L_{ij22}^{V8,LL} + \frac{784}{729} L_{ij11}^{V8,LR} + \frac{784}{729} L_{ij22}^{V8,LR} + \frac{448}{9} L_{ijii}^{V1,LR} \\
& + \frac{64}{9} L_{ijjj}^{V1,LR} - \frac{4832}{729} L_{ijii}^{V8,LR} - \frac{3968}{729} L_{ijjj}^{V8,LR} + \frac{4480}{243} L_{ijii}^{V,LL} + \frac{4480}{243} L_{ijjj}^{V,LL} \left. \right]
\end{aligned}$$

$$\begin{aligned}
& + \alpha^2 \left[ -\frac{8344}{729} L_{11ij}^{V,LL} - \frac{8344}{729} L_{22ij}^{V,LL} - \frac{8344}{729} L_{33ij}^{V,LL} - \frac{3736}{729} L_{ij11}^{V1,LL} - \frac{3736}{729} L_{ij22}^{V1,LL} \right. \\
& - \frac{2584}{729} L_{ij11}^{V1,LR} - \frac{2584}{729} L_{ij22}^{V1,LR} - \frac{4888}{729} L_{ij11}^{V,LR} - \frac{4888}{729} L_{ij22}^{V,LR} - \frac{4888}{729} L_{ij33}^{V,LR} \\
& \left. + \frac{69248}{729} L_{ijii}^{V1,LR} + \frac{4736}{729} L_{ijjj}^{V1,LR} - \frac{9728}{729} L_{ijii}^{V,LL} - \frac{9728}{729} L_{ijjj}^{V,LL} \right];
\end{aligned}$$

$$\begin{aligned}
\dot{L}_{ijii}^{V8,LR} = & g_s^2 \left[ \frac{2}{3} L_{ij11}^{V8,LL} + \frac{2}{3} L_{ij22}^{V8,LL} + \frac{2}{3} L_{ij11}^{V8,LR} + \frac{2}{3} L_{ij22}^{V8,LR} - 12 L_{ijii}^{V1,LR} \right. \\
& - \frac{40}{3} L_{ijii}^{V8,LR} + \frac{2}{3} L_{ijjj}^{V8,LR} + \frac{8}{3} L_{ijii}^{V,LL} + \frac{8}{3} L_{ijjj}^{V,LL} \left. \right] - \frac{16}{3} e^2 L_{ijii}^{V8,LR} + \alpha_s^2 \left[ -\frac{2}{3} L_{ij11}^{V1,LL} \right. \\
& - \frac{2}{3} L_{ij22}^{V1,LL} - \frac{22}{3} L_{ij11}^{V1,LR} - \frac{22}{3} L_{ij22}^{V1,LR} + \frac{619}{81} L_{ij11}^{V8,LL} + \frac{619}{81} L_{ij22}^{V8,LL} + \frac{799}{81} L_{ij11}^{V8,LR} \\
& + \frac{799}{81} L_{ij22}^{V8,LR} - 132 L_{ijii}^{V1,LR} - \frac{22}{3} L_{ijjj}^{V1,LR} - \frac{25177}{162} L_{ijii}^{V8,LR} + \frac{799}{81} L_{ijjj}^{V8,LR} + \frac{1210}{27} L_{ijii}^{V,LL} \\
& \left. + \frac{1210}{27} L_{ijjj}^{V,LL} \right] + \alpha_s \alpha \left[ -\frac{520}{81} L_{11ij}^{V,LL} - \frac{520}{81} L_{22ij}^{V,LL} - \frac{520}{81} L_{33ij}^{V,LL} - \frac{520}{81} L_{ij11}^{V1,LL} \right. \\
& - \frac{520}{81} L_{ij22}^{V1,LL} - \frac{520}{81} L_{ij11}^{V1,LR} - \frac{520}{81} L_{ij22}^{V1,LR} + \frac{170}{27} L_{ij11}^{V8,LL} + \frac{170}{27} L_{ij22}^{V8,LL} + \frac{22}{9} L_{ij11}^{V8,LR} \\
& + \frac{22}{9} L_{ij22}^{V8,LR} - \frac{520}{81} L_{ij11}^{V,LR} - \frac{520}{81} L_{ij22}^{V,LR} - \frac{520}{81} L_{ij33}^{V,LR} + \frac{608}{81} L_{ijii}^{V1,LR} + \frac{1040}{81} L_{ijjj}^{V1,LR} \\
& \left. - \frac{16}{3} L_{ijii}^{V8,LR} + \frac{56}{9} L_{ijjj}^{V8,LR} + \frac{1168}{81} L_{ijii}^{V,LL} + \frac{1168}{81} L_{ijjj}^{V,LL} \right] + \frac{7168}{81} \alpha^2 L_{ijii}^{V8,LR};
\end{aligned}$$

$$\begin{aligned}
\dot{L}_{11ij}^{S,RL} = & -8g_s^2 L_{11ij}^{S,RL} - \frac{26}{3} e^2 L_{11ij}^{S,RL} - \frac{1012}{9} \alpha_s^2 L_{11ij}^{S,RL} - \frac{32}{9} \alpha_s \alpha L_{11ij}^{S,RL} \\
& + \frac{473}{81} \alpha^2 L_{11ij}^{S,RL};
\end{aligned}$$

$$\begin{aligned}
\dot{L}_{22ij}^{S,RL} = & -8g_s^2 L_{22ij}^{S,RL} - \frac{26}{3} e^2 L_{22ij}^{S,RL} - \frac{1012}{9} \alpha_s^2 L_{22ij}^{S,RL} - \frac{32}{9} \alpha_s \alpha L_{22ij}^{S,RL} \\
& + \frac{473}{81} \alpha^2 L_{22ij}^{S,RL};
\end{aligned}$$

$$\begin{aligned}
\dot{L}_{33ij}^{S,RL} = & -8g_s^2 L_{33ij}^{S,RL} - \frac{26}{3} e^2 L_{33ij}^{S,RL} - \frac{1012}{9} \alpha_s^2 L_{33ij}^{S,RL} - \frac{32}{9} \alpha_s \alpha L_{33ij}^{S,RL} \\
& + \frac{473}{81} \alpha^2 L_{33ij}^{S,RL};
\end{aligned}$$

$$\begin{aligned}
\dot{L}_{i11j}^{V1,LR} &= -\frac{8}{3}g_s^2 L_{i11j}^{V8,LR} - \frac{10}{3}e^2 L_{i11j}^{V1,LR} + \alpha_s^2 \left[ -\frac{28}{3}L_{i11j}^{V1,LR} - \frac{2044}{27}L_{i11j}^{V8,LR} \right] \\
&\quad + \alpha_s \alpha \left[ \frac{8}{3}L_{i11j}^{V1,LR} - \frac{128}{27}L_{i11j}^{V8,LR} \right] + \frac{169}{81}\alpha^2 L_{i11j}^{V1,LR} ; \\
\dot{L}_{i11j}^{V8,LR} &= g_s^2 \left[ -12L_{i11j}^{V1,LR} - 14L_{i11j}^{V8,LR} \right] - \frac{10}{3}e^2 L_{i11j}^{V8,LR} + \alpha_s^2 \left[ -\frac{374}{3}L_{i11j}^{V1,LR} \right. \\
&\quad \left. - \frac{2975}{18}L_{i11j}^{V8,LR} \right] + \alpha_s \alpha \left[ \frac{16}{9}L_{i11j}^{V8,LR} - \frac{64}{3}L_{i11j}^{V1,LR} \right] + \frac{169}{81}\alpha^2 L_{i11j}^{V8,LR} ; \\
\dot{L}_{i22j}^{V1,LR} &= -\frac{8}{3}g_s^2 L_{i22j}^{V8,LR} - \frac{10}{3}e^2 L_{i22j}^{V1,LR} + \alpha_s^2 \left[ -\frac{28}{3}L_{i22j}^{V1,LR} - \frac{2044}{27}L_{i22j}^{V8,LR} \right] \\
&\quad + \alpha_s \alpha \left[ \frac{8}{3}L_{i22j}^{V1,LR} - \frac{128}{27}L_{i22j}^{V8,LR} \right] + \frac{169}{81}\alpha^2 L_{i22j}^{V1,LR} ; \\
\dot{L}_{i22j}^{V8,LR} &= g_s^2 \left[ -12L_{i22j}^{V1,LR} - 14L_{i22j}^{V8,LR} \right] - \frac{10}{3}e^2 L_{i22j}^{V8,LR} + \alpha_s^2 \left[ -\frac{374}{3}L_{i22j}^{V1,LR} \right. \\
&\quad \left. - \frac{2975}{18}L_{i22j}^{V8,LR} \right] + \alpha_s \alpha \left[ \frac{16}{9}L_{i22j}^{V8,LR} - \frac{64}{3}L_{i22j}^{V1,LR} \right] + \frac{169}{81}\alpha^2 L_{i22j}^{V8,LR} ; \\
\dot{L}_{11ij}^{S,RR} &= -8g_s^2 L_{11ij}^{S,RR} + e^2 \left[ 64L_{11ij}^{T,RR} - \frac{26}{3}L_{11ij}^{S,RR} \right] - \frac{1012}{9}\alpha_s^2 L_{11ij}^{S,RR} \\
&\quad + \alpha_s \alpha \left[ -\frac{32}{9}L_{11ij}^{S,RR} - \frac{3584}{9}L_{11ij}^{T,RR} \right] + \alpha^2 \left[ -\frac{2839}{81}L_{11ij}^{S,RR} - \frac{11264}{9}L_{11ij}^{T,RR} \right] ; \\
\dot{L}_{11ij}^{T,RR} &= \frac{8}{3}g_s^2 L_{11ij}^{T,RR} + e^2 \left[ \frac{4}{3}L_{11ij}^{S,RR} + \frac{26}{9}L_{11ij}^{T,RR} \right] + \frac{1652}{27}\alpha_s^2 L_{11ij}^{T,RR} \\
&\quad + \alpha_s \alpha \left[ -\frac{32}{3}L_{11ij}^{S,RR} - \frac{608}{27}L_{11ij}^{T,RR} \right] + \alpha^2 \left[ -\frac{1376}{81}L_{11ij}^{S,RR} - \frac{20677}{243}L_{11ij}^{T,RR} \right] ; \\
\dot{L}_{22ij}^{S,RR} &= -8g_s^2 L_{22ij}^{S,RR} + e^2 \left[ 64L_{22ij}^{T,RR} - \frac{26}{3}L_{22ij}^{S,RR} \right] - \frac{1012}{9}\alpha_s^2 L_{22ij}^{S,RR} \\
&\quad + \alpha_s \alpha \left[ -\frac{32}{9}L_{22ij}^{S,RR} - \frac{3584}{9}L_{22ij}^{T,RR} \right] + \alpha^2 \left[ -\frac{2839}{81}L_{22ij}^{S,RR} - \frac{11264}{9}L_{22ij}^{T,RR} \right] ;
\end{aligned}$$

$$\begin{aligned}
\dot{L}_{22ij}^{T,RR} &= \frac{8}{3}g_s^2 L_{22ij}^{T,RR} + e^2 \left[ \frac{4}{3}L_{22ij}^{S,RR} + \frac{26}{9}L_{22ij}^{T,RR} \right] + \frac{1652}{27}\alpha_s^2 L_{22ij}^{T,RR} \\
&\quad + \alpha_s \alpha \left[ -\frac{32}{3}L_{22ij}^{S,RR} - \frac{608}{27}L_{22ij}^{T,RR} \right] + \alpha^2 \left[ -\frac{1376}{81}L_{22ij}^{S,RR} - \frac{20677}{243}L_{22ij}^{T,RR} \right]; \\
\dot{L}_{33ij}^{S,RR} &= -8g_s^2 L_{33ij}^{S,RR} + e^2 \left[ 64L_{33ij}^{T,RR} - \frac{26}{3}L_{33ij}^{S,RR} \right] - \frac{1012}{9}\alpha_s^2 L_{33ij}^{S,RR} \\
&\quad + \alpha_s \alpha \left[ -\frac{32}{9}L_{33ij}^{S,RR} - \frac{3584}{9}L_{33ij}^{T,RR} \right] + \alpha^2 \left[ -\frac{2839}{81}L_{33ij}^{S,RR} - \frac{11264}{9}L_{33ij}^{T,RR} \right]; \\
\dot{L}_{33ij}^{T,RR} &= \frac{8}{3}g_s^2 L_{33ij}^{T,RR} + e^2 \left[ \frac{4}{3}L_{33ij}^{S,RR} + \frac{26}{9}L_{33ij}^{T,RR} \right] + \frac{1652}{27}\alpha_s^2 L_{33ij}^{T,RR} \\
&\quad + \alpha_s \alpha \left[ -\frac{32}{3}L_{33ij}^{S,RR} - \frac{608}{27}L_{33ij}^{T,RR} \right] + \alpha^2 \left[ -\frac{1376}{81}L_{33ij}^{S,RR} - \frac{20677}{243}L_{33ij}^{T,RR} \right]; \\
\dot{L}_{ij11}^{S1,RR} &= g_s^2 \left[ \frac{64}{9}L_{i11j}^{S1,RR} + \frac{112}{27}L_{i11j}^{S8,RR} - 16L_{ij11}^{S1,RR} + \frac{16}{9}L_{ij11}^{S8,RR} \right] \\
&\quad + e^2 \left[ \frac{4}{27}L_{i11j}^{S1,RR} + \frac{16}{81}L_{i11j}^{S8,RR} - \frac{46}{9}L_{ij11}^{S1,RR} \right] + \alpha_s^2 \left[ \frac{9472}{81}L_{i11j}^{S1,RR} + \frac{16576}{243}L_{i11j}^{S8,RR} \right. \\
&\quad \left. - \frac{2120}{9}L_{ij11}^{S1,RR} + \frac{928}{81}L_{ij11}^{S8,RR} \right] + \alpha_s \alpha \left[ \frac{1888}{81}L_{i11j}^{S1,RR} + \frac{3808}{243}L_{i11j}^{S8,RR} + \frac{136}{27}L_{ij11}^{S1,RR} \right. \\
&\quad \left. + \frac{224}{81}L_{ij11}^{S8,RR} \right] + \alpha^2 \left[ \frac{106}{729}L_{i11j}^{S1,RR} + \frac{424}{2187}L_{i11j}^{S8,RR} + \frac{6059}{243}L_{ij11}^{S1,RR} \right]; \\
\dot{L}_{ij11}^{S8,RR} &= g_s^2 \left[ -\frac{16}{3}L_{i11j}^{S1,RR} + \frac{44}{9}L_{i11j}^{S8,RR} + 8L_{ij11}^{S1,RR} + \frac{16}{3}L_{ij11}^{S8,RR} \right] \\
&\quad + e^2 \left[ \frac{8}{9}L_{i11j}^{S1,RR} - \frac{4}{27}L_{i11j}^{S8,RR} - \frac{46}{9}L_{ij11}^{S8,RR} \right] + \alpha_s^2 \left[ -\frac{856}{27}L_{i11j}^{S1,RR} - \frac{2506}{81}L_{i11j}^{S8,RR} \right. \\
&\quad \left. + \frac{248}{9}L_{ij11}^{S1,RR} + \frac{2995}{27}L_{ij11}^{S8,RR} \right] + \alpha_s \alpha \left[ -\frac{868}{27}L_{i11j}^{S1,RR} + \frac{1370}{81}L_{i11j}^{S8,RR} + \frac{112}{9}L_{ij11}^{S1,RR} \right. \\
&\quad \left. + \frac{224}{9}L_{ij11}^{S8,RR} \right] + \alpha^2 \left[ \frac{212}{243}L_{i11j}^{S1,RR} - \frac{106}{729}L_{i11j}^{S8,RR} + \frac{6059}{243}L_{ij11}^{S8,RR} \right];
\end{aligned}$$

$$\begin{aligned}
\dot{L}_{uddu\ i11j}^{S1,RR} = & g_s^2 \left[ -16L_{uddu\ i11j}^{S1,RR} + \frac{16}{9}L_{uddu\ i11j}^{S8,RR} + \frac{64}{9}L_{ud\ ij11}^{S1,RR} + \frac{112}{27}L_{ud\ ij11}^{S8,RR} \right] \\
& + e^2 \left[ \frac{26}{9}L_{uddu\ i11j}^{S1,RR} - \frac{32}{27}L_{ud\ ij11}^{S1,RR} - \frac{128}{81}L_{ud\ ij11}^{S8,RR} \right] + \alpha_s^2 \left[ -\frac{2120}{9}L_{uddu\ i11j}^{S1,RR} + \frac{928}{81}L_{uddu\ i11j}^{S8,RR} \right. \\
& + \frac{9472}{81}L_{ud\ ij11}^{S1,RR} + \frac{16576}{243}L_{ud\ ij11}^{S8,RR} \left. \right] + \alpha_s \alpha \left[ \frac{712}{27}L_{uddu\ i11j}^{S1,RR} - \frac{64}{81}L_{uddu\ i11j}^{S8,RR} - \frac{2144}{81}L_{ud\ ij11}^{S1,RR} \right. \\
& \left. - \frac{7784}{243}L_{ud\ ij11}^{S8,RR} \right] + \alpha^2 \left[ -\frac{13201}{243}L_{uddu\ i11j}^{S1,RR} + \frac{5200}{729}L_{ud\ ij11}^{S1,RR} + \frac{20800}{2187}L_{ud\ ij11}^{S8,RR} \right];
\end{aligned}$$

$$\begin{aligned}
\dot{L}_{uddu\ i11j}^{S8,RR} = & g_s^2 \left[ 8L_{uddu\ i11j}^{S1,RR} + \frac{16}{3}L_{uddu\ i11j}^{S8,RR} - \frac{16}{3}L_{ud\ ij11}^{S1,RR} + \frac{44}{9}L_{ud\ ij11}^{S8,RR} \right] \\
& + e^2 \left[ \frac{26}{9}L_{uddu\ i11j}^{S8,RR} - \frac{64}{9}L_{ud\ ij11}^{S1,RR} + \frac{32}{27}L_{ud\ ij11}^{S8,RR} \right] + \alpha_s^2 \left[ \frac{248}{9}L_{uddu\ i11j}^{S1,RR} + \frac{2995}{27}L_{uddu\ i11j}^{S8,RR} \right. \\
& \left. - \frac{856}{27}L_{ud\ ij11}^{S1,RR} - \frac{2506}{81}L_{ud\ ij11}^{S8,RR} \right] + \alpha_s \alpha \left[ -\frac{32}{9}L_{uddu\ i11j}^{S1,RR} - \frac{400}{9}L_{uddu\ i11j}^{S8,RR} + \frac{3704}{27}L_{ud\ ij11}^{S1,RR} \right. \\
& \left. - \frac{2050}{81}L_{ud\ ij11}^{S8,RR} \right] + \alpha^2 \left[ -\frac{13201}{243}L_{uddu\ i11j}^{S8,RR} + \frac{10400}{243}L_{ud\ ij11}^{S1,RR} - \frac{5200}{729}L_{ud\ ij11}^{S8,RR} \right];
\end{aligned}$$

$$\begin{aligned}
\dot{L}_{ud\ ij22}^{S1,RR} = & g_s^2 \left[ \frac{64}{9}L_{uddu\ i22j}^{S1,RR} + \frac{112}{27}L_{uddu\ i22j}^{S8,RR} - 16L_{ud\ ij22}^{S1,RR} + \frac{16}{9}L_{ud\ ij22}^{S8,RR} \right] \\
& + e^2 \left[ \frac{4}{27}L_{uddu\ i22j}^{S1,RR} + \frac{16}{81}L_{uddu\ i22j}^{S8,RR} - \frac{46}{9}L_{ud\ ij22}^{S1,RR} \right] + \alpha_s^2 \left[ \frac{9472}{81}L_{uddu\ i22j}^{S1,RR} + \frac{16576}{243}L_{uddu\ i22j}^{S8,RR} \right. \\
& \left. - \frac{2120}{9}L_{ud\ ij22}^{S1,RR} + \frac{928}{81}L_{ud\ ij22}^{S8,RR} \right] + \alpha_s \alpha \left[ \frac{1888}{81}L_{uddu\ i22j}^{S1,RR} + \frac{3808}{243}L_{uddu\ i22j}^{S8,RR} + \frac{136}{27}L_{ud\ ij22}^{S1,RR} \right. \\
& \left. + \frac{224}{81}L_{ud\ ij22}^{S8,RR} \right] + \alpha^2 \left[ \frac{106}{729}L_{uddu\ i22j}^{S1,RR} + \frac{424}{2187}L_{uddu\ i22j}^{S8,RR} + \frac{6059}{243}L_{ud\ ij22}^{S1,RR} \right];
\end{aligned}$$

$$\begin{aligned}
\dot{L}_{ud\ ij22}^{S8,RR} = & g_s^2 \left[ -\frac{16}{3}L_{uddu\ i22j}^{S1,RR} + \frac{44}{9}L_{uddu\ i22j}^{S8,RR} + 8L_{ud\ ij22}^{S1,RR} + \frac{16}{3}L_{ud\ ij22}^{S8,RR} \right] \\
& + e^2 \left[ \frac{8}{9}L_{uddu\ i22j}^{S1,RR} - \frac{4}{27}L_{uddu\ i22j}^{S8,RR} - \frac{46}{9}L_{ud\ ij22}^{S8,RR} \right] + \alpha_s^2 \left[ -\frac{856}{27}L_{uddu\ i22j}^{S1,RR} - \frac{2506}{81}L_{uddu\ i22j}^{S8,RR} \right]
\end{aligned}$$

$$\begin{aligned}
& + \frac{248}{9} L_{ij22}^{S1,RR} + \frac{2995}{27} L_{ij22}^{S8,RR} \Big] + \alpha_s \alpha \Big[ - \frac{868}{27} L_{i22j}^{S1,RR} + \frac{1370}{81} L_{i22j}^{S8,RR} + \frac{112}{9} L_{ij22}^{S1,RR} \\
& + \frac{224}{9} L_{ij22}^{S8,RR} \Big] + \alpha^2 \Big[ \frac{212}{243} L_{i22j}^{S1,RR} - \frac{106}{729} L_{i22j}^{S8,RR} + \frac{6059}{243} L_{ij22}^{S8,RR} \Big] ; \\
\dot{L}_{i22j}^{S1,RR} & = g_s^2 \Big[ -16 L_{i22j}^{S1,RR} + \frac{16}{9} L_{i22j}^{S8,RR} + \frac{64}{9} L_{ij22}^{S1,RR} + \frac{112}{27} L_{ij22}^{S8,RR} \Big] \\
& + e^2 \Big[ \frac{26}{9} L_{i22j}^{S1,RR} - \frac{32}{27} L_{ij22}^{S1,RR} - \frac{128}{81} L_{ij22}^{S8,RR} \Big] + \alpha_s^2 \Big[ - \frac{2120}{9} L_{i22j}^{S1,RR} + \frac{928}{81} L_{i22j}^{S8,RR} \\
& + \frac{9472}{81} L_{ij22}^{S1,RR} + \frac{16576}{243} L_{ij22}^{S8,RR} \Big] + \alpha_s \alpha \Big[ \frac{712}{27} L_{i22j}^{S1,RR} - \frac{64}{81} L_{i22j}^{S8,RR} - \frac{2144}{81} L_{ij22}^{S1,RR} \\
& - \frac{7784}{243} L_{ij22}^{S8,RR} \Big] + \alpha^2 \Big[ - \frac{13201}{243} L_{i22j}^{S1,RR} + \frac{5200}{729} L_{ij22}^{S1,RR} + \frac{20800}{2187} L_{ij22}^{S8,RR} \Big] ; \\
\dot{L}_{i22j}^{S8,RR} & = g_s^2 \Big[ 8 L_{i22j}^{S1,RR} + \frac{16}{3} L_{i22j}^{S8,RR} - \frac{16}{3} L_{ij22}^{S1,RR} + \frac{44}{9} L_{ij22}^{S8,RR} \Big] \\
& + e^2 \Big[ \frac{26}{9} L_{i22j}^{S8,RR} - \frac{64}{9} L_{ij22}^{S1,RR} + \frac{32}{27} L_{ij22}^{S8,RR} \Big] + \alpha_s^2 \Big[ \frac{248}{9} L_{i22j}^{S1,RR} + \frac{2995}{27} L_{i22j}^{S8,RR} \\
& - \frac{856}{27} L_{ij22}^{S1,RR} - \frac{2506}{81} L_{ij22}^{S8,RR} \Big] + \alpha_s \alpha \Big[ - \frac{32}{9} L_{i22j}^{S1,RR} - \frac{400}{9} L_{i22j}^{S8,RR} + \frac{3704}{27} L_{ij22}^{S1,RR} \\
& - \frac{2050}{81} L_{ij22}^{S8,RR} \Big] + \alpha^2 \Big[ - \frac{13201}{243} L_{i22j}^{S8,RR} + \frac{10400}{243} L_{ij22}^{S1,RR} - \frac{5200}{729} L_{ij22}^{S8,RR} \Big] ; \\
\dot{L}_{ijjj}^{S1,RR} & = g_s^2 \Big[ \frac{160}{27} L_{ijjj}^{S8,RR} - \frac{80}{9} L_{ijjj}^{S1,RR} \Big] + e^2 \Big[ \frac{16}{27} L_{ijjj}^{S1,RR} + \frac{256}{81} L_{ijjj}^{S8,RR} \Big] \\
& + \alpha_s^2 \Big[ \frac{19360}{243} L_{ijjj}^{S8,RR} - \frac{9608}{81} L_{ijjj}^{S1,RR} \Big] + \alpha_s \alpha \Big[ \frac{1408}{243} L_{ijjj}^{S8,RR} - \frac{4160}{81} L_{ijjj}^{S1,RR} \Big] \\
& + \alpha^2 \Big[ \frac{5824}{729} L_{ijjj}^{S1,RR} - \frac{22016}{2187} L_{ijjj}^{S8,RR} \Big] ; \\
\dot{L}_{ijjj}^{S8,RR} & = g_s^2 \Big[ \frac{8}{3} L_{ijjj}^{S1,RR} + \frac{92}{9} L_{ijjj}^{S8,RR} \Big] + e^2 \Big[ \frac{128}{9} L_{ijjj}^{S1,RR} - \frac{112}{27} L_{ijjj}^{S8,RR} \Big]
\end{aligned}$$



$$\begin{aligned}
& + \alpha_s^2 \left[ \frac{6479}{81} L_{ijjj}^{S8,RR} - \frac{112}{27} L_{ijjj}^{S1,RR} \right] + \alpha_s \alpha \left[ -\frac{7360}{27} L_{ijjj}^{S1,RR} - \frac{832}{81} L_{ijjj}^{S8,RR} \right] \\
& + \alpha^2 \left[ \frac{16832}{729} L_{ijjj}^{S8,RR} - \frac{11008}{243} L_{ijjj}^{S1,RR} \right] ; \\
\dot{L}_{ijii}^{S1,RR} & = g_s^2 \left[ \frac{160}{27} L_{ijii}^{S8,RR} - \frac{80}{9} L_{ijii}^{S1,RR} \right] + e^2 \left[ \frac{16}{27} L_{ijii}^{S1,RR} + \frac{256}{81} L_{ijii}^{S8,RR} \right] \\
& + \alpha_s^2 \left[ \frac{19360}{243} L_{ijii}^{S8,RR} - \frac{9608}{81} L_{ijii}^{S1,RR} \right] + \alpha_s \alpha \left[ \frac{1408}{243} L_{ijii}^{S8,RR} - \frac{4160}{81} L_{ijii}^{S1,RR} \right] \\
& + \alpha^2 \left[ \frac{5824}{729} L_{ijii}^{S1,RR} - \frac{22016}{2187} L_{ijii}^{S8,RR} \right] ; \\
\dot{L}_{ijii}^{S8,RR} & = g_s^2 \left[ \frac{8}{3} L_{ijii}^{S1,RR} + \frac{92}{9} L_{ijii}^{S8,RR} \right] + e^2 \left[ \frac{128}{9} L_{ijii}^{S1,RR} - \frac{112}{27} L_{ijii}^{S8,RR} \right] \\
& + \alpha_s^2 \left[ \frac{6479}{81} L_{ijii}^{S8,RR} - \frac{112}{27} L_{ijii}^{S1,RR} \right] + \alpha_s \alpha \left[ -\frac{7360}{27} L_{ijii}^{S1,RR} - \frac{832}{81} L_{ijii}^{S8,RR} \right] \\
& + \alpha^2 \left[ \frac{16832}{729} L_{ijii}^{S8,RR} - \frac{11008}{243} L_{ijii}^{S1,RR} \right] ; \\
\dot{L}_{11ij}^{V,RR} & = e^2 \left[ \frac{4}{3} L_{11ij}^{V1,LR} + \frac{4}{3} L_{22ij}^{V1,LR} + \frac{4}{3} L_{11ij}^{V,LR} + \frac{4}{3} L_{22ij}^{V,LR} + \frac{4}{3} L_{33ij}^{V,LR} \right. \\
& - \frac{20}{3} L_{11ij}^{V,RR} + \frac{4}{3} L_{22ij}^{V,RR} + \frac{4}{3} L_{33ij}^{V,RR} + \frac{4}{3} L_{ij11}^{V1,RR} + \frac{4}{3} L_{ij22}^{V1,RR} - \frac{8}{3} L_{ijij}^{V1,LR} \\
& - \frac{8}{3} L_{jjij}^{V1,LR} - \frac{64}{9} L_{ijii}^{V,RR} - \frac{64}{9} L_{ijjj}^{V,RR} \left. \right] + \alpha_s \alpha \left[ \frac{16}{3} L_{11ij}^{V1,LR} + \frac{16}{3} L_{22ij}^{V1,LR} \right. \\
& - \frac{392}{243} L_{11ij}^{V8,LR} - \frac{392}{243} L_{22ij}^{V8,LR} + 32 L_{11ij}^{V,RR} + \frac{16}{3} L_{ij11}^{V1,RR} + \frac{16}{3} L_{ij22}^{V1,RR} + \frac{328}{243} L_{ij11}^{V8,RR} \\
& + \frac{328}{243} L_{ij22}^{V8,RR} - \frac{32}{3} L_{ijii}^{V1,LR} - \frac{32}{3} L_{jjij}^{V1,LR} + \frac{1984}{243} L_{ijii}^{V8,LR} + \frac{1984}{243} L_{jjij}^{V8,LR} \\
& - \frac{2240}{81} L_{ijii}^{V,RR} - \frac{2240}{81} L_{ijjj}^{V,RR} \left. \right] + \alpha^2 \left[ -\frac{832}{243} L_{11ij}^{V1,LR} - \frac{832}{243} L_{22ij}^{V1,LR} - \frac{328}{243} L_{11ij}^{V,LR} \right. \\
& - \frac{328}{243} L_{22ij}^{V,LR} - \frac{328}{243} L_{33ij}^{V,LR} + \frac{4496}{243} L_{11ij}^{V,RR} + \frac{3344}{243} L_{22ij}^{V,RR} + \frac{3344}{243} L_{33ij}^{V,RR}
\end{aligned}$$

$$\begin{aligned}
& + \frac{392}{243} L_{ij11}^{V1,RR} + \frac{392}{243} L_{ij22}^{V1,RR} - \frac{64}{243} L_{iijj}^{V1,LR} - \frac{64}{243} L_{jjij}^{V1,LR} + \frac{25888}{243} L_{iijj}^{V,RR} \\
& + \frac{25888}{243} L_{iijj}^{V,RR} \Big] ;
\end{aligned}$$

$$\begin{aligned}
\dot{L}_{22ij}^{V,RR} = & e^2 \left[ \frac{4}{3} L_{11ij}^{V1,LR} + \frac{4}{3} L_{22ij}^{V1,LR} + \frac{4}{3} L_{11ij}^{V,LR} + \frac{4}{3} L_{22ij}^{V,LR} + \frac{4}{3} L_{33ij}^{V,LR} \right. \\
& + \frac{4}{3} L_{11ij}^{V,RR} - \frac{20}{3} L_{22ij}^{V,RR} + \frac{4}{3} L_{33ij}^{V,RR} + \frac{4}{3} L_{ij11}^{V1,RR} + \frac{4}{3} L_{ij22}^{V1,RR} - \frac{8}{3} L_{iijj}^{V1,LR} \\
& - \frac{8}{3} L_{jjij}^{V1,LR} - \frac{64}{9} L_{iijj}^{V,RR} - \frac{64}{9} L_{jjij}^{V,RR} \Big] + \alpha_s \alpha \left[ \frac{16}{3} L_{11ij}^{V1,LR} + \frac{16}{3} L_{22ij}^{V1,LR} \right. \\
& - \frac{392}{243} L_{11ij}^{V8,LR} - \frac{392}{243} L_{22ij}^{V8,LR} + 32 L_{22ij}^{V,RR} + \frac{16}{3} L_{ij11}^{V1,RR} + \frac{16}{3} L_{ij22}^{V1,RR} + \frac{328}{243} L_{ij11}^{V8,RR} \\
& + \frac{328}{243} L_{ij22}^{V8,RR} - \frac{32}{3} L_{iijj}^{V1,LR} - \frac{32}{3} L_{jjij}^{V1,LR} + \frac{1984}{243} L_{iijj}^{V8,LR} + \frac{1984}{243} L_{jjij}^{V8,LR} \\
& - \frac{2240}{81} L_{iijj}^{V,RR} - \frac{2240}{81} L_{jjij}^{V,RR} \Big] + \alpha^2 \left[ - \frac{832}{243} L_{11ij}^{V1,LR} - \frac{832}{243} L_{22ij}^{V1,LR} - \frac{328}{243} L_{11ij}^{V,LR} \right. \\
& - \frac{328}{243} L_{22ij}^{V,LR} - \frac{328}{243} L_{33ij}^{V,LR} + \frac{3344}{243} L_{11ij}^{V,RR} + \frac{4496}{243} L_{22ij}^{V,RR} + \frac{3344}{243} L_{33ij}^{V,RR} \\
& + \frac{392}{243} L_{ij11}^{V1,RR} + \frac{392}{243} L_{ij22}^{V1,RR} - \frac{64}{243} L_{iijj}^{V1,LR} - \frac{64}{243} L_{jjij}^{V1,LR} + \frac{25888}{243} L_{iijj}^{V,RR} \\
& \left. + \frac{25888}{243} L_{jjij}^{V,RR} \right] ;
\end{aligned}$$

$$\begin{aligned}
\dot{L}_{33ij}^{V,RR} = & e^2 \left[ \frac{4}{3} L_{11ij}^{V1,LR} + \frac{4}{3} L_{22ij}^{V1,LR} + \frac{4}{3} L_{11ij}^{V,LR} + \frac{4}{3} L_{22ij}^{V,LR} + \frac{4}{3} L_{33ij}^{V,LR} \right. \\
& + \frac{4}{3} L_{11ij}^{V,RR} + \frac{4}{3} L_{22ij}^{V,RR} - \frac{20}{3} L_{33ij}^{V,RR} + \frac{4}{3} L_{ij11}^{V1,RR} + \frac{4}{3} L_{ij22}^{V1,RR} - \frac{8}{3} L_{iijj}^{V1,LR} \\
& - \frac{8}{3} L_{jjij}^{V1,LR} - \frac{64}{9} L_{iijj}^{V,RR} - \frac{64}{9} L_{jjij}^{V,RR} \Big] + \alpha_s \alpha \left[ \frac{16}{3} L_{11ij}^{V1,LR} + \frac{16}{3} L_{22ij}^{V1,LR} \right. \\
& - \frac{392}{243} L_{11ij}^{V8,LR} - \frac{392}{243} L_{22ij}^{V8,LR} + 32 L_{33ij}^{V,RR} + \frac{16}{3} L_{ij11}^{V1,RR} + \frac{16}{3} L_{ij22}^{V1,RR} + \frac{328}{243} L_{ij11}^{V8,RR} \\
& + \frac{328}{243} L_{ij22}^{V8,RR} - \frac{32}{3} L_{iijj}^{V1,LR} - \frac{32}{3} L_{jjij}^{V1,LR} + \frac{1984}{243} L_{iijj}^{V8,LR} + \frac{1984}{243} L_{jjij}^{V8,LR}
\end{aligned}$$

$$\begin{aligned}
& -\frac{2240}{81}L_{ij\bar{i}\bar{i}}^{V,RR} - \frac{2240}{81}L_{ij\bar{j}\bar{j}}^{V,RR} \Big] + \alpha^2 \Big[ -\frac{832}{243}L_{11ij}^{V1,LR} - \frac{832}{243}L_{22ij}^{V1,LR} - \frac{328}{243}L_{11ij}^{V,LR} \\
& -\frac{328}{243}L_{22ij}^{V,LR} - \frac{328}{243}L_{33ij}^{V,LR} + \frac{3344}{243}L_{11ij}^{V,RR} + \frac{3344}{243}L_{22ij}^{V,RR} + \frac{4496}{243}L_{33ij}^{V,RR} \\
& + \frac{392}{243}L_{ud11}^{V1,RR} + \frac{392}{243}L_{ud22}^{V1,RR} - \frac{64}{243}L_{i\bar{i}ij}^{V1,LR} - \frac{64}{243}L_{j\bar{j}ij}^{V1,LR} + \frac{25888}{243}L_{ij\bar{i}\bar{i}}^{V,RR} \\
& + \frac{25888}{243}L_{ij\bar{j}\bar{j}}^{V,RR} \Big] ;
\end{aligned}$$

$$\begin{aligned}
\dot{L}_{ij11}^{V1,RR} &= \frac{8}{3}g_s^2L_{ij11}^{V8,RR} + e^2 \Big[ \frac{4}{9}L_{11ij}^{V1,LR} + \frac{4}{9}L_{22ij}^{V1,LR} + \frac{4}{9}L_{11ij}^{V,LR} + \frac{4}{9}L_{22ij}^{V,LR} \\
& + \frac{4}{9}L_{33ij}^{V,LR} + \frac{4}{9}L_{11ij}^{V,RR} + \frac{4}{9}L_{22ij}^{V,RR} + \frac{4}{9}L_{33ij}^{V,RR} - \frac{20}{9}L_{ud11}^{V1,RR} + \frac{4}{9}L_{ij22}^{V1,RR} \\
& - \frac{8}{9}L_{i\bar{i}ij}^{V1,LR} - \frac{8}{9}L_{j\bar{j}ij}^{V1,LR} - \frac{64}{27}L_{i\bar{i}ij}^{V,RR} - \frac{64}{27}L_{j\bar{j}ij}^{V,RR} \Big] + \alpha_s^2 \Big[ -8L_{11ij}^{V1,LR} \\
& - 8L_{22ij}^{V1,LR} + \frac{4}{27}L_{11ij}^{V8,LR} + \frac{4}{27}L_{22ij}^{V8,LR} - \frac{4}{3}L_{ud11}^{V1,RR} + 8L_{ij22}^{V1,RR} + \frac{86}{27}L_{ud11}^{V8,RR} \\
& + \frac{4}{27}L_{ud22}^{V8,RR} - 8L_{i\bar{i}ij}^{V1,LR} - 8L_{j\bar{j}ij}^{V1,LR} + \frac{4}{27}L_{i\bar{i}ij}^{V8,LR} + \frac{4}{27}L_{j\bar{j}ij}^{V8,LR} + \frac{328}{9}L_{ij\bar{i}\bar{i}}^{V,RR} \\
& + \frac{328}{9}L_{ij\bar{j}\bar{j}}^{V,RR} \Big] + \alpha_s\alpha \Big[ \frac{16}{9}L_{11ij}^{V1,LR} + \frac{16}{9}L_{22ij}^{V1,LR} - \frac{392}{729}L_{11ij}^{V8,LR} - \frac{392}{729}L_{22ij}^{V8,LR} \\
& + \frac{208}{9}L_{ud11}^{V1,RR} + \frac{16}{9}L_{ij22}^{V1,RR} + \frac{112}{729}L_{ud11}^{V8,RR} + \frac{328}{729}L_{ij22}^{V8,RR} - \frac{32}{9}L_{i\bar{i}ij}^{V1,LR} - \frac{32}{9}L_{j\bar{j}ij}^{V1,LR} \\
& + \frac{1984}{729}L_{i\bar{i}ij}^{V8,LR} + \frac{1984}{729}L_{j\bar{j}ij}^{V8,LR} - \frac{2240}{243}L_{ij\bar{i}\bar{i}}^{V,RR} - \frac{2240}{243}L_{ij\bar{j}\bar{j}}^{V,RR} \Big] + \alpha^2 \Big[ -\frac{40}{729}L_{11ij}^{V1,LR} \\
& - \frac{40}{729}L_{22ij}^{V1,LR} + \frac{1760}{729}L_{11ij}^{V,LR} + \frac{1760}{729}L_{22ij}^{V,LR} + \frac{1760}{729}L_{33ij}^{V,LR} + \frac{1544}{729}L_{11ij}^{V,RR} \\
& + \frac{1544}{729}L_{22ij}^{V,RR} + \frac{1544}{729}L_{33ij}^{V,RR} - \frac{1120}{729}L_{ud11}^{V1,RR} - \frac{112}{729}L_{ij22}^{V1,RR} + \frac{2240}{729}L_{i\bar{i}ij}^{V1,LR} \\
& + \frac{2240}{729}L_{j\bar{j}ij}^{V1,LR} + \frac{11488}{729}L_{ij\bar{i}\bar{i}}^{V,RR} + \frac{11488}{729}L_{ij\bar{j}\bar{j}}^{V,RR} \Big] ;
\end{aligned}$$

$$\dot{L}_{ij11}^{V8,RR} = g_s^2 \Big[ \frac{2}{3}L_{11ij}^{V8,LR} + \frac{2}{3}L_{22ij}^{V8,LR} + 12L_{ud11}^{V1,RR} - \frac{10}{3}L_{ij11}^{V8,RR} + \frac{2}{3}L_{ij22}^{V8,RR}
\end{aligned}$$

$$\begin{aligned}
& + \frac{2}{3} L_{\bar{u}\bar{u}j}^{V8,LR} + \frac{2}{3} L_{\bar{j}\bar{j}i}^{V8,LR} + \frac{8}{3} L_{\bar{u}\bar{i}i}^{V,RR} + \frac{8}{3} L_{\bar{i}\bar{j}j}^{V,RR} \Big] - \frac{8}{3} e^2 L_{\bar{u}\bar{j}11}^{V8,RR} + \alpha_s^2 \Big[ - \frac{22}{3} L_{\bar{u}\bar{i}1j}^{V1,LR} \\
& - \frac{22}{3} L_{\bar{u}\bar{j}22}^{V1,LR} + \frac{169}{81} L_{\bar{u}\bar{i}1j}^{V8,LR} + \frac{169}{81} L_{\bar{u}\bar{j}22}^{V8,LR} + 13 L_{\bar{u}\bar{i}11}^{V1,RR} - \frac{2}{3} L_{\bar{u}\bar{j}22}^{V1,RR} - \frac{326}{81} L_{\bar{u}\bar{i}11}^{V8,RR} \\
& + \frac{799}{81} L_{\bar{u}\bar{j}22}^{V8,RR} - \frac{22}{3} L_{\bar{u}\bar{i}i}^{V1,LR} - \frac{22}{3} L_{\bar{u}\bar{j}j}^{V1,LR} + \frac{169}{81} L_{\bar{u}\bar{i}i}^{V8,LR} + \frac{169}{81} L_{\bar{u}\bar{j}j}^{V8,LR} + \frac{1930}{27} L_{\bar{u}\bar{i}i}^{V,RR} \\
& + \frac{1930}{27} L_{\bar{u}\bar{j}j}^{V,RR} \Big] + \alpha_s \alpha \Big[ \frac{308}{81} L_{\bar{u}\bar{i}1j}^{V1,LR} + \frac{308}{81} L_{\bar{u}\bar{j}22}^{V1,LR} + \frac{10}{27} L_{\bar{u}\bar{i}1j}^{V8,LR} + \frac{10}{27} L_{\bar{u}\bar{j}22}^{V8,LR} \\
& + \frac{308}{81} L_{\bar{u}\bar{i}1j}^{V,LR} + \frac{308}{81} L_{\bar{u}\bar{j}22}^{V,LR} + \frac{308}{81} L_{\bar{u}\bar{i}i}^{V,LR} + \frac{308}{81} L_{\bar{u}\bar{j}j}^{V,LR} + \frac{308}{81} L_{\bar{u}\bar{i}i}^{V,RR} + \frac{308}{81} L_{\bar{u}\bar{j}j}^{V,RR} \\
& + \frac{200}{81} L_{\bar{u}\bar{i}11}^{V1,RR} + \frac{308}{81} L_{\bar{u}\bar{j}22}^{V1,RR} - \frac{11}{3} L_{\bar{u}\bar{i}11}^{V8,RR} + \frac{14}{9} L_{\bar{u}\bar{j}22}^{V8,RR} - \frac{616}{81} L_{\bar{u}\bar{i}i}^{V1,LR} - \frac{616}{81} L_{\bar{u}\bar{j}j}^{V1,LR} \\
& + \frac{4}{27} L_{\bar{u}\bar{i}i}^{V8,LR} + \frac{4}{27} L_{\bar{u}\bar{j}j}^{V8,LR} - \frac{4808}{81} L_{\bar{u}\bar{i}i}^{V,RR} - \frac{4808}{81} L_{\bar{u}\bar{j}j}^{V,RR} \Big] - \frac{112}{81} \alpha^2 L_{\bar{u}\bar{i}11}^{V8,RR} ;
\end{aligned}$$

$$\begin{aligned}
\dot{L}_{\bar{u}\bar{j}22}^{V1,RR} = & \frac{8}{3} g_s^2 L_{\bar{u}\bar{j}22}^{V8,RR} + e^2 \Big[ \frac{4}{9} L_{\bar{u}\bar{i}1j}^{V1,LR} + \frac{4}{9} L_{\bar{u}\bar{j}22}^{V1,LR} + \frac{4}{9} L_{\bar{u}\bar{i}i}^{V,LR} + \frac{4}{9} L_{\bar{u}\bar{j}j}^{V,LR} \\
& + \frac{4}{9} L_{\bar{u}\bar{i}i}^{V,RR} + \frac{4}{9} L_{\bar{u}\bar{j}j}^{V,RR} + \frac{4}{9} L_{\bar{u}\bar{i}i}^{V,RR} + \frac{4}{9} L_{\bar{u}\bar{j}j}^{V,RR} + \frac{4}{9} L_{\bar{u}\bar{i}11}^{V1,RR} - \frac{20}{9} L_{\bar{u}\bar{j}22}^{V1,RR} \\
& - \frac{8}{9} L_{\bar{u}\bar{i}i}^{V1,LR} - \frac{8}{9} L_{\bar{u}\bar{j}j}^{V1,LR} - \frac{64}{27} L_{\bar{u}\bar{i}i}^{V,RR} - \frac{64}{27} L_{\bar{u}\bar{j}j}^{V,RR} \Big] + \alpha_s^2 \Big[ - 8 L_{\bar{u}\bar{i}1j}^{V1,LR} \\
& - 8 L_{\bar{u}\bar{j}22}^{V1,LR} + \frac{4}{27} L_{\bar{u}\bar{i}1j}^{V8,LR} + \frac{4}{27} L_{\bar{u}\bar{j}22}^{V8,LR} + 8 L_{\bar{u}\bar{i}11}^{V1,RR} - \frac{4}{3} L_{\bar{u}\bar{j}22}^{V1,RR} + \frac{4}{27} L_{\bar{u}\bar{i}11}^{V8,RR} \\
& + \frac{86}{27} L_{\bar{u}\bar{j}22}^{V8,RR} - 8 L_{\bar{u}\bar{i}i}^{V1,LR} - 8 L_{\bar{u}\bar{j}j}^{V1,LR} + \frac{4}{27} L_{\bar{u}\bar{i}i}^{V8,LR} + \frac{4}{27} L_{\bar{u}\bar{j}j}^{V8,LR} + \frac{328}{9} L_{\bar{u}\bar{i}i}^{V,RR} \\
& + \frac{328}{9} L_{\bar{u}\bar{j}j}^{V,RR} \Big] + \alpha_s \alpha \Big[ \frac{16}{9} L_{\bar{u}\bar{i}1j}^{V1,LR} + \frac{16}{9} L_{\bar{u}\bar{j}22}^{V1,LR} - \frac{392}{729} L_{\bar{u}\bar{i}1j}^{V8,LR} - \frac{392}{729} L_{\bar{u}\bar{j}22}^{V8,LR} \\
& + \frac{16}{9} L_{\bar{u}\bar{i}11}^{V1,RR} + \frac{208}{9} L_{\bar{u}\bar{j}22}^{V1,RR} + \frac{328}{729} L_{\bar{u}\bar{i}11}^{V8,RR} + \frac{112}{729} L_{\bar{u}\bar{j}22}^{V8,RR} - \frac{32}{9} L_{\bar{u}\bar{i}i}^{V1,LR} - \frac{32}{9} L_{\bar{u}\bar{j}j}^{V1,LR} \\
& + \frac{1984}{729} L_{\bar{u}\bar{i}i}^{V8,LR} + \frac{1984}{729} L_{\bar{u}\bar{j}j}^{V8,LR} - \frac{2240}{243} L_{\bar{u}\bar{i}i}^{V,RR} - \frac{2240}{243} L_{\bar{u}\bar{j}j}^{V,RR} \Big] + \alpha^2 \Big[ - \frac{40}{729} L_{\bar{u}\bar{i}1j}^{V1,LR} \\
& - \frac{40}{729} L_{\bar{u}\bar{j}22}^{V1,LR} + \frac{1760}{729} L_{\bar{u}\bar{i}i}^{V,LR} + \frac{1760}{729} L_{\bar{u}\bar{j}j}^{V,LR} + \frac{1760}{729} L_{\bar{u}\bar{i}i}^{V,RR} + \frac{1760}{729} L_{\bar{u}\bar{j}j}^{V,RR} + \frac{1544}{729} L_{\bar{u}\bar{i}i}^{V,RR} \\
& + \frac{1544}{729} L_{\bar{u}\bar{j}j}^{V,RR} \Big]
\end{aligned}$$

$$\begin{aligned}
& + \frac{1544}{729} L_{22ij}^{V,RR} + \frac{1544}{729} L_{33ij}^{V,RR} - \frac{112}{729} L_{ij11}^{V1,RR} - \frac{1120}{729} L_{ij22}^{V1,RR} + \frac{2240}{729} L_{iii}^{V1,LR} \\
& + \frac{2240}{729} L_{jjj}^{V1,LR} + \frac{11488}{729} L_{ijii}^{V,RR} + \frac{11488}{729} L_{ijjj}^{V,RR} \Big] ;
\end{aligned}$$

$$\begin{aligned}
\dot{L}_{ud}^{V8,RR} = & g_s^2 \left[ \frac{2}{3} L_{11ij}^{V8,LR} + \frac{2}{3} L_{22ij}^{V8,LR} + 12 L_{ij22}^{V1,RR} + \frac{2}{3} L_{ij11}^{V8,RR} - \frac{10}{3} L_{ij22}^{V8,RR} \right. \\
& + \frac{2}{3} L_{iii}^{V8,LR} + \frac{2}{3} L_{jjj}^{V8,LR} + \frac{8}{3} L_{ijii}^{V,RR} + \frac{8}{3} L_{ijjj}^{V,RR} \Big] - \frac{8}{3} e^2 L_{ij22}^{V8,RR} + \alpha_s^2 \left[ -\frac{22}{3} L_{11ij}^{V1,LR} \right. \\
& - \frac{22}{3} L_{22ij}^{V1,LR} + \frac{169}{81} L_{11ij}^{V8,LR} + \frac{169}{81} L_{22ij}^{V8,LR} - \frac{2}{3} L_{ij11}^{V1,RR} + 13 L_{ij22}^{V1,RR} + \frac{799}{81} L_{ij11}^{V8,RR} \\
& - \frac{326}{81} L_{ij22}^{V8,RR} - \frac{22}{3} L_{iii}^{V1,LR} - \frac{22}{3} L_{jjj}^{V1,LR} + \frac{169}{81} L_{iii}^{V8,LR} + \frac{169}{81} L_{jjj}^{V8,LR} + \frac{1930}{27} L_{ijii}^{V,RR} \\
& + \frac{1930}{27} L_{ijjj}^{V,RR} \Big] + \alpha_s \alpha \left[ \frac{308}{81} L_{11ij}^{V1,LR} + \frac{308}{81} L_{22ij}^{V1,LR} + \frac{10}{27} L_{11ij}^{V8,LR} + \frac{10}{27} L_{22ij}^{V8,LR} \right. \\
& + \frac{308}{81} L_{11ij}^{V,LR} + \frac{308}{81} L_{22ij}^{V,LR} + \frac{308}{81} L_{33ij}^{V,LR} + \frac{308}{81} L_{11ij}^{V,RR} + \frac{308}{81} L_{22ij}^{V,RR} + \frac{308}{81} L_{33ij}^{V,RR} \\
& + \frac{308}{81} L_{ij11}^{V1,RR} + \frac{200}{81} L_{ij22}^{V1,RR} + \frac{14}{9} L_{ij11}^{V8,RR} - \frac{11}{3} L_{ij22}^{V8,RR} - \frac{616}{81} L_{iii}^{V1,LR} - \frac{616}{81} L_{jjj}^{V1,LR} \\
& + \frac{4}{27} L_{iii}^{V8,LR} + \frac{4}{27} L_{jjj}^{V8,LR} - \frac{4808}{81} L_{ijii}^{V,RR} - \frac{4808}{81} L_{ijjj}^{V,RR} \Big] - \frac{112}{81} \alpha^2 L_{ij22}^{V8,RR} ;
\end{aligned}$$

$$\begin{aligned}
\dot{L}_{uu}^{V,RR} = & g_s^2 \left[ \frac{1}{9} L_{11ij}^{V8,LR} + \frac{1}{9} L_{22ij}^{V8,LR} + \frac{1}{9} L_{ij11}^{V8,RR} + \frac{1}{9} L_{ij22}^{V8,RR} + \frac{1}{9} L_{iii}^{V8,LR} \right. \\
& + \frac{1}{9} L_{jjj}^{V8,LR} + \frac{4}{9} L_{ijii}^{V,RR} + \frac{40}{9} L_{ijjj}^{V,RR} \Big] + e^2 \left[ -\frac{4}{9} L_{11ij}^{V1,LR} - \frac{4}{9} L_{22ij}^{V1,LR} \right. \\
& - \frac{4}{9} L_{11ij}^{V,LR} - \frac{4}{9} L_{22ij}^{V,LR} - \frac{4}{9} L_{33ij}^{V,LR} - \frac{4}{9} L_{11ij}^{V,RR} - \frac{4}{9} L_{22ij}^{V,RR} - \frac{4}{9} L_{33ij}^{V,RR} \\
& - \frac{4}{9} L_{ij11}^{V1,RR} - \frac{4}{9} L_{ij22}^{V1,RR} + \frac{8}{9} L_{iii}^{V1,LR} + \frac{8}{9} L_{jjj}^{V1,LR} + \frac{64}{27} L_{ijii}^{V,RR} + \frac{208}{27} L_{ijjj}^{V,RR} \Big] \\
& + \alpha_s^2 \left[ -\frac{47}{9} L_{11ij}^{V1,LR} - \frac{47}{9} L_{22ij}^{V1,LR} + \frac{205}{486} L_{11ij}^{V8,LR} + \frac{205}{486} L_{22ij}^{V8,LR} + \frac{35}{9} L_{ij11}^{V1,RR} \right. \\
& + \frac{35}{9} L_{ij22}^{V1,RR} + \frac{835}{486} L_{ij11}^{V8,RR} + \frac{835}{486} L_{ij22}^{V8,RR} - \frac{47}{9} L_{iii}^{V1,LR} - \frac{47}{9} L_{jjj}^{V1,LR} + \frac{205}{486} L_{iii}^{V8,LR}
\end{aligned}$$

$$\begin{aligned}
& + \frac{205}{486} L_{jjij}^{V8,LR} + \frac{2441}{81} L_{ijii}^{V,RR} + \frac{2054}{81} L_{ijjj}^{V,RR} \Big] + \alpha_s \alpha \Bigg[ - \frac{332}{243} L_{11ij}^{V1,LR} - \frac{332}{243} L_{22ij}^{V1,LR} \\
& + \frac{977}{729} L_{11ij}^{V8,LR} + \frac{977}{729} L_{22ij}^{V8,LR} + \frac{100}{243} L_{11ij}^{V,LR} + \frac{100}{243} L_{22ij}^{V,LR} + \frac{100}{243} L_{33ij}^{V,LR} \\
& + \frac{100}{243} L_{11ij}^{V,RR} + \frac{100}{243} L_{22ij}^{V,RR} + \frac{100}{243} L_{33ij}^{V,RR} - \frac{332}{243} L_{ij11}^{V1,RR} - \frac{332}{243} L_{ij22}^{V1,RR} \\
& - \frac{571}{729} L_{ij11}^{V8,RR} - \frac{571}{729} L_{ij22}^{V8,RR} + \frac{664}{243} L_{iijj}^{V1,LR} + \frac{664}{243} L_{jjij}^{V1,LR} - \frac{2884}{729} L_{iijj}^{V8,LR} \\
& - \frac{2884}{729} L_{jjij}^{V8,LR} + \frac{3832}{243} L_{iijj}^{V,RR} - \frac{12152}{243} L_{ijjj}^{V,RR} \Big] + \alpha^2 \Bigg[ - \frac{1148}{729} L_{11ij}^{V1,LR} - \frac{1148}{729} L_{22ij}^{V1,LR} \\
& - \frac{4892}{729} L_{11ij}^{V,LR} - \frac{4892}{729} L_{22ij}^{V,LR} - \frac{4892}{729} L_{33ij}^{V,LR} + \frac{1156}{729} L_{11ij}^{V,RR} + \frac{1156}{729} L_{22ij}^{V,RR} \\
& + \frac{1156}{729} L_{33ij}^{V,RR} + \frac{868}{729} L_{ij11}^{V1,RR} + \frac{868}{729} L_{ij22}^{V1,RR} - \frac{5696}{729} L_{iijj}^{V1,LR} - \frac{5696}{729} L_{jjij}^{V1,LR} \\
& + \frac{10112}{729} L_{iijj}^{V,RR} - \frac{832}{729} L_{ijjj}^{V,RR} \Big] ;
\end{aligned}$$

$$\begin{aligned}
\dot{L}_{iijj}^{V,RR} &= g_s^2 \Bigg[ \frac{1}{9} L_{11ij}^{V8,LR} + \frac{1}{9} L_{22ij}^{V8,LR} + \frac{1}{9} L_{ij11}^{V8,RR} + \frac{1}{9} L_{ij22}^{V8,RR} + \frac{1}{9} L_{iijj}^{V8,LR} \\
& + \frac{1}{9} L_{jjij}^{V8,LR} + \frac{40}{9} L_{ijii}^{V,RR} + \frac{4}{9} L_{ijjj}^{V,RR} \Big] + e^2 \Bigg[ - \frac{4}{9} L_{11ij}^{V1,LR} - \frac{4}{9} L_{22ij}^{V1,LR} \\
& - \frac{4}{9} L_{11ij}^{V,LR} - \frac{4}{9} L_{22ij}^{V,LR} - \frac{4}{9} L_{33ij}^{V,LR} - \frac{4}{9} L_{11ij}^{V,RR} - \frac{4}{9} L_{22ij}^{V,RR} - \frac{4}{9} L_{33ij}^{V,RR} \\
& - \frac{4}{9} L_{ij11}^{V1,RR} - \frac{4}{9} L_{ij22}^{V1,RR} + \frac{8}{9} L_{iijj}^{V1,LR} + \frac{8}{9} L_{jjij}^{V1,LR} + \frac{208}{27} L_{ijii}^{V,RR} + \frac{64}{27} L_{ijjj}^{V,RR} \Big] \\
& + \alpha_s^2 \Bigg[ - \frac{47}{9} L_{11ij}^{V1,LR} - \frac{47}{9} L_{22ij}^{V1,LR} + \frac{205}{486} L_{11ij}^{V8,LR} + \frac{205}{486} L_{22ij}^{V8,LR} + \frac{35}{9} L_{ij11}^{V1,RR} \\
& + \frac{35}{9} L_{ij22}^{V1,RR} + \frac{835}{486} L_{ij11}^{V8,RR} + \frac{835}{486} L_{ij22}^{V8,RR} - \frac{47}{9} L_{iijj}^{V1,LR} - \frac{47}{9} L_{jjij}^{V1,LR} + \frac{205}{486} L_{iijj}^{V8,LR} \\
& + \frac{205}{486} L_{jjij}^{V8,LR} + \frac{2054}{81} L_{ijii}^{V,RR} + \frac{2441}{81} L_{ijjj}^{V,RR} \Big] + \alpha_s \alpha \Bigg[ - \frac{332}{243} L_{11ij}^{V1,LR} - \frac{332}{243} L_{22ij}^{V1,LR} \\
& + \frac{977}{729} L_{11ij}^{V8,LR} + \frac{977}{729} L_{22ij}^{V8,LR} + \frac{100}{243} L_{11ij}^{V,LR} + \frac{100}{243} L_{22ij}^{V,LR} + \frac{100}{243} L_{33ij}^{V,LR}
\end{aligned}$$

$$\begin{aligned}
& + \frac{100}{243} L_{11ij}^{V,RR} + \frac{100}{243} L_{22ij}^{V,RR} + \frac{100}{243} L_{33ij}^{V,RR} - \frac{332}{243} L_{ij11}^{V1,RR} - \frac{332}{243} L_{ij22}^{V1,RR} \\
& - \frac{571}{729} L_{ij11}^{V8,RR} - \frac{571}{729} L_{ij22}^{V8,RR} + \frac{664}{243} L_{iiij}^{V1,LR} + \frac{664}{243} L_{jjij}^{V1,LR} - \frac{2884}{729} L_{iiij}^{V8,LR} \\
& - \frac{2884}{729} L_{jjij}^{V8,LR} - \frac{12152}{243} L_{ijii}^{V,RR} + \frac{3832}{243} L_{ijjj}^{V,RR} \Big] + \alpha^2 \Big[ - \frac{1148}{729} L_{11ij}^{V1,LR} - \frac{1148}{729} L_{22ij}^{V1,LR} \\
& - \frac{4892}{729} L_{11ij}^{V,LR} - \frac{4892}{729} L_{22ij}^{V,LR} - \frac{4892}{729} L_{33ij}^{V,LR} + \frac{1156}{729} L_{11ij}^{V,RR} + \frac{1156}{729} L_{22ij}^{V,RR} \\
& + \frac{1156}{729} L_{33ij}^{V,RR} + \frac{868}{729} L_{ij11}^{V1,RR} + \frac{868}{729} L_{ij22}^{V1,RR} - \frac{5696}{729} L_{iiij}^{V1,LR} - \frac{5696}{729} L_{jjij}^{V1,LR} \\
& - \frac{832}{729} L_{ijii}^{V,RR} + \frac{10112}{729} L_{ijjj}^{V,RR} \Big] ;
\end{aligned}$$

$$\begin{aligned}
\dot{L}_{11ij}^{V,LR} &= e^2 \Big[ \frac{4}{3} L_{11ij}^{V1,LR} + \frac{4}{3} L_{22ij}^{V1,LR} + \frac{28}{3} L_{11ij}^{V,LR} + \frac{4}{3} L_{22ij}^{V,LR} + \frac{4}{3} L_{33ij}^{V,LR} \\
& + \frac{4}{3} L_{11ij}^{V,RR} + \frac{4}{3} L_{22ij}^{V,RR} + \frac{4}{3} L_{33ij}^{V,RR} + \frac{4}{3} L_{ij11}^{V1,RR} + \frac{4}{3} L_{ij22}^{V1,RR} - \frac{8}{3} L_{iiij}^{V1,LR} \\
& - \frac{8}{3} L_{jjij}^{V1,LR} - \frac{64}{9} L_{ijii}^{V,RR} - \frac{64}{9} L_{ijjj}^{V,RR} \Big] + \alpha_s \alpha \Big[ \frac{16}{3} L_{11ij}^{V1,LR} + \frac{16}{3} L_{22ij}^{V1,LR} \\
& - \frac{392}{243} L_{11ij}^{V8,LR} - \frac{392}{243} L_{22ij}^{V8,LR} - 32 L_{11ij}^{V,LR} + \frac{16}{3} L_{ij11}^{V1,RR} + \frac{16}{3} L_{ij22}^{V1,RR} + \frac{328}{243} L_{ij11}^{V8,RR} \\
& + \frac{328}{243} L_{ij22}^{V8,RR} - \frac{32}{3} L_{iiij}^{V1,LR} - \frac{32}{3} L_{jjij}^{V1,LR} + \frac{1984}{243} L_{iiij}^{V8,LR} + \frac{1984}{243} L_{jjij}^{V8,LR} \\
& - \frac{2240}{81} L_{ijii}^{V,RR} - \frac{2240}{81} L_{ijjj}^{V,RR} \Big] + \alpha^2 \Big[ - \frac{1048}{243} L_{11ij}^{V1,LR} - \frac{1048}{243} L_{22ij}^{V1,LR} - \frac{39712}{243} L_{11ij}^{V,LR} \\
& + \frac{3344}{243} L_{22ij}^{V,LR} + \frac{3344}{243} L_{33ij}^{V,LR} - \frac{4648}{243} L_{11ij}^{V,RR} - \frac{4648}{243} L_{22ij}^{V,RR} - \frac{4648}{243} L_{33ij}^{V,RR} \\
& - \frac{3712}{243} L_{ij11}^{V1,RR} - \frac{3712}{243} L_{ij22}^{V1,RR} + \frac{12032}{243} L_{iiij}^{V1,LR} + \frac{12032}{243} L_{jjij}^{V1,LR} + \frac{3424}{243} L_{ijii}^{V,RR} \\
& + \frac{3424}{243} L_{ijjj}^{V,RR} \Big] ;
\end{aligned}$$

$$\dot{L}_{22ij}^{V,LR} = e^2 \Big[ \frac{4}{3} L_{11ij}^{V1,LR} + \frac{4}{3} L_{22ij}^{V1,LR} + \frac{4}{3} L_{11ij}^{V,LR} + \frac{28}{3} L_{22ij}^{V,LR} + \frac{4}{3} L_{33ij}^{V,LR}$$

$$\begin{aligned}
& + \frac{4}{3}L_{11ij}^{V,RR} + \frac{4}{3}L_{22ij}^{V,RR} + \frac{4}{3}L_{33ij}^{V,RR} + \frac{4}{3}L_{ij11}^{V1,RR} + \frac{4}{3}L_{ij22}^{V1,RR} - \frac{8}{3}L_{iiij}^{V1,LR} \\
& - \frac{8}{3}L_{jjij}^{V1,LR} - \frac{64}{9}L_{ijii}^{V,RR} - \frac{64}{9}L_{ijjj}^{V,RR} \Big] + \alpha_s \alpha \Big[ \frac{16}{3}L_{11ij}^{V1,LR} + \frac{16}{3}L_{22ij}^{V1,LR} \\
& - \frac{392}{243}L_{11ij}^{V8,LR} - \frac{392}{243}L_{22ij}^{V8,LR} - 32L_{22ij}^{V,LR} + \frac{16}{3}L_{ij11}^{V1,RR} + \frac{16}{3}L_{ij22}^{V1,RR} + \frac{328}{243}L_{ij11}^{V8,RR} \\
& + \frac{328}{243}L_{ij22}^{V8,RR} - \frac{32}{3}L_{iiij}^{V1,LR} - \frac{32}{3}L_{jjij}^{V1,LR} + \frac{1984}{243}L_{iiij}^{V8,LR} + \frac{1984}{243}L_{jjij}^{V8,LR} \\
& - \frac{2240}{81}L_{ijii}^{V,RR} - \frac{2240}{81}L_{ijjj}^{V,RR} \Big] + \alpha^2 \Big[ -\frac{1048}{243}L_{11ij}^{V1,LR} - \frac{1048}{243}L_{22ij}^{V1,LR} + \frac{3344}{243}L_{11ij}^{V,LR} \\
& - \frac{39712}{243}L_{22ij}^{V,LR} + \frac{3344}{243}L_{33ij}^{V,LR} - \frac{4648}{243}L_{11ij}^{V,RR} - \frac{4648}{243}L_{22ij}^{V,RR} - \frac{4648}{243}L_{33ij}^{V,RR} \\
& - \frac{3712}{243}L_{ij11}^{V1,RR} - \frac{3712}{243}L_{ij22}^{V1,RR} + \frac{12032}{243}L_{iiij}^{V1,LR} + \frac{12032}{243}L_{jjij}^{V1,LR} + \frac{3424}{243}L_{ijii}^{V,RR} \\
& + \frac{3424}{243}L_{ijjj}^{V,RR} \Big] ;
\end{aligned}$$

$$\begin{aligned}
\dot{L}_{33ij}^{V,LR} & = e^2 \Big[ \frac{4}{3}L_{11ij}^{V1,LR} + \frac{4}{3}L_{22ij}^{V1,LR} + \frac{4}{3}L_{11ij}^{V,LR} + \frac{4}{3}L_{22ij}^{V,LR} + \frac{28}{3}L_{33ij}^{V,LR} \\
& + \frac{4}{3}L_{11ij}^{V,RR} + \frac{4}{3}L_{22ij}^{V,RR} + \frac{4}{3}L_{33ij}^{V,RR} + \frac{4}{3}L_{ij11}^{V1,RR} + \frac{4}{3}L_{ij22}^{V1,RR} - \frac{8}{3}L_{iiij}^{V1,LR} \\
& - \frac{8}{3}L_{jjij}^{V1,LR} - \frac{64}{9}L_{ijii}^{V,RR} - \frac{64}{9}L_{ijjj}^{V,RR} \Big] + \alpha_s \alpha \Big[ \frac{16}{3}L_{11ij}^{V1,LR} + \frac{16}{3}L_{22ij}^{V1,LR} \\
& - \frac{392}{243}L_{11ij}^{V8,LR} - \frac{392}{243}L_{22ij}^{V8,LR} - 32L_{33ij}^{V,LR} + \frac{16}{3}L_{ij11}^{V1,RR} + \frac{16}{3}L_{ij22}^{V1,RR} + \frac{328}{243}L_{ij11}^{V8,RR} \\
& + \frac{328}{243}L_{ij22}^{V8,RR} - \frac{32}{3}L_{iiij}^{V1,LR} - \frac{32}{3}L_{jjij}^{V1,LR} + \frac{1984}{243}L_{iiij}^{V8,LR} + \frac{1984}{243}L_{jjij}^{V8,LR} \\
& - \frac{2240}{81}L_{ijii}^{V,RR} - \frac{2240}{81}L_{ijjj}^{V,RR} \Big] + \alpha^2 \Big[ -\frac{1048}{243}L_{11ij}^{V1,LR} - \frac{1048}{243}L_{22ij}^{V1,LR} + \frac{3344}{243}L_{11ij}^{V,LR} \\
& + \frac{3344}{243}L_{22ij}^{V,LR} - \frac{39712}{243}L_{33ij}^{V,LR} - \frac{4648}{243}L_{11ij}^{V,RR} - \frac{4648}{243}L_{22ij}^{V,RR} - \frac{4648}{243}L_{33ij}^{V,RR} \\
& - \frac{3712}{243}L_{ij11}^{V1,RR} - \frac{3712}{243}L_{ij22}^{V1,RR} + \frac{12032}{243}L_{iiij}^{V1,LR} + \frac{12032}{243}L_{jjij}^{V1,LR} + \frac{3424}{243}L_{ijii}^{V,RR} \\
& + \frac{3424}{243}L_{ijjj}^{V,RR} \Big] ;
\end{aligned}$$



$$\begin{aligned}
& + \frac{3424}{243} L_{ijjj}^{V,RR} \Big] ; \\
\dot{L}_{11ij}^{V1,LR} = & -\frac{8}{3} g_s^2 L_{11ij}^{V8,LR} + e^2 \left[ \frac{28}{9} L_{11ij}^{V1,LR} + \frac{4}{9} L_{22ij}^{V1,LR} + \frac{4}{9} L_{11ij}^{V,LR} + \frac{4}{9} L_{22ij}^{V,LR} \right. \\
& + \frac{4}{9} L_{33ij}^{V,LR} + \frac{4}{9} L_{11ij}^{V,RR} + \frac{4}{9} L_{22ij}^{V,RR} + \frac{4}{9} L_{33ij}^{V,RR} + \frac{4}{9} L_{ij11}^{V1,RR} + \frac{4}{9} L_{ij22}^{V1,RR} \\
& - \frac{8}{9} L_{iii}^{V1,LR} - \frac{8}{9} L_{jjj}^{V1,LR} - \frac{64}{27} L_{ijii}^{V,RR} - \frac{64}{27} L_{ijjj}^{V,RR} \Big] + \alpha_s^2 \left[ -\frac{4}{3} L_{11ij}^{V1,LR} \right. \\
& + 8 L_{22ij}^{V1,LR} - \frac{2000}{27} L_{11ij}^{V8,LR} + \frac{44}{27} L_{22ij}^{V8,LR} - 8 L_{ij11}^{V1,RR} - 8 L_{ij22}^{V1,RR} + \frac{44}{27} L_{ij11}^{V8,RR} \\
& + \frac{44}{27} L_{ij22}^{V8,RR} + 8 L_{iii}^{V1,LR} + 8 L_{jjj}^{V1,LR} + \frac{44}{27} L_{ijii}^{V8,LR} + \frac{44}{27} L_{jjjj}^{V8,LR} - \frac{232}{9} L_{ijii}^{V,RR} \\
& - \frac{232}{9} L_{ijjj}^{V,RR} \Big] + \alpha_s \alpha \left[ -\frac{176}{9} L_{11ij}^{V1,LR} + \frac{16}{9} L_{22ij}^{V1,LR} + \frac{5872}{729} L_{11ij}^{V8,LR} - \frac{392}{729} L_{22ij}^{V8,LR} \right. \\
& + \frac{16}{9} L_{ij11}^{V1,RR} + \frac{16}{9} L_{ij22}^{V1,RR} + \frac{328}{729} L_{ij11}^{V8,RR} + \frac{328}{729} L_{ij22}^{V8,RR} - \frac{32}{9} L_{iii}^{V1,LR} - \frac{32}{9} L_{jjj}^{V1,LR} \\
& + \frac{1984}{729} L_{ijii}^{V8,LR} + \frac{1984}{729} L_{jjjj}^{V8,LR} - \frac{2240}{243} L_{ijii}^{V,RR} - \frac{2240}{243} L_{ijjj}^{V,RR} \Big] + \alpha^2 \left[ -\frac{34960}{729} L_{11ij}^{V1,LR} \right. \\
& - \frac{112}{729} L_{22ij}^{V1,LR} + \frac{2984}{729} L_{11ij}^{V,LR} + \frac{2984}{729} L_{22ij}^{V,LR} + \frac{2984}{729} L_{33ij}^{V,LR} - \frac{1120}{729} L_{11ij}^{V,RR} \\
& - \frac{1120}{729} L_{22ij}^{V,RR} - \frac{1120}{729} L_{33ij}^{V,RR} - \frac{1480}{729} L_{ij11}^{V1,RR} - \frac{1480}{729} L_{ij22}^{V1,RR} + \frac{6272}{729} L_{iii}^{V1,LR} \\
& + \frac{6272}{729} L_{jjj}^{V1,LR} + \frac{4000}{729} L_{ijii}^{V,RR} + \frac{4000}{729} L_{ijjj}^{V,RR} \Big] ; \\
\dot{L}_{11ij}^{V8,LR} = & g_s^2 \left[ -12 L_{11ij}^{V1,LR} - \frac{40}{3} L_{11ij}^{V8,LR} + \frac{2}{3} L_{22ij}^{V8,LR} + \frac{2}{3} L_{ij11}^{V8,RR} + \frac{2}{3} L_{ij22}^{V8,RR} \right. \\
& + \frac{2}{3} L_{iii}^{V8,LR} + \frac{2}{3} L_{jjj}^{V8,LR} + \frac{8}{3} L_{ijii}^{V,RR} + \frac{8}{3} L_{ijjj}^{V,RR} \Big] + \frac{8}{3} e^2 L_{11ij}^{V8,LR} + \alpha_s^2 \left[ -132 L_{11ij}^{V1,LR} \right. \\
& - \frac{22}{3} L_{22ij}^{V1,LR} - \frac{25177}{162} L_{11ij}^{V8,LR} + \frac{799}{81} L_{22ij}^{V8,LR} - \frac{2}{3} L_{ij11}^{V1,RR} - \frac{2}{3} L_{ij22}^{V1,RR} + \frac{619}{81} L_{ij11}^{V8,RR} \\
& + \frac{619}{81} L_{ij22}^{V8,RR} - \frac{22}{3} L_{iii}^{V1,LR} - \frac{22}{3} L_{jjj}^{V1,LR} + \frac{799}{81} L_{ijii}^{V8,LR} + \frac{799}{81} L_{jjjj}^{V8,LR} + \frac{1210}{27} L_{ijii}^{V,RR} \\
& + \frac{1210}{27} L_{ijjj}^{V,RR} \Big] ;
\end{aligned}$$

$$\begin{aligned}
& + \frac{1210}{27} L_{ijjj}^{V,RR} \Big] + \alpha_s \alpha \Big[ \frac{3800}{81} L_{11ij}^{V1,LR} + \frac{668}{81} L_{22ij}^{V1,LR} + \frac{67}{3} L_{11ij}^{V8,LR} + \frac{14}{9} L_{22ij}^{V8,LR} \\
& + \frac{668}{81} L_{11ij}^{V,LR} + \frac{668}{81} L_{22ij}^{V,LR} + \frac{668}{81} L_{33ij}^{V,LR} + \frac{668}{81} L_{11ij}^{V,RR} + \frac{668}{81} L_{22ij}^{V,RR} + \frac{668}{81} L_{33ij}^{V,RR} \\
& + \frac{668}{81} L_{ud11}^{V1,RR} + \frac{668}{81} L_{ij22}^{V1,RR} - \frac{70}{27} L_{ij11}^{V8,RR} - \frac{70}{27} L_{ij22}^{V8,RR} - \frac{1336}{81} L_{iii}^{V1,LR} - \frac{1336}{81} L_{jjj}^{V1,LR} \\
& - \frac{20}{3} L_{iii}^{V8,LR} - \frac{20}{3} L_{jjj}^{V8,LR} - \frac{3800}{81} L_{ijii}^{V,RR} - \frac{3800}{81} L_{ijjj}^{V,RR} \Big] - \frac{3872}{81} \alpha^2 L_{11ij}^{V8,LR} ; \\
\dot{L}_{22ij}^{V1,LR} = & - \frac{8}{3} g_s^2 L_{22ij}^{V8,LR} + e^2 \Big[ \frac{4}{9} L_{11ij}^{V1,LR} + \frac{28}{9} L_{22ij}^{V1,LR} + \frac{4}{9} L_{11ij}^{V,LR} + \frac{4}{9} L_{22ij}^{V,LR} \\
& + \frac{4}{9} L_{33ij}^{V,LR} + \frac{4}{9} L_{11ij}^{V,RR} + \frac{4}{9} L_{22ij}^{V,RR} + \frac{4}{9} L_{33ij}^{V,RR} + \frac{4}{9} L_{ij11}^{V1,RR} + \frac{4}{9} L_{ij22}^{V1,RR} \\
& - \frac{8}{9} L_{iii}^{V1,LR} - \frac{8}{9} L_{jjj}^{V1,LR} - \frac{64}{27} L_{ijii}^{V,RR} - \frac{64}{27} L_{ijjj}^{V,RR} \Big] + \alpha_s^2 \Big[ 8 L_{11ij}^{V1,LR} \\
& - \frac{4}{3} L_{22ij}^{V1,LR} + \frac{44}{27} L_{11ij}^{V8,LR} - \frac{2000}{27} L_{22ij}^{V8,LR} - 8 L_{ij11}^{V1,RR} - 8 L_{ij22}^{V1,RR} + \frac{44}{27} L_{ij11}^{V8,RR} \\
& + \frac{44}{27} L_{ij22}^{V8,RR} + 8 L_{iii}^{V1,LR} + 8 L_{jjj}^{V1,LR} + \frac{44}{27} L_{iii}^{V8,LR} + \frac{44}{27} L_{jjj}^{V8,LR} - \frac{232}{9} L_{ijii}^{V,RR} \\
& - \frac{232}{9} L_{ijjj}^{V,RR} \Big] + \alpha_s \alpha \Big[ \frac{16}{9} L_{11ij}^{V1,LR} - \frac{176}{9} L_{22ij}^{V1,LR} - \frac{392}{729} L_{11ij}^{V8,LR} + \frac{5872}{729} L_{22ij}^{V8,LR} \\
& + \frac{16}{9} L_{ij11}^{V1,RR} + \frac{16}{9} L_{ij22}^{V1,RR} + \frac{328}{729} L_{ij11}^{V8,RR} + \frac{328}{729} L_{ij22}^{V8,RR} - \frac{32}{9} L_{iii}^{V1,LR} - \frac{32}{9} L_{jjj}^{V1,LR} \\
& + \frac{1984}{729} L_{iii}^{V8,LR} + \frac{1984}{729} L_{jjj}^{V8,LR} - \frac{2240}{243} L_{ijii}^{V,RR} - \frac{2240}{243} L_{ijjj}^{V,RR} \Big] + \alpha^2 \Big[ - \frac{112}{729} L_{11ij}^{V1,LR} \\
& - \frac{34960}{729} L_{22ij}^{V1,LR} + \frac{2984}{729} L_{11ij}^{V,LR} + \frac{2984}{729} L_{22ij}^{V,LR} + \frac{2984}{729} L_{33ij}^{V,LR} - \frac{1120}{729} L_{11ij}^{V,RR} \\
& - \frac{1120}{729} L_{22ij}^{V,RR} - \frac{1120}{729} L_{33ij}^{V,RR} - \frac{1480}{729} L_{ij11}^{V1,RR} - \frac{1480}{729} L_{ij22}^{V1,RR} + \frac{6272}{729} L_{iii}^{V1,LR} \\
& + \frac{6272}{729} L_{jjj}^{V1,LR} + \frac{4000}{729} L_{ijii}^{V,RR} + \frac{4000}{729} L_{ijjj}^{V,RR} \Big] ; \\
\dot{L}_{22ij}^{V8,LR} = & g_s^2 \Big[ - 12 L_{22ij}^{V1,LR} + \frac{2}{3} L_{11ij}^{V8,LR} - \frac{40}{3} L_{22ij}^{V8,LR} + \frac{2}{3} L_{ij11}^{V8,RR} + \frac{2}{3} L_{ij22}^{V8,RR}
\end{aligned}$$

$$\begin{aligned}
& + \frac{2}{3} L_{\bar{u}\bar{u}}^{V8,LR} + \frac{2}{3} L_{\bar{j}\bar{j}}^{V8,LR} + \frac{8}{3} L_{\bar{u}\bar{i}}^{V,RR} + \frac{8}{3} L_{\bar{i}\bar{j}}^{V,RR} \left] + \frac{8}{3} e^2 L_{\bar{d}\bar{u}}^{V8,LR} + \alpha_s^2 \left[ -\frac{22}{3} L_{\bar{d}\bar{u}}^{V1,LR} \right. \right. \\
& - 132 L_{\bar{d}\bar{u}}^{V1,LR} + \frac{799}{81} L_{\bar{d}\bar{u}}^{V8,LR} - \frac{25177}{162} L_{\bar{d}\bar{u}}^{V8,LR} - \frac{2}{3} L_{\bar{u}\bar{d}}^{V1,RR} - \frac{2}{3} L_{\bar{u}\bar{d}}^{V1,RR} + \frac{619}{81} L_{\bar{u}\bar{d}}^{V8,RR} \\
& + \frac{619}{81} L_{\bar{u}\bar{d}}^{V8,RR} - \frac{22}{3} L_{\bar{u}\bar{u}}^{V1,LR} - \frac{22}{3} L_{\bar{j}\bar{j}}^{V1,LR} + \frac{799}{81} L_{\bar{u}\bar{u}}^{V8,LR} + \frac{799}{81} L_{\bar{j}\bar{j}}^{V8,LR} + \frac{1210}{27} L_{\bar{u}\bar{u}}^{V,RR} \\
& \left. + \frac{1210}{27} L_{\bar{j}\bar{j}}^{V,RR} \right] + \alpha_s \alpha \left[ \frac{668}{81} L_{\bar{d}\bar{u}}^{V1,LR} + \frac{3800}{81} L_{\bar{d}\bar{u}}^{V1,LR} + \frac{14}{9} L_{\bar{d}\bar{u}}^{V8,LR} + \frac{67}{3} L_{\bar{d}\bar{u}}^{V8,LR} \right. \\
& + \frac{668}{81} L_{\bar{u}\bar{u}}^{V,LR} + \frac{668}{81} L_{\bar{u}\bar{u}}^{V,LR} + \frac{668}{81} L_{\bar{u}\bar{u}}^{V,LR} + \frac{668}{81} L_{\bar{u}\bar{u}}^{V,RR} + \frac{668}{81} L_{\bar{u}\bar{u}}^{V,RR} + \frac{668}{81} L_{\bar{u}\bar{u}}^{V,RR} \\
& + \frac{668}{81} L_{\bar{u}\bar{d}}^{V1,RR} + \frac{668}{81} L_{\bar{u}\bar{d}}^{V1,RR} - \frac{70}{27} L_{\bar{u}\bar{d}}^{V8,RR} - \frac{70}{27} L_{\bar{u}\bar{d}}^{V8,RR} - \frac{1336}{81} L_{\bar{u}\bar{u}}^{V1,LR} - \frac{1336}{81} L_{\bar{u}\bar{u}}^{V1,LR} \\
& \left. - \frac{20}{3} L_{\bar{u}\bar{u}}^{V8,LR} - \frac{20}{3} L_{\bar{j}\bar{j}}^{V8,LR} - \frac{3800}{81} L_{\bar{u}\bar{u}}^{V,RR} - \frac{3800}{81} L_{\bar{j}\bar{j}}^{V,RR} \right] - \frac{3872}{81} \alpha^2 L_{\bar{d}\bar{u}}^{V8,LR} ; \\
\dot{L}_{\bar{u}\bar{u}}^{V1,LR} & = -\frac{8}{3} g_s^2 L_{\bar{u}\bar{u}}^{V8,LR} + e^2 \left[ -\frac{8}{9} L_{\bar{d}\bar{u}}^{V1,LR} - \frac{8}{9} L_{\bar{d}\bar{u}}^{V1,LR} - \frac{8}{9} L_{\bar{u}\bar{u}}^{V,LR} - \frac{8}{9} L_{\bar{u}\bar{u}}^{V,LR} \right. \\
& - \frac{8}{9} L_{\bar{u}\bar{u}}^{V,LR} - \frac{8}{9} L_{\bar{u}\bar{u}}^{V,RR} - \frac{8}{9} L_{\bar{u}\bar{u}}^{V,RR} - \frac{8}{9} L_{\bar{u}\bar{u}}^{V,RR} - \frac{8}{9} L_{\bar{u}\bar{d}}^{V1,RR} - \frac{8}{9} L_{\bar{u}\bar{d}}^{V1,RR} \\
& + \frac{16}{9} L_{\bar{u}\bar{u}}^{V1,LR} - \frac{32}{9} L_{\bar{u}\bar{u}}^{V1,LR} + \frac{128}{27} L_{\bar{u}\bar{u}}^{V,RR} + \frac{128}{27} L_{\bar{u}\bar{u}}^{V,RR} \left] + \alpha_s^2 \left[ 8 L_{\bar{d}\bar{u}}^{V1,LR} \right. \right. \\
& + 8 L_{\bar{d}\bar{u}}^{V1,LR} + \frac{44}{27} L_{\bar{d}\bar{u}}^{V8,LR} + \frac{44}{27} L_{\bar{d}\bar{u}}^{V8,LR} - 8 L_{\bar{u}\bar{d}}^{V1,RR} - 8 L_{\bar{u}\bar{d}}^{V1,RR} + \frac{44}{27} L_{\bar{u}\bar{d}}^{V8,RR} \\
& + \frac{44}{27} L_{\bar{u}\bar{d}}^{V8,RR} + 8 L_{\bar{u}\bar{u}}^{V1,LR} - \frac{4}{3} L_{\bar{u}\bar{u}}^{V1,LR} + \frac{44}{27} L_{\bar{u}\bar{u}}^{V8,LR} - \frac{2000}{27} L_{\bar{u}\bar{u}}^{V8,LR} - \frac{232}{9} L_{\bar{u}\bar{u}}^{V,RR} \\
& \left. - \frac{232}{9} L_{\bar{u}\bar{u}}^{V,RR} \right] + \alpha_s \alpha \left[ -\frac{32}{9} L_{\bar{d}\bar{u}}^{V1,LR} - \frac{32}{9} L_{\bar{d}\bar{u}}^{V1,LR} + \frac{784}{729} L_{\bar{d}\bar{u}}^{V8,LR} + \frac{784}{729} L_{\bar{d}\bar{u}}^{V8,LR} \right. \\
& - \frac{32}{9} L_{\bar{u}\bar{d}}^{V1,RR} - \frac{32}{9} L_{\bar{u}\bar{d}}^{V1,RR} - \frac{656}{729} L_{\bar{u}\bar{d}}^{V8,RR} - \frac{656}{729} L_{\bar{u}\bar{d}}^{V8,RR} + \frac{64}{9} L_{\bar{u}\bar{u}}^{V1,LR} + \frac{448}{9} L_{\bar{u}\bar{u}}^{V1,LR} \\
& \left. - \frac{3968}{729} L_{\bar{u}\bar{u}}^{V8,LR} - \frac{4832}{729} L_{\bar{u}\bar{u}}^{V8,LR} + \frac{4480}{243} L_{\bar{u}\bar{u}}^{V,RR} + \frac{4480}{243} L_{\bar{u}\bar{u}}^{V,RR} \right] + \alpha^2 \left[ -\frac{2584}{729} L_{\bar{d}\bar{u}}^{V1,LR} \right. \\
& - \frac{2584}{729} L_{\bar{d}\bar{u}}^{V1,LR} - \frac{4888}{729} L_{\bar{u}\bar{u}}^{V,LR} - \frac{4888}{729} L_{\bar{u}\bar{u}}^{V,LR} - \frac{4888}{729} L_{\bar{u}\bar{u}}^{V,LR} - \frac{4888}{729} L_{\bar{u}\bar{u}}^{V,LR} - \frac{8344}{729} L_{\bar{u}\bar{u}}^{V,RR}
\end{aligned}$$

$$\begin{aligned}
& -\frac{8344}{729}L_{22ij}^{V,RR} - \frac{8344}{729}L_{33ij}^{V,RR} - \frac{3736}{729}L_{ij11}^{V1,RR} - \frac{3736}{729}L_{ij22}^{V1,RR} + \frac{4736}{729}L_{iiij}^{V1,LR} \\
& + \frac{69248}{729}L_{jjij}^{V1,LR} - \frac{9728}{729}L_{ijii}^{V,RR} - \frac{9728}{729}L_{ijjj}^{V,RR} \Big] ;
\end{aligned}$$

$$\begin{aligned}
\dot{L}_{jjij}^{V8,LR} = & g_s^2 \left[ \frac{2}{3}L_{11ij}^{V8,LR} + \frac{2}{3}L_{22ij}^{V8,LR} + \frac{2}{3}L_{ij11}^{V8,RR} + \frac{2}{3}L_{ij22}^{V8,RR} - 12L_{jjij}^{V1,LR} \right. \\
& + \frac{2}{3}L_{iiij}^{V8,LR} - \frac{40}{3}L_{jjij}^{V8,LR} + \frac{8}{3}L_{ijii}^{V,RR} + \frac{8}{3}L_{ijjj}^{V,RR} \Big] - \frac{16}{3}e^2L_{jjij}^{V8,LR} + \alpha_s^2 \left[ -\frac{22}{3}L_{11ij}^{V1,LR} \right. \\
& - \frac{22}{3}L_{22ij}^{V1,LR} + \frac{799}{81}L_{11ij}^{V8,LR} + \frac{799}{81}L_{22ij}^{V8,LR} - \frac{2}{3}L_{ij11}^{V1,RR} - \frac{2}{3}L_{ij22}^{V1,RR} + \frac{619}{81}L_{ij11}^{V8,RR} \\
& + \frac{619}{81}L_{ij22}^{V8,RR} - \frac{22}{3}L_{iiij}^{V1,LR} - 132L_{jjij}^{V1,LR} + \frac{799}{81}L_{iiij}^{V8,LR} - \frac{25177}{162}L_{jjij}^{V8,LR} + \frac{1210}{27}L_{ijii}^{V,RR} \\
& + \frac{1210}{27}L_{ijjj}^{V,RR} \Big] + \alpha_s \alpha \left[ -\frac{520}{81}L_{11ij}^{V1,LR} - \frac{520}{81}L_{22ij}^{V1,LR} + \frac{22}{9}L_{11ij}^{V8,LR} + \frac{22}{9}L_{22ij}^{V8,LR} \right. \\
& - \frac{520}{81}L_{11ij}^{V,LR} - \frac{520}{81}L_{22ij}^{V,LR} - \frac{520}{81}L_{33ij}^{V,LR} - \frac{520}{81}L_{11ij}^{V,RR} - \frac{520}{81}L_{22ij}^{V,RR} - \frac{520}{81}L_{33ij}^{V,RR} \\
& - \frac{520}{81}L_{ij11}^{V1,RR} - \frac{520}{81}L_{ij22}^{V1,RR} + \frac{170}{27}L_{ij11}^{V8,RR} + \frac{170}{27}L_{ij22}^{V8,RR} + \frac{1040}{81}L_{iiij}^{V1,LR} \\
& + \frac{608}{81}L_{jjij}^{V1,LR} + \frac{56}{9}L_{iiij}^{V8,LR} - \frac{16}{3}L_{jjij}^{V8,LR} + \frac{1168}{81}L_{ijii}^{V,RR} + \frac{1168}{81}L_{ijjj}^{V,RR} \Big] \\
& + \frac{7168}{81}\alpha^2L_{jjij}^{V8,LR} ;
\end{aligned}$$

$$\begin{aligned}
\dot{L}_{iiij}^{V1,LR} = & -\frac{8}{3}g_s^2L_{iiij}^{V8,LR} + e^2 \left[ -\frac{8}{9}L_{11ij}^{V1,LR} - \frac{8}{9}L_{22ij}^{V1,LR} - \frac{8}{9}L_{11ij}^{V,LR} - \frac{8}{9}L_{22ij}^{V,LR} \right. \\
& - \frac{8}{9}L_{33ij}^{V,LR} - \frac{8}{9}L_{11ij}^{V,RR} - \frac{8}{9}L_{22ij}^{V,RR} - \frac{8}{9}L_{33ij}^{V,RR} - \frac{8}{9}L_{ij11}^{V1,RR} - \frac{8}{9}L_{ij22}^{V1,RR} \\
& - \frac{32}{9}L_{iiij}^{V1,LR} + \frac{16}{9}L_{jjij}^{V1,LR} + \frac{128}{27}L_{ijii}^{V,RR} + \frac{128}{27}L_{ijjj}^{V,RR} \Big] + \alpha_s^2 \left[ 8L_{11ij}^{V1,LR} \right. \\
& + 8L_{22ij}^{V1,LR} + \frac{44}{27}L_{11ij}^{V8,LR} + \frac{44}{27}L_{22ij}^{V8,LR} - 8L_{ij11}^{V1,RR} - 8L_{ij22}^{V1,RR} + \frac{44}{27}L_{ij11}^{V8,RR} \\
& + \frac{44}{27}L_{ij22}^{V8,RR} - \frac{4}{3}L_{iiij}^{V1,LR} + 8L_{jjij}^{V1,LR} - \frac{2000}{27}L_{iiij}^{V8,LR} + \frac{44}{27}L_{jjij}^{V8,LR} - \frac{232}{9}L_{ijii}^{V,RR} \\
& \left. - \frac{232}{9}L_{ijjj}^{V,RR} \right]
\end{aligned}$$

$$\begin{aligned}
& -\frac{232}{9}L_{ijjj}^{V,RR} \Big] + \alpha_s \alpha \Big[ -\frac{32}{9}L_{11ij}^{V1,LR} - \frac{32}{9}L_{22ij}^{V1,LR} + \frac{784}{729}L_{11ij}^{V8,LR} + \frac{784}{729}L_{22ij}^{V8,LR} \\
& -\frac{32}{9}L_{ud11}^{V1,RR} - \frac{32}{9}L_{ud22}^{V1,RR} - \frac{656}{729}L_{ud11}^{V8,RR} - \frac{656}{729}L_{ud22}^{V8,RR} + \frac{448}{9}L_{uu\bar{u}\bar{j}}^{V1,LR} + \frac{64}{9}L_{jj\bar{i}\bar{j}}^{V1,LR} \\
& -\frac{4832}{729}L_{uu\bar{u}\bar{j}}^{V8,LR} - \frac{3968}{729}L_{jj\bar{i}\bar{j}}^{V8,LR} + \frac{4480}{243}L_{ij\bar{i}\bar{i}}^{V,RR} + \frac{4480}{243}L_{ij\bar{j}\bar{j}}^{V,RR} \Big] + \alpha^2 \Big[ -\frac{2584}{729}L_{11ij}^{V1,LR} \\
& -\frac{2584}{729}L_{22ij}^{V1,LR} - \frac{4888}{729}L_{11ij}^{V,LR} - \frac{4888}{729}L_{22ij}^{V,LR} - \frac{4888}{729}L_{33ij}^{V,LR} - \frac{8344}{729}L_{11ij}^{V,RR} \\
& -\frac{8344}{729}L_{22ij}^{V,RR} - \frac{8344}{729}L_{33ij}^{V,RR} - \frac{3736}{729}L_{ud11}^{V1,RR} - \frac{3736}{729}L_{ud22}^{V1,RR} + \frac{69248}{729}L_{uu\bar{u}\bar{j}}^{V1,LR} \\
& + \frac{4736}{729}L_{jj\bar{i}\bar{j}}^{V1,LR} - \frac{9728}{729}L_{uu\bar{u}\bar{i}}^{V,RR} - \frac{9728}{729}L_{ij\bar{j}\bar{j}}^{V,RR} \Big] ;
\end{aligned}$$

$$\begin{aligned}
\dot{L}_{uu\bar{u}\bar{j}}^{V8,LR} &= g_s^2 \Big[ \frac{2}{3}L_{11ij}^{V8,LR} + \frac{2}{3}L_{22ij}^{V8,LR} + \frac{2}{3}L_{ud11}^{V8,RR} + \frac{2}{3}L_{ud22}^{V8,RR} - 12L_{uu\bar{u}\bar{j}}^{V1,LR} \\
& -\frac{40}{3}L_{uu\bar{u}\bar{j}}^{V8,LR} + \frac{2}{3}L_{jj\bar{i}\bar{j}}^{V8,LR} + \frac{8}{3}L_{ij\bar{i}\bar{i}}^{V,RR} + \frac{8}{3}L_{ij\bar{j}\bar{j}}^{V,RR} \Big] - \frac{16}{3}e^2L_{uu\bar{u}\bar{j}}^{V8,LR} + \alpha_s^2 \Big[ -\frac{22}{3}L_{11ij}^{V1,LR} \\
& -\frac{22}{3}L_{22ij}^{V1,LR} + \frac{799}{81}L_{11ij}^{V8,LR} + \frac{799}{81}L_{22ij}^{V8,LR} - \frac{2}{3}L_{ud11}^{V1,RR} - \frac{2}{3}L_{ud22}^{V1,RR} + \frac{619}{81}L_{ud11}^{V8,RR} \\
& + \frac{619}{81}L_{ud22}^{V8,RR} - 132L_{uu\bar{u}\bar{j}}^{V1,LR} - \frac{22}{3}L_{jj\bar{i}\bar{j}}^{V1,LR} - \frac{25177}{162}L_{uu\bar{u}\bar{j}}^{V8,LR} + \frac{799}{81}L_{jj\bar{i}\bar{j}}^{V8,LR} + \frac{1210}{27}L_{ij\bar{i}\bar{i}}^{V,RR} \\
& + \frac{1210}{27}L_{ij\bar{j}\bar{j}}^{V,RR} \Big] + \alpha_s \alpha \Big[ -\frac{520}{81}L_{11ij}^{V1,LR} - \frac{520}{81}L_{22ij}^{V1,LR} + \frac{22}{9}L_{11ij}^{V8,LR} + \frac{22}{9}L_{22ij}^{V8,LR} \\
& -\frac{520}{81}L_{11ij}^{V,LR} - \frac{520}{81}L_{22ij}^{V,LR} - \frac{520}{81}L_{33ij}^{V,LR} - \frac{520}{81}L_{11ij}^{V,RR} - \frac{520}{81}L_{22ij}^{V,RR} - \frac{520}{81}L_{33ij}^{V,RR} \\
& -\frac{520}{81}L_{ud11}^{V1,RR} - \frac{520}{81}L_{ud22}^{V1,RR} + \frac{170}{27}L_{ud11}^{V8,RR} + \frac{170}{27}L_{ud22}^{V8,RR} + \frac{608}{81}L_{uu\bar{u}\bar{j}}^{V1,LR} + \frac{1040}{81}L_{jj\bar{i}\bar{j}}^{V1,LR} \\
& -\frac{16}{3}L_{uu\bar{u}\bar{j}}^{V8,LR} + \frac{56}{9}L_{jj\bar{i}\bar{j}}^{V8,LR} + \frac{1168}{81}L_{ij\bar{i}\bar{i}}^{V,RR} + \frac{1168}{81}L_{ij\bar{j}\bar{j}}^{V,RR} \Big] + \frac{7168}{81}\alpha^2L_{uu\bar{u}\bar{j}}^{V8,LR} ;
\end{aligned}$$

$$\dot{L}_{11ij}^{V,LL} = 0 ;$$

$$\dot{L}_{22ij}^{V,LL} = 0 ;$$

$$\dot{L}_{33ij}^{V,LL} = 0 ;$$

$$\begin{aligned}
\dot{L}_{11ij}^{V,LR} &= 0 ; \\
\dot{L}_{22ij}^{V,LR} &= 0 ; \\
\dot{L}_{33ij}^{V,LR} &= 0 ; \\
\dot{L}_{11ij}^{S,LR} &= -8g_s^2 L_{11ij}^{S,LR} - \frac{8}{3}e^2 L_{11ij}^{S,LR} - \frac{1012}{9}\alpha_s^2 L_{11ij}^{S,LR} - \frac{32}{9}\alpha_s \alpha L_{11ij}^{S,LR} \\
&\quad + \frac{1472}{81}\alpha^2 L_{11ij}^{S,LR} ; \\
\dot{L}_{22ij}^{S,LR} &= -8g_s^2 L_{22ij}^{S,LR} - \frac{8}{3}e^2 L_{22ij}^{S,LR} - \frac{1012}{9}\alpha_s^2 L_{22ij}^{S,LR} - \frac{32}{9}\alpha_s \alpha L_{22ij}^{S,LR} \\
&\quad + \frac{1472}{81}\alpha^2 L_{22ij}^{S,LR} ; \\
\dot{L}_{33ij}^{S,LR} &= -8g_s^2 L_{33ij}^{S,LR} - \frac{8}{3}e^2 L_{33ij}^{S,LR} - \frac{1012}{9}\alpha_s^2 L_{33ij}^{S,LR} - \frac{32}{9}\alpha_s \alpha L_{33ij}^{S,LR} \\
&\quad + \frac{1472}{81}\alpha^2 L_{33ij}^{S,LR} ; \\
\dot{L}_{11ij}^{S,LL} &= -8g_s^2 L_{11ij}^{S,LL} - \frac{8}{3}e^2 L_{11ij}^{S,LL} - \frac{1012}{9}\alpha_s^2 L_{11ij}^{S,LL} - \frac{32}{9}\alpha_s \alpha L_{11ij}^{S,LL} \\
&\quad + \frac{1472}{81}\alpha^2 L_{11ij}^{S,LL} ; \\
\dot{L}_{11ij}^{T,LL} &= \frac{8}{3}g_s^2 L_{11ij}^{T,LL} + \frac{8}{9}e^2 L_{11ij}^{T,LL} + \frac{1652}{27}\alpha_s^2 L_{11ij}^{T,LL} - \frac{608}{27}\alpha_s \alpha L_{11ij}^{T,LL} \\
&\quad - \frac{4864}{243}\alpha^2 L_{11ij}^{T,LL} ; \\
\dot{L}_{22ij}^{S,LL} &= -8g_s^2 L_{22ij}^{S,LL} - \frac{8}{3}e^2 L_{22ij}^{S,LL} - \frac{1012}{9}\alpha_s^2 L_{22ij}^{S,LL} - \frac{32}{9}\alpha_s \alpha L_{22ij}^{S,LL} \\
&\quad + \frac{1472}{81}\alpha^2 L_{22ij}^{S,LL} ; \\
\dot{L}_{22ij}^{T,LL} &= \frac{8}{3}g_s^2 L_{22ij}^{T,LL} + \frac{8}{9}e^2 L_{22ij}^{T,LL} + \frac{1652}{27}\alpha_s^2 L_{22ij}^{T,LL} - \frac{608}{27}\alpha_s \alpha L_{22ij}^{T,LL} \\
&\quad - \frac{4864}{243}\alpha^2 L_{22ij}^{T,LL} ; \\
\dot{L}_{33ij}^{S,LL} &= -8g_s^2 L_{33ij}^{S,LL} - \frac{8}{3}e^2 L_{33ij}^{S,LL} - \frac{1012}{9}\alpha_s^2 L_{33ij}^{S,LL} - \frac{32}{9}\alpha_s \alpha L_{33ij}^{S,LL} \\
&\quad + \frac{1472}{81}\alpha^2 L_{33ij}^{S,LL} ;
\end{aligned}$$

$$\begin{aligned}\dot{L}_{33ij}^{T,LL} &= \frac{8}{3}g_s^2 L_{33ij}^{T,LL} + \frac{8}{9}e^2 L_{33ij}^{T,LL} + \frac{1652}{27}\alpha_s^2 L_{33ij}^{T,LL} - \frac{608}{27}\alpha_s \alpha L_{33ij}^{T,LL} \\ &\quad - \frac{4864}{243}\alpha^2 L_{33ij}^{T,LL};\end{aligned}$$

## 2.7 $\Delta F = 1^{ff} : e\text{-type } (\bar{e}_i e_j \bar{f}_k f_k)$

$$\begin{aligned}\dot{L}_{ij11}^{V,LL} &= e^2 \left[ \frac{16}{9} L_{ijkk}^{V,LL} + \frac{4}{9} L_{ijkk}^{V,LR} + \frac{40}{9} L_{ij11}^{V,LL} + \frac{4}{9} L_{ij22}^{V,LL} + \frac{4}{9} L_{ij11}^{V,LR} \right. \\ &\quad + \frac{4}{9} L_{ij22}^{V,LR} + \frac{16}{9} L_{ijii}^{V,LL} + \frac{16}{9} L_{ijjj}^{V,LL} + \frac{4}{9} L_{ijii}^{V,LR} + \frac{4}{9} L_{ijjj}^{V,LR} - \frac{8}{9} L_{ij11}^{V,LL} \\ &\quad \left. - \frac{8}{9} L_{ij22}^{V,LL} - \frac{8}{9} L_{ij11}^{V,LR} - \frac{8}{9} L_{ij22}^{V,LR} \right] + \alpha_s^2 \left[ 8 L_{ij11}^{V,LL} + 8 L_{ij22}^{V,LL} \right. \\ &\quad \left. - 8 L_{ij11}^{V,LR} - 8 L_{ij22}^{V,LR} + 8 L_{ij11}^{V,LL} + 8 L_{ij22}^{V,LL} - 8 L_{ij11}^{V,LR} - 8 L_{ij22}^{V,LR} \right] \\ &\quad + \alpha_s \alpha \left[ -\frac{128}{9} L_{ij11}^{V,LL} + \frac{16}{9} L_{ij22}^{V,LL} + \frac{16}{9} L_{ij11}^{V,LR} + \frac{16}{9} L_{ij22}^{V,LR} - \frac{32}{9} L_{ij11}^{V,LL} \right. \\ &\quad \left. - \frac{32}{9} L_{ij22}^{V,LL} - \frac{32}{9} L_{ij11}^{V,LR} - \frac{32}{9} L_{ij22}^{V,LR} \right] + \alpha^2 \left[ \frac{224}{81} L_{ijkk}^{V,LL} - \frac{520}{81} L_{ijkk}^{V,LR} \right. \\ &\quad - \frac{3110}{243} L_{ij11}^{V,LL} - \frac{104}{243} L_{ij22}^{V,LL} - \frac{200}{243} L_{ij11}^{V,LR} - \frac{200}{243} L_{ij22}^{V,LR} + \frac{32}{81} L_{ijii}^{V,LL} + \frac{32}{81} L_{ijjj}^{V,LL} \\ &\quad - \frac{520}{81} L_{ijii}^{V,LR} - \frac{520}{81} L_{ijjj}^{V,LR} - \frac{1016}{243} L_{ij11}^{V,LL} - \frac{1016}{243} L_{ij22}^{V,LL} - \frac{1400}{243} L_{ij11}^{V,LR} \\ &\quad \left. - \frac{1400}{243} L_{ij22}^{V,LR} \right];\end{aligned}$$

$$\begin{aligned}\dot{L}_{ij22}^{V,LL} &= e^2 \left[ \frac{16}{9} L_{ijkk}^{V,LL} + \frac{4}{9} L_{ijkk}^{V,LR} + \frac{4}{9} L_{ij11}^{V,LL} + \frac{40}{9} L_{ij22}^{V,LL} + \frac{4}{9} L_{ij11}^{V,LR} \right. \\ &\quad + \frac{4}{9} L_{ij22}^{V,LR} + \frac{16}{9} L_{ijii}^{V,LL} + \frac{16}{9} L_{ijjj}^{V,LL} + \frac{4}{9} L_{ijii}^{V,LR} + \frac{4}{9} L_{ijjj}^{V,LR} - \frac{8}{9} L_{ij11}^{V,LL} \\ &\quad \left. - \frac{8}{9} L_{ij22}^{V,LL} - \frac{8}{9} L_{ij11}^{V,LR} - \frac{8}{9} L_{ij22}^{V,LR} \right] + \alpha_s^2 \left[ 8 L_{ij11}^{V,LL} + 8 L_{ij22}^{V,LL} \right. \\ &\quad \left. - 8 L_{ij11}^{V,LR} - 8 L_{ij22}^{V,LR} + 8 L_{ij11}^{V,LL} + 8 L_{ij22}^{V,LL} - 8 L_{ij11}^{V,LR} - 8 L_{ij22}^{V,LR} \right]\end{aligned}$$

$$\begin{aligned}
& -8L_{ij11}^{V,LR} - 8L_{ij22}^{V,LR} + 8L_{ij11}^{V,LL} + 8L_{ij22}^{V,LL} - 8L_{ij11}^{V,LR} - 8L_{ij22}^{V,LR} \Big] \\
& + \alpha_s \alpha \left[ \frac{16}{9} L_{ij11}^{V,LL} - \frac{128}{9} L_{ij22}^{V,LL} + \frac{16}{9} L_{ij11}^{V,LR} + \frac{16}{9} L_{ij22}^{V,LR} - \frac{32}{9} L_{ij11}^{V,LL} \right. \\
& \quad \left. - \frac{32}{9} L_{ij22}^{V,LL} - \frac{32}{9} L_{ij11}^{V,LR} - \frac{32}{9} L_{ij22}^{V,LR} \right] + \alpha^2 \left[ \frac{224}{81} L_{ijkk}^{V,LL} - \frac{520}{81} L_{ijkk}^{V,LR} \right. \\
& \quad - \frac{104}{243} L_{ij11}^{V,LL} - \frac{3110}{243} L_{ij22}^{V,LL} - \frac{200}{243} L_{ij11}^{V,LR} - \frac{200}{243} L_{ij22}^{V,LR} + \frac{32}{81} L_{ijii}^{V,LL} + \frac{32}{81} L_{ijjj}^{V,LL} \\
& \quad - \frac{520}{81} L_{ijii}^{V,LR} - \frac{520}{81} L_{ijjj}^{V,LR} - \frac{1016}{243} L_{ij11}^{V,LL} - \frac{1016}{243} L_{ij22}^{V,LL} - \frac{1400}{243} L_{ij11}^{V,LR} \\
& \quad \left. - \frac{1400}{243} L_{ij22}^{V,LR} \right]; \\
\dot{L}_{ij11}^{V,LL} & = e^2 \left[ -\frac{32}{9} L_{ijkk}^{V,LL} - \frac{8}{9} L_{ijkk}^{V,LR} - \frac{8}{9} L_{ij11}^{V,LL} - \frac{8}{9} L_{ij22}^{V,LL} - \frac{8}{9} L_{ij11}^{V,LR} \right. \\
& \quad - \frac{8}{9} L_{ij22}^{V,LR} - \frac{32}{9} L_{ijii}^{V,LL} - \frac{32}{9} L_{ijjj}^{V,LL} - \frac{8}{9} L_{ijii}^{V,LR} - \frac{8}{9} L_{ijjj}^{V,LR} - \frac{56}{9} L_{ij11}^{V,LL} \\
& \quad \left. + \frac{16}{9} L_{ij22}^{V,LL} + \frac{16}{9} L_{ij11}^{V,LR} + \frac{16}{9} L_{ij22}^{V,LR} \right] + \alpha_s^2 \left[ 8L_{ij11}^{V,LL} + 8L_{ij22}^{V,LL} \right. \\
& \quad \left. - 8L_{ij11}^{V,LR} - 8L_{ij22}^{V,LR} + 8L_{ij11}^{V,LL} + 8L_{ij22}^{V,LL} - 8L_{ij11}^{V,LR} - 8L_{ij22}^{V,LR} \right] \\
& + \alpha_s \alpha \left[ -\frac{32}{9} L_{ij11}^{V,LL} - \frac{32}{9} L_{ij22}^{V,LL} - \frac{32}{9} L_{ij11}^{V,LR} - \frac{32}{9} L_{ij22}^{V,LR} + \frac{352}{9} L_{ij11}^{V,LL} \right. \\
& \quad \left. + \frac{64}{9} L_{ij22}^{V,LL} + \frac{64}{9} L_{ij11}^{V,LR} + \frac{64}{9} L_{ij22}^{V,LR} \right] + \alpha^2 \left[ \frac{2432}{81} L_{ijkk}^{V,LL} + \frac{464}{81} L_{ijkk}^{V,LR} \right. \\
& \quad + \frac{2512}{243} L_{ij11}^{V,LL} + \frac{2512}{243} L_{ij22}^{V,LL} + \frac{1408}{243} L_{ij11}^{V,LR} + \frac{1408}{243} L_{ij22}^{V,LR} + \frac{3680}{81} L_{ijii}^{V,LL} \\
& \quad + \frac{3680}{81} L_{ijjj}^{V,LL} + \frac{464}{81} L_{ijii}^{V,LR} + \frac{464}{81} L_{ijjj}^{V,LR} + \frac{2464}{243} L_{ij11}^{V,LL} + \frac{1312}{243} L_{ij22}^{V,LL} - \frac{3104}{243} L_{ij11}^{V,LR} \\
& \quad \left. - \frac{3104}{243} L_{ij22}^{V,LR} \right];
\end{aligned}$$



$$\begin{aligned}
\dot{L}_{ij22}^{V,LL} = & e^2 \left[ -\frac{32}{9} L_{ijkk}^{V,LL} - \frac{8}{9} L_{ijkk}^{V,LR} - \frac{8}{9} L_{ij11}^{V,LL} - \frac{8}{9} L_{ij22}^{V,LL} - \frac{8}{9} L_{ij11}^{V,LR} \right. \\
& - \frac{8}{9} L_{ij22}^{V,LR} - \frac{32}{9} L_{ijii}^{V,LL} - \frac{32}{9} L_{ijjj}^{V,LL} - \frac{8}{9} L_{ijii}^{V,LR} - \frac{8}{9} L_{ijjj}^{V,LR} + \frac{16}{9} L_{ij11}^{V,LL} \\
& \left. - \frac{56}{9} L_{ij22}^{V,LL} + \frac{16}{9} L_{ij11}^{V,LR} + \frac{16}{9} L_{ij22}^{V,LR} \right] + \alpha_s^2 \left[ 8L_{ij11}^{V,LL} + 8L_{ij22}^{V,LL} \right. \\
& \left. - 8L_{ij11}^{V,LR} - 8L_{ij22}^{V,LR} + 8L_{ij11}^{V,LL} + 8L_{ij22}^{V,LL} - 8L_{ij11}^{V,LR} - 8L_{ij22}^{V,LR} \right] \\
& + \alpha_s \alpha \left[ -\frac{32}{9} L_{ij11}^{V,LL} - \frac{32}{9} L_{ij22}^{V,LL} - \frac{32}{9} L_{ij11}^{V,LR} - \frac{32}{9} L_{ij22}^{V,LR} + \frac{64}{9} L_{ij11}^{V,LL} \right. \\
& + \frac{352}{9} L_{ij22}^{V,LL} + \frac{64}{9} L_{ij11}^{V,LR} + \frac{64}{9} L_{ij22}^{V,LR} \left. \right] + \alpha^2 \left[ \frac{2432}{81} L_{ijkk}^{V,LL} + \frac{464}{81} L_{ijkk}^{V,LR} \right. \\
& + \frac{2512}{243} L_{ij11}^{V,LL} + \frac{2512}{243} L_{ij22}^{V,LL} + \frac{1408}{243} L_{ij11}^{V,LR} + \frac{1408}{243} L_{ij22}^{V,LR} + \frac{3680}{81} L_{ijii}^{V,LL} \\
& + \frac{3680}{81} L_{ijjj}^{V,LL} + \frac{464}{81} L_{ijii}^{V,LR} + \frac{464}{81} L_{ijjj}^{V,LR} + \frac{1312}{243} L_{ij11}^{V,LL} + \frac{2464}{243} L_{ij22}^{V,LL} - \frac{3104}{243} L_{ij11}^{V,LR} \\
& \left. - \frac{3104}{243} L_{ij22}^{V,LR} \right];
\end{aligned}$$

$$\begin{aligned}
\dot{L}_{ijkk}^{V,LL} = & e^2 \left[ \frac{40}{3} L_{ijkk}^{V,LL} + \frac{1}{3} L_{ijkk}^{V,LR} + \frac{1}{3} L_{ij11}^{V,LL} + \frac{1}{3} L_{ij22}^{V,LL} + \frac{1}{3} L_{ij11}^{V,LR} \right. \\
& + \frac{1}{3} L_{ij22}^{V,LR} + \frac{4}{3} L_{ijii}^{V,LL} + \frac{4}{3} L_{ijjj}^{V,LL} + \frac{1}{3} L_{ijii}^{V,LR} + \frac{1}{3} L_{ijjj}^{V,LR} - \frac{2}{3} L_{ij11}^{V,LL} \\
& \left. - \frac{2}{3} L_{ij22}^{V,LL} - \frac{2}{3} L_{ij11}^{V,LR} - \frac{2}{3} L_{ij22}^{V,LR} \right] + \alpha_s \alpha \left[ \frac{4}{3} L_{ij11}^{V,LL} + \frac{4}{3} L_{ij22}^{V,LL} \right. \\
& + \frac{4}{3} L_{ij11}^{V,LR} + \frac{4}{3} L_{ij22}^{V,LR} - \frac{8}{3} L_{ij11}^{V,LL} - \frac{8}{3} L_{ij22}^{V,LL} - \frac{8}{3} L_{ij11}^{V,LR} - \frac{8}{3} L_{ij22}^{V,LR} \left. \right] \\
& + \alpha^2 \left[ -\frac{2326}{27} L_{ijkk}^{V,LL} - \frac{178}{27} L_{ijkk}^{V,LR} + \frac{166}{81} L_{ij11}^{V,LL} + \frac{166}{81} L_{ij22}^{V,LL} + \frac{34}{81} L_{ij11}^{V,LR} \right. \\
& \left. + \frac{34}{81} L_{ij22}^{V,LR} + \frac{320}{27} L_{ijii}^{V,LL} + \frac{320}{27} L_{ijjj}^{V,LL} - \frac{178}{27} L_{ijii}^{V,LR} - \frac{178}{27} L_{ijjj}^{V,LR} - \frac{314}{81} L_{ij11}^{V,LL} \right.
\end{aligned}$$

$$\begin{aligned}
& -\frac{314}{81}L_{ij22}^{V,LL} - \frac{842}{81}L_{ij11}^{V,LR} - \frac{842}{81}L_{ij22}^{V,LR} \Big] ; \\
\dot{L}_{ijj}^{V,LL} = & e^2 \left[ \frac{8}{3}L_{ijkk}^{V,LL} + \frac{2}{3}L_{ijkk}^{V,LR} + \frac{2}{3}L_{ij11}^{V,LL} + \frac{2}{3}L_{ij22}^{V,LL} + \frac{2}{3}L_{ij11}^{V,LR} \right. \\
& + \frac{2}{3}L_{ij22}^{V,LR} + \frac{8}{3}L_{ijii}^{V,LL} + \frac{44}{3}L_{ijjj}^{V,LL} + \frac{2}{3}L_{ijjj}^{V,LR} + \frac{2}{3}L_{ijjj}^{V,LR} - \frac{4}{3}L_{ij11}^{V,LL} \\
& \left. - \frac{4}{3}L_{ij22}^{V,LL} - \frac{4}{3}L_{ij11}^{V,LR} - \frac{4}{3}L_{ij22}^{V,LR} \right] + \alpha_s \alpha \left[ \frac{8}{3}L_{ij11}^{V,LL} + \frac{8}{3}L_{ij22}^{V,LL} \right. \\
& + \frac{8}{3}L_{ij11}^{V,LR} + \frac{8}{3}L_{ij22}^{V,LR} - \frac{16}{3}L_{ij11}^{V,LL} - \frac{16}{3}L_{ij22}^{V,LL} - \frac{16}{3}L_{ij11}^{V,LR} - \frac{16}{3}L_{ij22}^{V,LR} \Big] \\
& + \alpha^2 \left[ \frac{592}{27}L_{ijkk}^{V,LL} - \frac{356}{27}L_{ijkk}^{V,LR} + \frac{332}{81}L_{ij11}^{V,LL} + \frac{332}{81}L_{ij22}^{V,LL} + \frac{68}{81}L_{ij11}^{V,LR} \right. \\
& + \frac{68}{81}L_{ij22}^{V,LR} + \frac{640}{27}L_{ijii}^{V,LL} - \frac{1982}{27}L_{ijjj}^{V,LL} - \frac{356}{27}L_{ijii}^{V,LR} - \frac{356}{27}L_{ijjj}^{V,LR} - \frac{628}{81}L_{ij11}^{V,LL} \\
& \left. - \frac{628}{81}L_{ij22}^{V,LL} - \frac{1684}{81}L_{ij11}^{V,LR} - \frac{1684}{81}L_{ij22}^{V,LR} \right] ; \\
\dot{L}_{iji}^{V,LL} = & e^2 \left[ \frac{8}{3}L_{ijkk}^{V,LL} + \frac{2}{3}L_{ijkk}^{V,LR} + \frac{2}{3}L_{ij11}^{V,LL} + \frac{2}{3}L_{ij22}^{V,LL} + \frac{2}{3}L_{ij11}^{V,LR} \right. \\
& + \frac{2}{3}L_{ij22}^{V,LR} + \frac{44}{3}L_{ijii}^{V,LL} + \frac{8}{3}L_{ijjj}^{V,LL} + \frac{2}{3}L_{ijjj}^{V,LR} + \frac{2}{3}L_{ijjj}^{V,LR} - \frac{4}{3}L_{ij11}^{V,LL} \\
& \left. - \frac{4}{3}L_{ij22}^{V,LL} - \frac{4}{3}L_{ij11}^{V,LR} - \frac{4}{3}L_{ij22}^{V,LR} \right] + \alpha_s \alpha \left[ \frac{8}{3}L_{ij11}^{V,LL} + \frac{8}{3}L_{ij22}^{V,LL} \right. \\
& + \frac{8}{3}L_{ij11}^{V,LR} + \frac{8}{3}L_{ij22}^{V,LR} - \frac{16}{3}L_{ij11}^{V,LL} - \frac{16}{3}L_{ij22}^{V,LL} - \frac{16}{3}L_{ij11}^{V,LR} - \frac{16}{3}L_{ij22}^{V,LR} \Big] \\
& + \alpha^2 \left[ \frac{592}{27}L_{ijkk}^{V,LL} - \frac{356}{27}L_{ijkk}^{V,LR} + \frac{332}{81}L_{ij11}^{V,LL} + \frac{332}{81}L_{ij22}^{V,LL} + \frac{68}{81}L_{ij11}^{V,LR} \right. \\
& + \frac{68}{81}L_{ij22}^{V,LR} - \frac{1982}{27}L_{ijii}^{V,LL} + \frac{640}{27}L_{ijjj}^{V,LL} - \frac{356}{27}L_{ijii}^{V,LR} - \frac{356}{27}L_{ijjj}^{V,LR} - \frac{628}{81}L_{ij11}^{V,LL} \\
& \left. - \frac{628}{81}L_{ij22}^{V,LL} - \frac{1684}{81}L_{ij11}^{V,LR} - \frac{1684}{81}L_{ij22}^{V,LR} \right] ;
\end{aligned}$$

$$\begin{aligned}
\dot{L}_{ed,ij11}^{V,LR} = & e^2 \left[ \frac{16}{9} L_{ijkk}^{V,LL} + \frac{4}{9} L_{ijkk}^{V,LR} + \frac{4}{9} L_{ij11}^{V,LL} + \frac{4}{9} L_{ij22}^{V,LL} - \frac{32}{9} L_{ij11}^{V,LR} \right. \\
& + \frac{4}{9} L_{ij22}^{V,LR} + \frac{16}{9} L_{ijii}^{V,LL} + \frac{16}{9} L_{ijjj}^{V,LL} + \frac{4}{9} L_{ijii}^{V,LR} + \frac{4}{9} L_{ijjj}^{V,LR} - \frac{8}{9} L_{ij11}^{V,LL} \\
& \left. - \frac{8}{9} L_{ij22}^{V,LL} - \frac{8}{9} L_{ij11}^{V,LR} - \frac{8}{9} L_{ij22}^{V,LR} \right] + \alpha_s^2 \left[ -8 L_{ij11}^{V,LL} - 8 L_{ij22}^{V,LL} \right. \\
& + 8 L_{ij11}^{V,LR} + 8 L_{ij22}^{V,LR} - 8 L_{ij11}^{V,LL} - 8 L_{ij22}^{V,LL} + 8 L_{ij11}^{V,LR} + 8 L_{ij22}^{V,LR} \left. \right] \\
& + \alpha_s \alpha \left[ \frac{16}{9} L_{ij11}^{V,LL} + \frac{16}{9} L_{ij22}^{V,LL} + \frac{160}{9} L_{ij11}^{V,LR} + \frac{16}{9} L_{ij22}^{V,LR} - \frac{32}{9} L_{ij11}^{V,LL} \right. \\
& \left. - \frac{32}{9} L_{ij22}^{V,LL} - \frac{32}{9} L_{ij11}^{V,LR} - \frac{32}{9} L_{ij22}^{V,LR} \right] + \alpha^2 \left[ -\frac{160}{81} L_{ijkk}^{V,LL} - \frac{184}{81} L_{ijkk}^{V,LR} \right. \\
& - \frac{440}{243} L_{ij11}^{V,LL} - \frac{440}{243} L_{ij22}^{V,LL} + \frac{17050}{243} L_{ij11}^{V,LR} - \frac{104}{243} L_{ij22}^{V,LR} - \frac{640}{81} L_{ijii}^{V,LL} \\
& - \frac{640}{81} L_{ijjj}^{V,LL} - \frac{184}{81} L_{ijii}^{V,LR} - \frac{184}{81} L_{ijjj}^{V,LR} - \frac{1640}{243} L_{ij11}^{V,LL} - \frac{1640}{243} L_{ij22}^{V,LL} - \frac{296}{243} L_{ij11}^{V,LR} \\
& \left. - \frac{296}{243} L_{ij22}^{V,LR} \right];
\end{aligned}$$

$$\begin{aligned}
\dot{L}_{ed,ij22}^{V,LR} = & e^2 \left[ \frac{16}{9} L_{ijkk}^{V,LL} + \frac{4}{9} L_{ijkk}^{V,LR} + \frac{4}{9} L_{ij11}^{V,LL} + \frac{4}{9} L_{ij22}^{V,LL} + \frac{4}{9} L_{ij11}^{V,LR} \right. \\
& - \frac{32}{9} L_{ij22}^{V,LR} + \frac{16}{9} L_{ijii}^{V,LL} + \frac{16}{9} L_{ijjj}^{V,LL} + \frac{4}{9} L_{ijii}^{V,LR} + \frac{4}{9} L_{ijjj}^{V,LR} - \frac{8}{9} L_{ij11}^{V,LL} \\
& \left. - \frac{8}{9} L_{ij22}^{V,LL} - \frac{8}{9} L_{ij11}^{V,LR} - \frac{8}{9} L_{ij22}^{V,LR} \right] + \alpha_s^2 \left[ -8 L_{ij11}^{V,LL} - 8 L_{ij22}^{V,LL} \right. \\
& + 8 L_{ij11}^{V,LR} + 8 L_{ij22}^{V,LR} - 8 L_{ij11}^{V,LL} - 8 L_{ij22}^{V,LL} + 8 L_{ij11}^{V,LR} + 8 L_{ij22}^{V,LR} \left. \right] \\
& + \alpha_s \alpha \left[ \frac{16}{9} L_{ij11}^{V,LL} + \frac{16}{9} L_{ij22}^{V,LL} + \frac{16}{9} L_{ij11}^{V,LR} + \frac{160}{9} L_{ij22}^{V,LR} - \frac{32}{9} L_{ij11}^{V,LL} \right. \\
& \left. - \frac{32}{9} L_{ij22}^{V,LL} - \frac{32}{9} L_{ij11}^{V,LR} - \frac{32}{9} L_{ij22}^{V,LR} \right] + \alpha^2 \left[ -\frac{160}{81} L_{ijkk}^{V,LL} - \frac{184}{81} L_{ijkk}^{V,LR} \right.
\end{aligned}$$

$$\begin{aligned}
& -\frac{440}{243}L_{ij11}^{V,LL} - \frac{440}{243}L_{ij22}^{V,LL} - \frac{104}{243}L_{ij11}^{V,LR} + \frac{17050}{243}L_{ij22}^{V,LR} - \frac{640}{81}L_{ijii}^{V,LL} \\
& -\frac{640}{81}L_{ijjj}^{V,LL} - \frac{184}{81}L_{ijii}^{V,LR} - \frac{184}{81}L_{ijjj}^{V,LR} - \frac{1640}{243}L_{ij11}^{V,LL} - \frac{1640}{243}L_{ij22}^{V,LL} - \frac{296}{243}L_{ij11}^{V,LR} \\
& -\frac{296}{243}L_{ij22}^{V,LR} \Big] ;
\end{aligned}$$

$$\begin{aligned}
\dot{L}_{ij11}^{V,LR} = & e^2 \left[ -\frac{32}{9}L_{ijkk}^{V,LL} - \frac{8}{9}L_{ijkk}^{V,LR} - \frac{8}{9}L_{ij11}^{V,LL} - \frac{8}{9}L_{ij22}^{V,LL} - \frac{8}{9}L_{ij11}^{V,LR} \right. \\
& -\frac{8}{9}L_{ij22}^{V,LR} - \frac{32}{9}L_{ijii}^{V,LL} - \frac{32}{9}L_{ijjj}^{V,LL} - \frac{8}{9}L_{ijii}^{V,LR} - \frac{8}{9}L_{ijjj}^{V,LR} + \frac{16}{9}L_{ij11}^{V,LL} \\
& + \frac{16}{9}L_{ij22}^{V,LL} + \frac{88}{9}L_{ij11}^{V,LR} + \frac{16}{9}L_{ij22}^{V,LR} \Big] + \alpha_s^2 \left[ -8L_{ij11}^{V,LL} - 8L_{ij22}^{V,LL} \right. \\
& + 8L_{ij11}^{V,LR} + 8L_{ij22}^{V,LR} - 8L_{ij11}^{V,LL} - 8L_{ij22}^{V,LL} + 8L_{ij11}^{V,LR} + 8L_{ij22}^{V,LR} \Big] \\
& + \alpha_s \alpha \left[ -\frac{32}{9}L_{ij11}^{V,LL} - \frac{32}{9}L_{ij22}^{V,LL} - \frac{32}{9}L_{ij11}^{V,LR} - \frac{32}{9}L_{ij22}^{V,LR} + \frac{64}{9}L_{ij11}^{V,LL} \right. \\
& + \frac{64}{9}L_{ij22}^{V,LL} - \frac{224}{9}L_{ij11}^{V,LR} + \frac{64}{9}L_{ij22}^{V,LR} \Big] + \alpha^2 \left[ \frac{896}{81}L_{ijkk}^{V,LL} + \frac{1808}{81}L_{ijkk}^{V,LR} \right. \\
& + \frac{1168}{243}L_{ij11}^{V,LL} + \frac{1168}{243}L_{ij22}^{V,LL} + \frac{1792}{243}L_{ij11}^{V,LR} + \frac{1792}{243}L_{ij22}^{V,LR} + \frac{992}{81}L_{ijii}^{V,LL} \\
& + \frac{992}{81}L_{ijjj}^{V,LL} + \frac{1808}{81}L_{ijii}^{V,LR} + \frac{1808}{81}L_{ijjj}^{V,LR} - \frac{1184}{243}L_{ij11}^{V,LL} - \frac{1184}{243}L_{ij22}^{V,LL} \\
& \left. - \frac{41744}{243}L_{ij11}^{V,LR} + \frac{1312}{243}L_{ij22}^{V,LR} \right] ;
\end{aligned}$$

$$\begin{aligned}
\dot{L}_{ij22}^{V,LR} = & e^2 \left[ -\frac{32}{9}L_{ijkk}^{V,LL} - \frac{8}{9}L_{ijkk}^{V,LR} - \frac{8}{9}L_{ij11}^{V,LL} - \frac{8}{9}L_{ij22}^{V,LL} - \frac{8}{9}L_{ij11}^{V,LR} \right. \\
& -\frac{8}{9}L_{ij22}^{V,LR} - \frac{32}{9}L_{ijii}^{V,LL} - \frac{32}{9}L_{ijjj}^{V,LL} - \frac{8}{9}L_{ijii}^{V,LR} - \frac{8}{9}L_{ijjj}^{V,LR} + \frac{16}{9}L_{ij11}^{V,LL} \\
& + \frac{16}{9}L_{ij22}^{V,LL} + \frac{16}{9}L_{ij11}^{V,LR} + \frac{88}{9}L_{ij22}^{V,LR} \Big] + \alpha_s^2 \left[ -8L_{ij11}^{V,LL} - 8L_{ij22}^{V,LL} \right.
\end{aligned}$$

$$\begin{aligned}
& + 8L_{ed\,ij11}^{V,LR} + 8L_{ed\,ij22}^{V,LR} - 8L_{eu\,ij11}^{V,LL} - 8L_{eu\,ij22}^{V,LL} + 8L_{eu\,ij11}^{V,LR} + 8L_{eu\,ij22}^{V,LR} \Big] \\
& + \alpha_s \alpha \left[ -\frac{32}{9}L_{ed\,ij11}^{V,LL} - \frac{32}{9}L_{ed\,ij22}^{V,LL} - \frac{32}{9}L_{ed\,ij11}^{V,LR} - \frac{32}{9}L_{ed\,ij22}^{V,LR} + \frac{64}{9}L_{eu\,ij11}^{V,LL} \right. \\
& + \frac{64}{9}L_{eu\,ij22}^{V,LL} + \frac{64}{9}L_{eu\,ij11}^{V,LR} - \frac{224}{9}L_{eu\,ij22}^{V,LR} \Big] + \alpha^2 \left[ \frac{896}{81}L_{ee\,ijkk}^{V,LL} + \frac{1808}{81}L_{ee\,ijkk}^{V,LR} \right. \\
& + \frac{1168}{243}L_{ed\,ij11}^{V,LL} + \frac{1168}{243}L_{ed\,ij22}^{V,LL} + \frac{1792}{243}L_{ed\,ij11}^{V,LR} + \frac{1792}{243}L_{ed\,ij22}^{V,LR} + \frac{992}{81}L_{ee\,ijii}^{V,LL} \\
& + \frac{992}{81}L_{ee\,ijjj}^{V,LL} + \frac{1808}{81}L_{ee\,ijii}^{V,LR} + \frac{1808}{81}L_{ee\,ijjj}^{V,LR} - \frac{1184}{243}L_{eu\,ij11}^{V,LL} - \frac{1184}{243}L_{eu\,ij22}^{V,LL} \\
& \left. + \frac{1312}{243}L_{eu\,ij11}^{V,LR} - \frac{41744}{243}L_{eu\,ij22}^{V,LR} \right] ; \\
\dot{L}_{ee\,ijkk}^{V,LR} & = e^2 \left[ \frac{16}{3}L_{ee\,ijkk}^{V,LL} - \frac{32}{3}L_{ee\,ijkk}^{V,LR} + \frac{4}{3}L_{ed\,ij11}^{V,LL} + \frac{4}{3}L_{ed\,ij22}^{V,LL} + \frac{4}{3}L_{ed\,ij11}^{V,LR} \right. \\
& + \frac{4}{3}L_{ed\,ij22}^{V,LR} + \frac{16}{3}L_{ee\,ijii}^{V,LL} + \frac{16}{3}L_{ee\,ijjj}^{V,LL} + \frac{4}{3}L_{ee\,ijii}^{V,LR} + \frac{4}{3}L_{ee\,ijjj}^{V,LR} - \frac{8}{3}L_{eu\,ij11}^{V,LL} \\
& - \frac{8}{3}L_{eu\,ij22}^{V,LL} - \frac{8}{3}L_{eu\,ij11}^{V,LR} - \frac{8}{3}L_{eu\,ij22}^{V,LR} \Big] + \alpha_s \alpha \left[ \frac{16}{3}L_{ed\,ij11}^{V,LL} + \frac{16}{3}L_{ed\,ij22}^{V,LL} \right. \\
& + \frac{16}{3}L_{ed\,ij11}^{V,LR} + \frac{16}{3}L_{ed\,ij22}^{V,LR} - \frac{32}{3}L_{eu\,ij11}^{V,LL} - \frac{32}{3}L_{eu\,ij22}^{V,LL} - \frac{32}{3}L_{eu\,ij11}^{V,LR} - \frac{32}{3}L_{eu\,ij22}^{V,LR} \Big] \\
& + \alpha^2 \left[ \frac{32}{27}L_{ee\,ijkk}^{V,LL} + \frac{6122}{27}L_{ee\,ijkk}^{V,LR} - \frac{344}{81}L_{ed\,ij11}^{V,LL} - \frac{344}{81}L_{ed\,ij22}^{V,LL} + \frac{424}{81}L_{ed\,ij11}^{V,LR} \right. \\
& + \frac{424}{81}L_{ed\,ij22}^{V,LR} - \frac{736}{27}L_{ee\,ijii}^{V,LL} - \frac{736}{27}L_{ee\,ijjj}^{V,LL} + \frac{296}{27}L_{ee\,ijii}^{V,LR} + \frac{296}{27}L_{ee\,ijjj}^{V,LR} - \frac{3128}{81}L_{eu\,ij11}^{V,LL} \\
& \left. - \frac{3128}{81}L_{eu\,ij22}^{V,LL} - \frac{56}{81}L_{eu\,ij11}^{V,LR} - \frac{56}{81}L_{eu\,ij22}^{V,LR} \right] ; \\
\dot{L}_{ee\,ijjj}^{V,LR} & = e^2 \left[ \frac{16}{3}L_{ee\,ijkk}^{V,LL} + \frac{4}{3}L_{ee\,ijkk}^{V,LR} + \frac{4}{3}L_{ed\,ij11}^{V,LL} + \frac{4}{3}L_{ed\,ij22}^{V,LL} + \frac{4}{3}L_{ed\,ij11}^{V,LR} \right. \\
& + \frac{4}{3}L_{ed\,ij22}^{V,LR} + \frac{16}{3}L_{ee\,ijii}^{V,LL} + \frac{16}{3}L_{ee\,ijjj}^{V,LL} + \frac{4}{3}L_{ee\,ijii}^{V,LR} - \frac{32}{3}L_{ee\,ijjj}^{V,LR} - \frac{8}{3}L_{eu\,ij11}^{V,LL} \\
& \left. - \frac{8}{3}L_{eu\,ij22}^{V,LL} - \frac{8}{3}L_{eu\,ij11}^{V,LR} - \frac{8}{3}L_{eu\,ij22}^{V,LR} \right] ;
\end{aligned}$$

$$\begin{aligned}
& -\frac{8}{3}L_{ij22}^{V,LL} - \frac{8}{3}L_{ij11}^{V,LR} - \frac{8}{3}L_{ij22}^{V,LR} \Big] + \alpha_s \alpha \Big[ \frac{16}{3}L_{ij11}^{V,LL} + \frac{16}{3}L_{ij22}^{V,LL} \\
& + \frac{16}{3}L_{ij11}^{V,LR} + \frac{16}{3}L_{ij22}^{V,LR} - \frac{32}{3}L_{ij11}^{V,LL} - \frac{32}{3}L_{ij22}^{V,LL} - \frac{32}{3}L_{ij11}^{V,LR} - \frac{32}{3}L_{ij22}^{V,LR} \Big] \\
& + \alpha^2 \Big[ \frac{32}{27}L_{ijkk}^{V,LL} + \frac{296}{27}L_{ijkk}^{V,LR} - \frac{344}{81}L_{ij11}^{V,LL} - \frac{344}{81}L_{ij22}^{V,LL} + \frac{424}{81}L_{ij11}^{V,LR} \\
& + \frac{424}{81}L_{ij22}^{V,LR} - \frac{736}{27}L_{ijii}^{V,LL} - \frac{736}{27}L_{ijjj}^{V,LL} + \frac{296}{27}L_{ijii}^{V,LR} + \frac{6122}{27}L_{ijjj}^{V,LR} - \frac{3128}{81}L_{ij11}^{V,LL} \\
& - \frac{3128}{81}L_{ij22}^{V,LL} - \frac{56}{81}L_{ij11}^{V,LR} - \frac{56}{81}L_{ij22}^{V,LR} \Big] ; \\
\dot{L}_{ijii}^{V,LR} & = e^2 \Big[ \frac{16}{3}L_{ijkk}^{V,LL} + \frac{4}{3}L_{ijkk}^{V,LR} + \frac{4}{3}L_{ij11}^{V,LL} + \frac{4}{3}L_{ij22}^{V,LL} + \frac{4}{3}L_{ij11}^{V,LR} \\
& + \frac{4}{3}L_{ij22}^{V,LR} + \frac{16}{3}L_{ijii}^{V,LL} + \frac{16}{3}L_{ijjj}^{V,LL} - \frac{32}{3}L_{ijii}^{V,LR} + \frac{4}{3}L_{ijjj}^{V,LR} - \frac{8}{3}L_{ij11}^{V,LL} \\
& - \frac{8}{3}L_{ij22}^{V,LL} - \frac{8}{3}L_{ij11}^{V,LR} - \frac{8}{3}L_{ij22}^{V,LR} \Big] + \alpha_s \alpha \Big[ \frac{16}{3}L_{ij11}^{V,LL} + \frac{16}{3}L_{ij22}^{V,LL} \\
& + \frac{16}{3}L_{ij11}^{V,LR} + \frac{16}{3}L_{ij22}^{V,LR} - \frac{32}{3}L_{ij11}^{V,LL} - \frac{32}{3}L_{ij22}^{V,LL} - \frac{32}{3}L_{ij11}^{V,LR} - \frac{32}{3}L_{ij22}^{V,LR} \Big] \\
& + \alpha^2 \Big[ \frac{32}{27}L_{ijkk}^{V,LL} + \frac{296}{27}L_{ijkk}^{V,LR} - \frac{344}{81}L_{ij11}^{V,LL} - \frac{344}{81}L_{ij22}^{V,LL} + \frac{424}{81}L_{ij11}^{V,LR} \\
& + \frac{424}{81}L_{ij22}^{V,LR} - \frac{736}{27}L_{ijii}^{V,LL} - \frac{736}{27}L_{ijjj}^{V,LL} + \frac{6122}{27}L_{ijii}^{V,LR} + \frac{296}{27}L_{ijjj}^{V,LR} - \frac{3128}{81}L_{ij11}^{V,LL} \\
& - \frac{3128}{81}L_{ij22}^{V,LL} - \frac{56}{81}L_{ij11}^{V,LR} - \frac{56}{81}L_{ij22}^{V,LR} \Big] ; \\
\dot{L}_{ij11}^{S,RL} & = -8g_s^2 L_{ij11}^{S,RL} - \frac{20}{3}e^2 L_{ij11}^{S,RL} - \frac{1012}{9}\alpha_s^2 L_{ij11}^{S,RL} - \frac{8}{9}\alpha_s \alpha L_{ij11}^{S,RL} \\
& + \frac{6614}{81}\alpha^2 L_{ij11}^{S,RL} ; \\
\dot{L}_{ij22}^{S,RL} & = -8g_s^2 L_{ij22}^{S,RL} - \frac{20}{3}e^2 L_{ij22}^{S,RL} - \frac{1012}{9}\alpha_s^2 L_{ij22}^{S,RL} - \frac{8}{9}\alpha_s \alpha L_{ij22}^{S,RL} \\
& + \frac{6614}{81}\alpha^2 L_{ij22}^{S,RL} ;
\end{aligned}$$

$$\begin{aligned}
\dot{L}_{ij11}^{S,RL} &= -8g_s^2 L_{ij11}^{S,RL} - \frac{26}{3} e^2 L_{ij11}^{S,RL} - \frac{1012}{9} \alpha_s^2 L_{ij11}^{S,RL} - \frac{32}{9} \alpha_s \alpha L_{ij11}^{S,RL} \\
&\quad + \frac{473}{81} \alpha^2 L_{ij11}^{S,RL} ; \\
\dot{L}_{ij22}^{S,RL} &= -8g_s^2 L_{ij22}^{S,RL} - \frac{26}{3} e^2 L_{ij22}^{S,RL} - \frac{1012}{9} \alpha_s^2 L_{ij22}^{S,RL} - \frac{32}{9} \alpha_s \alpha L_{ij22}^{S,RL} \\
&\quad + \frac{473}{81} \alpha^2 L_{ij22}^{S,RL} ; \\
\dot{L}_{kjik}^{V,LR} &= \frac{1942}{9} \alpha^2 L_{kjik}^{V,LR} - 12e^2 L_{kjik}^{V,LR} ; \\
\dot{L}_{ij11}^{S,RR} &= -8g_s^2 L_{ij11}^{S,RR} + e^2 \left[ -\frac{20}{3} L_{ij11}^{S,RR} - 32 L_{ij11}^{T,RR} \right] - \frac{1012}{9} \alpha_s^2 L_{ij11}^{S,RR} \\
&\quad + \alpha_s \alpha \left[ \frac{1792}{9} L_{ij11}^{T,RR} - \frac{8}{9} L_{ij11}^{S,RR} \right] + \alpha^2 \left[ \frac{1682}{81} L_{ij11}^{S,RR} + 704 L_{ij11}^{T,RR} \right] ; \\
\dot{L}_{ij11}^{T,RR} &= \frac{8}{3} g_s^2 L_{ij11}^{T,RR} + e^2 \left[ \frac{20}{9} L_{ij11}^{T,RR} - \frac{2}{3} L_{ij11}^{S,RR} \right] + \frac{1652}{27} \alpha_s^2 L_{ij11}^{T,RR} \\
&\quad + \alpha_s \alpha \left[ \frac{16}{3} L_{ij11}^{S,RR} - \frac{152}{27} L_{ij11}^{T,RR} \right] + \alpha^2 \left[ \frac{364}{81} L_{ij11}^{S,RR} - \frac{6922}{243} L_{ij11}^{T,RR} \right] ; \\
\dot{L}_{ij22}^{S,RR} &= -8g_s^2 L_{ij22}^{S,RR} + e^2 \left[ -\frac{20}{3} L_{ij22}^{S,RR} - 32 L_{ij22}^{T,RR} \right] - \frac{1012}{9} \alpha_s^2 L_{ij22}^{S,RR} \\
&\quad + \alpha_s \alpha \left[ \frac{1792}{9} L_{ij22}^{T,RR} - \frac{8}{9} L_{ij22}^{S,RR} \right] + \alpha^2 \left[ \frac{1682}{81} L_{ij22}^{S,RR} + 704 L_{ij22}^{T,RR} \right] ; \\
\dot{L}_{ij22}^{T,RR} &= \frac{8}{3} g_s^2 L_{ij22}^{T,RR} + e^2 \left[ \frac{20}{9} L_{ij22}^{T,RR} - \frac{2}{3} L_{ij22}^{S,RR} \right] + \frac{1652}{27} \alpha_s^2 L_{ij22}^{T,RR} \\
&\quad + \alpha_s \alpha \left[ \frac{16}{3} L_{ij22}^{S,RR} - \frac{152}{27} L_{ij22}^{T,RR} \right] + \alpha^2 \left[ \frac{364}{81} L_{ij22}^{S,RR} - \frac{6922}{243} L_{ij22}^{T,RR} \right] ; \\
\dot{L}_{ij11}^{S,RR} &= -8g_s^2 L_{ij11}^{S,RR} + e^2 \left[ 64 L_{ij11}^{T,RR} - \frac{26}{3} L_{ij11}^{S,RR} \right] - \frac{1012}{9} \alpha_s^2 L_{ij11}^{S,RR} \\
&\quad + \alpha_s \alpha \left[ -\frac{32}{9} L_{ij11}^{S,RR} - \frac{3584}{9} L_{ij11}^{T,RR} \right] + \alpha^2 \left[ -\frac{2839}{81} L_{ij11}^{S,RR} - \frac{11264}{9} L_{ij11}^{T,RR} \right] ;
\end{aligned}$$

$$\begin{aligned}
\dot{L}_{ij11}^{T,RR} &= \frac{8}{3}g_s^2 L_{ij11}^{T,RR} + e^2 \left[ \frac{4}{3}L_{ij11}^{S,RR} + \frac{26}{9}L_{ij11}^{T,RR} \right] + \frac{1652}{27}\alpha_s^2 L_{ij11}^{T,RR} \\
&\quad + \alpha_s \alpha \left[ -\frac{32}{3}L_{ij11}^{S,RR} - \frac{608}{27}L_{ij11}^{T,RR} \right] + \alpha^2 \left[ -\frac{1376}{81}L_{ij11}^{S,RR} - \frac{20677}{243}L_{ij11}^{T,RR} \right]; \\
\dot{L}_{ij22}^{S,RR} &= -8g_s^2 L_{ij22}^{S,RR} + e^2 \left[ 64L_{ij22}^{T,RR} - \frac{26}{3}L_{ij22}^{S,RR} \right] - \frac{1012}{9}\alpha_s^2 L_{ij22}^{S,RR} \\
&\quad + \alpha_s \alpha \left[ -\frac{32}{9}L_{ij22}^{S,RR} - \frac{3584}{9}L_{ij22}^{T,RR} \right] + \alpha^2 \left[ -\frac{2839}{81}L_{ij22}^{S,RR} - \frac{11264}{9}L_{ij22}^{T,RR} \right]; \\
\dot{L}_{ij22}^{T,RR} &= \frac{8}{3}g_s^2 L_{ij22}^{T,RR} + e^2 \left[ \frac{4}{3}L_{ij22}^{S,RR} + \frac{26}{9}L_{ij22}^{T,RR} \right] + \frac{1652}{27}\alpha_s^2 L_{ij22}^{T,RR} \\
&\quad + \alpha_s \alpha \left[ -\frac{32}{3}L_{ij22}^{S,RR} - \frac{608}{27}L_{ij22}^{T,RR} \right] + \alpha^2 \left[ -\frac{1376}{81}L_{ij22}^{S,RR} - \frac{20677}{243}L_{ij22}^{T,RR} \right]; \\
\dot{L}_{ijkk}^{S,RR} &= -4e^2 L_{ijkk}^{S,RR} - \frac{5530}{27}\alpha^2 L_{ijkk}^{S,RR}; \\
\dot{L}_{ikkj}^{S,RR} &= \frac{608}{9}\alpha^2 L_{ikkj}^{S,RR} - 4e^2 L_{ikkj}^{S,RR}; \\
\dot{L}_{ijjj}^{S,RR} &= -4e^2 L_{ijjj}^{S,RR} - \frac{1853}{27}\alpha^2 L_{ijjj}^{S,RR}; \\
\dot{L}_{ijii}^{S,RR} &= -4e^2 L_{ijii}^{S,RR} - \frac{1853}{27}\alpha^2 L_{ijii}^{S,RR}; \\
\dot{L}_{edij11}^{V,RR} &= e^2 \left[ \frac{4}{9}L_{edij11}^{V,LR} + \frac{16}{9}L_{edij11}^{V,RR} + \frac{4}{9}L_{edij11}^{V,LR} + \frac{4}{9}L_{edij11}^{V,LR} + \frac{40}{9}L_{edij11}^{V,RR} \right. \\
&\quad + \frac{4}{9}L_{edij22}^{V,RR} + \frac{4}{9}L_{edij22}^{V,LR} + \frac{4}{9}L_{edij22}^{V,LR} + \frac{16}{9}L_{edij22}^{V,RR} + \frac{16}{9}L_{edij22}^{V,RR} - \frac{8}{9}L_{edij11}^{V,RR} \\
&\quad - \frac{8}{9}L_{edij22}^{V,RR} - \frac{8}{9}L_{edij22}^{V,LR} - \frac{8}{9}L_{edij22}^{V,LR} \left. \right] + \alpha_s^2 \left[ -8L_{edij11}^{V,LR} - 8L_{edij22}^{V,LR} \right. \\
&\quad + 8L_{edij11}^{V,RR} + 8L_{edij22}^{V,RR} + 8L_{edij11}^{V,RR} + 8L_{edij22}^{V,RR} - 8L_{edij11}^{V,LR} - 8L_{edij22}^{V,LR} \left. \right] \\
&\quad + \alpha_s \alpha \left[ \frac{16}{9}L_{edij11}^{V,LR} + \frac{16}{9}L_{edij22}^{V,LR} - \frac{128}{9}L_{edij11}^{V,RR} + \frac{16}{9}L_{edij22}^{V,RR} - \frac{32}{9}L_{edij11}^{V,RR} \right.
\end{aligned}$$



$$\begin{aligned}
& -\frac{32}{9}L_{ij22}^{V,RR} - \frac{32}{9}L_{11ij}^{V,LR} - \frac{32}{9}L_{22ij}^{V,LR} \Big] + \alpha^2 \Big[ -\frac{520}{81}L_{kkij}^{V,LR} + \frac{224}{81}L_{ijkk}^{V,RR} \\
& -\frac{200}{243}L_{11ij}^{V,LR} - \frac{200}{243}L_{22ij}^{V,LR} - \frac{3110}{243}L_{ij11}^{V,RR} - \frac{104}{243}L_{ij22}^{V,RR} - \frac{520}{81}L_{iiij}^{V,LR} - \frac{520}{81}L_{jjij}^{V,LR} \\
& + \frac{32}{81}L_{ijii}^{V,RR} + \frac{32}{81}L_{ijjj}^{V,RR} - \frac{1016}{243}L_{ij11}^{V,RR} - \frac{1016}{243}L_{ij22}^{V,RR} - \frac{1400}{243}L_{11ij}^{V,LR} - \frac{1400}{243}L_{22ij}^{V,LR} \Big] ; \\
\dot{L}_{ij22}^{V,RR} & = e^2 \Big[ \frac{4}{9}L_{kkij}^{V,LR} + \frac{16}{9}L_{ijkk}^{V,RR} + \frac{4}{9}L_{11ij}^{V,LR} + \frac{4}{9}L_{22ij}^{V,LR} + \frac{4}{9}L_{ij11}^{V,RR} \\
& + \frac{40}{9}L_{ij22}^{V,RR} + \frac{4}{9}L_{iiij}^{V,LR} + \frac{4}{9}L_{jjij}^{V,LR} + \frac{16}{9}L_{ijii}^{V,RR} + \frac{16}{9}L_{ijjj}^{V,RR} - \frac{8}{9}L_{ij11}^{V,RR} \\
& - \frac{8}{9}L_{ij22}^{V,RR} - \frac{8}{9}L_{11ij}^{V,LR} - \frac{8}{9}L_{22ij}^{V,LR} \Big] + \alpha_s^2 \Big[ -8L_{11ij}^{V,LR} - 8L_{22ij}^{V,LR} \\
& + 8L_{ij11}^{V,RR} + 8L_{ij22}^{V,RR} + 8L_{ij11}^{V,RR} + 8L_{ij22}^{V,RR} - 8L_{11ij}^{V,LR} - 8L_{22ij}^{V,LR} \Big] \\
& + \alpha_s \alpha \Big[ \frac{16}{9}L_{11ij}^{V,LR} + \frac{16}{9}L_{22ij}^{V,LR} + \frac{16}{9}L_{ij11}^{V,RR} - \frac{128}{9}L_{ij22}^{V,RR} - \frac{32}{9}L_{ij11}^{V,RR} \\
& - \frac{32}{9}L_{ij22}^{V,RR} - \frac{32}{9}L_{11ij}^{V,LR} - \frac{32}{9}L_{22ij}^{V,LR} \Big] + \alpha^2 \Big[ -\frac{520}{81}L_{kkij}^{V,LR} + \frac{224}{81}L_{ijkk}^{V,RR} \\
& - \frac{200}{243}L_{11ij}^{V,LR} - \frac{200}{243}L_{22ij}^{V,LR} - \frac{104}{243}L_{ij11}^{V,RR} - \frac{3110}{243}L_{ij22}^{V,RR} - \frac{520}{81}L_{iiij}^{V,LR} - \frac{520}{81}L_{jjij}^{V,LR} \\
& + \frac{32}{81}L_{ijii}^{V,RR} + \frac{32}{81}L_{ijjj}^{V,RR} - \frac{1016}{243}L_{ij11}^{V,RR} - \frac{1016}{243}L_{ij22}^{V,RR} - \frac{1400}{243}L_{11ij}^{V,LR} - \frac{1400}{243}L_{22ij}^{V,LR} \Big] ; \\
\dot{L}_{ij11}^{V,RR} & = e^2 \Big[ -\frac{8}{9}L_{kkij}^{V,LR} - \frac{32}{9}L_{ijkk}^{V,RR} - \frac{8}{9}L_{11ij}^{V,LR} - \frac{8}{9}L_{22ij}^{V,LR} - \frac{8}{9}L_{ij11}^{V,RR} \\
& - \frac{8}{9}L_{ij22}^{V,RR} - \frac{8}{9}L_{iiij}^{V,LR} - \frac{8}{9}L_{jjij}^{V,LR} - \frac{32}{9}L_{ijii}^{V,RR} - \frac{32}{9}L_{ijjj}^{V,RR} - \frac{56}{9}L_{ij11}^{V,RR} \\
& + \frac{16}{9}L_{ij22}^{V,RR} + \frac{16}{9}L_{11ij}^{V,LR} + \frac{16}{9}L_{22ij}^{V,LR} \Big] + \alpha_s^2 \Big[ -8L_{11ij}^{V,LR} - 8L_{22ij}^{V,LR} \\
& + 8L_{ij11}^{V,RR} + 8L_{ij22}^{V,RR} + 8L_{ij11}^{V,RR} + 8L_{ij22}^{V,RR} - 8L_{11ij}^{V,LR} - 8L_{22ij}^{V,LR} \Big]
\end{aligned}$$

$$\begin{aligned}
& + \alpha_s \alpha \left[ -\frac{32}{9} L_{11ij}^{V,LR} - \frac{32}{9} L_{22ij}^{V,LR} - \frac{32}{9} L_{ij11}^{V,RR} - \frac{32}{9} L_{ij22}^{V,RR} + \frac{352}{9} L_{ij11}^{V,RR} \right. \\
& + \frac{64}{9} L_{ij22}^{V,RR} + \frac{64}{9} L_{11ij}^{V,LR} + \frac{64}{9} L_{22ij}^{V,LR} \left. \right] + \alpha^2 \left[ \frac{464}{81} L_{kkij}^{V,LR} + \frac{2432}{81} L_{ijkk}^{V,RR} \right. \\
& + \frac{1408}{243} L_{11ij}^{V,LR} + \frac{1408}{243} L_{22ij}^{V,LR} + \frac{2512}{243} L_{ij11}^{V,RR} + \frac{2512}{243} L_{ij22}^{V,RR} + \frac{464}{81} L_{iiij}^{V,LR} \\
& + \frac{464}{81} L_{jjij}^{V,LR} + \frac{3680}{81} L_{ijii}^{V,RR} + \frac{3680}{81} L_{ijjj}^{V,RR} + \frac{2464}{243} L_{ij11}^{V,RR} + \frac{1312}{243} L_{ij22}^{V,RR} \\
& \left. - \frac{3104}{243} L_{11ij}^{V,LR} - \frac{3104}{243} L_{22ij}^{V,LR} \right]; \\
\dot{L}_{ij22}^{V,RR} & = e^2 \left[ -\frac{8}{9} L_{kkij}^{V,LR} - \frac{32}{9} L_{ijkk}^{V,RR} - \frac{8}{9} L_{11ij}^{V,LR} - \frac{8}{9} L_{22ij}^{V,LR} - \frac{8}{9} L_{ij11}^{V,RR} \right. \\
& - \frac{8}{9} L_{ij22}^{V,RR} - \frac{8}{9} L_{iiij}^{V,LR} - \frac{8}{9} L_{jjij}^{V,LR} - \frac{32}{9} L_{ijii}^{V,RR} - \frac{32}{9} L_{ijjj}^{V,RR} + \frac{16}{9} L_{ij11}^{V,RR} \\
& - \frac{56}{9} L_{ij22}^{V,RR} + \frac{16}{9} L_{11ij}^{V,LR} + \frac{16}{9} L_{22ij}^{V,LR} \left. \right] + \alpha_s^2 \left[ -8 L_{11ij}^{V,LR} - 8 L_{22ij}^{V,LR} \right. \\
& + 8 L_{ij11}^{V,RR} + 8 L_{ij22}^{V,RR} + 8 L_{ij11}^{V,RR} + 8 L_{ij22}^{V,RR} - 8 L_{11ij}^{V,LR} - 8 L_{22ij}^{V,LR} \left. \right] \\
& + \alpha_s \alpha \left[ -\frac{32}{9} L_{11ij}^{V,LR} - \frac{32}{9} L_{22ij}^{V,LR} - \frac{32}{9} L_{ij11}^{V,RR} - \frac{32}{9} L_{ij22}^{V,RR} + \frac{64}{9} L_{ij11}^{V,RR} \right. \\
& + \frac{352}{9} L_{ij22}^{V,RR} + \frac{64}{9} L_{11ij}^{V,LR} + \frac{64}{9} L_{22ij}^{V,LR} \left. \right] + \alpha^2 \left[ \frac{464}{81} L_{kkij}^{V,LR} + \frac{2432}{81} L_{ijkk}^{V,RR} \right. \\
& + \frac{1408}{243} L_{11ij}^{V,LR} + \frac{1408}{243} L_{22ij}^{V,LR} + \frac{2512}{243} L_{ij11}^{V,RR} + \frac{2512}{243} L_{ij22}^{V,RR} + \frac{464}{81} L_{iiij}^{V,LR} \\
& + \frac{464}{81} L_{jjij}^{V,LR} + \frac{3680}{81} L_{ijii}^{V,RR} + \frac{3680}{81} L_{ijjj}^{V,RR} + \frac{1312}{243} L_{ij11}^{V,RR} + \frac{2464}{243} L_{ij22}^{V,RR} \\
& \left. - \frac{3104}{243} L_{11ij}^{V,LR} - \frac{3104}{243} L_{22ij}^{V,LR} \right]; \\
\dot{L}_{ijkk}^{V,RR} & = e^2 \left[ \frac{1}{3} L_{kkij}^{V,LR} + \frac{40}{3} L_{ijkk}^{V,RR} + \frac{1}{3} L_{11ij}^{V,LR} + \frac{1}{3} L_{22ij}^{V,LR} + \frac{1}{3} L_{ij11}^{V,RR} \right.
\end{aligned}$$

$$\begin{aligned}
& + \frac{1}{3}L_{ij22}^{V,RR} + \frac{1}{3}L_{iij}^{V,LR} + \frac{1}{3}L_{jjij}^{V,LR} + \frac{4}{3}L_{ijii}^{V,RR} + \frac{4}{3}L_{ijjj}^{V,RR} - \frac{2}{3}L_{ij11}^{V,RR} \\
& - \frac{2}{3}L_{ij22}^{V,RR} - \frac{2}{3}L_{11ij}^{V,LR} - \frac{2}{3}L_{22ij}^{V,LR} \Big] + \alpha_s \alpha \Big[ \frac{4}{3}L_{11ij}^{V,LR} + \frac{4}{3}L_{22ij}^{V,LR} \\
& + \frac{4}{3}L_{ij11}^{V,RR} + \frac{4}{3}L_{ij22}^{V,RR} - \frac{8}{3}L_{ij11}^{V,RR} - \frac{8}{3}L_{ij22}^{V,RR} - \frac{8}{3}L_{11ij}^{V,LR} - \frac{8}{3}L_{22ij}^{V,LR} \Big] \\
& + \alpha^2 \Big[ -\frac{178}{27}L_{kkij}^{V,LR} - \frac{2326}{27}L_{ijkk}^{V,RR} + \frac{34}{81}L_{11ij}^{V,LR} + \frac{34}{81}L_{22ij}^{V,LR} + \frac{166}{81}L_{ij11}^{V,RR} \\
& + \frac{166}{81}L_{ij22}^{V,RR} - \frac{178}{27}L_{iij}^{V,LR} - \frac{178}{27}L_{jjij}^{V,LR} + \frac{320}{27}L_{ijii}^{V,RR} + \frac{320}{27}L_{ijjj}^{V,RR} - \frac{314}{81}L_{ij11}^{V,RR} \\
& - \frac{314}{81}L_{ij22}^{V,RR} - \frac{842}{81}L_{11ij}^{V,LR} - \frac{842}{81}L_{22ij}^{V,LR} \Big] ; \\
\dot{L}_{ijjj}^{V,RR} & = e^2 \Big[ \frac{2}{3}L_{kkij}^{V,LR} + \frac{8}{3}L_{ijkk}^{V,RR} + \frac{2}{3}L_{11ij}^{V,LR} + \frac{2}{3}L_{22ij}^{V,LR} + \frac{2}{3}L_{ij11}^{V,RR} \\
& + \frac{2}{3}L_{ij22}^{V,RR} + \frac{2}{3}L_{iij}^{V,LR} + \frac{2}{3}L_{jjij}^{V,LR} + \frac{8}{3}L_{ijii}^{V,RR} + \frac{44}{3}L_{ijjj}^{V,RR} - \frac{4}{3}L_{ij11}^{V,RR} \\
& - \frac{4}{3}L_{ij22}^{V,RR} - \frac{4}{3}L_{11ij}^{V,LR} - \frac{4}{3}L_{22ij}^{V,LR} \Big] + \alpha_s \alpha \Big[ \frac{8}{3}L_{11ij}^{V,LR} + \frac{8}{3}L_{22ij}^{V,LR} \\
& + \frac{8}{3}L_{ij11}^{V,RR} + \frac{8}{3}L_{ij22}^{V,RR} - \frac{16}{3}L_{ij11}^{V,RR} - \frac{16}{3}L_{ij22}^{V,RR} - \frac{16}{3}L_{11ij}^{V,LR} - \frac{16}{3}L_{22ij}^{V,LR} \Big] \\
& + \alpha^2 \Big[ -\frac{356}{27}L_{kkij}^{V,LR} + \frac{592}{27}L_{ijkk}^{V,RR} + \frac{68}{81}L_{11ij}^{V,LR} + \frac{68}{81}L_{22ij}^{V,LR} + \frac{332}{81}L_{ij11}^{V,RR} \\
& + \frac{332}{81}L_{ij22}^{V,RR} - \frac{356}{27}L_{iij}^{V,LR} - \frac{356}{27}L_{jjij}^{V,LR} + \frac{640}{27}L_{ijii}^{V,RR} - \frac{1982}{27}L_{ijjj}^{V,RR} - \frac{628}{81}L_{ij11}^{V,RR} \\
& - \frac{628}{81}L_{ij22}^{V,RR} - \frac{1684}{81}L_{11ij}^{V,LR} - \frac{1684}{81}L_{22ij}^{V,LR} \Big] ; \\
\dot{L}_{ijii}^{V,RR} & = e^2 \Big[ \frac{2}{3}L_{kkij}^{V,LR} + \frac{8}{3}L_{ijkk}^{V,RR} + \frac{2}{3}L_{11ij}^{V,LR} + \frac{2}{3}L_{22ij}^{V,LR} + \frac{2}{3}L_{ij11}^{V,RR} \\
& + \frac{2}{3}L_{ij22}^{V,RR} + \frac{2}{3}L_{iij}^{V,LR} + \frac{2}{3}L_{jjij}^{V,LR} + \frac{44}{3}L_{ijii}^{V,RR} + \frac{8}{3}L_{ijjj}^{V,RR} - \frac{4}{3}L_{ij11}^{V,RR} \\
& - \frac{4}{3}L_{ij22}^{V,RR} - \frac{4}{3}L_{11ij}^{V,LR} - \frac{4}{3}L_{22ij}^{V,LR} \Big] + \alpha_s \alpha \Big[ \frac{8}{3}L_{11ij}^{V,LR} + \frac{8}{3}L_{22ij}^{V,LR} \\
& + \frac{8}{3}L_{ij11}^{V,RR} + \frac{8}{3}L_{ij22}^{V,RR} - \frac{16}{3}L_{ij11}^{V,RR} - \frac{16}{3}L_{ij22}^{V,RR} - \frac{16}{3}L_{11ij}^{V,LR} - \frac{16}{3}L_{22ij}^{V,LR} \Big] \\
& + \alpha^2 \Big[ -\frac{356}{27}L_{kkij}^{V,LR} + \frac{592}{27}L_{ijkk}^{V,RR} + \frac{68}{81}L_{11ij}^{V,LR} + \frac{68}{81}L_{22ij}^{V,LR} + \frac{332}{81}L_{ij11}^{V,RR} \\
& + \frac{332}{81}L_{ij22}^{V,RR} - \frac{356}{27}L_{iij}^{V,LR} - \frac{356}{27}L_{jjij}^{V,LR} + \frac{640}{27}L_{ijii}^{V,RR} - \frac{1982}{27}L_{ijjj}^{V,RR} - \frac{628}{81}L_{ij11}^{V,RR} \\
& - \frac{628}{81}L_{ij22}^{V,RR} - \frac{1684}{81}L_{11ij}^{V,LR} - \frac{1684}{81}L_{22ij}^{V,LR} \Big] ;
\end{aligned}$$

$$\begin{aligned}
& -\frac{4}{3}L_{ij22}^{V,RR} - \frac{4}{3}L_{11ij}^{V,LR} - \frac{4}{3}L_{22ij}^{V,LR} \Big] + \alpha_s \alpha \Big[ \frac{8}{3}L_{11ij}^{V,LR} + \frac{8}{3}L_{22ij}^{V,LR} \\
& + \frac{8}{3}L_{edij11}^{V,RR} + \frac{8}{3}L_{ij22}^{V,RR} - \frac{16}{3}L_{ij11}^{V,RR} - \frac{16}{3}L_{ij22}^{V,RR} - \frac{16}{3}L_{11ij}^{V,LR} - \frac{16}{3}L_{22ij}^{V,LR} \Big] \\
& + \alpha^2 \Big[ -\frac{356}{27}L_{kkij}^{V,LR} + \frac{592}{27}L_{ijkk}^{V,RR} + \frac{68}{81}L_{11ij}^{V,LR} + \frac{68}{81}L_{22ij}^{V,LR} + \frac{332}{81}L_{ij11}^{V,RR} \\
& + \frac{332}{81}L_{ij22}^{V,RR} - \frac{356}{27}L_{iij}^{V,LR} - \frac{356}{27}L_{jjij}^{V,LR} - \frac{1982}{27}L_{ijii}^{V,RR} + \frac{640}{27}L_{ijjj}^{V,RR} - \frac{628}{81}L_{ij11}^{V,RR} \\
& - \frac{628}{81}L_{ij22}^{V,RR} - \frac{1684}{81}L_{11ij}^{V,LR} - \frac{1684}{81}L_{22ij}^{V,LR} \Big] ; \\
\dot{L}_{11ij}^{V,LR} & = e^2 \Big[ \frac{4}{9}L_{kkij}^{V,LR} + \frac{16}{9}L_{ijkk}^{V,RR} - \frac{32}{9}L_{11ij}^{V,LR} + \frac{4}{9}L_{22ij}^{V,LR} + \frac{4}{9}L_{ij11}^{V,RR} \\
& + \frac{4}{9}L_{ij22}^{V,RR} + \frac{4}{9}L_{iij}^{V,LR} + \frac{4}{9}L_{jjij}^{V,LR} + \frac{16}{9}L_{ijii}^{V,RR} + \frac{16}{9}L_{ijjj}^{V,RR} - \frac{8}{9}L_{ij11}^{V,RR} \\
& - \frac{8}{9}L_{ij22}^{V,RR} - \frac{8}{9}L_{11ij}^{V,LR} - \frac{8}{9}L_{22ij}^{V,LR} \Big] + \alpha_s^2 \Big[ 8L_{11ij}^{V,LR} + 8L_{22ij}^{V,LR} \\
& - 8L_{edij11}^{V,RR} - 8L_{ij22}^{V,RR} - 8L_{ij11}^{V,RR} - 8L_{ij22}^{V,RR} + 8L_{11ij}^{V,LR} + 8L_{22ij}^{V,LR} \Big] \\
& + \alpha_s \alpha \Big[ \frac{160}{9}L_{11ij}^{V,LR} + \frac{16}{9}L_{22ij}^{V,LR} + \frac{16}{9}L_{ij11}^{V,RR} + \frac{16}{9}L_{ij22}^{V,RR} - \frac{32}{9}L_{ij11}^{V,RR} \\
& - \frac{32}{9}L_{ij22}^{V,RR} - \frac{32}{9}L_{11ij}^{V,LR} - \frac{32}{9}L_{22ij}^{V,LR} \Big] + \alpha^2 \Big[ -\frac{184}{81}L_{kkij}^{V,LR} - \frac{160}{81}L_{ijkk}^{V,RR} \\
& + \frac{17050}{243}L_{11ij}^{V,LR} - \frac{104}{243}L_{22ij}^{V,LR} - \frac{440}{243}L_{ij11}^{V,RR} - \frac{440}{243}L_{ij22}^{V,RR} - \frac{184}{81}L_{iij}^{V,LR} \\
& - \frac{184}{81}L_{jjij}^{V,LR} - \frac{640}{81}L_{ijii}^{V,RR} - \frac{640}{81}L_{ijjj}^{V,RR} - \frac{1640}{243}L_{ij11}^{V,RR} - \frac{1640}{243}L_{ij22}^{V,RR} - \frac{296}{243}L_{ij11}^{V,RR} \\
& - \frac{296}{243}L_{ij22}^{V,RR} \Big] ; \\
\dot{L}_{22ij}^{V,LR} & = e^2 \Big[ \frac{4}{9}L_{kkij}^{V,LR} + \frac{16}{9}L_{ijkk}^{V,RR} + \frac{4}{9}L_{11ij}^{V,LR} - \frac{32}{9}L_{22ij}^{V,LR} + \frac{4}{9}L_{ij11}^{V,RR}
\end{aligned}$$

$$\begin{aligned}
& + \frac{4}{9}L_{ij22}^{V,RR} + \frac{4}{9}L_{iij}^{V,LR} + \frac{4}{9}L_{jjij}^{V,LR} + \frac{16}{9}L_{ijii}^{V,RR} + \frac{16}{9}L_{ijjj}^{V,RR} - \frac{8}{9}L_{ij11}^{V,RR} \\
& - \frac{8}{9}L_{ij22}^{V,RR} - \frac{8}{9}L_{11ij}^{V,LR} - \frac{8}{9}L_{22ij}^{V,LR} \Big] + \alpha_s^2 \Big[ 8L_{11ij}^{V,LR} + 8L_{22ij}^{V,LR} \\
& - 8L_{ij11}^{V,RR} - 8L_{ij22}^{V,RR} - 8L_{ij11}^{V,RR} - 8L_{ij22}^{V,RR} + 8L_{11ij}^{V,LR} + 8L_{22ij}^{V,LR} \Big] \\
& + \alpha_s \alpha \Big[ \frac{16}{9}L_{de}^{V,LR} + \frac{160}{9}L_{22ij}^{V,LR} + \frac{16}{9}L_{ij11}^{V,RR} + \frac{16}{9}L_{ij22}^{V,RR} - \frac{32}{9}L_{ij11}^{V,RR} \\
& - \frac{32}{9}L_{ij22}^{V,RR} - \frac{32}{9}L_{11ij}^{V,LR} - \frac{32}{9}L_{22ij}^{V,LR} \Big] + \alpha^2 \Big[ -\frac{184}{81}L_{kkij}^{V,LR} - \frac{160}{81}L_{ijkk}^{V,RR} \\
& - \frac{104}{243}L_{11ij}^{V,LR} + \frac{17050}{243}L_{22ij}^{V,LR} - \frac{440}{243}L_{ij11}^{V,RR} - \frac{440}{243}L_{ij22}^{V,RR} - \frac{184}{81}L_{iij}^{V,LR} \\
& - \frac{184}{81}L_{jjij}^{V,LR} - \frac{640}{81}L_{ijii}^{V,RR} - \frac{640}{81}L_{ijjj}^{V,RR} - \frac{1640}{243}L_{ij11}^{V,RR} - \frac{1640}{243}L_{ij22}^{V,RR} - \frac{296}{243}L_{11ij}^{V,LR} \\
& - \frac{296}{243}L_{22ij}^{V,LR} \Big] ;
\end{aligned}$$

$$\begin{aligned}
\dot{L}_{11ij}^{V,LR} &= e^2 \Big[ -\frac{8}{9}L_{kkij}^{V,LR} - \frac{32}{9}L_{ijkk}^{V,RR} - \frac{8}{9}L_{11ij}^{V,LR} - \frac{8}{9}L_{22ij}^{V,LR} - \frac{8}{9}L_{ij11}^{V,RR} \\
& - \frac{8}{9}L_{ij22}^{V,RR} - \frac{8}{9}L_{iij}^{V,LR} - \frac{8}{9}L_{jjij}^{V,LR} - \frac{32}{9}L_{ijii}^{V,RR} - \frac{32}{9}L_{ijjj}^{V,RR} + \frac{16}{9}L_{ij11}^{V,RR} \\
& + \frac{16}{9}L_{ij22}^{V,RR} + \frac{88}{9}L_{11ij}^{V,LR} + \frac{16}{9}L_{22ij}^{V,LR} \Big] + \alpha_s^2 \Big[ 8L_{11ij}^{V,LR} + 8L_{22ij}^{V,LR} \\
& - 8L_{ij11}^{V,RR} - 8L_{ij22}^{V,RR} - 8L_{ij11}^{V,RR} - 8L_{ij22}^{V,RR} + 8L_{11ij}^{V,LR} + 8L_{22ij}^{V,LR} \Big] \\
& + \alpha_s \alpha \Big[ -\frac{32}{9}L_{de}^{V,LR} - \frac{32}{9}L_{22ij}^{V,LR} - \frac{32}{9}L_{ij11}^{V,RR} - \frac{32}{9}L_{ij22}^{V,RR} + \frac{64}{9}L_{ij11}^{V,RR} \\
& + \frac{64}{9}L_{ij22}^{V,RR} - \frac{224}{9}L_{11ij}^{V,LR} + \frac{64}{9}L_{22ij}^{V,LR} \Big] + \alpha^2 \Big[ \frac{1808}{81}L_{kkij}^{V,LR} + \frac{896}{81}L_{ijkk}^{V,RR} \\
& + \frac{1792}{243}L_{11ij}^{V,LR} + \frac{1792}{243}L_{22ij}^{V,LR} + \frac{1168}{243}L_{ij11}^{V,RR} + \frac{1168}{243}L_{ij22}^{V,RR} + \frac{1808}{81}L_{iij}^{V,LR}
\end{aligned}$$

$$\begin{aligned}
& + \frac{1808}{81} L_{jjij}^{V,LR} + \frac{992}{81} L_{ijii}^{V,RR} + \frac{992}{81} L_{ijjj}^{V,RR} - \frac{1184}{243} L_{ij11}^{V,RR} - \frac{1184}{243} L_{ij22}^{V,RR} - \frac{41744}{243} L_{11ij}^{V,LR} \\
& + \frac{1312}{243} L_{22ij}^{V,LR} \Big] ; \\
\dot{L}_{ue22ij}^{V,LR} = & e^2 \left[ -\frac{8}{9} L_{kkij}^{V,LR} - \frac{32}{9} L_{ijkk}^{V,RR} - \frac{8}{9} L_{11ij}^{V,LR} - \frac{8}{9} L_{22ij}^{V,LR} - \frac{8}{9} L_{ij11}^{V,RR} \right. \\
& - \frac{8}{9} L_{ij22}^{V,RR} - \frac{8}{9} L_{iiij}^{V,LR} - \frac{8}{9} L_{jjij}^{V,LR} - \frac{32}{9} L_{ijii}^{V,RR} - \frac{32}{9} L_{ijjj}^{V,RR} + \frac{16}{9} L_{ij11}^{V,RR} \\
& + \frac{16}{9} L_{ij22}^{V,RR} + \frac{16}{9} L_{11ij}^{V,LR} + \frac{88}{9} L_{22ij}^{V,LR} \Big] + \alpha_s^2 \left[ 8 L_{11ij}^{V,LR} + 8 L_{22ij}^{V,LR} \right. \\
& - 8 L_{ij11}^{V,RR} - 8 L_{ij22}^{V,RR} - 8 L_{ij11}^{V,RR} - 8 L_{ij22}^{V,RR} + 8 L_{11ij}^{V,LR} + 8 L_{22ij}^{V,LR} \Big] \\
& + \alpha_s \alpha \left[ -\frac{32}{9} L_{11ij}^{V,LR} - \frac{32}{9} L_{22ij}^{V,LR} - \frac{32}{9} L_{ij11}^{V,RR} - \frac{32}{9} L_{ij22}^{V,RR} + \frac{64}{9} L_{ij11}^{V,RR} \right. \\
& + \frac{64}{9} L_{ij22}^{V,RR} + \frac{64}{9} L_{11ij}^{V,LR} - \frac{224}{9} L_{22ij}^{V,LR} \Big] + \alpha^2 \left[ \frac{1808}{81} L_{kkij}^{V,LR} + \frac{896}{81} L_{ijkk}^{V,RR} \right. \\
& + \frac{1792}{243} L_{11ij}^{V,LR} + \frac{1792}{243} L_{22ij}^{V,LR} + \frac{1168}{243} L_{ij11}^{V,RR} + \frac{1168}{243} L_{ij22}^{V,RR} + \frac{1808}{81} L_{iiij}^{V,LR} \\
& + \frac{1808}{81} L_{jjij}^{V,LR} + \frac{992}{81} L_{ijii}^{V,RR} + \frac{992}{81} L_{ijjj}^{V,RR} - \frac{1184}{243} L_{ij11}^{V,RR} - \frac{1184}{243} L_{ij22}^{V,RR} + \frac{1312}{243} L_{11ij}^{V,LR} \\
& \left. - \frac{41744}{243} L_{22ij}^{V,LR} \right] ; \\
\dot{L}_{ee kkij}^{V,LR} = & e^2 \left[ -\frac{32}{3} L_{kkij}^{V,LR} + \frac{16}{3} L_{ijkk}^{V,RR} + \frac{4}{3} L_{11ij}^{V,LR} + \frac{4}{3} L_{22ij}^{V,LR} + \frac{4}{3} L_{ij11}^{V,RR} \right. \\
& + \frac{4}{3} L_{ij22}^{V,RR} + \frac{4}{3} L_{iiij}^{V,LR} + \frac{4}{3} L_{jjij}^{V,LR} + \frac{16}{3} L_{ijii}^{V,RR} + \frac{16}{3} L_{ijjj}^{V,RR} - \frac{8}{3} L_{ij11}^{V,RR} \\
& - \frac{8}{3} L_{ij22}^{V,RR} - \frac{8}{3} L_{11ij}^{V,LR} - \frac{8}{3} L_{22ij}^{V,LR} \Big] + \alpha_s \alpha \left[ \frac{16}{3} L_{11ij}^{V,LR} + \frac{16}{3} L_{22ij}^{V,LR} \right. \\
& \left. + \frac{16}{3} L_{ij11}^{V,RR} + \frac{16}{3} L_{ij22}^{V,RR} - \frac{32}{3} L_{ij11}^{V,RR} - \frac{32}{3} L_{ij22}^{V,RR} - \frac{32}{3} L_{11ij}^{V,LR} - \frac{32}{3} L_{22ij}^{V,LR} \right]
\end{aligned}$$

$$\begin{aligned}
& + \alpha^2 \left[ \frac{6122}{27} L_{kkij}^{V,LR} + \frac{32}{27} L_{ijkk}^{V,RR} + \frac{424}{81} L_{11ij}^{V,LR} + \frac{424}{81} L_{22ij}^{V,LR} - \frac{344}{81} L_{ij11}^{V,RR} \right. \\
& - \frac{344}{81} L_{ij22}^{V,RR} + \frac{296}{27} L_{iij}^{V,LR} + \frac{296}{27} L_{jjj}^{V,LR} - \frac{736}{27} L_{ijii}^{V,RR} - \frac{736}{27} L_{ijjj}^{V,RR} - \frac{3128}{81} L_{ij11}^{V,RR} \\
& \left. - \frac{3128}{81} L_{ij22}^{V,RR} - \frac{56}{81} L_{11ij}^{V,LR} - \frac{56}{81} L_{22ij}^{V,LR} \right]; \\
\dot{L}_{jjij}^{V,LR} & = e^2 \left[ \frac{4}{3} L_{kkij}^{V,LR} + \frac{16}{3} L_{ijkk}^{V,RR} + \frac{4}{3} L_{11ij}^{V,LR} + \frac{4}{3} L_{22ij}^{V,LR} + \frac{4}{3} L_{ij11}^{V,RR} \right. \\
& + \frac{4}{3} L_{ij22}^{V,RR} + \frac{4}{3} L_{iij}^{V,LR} - \frac{32}{3} L_{jjj}^{V,LR} + \frac{16}{3} L_{ijii}^{V,RR} + \frac{16}{3} L_{ijjj}^{V,RR} - \frac{8}{3} L_{ij11}^{V,RR} \\
& - \frac{8}{3} L_{ij22}^{V,RR} - \frac{8}{3} L_{11ij}^{V,LR} - \frac{8}{3} L_{22ij}^{V,LR} \left. \right] + \alpha_s \alpha \left[ \frac{16}{3} L_{11ij}^{V,LR} + \frac{16}{3} L_{22ij}^{V,LR} \right. \\
& + \frac{16}{3} L_{ij11}^{V,RR} + \frac{16}{3} L_{ij22}^{V,RR} - \frac{32}{3} L_{ij11}^{V,RR} - \frac{32}{3} L_{ij22}^{V,RR} - \frac{32}{3} L_{11ij}^{V,LR} - \frac{32}{3} L_{22ij}^{V,LR} \left. \right] \\
& + \alpha^2 \left[ \frac{296}{27} L_{kkij}^{V,LR} + \frac{32}{27} L_{ijkk}^{V,RR} + \frac{424}{81} L_{11ij}^{V,LR} + \frac{424}{81} L_{22ij}^{V,LR} - \frac{344}{81} L_{ij11}^{V,RR} \right. \\
& - \frac{344}{81} L_{ij22}^{V,RR} + \frac{296}{27} L_{iij}^{V,LR} + \frac{6122}{27} L_{jjj}^{V,LR} - \frac{736}{27} L_{ijii}^{V,RR} - \frac{736}{27} L_{ijjj}^{V,RR} - \frac{3128}{81} L_{ij11}^{V,RR} \\
& \left. - \frac{3128}{81} L_{ij22}^{V,RR} - \frac{56}{81} L_{11ij}^{V,LR} - \frac{56}{81} L_{22ij}^{V,LR} \right]; \\
\dot{L}_{iij}^{V,LR} & = e^2 \left[ \frac{4}{3} L_{kkij}^{V,LR} + \frac{16}{3} L_{ijkk}^{V,RR} + \frac{4}{3} L_{11ij}^{V,LR} + \frac{4}{3} L_{22ij}^{V,LR} + \frac{4}{3} L_{ij11}^{V,RR} \right. \\
& + \frac{4}{3} L_{ij22}^{V,RR} - \frac{32}{3} L_{iij}^{V,LR} + \frac{4}{3} L_{jjj}^{V,LR} + \frac{16}{3} L_{ijii}^{V,RR} + \frac{16}{3} L_{ijjj}^{V,RR} - \frac{8}{3} L_{ij11}^{V,RR} \\
& - \frac{8}{3} L_{ij22}^{V,RR} - \frac{8}{3} L_{11ij}^{V,LR} - \frac{8}{3} L_{22ij}^{V,LR} \left. \right] + \alpha_s \alpha \left[ \frac{16}{3} L_{11ij}^{V,LR} + \frac{16}{3} L_{22ij}^{V,LR} \right. \\
& + \frac{16}{3} L_{ij11}^{V,RR} + \frac{16}{3} L_{ij22}^{V,RR} - \frac{32}{3} L_{ij11}^{V,RR} - \frac{32}{3} L_{ij22}^{V,RR} - \frac{32}{3} L_{11ij}^{V,LR} - \frac{32}{3} L_{22ij}^{V,LR} \left. \right] \\
& + \alpha^2 \left[ \frac{296}{27} L_{kkij}^{V,LR} + \frac{32}{27} L_{ijkk}^{V,RR} + \frac{424}{81} L_{11ij}^{V,LR} + \frac{424}{81} L_{22ij}^{V,LR} - \frac{344}{81} L_{ij11}^{V,RR} \right.
\end{aligned}$$

$$\begin{aligned}
& -\frac{344}{81}L_{ij22}^{V,RR} + \frac{6122}{27}L_{iiij}^{V,LR} + \frac{296}{27}L_{jjij}^{V,LR} - \frac{736}{27}L_{ijii}^{V,RR} - \frac{736}{27}L_{ijjj}^{V,RR} - \frac{3128}{81}L_{ij11}^{V,RR} \\
& -\frac{3128}{81}L_{ij22}^{V,RR} - \frac{56}{81}L_{11ij}^{V,LR} - \frac{56}{81}L_{22ij}^{V,LR} \Bigg] ;
\end{aligned}$$

$$\begin{aligned}
\dot{L}_{jkki}^{V,LR} &= -8g_s^2 L_{jkki}^{V,LR} - \frac{20}{3}e^2 L_{jkki}^{V,LR} - \frac{1012}{9}\alpha_s^2 L_{jkki}^{V,LR} - \frac{8}{9}\alpha_s \alpha L_{jkki}^{V,LR} \\
&+ \frac{1682}{81}\alpha^2 L_{jkki}^{V,LR} ;
\end{aligned}$$

$$\dot{L}_{11ij}^{V,LL} = 0 ;$$

$$\dot{L}_{22ij}^{V,LL} = 0 ;$$

$$\dot{L}_{33ij}^{V,LL} = 0 ;$$

$$\dot{L}_{11ij}^{V,LR} = 0 ;$$

$$\dot{L}_{22ij}^{V,LR} = 0 ;$$

$$\dot{L}_{33ij}^{V,LR} = 0 ;$$

$$\dot{L}_{11ij}^{S,LR} = \frac{353}{9}\alpha^2 L_{11ij}^{S,LR} - 6e^2 L_{11ij}^{S,LR} ;$$

$$\dot{L}_{22ij}^{S,LR} = \frac{353}{9}\alpha^2 L_{22ij}^{S,LR} - 6e^2 L_{22ij}^{S,LR} ;$$

$$\dot{L}_{33ij}^{S,LR} = \frac{353}{9}\alpha^2 L_{33ij}^{S,LR} - 6e^2 L_{33ij}^{S,LR} ;$$

$$\dot{L}_{11ij}^{S,LL} = \frac{353}{9}\alpha^2 L_{11ij}^{S,LL} - 6e^2 L_{11ij}^{S,LL} ;$$

$$\dot{L}_{11ij}^{T,LL} = 2e^2 L_{11ij}^{T,LL} - \frac{1501}{27}\alpha^2 L_{11ij}^{T,LL} ;$$

$$\dot{L}_{22ij}^{S,LL} = \frac{353}{9}\alpha^2 L_{22ij}^{S,LL} - 6e^2 L_{22ij}^{S,LL} ;$$

$$\dot{L}_{22ij}^{T,LL} = 2e^2 L_{22ij}^{T,LL} - \frac{1501}{27}\alpha^2 L_{22ij}^{T,LL} ;$$

$$\dot{L}_{33ij}^{S,LL} = \frac{353}{9}\alpha^2 L_{33ij}^{S,LL} - 6e^2 L_{33ij}^{S,LL} ;$$

$$\dot{L}_{33ij}^{T,LL} = 2e^2 L_{33ij}^{T,LL} - \frac{1501}{27}\alpha^2 L_{33ij}^{T,LL} ;$$



## 2.8 $\Delta F = 1^{\bar{f}f} : \nu\text{-type } (\bar{\nu}_i \nu_j \bar{f}_k f_k)$

$$\begin{aligned}
\dot{L}_{ij11}^{V,LL} = & e^2 \left[ \frac{4}{3} L_{\nu d, ij11}^{V,LL} + \frac{4}{3} L_{\nu d, ij22}^{V,LL} + \frac{4}{3} L_{\nu d, ij11}^{V,LR} + \frac{4}{3} L_{\nu d, ij22}^{V,LR} + \frac{4}{3} L_{\nu e, ij11}^{V,LL} \right. \\
& + \frac{4}{3} L_{\nu e, ij22}^{V,LL} + \frac{4}{3} L_{\nu e, ij33}^{V,LL} + \frac{4}{3} L_{\nu e, ij11}^{V,LR} + \frac{4}{3} L_{\nu e, ij22}^{V,LR} + \frac{4}{3} L_{\nu e, ij33}^{V,LR} - \frac{8}{3} L_{\nu u, ij11}^{V,LL} \\
& - \frac{8}{3} L_{\nu u, ij22}^{V,LL} - \frac{8}{3} L_{\nu u, ij11}^{V,LR} - \frac{8}{3} L_{\nu u, ij22}^{V,LR} \left. \right] + \alpha_s \alpha \left[ \frac{16}{3} L_{\nu d, ij11}^{V,LL} + \frac{16}{3} L_{\nu d, ij22}^{V,LL} \right. \\
& + \frac{16}{3} L_{\nu d, ij11}^{V,LR} + \frac{16}{3} L_{\nu d, ij22}^{V,LR} - \frac{32}{3} L_{\nu u, ij11}^{V,LL} - \frac{32}{3} L_{\nu u, ij22}^{V,LL} - \frac{32}{3} L_{\nu u, ij11}^{V,LR} - \frac{32}{3} L_{\nu u, ij22}^{V,LR} \left. \right] \\
& + \alpha^2 \left[ \frac{40}{9} L_{\nu d, ij11}^{V,LL} + \frac{40}{9} L_{\nu d, ij22}^{V,LL} - \frac{32}{9} L_{\nu d, ij11}^{V,LR} - \frac{32}{9} L_{\nu d, ij22}^{V,LR} + 16 L_{\nu e, ij11}^{V,LL} \right. \\
& + 16 L_{\nu e, ij22}^{V,LL} + 16 L_{\nu e, ij33}^{V,LL} - 8 L_{\nu e, ij11}^{V,LR} - 8 L_{\nu e, ij22}^{V,LR} - 8 L_{\nu e, ij33}^{V,LR} + \frac{112}{9} L_{\nu u, ij11}^{V,LL} \\
& + \frac{112}{9} L_{\nu u, ij22}^{V,LL} - \frac{176}{9} L_{\nu u, ij11}^{V,LR} - \frac{176}{9} L_{\nu u, ij22}^{V,LR} \left. \right];
\end{aligned}$$

$$\begin{aligned}
\dot{L}_{ij22}^{V,LL} = & e^2 \left[ \frac{4}{3} L_{\nu d, ij11}^{V,LL} + \frac{4}{3} L_{\nu d, ij22}^{V,LL} + \frac{4}{3} L_{\nu d, ij11}^{V,LR} + \frac{4}{3} L_{\nu d, ij22}^{V,LR} + \frac{4}{3} L_{\nu e, ij11}^{V,LL} \right. \\
& + \frac{4}{3} L_{\nu e, ij22}^{V,LL} + \frac{4}{3} L_{\nu e, ij33}^{V,LL} + \frac{4}{3} L_{\nu e, ij11}^{V,LR} + \frac{4}{3} L_{\nu e, ij22}^{V,LR} + \frac{4}{3} L_{\nu e, ij33}^{V,LR} - \frac{8}{3} L_{\nu u, ij11}^{V,LL} \\
& - \frac{8}{3} L_{\nu u, ij22}^{V,LL} - \frac{8}{3} L_{\nu u, ij11}^{V,LR} - \frac{8}{3} L_{\nu u, ij22}^{V,LR} \left. \right] + \alpha_s \alpha \left[ \frac{16}{3} L_{\nu d, ij11}^{V,LL} + \frac{16}{3} L_{\nu d, ij22}^{V,LL} \right. \\
& + \frac{16}{3} L_{\nu d, ij11}^{V,LR} + \frac{16}{3} L_{\nu d, ij22}^{V,LR} - \frac{32}{3} L_{\nu u, ij11}^{V,LL} - \frac{32}{3} L_{\nu u, ij22}^{V,LL} - \frac{32}{3} L_{\nu u, ij11}^{V,LR} - \frac{32}{3} L_{\nu u, ij22}^{V,LR} \left. \right] \\
& + \alpha^2 \left[ \frac{40}{9} L_{\nu d, ij11}^{V,LL} + \frac{40}{9} L_{\nu d, ij22}^{V,LL} - \frac{32}{9} L_{\nu d, ij11}^{V,LR} - \frac{32}{9} L_{\nu d, ij22}^{V,LR} + 16 L_{\nu e, ij11}^{V,LL} \right. \\
& + 16 L_{\nu e, ij22}^{V,LL} + 16 L_{\nu e, ij33}^{V,LL} - 8 L_{\nu e, ij11}^{V,LR} - 8 L_{\nu e, ij22}^{V,LR} - 8 L_{\nu e, ij33}^{V,LR} + \frac{112}{9} L_{\nu u, ij11}^{V,LL} \\
& + \frac{112}{9} L_{\nu u, ij22}^{V,LL} - \frac{176}{9} L_{\nu u, ij11}^{V,LR} - \frac{176}{9} L_{\nu u, ij22}^{V,LR} \left. \right];
\end{aligned}$$

$$\begin{aligned}
\dot{L}_{ij33}^{V,LL} = & e^2 \left[ \frac{4}{3} L_{ij11}^{V,LL} + \frac{4}{3} L_{ij22}^{V,LL} + \frac{4}{3} L_{ij11}^{V,LR} + \frac{4}{3} L_{ij22}^{V,LR} + \frac{4}{3} L_{ij11}^{V,LL} \right. \\
& + \frac{4}{3} L_{ij22}^{V,LL} + \frac{4}{3} L_{ij33}^{V,LL} + \frac{4}{3} L_{ij11}^{V,LR} + \frac{4}{3} L_{ij22}^{V,LR} + \frac{4}{3} L_{ij33}^{V,LR} - \frac{8}{3} L_{ij11}^{V,LL} \\
& \left. - \frac{8}{3} L_{ij22}^{V,LL} - \frac{8}{3} L_{ij11}^{V,LR} - \frac{8}{3} L_{ij22}^{V,LR} \right] + \alpha_s \alpha \left[ \frac{16}{3} L_{ij11}^{V,LL} + \frac{16}{3} L_{ij22}^{V,LL} \right. \\
& + \frac{16}{3} L_{ij11}^{V,LR} + \frac{16}{3} L_{ij22}^{V,LR} - \frac{32}{3} L_{ij11}^{V,LL} - \frac{32}{3} L_{ij22}^{V,LL} - \frac{32}{3} L_{ij11}^{V,LR} - \frac{32}{3} L_{ij22}^{V,LR} \left. \right] \\
& + \alpha^2 \left[ \frac{40}{9} L_{ij11}^{V,LL} + \frac{40}{9} L_{ij22}^{V,LL} - \frac{32}{9} L_{ij11}^{V,LR} - \frac{32}{9} L_{ij22}^{V,LR} + 16 L_{ij11}^{V,LL} \right. \\
& + 16 L_{ij22}^{V,LL} + 16 L_{ij33}^{V,LL} - 8 L_{ij11}^{V,LR} - 8 L_{ij22}^{V,LR} - 8 L_{ij33}^{V,LR} + \frac{112}{9} L_{ij11}^{V,LL} \\
& \left. + \frac{112}{9} L_{ij22}^{V,LL} - \frac{176}{9} L_{ij11}^{V,LR} - \frac{176}{9} L_{ij22}^{V,LR} \right];
\end{aligned}$$

$$\begin{aligned}
\dot{L}_{ij11}^{V,LL} = & e^2 \left[ \frac{4}{9} L_{ij11}^{V,LL} + \frac{4}{9} L_{ij22}^{V,LL} + \frac{4}{9} L_{ij11}^{V,LR} + \frac{4}{9} L_{ij22}^{V,LR} + \frac{4}{9} L_{ij11}^{V,LL} \right. \\
& + \frac{4}{9} L_{ij22}^{V,LL} + \frac{4}{9} L_{ij33}^{V,LL} + \frac{4}{9} L_{ij11}^{V,LR} + \frac{4}{9} L_{ij22}^{V,LR} + \frac{4}{9} L_{ij33}^{V,LR} - \frac{8}{9} L_{ij11}^{V,LL} \\
& \left. - \frac{8}{9} L_{ij22}^{V,LL} - \frac{8}{9} L_{ij11}^{V,LR} - \frac{8}{9} L_{ij22}^{V,LR} \right] + \alpha_s^2 \left[ 8 L_{ij11}^{V,LL} + 8 L_{ij22}^{V,LL} \right. \\
& - 8 L_{ij11}^{V,LR} - 8 L_{ij22}^{V,LR} + 8 L_{ij11}^{V,LL} + 8 L_{ij22}^{V,LL} - 8 L_{ij11}^{V,LR} - 8 L_{ij22}^{V,LR} \left. \right] \\
& + \alpha_s \alpha \left[ \frac{16}{9} L_{ij11}^{V,LL} + \frac{16}{9} L_{ij22}^{V,LL} + \frac{16}{9} L_{ij11}^{V,LR} + \frac{16}{9} L_{ij22}^{V,LR} - \frac{32}{9} L_{ij11}^{V,LL} \right. \\
& - \frac{32}{9} L_{ij22}^{V,LL} - \frac{32}{9} L_{ij11}^{V,LR} - \frac{32}{9} L_{ij22}^{V,LR} \left. \right] + \alpha^2 \left[ \frac{16}{27} L_{ij11}^{V,LL} + \frac{16}{27} L_{ij22}^{V,LL} \right. \\
& - \frac{8}{27} L_{ij11}^{V,LR} - \frac{8}{27} L_{ij22}^{V,LR} + \frac{8}{3} L_{ij11}^{V,LL} + \frac{8}{3} L_{ij22}^{V,LL} + \frac{8}{3} L_{ij33}^{V,LL} + \frac{16}{27} L_{ij11}^{V,LL} \\
& \left. + \frac{16}{27} L_{ij22}^{V,LL} - \frac{80}{27} L_{ij11}^{V,LR} - \frac{80}{27} L_{ij22}^{V,LR} \right];
\end{aligned}$$

$$\begin{aligned}
\dot{L}_{ij22}^{V,LL} = & e^2 \left[ \frac{4}{9} L_{ij11}^{V,LL} + \frac{4}{9} L_{ij22}^{V,LL} + \frac{4}{9} L_{ij11}^{V,LR} + \frac{4}{9} L_{ij22}^{V,LR} + \frac{4}{9} L_{ij11}^{V,LL} \right. \\
& + \frac{4}{9} L_{ij22}^{V,LL} + \frac{4}{9} L_{ij33}^{V,LL} + \frac{4}{9} L_{ij11}^{V,LR} + \frac{4}{9} L_{ij22}^{V,LR} + \frac{4}{9} L_{ij33}^{V,LR} - \frac{8}{9} L_{ij11}^{V,LL} \\
& \left. - \frac{8}{9} L_{ij22}^{V,LL} - \frac{8}{9} L_{ij11}^{V,LR} - \frac{8}{9} L_{ij22}^{V,LR} \right] + \alpha_s^2 \left[ 8 L_{ij11}^{V,LL} + 8 L_{ij22}^{V,LL} \right. \\
& \left. - 8 L_{ij11}^{V,LR} - 8 L_{ij22}^{V,LR} + 8 L_{ij11}^{V,LL} + 8 L_{ij22}^{V,LL} - 8 L_{ij11}^{V,LR} - 8 L_{ij22}^{V,LR} \right] \\
& + \alpha_s \alpha \left[ \frac{16}{9} L_{ij11}^{V,LL} + \frac{16}{9} L_{ij22}^{V,LL} + \frac{16}{9} L_{ij11}^{V,LR} + \frac{16}{9} L_{ij22}^{V,LR} - \frac{32}{9} L_{ij11}^{V,LL} \right. \\
& \left. - \frac{32}{9} L_{ij22}^{V,LL} - \frac{32}{9} L_{ij11}^{V,LR} - \frac{32}{9} L_{ij22}^{V,LR} \right] + \alpha^2 \left[ \frac{16}{27} L_{ij11}^{V,LL} + \frac{16}{27} L_{ij22}^{V,LL} \right. \\
& - \frac{8}{27} L_{ij11}^{V,LR} - \frac{8}{27} L_{ij22}^{V,LR} + \frac{8}{3} L_{ij11}^{V,LL} + \frac{8}{3} L_{ij22}^{V,LL} + \frac{8}{3} L_{ij33}^{V,LL} + \frac{16}{27} L_{ij11}^{V,LL} \\
& \left. + \frac{16}{27} L_{ij22}^{V,LL} - \frac{80}{27} L_{ij11}^{V,LR} - \frac{80}{27} L_{ij22}^{V,LR} \right];
\end{aligned}$$

$$\begin{aligned}
\dot{L}_{ij11}^{V,LL} = & e^2 \left[ -\frac{8}{9} L_{ij11}^{V,LL} - \frac{8}{9} L_{ij22}^{V,LL} - \frac{8}{9} L_{ij11}^{V,LR} - \frac{8}{9} L_{ij22}^{V,LR} - \frac{8}{9} L_{ij11}^{V,LL} \right. \\
& - \frac{8}{9} L_{ij22}^{V,LL} - \frac{8}{9} L_{ij33}^{V,LL} - \frac{8}{9} L_{ij11}^{V,LR} - \frac{8}{9} L_{ij22}^{V,LR} - \frac{8}{9} L_{ij33}^{V,LR} + \frac{16}{9} L_{ij11}^{V,LL} \\
& \left. + \frac{16}{9} L_{ij22}^{V,LL} + \frac{16}{9} L_{ij11}^{V,LR} + \frac{16}{9} L_{ij22}^{V,LR} \right] + \alpha_s^2 \left[ 8 L_{ij11}^{V,LL} + 8 L_{ij22}^{V,LL} \right. \\
& \left. - 8 L_{ij11}^{V,LR} - 8 L_{ij22}^{V,LR} + 8 L_{ij11}^{V,LL} + 8 L_{ij22}^{V,LL} - 8 L_{ij11}^{V,LR} - 8 L_{ij22}^{V,LR} \right] \\
& + \alpha_s \alpha \left[ -\frac{32}{9} L_{ij11}^{V,LL} - \frac{32}{9} L_{ij22}^{V,LL} - \frac{32}{9} L_{ij11}^{V,LR} - \frac{32}{9} L_{ij22}^{V,LR} + \frac{64}{9} L_{ij11}^{V,LL} \right. \\
& \left. + \frac{64}{9} L_{ij22}^{V,LL} + \frac{64}{9} L_{ij11}^{V,LR} + \frac{64}{9} L_{ij22}^{V,LR} \right] + \alpha^2 \left[ \frac{40}{27} L_{ij11}^{V,LL} + \frac{40}{27} L_{ij22}^{V,LL} \right. \\
& \left. - \frac{56}{27} L_{ij11}^{V,LR} - \frac{56}{27} L_{ij22}^{V,LR} + \frac{8}{3} L_{ij11}^{V,LL} + \frac{8}{3} L_{ij22}^{V,LL} + \frac{8}{3} L_{ij33}^{V,LL} - 8 L_{ij11}^{V,LR} \right]
\end{aligned}$$

$$\begin{aligned}
& -8L_{ij22}^{V,LR} - 8L_{ij33}^{V,LR} + \frac{256}{27}L_{ij11}^{V,LL} + \frac{256}{27}L_{ij22}^{V,LL} - \frac{128}{27}L_{ij11}^{V,LR} \\
& - \frac{128}{27}L_{ij22}^{V,LR} \Big] ; \\
\dot{L}_{ij22}^{V,LL} &= e^2 \Bigg[ -\frac{8}{9}L_{ij11}^{V,LL} - \frac{8}{9}L_{ij22}^{V,LL} - \frac{8}{9}L_{ij11}^{V,LR} - \frac{8}{9}L_{ij22}^{V,LR} - \frac{8}{9}L_{ij11}^{V,LL} \\
& - \frac{8}{9}L_{ij22}^{V,LL} - \frac{8}{9}L_{ij33}^{V,LL} - \frac{8}{9}L_{ij11}^{V,LR} - \frac{8}{9}L_{ij22}^{V,LR} - \frac{8}{9}L_{ij33}^{V,LR} + \frac{16}{9}L_{ij11}^{V,LL} \\
& + \frac{16}{9}L_{ij22}^{V,LL} + \frac{16}{9}L_{ij11}^{V,LR} + \frac{16}{9}L_{ij22}^{V,LR} \Big] + \alpha_s^2 \Bigg[ 8L_{ij11}^{V,LL} + 8L_{ij22}^{V,LL} \\
& - 8L_{ij11}^{V,LR} - 8L_{ij22}^{V,LR} + 8L_{ij11}^{V,LL} + 8L_{ij22}^{V,LL} - 8L_{ij11}^{V,LR} - 8L_{ij22}^{V,LR} \Big] \\
& + \alpha_s \alpha \Bigg[ -\frac{32}{9}L_{ij11}^{V,LL} - \frac{32}{9}L_{ij22}^{V,LL} - \frac{32}{9}L_{ij11}^{V,LR} - \frac{32}{9}L_{ij22}^{V,LR} + \frac{64}{9}L_{ij11}^{V,LL} \\
& + \frac{64}{9}L_{ij22}^{V,LL} + \frac{64}{9}L_{ij11}^{V,LR} + \frac{64}{9}L_{ij22}^{V,LR} \Big] + \alpha^2 \Bigg[ \frac{40}{27}L_{ij11}^{V,LL} + \frac{40}{27}L_{ij22}^{V,LL} \\
& - \frac{56}{27}L_{ij11}^{V,LR} - \frac{56}{27}L_{ij22}^{V,LR} + \frac{8}{3}L_{ij11}^{V,LL} + \frac{8}{3}L_{ij22}^{V,LL} + \frac{8}{3}L_{ij33}^{V,LL} - 8L_{ij11}^{V,LR} \\
& - 8L_{ij22}^{V,LR} - 8L_{ij33}^{V,LR} + \frac{256}{27}L_{ij11}^{V,LL} + \frac{256}{27}L_{ij22}^{V,LL} - \frac{128}{27}L_{ij11}^{V,LR} \\
& - \frac{128}{27}L_{ij22}^{V,LR} \Big] ; \\
\dot{L}_{ij11}^{V,LR} &= e^2 \Bigg[ \frac{4}{3}L_{ij11}^{V,LL} + \frac{4}{3}L_{ij22}^{V,LL} + \frac{4}{3}L_{ij11}^{V,LR} + \frac{4}{3}L_{ij22}^{V,LR} + \frac{4}{3}L_{ij11}^{V,LL} \\
& + \frac{4}{3}L_{ij22}^{V,LL} + \frac{4}{3}L_{ij33}^{V,LL} + \frac{4}{3}L_{ij11}^{V,LR} + \frac{4}{3}L_{ij22}^{V,LR} + \frac{4}{3}L_{ij33}^{V,LR} - \frac{8}{3}L_{ij11}^{V,LL} \\
& - \frac{8}{3}L_{ij22}^{V,LL} - \frac{8}{3}L_{ij11}^{V,LR} - \frac{8}{3}L_{ij22}^{V,LR} \Big] + \alpha_s \alpha \Bigg[ \frac{16}{3}L_{ij11}^{V,LL} + \frac{16}{3}L_{ij22}^{V,LL} \\
& + \frac{16}{3}L_{ij11}^{V,LR} + \frac{16}{3}L_{ij22}^{V,LR} - \frac{32}{3}L_{ij11}^{V,LL} - \frac{32}{3}L_{ij22}^{V,LL} - \frac{32}{3}L_{ij11}^{V,LR} - \frac{32}{3}L_{ij22}^{V,LR} \Big]
\end{aligned}$$

$$\begin{aligned}
& + \alpha^2 \left[ -\frac{32}{9} L_{ij11}^{V,LL} - \frac{32}{9} L_{ij22}^{V,LL} + \frac{40}{9} L_{ij11}^{V,LR} + \frac{40}{9} L_{ij22}^{V,LR} - 8 L_{ij11}^{V,LL} \right. \\
& - 8 L_{ij22}^{V,LL} - 8 L_{ij33}^{V,LL} + 16 L_{ij11}^{V,LR} + 16 L_{ij22}^{V,LR} + 16 L_{ij33}^{V,LR} - \frac{176}{9} L_{ij11}^{V,LL} \\
& \left. - \frac{176}{9} L_{ij22}^{V,LL} + \frac{112}{9} L_{ij11}^{V,LR} + \frac{112}{9} L_{ij22}^{V,LR} \right];
\end{aligned}$$

$$\begin{aligned}
\dot{L}_{ij22}^{V,LR} &= e^2 \left[ \frac{4}{3} L_{ij11}^{V,LL} + \frac{4}{3} L_{ij22}^{V,LL} + \frac{4}{3} L_{ij11}^{V,LR} + \frac{4}{3} L_{ij22}^{V,LR} + \frac{4}{3} L_{ij11}^{V,LL} \right. \\
& + \frac{4}{3} L_{ij22}^{V,LL} + \frac{4}{3} L_{ij33}^{V,LL} + \frac{4}{3} L_{ij11}^{V,LR} + \frac{4}{3} L_{ij22}^{V,LR} + \frac{4}{3} L_{ij33}^{V,LR} - \frac{8}{3} L_{ij11}^{V,LL} \\
& \left. - \frac{8}{3} L_{ij22}^{V,LL} - \frac{8}{3} L_{ij11}^{V,LR} - \frac{8}{3} L_{ij22}^{V,LR} \right] + \alpha_s \alpha \left[ \frac{16}{3} L_{ij11}^{V,LL} + \frac{16}{3} L_{ij22}^{V,LL} \right. \\
& + \frac{16}{3} L_{ij11}^{V,LR} + \frac{16}{3} L_{ij22}^{V,LR} - \frac{32}{3} L_{ij11}^{V,LL} - \frac{32}{3} L_{ij22}^{V,LL} - \frac{32}{3} L_{ij11}^{V,LR} - \frac{32}{3} L_{ij22}^{V,LR} \\
& + \alpha^2 \left[ -\frac{32}{9} L_{ij11}^{V,LL} - \frac{32}{9} L_{ij22}^{V,LL} + \frac{40}{9} L_{ij11}^{V,LR} + \frac{40}{9} L_{ij22}^{V,LR} - 8 L_{ij11}^{V,LL} \right. \\
& - 8 L_{ij22}^{V,LL} - 8 L_{ij33}^{V,LL} + 16 L_{ij11}^{V,LR} + 16 L_{ij22}^{V,LR} + 16 L_{ij33}^{V,LR} - \frac{176}{9} L_{ij11}^{V,LL} \\
& \left. - \frac{176}{9} L_{ij22}^{V,LL} + \frac{112}{9} L_{ij11}^{V,LR} + \frac{112}{9} L_{ij22}^{V,LR} \right];
\end{aligned}$$

$$\begin{aligned}
\dot{L}_{ij33}^{V,LR} &= e^2 \left[ \frac{4}{3} L_{ij11}^{V,LL} + \frac{4}{3} L_{ij22}^{V,LL} + \frac{4}{3} L_{ij11}^{V,LR} + \frac{4}{3} L_{ij22}^{V,LR} + \frac{4}{3} L_{ij11}^{V,LL} \right. \\
& + \frac{4}{3} L_{ij22}^{V,LL} + \frac{4}{3} L_{ij33}^{V,LL} + \frac{4}{3} L_{ij11}^{V,LR} + \frac{4}{3} L_{ij22}^{V,LR} + \frac{4}{3} L_{ij33}^{V,LR} - \frac{8}{3} L_{ij11}^{V,LL} \\
& \left. - \frac{8}{3} L_{ij22}^{V,LL} - \frac{8}{3} L_{ij11}^{V,LR} - \frac{8}{3} L_{ij22}^{V,LR} \right] + \alpha_s \alpha \left[ \frac{16}{3} L_{ij11}^{V,LL} + \frac{16}{3} L_{ij22}^{V,LL} \right. \\
& + \frac{16}{3} L_{ij11}^{V,LR} + \frac{16}{3} L_{ij22}^{V,LR} - \frac{32}{3} L_{ij11}^{V,LL} - \frac{32}{3} L_{ij22}^{V,LL} - \frac{32}{3} L_{ij11}^{V,LR} - \frac{32}{3} L_{ij22}^{V,LR} \\
& + \alpha^2 \left[ -\frac{32}{9} L_{ij11}^{V,LL} - \frac{32}{9} L_{ij22}^{V,LL} + \frac{40}{9} L_{ij11}^{V,LR} + \frac{40}{9} L_{ij22}^{V,LR} - 8 L_{ij11}^{V,LL} \right. \\
& - 8 L_{ij22}^{V,LL} - 8 L_{ij33}^{V,LL} + 16 L_{ij11}^{V,LR} + 16 L_{ij22}^{V,LR} + 16 L_{ij33}^{V,LR} - \frac{176}{9} L_{ij11}^{V,LL} \\
& \left. - \frac{176}{9} L_{ij22}^{V,LL} + \frac{112}{9} L_{ij11}^{V,LR} + \frac{112}{9} L_{ij22}^{V,LR} \right];
\end{aligned}$$

$$\begin{aligned}
& -8L_{ij22}^{V,LL} - 8L_{ij33}^{V,LL} + 16L_{ij11}^{V,LR} + 16L_{ij22}^{V,LR} + 16L_{ij33}^{V,LR} - \frac{176}{9}L_{ij11}^{V,LL} \\
& - \frac{176}{9}L_{ij22}^{V,LL} + \frac{112}{9}L_{ij11}^{V,LR} + \frac{112}{9}L_{ij22}^{V,LR} \Big] ; \\
\dot{L}_{ij11}^{V,LR} = & e^2 \left[ \frac{4}{9}L_{ij11}^{V,LL} + \frac{4}{9}L_{ij22}^{V,LL} + \frac{4}{9}L_{ij11}^{V,LR} + \frac{4}{9}L_{ij22}^{V,LR} + \frac{4}{9}L_{ij11}^{V,LL} \right. \\
& + \frac{4}{9}L_{ij22}^{V,LL} + \frac{4}{9}L_{ij33}^{V,LL} + \frac{4}{9}L_{ij11}^{V,LR} + \frac{4}{9}L_{ij22}^{V,LR} + \frac{4}{9}L_{ij33}^{V,LR} - \frac{8}{9}L_{ij11}^{V,LL} \\
& \left. - \frac{8}{9}L_{ij22}^{V,LL} - \frac{8}{9}L_{ij11}^{V,LR} - \frac{8}{9}L_{ij22}^{V,LR} \right] + \alpha_s^2 \left[ -8L_{ij11}^{V,LL} - 8L_{ij22}^{V,LL} \right. \\
& \left. + 8L_{ij11}^{V,LR} + 8L_{ij22}^{V,LR} - 8L_{ij11}^{V,LL} - 8L_{ij22}^{V,LL} + 8L_{ij11}^{V,LR} + 8L_{ij22}^{V,LR} \right] \\
& + \alpha_s \alpha \left[ \frac{16}{9}L_{ij11}^{V,LL} + \frac{16}{9}L_{ij22}^{V,LL} + \frac{16}{9}L_{ij11}^{V,LR} + \frac{16}{9}L_{ij22}^{V,LR} - \frac{32}{9}L_{ij11}^{V,LL} \right. \\
& \left. - \frac{32}{9}L_{ij22}^{V,LL} - \frac{32}{9}L_{ij11}^{V,LR} - \frac{32}{9}L_{ij22}^{V,LR} \right] + \alpha^2 \left[ -\frac{8}{27}L_{ij11}^{V,LL} - \frac{8}{27}L_{ij22}^{V,LL} \right. \\
& + \frac{16}{27}L_{ij11}^{V,LR} + \frac{16}{27}L_{ij22}^{V,LR} + \frac{8}{3}L_{ij11}^{V,LR} + \frac{8}{3}L_{ij22}^{V,LR} + \frac{8}{3}L_{ij33}^{V,LR} - \frac{80}{27}L_{ij11}^{V,LL} \\
& \left. - \frac{80}{27}L_{ij22}^{V,LL} + \frac{16}{27}L_{ij11}^{V,LR} + \frac{16}{27}L_{ij22}^{V,LR} \right] ; \\
\dot{L}_{ij22}^{V,LR} = & e^2 \left[ \frac{4}{9}L_{ij11}^{V,LL} + \frac{4}{9}L_{ij22}^{V,LL} + \frac{4}{9}L_{ij11}^{V,LR} + \frac{4}{9}L_{ij22}^{V,LR} + \frac{4}{9}L_{ij11}^{V,LL} \right. \\
& + \frac{4}{9}L_{ij22}^{V,LL} + \frac{4}{9}L_{ij33}^{V,LL} + \frac{4}{9}L_{ij11}^{V,LR} + \frac{4}{9}L_{ij22}^{V,LR} + \frac{4}{9}L_{ij33}^{V,LR} - \frac{8}{9}L_{ij11}^{V,LL} \\
& \left. - \frac{8}{9}L_{ij22}^{V,LL} - \frac{8}{9}L_{ij11}^{V,LR} - \frac{8}{9}L_{ij22}^{V,LR} \right] + \alpha_s^2 \left[ -8L_{ij11}^{V,LL} - 8L_{ij22}^{V,LL} \right. \\
& \left. + 8L_{ij11}^{V,LR} + 8L_{ij22}^{V,LR} - 8L_{ij11}^{V,LL} - 8L_{ij22}^{V,LL} + 8L_{ij11}^{V,LR} + 8L_{ij22}^{V,LR} \right] \\
& + \alpha_s \alpha \left[ \frac{16}{9}L_{ij11}^{V,LL} + \frac{16}{9}L_{ij22}^{V,LL} + \frac{16}{9}L_{ij11}^{V,LR} + \frac{16}{9}L_{ij22}^{V,LR} - \frac{32}{9}L_{ij11}^{V,LL} \right. \\
& \left. - \frac{32}{9}L_{ij22}^{V,LL} - \frac{32}{9}L_{ij11}^{V,LR} - \frac{32}{9}L_{ij22}^{V,LR} \right] + \alpha^2 \left[ -\frac{8}{27}L_{ij11}^{V,LL} - \frac{8}{27}L_{ij22}^{V,LL} \right. \\
& + \frac{16}{27}L_{ij11}^{V,LR} + \frac{16}{27}L_{ij22}^{V,LR} + \frac{8}{3}L_{ij11}^{V,LR} + \frac{8}{3}L_{ij22}^{V,LR} + \frac{8}{3}L_{ij33}^{V,LR} - \frac{80}{27}L_{ij11}^{V,LL} \\
& \left. - \frac{80}{27}L_{ij22}^{V,LL} + \frac{16}{27}L_{ij11}^{V,LR} + \frac{16}{27}L_{ij22}^{V,LR} \right] ;
\end{aligned}$$

$$\begin{aligned}
& -\frac{32}{9}L_{ij22}^{V,LL} - \frac{32}{9}L_{ij11}^{V,LR} - \frac{32}{9}L_{ij22}^{V,LR} \Big] + \alpha^2 \Big[ -\frac{8}{27}L_{ij11}^{V,LL} - \frac{8}{27}L_{ij22}^{V,LL} \\
& + \frac{16}{27}L_{ij11}^{V,LR} + \frac{16}{27}L_{ij22}^{V,LR} + \frac{8}{3}L_{ij11}^{V,LR} + \frac{8}{3}L_{ij22}^{V,LR} + \frac{8}{3}L_{ij33}^{V,LR} - \frac{80}{27}L_{ij11}^{V,LL} \\
& - \frac{80}{27}L_{ij22}^{V,LL} + \frac{16}{27}L_{ij11}^{V,LR} + \frac{16}{27}L_{ij22}^{V,LR} \Big] ; \\
\dot{L}_{ij11}^{V,LR} & = e^2 \Big[ -\frac{8}{9}L_{ij11}^{V,LL} - \frac{8}{9}L_{ij22}^{V,LL} - \frac{8}{9}L_{ij11}^{V,LR} - \frac{8}{9}L_{ij22}^{V,LR} - \frac{8}{9}L_{ij11}^{V,LL} \\
& - \frac{8}{9}L_{ij22}^{V,LL} - \frac{8}{9}L_{ij33}^{V,LL} - \frac{8}{9}L_{ij11}^{V,LR} - \frac{8}{9}L_{ij22}^{V,LR} - \frac{8}{9}L_{ij33}^{V,LR} + \frac{16}{9}L_{ij11}^{V,LL} \\
& + \frac{16}{9}L_{ij22}^{V,LL} + \frac{16}{9}L_{ij11}^{V,LR} + \frac{16}{9}L_{ij22}^{V,LR} \Big] + \alpha_s^2 \Big[ -8L_{ij11}^{V,LL} - 8L_{ij22}^{V,LL} \\
& + 8L_{ij11}^{V,LR} + 8L_{ij22}^{V,LR} - 8L_{ij11}^{V,LL} - 8L_{ij22}^{V,LL} + 8L_{ij11}^{V,LR} + 8L_{ij22}^{V,LR} \Big] \\
& + \alpha_s \alpha \Big[ -\frac{32}{9}L_{ij11}^{V,LL} - \frac{32}{9}L_{ij22}^{V,LL} - \frac{32}{9}L_{ij11}^{V,LR} - \frac{32}{9}L_{ij22}^{V,LR} + \frac{64}{9}L_{ij11}^{V,LL} \\
& + \frac{64}{9}L_{ij22}^{V,LL} + \frac{64}{9}L_{ij11}^{V,LR} + \frac{64}{9}L_{ij22}^{V,LR} \Big] + \alpha^2 \Big[ -\frac{56}{27}L_{ij11}^{V,LL} - \frac{56}{27}L_{ij22}^{V,LL} \\
& + \frac{40}{27}L_{ij11}^{V,LR} + \frac{40}{27}L_{ij22}^{V,LR} - 8L_{ij11}^{V,LL} - 8L_{ij22}^{V,LL} - 8L_{ij33}^{V,LL} + \frac{8}{3}L_{ij11}^{V,LR} \\
& + \frac{8}{3}L_{ij22}^{V,LR} + \frac{8}{3}L_{ij33}^{V,LR} - \frac{128}{27}L_{ij11}^{V,LL} - \frac{128}{27}L_{ij22}^{V,LL} + \frac{256}{27}L_{ij11}^{V,LR} \\
& + \frac{256}{27}L_{ij22}^{V,LR} \Big] ; \\
\dot{L}_{ij22}^{V,LR} & = e^2 \Big[ -\frac{8}{9}L_{ij11}^{V,LL} - \frac{8}{9}L_{ij22}^{V,LL} - \frac{8}{9}L_{ij11}^{V,LR} - \frac{8}{9}L_{ij22}^{V,LR} - \frac{8}{9}L_{ij11}^{V,LL} \\
& - \frac{8}{9}L_{ij22}^{V,LL} - \frac{8}{9}L_{ij33}^{V,LL} - \frac{8}{9}L_{ij11}^{V,LR} - \frac{8}{9}L_{ij22}^{V,LR} - \frac{8}{9}L_{ij33}^{V,LR} + \frac{16}{9}L_{ij11}^{V,LL} \\
& + \frac{16}{9}L_{ij22}^{V,LL} + \frac{16}{9}L_{ij11}^{V,LR} + \frac{16}{9}L_{ij22}^{V,LR} \Big] + \alpha_s^2 \Big[ -8L_{ij11}^{V,LL} - 8L_{ij22}^{V,LL}
\end{aligned}$$

$$\begin{aligned}
& + 8L_{ij11}^{V,LR} + 8L_{ij22}^{V,LR} - 8L_{ij11}^{V,LL} - 8L_{ij22}^{V,LL} + 8L_{ij11}^{V,LR} + 8L_{ij22}^{V,LR} \Big] \\
& + \alpha_s \alpha \left[ -\frac{32}{9}L_{ij11}^{V,LL} - \frac{32}{9}L_{ij22}^{V,LL} - \frac{32}{9}L_{ij11}^{V,LR} - \frac{32}{9}L_{ij22}^{V,LR} + \frac{64}{9}L_{ij11}^{V,LL} \right. \\
& + \frac{64}{9}L_{ij22}^{V,LL} + \frac{64}{9}L_{ij11}^{V,LR} + \frac{64}{9}L_{ij22}^{V,LR} \Big] + \alpha^2 \left[ -\frac{56}{27}L_{ij11}^{V,LL} - \frac{56}{27}L_{ij22}^{V,LL} \right. \\
& + \frac{40}{27}L_{ij11}^{V,LR} + \frac{40}{27}L_{ij22}^{V,LR} - 8L_{ij11}^{V,LL} - 8L_{ij22}^{V,LL} - 8L_{ij33}^{V,LL} + \frac{8}{3}L_{ij11}^{V,LR} \\
& + \frac{8}{3}L_{ij22}^{V,LR} + \frac{8}{3}L_{ij33}^{V,LR} - \frac{128}{27}L_{ij11}^{V,LL} - \frac{128}{27}L_{ij22}^{V,LL} + \frac{256}{27}L_{ij11}^{V,LR} \\
& \left. + \frac{256}{27}L_{ij22}^{V,LR} \right] ;
\end{aligned}$$

$$\dot{L}_{ij11}^{S,LR} = \frac{353}{9}\alpha^2 L_{ij11}^{S,LR} - 6e^2 L_{ij11}^{S,LR} ;$$

$$\dot{L}_{ij22}^{S,LR} = \frac{353}{9}\alpha^2 L_{ij22}^{S,LR} - 6e^2 L_{ij22}^{S,LR} ;$$

$$\dot{L}_{ij33}^{S,LR} = \frac{353}{9}\alpha^2 L_{ij33}^{S,LR} - 6e^2 L_{ij33}^{S,LR} ;$$

$$\begin{aligned}
\dot{L}_{ij11}^{S,LR} & = -8g_s^2 L_{ij11}^{S,LR} - \frac{2}{3}e^2 L_{ij11}^{S,LR} - \frac{1012}{9}\alpha_s^2 L_{ij11}^{S,LR} - \frac{8}{9}\alpha_s \alpha L_{ij11}^{S,LR} \\
& + \frac{377}{81}\alpha^2 L_{ij11}^{S,LR} ;
\end{aligned}$$

$$\begin{aligned}
\dot{L}_{ij22}^{S,LR} & = -8g_s^2 L_{ij22}^{S,LR} - \frac{2}{3}e^2 L_{ij22}^{S,LR} - \frac{1012}{9}\alpha_s^2 L_{ij22}^{S,LR} - \frac{8}{9}\alpha_s \alpha L_{ij22}^{S,LR} \\
& + \frac{377}{81}\alpha^2 L_{ij22}^{S,LR} ;
\end{aligned}$$

$$\begin{aligned}
\dot{L}_{ij11}^{S,LR} & = -8g_s^2 L_{ij11}^{S,LR} - \frac{8}{3}e^2 L_{ij11}^{S,LR} - \frac{1012}{9}\alpha_s^2 L_{ij11}^{S,LR} - \frac{32}{9}\alpha_s \alpha L_{ij11}^{S,LR} \\
& + \frac{1472}{81}\alpha^2 L_{ij11}^{S,LR} ;
\end{aligned}$$

$$\begin{aligned}
\dot{L}_{ij22}^{S,LR} & = -8g_s^2 L_{ij22}^{S,LR} - \frac{8}{3}e^2 L_{ij22}^{S,LR} - \frac{1012}{9}\alpha_s^2 L_{ij22}^{S,LR} - \frac{32}{9}\alpha_s \alpha L_{ij22}^{S,LR} \\
& + \frac{1472}{81}\alpha^2 L_{ij22}^{S,LR} ;
\end{aligned}$$



$$\begin{aligned}
\dot{L}_{ij11}^{S,LL} &= \frac{353}{9} \alpha^2 L_{ij11}^{S,LL} - 6e^2 L_{ij11}^{S,LL} ; \\
\dot{L}_{ij11}^{T,LL} &= 2e^2 L_{ij11}^{T,LL} - \frac{1501}{27} \alpha^2 L_{ij11}^{T,LL} ; \\
\dot{L}_{ij22}^{S,LL} &= \frac{353}{9} \alpha^2 L_{ij22}^{S,LL} - 6e^2 L_{ij22}^{S,LL} ; \\
\dot{L}_{ij22}^{T,LL} &= 2e^2 L_{ij22}^{T,LL} - \frac{1501}{27} \alpha^2 L_{ij22}^{T,LL} ; \\
\dot{L}_{ij33}^{S,LL} &= \frac{353}{9} \alpha^2 L_{ij33}^{S,LL} - 6e^2 L_{ij33}^{S,LL} ; \\
\dot{L}_{ij33}^{T,LL} &= 2e^2 L_{ij33}^{T,LL} - \frac{1501}{27} \alpha^2 L_{ij33}^{T,LL} ; \\
\dot{L}_{ij11}^{S,LL} &= -8g_s^2 L_{ij11}^{S,LL} - \frac{2}{3} e^2 L_{ij11}^{S,LL} - \frac{1012}{9} \alpha_s^2 L_{ij11}^{S,LL} - \frac{8}{9} \alpha_s \alpha L_{ij11}^{S,LL} \\
&\quad + \frac{377}{81} \alpha^2 L_{ij11}^{S,LL} ; \\
\dot{L}_{ij11}^{T,LL} &= \frac{8}{3} g_s^2 L_{ij11}^{T,LL} + \frac{2}{9} e^2 L_{ij11}^{T,LL} + \frac{1652}{27} \alpha_s^2 L_{ij11}^{T,LL} - \frac{152}{27} \alpha_s \alpha L_{ij11}^{T,LL} \\
&\quad - \frac{1045}{243} \alpha^2 L_{ij11}^{T,LL} ; \\
\dot{L}_{ij22}^{S,LL} &= -8g_s^2 L_{ij22}^{S,LL} - \frac{2}{3} e^2 L_{ij22}^{S,LL} - \frac{1012}{9} \alpha_s^2 L_{ij22}^{S,LL} - \frac{8}{9} \alpha_s \alpha L_{ij22}^{S,LL} \\
&\quad + \frac{377}{81} \alpha^2 L_{ij22}^{S,LL} ; \\
\dot{L}_{ij22}^{T,LL} &= \frac{8}{3} g_s^2 L_{ij22}^{T,LL} + \frac{2}{9} e^2 L_{ij22}^{T,LL} + \frac{1652}{27} \alpha_s^2 L_{ij22}^{T,LL} - \frac{152}{27} \alpha_s \alpha L_{ij22}^{T,LL} \\
&\quad - \frac{1045}{243} \alpha^2 L_{ij22}^{T,LL} ; \\
\dot{L}_{ij11}^{S,LL} &= -8g_s^2 L_{ij11}^{S,LL} - \frac{8}{3} e^2 L_{ij11}^{S,LL} - \frac{1012}{9} \alpha_s^2 L_{ij11}^{S,LL} - \frac{32}{9} \alpha_s \alpha L_{ij11}^{S,LL} \\
&\quad + \frac{1472}{81} \alpha^2 L_{ij11}^{S,LL} ; \\
\dot{L}_{ij11}^{T,LL} &= \frac{8}{3} g_s^2 L_{ij11}^{T,LL} + \frac{8}{9} e^2 L_{ij11}^{T,LL} + \frac{1652}{27} \alpha_s^2 L_{ij11}^{T,LL} - \frac{608}{27} \alpha_s \alpha L_{ij11}^{T,LL} \\
&\quad - \frac{4864}{243} \alpha^2 L_{ij11}^{T,LL} ;
\end{aligned}$$

$$\begin{aligned}
\dot{L}_{ij22}^{S,LL} &= -8g_s^2 L_{ij22}^{S,LL} - \frac{8}{3}e^2 L_{ij22}^{S,LL} - \frac{1012}{9}\alpha_s^2 L_{ij22}^{S,LL} - \frac{32}{9}\alpha_s \alpha L_{ij22}^{S,LL} \\
&\quad + \frac{1472}{81}\alpha^2 L_{ij22}^{S,LL} ; \\
\dot{L}_{ij22}^{T,LL} &= \frac{8}{3}g_s^2 L_{ij22}^{T,LL} + \frac{8}{9}e^2 L_{ij22}^{T,LL} + \frac{1652}{27}\alpha_s^2 L_{ij22}^{T,LL} - \frac{608}{27}\alpha_s \alpha L_{ij22}^{T,LL} \\
&\quad - \frac{4864}{243}\alpha^2 L_{ij22}^{T,LL} ; \\
\dot{L}_{ijkk}^{V,LL} &= 0 ; \\
\dot{L}_{ijjj}^{V,LL} &= 0 ; \\
\dot{L}_{ijii}^{V,LL} &= 0 ; \\
\dot{L}_{ijkk}^{S,LL} &= 0 ; \\
\dot{L}_{ikkk}^{S,LL} &= 0 ; \\
\dot{L}_{ijjj}^{S,LL} &= 0 ; \\
\dot{L}_{ijii}^{S,LL} &= 0 ;
\end{aligned}$$

## 2.9 $\Delta F = 0$ Transitions ( $\bar{f}_i f_i \bar{f}_j f_j$ )

$$\begin{aligned}
\dot{L}_{ijjj}^{S,RL} &= -8g_s^2 L_{ijjj}^{S,RL} - \frac{20}{3}e^2 L_{ijjj}^{S,RL} - \frac{1012}{9}\alpha_s^2 L_{ijjj}^{S,RL} - \frac{8}{9}\alpha_s \alpha L_{ijjj}^{S,RL} \\
&\quad + \frac{6614}{81}\alpha^2 L_{ijjj}^{S,RL} ; \\
\dot{L}_{ijjj}^{S,RL} &= -8g_s^2 L_{ijjj}^{S,RL} - \frac{26}{3}e^2 L_{ijjj}^{S,RL} - \frac{1012}{9}\alpha_s^2 L_{ijjj}^{S,RL} - \frac{32}{9}\alpha_s \alpha L_{ijjj}^{S,RL} \\
&\quad + \frac{473}{81}\alpha^2 L_{ijjj}^{S,RL} ; \\
\dot{L}_{ijjj}^{S,LR} &= -6e^2 L_{ijjj}^{S,LR} ; \\
\dot{L}_{ijjj}^{S,LR} &= -8g_s^2 L_{ijjj}^{S,LR} - \frac{2}{3}e^2 L_{ijjj}^{S,LR} - \frac{1012}{9}\alpha_s^2 L_{ijjj}^{S,LR} - \frac{8}{9}\alpha_s \alpha L_{ijjj}^{S,LR} \\
&\quad + \frac{377}{81}\alpha^2 L_{ijjj}^{S,LR} ;
\end{aligned}$$

$$\begin{aligned}
\dot{L}_{\nu u}^{S,LR}{}_{ijji} &= -8g_s^2 L_{\nu u}^{S,LR}{}_{ijji} - \frac{8}{3}e^2 L_{\nu u}^{S,LR}{}_{ijji} - \frac{1012}{9}\alpha_s^2 L_{\nu u}^{S,LR}{}_{ijji} - \frac{32}{9}\alpha_s\alpha L_{\nu u}^{S,LR}{}_{ijji} \\
&\quad + \frac{1472}{81}\alpha^2 L_{\nu u}^{S,LR}{}_{ijji} ; \\
\dot{L}_{uddu}^{V1,LR}{}_{ijji} &= -\frac{8}{3}g_s^2 L_{uddu}^{V8,LR}{}_{ijji} - \frac{10}{3}e^2 L_{uddu}^{V1,LR}{}_{ijji} + \alpha_s^2 \left[ -\frac{28}{3}L_{uddu}^{V1,LR}{}_{ijji} - \frac{2044}{27}L_{uddu}^{V8,LR}{}_{ijji} \right] \\
&\quad + \alpha_s\alpha \left[ \frac{8}{3}L_{uddu}^{V1,LR}{}_{ijji} - \frac{128}{27}L_{uddu}^{V8,LR}{}_{ijji} \right] + \frac{169}{81}\alpha^2 L_{uddu}^{V1,LR}{}_{ijji} ; \\
\dot{L}_{uddu}^{V8,LR}{}_{ijji} &= g_s^2 \left[ -12L_{uddu}^{V1,LR}{}_{ijji} - 14L_{uddu}^{V8,LR}{}_{ijji} \right] - \frac{10}{3}e^2 L_{uddu}^{V8,LR}{}_{ijji} + \alpha_s^2 \left[ -\frac{374}{3}L_{uddu}^{V1,LR}{}_{ijji} \right. \\
&\quad \left. - \frac{2975}{18}L_{uddu}^{V8,LR}{}_{ijji} \right] + \alpha_s\alpha \left[ \frac{16}{9}L_{uddu}^{V8,LR}{}_{ijji} - \frac{64}{3}L_{uddu}^{V1,LR}{}_{ijji} \right] + \frac{169}{81}\alpha^2 L_{uddu}^{V8,LR}{}_{ijji} ; \\
\dot{L}_{dd}^{V1,LR}{}_{ijji} &= -\frac{8}{3}g_s^2 L_{dd}^{V8,LR}{}_{ijji} - \frac{4}{3}e^2 L_{dd}^{V1,LR}{}_{ijji} + \alpha_s^2 \left[ -\frac{28}{3}L_{dd}^{V1,LR}{}_{ijji} - \frac{2044}{27}L_{dd}^{V8,LR}{}_{ijji} \right] \\
&\quad + \alpha_s\alpha \left[ \frac{32}{3}L_{dd}^{V1,LR}{}_{ijji} - \frac{8}{27}L_{dd}^{V8,LR}{}_{ijji} \right] + \frac{1702}{81}\alpha^2 L_{dd}^{V1,LR}{}_{ijji} ; \\
\dot{L}_{dd}^{V8,LR}{}_{ijji} &= g_s^2 \left[ -12L_{dd}^{V1,LR}{}_{ijji} - 14L_{dd}^{V8,LR}{}_{ijji} \right] - \frac{4}{3}e^2 L_{dd}^{V8,LR}{}_{ijji} + \alpha_s^2 \left[ -\frac{374}{3}L_{dd}^{V1,LR}{}_{ijji} \right. \\
&\quad \left. - \frac{2975}{18}L_{dd}^{V8,LR}{}_{ijji} \right] + \alpha_s\alpha \left[ -\frac{4}{3}L_{dd}^{V1,LR}{}_{ijji} - \frac{26}{9}L_{dd}^{V8,LR}{}_{ijji} \right] + \frac{1702}{81}\alpha^2 L_{dd}^{V8,LR}{}_{ijji} ; \\
\dot{L}_{uu}^{V1,LR}{}_{ijji} &= -\frac{8}{3}g_s^2 L_{uu}^{V8,LR}{}_{ijji} - \frac{16}{3}e^2 L_{uu}^{V1,LR}{}_{ijji} + \alpha_s^2 \left[ -\frac{28}{3}L_{uu}^{V1,LR}{}_{ijji} - \frac{2044}{27}L_{uu}^{V8,LR}{}_{ijji} \right] \\
&\quad + \alpha_s\alpha \left[ \frac{128}{3}L_{uu}^{V1,LR}{}_{ijji} - \frac{32}{27}L_{uu}^{V8,LR}{}_{ijji} \right] + \frac{7168}{81}\alpha^2 L_{uu}^{V1,LR}{}_{ijji} ; \\
\dot{L}_{uu}^{V8,LR}{}_{ijji} &= g_s^2 \left[ -12L_{uu}^{V1,LR}{}_{ijji} - 14L_{uu}^{V8,LR}{}_{ijji} \right] - \frac{16}{3}e^2 L_{uu}^{V8,LR}{}_{ijji} + \alpha_s^2 \left[ -\frac{374}{3}L_{uu}^{V1,LR}{}_{ijji} \right. \\
&\quad \left. - \frac{2975}{18}L_{uu}^{V8,LR}{}_{ijji} \right] + \alpha_s\alpha \left[ -\frac{16}{3}L_{uu}^{V1,LR}{}_{ijji} - \frac{104}{9}L_{uu}^{V8,LR}{}_{ijji} \right] + \frac{7168}{81}\alpha^2 L_{uu}^{V8,LR}{}_{ijji} ; \\
\dot{L}_{ee}^{V,LR}{}_{ijji} &= \frac{1942}{9}\alpha^2 L_{ee}^{V,LR}{}_{ijji} - 12e^2 L_{ee}^{V,LR}{}_{ijji} ;
\end{aligned}$$

$$\begin{aligned}
\dot{L}_{ed}^{S,RL} &= -8g_s^2 L_{ed}^{S,RL} - \frac{20}{3} e^2 L_{ed}^{S,RL} - \frac{1012}{9} \alpha_s^2 L_{ed}^{S,RL} - \frac{8}{9} \alpha_s \alpha L_{ed}^{S,RL} \\
&\quad + \frac{6614}{81} \alpha^2 L_{ed}^{S,RL} ; \\
\dot{L}_{eu}^{S,RL} &= -8g_s^2 L_{eu}^{S,RL} - \frac{26}{3} e^2 L_{eu}^{S,RL} - \frac{1012}{9} \alpha_s^2 L_{eu}^{S,RL} - \frac{32}{9} \alpha_s \alpha L_{eu}^{S,RL} \\
&\quad + \frac{473}{81} \alpha^2 L_{eu}^{S,RL} ; \\
\dot{L}_{\nu e}^{S,LR} &= -6e^2 L_{\nu e}^{S,LR} ; \\
\dot{L}_{\nu d}^{S,LR} &= -8g_s^2 L_{\nu d}^{S,LR} - \frac{2}{3} e^2 L_{\nu d}^{S,LR} - \frac{1012}{9} \alpha_s^2 L_{\nu d}^{S,LR} - \frac{8}{9} \alpha_s \alpha L_{\nu d}^{S,LR} \\
&\quad + \frac{377}{81} \alpha^2 L_{\nu d}^{S,LR} ; \\
\dot{L}_{\nu u}^{S,LR} &= -8g_s^2 L_{\nu u}^{S,LR} - \frac{8}{3} e^2 L_{\nu u}^{S,LR} - \frac{1012}{9} \alpha_s^2 L_{\nu u}^{S,LR} - \frac{32}{9} \alpha_s \alpha L_{\nu u}^{S,LR} \\
&\quad + \frac{1472}{81} \alpha^2 L_{\nu u}^{S,LR} ; \\
\dot{L}_{uddu}^{V1,LR} &= -\frac{8}{3} g_s^2 L_{uddu}^{V8,LR} - \frac{10}{3} e^2 L_{uddu}^{V1,LR} + \alpha_s^2 \left[ -\frac{28}{3} L_{uddu}^{V1,LR} - \frac{2044}{27} L_{uddu}^{V8,LR} \right] \\
&\quad + \alpha_s \alpha \left[ \frac{8}{3} L_{uddu}^{V1,LR} - \frac{128}{27} L_{uddu}^{V8,LR} \right] + \frac{169}{81} \alpha^2 L_{uddu}^{V1,LR} ; \\
\dot{L}_{jij}^{V8,LR} &= g_s^2 \left[ -12 L_{uddu}^{V1,LR} - 14 L_{uddu}^{V8,LR} \right] - \frac{10}{3} e^2 L_{uddu}^{V8,LR} + \alpha_s^2 \left[ -\frac{374}{3} L_{uddu}^{V1,LR} \right. \\
&\quad \left. - \frac{2975}{18} L_{uddu}^{V8,LR} \right] + \alpha_s \alpha \left[ \frac{16}{9} L_{uddu}^{V8,LR} - \frac{64}{3} L_{uddu}^{V1,LR} \right] + \frac{169}{81} \alpha^2 L_{uddu}^{V8,LR} ; \\
\dot{L}_{dd}^{V1,LR} &= -\frac{8}{3} g_s^2 L_{dd}^{V8,LR} - \frac{4}{3} e^2 L_{dd}^{V1,LR} + \alpha_s^2 \left[ -\frac{28}{3} L_{dd}^{V1,LR} - \frac{2044}{27} L_{dd}^{V8,LR} \right] \\
&\quad + \alpha_s \alpha \left[ \frac{32}{3} L_{dd}^{V1,LR} - \frac{8}{27} L_{dd}^{V8,LR} \right] + \frac{1702}{81} \alpha^2 L_{dd}^{V1,LR} ; \\
\dot{L}_{dd}^{V8,LR} &= g_s^2 \left[ -12 L_{dd}^{V1,LR} - 14 L_{dd}^{V8,LR} \right] - \frac{4}{3} e^2 L_{dd}^{V8,LR} + \alpha_s^2 \left[ -\frac{374}{3} L_{dd}^{V1,LR} \right.
\end{aligned}$$

$$\begin{aligned}
& -\frac{2975}{18}L_{\ddot{u}j}^{V8,LR} \Big] + \alpha_s \alpha \left[ -\frac{4}{3}L_{\ddot{u}j}^{V1,LR} - \frac{26}{9}L_{\ddot{u}j}^{V8,LR} \right] + \frac{1702}{81}\alpha^2 L_{\ddot{u}j}^{V8,LR} ; \\
\dot{L}_{\ddot{u}j}^{V1,LR} &= -\frac{8}{3}g_s^2 L_{\ddot{u}j}^{V8,LR} - \frac{16}{3}e^2 L_{\ddot{u}j}^{V1,LR} + \alpha_s^2 \left[ -\frac{28}{3}L_{\ddot{u}j}^{V1,LR} - \frac{2044}{27}L_{\ddot{u}j}^{V8,LR} \right] \\
& + \alpha_s \alpha \left[ \frac{128}{3}L_{\ddot{u}j}^{V1,LR} - \frac{32}{27}L_{\ddot{u}j}^{V8,LR} \right] + \frac{7168}{81}\alpha^2 L_{\ddot{u}j}^{V1,LR} ; \\
\dot{L}_{\ddot{u}j}^{V8,LR} &= g_s^2 \left[ -12L_{\ddot{u}j}^{V1,LR} - 14L_{\ddot{u}j}^{V8,LR} \right] - \frac{16}{3}e^2 L_{\ddot{u}j}^{V8,LR} + \alpha_s^2 \left[ -\frac{374}{3}L_{\ddot{u}j}^{V1,LR} \right. \\
& \left. - \frac{2975}{18}L_{\ddot{u}j}^{V8,LR} \right] + \alpha_s \alpha \left[ -\frac{16}{3}L_{\ddot{u}j}^{V1,LR} - \frac{104}{9}L_{\ddot{u}j}^{V8,LR} \right] + \frac{7168}{81}\alpha^2 L_{\ddot{u}j}^{V8,LR} ; \\
\dot{L}_{\ddot{u}j}^{V,LR} &= \frac{1942}{9}\alpha^2 L_{\ddot{u}j}^{V,LR} - 12e^2 L_{\ddot{u}j}^{V,LR} ; \\
\dot{L}_{\ddot{u}j}^{S,RR} &= -8g_s^2 L_{\ddot{u}j}^{S,RR} + e^2 \left[ -\frac{20}{3}L_{\ddot{u}j}^{S,RR} - 32L_{\ddot{u}j}^{T,RR} \right] - \frac{1012}{9}\alpha_s^2 L_{\ddot{u}j}^{S,RR} \\
& + \alpha_s \alpha \left[ \frac{1792}{9}L_{\ddot{u}j}^{T,RR} - \frac{8}{9}L_{\ddot{u}j}^{S,RR} \right] + \alpha^2 \left[ \frac{1682}{81}L_{\ddot{u}j}^{S,RR} + 704L_{\ddot{u}j}^{T,RR} \right] ; \\
\dot{L}_{\ddot{u}j}^{T,RR} &= \frac{8}{3}g_s^2 L_{\ddot{u}j}^{T,RR} + e^2 \left[ \frac{20}{9}L_{\ddot{u}j}^{T,RR} - \frac{2}{3}L_{\ddot{u}j}^{S,RR} \right] + \frac{1652}{27}\alpha_s^2 L_{\ddot{u}j}^{T,RR} \\
& + \alpha_s \alpha \left[ \frac{16}{3}L_{\ddot{u}j}^{S,RR} - \frac{152}{27}L_{\ddot{u}j}^{T,RR} \right] + \alpha^2 \left[ \frac{364}{81}L_{\ddot{u}j}^{S,RR} - \frac{6922}{243}L_{\ddot{u}j}^{T,RR} \right] ; \\
\dot{L}_{\ddot{u}j}^{S,RR} &= -8g_s^2 L_{\ddot{u}j}^{S,RR} + e^2 \left[ 64L_{\ddot{u}j}^{T,RR} - \frac{26}{3}L_{\ddot{u}j}^{S,RR} \right] - \frac{1012}{9}\alpha_s^2 L_{\ddot{u}j}^{S,RR} \\
& + \alpha_s \alpha \left[ -\frac{32}{9}L_{\ddot{u}j}^{S,RR} - \frac{3584}{9}L_{\ddot{u}j}^{T,RR} \right] + \alpha^2 \left[ -\frac{2839}{81}L_{\ddot{u}j}^{S,RR} - \frac{11264}{9}L_{\ddot{u}j}^{T,RR} \right] ; \\
\dot{L}_{\ddot{u}j}^{T,RR} &= \frac{8}{3}g_s^2 L_{\ddot{u}j}^{T,RR} + e^2 \left[ \frac{4}{3}L_{\ddot{u}j}^{S,RR} + \frac{26}{9}L_{\ddot{u}j}^{T,RR} \right] + \frac{1652}{27}\alpha_s^2 L_{\ddot{u}j}^{T,RR} \\
& + \alpha_s \alpha \left[ -\frac{32}{3}L_{\ddot{u}j}^{S,RR} - \frac{608}{27}L_{\ddot{u}j}^{T,RR} \right] + \alpha^2 \left[ -\frac{1376}{81}L_{\ddot{u}j}^{S,RR} - \frac{20677}{243}L_{\ddot{u}j}^{T,RR} \right] ; \\
\dot{L}_{\ddot{u}j}^{S,LL} &= \frac{353}{9}\alpha^2 L_{\ddot{u}j}^{S,LL} - 6e^2 L_{\ddot{u}j}^{S,LL} ;
\end{aligned}$$

$$\dot{L}_{\nu e ij}^{T,LL} = 2e^2 L_{\nu e ij}^{T,LL} - \frac{1501}{27} \alpha^2 L_{\nu e ij}^{T,LL} ;$$

$$\begin{aligned} \dot{L}_{\nu d ij}^{S,LL} = & -8g_s^2 L_{\nu d ij}^{S,LL} - \frac{2}{3} e^2 L_{\nu d ij}^{S,LL} - \frac{1012}{9} \alpha_s^2 L_{\nu d ij}^{S,LL} - \frac{8}{9} \alpha_s \alpha L_{\nu d ij}^{S,LL} \\ & + \frac{377}{81} \alpha^2 L_{\nu d ij}^{S,LL} ; \end{aligned}$$

$$\begin{aligned} \dot{L}_{\nu d ij}^{T,LL} = & \frac{8}{3} g_s^2 L_{\nu d ij}^{T,LL} + \frac{2}{9} e^2 L_{\nu d ij}^{T,LL} + \frac{1652}{27} \alpha_s^2 L_{\nu d ij}^{T,LL} - \frac{152}{27} \alpha_s \alpha L_{\nu d ij}^{T,LL} \\ & - \frac{1045}{243} \alpha^2 L_{\nu d ij}^{T,LL} ; \end{aligned}$$

$$\begin{aligned} \dot{L}_{\nu u ij}^{S,LL} = & -8g_s^2 L_{\nu u ij}^{S,LL} - \frac{8}{3} e^2 L_{\nu u ij}^{S,LL} - \frac{1012}{9} \alpha_s^2 L_{\nu u ij}^{S,LL} - \frac{32}{9} \alpha_s \alpha L_{\nu u ij}^{S,LL} \\ & + \frac{1472}{81} \alpha^2 L_{\nu u ij}^{S,LL} ; \end{aligned}$$

$$\begin{aligned} \dot{L}_{\nu u ij}^{T,LL} = & \frac{8}{3} g_s^2 L_{\nu u ij}^{T,LL} + \frac{8}{9} e^2 L_{\nu u ij}^{T,LL} + \frac{1652}{27} \alpha_s^2 L_{\nu u ij}^{T,LL} - \frac{608}{27} \alpha_s \alpha L_{\nu u ij}^{T,LL} \\ & - \frac{4864}{243} \alpha^2 L_{\nu u ij}^{T,LL} ; \end{aligned}$$

$$\begin{aligned} \dot{L}_{ud ij}^{S1,RR} = & g_s^2 \left[ \frac{64}{9} L_{uddu ij}^{S1,RR} + \frac{112}{27} L_{uddu ij}^{S8,RR} - 16 L_{ud ij}^{S1,RR} + \frac{16}{9} L_{ud ij}^{S8,RR} \right] \\ & + e^2 \left[ \frac{4}{27} L_{uddu ij}^{S1,RR} + \frac{16}{81} L_{uddu ij}^{S8,RR} - \frac{46}{9} L_{ud ij}^{S1,RR} \right] + \alpha_s^2 \left[ \frac{9472}{81} L_{uddu ij}^{S1,RR} + \frac{16576}{243} L_{uddu ij}^{S8,RR} \right. \\ & \left. - \frac{2120}{9} L_{ud ij}^{S1,RR} + \frac{928}{81} L_{ud ij}^{S8,RR} \right] + \alpha_s \alpha \left[ \frac{1888}{81} L_{uddu ij}^{S1,RR} + \frac{3808}{243} L_{uddu ij}^{S8,RR} + \frac{136}{27} L_{ud ij}^{S1,RR} \right. \\ & \left. + \frac{224}{81} L_{ud ij}^{S8,RR} \right] + \alpha^2 \left[ \frac{106}{729} L_{uddu ij}^{S1,RR} + \frac{424}{2187} L_{uddu ij}^{S8,RR} + \frac{6059}{243} L_{ud ij}^{S1,RR} \right] ; \end{aligned}$$

$$\begin{aligned} \dot{L}_{ud ij}^{S8,RR} = & g_s^2 \left[ -\frac{16}{3} L_{uddu ij}^{S1,RR} + \frac{44}{9} L_{uddu ij}^{S8,RR} + 8 L_{ud ij}^{S1,RR} + \frac{16}{3} L_{ud ij}^{S8,RR} \right] \\ & + e^2 \left[ \frac{8}{9} L_{uddu ij}^{S1,RR} - \frac{4}{27} L_{uddu ij}^{S8,RR} - \frac{46}{9} L_{ud ij}^{S8,RR} \right] + \alpha_s^2 \left[ -\frac{856}{27} L_{uddu ij}^{S1,RR} - \frac{2506}{81} L_{uddu ij}^{S8,RR} \right. \\ & \left. + \frac{248}{9} L_{ud ij}^{S1,RR} + \frac{2995}{27} L_{ud ij}^{S8,RR} \right] + \alpha_s \alpha \left[ -\frac{868}{27} L_{uddu ij}^{S1,RR} + \frac{1370}{81} L_{uddu ij}^{S8,RR} + \frac{112}{9} L_{ud ij}^{S1,RR} \right. \\ & \left. + \frac{112}{9} L_{ud ij}^{S8,RR} \right] ; \end{aligned}$$

$$\begin{aligned}
& + \frac{224}{9} L_{ijj}^{S8,RR} \Big] + \alpha^2 \left[ \frac{212}{243} L_{ijji}^{S1,RR} - \frac{106}{729} L_{ijji}^{S8,RR} + \frac{6059}{243} L_{ijji}^{S8,RR} \right]; \\
\dot{L}_{ijji}^{S1,RR} &= g_s^2 \left[ -16 L_{ijji}^{S1,RR} + \frac{16}{9} L_{ijji}^{S8,RR} + \frac{64}{9} L_{ijji}^{S1,RR} + \frac{112}{27} L_{ijji}^{S8,RR} \right] \\
& + e^2 \left[ \frac{26}{9} L_{ijji}^{S1,RR} - \frac{32}{27} L_{ijji}^{S1,RR} - \frac{128}{81} L_{ijji}^{S8,RR} \right] + \alpha_s^2 \left[ -\frac{2120}{9} L_{ijji}^{S1,RR} + \frac{928}{81} L_{ijji}^{S8,RR} \right. \\
& + \frac{9472}{81} L_{ijji}^{S1,RR} + \frac{16576}{243} L_{ijji}^{S8,RR} \Big] + \alpha_s \alpha \left[ \frac{712}{27} L_{ijji}^{S1,RR} - \frac{64}{81} L_{ijji}^{S8,RR} - \frac{2144}{81} L_{ijji}^{S1,RR} \right. \\
& - \frac{7784}{243} L_{ijji}^{S8,RR} \Big] + \alpha^2 \left[ -\frac{13201}{243} L_{ijji}^{S1,RR} + \frac{5200}{729} L_{ijji}^{S1,RR} + \frac{20800}{2187} L_{ijji}^{S8,RR} \right]; \\
\dot{L}_{ijji}^{S8,RR} &= g_s^2 \left[ 8 L_{ijji}^{S1,RR} + \frac{16}{3} L_{ijji}^{S8,RR} - \frac{16}{3} L_{ijji}^{S1,RR} + \frac{44}{9} L_{ijji}^{S8,RR} \right] \\
& + e^2 \left[ \frac{26}{9} L_{ijji}^{S8,RR} - \frac{64}{9} L_{ijji}^{S1,RR} + \frac{32}{27} L_{ijji}^{S8,RR} \right] + \alpha_s^2 \left[ \frac{248}{9} L_{ijji}^{S1,RR} + \frac{2995}{27} L_{ijji}^{S8,RR} \right. \\
& - \frac{856}{27} L_{ijji}^{S1,RR} - \frac{2506}{81} L_{ijji}^{S8,RR} \Big] + \alpha_s \alpha \left[ -\frac{32}{9} L_{ijji}^{S1,RR} - \frac{400}{9} L_{ijji}^{S8,RR} + \frac{3704}{27} L_{ijji}^{S1,RR} \right. \\
& - \frac{2050}{81} L_{ijji}^{S8,RR} \Big] + \alpha^2 \left[ -\frac{13201}{243} L_{ijji}^{S8,RR} + \frac{10400}{243} L_{ijji}^{S1,RR} - \frac{5200}{729} L_{ijji}^{S8,RR} \right]; \\
\dot{L}_{jji}^{S,RR} &= -8g_s^2 L_{jji}^{S,RR} + e^2 \left[ -\frac{20}{3} L_{jji}^{S,RR} - 32 L_{jji}^{T,RR} \right] - \frac{1012}{9} \alpha_s^2 L_{jji}^{S,RR} \\
& + \alpha_s \alpha \left[ \frac{1792}{9} L_{jji}^{T,RR} - \frac{8}{9} L_{jji}^{S,RR} \right] + \alpha^2 \left[ \frac{1682}{81} L_{jji}^{S,RR} + 704 L_{jji}^{T,RR} \right]; \\
\dot{L}_{jji}^{T,RR} &= \frac{8}{3} g_s^2 L_{jji}^{T,RR} + e^2 \left[ \frac{20}{9} L_{jji}^{T,RR} - \frac{2}{3} L_{jji}^{S,RR} \right] + \frac{1652}{27} \alpha_s^2 L_{jji}^{T,RR} \\
& + \alpha_s \alpha \left[ \frac{16}{3} L_{jji}^{S,RR} - \frac{152}{27} L_{jji}^{T,RR} \right] + \alpha^2 \left[ \frac{364}{81} L_{jji}^{S,RR} - \frac{6922}{243} L_{jji}^{T,RR} \right]; \\
\dot{L}_{jji}^{eu,RR} &= -8g_s^2 L_{jji}^{eu,RR} + e^2 \left[ 64 L_{jji}^{eu,RR} - \frac{26}{3} L_{jji}^{eu,RR} \right] - \frac{1012}{9} \alpha_s^2 L_{jji}^{eu,RR}
\end{aligned}$$

$$\begin{aligned}
& + \alpha_s \alpha \left[ -\frac{32}{9} L_{jji}^{S,RR} - \frac{3584}{9} L_{jji}^{T,RR} \right] + \alpha^2 \left[ -\frac{2839}{81} L_{jji}^{S,RR} - \frac{11264}{9} L_{jji}^{T,RR} \right]; \\
\dot{L}_{jji}^{T,RR} &= \frac{8}{3} g_s^2 L_{jji}^{T,RR} + e^2 \left[ \frac{4}{3} L_{jji}^{S,RR} + \frac{26}{9} L_{jji}^{T,RR} \right] + \frac{1652}{27} \alpha_s^2 L_{jji}^{T,RR} \\
& + \alpha_s \alpha \left[ -\frac{32}{3} L_{jji}^{S,RR} - \frac{608}{27} L_{jji}^{T,RR} \right] + \alpha^2 \left[ -\frac{1376}{81} L_{jji}^{S,RR} - \frac{20677}{243} L_{jji}^{T,RR} \right]; \\
\dot{L}_{jji}^{S,LL} &= \frac{353}{9} \alpha^2 L_{jji}^{S,LL} - 6e^2 L_{jji}^{S,LL}; \\
\dot{L}_{jji}^{T,LL} &= 2e^2 L_{jji}^{T,LL} - \frac{1501}{27} \alpha^2 L_{jji}^{T,LL}; \\
\dot{L}_{jji}^{S,LL} &= -8g_s^2 L_{jji}^{S,LL} - \frac{2}{3} e^2 L_{jji}^{S,LL} - \frac{1012}{9} \alpha_s^2 L_{jji}^{S,LL} - \frac{8}{9} \alpha_s \alpha L_{jji}^{S,LL} \\
& + \frac{377}{81} \alpha^2 L_{jji}^{S,LL}; \\
\dot{L}_{jji}^{T,LL} &= \frac{8}{3} g_s^2 L_{jji}^{T,LL} + \frac{2}{9} e^2 L_{jji}^{T,LL} + \frac{1652}{27} \alpha_s^2 L_{jji}^{T,LL} - \frac{152}{27} \alpha_s \alpha L_{jji}^{T,LL} \\
& - \frac{1045}{243} \alpha^2 L_{jji}^{T,LL}; \\
\dot{L}_{jji}^{S,LL} &= -8g_s^2 L_{jji}^{S,LL} - \frac{8}{3} e^2 L_{jji}^{S,LL} - \frac{1012}{9} \alpha_s^2 L_{jji}^{S,LL} - \frac{32}{9} \alpha_s \alpha L_{jji}^{S,LL} \\
& + \frac{1472}{81} \alpha^2 L_{jji}^{S,LL}; \\
\dot{L}_{jji}^{T,LL} &= \frac{8}{3} g_s^2 L_{jji}^{T,LL} + \frac{8}{9} e^2 L_{jji}^{T,LL} + \frac{1652}{27} \alpha_s^2 L_{jji}^{T,LL} - \frac{608}{27} \alpha_s \alpha L_{jji}^{T,LL} \\
& - \frac{4864}{243} \alpha^2 L_{jji}^{T,LL}; \\
\dot{L}_{jji}^{S1,RR} &= g_s^2 \left[ \frac{64}{9} L_{jji}^{S1,RR} + \frac{112}{27} L_{jji}^{S8,RR} - 16 L_{jji}^{S1,RR} + \frac{16}{9} L_{jji}^{S8,RR} \right] \\
& + e^2 \left[ \frac{4}{27} L_{jji}^{S1,RR} + \frac{16}{81} L_{jji}^{S8,RR} - \frac{46}{9} L_{jji}^{S1,RR} \right] + \alpha_s^2 \left[ \frac{9472}{81} L_{jji}^{S1,RR} + \frac{16576}{243} L_{jji}^{S8,RR} \right. \\
& \left. - \frac{2120}{9} L_{jji}^{S1,RR} + \frac{928}{81} L_{jji}^{S8,RR} \right] + \alpha_s \alpha \left[ \frac{1888}{81} L_{jji}^{S1,RR} + \frac{3808}{243} L_{jji}^{S8,RR} + \frac{136}{27} L_{jji}^{S1,RR} \right]
\end{aligned}$$



$$\begin{aligned}
& + \frac{224}{81} L_{jji}^{S8,RR} \Big] + \alpha^2 \Big[ \frac{106}{729} L_{jij}^{S1,RR} + \frac{424}{2187} L_{jij}^{S8,RR} + \frac{6059}{243} L_{jji}^{S1,RR} \Big] ; \\
\dot{L}_{jji}^{S8,RR} &= g_s^2 \Big[ -\frac{16}{3} L_{jij}^{S1,RR} + \frac{44}{9} L_{jij}^{S8,RR} + 8 L_{jji}^{S1,RR} + \frac{16}{3} L_{jji}^{S8,RR} \Big] \\
& + e^2 \Big[ \frac{8}{9} L_{jij}^{S1,RR} - \frac{4}{27} L_{jij}^{S8,RR} - \frac{46}{9} L_{jji}^{S8,RR} \Big] + \alpha_s^2 \Big[ -\frac{856}{27} L_{jij}^{S1,RR} - \frac{2506}{81} L_{jij}^{S8,RR} \\
& + \frac{248}{9} L_{jji}^{S1,RR} + \frac{2995}{27} L_{jji}^{S8,RR} \Big] + \alpha_s \alpha \Big[ -\frac{868}{27} L_{jij}^{S1,RR} + \frac{1370}{81} L_{jij}^{S8,RR} + \frac{112}{9} L_{jji}^{S1,RR} \\
& + \frac{224}{9} L_{jji}^{S8,RR} \Big] + \alpha^2 \Big[ \frac{212}{243} L_{jij}^{S1,RR} - \frac{106}{729} L_{jij}^{S8,RR} + \frac{6059}{243} L_{jji}^{S8,RR} \Big] ; \\
\dot{L}_{jij}^{S1,RR} &= g_s^2 \Big[ -16 L_{jij}^{S1,RR} + \frac{16}{9} L_{jij}^{S8,RR} + \frac{64}{9} L_{jji}^{S1,RR} + \frac{112}{27} L_{jji}^{S8,RR} \Big] \\
& + e^2 \Big[ \frac{26}{9} L_{jij}^{S1,RR} - \frac{32}{27} L_{jji}^{S1,RR} - \frac{128}{81} L_{jji}^{S8,RR} \Big] + \alpha_s^2 \Big[ -\frac{2120}{9} L_{jij}^{S1,RR} + \frac{928}{81} L_{jij}^{S8,RR} \\
& + \frac{9472}{81} L_{jji}^{S1,RR} + \frac{16576}{243} L_{jji}^{S8,RR} \Big] + \alpha_s \alpha \Big[ \frac{712}{27} L_{jij}^{S1,RR} - \frac{64}{81} L_{jij}^{S8,RR} - \frac{2144}{81} L_{jji}^{S1,RR} \\
& - \frac{7784}{243} L_{jji}^{S8,RR} \Big] + \alpha^2 \Big[ -\frac{13201}{243} L_{jij}^{S1,RR} + \frac{5200}{729} L_{jji}^{S1,RR} + \frac{20800}{2187} L_{jji}^{S8,RR} \Big] ; \\
\dot{L}_{jij}^{S8,RR} &= g_s^2 \Big[ 8 L_{jij}^{S1,RR} + \frac{16}{3} L_{jij}^{S8,RR} - \frac{16}{3} L_{jji}^{S1,RR} + \frac{44}{9} L_{jji}^{S8,RR} \Big] \\
& + e^2 \Big[ \frac{26}{9} L_{jij}^{S8,RR} - \frac{64}{9} L_{jji}^{S1,RR} + \frac{32}{27} L_{jji}^{S8,RR} \Big] + \alpha_s^2 \Big[ \frac{248}{9} L_{jij}^{S1,RR} + \frac{2995}{27} L_{jij}^{S8,RR} \\
& - \frac{856}{27} L_{jji}^{S1,RR} - \frac{2506}{81} L_{jji}^{S8,RR} \Big] + \alpha_s \alpha \Big[ -\frac{32}{9} L_{jij}^{S1,RR} - \frac{400}{9} L_{jij}^{S8,RR} + \frac{3704}{27} L_{jji}^{S1,RR} \\
& - \frac{2050}{81} L_{jji}^{S8,RR} \Big] + \alpha^2 \Big[ -\frac{13201}{243} L_{jij}^{S8,RR} + \frac{10400}{243} L_{jji}^{S1,RR} - \frac{5200}{729} L_{jji}^{S8,RR} \Big] ; \\
\dot{L}_{ijj}^{S1,RR} &= g_s^2 \Big[ -16 L_{ijj}^{S1,RR} + \frac{64}{9} L_{ijj}^{S1,RR} + \frac{16}{9} L_{ijj}^{S8,RR} + \frac{112}{27} L_{ijj}^{S8,RR} \Big]
\end{aligned}$$

$$\begin{aligned}
& + e^2 \left[ -\frac{4}{9} L_{\ddot{ij}j}^{S1,RR} + \frac{16}{27} L_{\ddot{ij}ji}^{S1,RR} + \frac{64}{81} L_{\ddot{ij}ji}^{S8,RR} \right] + \alpha_s^2 \left[ -\frac{2120}{9} L_{\ddot{ij}j}^{S1,RR} + \frac{9472}{81} L_{\ddot{ij}ji}^{S1,RR} \right. \\
& + \frac{928}{81} L_{\ddot{ij}j}^{S8,RR} + \frac{16576}{243} L_{\ddot{ij}ji}^{S8,RR} \left. \right] + \alpha_s \alpha \left[ -\frac{176}{27} L_{\ddot{ij}j}^{S1,RR} - \frac{512}{81} L_{\ddot{ij}ji}^{S1,RR} - \frac{256}{81} L_{\ddot{ij}j}^{S8,RR} \right. \\
& + \frac{1120}{243} L_{\ddot{ij}ji}^{S8,RR} \left. \right] + \alpha^2 \left[ \frac{1718}{243} L_{\ddot{ij}j}^{S1,RR} - \frac{800}{729} L_{\ddot{ij}ji}^{S1,RR} - \frac{3200}{2187} L_{\ddot{ij}j}^{S8,RR} \right] ; \\
\dot{L}_{\ddot{ij}j}^{S8,RR} & = g_s^2 \left[ 8 L_{\ddot{ij}j}^{S1,RR} - \frac{16}{3} L_{\ddot{ij}ji}^{S1,RR} + \frac{16}{3} L_{\ddot{ij}j}^{S8,RR} + \frac{44}{9} L_{\ddot{ij}ji}^{S8,RR} \right] + e^2 \left[ \frac{32}{9} L_{\ddot{ij}j}^{S1,RR} \right. \\
& - \frac{4}{9} L_{\ddot{ij}j}^{S8,RR} - \frac{16}{27} L_{\ddot{ij}ji}^{S8,RR} \left. \right] + \alpha_s^2 \left[ \frac{248}{9} L_{\ddot{ij}j}^{S1,RR} - \frac{856}{27} L_{\ddot{ij}ji}^{S1,RR} + \frac{2995}{27} L_{\ddot{ij}j}^{S8,RR} \right. \\
& - \frac{2506}{81} L_{\ddot{ij}ji}^{S8,RR} \left. \right] + \alpha_s \alpha \left[ -\frac{128}{9} L_{\ddot{ij}j}^{S1,RR} - \frac{1456}{27} L_{\ddot{ij}ji}^{S1,RR} - \frac{16}{9} L_{\ddot{ij}j}^{S8,RR} - \frac{64}{81} L_{\ddot{ij}ji}^{S8,RR} \right] \\
& + \alpha^2 \left[ -\frac{1600}{243} L_{\ddot{ij}j}^{S1,RR} + \frac{1718}{243} L_{\ddot{ij}j}^{S8,RR} + \frac{800}{729} L_{\ddot{ij}ji}^{S8,RR} \right] ; \\
\dot{L}_{\ddot{ij}ji}^{S1,RR} & = g_s^2 \left[ \frac{64}{9} L_{\ddot{ij}j}^{S1,RR} - 16 L_{\ddot{ij}ji}^{S1,RR} + \frac{112}{27} L_{\ddot{ij}j}^{S8,RR} + \frac{16}{9} L_{\ddot{ij}ji}^{S8,RR} \right] \\
& + e^2 \left[ \frac{16}{27} L_{\ddot{ij}j}^{S1,RR} - \frac{4}{9} L_{\ddot{ij}ji}^{S1,RR} + \frac{64}{81} L_{\ddot{ij}j}^{S8,RR} \right] + \alpha_s^2 \left[ \frac{9472}{81} L_{\ddot{ij}j}^{S1,RR} - \frac{2120}{9} L_{\ddot{ij}ji}^{S1,RR} \right. \\
& + \frac{16576}{243} L_{\ddot{ij}j}^{S8,RR} + \frac{928}{81} L_{\ddot{ij}ji}^{S8,RR} \left. \right] + \alpha_s \alpha \left[ -\frac{512}{81} L_{\ddot{ij}j}^{S1,RR} - \frac{176}{27} L_{\ddot{ij}ji}^{S1,RR} + \frac{1120}{243} L_{\ddot{ij}j}^{S8,RR} \right. \\
& - \frac{256}{81} L_{\ddot{ij}ji}^{S8,RR} \left. \right] + \alpha^2 \left[ -\frac{800}{729} L_{\ddot{ij}j}^{S1,RR} + \frac{1718}{243} L_{\ddot{ij}ji}^{S1,RR} - \frac{3200}{2187} L_{\ddot{ij}j}^{S8,RR} \right] ; \\
\dot{L}_{\ddot{ij}ji}^{S8,RR} & = g_s^2 \left[ -\frac{16}{3} L_{\ddot{ij}j}^{S1,RR} + 8 L_{\ddot{ij}ji}^{S1,RR} + \frac{44}{9} L_{\ddot{ij}j}^{S8,RR} + \frac{16}{3} L_{\ddot{ij}ji}^{S8,RR} \right] \\
& + e^2 \left[ \frac{32}{9} L_{\ddot{ij}j}^{S1,RR} - \frac{16}{27} L_{\ddot{ij}j}^{S8,RR} - \frac{4}{9} L_{\ddot{ij}ji}^{S8,RR} \right] + \alpha_s^2 \left[ -\frac{856}{27} L_{\ddot{ij}j}^{S1,RR} + \frac{248}{9} L_{\ddot{ij}ji}^{S1,RR} \right. \\
& - \frac{2506}{81} L_{\ddot{ij}j}^{S8,RR} + \frac{2995}{27} L_{\ddot{ij}ji}^{S8,RR} \left. \right] + \alpha_s \alpha \left[ -\frac{1456}{27} L_{\ddot{ij}j}^{S1,RR} - \frac{128}{9} L_{\ddot{ij}ji}^{S1,RR} - \frac{64}{81} L_{\ddot{ij}j}^{S8,RR} \right.
\end{aligned}$$

$$\begin{aligned}
& -\frac{16}{9}L_{ijji}^{S8,RR} \Big] + \alpha^2 \Big[ -\frac{1600}{243}L_{ijj}^{S1,RR} + \frac{800}{729}L_{ijj}^{S8,RR} + \frac{1718}{243}L_{ijji}^{S8,RR} \Big] ; \\
\dot{L}_{dd\bar{iii}}^{S1,RR} &= g_s^2 \Big[ \frac{160}{27}L_{iii}^{S8,RR} - \frac{80}{9}L_{iii}^{S1,RR} \Big] + e^2 \Big[ \frac{4}{27}L_{iii}^{S1,RR} + \frac{64}{81}L_{iii}^{S8,RR} \Big] \\
& + \alpha_s^2 \Big[ \frac{19360}{243}L_{iii}^{S8,RR} - \frac{9608}{81}L_{iii}^{S1,RR} \Big] + \alpha_s \alpha \Big[ \frac{352}{243}L_{iii}^{S8,RR} - \frac{1040}{81}L_{iii}^{S1,RR} \Big] \\
& + \alpha^2 \Big[ \frac{4354}{729}L_{iii}^{S1,RR} - \frac{3200}{2187}L_{iii}^{S8,RR} \Big] ; \\
\dot{L}_{dd\bar{iii}}^{S8,RR} &= g_s^2 \Big[ \frac{8}{3}L_{iii}^{S1,RR} + \frac{92}{9}L_{iii}^{S8,RR} \Big] + e^2 \Big[ \frac{32}{9}L_{iii}^{S1,RR} - \frac{28}{27}L_{iii}^{S8,RR} \Big] \\
& + \alpha_s^2 \Big[ \frac{6479}{81}L_{iii}^{S8,RR} - \frac{112}{27}L_{iii}^{S1,RR} \Big] + \alpha_s \alpha \Big[ -\frac{1840}{27}L_{iii}^{S1,RR} - \frac{208}{81}L_{iii}^{S8,RR} \Big] \\
& + \alpha^2 \Big[ \frac{5954}{729}L_{iii}^{S8,RR} - \frac{1600}{243}L_{iii}^{S1,RR} \Big] ; \\
\dot{L}_{uu\bar{ijj}}^{S1,RR} &= g_s^2 \Big[ -16L_{ijj}^{S1,RR} + \frac{64}{9}L_{ijji}^{S1,RR} + \frac{16}{9}L_{ijj}^{S8,RR} + \frac{112}{27}L_{ijji}^{S8,RR} \Big] \\
& + e^2 \Big[ -\frac{16}{9}L_{ijj}^{S1,RR} + \frac{64}{27}L_{ijji}^{S1,RR} + \frac{256}{81}L_{ijji}^{S8,RR} \Big] + \alpha_s^2 \Big[ -\frac{2120}{9}L_{ijj}^{S1,RR} + \frac{9472}{81}L_{ijji}^{S1,RR} \\
& + \frac{928}{81}L_{ijj}^{S8,RR} + \frac{16576}{243}L_{ijji}^{S8,RR} \Big] + \alpha_s \alpha \Big[ -\frac{704}{27}L_{ijj}^{S1,RR} - \frac{2048}{81}L_{ijji}^{S1,RR} - \frac{1024}{81}L_{ijj}^{S8,RR} \\
& + \frac{4480}{243}L_{ijji}^{S8,RR} \Big] + \alpha^2 \Big[ \frac{3776}{243}L_{ijj}^{S1,RR} - \frac{5504}{729}L_{ijji}^{S1,RR} - \frac{22016}{2187}L_{ijji}^{S8,RR} \Big] ; \\
\dot{L}_{uu\bar{ijj}}^{S8,RR} &= g_s^2 \Big[ 8L_{ijj}^{S1,RR} - \frac{16}{3}L_{ijji}^{S1,RR} + \frac{16}{3}L_{ijj}^{S8,RR} + \frac{44}{9}L_{ijji}^{S8,RR} \Big] + e^2 \Big[ \frac{128}{9}L_{ijji}^{S1,RR} \\
& - \frac{16}{9}L_{ijj}^{S8,RR} - \frac{64}{27}L_{ijji}^{S8,RR} \Big] + \alpha_s^2 \Big[ \frac{248}{9}L_{ijj}^{S1,RR} - \frac{856}{27}L_{ijji}^{S1,RR} + \frac{2995}{27}L_{ijj}^{S8,RR} \\
& - \frac{2506}{81}L_{ijji}^{S8,RR} \Big] + \alpha_s \alpha \Big[ -\frac{512}{9}L_{ijj}^{S1,RR} - \frac{5824}{27}L_{ijji}^{S1,RR} - \frac{64}{9}L_{ijj}^{S8,RR} - \frac{256}{81}L_{ijji}^{S8,RR} \Big]
\end{aligned}$$

$$\begin{aligned}
& + \alpha^2 \left[ -\frac{11008}{243} L_{ijji}^{S1,RR} + \frac{3776}{243} L_{ijj}^{S8,RR} + \frac{5504}{729} L_{ijji}^{S8,RR} \right]; \\
\dot{L}_{ijji}^{S1,RR} &= g_s^2 \left[ \frac{64}{9} L_{ijj}^{S1,RR} - 16 L_{ijji}^{S1,RR} + \frac{112}{27} L_{ijj}^{S8,RR} + \frac{16}{9} L_{ijji}^{S8,RR} \right] \\
& + e^2 \left[ \frac{64}{27} L_{ijj}^{S1,RR} - \frac{16}{9} L_{ijji}^{S1,RR} + \frac{256}{81} L_{ijj}^{S8,RR} \right] + \alpha_s^2 \left[ \frac{9472}{81} L_{ijj}^{S1,RR} - \frac{2120}{9} L_{ijji}^{S1,RR} \right. \\
& + \frac{16576}{243} L_{ijj}^{S8,RR} + \frac{928}{81} L_{ijji}^{S8,RR} \left. \right] + \alpha_s \alpha \left[ -\frac{2048}{81} L_{ijj}^{S1,RR} - \frac{704}{27} L_{ijji}^{S1,RR} + \frac{4480}{243} L_{ijj}^{S8,RR} \right. \\
& - \frac{1024}{81} L_{ijji}^{S8,RR} \left. \right] + \alpha^2 \left[ -\frac{5504}{729} L_{ijj}^{S1,RR} + \frac{3776}{243} L_{ijji}^{S1,RR} - \frac{22016}{2187} L_{ijj}^{S8,RR} \right]; \\
\dot{L}_{ijji}^{S8,RR} &= g_s^2 \left[ -\frac{16}{3} L_{ijj}^{S1,RR} + 8 L_{ijji}^{S1,RR} + \frac{44}{9} L_{ijj}^{S8,RR} + \frac{16}{3} L_{ijji}^{S8,RR} \right] \\
& + e^2 \left[ \frac{128}{9} L_{ijj}^{S1,RR} - \frac{64}{27} L_{ijj}^{S8,RR} - \frac{16}{9} L_{ijji}^{S8,RR} \right] + \alpha_s^2 \left[ -\frac{856}{27} L_{ijj}^{S1,RR} + \frac{248}{9} L_{ijji}^{S1,RR} \right. \\
& - \frac{2506}{81} L_{ijj}^{S8,RR} + \frac{2995}{27} L_{ijji}^{S8,RR} \left. \right] + \alpha_s \alpha \left[ -\frac{5824}{27} L_{ijj}^{S1,RR} - \frac{512}{9} L_{ijji}^{S1,RR} - \frac{256}{81} L_{ijj}^{S8,RR} \right. \\
& - \frac{64}{9} L_{ijji}^{S8,RR} \left. \right] + \alpha^2 \left[ -\frac{11008}{243} L_{ijj}^{S1,RR} + \frac{5504}{729} L_{ijj}^{S8,RR} + \frac{3776}{243} L_{ijji}^{S8,RR} \right]; \\
\dot{L}_{iii}^{S1,RR} &= g_s^2 \left[ \frac{160}{27} L_{iii}^{S8,RR} - \frac{80}{9} L_{iii}^{S1,RR} \right] + e^2 \left[ \frac{16}{27} L_{iii}^{S1,RR} + \frac{256}{81} L_{iii}^{S8,RR} \right] \\
& + \alpha_s^2 \left[ \frac{19360}{243} L_{iii}^{S8,RR} - \frac{9608}{81} L_{iii}^{S1,RR} \right] + \alpha_s \alpha \left[ \frac{1408}{243} L_{iii}^{S8,RR} - \frac{4160}{81} L_{iii}^{S1,RR} \right] \\
& + \alpha^2 \left[ \frac{5824}{729} L_{iii}^{S1,RR} - \frac{22016}{2187} L_{iii}^{S8,RR} \right]; \\
\dot{L}_{iii}^{S8,RR} &= g_s^2 \left[ \frac{8}{3} L_{iii}^{S1,RR} + \frac{92}{9} L_{iii}^{S8,RR} \right] + e^2 \left[ \frac{128}{9} L_{iii}^{S1,RR} - \frac{112}{27} L_{iii}^{S8,RR} \right] \\
& + \alpha_s^2 \left[ \frac{6479}{81} L_{iii}^{S8,RR} - \frac{112}{27} L_{iii}^{S1,RR} \right] + \alpha_s \alpha \left[ -\frac{7360}{27} L_{iii}^{S1,RR} - \frac{832}{81} L_{iii}^{S8,RR} \right]
\end{aligned}$$

$$\begin{aligned}
& + \alpha^2 \left[ \frac{16832}{729} L_{iii}^{S8,RR} - \frac{11008}{243} L_{iii}^{S1,RR} \right]; \\
\dot{L}_{ijj}^{S,RR} &= e^2 \left[ 16 L_{ijji}^{S,RR} - 4 L_{ijj}^{S,RR} \right] - \frac{5530}{27} \alpha^2 L_{ijj}^{S,RR}; \\
\dot{L}_{ijji}^{S,RR} &= e^2 \left[ 16 L_{ijj}^{S,RR} - 4 L_{ijji}^{S,RR} \right] + \frac{608}{9} \alpha^2 L_{ijji}^{S,RR}; \\
\dot{L}_{iii}^{S,RR} &= 12 e^2 L_{iii}^{S,RR} - \frac{1853}{27} \alpha^2 L_{iii}^{S,RR}; \\
\dot{L}_{ijj}^{S,LL} &= 0; \\
\dot{L}_{ijji}^{S,LL} &= 0; \\
\dot{L}_{iii}^{S,LL} &= 0; \\
\dot{L}_{ed}^{V,LL} &= e^2 \left[ 4 L_{ijj}^{V,LL} + \frac{16}{9} L_{ijj}^{V,LL} + \frac{4}{9} L_{ijj}^{V,LR} + \frac{16}{9} L_{ikk}^{V,LL} + \frac{4}{9} L_{ikk}^{V,LR} \right. \\
& + \frac{4}{9} L_{ii11}^{V,LL} + \frac{4}{9} L_{ii22}^{V,LL} + \frac{4}{9} L_{ii11}^{V,LR} + \frac{4}{9} L_{ii22}^{V,LR} + \frac{16}{9} L_{iii}^{V,LL} + \frac{4}{9} L_{iii}^{V,LR} \\
& - \frac{8}{9} L_{ii11}^{V,LL} - \frac{8}{9} L_{ii22}^{V,LL} - \frac{8}{9} L_{ii11}^{V,LR} - \frac{8}{9} L_{ii22}^{V,LR} + \frac{8}{3} L_{jjjj}^{V1,LR} + \frac{64}{9} L_{jjjj}^{V,LL} \\
& + \frac{4}{3} L_{jj11}^{V,LR} + \frac{4}{3} L_{jj22}^{V,LR} + \frac{4}{3} L_{jj33}^{V,LR} - \frac{8}{3} L_{jj11}^{V1,LR} - \frac{8}{3} L_{jj22}^{V1,LR} + \frac{4}{3} L_{11jj}^{V,LL} \\
& + \frac{4}{3} L_{22jj}^{V,LL} + \frac{4}{3} L_{33jj}^{V,LL} - \frac{8}{3} L_{11jj}^{V1,LL} - \frac{8}{3} L_{22jj}^{V1,LL} \left. \right] + \alpha_s^2 \left[ 8 L_{ii11}^{V,LL} \right. \\
& + 8 L_{ii22}^{V,LL} - 8 L_{ii11}^{V,LR} - 8 L_{ii22}^{V,LR} + 8 L_{ii11}^{V,LL} + 8 L_{ii22}^{V,LL} - 8 L_{ii11}^{V,LR} \\
& - 8 L_{ii22}^{V,LR} \left. \right] + \alpha_s \alpha \left[ -16 L_{ijj}^{V,LL} + \frac{16}{9} L_{ii11}^{V,LL} + \frac{16}{9} L_{ii22}^{V,LL} + \frac{16}{9} L_{ii11}^{V,LR} \right. \\
& + \frac{16}{9} L_{ii22}^{V,LR} - \frac{32}{9} L_{ii11}^{V,LL} - \frac{32}{9} L_{ii22}^{V,LL} - \frac{32}{9} L_{ii11}^{V,LR} - \frac{32}{9} L_{ii22}^{V,LR} + \frac{32}{3} L_{jjjj}^{V1,LR} \\
& - \frac{2044}{243} L_{jjjj}^{V8,LR} + \frac{5152}{243} L_{jjjj}^{V,LL} - \frac{32}{3} L_{jj11}^{V1,LR} - \frac{32}{3} L_{jj22}^{V1,LR} + \frac{1354}{243} L_{jj11}^{V8,LR}
\end{aligned}$$

$$\begin{aligned}
& + \frac{1354}{243} L_{jj22}^{V8,LR} - \frac{32}{3} L_{11jj}^{V1,LL} - \frac{32}{3} L_{22jj}^{V1,LL} - \frac{86}{243} L_{11jj}^{V8,LL} - \frac{86}{243} L_{22jj}^{V8,LL} \Bigg] \\
& + \alpha^2 \Bigg[ - \frac{334}{27} L_{ijjj}^{V,LL} + \frac{224}{81} L_{ijjj}^{V,LL} - \frac{520}{81} L_{ijjj}^{V,LR} + \frac{224}{81} L_{iikk}^{V,LL} - \frac{520}{81} L_{iikk}^{V,LR} \\
& - \frac{104}{243} L_{ii11}^{V,LL} - \frac{104}{243} L_{ii22}^{V,LL} - \frac{200}{243} L_{ii11}^{V,LR} - \frac{200}{243} L_{ii22}^{V,LR} + \frac{32}{81} L_{iii}^{V,LL} - \frac{520}{81} L_{iii}^{V,LR} \\
& - \frac{1016}{243} L_{ii11}^{V,LL} - \frac{1016}{243} L_{ii22}^{V,LL} - \frac{1400}{243} L_{ii11}^{V,LR} - \frac{1400}{243} L_{ii22}^{V,LR} - \frac{2624}{243} L_{jjjj}^{V1,LR} \\
& + \frac{23296}{729} L_{jjjj}^{V,LL} - \frac{3184}{243} L_{jj11}^{V,LR} - \frac{3184}{243} L_{jj22}^{V,LR} - \frac{3184}{243} L_{jj33}^{V,LR} - \frac{6232}{243} L_{jj11}^{V1,LR} \\
& - \frac{6232}{243} L_{jj22}^{V1,LR} + \frac{3728}{243} L_{11jj}^{V,LL} + \frac{3728}{243} L_{22jj}^{V,LL} + \frac{3728}{243} L_{33jj}^{V,LL} + \frac{2984}{243} L_{11jj}^{V1,LL} \\
& + \frac{2984}{243} L_{22jj}^{V1,LL} \Bigg] ;
\end{aligned}$$

$$\begin{aligned}
\dot{L}_{ijj}^{V,LL} & = e^2 \Bigg[ - \frac{8}{9} L_{ii11}^{V,LL} - \frac{8}{9} L_{ii22}^{V,LL} - \frac{8}{9} L_{ii11}^{V,LR} - \frac{8}{9} L_{ii22}^{V,LR} - \frac{32}{9} L_{iii}^{V,LL} \\
& - \frac{32}{9} L_{ijj}^{V,LL} - \frac{32}{9} L_{iikk}^{V,LL} - \frac{8}{9} L_{iii}^{V,LR} - \frac{8}{9} L_{ijj}^{V,LR} - \frac{8}{9} L_{iikk}^{V,LR} + \frac{4}{3} L_{11jj}^{V,LL} \\
& + \frac{4}{3} L_{22jj}^{V,LL} + \frac{4}{3} L_{33jj}^{V,LL} + \frac{16}{9} L_{ii11}^{V,LL} + \frac{16}{9} L_{ii22}^{V,LL} - 8 L_{ijj}^{V,LL} + \frac{16}{9} L_{ii11}^{V,LR} \\
& + \frac{16}{9} L_{ii22}^{V,LR} + \frac{4}{3} L_{jj11}^{V1,LL} + \frac{4}{3} L_{jj22}^{V1,LL} + \frac{4}{3} L_{jj11}^{V1,LR} + \frac{4}{3} L_{jj22}^{V1,LR} + \frac{4}{3} L_{jj11}^{V,LR} \\
& + \frac{4}{3} L_{jj22}^{V,LR} + \frac{4}{3} L_{jj33}^{V,LR} - \frac{8}{3} L_{jjjj}^{V1,LR} - \frac{8}{3} L_{jjkk}^{V1,LR} - \frac{64}{9} L_{jjjj}^{V,LL} - \frac{16}{3} L_{jjkk}^{V,LL} \\
& - \frac{16}{9} L_{jjkk}^{V,LL} \Bigg] + \alpha_s^2 \Bigg[ 8 L_{ii11}^{V,LL} + 8 L_{ii22}^{V,LL} - 8 L_{ii11}^{V,LR} - 8 L_{ii22}^{V,LR} \\
& + 8 L_{ii11}^{V,LL} + 8 L_{ii22}^{V,LL} - 8 L_{ii11}^{V,LR} - 8 L_{ii22}^{V,LR} \Bigg] + \alpha_s \alpha \Bigg[ - \frac{32}{9} L_{ii11}^{V,LL} \\
& - \frac{32}{9} L_{ii22}^{V,LL} - \frac{32}{9} L_{ii11}^{V,LR} - \frac{32}{9} L_{ii22}^{V,LR} + \frac{64}{9} L_{ii11}^{V,LL} + \frac{64}{9} L_{ii22}^{V,LL} + 32 L_{ijj}^{V,LL} \\
& + \frac{64}{9} L_{ii11}^{V,LR} + \frac{64}{9} L_{ii22}^{V,LR} + \frac{16}{3} L_{jj11}^{V1,LL} + \frac{16}{3} L_{jj22}^{V1,LL} + \frac{16}{3} L_{jj11}^{V1,LR} - \frac{32}{3} L_{jj22}^{V1,LR} \\
& + \frac{388}{243} L_{jj11}^{V8,LL} + \frac{388}{243} L_{jj22}^{V8,LL} - \frac{332}{243} L_{jj11}^{V8,LR} + \frac{2044}{243} L_{jj22}^{V8,LR} - \frac{32}{3} L_{jjjj}^{V1,LR}
\end{aligned}$$

$$\begin{aligned}
& -\frac{32}{3}L_{jjkk}^{V1,LR} + \frac{2044}{243}L_{jjjj}^{V8,LR} + \frac{2044}{243}L_{jjkk}^{V8,LR} - \frac{2096}{81}L_{jjjj}^{V,LL} - 16L_{jjkk}^{V,LL} - \frac{128}{243}L_{jkkj}^{V,LL} \Big] \\
& + \alpha^2 \Big[ \frac{2512}{243}L_{ii11}^{V,LL} + \frac{2512}{243}L_{ii22}^{V,LL} + \frac{1408}{243}L_{ii11}^{V,LR} + \frac{1408}{243}L_{ii22}^{V,LR} + \frac{3680}{81}L_{iii}^{V,LL} \\
& + \frac{2432}{81}L_{iijj}^{V,LL} + \frac{2432}{81}L_{iikk}^{V,LL} + \frac{464}{81}L_{iii}^{V,LR} + \frac{464}{81}L_{iijj}^{V,LR} + \frac{464}{81}L_{iikk}^{V,LR} + \frac{3248}{243}L_{11jj}^{V,LL} \\
& + \frac{3248}{243}L_{22jj}^{V,LL} + \frac{3248}{243}L_{33jj}^{V,LL} + \frac{1312}{243}L_{ii11}^{V,LL} + \frac{1312}{243}L_{ii22}^{V,LL} + \frac{128}{27}L_{iijj}^{V,LL} \\
& - \frac{3104}{243}L_{ii11}^{V,LR} - \frac{3104}{243}L_{ii22}^{V,LR} + \frac{296}{243}L_{jj11}^{V1,LL} + \frac{296}{243}L_{jj22}^{V1,LL} - \frac{928}{243}L_{jj11}^{V1,LR} \\
& + \frac{416}{243}L_{jj22}^{V1,LR} - \frac{424}{243}L_{jj11}^{V,LR} - \frac{424}{243}L_{jj22}^{V,LR} - \frac{424}{243}L_{jj33}^{V,LR} + \frac{128}{243}L_{jjjj}^{V1,LR} \\
& + \frac{128}{243}L_{jjkk}^{V1,LR} + \frac{26272}{243}L_{jjjj}^{V,LL} + \frac{10048}{243}L_{jjkk}^{V,LL} + \frac{18304}{729}L_{jkkj}^{V,LL} \Big] ;
\end{aligned}$$

$$\begin{aligned}
\dot{L}_{iijj}^{V,LL} &= e^2 \Big[ \frac{4}{3}L_{ii11}^{V,LL} + \frac{4}{3}L_{ii22}^{V,LL} + \frac{4}{3}L_{ii11}^{V,LR} + \frac{4}{3}L_{ii22}^{V,LR} + \frac{4}{3}L_{iijj}^{V,LL} \\
& + \frac{4}{3}L_{iijj}^{V,LL} + \frac{4}{3}L_{iikk}^{V,LL} + \frac{4}{3}L_{iijj}^{V,LR} + \frac{4}{3}L_{iikk}^{V,LR} + \frac{4}{3}L_{iikk}^{V,LR} - \frac{8}{3}L_{iijj}^{V,LL} \\
& - \frac{8}{3}L_{iijj}^{V,LL} - \frac{8}{3}L_{iijj}^{V,LR} - \frac{8}{3}L_{iijj}^{V,LR} \Big] + \alpha_s \alpha \Big[ \frac{16}{3}L_{ii11}^{V,LL} + \frac{16}{3}L_{ii22}^{V,LL} \\
& + \frac{16}{3}L_{ii11}^{V,LR} + \frac{16}{3}L_{ii22}^{V,LR} - \frac{32}{3}L_{iijj}^{V,LL} - \frac{32}{3}L_{iijj}^{V,LL} - \frac{32}{3}L_{iijj}^{V,LR} - \frac{32}{3}L_{iijj}^{V,LR} \Big] \\
& + \alpha^2 \Big[ \frac{40}{9}L_{ii11}^{V,LL} + \frac{40}{9}L_{ii22}^{V,LL} - \frac{32}{9}L_{ii11}^{V,LR} - \frac{32}{9}L_{ii22}^{V,LR} + 16L_{iijj}^{V,LL} \\
& + 16L_{iijj}^{V,LL} + 16L_{iikk}^{V,LL} - 8L_{iijj}^{V,LR} - 8L_{iikk}^{V,LR} - 8L_{iikk}^{V,LR} + \frac{112}{9}L_{iijj}^{V,LL} \\
& + \frac{112}{9}L_{iijj}^{V,LL} - \frac{176}{9}L_{iijj}^{V,LR} - \frac{176}{9}L_{iijj}^{V,LR} \Big] ;
\end{aligned}$$

$$\begin{aligned}
\dot{L}_{iijj}^{V,LL} &= e^2 \Big[ \frac{4}{9}L_{ii11}^{V,LL} + \frac{4}{9}L_{ii22}^{V,LL} + \frac{4}{9}L_{ii11}^{V,LR} + \frac{4}{9}L_{ii22}^{V,LR} + \frac{4}{9}L_{iijj}^{V,LL} \\
& + \frac{4}{9}L_{iijj}^{V,LL} + \frac{4}{9}L_{iikk}^{V,LL} + \frac{4}{9}L_{iijj}^{V,LR} + \frac{4}{9}L_{iikk}^{V,LR} + \frac{4}{9}L_{iikk}^{V,LR} - \frac{8}{9}L_{iijj}^{V,LL} \\
& + \frac{112}{9}L_{iijj}^{V,LL} - \frac{176}{9}L_{iijj}^{V,LR} - \frac{176}{9}L_{iijj}^{V,LR} \Big] ;
\end{aligned}$$

$$\begin{aligned}
& -\frac{8}{9}L_{\nu u, ii22}^{V,LL} - \frac{8}{9}L_{\nu u, ii11}^{V,LR} - \frac{8}{9}L_{\nu u, ii22}^{V,LR} \Big] + \alpha_s^2 \Big[ 8L_{\nu d, ii11}^{V,LL} + 8L_{\nu d, ii22}^{V,LL} \\
& - 8L_{\nu d, ii11}^{V,LR} - 8L_{\nu d, ii22}^{V,LR} + 8L_{\nu u, ii11}^{V,LL} + 8L_{\nu u, ii22}^{V,LL} - 8L_{\nu u, ii11}^{V,LR} - 8L_{\nu u, ii22}^{V,LR} \Big] \\
& + \alpha_s \alpha \Big[ \frac{16}{9}L_{\nu d, ii11}^{V,LL} + \frac{16}{9}L_{\nu d, ii22}^{V,LL} + \frac{16}{9}L_{\nu d, ii11}^{V,LR} + \frac{16}{9}L_{\nu d, ii22}^{V,LR} - \frac{32}{9}L_{\nu u, ii11}^{V,LL} \\
& - \frac{32}{9}L_{\nu u, ii22}^{V,LL} - \frac{32}{9}L_{\nu u, ii11}^{V,LR} - \frac{32}{9}L_{\nu u, ii22}^{V,LR} \Big] + \alpha^2 \Big[ \frac{16}{27}L_{\nu d, ii11}^{V,LL} + \frac{16}{27}L_{\nu d, ii22}^{V,LL} \\
& - \frac{8}{27}L_{\nu d, ii11}^{V,LR} - \frac{8}{27}L_{\nu d, ii22}^{V,LR} + \frac{8}{3}L_{\nu e, ii11}^{V,LL} + \frac{8}{3}L_{\nu e, ii22}^{V,LL} + \frac{8}{3}L_{\nu e, ii33}^{V,LL} + \frac{16}{27}L_{\nu u, ii11}^{V,LL} \\
& + \frac{16}{27}L_{\nu u, ii22}^{V,LL} - \frac{80}{27}L_{\nu u, ii11}^{V,LR} - \frac{80}{27}L_{\nu u, ii22}^{V,LR} \Big] ; \\
\dot{L}_{\nu u, ij}^{V,LL} & = e^2 \Big[ -\frac{8}{9}L_{\nu d, ii11}^{V,LL} - \frac{8}{9}L_{\nu d, ii22}^{V,LL} - \frac{8}{9}L_{\nu d, ii11}^{V,LR} - \frac{8}{9}L_{\nu d, ii22}^{V,LR} - \frac{8}{9}L_{\nu e, ii11}^{V,LL} \\
& - \frac{8}{9}L_{\nu e, ii22}^{V,LL} - \frac{8}{9}L_{\nu e, ii33}^{V,LL} - \frac{8}{9}L_{\nu e, ii11}^{V,LR} - \frac{8}{9}L_{\nu e, ii22}^{V,LR} - \frac{8}{9}L_{\nu e, ii33}^{V,LR} + \frac{16}{9}L_{\nu u, ii11}^{V,LL} \\
& + \frac{16}{9}L_{\nu u, ii22}^{V,LL} + \frac{16}{9}L_{\nu u, ii11}^{V,LR} + \frac{16}{9}L_{\nu u, ii22}^{V,LR} \Big] + \alpha_s^2 \Big[ 8L_{\nu d, ii11}^{V,LL} + 8L_{\nu d, ii22}^{V,LL} \\
& - 8L_{\nu d, ii11}^{V,LR} - 8L_{\nu d, ii22}^{V,LR} + 8L_{\nu u, ii11}^{V,LL} + 8L_{\nu u, ii22}^{V,LL} - 8L_{\nu u, ii11}^{V,LR} - 8L_{\nu u, ii22}^{V,LR} \Big] \\
& + \alpha_s \alpha \Big[ -\frac{32}{9}L_{\nu d, ii11}^{V,LL} - \frac{32}{9}L_{\nu d, ii22}^{V,LL} - \frac{32}{9}L_{\nu d, ii11}^{V,LR} - \frac{32}{9}L_{\nu d, ii22}^{V,LR} + \frac{64}{9}L_{\nu u, ii11}^{V,LL} \\
& + \frac{64}{9}L_{\nu u, ii22}^{V,LL} + \frac{64}{9}L_{\nu u, ii11}^{V,LR} + \frac{64}{9}L_{\nu u, ii22}^{V,LR} \Big] + \alpha^2 \Big[ \frac{40}{27}L_{\nu d, ii11}^{V,LL} + \frac{40}{27}L_{\nu d, ii22}^{V,LL} \\
& - \frac{56}{27}L_{\nu d, ii11}^{V,LR} - \frac{56}{27}L_{\nu d, ii22}^{V,LR} + \frac{8}{3}L_{\nu e, ii11}^{V,LL} + \frac{8}{3}L_{\nu e, ii22}^{V,LL} + \frac{8}{3}L_{\nu e, ii33}^{V,LL} - 8L_{\nu e, ii11}^{V,LR} \\
& - 8L_{\nu e, ii22}^{V,LR} - 8L_{\nu e, ii33}^{V,LR} + \frac{256}{27}L_{\nu u, ii11}^{V,LL} + \frac{256}{27}L_{\nu u, ii22}^{V,LL} - \frac{128}{27}L_{\nu u, ii11}^{V,LR} \\
& - \frac{128}{27}L_{\nu u, ii22}^{V,LR} \Big] ;
\end{aligned}$$



$$\begin{aligned}
\dot{L}_{ud}^{V1,LL} = & \frac{8}{3} L_{ijj}^{V8,LL} g_s^2 + e^2 \left[ -\frac{16}{9} L_{jjj}^{V1,LR} - \frac{128}{27} L_{jjj}^{V,LL} - \frac{8}{9} L_{jj11}^{V,LR} - \frac{8}{9} L_{jj22}^{V,LR} \right. \\
& - \frac{8}{9} L_{jj33}^{V,LR} + \frac{16}{9} L_{jj11}^{V1,LR} + \frac{16}{9} L_{jj22}^{V1,LR} - \frac{8}{9} L_{11jj}^{V,LL} - \frac{8}{9} L_{22jj}^{V,LL} - \frac{8}{9} L_{33jj}^{V,LL} \\
& + \frac{4}{9} L_{11ii}^{V,LL} + \frac{4}{9} L_{22ii}^{V,LL} + \frac{4}{9} L_{33ii}^{V,LL} + \frac{16}{9} L_{11jj}^{V1,LL} + \frac{16}{9} L_{22jj}^{V1,LL} + \frac{4}{9} L_{ii11}^{V1,LL} \\
& + \frac{4}{9} L_{ii22}^{V1,LL} - \frac{8}{3} L_{iijj}^{V1,LL} + \frac{4}{9} L_{ii11}^{V1,LR} + \frac{4}{9} L_{ii22}^{V1,LR} + \frac{4}{9} L_{ii11}^{V,LR} + \frac{4}{9} L_{ii22}^{V,LR} \\
& \left. + \frac{4}{9} L_{ii33}^{V,LR} - \frac{8}{9} L_{iii}^{V1,LR} - \frac{8}{9} L_{ikk}^{V1,LR} - \frac{64}{27} L_{iii}^{V,LL} - \frac{16}{9} L_{ikk}^{V,LL} - \frac{16}{27} L_{ikki}^{V,LL} \right] \\
& + \alpha_s^2 \left[ -16 L_{jjj}^{V1,LR} + \frac{8}{27} L_{jjj}^{V8,LR} + \frac{1672}{27} L_{jjj}^{V,LL} - 8 L_{jj11}^{V1,LR} - 8 L_{jj22}^{V1,LR} \right. \\
& + \frac{4}{27} L_{jj11}^{V8,LR} + \frac{4}{27} L_{jj22}^{V8,LR} + 8 L_{11jj}^{V1,LL} + 8 L_{22jj}^{V1,LL} + 8 L_{ii11}^{V1,LL} + 8 L_{ii22}^{V1,LL} \\
& - \frac{28}{3} L_{iijj}^{V1,LL} - 8 L_{ii11}^{V1,LR} - 8 L_{ii22}^{V1,LR} + \frac{4}{27} L_{11jj}^{V8,LL} + \frac{4}{27} L_{22jj}^{V8,LL} + \frac{4}{27} L_{ii11}^{V8,LL} \\
& + \frac{4}{27} L_{ii22}^{V8,LL} + \frac{82}{27} L_{iijj}^{V8,LL} + \frac{4}{27} L_{ii11}^{V8,LR} + \frac{4}{27} L_{ii22}^{V8,LR} - 8 L_{iii}^{V1,LR} - 8 L_{ikk}^{V1,LR} \\
& + \frac{4}{27} L_{iii}^{V8,LR} + \frac{4}{27} L_{ikk}^{V8,LR} + \frac{328}{9} L_{iii}^{V,LL} + 16 L_{ikk}^{V,LL} + \frac{256}{27} L_{ikki}^{V,LL} \left. \right] + \alpha_s \alpha \left[ -\frac{64}{9} L_{jjj}^{V1,LR} \right. \\
& + \frac{4088}{729} L_{jjj}^{V8,LR} - \frac{10304}{729} L_{jjj}^{V,LL} + \frac{64}{9} L_{jj11}^{V1,LR} + \frac{64}{9} L_{jj22}^{V1,LR} - \frac{2708}{729} L_{jj11}^{V8,LR} \\
& - \frac{2708}{729} L_{jj22}^{V8,LR} + \frac{64}{9} L_{11jj}^{V1,LL} + \frac{64}{9} L_{22jj}^{V1,LL} + \frac{16}{9} L_{ii11}^{V1,LL} + \frac{16}{9} L_{ii22}^{V1,LL} + \frac{64}{3} L_{iijj}^{V1,LL} \\
& + \frac{16}{9} L_{ii11}^{V1,LR} - \frac{32}{9} L_{ii22}^{V1,LR} + \frac{172}{729} L_{11jj}^{V8,LL} + \frac{172}{729} L_{22jj}^{V8,LL} + \frac{388}{729} L_{ii11}^{V8,LL} + \frac{388}{729} L_{ii22}^{V8,LL} \\
& - \frac{8}{27} L_{iijj}^{V8,LL} - \frac{332}{729} L_{ii11}^{V8,LR} + \frac{2044}{729} L_{ii22}^{V8,LR} - \frac{32}{9} L_{iii}^{V1,LR} - \frac{32}{9} L_{ikk}^{V1,LR} + \frac{2044}{729} L_{iii}^{V8,LR} \\
& \left. + \frac{2044}{729} L_{ikk}^{V8,LR} - \frac{2096}{243} L_{iii}^{V,LL} - \frac{16}{3} L_{ikk}^{V,LL} - \frac{128}{729} L_{ikki}^{V,LL} \right] + \alpha^2 \left[ -\frac{512}{729} L_{jjj}^{V1,LR} \right. \\
& + \frac{40528}{2187} L_{jjj}^{V,LL} - \frac{2992}{729} L_{jj11}^{V,LR} - \frac{2992}{729} L_{jj22}^{V,LR} - \frac{2992}{729} L_{jj33}^{V,LR} - \frac{1216}{729} L_{jj11}^{V1,LR} \\
& - \frac{1216}{729} L_{jj22}^{V1,LR} + \frac{2624}{729} L_{11jj}^{V,LL} + \frac{2624}{729} L_{22jj}^{V,LL} + \frac{2624}{729} L_{33jj}^{V,LL} + \frac{1448}{729} L_{11ii}^{V,LL}
\end{aligned}$$

$$\begin{aligned}
& + \frac{1448}{729} L_{22ii}^{V,LL} + \frac{1448}{729} L_{33ii}^{V,LL} + \frac{6272}{729} L_{11jj}^{V1,LL} + \frac{6272}{729} L_{22jj}^{V1,LL} - \frac{208}{729} L_{ii11}^{V1,LL} \\
& - \frac{208}{729} L_{ii22}^{V1,LL} - \frac{112}{81} L_{iijj}^{V1,LL} - \frac{136}{729} L_{ii11}^{V1,LR} + \frac{2720}{729} L_{ii22}^{V1,LR} + \frac{1664}{729} L_{ii11}^{V,LR} \\
& + \frac{1664}{729} L_{ii22}^{V,LR} + \frac{1664}{729} L_{ii33}^{V,LR} + \frac{2432}{729} L_{iii}^{V1,LR} + \frac{2432}{729} L_{iikk}^{V1,LR} + \frac{11872}{729} L_{iii}^{V,LL} \\
& + \frac{4288}{729} L_{iikk}^{V,LL} + \frac{9088}{2187} L_{iikki}^{V,LL} \Bigg];
\end{aligned}$$

$$\begin{aligned}
\dot{L}_{ijj}^{V8,LL} &= g_s^2 \left[ 12 L_{ijj}^{V1,LL} - 4 L_{ijj}^{V8,LL} + \frac{2}{3} L_{iikk}^{V8,LR} + \frac{8}{3} L_{iikki}^{V,LL} + \frac{2}{3} L_{ii11}^{V8,LL} \right. \\
& + \frac{2}{3} L_{ii22}^{V8,LL} + \frac{2}{3} L_{ii11}^{V8,LR} + \frac{2}{3} L_{ii22}^{V8,LR} + \frac{2}{3} L_{iii}^{V8,LR} + \frac{8}{3} L_{iii}^{V,LL} + \frac{4}{3} L_{jjjj}^{V8,LR} \\
& + \frac{16}{3} L_{jjjj}^{V,LL} + \frac{2}{3} L_{jj11}^{V8,LR} + \frac{2}{3} L_{jj22}^{V8,LR} + \frac{2}{3} L_{11jj}^{V8,LL} + \frac{2}{3} L_{22jj}^{V8,LL} \Bigg] - \frac{8}{3} e^2 L_{ijj}^{V8,LL} \\
& + \alpha_s^2 \left[ \frac{41}{3} L_{ijj}^{V1,LL} - \frac{125}{9} L_{ijj}^{V8,LL} - \frac{22}{3} L_{iikk}^{V1,LR} + \frac{157}{81} L_{iikk}^{V8,LR} - \frac{28}{3} L_{iikk}^{V,LL} \right. \\
& + \frac{5248}{81} L_{iikki}^{V,LL} - \frac{2}{3} L_{ii11}^{V1,LL} - \frac{2}{3} L_{ii22}^{V1,LL} - \frac{22}{3} L_{ii11}^{V1,LR} - \frac{22}{3} L_{ii22}^{V1,LR} + \frac{787}{81} L_{ii11}^{V8,LL} \\
& + \frac{787}{81} L_{ii22}^{V8,LL} + \frac{157}{81} L_{ii11}^{V8,LR} + \frac{157}{81} L_{ii22}^{V8,LR} - \frac{22}{3} L_{iii}^{V1,LR} + \frac{157}{81} L_{iii}^{V8,LR} + \frac{1918}{27} L_{iii}^{V,LL} \\
& - \frac{44}{3} L_{jjjj}^{V1,LR} + \frac{314}{81} L_{jjjj}^{V8,LR} + \frac{10246}{81} L_{jjjj}^{V,LL} - \frac{22}{3} L_{jj11}^{V1,LR} - \frac{22}{3} L_{jj22}^{V1,LR} + \frac{157}{81} L_{jj11}^{V8,LR} \\
& + \frac{157}{81} L_{jj22}^{V8,LR} - \frac{2}{3} L_{11jj}^{V1,LL} - \frac{2}{3} L_{22jj}^{V1,LL} + \frac{787}{81} L_{11jj}^{V8,LL} + \frac{787}{81} L_{22jj}^{V8,LL} \Bigg] \\
& + \alpha_s \alpha \left[ - \frac{4}{3} L_{ijj}^{V1,LL} - \frac{47}{9} L_{ijj}^{V8,LL} - \frac{568}{81} L_{iikk}^{V1,LR} + \frac{4}{27} L_{iikk}^{V8,LR} - \frac{1136}{81} L_{iikk}^{V,LL} \right. \\
& - \frac{6560}{243} L_{iikki}^{V,LL} + \frac{284}{81} L_{11ii}^{V,LL} + \frac{284}{81} L_{22ii}^{V,LL} + \frac{284}{81} L_{33ii}^{V,LL} + \frac{284}{81} L_{ii11}^{V1,LL} + \frac{284}{81} L_{ii22}^{V1,LL} \\
& + \frac{284}{81} L_{ii11}^{V1,LR} - \frac{496}{81} L_{ii22}^{V1,LR} + \frac{14}{9} L_{ii11}^{V8,LL} + \frac{14}{9} L_{ii22}^{V8,LL} + \frac{10}{27} L_{ii11}^{V8,LR} + \frac{4}{27} L_{ii22}^{V8,LR} \\
& + \frac{284}{81} L_{ii11}^{V,LR} + \frac{284}{81} L_{ii22}^{V,LR} + \frac{284}{81} L_{ii33}^{V,LR} - \frac{568}{81} L_{iii}^{V1,LR} + \frac{4}{27} L_{iii}^{V8,LR} - \frac{4616}{81} L_{iii}^{V,LL} \\
& - \frac{392}{81} L_{jjjj}^{V1,LR} + \frac{104}{27} L_{jjjj}^{V8,LR} - \frac{15728}{243} L_{jjjj}^{V,LL} - \frac{196}{81} L_{jj11}^{V,LR} - \frac{196}{81} L_{jj22}^{V,LR} - \frac{196}{81} L_{jj33}^{V,LR}
\end{aligned}$$

$$\begin{aligned}
& + \frac{392}{81} L_{jj11}^{V1,LR} + \frac{392}{81} L_{jj22}^{V1,LR} - \frac{80}{27} L_{jj11}^{V8,LR} - \frac{80}{27} L_{jj22}^{V8,LR} - \frac{196}{81} L_{11jj}^{V,LL} - \frac{196}{81} L_{22jj}^{V,LL} \\
& - \frac{196}{81} L_{33jj}^{V,LL} + \frac{392}{81} L_{11jj}^{V1,LL} + \frac{392}{81} L_{22jj}^{V1,LL} + \frac{56}{9} L_{11jj}^{V8,LL} + \frac{56}{9} L_{22jj}^{V8,LL} \Big] \\
& - \frac{112}{81} \alpha^2 L_{iijj}^{V8,LL} ;
\end{aligned}$$

$$\begin{aligned}
\dot{L}_{ed,jji}^{V,LL} = & e^2 \Big[ \frac{4}{3} L_{dd,iijj}^{V1,LR} + \frac{8}{3} L_{dd,iijj}^{V,LL} + \frac{8}{9} L_{dd,ijji}^{V,LL} + 4 L_{ed,jjii}^{V,LL} + \frac{4}{3} L_{dd,iii}^{V1,LR} \\
& + \frac{32}{9} L_{dd,iii}^{V,LL} + \frac{4}{3} L_{de,ii11}^{V,LR} + \frac{4}{3} L_{de,ii22}^{V,LR} + \frac{4}{3} L_{de,ii33}^{V,LR} - \frac{8}{3} L_{du,ii11}^{V1,LR} - \frac{8}{3} L_{du,ii22}^{V1,LR} \\
& + \frac{4}{3} L_{11ii}^{V,LL} + \frac{4}{3} L_{22ii}^{V,LL} + \frac{4}{3} L_{33ii}^{V,LL} - \frac{8}{3} L_{ud,11ii}^{V1,LL} - \frac{8}{3} L_{ud,22ii}^{V1,LL} + \frac{16}{9} L_{jjkk}^{V,LL} \\
& + \frac{4}{9} L_{jjkk}^{V,LR} + \frac{4}{9} L_{jj11}^{V,LL} + \frac{4}{9} L_{jj22}^{V,LL} + \frac{4}{9} L_{jj11}^{V,LR} + \frac{4}{9} L_{jj22}^{V,LR} + \frac{8}{3} L_{jjjj}^{V,LL} \\
& + \frac{8}{9} L_{jjjj}^{V,LR} - \frac{8}{9} L_{jj11}^{V,LL} - \frac{8}{9} L_{jj22}^{V,LL} - \frac{8}{9} L_{jj11}^{V,LR} - \frac{8}{9} L_{jj22}^{V,LR} \Big] + \alpha_s^2 \Big[ 8 L_{ed,jj11}^{V,LL} \\
& + 8 L_{ed,jj22}^{V,LL} - 8 L_{ed,jj11}^{V,LR} - 8 L_{ed,jj22}^{V,LR} + 8 L_{eu,jj11}^{V,LL} + 8 L_{eu,jj22}^{V,LL} - 8 L_{eu,jj11}^{V,LR} \\
& - 8 L_{eu,jj22}^{V,LR} \Big] + \alpha_s \alpha \Big[ \frac{16}{3} L_{dd,iijj}^{V1,LR} - \frac{1022}{243} L_{dd,iijj}^{V8,LR} + 8 L_{dd,iijj}^{V,LL} + \frac{64}{243} L_{ijji}^{V,LL} \\
& - 16 L_{ed,jji}^{V,LL} + \frac{16}{3} L_{dd,iii}^{V1,LR} - \frac{1022}{243} L_{dd,iii}^{V8,LR} + \frac{1048}{81} L_{dd,iii}^{V,LL} - \frac{32}{3} L_{du,ii11}^{V1,LR} - \frac{32}{3} L_{du,ii22}^{V1,LR} \\
& + \frac{1354}{243} L_{du,ii11}^{V8,LR} + \frac{1354}{243} L_{du,ii22}^{V8,LR} - \frac{32}{3} L_{ud,11ii}^{V1,LL} - \frac{32}{3} L_{ud,22ii}^{V1,LL} - \frac{86}{243} L_{ud,11ii}^{V8,LL} - \frac{86}{243} L_{ud,22ii}^{V8,LL} \\
& + \frac{16}{9} L_{ed,jj11}^{V,LL} + \frac{16}{9} L_{ed,jj22}^{V,LL} + \frac{16}{9} L_{ed,jj11}^{V,LR} + \frac{16}{9} L_{ed,jj22}^{V,LR} - \frac{32}{9} L_{jj11}^{V,LL} - \frac{32}{9} L_{jj22}^{V,LL} \\
& - \frac{32}{9} L_{jj11}^{V,LR} - \frac{32}{9} L_{jj22}^{V,LR} \Big] + \alpha^2 \Big[ - \frac{1312}{243} L_{dd,iijj}^{V1,LR} + \frac{1984}{243} L_{dd,iijj}^{V,LL} + \frac{2896}{729} L_{ijji}^{V,LL} \\
& - \frac{334}{27} L_{ed,jji}^{V,LL} - \frac{1312}{243} L_{dd,iii}^{V1,LR} + \frac{4816}{243} L_{dd,iii}^{V,LL} - \frac{3184}{243} L_{de,ii11}^{V,LR} - \frac{3184}{243} L_{de,ii22}^{V,LR} \\
& - \frac{3184}{243} L_{de,ii33}^{V,LR} - \frac{6232}{243} L_{du,ii11}^{V1,LR} - \frac{6232}{243} L_{du,ii22}^{V1,LR} + \frac{3728}{243} L_{11ii}^{V,LL} + \frac{3728}{243} L_{22ii}^{V,LL} \\
& + \frac{3728}{243} L_{33ii}^{V,LL} + \frac{2984}{243} L_{ud,11ii}^{V1,LL} + \frac{2984}{243} L_{ud,22ii}^{V1,LL} + \frac{224}{81} L_{jjkk}^{V,LL} - \frac{520}{81} L_{jjkk}^{V,LR}
\end{aligned}$$

$$\begin{aligned}
& -\frac{104}{243}L_{jj11}^{V,LL} - \frac{104}{243}L_{jj22}^{V,LL} - \frac{200}{243}L_{jj11}^{V,LR} - \frac{200}{243}L_{jj22}^{V,LR} + \frac{16}{9}L_{jjjj}^{V,LL} - \frac{1040}{81}L_{jjjj}^{V,LR} \\
& - \frac{1016}{243}L_{jj11}^{V,LL} - \frac{1016}{243}L_{jj22}^{V,LL} - \frac{1400}{243}L_{jj11}^{V,LR} - \frac{1400}{243}L_{jj22}^{V,LR} \Big] ; \\
\dot{L}_{jj\dot{u}}^{V,LL} = & e^2 \Bigg[ -8L_{jj\dot{u}}^{V,LL} - \frac{8}{3}L_{i\dot{u}kk}^{V1,LR} - \frac{16}{3}L_{i\dot{u}kk}^{V,LL} - \frac{16}{9}L_{i\dot{u}kk}^{V,LL} + \frac{4}{3}L_{11\dot{u}}^{V,LL} \\
& + \frac{4}{3}L_{22\dot{u}}^{V,LL} + \frac{4}{3}L_{33\dot{u}}^{V,LL} + \frac{4}{3}L_{i\dot{u}11}^{V1,LL} + \frac{4}{3}L_{i\dot{u}22}^{V1,LL} + \frac{4}{3}L_{i\dot{u}11}^{V1,LR} + \frac{4}{3}L_{i\dot{u}22}^{V1,LR} \\
& + \frac{4}{3}L_{i\dot{u}11}^{V,LR} + \frac{4}{3}L_{i\dot{u}22}^{V,LR} + \frac{4}{3}L_{i\dot{u}33}^{V,LR} - \frac{8}{3}L_{i\dot{u}iii}^{V1,LR} - \frac{64}{9}L_{i\dot{u}iii}^{V,LL} - \frac{32}{9}L_{jjkk}^{V,LL} \\
& - \frac{8}{9}L_{jjkk}^{V,LR} - \frac{8}{9}L_{jj11}^{V,LL} - \frac{8}{9}L_{jj22}^{V,LL} - \frac{8}{9}L_{jj11}^{V,LR} - \frac{8}{9}L_{jj22}^{V,LR} - \frac{16}{3}L_{jjjj}^{V,LL} \\
& - \frac{16}{9}L_{jjjj}^{V,LR} + \frac{16}{9}L_{jj11}^{V,LL} + \frac{16}{9}L_{jj22}^{V,LL} + \frac{16}{9}L_{jj11}^{V,LR} + \frac{16}{9}L_{jj22}^{V,LR} \Big] + \alpha_s^2 \Bigg[ 8L_{jj11}^{V,LL} \\
& + 8L_{jj22}^{V,LL} - 8L_{jj11}^{V,LR} - 8L_{jj22}^{V,LR} + 8L_{jj11}^{V,LL} + 8L_{jj22}^{V,LL} - 8L_{jj11}^{V,LR} \\
& - 8L_{jj22}^{V,LR} \Big] + \alpha_s \alpha \Bigg[ 32L_{jj\dot{u}}^{V,LL} - \frac{32}{3}L_{i\dot{u}kk}^{V1,LR} + \frac{2044}{243}L_{i\dot{u}kk}^{V8,LR} - 16L_{i\dot{u}kk}^{V,LL} \\
& - \frac{128}{243}L_{i\dot{u}kk}^{V,LL} + \frac{16}{3}L_{i\dot{u}11}^{V1,LL} + \frac{16}{3}L_{i\dot{u}22}^{V1,LL} + \frac{16}{3}L_{i\dot{u}11}^{V1,LR} - \frac{32}{3}L_{i\dot{u}22}^{V1,LR} + \frac{388}{243}L_{i\dot{u}11}^{V8,LL} \\
& + \frac{388}{243}L_{i\dot{u}22}^{V8,LL} - \frac{332}{243}L_{i\dot{u}11}^{V8,LR} + \frac{2044}{243}L_{i\dot{u}22}^{V8,LR} - \frac{32}{3}L_{i\dot{u}iii}^{V1,LR} + \frac{2044}{243}L_{i\dot{u}iii}^{V8,LR} \\
& - \frac{2096}{81}L_{i\dot{u}iii}^{V,LL} - \frac{32}{9}L_{jj11}^{V,LL} - \frac{32}{9}L_{jj22}^{V,LL} - \frac{32}{9}L_{jj11}^{V,LR} - \frac{32}{9}L_{jj22}^{V,LR} + \frac{64}{9}L_{jj11}^{V,LL} \\
& + \frac{64}{9}L_{jj22}^{V,LL} + \frac{64}{9}L_{jj11}^{V,LR} + \frac{64}{9}L_{jj22}^{V,LR} \Big] + \alpha^2 \Bigg[ \frac{128}{27}L_{jj\dot{u}}^{V,LL} + \frac{128}{243}L_{i\dot{u}kk}^{V1,LR} \\
& + \frac{10048}{243}L_{i\dot{u}kk}^{V,LL} + \frac{18304}{729}L_{i\dot{u}kk}^{V,LL} + \frac{3248}{243}L_{11\dot{u}}^{V,LL} + \frac{3248}{243}L_{22\dot{u}}^{V,LL} + \frac{3248}{243}L_{33\dot{u}}^{V,LL} \\
& + \frac{296}{243}L_{i\dot{u}11}^{V1,LL} + \frac{296}{243}L_{i\dot{u}22}^{V1,LL} - \frac{928}{243}L_{i\dot{u}11}^{V1,LR} + \frac{416}{243}L_{i\dot{u}22}^{V1,LR} - \frac{424}{243}L_{i\dot{u}11}^{V,LR} \\
& - \frac{424}{243}L_{i\dot{u}22}^{V,LR} - \frac{424}{243}L_{i\dot{u}33}^{V,LR} + \frac{128}{243}L_{i\dot{u}iii}^{V1,LR} + \frac{26272}{243}L_{i\dot{u}iii}^{V,LL} + \frac{2432}{81}L_{jjkk}^{V,LL} \\
& + \frac{464}{81}L_{jjkk}^{V,LR} + \frac{2512}{243}L_{jj11}^{V,LL} + \frac{2512}{243}L_{jj22}^{V,LL} + \frac{1408}{243}L_{jj11}^{V,LR} + \frac{1408}{243}L_{jj22}^{V,LR}
\end{aligned}$$

$$\begin{aligned}
& + \frac{544}{9} L_{jjj}^{V,LL} + \frac{928}{81} L_{jjj}^{V,LR} + \frac{1312}{243} L_{jj11}^{V,LL} + \frac{1312}{243} L_{jj22}^{V,LL} - \frac{3104}{243} L_{jj11}^{V,LR} - \frac{3104}{243} L_{jj22}^{V,LR} \Big] ; \\
\dot{L}_{jj\ddot{i}}^{V,LL} &= e^2 \left[ \frac{4}{3} L_{jj11}^{V,LL} + \frac{4}{3} L_{jj22}^{V,LL} + \frac{4}{3} L_{jj11}^{V,LR} + \frac{4}{3} L_{jj22}^{V,LR} + \frac{4}{3} L_{jj11}^{V,LL} \right. \\
& + \frac{4}{3} L_{jj22}^{V,LL} + \frac{4}{3} L_{jj33}^{V,LL} + \frac{4}{3} L_{jj11}^{V,LR} + \frac{4}{3} L_{jj22}^{V,LR} + \frac{4}{3} L_{jj33}^{V,LR} - \frac{8}{3} L_{jj11}^{V,LL} \\
& - \frac{8}{3} L_{jj22}^{V,LL} - \frac{8}{3} L_{jj11}^{V,LR} - \frac{8}{3} L_{jj22}^{V,LR} \Big] + \alpha_s \alpha \left[ \frac{16}{3} L_{jj11}^{V,LL} + \frac{16}{3} L_{jj22}^{V,LL} \right. \\
& + \frac{16}{3} L_{jj11}^{V,LR} + \frac{16}{3} L_{jj22}^{V,LR} - \frac{32}{3} L_{jj11}^{V,LL} - \frac{32}{3} L_{jj22}^{V,LL} - \frac{32}{3} L_{jj11}^{V,LR} - \frac{32}{3} L_{jj22}^{V,LR} \Big] \\
& + \alpha^2 \left[ \frac{40}{9} L_{jj11}^{V,LL} + \frac{40}{9} L_{jj22}^{V,LL} - \frac{32}{9} L_{jj11}^{V,LR} - \frac{32}{9} L_{jj22}^{V,LR} + 16 L_{jj11}^{V,LL} \right. \\
& + 16 L_{jj22}^{V,LL} + 16 L_{jj33}^{V,LL} - 8 L_{jj11}^{V,LR} - 8 L_{jj22}^{V,LR} - 8 L_{jj33}^{V,LR} + \frac{112}{9} L_{jj11}^{V,LL} \\
& + \frac{112}{9} L_{jj22}^{V,LL} - \frac{176}{9} L_{jj11}^{V,LR} - \frac{176}{9} L_{jj22}^{V,LR} \Big] ; \\
\dot{L}_{jj\ddot{i}}^{V,LL} &= e^2 \left[ \frac{4}{9} L_{jj11}^{V,LL} + \frac{4}{9} L_{jj22}^{V,LL} + \frac{4}{9} L_{jj11}^{V,LR} + \frac{4}{9} L_{jj22}^{V,LR} + \frac{4}{9} L_{jj11}^{V,LL} \right. \\
& + \frac{4}{9} L_{jj22}^{V,LL} + \frac{4}{9} L_{jj33}^{V,LL} + \frac{4}{9} L_{jj11}^{V,LR} + \frac{4}{9} L_{jj22}^{V,LR} + \frac{4}{9} L_{jj33}^{V,LR} - \frac{8}{9} L_{jj11}^{V,LL} \\
& - \frac{8}{9} L_{jj22}^{V,LL} - \frac{8}{9} L_{jj11}^{V,LR} - \frac{8}{9} L_{jj22}^{V,LR} \Big] + \alpha_s^2 \left[ 8 L_{jj11}^{V,LL} + 8 L_{jj22}^{V,LL} \right. \\
& - 8 L_{jj11}^{V,LR} - 8 L_{jj22}^{V,LR} + 8 L_{jj11}^{V,LL} + 8 L_{jj22}^{V,LL} - 8 L_{jj11}^{V,LR} - 8 L_{jj22}^{V,LR} \Big] \\
& + \alpha_s \alpha \left[ \frac{16}{9} L_{jj11}^{V,LL} + \frac{16}{9} L_{jj22}^{V,LL} + \frac{16}{9} L_{jj11}^{V,LR} + \frac{16}{9} L_{jj22}^{V,LR} - \frac{32}{9} L_{jj11}^{V,LL} \right. \\
& - \frac{32}{9} L_{jj22}^{V,LL} - \frac{32}{9} L_{jj11}^{V,LR} - \frac{32}{9} L_{jj22}^{V,LR} \Big] + \alpha^2 \left[ \frac{16}{27} L_{jj11}^{V,LL} + \frac{16}{27} L_{jj22}^{V,LL} \right. \\
& - \frac{8}{27} L_{jj11}^{V,LR} - \frac{8}{27} L_{jj22}^{V,LR} + \frac{8}{3} L_{jj11}^{V,LL} + \frac{8}{3} L_{jj22}^{V,LL} + \frac{8}{3} L_{jj33}^{V,LL} + \frac{16}{27} L_{jj11}^{V,LL}
\end{aligned}$$

$$\begin{aligned}
& + \frac{16}{27} L_{jj22}^{V,LL} - \frac{80}{27} L_{jj11}^{V,LR} - \frac{80}{27} L_{jj22}^{V,LR} \Big] ; \\
\dot{L}_{jj\ddot{u}}^{V,LL} = & e^2 \left[ -\frac{8}{9} L_{jj11}^{V,LL} - \frac{8}{9} L_{jj22}^{V,LL} - \frac{8}{9} L_{jj11}^{V,LR} - \frac{8}{9} L_{jj22}^{V,LR} - \frac{8}{9} L_{jj11}^{V,LL} \right. \\
& - \frac{8}{9} L_{jj22}^{V,LL} - \frac{8}{9} L_{jj33}^{V,LL} - \frac{8}{9} L_{jj11}^{V,LR} - \frac{8}{9} L_{jj22}^{V,LR} - \frac{8}{9} L_{jj33}^{V,LR} + \frac{16}{9} L_{jj11}^{V,LL} \\
& + \frac{16}{9} L_{jj22}^{V,LL} + \frac{16}{9} L_{jj11}^{V,LR} + \frac{16}{9} L_{jj22}^{V,LR} \Big] + \alpha_s^2 \left[ 8 L_{jj11}^{V,LL} + 8 L_{jj22}^{V,LL} \right. \\
& - 8 L_{jj11}^{V,LR} - 8 L_{jj22}^{V,LR} + 8 L_{jj11}^{V,LL} + 8 L_{jj22}^{V,LL} - 8 L_{jj11}^{V,LR} - 8 L_{jj22}^{V,LR} \Big] \\
& + \alpha_s \alpha \left[ -\frac{32}{9} L_{jj11}^{V,LL} - \frac{32}{9} L_{jj22}^{V,LL} - \frac{32}{9} L_{jj11}^{V,LR} - \frac{32}{9} L_{jj22}^{V,LR} + \frac{64}{9} L_{jj11}^{V,LL} \right. \\
& + \frac{64}{9} L_{jj22}^{V,LL} + \frac{64}{9} L_{jj11}^{V,LR} + \frac{64}{9} L_{jj22}^{V,LR} \Big] + \alpha^2 \left[ \frac{40}{27} L_{jj11}^{V,LL} + \frac{40}{27} L_{jj22}^{V,LL} \right. \\
& - \frac{56}{27} L_{jj11}^{V,LR} - \frac{56}{27} L_{jj22}^{V,LR} + \frac{8}{3} L_{jj11}^{V,LL} + \frac{8}{3} L_{jj22}^{V,LL} + \frac{8}{3} L_{jj33}^{V,LL} - 8 L_{jj11}^{V,LR} \\
& - 8 L_{jj22}^{V,LR} - 8 L_{jj33}^{V,LR} + \frac{256}{27} L_{jj11}^{V,LL} + \frac{256}{27} L_{jj22}^{V,LL} - \frac{128}{27} L_{jj11}^{V,LR} \\
& \left. - \frac{128}{27} L_{jj22}^{V,LR} \right] ;
\end{aligned}$$

$$\begin{aligned}
\dot{L}_{jj\ddot{u}}^{V1,LL} = & \frac{8}{3} L_{jj\ddot{u}}^{V8,LL} g_s^2 + e^2 \left[ -\frac{8}{9} L_{\ddot{u}\ddot{u}}^{V1,LR} - \frac{8}{9} L_{\ddot{u}\ddot{u}}^{V1,LR} - \frac{64}{27} L_{\ddot{u}\ddot{u}}^{V,LL} - \frac{16}{9} L_{\ddot{u}\ddot{u}}^{V,LL} \right. \\
& - \frac{16}{27} L_{\ddot{u}\ddot{u}}^{V,LL} - \frac{8}{9} L_{\ddot{u}\ddot{u}}^{V,LR} - \frac{8}{9} L_{\ddot{u}\ddot{u}}^{V,LR} - \frac{8}{9} L_{\ddot{u}\ddot{u}}^{V,LR} + \frac{16}{9} L_{\ddot{u}\ddot{u}}^{V1,LR} + \frac{16}{9} L_{\ddot{u}\ddot{u}}^{V1,LR} \\
& - \frac{8}{9} L_{\ddot{u}\ddot{u}}^{V,LL} - \frac{8}{9} L_{\ddot{u}\ddot{u}}^{V,LL} - \frac{8}{9} L_{\ddot{u}\ddot{u}}^{V,LL} + \frac{4}{9} L_{\ddot{u}\ddot{u}}^{V,LL} + \frac{4}{9} L_{\ddot{u}\ddot{u}}^{V,LL} + \frac{4}{9} L_{\ddot{u}\ddot{u}}^{V,LL} \\
& + \frac{16}{9} L_{\ddot{u}\ddot{u}}^{V1,LL} + \frac{16}{9} L_{\ddot{u}\ddot{u}}^{V1,LL} + \frac{4}{9} L_{\ddot{u}\ddot{u}}^{V1,LL} + \frac{4}{9} L_{\ddot{u}\ddot{u}}^{V1,LL} - \frac{8}{3} L_{\ddot{u}\ddot{u}}^{V1,LL} + \frac{4}{9} L_{\ddot{u}\ddot{u}}^{V1,LR} \\
& + \frac{4}{9} L_{\ddot{u}\ddot{u}}^{V1,LR} + \frac{4}{9} L_{\ddot{u}\ddot{u}}^{V,LR} + \frac{4}{9} L_{\ddot{u}\ddot{u}}^{V,LR} + \frac{4}{9} L_{\ddot{u}\ddot{u}}^{V,LR} - \frac{8}{9} L_{\ddot{u}\ddot{u}}^{V1,LR} - \frac{8}{9} L_{\ddot{u}\ddot{u}}^{V1,LR} \\
& \left. - \frac{64}{27} L_{\ddot{u}\ddot{u}}^{V,LL} - \frac{16}{9} L_{\ddot{u}\ddot{u}}^{V,LL} - \frac{16}{27} L_{\ddot{u}\ddot{u}}^{V,LL} \right] + \alpha_s^2 \left[ -8 L_{\ddot{u}\ddot{u}}^{V1,LR} - 8 L_{\ddot{u}\ddot{u}}^{V1,LR} \right.
\end{aligned}$$

$$\begin{aligned}
& + \frac{4}{27} L_{\ddot{iii}}^{V8,LR} + \frac{4}{27} L_{\ddot{ijj}}^{V8,LR} + \frac{328}{9} L_{\ddot{iii}}^{V,LL} + 16 L_{\ddot{ijj}}^{V,LL} + \frac{256}{27} L_{\ddot{ijji}}^{V,LL} - 8 L_{\ddot{ii1}}^{V1,LR} \\
& - 8 L_{\ddot{ii22}}^{V1,LR} + \frac{4}{27} L_{\ddot{ii11}}^{V8,LR} + \frac{4}{27} L_{\ddot{ii22}}^{V8,LR} + 8 L_{\ddot{11ii}}^{V1,LL} + 8 L_{\ddot{22ii}}^{V1,LL} + 8 L_{\ddot{jj11}}^{V1,LL} \\
& + 8 L_{\ddot{jj22}}^{V1,LL} - \frac{28}{3} L_{\ddot{jjii}}^{V1,LL} - 8 L_{\ddot{jj11}}^{V1,LR} - 8 L_{\ddot{jj22}}^{V1,LR} + \frac{4}{27} L_{\ddot{11ii}}^{V8,LL} + \frac{4}{27} L_{\ddot{22ii}}^{V8,LL} \\
& + \frac{4}{27} L_{\ddot{jj11}}^{V8,LL} + \frac{4}{27} L_{\ddot{jj22}}^{V8,LL} + \frac{82}{27} L_{\ddot{jjii}}^{V8,LL} + \frac{4}{27} L_{\ddot{jj11}}^{V8,LR} + \frac{4}{27} L_{\ddot{jj22}}^{V8,LR} - 8 L_{\ddot{jjj}}^{V1,LR} \\
& - 8 L_{\ddot{jjkk}}^{V1,LR} + \frac{4}{27} L_{\ddot{jjjj}}^{V8,LR} + \frac{4}{27} L_{\ddot{jjkk}}^{V8,LR} + \frac{328}{9} L_{\ddot{jjjj}}^{V,LL} + 16 L_{\ddot{jjkk}}^{V,LL} + \frac{256}{27} L_{\ddot{jjkj}}^{V,LL} \Big] \\
& + \alpha_s \alpha \left[ - \frac{32}{9} L_{\ddot{iii}}^{V1,LR} - \frac{32}{9} L_{\ddot{ijj}}^{V1,LR} + \frac{2044}{729} L_{\ddot{iii}}^{V8,LR} + \frac{2044}{729} L_{\ddot{ijj}}^{V8,LR} - \frac{2096}{243} L_{\ddot{iii}}^{V,LL} \right. \\
& - \frac{16}{3} L_{\ddot{ijj}}^{V,LL} - \frac{128}{729} L_{\ddot{ijji}}^{V,LL} + \frac{64}{9} L_{\ddot{ii1}}^{V1,LR} + \frac{64}{9} L_{\ddot{ii22}}^{V1,LR} - \frac{2708}{729} L_{\ddot{ii11}}^{V8,LR} - \frac{2708}{729} L_{\ddot{ii22}}^{V8,LR} \\
& + \frac{64}{9} L_{\ddot{11ii}}^{V1,LL} + \frac{64}{9} L_{\ddot{22ii}}^{V1,LL} + \frac{16}{9} L_{\ddot{jj11}}^{V1,LL} + \frac{16}{9} L_{\ddot{jj22}}^{V1,LL} + \frac{64}{3} L_{\ddot{jjii}}^{V1,LL} + \frac{16}{9} L_{\ddot{jj11}}^{V1,LR} \\
& - \frac{32}{9} L_{\ddot{jj22}}^{V1,LR} + \frac{172}{729} L_{\ddot{11ii}}^{V8,LL} + \frac{172}{729} L_{\ddot{22ii}}^{V8,LL} + \frac{388}{729} L_{\ddot{jj11}}^{V8,LL} + \frac{388}{729} L_{\ddot{jj22}}^{V8,LL} \\
& - \frac{8}{27} L_{\ddot{jjii}}^{V8,LL} - \frac{332}{729} L_{\ddot{jj11}}^{V8,LR} + \frac{2044}{729} L_{\ddot{jj22}}^{V8,LR} - \frac{32}{9} L_{\ddot{jjj}}^{V1,LR} - \frac{32}{9} L_{\ddot{jjkk}}^{V1,LR} + \frac{2044}{729} L_{\ddot{jjjj}}^{V8,LR} \\
& + \frac{2044}{729} L_{\ddot{jjkk}}^{V8,LR} - \frac{2096}{243} L_{\ddot{jjjj}}^{V,LL} - \frac{16}{3} L_{\ddot{jjkk}}^{V,LL} - \frac{128}{729} L_{\ddot{jjkj}}^{V,LL} \Big] + \alpha^2 \left[ - \frac{256}{729} L_{\ddot{iii}}^{V1,LR} \right. \\
& - \frac{256}{729} L_{\ddot{ijj}}^{V1,LR} + \frac{8368}{729} L_{\ddot{iii}}^{V,LL} + \frac{3232}{729} L_{\ddot{ijj}}^{V,LL} + \frac{5728}{2187} L_{\ddot{ijji}}^{V,LL} - \frac{2992}{729} L_{\ddot{ii1}}^{V,LR} \\
& - \frac{2992}{729} L_{\ddot{ii22}}^{V,LR} - \frac{2992}{729} L_{\ddot{ii33}}^{V,LR} - \frac{1216}{729} L_{\ddot{ii11}}^{V1,LR} - \frac{1216}{729} L_{\ddot{ii22}}^{V1,LR} + \frac{2624}{729} L_{\ddot{11ii}}^{V,LL} \\
& + \frac{2624}{729} L_{\ddot{22ii}}^{V,LL} + \frac{2624}{729} L_{\ddot{33ii}}^{V,LL} + \frac{1448}{729} L_{\ddot{11jj}}^{V,LL} + \frac{1448}{729} L_{\ddot{22jj}}^{V,LL} + \frac{1448}{729} L_{\ddot{33jj}}^{V,LL} \\
& + \frac{6272}{729} L_{\ddot{11ii}}^{V1,LL} + \frac{6272}{729} L_{\ddot{22ii}}^{V1,LL} - \frac{208}{729} L_{\ddot{jj11}}^{V1,LL} - \frac{208}{729} L_{\ddot{jj22}}^{V1,LL} - \frac{112}{81} L_{\ddot{jjii}}^{V1,LL} \\
& - \frac{136}{729} L_{\ddot{jj11}}^{V1,LR} + \frac{2720}{729} L_{\ddot{jj22}}^{V1,LR} + \frac{1664}{729} L_{\ddot{jj11}}^{V,LR} + \frac{1664}{729} L_{\ddot{jj22}}^{V,LR} + \frac{1664}{729} L_{\ddot{jj33}}^{V,LR} \\
& + \frac{2432}{729} L_{\ddot{jjjj}}^{V1,LR} + \frac{2432}{729} L_{\ddot{jjkk}}^{V1,LR} + \frac{11872}{729} L_{\ddot{jjjj}}^{V,LL} + \frac{4288}{729} L_{\ddot{jjkk}}^{V,LL} + \frac{9088}{2187} L_{\ddot{jjkj}}^{V,LL} \Big] ;
\end{aligned}$$

$$\begin{aligned}
\dot{L}_{ud,jj\ddot{i}}^{V8,LL} = & g_s^2 \left[ \frac{2}{3} L_{\ddot{i}\ddot{i}\ddot{i}}^{V8,LR} + \frac{2}{3} L_{\ddot{i}j\ddot{j}}^{V8,LR} + \frac{8}{3} L_{\ddot{i}\ddot{i}\ddot{i}}^{V,LL} + \frac{8}{3} L_{\ddot{i}j\ddot{j}}^{V,LL} + \frac{2}{3} L_{\ddot{i}11}^{V8,LR} \right. \\
& + \frac{2}{3} L_{\ddot{i}22}^{V8,LR} + 12 L_{\ddot{i}j\ddot{i}}^{V1,LL} + \frac{2}{3} L_{\ddot{i}11}^{V8,LL} + \frac{2}{3} L_{\ddot{i}22}^{V8,LL} + \frac{2}{3} L_{\ddot{j}11}^{V8,LL} + \frac{2}{3} L_{\ddot{j}22}^{V8,LL} \\
& - 4 L_{\ddot{j}j\ddot{i}}^{V8,LL} + \frac{2}{3} L_{\ddot{j}j11}^{V8,LR} + \frac{2}{3} L_{\ddot{j}j22}^{V8,LR} + \frac{2}{3} L_{\ddot{j}\ddot{j}\ddot{j}}^{V8,LR} + \frac{2}{3} L_{\ddot{j}j\ddot{k}\ddot{k}}^{V8,LR} + \frac{8}{3} L_{\ddot{j}\ddot{j}\ddot{j}}^{V,LL} \\
& + \left. \frac{8}{3} L_{\ddot{j}k\ddot{k}j}^{V,LL} \right] - \frac{8}{3} L_{\ddot{j}j\ddot{i}}^{V8,LL} e^2 + \alpha_s^2 \left[ -\frac{22}{3} L_{\ddot{i}\ddot{i}\ddot{i}}^{V1,LR} - \frac{22}{3} L_{\ddot{i}j\ddot{j}}^{V1,LR} + \frac{157}{81} L_{\ddot{i}\ddot{i}\ddot{i}}^{V8,LR} \right. \\
& + \frac{157}{81} L_{\ddot{i}\ddot{j}\ddot{j}}^{V8,LR} + \frac{1918}{27} L_{\ddot{i}\ddot{i}\ddot{i}}^{V,LL} - \frac{28}{3} L_{\ddot{i}j\ddot{j}}^{V,LL} + \frac{5248}{81} L_{\ddot{i}\ddot{j}\ddot{i}}^{V,LL} - \frac{22}{3} L_{\ddot{i}11}^{V1,LR} - \frac{22}{3} L_{\ddot{i}22}^{V1,LR} \\
& + \frac{157}{81} L_{\ddot{i}11}^{V8,LR} + \frac{157}{81} L_{\ddot{i}22}^{V8,LR} - \frac{2}{3} L_{\ddot{i}11}^{V1,LL} - \frac{2}{3} L_{\ddot{i}22}^{V1,LL} - \frac{2}{3} L_{\ddot{j}11}^{V1,LL} - \frac{2}{3} L_{\ddot{j}22}^{V1,LL} \\
& + \frac{41}{3} L_{\ddot{j}j\ddot{i}}^{V1,LL} - \frac{22}{3} L_{\ddot{j}j11}^{V1,LR} - \frac{22}{3} L_{\ddot{j}j22}^{V1,LR} + \frac{787}{81} L_{\ddot{i}11}^{V8,LL} + \frac{787}{81} L_{\ddot{i}22}^{V8,LL} + \frac{787}{81} L_{\ddot{j}j11}^{V8,LL} \\
& + \frac{787}{81} L_{\ddot{j}j22}^{V8,LL} - \frac{125}{9} L_{\ddot{j}j\ddot{i}}^{V8,LL} + \frac{157}{81} L_{\ddot{j}j11}^{V8,LR} + \frac{157}{81} L_{\ddot{j}j22}^{V8,LR} - \frac{22}{3} L_{\ddot{j}\ddot{j}\ddot{j}}^{V1,LR} - \frac{22}{3} L_{\ddot{j}j\ddot{k}\ddot{k}}^{V1,LR} \\
& + \left. \frac{157}{81} L_{\ddot{j}\ddot{j}\ddot{j}}^{V8,LR} + \frac{157}{81} L_{\ddot{j}j\ddot{k}\ddot{k}}^{V8,LR} + \frac{1918}{27} L_{\ddot{j}\ddot{j}\ddot{j}}^{V,LL} - \frac{28}{3} L_{\ddot{j}j\ddot{k}\ddot{k}}^{V,LL} + \frac{5248}{81} L_{\ddot{j}k\ddot{k}j}^{V,LL} \right] \\
& + \alpha_s \alpha \left[ -\frac{196}{81} L_{\ddot{i}\ddot{i}\ddot{i}}^{V1,LR} - \frac{196}{81} L_{\ddot{i}j\ddot{j}}^{V1,LR} + \frac{52}{27} L_{\ddot{i}\ddot{i}\ddot{i}}^{V8,LR} + \frac{52}{27} L_{\ddot{i}j\ddot{j}}^{V8,LR} - \frac{3152}{81} L_{\ddot{i}\ddot{i}\ddot{i}}^{V,LL} \right. \\
& - \frac{392}{81} L_{\ddot{i}j\ddot{j}}^{V,LL} - \frac{5096}{243} L_{\ddot{i}j\ddot{j}}^{V,LL} - \frac{196}{81} L_{\ddot{i}11}^{V,LR} - \frac{196}{81} L_{\ddot{i}22}^{V,LR} - \frac{196}{81} L_{\ddot{i}33}^{V,LR} + \frac{392}{81} L_{\ddot{i}11}^{V1,LR} \\
& + \frac{392}{81} L_{\ddot{i}22}^{V1,LR} - \frac{80}{27} L_{\ddot{i}11}^{V8,LR} - \frac{80}{27} L_{\ddot{i}22}^{V8,LR} - \frac{196}{81} L_{\ddot{i}11}^{V,LL} - \frac{196}{81} L_{\ddot{i}22}^{V,LL} - \frac{196}{81} L_{\ddot{i}33}^{V,LL} \\
& + \frac{284}{81} L_{\ddot{i}11}^{V,LL} + \frac{284}{81} L_{\ddot{i}22}^{V,LL} + \frac{284}{81} L_{\ddot{i}33}^{V,LL} + \frac{392}{81} L_{\ddot{i}11}^{V1,LL} + \frac{392}{81} L_{\ddot{i}22}^{V1,LL} + \frac{284}{81} L_{\ddot{i}j11}^{V1,LL} \\
& + \frac{284}{81} L_{\ddot{j}j22}^{V1,LL} - \frac{4}{3} L_{\ddot{j}j\ddot{i}}^{V1,LL} + \frac{284}{81} L_{\ddot{j}j11}^{V1,LR} - \frac{496}{81} L_{\ddot{j}j22}^{V1,LR} + \frac{56}{9} L_{\ddot{i}11}^{V8,LL} + \frac{56}{9} L_{\ddot{i}22}^{V8,LL} \\
& + \frac{14}{9} L_{\ddot{j}j11}^{V8,LL} + \frac{14}{9} L_{\ddot{j}j22}^{V8,LL} - \frac{47}{9} L_{\ddot{j}j\ddot{i}}^{V8,LL} + \frac{10}{27} L_{\ddot{j}j11}^{V8,LR} + \frac{4}{27} L_{\ddot{j}j22}^{V8,LR} + \frac{284}{81} L_{\ddot{j}j11}^{V,LR} \\
& + \frac{284}{81} L_{\ddot{j}j22}^{V,LR} + \frac{284}{81} L_{\ddot{j}j33}^{V,LR} - \frac{568}{81} L_{\ddot{j}\ddot{j}\ddot{j}}^{V1,LR} - \frac{568}{81} L_{\ddot{j}j\ddot{k}\ddot{k}}^{V1,LR} + \frac{4}{27} L_{\ddot{j}\ddot{j}\ddot{j}}^{V8,LR} + \frac{4}{27} L_{\ddot{j}j\ddot{k}\ddot{k}}^{V8,LR} \\
& - \left. \frac{4616}{81} L_{\ddot{j}\ddot{j}\ddot{j}}^{V,LL} - \frac{1136}{81} L_{\ddot{j}j\ddot{k}\ddot{k}}^{V,LL} - \frac{6560}{243} L_{\ddot{j}k\ddot{k}j}^{V,LL} \right] - \frac{112}{81} L_{\ddot{j}j\ddot{i}}^{V8,LL} \alpha^2 ;
\end{aligned}$$



$$\begin{aligned}
\dot{L}_{dd\dot{u}jj}^{V,LL} = & g_s^2 \left[ -\frac{1}{18} L_{iii}^{V8,LR} - \frac{1}{18} L_{i\dot{u}jj}^{V8,LR} - \frac{1}{9} L_{jjjj}^{V8,LR} - \frac{2}{9} L_{iii}^{V,LL} - 2 L_{i\dot{u}jj}^{V,LL} \right. \\
& + \frac{52}{9} L_{i\dot{u}ji}^{V,LL} - \frac{4}{9} L_{jjj\dot{u}}^{V,LL} - \frac{1}{18} L_{i\dot{u}11}^{V8,LR} - \frac{1}{18} L_{i\dot{u}22}^{V8,LR} - \frac{1}{18} L_{j\dot{u}11}^{V8,LR} - \frac{1}{18} L_{j\dot{u}22}^{V8,LR} \\
& - \frac{1}{18} L_{11ii}^{V8,LL} - \frac{1}{18} L_{11jj}^{V8,LL} - \frac{1}{18} L_{22ii}^{V8,LL} - \left. \frac{1}{18} L_{22jj}^{V8,LL} \right] + e^2 \left[ \frac{2}{9} L_{iii}^{V1,LR} \right. \\
& + \frac{2}{9} L_{i\dot{u}jj}^{V1,LR} + \frac{4}{9} L_{jjj\dot{u}}^{V1,LR} + \frac{16}{27} L_{iii}^{V,LL} + \frac{16}{9} L_{i\dot{u}jj}^{V,LL} + \frac{4}{27} L_{i\dot{u}ji}^{V,LL} + \frac{32}{27} L_{jjj\dot{u}}^{V,LL} \\
& + \frac{2}{9} L_{i\dot{u}11}^{V,LR} + \frac{2}{9} L_{i\dot{u}22}^{V,LR} + \frac{2}{9} L_{i\dot{u}33}^{V,LR} + \frac{2}{9} L_{j\dot{u}11}^{V,LR} + \frac{2}{9} L_{j\dot{u}22}^{V,LR} + \frac{2}{9} L_{j\dot{u}33}^{V,LR} \\
& - \frac{4}{9} L_{i\dot{u}11}^{V1,LR} - \frac{4}{9} L_{i\dot{u}22}^{V1,LR} - \frac{4}{9} L_{j\dot{u}11}^{V1,LR} - \frac{4}{9} L_{j\dot{u}22}^{V1,LR} + \frac{2}{9} L_{11ii}^{V,LL} + \frac{2}{9} L_{11jj}^{V,LL} \\
& + \frac{2}{9} L_{22ii}^{V,LL} + \frac{2}{9} L_{22jj}^{V,LL} + \frac{2}{9} L_{33ii}^{V,LL} + \frac{2}{9} L_{33jj}^{V,LL} - \frac{4}{9} L_{11i\dot{u}}^{V1,LL} - \frac{4}{9} L_{11j\dot{u}}^{V1,LL} \\
& - \frac{4}{9} L_{22i\dot{u}}^{V1,LL} - \frac{4}{9} L_{22j\dot{u}}^{V1,LL} \left. \right] + \alpha_s^2 \left[ -\frac{61}{18} L_{iii}^{V1,LR} - \frac{61}{18} L_{i\dot{u}jj}^{V1,LR} - \frac{61}{9} L_{jjjj}^{V1,LR} \right. \\
& - \frac{85}{972} L_{iii}^{V8,LR} - \frac{85}{972} L_{i\dot{u}jj}^{V8,LR} - \frac{85}{486} L_{jjjj}^{V8,LR} + \frac{1993}{162} L_{iii}^{V,LL} - \frac{17}{6} L_{i\dot{u}jj}^{V,LL} + \frac{3001}{486} L_{i\dot{u}ji}^{V,LL} \\
& + \frac{9925}{486} L_{jjj\dot{u}}^{V,LL} - \frac{61}{18} L_{i\dot{u}11}^{V1,LR} - \frac{61}{18} L_{i\dot{u}22}^{V1,LR} - \frac{61}{18} L_{j\dot{u}11}^{V1,LR} - \frac{61}{18} L_{j\dot{u}22}^{V1,LR} - \frac{85}{972} L_{i\dot{u}11}^{V8,LR} \\
& - \frac{85}{972} L_{i\dot{u}22}^{V8,LR} - \frac{85}{972} L_{j\dot{u}11}^{V8,LR} + \frac{73}{18} L_{11ii}^{V1,LL} + \frac{73}{18} L_{11jj}^{V1,LL} + \frac{73}{18} L_{22ii}^{V1,LL} \\
& + \frac{73}{18} L_{22jj}^{V1,LL} - \frac{715}{972} L_{11ii}^{V8,LL} - \frac{715}{972} L_{11jj}^{V8,LL} - \frac{715}{972} L_{22ii}^{V8,LL} - \frac{715}{972} L_{22jj}^{V8,LL} \left. \right] \\
& + \alpha_s \alpha \left[ \frac{238}{243} L_{iii}^{V1,LR} + \frac{238}{243} L_{i\dot{u}jj}^{V1,LR} + \frac{476}{243} L_{jjjj}^{V1,LR} - \frac{797}{1458} L_{iii}^{V8,LR} - \frac{797}{1458} L_{i\dot{u}jj}^{V8,LR} \right. \\
& - \frac{797}{729} L_{jjjj}^{V8,LR} + \frac{313}{243} L_{iii}^{V,LL} - \frac{1522}{243} L_{i\dot{u}jj}^{V,LL} - \frac{6740}{729} L_{i\dot{u}ji}^{V,LL} + \frac{1621}{729} L_{jjj\dot{u}}^{V,LL} \\
& + \frac{22}{243} L_{i\dot{u}11}^{V,LR} + \frac{22}{243} L_{i\dot{u}22}^{V,LR} + \frac{22}{243} L_{i\dot{u}33}^{V,LR} + \frac{22}{243} L_{j\dot{u}11}^{V,LR} + \frac{22}{243} L_{j\dot{u}22}^{V,LR} + \frac{22}{243} L_{j\dot{u}33}^{V,LR} \\
& - \frac{476}{243} L_{i\dot{u}11}^{V1,LR} - \frac{476}{243} L_{i\dot{u}22}^{V1,LR} - \frac{476}{243} L_{j\dot{u}11}^{V1,LR} - \frac{476}{243} L_{j\dot{u}22}^{V1,LR} + \frac{715}{1458} L_{i\dot{u}11}^{V8,LR} \\
& + \frac{715}{1458} L_{i\dot{u}22}^{V8,LR} + \frac{715}{1458} L_{j\dot{u}11}^{V8,LR} + \frac{715}{1458} L_{j\dot{u}22}^{V8,LR} + \frac{22}{243} L_{11ii}^{V,LL} + \frac{22}{243} L_{11jj}^{V,LL}
\end{aligned}$$

$$\begin{aligned}
& + \frac{22}{243} L_{22ii}^{V,LL} + \frac{22}{243} L_{22jj}^{V,LL} + \frac{22}{243} L_{33ii}^{V,LL} + \frac{22}{243} L_{33jj}^{V,LL} - \frac{476}{243} L_{11ii}^{V1,LL} - \frac{476}{243} L_{11jj}^{V1,LL} \\
& - \frac{476}{243} L_{22ii}^{V1,LL} - \frac{476}{243} L_{22jj}^{V1,LL} + \frac{103}{1458} L_{11ii}^{V8,LL} + \frac{103}{1458} L_{11jj}^{V8,LL} + \frac{103}{1458} L_{22ii}^{V8,LL} \\
& + \frac{103}{1458} L_{22jj}^{V8,LL} \Big] + \alpha^2 \Big[ - \frac{368}{729} L_{iii}^{V1,LR} - \frac{368}{729} L_{iijj}^{V1,LR} - \frac{736}{729} L_{jjjj}^{V1,LR} + \frac{608}{729} L_{iii}^{V,LL} \\
& + \frac{614}{729} L_{iijj}^{V,LL} + \frac{296}{2187} L_{iijj}^{V,LL} + \frac{2936}{2187} L_{jjjj}^{V,LL} - \frac{656}{729} L_{ii11}^{V,LR} - \frac{656}{729} L_{ii22}^{V,LR} \\
& - \frac{656}{729} L_{ii33}^{V,LR} - \frac{656}{729} L_{jj11}^{V,LR} - \frac{656}{729} L_{jj22}^{V,LR} - \frac{656}{729} L_{jj33}^{V,LR} - \frac{1748}{729} L_{ii11}^{V1,LR} \\
& - \frac{1748}{729} L_{ii22}^{V1,LR} - \frac{1748}{729} L_{jj11}^{V1,LR} - \frac{1748}{729} L_{jj22}^{V1,LR} + \frac{856}{729} L_{11ii}^{V,LL} + \frac{856}{729} L_{11jj}^{V,LL} \\
& + \frac{856}{729} L_{22ii}^{V,LL} + \frac{856}{729} L_{22jj}^{V,LL} + \frac{856}{729} L_{33ii}^{V,LL} + \frac{856}{729} L_{33jj}^{V,LL} + \frac{268}{729} L_{11ii}^{V1,LL} \\
& + \frac{268}{729} L_{11jj}^{V1,LL} + \frac{268}{729} L_{22ii}^{V1,LL} + \frac{268}{729} L_{22jj}^{V1,LL} \Big] ;
\end{aligned}$$

$$\begin{aligned}
\dot{L}_{iijj}^{V,LL} & = g_s^2 \Big[ \frac{1}{6} L_{iijj}^{V8,LR} + 6 L_{iijj}^{V,LL} - \frac{4}{3} L_{iijj}^{V,LL} + \frac{1}{6} L_{iii}^{V8,LR} + \frac{2}{3} L_{iii}^{V,LL} \\
& + \frac{1}{6} L_{ii11}^{V8,LR} + \frac{1}{6} L_{ii22}^{V8,LR} + \frac{1}{6} L_{ii11}^{V8,LL} + \frac{1}{6} L_{ii22}^{V8,LL} + \frac{1}{3} L_{jjjj}^{V8,LR} + \frac{4}{3} L_{jjjj}^{V,LL} \\
& + \frac{1}{6} L_{jj11}^{V8,LR} + \frac{1}{6} L_{jj22}^{V8,LR} + \frac{1}{6} L_{jj11}^{V8,LL} + \frac{1}{6} L_{jj22}^{V8,LL} \Big] + \frac{4}{3} e^2 L_{iijj}^{V,LL} + \alpha_s^2 \Big[ - \frac{11}{6} L_{iijj}^{V1,LR} \\
& + \frac{157}{324} L_{iijj}^{V8,LR} + \frac{9}{2} L_{iijj}^{V,LL} + \frac{743}{162} L_{iijj}^{V,LL} - \frac{11}{6} L_{iii}^{V1,LR} + \frac{157}{324} L_{iii}^{V8,LR} + \frac{959}{54} L_{iii}^{V,LL} \\
& - \frac{11}{6} L_{ii11}^{V1,LR} - \frac{11}{6} L_{ii22}^{V1,LR} + \frac{157}{324} L_{ii11}^{V8,LR} + \frac{157}{324} L_{ii22}^{V8,LR} - \frac{1}{6} L_{11ii}^{V1,LL} - \frac{1}{6} L_{22ii}^{V1,LL} \\
& + \frac{787}{324} L_{11ii}^{V8,LL} + \frac{787}{324} L_{22ii}^{V8,LL} - \frac{11}{3} L_{jjjj}^{V1,LR} + \frac{157}{162} L_{jjjj}^{V8,LR} + \frac{5123}{162} L_{jjjj}^{V,LL} \\
& - \frac{11}{6} L_{jj11}^{V1,LR} - \frac{11}{6} L_{jj22}^{V1,LR} + \frac{157}{324} L_{jj11}^{V8,LR} + \frac{157}{324} L_{jj22}^{V8,LR} - \frac{1}{6} L_{11jj}^{V1,LL} - \frac{1}{6} L_{22jj}^{V1,LL} \\
& + \frac{787}{324} L_{11jj}^{V8,LL} + \frac{787}{324} L_{22jj}^{V8,LL} \Big] + \alpha_s \alpha \Big[ - \frac{22}{81} L_{iijj}^{V1,LR} - \frac{25}{54} L_{iijj}^{V8,LR} - \frac{746}{81} L_{iijj}^{V,LL} \\
& - \frac{1436}{243} L_{iijj}^{V,LL} - \frac{22}{81} L_{iii}^{V1,LR} - \frac{25}{54} L_{iii}^{V8,LR} + \frac{211}{81} L_{iii}^{V,LL} - \frac{22}{81} L_{ii11}^{V,LR} - \frac{22}{81} L_{ii22}^{V,LR}
\end{aligned}$$

$$\begin{aligned}
& -\frac{22}{81}L_{i33}^{V,LR} + \frac{44}{81}L_{ii11}^{V1,LR} + \frac{44}{81}L_{ii22}^{V1,LR} + \frac{71}{54}L_{ii11}^{V8,LR} + \frac{71}{54}L_{ii22}^{V8,LR} - \frac{22}{81}L_{11ii}^{V,LL} \\
& -\frac{22}{81}L_{22ii}^{V,LL} - \frac{22}{81}L_{33ii}^{V,LL} + \frac{44}{81}L_{11ii}^{V1,LL} + \frac{44}{81}L_{22ii}^{V1,LL} - \frac{7}{18}L_{11ii}^{V8,LL} - \frac{7}{18}L_{22ii}^{V8,LL} \\
& -\frac{44}{81}L_{jjjj}^{V1,LR} - \frac{25}{27}L_{jjjj}^{V8,LR} + \frac{955}{243}L_{jjjj}^{V,LL} - \frac{22}{81}L_{jj11}^{V,LR} - \frac{22}{81}L_{jj22}^{V,LR} - \frac{22}{81}L_{jj33}^{V,LR} \\
& + \frac{44}{81}L_{jj11}^{V1,LR} + \frac{44}{81}L_{jj22}^{V1,LR} + \frac{71}{54}L_{jj11}^{V8,LR} + \frac{71}{54}L_{jj22}^{V8,LR} - \frac{22}{81}L_{11jj}^{V,LL} - \frac{22}{81}L_{22jj}^{V,LL} \\
& -\frac{22}{81}L_{33jj}^{V,LL} + \frac{44}{81}L_{11jj}^{V1,LL} + \frac{44}{81}L_{22jj}^{V1,LL} - \frac{7}{18}L_{11jj}^{V8,LL} - \frac{7}{18}L_{22jj}^{V8,LL} \Big] + \frac{38}{81}\alpha^2 L_{ijji}^{V,LL} ;
\end{aligned}$$

$$\begin{aligned}
\dot{L}_{iii}^{V,LL} &= g_s^2 \left[ \frac{2}{9}L_{ijj}^{V8,LR} + \frac{8}{9}L_{ijji}^{V,LL} + \frac{2}{9}L_{iii}^{V8,LR} + \frac{44}{9}L_{iii}^{V,LL} + \frac{2}{9}L_{ii11}^{V8,LR} \right. \\
& + \frac{2}{9}L_{ii22}^{V8,LR} + \frac{2}{9}L_{11ii}^{V8,LL} + \frac{2}{9}L_{22ii}^{V8,LL} \Big] + e^2 \left[ \frac{4}{9}L_{ijj}^{V1,LR} + \frac{8}{9}L_{ijj}^{V,LL} \right. \\
& + \frac{8}{27}L_{ijji}^{V,LL} + \frac{4}{9}L_{iii}^{V1,LR} + \frac{68}{27}L_{iii}^{V,LL} + \frac{4}{9}L_{ii11}^{V,LR} + \frac{4}{9}L_{ii22}^{V,LR} + \frac{4}{9}L_{ii33}^{V,LR} \\
& - \frac{8}{9}L_{ii11}^{V1,LR} - \frac{8}{9}L_{ii22}^{V1,LR} + \frac{4}{9}L_{11ii}^{V,LL} + \frac{4}{9}L_{22ii}^{V,LL} + \frac{4}{9}L_{33ii}^{V,LL} - \frac{8}{9}L_{11ii}^{V1,LL} \\
& \left. - \frac{8}{9}L_{22ii}^{V1,LL} \right] + \alpha_s^2 \left[ -\frac{94}{9}L_{ijj}^{V1,LR} + \frac{193}{243}L_{ijj}^{V8,LR} + \frac{116}{9}L_{ijj}^{V,LL} + \frac{7552}{243}L_{ijji}^{V,LL} \right. \\
& - \frac{94}{9}L_{iii}^{V1,LR} + \frac{193}{243}L_{iii}^{V8,LR} + \frac{4483}{81}L_{iii}^{V,LL} - \frac{94}{9}L_{ii11}^{V1,LR} - \frac{94}{9}L_{ii22}^{V1,LR} + \frac{193}{243}L_{ii11}^{V8,LR} \\
& \left. + \frac{193}{243}L_{ii22}^{V8,LR} + \frac{70}{9}L_{11ii}^{V1,LL} + \frac{70}{9}L_{22ii}^{V1,LL} + \frac{823}{243}L_{11ii}^{V8,LL} + \frac{823}{243}L_{22ii}^{V8,LL} \right] \\
& + \alpha_s \alpha \left[ \frac{344}{243}L_{ijj}^{V1,LR} - \frac{1472}{729}L_{ijj}^{V8,LR} + \frac{472}{243}L_{ijj}^{V,LL} + \frac{1880}{729}L_{ijji}^{V,LL} + \frac{344}{243}L_{iii}^{V1,LR} \right. \\
& - \frac{1472}{729}L_{iii}^{V8,LR} - \frac{2104}{243}L_{iii}^{V,LL} - \frac{88}{243}L_{ii11}^{V,LR} - \frac{88}{243}L_{ii22}^{V,LR} - \frac{88}{243}L_{ii33}^{V,LR} - \frac{688}{243}L_{ii11}^{V1,LR} \\
& - \frac{688}{243}L_{ii22}^{V1,LR} + \frac{2632}{729}L_{ii11}^{V8,LR} + \frac{2632}{729}L_{ii22}^{V8,LR} - \frac{88}{243}L_{11ii}^{V,LL} - \frac{88}{243}L_{22ii}^{V,LL} \\
& \left. - \frac{88}{243}L_{33ii}^{V,LL} - \frac{688}{243}L_{11ii}^{V1,LL} - \frac{688}{243}L_{22ii}^{V1,LL} - \frac{464}{729}L_{11ii}^{V8,LL} - \frac{464}{729}L_{22ii}^{V8,LL} \right]
\end{aligned}$$

$$\begin{aligned}
& + \alpha^2 \left[ -\frac{736}{729} L_{ijj}^{V1,LR} + \frac{544}{729} L_{ijj}^{V,LL} + \frac{592}{2187} L_{ijji}^{V,LL} - \frac{736}{729} L_{iii}^{V1,LR} + \frac{1558}{729} L_{iii}^{V,LL} \right. \\
& - \frac{1312}{729} L_{ii11}^{V,LR} - \frac{1312}{729} L_{ii22}^{V,LR} - \frac{1312}{729} L_{ii33}^{V,LR} - \frac{3496}{729} L_{ii11}^{V1,LR} - \frac{3496}{729} L_{ii22}^{V1,LR} \\
& \left. + \frac{1712}{729} L_{11ii}^{V,LL} + \frac{1712}{729} L_{22ii}^{V,LL} + \frac{1712}{729} L_{33ii}^{V,LL} + \frac{536}{729} L_{11ii}^{V1,LL} + \frac{536}{729} L_{22ii}^{V1,LL} \right];
\end{aligned}$$

$$\begin{aligned}
\dot{L}_{ijj}^{V,LL} &= g_s^2 \left[ -\frac{1}{18} L_{ii11}^{V8,LL} - \frac{1}{18} L_{ii22}^{V8,LL} - \frac{1}{18} L_{jj11}^{V8,LL} - \frac{1}{18} L_{jj22}^{V8,LL} - \frac{1}{18} L_{ii11}^{V8,LR} \right. \\
& - \frac{1}{18} L_{ii22}^{V8,LR} - \frac{1}{18} L_{jj11}^{V8,LR} - \frac{1}{18} L_{jj22}^{V8,LR} - \frac{1}{18} L_{iii}^{V8,LR} - \frac{1}{18} L_{ikk}^{V8,LR} - \frac{1}{18} L_{jjj}^{V8,LR} \\
& - \frac{1}{18} L_{jjkk}^{V8,LR} - \frac{2}{9} L_{iii}^{V,LL} - 2L_{ijj}^{V,LL} + 6L_{iji}^{V,LL} - \frac{2}{9} L_{ikk}^{V,LL} - \frac{2}{9} L_{jjj}^{V,LL} \\
& \left. - \frac{2}{9} L_{jjkj}^{V,LL} \right] + e^2 \left[ -\frac{4}{9} L_{11ii}^{V,LL} - \frac{4}{9} L_{11jj}^{V,LL} - \frac{4}{9} L_{22ii}^{V,LL} - \frac{4}{9} L_{22jj}^{V,LL} - \frac{4}{9} L_{33ii}^{V,LL} \right. \\
& - \frac{4}{9} L_{33jj}^{V,LL} - \frac{4}{9} L_{ii11}^{V1,LL} - \frac{4}{9} L_{ii22}^{V1,LL} - \frac{4}{9} L_{jj11}^{V1,LL} - \frac{4}{9} L_{jj22}^{V1,LL} - \frac{4}{9} L_{ii11}^{V1,LR} \\
& - \frac{4}{9} L_{ii22}^{V1,LR} - \frac{4}{9} L_{jj11}^{V1,LR} - \frac{4}{9} L_{jj22}^{V1,LR} - \frac{4}{9} L_{ii11}^{V,LR} - \frac{4}{9} L_{ii22}^{V,LR} - \frac{4}{9} L_{ii33}^{V,LR} \\
& - \frac{4}{9} L_{jj11}^{V,LR} - \frac{4}{9} L_{jj22}^{V,LR} - \frac{4}{9} L_{jj33}^{V,LR} + \frac{8}{9} L_{iii}^{V1,LR} + \frac{8}{9} L_{ikk}^{V1,LR} + \frac{8}{9} L_{jjj}^{V1,LR} \\
& + \frac{8}{9} L_{jjkk}^{V1,LR} + \frac{64}{27} L_{iii}^{V,LL} + \frac{16}{3} L_{ijj}^{V,LL} + \frac{16}{9} L_{iik}^{V,LL} + \frac{16}{27} L_{ikk}^{V,LL} + \frac{64}{27} L_{jjj}^{V,LL} \\
& + \frac{16}{9} L_{jjkk}^{V,LL} + \frac{16}{27} L_{jjkj}^{V,LL} \left. \right] + \alpha_s^2 \left[ \frac{73}{18} L_{ii11}^{V1,LL} + \frac{73}{18} L_{ii22}^{V1,LL} + \frac{73}{18} L_{jj11}^{V1,LL} \right. \\
& + \frac{73}{18} L_{jj22}^{V1,LL} - \frac{61}{18} L_{ii11}^{V1,LR} - \frac{61}{18} L_{ii22}^{V1,LR} - \frac{61}{18} L_{jj11}^{V1,LR} - \frac{61}{18} L_{jj22}^{V1,LR} - \frac{715}{972} L_{ii11}^{V8,LL} \\
& - \frac{715}{972} L_{ii22}^{V8,LL} - \frac{715}{972} L_{jj11}^{V8,LL} - \frac{715}{972} L_{jj22}^{V8,LL} - \frac{85}{972} L_{ii11}^{V8,LR} - \frac{85}{972} L_{ii22}^{V8,LR} \\
& - \frac{85}{972} L_{jj11}^{V8,LR} - \frac{85}{972} L_{jj22}^{V8,LR} - \frac{61}{18} L_{iii}^{V1,LR} - \frac{61}{18} L_{ikk}^{V1,LR} - \frac{61}{18} L_{jjj}^{V1,LR} - \frac{61}{18} L_{jjkk}^{V1,LR} \\
& - \frac{85}{972} L_{iii}^{V8,LR} - \frac{85}{972} L_{ikk}^{V8,LR} - \frac{85}{972} L_{jjj}^{V8,LR} - \frac{85}{972} L_{jjkk}^{V8,LR} + \frac{1993}{162} L_{iii}^{V,LL} \\
& - \frac{209}{18} L_{ijj}^{V,LL} + \frac{79}{9} L_{iik}^{V,LL} + \frac{41}{6} L_{iji}^{V,LL} - \frac{160}{243} L_{ikk}^{V,LL} + \frac{1993}{162} L_{jjj}^{V,LL} + \frac{79}{9} L_{jjkk}^{V,LL}
\end{aligned}$$

$$\begin{aligned}
& -\frac{160}{243}L_{jkkj}^{V,LL} \Big] + \alpha_s \alpha \Bigg[ -\frac{44}{243}L_{11ii}^{V,LL} - \frac{44}{243}L_{11jj}^{V,LL} - \frac{44}{243}L_{22ii}^{V,LL} - \frac{44}{243}L_{22jj}^{V,LL} \\
& -\frac{44}{243}L_{33ii}^{V,LL} - \frac{44}{243}L_{33jj}^{V,LL} - \frac{476}{243}L_{ii11}^{V1,LL} - \frac{476}{243}L_{ii22}^{V1,LL} - \frac{476}{243}L_{jj11}^{V1,LL} \\
& -\frac{476}{243}L_{jj22}^{V1,LL} - \frac{476}{243}L_{ii11}^{V1,LR} + \frac{934}{243}L_{ii22}^{V1,LR} - \frac{476}{243}L_{jj11}^{V1,LR} + \frac{934}{243}L_{jj22}^{V1,LR} \\
& -\frac{533}{1458}L_{ii11}^{V8,LL} - \frac{533}{1458}L_{ii22}^{V8,LL} - \frac{533}{1458}L_{jj11}^{V8,LL} - \frac{533}{1458}L_{jj22}^{V8,LL} + \frac{79}{1458}L_{ii11}^{V8,LR} \\
& -\frac{1594}{729}L_{ii22}^{V8,LR} + \frac{79}{1458}L_{jj11}^{V8,LR} - \frac{1594}{729}L_{jj22}^{V8,LR} - \frac{44}{243}L_{ii11}^{V,LR} - \frac{44}{243}L_{ii22}^{V,LR} \\
& -\frac{44}{243}L_{jj11}^{V,LR} - \frac{44}{243}L_{jj22}^{V,LR} - \frac{44}{243}L_{jj33}^{V,LR} + \frac{952}{243}L_{iii}^{V1,LR} + \frac{952}{243}L_{ikk}^{V1,LR} \\
& + \frac{952}{243}L_{jjj}^{V1,LR} + \frac{952}{243}L_{jjk}^{V1,LR} - \frac{1594}{729}L_{iii}^{V8,LR} - \frac{1594}{729}L_{ikk}^{V8,LR} - \frac{1594}{729}L_{jjj}^{V8,LR} \\
& -\frac{1594}{729}L_{jjk}^{V8,LR} + \frac{1252}{243}L_{iii}^{V,LL} - \frac{280}{9}L_{ijj}^{V,LL} + \frac{1472}{243}L_{ikk}^{V,LL} - \frac{104}{3}L_{ijji}^{V,LL} - \frac{1688}{729}L_{ikki}^{V,LL} \\
& + \frac{1252}{243}L_{jjjj}^{V,LL} + \frac{1472}{243}L_{jjkk}^{V,LL} - \frac{1688}{729}L_{jjkj}^{V,LL} \Big] + \alpha^2 \Bigg[ \frac{1252}{729}L_{11ii}^{V,LL} + \frac{1252}{729}L_{11jj}^{V,LL} \\
& + \frac{1252}{729}L_{22ii}^{V,LL} + \frac{1252}{729}L_{22jj}^{V,LL} + \frac{1252}{729}L_{33ii}^{V,LL} + \frac{1252}{729}L_{33jj}^{V,LL} + \frac{964}{729}L_{ii11}^{V1,LL} \\
& + \frac{964}{729}L_{ii22}^{V1,LL} + \frac{964}{729}L_{jj11}^{V1,LL} + \frac{964}{729}L_{jj22}^{V1,LL} - \frac{1052}{729}L_{ii11}^{V1,LR} - \frac{6176}{729}L_{ii22}^{V1,LR} \\
& -\frac{1052}{729}L_{jj11}^{V1,LR} - \frac{6176}{729}L_{jj22}^{V1,LR} - \frac{4796}{729}L_{ii11}^{V,LR} - \frac{4796}{729}L_{ii22}^{V,LR} - \frac{4796}{729}L_{ii33}^{V,LR} \\
& -\frac{4796}{729}L_{jj11}^{V,LR} - \frac{4796}{729}L_{jj22}^{V,LR} - \frac{4796}{729}L_{jj33}^{V,LR} - \frac{5888}{729}L_{iii}^{V1,LR} - \frac{5888}{729}L_{ikk}^{V1,LR} \\
& -\frac{5888}{729}L_{jjj}^{V1,LR} - \frac{5888}{729}L_{jjk}^{V1,LR} + \frac{9728}{729}L_{iii}^{V,LL} - \frac{1216}{81}L_{ijj}^{V,LL} + \frac{4352}{729}L_{ikk}^{V,LL} \\
& + \frac{4736}{2187}L_{ikki}^{V,LL} + \frac{9728}{729}L_{jjjj}^{V,LL} + \frac{4352}{729}L_{jjkk}^{V,LL} + \frac{4736}{2187}L_{jjkj}^{V,LL} \Big] ;
\end{aligned}$$

$$\begin{aligned}
\dot{L}_{ijji}^{V,LL} &= g_s^2 \Bigg[ \frac{1}{6}L_{ii11}^{V8,LL} + \frac{1}{6}L_{ii22}^{V8,LL} + \frac{1}{6}L_{jj11}^{V8,LL} + \frac{1}{6}L_{jj22}^{V8,LL} + \frac{1}{6}L_{ii11}^{V8,LR} \\
& + \frac{1}{6}L_{ii22}^{V8,LR} + \frac{1}{6}L_{jj11}^{V8,LR} + \frac{1}{6}L_{jj22}^{V8,LR} + \frac{1}{6}L_{ikk}^{V8,LR} + \frac{1}{6}L_{jjj}^{V8,LR}
\end{aligned}$$

$$\begin{aligned}
& + \frac{1}{6} L_{jjkk}^{V8,LR} + \frac{2}{3} L_{iiii}^{V,LL} + 6 L_{iijj}^{V,LL} - 2 L_{ijji}^{V,LL} + \frac{2}{3} L_{ikki}^{V,LL} + \frac{2}{3} L_{jjjj}^{V,LL} \\
& + \frac{2}{3} L_{jjkj}^{V,LL} \Big] + \frac{16}{3} L_{ijji}^{V,LL} e^2 + \alpha_s^2 \Bigg[ - \frac{1}{6} L_{ii11}^{V1,LL} - \frac{1}{6} L_{ii22}^{V1,LL} - \frac{1}{6} L_{jj11}^{V1,LL} \\
& - \frac{1}{6} L_{jj22}^{V1,LL} - \frac{11}{6} L_{ud11}^{V1,LR} - \frac{11}{6} L_{ud22}^{V1,LR} - \frac{11}{6} L_{jj11}^{V1,LR} - \frac{11}{6} L_{jj22}^{V1,LR} + \frac{787}{324} L_{ii11}^{V8,LL} \\
& + \frac{787}{324} L_{ii22}^{V8,LL} + \frac{787}{324} L_{jj11}^{V8,LL} + \frac{787}{324} L_{jj22}^{V8,LL} + \frac{157}{324} L_{ii11}^{V8,LR} + \frac{157}{324} L_{ii22}^{V8,LR} \\
& + \frac{157}{324} L_{jj11}^{V8,LR} + \frac{157}{324} L_{jj22}^{V8,LR} - \frac{11}{6} L_{iii}^{V1,LR} - \frac{11}{6} L_{iik}^{V1,LR} - \frac{11}{6} L_{jjj}^{V1,LR} - \frac{11}{6} L_{jjk}^{V1,LR} \\
& + \frac{157}{324} L_{iii}^{V8,LR} + \frac{157}{324} L_{iik}^{V8,LR} + \frac{157}{324} L_{jjj}^{V8,LR} + \frac{157}{324} L_{jjk}^{V8,LR} + \frac{959}{54} L_{iii}^{V,LL} \\
& + \frac{41}{6} L_{iijj}^{V,LL} - \frac{7}{3} L_{iikk}^{V,LL} - \frac{209}{18} L_{ijji}^{V,LL} + \frac{1312}{81} L_{ikki}^{V,LL} + \frac{959}{54} L_{jjjj}^{V,LL} - \frac{7}{3} L_{jjkk}^{V,LL} \\
& + \frac{1312}{81} L_{jjkj}^{V,LL} \Big] + \alpha_s \alpha \Bigg[ \frac{44}{81} L_{11ii}^{V,LL} + \frac{44}{81} L_{11jj}^{V,LL} + \frac{44}{81} L_{22ii}^{V,LL} + \frac{44}{81} L_{22jj}^{V,LL} \\
& + \frac{44}{81} L_{33ii}^{V,LL} + \frac{44}{81} L_{33jj}^{V,LL} + \frac{44}{81} L_{ii11}^{V1,LL} + \frac{44}{81} L_{ii22}^{V1,LL} + \frac{44}{81} L_{jj11}^{V1,LL} + \frac{44}{81} L_{jj22}^{V1,LL} \\
& + \frac{44}{81} L_{ii11}^{V1,LR} - \frac{70}{81} L_{ii22}^{V1,LR} + \frac{44}{81} L_{jj11}^{V1,LR} - \frac{70}{81} L_{jj22}^{V1,LR} - \frac{1}{2} L_{ii11}^{V8,LL} - \frac{1}{2} L_{ii22}^{V8,LL} \\
& - \frac{1}{2} L_{jj11}^{V8,LL} - \frac{1}{2} L_{jj22}^{V8,LL} + \frac{65}{54} L_{ii11}^{V8,LR} - \frac{50}{27} L_{ii22}^{V8,LR} + \frac{65}{54} L_{jj11}^{V8,LR} - \frac{50}{27} L_{jj22}^{V8,LR} \\
& + \frac{44}{81} L_{ii11}^{V,LR} + \frac{44}{81} L_{ii22}^{V,LR} + \frac{44}{81} L_{ii33}^{V,LR} + \frac{44}{81} L_{jj11}^{V,LR} + \frac{44}{81} L_{jj22}^{V,LR} + \frac{44}{81} L_{jj33}^{V,LR} \\
& - \frac{88}{81} L_{iii}^{V1,LR} - \frac{88}{81} L_{iik}^{V1,LR} - \frac{88}{81} L_{jjj}^{V1,LR} - \frac{88}{81} L_{jjk}^{V1,LR} - \frac{50}{27} L_{iii}^{V8,LR} - \frac{50}{27} L_{iik}^{V8,LR} \\
& - \frac{50}{27} L_{jjj}^{V8,LR} - \frac{50}{27} L_{jjk}^{V8,LR} + \frac{844}{81} L_{iii}^{V,LL} - \frac{104}{3} L_{iijj}^{V,LL} - \frac{176}{81} L_{iikk}^{V,LL} - \frac{280}{9} L_{ijji}^{V,LL} \\
& + \frac{1816}{243} L_{ikki}^{V,LL} + \frac{844}{81} L_{jjjj}^{V,LL} - \frac{176}{81} L_{jjkk}^{V,LL} + \frac{1816}{243} L_{jjkj}^{V,LL} \Big] - \frac{1216}{81} L_{ijji}^{V,LL} \\
& \alpha^2 ;
\end{aligned}$$

$$\dot{L}_{iii}^{V,LL} = g_s^2 \left[ \frac{2}{9} L_{iik}^{V8,LR} + \frac{8}{9} L_{iikk}^{V,LL} + \frac{2}{9} L_{ii11}^{V8,LL} + \frac{2}{9} L_{ii22}^{V8,LL} + \frac{2}{9} L_{ii11}^{V8,LR} \right]$$

$$\begin{aligned}
& + \frac{2}{9} L_{ud\,ii22}^{V8,LR} + \frac{2}{9} L_{uu\,iiii}^{V8,LR} + \frac{44}{9} L_{uu\,iii}^{V,LL} \Big] + e^2 \Big[ \frac{16}{9} L_{uu\,ikk}^{V1,LR} + \frac{32}{9} L_{uu\,ikk}^{V,LL} \\
& + \frac{32}{27} L_{uu\,ikki}^{V,LL} - \frac{8}{9} L_{eu\,11ii}^{V,LL} - \frac{8}{9} L_{eu\,22ii}^{V,LL} - \frac{8}{9} L_{eu\,33ii}^{V,LL} - \frac{8}{9} L_{ud\,ii11}^{V1,LL} - \frac{8}{9} L_{ud\,ii22}^{V1,LL} \\
& - \frac{8}{9} L_{ud\,ii11}^{V1,LR} - \frac{8}{9} L_{ud\,ii22}^{V1,LR} - \frac{8}{9} L_{ue\,ii11}^{V,LR} - \frac{8}{9} L_{ue\,ii22}^{V,LR} - \frac{8}{9} L_{ue\,ii33}^{V,LR} + \frac{16}{9} L_{uu\,iii}^{V1,LR} \\
& + \frac{272}{27} L_{uu\,iii}^{V,LL} \Big] + \alpha_s^2 \Big[ -\frac{94}{9} L_{uu\,ikk}^{V1,LR} + \frac{193}{243} L_{uu\,ikk}^{V8,LR} + \frac{116}{9} L_{uu\,ikk}^{V,LL} + \frac{7552}{243} L_{uu\,ikki}^{V,LL} \\
& + \frac{70}{9} L_{ud\,ii11}^{V1,LL} + \frac{70}{9} L_{ud\,ii22}^{V1,LL} - \frac{94}{9} L_{ud\,ii11}^{V1,LR} - \frac{94}{9} L_{ud\,ii22}^{V1,LR} + \frac{823}{243} L_{ud\,ii11}^{V8,LL} + \frac{823}{243} L_{ud\,ii22}^{V8,LL} \\
& + \frac{193}{243} L_{ud\,ii11}^{V8,LR} + \frac{193}{243} L_{ud\,ii22}^{V8,LR} - \frac{94}{9} L_{uu\,iii}^{V1,LR} + \frac{193}{243} L_{uu\,iii}^{V8,LR} + \frac{4483}{81} L_{uu\,iii}^{V,LL} \Big] \\
& + \alpha_s \alpha \Big[ \frac{1376}{243} L_{uu\,ikk}^{V1,LR} - \frac{5888}{729} L_{uu\,ikk}^{V8,LR} + \frac{1888}{243} L_{uu\,ikk}^{V,LL} + \frac{7520}{729} L_{uu\,ikki}^{V,LL} + \frac{176}{243} L_{eu\,11ii}^{V,LL} \\
& + \frac{176}{243} L_{eu\,22ii}^{V,LL} + \frac{176}{243} L_{eu\,33ii}^{V,LL} - \frac{688}{243} L_{ud\,ii11}^{V1,LL} - \frac{688}{243} L_{ud\,ii22}^{V1,LL} - \frac{688}{243} L_{ud\,ii11}^{V1,LR} \\
& + \frac{1448}{243} L_{ud\,ii22}^{V1,LR} - \frac{1262}{729} L_{ud\,ii11}^{V8,LL} - \frac{1262}{729} L_{ud\,ii22}^{V8,LL} + \frac{1834}{729} L_{ud\,ii11}^{V8,LR} - \frac{5888}{729} L_{ud\,ii22}^{V8,LR} \\
& + \frac{176}{243} L_{ue\,ii11}^{V,LR} + \frac{176}{243} L_{ue\,ii22}^{V,LR} + \frac{176}{243} L_{ue\,ii33}^{V,LR} + \frac{1376}{243} L_{uu\,iii}^{V1,LR} - \frac{5888}{729} L_{uu\,iii}^{V8,LR} \\
& - \frac{8416}{243} L_{uu\,iii}^{V,LL} \Big] + \alpha^2 \Big[ -\frac{11776}{729} L_{uu\,ikk}^{V1,LR} + \frac{8704}{729} L_{uu\,ikk}^{V,LL} + \frac{9472}{2187} L_{uu\,ikki}^{V,LL} + \frac{2504}{729} L_{eu\,11ii}^{V,LL} \\
& + \frac{2504}{729} L_{eu\,22ii}^{V,LL} + \frac{2504}{729} L_{eu\,33ii}^{V,LL} + \frac{1928}{729} L_{ud\,ii11}^{V1,LL} + \frac{1928}{729} L_{ud\,ii22}^{V1,LL} - \frac{2104}{729} L_{ud\,ii11}^{V1,LR} \\
& - \frac{12352}{729} L_{ud\,ii22}^{V1,LR} - \frac{9592}{729} L_{ue\,ii11}^{V,LR} - \frac{9592}{729} L_{ue\,ii22}^{V,LR} - \frac{9592}{729} L_{ue\,ii33}^{V,LR} - \frac{11776}{729} L_{uu\,iii}^{V1,LR} \\
& + \frac{8512}{729} L_{uu\,iii}^{V,LL} \Big] ;
\end{aligned}$$

$$\begin{aligned}
\dot{L}_{ee\,ijj}^{V,LL} &= e^2 \Big[ \frac{40}{3} L_{ee\,ijj}^{V,LL} + \frac{1}{3} L_{ee\,ijj}^{V,LR} + \frac{4}{3} L_{ee\,ikk}^{V,LL} + \frac{1}{3} L_{ee\,ikk}^{V,LR} + \frac{1}{3} L_{ed\,ii11}^{V,LL} \\
& + \frac{1}{3} L_{ed\,ii22}^{V,LL} + \frac{1}{3} L_{ed\,ii11}^{V,LR} + \frac{1}{3} L_{ed\,ii22}^{V,LR} + \frac{4}{3} L_{ee\,iii}^{V,LL} + \frac{1}{3} L_{ee\,iii}^{V,LR} - \frac{2}{3} L_{eu\,ii11}^{V,LL} \\
& - \frac{2}{3} L_{eu\,ii22}^{V,LL} - \frac{2}{3} L_{eu\,ii11}^{V,LR} - \frac{2}{3} L_{eu\,ii22}^{V,LR} + \frac{4}{3} L_{jjkk}^{V,LL} + \frac{1}{3} L_{jjkk}^{V,LR} + \frac{1}{3} L_{ed\,jj11}^{V,LL} \Big]
\end{aligned}$$

$$\begin{aligned}
& + \frac{1}{3}L_{ed,jj22}^{V,LL} + \frac{1}{3}L_{ed,jj11}^{V,LR} + \frac{1}{3}L_{ed,jj22}^{V,LR} + 2L_{ee,jjjj}^{V,LL} + \frac{2}{3}L_{ee,jjjj}^{V,LR} - \frac{2}{3}L_{eu,jj11}^{V,LL} \\
& - \frac{2}{3}L_{eu,jj22}^{V,LL} - \frac{2}{3}L_{eu,jj11}^{V,LR} - \frac{2}{3}L_{eu,jj22}^{V,LR} \Big] + \alpha_s \alpha \Big[ \frac{4}{3}L_{ed,ii11}^{V,LL} + \frac{4}{3}L_{ed,ii22}^{V,LL} \\
& + \frac{4}{3}L_{ed,ii11}^{V,LR} + \frac{4}{3}L_{ed,ii22}^{V,LR} - \frac{8}{3}L_{eu,ii11}^{V,LL} - \frac{8}{3}L_{eu,ii22}^{V,LL} - \frac{8}{3}L_{eu,ii11}^{V,LR} - \frac{8}{3}L_{eu,ii22}^{V,LR} \\
& + \frac{4}{3}L_{ed,jj11}^{V,LL} + \frac{4}{3}L_{ed,jj22}^{V,LL} + \frac{4}{3}L_{ed,jj11}^{V,LR} + \frac{4}{3}L_{ed,jj22}^{V,LR} - \frac{8}{3}L_{eu,jj11}^{V,LL} - \frac{8}{3}L_{eu,jj22}^{V,LL} \\
& - \frac{8}{3}L_{eu,jj11}^{V,LR} - \frac{8}{3}L_{eu,jj22}^{V,LR} \Big] + \alpha^2 \Big[ -\frac{2326}{27}L_{ee,ijj}^{V,LL} - \frac{178}{27}L_{ee,ijj}^{V,LR} + \frac{296}{27}L_{ee,iikk}^{V,LL} \\
& - \frac{178}{27}L_{ee,iikk}^{V,LR} + \frac{166}{81}L_{ed,ii11}^{V,LL} + \frac{166}{81}L_{ed,ii22}^{V,LL} + \frac{34}{81}L_{ed,ii11}^{V,LR} + \frac{34}{81}L_{ed,ii22}^{V,LR} + \frac{320}{27}L_{ee,iii}^{V,LL} \\
& - \frac{178}{27}L_{ee,iii}^{V,LR} - \frac{314}{81}L_{eu,ii11}^{V,LL} - \frac{314}{81}L_{eu,ii22}^{V,LL} - \frac{842}{81}L_{eu,ii11}^{V,LR} - \frac{842}{81}L_{eu,ii22}^{V,LR} + \frac{296}{27}L_{ee,jjkk}^{V,LL} \\
& - \frac{178}{27}L_{ee,jjkk}^{V,LR} + \frac{166}{81}L_{ed,jj11}^{V,LL} + \frac{166}{81}L_{ed,jj22}^{V,LL} + \frac{34}{81}L_{ed,jj11}^{V,LR} + \frac{34}{81}L_{ed,jj22}^{V,LR} + \frac{52}{3}L_{ee,jjjj}^{V,LL} \\
& - \frac{356}{27}L_{ee,jjjj}^{V,LR} - \frac{314}{81}L_{eu,jj11}^{V,LL} - \frac{314}{81}L_{eu,jj22}^{V,LL} - \frac{842}{81}L_{eu,jj11}^{V,LR} - \frac{842}{81}L_{eu,jj22}^{V,LR} \Big] ;
\end{aligned}$$

$$\begin{aligned}
\dot{L}_{ee,iii}^{V,LL} & = e^2 \Big[ \frac{16}{3}L_{ee,ijj}^{V,LL} + \frac{4}{3}L_{ee,ijj}^{V,LR} + \frac{16}{3}L_{ee,iikk}^{V,LL} + \frac{4}{3}L_{ee,iikk}^{V,LR} + \frac{4}{3}L_{ed,ii11}^{V,LL} \\
& + \frac{4}{3}L_{ed,ii22}^{V,LL} + \frac{4}{3}L_{ed,ii11}^{V,LR} + \frac{4}{3}L_{ed,ii22}^{V,LR} + \frac{52}{3}L_{ee,iii}^{V,LL} + \frac{4}{3}L_{ee,iii}^{V,LR} - \frac{8}{3}L_{eu,ii11}^{V,LL} \\
& - \frac{8}{3}L_{eu,ii22}^{V,LL} - \frac{8}{3}L_{eu,ii11}^{V,LR} - \frac{8}{3}L_{eu,ii22}^{V,LR} \Big] + \alpha_s \alpha \Big[ \frac{16}{3}L_{ed,ii11}^{V,LL} + \frac{16}{3}L_{ed,ii22}^{V,LL} \\
& + \frac{16}{3}L_{ed,ii11}^{V,LR} + \frac{16}{3}L_{ed,ii22}^{V,LR} - \frac{32}{3}L_{eu,ii11}^{V,LL} - \frac{32}{3}L_{eu,ii22}^{V,LL} - \frac{32}{3}L_{eu,ii11}^{V,LR} - \frac{32}{3}L_{eu,ii22}^{V,LR} \Big] \\
& + \alpha^2 \Big[ \frac{1184}{27}L_{ee,ijj}^{V,LL} - \frac{712}{27}L_{ee,ijj}^{V,LR} + \frac{1184}{27}L_{ee,iikk}^{V,LL} - \frac{712}{27}L_{ee,iikk}^{V,LR} + \frac{664}{81}L_{ed,ii11}^{V,LL} \\
& + \frac{664}{81}L_{ed,ii22}^{V,LL} + \frac{136}{81}L_{ed,ii11}^{V,LR} + \frac{136}{81}L_{ed,ii22}^{V,LR} - \frac{1342}{27}L_{ee,iii}^{V,LL} - \frac{712}{27}L_{ee,iii}^{V,LR} - \frac{1256}{81}L_{eu,ii11}^{V,LL} \\
& - \frac{1256}{81}L_{eu,ii22}^{V,LL} - \frac{3368}{81}L_{eu,ii11}^{V,LR} - \frac{3368}{81}L_{eu,ii22}^{V,LR} \Big] ;
\end{aligned}$$



$$\dot{L}_{\nu\nu ij}^{V,LL} = 0;$$

$$\dot{L}_{\nu\nu iii}^{V,LL} = 0;$$

$$\begin{aligned} \dot{L}_{de ij}^{V,LR} = & e^2 \left[ \frac{4}{3} L_{ijj}^{V1,LR} + \frac{8}{3} L_{ijj}^{V,LL} + \frac{8}{9} L_{ijji}^{V,LL} - 4 L_{ijj}^{V,LR} + \frac{4}{3} L_{iii}^{V1,LR} \right. \\ & + \frac{32}{9} L_{iii}^{V,LL} + \frac{4}{3} L_{i11}^{V,LR} + \frac{4}{3} L_{i22}^{V,LR} + \frac{4}{3} L_{i33}^{V,LR} - \frac{8}{3} L_{i11}^{V1,LR} - \frac{8}{3} L_{i22}^{V1,LR} \\ & + \frac{4}{3} L_{11i}^{V,LL} + \frac{4}{3} L_{22i}^{V,LL} + \frac{4}{3} L_{33i}^{V,LL} - \frac{8}{3} L_{11i}^{V1,LL} - \frac{8}{3} L_{22i}^{V1,LL} + \frac{4}{9} L_{kkj}^{V,LR} \\ & + \frac{16}{9} L_{jjk}^{V,RR} + \frac{4}{9} L_{11j}^{V,LR} + \frac{4}{9} L_{22j}^{V,LR} + \frac{4}{9} L_{jj11}^{V,RR} + \frac{4}{9} L_{jj22}^{V,RR} + \frac{8}{9} L_{jjj}^{V,LR} \\ & + \frac{8}{3} L_{jjj}^{V,RR} - \frac{8}{9} L_{jj11}^{V,RR} - \frac{8}{9} L_{jj22}^{V,RR} - \frac{8}{9} L_{11jj}^{V,LR} - \frac{8}{9} L_{22jj}^{V,LR} \left. \right] + \alpha_s^2 \left[ 8 L_{11j}^{V,LR} \right. \\ & + 8 L_{22j}^{V,LR} - 8 L_{jj11}^{V,RR} - 8 L_{jj22}^{V,RR} - 8 L_{jj11}^{V,RR} - 8 L_{jj22}^{V,RR} + 8 L_{11jj}^{V,RR} \\ & + 8 L_{22jj}^{V,RR} \left. \right] + \alpha_s \alpha \left[ \frac{16}{3} L_{ijj}^{V1,LR} - \frac{1022}{243} L_{ijj}^{V8,LR} + 8 L_{ijj}^{V,LL} + \frac{64}{243} L_{ijji}^{V,LL} \right. \\ & + 16 L_{ijj}^{V,LR} + \frac{16}{3} L_{iii}^{V1,LR} - \frac{1022}{243} L_{iii}^{V8,LR} + \frac{1048}{81} L_{iii}^{V,LL} - \frac{32}{3} L_{i11}^{V1,LR} - \frac{32}{3} L_{i22}^{V1,LR} \\ & + \frac{1354}{243} L_{i11}^{V8,LR} + \frac{1354}{243} L_{i22}^{V8,LR} - \frac{32}{3} L_{11i}^{V1,LL} - \frac{32}{3} L_{22i}^{V1,LL} - \frac{86}{243} L_{11i}^{V8,LL} - \frac{86}{243} L_{22i}^{V8,LL} \\ & + \frac{16}{9} L_{11j}^{V,LR} + \frac{16}{9} L_{22j}^{V,LR} + \frac{16}{9} L_{jj11}^{V,RR} + \frac{16}{9} L_{jj22}^{V,RR} - \frac{32}{9} L_{jj11}^{V,RR} - \frac{32}{9} L_{jj22}^{V,RR} \\ & - \frac{32}{9} L_{11jj}^{V,LR} - \frac{32}{9} L_{22jj}^{V,LR} \left. \right] + \alpha^2 \left[ \frac{1712}{243} L_{ijj}^{V1,LR} + \frac{256}{243} L_{ijj}^{V,LL} - \frac{1424}{729} L_{ijji}^{V,LL} \right. \\ & + \frac{1906}{27} L_{ijj}^{V,LR} + \frac{1712}{243} L_{iii}^{V1,LR} - \frac{800}{243} L_{iii}^{V,LL} + \frac{3728}{243} L_{i11}^{V,LR} + \frac{3728}{243} L_{i22}^{V,LR} \\ & + \frac{3728}{243} L_{i33}^{V,LR} - \frac{616}{243} L_{i11}^{V1,LR} - \frac{616}{243} L_{i22}^{V1,LR} - \frac{1024}{243} L_{i11}^{V,LL} - \frac{1024}{243} L_{i22}^{V,LL} \\ & - \frac{1024}{243} L_{i33}^{V,LL} - \frac{6952}{243} L_{11i}^{V1,LL} - \frac{6952}{243} L_{22i}^{V1,LL} - \frac{184}{81} L_{kkj}^{V,LR} - \frac{160}{81} L_{jjk}^{V,RR} \\ & - \frac{104}{243} L_{11j}^{V,LR} - \frac{104}{243} L_{22j}^{V,LR} - \frac{440}{243} L_{jj11}^{V,RR} - \frac{440}{243} L_{jj22}^{V,RR} - \frac{368}{81} L_{jjj}^{V,LR} - \frac{80}{9} L_{jjj}^{V,RR} \end{aligned}$$

$$\begin{aligned}
& -\frac{1640}{243}L_{jj11}^{V,RR} - \frac{1640}{243}L_{jj22}^{V,RR} - \frac{296}{243}L_{11jj}^{V,LR} - \frac{296}{243}L_{22jj}^{V,LR} \Big] ; \\
\dot{L}_{ue\bar{u}jj}^{V,LR} = & e^2 \Bigg[ 8L_{ue\bar{u}jj}^{V,LR} - \frac{8}{3}L_{u\bar{u}kk}^{V1,LR} - \frac{16}{3}L_{u\bar{u}kk}^{V,LL} - \frac{16}{9}L_{u\bar{u}kk}^{V,LL} + \frac{4}{3}L_{11\bar{u}i}^{V,LL} \\
& + \frac{4}{3}L_{22\bar{u}i}^{V,LL} + \frac{4}{3}L_{33\bar{u}i}^{V,LL} + \frac{4}{3}L_{u\bar{u}11}^{V1,LL} + \frac{4}{3}L_{u\bar{u}22}^{V1,LL} + \frac{4}{3}L_{u\bar{u}11}^{V1,LR} + \frac{4}{3}L_{u\bar{u}22}^{V1,LR} \\
& + \frac{4}{3}L_{ue\bar{u}11}^{V,LR} + \frac{4}{3}L_{ue\bar{u}22}^{V,LR} + \frac{4}{3}L_{ue\bar{u}33}^{V,LR} - \frac{8}{3}L_{u\bar{u}iii}^{V1,LR} - \frac{64}{9}L_{u\bar{u}iii}^{V,LL} - \frac{8}{9}L_{kkjj}^{V,LR} \\
& - \frac{32}{9}L_{jjkk}^{V,RR} - \frac{8}{9}L_{11jj}^{V,LR} - \frac{8}{9}L_{22jj}^{V,LR} - \frac{8}{9}L_{jj11}^{V,RR} - \frac{8}{9}L_{jj22}^{V,RR} - \frac{16}{9}L_{jjjj}^{V,LR} \\
& - \frac{16}{3}L_{jjjj}^{V,RR} + \frac{16}{9}L_{jj11}^{V,RR} + \frac{16}{9}L_{jj22}^{V,RR} + \frac{16}{9}L_{11jj}^{V,LR} + \frac{16}{9}L_{22jj}^{V,LR} \Big] + \alpha_s^2 \Bigg[ 8L_{de\bar{u}jj}^{V,LR} \\
& + 8L_{de\bar{u}jj}^{V,LR} - 8L_{ed\bar{u}jj}^{V,RR} - 8L_{ed\bar{u}jj}^{V,RR} - 8L_{ed\bar{u}jj}^{V,RR} - 8L_{ed\bar{u}jj}^{V,RR} + 8L_{ue\bar{u}11}^{V,LR} \\
& + 8L_{ue\bar{u}22}^{V,LR} \Big] + \alpha_s \alpha \Bigg[ -32L_{ue\bar{u}jj}^{V,LR} - \frac{32}{3}L_{u\bar{u}kk}^{V1,LR} + \frac{2044}{243}L_{u\bar{u}kk}^{V8,LR} - 16L_{u\bar{u}kk}^{V,LL} \\
& - \frac{128}{243}L_{u\bar{u}kk}^{V,LL} + \frac{16}{3}L_{u\bar{u}11}^{V1,LL} + \frac{16}{3}L_{u\bar{u}22}^{V1,LL} + \frac{16}{3}L_{u\bar{u}11}^{V1,LR} - \frac{32}{3}L_{u\bar{u}22}^{V1,LR} + \frac{388}{243}L_{u\bar{u}11}^{V8,LL} \\
& + \frac{388}{243}L_{u\bar{u}22}^{V8,LL} - \frac{332}{243}L_{u\bar{u}11}^{V8,LR} + \frac{2044}{243}L_{u\bar{u}22}^{V8,LR} - \frac{32}{3}L_{u\bar{u}iii}^{V1,LR} + \frac{2044}{243}L_{u\bar{u}iii}^{V8,LR} \\
& - \frac{2096}{81}L_{u\bar{u}iii}^{V,LL} - \frac{32}{9}L_{de\bar{u}11}^{V,LR} - \frac{32}{9}L_{de\bar{u}22}^{V,LR} - \frac{32}{9}L_{ed\bar{u}11}^{V,RR} - \frac{32}{9}L_{ed\bar{u}22}^{V,RR} + \frac{64}{9}L_{jj11}^{V,RR} \\
& + \frac{64}{9}L_{jj22}^{V,RR} + \frac{64}{9}L_{11jj}^{V,LR} + \frac{64}{9}L_{22jj}^{V,LR} \Big] + \alpha^2 \Bigg[ -\frac{4784}{27}L_{ue\bar{u}jj}^{V,LR} + \frac{12224}{243}L_{u\bar{u}kk}^{V1,LR} \\
& + \frac{3136}{243}L_{u\bar{u}kk}^{V,LL} + \frac{1024}{729}L_{u\bar{u}kk}^{V,LL} - \frac{4744}{243}L_{11\bar{u}i}^{V,LL} - \frac{4744}{243}L_{22\bar{u}i}^{V,LL} - \frac{4744}{243}L_{33\bar{u}i}^{V,LL} \\
& - \frac{3808}{243}L_{u\bar{u}11}^{V1,LL} - \frac{3808}{243}L_{u\bar{u}22}^{V1,LL} - \frac{1144}{243}L_{u\bar{u}11}^{V1,LR} + \frac{12512}{243}L_{u\bar{u}22}^{V1,LR} + \frac{3248}{243}L_{ue\bar{u}11}^{V,LR} \\
& + \frac{3248}{243}L_{ue\bar{u}22}^{V,LR} + \frac{3248}{243}L_{ue\bar{u}33}^{V,LR} + \frac{12224}{243}L_{u\bar{u}iii}^{V1,LR} + \frac{3808}{243}L_{u\bar{u}iii}^{V,LL} + \frac{1808}{81}L_{kkjj}^{V,LR} \\
& + \frac{896}{81}L_{jjkk}^{V,RR} + \frac{1792}{243}L_{de\bar{u}jj}^{V,LR} + \frac{1792}{243}L_{de\bar{u}jj}^{V,LR} + \frac{1168}{243}L_{ed\bar{u}jj}^{V,RR} + \frac{1168}{243}L_{ed\bar{u}jj}^{V,RR} \\
& + \frac{3616}{81}L_{jjjj}^{V,LR} + \frac{160}{9}L_{jjjj}^{V,RR} - \frac{1184}{243}L_{jj11}^{V,RR} - \frac{1184}{243}L_{jj22}^{V,RR} + \frac{1312}{243}L_{11jj}^{V,LR}
\end{aligned}$$

$$\begin{aligned}
& + \frac{1312}{243} L_{22jj}^{V,LR} \Big] ; \\
\dot{L}_{\dot{ii}jj}^{V,LR} = & e^2 \left[ \frac{4}{3} L_{\dot{ii}11}^{V,LL} + \frac{4}{3} L_{\dot{ii}22}^{V,LL} + \frac{4}{3} L_{\dot{ii}11}^{V,LR} + \frac{4}{3} L_{\dot{ii}22}^{V,LR} + \frac{4}{3} L_{\dot{ii}11}^{V,LL} \right. \\
& + \frac{4}{3} L_{\dot{ii}22}^{V,LL} + \frac{4}{3} L_{\dot{ii}33}^{V,LL} + \frac{4}{3} L_{\dot{ii}11}^{V,LR} + \frac{4}{3} L_{\dot{ii}22}^{V,LR} + \frac{4}{3} L_{\dot{ii}33}^{V,LR} - \frac{8}{3} L_{\dot{ii}11}^{V,LL} \\
& \left. - \frac{8}{3} L_{\dot{ii}22}^{V,LL} - \frac{8}{3} L_{\dot{ii}11}^{V,LR} - \frac{8}{3} L_{\dot{ii}22}^{V,LR} \right] + \alpha_s \alpha \left[ \frac{16}{3} L_{\dot{ii}11}^{V,LL} + \frac{16}{3} L_{\dot{ii}22}^{V,LL} \right. \\
& + \frac{16}{3} L_{\dot{ii}11}^{V,LR} + \frac{16}{3} L_{\dot{ii}22}^{V,LR} - \frac{32}{3} L_{\dot{ii}11}^{V,LL} - \frac{32}{3} L_{\dot{ii}22}^{V,LL} - \frac{32}{3} L_{\dot{ii}11}^{V,LR} - \frac{32}{3} L_{\dot{ii}22}^{V,LR} \Big] \\
& + \alpha^2 \left[ -\frac{32}{9} L_{\dot{ii}11}^{V,LL} - \frac{32}{9} L_{\dot{ii}22}^{V,LL} + \frac{40}{9} L_{\dot{ii}11}^{V,LR} + \frac{40}{9} L_{\dot{ii}22}^{V,LR} - 8 L_{\dot{ii}11}^{V,LL} \right. \\
& - 8 L_{\dot{ii}22}^{V,LL} - 8 L_{\dot{ii}33}^{V,LL} + 16 L_{\dot{ii}11}^{V,LR} + 16 L_{\dot{ii}22}^{V,LR} + 16 L_{\dot{ii}33}^{V,LR} - \frac{176}{9} L_{\dot{ii}11}^{V,LL} \\
& \left. - \frac{176}{9} L_{\dot{ii}22}^{V,LL} + \frac{112}{9} L_{\dot{ii}11}^{V,LR} + \frac{112}{9} L_{\dot{ii}22}^{V,LR} \right] ; \\
\dot{L}_{\dot{ii}jj}^{V,LR} = & e^2 \left[ \frac{4}{9} L_{\dot{ii}11}^{V,LL} + \frac{4}{9} L_{\dot{ii}22}^{V,LL} + \frac{4}{9} L_{\dot{ii}11}^{V,LR} + \frac{4}{9} L_{\dot{ii}22}^{V,LR} + \frac{4}{9} L_{\dot{ii}11}^{V,LL} \right. \\
& + \frac{4}{9} L_{\dot{ii}22}^{V,LL} + \frac{4}{9} L_{\dot{ii}33}^{V,LL} + \frac{4}{9} L_{\dot{ii}11}^{V,LR} + \frac{4}{9} L_{\dot{ii}22}^{V,LR} + \frac{4}{9} L_{\dot{ii}33}^{V,LR} - \frac{8}{9} L_{\dot{ii}11}^{V,LL} \\
& \left. - \frac{8}{9} L_{\dot{ii}22}^{V,LL} - \frac{8}{9} L_{\dot{ii}11}^{V,LR} - \frac{8}{9} L_{\dot{ii}22}^{V,LR} \right] + \alpha_s^2 \left[ -8 L_{\dot{ii}11}^{V,LL} - 8 L_{\dot{ii}22}^{V,LL} \right. \\
& + 8 L_{\dot{ii}11}^{V,LR} + 8 L_{\dot{ii}22}^{V,LR} - 8 L_{\dot{ii}11}^{V,LL} - 8 L_{\dot{ii}22}^{V,LL} + 8 L_{\dot{ii}11}^{V,LR} + 8 L_{\dot{ii}22}^{V,LR} \Big] \\
& + \alpha_s \alpha \left[ \frac{16}{9} L_{\dot{ii}11}^{V,LL} + \frac{16}{9} L_{\dot{ii}22}^{V,LL} + \frac{16}{9} L_{\dot{ii}11}^{V,LR} + \frac{16}{9} L_{\dot{ii}22}^{V,LR} - \frac{32}{9} L_{\dot{ii}11}^{V,LL} \right. \\
& - \frac{32}{9} L_{\dot{ii}22}^{V,LL} - \frac{32}{9} L_{\dot{ii}11}^{V,LR} - \frac{32}{9} L_{\dot{ii}22}^{V,LR} \Big] + \alpha^2 \left[ -\frac{8}{27} L_{\dot{ii}11}^{V,LL} - \frac{8}{27} L_{\dot{ii}22}^{V,LL} \right. \\
& + \frac{16}{27} L_{\dot{ii}11}^{V,LR} + \frac{16}{27} L_{\dot{ii}22}^{V,LR} + \frac{8}{3} L_{\dot{ii}11}^{V,LR} + \frac{8}{3} L_{\dot{ii}22}^{V,LR} + \frac{8}{3} L_{\dot{ii}33}^{V,LR} - \frac{80}{27} L_{\dot{ii}11}^{V,LL}
\end{aligned}$$

$$\begin{aligned}
& -\frac{80}{27}L_{\nu u, ii22}^{V,LL} + \frac{16}{27}L_{\nu u, ii11}^{V,LR} + \frac{16}{27}L_{\nu u, ii22}^{V,LR} \Big] ; \\
\dot{L}_{\nu u, ij}^{V,LR} = & e^2 \Bigg[ -\frac{8}{9}L_{\nu d, ii11}^{V,LL} - \frac{8}{9}L_{\nu d, ii22}^{V,LL} - \frac{8}{9}L_{\nu d, ii11}^{V,LR} - \frac{8}{9}L_{\nu d, ii22}^{V,LR} - \frac{8}{9}L_{\nu e, ii11}^{V,LL} \\
& - \frac{8}{9}L_{\nu e, ii22}^{V,LL} - \frac{8}{9}L_{\nu e, ii33}^{V,LL} - \frac{8}{9}L_{\nu e, ii11}^{V,LR} - \frac{8}{9}L_{\nu e, ii22}^{V,LR} - \frac{8}{9}L_{\nu e, ii33}^{V,LR} + \frac{16}{9}L_{\nu u, ii11}^{V,LL} \\
& + \frac{16}{9}L_{\nu u, ii22}^{V,LL} + \frac{16}{9}L_{\nu u, ii11}^{V,LR} + \frac{16}{9}L_{\nu u, ii22}^{V,LR} \Big] + \alpha_s^2 \Bigg[ -8L_{\nu d, ii11}^{V,LL} - 8L_{\nu d, ii22}^{V,LL} \\
& + 8L_{\nu d, ii11}^{V,LR} + 8L_{\nu d, ii22}^{V,LR} - 8L_{\nu u, ii11}^{V,LL} - 8L_{\nu u, ii22}^{V,LL} + 8L_{\nu u, ii11}^{V,LR} + 8L_{\nu u, ii22}^{V,LR} \Big] \\
& + \alpha_s \alpha \Bigg[ -\frac{32}{9}L_{\nu d, ii11}^{V,LL} - \frac{32}{9}L_{\nu d, ii22}^{V,LL} - \frac{32}{9}L_{\nu d, ii11}^{V,LR} - \frac{32}{9}L_{\nu d, ii22}^{V,LR} + \frac{64}{9}L_{\nu u, ii11}^{V,LL} \\
& + \frac{64}{9}L_{\nu u, ii22}^{V,LL} + \frac{64}{9}L_{\nu u, ii11}^{V,LR} + \frac{64}{9}L_{\nu u, ii22}^{V,LR} \Big] + \alpha^2 \Bigg[ -\frac{56}{27}L_{\nu d, ii11}^{V,LL} - \frac{56}{27}L_{\nu d, ii22}^{V,LL} \\
& + \frac{40}{27}L_{\nu d, ii11}^{V,LR} + \frac{40}{27}L_{\nu d, ii22}^{V,LR} - 8L_{\nu e, ii11}^{V,LL} - 8L_{\nu e, ii22}^{V,LL} - 8L_{\nu e, ii33}^{V,LL} + \frac{8}{3}L_{\nu e, ii11}^{V,LR} \\
& + \frac{8}{3}L_{\nu e, ii22}^{V,LR} + \frac{8}{3}L_{\nu e, ii33}^{V,LR} - \frac{128}{27}L_{\nu u, ii11}^{V,LL} - \frac{128}{27}L_{\nu u, ii22}^{V,LL} + \frac{256}{27}L_{\nu u, ii11}^{V,LR} \\
& + \frac{256}{27}L_{\nu u, ii22}^{V,LR} \Big] ;
\end{aligned}$$

$$\begin{aligned}
\dot{L}_{du, ij}^{V1,LR} = & -\frac{8}{3}L_{du, ij}^{V8,LR} g_s^2 + e^2 \Bigg[ -\frac{8}{9}L_{dd, iii}^{V1,LR} - \frac{8}{9}L_{dd, ij}^{V1,LR} - \frac{64}{27}L_{dd, iii}^{V,LL} - \frac{16}{9}L_{dd, ij}^{V,LL} \\
& - \frac{16}{27}L_{dd, ij}^{V,LL} - \frac{8}{9}L_{de, ii11}^{V,LR} - \frac{8}{9}L_{de, ii22}^{V,LR} - \frac{8}{9}L_{de, ii33}^{V,LR} + \frac{4}{9}L_{du, 11jj}^{V1,LR} + \frac{4}{9}L_{du, 22jj}^{V1,LR} \\
& + \frac{16}{9}L_{du, ii11}^{V1,LR} + \frac{16}{9}L_{du, ii22}^{V1,LR} + \frac{8}{3}L_{du, ij}^{V1,LR} - \frac{8}{9}L_{ed, 11ii}^{V,LL} - \frac{8}{9}L_{ed, 22ii}^{V,LL} - \frac{8}{9}L_{ed, 33ii}^{V,LL} \\
& + \frac{4}{9}L_{eu, 11jj}^{V,LR} + \frac{4}{9}L_{eu, 22jj}^{V,LR} + \frac{4}{9}L_{eu, 33jj}^{V,LR} + \frac{4}{9}L_{eu, 11jj}^{V,RR} + \frac{4}{9}L_{eu, 22jj}^{V,RR} + \frac{4}{9}L_{eu, 33jj}^{V,RR} \\
& + \frac{16}{9}L_{ud, 11ii}^{V1,LL} + \frac{16}{9}L_{ud, 22ii}^{V1,LL} + \frac{4}{9}L_{ud, jj11}^{V1,RR} + \frac{4}{9}L_{ud, jj22}^{V1,RR} - \frac{8}{9}L_{uu, jjjj}^{V1,LR} - \frac{8}{9}L_{uu, kkjj}^{V1,LR} \\
& - \frac{64}{27}L_{uu, jjjj}^{V,RR} - \frac{16}{9}L_{uu, jjkk}^{V,RR} - \frac{16}{27}L_{uu, jkkj}^{V,RR} \Big] + \alpha_s^2 \Bigg[ 8L_{dd, iii}^{V1,LR} + 8L_{dd, ij}^{V1,LR}
\end{aligned}$$

$$\begin{aligned}
& + \frac{44}{27} L_{\ddot{iii}}^{V8,LR} + \frac{44}{27} L_{\ddot{ijj}}^{V8,LR} - \frac{232}{9} L_{\ddot{iii}}^{V,LL} - 16 L_{\ddot{ijj}}^{V,LL} - \frac{64}{27} L_{\ddot{ijji}}^{V,LL} + 8 L_{\ddot{11jj}}^{V1,LR} \\
& + 8 L_{\ddot{22jj}}^{V1,LR} + 8 L_{\ddot{ii11}}^{V1,LR} + 8 L_{\ddot{ii22}}^{V1,LR} - \frac{28}{3} L_{\ddot{ijj}}^{V1,LR} + \frac{44}{27} L_{\ddot{11jj}}^{V8,LR} + \frac{44}{27} L_{\ddot{22jj}}^{V8,LR} \\
& + \frac{44}{27} L_{\ddot{ii11}}^{V8,LR} + \frac{44}{27} L_{\ddot{ii22}}^{V8,LR} - \frac{2044}{27} L_{\ddot{ijj}}^{V8,LR} - 8 L_{\ddot{11ii}}^{V1,LL} - 8 L_{\ddot{22ii}}^{V1,LL} - 8 L_{\ddot{jj11}}^{V1,RR} \\
& - 8 L_{\ddot{jj22}}^{V1,RR} + \frac{44}{27} L_{\ddot{11ii}}^{V8,LL} + \frac{44}{27} L_{\ddot{22ii}}^{V8,LL} + \frac{44}{27} L_{\ddot{jj11}}^{V8,RR} + \frac{44}{27} L_{\ddot{jj22}}^{V8,RR} + 8 L_{\ddot{jjjj}}^{V1,LR} \\
& + 8 L_{\ddot{kkjj}}^{V1,LR} + \frac{44}{27} L_{\ddot{jjjj}}^{V8,LR} + \frac{44}{27} L_{\ddot{kkjj}}^{V8,LR} - \frac{232}{9} L_{\ddot{jjjj}}^{V,RR} - 16 L_{\ddot{jjkk}}^{V,RR} - \frac{64}{27} L_{\ddot{jjkj}}^{V,RR} \Big] \\
& + \alpha_s \alpha \left[ - \frac{32}{9} L_{\ddot{iii}}^{V1,LR} - \frac{32}{9} L_{\ddot{ijj}}^{V1,LR} + \frac{2044}{729} L_{\ddot{iii}}^{V8,LR} + \frac{2044}{729} L_{\ddot{ijj}}^{V8,LR} - \frac{2096}{243} L_{\ddot{iii}}^{V,LL} \right. \\
& - \frac{16}{3} L_{\ddot{ijj}}^{V,LL} - \frac{128}{729} L_{\ddot{ijji}}^{V,LL} + \frac{16}{9} L_{\ddot{11jj}}^{V1,LR} - \frac{32}{9} L_{\ddot{22jj}}^{V1,LR} + \frac{64}{9} L_{\ddot{ii11}}^{V1,LR} + \frac{64}{9} L_{\ddot{ii22}}^{V1,LR} \\
& - \frac{64}{3} L_{\ddot{ijj}}^{V1,LR} - \frac{332}{729} L_{\ddot{11jj}}^{V8,LR} + \frac{2044}{729} L_{\ddot{22jj}}^{V8,LR} - \frac{2708}{729} L_{\ddot{ii11}}^{V8,LR} - \frac{2708}{729} L_{\ddot{ii22}}^{V8,LR} \\
& + \frac{232}{27} L_{\ddot{ijj}}^{V8,LR} + \frac{64}{9} L_{\ddot{11ii}}^{V1,LL} + \frac{64}{9} L_{\ddot{22ii}}^{V1,LL} + \frac{16}{9} L_{\ddot{jj11}}^{V1,RR} + \frac{16}{9} L_{\ddot{jj22}}^{V1,RR} + \frac{172}{729} L_{\ddot{11ii}}^{V8,LL} \\
& + \frac{172}{729} L_{\ddot{22ii}}^{V8,LL} + \frac{388}{729} L_{\ddot{jj11}}^{V8,RR} + \frac{388}{729} L_{\ddot{jj22}}^{V8,RR} - \frac{32}{9} L_{\ddot{jjjj}}^{V1,LR} - \frac{32}{9} L_{\ddot{kkjj}}^{V1,LR} + \frac{2044}{729} L_{\ddot{jjjj}}^{V8,LR} \\
& + \frac{2044}{729} L_{\ddot{kkjj}}^{V8,LR} - \frac{2096}{243} L_{\ddot{jjjj}}^{V,RR} - \frac{16}{3} L_{\ddot{jjkk}}^{V,RR} - \frac{128}{729} L_{\ddot{jjkj}}^{V,RR} \Big] + \alpha^2 \left[ \frac{3776}{729} L_{\ddot{iii}}^{V1,LR} \right. \\
& + \frac{3776}{729} L_{\ddot{ijj}}^{V1,LR} + \frac{880}{729} L_{\ddot{iii}}^{V,LL} + \frac{928}{729} L_{\ddot{ijj}}^{V,LL} - \frac{32}{2187} L_{\ddot{ijji}}^{V,LL} + \frac{6224}{729} L_{\ddot{ii11}}^{V,LR} \\
& + \frac{6224}{729} L_{\ddot{ii22}}^{V,LR} + \frac{6224}{729} L_{\ddot{ii33}}^{V,LR} - \frac{208}{729} L_{\ddot{11jj}}^{V1,LR} + \frac{6752}{729} L_{\ddot{22jj}}^{V1,LR} + \frac{6272}{729} L_{\ddot{ii11}}^{V1,LR} \\
& + \frac{6272}{729} L_{\ddot{ii22}}^{V1,LR} - \frac{3872}{81} L_{\ddot{ii33}}^{V1,LR} - \frac{3712}{729} L_{\ddot{11ii}}^{V,LL} - \frac{3712}{729} L_{\ddot{22ii}}^{V,LL} - \frac{3712}{729} L_{\ddot{33ii}}^{V,LL} \\
& + \frac{2888}{729} L_{\ddot{11jj}}^{V,LR} + \frac{2888}{729} L_{\ddot{22jj}}^{V,LR} + \frac{2888}{729} L_{\ddot{33jj}}^{V,LR} - \frac{1216}{729} L_{\ddot{11jj}}^{V,RR} - \frac{1216}{729} L_{\ddot{22jj}}^{V,RR} \\
& - \frac{1216}{729} L_{\ddot{33jj}}^{V,RR} - \frac{6976}{729} L_{\ddot{11ii}}^{V1,LL} - \frac{6976}{729} L_{\ddot{22ii}}^{V1,LL} - \frac{1576}{729} L_{\ddot{jj11}}^{V1,RR} - \frac{1576}{729} L_{\ddot{jj22}}^{V1,RR} \\
& + \frac{6464}{729} L_{\ddot{jjjj}}^{V1,LR} + \frac{6464}{729} L_{\ddot{kkjj}}^{V1,LR} + \frac{4384}{729} L_{\ddot{jjjj}}^{V,RR} + \frac{1984}{729} L_{\ddot{jjkk}}^{V,RR} + \frac{3328}{2187} L_{\ddot{jjkj}}^{V,RR} \Big] ;
\end{aligned}$$

$$\begin{aligned}
\dot{L}_{ijj}^{V8,LR} = & g_s^2 \left[ \frac{2}{3} L_{iii}^{V8,LR} + \frac{2}{3} L_{ijj}^{V8,LR} + \frac{8}{3} L_{iii}^{V,LL} + \frac{8}{3} L_{ijj}^{V,LL} - 12 L_{ijj}^{V1,LR} \right. \\
& + \frac{2}{3} L_{11jj}^{V8,LR} + \frac{2}{3} L_{22jj}^{V8,LR} + \frac{2}{3} L_{ii11}^{V8,LR} + \frac{2}{3} L_{ii22}^{V8,LR} - 14 L_{ijj}^{V8,LR} + \frac{2}{3} L_{11ii}^{V8,LL} \\
& + \frac{2}{3} L_{22ii}^{V8,LL} + \frac{2}{3} L_{jj11}^{V8,RR} + \frac{2}{3} L_{jj22}^{V8,RR} + \frac{2}{3} L_{jjjj}^{V8,LR} + \frac{2}{3} L_{kkjj}^{V8,LR} + \frac{8}{3} L_{jjjj}^{V,RR} \\
& \left. + \frac{8}{3} L_{jkkj}^{V,RR} \right] + \frac{8}{3} L_{ijj}^{V8,LR} e^2 + \alpha_s^2 \left[ -\frac{22}{3} L_{iii}^{V1,LR} - \frac{22}{3} L_{ijj}^{V1,LR} + \frac{787}{81} L_{iii}^{V8,LR} \right. \\
& + \frac{787}{81} L_{ijj}^{V8,LR} + \frac{1198}{27} L_{iii}^{V,LL} - \frac{28}{3} L_{ijj}^{V,LL} + \frac{3448}{81} L_{ijj}^{V,LL} - \frac{22}{3} L_{11jj}^{V1,LR} - \frac{22}{3} L_{22jj}^{V1,LR} \\
& - \frac{22}{3} L_{ii11}^{V1,LR} - \frac{22}{3} L_{ii22}^{V1,LR} - \frac{374}{3} L_{ijj}^{V1,LR} + \frac{787}{81} L_{11jj}^{V8,LR} + \frac{787}{81} L_{22jj}^{V8,LR} + \frac{787}{81} L_{ii11}^{V8,LR} \\
& + \frac{787}{81} L_{ii22}^{V8,LR} - \frac{2975}{18} L_{ijj}^{V8,LR} - \frac{2}{3} L_{11ii}^{V1,LL} - \frac{2}{3} L_{22ii}^{V1,LL} - \frac{2}{3} L_{jj11}^{V1,RR} - \frac{2}{3} L_{jj22}^{V1,RR} \\
& + \frac{607}{81} L_{11ii}^{V8,LL} + \frac{607}{81} L_{22ii}^{V8,LL} + \frac{607}{81} L_{jj11}^{V8,RR} + \frac{607}{81} L_{jj22}^{V8,RR} - \frac{22}{3} L_{jjjj}^{V1,LR} - \frac{22}{3} L_{kkjj}^{V1,LR} \\
& \left. + \frac{787}{81} L_{jjjj}^{V8,LR} + \frac{787}{81} L_{kkjj}^{V8,LR} + \frac{1198}{27} L_{jjjj}^{V,RR} - \frac{28}{3} L_{jjkk}^{V,RR} + \frac{3448}{81} L_{jkkj}^{V,RR} \right] \\
& + \alpha_s \alpha \left[ -\frac{916}{81} L_{iii}^{V1,LR} - \frac{916}{81} L_{ijj}^{V1,LR} - \frac{44}{9} L_{iii}^{V8,LR} - \frac{44}{9} L_{ijj}^{V8,LR} - \frac{2144}{81} L_{iii}^{V,LL} \right. \\
& - \frac{1832}{81} L_{ijj}^{V,LL} + \frac{664}{243} L_{ijji}^{V,LL} - \frac{916}{81} L_{ii11}^{V,LR} - \frac{916}{81} L_{ii22}^{V,LR} - \frac{916}{81} L_{ii33}^{V,LR} + \frac{644}{81} L_{11jj}^{V1,LR} \\
& - \frac{1216}{81} L_{22jj}^{V1,LR} + \frac{1832}{81} L_{ii11}^{V1,LR} + \frac{1832}{81} L_{ii22}^{V1,LR} + \frac{116}{3} L_{ijj}^{V1,LR} + \frac{14}{9} L_{11jj}^{V8,LR} - \frac{20}{3} L_{22jj}^{V8,LR} \\
& + \frac{56}{9} L_{ii11}^{V8,LR} + \frac{56}{9} L_{ii22}^{V8,LR} + \frac{187}{9} L_{ijj}^{V8,LR} - \frac{916}{81} L_{11ii}^{V,LL} - \frac{916}{81} L_{22ii}^{V,LL} - \frac{916}{81} L_{33ii}^{V,LL} \\
& + \frac{644}{81} L_{11jj}^{V,LR} + \frac{644}{81} L_{22jj}^{V,LR} + \frac{644}{81} L_{33jj}^{V,LR} + \frac{644}{81} L_{11jj}^{V,RR} + \frac{644}{81} L_{22jj}^{V,RR} + \frac{644}{81} L_{33jj}^{V,RR} \\
& + \frac{1832}{81} L_{11ii}^{V1,LL} + \frac{1832}{81} L_{22ii}^{V1,LL} + \frac{644}{81} L_{jj11}^{V1,RR} + \frac{644}{81} L_{jj22}^{V1,RR} - \frac{160}{27} L_{11ii}^{V8,LL} \\
& - \frac{160}{27} L_{22ii}^{V8,LL} - \frac{70}{27} L_{jj11}^{V8,RR} - \frac{70}{27} L_{jj22}^{V8,RR} - \frac{1288}{81} L_{jjjj}^{V1,LR} - \frac{1288}{81} L_{kkjj}^{V1,LR} - \frac{20}{3} L_{jjjj}^{V8,LR} \\
& \left. - \frac{20}{3} L_{kkjj}^{V8,LR} - \frac{3608}{81} L_{jjjj}^{V,RR} - \frac{2576}{81} L_{jjkk}^{V,RR} - \frac{800}{243} L_{jkkj}^{V,RR} \right] - \frac{3872}{81} L_{ijj}^{V8,LR}
\end{aligned}$$

$$\alpha^2 ;$$

$$\begin{aligned}
\dot{L}_{de}^{V,LR}{}_{jji} = & e^2 \left[ -4L_{de}^{V,LR}{}_{jji} + \frac{4}{9}L_{jji}^{V,LR} + \frac{16}{9}L_{ijj}^{V,RR} + \frac{4}{9}L_{kii}^{V,LR} + \frac{16}{9}L_{ikk}^{V,RR} \right. \\
& + \frac{4}{9}L_{11ii}^{V,LR} + \frac{4}{9}L_{22ii}^{V,LR} + \frac{4}{9}L_{ii11}^{V,RR} + \frac{4}{9}L_{ii22}^{V,RR} + \frac{4}{9}L_{iii}^{V,LR} + \frac{16}{9}L_{iii}^{V,RR} \\
& - \frac{8}{9}L_{ii11}^{V,RR} - \frac{8}{9}L_{ii22}^{V,RR} - \frac{8}{9}L_{11ii}^{V,LR} - \frac{8}{9}L_{22ii}^{V,LR} + \frac{8}{3}L_{jjjj}^{V1,LR} + \frac{64}{9}L_{jjjj}^{V,LL} \\
& + \frac{4}{3}L_{jj11}^{V,LR} + \frac{4}{3}L_{jj22}^{V,LR} + \frac{4}{3}L_{jj33}^{V,LR} - \frac{8}{3}L_{jj11}^{V1,LR} - \frac{8}{3}L_{jj22}^{V1,LR} + \frac{4}{3}L_{11jj}^{V,LL} \\
& + \frac{4}{3}L_{22jj}^{V,LL} + \frac{4}{3}L_{33jj}^{V,LL} - \frac{8}{3}L_{11jj}^{V1,LL} - \frac{8}{3}L_{22jj}^{V1,LL} \left. \right] + \alpha_s^2 \left[ 8L_{11ii}^{V,LR} \right. \\
& + 8L_{22ii}^{V,LR} - 8L_{ii11}^{V,RR} - 8L_{ii22}^{V,RR} - 8L_{ii11}^{V,RR} - 8L_{ii22}^{V,RR} + 8L_{11ii}^{V,RR} \\
& + 8L_{22ii}^{V,RR} \left. \right] + \alpha_s \alpha \left[ 16L_{jji}^{V,LR} + \frac{16}{9}L_{11ii}^{V,LR} + \frac{16}{9}L_{22ii}^{V,LR} + \frac{16}{9}L_{ii11}^{V,RR} \right. \\
& + \frac{16}{9}L_{ii22}^{V,RR} - \frac{32}{9}L_{ii11}^{V,RR} - \frac{32}{9}L_{ii22}^{V,RR} - \frac{32}{9}L_{11ii}^{V,LR} - \frac{32}{9}L_{22ii}^{V,LR} + \frac{32}{3}L_{jjjj}^{V1,LR} \\
& - \frac{2044}{243}L_{jjjj}^{V8,LR} + \frac{5152}{243}L_{jjjj}^{V,LL} - \frac{32}{3}L_{jj11}^{V1,LR} - \frac{32}{3}L_{jj22}^{V1,LR} + \frac{1354}{243}L_{jj11}^{V8,LR} \\
& + \frac{1354}{243}L_{jj22}^{V8,LR} - \frac{32}{3}L_{11jj}^{V1,LL} - \frac{32}{3}L_{22jj}^{V1,LL} - \frac{86}{243}L_{11jj}^{V8,LL} - \frac{86}{243}L_{22jj}^{V8,LL} \left. \right] \\
& + \alpha^2 \left[ \frac{1906}{27}L_{jji}^{V,LR} - \frac{184}{81}L_{jji}^{V,LR} - \frac{160}{81}L_{ijj}^{V,RR} - \frac{184}{81}L_{kii}^{V,LR} - \frac{160}{81}L_{ikk}^{V,RR} \right. \\
& - \frac{104}{243}L_{11ii}^{V,LR} - \frac{104}{243}L_{22ii}^{V,LR} - \frac{440}{243}L_{ii11}^{V,RR} - \frac{440}{243}L_{ii22}^{V,RR} - \frac{184}{81}L_{iii}^{V,LR} - \frac{640}{81}L_{iii}^{V,RR} \\
& - \frac{1640}{243}L_{ii11}^{V,RR} - \frac{1640}{243}L_{ii22}^{V,RR} - \frac{296}{243}L_{11ii}^{V,LR} - \frac{296}{243}L_{22ii}^{V,LR} + \frac{3424}{243}L_{jjjj}^{V1,LR} \\
& - \frac{3056}{729}L_{jjjj}^{V,LL} + \frac{3728}{243}L_{jj11}^{V,LR} + \frac{3728}{243}L_{jj22}^{V,LR} + \frac{3728}{243}L_{jj33}^{V,LR} - \frac{616}{243}L_{jj11}^{V1,LR} \\
& - \frac{616}{243}L_{jj22}^{V1,LR} - \frac{1024}{243}L_{11jj}^{V,LL} - \frac{1024}{243}L_{22jj}^{V,LL} - \frac{1024}{243}L_{33jj}^{V,LL} - \frac{6952}{243}L_{11jj}^{V1,LL} \\
& \left. - \frac{6952}{243}L_{22jj}^{V1,LL} \right] ;
\end{aligned}$$

$$\begin{aligned}
\dot{L}_{ue,jji}^{V,LR} = & e^2 \left[ -\frac{8}{9}L_{de,11ii}^{V,LR} - \frac{8}{9}L_{de,22ii}^{V,LR} - \frac{8}{9}L_{ed,ii11}^{V,RR} - \frac{8}{9}L_{ed,ii22}^{V,RR} - \frac{8}{9}L_{ee,iii}^{V,LR} \right. \\
& - \frac{8}{9}L_{ee,jji}^{V,LR} - \frac{8}{9}L_{ee,kkii}^{V,LR} - \frac{32}{9}L_{ee,iii}^{V,RR} - \frac{32}{9}L_{ee,ijj}^{V,RR} - \frac{32}{9}L_{ee,iik}^{V,RR} + \frac{4}{3}L_{eu,11jj}^{V,LL} \\
& + \frac{4}{3}L_{eu,22jj}^{V,LL} + \frac{4}{3}L_{eu,33jj}^{V,LL} + \frac{16}{9}L_{eu,ii11}^{V,RR} + \frac{16}{9}L_{eu,ii22}^{V,RR} + \frac{4}{3}L_{ud,jj11}^{V1,LL} + \frac{4}{3}L_{ud,jj22}^{V1,LL} \\
& + \frac{4}{3}L_{ud,jj11}^{V1,LR} + \frac{4}{3}L_{ud,jj22}^{V1,LR} + \frac{16}{9}L_{ue,11ii}^{V,LR} + \frac{16}{9}L_{ue,22ii}^{V,LR} + \frac{4}{3}L_{ue,jj11}^{V,LR} + \frac{4}{3}L_{ue,jj22}^{V,LR} \\
& + \frac{4}{3}L_{ue,jj33}^{V,LR} + 8L_{ue,jji}^{V,LR} - \frac{8}{3}L_{uu,jjj}^{V1,LR} - \frac{8}{3}L_{uu,jjkk}^{V1,LR} - \frac{64}{9}L_{uu,jjj}^{V,LL} - \frac{16}{3}L_{uu,jjkk}^{V,LL} \\
& \left. - \frac{16}{9}L_{uu,jkkj}^{V,LL} \right] + \alpha_s^2 \left[ 8L_{de,11ii}^{V,LR} + 8L_{de,22ii}^{V,LR} - 8L_{ed,ii11}^{V,RR} - 8L_{ed,ii22}^{V,RR} \right. \\
& - 8L_{eu,ii11}^{V,RR} - 8L_{eu,ii22}^{V,RR} + 8L_{ue,11ii}^{V,LR} + 8L_{ue,22ii}^{V,LR} \left. \right] + \alpha_s \alpha \left[ -\frac{32}{9}L_{de,11ii}^{V,LR} \right. \\
& - \frac{32}{9}L_{de,22ii}^{V,LR} - \frac{32}{9}L_{ed,ii11}^{V,RR} - \frac{32}{9}L_{ed,ii22}^{V,RR} + \frac{64}{9}L_{eu,ii11}^{V,RR} + \frac{64}{9}L_{eu,ii22}^{V,RR} + \frac{16}{3}L_{ud,jj11}^{V1,LL} \\
& + \frac{16}{3}L_{ud,jj22}^{V1,LL} + \frac{16}{3}L_{ud,jj11}^{V1,LR} - \frac{32}{3}L_{ud,jj22}^{V1,LR} + \frac{388}{243}L_{ud,jj11}^{V8,LL} + \frac{388}{243}L_{ud,jj22}^{V8,LL} - \frac{332}{243}L_{ud,jj11}^{V8,LR} \\
& + \frac{2044}{243}L_{ud,jj22}^{V8,LR} + \frac{64}{9}L_{ue,11ii}^{V,LR} + \frac{64}{9}L_{ue,22ii}^{V,LR} - 32L_{ue,jji}^{V,LR} - \frac{32}{3}L_{uu,jjj}^{V1,LR} - \frac{32}{3}L_{uu,jjkk}^{V1,LR} \\
& \left. + \frac{2044}{243}L_{uu,jjj}^{V8,LR} + \frac{2044}{243}L_{uu,jjkk}^{V8,LR} - \frac{2096}{81}L_{uu,jjj}^{V,LL} - 16L_{uu,jjkk}^{V,LL} - \frac{128}{243}L_{uu,jkkj}^{V,LL} \right] \\
& + \alpha^2 \left[ \frac{1792}{243}L_{de,11ii}^{V,LR} + \frac{1792}{243}L_{de,22ii}^{V,LR} + \frac{1168}{243}L_{ed,ii11}^{V,RR} + \frac{1168}{243}L_{ed,ii22}^{V,RR} + \frac{1808}{81}L_{ee,iii}^{V,LR} \right. \\
& + \frac{1808}{81}L_{ee,jji}^{V,LR} + \frac{1808}{81}L_{ee,kkii}^{V,LR} + \frac{992}{81}L_{ee,iii}^{V,RR} + \frac{896}{81}L_{ee,ijj}^{V,RR} + \frac{896}{81}L_{ee,iik}^{V,RR} - \frac{4744}{243}L_{eu,11jj}^{V,LL} \\
& - \frac{4744}{243}L_{eu,22jj}^{V,LL} - \frac{4744}{243}L_{eu,33jj}^{V,LL} - \frac{1184}{243}L_{eu,ii11}^{V,RR} - \frac{1184}{243}L_{eu,ii22}^{V,RR} - \frac{3808}{243}L_{ud,jj11}^{V1,LL} \\
& - \frac{3808}{243}L_{ud,jj22}^{V1,LL} - \frac{1144}{243}L_{ud,jj11}^{V1,LR} + \frac{12512}{243}L_{ud,jj22}^{V1,LR} + \frac{1312}{243}L_{ue,11ii}^{V,LR} + \frac{1312}{243}L_{ue,22ii}^{V,LR} \\
& + \frac{3248}{243}L_{ue,jj11}^{V,LR} + \frac{3248}{243}L_{ue,jj22}^{V,LR} + \frac{3248}{243}L_{ue,jj33}^{V,LR} - \frac{4784}{27}L_{ue,jji}^{V,LR} + \frac{12224}{243}L_{uu,jjj}^{V1,LR} \\
& \left. + \frac{12224}{243}L_{uu,jjkk}^{V1,LR} + \frac{3808}{243}L_{uu,jjj}^{V,LL} + \frac{3136}{243}L_{uu,jjkk}^{V,LL} + \frac{1024}{729}L_{uu,jkkj}^{V,LL} \right];
\end{aligned}$$



$$\begin{aligned}
\dot{L}_{jj\bar{i}}^{V,LR} = & e^2 \left[ \frac{4}{3} L_{jj11}^{V,LL} + \frac{4}{3} L_{jj22}^{V,LL} + \frac{4}{3} L_{jj11}^{V,LR} + \frac{4}{3} L_{jj22}^{V,LR} + \frac{4}{3} L_{jj11}^{V,LL} \right. \\
& + \frac{4}{3} L_{jj22}^{V,LL} + \frac{4}{3} L_{jj33}^{V,LL} + \frac{4}{3} L_{jj11}^{V,LR} + \frac{4}{3} L_{jj22}^{V,LR} + \frac{4}{3} L_{jj33}^{V,LR} - \frac{8}{3} L_{jj11}^{V,LL} \\
& \left. - \frac{8}{3} L_{jj22}^{V,LL} - \frac{8}{3} L_{jj11}^{V,LR} - \frac{8}{3} L_{jj22}^{V,LR} \right] + \alpha_s \alpha \left[ \frac{16}{3} L_{jj11}^{V,LL} + \frac{16}{3} L_{jj22}^{V,LL} \right. \\
& + \frac{16}{3} L_{jj11}^{V,LR} + \frac{16}{3} L_{jj22}^{V,LR} - \frac{32}{3} L_{jj11}^{V,LL} - \frac{32}{3} L_{jj22}^{V,LL} - \frac{32}{3} L_{jj11}^{V,LR} - \frac{32}{3} L_{jj22}^{V,LR} \left. \right] \\
& + \alpha^2 \left[ -\frac{32}{9} L_{jj11}^{V,LL} - \frac{32}{9} L_{jj22}^{V,LL} + \frac{40}{9} L_{jj11}^{V,LR} + \frac{40}{9} L_{jj22}^{V,LR} - 8 L_{jj11}^{V,LL} \right. \\
& - 8 L_{jj22}^{V,LL} - 8 L_{jj33}^{V,LL} + 16 L_{jj11}^{V,LR} + 16 L_{jj22}^{V,LR} + 16 L_{jj33}^{V,LR} - \frac{176}{9} L_{jj11}^{V,LL} \\
& \left. - \frac{176}{9} L_{jj22}^{V,LL} + \frac{112}{9} L_{jj11}^{V,LR} + \frac{112}{9} L_{jj22}^{V,LR} \right];
\end{aligned}$$

$$\begin{aligned}
\dot{L}_{jj\bar{i}}^{V,LR} = & e^2 \left[ \frac{4}{9} L_{jj11}^{V,LL} + \frac{4}{9} L_{jj22}^{V,LL} + \frac{4}{9} L_{jj11}^{V,LR} + \frac{4}{9} L_{jj22}^{V,LR} + \frac{4}{9} L_{jj11}^{V,LL} \right. \\
& + \frac{4}{9} L_{jj22}^{V,LL} + \frac{4}{9} L_{jj33}^{V,LL} + \frac{4}{9} L_{jj11}^{V,LR} + \frac{4}{9} L_{jj22}^{V,LR} + \frac{4}{9} L_{jj33}^{V,LR} - \frac{8}{9} L_{jj11}^{V,LL} \\
& \left. - \frac{8}{9} L_{jj22}^{V,LL} - \frac{8}{9} L_{jj11}^{V,LR} - \frac{8}{9} L_{jj22}^{V,LR} \right] + \alpha_s^2 \left[ -8 L_{jj11}^{V,LL} - 8 L_{jj22}^{V,LL} \right. \\
& + 8 L_{jj11}^{V,LR} + 8 L_{jj22}^{V,LR} - 8 L_{jj11}^{V,LL} - 8 L_{jj22}^{V,LL} + 8 L_{jj11}^{V,LR} + 8 L_{jj22}^{V,LR} \left. \right] \\
& + \alpha_s \alpha \left[ \frac{16}{9} L_{jj11}^{V,LL} + \frac{16}{9} L_{jj22}^{V,LL} + \frac{16}{9} L_{jj11}^{V,LR} + \frac{16}{9} L_{jj22}^{V,LR} - \frac{32}{9} L_{jj11}^{V,LL} \right. \\
& - \frac{32}{9} L_{jj22}^{V,LL} - \frac{32}{9} L_{jj11}^{V,LR} - \frac{32}{9} L_{jj22}^{V,LR} \left. \right] + \alpha^2 \left[ -\frac{8}{27} L_{jj11}^{V,LL} - \frac{8}{27} L_{jj22}^{V,LL} \right. \\
& + \frac{16}{27} L_{jj11}^{V,LR} + \frac{16}{27} L_{jj22}^{V,LR} + \frac{8}{3} L_{jj11}^{V,LR} + \frac{8}{3} L_{jj22}^{V,LR} + \frac{8}{3} L_{jj33}^{V,LR} - \frac{80}{27} L_{jj11}^{V,LL} \\
& \left. - \frac{80}{27} L_{jj22}^{V,LL} + \frac{16}{27} L_{jj11}^{V,LR} + \frac{16}{27} L_{jj22}^{V,LR} \right];
\end{aligned}$$

$$\begin{aligned}
\dot{L}_{jj\ddot{i}}^{V,LR} = & e^2 \left[ -\frac{8}{9}L_{jj11}^{V,LL} - \frac{8}{9}L_{jj22}^{V,LL} - \frac{8}{9}L_{jj11}^{V,LR} - \frac{8}{9}L_{jj22}^{V,LR} - \frac{8}{9}L_{jj11}^{V,LL} \right. \\
& - \frac{8}{9}L_{jj22}^{V,LL} - \frac{8}{9}L_{jj33}^{V,LL} - \frac{8}{9}L_{jj11}^{V,LR} - \frac{8}{9}L_{jj22}^{V,LR} - \frac{8}{9}L_{jj33}^{V,LR} + \frac{16}{9}L_{jj11}^{V,LL} \\
& + \frac{16}{9}L_{jj22}^{V,LL} + \frac{16}{9}L_{jj11}^{V,LR} + \frac{16}{9}L_{jj22}^{V,LR} \left. \right] + \alpha_s^2 \left[ -8L_{jj11}^{V,LL} - 8L_{jj22}^{V,LL} \right. \\
& + 8L_{jj11}^{V,LR} + 8L_{jj22}^{V,LR} - 8L_{jj11}^{V,LL} - 8L_{jj22}^{V,LL} + 8L_{jj11}^{V,LR} + 8L_{jj22}^{V,LR} \left. \right] \\
& + \alpha_s \alpha \left[ -\frac{32}{9}L_{jj11}^{V,LL} - \frac{32}{9}L_{jj22}^{V,LL} - \frac{32}{9}L_{jj11}^{V,LR} - \frac{32}{9}L_{jj22}^{V,LR} + \frac{64}{9}L_{jj11}^{V,LL} \right. \\
& + \frac{64}{9}L_{jj22}^{V,LL} + \frac{64}{9}L_{jj11}^{V,LR} + \frac{64}{9}L_{jj22}^{V,LR} \left. \right] + \alpha^2 \left[ -\frac{56}{27}L_{jj11}^{V,LL} - \frac{56}{27}L_{jj22}^{V,LL} \right. \\
& + \frac{40}{27}L_{jj11}^{V,LR} + \frac{40}{27}L_{jj22}^{V,LR} - 8L_{jj11}^{V,LL} - 8L_{jj22}^{V,LL} - 8L_{jj33}^{V,LL} + \frac{8}{3}L_{jj11}^{V,LR} \\
& + \frac{8}{3}L_{jj22}^{V,LR} + \frac{8}{3}L_{jj33}^{V,LR} - \frac{128}{27}L_{jj11}^{V,LL} - \frac{128}{27}L_{jj22}^{V,LL} + \frac{256}{27}L_{jj11}^{V,LR} \\
& \left. + \frac{256}{27}L_{jj22}^{V,LR} \right] ;
\end{aligned}$$

$$\begin{aligned}
\dot{L}_{jj\ddot{i}}^{V1,LR} = & -\frac{8}{3}L_{jj\ddot{i}}^{V8,LR}g_s^2 + e^2 \left[ -\frac{16}{9}L_{jjj}^{V1,LR} - \frac{128}{27}L_{jjj}^{V,LL} - \frac{8}{9}L_{jj11}^{V,LR} - \frac{8}{9}L_{jj22}^{V,LR} \right. \\
& - \frac{8}{9}L_{jj33}^{V,LR} + \frac{4}{9}L_{11\ddot{i}}^{V1,LR} + \frac{4}{9}L_{22\ddot{i}}^{V1,LR} + \frac{16}{9}L_{jj11}^{V1,LR} + \frac{16}{9}L_{jj22}^{V1,LR} + \frac{8}{3}L_{jj\ddot{i}}^{V1,LR} \\
& - \frac{8}{9}L_{11jj}^{V,LL} - \frac{8}{9}L_{22jj}^{V,LL} - \frac{8}{9}L_{33jj}^{V,LL} + \frac{4}{9}L_{11\ddot{i}}^{V,LR} + \frac{4}{9}L_{22\ddot{i}}^{V,LR} + \frac{4}{9}L_{33\ddot{i}}^{V,LR} \\
& + \frac{4}{9}L_{11\ddot{i}}^{V,RR} + \frac{4}{9}L_{22\ddot{i}}^{V,RR} + \frac{4}{9}L_{33\ddot{i}}^{V,RR} + \frac{16}{9}L_{ud}^{V1,LL} + \frac{16}{9}L_{22jj}^{V1,LL} + \frac{4}{9}L_{ii11}^{V1,RR} \\
& + \frac{4}{9}L_{ud}^{V1,RR} - \frac{8}{9}L_{uu}^{V1,LR} - \frac{8}{9}L_{kk\ddot{i}}^{V1,LR} - \frac{64}{27}L_{uu}^{V,RR} - \frac{16}{9}L_{u\ddot{i}}^{V,RR} - \frac{16}{27}L_{u\ddot{i}}^{V,RR} \left. \right] \\
& + \alpha_s^2 \left[ 16L_{jjj}^{V1,LR} + \frac{88}{27}L_{jjj}^{V8,LR} - \frac{1192}{27}L_{jjj}^{V,LL} + 8L_{11\ddot{i}}^{V1,LR} + 8L_{22\ddot{i}}^{V1,LR} \right. \\
& + 8L_{jj11}^{V1,LR} + 8L_{jj22}^{V1,LR} - \frac{28}{3}L_{jj\ddot{i}}^{V1,LR} + \frac{44}{27}L_{11\ddot{i}}^{V8,LR} + \frac{44}{27}L_{22\ddot{i}}^{V8,LR} + \frac{44}{27}L_{jj11}^{V8,LR} \\
& \left. + \frac{44}{27}L_{jj22}^{V8,LR} \right]
\end{aligned}$$

$$\begin{aligned}
& + \frac{44}{27} L_{jj22}^{V8,LR} - \frac{2044}{27} L_{jjii}^{V8,LR} - 8 L_{11jj}^{V1,LL} - 8 L_{22jj}^{V1,LL} - 8 L_{ii11}^{V1,RR} - 8 L_{ii22}^{V1,RR} \\
& + \frac{44}{27} L_{11jj}^{V8,LL} + \frac{44}{27} L_{22jj}^{V8,LL} + \frac{44}{27} L_{ii11}^{V8,RR} + \frac{44}{27} L_{ii22}^{V8,RR} + 8 L_{iii}^{V1,LR} + 8 L_{kkii}^{V1,LR} \\
& + \frac{44}{27} L_{iii}^{V8,LR} + \frac{44}{27} L_{kkii}^{V8,LR} - \frac{232}{9} L_{iii}^{V,RR} - 16 L_{ikk}^{V,RR} - \frac{64}{27} L_{ikki}^{V,RR} \Big] + \alpha_s \alpha \Bigg[ - \frac{64}{9} L_{jjjj}^{V1,LR} \\
& + \frac{4088}{729} L_{jjjj}^{V8,LR} - \frac{10304}{729} L_{jjjj}^{V,LL} + \frac{16}{9} L_{11ii}^{V1,LR} - \frac{32}{9} L_{22ii}^{V1,LR} + \frac{64}{9} L_{jj11}^{V1,LR} + \frac{64}{9} L_{jj22}^{V1,LR} \\
& - \frac{64}{3} L_{jjii}^{V1,LR} - \frac{332}{729} L_{11ii}^{V8,LR} + \frac{2044}{729} L_{22ii}^{V8,LR} - \frac{2708}{729} L_{jj11}^{V8,LR} - \frac{2708}{729} L_{jj22}^{V8,LR} \\
& + \frac{232}{27} L_{jjii}^{V8,LR} + \frac{64}{9} L_{11jj}^{V1,LL} + \frac{64}{9} L_{22jj}^{V1,LL} + \frac{16}{9} L_{ii11}^{V1,RR} + \frac{16}{9} L_{ii22}^{V1,RR} + \frac{172}{729} L_{11jj}^{V8,LL} \\
& + \frac{172}{729} L_{22jj}^{V8,LL} + \frac{388}{729} L_{ii11}^{V8,RR} + \frac{388}{729} L_{ii22}^{V8,RR} - \frac{32}{9} L_{iii}^{V1,LR} - \frac{32}{9} L_{kkii}^{V1,LR} + \frac{2044}{729} L_{iii}^{V8,LR} \\
& + \frac{2044}{729} L_{kkii}^{V8,LR} - \frac{2096}{243} L_{iii}^{V,RR} - \frac{16}{3} L_{ikk}^{V,RR} - \frac{128}{729} L_{ikki}^{V,RR} \Big] + \alpha^2 \Bigg[ \frac{7552}{729} L_{jjjj}^{V1,LR} \\
& + \frac{5392}{2187} L_{jjjj}^{V,LL} + \frac{6224}{729} L_{jj11}^{V,LR} + \frac{6224}{729} L_{jj22}^{V,LR} + \frac{6224}{729} L_{jj33}^{V,LR} - \frac{208}{729} L_{11ii}^{V1,LR} \\
& + \frac{6752}{729} L_{22ii}^{V1,LR} + \frac{6272}{729} L_{jj11}^{V1,LR} + \frac{6272}{729} L_{jj22}^{V1,LR} - \frac{3872}{81} L_{jjii}^{V1,LR} - \frac{3712}{729} L_{11jj}^{V,LL} \\
& - \frac{3712}{729} L_{22jj}^{V,LL} - \frac{3712}{729} L_{33jj}^{V,LL} + \frac{2888}{729} L_{11ii}^{V,LR} + \frac{2888}{729} L_{22ii}^{V,LR} + \frac{2888}{729} L_{33ii}^{V,LR} \\
& - \frac{1216}{729} L_{11ii}^{V,RR} - \frac{1216}{729} L_{22ii}^{V,RR} - \frac{1216}{729} L_{33ii}^{V,RR} - \frac{6976}{729} L_{11jj}^{V1,LL} - \frac{6976}{729} L_{22jj}^{V1,LL} \\
& - \frac{1576}{729} L_{ii11}^{V1,RR} - \frac{1576}{729} L_{ii22}^{V1,RR} + \frac{6464}{729} L_{iii}^{V1,LR} + \frac{6464}{729} L_{kkii}^{V1,LR} + \frac{4384}{729} L_{iii}^{V,RR} \\
& + \frac{1984}{729} L_{ikk}^{V,RR} + \frac{3328}{2187} L_{ikki}^{V,RR} \Big] ;
\end{aligned}$$

$$\begin{aligned}
\dot{L}_{jjii}^{V8,LR} &= g_s^2 \Bigg[ -12 L_{jjii}^{V1,LR} - 14 L_{jjii}^{V8,LR} + \frac{2}{3} L_{kkii}^{V8,LR} + \frac{8}{3} L_{ikki}^{V,RR} + \frac{2}{3} L_{11ii}^{V8,LR} \\
& + \frac{2}{3} L_{22ii}^{V8,LR} + \frac{2}{3} L_{ii11}^{V8,RR} + \frac{2}{3} L_{ii22}^{V8,RR} + \frac{2}{3} L_{iii}^{V8,LR} + \frac{8}{3} L_{iii}^{V,RR} + \frac{4}{3} L_{jjjj}^{V8,LR} \\
& + \frac{16}{3} L_{jjjj}^{V,LL} + \frac{2}{3} L_{jj11}^{V8,LR} + \frac{2}{3} L_{jj22}^{V8,LR} + \frac{2}{3} L_{11jj}^{V8,LL} + \frac{2}{3} L_{22jj}^{V8,LL} \Big] + \frac{8}{3} e^2 L_{jjii}^{V8,LR}
\end{aligned}$$

$$\begin{aligned}
& + \alpha_s^2 \left[ -\frac{374}{3} L_{jjii}^{V1,LR} - \frac{2975}{18} L_{jjii}^{V8,LR} - \frac{22}{3} L_{kkii}^{V1,LR} + \frac{787}{81} L_{kkii}^{V8,LR} - \frac{28}{3} L_{iikk}^{V,RR} \right. \\
& + \frac{3448}{81} L_{iikk}^{V,RR} - \frac{22}{3} L_{11ii}^{V1,LR} - \frac{22}{3} L_{22ii}^{V1,LR} + \frac{787}{81} L_{11ii}^{V8,LR} + \frac{787}{81} L_{22ii}^{V8,LR} - \frac{2}{3} L_{ii11}^{V1,RR} \\
& - \frac{2}{3} L_{ii22}^{V1,RR} + \frac{607}{81} L_{ii11}^{V8,RR} + \frac{607}{81} L_{ii22}^{V8,RR} - \frac{22}{3} L_{iiii}^{V1,LR} + \frac{787}{81} L_{iiii}^{V8,LR} + \frac{1198}{27} L_{iiii}^{V,RR} \\
& - \frac{44}{3} L_{jjjj}^{V1,LR} + \frac{1574}{81} L_{jjjj}^{V8,LR} + \frac{6286}{81} L_{jjjj}^{V,LL} - \frac{22}{3} L_{jj11}^{V1,LR} - \frac{22}{3} L_{jj22}^{V1,LR} + \frac{787}{81} L_{jj11}^{V8,LR} \\
& \left. + \frac{787}{81} L_{jj22}^{V8,LR} - \frac{2}{3} L_{11jj}^{V1,LL} - \frac{2}{3} L_{22jj}^{V1,LL} + \frac{607}{81} L_{11jj}^{V8,LL} + \frac{607}{81} L_{22jj}^{V8,LL} \right] \\
& + \alpha_s \alpha \left[ \frac{116}{3} L_{jjii}^{V1,LR} + \frac{187}{9} L_{jjii}^{V8,LR} - \frac{1288}{81} L_{kkii}^{V1,LR} - \frac{20}{3} L_{kkii}^{V8,LR} - \frac{2576}{81} L_{iikk}^{V,RR} \right. \\
& - \frac{800}{243} L_{iikk}^{V,RR} + \frac{644}{81} L_{11ii}^{V1,LR} - \frac{1216}{81} L_{22ii}^{V1,LR} + \frac{14}{9} L_{11ii}^{V8,LR} - \frac{20}{3} L_{22ii}^{V8,LR} + \frac{644}{81} L_{11ii}^{V,LR} \\
& + \frac{644}{81} L_{22ii}^{V,LR} + \frac{644}{81} L_{33ii}^{V,LR} + \frac{644}{81} L_{11ii}^{V,RR} + \frac{644}{81} L_{22ii}^{V,RR} + \frac{644}{81} L_{33ii}^{V,RR} + \frac{644}{81} L_{ii11}^{V1,RR} \\
& + \frac{644}{81} L_{ii22}^{V1,RR} - \frac{70}{27} L_{ii11}^{V8,RR} - \frac{70}{27} L_{ii22}^{V8,RR} - \frac{1288}{81} L_{iiii}^{V1,LR} - \frac{20}{3} L_{iiii}^{V8,LR} - \frac{3608}{81} L_{iiii}^{V,RR} \\
& - \frac{1832}{81} L_{jjjj}^{V1,LR} - \frac{88}{9} L_{jjjj}^{V8,LR} - \frac{11264}{243} L_{jjjj}^{V,LL} - \frac{916}{81} L_{jj11}^{V,LR} - \frac{916}{81} L_{jj22}^{V,LR} - \frac{916}{81} L_{jj33}^{V,LR} \\
& + \frac{1832}{81} L_{jj11}^{V1,LR} + \frac{1832}{81} L_{jj22}^{V1,LR} + \frac{56}{9} L_{jj11}^{V8,LR} + \frac{56}{9} L_{jj22}^{V8,LR} - \frac{916}{81} L_{11jj}^{V,LL} - \frac{916}{81} L_{22jj}^{V,LL} \\
& - \frac{916}{81} L_{33jj}^{V,LL} + \frac{1832}{81} L_{11jj}^{V1,LL} + \frac{1832}{81} L_{22jj}^{V1,LL} - \frac{160}{27} L_{11jj}^{V8,LL} - \frac{160}{27} L_{22jj}^{V8,LL} \left. \right] \\
& - \frac{3872}{81} \alpha^2 L_{jjii}^{V8,LR} ;
\end{aligned}$$

$$\begin{aligned}
\dot{L}_{ijj}^{V1,LR} &= -\frac{8}{3} L_{ijj}^{V8,LR} g_s^2 + e^2 \left[ \frac{4}{9} L_{iii}^{V1,LR} - \frac{8}{9} L_{ijj}^{V1,LR} + \frac{8}{9} L_{jjj}^{V1,LR} + \frac{32}{27} L_{iii}^{V,LL} \right. \\
& + \frac{8}{9} L_{ijj}^{V,LL} + \frac{8}{27} L_{ijji}^{V,LL} + \frac{64}{27} L_{jjjj}^{V,RR} + \frac{4}{9} L_{ii11}^{V,LR} + \frac{4}{9} L_{ii22}^{V,LR} + \frac{4}{9} L_{ii33}^{V,LR} \\
& - \frac{8}{9} L_{ii11}^{V1,LR} - \frac{8}{9} L_{ii22}^{V1,LR} + \frac{4}{9} L_{11ii}^{V,LL} + \frac{4}{9} L_{22ii}^{V,LL} + \frac{4}{9} L_{33ii}^{V,LL} + \frac{4}{9} L_{11jj}^{V,LR} \\
& \left. + \frac{4}{9} L_{22jj}^{V,LR} + \frac{4}{9} L_{33jj}^{V,LR} + \frac{4}{9} L_{11jj}^{V,RR} + \frac{4}{9} L_{22jj}^{V,RR} + \frac{4}{9} L_{33jj}^{V,RR} - \frac{8}{9} L_{11ii}^{V1,LL} \right]
\end{aligned}$$

$$\begin{aligned}
& -\frac{8}{9}L_{22ii}^{V1,LL} - \frac{8}{9}L_{11jj}^{V1,LR} - \frac{8}{9}L_{22jj}^{V1,LR} - \frac{8}{9}L_{11jj}^{V1,RR} - \frac{8}{9}L_{22jj}^{V1,RR} \Big] + \alpha_s^2 \Big[ 8L_{iii}^{V1,LR} \\
& - \frac{4}{3}L_{ijj}^{V1,LR} + 16L_{jjj}^{V1,LR} + \frac{44}{27}L_{iii}^{V8,LR} - \frac{2000}{27}L_{ijj}^{V8,LR} + \frac{88}{27}L_{jjj}^{V8,LR} - \frac{232}{9}L_{iii}^{V,LL} \\
& - 16L_{ijj}^{V,LL} - \frac{64}{27}L_{ijji}^{V,LL} - \frac{1192}{27}L_{jjjj}^{V,RR} + 8L_{ii11}^{V1,LR} + 8L_{ii22}^{V1,LR} + \frac{44}{27}L_{ii11}^{V8,LR} \\
& + \frac{44}{27}L_{ii22}^{V8,LR} - 8L_{11ii}^{V1,LL} - 8L_{22ii}^{V1,LL} + 8L_{11jj}^{V1,LR} + 8L_{22jj}^{V1,LR} - 8L_{11jj}^{V1,RR} \\
& - 8L_{22jj}^{V1,RR} + \frac{44}{27}L_{11ii}^{V8,LL} + \frac{44}{27}L_{22ii}^{V8,LL} + \frac{44}{27}L_{11jj}^{V8,LR} + \frac{44}{27}L_{22jj}^{V8,LR} + \frac{44}{27}L_{11jj}^{V8,RR} \\
& + \frac{44}{27}L_{22jj}^{V8,RR} \Big] + \alpha_s \alpha \Big[ \frac{16}{9}L_{iii}^{V1,LR} + \frac{112}{9}L_{ijj}^{V1,LR} + \frac{32}{9}L_{jjjj}^{V1,LR} - \frac{1022}{729}L_{iii}^{V8,LR} \\
& - \frac{1238}{729}L_{ijj}^{V8,LR} - \frac{2044}{729}L_{jjj}^{V8,LR} + \frac{1048}{243}L_{iii}^{V,LL} + \frac{8}{3}L_{ijj}^{V,LL} + \frac{64}{729}L_{ijji}^{V,LL} + \frac{5152}{729}L_{jjjj}^{V,RR} \\
& - \frac{32}{9}L_{ii11}^{V1,LR} - \frac{32}{9}L_{ii22}^{V1,LR} + \frac{1354}{729}L_{ii11}^{V8,LR} + \frac{1354}{729}L_{ii22}^{V8,LR} - \frac{32}{9}L_{11ii}^{V1,LL} - \frac{32}{9}L_{22ii}^{V1,LL} \\
& - \frac{32}{9}L_{11jj}^{V1,LR} - \frac{32}{9}L_{22jj}^{V1,LR} - \frac{32}{9}L_{11jj}^{V1,RR} - \frac{32}{9}L_{22jj}^{V1,RR} - \frac{86}{729}L_{ii11}^{V8,LL} - \frac{86}{729}L_{ii22}^{V8,LL} \\
& + \frac{1354}{729}L_{11jj}^{V8,LR} + \frac{1354}{729}L_{22jj}^{V8,LR} - \frac{86}{729}L_{11jj}^{V8,RR} - \frac{86}{729}L_{22jj}^{V8,RR} \Big] + \alpha^2 \Big[ \frac{272}{729}L_{iii}^{V1,LR} \\
& + \frac{15590}{729}L_{ijj}^{V1,LR} + \frac{544}{729}L_{jjj}^{V1,LR} - \frac{656}{729}L_{iii}^{V,LL} - \frac{32}{729}L_{ijj}^{V,LL} - \frac{848}{2187}L_{ijji}^{V,LL} \\
& - \frac{2912}{2187}L_{jjjj}^{V,RR} + \frac{992}{729}L_{ii11}^{V,LR} + \frac{992}{729}L_{ii22}^{V,LR} + \frac{992}{729}L_{ii33}^{V,LR} - \frac{1624}{729}L_{ii11}^{V1,LR} \\
& - \frac{1624}{729}L_{ii22}^{V1,LR} + \frac{128}{729}L_{11ii}^{V,LL} + \frac{128}{729}L_{22ii}^{V,LL} + \frac{128}{729}L_{33ii}^{V,LL} + \frac{992}{729}L_{11jj}^{V,LR} \\
& + \frac{992}{729}L_{22jj}^{V,LR} + \frac{992}{729}L_{33jj}^{V,LR} + \frac{128}{729}L_{11jj}^{V,RR} + \frac{128}{729}L_{22jj}^{V,RR} + \frac{128}{729}L_{33jj}^{V,RR} - \frac{2776}{729}L_{11ii}^{V1,LL} \\
& - \frac{2776}{729}L_{22ii}^{V1,LL} - \frac{1624}{729}L_{11jj}^{V1,LR} - \frac{1624}{729}L_{22jj}^{V1,LR} - \frac{2776}{729}L_{11jj}^{V1,RR} - \frac{2776}{729}L_{22jj}^{V1,RR} \Big] ;
\end{aligned}$$

$$\begin{aligned}
\dot{L}_{ijj}^{V8,LR} &= g_s^2 \Big[ -12L_{ijj}^{V1,LR} - \frac{40}{3}L_{ijj}^{V8,LR} + \frac{8}{3}L_{ijji}^{V,LL} + \frac{2}{3}L_{iii}^{V8,LR} + \frac{8}{3}L_{iii}^{V,LL} \\
& + \frac{2}{3}L_{ii11}^{V8,LR} + \frac{2}{3}L_{ii22}^{V8,LR} + \frac{2}{3}L_{11ii}^{V8,LL} + \frac{2}{3}L_{22ii}^{V8,LL} + \frac{4}{3}L_{jjjj}^{V8,LR} + \frac{16}{3}L_{jjjj}^{V,RR} \Big]
\end{aligned}$$

$$\begin{aligned}
& + \frac{2}{3} L_{11jj}^{V8,LR} + \frac{2}{3} L_{22jj}^{V8,LR} + \frac{2}{3} L_{11jj}^{V8,RR} + \frac{2}{3} L_{22jj}^{V8,RR} \Big] - \frac{4}{3} e^2 L_{ijj}^{V8,LR} + \alpha_s^2 \Big[ - 132 L_{ijj}^{V1,LR} \\
& - \frac{25201}{162} L_{ijj}^{V8,LR} - \frac{28}{3} L_{ijj}^{V,LL} + \frac{3448}{81} L_{ijj}^{V,LL} - \frac{22}{3} L_{iii}^{V1,LR} + \frac{787}{81} L_{iii}^{V8,LR} + \frac{1198}{27} L_{iii}^{V,LL} \\
& - \frac{22}{3} L_{du}^{V1,LR} - \frac{22}{3} L_{du}^{V1,LR} + \frac{787}{81} L_{du}^{V8,LR} + \frac{787}{81} L_{du}^{V8,LR} - \frac{2}{3} L_{11ii}^{V1,LL} - \frac{2}{3} L_{22ii}^{V1,LL} \\
& + \frac{607}{81} L_{11ii}^{V8,LL} + \frac{607}{81} L_{22ii}^{V8,LL} - \frac{44}{3} L_{jjj}^{V1,LR} + \frac{1574}{81} L_{jjj}^{V8,LR} + \frac{6286}{81} L_{jjj}^{V,RR} - \frac{22}{3} L_{11jj}^{V1,LR} \\
& - \frac{22}{3} L_{22jj}^{V1,LR} - \frac{2}{3} L_{11jj}^{V1,RR} - \frac{2}{3} L_{22jj}^{V1,RR} + \frac{787}{81} L_{11jj}^{V8,LR} + \frac{787}{81} L_{22jj}^{V8,LR} + \frac{607}{81} L_{11jj}^{V8,RR} \\
& + \frac{607}{81} L_{22jj}^{V8,RR} \Big] + \alpha_s \alpha \Big[ \frac{164}{81} L_{ijj}^{V1,LR} - \frac{4}{3} L_{ijj}^{V8,LR} + \frac{544}{81} L_{ijj}^{V,LL} - \frac{1064}{243} L_{ijj}^{V,LL} \\
& + \frac{272}{81} L_{iii}^{V1,LR} + \frac{14}{9} L_{iii}^{V8,LR} + \frac{340}{81} L_{iii}^{V,LL} + \frac{272}{81} L_{de}^{V,LR} + \frac{272}{81} L_{de}^{V,LR} + \frac{272}{81} L_{de}^{V,LR} \\
& - \frac{544}{81} L_{du}^{V1,LR} - \frac{544}{81} L_{du}^{V1,LR} + \frac{2}{3} L_{du}^{V8,LR} + \frac{2}{3} L_{du}^{V8,LR} + \frac{272}{81} L_{11ii}^{V,LL} + \frac{272}{81} L_{22ii}^{V,LL} \\
& + \frac{272}{81} L_{33ii}^{V,LL} - \frac{544}{81} L_{11ii}^{V1,LL} - \frac{544}{81} L_{22ii}^{V1,LL} + \frac{122}{27} L_{11ii}^{V8,LL} + \frac{122}{27} L_{22ii}^{V8,LL} + \frac{544}{81} L_{jjj}^{V1,LR} \\
& + \frac{28}{9} L_{jjj}^{V8,LR} + \frac{1588}{243} L_{jjj}^{V,RR} + \frac{272}{81} L_{11jj}^{V,LR} + \frac{272}{81} L_{22jj}^{V,LR} + \frac{272}{81} L_{33jj}^{V,LR} + \frac{272}{81} L_{11jj}^{V,RR} \\
& + \frac{272}{81} L_{22jj}^{V,RR} + \frac{272}{81} L_{33jj}^{V,RR} - \frac{544}{81} L_{11jj}^{V1,LR} - \frac{544}{81} L_{22jj}^{V1,LR} - \frac{544}{81} L_{11jj}^{V1,RR} - \frac{544}{81} L_{22jj}^{V1,RR} \\
& + \frac{2}{3} L_{11jj}^{V8,LR} + \frac{2}{3} L_{22jj}^{V8,LR} + \frac{122}{27} L_{11jj}^{V8,RR} + \frac{122}{27} L_{22jj}^{V8,RR} \Big] + \frac{1702}{81} \alpha^2 L_{ijj}^{V8,LR} ;
\end{aligned}$$

$$\begin{aligned}
\dot{L}_{iii}^{V1,LR} = & - \frac{8}{3} L_{iii}^{V8,LR} g_s^2 + e^2 \Big[ - \frac{4}{9} L_{iii}^{V1,LR} + \frac{4}{9} L_{ijj}^{V1,LR} + \frac{4}{9} L_{jji}^{V1,LR} + \frac{32}{27} L_{iii}^{V,LL} \\
& + \frac{8}{9} L_{ijj}^{V,LL} + \frac{8}{27} L_{ijj}^{V,LL} + \frac{32}{27} L_{iii}^{V,RR} + \frac{8}{9} L_{ijj}^{V,RR} + \frac{8}{27} L_{ijj}^{V,RR} + \frac{4}{9} L_{de}^{V,LR} \\
& + \frac{4}{9} L_{de}^{V,LR} + \frac{4}{9} L_{de}^{V,LR} - \frac{8}{9} L_{du}^{V1,LR} - \frac{8}{9} L_{du}^{V1,LR} + \frac{4}{9} L_{11ii}^{V,LL} + \frac{4}{9} L_{22ii}^{V,LL} \\
& + \frac{4}{9} L_{33ii}^{V,LL} + \frac{4}{9} L_{11ii}^{V,LR} + \frac{4}{9} L_{22ii}^{V,LR} + \frac{4}{9} L_{33ii}^{V,LR} + \frac{4}{9} L_{11ii}^{V,RR} + \frac{4}{9} L_{22ii}^{V,RR} \\
& + \frac{4}{9} L_{33ii}^{V,RR} - \frac{8}{9} L_{11ii}^{V1,LL} - \frac{8}{9} L_{22ii}^{V1,LL} - \frac{8}{9} L_{11ii}^{V1,LR} - \frac{8}{9} L_{22ii}^{V1,LR} - \frac{8}{9} L_{11ii}^{V1,RR}
\end{aligned}$$

$$\begin{aligned}
& -\frac{8}{9}L_{22ii}^{V1,RR} \Big] + \alpha_s^2 \Big[ \frac{20}{3}L_{iii}^{V1,LR} + 8L_{ijj}^{V1,LR} + 8L_{jji}^{V1,LR} - \frac{652}{9}L_{iii}^{V8,LR} \\
& + \frac{44}{27}L_{ijj}^{V8,LR} + \frac{44}{27}L_{jji}^{V8,LR} - \frac{232}{9}L_{iii}^{V,LL} - 16L_{ijj}^{V,LL} - \frac{64}{27}L_{jji}^{V,LL} - \frac{232}{9}L_{iii}^{V,RR} \\
& - 16L_{ijj}^{V,RR} - \frac{64}{27}L_{jji}^{V,RR} + 8L_{ii1}^{V1,LR} + 8L_{ii2}^{V1,LR} + \frac{44}{27}L_{ii1}^{V8,LR} + \frac{44}{27}L_{ii2}^{V8,LR} \\
& - 8L_{11ii}^{V1,LL} - 8L_{22ii}^{V1,LL} + 8L_{11ii}^{V1,LR} + 8L_{22ii}^{V1,LR} - 8L_{11ii}^{V1,RR} - 8L_{22ii}^{V1,RR} \\
& + \frac{44}{27}L_{11ii}^{V8,LL} + \frac{44}{27}L_{22ii}^{V8,LL} + \frac{44}{27}L_{11ii}^{V8,LR} + \frac{44}{27}L_{22ii}^{V8,LR} + \frac{44}{27}L_{11ii}^{V8,RR} + \frac{44}{27}L_{22ii}^{V8,RR} \Big] \\
& + \alpha_s \alpha \Big[ \frac{128}{9}L_{iii}^{V1,LR} + \frac{16}{9}L_{ijj}^{V1,LR} + \frac{16}{9}L_{jji}^{V1,LR} - \frac{2260}{729}L_{iii}^{V8,LR} - \frac{1022}{729}L_{ijj}^{V8,LR} \\
& - \frac{1022}{729}L_{jji}^{V8,LR} + \frac{1048}{243}L_{iii}^{V,LL} + \frac{8}{3}L_{ijj}^{V,LL} + \frac{64}{729}L_{jji}^{V,LL} + \frac{1048}{243}L_{iii}^{V,RR} + \frac{8}{3}L_{ijj}^{V,RR} \\
& + \frac{64}{729}L_{jji}^{V,RR} - \frac{32}{9}L_{ii1}^{V1,LR} - \frac{32}{9}L_{ii2}^{V1,LR} + \frac{1354}{729}L_{ii1}^{V8,LR} + \frac{1354}{729}L_{ii2}^{V8,LR} - \frac{32}{9}L_{11ii}^{V1,LL} \\
& - \frac{32}{9}L_{22ii}^{V1,LL} - \frac{32}{9}L_{11ii}^{V1,LR} - \frac{32}{9}L_{22ii}^{V1,LR} - \frac{32}{9}L_{11ii}^{V1,RR} - \frac{32}{9}L_{22ii}^{V1,RR} - \frac{86}{729}L_{11ii}^{V8,LL} \\
& - \frac{86}{729}L_{22ii}^{V8,LL} + \frac{1354}{729}L_{11ii}^{V8,LR} + \frac{1354}{729}L_{22ii}^{V8,LR} - \frac{86}{729}L_{11ii}^{V8,RR} - \frac{86}{729}L_{22ii}^{V8,RR} \Big] \\
& + \alpha^2 \Big[ \frac{15862}{729}L_{iii}^{V1,LR} + \frac{272}{729}L_{ijj}^{V1,LR} + \frac{272}{729}L_{jji}^{V1,LR} - \frac{656}{729}L_{iii}^{V,LL} - \frac{32}{729}L_{ijj}^{V,LL} \\
& - \frac{848}{2187}L_{jji}^{V,LL} - \frac{656}{729}L_{iii}^{V,RR} - \frac{32}{729}L_{ijj}^{V,RR} - \frac{848}{2187}L_{jji}^{V,RR} + \frac{992}{729}L_{ii1}^{V,LR} \\
& + \frac{992}{729}L_{ii2}^{V,LR} + \frac{992}{729}L_{ii3}^{V,LR} - \frac{1624}{729}L_{ii1}^{V1,LR} - \frac{1624}{729}L_{ii2}^{V1,LR} + \frac{128}{729}L_{11ii}^{V,LL} \\
& + \frac{128}{729}L_{22ii}^{V,LL} + \frac{128}{729}L_{33ii}^{V,LL} + \frac{992}{729}L_{11ii}^{V,LR} + \frac{992}{729}L_{22ii}^{V,LR} + \frac{992}{729}L_{33ii}^{V,LR} + \frac{128}{729}L_{11ii}^{V,RR} \\
& + \frac{128}{729}L_{22ii}^{V,RR} + \frac{128}{729}L_{33ii}^{V,RR} - \frac{2776}{729}L_{11ii}^{V1,LL} - \frac{2776}{729}L_{22ii}^{V1,LL} - \frac{1624}{729}L_{11ii}^{V1,LR} \\
& - \frac{1624}{729}L_{22ii}^{V1,LR} - \frac{2776}{729}L_{11ii}^{V1,RR} - \frac{2776}{729}L_{22ii}^{V1,RR} \Big] ;
\end{aligned}$$

$$\begin{aligned}
\dot{L}_{dd\bar{iii}}^{V8,LR} = & g_s^2 \left[ \frac{2}{3} L_{ij\bar{j}}^{V8,LR} + \frac{2}{3} L_{jj\bar{i}}^{V8,LR} + \frac{8}{3} L_{ij\bar{j}}^{V,LL} + \frac{8}{3} L_{ij\bar{j}}^{V,RR} - 12 L_{iii}^{V1,LR} \right. \\
& - \frac{38}{3} L_{iii}^{V8,LR} + \frac{8}{3} L_{iii}^{V,LL} + \frac{8}{3} L_{iii}^{V,RR} + \frac{2}{3} L_{ii1}^{V8,LR} + \frac{2}{3} L_{ii2}^{V8,LR} + \frac{2}{3} L_{11i}^{V8,LL} \\
& + \frac{2}{3} L_{22i}^{V8,LL} + \frac{2}{3} L_{11i}^{V8,LR} + \frac{2}{3} L_{22i}^{V8,LR} + \frac{2}{3} L_{11i}^{V8,RR} + \left. \frac{2}{3} L_{22i}^{V8,RR} \right] - \frac{4}{3} e^2 L_{iii}^{V8,LR} \\
& + \alpha_s^2 \left[ -\frac{22}{3} L_{ij\bar{j}}^{V1,LR} - \frac{22}{3} L_{jj\bar{i}}^{V1,LR} + \frac{787}{81} L_{ij\bar{j}}^{V8,LR} + \frac{787}{81} L_{jj\bar{i}}^{V8,LR} - \frac{28}{3} L_{ij\bar{j}}^{V,LL} \right. \\
& + \frac{3448}{81} L_{ij\bar{j}}^{V,LL} - \frac{28}{3} L_{ij\bar{j}}^{V,RR} + \frac{3448}{81} L_{ij\bar{j}}^{V,RR} - \frac{418}{3} L_{iii}^{V1,LR} - \frac{23627}{162} L_{iii}^{V8,LR} + \frac{1198}{27} L_{iii}^{V,LL} \\
& + \frac{1198}{27} L_{iii}^{V,RR} - \frac{22}{3} L_{ii1}^{V1,LR} - \frac{22}{3} L_{ii2}^{V1,LR} + \frac{787}{81} L_{ii1}^{V8,LR} + \frac{787}{81} L_{ii2}^{V8,LR} - \frac{2}{3} L_{11i}^{V1,LL} \\
& - \frac{2}{3} L_{22i}^{V1,LL} - \frac{22}{3} L_{11i}^{V1,LR} - \frac{22}{3} L_{22i}^{V1,LR} - \frac{2}{3} L_{11i}^{V1,RR} - \frac{2}{3} L_{22i}^{V1,RR} + \frac{607}{81} L_{11i}^{V8,LL} \\
& + \left. \frac{607}{81} L_{22i}^{V8,LL} + \frac{787}{81} L_{11i}^{V8,LR} + \frac{787}{81} L_{22i}^{V8,LR} + \frac{607}{81} L_{11i}^{V8,RR} + \frac{607}{81} L_{22i}^{V8,RR} \right] \\
& + \alpha_s \alpha \left[ \frac{272}{81} L_{ij\bar{j}}^{V1,LR} + \frac{272}{81} L_{jj\bar{i}}^{V1,LR} + \frac{14}{9} L_{ij\bar{j}}^{V8,LR} + \frac{14}{9} L_{jj\bar{i}}^{V8,LR} + \frac{544}{81} L_{ij\bar{j}}^{V,LL} \right. \\
& - \frac{1064}{243} L_{ij\bar{j}}^{V,LL} + \frac{544}{81} L_{ij\bar{j}}^{V,RR} - \frac{1064}{243} L_{ij\bar{j}}^{V,RR} + \frac{436}{81} L_{iii}^{V1,LR} + \frac{2}{9} L_{iii}^{V8,LR} + \frac{340}{81} L_{iii}^{V,LL} \\
& + \frac{340}{81} L_{iii}^{V,RR} + \frac{272}{81} L_{ii1}^{V,LR} + \frac{272}{81} L_{ii2}^{V,LR} + \frac{272}{81} L_{ii3}^{V,LR} - \frac{544}{81} L_{ii1}^{V1,LR} - \frac{544}{81} L_{ii2}^{V1,LR} \\
& + \frac{2}{3} L_{ii1}^{V8,LR} + \frac{2}{3} L_{ii2}^{V8,LR} + \frac{272}{81} L_{11i}^{V,LL} + \frac{272}{81} L_{22i}^{V,LL} + \frac{272}{81} L_{33i}^{V,LL} + \frac{272}{81} L_{11i}^{V,LR} \\
& + \frac{272}{81} L_{22i}^{V,LR} + \frac{272}{81} L_{33i}^{V,LR} + \frac{272}{81} L_{11i}^{V,RR} + \frac{272}{81} L_{22i}^{V,RR} + \frac{272}{81} L_{33i}^{V,RR} - \frac{544}{81} L_{11i}^{V1,LL} \\
& - \frac{544}{81} L_{22i}^{V1,LL} - \frac{544}{81} L_{11i}^{V1,LR} - \frac{544}{81} L_{22i}^{V1,LR} - \frac{544}{81} L_{11i}^{V1,RR} - \frac{544}{81} L_{22i}^{V1,RR} + \frac{122}{27} L_{11i}^{V8,LL} \\
& + \left. \frac{122}{27} L_{22i}^{V8,LL} + \frac{2}{3} L_{11i}^{V8,LR} + \frac{2}{3} L_{22i}^{V8,LR} + \frac{122}{27} L_{11i}^{V8,RR} + \frac{122}{27} L_{22i}^{V8,RR} \right] \\
& + \frac{1702}{81} \alpha^2 L_{iii}^{V8,LR} ;
\end{aligned}$$



$$\begin{aligned}
\dot{L}_{uu,ijj}^{V1,LR} = & -\frac{8}{3}L_{uu,ijj}^{V8,LR}g_s^2 + e^2 \left[ -\frac{8}{9}L_{du,11jj}^{V1,LR} - \frac{8}{9}L_{du,22jj}^{V1,LR} - \frac{8}{9}L_{eu,11ii}^{V,LL} - \frac{8}{9}L_{eu,22ii}^{V,LL} \right. \\
& - \frac{8}{9}L_{eu,33ii}^{V,LL} - \frac{8}{9}L_{eu,11jj}^{V,LR} - \frac{8}{9}L_{eu,22jj}^{V,LR} - \frac{8}{9}L_{eu,33jj}^{V,LR} - \frac{8}{9}L_{eu,11jj}^{V,RR} - \frac{8}{9}L_{eu,22jj}^{V,RR} \\
& - \frac{8}{9}L_{eu,33jj}^{V,RR} - \frac{8}{9}L_{ud,ii11}^{V1,LL} - \frac{8}{9}L_{ud,ii22}^{V1,LL} - \frac{8}{9}L_{ud,ii11}^{V1,LR} - \frac{8}{9}L_{ud,ii22}^{V1,LR} - \frac{8}{9}L_{ud,ii11}^{V1,RR} \\
& - \frac{8}{9}L_{ud,jj22}^{V1,RR} - \frac{8}{9}L_{ue,ii11}^{V,LR} - \frac{8}{9}L_{ue,ii22}^{V,LR} - \frac{8}{9}L_{ue,ii33}^{V,LR} + \frac{16}{9}L_{uu,iii}^{V1,LR} - \frac{16}{3}L_{uu,ijj}^{V1,LR} \\
& + \frac{16}{9}L_{uu,ikk}^{V1,LR} + \frac{16}{9}L_{uu,jjj}^{V1,LR} + \frac{16}{9}L_{kkjj}^{V1,LR} + \frac{128}{27}L_{uu,iii}^{V,LL} + \frac{32}{9}L_{uu,ikk}^{V,LL} + \frac{32}{27}L_{uu,ikk}^{V,LL} \\
& + \frac{128}{27}L_{uu,jjjj}^{V,RR} + \frac{32}{9}L_{jjkk}^{V,RR} + \frac{32}{27}L_{jjkk}^{V,RR} \left. \right] + \alpha_s^2 \left[ 8L_{du,11jj}^{V1,LR} + 8L_{du,22jj}^{V1,LR} \right. \\
& + \frac{44}{27}L_{du,11jj}^{V8,LR} + \frac{44}{27}L_{du,22jj}^{V8,LR} - 8L_{ud,ii11}^{V1,LL} - 8L_{ud,ii22}^{V1,LL} + 8L_{ud,ii11}^{V1,LR} + 8L_{ud,ii22}^{V1,LR} \\
& - 8L_{ud,jj11}^{V1,RR} - 8L_{ud,jj22}^{V1,RR} + \frac{44}{27}L_{ud,ii11}^{V8,LL} + \frac{44}{27}L_{ud,ii22}^{V8,LL} + \frac{44}{27}L_{ud,ii11}^{V8,LR} + \frac{44}{27}L_{ud,ii22}^{V8,LR} \\
& + \frac{44}{27}L_{ud,jj11}^{V8,RR} + \frac{44}{27}L_{ud,jj22}^{V8,RR} + 8L_{uu,iii}^{V1,LR} - \frac{28}{3}L_{uu,ijj}^{V1,LR} + 8L_{uu,ikk}^{V1,LR} + 8L_{uu,jjj}^{V1,LR} \\
& + 8L_{kkjj}^{V1,LR} + \frac{44}{27}L_{uu,iii}^{V8,LR} - \frac{2044}{27}L_{uu,ijj}^{V8,LR} + \frac{44}{27}L_{uu,ikk}^{V8,LR} + \frac{44}{27}L_{uu,jjj}^{V8,LR} + \frac{44}{27}L_{kkjj}^{V8,LR} \\
& - \frac{232}{9}L_{uu,iii}^{V,LL} - 16L_{uu,ikk}^{V,LL} - \frac{64}{27}L_{uu,ikk}^{V,LL} - \frac{232}{9}L_{uu,jjj}^{V,RR} - 16L_{uu,jjkk}^{V,RR} - \frac{64}{27}L_{uu,jjkk}^{V,RR} \left. \right] \\
& + \alpha_s \alpha \left[ -\frac{32}{9}L_{du,11jj}^{V1,LR} + \frac{64}{9}L_{du,22jj}^{V1,LR} + \frac{664}{729}L_{du,11jj}^{V8,LR} - \frac{4088}{729}L_{du,22jj}^{V8,LR} - \frac{32}{9}L_{ud,ii11}^{V1,LL} \right. \\
& - \frac{32}{9}L_{ud,ii22}^{V1,LL} - \frac{32}{9}L_{ud,ii11}^{V1,LR} + \frac{64}{9}L_{ud,ii22}^{V1,LR} - \frac{32}{9}L_{ud,jj11}^{V1,RR} - \frac{32}{9}L_{ud,jj22}^{V1,RR} - \frac{776}{729}L_{ud,ii11}^{V8,LL} \\
& - \frac{776}{729}L_{ud,ii22}^{V8,LL} + \frac{664}{729}L_{ud,ii11}^{V8,LR} - \frac{4088}{729}L_{ud,ii22}^{V8,LR} - \frac{776}{729}L_{ud,jj11}^{V8,RR} - \frac{776}{729}L_{ud,jj22}^{V8,RR} \\
& + \frac{64}{9}L_{uu,iii}^{V1,LR} + \frac{128}{3}L_{uu,ijj}^{V1,LR} + \frac{64}{9}L_{uu,ikk}^{V1,LR} + \frac{64}{9}L_{uu,jjj}^{V1,LR} + \frac{64}{9}L_{kkjj}^{V1,LR} - \frac{4088}{729}L_{uu,iii}^{V8,LR} \\
& - \frac{32}{27}L_{uu,ijj}^{V8,LR} - \frac{4088}{729}L_{uu,ikk}^{V8,LR} - \frac{4088}{729}L_{uu,jjj}^{V8,LR} - \frac{4088}{729}L_{kkjj}^{V8,LR} + \frac{4192}{243}L_{uu,iii}^{V,LL} \\
& \left. + \frac{32}{3}L_{uu,ikk}^{V,LL} + \frac{256}{729}L_{uu,ikk}^{V,LL} + \frac{4192}{243}L_{uu,jjj}^{V,RR} + \frac{32}{3}L_{jjkk}^{V,RR} + \frac{256}{729}L_{jjkk}^{V,RR} \right]
\end{aligned}$$

$$\begin{aligned}
& + \alpha^2 \left[ -\frac{2392}{729} L_{11jj}^{V1,LR} + \frac{3776}{729} L_{22jj}^{V1,LR} - \frac{8152}{729} L_{11ii}^{V,LL} - \frac{8152}{729} L_{22ii}^{V,LL} - \frac{8152}{729} L_{33ii}^{V,LL} \right. \\
& - \frac{4696}{729} L_{11jj}^{V,LR} - \frac{4696}{729} L_{22jj}^{V,LR} - \frac{4696}{729} L_{33jj}^{V,LR} - \frac{8152}{729} L_{11jj}^{V,RR} - \frac{8152}{729} L_{22jj}^{V,RR} \\
& - \frac{8152}{729} L_{33jj}^{V,RR} - \frac{3544}{729} L_{ud11}^{V1,LL} - \frac{3544}{729} L_{ud22}^{V1,LL} - \frac{2392}{729} L_{ud11}^{V1,LR} + \frac{3776}{729} L_{ud22}^{V1,LR} \\
& - \frac{3544}{729} L_{jj11}^{V1,RR} - \frac{3544}{729} L_{jj22}^{V1,RR} - \frac{4696}{729} L_{ii11}^{V,LR} - \frac{4696}{729} L_{ii22}^{V,LR} - \frac{4696}{729} L_{ii33}^{V,LR} \\
& + \frac{4352}{729} L_{iii}^{V1,LR} + \frac{7168}{81} L_{iijj}^{V1,LR} + \frac{4352}{729} L_{ikk}^{V1,LR} + \frac{4352}{729} L_{jjjj}^{V1,LR} + \frac{4352}{729} L_{kkjj}^{V1,LR} \\
& - \frac{10496}{729} L_{iii}^{V,LL} - \frac{512}{729} L_{ikk}^{V,LL} - \frac{13568}{2187} L_{ikki}^{V,LL} - \frac{10496}{729} L_{jjjj}^{V,RR} - \frac{512}{729} L_{jjkk}^{V,RR} \\
& \left. - \frac{13568}{2187} L_{jjkk}^{V,RR} \right];
\end{aligned}$$

$$\begin{aligned}
\dot{L}_{iijj}^{V8,LR} & = g_s^2 \left[ \frac{2}{3} L_{11jj}^{V8,LR} + \frac{2}{3} L_{22jj}^{V8,LR} + \frac{2}{3} L_{ud11}^{V8,LL} + \frac{2}{3} L_{ud22}^{V8,LL} + \frac{2}{3} L_{ii11}^{V8,LR} \right. \\
& + \frac{2}{3} L_{ii22}^{V8,LR} + \frac{2}{3} L_{jj11}^{V8,RR} + \frac{2}{3} L_{jj22}^{V8,RR} - 12 L_{iijj}^{V1,LR} + \frac{2}{3} L_{iii}^{V8,LR} - 14 L_{iijj}^{V8,LR} \\
& + \frac{2}{3} L_{ikk}^{V8,LR} + \frac{2}{3} L_{jjjj}^{V8,LR} + \frac{2}{3} L_{kkjj}^{V8,LR} + \frac{8}{3} L_{iii}^{V,LL} + \frac{8}{3} L_{ikki}^{V,LL} + \frac{8}{3} L_{jjjj}^{V,RR} \\
& \left. + \frac{8}{3} L_{jjkk}^{V,RR} \right] - \frac{16}{3} L_{iijj}^{V8,LR} e^2 + \alpha_s^2 \left[ -\frac{22}{3} L_{11jj}^{V1,LR} - \frac{22}{3} L_{22jj}^{V1,LR} + \frac{787}{81} L_{11jj}^{V8,LR} \right. \\
& + \frac{787}{81} L_{22jj}^{V8,LR} - \frac{2}{3} L_{ud11}^{V1,LL} - \frac{2}{3} L_{ud22}^{V1,LL} - \frac{22}{3} L_{ii11}^{V1,LR} - \frac{22}{3} L_{ii22}^{V1,LR} - \frac{2}{3} L_{jj11}^{V1,RR} \\
& - \frac{2}{3} L_{jj22}^{V1,RR} + \frac{607}{81} L_{ud11}^{V8,LL} + \frac{607}{81} L_{ud22}^{V8,LL} + \frac{787}{81} L_{ii11}^{V8,LR} + \frac{787}{81} L_{ii22}^{V8,LR} + \frac{607}{81} L_{jj11}^{V8,RR} \\
& + \frac{607}{81} L_{jj22}^{V8,RR} - \frac{22}{3} L_{iii}^{V1,LR} - \frac{374}{3} L_{iijj}^{V1,LR} - \frac{22}{3} L_{ikk}^{V1,LR} - \frac{22}{3} L_{jjjj}^{V1,LR} - \frac{22}{3} L_{kkjj}^{V1,LR} \\
& + \frac{787}{81} L_{iii}^{V8,LR} - \frac{2975}{18} L_{iijj}^{V8,LR} + \frac{787}{81} L_{ikk}^{V8,LR} + \frac{787}{81} L_{jjjj}^{V8,LR} + \frac{787}{81} L_{kkjj}^{V8,LR} \\
& \left. + \frac{1198}{27} L_{iii}^{V,LL} - \frac{28}{3} L_{ikk}^{V,LL} + \frac{3448}{81} L_{ikki}^{V,LL} + \frac{1198}{27} L_{jjjj}^{V,RR} - \frac{28}{3} L_{jjkk}^{V,RR} + \frac{3448}{81} L_{jjkk}^{V,RR} \right] \\
& + \alpha_s \alpha \left[ -\frac{544}{81} L_{11jj}^{V1,LR} + \frac{1160}{81} L_{22jj}^{V1,LR} + \frac{22}{9} L_{11jj}^{V8,LR} + \frac{56}{9} L_{22jj}^{V8,LR} - \frac{544}{81} L_{11ii}^{V,LL} \right.
\end{aligned}$$

$$\begin{aligned}
& -\frac{544}{81}L_{22ii}^{V,LL} - \frac{544}{81}L_{33ii}^{V,LL} - \frac{544}{81}L_{11jj}^{V,LR} - \frac{544}{81}L_{22jj}^{V,LR} - \frac{544}{81}L_{33jj}^{V,LR} - \frac{544}{81}L_{11jj}^{V,RR} \\
& - \frac{544}{81}L_{22jj}^{V,RR} - \frac{544}{81}L_{33jj}^{V,RR} - \frac{544}{81}L_{ii11}^{V1,LL} - \frac{544}{81}L_{ii22}^{V1,LL} - \frac{544}{81}L_{ii11}^{V1,LR} + \frac{1160}{81}L_{ii22}^{V1,LR} \\
& - \frac{544}{81}L_{jj11}^{V1,RR} - \frac{544}{81}L_{jj22}^{V1,RR} + \frac{170}{27}L_{ii11}^{V8,LL} + \frac{170}{27}L_{ii22}^{V8,LL} + \frac{22}{9}L_{ii11}^{V8,LR} + \frac{56}{9}L_{ii22}^{V8,LR} \\
& + \frac{170}{27}L_{jj11}^{V8,RR} + \frac{170}{27}L_{jj22}^{V8,RR} - \frac{544}{81}L_{ii11}^{V,LR} - \frac{544}{81}L_{ii22}^{V,LR} - \frac{544}{81}L_{ii33}^{V,LR} + \frac{1088}{81}L_{iii}^{V1,LR} \\
& - \frac{16}{3}L_{ijj}^{V1,LR} + \frac{1088}{81}L_{iikk}^{V1,LR} + \frac{1088}{81}L_{jjj}^{V1,LR} + \frac{1088}{81}L_{kkjj}^{V1,LR} + \frac{56}{9}L_{iii}^{V8,LR} - \frac{104}{9}L_{ijj}^{V8,LR} \\
& + \frac{56}{9}L_{iikk}^{V8,LR} + \frac{56}{9}L_{jjjj}^{V8,LR} + \frac{56}{9}L_{kkjj}^{V8,LR} + \frac{1360}{81}L_{iii}^{V,LL} + \frac{2176}{81}L_{iikk}^{V,LL} - \frac{4256}{243}L_{ikki}^{V,LL} \\
& + \frac{1360}{81}L_{jjjj}^{V,RR} + \frac{2176}{81}L_{jjkk}^{V,RR} - \frac{4256}{243}L_{jjkk}^{V,RR} \Big] + \frac{7168}{81}L_{ijj}^{V8,LR}\alpha^2 ;
\end{aligned}$$

$$\begin{aligned}
\dot{L}_{uu}^{V1,LR} &= -\frac{8}{3}L_{iii}^{V8,LR}g_s^2 + e^2 \Bigg[ -\frac{8}{9}L_{11ii}^{V1,LR} - \frac{8}{9}L_{22ii}^{V1,LR} - \frac{8}{9}L_{11ii}^{V,LL} - \frac{8}{9}L_{22ii}^{V,LL} \\
& - \frac{8}{9}L_{33ii}^{V,LL} - \frac{8}{9}L_{11ii}^{V,LR} - \frac{8}{9}L_{22ii}^{V,LR} - \frac{8}{9}L_{33ii}^{V,LR} - \frac{8}{9}L_{22ii}^{V,RR} - \frac{8}{9}L_{33ii}^{V,RR} \\
& - \frac{8}{9}L_{33ii}^{V,RR} - \frac{8}{9}L_{ii11}^{V1,LL} - \frac{8}{9}L_{ii22}^{V1,LL} - \frac{8}{9}L_{ii11}^{V1,LR} - \frac{8}{9}L_{ii22}^{V1,LR} - \frac{8}{9}L_{ii11}^{V1,RR} \\
& - \frac{8}{9}L_{ii22}^{V1,RR} - \frac{8}{9}L_{ii11}^{V,LR} - \frac{8}{9}L_{ii22}^{V,LR} - \frac{8}{9}L_{ii33}^{V,LR} - \frac{16}{9}L_{iii}^{V1,LR} + \frac{16}{9}L_{iikk}^{V1,LR} \\
& + \frac{16}{9}L_{kkii}^{V1,LR} + \frac{128}{27}L_{iii}^{V,LL} + \frac{32}{9}L_{iikk}^{V,LL} + \frac{32}{27}L_{ikki}^{V,LL} + \frac{128}{27}L_{iii}^{V,RR} + \frac{32}{9}L_{iikk}^{V,RR} \\
& + \frac{32}{27}L_{ikki}^{V,RR} \Big] + \alpha_s^2 \Bigg[ 8L_{11ii}^{V1,LR} + 8L_{22ii}^{V1,LR} + \frac{44}{27}L_{11ii}^{V8,LR} + \frac{44}{27}L_{22ii}^{V8,LR} \\
& - 8L_{ii11}^{V1,LL} - 8L_{ii22}^{V1,LL} + 8L_{ii11}^{V1,LR} + 8L_{ii22}^{V1,LR} - 8L_{ii11}^{V1,RR} - 8L_{ii22}^{V1,RR} \\
& + \frac{44}{27}L_{ii11}^{V8,LL} + \frac{44}{27}L_{ii22}^{V8,LL} + \frac{44}{27}L_{ii11}^{V8,LR} + \frac{44}{27}L_{ii22}^{V8,LR} + \frac{44}{27}L_{ii11}^{V8,RR} + \frac{44}{27}L_{ii22}^{V8,RR} \\
& + \frac{20}{3}L_{iii}^{V1,LR} + 8L_{iikk}^{V1,LR} + 8L_{kkii}^{V1,LR} - \frac{652}{9}L_{iii}^{V8,LR} + \frac{44}{27}L_{iikk}^{V8,LR} + \frac{44}{27}L_{kkii}^{V8,LR} \\
& - \frac{232}{9}L_{iii}^{V,LL} - 16L_{iikk}^{V,LL} - \frac{64}{27}L_{ikki}^{V,LL} - \frac{232}{9}L_{iii}^{V,RR} - 16L_{iikk}^{V,RR} - \frac{64}{27}L_{ikki}^{V,RR} \Big]
\end{aligned}$$

$$\begin{aligned}
& + \alpha_s \alpha \left[ -\frac{32}{9} L_{11ii}^{V1,LR} + \frac{64}{9} L_{22ii}^{V1,LR} + \frac{664}{729} L_{11ii}^{V8,LR} - \frac{4088}{729} L_{22ii}^{V8,LR} - \frac{32}{9} L_{ii11}^{V1,LL} \right. \\
& - \frac{32}{9} L_{ii22}^{V1,LL} - \frac{32}{9} L_{ii11}^{V1,LR} + \frac{64}{9} L_{ii22}^{V1,LR} - \frac{32}{9} L_{ii11}^{V1,RR} - \frac{32}{9} L_{ii22}^{V1,RR} - \frac{776}{729} L_{ii11}^{V8,LL} \\
& - \frac{776}{729} L_{ii22}^{V8,LL} + \frac{664}{729} L_{ii11}^{V8,LR} - \frac{4088}{729} L_{ii22}^{V8,LR} - \frac{776}{729} L_{ii11}^{V8,RR} - \frac{776}{729} L_{ii22}^{V8,RR} \\
& + \frac{512}{9} L_{iii}^{V1,LR} + \frac{64}{9} L_{ikk}^{V1,LR} + \frac{64}{9} L_{kkii}^{V1,LR} - \frac{9040}{729} L_{iii}^{V8,LR} - \frac{4088}{729} L_{ikk}^{V8,LR} - \frac{4088}{729} L_{kkii}^{V8,LR} \\
& \left. + \frac{4192}{243} L_{iii}^{V,LL} + \frac{32}{3} L_{ikk}^{V,LL} + \frac{256}{729} L_{ikk}^{V,LL} + \frac{4192}{243} L_{iii}^{V,RR} + \frac{32}{3} L_{ikk}^{V,RR} + \frac{256}{729} L_{ikk}^{V,RR} \right] \\
& + \alpha^2 \left[ -\frac{2392}{729} L_{du}^{V1,LR} + \frac{3776}{729} L_{22ii}^{V1,LR} - \frac{8152}{729} L_{11ii}^{V,LL} - \frac{8152}{729} L_{22ii}^{V,LL} - \frac{8152}{729} L_{33ii}^{V,LL} \right. \\
& - \frac{4696}{729} L_{11ii}^{V,LR} - \frac{4696}{729} L_{22ii}^{V,LR} - \frac{4696}{729} L_{33ii}^{V,LR} - \frac{8152}{729} L_{11ii}^{V,RR} - \frac{8152}{729} L_{22ii}^{V,RR} \\
& - \frac{8152}{729} L_{33ii}^{V,RR} - \frac{3544}{729} L_{ii11}^{V1,LL} - \frac{3544}{729} L_{ii22}^{V1,LL} - \frac{2392}{729} L_{ii11}^{V1,LR} + \frac{3776}{729} L_{ii22}^{V1,LR} \\
& - \frac{3544}{729} L_{ii11}^{V1,RR} - \frac{3544}{729} L_{ii22}^{V1,RR} - \frac{4696}{729} L_{ii11}^{V,LR} - \frac{4696}{729} L_{ii22}^{V,LR} - \frac{4696}{729} L_{ii33}^{V,LR} \\
& + \frac{73216}{729} L_{iii}^{V1,LR} + \frac{4352}{729} L_{ikk}^{V1,LR} + \frac{4352}{729} L_{kkii}^{V1,LR} - \frac{10496}{729} L_{iii}^{V,LL} - \frac{512}{729} L_{ikk}^{V,LL} \\
& \left. - \frac{13568}{2187} L_{ikk}^{V,LL} - \frac{10496}{729} L_{iii}^{V,RR} - \frac{512}{729} L_{ikk}^{V,RR} - \frac{13568}{2187} L_{ikk}^{V,RR} \right];
\end{aligned}$$

$$\begin{aligned}
\dot{L}_{uu}^{V8,LR} & = g_s^2 \left[ \frac{2}{3} L_{ikk}^{V8,LR} + \frac{2}{3} L_{kkii}^{V8,LR} + \frac{8}{3} L_{ikk}^{V,LL} + \frac{8}{3} L_{ikk}^{V,RR} + \frac{2}{3} L_{11ii}^{V8,LR} \right. \\
& + \frac{2}{3} L_{22ii}^{V8,LR} + \frac{2}{3} L_{ii11}^{V8,LL} + \frac{2}{3} L_{ii22}^{V8,LL} + \frac{2}{3} L_{ii11}^{V8,LR} + \frac{2}{3} L_{ii22}^{V8,LR} + \frac{2}{3} L_{ii11}^{V8,RR} \\
& \left. + \frac{2}{3} L_{ii22}^{V8,RR} - 12 L_{iii}^{V1,LR} - \frac{38}{3} L_{iii}^{V8,LR} + \frac{8}{3} L_{iii}^{V,LL} + \frac{8}{3} L_{iii}^{V,RR} \right] - \frac{16}{3} e^2 L_{iii}^{V8,LR} \\
& + \alpha_s^2 \left[ -\frac{22}{3} L_{ikk}^{V1,LR} - \frac{22}{3} L_{kkii}^{V1,LR} + \frac{787}{81} L_{ikk}^{V8,LR} + \frac{787}{81} L_{kkii}^{V8,LR} - \frac{28}{3} L_{ikk}^{V,LL} \right. \\
& + \frac{3448}{81} L_{ikk}^{V,LL} - \frac{28}{3} L_{ikk}^{V,RR} + \frac{3448}{81} L_{ikk}^{V,RR} - \frac{22}{3} L_{11ii}^{V1,LR} - \frac{22}{3} L_{22ii}^{V1,LR} + \frac{787}{81} L_{11ii}^{V8,LR} \\
& \left. + \frac{787}{81} L_{22ii}^{V8,LR} - \frac{2}{3} L_{ii11}^{V1,LL} - \frac{2}{3} L_{ii22}^{V1,LL} - \frac{22}{3} L_{ii11}^{V1,LR} - \frac{22}{3} L_{ii22}^{V1,LR} - \frac{2}{3} L_{ii11}^{V1,RR} \right]
\end{aligned}$$

$$\begin{aligned}
& -\frac{2}{3}L_{ud\ i22}^{V1,RR} + \frac{607}{81}L_{ud\ i11}^{V8,LL} + \frac{607}{81}L_{ud\ i22}^{V8,LL} + \frac{787}{81}L_{ud\ i11}^{V8,LR} + \frac{787}{81}L_{ud\ i22}^{V8,LR} + \frac{607}{81}L_{ud\ i11}^{V8,RR} \\
& + \frac{607}{81}L_{ud\ i22}^{V8,RR} - \frac{418}{3}L_{uu\ iiii}^{V1,LR} - \frac{23627}{162}L_{uu\ iiii}^{V8,LR} + \frac{1198}{27}L_{uu\ iiii}^{V,LL} + \frac{1198}{27}L_{uu\ iiii}^{V,RR} \Big] \\
& + \alpha_s \alpha \left[ \frac{1088}{81}L_{uu\ iikk}^{V1,LR} + \frac{1088}{81}L_{uu\ kkii}^{V1,LR} + \frac{56}{9}L_{uu\ iikk}^{V8,LR} + \frac{56}{9}L_{uu\ kkii}^{V8,LR} + \frac{2176}{81}L_{uu\ iikk}^{V,LL} \right. \\
& - \frac{4256}{243}L_{uu\ iikk}^{V,LL} + \frac{2176}{81}L_{uu\ iikk}^{V,RR} - \frac{4256}{243}L_{uu\ iikk}^{V,RR} - \frac{544}{81}L_{11ii}^{V1,LR} + \frac{1160}{81}L_{22ii}^{V1,LR} \\
& + \frac{22}{9}L_{11ii}^{V8,LR} + \frac{56}{9}L_{22ii}^{V8,LR} - \frac{544}{81}L_{11ii}^{V,LL} - \frac{544}{81}L_{22ii}^{V,LL} - \frac{544}{81}L_{33ii}^{V,LL} - \frac{544}{81}L_{11ii}^{V,LR} \\
& - \frac{544}{81}L_{22ii}^{V,LR} - \frac{544}{81}L_{33ii}^{V,LR} - \frac{544}{81}L_{11ii}^{V,RR} - \frac{544}{81}L_{22ii}^{V,RR} - \frac{544}{81}L_{33ii}^{V,RR} - \frac{544}{81}L_{ud\ i11}^{V1,LL} \\
& - \frac{544}{81}L_{ud\ i22}^{V1,LL} - \frac{544}{81}L_{ud\ i11}^{V1,LR} + \frac{1160}{81}L_{ud\ i22}^{V1,LR} - \frac{544}{81}L_{ud\ i11}^{V1,RR} - \frac{544}{81}L_{ud\ i22}^{V1,RR} \\
& + \frac{170}{27}L_{ud\ i11}^{V8,LL} + \frac{170}{27}L_{ud\ i22}^{V8,LL} + \frac{22}{9}L_{ud\ i11}^{V8,LR} + \frac{56}{9}L_{ud\ i22}^{V8,LR} + \frac{170}{27}L_{ud\ i11}^{V8,RR} + \frac{170}{27}L_{ud\ i22}^{V8,RR} \\
& - \frac{544}{81}L_{ue\ i11}^{V,LR} - \frac{544}{81}L_{ue\ i22}^{V,LR} - \frac{544}{81}L_{ue\ i33}^{V,LR} + \frac{1744}{81}L_{uu\ iiii}^{V1,LR} + \frac{8}{9}L_{uu\ iiii}^{V8,LR} + \frac{1360}{81}L_{uu\ iiii}^{V,LL} \\
& \left. + \frac{1360}{81}L_{uu\ iiii}^{V,RR} \right] + \frac{7168}{81}\alpha^2 L_{uu\ iiii}^{V8,LR} ;
\end{aligned}$$

$$\begin{aligned}
\dot{L}_{ee\ ij}^{V,LR} & = e^2 \left[ \frac{16}{3}L_{ee\ ij}^{V,LL} - \frac{32}{3}L_{ee\ ij}^{V,LR} + \frac{16}{3}L_{ee\ iikk}^{V,LL} + \frac{4}{3}L_{ee\ iikk}^{V,LR} + \frac{4}{3}L_{ed\ i11}^{V,LL} \right. \\
& + \frac{4}{3}L_{ed\ i22}^{V,LL} + \frac{4}{3}L_{ed\ i11}^{V,LR} + \frac{4}{3}L_{ed\ i22}^{V,LR} + \frac{16}{3}L_{ee\ iiii}^{V,LL} + \frac{4}{3}L_{ee\ iiii}^{V,LR} - \frac{8}{3}L_{ed\ i11}^{V,LL} \\
& - \frac{8}{3}L_{ed\ i22}^{V,LL} - \frac{8}{3}L_{ed\ i11}^{V,LR} - \frac{8}{3}L_{ed\ i22}^{V,LR} + \frac{4}{3}L_{ee\ kkjj}^{V,LR} + \frac{16}{3}L_{ee\ jjkk}^{V,RR} + \frac{4}{3}L_{de\ 11jj}^{V,LR} \\
& + \frac{4}{3}L_{de\ 22jj}^{V,LR} + \frac{4}{3}L_{ed\ jj11}^{V,RR} + \frac{4}{3}L_{ed\ jj22}^{V,RR} + \frac{8}{3}L_{ee\ jjjj}^{V,LR} + 8L_{ee\ jjjj}^{V,RR} - \frac{8}{3}L_{ed\ jj11}^{V,RR} \\
& \left. - \frac{8}{3}L_{ed\ jj22}^{V,RR} - \frac{8}{3}L_{ue\ 11jj}^{V,LR} - \frac{8}{3}L_{ue\ 22jj}^{V,LR} \right] + \alpha_s \alpha \left[ \frac{16}{3}L_{ed\ i11}^{V,LL} + \frac{16}{3}L_{ed\ i22}^{V,LL} \right. \\
& + \frac{16}{3}L_{ed\ i11}^{V,LR} + \frac{16}{3}L_{ed\ i22}^{V,LR} - \frac{32}{3}L_{ed\ i11}^{V,LL} - \frac{32}{3}L_{ed\ i22}^{V,LL} - \frac{32}{3}L_{ed\ i11}^{V,LR} - \frac{32}{3}L_{ed\ i22}^{V,LR} \\
& + \frac{16}{3}L_{de\ 11jj}^{V,LR} + \frac{16}{3}L_{de\ 22jj}^{V,LR} + \frac{16}{3}L_{ed\ jj11}^{V,RR} + \frac{16}{3}L_{ed\ jj22}^{V,RR} - \frac{32}{3}L_{ed\ jj11}^{V,RR} - \frac{32}{3}L_{ed\ jj22}^{V,RR}
\end{aligned}$$

$$\begin{aligned}
& -\frac{32}{3}L_{11jj}^{V,LR} - \frac{32}{3}L_{22jj}^{V,LR} \Big] + \alpha^2 \Big[ \frac{32}{27}L_{iijj}^{V,LL} + \frac{6122}{27}L_{ijjj}^{V,LR} + \frac{32}{27}L_{iikk}^{V,LL} \\
& + \frac{296}{27}L_{iikk}^{V,LR} - \frac{344}{81}L_{ii11}^{V,LL} - \frac{344}{81}L_{ii22}^{V,LL} + \frac{424}{81}L_{ii11}^{V,LR} + \frac{424}{81}L_{ii22}^{V,LR} - \frac{736}{27}L_{iii}^{V,LL} \\
& + \frac{296}{27}L_{iii}^{V,LR} - \frac{3128}{81}L_{ii11}^{V,LL} - \frac{3128}{81}L_{ii22}^{V,LL} - \frac{56}{81}L_{ii11}^{V,LR} - \frac{56}{81}L_{ii22}^{V,LR} + \frac{296}{27}L_{kkjj}^{V,LR} \\
& + \frac{32}{27}L_{jjkk}^{V,RR} + \frac{424}{81}L_{11jj}^{V,LR} + \frac{424}{81}L_{22jj}^{V,LR} - \frac{344}{81}L_{jj11}^{V,RR} - \frac{344}{81}L_{jj22}^{V,RR} + \frac{592}{27}L_{jjjj}^{V,LR} \\
& - \frac{80}{3}L_{jjjj}^{V,RR} - \frac{3128}{81}L_{jj11}^{V,RR} - \frac{3128}{81}L_{jj22}^{V,RR} - \frac{56}{81}L_{11jj}^{V,LR} - \frac{56}{81}L_{22jj}^{V,LR} \Big] ;
\end{aligned}$$

$$\begin{aligned}
\dot{L}_{iii}^{V,LR} &= e^2 \Big[ \frac{16}{3}L_{iijj}^{V,LL} + \frac{4}{3}L_{iijj}^{V,LR} + \frac{4}{3}L_{jjii}^{V,LR} + \frac{16}{3}L_{ijjj}^{V,RR} + \frac{16}{3}L_{iikk}^{V,LL} \\
& + \frac{4}{3}L_{iikk}^{V,LR} + \frac{4}{3}L_{kkii}^{V,LR} + \frac{16}{3}L_{iikk}^{V,RR} + \frac{4}{3}L_{11ii}^{V,LR} + \frac{4}{3}L_{22ii}^{V,LR} + \frac{4}{3}L_{ii11}^{V,LL} \\
& + \frac{4}{3}L_{ii22}^{V,LL} + \frac{4}{3}L_{ii11}^{V,LR} + \frac{4}{3}L_{ii22}^{V,LR} + \frac{4}{3}L_{ii11}^{V,RR} + \frac{4}{3}L_{ii22}^{V,RR} + \frac{16}{3}L_{iii}^{V,LL} \\
& - \frac{28}{3}L_{iii}^{V,LR} + \frac{16}{3}L_{iii}^{V,RR} - \frac{8}{3}L_{ii11}^{V,LL} - \frac{8}{3}L_{ii22}^{V,LL} - \frac{8}{3}L_{ii11}^{V,LR} - \frac{8}{3}L_{ii22}^{V,LR} \\
& - \frac{8}{3}L_{ii11}^{V,RR} - \frac{8}{3}L_{ii22}^{V,RR} - \frac{8}{3}L_{11ii}^{V,LR} - \frac{8}{3}L_{22ii}^{V,LR} \Big] + \alpha_s \alpha \Big[ \frac{16}{3}L_{11ii}^{V,LR} \\
& + \frac{16}{3}L_{22ii}^{V,LR} + \frac{16}{3}L_{ii11}^{V,LL} + \frac{16}{3}L_{ii22}^{V,LL} + \frac{16}{3}L_{ii11}^{V,LR} + \frac{16}{3}L_{ii22}^{V,LR} + \frac{16}{3}L_{ii11}^{V,RR} \\
& + \frac{16}{3}L_{ii22}^{V,RR} - \frac{32}{3}L_{ii11}^{V,LL} - \frac{32}{3}L_{ii22}^{V,LL} - \frac{32}{3}L_{ii11}^{V,LR} - \frac{32}{3}L_{ii22}^{V,LR} - \frac{32}{3}L_{ii11}^{V,RR} \\
& - \frac{32}{3}L_{ii22}^{V,RR} - \frac{32}{3}L_{11ii}^{V,LR} - \frac{32}{3}L_{22ii}^{V,LR} \Big] + \alpha^2 \Big[ \frac{32}{27}L_{iijj}^{V,LL} + \frac{296}{27}L_{ijjj}^{V,LR} \\
& + \frac{296}{27}L_{iikk}^{V,LR} + \frac{32}{27}L_{iijj}^{V,RR} + \frac{32}{27}L_{iikk}^{V,LL} + \frac{296}{27}L_{iikk}^{V,LR} + \frac{32}{27}L_{kkii}^{V,LR} + \frac{32}{27}L_{iikk}^{V,RR} \\
& + \frac{424}{81}L_{11ii}^{V,LR} + \frac{424}{81}L_{22ii}^{V,LR} - \frac{344}{81}L_{ii11}^{V,LL} - \frac{344}{81}L_{ii22}^{V,LL} + \frac{424}{81}L_{ii11}^{V,LR} + \frac{424}{81}L_{ii22}^{V,LR} \\
& - \frac{344}{81}L_{ii11}^{V,RR} - \frac{344}{81}L_{ii22}^{V,RR} - \frac{736}{27}L_{iii}^{V,LL} + \frac{6418}{27}L_{iii}^{V,LR} - \frac{736}{27}L_{iii}^{V,RR} - \frac{3128}{81}L_{ii11}^{V,LL} \\
& - \frac{3128}{81}L_{ii22}^{V,LL} - \frac{56}{81}L_{ii11}^{V,LR} - \frac{56}{81}L_{ii22}^{V,LR} - \frac{3128}{81}L_{ii11}^{V,RR} - \frac{3128}{81}L_{ii22}^{V,RR} - \frac{56}{81}L_{11ii}^{V,LR}
\end{aligned}$$

$$\begin{aligned}
& -\frac{56}{81}L_{22ii}^{V,LR} \Big] ; \\
\dot{L}_{ed\,ijj}^{V,RR} = & e^2 \Bigg[ 4L_{ed\,ijj}^{V,RR} + \frac{4}{9}L_{jjii}^{V,LR} + \frac{16}{9}L_{ijjj}^{V,RR} + \frac{4}{9}L_{kkii}^{V,LR} + \frac{16}{9}L_{iikk}^{V,RR} \\
& + \frac{4}{9}L_{11ii}^{V,LR} + \frac{4}{9}L_{22ii}^{V,LR} + \frac{4}{9}L_{ii11}^{V,RR} + \frac{4}{9}L_{ii22}^{V,RR} + \frac{4}{9}L_{iiii}^{V,LR} + \frac{16}{9}L_{iiii}^{V,RR} \\
& - \frac{8}{9}L_{ii11}^{V,RR} - \frac{8}{9}L_{ii22}^{V,RR} - \frac{8}{9}L_{ii11}^{V,LR} - \frac{8}{9}L_{ii22}^{V,LR} + \frac{8}{3}L_{jjjj}^{V1,LR} + \frac{64}{9}L_{jjjj}^{V,RR} \\
& + \frac{4}{3}L_{11jj}^{V,LR} + \frac{4}{3}L_{22jj}^{V,LR} + \frac{4}{3}L_{33jj}^{V,LR} + \frac{4}{3}L_{11jj}^{V,RR} + \frac{4}{3}L_{22jj}^{V,RR} + \frac{4}{3}L_{33jj}^{V,RR} \\
& - \frac{8}{3}L_{11jj}^{V1,LR} - \frac{8}{3}L_{22jj}^{V1,LR} - \frac{8}{3}L_{11jj}^{V1,RR} - \frac{8}{3}L_{22jj}^{V1,RR} \Bigg] + \alpha_s^2 \Bigg[ -8L_{11ii}^{V,LR} \\
& - 8L_{22ii}^{V,LR} + 8L_{ii11}^{V,RR} + 8L_{ii22}^{V,RR} + 8L_{ii11}^{V,RR} + 8L_{ii22}^{V,RR} - 8L_{11ii}^{V,LR} \\
& - 8L_{22ii}^{V,LR} \Bigg] + \alpha_s \alpha \Bigg[ -16L_{ijjj}^{V,RR} + \frac{16}{9}L_{11ii}^{V,LR} + \frac{16}{9}L_{22ii}^{V,LR} + \frac{16}{9}L_{ii11}^{V,RR} \\
& + \frac{16}{9}L_{ii22}^{V,RR} - \frac{32}{9}L_{ii11}^{V,RR} - \frac{32}{9}L_{ii22}^{V,RR} - \frac{32}{9}L_{11ii}^{V,LR} - \frac{32}{9}L_{22ii}^{V,LR} + \frac{32}{3}L_{jjjj}^{V1,LR} \\
& - \frac{2044}{243}L_{jjjj}^{V8,LR} + \frac{5152}{243}L_{jjjj}^{V,RR} - \frac{32}{3}L_{11jj}^{V1,LR} - \frac{32}{3}L_{22jj}^{V1,LR} - \frac{32}{3}L_{11jj}^{V1,RR} - \frac{32}{3}L_{22jj}^{V1,RR} \\
& + \frac{1354}{243}L_{11jj}^{V8,LR} + \frac{1354}{243}L_{22jj}^{V8,LR} - \frac{86}{243}L_{11jj}^{V8,RR} - \frac{86}{243}L_{22jj}^{V8,RR} \Bigg] + \alpha^2 \Bigg[ -\frac{334}{27}L_{ijjj}^{V,RR} \\
& - \frac{520}{81}L_{jjii}^{V,LR} + \frac{224}{81}L_{ijjj}^{V,RR} - \frac{520}{81}L_{kkii}^{V,LR} + \frac{224}{81}L_{iikk}^{V,RR} - \frac{200}{243}L_{11ii}^{V,LR} - \frac{200}{243}L_{22ii}^{V,LR} \\
& - \frac{104}{243}L_{ii11}^{V,RR} - \frac{104}{243}L_{ii22}^{V,RR} - \frac{520}{81}L_{iiii}^{V,LR} + \frac{32}{81}L_{iiii}^{V,RR} - \frac{1016}{243}L_{ii11}^{V,RR} - \frac{1016}{243}L_{ii22}^{V,RR} \\
& - \frac{1400}{243}L_{11ii}^{V,LR} - \frac{1400}{243}L_{22ii}^{V,LR} - \frac{2624}{243}L_{jjjj}^{V1,LR} + \frac{23296}{729}L_{jjjj}^{V,RR} - \frac{3184}{243}L_{11jj}^{V,LR} \\
& - \frac{3184}{243}L_{22jj}^{V,LR} - \frac{3184}{243}L_{33jj}^{V,LR} + \frac{3728}{243}L_{11jj}^{V,RR} + \frac{3728}{243}L_{22jj}^{V,RR} + \frac{3728}{243}L_{33jj}^{V,RR} \\
& - \frac{6232}{243}L_{11jj}^{V1,LR} - \frac{6232}{243}L_{22jj}^{V1,LR} + \frac{2984}{243}L_{11jj}^{V1,RR} + \frac{2984}{243}L_{22jj}^{V1,RR} \Bigg] ;
\end{aligned}$$

$$\begin{aligned}
\dot{L}_{ijj}^{V,RR} = & e^2 \left[ -\frac{8}{9} L_{11ii}^{V,LR} - \frac{8}{9} L_{22ii}^{V,LR} + \frac{4}{3} L_{11jj}^{V1,LR} + \frac{4}{3} L_{22jj}^{V1,LR} - \frac{8}{9} L_{ii11}^{V,RR} \right. \\
& - \frac{8}{9} L_{ii22}^{V,RR} - \frac{8}{9} L_{iii}^{V,LR} - \frac{8}{9} L_{jji}^{V,LR} - \frac{8}{9} L_{kii}^{V,LR} - \frac{32}{9} L_{iii}^{V,RR} - \frac{32}{9} L_{ijj}^{V,RR} \\
& - \frac{32}{9} L_{ikk}^{V,RR} + \frac{4}{3} L_{11jj}^{V,LR} + \frac{4}{3} L_{22jj}^{V,LR} + \frac{4}{3} L_{33jj}^{V,LR} + \frac{4}{3} L_{11jj}^{V,RR} + \frac{4}{3} L_{22jj}^{V,RR} \\
& + \frac{4}{3} L_{33jj}^{V,RR} + \frac{16}{9} L_{ii11}^{V,RR} + \frac{16}{9} L_{ii22}^{V,RR} - 8 L_{ijj}^{V,RR} + \frac{4}{3} L_{jj11}^{V1,RR} + \frac{4}{3} L_{jj22}^{V1,RR} \\
& + \frac{16}{9} L_{11ii}^{V,LR} + \frac{16}{9} L_{22ii}^{V,LR} - \frac{8}{3} L_{jjjj}^{V1,LR} - \frac{8}{3} L_{kkjj}^{V1,LR} - \frac{64}{9} L_{jjjj}^{V,RR} - \frac{16}{3} L_{jjkk}^{V,RR} \\
& \left. - \frac{16}{9} L_{jkkj}^{V,RR} \right] + \alpha_s^2 \left[ -8 L_{11ii}^{V,LR} - 8 L_{22ii}^{V,LR} + 8 L_{ii11}^{V,RR} + 8 L_{ii22}^{V,RR} \right. \\
& + 8 L_{ii11}^{V,RR} + 8 L_{ii22}^{V,RR} - 8 L_{11ii}^{V,LR} - 8 L_{22ii}^{V,LR} \left. \right] + \alpha_s \alpha \left[ -\frac{32}{9} L_{11ii}^{V,LR} \right. \\
& - \frac{32}{9} L_{22ii}^{V,LR} + \frac{16}{3} L_{11jj}^{V1,LR} - \frac{32}{3} L_{22jj}^{V1,LR} - \frac{332}{243} L_{11jj}^{V8,LR} + \frac{2044}{243} L_{22jj}^{V8,LR} - \frac{32}{9} L_{ii11}^{V,RR} \\
& - \frac{32}{9} L_{ii22}^{V,RR} + \frac{64}{9} L_{ii11}^{V,RR} + \frac{64}{9} L_{ii22}^{V,RR} + 32 L_{ijj}^{V,RR} + \frac{16}{3} L_{jj11}^{V1,RR} + \frac{16}{3} L_{jj22}^{V1,RR} \\
& + \frac{388}{243} L_{jj11}^{V8,RR} + \frac{388}{243} L_{jj22}^{V8,RR} + \frac{64}{9} L_{11ii}^{V,LR} + \frac{64}{9} L_{22ii}^{V,LR} - \frac{32}{3} L_{jjjj}^{V1,LR} - \frac{32}{3} L_{kkjj}^{V1,LR} \\
& \left. + \frac{2044}{243} L_{jjjj}^{V8,LR} + \frac{2044}{243} L_{kkjj}^{V8,LR} - \frac{2096}{81} L_{jjjj}^{V,RR} - 16 L_{jjkk}^{V,RR} - \frac{128}{243} L_{jkkj}^{V,RR} \right] \\
& + \alpha^2 \left[ \frac{1408}{243} L_{11ii}^{V,LR} + \frac{1408}{243} L_{22ii}^{V,LR} - \frac{928}{243} L_{11jj}^{V1,LR} + \frac{416}{243} L_{22jj}^{V1,LR} + \frac{2512}{243} L_{ii11}^{V,RR} \right. \\
& + \frac{2512}{243} L_{ii22}^{V,RR} + \frac{464}{81} L_{iii}^{V,LR} + \frac{464}{81} L_{jji}^{V,LR} + \frac{464}{81} L_{kii}^{V,LR} + \frac{3680}{81} L_{iii}^{V,RR} + \frac{2432}{81} L_{ijj}^{V,RR} \\
& + \frac{2432}{81} L_{ikk}^{V,RR} - \frac{424}{243} L_{11jj}^{V,LR} - \frac{424}{243} L_{22jj}^{V,LR} - \frac{424}{243} L_{33jj}^{V,LR} + \frac{3248}{243} L_{11jj}^{V,RR} \\
& + \frac{3248}{243} L_{22jj}^{V,RR} + \frac{3248}{243} L_{33jj}^{V,RR} + \frac{1312}{243} L_{ii11}^{V,RR} + \frac{1312}{243} L_{ii22}^{V,RR} + \frac{128}{27} L_{ijj}^{V,RR} \\
& + \frac{296}{243} L_{jj11}^{V1,RR} + \frac{296}{243} L_{jj22}^{V1,RR} - \frac{3104}{243} L_{11ii}^{V,LR} - \frac{3104}{243} L_{22ii}^{V,LR} + \frac{128}{243} L_{jjjj}^{V1,LR} \\
& \left. + \frac{128}{243} L_{kkjj}^{V1,LR} + \frac{26272}{243} L_{jjjj}^{V,RR} + \frac{10048}{243} L_{jjkk}^{V,RR} + \frac{18304}{729} L_{jkkj}^{V,RR} \right];
\end{aligned}$$



$$\begin{aligned}
\dot{L}_{ijj}^{V1,RR} = & \frac{8}{3} L_{ijj}^{V8,RR} g_s^2 + e^2 \left[ -\frac{16}{9} L_{jjj}^{V1,LR} - \frac{128}{27} L_{jjj}^{V,RR} + \frac{4}{9} L_{11i}^{V1,LR} + \frac{4}{9} L_{22i}^{V1,LR} \right. \\
& - \frac{8}{9} L_{11j}^{V,LR} - \frac{8}{9} L_{22j}^{V,LR} - \frac{8}{9} L_{33j}^{V,LR} - \frac{8}{9} L_{11j}^{V,RR} - \frac{8}{9} L_{22j}^{V,RR} - \frac{8}{9} L_{33j}^{V,RR} \\
& + \frac{4}{9} L_{11i}^{V,LR} + \frac{4}{9} L_{22i}^{V,LR} + \frac{4}{9} L_{33i}^{V,LR} + \frac{4}{9} L_{11i}^{V,RR} + \frac{4}{9} L_{22i}^{V,RR} + \frac{4}{9} L_{33i}^{V,RR} \\
& + \frac{16}{9} L_{11j}^{V1,LR} + \frac{16}{9} L_{22j}^{V1,LR} + \frac{16}{9} L_{11j}^{V1,RR} + \frac{16}{9} L_{22j}^{V1,RR} + \frac{4}{9} L_{i11}^{V1,RR} + \frac{4}{9} L_{i22}^{V1,RR} \\
& \left. - \frac{8}{3} L_{ijj}^{V1,RR} - \frac{8}{9} L_{iii}^{V1,LR} - \frac{8}{9} L_{kii}^{V1,LR} - \frac{64}{27} L_{iii}^{V,RR} - \frac{16}{9} L_{iik}^{V,RR} - \frac{16}{27} L_{ikki}^{V,RR} \right] \\
& + \alpha_s^2 \left[ -16 L_{jjj}^{V1,LR} + \frac{8}{27} L_{jjj}^{V8,LR} + \frac{1672}{27} L_{jjj}^{V,RR} - 8 L_{11i}^{V1,LR} - 8 L_{22i}^{V1,LR} \right. \\
& + \frac{4}{27} L_{11i}^{V8,LR} + \frac{4}{27} L_{22i}^{V8,LR} - 8 L_{11j}^{V1,LR} - 8 L_{22j}^{V1,LR} + 8 L_{11j}^{V1,RR} + 8 L_{22j}^{V1,RR} \\
& + 8 L_{i11}^{V1,RR} + 8 L_{i22}^{V1,RR} - \frac{28}{3} L_{ijj}^{V1,RR} + \frac{4}{27} L_{11j}^{V8,LR} + \frac{4}{27} L_{22j}^{V8,LR} + \frac{4}{27} L_{11j}^{V8,RR} \\
& + \frac{4}{27} L_{22j}^{V8,RR} + \frac{4}{27} L_{i11}^{V8,RR} + \frac{4}{27} L_{i22}^{V8,RR} + \frac{82}{27} L_{ijj}^{V8,RR} - 8 L_{iii}^{V1,LR} - 8 L_{kii}^{V1,LR} \\
& + \frac{4}{27} L_{iii}^{V8,RR} + \frac{4}{27} L_{kii}^{V8,RR} + \frac{328}{9} L_{iii}^{V,RR} + 16 L_{iik}^{V,RR} + \frac{256}{27} L_{ikki}^{V,RR} \left. \right] + \alpha_s \alpha \left[ -\frac{64}{9} L_{jjj}^{V1,LR} \right. \\
& + \frac{4088}{729} L_{jjj}^{V8,LR} - \frac{10304}{729} L_{jjj}^{V,RR} + \frac{16}{9} L_{11i}^{V1,LR} - \frac{32}{9} L_{22i}^{V1,LR} - \frac{332}{729} L_{11i}^{V8,LR} \\
& + \frac{2044}{729} L_{22i}^{V8,LR} + \frac{64}{9} L_{11j}^{V1,LR} + \frac{64}{9} L_{22j}^{V1,LR} + \frac{64}{9} L_{11j}^{V1,RR} + \frac{64}{9} L_{22j}^{V1,RR} + \frac{16}{9} L_{i11}^{V1,RR} \\
& + \frac{16}{9} L_{i22}^{V1,RR} + \frac{64}{3} L_{ijj}^{V1,RR} - \frac{2708}{729} L_{11j}^{V8,LR} - \frac{2708}{729} L_{22j}^{V8,LR} + \frac{172}{729} L_{11j}^{V8,RR} \\
& + \frac{172}{729} L_{22j}^{V8,RR} + \frac{388}{729} L_{i11}^{V8,RR} + \frac{388}{729} L_{i22}^{V8,RR} - \frac{8}{27} L_{ijj}^{V8,RR} - \frac{32}{9} L_{iii}^{V1,LR} - \frac{32}{9} L_{kii}^{V1,LR} \\
& \left. + \frac{2044}{729} L_{iii}^{V8,LR} + \frac{2044}{729} L_{kii}^{V8,LR} - \frac{2096}{243} L_{iii}^{V,RR} - \frac{16}{3} L_{iik}^{V,RR} - \frac{128}{729} L_{ikki}^{V,RR} \right] \\
& + \alpha^2 \left[ -\frac{512}{729} L_{jjj}^{V1,LR} + \frac{40528}{2187} L_{jjj}^{V,RR} - \frac{136}{729} L_{11i}^{V1,LR} + \frac{2720}{729} L_{22i}^{V1,LR} - \frac{2992}{729} L_{11j}^{V,LR} \right.
\end{aligned}$$

$$\begin{aligned}
& -\frac{2992}{729}L_{22jj}^{V,LR} - \frac{2992}{729}L_{33jj}^{V,LR} + \frac{2624}{729}L_{11jj}^{V,RR} + \frac{2624}{729}L_{22jj}^{V,RR} + \frac{2624}{729}L_{33jj}^{V,RR} \\
& + \frac{1664}{729}L_{11ii}^{V,LR} + \frac{1664}{729}L_{22ii}^{V,LR} + \frac{1664}{729}L_{33ii}^{V,LR} + \frac{1448}{729}L_{11ii}^{V,RR} + \frac{1448}{729}L_{22ii}^{V,RR} \\
& + \frac{1448}{729}L_{33ii}^{V,RR} - \frac{1216}{729}L_{11jj}^{V1,LR} - \frac{1216}{729}L_{22jj}^{V1,LR} + \frac{6272}{729}L_{11jj}^{V1,RR} + \frac{6272}{729}L_{22jj}^{V1,RR} \\
& - \frac{208}{729}L_{ii11}^{V1,RR} - \frac{208}{729}L_{ii22}^{V1,RR} - \frac{112}{81}L_{ijjj}^{V1,RR} + \frac{2432}{729}L_{uu}^{V1,LR} + \frac{2432}{729}L_{kkii}^{V1,LR} \\
& + \frac{11872}{729}L_{iii}^{V,RR} + \frac{4288}{729}L_{ikk}^{V,RR} + \frac{9088}{2187}L_{ikki}^{V,RR} \Big] ;
\end{aligned}$$

$$\begin{aligned}
\dot{L}_{ijj}^{V8,RR} &= g_s^2 \Bigg[ 12L_{ijj}^{V1,RR} - 4L_{ijj}^{V8,RR} + \frac{2}{3}L_{kkii}^{V8,LR} + \frac{8}{3}L_{ikki}^{V,RR} + \frac{2}{3}L_{11ii}^{V8,LR} \\
& + \frac{2}{3}L_{22ii}^{V8,LR} + \frac{2}{3}L_{ii11}^{V8,RR} + \frac{2}{3}L_{ii22}^{V8,RR} + \frac{2}{3}L_{iii}^{V8,LR} + \frac{8}{3}L_{iii}^{V,RR} + \frac{4}{3}L_{jjjj}^{V8,LR} \\
& + \frac{16}{3}L_{jjjj}^{V,RR} + \frac{2}{3}L_{11jj}^{V8,LR} + \frac{2}{3}L_{22jj}^{V8,LR} + \frac{2}{3}L_{11jj}^{V8,RR} + \frac{2}{3}L_{22jj}^{V8,RR} \Bigg] - \frac{8}{3}e^2L_{ijj}^{V8,RR} \\
& + \alpha_s^2 \Bigg[ \frac{41}{3}L_{ijj}^{V1,RR} - \frac{125}{9}L_{ijj}^{V8,RR} - \frac{22}{3}L_{kkii}^{V1,LR} + \frac{157}{81}L_{kkii}^{V8,LR} - \frac{28}{3}L_{ikk}^{V,RR} \\
& + \frac{5248}{81}L_{ikki}^{V,RR} - \frac{22}{3}L_{11ii}^{V1,LR} - \frac{22}{3}L_{22ii}^{V1,LR} + \frac{157}{81}L_{11ii}^{V8,LR} + \frac{157}{81}L_{22ii}^{V8,LR} - \frac{2}{3}L_{ii11}^{V1,RR} \\
& - \frac{2}{3}L_{ii22}^{V1,RR} + \frac{787}{81}L_{ii11}^{V8,RR} + \frac{787}{81}L_{ii22}^{V8,RR} - \frac{22}{3}L_{iii}^{V1,LR} + \frac{157}{81}L_{iii}^{V8,LR} + \frac{1918}{27}L_{iii}^{V,RR} \\
& - \frac{44}{3}L_{jjjj}^{V1,LR} + \frac{314}{81}L_{jjjj}^{V8,LR} + \frac{10246}{81}L_{jjjj}^{V,RR} - \frac{22}{3}L_{11jj}^{V1,LR} - \frac{22}{3}L_{22jj}^{V1,LR} - \frac{2}{3}L_{11jj}^{V1,RR} \\
& - \frac{2}{3}L_{22jj}^{V1,RR} + \frac{157}{81}L_{11jj}^{V8,LR} + \frac{157}{81}L_{22jj}^{V8,LR} + \frac{787}{81}L_{11jj}^{V8,RR} + \frac{787}{81}L_{22jj}^{V8,RR} \Bigg] \\
& + \alpha_s \alpha \Bigg[ -\frac{4}{3}L_{ijj}^{V1,RR} - \frac{47}{9}L_{ijj}^{V8,RR} - \frac{568}{81}L_{kkii}^{V1,LR} + \frac{4}{27}L_{kkii}^{V8,LR} - \frac{1136}{81}L_{ikk}^{V,RR} \\
& - \frac{6560}{243}L_{ikki}^{V,RR} + \frac{284}{81}L_{11ii}^{V1,LR} - \frac{496}{81}L_{22ii}^{V1,LR} + \frac{10}{27}L_{11ii}^{V8,LR} + \frac{4}{27}L_{22ii}^{V8,LR} + \frac{284}{81}L_{11ii}^{V,LR} \\
& + \frac{284}{81}L_{22ii}^{V,LR} + \frac{284}{81}L_{33ii}^{V,LR} + \frac{284}{81}L_{11ii}^{V,RR} + \frac{284}{81}L_{22ii}^{V,RR} + \frac{284}{81}L_{33ii}^{V,RR} + \frac{284}{81}L_{ii11}^{V1,RR} \\
& + \frac{284}{81}L_{ii22}^{V1,RR} + \frac{14}{9}L_{ii11}^{V8,RR} + \frac{14}{9}L_{ii22}^{V8,RR} - \frac{568}{81}L_{iii}^{V1,LR} + \frac{4}{27}L_{iii}^{V8,LR} - \frac{4616}{81}L_{iii}^{V,RR}
\end{aligned}$$

$$\begin{aligned}
& -\frac{392}{81}L_{jjjj}^{V1,LR} + \frac{104}{27}L_{jjjj}^{V8,LR} - \frac{15728}{243}L_{jjjj}^{V,RR} - \frac{196}{81}L_{11jj}^{V,LR} - \frac{196}{81}L_{22jj}^{V,LR} - \frac{196}{81}L_{33jj}^{V,LR} \\
& -\frac{196}{81}L_{11jj}^{V,RR} - \frac{196}{81}L_{22jj}^{V,RR} - \frac{196}{81}L_{33jj}^{V,RR} + \frac{392}{81}L_{11jj}^{V1,LR} + \frac{392}{81}L_{22jj}^{V1,LR} + \frac{392}{81}L_{11jj}^{V1,RR} \\
& + \frac{392}{81}L_{22jj}^{V1,RR} - \frac{80}{27}L_{11jj}^{V8,LR} - \frac{80}{27}L_{22jj}^{V8,LR} + \frac{56}{9}L_{11jj}^{V8,RR} + \frac{56}{9}L_{22jj}^{V8,RR} \Big] \\
& - \frac{112}{81}\alpha^2 L_{ijjj}^{V8,RR} ;
\end{aligned}$$

$$\begin{aligned}
\dot{L}_{jjii}^{V,RR} = & e^2 \Bigg[ \frac{4}{3}L_{jjii}^{V1,LR} + \frac{8}{3}L_{ijjj}^{V,RR} + \frac{8}{9}L_{ijji}^{V,RR} + 4L_{jjii}^{V,RR} + \frac{4}{3}L_{iiii}^{V1,LR} \\
& + \frac{32}{9}L_{iiii}^{V,RR} + \frac{4}{3}L_{11ii}^{V,LR} + \frac{4}{3}L_{22ii}^{V,LR} + \frac{4}{3}L_{33ii}^{V,LR} + \frac{4}{3}L_{11ii}^{V,RR} + \frac{4}{3}L_{22ii}^{V,RR} \\
& + \frac{4}{3}L_{33ii}^{V,RR} - \frac{8}{3}L_{11ii}^{V1,LR} - \frac{8}{3}L_{22ii}^{V1,LR} - \frac{8}{3}L_{33ii}^{V1,RR} - \frac{8}{3}L_{11ii}^{V1,RR} + \frac{4}{9}L_{kkjj}^{V,LR} \\
& + \frac{16}{9}L_{jjkk}^{V,RR} + \frac{4}{9}L_{11jj}^{V,LR} + \frac{4}{9}L_{22jj}^{V,LR} + \frac{4}{9}L_{jj11}^{V,RR} + \frac{4}{9}L_{jj22}^{V,RR} + \frac{8}{9}L_{jjjj}^{V,LR} \\
& + \frac{8}{3}L_{jjjj}^{V,RR} - \frac{8}{9}L_{jj11}^{V,RR} - \frac{8}{9}L_{jj22}^{V,RR} - \frac{8}{9}L_{11jj}^{V,LR} - \frac{8}{9}L_{22jj}^{V,LR} \Big] + \alpha_s^2 \Bigg[ -8L_{11jj}^{V,LR} \\
& - 8L_{22jj}^{V,LR} + 8L_{jj11}^{V,RR} + 8L_{jj22}^{V,RR} + 8L_{jj11}^{V,RR} + 8L_{jj22}^{V,RR} - 8L_{11jj}^{V,LR} \\
& - 8L_{22jj}^{V,LR} \Big] + \alpha_s \alpha \Bigg[ \frac{16}{3}L_{jjii}^{V1,LR} - \frac{1022}{243}L_{jjii}^{V8,LR} + 8L_{ijjj}^{V,RR} + \frac{64}{243}L_{ijji}^{V,RR} \\
& - 16L_{jjii}^{V,RR} + \frac{16}{3}L_{iiii}^{V1,LR} - \frac{1022}{243}L_{iiii}^{V8,LR} + \frac{1048}{81}L_{iiii}^{V,RR} - \frac{32}{3}L_{11ii}^{V1,LR} - \frac{32}{3}L_{22ii}^{V1,LR} \\
& - \frac{32}{3}L_{33ii}^{V1,RR} - \frac{32}{3}L_{11ii}^{V1,RR} + \frac{1354}{243}L_{11ii}^{V8,LR} + \frac{1354}{243}L_{22ii}^{V8,LR} - \frac{86}{243}L_{11ii}^{V8,RR} - \frac{86}{243}L_{22ii}^{V8,RR} \\
& + \frac{16}{9}L_{11jj}^{V,LR} + \frac{16}{9}L_{22jj}^{V,LR} + \frac{16}{9}L_{jj11}^{V,RR} + \frac{16}{9}L_{jj22}^{V,RR} - \frac{32}{9}L_{jj11}^{V,RR} - \frac{32}{9}L_{jj22}^{V,RR} \\
& - \frac{32}{9}L_{11jj}^{V,LR} - \frac{32}{9}L_{22jj}^{V,LR} \Big] + \alpha^2 \Bigg[ -\frac{1312}{243}L_{jjii}^{V1,LR} + \frac{1984}{243}L_{ijjj}^{V,RR} + \frac{2896}{729}L_{ijji}^{V,RR} \\
& - \frac{334}{27}L_{jjii}^{V,RR} - \frac{1312}{243}L_{iiii}^{V1,LR} + \frac{4816}{243}L_{iiii}^{V,RR} - \frac{3184}{243}L_{11ii}^{V,LR} - \frac{3184}{243}L_{22ii}^{V,LR} \\
& - \frac{3184}{243}L_{33ii}^{V,LR} + \frac{3728}{243}L_{11ii}^{V,RR} + \frac{3728}{243}L_{22ii}^{V,RR} + \frac{3728}{243}L_{33ii}^{V,RR} - \frac{6232}{243}L_{11ii}^{V1,LR}
\end{aligned}$$

$$\begin{aligned}
& -\frac{6232}{243}L_{ud,22ii}^{V1,LR} + \frac{2984}{243}L_{ud,11ii}^{V1,RR} + \frac{2984}{243}L_{ud,22ii}^{V1,RR} - \frac{520}{81}L_{kkjj}^{V,LR} + \frac{224}{81}L_{jjkk}^{V,RR} \\
& -\frac{200}{243}L_{de,11jj}^{V,LR} - \frac{200}{243}L_{de,22jj}^{V,LR} - \frac{104}{243}L_{jj11}^{V,RR} - \frac{104}{243}L_{jj22}^{V,RR} - \frac{1040}{81}L_{jjjj}^{V,LR} + \frac{16}{9}L_{jjjj}^{V,RR} \\
& -\frac{1016}{243}L_{jj11}^{V,RR} - \frac{1016}{243}L_{jj22}^{V,RR} - \frac{1400}{243}L_{11jj}^{V,LR} - \frac{1400}{243}L_{22jj}^{V,LR} \Bigg]; \\
\dot{L}_{jjii}^{V,RR} &= e^2 \Bigg[ -8L_{jjii}^{V,RR} - \frac{8}{3}L_{kkii}^{V1,LR} - \frac{16}{3}L_{iikk}^{V,RR} - \frac{16}{9}L_{iikki}^{V,RR} + \frac{4}{3}L_{11ii}^{V1,LR} \\
& + \frac{4}{3}L_{22ii}^{V1,LR} + \frac{4}{3}L_{11ii}^{V,LR} + \frac{4}{3}L_{22ii}^{V,LR} + \frac{4}{3}L_{33ii}^{V,LR} + \frac{4}{3}L_{11ii}^{V,RR} + \frac{4}{3}L_{22ii}^{V,RR} \\
& + \frac{4}{3}L_{33ii}^{V,RR} + \frac{4}{3}L_{ii11}^{V1,RR} + \frac{4}{3}L_{ii22}^{V1,RR} - \frac{8}{3}L_{iii}^{V1,LR} - \frac{64}{9}L_{iii}^{V,RR} - \frac{8}{9}L_{kkjj}^{V,LR} \\
& - \frac{32}{9}L_{jjkk}^{V,RR} - \frac{8}{9}L_{11jj}^{V,LR} - \frac{8}{9}L_{22jj}^{V,LR} - \frac{8}{9}L_{jj11}^{V,RR} - \frac{8}{9}L_{jj22}^{V,RR} - \frac{16}{9}L_{jjjj}^{V,LR} \\
& - \frac{16}{3}L_{jjjj}^{V,RR} + \frac{16}{9}L_{jj11}^{V,RR} + \frac{16}{9}L_{jj22}^{V,RR} + \frac{16}{9}L_{11jj}^{V,LR} + \frac{16}{9}L_{22jj}^{V,LR} \Bigg] + \alpha_s^2 \Bigg[ -8L_{11jj}^{V,LR} \\
& -8L_{22jj}^{V,LR} + 8L_{jj11}^{V,RR} + 8L_{jj22}^{V,RR} + 8L_{jj11}^{V,RR} + 8L_{jj22}^{V,RR} - 8L_{11jj}^{V,LR} \\
& -8L_{22jj}^{V,LR} \Bigg] + \alpha_s \alpha \Bigg[ 32L_{jjii}^{V,RR} - \frac{32}{3}L_{kkii}^{V1,LR} + \frac{2044}{243}L_{kkii}^{V8,LR} - 16L_{iikk}^{V,RR} \\
& - \frac{128}{243}L_{iikki}^{V,RR} + \frac{16}{3}L_{11ii}^{V1,LR} - \frac{32}{3}L_{22ii}^{V1,LR} - \frac{332}{243}L_{11ii}^{V8,LR} + \frac{2044}{243}L_{22ii}^{V8,LR} + \frac{16}{3}L_{ii11}^{V1,RR} \\
& + \frac{16}{3}L_{ii22}^{V1,RR} + \frac{388}{243}L_{ii11}^{V8,RR} + \frac{388}{243}L_{ii22}^{V8,RR} - \frac{32}{3}L_{iii}^{V1,LR} + \frac{2044}{243}L_{iii}^{V8,LR} - \frac{2096}{81}L_{iii}^{V,RR} \\
& - \frac{32}{9}L_{11jj}^{V,LR} - \frac{32}{9}L_{22jj}^{V,LR} - \frac{32}{9}L_{jj11}^{V,RR} - \frac{32}{9}L_{jj22}^{V,RR} + \frac{64}{9}L_{jj11}^{V,RR} + \frac{64}{9}L_{jj22}^{V,RR} \\
& + \frac{64}{9}L_{11jj}^{V,LR} + \frac{64}{9}L_{22jj}^{V,LR} \Bigg] + \alpha^2 \Bigg[ \frac{128}{27}L_{jjii}^{V,RR} + \frac{128}{243}L_{kkii}^{V1,LR} + \frac{10048}{243}L_{iikk}^{V,RR} \\
& + \frac{18304}{729}L_{iikki}^{V,RR} - \frac{928}{243}L_{11ii}^{V1,LR} + \frac{416}{243}L_{22ii}^{V1,LR} - \frac{424}{243}L_{11ii}^{V,LR} - \frac{424}{243}L_{22ii}^{V,LR} \\
& - \frac{424}{243}L_{33ii}^{V,LR} + \frac{3248}{243}L_{11ii}^{V,RR} + \frac{3248}{243}L_{22ii}^{V,RR} + \frac{3248}{243}L_{33ii}^{V,RR} + \frac{296}{243}L_{ii11}^{V1,RR} \\
& + \frac{296}{243}L_{ii22}^{V1,RR} + \frac{128}{243}L_{iii}^{V1,LR} + \frac{26272}{243}L_{iii}^{V,RR} + \frac{464}{81}L_{kkjj}^{V,LR} + \frac{2432}{81}L_{jjkk}^{V,RR}
\end{aligned}$$

$$\begin{aligned}
& + \frac{1408}{243} L_{11jj}^{V,LR} + \frac{1408}{243} L_{22jj}^{V,LR} + \frac{2512}{243} L_{jj11}^{V,RR} + \frac{2512}{243} L_{jj22}^{V,RR} + \frac{928}{81} L_{jjjj}^{V,LR} \\
& + \frac{544}{9} L_{jjjj}^{V,RR} + \frac{1312}{243} L_{jj11}^{V,RR} + \frac{1312}{243} L_{jj22}^{V,RR} - \frac{3104}{243} L_{11jj}^{V,LR} - \frac{3104}{243} L_{22jj}^{V,LR} \Big] ;
\end{aligned}$$

$$\begin{aligned}
\dot{L}_{jjii}^{V1,RR} = & \frac{8}{3} L_{jjii}^{V8,RR} g_s^2 + e^2 \Bigg[ -\frac{8}{9} L_{iii}^{V1,LR} - \frac{8}{9} L_{jjii}^{V1,LR} - \frac{64}{27} L_{iii}^{V,RR} - \frac{16}{9} L_{ijjj}^{V,RR} \\
& - \frac{16}{27} L_{ijji}^{V,RR} + \frac{4}{9} L_{du}^{V1,LR} + \frac{4}{9} L_{22jj}^{V1,LR} - \frac{8}{9} L_{ed}^{V,LR} - \frac{8}{9} L_{22ii}^{V,LR} - \frac{8}{9} L_{33ii}^{V,LR} \\
& - \frac{8}{9} L_{11ii}^{V,RR} - \frac{8}{9} L_{22ii}^{V,RR} - \frac{8}{9} L_{33ii}^{V,RR} + \frac{4}{9} L_{11jj}^{V,LR} + \frac{4}{9} L_{22jj}^{V,LR} + \frac{4}{9} L_{33jj}^{V,LR} \\
& + \frac{4}{9} L_{11jj}^{V,RR} + \frac{4}{9} L_{22jj}^{V,RR} + \frac{4}{9} L_{33jj}^{V,RR} + \frac{16}{9} L_{ud}^{V1,LR} + \frac{16}{9} L_{22ii}^{V1,LR} + \frac{16}{9} L_{11ii}^{V,RR} \\
& + \frac{16}{9} L_{22ii}^{V1,RR} + \frac{4}{9} L_{jj11}^{V1,RR} + \frac{4}{9} L_{jj22}^{V1,RR} - \frac{8}{3} L_{jjii}^{V1,RR} - \frac{8}{9} L_{jjjj}^{V1,LR} - \frac{8}{9} L_{kkjj}^{V1,LR} \\
& - \frac{64}{27} L_{jjjj}^{V,RR} - \frac{16}{9} L_{jjkk}^{V,RR} - \frac{16}{27} L_{jjkk}^{V,RR} \Big] + \alpha_s^2 \Bigg[ -8 L_{iii}^{V1,LR} - 8 L_{jjii}^{V1,LR} \\
& + \frac{4}{27} L_{iii}^{V8,LR} + \frac{4}{27} L_{jjii}^{V8,LR} + \frac{328}{9} L_{iii}^{V,RR} + 16 L_{ijjj}^{V,RR} + \frac{256}{27} L_{ijji}^{V,RR} - 8 L_{du}^{V1,LR} \\
& - 8 L_{22jj}^{V1,LR} + \frac{4}{27} L_{11jj}^{V8,LR} + \frac{4}{27} L_{22jj}^{V8,LR} - 8 L_{ud}^{V1,LR} - 8 L_{22ii}^{V1,LR} + 8 L_{11ii}^{V1,RR} \\
& + 8 L_{22ii}^{V1,RR} + 8 L_{jj11}^{V1,RR} + 8 L_{jj22}^{V1,RR} - \frac{28}{3} L_{jjii}^{V1,RR} + \frac{4}{27} L_{11ii}^{V8,LR} + \frac{4}{27} L_{22ii}^{V8,LR} \\
& + \frac{4}{27} L_{11ii}^{V8,RR} + \frac{4}{27} L_{22ii}^{V8,RR} + \frac{4}{27} L_{jj11}^{V8,RR} + \frac{4}{27} L_{jj22}^{V8,RR} + \frac{82}{27} L_{jjii}^{V8,RR} - 8 L_{uu}^{V1,LR} \\
& - 8 L_{kkjj}^{V1,LR} + \frac{4}{27} L_{jjjj}^{V8,LR} + \frac{4}{27} L_{kkjj}^{V8,LR} + \frac{328}{9} L_{jjjj}^{V,RR} + 16 L_{jjkk}^{V,RR} + \frac{256}{27} L_{jjkk}^{V,RR} \Big] \\
& + \alpha_s \alpha \Bigg[ -\frac{32}{9} L_{iii}^{V1,LR} - \frac{32}{9} L_{jjii}^{V1,LR} + \frac{2044}{729} L_{iii}^{V8,LR} + \frac{2044}{729} L_{jjii}^{V8,LR} - \frac{2096}{243} L_{iii}^{V,RR} \\
& - \frac{16}{3} L_{ijjj}^{V,RR} - \frac{128}{729} L_{ijji}^{V,RR} + \frac{16}{9} L_{du}^{V1,LR} - \frac{32}{9} L_{22jj}^{V1,LR} - \frac{332}{729} L_{11jj}^{V8,LR} + \frac{2044}{729} L_{22jj}^{V8,LR} \\
& + \frac{64}{9} L_{11ii}^{V1,LR} + \frac{64}{9} L_{22ii}^{V1,LR} + \frac{64}{9} L_{11ii}^{V1,RR} + \frac{64}{9} L_{22ii}^{V1,RR} + \frac{16}{9} L_{jj11}^{V1,RR} + \frac{16}{9} L_{jj22}^{V1,RR} \\
& + \frac{64}{3} L_{jjii}^{V1,RR} - \frac{2708}{729} L_{11ii}^{V8,LR} - \frac{2708}{729} L_{22ii}^{V8,LR} + \frac{172}{729} L_{11ii}^{V8,RR} + \frac{172}{729} L_{22ii}^{V8,RR}
\end{aligned}$$

$$\begin{aligned}
& + \frac{388}{729} L_{ud}^{V8,RR} + \frac{388}{729} L_{jj22}^{V8,RR} - \frac{8}{27} L_{jjii}^{V8,RR} - \frac{32}{9} L_{jjjj}^{V1,LR} - \frac{32}{9} L_{kkjj}^{V1,LR} + \frac{2044}{729} L_{jjjj}^{V8,LR} \\
& + \frac{2044}{729} L_{kkjj}^{V8,LR} - \frac{2096}{243} L_{jjjj}^{V,RR} - \frac{16}{3} L_{jjkk}^{V,RR} - \frac{128}{729} L_{jjkk}^{V,RR} \Big] + \alpha^2 \Big[ - \frac{256}{729} L_{iiii}^{V1,LR} \\
& - \frac{256}{729} L_{jjii}^{V1,LR} + \frac{8368}{729} L_{iiii}^{V,RR} + \frac{3232}{729} L_{ijjj}^{V,RR} + \frac{5728}{2187} L_{ijji}^{V,RR} - \frac{136}{729} L_{11jj}^{V1,LR} \\
& + \frac{2720}{729} L_{22jj}^{V1,LR} - \frac{2992}{729} L_{11ii}^{V,LR} - \frac{2992}{729} L_{22ii}^{V,LR} - \frac{2992}{729} L_{33ii}^{V,LR} + \frac{2624}{729} L_{11ii}^{V,RR} \\
& + \frac{2624}{729} L_{22ii}^{V,RR} + \frac{2624}{729} L_{33ii}^{V,RR} + \frac{1664}{729} L_{11jj}^{V,LR} + \frac{1664}{729} L_{22jj}^{V,LR} + \frac{1664}{729} L_{33jj}^{V,LR} \\
& + \frac{1448}{729} L_{11jj}^{V,RR} + \frac{1448}{729} L_{22jj}^{V,RR} + \frac{1448}{729} L_{33jj}^{V,RR} - \frac{1216}{729} L_{11ii}^{V1,LR} - \frac{1216}{729} L_{22ii}^{V1,LR} \\
& + \frac{6272}{729} L_{11ii}^{V1,RR} + \frac{6272}{729} L_{22ii}^{V1,RR} - \frac{208}{729} L_{jj11}^{V1,RR} - \frac{208}{729} L_{jj22}^{V1,RR} - \frac{112}{81} L_{jjii}^{V1,RR} \\
& + \frac{2432}{729} L_{jjjj}^{V1,LR} + \frac{2432}{729} L_{kkjj}^{V1,LR} + \frac{11872}{729} L_{jjjj}^{V,RR} + \frac{4288}{729} L_{jjkk}^{V,RR} + \frac{9088}{2187} L_{jjkk}^{V,RR} \Big] ;
\end{aligned}$$

$$\begin{aligned}
\dot{L}_{ud}^{V8,RR} &= g_s^2 \Big[ \frac{2}{3} L_{iiii}^{V8,LR} + \frac{2}{3} L_{jjii}^{V8,LR} + \frac{8}{3} L_{iiii}^{V,RR} + \frac{8}{3} L_{ijji}^{V,RR} + \frac{2}{3} L_{11jj}^{V8,LR} \\
& + \frac{2}{3} L_{22jj}^{V8,LR} + 12 L_{jjii}^{V1,RR} + \frac{2}{3} L_{11ii}^{V8,LR} + \frac{2}{3} L_{22ii}^{V8,LR} + \frac{2}{3} L_{11ii}^{V8,RR} + \frac{2}{3} L_{22ii}^{V8,RR} \\
& + \frac{2}{3} L_{jj11}^{V8,RR} + \frac{2}{3} L_{jj22}^{V8,RR} - 4 L_{jjii}^{V8,RR} + \frac{2}{3} L_{jjjj}^{V8,LR} + \frac{2}{3} L_{kkjj}^{V8,LR} + \frac{8}{3} L_{jjjj}^{V,RR} \\
& + \frac{8}{3} L_{jjkk}^{V,RR} \Big] - \frac{8}{3} L_{jjii}^{V8,RR} e^2 + \alpha_s^2 \Big[ - \frac{22}{3} L_{iiii}^{V1,LR} - \frac{22}{3} L_{jjii}^{V1,LR} + \frac{157}{81} L_{iiii}^{V8,LR} \\
& + \frac{157}{81} L_{jjii}^{V8,LR} + \frac{1918}{27} L_{iiii}^{V,RR} - \frac{28}{3} L_{ijjj}^{V,RR} + \frac{5248}{81} L_{ijji}^{V,RR} - \frac{22}{3} L_{11jj}^{V1,LR} - \frac{22}{3} L_{22jj}^{V1,LR} \\
& + \frac{157}{81} L_{11jj}^{V8,LR} + \frac{157}{81} L_{22jj}^{V8,LR} - \frac{22}{3} L_{11ii}^{V1,LR} - \frac{22}{3} L_{22ii}^{V1,LR} - \frac{2}{3} L_{11ii}^{V1,RR} - \frac{2}{3} L_{22ii}^{V1,RR} \\
& - \frac{2}{3} L_{jj11}^{V1,RR} - \frac{2}{3} L_{jj22}^{V1,RR} + \frac{41}{3} L_{jjii}^{V1,RR} + \frac{157}{81} L_{11ii}^{V8,LR} + \frac{157}{81} L_{22ii}^{V8,LR} + \frac{787}{81} L_{11ii}^{V8,RR} \\
& + \frac{787}{81} L_{22ii}^{V8,RR} + \frac{787}{81} L_{jj11}^{V8,RR} + \frac{787}{81} L_{jj22}^{V8,RR} - \frac{125}{9} L_{jjii}^{V8,RR} - \frac{22}{3} L_{jjjj}^{V1,LR} - \frac{22}{3} L_{kkjj}^{V1,LR} \\
& + \frac{157}{81} L_{jjjj}^{V8,LR} + \frac{157}{81} L_{kkjj}^{V8,LR} + \frac{1918}{27} L_{jjjj}^{V,RR} - \frac{28}{3} L_{jjkk}^{V,RR} + \frac{5248}{81} L_{jjkk}^{V,RR} \Big]
\end{aligned}$$

$$\begin{aligned}
& + \alpha_s \alpha \left[ -\frac{196}{81} L_{\overline{iii}}^{V1,LR} - \frac{196}{81} L_{\overline{jji}}^{V1,LR} + \frac{52}{27} L_{\overline{iii}}^{V8,LR} + \frac{52}{27} L_{\overline{jji}}^{V8,LR} - \frac{3152}{81} L_{\overline{iii}}^{V,RR} \right. \\
& - \frac{392}{81} L_{\overline{ijj}}^{V,RR} - \frac{5096}{243} L_{\overline{ijji}}^{V,RR} + \frac{284}{81} L_{\overline{11jj}}^{V1,LR} - \frac{496}{81} L_{\overline{22jj}}^{V1,LR} + \frac{10}{27} L_{\overline{11jj}}^{V8,LR} + \frac{4}{27} L_{\overline{22jj}}^{V8,LR} \\
& - \frac{196}{81} L_{\overline{11ii}}^{V,LR} - \frac{196}{81} L_{\overline{22ii}}^{V,LR} - \frac{196}{81} L_{\overline{33ii}}^{V,LR} - \frac{196}{81} L_{\overline{11ii}}^{V,RR} - \frac{196}{81} L_{\overline{22ii}}^{V,RR} - \frac{196}{81} L_{\overline{33ii}}^{V,RR} \\
& + \frac{284}{81} L_{\overline{11jj}}^{V,LR} + \frac{284}{81} L_{\overline{22jj}}^{V,LR} + \frac{284}{81} L_{\overline{33jj}}^{V,LR} + \frac{284}{81} L_{\overline{11jj}}^{V,RR} + \frac{284}{81} L_{\overline{22jj}}^{V,RR} + \frac{284}{81} L_{\overline{33jj}}^{V,RR} \\
& + \frac{392}{81} L_{\overline{11ii}}^{V1,LR} + \frac{392}{81} L_{\overline{22ii}}^{V1,LR} + \frac{392}{81} L_{\overline{11ii}}^{V1,RR} + \frac{392}{81} L_{\overline{22ii}}^{V1,RR} + \frac{284}{81} L_{\overline{jj11}}^{V1,RR} + \frac{284}{81} L_{\overline{jj22}}^{V1,RR} \\
& - \frac{4}{3} L_{\overline{jji}}^{V1,RR} - \frac{80}{27} L_{\overline{11ii}}^{V8,LR} - \frac{80}{27} L_{\overline{22ii}}^{V8,LR} + \frac{56}{9} L_{\overline{11ii}}^{V8,RR} + \frac{56}{9} L_{\overline{22ii}}^{V8,RR} + \frac{14}{9} L_{\overline{jj11}}^{V8,RR} \\
& + \frac{14}{9} L_{\overline{jj22}}^{V8,RR} - \frac{47}{9} L_{\overline{jjii}}^{V8,RR} - \frac{568}{81} L_{\overline{jjjj}}^{V1,LR} - \frac{568}{81} L_{\overline{kkjj}}^{V1,LR} + \frac{4}{27} L_{\overline{jjjj}}^{V8,LR} + \frac{4}{27} L_{\overline{kkjj}}^{V8,LR} \\
& \left. - \frac{4616}{81} L_{\overline{jjjj}}^{V,RR} - \frac{1136}{81} L_{\overline{jjkk}}^{V,RR} - \frac{6560}{243} L_{\overline{jjkk}}^{V,RR} \right] - \frac{112}{81} L_{\overline{jjii}}^{V8,RR} \alpha^2 ;
\end{aligned}$$

$$\begin{aligned}
\dot{L}_{\overline{ijj}}^{V,RR} &= g_s^2 \left[ -\frac{1}{18} L_{\overline{iii}}^{V8,LR} - \frac{1}{18} L_{\overline{jji}}^{V8,LR} - \frac{1}{9} L_{\overline{jjjj}}^{V8,LR} - \frac{2}{9} L_{\overline{iii}}^{V,RR} - 2 L_{\overline{ijj}}^{V,RR} \right. \\
& + \frac{52}{9} L_{\overline{ijji}}^{V,RR} - \frac{4}{9} L_{\overline{jjjj}}^{V,RR} - \frac{1}{18} L_{\overline{11ii}}^{V8,LR} - \frac{1}{18} L_{\overline{11jj}}^{V8,LR} - \frac{1}{18} L_{\overline{22ii}}^{V8,LR} - \frac{1}{18} L_{\overline{22jj}}^{V8,LR} \\
& \left. - \frac{1}{18} L_{\overline{11ii}}^{V8,RR} - \frac{1}{18} L_{\overline{11jj}}^{V8,RR} - \frac{1}{18} L_{\overline{22ii}}^{V8,RR} - \frac{1}{18} L_{\overline{22jj}}^{V8,RR} \right] + e^2 \left[ \frac{2}{9} L_{\overline{iii}}^{V1,LR} \right. \\
& + \frac{2}{9} L_{\overline{jji}}^{V1,LR} + \frac{4}{9} L_{\overline{jjjj}}^{V1,LR} + \frac{16}{27} L_{\overline{iii}}^{V,RR} + \frac{16}{9} L_{\overline{ijj}}^{V,RR} + \frac{4}{27} L_{\overline{ijji}}^{V,RR} + \frac{32}{27} L_{\overline{jjjj}}^{V,RR} \\
& + \frac{2}{9} L_{\overline{11ii}}^{V,LR} + \frac{2}{9} L_{\overline{11jj}}^{V,LR} + \frac{2}{9} L_{\overline{22ii}}^{V,LR} + \frac{2}{9} L_{\overline{22jj}}^{V,LR} + \frac{2}{9} L_{\overline{33ii}}^{V,LR} + \frac{2}{9} L_{\overline{33jj}}^{V,LR} \\
& + \frac{2}{9} L_{\overline{11ii}}^{V,RR} + \frac{2}{9} L_{\overline{11jj}}^{V,RR} + \frac{2}{9} L_{\overline{22ii}}^{V,RR} + \frac{2}{9} L_{\overline{22jj}}^{V,RR} + \frac{2}{9} L_{\overline{33ii}}^{V,RR} + \frac{2}{9} L_{\overline{33jj}}^{V,RR} \\
& - \frac{4}{9} L_{\overline{11ii}}^{V1,LR} - \frac{4}{9} L_{\overline{11jj}}^{V1,LR} - \frac{4}{9} L_{\overline{22ii}}^{V1,LR} - \frac{4}{9} L_{\overline{22jj}}^{V1,LR} - \frac{4}{9} L_{\overline{11ii}}^{V1,RR} - \frac{4}{9} L_{\overline{11jj}}^{V1,RR} \\
& \left. - \frac{4}{9} L_{\overline{22ii}}^{V1,RR} - \frac{4}{9} L_{\overline{22jj}}^{V1,RR} \right] + \alpha_s^2 \left[ -\frac{61}{18} L_{\overline{iii}}^{V1,LR} - \frac{61}{18} L_{\overline{jji}}^{V1,LR} - \frac{61}{9} L_{\overline{jjjj}}^{V1,LR} \right. \\
& - \frac{85}{972} L_{\overline{iii}}^{V8,LR} - \frac{85}{972} L_{\overline{jji}}^{V8,LR} - \frac{85}{486} L_{\overline{jjjj}}^{V8,LR} + \frac{1993}{162} L_{\overline{iii}}^{V,RR} - \frac{17}{6} L_{\overline{ijj}}^{V,RR} + \frac{3001}{486} L_{\overline{ijji}}^{V,RR} \\
& \left. - \frac{17}{6} L_{\overline{ijj}}^{V,RR} + \frac{3001}{486} L_{\overline{ijji}}^{V,RR} \right]
\end{aligned}$$

$$\begin{aligned}
& + \frac{9925}{486} L_{jjjj}^{V,RR} - \frac{61}{18} L_{11ii}^{V1,LR} - \frac{61}{18} L_{11jj}^{V1,LR} - \frac{61}{18} L_{22ii}^{V1,LR} - \frac{61}{18} L_{22jj}^{V1,LR} + \frac{73}{18} L_{11ii}^{V1,RR} \\
& + \frac{73}{18} L_{11jj}^{V1,RR} + \frac{73}{18} L_{22ii}^{V1,RR} + \frac{73}{18} L_{22jj}^{V1,RR} - \frac{85}{972} L_{11ii}^{V8,LR} - \frac{85}{972} L_{11jj}^{V8,LR} - \frac{85}{972} L_{22ii}^{V8,LR} \\
& - \frac{85}{972} L_{22jj}^{V8,LR} - \frac{715}{972} L_{11ii}^{V8,RR} - \frac{715}{972} L_{11jj}^{V8,RR} - \frac{715}{972} L_{22ii}^{V8,RR} - \frac{715}{972} L_{22jj}^{V8,RR} \Big] \\
& + \alpha_s \alpha \left[ \frac{238}{243} L_{iiii}^{V1,LR} + \frac{238}{243} L_{jjii}^{V1,LR} + \frac{476}{243} L_{jjjj}^{V1,LR} - \frac{797}{1458} L_{iiii}^{V8,LR} - \frac{797}{1458} L_{jjii}^{V8,LR} \right. \\
& - \frac{797}{729} L_{jjjj}^{V8,LR} + \frac{313}{243} L_{dd}^{V,RR} - \frac{1522}{243} L_{ijjj}^{V,RR} - \frac{6740}{729} L_{ijjj}^{V,RR} + \frac{1621}{729} L_{jjjj}^{V,RR} \\
& + \frac{22}{243} L_{11ii}^{V,LR} + \frac{22}{243} L_{11jj}^{V,LR} + \frac{22}{243} L_{22ii}^{V,LR} + \frac{22}{243} L_{22jj}^{V,LR} + \frac{22}{243} L_{33ii}^{V,LR} + \frac{22}{243} L_{33jj}^{V,LR} \\
& + \frac{22}{243} L_{11ii}^{V,RR} + \frac{22}{243} L_{11jj}^{V,RR} + \frac{22}{243} L_{22ii}^{V,RR} + \frac{22}{243} L_{22jj}^{V,RR} + \frac{22}{243} L_{33ii}^{V,RR} + \frac{22}{243} L_{33jj}^{V,RR} \\
& - \frac{476}{243} L_{11ii}^{V1,LR} - \frac{476}{243} L_{11jj}^{V1,LR} - \frac{476}{243} L_{22ii}^{V1,LR} - \frac{476}{243} L_{22jj}^{V1,LR} - \frac{476}{243} L_{11ii}^{V1,RR} \\
& - \frac{476}{243} L_{11jj}^{V1,RR} - \frac{476}{243} L_{22ii}^{V1,RR} - \frac{476}{243} L_{22jj}^{V1,RR} + \frac{715}{1458} L_{11ii}^{V8,LR} + \frac{715}{1458} L_{11jj}^{V8,LR} \\
& + \frac{715}{1458} L_{22ii}^{V8,LR} + \frac{715}{1458} L_{22jj}^{V8,LR} + \frac{103}{1458} L_{11ii}^{V8,RR} + \frac{103}{1458} L_{11jj}^{V8,RR} + \frac{103}{1458} L_{22ii}^{V8,RR} \\
& + \frac{103}{1458} L_{22jj}^{V8,RR} \Big] + \alpha^2 \left[ - \frac{368}{729} L_{iiii}^{V1,LR} - \frac{368}{729} L_{jjii}^{V1,LR} - \frac{736}{729} L_{jjjj}^{V1,LR} + \frac{608}{729} L_{iiii}^{V,RR} \right. \\
& + \frac{614}{729} L_{ijjj}^{V,RR} + \frac{296}{2187} L_{ijjj}^{V,RR} + \frac{2936}{2187} L_{jjjj}^{V,RR} - \frac{656}{729} L_{11ii}^{V,LR} - \frac{656}{729} L_{11jj}^{V,LR} \\
& - \frac{656}{729} L_{22ii}^{V,LR} - \frac{656}{729} L_{22jj}^{V,LR} - \frac{656}{729} L_{33ii}^{V,LR} - \frac{656}{729} L_{33jj}^{V,LR} + \frac{856}{729} L_{11ii}^{V,RR} + \frac{856}{729} L_{11jj}^{V,RR} \\
& + \frac{856}{729} L_{22ii}^{V,RR} + \frac{856}{729} L_{22jj}^{V,RR} + \frac{856}{729} L_{33ii}^{V,RR} + \frac{856}{729} L_{33jj}^{V,RR} - \frac{1748}{729} L_{11ii}^{V1,LR} \\
& - \frac{1748}{729} L_{11jj}^{V1,LR} - \frac{1748}{729} L_{22ii}^{V1,LR} - \frac{1748}{729} L_{22jj}^{V1,LR} + \frac{268}{729} L_{11ii}^{V1,RR} + \frac{268}{729} L_{11jj}^{V1,RR} \\
& + \frac{268}{729} L_{22ii}^{V1,RR} + \frac{268}{729} L_{22jj}^{V1,RR} \Big] ;
\end{aligned}$$

$$\dot{L}_{ijji}^{V,RR} = g_s^2 \left[ \frac{1}{6} L_{jjii}^{V8,LR} + 6 L_{ijjj}^{V,RR} - \frac{4}{3} L_{ijji}^{V,RR} + \frac{1}{6} L_{iiii}^{V8,LR} + \frac{2}{3} L_{iiii}^{V,RR} \right]$$



$$\begin{aligned}
& + \frac{1}{6} L_{11ii}^{V8,LR} + \frac{1}{6} L_{22ii}^{V8,LR} + \frac{1}{6} L_{11ii}^{V8,RR} + \frac{1}{6} L_{22ii}^{V8,RR} + \frac{1}{3} L_{jjjj}^{V8,LR} + \frac{4}{3} L_{jjjj}^{V,RR} \\
& + \frac{1}{6} L_{11jj}^{V8,LR} + \frac{1}{6} L_{22jj}^{V8,LR} + \frac{1}{6} L_{11jj}^{V8,RR} + \frac{1}{6} L_{22jj}^{V8,RR} \Big] + \frac{4}{3} e^2 L_{ijji}^{V,RR} + \alpha_s^2 \Big[ - \frac{11}{6} L_{jjii}^{V1,LR} \\
& + \frac{157}{324} L_{jjii}^{V8,LR} + \frac{9}{2} L_{ijji}^{V,RR} + \frac{743}{162} L_{ijji}^{V,RR} - \frac{11}{6} L_{iiii}^{V1,LR} + \frac{157}{324} L_{iiii}^{V8,LR} + \frac{959}{54} L_{iiii}^{V,RR} \\
& - \frac{11}{6} L_{11ii}^{V1,LR} - \frac{11}{6} L_{22ii}^{V1,LR} - \frac{1}{6} L_{11ii}^{V1,RR} - \frac{1}{6} L_{22ii}^{V1,RR} + \frac{157}{324} L_{11ii}^{V8,LR} + \frac{157}{324} L_{22ii}^{V8,LR} \\
& + \frac{787}{324} L_{11ii}^{V8,RR} + \frac{787}{324} L_{22ii}^{V8,RR} - \frac{11}{3} L_{jjjj}^{V1,LR} + \frac{157}{162} L_{jjjj}^{V8,LR} + \frac{5123}{162} L_{jjjj}^{V,RR} \\
& - \frac{11}{6} L_{11jj}^{V1,LR} - \frac{11}{6} L_{22jj}^{V1,LR} - \frac{1}{6} L_{11jj}^{V1,RR} - \frac{1}{6} L_{22jj}^{V1,RR} + \frac{157}{324} L_{11jj}^{V8,LR} + \frac{157}{324} L_{22jj}^{V8,LR} \\
& + \frac{787}{324} L_{11jj}^{V8,RR} + \frac{787}{324} L_{22jj}^{V8,RR} \Big] + \alpha_s \alpha \Big[ - \frac{22}{81} L_{jjii}^{V1,LR} - \frac{25}{54} L_{jjii}^{V8,LR} - \frac{746}{81} L_{ijji}^{V,RR} \\
& - \frac{1436}{243} L_{ijji}^{V,RR} - \frac{22}{81} L_{iiii}^{V1,LR} - \frac{25}{54} L_{iiii}^{V8,LR} + \frac{211}{81} L_{iiii}^{V,RR} - \frac{22}{81} L_{11ii}^{V,LR} - \frac{22}{81} L_{22ii}^{V,LR} \\
& - \frac{22}{81} L_{33ii}^{V,LR} - \frac{22}{81} L_{ed}^{V,RR} - \frac{22}{81} L_{ed}^{V,RR} - \frac{22}{81} L_{ed}^{V,RR} + \frac{44}{81} L_{11ii}^{V1,LR} + \frac{44}{81} L_{22ii}^{V1,LR} \\
& + \frac{44}{81} L_{11ii}^{V1,RR} + \frac{44}{81} L_{22ii}^{V1,RR} + \frac{71}{54} L_{11ii}^{V8,LR} + \frac{71}{54} L_{22ii}^{V8,LR} - \frac{7}{18} L_{11ii}^{V8,RR} - \frac{7}{18} L_{22ii}^{V8,RR} \\
& - \frac{44}{81} L_{jjjj}^{V1,LR} - \frac{25}{27} L_{jjjj}^{V8,LR} + \frac{955}{243} L_{jjjj}^{V,RR} - \frac{22}{81} L_{11jj}^{V,LR} - \frac{22}{81} L_{22jj}^{V,LR} - \frac{22}{81} L_{33jj}^{V,LR} \\
& - \frac{22}{81} L_{11jj}^{V,RR} - \frac{22}{81} L_{22jj}^{V,RR} - \frac{22}{81} L_{33jj}^{V,RR} + \frac{44}{81} L_{11jj}^{V1,LR} + \frac{44}{81} L_{22jj}^{V1,LR} + \frac{44}{81} L_{11jj}^{V1,RR} \\
& + \frac{44}{81} L_{22jj}^{V1,RR} + \frac{71}{54} L_{11jj}^{V8,LR} + \frac{71}{54} L_{22jj}^{V8,LR} - \frac{7}{18} L_{11jj}^{V8,RR} - \frac{7}{18} L_{22jj}^{V8,RR} \Big] + \frac{38}{81} \alpha^2 L_{ijji}^{V,RR} ;
\end{aligned}$$

$$\begin{aligned}
\dot{L}_{dd}^{V,RR} & = g_s^2 \Big[ \frac{2}{9} L_{jjii}^{V8,LR} + \frac{8}{9} L_{ijji}^{V,RR} + \frac{2}{9} L_{iiii}^{V8,LR} + \frac{44}{9} L_{iiii}^{V,RR} + \frac{2}{9} L_{11ii}^{V8,LR} \\
& + \frac{2}{9} L_{22ii}^{V8,LR} + \frac{2}{9} L_{11ii}^{V8,RR} + \frac{2}{9} L_{22ii}^{V8,RR} \Big] + e^2 \Big[ \frac{4}{9} L_{jjii}^{V1,LR} + \frac{8}{9} L_{ijji}^{V,RR} \\
& + \frac{8}{27} L_{ijji}^{V,RR} + \frac{4}{9} L_{iiii}^{V1,LR} + \frac{68}{27} L_{iiii}^{V,RR} + \frac{4}{9} L_{11ii}^{V,LR} + \frac{4}{9} L_{22ii}^{V,LR} + \frac{4}{9} L_{33ii}^{V,LR} \\
& + \frac{4}{9} L_{11ii}^{V,RR} + \frac{4}{9} L_{22ii}^{V,RR} + \frac{4}{9} L_{33ii}^{V,RR} - \frac{8}{9} L_{11ii}^{V1,LR} - \frac{8}{9} L_{22ii}^{V1,LR} - \frac{8}{9} L_{11ii}^{V1,RR}
\end{aligned}$$

$$\begin{aligned}
& -\frac{8}{9}L_{22ii}^{V1,RR} \Big] + \alpha_s^2 \Big[ -\frac{94}{9}L_{jjii}^{V1,LR} + \frac{193}{243}L_{jjii}^{V8,LR} + \frac{116}{9}L_{ijjj}^{V,RR} + \frac{7552}{243}L_{ijji}^{V,RR} \\
& -\frac{94}{9}L_{iiii}^{V1,LR} + \frac{193}{243}L_{iiii}^{V8,LR} + \frac{4483}{81}L_{iiii}^{V,RR} - \frac{94}{9}L_{11ii}^{V1,LR} - \frac{94}{9}L_{22ii}^{V1,LR} + \frac{70}{9}L_{11ii}^{V1,RR} \\
& + \frac{70}{9}L_{22ii}^{V1,RR} + \frac{193}{243}L_{11ii}^{V8,LR} + \frac{193}{243}L_{22ii}^{V8,LR} + \frac{823}{243}L_{11ii}^{V8,RR} + \frac{823}{243}L_{22ii}^{V8,RR} \Big] \\
& + \alpha_s \alpha \Big[ \frac{344}{243}L_{jjii}^{V1,LR} - \frac{1472}{729}L_{jjii}^{V8,LR} + \frac{472}{243}L_{ijjj}^{V,RR} + \frac{1880}{729}L_{ijji}^{V,RR} + \frac{344}{243}L_{iiii}^{V1,LR} \\
& - \frac{1472}{729}L_{iiii}^{V8,LR} - \frac{2104}{243}L_{iiii}^{V,RR} - \frac{88}{243}L_{11ii}^{V,LR} - \frac{88}{243}L_{22ii}^{V,LR} - \frac{88}{243}L_{33ii}^{V,LR} - \frac{88}{243}L_{11ii}^{V,RR} \\
& - \frac{88}{243}L_{22ii}^{V,RR} - \frac{88}{243}L_{33ii}^{V,RR} - \frac{688}{243}L_{11ii}^{V1,LR} - \frac{688}{243}L_{22ii}^{V1,LR} - \frac{688}{243}L_{11ii}^{V1,RR} \\
& - \frac{688}{243}L_{22ii}^{V1,RR} + \frac{2632}{729}L_{11ii}^{V8,LR} + \frac{2632}{729}L_{22ii}^{V8,LR} - \frac{464}{729}L_{11ii}^{V8,RR} - \frac{464}{729}L_{22ii}^{V8,RR} \Big] \\
& + \alpha^2 \Big[ -\frac{736}{729}L_{jjii}^{V1,LR} + \frac{544}{729}L_{ijjj}^{V,RR} + \frac{592}{2187}L_{ijji}^{V,RR} - \frac{736}{729}L_{iiii}^{V1,LR} + \frac{1558}{729}L_{iiii}^{V,RR} \\
& - \frac{1312}{729}L_{11ii}^{V,LR} - \frac{1312}{729}L_{22ii}^{V,LR} - \frac{1312}{729}L_{33ii}^{V,LR} + \frac{1712}{729}L_{11ii}^{V,RR} + \frac{1712}{729}L_{22ii}^{V,RR} \\
& + \frac{1712}{729}L_{33ii}^{V,RR} - \frac{3496}{729}L_{11ii}^{V1,LR} - \frac{3496}{729}L_{22ii}^{V1,LR} + \frac{536}{729}L_{11ii}^{V1,RR} + \frac{536}{729}L_{22ii}^{V1,RR} \Big] ;
\end{aligned}$$

$$\begin{aligned}
\dot{L}_{ijjj}^{V,RR} &= g_s^2 \Big[ -\frac{1}{18}L_{11ii}^{V8,LR} - \frac{1}{18}L_{11jj}^{V8,LR} - \frac{1}{18}L_{22ii}^{V8,LR} - \frac{1}{18}L_{22jj}^{V8,LR} - \frac{1}{18}L_{ii11}^{V8,RR} \\
& - \frac{1}{18}L_{ii22}^{V8,RR} - \frac{1}{18}L_{jj11}^{V8,RR} - \frac{1}{18}L_{jj22}^{V8,RR} - \frac{1}{18}L_{iiii}^{V8,LR} - \frac{1}{18}L_{jjjj}^{V8,LR} - \frac{1}{18}L_{kkii}^{V8,LR} \\
& - \frac{1}{18}L_{kkjj}^{V8,LR} - \frac{2}{9}L_{iiii}^{V,RR} - 2L_{ijjj}^{V,RR} + 6L_{ijji}^{V,RR} - \frac{2}{9}L_{ikki}^{V,RR} - \frac{2}{9}L_{jjjj}^{V,RR} \\
& - \frac{2}{9}L_{jjkk}^{V,RR} \Big] + e^2 \Big[ -\frac{4}{9}L_{11ii}^{V1,LR} - \frac{4}{9}L_{11jj}^{V1,LR} - \frac{4}{9}L_{22ii}^{V1,LR} - \frac{4}{9}L_{22jj}^{V1,LR} \\
& - \frac{4}{9}L_{11ii}^{V,LR} - \frac{4}{9}L_{11jj}^{V,LR} - \frac{4}{9}L_{22ii}^{V,LR} - \frac{4}{9}L_{22jj}^{V,LR} - \frac{4}{9}L_{33ii}^{V,LR} - \frac{4}{9}L_{33jj}^{V,LR} \\
& - \frac{4}{9}L_{11ii}^{V,RR} - \frac{4}{9}L_{11jj}^{V,RR} - \frac{4}{9}L_{22ii}^{V,RR} - \frac{4}{9}L_{22jj}^{V,RR} - \frac{4}{9}L_{33ii}^{V,RR} - \frac{4}{9}L_{33jj}^{V,RR}
\end{aligned}$$

$$\begin{aligned}
& -\frac{4}{9}L_{\frac{ud}{ii11}}^{V1,RR} - \frac{4}{9}L_{\frac{ud}{ii22}}^{V1,RR} - \frac{4}{9}L_{\frac{ud}{jj11}}^{V1,RR} - \frac{4}{9}L_{\frac{ud}{jj22}}^{V1,RR} + \frac{8}{9}L_{\frac{uu}{iii}}^{V1,LR} + \frac{8}{9}L_{\frac{uu}{jjj}}^{V1,LR} \\
& + \frac{8}{9}L_{\frac{uu}{kkii}}^{V1,LR} + \frac{8}{9}L_{\frac{uu}{kkjj}}^{V1,LR} + \frac{64}{27}L_{\frac{uu}{iii}}^{V,RR} + \frac{16}{3}L_{\frac{uu}{ijj}}^{V,RR} + \frac{16}{9}L_{\frac{uu}{ikk}}^{V,RR} + \frac{16}{27}L_{\frac{uu}{ikki}}^{V,RR} \\
& + \frac{64}{27}L_{\frac{uu}{jjjj}}^{V,RR} + \frac{16}{9}L_{\frac{uu}{jjkk}}^{V,RR} + \frac{16}{27}L_{\frac{uu}{jkkj}}^{V,RR} \Big] + \alpha_s^2 \Bigg[ -\frac{61}{18}L_{\frac{du}{11ii}}^{V1,LR} - \frac{61}{18}L_{\frac{du}{11jj}}^{V1,LR} \\
& - \frac{61}{18}L_{\frac{du}{22ii}}^{V1,LR} - \frac{61}{18}L_{\frac{du}{22jj}}^{V1,LR} - \frac{85}{972}L_{\frac{du}{11ii}}^{V8,LR} - \frac{85}{972}L_{\frac{du}{11jj}}^{V8,LR} - \frac{85}{972}L_{\frac{du}{22ii}}^{V8,LR} - \frac{85}{972}L_{\frac{du}{22jj}}^{V8,LR} \\
& + \frac{73}{18}L_{\frac{ud}{ii11}}^{V1,RR} + \frac{73}{18}L_{\frac{ud}{ii22}}^{V1,RR} + \frac{73}{18}L_{\frac{ud}{jj11}}^{V1,RR} + \frac{73}{18}L_{\frac{ud}{jj22}}^{V1,RR} - \frac{715}{972}L_{\frac{ud}{ii11}}^{V8,RR} - \frac{715}{972}L_{\frac{ud}{ii22}}^{V8,RR} \\
& - \frac{715}{972}L_{\frac{ud}{jj11}}^{V8,RR} - \frac{715}{972}L_{\frac{ud}{jj22}}^{V8,RR} - \frac{61}{18}L_{\frac{uu}{iii}}^{V1,LR} - \frac{61}{18}L_{\frac{uu}{jjj}}^{V1,LR} - \frac{61}{18}L_{\frac{uu}{kkii}}^{V1,LR} - \frac{61}{18}L_{\frac{uu}{kkjj}}^{V1,LR} \\
& - \frac{85}{972}L_{\frac{uu}{iii}}^{V8,LR} - \frac{85}{972}L_{\frac{uu}{jjj}}^{V8,LR} - \frac{85}{972}L_{\frac{uu}{kkii}}^{V8,LR} - \frac{85}{972}L_{\frac{uu}{kkjj}}^{V8,LR} + \frac{1993}{162}L_{\frac{uu}{iii}}^{V,RR} \\
& - \frac{209}{18}L_{\frac{uu}{ijj}}^{V,RR} + \frac{79}{9}L_{\frac{uu}{ikk}}^{V,RR} + \frac{41}{6}L_{\frac{uu}{ijji}}^{V,RR} - \frac{160}{243}L_{\frac{uu}{ikki}}^{V,RR} + \frac{1993}{162}L_{\frac{uu}{jjjj}}^{V,RR} + \frac{79}{9}L_{\frac{uu}{jjkk}}^{V,RR} \\
& - \frac{160}{243}L_{\frac{uu}{jkkj}}^{V,RR} \Big] + \alpha_s \alpha \Bigg[ -\frac{476}{243}L_{\frac{du}{11ii}}^{V1,LR} - \frac{476}{243}L_{\frac{du}{11jj}}^{V1,LR} + \frac{934}{243}L_{\frac{du}{22ii}}^{V1,LR} + \frac{934}{243}L_{\frac{du}{22jj}}^{V1,LR} \\
& + \frac{79}{1458}L_{\frac{du}{11ii}}^{V8,LR} + \frac{79}{1458}L_{\frac{du}{11jj}}^{V8,LR} - \frac{1594}{729}L_{\frac{du}{22ii}}^{V8,LR} - \frac{1594}{729}L_{\frac{du}{22jj}}^{V8,LR} - \frac{44}{243}L_{\frac{eu}{11ii}}^{V,LR} \\
& - \frac{44}{243}L_{\frac{eu}{11jj}}^{V,LR} - \frac{44}{243}L_{\frac{eu}{22ii}}^{V,LR} - \frac{44}{243}L_{\frac{eu}{22jj}}^{V,LR} - \frac{44}{243}L_{\frac{eu}{33ii}}^{V,LR} - \frac{44}{243}L_{\frac{eu}{33jj}}^{V,LR} - \frac{44}{243}L_{\frac{eu}{11ii}}^{V,RR} \\
& - \frac{44}{243}L_{\frac{eu}{11jj}}^{V,RR} - \frac{44}{243}L_{\frac{eu}{22ii}}^{V,RR} - \frac{44}{243}L_{\frac{eu}{22jj}}^{V,RR} - \frac{44}{243}L_{\frac{eu}{33ii}}^{V,RR} - \frac{44}{243}L_{\frac{eu}{33jj}}^{V,RR} - \frac{476}{243}L_{\frac{ud}{ii11}}^{V1,RR} \\
& - \frac{476}{243}L_{\frac{ud}{ii22}}^{V1,RR} - \frac{476}{243}L_{\frac{ud}{jj11}}^{V1,RR} - \frac{476}{243}L_{\frac{ud}{jj22}}^{V1,RR} - \frac{533}{1458}L_{\frac{ud}{ii11}}^{V8,RR} - \frac{533}{1458}L_{\frac{ud}{ii22}}^{V8,RR} \\
& - \frac{533}{1458}L_{\frac{ud}{jj11}}^{V8,RR} - \frac{533}{1458}L_{\frac{ud}{jj22}}^{V8,RR} + \frac{952}{243}L_{\frac{uu}{iii}}^{V1,LR} + \frac{952}{243}L_{\frac{uu}{jjj}}^{V1,LR} + \frac{952}{243}L_{\frac{uu}{kkii}}^{V1,LR} \\
& + \frac{952}{243}L_{\frac{uu}{kkjj}}^{V1,LR} - \frac{1594}{729}L_{\frac{uu}{iii}}^{V8,LR} - \frac{1594}{729}L_{\frac{uu}{jjj}}^{V8,LR} - \frac{1594}{729}L_{\frac{uu}{kkii}}^{V8,LR} - \frac{1594}{729}L_{\frac{uu}{kkjj}}^{V8,LR} \\
& + \frac{1252}{243}L_{\frac{uu}{iii}}^{V,RR} - \frac{280}{9}L_{\frac{uu}{ijj}}^{V,RR} + \frac{1472}{243}L_{\frac{uu}{ikk}}^{V,RR} - \frac{104}{3}L_{\frac{uu}{ijji}}^{V,RR} - \frac{1688}{729}L_{\frac{uu}{ikki}}^{V,RR} + \frac{1252}{243}L_{\frac{uu}{jjjj}}^{V,RR} \\
& + \frac{1472}{243}L_{\frac{uu}{jjkk}}^{V,RR} - \frac{1688}{729}L_{\frac{uu}{jkkj}}^{V,RR} \Big] + \alpha^2 \Bigg[ -\frac{1052}{729}L_{\frac{du}{11ii}}^{V1,LR} - \frac{1052}{729}L_{\frac{du}{11jj}}^{V1,LR} - \frac{6176}{729}L_{\frac{du}{22ii}}^{V1,LR}
\end{aligned}$$

$$\begin{aligned}
& -\frac{6176}{729}L_{22jj}^{V1,LR} - \frac{4796}{729}L_{11ii}^{V,LR} - \frac{4796}{729}L_{11jj}^{V,LR} - \frac{4796}{729}L_{22ii}^{V,LR} - \frac{4796}{729}L_{22jj}^{V,LR} \\
& - \frac{4796}{729}L_{33ii}^{V,LR} - \frac{4796}{729}L_{33jj}^{V,LR} + \frac{1252}{729}L_{11ii}^{V,RR} + \frac{1252}{729}L_{11jj}^{V,RR} + \frac{1252}{729}L_{22ii}^{V,RR} \\
& + \frac{1252}{729}L_{22jj}^{V,RR} + \frac{1252}{729}L_{33ii}^{V,RR} + \frac{1252}{729}L_{33jj}^{V,RR} + \frac{964}{729}L_{ii11}^{V1,RR} + \frac{964}{729}L_{ii22}^{V1,RR} \\
& + \frac{964}{729}L_{jj11}^{V1,RR} + \frac{964}{729}L_{jj22}^{V1,RR} - \frac{5888}{729}L_{iii}^{V1,LR} - \frac{5888}{729}L_{jjj}^{V1,LR} - \frac{5888}{729}L_{kkii}^{V1,LR} \\
& - \frac{5888}{729}L_{kkjj}^{V1,LR} + \frac{9728}{729}L_{iii}^{V,RR} - \frac{1216}{81}L_{ijj}^{V,RR} + \frac{4352}{729}L_{iik}^{V,RR} + \frac{4736}{2187}L_{ikk}^{V,RR} \\
& + \frac{9728}{729}L_{jjj}^{V,RR} + \frac{4352}{729}L_{jjk}^{V,RR} + \frac{4736}{2187}L_{jkk}^{V,RR} \Big] ;
\end{aligned}$$

$$\begin{aligned}
\dot{L}_{ijji}^{V,RR} &= g_s^2 \Bigg[ \frac{1}{6}L_{11ii}^{V8,LR} + \frac{1}{6}L_{11jj}^{V8,LR} + \frac{1}{6}L_{22ii}^{V8,LR} + \frac{1}{6}L_{22jj}^{V8,LR} + \frac{1}{6}L_{ii11}^{V8,RR} \\
& + \frac{1}{6}L_{ii22}^{V8,RR} + \frac{1}{6}L_{jj11}^{V8,RR} + \frac{1}{6}L_{jj22}^{V8,RR} + \frac{1}{6}L_{iii}^{V8,LR} + \frac{1}{6}L_{jjj}^{V8,LR} + \frac{1}{6}L_{kkii}^{V8,LR} \\
& + \frac{1}{6}L_{kkjj}^{V8,LR} + \frac{2}{3}L_{iii}^{V,RR} + 6L_{ijj}^{V,RR} - 2L_{ijji}^{V,RR} + \frac{2}{3}L_{iik}^{V,RR} + \frac{2}{3}L_{jjj}^{V,RR} \\
& + \frac{2}{3}L_{jkk}^{V,RR} \Big] + \frac{16}{3}L_{ijji}^{V,RR}e^2 + \alpha_s^2 \Bigg[ -\frac{11}{6}L_{11ii}^{V1,LR} - \frac{11}{6}L_{11jj}^{V1,LR} - \frac{11}{6}L_{22ii}^{V1,LR} \\
& - \frac{11}{6}L_{22jj}^{V1,LR} + \frac{157}{324}L_{11ii}^{V8,LR} + \frac{157}{324}L_{11jj}^{V8,LR} + \frac{157}{324}L_{22ii}^{V8,LR} + \frac{157}{324}L_{22jj}^{V8,LR} \\
& - \frac{1}{6}L_{ii11}^{V1,RR} - \frac{1}{6}L_{ii22}^{V1,RR} - \frac{1}{6}L_{jj11}^{V1,RR} - \frac{1}{6}L_{jj22}^{V1,RR} + \frac{787}{324}L_{ii11}^{V8,RR} + \frac{787}{324}L_{ii22}^{V8,RR} \\
& + \frac{787}{324}L_{jj11}^{V8,RR} + \frac{787}{324}L_{jj22}^{V8,RR} - \frac{11}{6}L_{iii}^{V1,LR} - \frac{11}{6}L_{jjj}^{V1,LR} - \frac{11}{6}L_{kkii}^{V1,LR} - \frac{11}{6}L_{kkjj}^{V1,LR} \\
& + \frac{157}{324}L_{iii}^{V8,LR} + \frac{157}{324}L_{jjj}^{V8,LR} + \frac{157}{324}L_{kkii}^{V8,LR} + \frac{157}{324}L_{kkjj}^{V8,LR} + \frac{959}{54}L_{iii}^{V,RR} \\
& + \frac{41}{6}L_{ijj}^{V,RR} - \frac{7}{3}L_{iik}^{V,RR} - \frac{209}{18}L_{ijji}^{V,RR} + \frac{1312}{81}L_{iik}^{V,RR} + \frac{959}{54}L_{jjj}^{V,RR} - \frac{7}{3}L_{jkk}^{V,RR} \\
& + \frac{1312}{81}L_{jkk}^{V,RR} \Big] + \alpha_s \alpha \Bigg[ \frac{44}{81}L_{11ii}^{V1,LR} + \frac{44}{81}L_{11jj}^{V1,LR} - \frac{70}{81}L_{22ii}^{V1,LR} - \frac{70}{81}L_{22jj}^{V1,LR} \\
& + \frac{65}{54}L_{11ii}^{V8,LR} + \frac{65}{54}L_{11jj}^{V8,LR} - \frac{50}{27}L_{22ii}^{V8,LR} - \frac{50}{27}L_{22jj}^{V8,LR} + \frac{44}{81}L_{11ii}^{V,LR} + \frac{44}{81}L_{11jj}^{V,LR}
\end{aligned}$$

$$\begin{aligned}
& + \frac{44}{81} L_{22ii}^{V,LR} + \frac{44}{81} L_{22jj}^{V,LR} + \frac{44}{81} L_{33ii}^{V,LR} + \frac{44}{81} L_{33jj}^{V,LR} + \frac{44}{81} L_{11ii}^{V,RR} + \frac{44}{81} L_{11jj}^{V,RR} \\
& + \frac{44}{81} L_{22ii}^{V,RR} + \frac{44}{81} L_{22jj}^{V,RR} + \frac{44}{81} L_{33ii}^{V,RR} + \frac{44}{81} L_{33jj}^{V,RR} + \frac{44}{81} L_{ii11}^{V1,RR} + \frac{44}{81} L_{ii22}^{V1,RR} \\
& + \frac{44}{81} L_{jj11}^{V1,RR} + \frac{44}{81} L_{jj22}^{V1,RR} - \frac{1}{2} L_{ii11}^{V8,RR} - \frac{1}{2} L_{ii22}^{V8,RR} - \frac{1}{2} L_{jj11}^{V8,RR} - \frac{1}{2} L_{jj22}^{V8,RR} \\
& - \frac{88}{81} L_{iii}^{V1,LR} - \frac{88}{81} L_{jjj}^{V1,LR} - \frac{88}{81} L_{kkii}^{V1,LR} - \frac{88}{81} L_{kkjj}^{V1,LR} - \frac{50}{27} L_{iii}^{V8,LR} - \frac{50}{27} L_{jjj}^{V8,LR} \\
& - \frac{50}{27} L_{kkii}^{V8,LR} - \frac{50}{27} L_{kkjj}^{V8,LR} + \frac{844}{81} L_{iii}^{V,RR} - \frac{104}{3} L_{ijj}^{V,RR} - \frac{176}{81} L_{ikk}^{V,RR} - \frac{280}{9} L_{ijji}^{V,RR} \\
& + \frac{1816}{243} L_{uu}^{V,RR} + \frac{844}{81} L_{jjj}^{V,RR} - \frac{176}{81} L_{jjkk}^{V,RR} + \frac{1816}{243} L_{jkkj}^{V,RR} \Big] - \frac{1216}{81} L_{ijji}^{V,RR}
\end{aligned}$$

$$\alpha^2 ;$$

$$\begin{aligned}
\dot{L}_{uu}^{V,RR} &= g_s^2 \left[ \frac{2}{9} L_{kkii}^{V8,LR} + \frac{8}{9} L_{ikk}^{V,RR} + \frac{2}{9} L_{11ii}^{V8,LR} + \frac{2}{9} L_{22ii}^{V8,LR} + \frac{2}{9} L_{ii11}^{V8,RR} \right. \\
& + \frac{2}{9} L_{ii22}^{V8,RR} + \frac{2}{9} L_{iii}^{V8,LR} + \frac{44}{9} L_{iii}^{V,RR} \Big] + e^2 \left[ \frac{16}{9} L_{kkii}^{V1,LR} + \frac{32}{9} L_{ikk}^{V,RR} \right. \\
& + \frac{32}{27} L_{ikk}^{V,RR} - \frac{8}{9} L_{11ii}^{V1,LR} - \frac{8}{9} L_{22ii}^{V1,LR} - \frac{8}{9} L_{11ii}^{V,LR} - \frac{8}{9} L_{22ii}^{V,LR} - \frac{8}{9} L_{33ii}^{V,LR} \\
& - \frac{8}{9} L_{11ii}^{V,RR} - \frac{8}{9} L_{22ii}^{V,RR} - \frac{8}{9} L_{33ii}^{V,RR} - \frac{8}{9} L_{ii11}^{V1,RR} - \frac{8}{9} L_{ii22}^{V1,RR} + \frac{16}{9} L_{iii}^{V1,LR} \\
& + \frac{272}{27} L_{iii}^{V,RR} \Big] + \alpha_s^2 \left[ -\frac{94}{9} L_{kkii}^{V1,LR} + \frac{193}{243} L_{kkii}^{V8,LR} + \frac{116}{9} L_{ikk}^{V,RR} + \frac{7552}{243} L_{ikk}^{V,RR} \right. \\
& - \frac{94}{9} L_{11ii}^{V1,LR} - \frac{94}{9} L_{22ii}^{V1,LR} + \frac{193}{243} L_{11ii}^{V8,LR} + \frac{193}{243} L_{22ii}^{V8,LR} + \frac{70}{9} L_{ii11}^{V1,RR} + \frac{70}{9} L_{ii22}^{V1,RR} \\
& + \frac{823}{243} L_{ii11}^{V8,RR} + \frac{823}{243} L_{ii22}^{V8,RR} - \frac{94}{9} L_{iii}^{V1,LR} + \frac{193}{243} L_{iii}^{V8,LR} + \frac{4483}{81} L_{iii}^{V,RR} \Big] \\
& + \alpha_s \alpha \left[ \frac{1376}{243} L_{kkii}^{V1,LR} - \frac{5888}{729} L_{kkii}^{V8,LR} + \frac{1888}{243} L_{ikk}^{V,RR} + \frac{7520}{729} L_{ikk}^{V,RR} - \frac{688}{243} L_{11ii}^{V1,LR} \right. \\
& + \frac{1448}{243} L_{22ii}^{V1,LR} + \frac{1834}{729} L_{11ii}^{V8,LR} - \frac{5888}{729} L_{22ii}^{V8,LR} + \frac{176}{243} L_{11ii}^{V,LR} + \frac{176}{243} L_{22ii}^{V,LR} \\
& + \frac{176}{243} L_{33ii}^{V,LR} + \frac{176}{243} L_{11ii}^{V,RR} + \frac{176}{243} L_{22ii}^{V,RR} + \frac{176}{243} L_{33ii}^{V,RR} - \frac{688}{243} L_{ii11}^{V1,RR}
\end{aligned}$$

$$\begin{aligned}
& -\frac{688}{243}L_{ud\ ii22}^{V1,RR} - \frac{1262}{729}L_{ud\ ii11}^{V8,RR} - \frac{1262}{729}L_{ud\ ii22}^{V8,RR} + \frac{1376}{243}L_{uu\ iiii}^{V1,LR} - \frac{5888}{729}L_{uu\ iiii}^{V8,LR} \\
& - \frac{8416}{243}L_{uu\ iiii}^{V,RR} \Big] + \alpha^2 \Bigg[ -\frac{11776}{729}L_{uu\ kkii}^{V1,LR} + \frac{8704}{729}L_{uu\ iikk}^{V,RR} + \frac{9472}{2187}L_{uu\ ikki}^{V,RR} - \frac{2104}{729}L_{du\ 11ii}^{V1,LR} \\
& - \frac{12352}{729}L_{du\ 22ii}^{V1,LR} - \frac{9592}{729}L_{eu\ 11ii}^{V,LR} - \frac{9592}{729}L_{eu\ 22ii}^{V,LR} - \frac{9592}{729}L_{eu\ 33ii}^{V,LR} + \frac{2504}{729}L_{eu\ 11ii}^{V,RR} \\
& + \frac{2504}{729}L_{eu\ 22ii}^{V,RR} + \frac{2504}{729}L_{eu\ 33ii}^{V,RR} + \frac{1928}{729}L_{ud\ ii11}^{V1,RR} + \frac{1928}{729}L_{ud\ ii22}^{V1,RR} - \frac{11776}{729}L_{uu\ iiii}^{V1,LR} \\
& + \frac{8512}{729}L_{uu\ iiii}^{V,RR} \Big] ;
\end{aligned}$$

$$\begin{aligned}
\dot{L}_{ee\ ij}^{V,RR} &= e^2 \Bigg[ \frac{1}{3}L_{ee\ jjii}^{V,LR} + \frac{40}{3}L_{ee\ iijj}^{V,RR} + \frac{1}{3}L_{ee\ kkii}^{V,LR} + \frac{4}{3}L_{ee\ iikk}^{V,RR} + \frac{1}{3}L_{de\ 11ii}^{V,LR} \\
& + \frac{1}{3}L_{de\ 22ii}^{V,LR} + \frac{1}{3}L_{ed\ ii11}^{V,RR} + \frac{1}{3}L_{ed\ ii22}^{V,RR} + \frac{1}{3}L_{ee\ iiii}^{V,LR} + \frac{4}{3}L_{ee\ iiii}^{V,RR} - \frac{2}{3}L_{eu\ ii11}^{V,RR} \\
& - \frac{2}{3}L_{eu\ ii22}^{V,RR} - \frac{2}{3}L_{ue\ 11ii}^{V,LR} - \frac{2}{3}L_{ue\ 22ii}^{V,LR} + \frac{1}{3}L_{ee\ kkjj}^{V,LR} + \frac{4}{3}L_{ee\ jjkk}^{V,RR} + \frac{1}{3}L_{de\ 11jj}^{V,LR} \\
& + \frac{1}{3}L_{de\ 22jj}^{V,LR} + \frac{1}{3}L_{ed\ jj11}^{V,RR} + \frac{1}{3}L_{ed\ jj22}^{V,RR} + \frac{2}{3}L_{ee\ jjjj}^{V,LR} + 2L_{ee\ jjjj}^{V,RR} - \frac{2}{3}L_{eu\ jj11}^{V,RR} \\
& - \frac{2}{3}L_{eu\ jj22}^{V,RR} - \frac{2}{3}L_{ue\ 11jj}^{V,LR} - \frac{2}{3}L_{ue\ 22jj}^{V,LR} \Big] + \alpha_s \alpha \Bigg[ \frac{4}{3}L_{de\ 11ii}^{V,LR} + \frac{4}{3}L_{de\ 22ii}^{V,LR} \\
& + \frac{4}{3}L_{ed\ ii11}^{V,RR} + \frac{4}{3}L_{ed\ ii22}^{V,RR} - \frac{8}{3}L_{eu\ ii11}^{V,RR} - \frac{8}{3}L_{eu\ ii22}^{V,RR} - \frac{8}{3}L_{ue\ 11ii}^{V,LR} - \frac{8}{3}L_{ue\ 22ii}^{V,LR} \\
& + \frac{4}{3}L_{de\ 11jj}^{V,LR} + \frac{4}{3}L_{de\ 22jj}^{V,LR} + \frac{4}{3}L_{ed\ jj11}^{V,RR} + \frac{4}{3}L_{ed\ jj22}^{V,RR} - \frac{8}{3}L_{eu\ jj11}^{V,RR} - \frac{8}{3}L_{eu\ jj22}^{V,RR} \\
& - \frac{8}{3}L_{ue\ 11jj}^{V,LR} - \frac{8}{3}L_{ue\ 22jj}^{V,LR} \Big] + \alpha^2 \Bigg[ -\frac{178}{27}L_{ee\ jjii}^{V,LR} - \frac{2326}{27}L_{ee\ iijj}^{V,RR} - \frac{178}{27}L_{ee\ kkii}^{V,LR} \\
& + \frac{296}{27}L_{ee\ iikk}^{V,RR} + \frac{34}{81}L_{de\ 11ii}^{V,LR} + \frac{34}{81}L_{de\ 22ii}^{V,LR} + \frac{166}{81}L_{ed\ ii11}^{V,RR} + \frac{166}{81}L_{ed\ ii22}^{V,RR} - \frac{178}{27}L_{ee\ iiii}^{V,LR} \\
& + \frac{320}{27}L_{ee\ iiii}^{V,RR} - \frac{314}{81}L_{eu\ ii11}^{V,RR} - \frac{314}{81}L_{eu\ ii22}^{V,RR} - \frac{842}{81}L_{ue\ 11ii}^{V,LR} - \frac{842}{81}L_{ue\ 22ii}^{V,LR} - \frac{178}{27}L_{ee\ kkjj}^{V,LR} \\
& + \frac{296}{27}L_{ee\ jjkk}^{V,RR} + \frac{34}{81}L_{de\ 11jj}^{V,LR} + \frac{34}{81}L_{de\ 22jj}^{V,LR} + \frac{166}{81}L_{ed\ jj11}^{V,RR} + \frac{166}{81}L_{ed\ jj22}^{V,RR} - \frac{356}{27}L_{ee\ jjjj}^{V,LR} \\
& + \frac{52}{3}L_{ee\ jjjj}^{V,RR} - \frac{314}{81}L_{eu\ jj11}^{V,RR} - \frac{314}{81}L_{eu\ jj22}^{V,RR} - \frac{842}{81}L_{ue\ 11jj}^{V,LR} - \frac{842}{81}L_{ue\ 22jj}^{V,LR} \Big] ;
\end{aligned}$$

$$\begin{aligned}
\dot{L}_{ee\bar{iii}}^{V,RR} = & e^2 \left[ \frac{4}{3} L_{jj\bar{ii}}^{V,LR} + \frac{16}{3} L_{ij\bar{jj}}^{V,RR} + \frac{4}{3} L_{kk\bar{ii}}^{V,LR} + \frac{16}{3} L_{ikk\bar{kk}}^{V,RR} + \frac{4}{3} L_{11\bar{ii}}^{V,LR} \right. \\
& + \frac{4}{3} L_{22\bar{ii}}^{V,LR} + \frac{4}{3} L_{ii\bar{11}}^{V,RR} + \frac{4}{3} L_{ed\bar{ii22}}^{V,RR} + \frac{4}{3} L_{ee\bar{iii}}^{V,LR} + \frac{52}{3} L_{iii\bar{iii}}^{V,RR} - \frac{8}{3} L_{ii\bar{11}}^{V,RR} \\
& \left. - \frac{8}{3} L_{ii\bar{22}}^{V,RR} - \frac{8}{3} L_{11\bar{ii}}^{V,LR} - \frac{8}{3} L_{22\bar{ii}}^{V,LR} \right] + \alpha_s \alpha \left[ \frac{16}{3} L_{11\bar{ii}}^{V,LR} + \frac{16}{3} L_{22\bar{ii}}^{V,LR} \right. \\
& + \frac{16}{3} L_{ed\bar{ii11}}^{V,RR} + \frac{16}{3} L_{ed\bar{ii22}}^{V,RR} - \frac{32}{3} L_{eu\bar{ii11}}^{V,RR} - \frac{32}{3} L_{eu\bar{ii22}}^{V,RR} - \frac{32}{3} L_{ue\bar{11ii}}^{V,LR} - \frac{32}{3} L_{ue\bar{22ii}}^{V,LR} \left. \right] \\
& + \alpha^2 \left[ -\frac{712}{27} L_{jj\bar{ii}}^{V,LR} + \frac{1184}{27} L_{ij\bar{jj}}^{V,RR} - \frac{712}{27} L_{kk\bar{ii}}^{V,LR} + \frac{1184}{27} L_{ikk\bar{kk}}^{V,RR} + \frac{136}{81} L_{11\bar{ii}}^{V,LR} \right. \\
& + \frac{136}{81} L_{22\bar{ii}}^{V,LR} + \frac{664}{81} L_{ii\bar{11}}^{V,RR} + \frac{664}{81} L_{ed\bar{ii22}}^{V,RR} - \frac{712}{27} L_{ee\bar{iii}}^{V,LR} - \frac{1342}{27} L_{iii\bar{iii}}^{V,RR} - \frac{1256}{81} L_{ii\bar{11}}^{V,RR} \\
& \left. - \frac{1256}{81} L_{ii\bar{22}}^{V,RR} - \frac{3368}{81} L_{11\bar{ii}}^{V,LR} - \frac{3368}{81} L_{22\bar{ii}}^{V,LR} \right];
\end{aligned}$$

$$\begin{aligned}
\dot{L}_{ed\bar{ijj}}^{V,LR} = & e^2 \left[ -4 L_{ed\bar{ijj}}^{V,LR} + \frac{16}{9} L_{ee\bar{ijj}}^{V,LL} + \frac{4}{9} L_{ee\bar{ijj}}^{V,LR} + \frac{16}{9} L_{ikk\bar{kk}}^{V,LL} + \frac{4}{9} L_{ikk\bar{kk}}^{V,LR} \right. \\
& + \frac{4}{9} L_{ii\bar{11}}^{V,LL} + \frac{4}{9} L_{ii\bar{22}}^{V,LL} + \frac{4}{9} L_{ed\bar{ii11}}^{V,LR} + \frac{4}{9} L_{ed\bar{ii22}}^{V,LR} + \frac{16}{9} L_{iii\bar{iii}}^{V,LL} + \frac{4}{9} L_{iii\bar{iii}}^{V,LR} \\
& - \frac{8}{9} L_{ii\bar{11}}^{V,LL} - \frac{8}{9} L_{ii\bar{22}}^{V,LL} - \frac{8}{9} L_{ii\bar{11}}^{V,LR} - \frac{8}{9} L_{ii\bar{22}}^{V,LR} + \frac{8}{3} L_{jj\bar{jj}}^{V1,LR} + \frac{64}{9} L_{jj\bar{jj}}^{V,RR} \\
& + \frac{4}{3} L_{11\bar{jj}}^{V,LR} + \frac{4}{3} L_{22\bar{jj}}^{V,LR} + \frac{4}{3} L_{33\bar{jj}}^{V,LR} + \frac{4}{3} L_{11\bar{jj}}^{V,RR} + \frac{4}{3} L_{22\bar{jj}}^{V,RR} + \frac{4}{3} L_{33\bar{jj}}^{V,RR} \\
& \left. - \frac{8}{3} L_{ud\bar{11jj}}^{V1,LR} - \frac{8}{3} L_{ud\bar{22jj}}^{V1,LR} - \frac{8}{3} L_{ud\bar{11jj}}^{V1,RR} - \frac{8}{3} L_{ud\bar{22jj}}^{V1,RR} \right] + \alpha_s^2 \left[ -8 L_{ii\bar{11}}^{V,LL} \right. \\
& - 8 L_{ii\bar{22}}^{V,LL} + 8 L_{ii\bar{11}}^{V,LR} + 8 L_{ii\bar{22}}^{V,LR} - 8 L_{eu\bar{ii11}}^{V,LL} - 8 L_{eu\bar{ii22}}^{V,LL} + 8 L_{eu\bar{ii11}}^{V,LR} \\
& \left. + 8 L_{eu\bar{ii22}}^{V,LR} \right] + \alpha_s \alpha \left[ 16 L_{ed\bar{ijj}}^{V,LR} + \frac{16}{9} L_{ed\bar{ii11}}^{V,LL} + \frac{16}{9} L_{ed\bar{ii22}}^{V,LL} + \frac{16}{9} L_{ed\bar{ii11}}^{V,LR} \right. \\
& + \frac{16}{9} L_{ed\bar{ii22}}^{V,LR} - \frac{32}{9} L_{ii\bar{11}}^{V,LL} - \frac{32}{9} L_{ii\bar{22}}^{V,LL} - \frac{32}{9} L_{ii\bar{11}}^{V,LR} - \frac{32}{9} L_{ii\bar{22}}^{V,LR} + \frac{32}{3} L_{jj\bar{jj}}^{V1,LR} \\
& \left. - \frac{2044}{243} L_{jj\bar{jj}}^{V8,LR} + \frac{5152}{243} L_{jj\bar{jj}}^{V,RR} - \frac{32}{3} L_{ud\bar{11jj}}^{V1,LR} - \frac{32}{3} L_{ud\bar{22jj}}^{V1,LR} - \frac{32}{3} L_{ud\bar{11jj}}^{V1,RR} - \frac{32}{3} L_{ud\bar{22jj}}^{V1,RR} \right]
\end{aligned}$$

$$\begin{aligned}
& + \frac{1354}{243} L_{11jj}^{V8,LR} + \frac{1354}{243} L_{22jj}^{V8,LR} - \frac{86}{243} L_{11jj}^{V8,RR} - \frac{86}{243} L_{22jj}^{V8,RR} \Big] + \alpha^2 \Big[ \frac{1906}{27} L_{ijj}^{V,LR} \\
& - \frac{160}{81} L_{ijj}^{V,LL} - \frac{184}{81} L_{ijj}^{V,LR} - \frac{160}{81} L_{ikk}^{V,LL} - \frac{184}{81} L_{ikk}^{V,LR} - \frac{440}{243} L_{ii11}^{V,LL} - \frac{440}{243} L_{ii22}^{V,LL} \\
& - \frac{104}{243} L_{ii11}^{V,LR} - \frac{104}{243} L_{ii22}^{V,LR} - \frac{640}{81} L_{iii}^{V,LL} - \frac{184}{81} L_{iii}^{V,LR} - \frac{1640}{243} L_{ii11}^{V,LL} - \frac{1640}{243} L_{ii22}^{V,LL} \\
& - \frac{296}{243} L_{ii11}^{V,LR} - \frac{296}{243} L_{ii22}^{V,LR} + \frac{3424}{243} L_{jjj}^{V1,LR} - \frac{3056}{729} L_{jjj}^{V,RR} + \frac{3728}{243} L_{11j}^{V,LR} \\
& + \frac{3728}{243} L_{22j}^{V,LR} + \frac{3728}{243} L_{33j}^{V,LR} - \frac{1024}{243} L_{11j}^{V,RR} - \frac{1024}{243} L_{22j}^{V,RR} - \frac{1024}{243} L_{33j}^{V,RR} \\
& - \frac{616}{243} L_{11jj}^{V1,LR} - \frac{616}{243} L_{22jj}^{V1,LR} - \frac{6952}{243} L_{11jj}^{V1,RR} - \frac{6952}{243} L_{22jj}^{V1,RR} \Big] ;
\end{aligned}$$

$$\begin{aligned}
\dot{L}_{ijj}^{V,LR} &= e^2 \Big[ \frac{4}{3} L_{11jj}^{V1,LR} + \frac{4}{3} L_{22jj}^{V1,LR} - \frac{8}{9} L_{ii11}^{V,LL} - \frac{8}{9} L_{ii22}^{V,LL} - \frac{8}{9} L_{ii11}^{V,LR} \\
& - \frac{8}{9} L_{ii22}^{V,LR} - \frac{32}{9} L_{iii}^{V,LL} - \frac{32}{9} L_{ijj}^{V,LL} - \frac{32}{9} L_{ikk}^{V,LL} - \frac{8}{9} L_{iii}^{V,LR} - \frac{8}{9} L_{ijj}^{V,LR} \\
& - \frac{8}{9} L_{ikk}^{V,LR} + \frac{16}{9} L_{ii11}^{V,LL} + \frac{16}{9} L_{ii22}^{V,LL} + \frac{4}{3} L_{11jj}^{V,LR} + \frac{4}{3} L_{22jj}^{V,LR} + \frac{4}{3} L_{33jj}^{V,LR} \\
& + \frac{16}{9} L_{ii11}^{V,LR} + \frac{16}{9} L_{ii22}^{V,LR} + 8 L_{ijj}^{V,LR} + \frac{4}{3} L_{11jj}^{V,RR} + \frac{4}{3} L_{22jj}^{V,RR} + \frac{4}{3} L_{33jj}^{V,RR} \\
& + \frac{4}{3} L_{jj11}^{V1,RR} + \frac{4}{3} L_{jj22}^{V1,RR} - \frac{8}{3} L_{jjj}^{V1,LR} - \frac{8}{3} L_{kkj}^{V1,LR} - \frac{64}{9} L_{jjj}^{V,RR} - \frac{16}{3} L_{jjk}^{V,RR} \\
& - \frac{16}{9} L_{jjk}^{V,RR} \Big] + \alpha_s^2 \Big[ -8 L_{ii11}^{V,LL} - 8 L_{ii22}^{V,LL} + 8 L_{ii11}^{V,LR} + 8 L_{ii22}^{V,LR} \\
& - 8 L_{ii11}^{V,LL} - 8 L_{ii22}^{V,LL} + 8 L_{ii11}^{V,LR} + 8 L_{ii22}^{V,LR} \Big] + \alpha_s \alpha \Big[ \frac{16}{3} L_{11j}^{V1,LR} \\
& - \frac{32}{3} L_{22j}^{V1,LR} - \frac{332}{243} L_{11jj}^{V8,LR} + \frac{2044}{243} L_{22jj}^{V8,LR} - \frac{32}{9} L_{ii11}^{V,LL} - \frac{32}{9} L_{ii22}^{V,LL} - \frac{32}{9} L_{ii11}^{V,LR} \\
& - \frac{32}{9} L_{ii22}^{V,LR} + \frac{64}{9} L_{ii11}^{V,LL} + \frac{64}{9} L_{ii22}^{V,LL} + \frac{64}{9} L_{ii11}^{V,LR} + \frac{64}{9} L_{ii22}^{V,LR} - 32 L_{ijj}^{V,LR} \\
& + \frac{16}{3} L_{jj11}^{V1,RR} + \frac{16}{3} L_{jj22}^{V1,RR} + \frac{388}{243} L_{jj11}^{V8,RR} + \frac{388}{243} L_{jj22}^{V8,RR} - \frac{32}{3} L_{jjj}^{V1,LR} - \frac{32}{3} L_{kkj}^{V1,LR} \\
& + \frac{2044}{243} L_{jjj}^{V8,LR} + \frac{2044}{243} L_{kkj}^{V8,LR} - \frac{2096}{81} L_{jjj}^{V,RR} - 16 L_{jjk}^{V,RR} - \frac{128}{243} L_{jjk}^{V,RR} \Big]
\end{aligned}$$



$$\begin{aligned}
& + \alpha^2 \left[ -\frac{1144}{243} L_{11jj}^{V1,LR} + \frac{12512}{243} L_{22jj}^{V1,LR} + \frac{1168}{243} L_{ii11}^{V,LL} + \frac{1168}{243} L_{ii22}^{V,LL} + \frac{1792}{243} L_{ii11}^{V,LR} \right. \\
& + \frac{1792}{243} L_{ii22}^{V,LR} + \frac{992}{81} L_{iii}^{V,LL} + \frac{896}{81} L_{ijj}^{V,LL} + \frac{896}{81} L_{ikk}^{V,LL} + \frac{1808}{81} L_{iii}^{V,LR} + \frac{1808}{81} L_{ijj}^{V,LR} \\
& + \frac{1808}{81} L_{ikk}^{V,LR} - \frac{1184}{243} L_{ii11}^{V,LL} - \frac{1184}{243} L_{ii22}^{V,LL} + \frac{3248}{243} L_{11jj}^{V,LR} + \frac{3248}{243} L_{22jj}^{V,LR} \\
& + \frac{3248}{243} L_{33jj}^{V,LR} + \frac{1312}{243} L_{ii11}^{V,LR} + \frac{1312}{243} L_{ii22}^{V,LR} - \frac{4784}{27} L_{ijj}^{V,LR} - \frac{4744}{243} L_{11jj}^{V,RR} \\
& - \frac{4744}{243} L_{22jj}^{V,RR} - \frac{4744}{243} L_{33jj}^{V,RR} - \frac{3808}{243} L_{jj11}^{V1,RR} - \frac{3808}{243} L_{jj22}^{V1,RR} + \frac{12224}{243} L_{jjjj}^{V1,LR} \\
& \left. + \frac{12224}{243} L_{kkjj}^{V1,LR} + \frac{3808}{243} L_{jjjj}^{V,RR} + \frac{3136}{243} L_{jjkk}^{V,RR} + \frac{1024}{729} L_{jjkk}^{V,RR} \right];
\end{aligned}$$

$$\begin{aligned}
\dot{L}_{ijj}^{V1,LR} = & -\frac{8}{3} L_{ijj}^{V8,LR} g_s^2 + e^2 \left[ -\frac{16}{9} L_{jjj}^{V1,LR} - \frac{128}{27} L_{jjj}^{V,RR} - \frac{8}{9} L_{11jj}^{V,LR} - \frac{8}{9} L_{22jj}^{V,LR} \right. \\
& - \frac{8}{9} L_{33jj}^{V,LR} - \frac{8}{9} L_{11jj}^{V,RR} - \frac{8}{9} L_{22jj}^{V,RR} - \frac{8}{9} L_{33jj}^{V,RR} + \frac{4}{9} L_{11ii}^{V,LL} + \frac{4}{9} L_{22ii}^{V,LL} \\
& + \frac{4}{9} L_{33ii}^{V,LL} + \frac{4}{9} L_{ii11}^{V1,LL} + \frac{4}{9} L_{ii22}^{V1,LL} + \frac{16}{9} L_{11jj}^{V1,LR} + \frac{16}{9} L_{22jj}^{V1,LR} + \frac{4}{9} L_{ii11}^{V1,LR} \\
& + \frac{4}{9} L_{ii22}^{V1,LR} + \frac{8}{3} L_{ijj}^{V1,LR} + \frac{16}{9} L_{11jj}^{V1,RR} + \frac{16}{9} L_{22jj}^{V1,RR} + \frac{4}{9} L_{ii11}^{V,LR} + \frac{4}{9} L_{ii22}^{V,LR} \\
& \left. + \frac{4}{9} L_{ii33}^{V,LR} - \frac{8}{9} L_{iii}^{V1,LR} - \frac{8}{9} L_{ikk}^{V1,LR} - \frac{64}{27} L_{iii}^{V,LL} - \frac{16}{9} L_{ikk}^{V,LL} - \frac{16}{27} L_{ikki}^{V,LL} \right] \\
& + \alpha_s^2 \left[ 16 L_{jjjj}^{V1,LR} + \frac{88}{27} L_{jjjj}^{V8,LR} - \frac{1192}{27} L_{jjjj}^{V,RR} - 8 L_{ii11}^{V1,LL} - 8 L_{ii22}^{V1,LL} \right. \\
& + 8 L_{11jj}^{V1,LR} + 8 L_{22jj}^{V1,LR} + 8 L_{ii11}^{V1,LR} + 8 L_{ii22}^{V1,LR} - \frac{28}{3} L_{ijj}^{V1,LR} - 8 L_{11jj}^{V1,RR} \\
& - 8 L_{22jj}^{V1,RR} + \frac{44}{27} L_{ii11}^{V8,LL} + \frac{44}{27} L_{ii22}^{V8,LL} + \frac{44}{27} L_{11jj}^{V8,LR} + \frac{44}{27} L_{22jj}^{V8,LR} + \frac{44}{27} L_{ii11}^{V8,LR} \\
& + \frac{44}{27} L_{ii22}^{V8,LR} - \frac{2044}{27} L_{ijj}^{V8,LR} + \frac{44}{27} L_{11jj}^{V8,RR} + \frac{44}{27} L_{22jj}^{V8,RR} + 8 L_{iii}^{V1,LR} + 8 L_{ikk}^{V1,LR} \\
& \left. + \frac{44}{27} L_{iii}^{V8,LR} + \frac{44}{27} L_{ikk}^{V8,LR} - \frac{232}{9} L_{iii}^{V,LL} - 16 L_{ikk}^{V,LL} - \frac{64}{27} L_{ikki}^{V,LL} \right] + \alpha_s \alpha \left[ -\frac{64}{9} L_{jjj}^{V1,LR} \right.
\end{aligned}$$

$$\begin{aligned}
& + \frac{4088}{729} L_{jjjj}^{V8,LR} - \frac{10304}{729} L_{jjjj}^{V,RR} + \frac{16}{9} L_{ii11}^{V1,LL} + \frac{16}{9} L_{ii22}^{V1,LL} + \frac{64}{9} L_{11jj}^{V1,LR} + \frac{64}{9} L_{22jj}^{V1,LR} \\
& + \frac{16}{9} L_{ii11}^{V1,LR} - \frac{32}{9} L_{ii22}^{V1,LR} - \frac{64}{3} L_{ijjj}^{V1,LR} + \frac{64}{9} L_{11jj}^{V1,RR} + \frac{64}{9} L_{22jj}^{V1,RR} + \frac{388}{729} L_{ii11}^{V8,LL} \\
& + \frac{388}{729} L_{ii22}^{V8,LL} - \frac{2708}{729} L_{11jj}^{V8,LR} - \frac{2708}{729} L_{22jj}^{V8,LR} - \frac{332}{729} L_{ii11}^{V8,LR} + \frac{2044}{729} L_{ii22}^{V8,LR} \\
& + \frac{232}{27} L_{ijjj}^{V8,LR} + \frac{172}{729} L_{11jj}^{V8,RR} + \frac{172}{729} L_{22jj}^{V8,RR} - \frac{32}{9} L_{iii}^{V1,LR} - \frac{32}{9} L_{ikk}^{V1,LR} + \frac{2044}{729} L_{iii}^{V8,LR} \\
& + \frac{2044}{729} L_{ikk}^{V8,LR} - \frac{2096}{243} L_{iii}^{V,LL} - \frac{16}{3} L_{ikk}^{V,LL} - \frac{128}{729} L_{ikki}^{V,LL} \Big] + \alpha^2 \Big[ \frac{7552}{729} L_{jjjj}^{V1,LR} \\
& + \frac{5392}{2187} L_{jjjj}^{V,RR} + \frac{6224}{729} L_{11jj}^{V,LR} + \frac{6224}{729} L_{22jj}^{V,LR} + \frac{6224}{729} L_{33jj}^{V,LR} - \frac{3712}{729} L_{11jj}^{V,RR} \\
& - \frac{3712}{729} L_{22jj}^{V,RR} - \frac{3712}{729} L_{33jj}^{V,RR} - \frac{1216}{729} L_{11ii}^{V,LL} - \frac{1216}{729} L_{22ii}^{V,LL} - \frac{1216}{729} L_{33ii}^{V,LL} \\
& - \frac{1576}{729} L_{ii11}^{V1,LL} - \frac{1576}{729} L_{ii22}^{V1,LL} + \frac{6272}{729} L_{11jj}^{V1,LR} + \frac{6272}{729} L_{22jj}^{V1,LR} - \frac{208}{729} L_{ii11}^{V1,LR} \\
& + \frac{6752}{729} L_{ii22}^{V1,LR} - \frac{3872}{81} L_{ijjj}^{V1,LR} - \frac{6976}{729} L_{11jj}^{V1,RR} - \frac{6976}{729} L_{22jj}^{V1,RR} + \frac{2888}{729} L_{ii11}^{V,LR} \\
& + \frac{2888}{729} L_{ii22}^{V,LR} + \frac{2888}{729} L_{ii33}^{V,LR} + \frac{6464}{729} L_{iii}^{V1,LR} + \frac{6464}{729} L_{ikk}^{V1,LR} + \frac{4384}{729} L_{iii}^{V,LL} \\
& + \frac{1984}{729} L_{ikk}^{V,LL} + \frac{3328}{2187} L_{ikki}^{V,LL} \Big] ;
\end{aligned}$$

$$\begin{aligned}
\dot{L}_{ijj}^{V8,LR} & = g_s^2 \Big[ -12 L_{ijj}^{V1,LR} - 14 L_{ijj}^{V8,LR} + \frac{2}{3} L_{ikk}^{V8,LR} + \frac{8}{3} L_{ikki}^{V,LL} + \frac{2}{3} L_{ii11}^{V8,LL} \\
& + \frac{2}{3} L_{ii22}^{V8,LL} + \frac{2}{3} L_{ii11}^{V8,LR} + \frac{2}{3} L_{ii22}^{V8,LR} + \frac{2}{3} L_{iii}^{V8,LR} + \frac{8}{3} L_{iii}^{V,LL} + \frac{4}{3} L_{jjjj}^{V8,LR} \\
& + \frac{16}{3} L_{jjjj}^{V,RR} + \frac{2}{3} L_{11jj}^{V8,LR} + \frac{2}{3} L_{22jj}^{V8,LR} + \frac{2}{3} L_{11jj}^{V8,RR} + \frac{2}{3} L_{22jj}^{V8,RR} \Big] + \frac{8}{3} e^2 L_{ijj}^{V8,LR} \\
& + \alpha_s^2 \Big[ -\frac{374}{3} L_{ijj}^{V1,LR} - \frac{2975}{18} L_{ijj}^{V8,LR} - \frac{22}{3} L_{ikk}^{V1,LR} + \frac{787}{81} L_{ikk}^{V8,LR} - \frac{28}{3} L_{ikk}^{V,LL} \\
& + \frac{3448}{81} L_{ikki}^{V,LL} - \frac{2}{3} L_{ii11}^{V1,LL} - \frac{2}{3} L_{ii22}^{V1,LL} - \frac{22}{3} L_{ii11}^{V1,LR} - \frac{22}{3} L_{ii22}^{V1,LR} + \frac{607}{81} L_{ii11}^{V8,LL} \\
& + \frac{607}{81} L_{ii22}^{V8,LL} + \frac{787}{81} L_{ii11}^{V8,LR} + \frac{787}{81} L_{ii22}^{V8,LR} - \frac{22}{3} L_{iii}^{V1,LR} + \frac{787}{81} L_{iii}^{V8,LR} + \frac{1198}{27} L_{iii}^{V,LL}
\end{aligned}$$

$$\begin{aligned}
& -\frac{44}{3}L_{jjjj}^{V1,LR} + \frac{1574}{81}L_{jjjj}^{V8,LR} + \frac{6286}{81}L_{jjjj}^{V,RR} - \frac{22}{3}L_{11jj}^{V1,LR} - \frac{22}{3}L_{22jj}^{V1,LR} - \frac{2}{3}L_{11jj}^{V1,RR} \\
& - \frac{2}{3}L_{22jj}^{V1,RR} + \frac{787}{81}L_{11jj}^{V8,LR} + \frac{787}{81}L_{22jj}^{V8,LR} + \frac{607}{81}L_{11jj}^{V8,RR} + \frac{607}{81}L_{22jj}^{V8,RR} \Big] \\
& + \alpha_s \alpha \left[ \frac{116}{3}L_{iijj}^{V1,LR} + \frac{187}{9}L_{iijj}^{V8,LR} - \frac{1288}{81}L_{iikk}^{V1,LR} - \frac{20}{3}L_{iikk}^{V8,LR} - \frac{2576}{81}L_{iikk}^{V,LL} \right. \\
& - \frac{800}{243}L_{iikk}^{V,LL} + \frac{644}{81}L_{11ii}^{V,LL} + \frac{644}{81}L_{22ii}^{V,LL} + \frac{644}{81}L_{33ii}^{V,LL} + \frac{644}{81}L_{ii11}^{V1,LL} + \frac{644}{81}L_{ii22}^{V1,LL} \\
& + \frac{644}{81}L_{ii11}^{V1,LR} - \frac{1216}{81}L_{ii22}^{V1,LR} - \frac{70}{27}L_{ii11}^{V8,LL} - \frac{70}{27}L_{ii22}^{V8,LL} + \frac{14}{9}L_{ii11}^{V8,LR} - \frac{20}{3}L_{ii22}^{V8,LR} \\
& + \frac{644}{81}L_{ii11}^{V,LR} + \frac{644}{81}L_{ii22}^{V,LR} + \frac{644}{81}L_{ii33}^{V,LR} - \frac{1288}{81}L_{iii}^{V1,LR} - \frac{20}{3}L_{iii}^{V8,LR} - \frac{3608}{81}L_{iii}^{V,LL} \\
& - \frac{1832}{81}L_{jjjj}^{V1,LR} - \frac{88}{9}L_{jjjj}^{V8,LR} - \frac{11264}{243}L_{jjjj}^{V,RR} - \frac{916}{81}L_{11jj}^{V,LR} - \frac{916}{81}L_{22jj}^{V,LR} - \frac{916}{81}L_{33jj}^{V,LR} \\
& - \frac{916}{81}L_{11jj}^{V,RR} - \frac{916}{81}L_{22jj}^{V,RR} - \frac{916}{81}L_{33jj}^{V,RR} + \frac{1832}{81}L_{11jj}^{V1,LR} + \frac{1832}{81}L_{22jj}^{V1,LR} + \frac{1832}{81}L_{11jj}^{V1,RR} \\
& + \frac{1832}{81}L_{22jj}^{V1,RR} + \frac{56}{9}L_{11jj}^{V8,LR} + \frac{56}{9}L_{22jj}^{V8,LR} - \frac{160}{27}L_{11jj}^{V8,RR} - \frac{160}{27}L_{22jj}^{V8,RR} \Big] \\
& - \frac{3872}{81}\alpha^2 L_{iijj}^{V8,LR} ;
\end{aligned}$$

$$\begin{aligned}
\dot{L}_{jjii}^{V,LR} & = e^2 \left[ \frac{4}{3}L_{jjii}^{V1,LR} + \frac{8}{3}L_{iijj}^{V,RR} + \frac{8}{9}L_{ijji}^{V,RR} - 4L_{jjii}^{V,LR} + \frac{4}{3}L_{iii}^{V1,LR} \right. \\
& + \frac{32}{9}L_{iii}^{V,RR} + \frac{4}{3}L_{11ii}^{V,LR} + \frac{4}{3}L_{22ii}^{V,LR} + \frac{4}{3}L_{33ii}^{V,LR} + \frac{4}{3}L_{11ii}^{V,RR} + \frac{4}{3}L_{22ii}^{V,RR} \\
& + \frac{4}{3}L_{33ii}^{V,RR} - \frac{8}{3}L_{11ii}^{V1,LR} - \frac{8}{3}L_{22ii}^{V1,LR} - \frac{8}{3}L_{11ii}^{V1,RR} - \frac{8}{3}L_{22ii}^{V1,RR} + \frac{16}{9}L_{jjkk}^{V,LL} \\
& + \frac{4}{9}L_{jjkk}^{V,LR} + \frac{4}{9}L_{jj11}^{V,LL} + \frac{4}{9}L_{jj22}^{V,LL} + \frac{4}{9}L_{jj11}^{V,LR} + \frac{4}{9}L_{jj22}^{V,LR} + \frac{8}{3}L_{jjjj}^{V,LL} \\
& + \frac{8}{9}L_{jjjj}^{V,LR} - \frac{8}{9}L_{jj11}^{V,LL} - \frac{8}{9}L_{jj22}^{V,LL} - \frac{8}{9}L_{jj11}^{V,LR} - \frac{8}{9}L_{jj22}^{V,LR} \Big] + \alpha_s^2 \left[ -8L_{jj11}^{V,LL} \right. \\
& - 8L_{jj22}^{V,LL} + 8L_{jj11}^{V,LR} + 8L_{jj22}^{V,LR} - 8L_{jj11}^{V,LL} - 8L_{jj22}^{V,LL} + 8L_{jj11}^{V,LR} \\
& \left. + 8L_{jj22}^{V,LR} \right] + \alpha_s \alpha \left[ \frac{16}{3}L_{jjii}^{V1,LR} - \frac{1022}{243}L_{jjii}^{V8,LR} + 8L_{iijj}^{V,RR} + \frac{64}{243}L_{ijji}^{V,RR} \right.
\end{aligned}$$

$$\begin{aligned}
& + 16L_{jj\bar{i}i}^{V,LR} + \frac{16}{3}L_{iii}^{V1,LR} - \frac{1022}{243}L_{iii}^{V8,LR} + \frac{1048}{81}L_{iii}^{V,RR} - \frac{32}{3}L_{11\bar{i}i}^{V1,LR} - \frac{32}{3}L_{22\bar{i}i}^{V1,LR} \\
& - \frac{32}{3}L_{11\bar{i}i}^{V1,RR} - \frac{32}{3}L_{22\bar{i}i}^{V1,RR} + \frac{1354}{243}L_{11\bar{i}i}^{V8,LR} + \frac{1354}{243}L_{22\bar{i}i}^{V8,LR} - \frac{86}{243}L_{11\bar{i}i}^{V8,RR} - \frac{86}{243}L_{22\bar{i}i}^{V8,RR} \\
& + \frac{16}{9}L_{jj11}^{V,LL} + \frac{16}{9}L_{jj22}^{V,LL} + \frac{16}{9}L_{jj11}^{V,LR} + \frac{16}{9}L_{jj22}^{V,LR} - \frac{32}{9}L_{jj11}^{V,LL} - \frac{32}{9}L_{jj22}^{V,LL} \\
& - \frac{32}{9}L_{jj11}^{V,LR} - \frac{32}{9}L_{jj22}^{V,LR} \Big] + \alpha^2 \Big[ \frac{1712}{243}L_{jj\bar{i}i}^{V1,LR} + \frac{256}{243}L_{i\bar{j}j}^{V,RR} - \frac{1424}{729}L_{i\bar{j}j}^{V,RR} \\
& + \frac{1906}{27}L_{jj\bar{i}i}^{V,LR} + \frac{1712}{243}L_{dd}^{V1,LR} - \frac{800}{243}L_{dd}^{V,RR} + \frac{3728}{243}L_{11\bar{i}i}^{V,LR} + \frac{3728}{243}L_{22\bar{i}i}^{V,LR} \\
& + \frac{3728}{243}L_{33\bar{i}i}^{V,LR} - \frac{1024}{243}L_{11\bar{i}i}^{V,RR} - \frac{1024}{243}L_{22\bar{i}i}^{V,RR} - \frac{1024}{243}L_{33\bar{i}i}^{V,RR} - \frac{616}{243}L_{11\bar{i}i}^{V1,LR} \\
& - \frac{616}{243}L_{22\bar{i}i}^{V1,LR} - \frac{6952}{243}L_{11\bar{i}i}^{V1,RR} - \frac{6952}{243}L_{22\bar{i}i}^{V1,RR} - \frac{160}{81}L_{jj\bar{k}k}^{V,LL} - \frac{184}{81}L_{jj\bar{k}k}^{V,LR} \\
& - \frac{440}{243}L_{jj11}^{V,LL} - \frac{440}{243}L_{jj22}^{V,LL} - \frac{104}{243}L_{jj11}^{V,LR} - \frac{104}{243}L_{jj22}^{V,LR} - \frac{80}{9}L_{jjjj}^{V,LL} - \frac{368}{81}L_{jjjj}^{V,LR} \\
& - \frac{1640}{243}L_{jj11}^{V,LL} - \frac{1640}{243}L_{jj22}^{V,LL} - \frac{296}{243}L_{jj11}^{V,LR} - \frac{296}{243}L_{jj22}^{V,LR} \Big] ;
\end{aligned}$$

$$\begin{aligned}
\dot{L}_{jj\bar{i}i}^{V,LR} &= e^2 \Big[ 8L_{jj\bar{i}i}^{V,LR} - \frac{8}{3}L_{kk\bar{i}i}^{V1,LR} - \frac{16}{3}L_{i\bar{u}k}^{V,RR} - \frac{16}{9}L_{i\bar{k}k}^{V,RR} + \frac{4}{3}L_{11\bar{i}i}^{V1,LR} \\
& + \frac{4}{3}L_{22\bar{i}i}^{V1,LR} + \frac{4}{3}L_{11\bar{i}i}^{V,LR} + \frac{4}{3}L_{22\bar{i}i}^{V,LR} + \frac{4}{3}L_{33\bar{i}i}^{V,RR} + \frac{4}{3}L_{11\bar{i}i}^{V,RR} + \frac{4}{3}L_{22\bar{i}i}^{V,RR} \\
& + \frac{4}{3}L_{33\bar{i}i}^{V,RR} + \frac{4}{3}L_{i\bar{i}11}^{V1,RR} + \frac{4}{3}L_{i\bar{i}22}^{V1,RR} - \frac{8}{3}L_{i\bar{u}i}^{V1,LR} - \frac{64}{9}L_{i\bar{u}i}^{V,RR} - \frac{32}{9}L_{jj\bar{k}k}^{V,LL} \\
& - \frac{8}{9}L_{jj\bar{k}k}^{V,LR} - \frac{8}{9}L_{jj11}^{V,LL} - \frac{8}{9}L_{jj22}^{V,LL} - \frac{8}{9}L_{jj11}^{V,LR} - \frac{8}{9}L_{jj22}^{V,LR} - \frac{16}{3}L_{jjjj}^{V,LL} \\
& - \frac{16}{9}L_{jjjj}^{V,LR} + \frac{16}{9}L_{jj11}^{V,LL} + \frac{16}{9}L_{jj22}^{V,LL} + \frac{16}{9}L_{jj11}^{V,LR} + \frac{16}{9}L_{jj22}^{V,LR} \Big] + \alpha_s^2 \Big[ -8L_{jj11}^{V,LL} \\
& - 8L_{jj22}^{V,LL} + 8L_{jj11}^{V,LR} + 8L_{jj22}^{V,LR} - 8L_{jj11}^{V,LL} - 8L_{jj22}^{V,LL} + 8L_{jj11}^{V,LR} \\
& + 8L_{jj22}^{V,LR} \Big] + \alpha_s \alpha \Big[ -32L_{jj\bar{i}i}^{V,LR} - \frac{32}{3}L_{kk\bar{i}i}^{V1,LR} + \frac{2044}{243}L_{kk\bar{i}i}^{V8,LR} - 16L_{i\bar{k}k}^{V,RR} \\
& - \frac{128}{243}L_{i\bar{k}k}^{V,RR} + \frac{16}{3}L_{11\bar{i}i}^{V1,LR} - \frac{32}{3}L_{22\bar{i}i}^{V1,LR} - \frac{332}{243}L_{11\bar{i}i}^{V8,LR} + \frac{2044}{243}L_{22\bar{i}i}^{V8,LR} + \frac{16}{3}L_{i\bar{i}11}^{V1,RR}
\end{aligned}$$

$$\begin{aligned}
& + \frac{16}{3} L_{ud}^{V1,RR} + \frac{388}{243} L_{ii11}^{V8,RR} + \frac{388}{243} L_{ii22}^{V8,RR} - \frac{32}{3} L_{iii}^{V1,LR} + \frac{2044}{243} L_{iii}^{V8,LR} - \frac{2096}{81} L_{iii}^{V,RR} \\
& - \frac{32}{9} L_{jj11}^{V,LL} - \frac{32}{9} L_{jj22}^{V,LL} - \frac{32}{9} L_{jj11}^{V,LR} - \frac{32}{9} L_{jj22}^{V,LR} + \frac{64}{9} L_{jj11}^{V,LL} + \frac{64}{9} L_{jj22}^{V,LL} \\
& + \frac{64}{9} L_{jj11}^{V,LR} + \frac{64}{9} L_{jj22}^{V,LR} \Big] + \alpha^2 \Bigg[ - \frac{4784}{27} L_{jji}^{V,LR} + \frac{12224}{243} L_{kkii}^{V1,LR} + \frac{3136}{243} L_{iikk}^{V,RR} \\
& + \frac{1024}{729} L_{iikk}^{V,RR} - \frac{1144}{243} L_{11ii}^{V1,LR} + \frac{12512}{243} L_{22ii}^{V1,LR} + \frac{3248}{243} L_{11ii}^{V,LR} + \frac{3248}{243} L_{22ii}^{V,LR} \\
& + \frac{3248}{243} L_{33ii}^{V,LR} - \frac{4744}{243} L_{11ii}^{V,RR} - \frac{4744}{243} L_{22ii}^{V,RR} - \frac{4744}{243} L_{33ii}^{V,RR} - \frac{3808}{243} L_{ii11}^{V1,RR} \\
& - \frac{3808}{243} L_{ii22}^{V1,RR} + \frac{12224}{243} L_{iii}^{V1,LR} + \frac{3808}{243} L_{iii}^{V,RR} + \frac{896}{81} L_{jjkk}^{V,LL} + \frac{1808}{81} L_{jjkk}^{V,LR} \\
& + \frac{1168}{243} L_{jj11}^{V,LL} + \frac{1168}{243} L_{jj22}^{V,LL} + \frac{1792}{243} L_{jj11}^{V,LR} + \frac{1792}{243} L_{jj22}^{V,LR} + \frac{160}{9} L_{jjjj}^{V,LL} \\
& + \frac{3616}{81} L_{jjjj}^{V,LR} - \frac{1184}{243} L_{jj11}^{V,LL} - \frac{1184}{243} L_{jj22}^{V,LL} + \frac{1312}{243} L_{jj11}^{V,LR} + \frac{1312}{243} L_{jj22}^{V,LR} \Big] ;
\end{aligned}$$

$$\begin{aligned}
\dot{L}_{ud}^{V1,LR} = & - \frac{8}{3} L_{jji}^{V8,LR} g_s^2 + e^2 \Bigg[ - \frac{8}{9} L_{iii}^{V1,LR} - \frac{8}{9} L_{jji}^{V1,LR} - \frac{64}{27} L_{iii}^{V,RR} - \frac{16}{9} L_{ijj}^{V,RR} \\
& - \frac{16}{27} L_{ijj}^{V,RR} - \frac{8}{9} L_{11ii}^{V,LR} - \frac{8}{9} L_{22ii}^{V,LR} - \frac{8}{9} L_{33ii}^{V,LR} - \frac{8}{9} L_{11ii}^{V,RR} - \frac{8}{9} L_{22ii}^{V,RR} \\
& - \frac{8}{9} L_{33ii}^{V,RR} + \frac{4}{9} L_{11jj}^{V,LL} + \frac{4}{9} L_{22jj}^{V,LL} + \frac{4}{9} L_{33jj}^{V,LL} + \frac{4}{9} L_{ud}^{V1,LL} + \frac{4}{9} L_{jj22}^{V1,LL} \\
& + \frac{16}{9} L_{11ii}^{V1,LR} + \frac{16}{9} L_{22ii}^{V1,LR} + \frac{4}{9} L_{jj11}^{V1,LR} + \frac{4}{9} L_{jj22}^{V1,LR} + \frac{8}{3} L_{jji}^{V1,LR} + \frac{16}{9} L_{11ii}^{V1,RR} \\
& + \frac{16}{9} L_{22ii}^{V1,RR} + \frac{4}{9} L_{jj11}^{V,LR} + \frac{4}{9} L_{jj22}^{V,LR} + \frac{4}{9} L_{jj33}^{V,LR} - \frac{8}{9} L_{jjjj}^{V1,LR} - \frac{8}{9} L_{jjkk}^{V1,LR} \\
& - \frac{64}{27} L_{jjjj}^{V,LL} - \frac{16}{9} L_{jjkk}^{V,LL} - \frac{16}{27} L_{jjkk}^{V,LL} \Big] + \alpha_s^2 \Bigg[ 8 L_{iii}^{V1,LR} + 8 L_{jji}^{V1,LR} \\
& + \frac{44}{27} L_{iii}^{V8,LR} + \frac{44}{27} L_{jji}^{V8,LR} - \frac{232}{9} L_{iii}^{V,RR} - 16 L_{ijj}^{V,RR} - \frac{64}{27} L_{ijj}^{V,RR} - 8 L_{ud}^{V1,LL} \\
& - 8 L_{jj22}^{V1,LL} + 8 L_{11ii}^{V1,LR} + 8 L_{22ii}^{V1,LR} + 8 L_{jj11}^{V1,LR} + 8 L_{jj22}^{V1,LR} - \frac{28}{3} L_{jji}^{V1,LR} \\
& - 8 L_{11ii}^{V1,RR} - 8 L_{22ii}^{V1,RR} + \frac{44}{27} L_{jj11}^{V8,LL} + \frac{44}{27} L_{jj22}^{V8,LL} + \frac{44}{27} L_{11ii}^{V8,LR} + \frac{44}{27} L_{22ii}^{V8,LR}
\end{aligned}$$

$$\begin{aligned}
& + \frac{44}{27} L_{jj11}^{V8,LR} + \frac{44}{27} L_{jj22}^{V8,LR} - \frac{2044}{27} L_{jjii}^{V8,LR} + \frac{44}{27} L_{11ii}^{V8,RR} + \frac{44}{27} L_{22ii}^{V8,RR} + 8 L_{jjjj}^{V1,LR} \\
& + 8 L_{jjkk}^{V1,LR} + \frac{44}{27} L_{jjjj}^{V8,LR} + \frac{44}{27} L_{jjkk}^{V8,LR} - \frac{232}{9} L_{jjjj}^{V,LL} - 16 L_{jjkk}^{V,LL} - \frac{64}{27} L_{jjkj}^{V,LL} \Big] \\
& + \alpha_s \alpha \left[ -\frac{32}{9} L_{iii}^{V1,LR} - \frac{32}{9} L_{jjii}^{V1,LR} + \frac{2044}{729} L_{iii}^{V8,LR} + \frac{2044}{729} L_{jjii}^{V8,LR} - \frac{2096}{243} L_{iii}^{V,RR} \right. \\
& - \frac{16}{3} L_{ijj}^{V,RR} - \frac{128}{729} L_{ijji}^{V,RR} + \frac{16}{9} L_{jj11}^{V1,LL} + \frac{16}{9} L_{jj22}^{V1,LL} + \frac{64}{9} L_{11ii}^{V1,LR} + \frac{64}{9} L_{22ii}^{V1,LR} \\
& + \frac{16}{9} L_{jj11}^{V1,LR} - \frac{32}{9} L_{jj22}^{V1,LR} - \frac{64}{3} L_{jjii}^{V1,LR} + \frac{64}{9} L_{11ii}^{V1,RR} + \frac{64}{9} L_{22ii}^{V1,RR} + \frac{388}{729} L_{jj11}^{V8,LL} \\
& + \frac{388}{729} L_{jj22}^{V8,LL} - \frac{2708}{729} L_{11ii}^{V8,LR} - \frac{2708}{729} L_{22ii}^{V8,LR} - \frac{332}{729} L_{jj11}^{V8,LR} + \frac{2044}{729} L_{jj22}^{V8,LR} \\
& + \frac{232}{27} L_{jjii}^{V8,LR} + \frac{172}{729} L_{11ii}^{V8,RR} + \frac{172}{729} L_{22ii}^{V8,RR} - \frac{32}{9} L_{jjjj}^{V1,LR} - \frac{32}{9} L_{jjkk}^{V1,LR} + \frac{2044}{729} L_{jjjj}^{V8,LR} \\
& + \frac{2044}{729} L_{jjkk}^{V8,LR} - \frac{2096}{243} L_{jjjj}^{V,LL} - \frac{16}{3} L_{jjkk}^{V,LL} - \frac{128}{729} L_{jjkj}^{V,LL} \Big] + \alpha^2 \left[ \frac{3776}{729} L_{iii}^{V1,LR} \right. \\
& + \frac{3776}{729} L_{jjii}^{V1,LR} + \frac{880}{729} L_{iii}^{V,RR} + \frac{928}{729} L_{ijj}^{V,RR} - \frac{32}{2187} L_{ijji}^{V,RR} + \frac{6224}{729} L_{11ii}^{V,LR} \\
& + \frac{6224}{729} L_{22ii}^{V,LR} + \frac{6224}{729} L_{33ii}^{V,LR} - \frac{3712}{729} L_{11ii}^{V,RR} - \frac{3712}{729} L_{22ii}^{V,RR} - \frac{3712}{729} L_{33ii}^{V,RR} \\
& - \frac{1216}{729} L_{11jj}^{V,LL} - \frac{1216}{729} L_{22jj}^{V,LL} - \frac{1216}{729} L_{33jj}^{V,LL} - \frac{1576}{729} L_{jj11}^{V1,LL} - \frac{1576}{729} L_{jj22}^{V1,LL} \\
& + \frac{6272}{729} L_{11ii}^{V1,LR} + \frac{6272}{729} L_{22ii}^{V1,LR} - \frac{208}{729} L_{jj11}^{V1,LR} + \frac{6752}{729} L_{jj22}^{V1,LR} - \frac{3872}{81} L_{jjii}^{V1,LR} \\
& - \frac{6976}{729} L_{11ii}^{V1,RR} - \frac{6976}{729} L_{22ii}^{V1,RR} + \frac{2888}{729} L_{jj11}^{V,LR} + \frac{2888}{729} L_{jj22}^{V,LR} + \frac{2888}{729} L_{jj33}^{V,LR} \\
& + \frac{6464}{729} L_{jjjj}^{V1,LR} + \frac{6464}{729} L_{jjkk}^{V1,LR} + \frac{4384}{729} L_{jjjj}^{V,LL} + \frac{1984}{729} L_{jjkk}^{V,LL} + \frac{3328}{2187} L_{jjkj}^{V,LL} \Big] ;
\end{aligned}$$

$$\begin{aligned}
\dot{L}_{jjii}^{V8,LR} & = g_s^2 \left[ \frac{2}{3} L_{iii}^{V8,LR} + \frac{2}{3} L_{jjii}^{V8,LR} + \frac{8}{3} L_{iii}^{V,RR} + \frac{8}{3} L_{ijji}^{V,RR} - 12 L_{jjii}^{V1,LR} \right. \\
& + \frac{2}{3} L_{jj11}^{V8,LL} + \frac{2}{3} L_{jj22}^{V8,LL} + \frac{2}{3} L_{11ii}^{V8,LR} + \frac{2}{3} L_{22ii}^{V8,LR} + \frac{2}{3} L_{jj11}^{V8,LR} + \frac{2}{3} L_{jj22}^{V8,LR} \\
& \left. - 14 L_{jjii}^{V8,LR} + \frac{2}{3} L_{11ii}^{V8,RR} + \frac{2}{3} L_{22ii}^{V8,RR} + \frac{2}{3} L_{jjjj}^{V8,LR} + \frac{2}{3} L_{jjkk}^{V8,LR} + \frac{8}{3} L_{jjjj}^{V,LL} \right]
\end{aligned}$$

$$\begin{aligned}
& + \frac{8}{3} L_{jkkj}^{V,LL} \Big] + \frac{8}{3} L_{jjii}^{V8,LR} e^2 + \alpha_s^2 \Bigg[ - \frac{22}{3} L_{iii}^{V1,LR} - \frac{22}{3} L_{jjii}^{V1,LR} + \frac{787}{81} L_{iii}^{V8,LR} \\
& + \frac{787}{81} L_{jjii}^{V8,LR} + \frac{1198}{27} L_{iii}^{V,RR} - \frac{28}{3} L_{ijji}^{V,RR} + \frac{3448}{81} L_{ijji}^{V,RR} - \frac{2}{3} L_{jj11}^{V1,LL} - \frac{2}{3} L_{jj22}^{V1,LL} \\
& - \frac{22}{3} L_{11ii}^{V1,LR} - \frac{22}{3} L_{22ii}^{V1,LR} - \frac{22}{3} L_{jj11}^{V1,LR} - \frac{22}{3} L_{jj22}^{V1,LR} - \frac{374}{3} L_{jjii}^{V1,LR} - \frac{2}{3} L_{11ii}^{V1,RR} \\
& - \frac{2}{3} L_{22ii}^{V1,RR} + \frac{607}{81} L_{jj11}^{V8,LL} + \frac{607}{81} L_{jj22}^{V8,LL} + \frac{787}{81} L_{11ii}^{V8,LR} + \frac{787}{81} L_{22ii}^{V8,LR} + \frac{787}{81} L_{jj11}^{V8,LR} \\
& + \frac{787}{81} L_{jj22}^{V8,LR} - \frac{2975}{18} L_{jjii}^{V8,LR} + \frac{607}{81} L_{11ii}^{V8,RR} + \frac{607}{81} L_{22ii}^{V8,RR} - \frac{22}{3} L_{jjj}^{V1,LR} - \frac{22}{3} L_{jjk}^{V1,LR} \\
& + \frac{787}{81} L_{jjjj}^{V8,LR} + \frac{787}{81} L_{jjkk}^{V8,LR} + \frac{1198}{27} L_{jjjj}^{V,LL} - \frac{28}{3} L_{jjkk}^{V,LL} + \frac{3448}{81} L_{jkkj}^{V,LL} \Big] \\
& + \alpha_s \alpha \Bigg[ - \frac{916}{81} L_{iii}^{V1,LR} - \frac{916}{81} L_{jjii}^{V1,LR} - \frac{44}{9} L_{iii}^{V8,LR} - \frac{44}{9} L_{jjii}^{V8,LR} - \frac{2144}{81} L_{iii}^{V,RR} \\
& - \frac{1832}{81} L_{ijji}^{V,RR} + \frac{664}{243} L_{ijji}^{V,RR} - \frac{916}{81} L_{11ii}^{V,LR} - \frac{916}{81} L_{22ii}^{V,LR} - \frac{916}{81} L_{33ii}^{V,LR} - \frac{916}{81} L_{11ii}^{V,RR} \\
& - \frac{916}{81} L_{22ii}^{V,RR} - \frac{916}{81} L_{33ii}^{V,RR} + \frac{644}{81} L_{11jj}^{V,LL} + \frac{644}{81} L_{22jj}^{V,LL} + \frac{644}{81} L_{33jj}^{V,LL} + \frac{644}{81} L_{jj11}^{V1,LL} \\
& + \frac{644}{81} L_{jj22}^{V1,LL} + \frac{1832}{81} L_{11ii}^{V1,LR} + \frac{1832}{81} L_{22ii}^{V1,LR} + \frac{644}{81} L_{jj11}^{V1,LR} - \frac{1216}{81} L_{jj22}^{V1,LR} \\
& + \frac{116}{3} L_{jjii}^{V1,LR} + \frac{1832}{81} L_{11ii}^{V1,RR} + \frac{1832}{81} L_{22ii}^{V1,RR} - \frac{70}{27} L_{jj11}^{V8,LL} - \frac{70}{27} L_{jj22}^{V8,LL} + \frac{56}{9} L_{11ii}^{V8,LR} \\
& + \frac{56}{9} L_{22ii}^{V8,LR} + \frac{14}{9} L_{jj11}^{V8,LR} - \frac{20}{3} L_{jj22}^{V8,LR} + \frac{187}{9} L_{jjii}^{V8,LR} - \frac{160}{27} L_{11ii}^{V8,RR} - \frac{160}{27} L_{22ii}^{V8,RR} \\
& + \frac{644}{81} L_{jj11}^{V,LR} + \frac{644}{81} L_{jj22}^{V,LR} + \frac{644}{81} L_{jj33}^{V,LR} - \frac{1288}{81} L_{jjjj}^{V1,LR} - \frac{1288}{81} L_{jjkk}^{V1,LR} - \frac{20}{3} L_{jjjj}^{V8,LR} \\
& - \frac{20}{3} L_{jjkk}^{V8,LR} - \frac{3608}{81} L_{jjjj}^{V,LL} - \frac{2576}{81} L_{jjkk}^{V,LL} - \frac{800}{243} L_{jkkj}^{V,LL} \Big] - \frac{3872}{81} L_{jjii}^{V8,LR} \\
& \alpha^2 ;
\end{aligned}$$

$$\begin{aligned}
\dot{L}_{jjii}^{V1,LR} &= - \frac{8}{3} L_{jjii}^{V8,LR} g_s^2 + e^2 \Bigg[ \frac{4}{9} L_{iii}^{V1,LR} - \frac{8}{9} L_{jjii}^{V1,LR} + \frac{8}{9} L_{jjjj}^{V1,LR} + \frac{64}{27} L_{jjjj}^{V,LL} \\
& + \frac{32}{27} L_{iii}^{V,RR} + \frac{8}{9} L_{ijji}^{V,RR} + \frac{8}{27} L_{ijji}^{V,RR} + \frac{4}{9} L_{jj11}^{V,LR} + \frac{4}{9} L_{jj22}^{V,LR} + \frac{4}{9} L_{jj33}^{V,LR}
\end{aligned}$$

$$\begin{aligned}
& -\frac{8}{9}L_{\frac{du}{jj11}}^{V1,LR} - \frac{8}{9}L_{\frac{du}{jj22}}^{V1,LR} + \frac{4}{9}L_{\frac{ed}{11jj}}^{V,LL} + \frac{4}{9}L_{\frac{ed}{22jj}}^{V,LL} + \frac{4}{9}L_{\frac{ed}{33jj}}^{V,LL} + \frac{4}{9}L_{\frac{ed}{11ii}}^{V,LR} \\
& + \frac{4}{9}L_{\frac{ed}{22ii}}^{V,LR} + \frac{4}{9}L_{\frac{ed}{33ii}}^{V,LR} + \frac{4}{9}L_{\frac{ed}{11ii}}^{V,RR} + \frac{4}{9}L_{\frac{ed}{22ii}}^{V,RR} + \frac{4}{9}L_{\frac{ed}{33ii}}^{V,RR} - \frac{8}{9}L_{\frac{ud}{11jj}}^{V1,LL} \\
& - \frac{8}{9}L_{\frac{ud}{22jj}}^{V1,LL} - \frac{8}{9}L_{\frac{ud}{11ii}}^{V1,LR} - \frac{8}{9}L_{\frac{ud}{22ii}}^{V1,LR} - \frac{8}{9}L_{\frac{ud}{11ii}}^{V1,RR} - \frac{8}{9}L_{\frac{ud}{22ii}}^{V1,RR} \Big] + \alpha_s^2 \Big[ 8L_{\frac{dd}{iii}}^{V1,LR} \\
& - \frac{4}{3}L_{\frac{dd}{jjii}}^{V1,LR} + 16L_{\frac{dd}{jjjj}}^{V1,LR} + \frac{44}{27}L_{\frac{dd}{iii}}^{V8,LR} - \frac{2000}{27}L_{\frac{dd}{jjii}}^{V8,LR} + \frac{88}{27}L_{\frac{dd}{jjjj}}^{V8,LR} - \frac{1192}{27}L_{\frac{dd}{jjjj}}^{V,LL} \\
& - \frac{232}{9}L_{\frac{dd}{iii}}^{V,RR} - 16L_{\frac{dd}{ijjj}}^{V,RR} - \frac{64}{27}L_{\frac{dd}{ijji}}^{V,RR} + 8L_{\frac{du}{jj11}}^{V1,LR} + 8L_{\frac{du}{jj22}}^{V1,LR} + \frac{44}{27}L_{\frac{du}{jj11}}^{V8,LR} \\
& + \frac{44}{27}L_{\frac{du}{jj22}}^{V8,LR} - 8L_{\frac{ud}{11jj}}^{V1,LL} - 8L_{\frac{ud}{22jj}}^{V1,LL} + 8L_{\frac{ud}{11ii}}^{V1,LR} + 8L_{\frac{ud}{22ii}}^{V1,LR} - 8L_{\frac{ud}{11ii}}^{V1,RR} \\
& - 8L_{\frac{ud}{22ii}}^{V1,RR} + \frac{44}{27}L_{\frac{ud}{11jj}}^{V8,LL} + \frac{44}{27}L_{\frac{ud}{22jj}}^{V8,LL} + \frac{44}{27}L_{\frac{ud}{11ii}}^{V8,LR} + \frac{44}{27}L_{\frac{ud}{22ii}}^{V8,LR} + \frac{44}{27}L_{\frac{ud}{11ii}}^{V8,RR} \\
& + \frac{44}{27}L_{\frac{ud}{22ii}}^{V8,RR} \Big] + \alpha_s \alpha \Big[ \frac{16}{9}L_{\frac{dd}{iii}}^{V1,LR} + \frac{112}{9}L_{\frac{dd}{jjii}}^{V1,LR} + \frac{32}{9}L_{\frac{dd}{jjjj}}^{V1,LR} - \frac{1022}{729}L_{\frac{dd}{iii}}^{V8,LR} \\
& - \frac{1238}{729}L_{\frac{dd}{jjii}}^{V8,LR} - \frac{2044}{729}L_{\frac{dd}{jjjj}}^{V8,LR} + \frac{5152}{729}L_{\frac{dd}{jjjj}}^{V,LL} + \frac{1048}{243}L_{\frac{dd}{iii}}^{V,RR} + \frac{8}{3}L_{\frac{dd}{ijjj}}^{V,RR} \\
& + \frac{64}{729}L_{\frac{dd}{ijji}}^{V,RR} - \frac{32}{9}L_{\frac{du}{jj11}}^{V1,LR} - \frac{32}{9}L_{\frac{du}{jj22}}^{V1,LR} + \frac{1354}{729}L_{\frac{du}{jj11}}^{V8,LR} + \frac{1354}{729}L_{\frac{du}{jj22}}^{V8,LR} - \frac{32}{9}L_{\frac{ud}{11jj}}^{V1,LL} \\
& - \frac{32}{9}L_{\frac{ud}{22jj}}^{V1,LL} - \frac{32}{9}L_{\frac{ud}{11ii}}^{V1,LR} - \frac{32}{9}L_{\frac{ud}{22ii}}^{V1,LR} - \frac{32}{9}L_{\frac{ud}{11ii}}^{V1,RR} - \frac{32}{9}L_{\frac{ud}{22ii}}^{V1,RR} - \frac{86}{729}L_{\frac{ud}{11jj}}^{V8,LL} \\
& - \frac{86}{729}L_{\frac{ud}{22jj}}^{V8,LL} + \frac{1354}{729}L_{\frac{ud}{11ii}}^{V8,LR} + \frac{1354}{729}L_{\frac{ud}{22ii}}^{V8,LR} - \frac{86}{729}L_{\frac{ud}{11ii}}^{V8,RR} - \frac{86}{729}L_{\frac{ud}{22ii}}^{V8,RR} \Big] \\
& + \alpha^2 \Big[ \frac{272}{729}L_{\frac{dd}{iii}}^{V1,LR} + \frac{15590}{729}L_{\frac{dd}{jjii}}^{V1,LR} + \frac{544}{729}L_{\frac{dd}{jjjj}}^{V1,LR} - \frac{2912}{2187}L_{\frac{dd}{jjjj}}^{V,LL} - \frac{656}{729}L_{\frac{dd}{iii}}^{V,RR} \\
& - \frac{32}{729}L_{\frac{dd}{ijjj}}^{V,RR} - \frac{848}{2187}L_{\frac{dd}{ijji}}^{V,RR} + \frac{992}{729}L_{\frac{de}{jj11}}^{V,LR} + \frac{992}{729}L_{\frac{de}{jj22}}^{V,LR} + \frac{992}{729}L_{\frac{de}{jj33}}^{V,LR} - \frac{1624}{729}L_{\frac{du}{jj11}}^{V1,LR} \\
& - \frac{1624}{729}L_{\frac{du}{jj22}}^{V1,LR} + \frac{128}{729}L_{\frac{ed}{11jj}}^{V,LL} + \frac{128}{729}L_{\frac{ed}{22jj}}^{V,LL} + \frac{128}{729}L_{\frac{ed}{33jj}}^{V,LL} + \frac{992}{729}L_{\frac{ed}{11ii}}^{V,LR} \\
& + \frac{992}{729}L_{\frac{ed}{22ii}}^{V,LR} + \frac{992}{729}L_{\frac{ed}{33ii}}^{V,LR} + \frac{128}{729}L_{\frac{ed}{11ii}}^{V,RR} + \frac{128}{729}L_{\frac{ed}{22ii}}^{V,RR} + \frac{128}{729}L_{\frac{ed}{33ii}}^{V,RR} - \frac{2776}{729}L_{\frac{ud}{11jj}}^{V1,LL} \\
& - \frac{2776}{729}L_{\frac{ud}{22jj}}^{V1,LL} - \frac{1624}{729}L_{\frac{ud}{11ii}}^{V1,LR} - \frac{1624}{729}L_{\frac{ud}{22ii}}^{V1,LR} - \frac{2776}{729}L_{\frac{ud}{11ii}}^{V1,RR} - \frac{2776}{729}L_{\frac{ud}{22ii}}^{V1,RR} \Big] ;
\end{aligned}$$



$$\begin{aligned}
\dot{L}_{dd,jji}^{V8,LR} = & g_s^2 \left[ -12L_{dd,jji}^{V1,LR} - \frac{40}{3}L_{dd,jji}^{V8,LR} + \frac{8}{3}L_{ijji}^{V,RR} + \frac{2}{3}L_{iii}^{V8,LR} + \frac{8}{3}L_{iii}^{V,RR} \right. \\
& + \frac{2}{3}L_{11ii}^{V8,LR} + \frac{2}{3}L_{22ii}^{V8,LR} + \frac{2}{3}L_{11ii}^{V8,RR} + \frac{2}{3}L_{22ii}^{V8,RR} + \frac{4}{3}L_{jjjj}^{V8,LR} + \frac{16}{3}L_{jjjj}^{V,LL} \\
& + \frac{2}{3}L_{jj11}^{V8,LR} + \frac{2}{3}L_{jj22}^{V8,LR} + \frac{2}{3}L_{11jj}^{V8,LL} + \frac{2}{3}L_{22jj}^{V8,LL} \left. \right] - \frac{4}{3}e^2L_{dd,jji}^{V8,LR} + \alpha_s^2 \left[ -132L_{dd,jji}^{V1,LR} \right. \\
& - \frac{25201}{162}L_{dd,jji}^{V8,LR} - \frac{28}{3}L_{ijji}^{V,RR} + \frac{3448}{81}L_{ijji}^{V,RR} - \frac{22}{3}L_{iii}^{V1,LR} + \frac{787}{81}L_{iii}^{V8,LR} + \frac{1198}{27}L_{iii}^{V,RR} \\
& - \frac{22}{3}L_{11ii}^{V1,LR} - \frac{22}{3}L_{22ii}^{V1,LR} - \frac{2}{3}L_{11ii}^{V1,RR} - \frac{2}{3}L_{22ii}^{V1,RR} + \frac{787}{81}L_{11ii}^{V8,LR} + \frac{787}{81}L_{22ii}^{V8,LR} \\
& + \frac{607}{81}L_{11ii}^{V8,RR} + \frac{607}{81}L_{22ii}^{V8,RR} - \frac{44}{3}L_{jjjj}^{V1,LR} + \frac{1574}{81}L_{jjjj}^{V8,LR} + \frac{6286}{81}L_{jjjj}^{V,LL} - \frac{22}{3}L_{jj11}^{V1,LR} \\
& - \frac{22}{3}L_{jj22}^{V1,LR} + \frac{787}{81}L_{jj11}^{V8,LR} + \frac{787}{81}L_{jj22}^{V8,LR} - \frac{2}{3}L_{11jj}^{V1,LL} - \frac{2}{3}L_{22jj}^{V1,LL} + \frac{607}{81}L_{11jj}^{V8,LL} \\
& + \frac{607}{81}L_{22jj}^{V8,LL} \left. \right] + \alpha_s \alpha \left[ \frac{164}{81}L_{dd,jji}^{V1,LR} - \frac{4}{3}L_{dd,jji}^{V8,LR} + \frac{544}{81}L_{ijji}^{V,RR} - \frac{1064}{243}L_{ijji}^{V,RR} \right. \\
& + \frac{272}{81}L_{iii}^{V1,LR} + \frac{14}{9}L_{iii}^{V8,LR} + \frac{340}{81}L_{iii}^{V,RR} + \frac{272}{81}L_{11ii}^{V,LR} + \frac{272}{81}L_{22ii}^{V,LR} + \frac{272}{81}L_{33ii}^{V,LR} \\
& + \frac{272}{81}L_{11ii}^{V,RR} + \frac{272}{81}L_{22ii}^{V,RR} + \frac{272}{81}L_{33ii}^{V,RR} - \frac{544}{81}L_{11ii}^{V1,LR} - \frac{544}{81}L_{22ii}^{V1,LR} - \frac{544}{81}L_{11ii}^{V1,RR} \\
& - \frac{544}{81}L_{22ii}^{V1,RR} + \frac{2}{3}L_{11ii}^{V8,LR} + \frac{2}{3}L_{22ii}^{V8,LR} + \frac{122}{27}L_{11ii}^{V8,RR} + \frac{122}{27}L_{22ii}^{V8,RR} + \frac{544}{81}L_{jjjj}^{V1,LR} \\
& + \frac{28}{9}L_{jjjj}^{V8,LR} + \frac{1588}{243}L_{jjjj}^{V,LL} + \frac{272}{81}L_{jj11}^{V,LR} + \frac{272}{81}L_{jj22}^{V,LR} + \frac{272}{81}L_{jj33}^{V,LR} - \frac{544}{81}L_{jj11}^{V1,LR} \\
& - \frac{544}{81}L_{jj22}^{V1,LR} + \frac{2}{3}L_{jj11}^{V8,LR} + \frac{2}{3}L_{jj22}^{V8,LR} + \frac{272}{81}L_{11jj}^{V,LL} + \frac{272}{81}L_{22jj}^{V,LL} + \frac{272}{81}L_{33jj}^{V,LL} \\
& - \frac{544}{81}L_{11jj}^{V1,LL} - \frac{544}{81}L_{22jj}^{V1,LL} + \frac{122}{27}L_{11jj}^{V8,LL} + \frac{122}{27}L_{22jj}^{V8,LL} \left. \right] + \frac{1702}{81}\alpha^2L_{dd,jji}^{V8,LR} ; \\
\dot{L}_{uu,jji}^{V1,LR} = & -\frac{8}{3}L_{uu,jji}^{V8,LR}g_s^2 + e^2 \left[ -\frac{8}{9}L_{11ii}^{V1,LR} - \frac{8}{9}L_{22ii}^{V1,LR} - \frac{8}{9}L_{11jj}^{V,LL} - \frac{8}{9}L_{22jj}^{V,LL} \right. \\
& - \frac{8}{9}L_{33jj}^{V,LL} - \frac{8}{9}L_{11ii}^{V,LR} - \frac{8}{9}L_{22ii}^{V,LR} - \frac{8}{9}L_{33ii}^{V,LR} - \frac{8}{9}L_{11ii}^{V,RR} - \frac{8}{9}L_{22ii}^{V,RR} \\
& - \frac{8}{9}L_{33ii}^{V,RR} - \frac{8}{9}L_{jj11}^{V1,LL} - \frac{8}{9}L_{jj22}^{V1,LL} - \frac{8}{9}L_{jj11}^{V1,LR} - \frac{8}{9}L_{jj22}^{V1,LR} - \frac{8}{9}L_{ii11}^{V1,RR}
\end{aligned}$$

$$\begin{aligned}
& -\frac{8}{9}L_{ud\ i\bar{i}22}^{V1,RR} - \frac{8}{9}L_{jj11}^{V,LR} - \frac{8}{9}L_{jj22}^{V,LR} - \frac{8}{9}L_{jj33}^{V,LR} + \frac{16}{9}L_{uu\ i\bar{i}\bar{i}\bar{i}}^{V1,LR} - \frac{16}{3}L_{jj\bar{i}\bar{i}}^{V1,LR} \\
& + \frac{16}{9}L_{uu\ j\bar{j}\bar{j}\bar{j}}^{V1,LR} + \frac{16}{9}L_{uu\ j\bar{j}k\bar{k}}^{V1,LR} + \frac{16}{9}L_{uu\ k\bar{k}i\bar{i}}^{V1,LR} + \frac{128}{27}L_{uu\ j\bar{j}\bar{j}\bar{j}}^{V,LL} + \frac{32}{9}L_{uu\ j\bar{j}k\bar{k}}^{V,LL} + \frac{32}{27}L_{uu\ j\bar{k}k\bar{j}}^{V,LL} \\
& + \frac{128}{27}L_{uu\ i\bar{i}\bar{i}\bar{i}}^{V,RR} + \frac{32}{9}L_{uu\ i\bar{i}k\bar{k}}^{V,RR} + \frac{32}{27}L_{uu\ i\bar{k}k\bar{i}}^{V,RR} \Big] + \alpha_s^2 \Big[ 8L_{11i\bar{i}}^{V1,LR} + 8L_{22i\bar{i}}^{V1,LR} \\
& + \frac{44}{27}L_{11i\bar{i}}^{V8,LR} + \frac{44}{27}L_{22i\bar{i}}^{V8,LR} - 8L_{jj11}^{V1,LL} - 8L_{jj22}^{V1,LL} + 8L_{jj11}^{V1,LR} + 8L_{jj22}^{V1,LR} \\
& - 8L_{i\bar{i}11}^{V1,RR} - 8L_{i\bar{i}22}^{V1,RR} + \frac{44}{27}L_{jj11}^{V8,LL} + \frac{44}{27}L_{jj22}^{V8,LL} + \frac{44}{27}L_{jj11}^{V8,LR} + \frac{44}{27}L_{jj22}^{V8,LR} \\
& + \frac{44}{27}L_{i\bar{i}11}^{V8,RR} + \frac{44}{27}L_{i\bar{i}22}^{V8,RR} + 8L_{uu\ i\bar{i}\bar{i}\bar{i}}^{V1,LR} - \frac{28}{3}L_{jj\bar{i}\bar{i}}^{V1,LR} + 8L_{jj\bar{j}\bar{j}}^{V1,LR} + 8L_{jjk\bar{k}}^{V1,LR} \\
& + 8L_{kk\bar{i}\bar{i}}^{V1,LR} + \frac{44}{27}L_{uu\ i\bar{i}\bar{i}\bar{i}}^{V8,LR} - \frac{2044}{27}L_{jj\bar{i}\bar{i}}^{V8,LR} + \frac{44}{27}L_{jj\bar{j}\bar{j}}^{V8,LR} + \frac{44}{27}L_{jjk\bar{k}}^{V8,LR} + \frac{44}{27}L_{kk\bar{i}\bar{i}}^{V8,LR} \\
& - \frac{232}{9}L_{jj\bar{j}\bar{j}}^{V,LL} - 16L_{jjk\bar{k}}^{V,LL} - \frac{64}{27}L_{j\bar{k}k\bar{j}}^{V,LL} - \frac{232}{9}L_{uu\ i\bar{i}\bar{i}\bar{i}}^{V,RR} - 16L_{uu\ i\bar{i}k\bar{k}}^{V,RR} - \frac{64}{27}L_{uu\ i\bar{k}k\bar{i}}^{V,RR} \Big] \\
& + \alpha_s \alpha \Big[ -\frac{32}{9}L_{du\ 11i\bar{i}}^{V1,LR} + \frac{64}{9}L_{du\ 22i\bar{i}}^{V1,LR} + \frac{664}{729}L_{du\ 11i\bar{i}}^{V8,LR} - \frac{4088}{729}L_{du\ 22i\bar{i}}^{V8,LR} - \frac{32}{9}L_{jj11}^{V1,LL} \\
& - \frac{32}{9}L_{jj22}^{V1,LL} - \frac{32}{9}L_{jj11}^{V1,LR} + \frac{64}{9}L_{jj22}^{V1,LR} - \frac{32}{9}L_{i\bar{i}11}^{V1,RR} - \frac{32}{9}L_{i\bar{i}22}^{V1,RR} - \frac{776}{729}L_{jj11}^{V8,LL} \\
& - \frac{776}{729}L_{jj22}^{V8,LL} + \frac{664}{729}L_{jj11}^{V8,LR} - \frac{4088}{729}L_{jj22}^{V8,LR} - \frac{776}{729}L_{i\bar{i}11}^{V8,RR} - \frac{776}{729}L_{i\bar{i}22}^{V8,RR} \\
& + \frac{64}{9}L_{uu\ i\bar{i}\bar{i}\bar{i}}^{V1,LR} + \frac{128}{3}L_{jj\bar{i}\bar{i}}^{V1,LR} + \frac{64}{9}L_{jj\bar{j}\bar{j}}^{V1,LR} + \frac{64}{9}L_{jjk\bar{k}}^{V1,LR} + \frac{64}{9}L_{kk\bar{i}\bar{i}}^{V1,LR} - \frac{4088}{729}L_{uu\ i\bar{i}\bar{i}\bar{i}}^{V8,LR} \\
& - \frac{32}{27}L_{jj\bar{i}\bar{i}}^{V8,LR} - \frac{4088}{729}L_{jj\bar{j}\bar{j}}^{V8,LR} - \frac{4088}{729}L_{jjk\bar{k}}^{V8,LR} - \frac{4088}{729}L_{kk\bar{i}\bar{i}}^{V8,LR} + \frac{4192}{243}L_{jj\bar{j}\bar{j}}^{V,LL} \\
& + \frac{32}{3}L_{jjk\bar{k}}^{V,LL} + \frac{256}{729}L_{j\bar{k}k\bar{j}}^{V,LL} + \frac{4192}{243}L_{uu\ i\bar{i}\bar{i}\bar{i}}^{V,RR} + \frac{32}{3}L_{uu\ i\bar{i}k\bar{k}}^{V,RR} + \frac{256}{729}L_{uu\ i\bar{k}k\bar{i}}^{V,RR} \Big] \\
& + \alpha^2 \Big[ -\frac{2392}{729}L_{du\ 11i\bar{i}}^{V1,LR} + \frac{3776}{729}L_{du\ 22i\bar{i}}^{V1,LR} - \frac{8152}{729}L_{11j\bar{j}}^{V,LL} - \frac{8152}{729}L_{22j\bar{j}}^{V,LL} - \frac{8152}{729}L_{33j\bar{j}}^{V,LL} \\
& - \frac{4696}{729}L_{11i\bar{i}}^{V,LR} - \frac{4696}{729}L_{22i\bar{i}}^{V,LR} - \frac{4696}{729}L_{33i\bar{i}}^{V,LR} - \frac{8152}{729}L_{11i\bar{i}}^{V,RR} - \frac{8152}{729}L_{22i\bar{i}}^{V,RR} \\
& - \frac{8152}{729}L_{33i\bar{i}}^{V,RR} - \frac{3544}{729}L_{jj11}^{V1,LL} - \frac{3544}{729}L_{jj22}^{V1,LL} - \frac{2392}{729}L_{jj11}^{V1,LR} + \frac{3776}{729}L_{jj22}^{V1,LR}
\end{aligned}$$

$$\begin{aligned}
& -\frac{3544}{729}L_{ud\ i11}^{V1,RR} - \frac{3544}{729}L_{ud\ i22}^{V1,RR} - \frac{4696}{729}L_{ue\ jj11}^{V,LR} - \frac{4696}{729}L_{ue\ jj22}^{V,LR} - \frac{4696}{729}L_{ue\ jj33}^{V,LR} \\
& + \frac{4352}{729}L_{uu\ iii}^{V1,LR} + \frac{7168}{81}L_{uu\ jjii}^{V1,LR} + \frac{4352}{729}L_{uu\ jjjj}^{V1,LR} + \frac{4352}{729}L_{uu\ jjkk}^{V1,LR} + \frac{4352}{729}L_{uu\ kkii}^{V1,LR} \\
& - \frac{10496}{729}L_{uu\ jjjj}^{V,LL} - \frac{512}{729}L_{uu\ jjkk}^{V,LL} - \frac{13568}{2187}L_{uu\ jkkj}^{V,LL} - \frac{10496}{729}L_{uu\ iii}^{V,RR} - \frac{512}{729}L_{uu\ iikk}^{V,RR} \\
& - \frac{13568}{2187}L_{uu\ ikki}^{V,RR} \Bigg];
\end{aligned}$$

$$\begin{aligned}
\dot{L}_{uu\ jjii}^{V8,LR} = & g_s^2 \left[ \frac{2}{3}L_{du\ 11ii}^{V8,LR} + \frac{2}{3}L_{du\ 22ii}^{V8,LR} + \frac{2}{3}L_{ud\ jj11}^{V8,LL} + \frac{2}{3}L_{ud\ jj22}^{V8,LL} + \frac{2}{3}L_{ud\ jj11}^{V8,LR} \right. \\
& + \frac{2}{3}L_{ud\ jj22}^{V8,LR} + \frac{2}{3}L_{ud\ ii11}^{V8,RR} + \frac{2}{3}L_{ud\ ii22}^{V8,RR} - 12L_{uu\ jjii}^{V1,LR} + \frac{2}{3}L_{uu\ iii}^{V8,LR} - 14L_{uu\ jjii}^{V8,LR} \\
& + \frac{2}{3}L_{uu\ jjjj}^{V8,LR} + \frac{2}{3}L_{uu\ jjkk}^{V8,LR} + \frac{2}{3}L_{uu\ kkii}^{V8,LR} + \frac{8}{3}L_{uu\ jjjj}^{V,LL} + \frac{8}{3}L_{uu\ jkkj}^{V,LL} + \frac{8}{3}L_{uu\ iii}^{V,RR} \\
& \left. + \frac{8}{3}L_{uu\ ikki}^{V,RR} \right] - \frac{16}{3}L_{uu\ jjii}^{V8,LR}e^2 + \alpha_s^2 \left[ -\frac{22}{3}L_{du\ 11ii}^{V1,LR} - \frac{22}{3}L_{du\ 22ii}^{V1,LR} + \frac{787}{81}L_{du\ 11ii}^{V8,LR} \right. \\
& + \frac{787}{81}L_{du\ 22ii}^{V8,LR} - \frac{2}{3}L_{ud\ jj11}^{V1,LL} - \frac{2}{3}L_{ud\ jj22}^{V1,LL} - \frac{22}{3}L_{ud\ jj11}^{V1,LR} - \frac{22}{3}L_{ud\ jj22}^{V1,LR} - \frac{2}{3}L_{ud\ ii11}^{V1,RR} \\
& - \frac{2}{3}L_{ud\ ii22}^{V1,RR} + \frac{607}{81}L_{ud\ jj11}^{V8,LL} + \frac{607}{81}L_{ud\ jj22}^{V8,LL} + \frac{787}{81}L_{ud\ jj11}^{V8,LR} + \frac{787}{81}L_{ud\ jj22}^{V8,LR} + \frac{607}{81}L_{ud\ ii11}^{V8,RR} \\
& + \frac{607}{81}L_{ud\ ii22}^{V8,RR} - \frac{22}{3}L_{uu\ iii}^{V1,LR} - \frac{374}{3}L_{uu\ jjii}^{V1,LR} - \frac{22}{3}L_{uu\ jjjj}^{V1,LR} - \frac{22}{3}L_{uu\ jjkk}^{V1,LR} - \frac{22}{3}L_{uu\ kkii}^{V1,LR} \\
& + \frac{787}{81}L_{uu\ iii}^{V8,LR} - \frac{2975}{18}L_{uu\ jjii}^{V8,LR} + \frac{787}{81}L_{uu\ jjjj}^{V8,LR} + \frac{787}{81}L_{uu\ jjkk}^{V8,LR} + \frac{787}{81}L_{uu\ kkii}^{V8,LR} \\
& \left. + \frac{1198}{27}L_{uu\ jjjj}^{V,LL} - \frac{28}{3}L_{uu\ jjkk}^{V,LL} + \frac{3448}{81}L_{uu\ jkkj}^{V,LL} + \frac{1198}{27}L_{uu\ iii}^{V,RR} - \frac{28}{3}L_{uu\ iikk}^{V,RR} + \frac{3448}{81}L_{uu\ ikki}^{V,RR} \right] \\
& + \alpha_s \alpha \left[ -\frac{544}{81}L_{du\ 11ii}^{V1,LR} + \frac{1160}{81}L_{du\ 22ii}^{V1,LR} + \frac{22}{9}L_{du\ 11ii}^{V8,LR} + \frac{56}{9}L_{du\ 22ii}^{V8,LR} - \frac{544}{81}L_{eu\ 11jj}^{V,LL} \right. \\
& - \frac{544}{81}L_{eu\ 22jj}^{V,LL} - \frac{544}{81}L_{eu\ 33jj}^{V,LL} - \frac{544}{81}L_{eu\ 11ii}^{V,LR} - \frac{544}{81}L_{eu\ 22ii}^{V,LR} - \frac{544}{81}L_{eu\ 33ii}^{V,LR} - \frac{544}{81}L_{eu\ 11ii}^{V,RR} \\
& - \frac{544}{81}L_{eu\ 22ii}^{V,RR} - \frac{544}{81}L_{eu\ 33ii}^{V,RR} - \frac{544}{81}L_{ud\ jj11}^{V1,LL} - \frac{544}{81}L_{ud\ jj22}^{V1,LL} - \frac{544}{81}L_{ud\ jj11}^{V1,LR} + \frac{1160}{81}L_{ud\ jj22}^{V1,LR} \\
& \left. - \frac{544}{81}L_{ud\ ii11}^{V1,RR} - \frac{544}{81}L_{ud\ ii22}^{V1,RR} + \frac{170}{27}L_{ud\ jj11}^{V8,LL} + \frac{170}{27}L_{ud\ jj22}^{V8,LL} + \frac{22}{9}L_{ud\ jj11}^{V8,LR} + \frac{56}{9}L_{ud\ jj22}^{V8,LR} \right]
\end{aligned}$$

$$\begin{aligned}
& + \frac{170}{27} L_{ud\ i11}^{V8,RR} + \frac{170}{27} L_{ud\ i22}^{V8,RR} - \frac{544}{81} L_{jj11}^{V,LR} - \frac{544}{81} L_{jj22}^{V,LR} - \frac{544}{81} L_{jj33}^{V,LR} + \frac{1088}{81} L_{iii}^{V1,LR} \\
& - \frac{16}{3} L_{jjii}^{V1,LR} + \frac{1088}{81} L_{jjjj}^{V1,LR} + \frac{1088}{81} L_{jjkk}^{V1,LR} + \frac{1088}{81} L_{kkii}^{V1,LR} + \frac{56}{9} L_{iii}^{V8,LR} - \frac{104}{9} L_{jjii}^{V8,LR} \\
& + \frac{56}{9} L_{jjjj}^{V8,LR} + \frac{56}{9} L_{jjkk}^{V8,LR} + \frac{56}{9} L_{kkii}^{V8,LR} + \frac{1360}{81} L_{jjjj}^{V,LL} + \frac{2176}{81} L_{jjkk}^{V,LL} - \frac{4256}{243} L_{jjkk}^{V,LL} \\
& + \frac{1360}{81} L_{iii}^{V,RR} + \frac{2176}{81} L_{ikk}^{V,RR} - \frac{4256}{243} L_{ikk}^{V,RR} \Big] + \frac{7168}{81} L_{jjii}^{V8,LR} \alpha^2 ;
\end{aligned}$$

$$\begin{aligned}
\dot{L}_{jjii}^{V,LR} &= e^2 \Bigg[ -\frac{32}{3} L_{jjii}^{V,LR} + \frac{16}{3} L_{ijjj}^{V,RR} + \frac{4}{3} L_{kkii}^{V,LR} + \frac{16}{3} L_{ikk}^{V,RR} + \frac{4}{3} L_{11ii}^{V,LR} \\
& + \frac{4}{3} L_{22ii}^{V,LR} + \frac{4}{3} L_{ii11}^{V,RR} + \frac{4}{3} L_{ii22}^{V,RR} + \frac{4}{3} L_{iii}^{V,LR} + \frac{16}{3} L_{iii}^{V,RR} - \frac{8}{3} L_{ii11}^{V,RR} \\
& - \frac{8}{3} L_{ii22}^{V,RR} - \frac{8}{3} L_{11ii}^{V,LR} - \frac{8}{3} L_{22ii}^{V,LR} + \frac{16}{3} L_{jjkk}^{V,LL} + \frac{4}{3} L_{jjkk}^{V,LR} + \frac{4}{3} L_{jj11}^{V,LL} \\
& + \frac{4}{3} L_{jj22}^{V,LL} + \frac{4}{3} L_{jj11}^{V,LR} + \frac{4}{3} L_{jj22}^{V,LR} + 8 L_{jjjj}^{V,LL} + \frac{8}{3} L_{jjjj}^{V,LR} - \frac{8}{3} L_{jj11}^{V,LL} \\
& - \frac{8}{3} L_{jj22}^{V,LL} - \frac{8}{3} L_{jj11}^{V,LR} - \frac{8}{3} L_{jj22}^{V,LR} \Big] + \alpha_s \alpha \Bigg[ \frac{16}{3} L_{11ii}^{V,LR} + \frac{16}{3} L_{22ii}^{V,LR} \\
& + \frac{16}{3} L_{ii11}^{V,RR} + \frac{16}{3} L_{ii22}^{V,RR} - \frac{32}{3} L_{ii11}^{V,RR} - \frac{32}{3} L_{ii22}^{V,RR} - \frac{32}{3} L_{11ii}^{V,LR} - \frac{32}{3} L_{22ii}^{V,LR} \\
& + \frac{16}{3} L_{jj11}^{V,LL} + \frac{16}{3} L_{jj22}^{V,LL} + \frac{16}{3} L_{jj11}^{V,LR} + \frac{16}{3} L_{jj22}^{V,LR} - \frac{32}{3} L_{jj11}^{V,LL} - \frac{32}{3} L_{jj22}^{V,LL} \\
& - \frac{32}{3} L_{jj11}^{V,LR} - \frac{32}{3} L_{jj22}^{V,LR} \Big] + \alpha^2 \Bigg[ \frac{6122}{27} L_{jjii}^{V,LR} + \frac{32}{27} L_{ijjj}^{V,RR} + \frac{296}{27} L_{kkii}^{V,LR} \\
& + \frac{32}{27} L_{ikk}^{V,RR} + \frac{424}{81} L_{11ii}^{V,LR} + \frac{424}{81} L_{22ii}^{V,LR} - \frac{344}{81} L_{ii11}^{V,RR} - \frac{344}{81} L_{ii22}^{V,RR} + \frac{296}{27} L_{iii}^{V,LR} \\
& - \frac{736}{27} L_{iii}^{V,RR} - \frac{3128}{81} L_{ii11}^{V,RR} - \frac{3128}{81} L_{ii22}^{V,RR} - \frac{56}{81} L_{11ii}^{V,LR} - \frac{56}{81} L_{22ii}^{V,LR} + \frac{32}{27} L_{jjkk}^{V,LL} \\
& + \frac{296}{27} L_{jjkk}^{V,LR} - \frac{344}{81} L_{jj11}^{V,LL} - \frac{344}{81} L_{jj22}^{V,LL} + \frac{424}{81} L_{jj11}^{V,LR} + \frac{424}{81} L_{jj22}^{V,LR} - \frac{80}{3} L_{jjjj}^{V,LL} \\
& + \frac{592}{27} L_{jjjj}^{V,LR} - \frac{3128}{81} L_{jj11}^{V,LL} - \frac{3128}{81} L_{jj22}^{V,LL} - \frac{56}{81} L_{jj11}^{V,LR} - \frac{56}{81} L_{jj22}^{V,LR} \Big] ;
\end{aligned}$$

## 2.10 $\Delta L = 2$ Transitions ( $\bar{\nu}_i^c \nu_j \bar{f}_k f_l$ or $\bar{\nu}_i^c e_j \bar{d}_k u_l$ )

$$\begin{aligned} \dot{L}_{\nu d,ijkl}^{S,LR} = & -8g_s^2 L_{\nu d,ijkl}^{S,LR} - \frac{2}{3}e^2 L_{\nu d,ijkl}^{S,LR} - \frac{1012}{9}\alpha_s^2 L_{\nu d,ijkl}^{S,LR} - \frac{8}{9}\alpha_s \alpha L_{\nu d,ijkl}^{S,LR} \\ & + \frac{377}{81}\alpha^2 L_{\nu d,ijkl}^{S,LR} ; \end{aligned}$$

$$\begin{aligned} \dot{L}_{\nu d,ijkl}^{S,LL} = & -8g_s^2 L_{\nu d,ijkl}^{S,LL} - \frac{2}{3}e^2 L_{\nu d,ijkl}^{S,LL} - \frac{1012}{9}\alpha_s^2 L_{\nu d,ijkl}^{S,LL} - \frac{8}{9}\alpha_s \alpha L_{\nu d,ijkl}^{S,LL} \\ & + \frac{377}{81}\alpha^2 L_{\nu d,ijkl}^{S,LL} ; \end{aligned}$$

$$\begin{aligned} \dot{L}_{\nu d,ijkl}^{T,LL} = & \frac{8}{3}g_s^2 L_{\nu d,ijkl}^{T,LL} + \frac{2}{9}e^2 L_{\nu d,ijkl}^{T,LL} + \frac{1652}{27}\alpha_s^2 L_{\nu d,ijkl}^{T,LL} - \frac{152}{27}\alpha_s \alpha L_{\nu d,ijkl}^{T,LL} \\ & - \frac{1045}{243}\alpha^2 L_{\nu d,ijkl}^{T,LL} ; \end{aligned}$$

$$\begin{aligned} \dot{L}_{\nu u,ijkl}^{S,LR} = & -8g_s^2 L_{\nu u,ijkl}^{S,LR} - \frac{8}{3}e^2 L_{\nu u,ijkl}^{S,LR} - \frac{1012}{9}\alpha_s^2 L_{\nu u,ijkl}^{S,LR} - \frac{32}{9}\alpha_s \alpha L_{\nu u,ijkl}^{S,LR} \\ & + \frac{1472}{81}\alpha^2 L_{\nu u,ijkl}^{S,LR} ; \end{aligned}$$

$$\begin{aligned} \dot{L}_{\nu u,ijkl}^{S,LL} = & -8g_s^2 L_{\nu u,ijkl}^{S,LL} - \frac{8}{3}e^2 L_{\nu u,ijkl}^{S,LL} - \frac{1012}{9}\alpha_s^2 L_{\nu u,ijkl}^{S,LL} - \frac{32}{9}\alpha_s \alpha L_{\nu u,ijkl}^{S,LL} \\ & + \frac{1472}{81}\alpha^2 L_{\nu u,ijkl}^{S,LL} ; \end{aligned}$$

$$\begin{aligned} \dot{L}_{\nu u,ijkl}^{T,LL} = & \frac{8}{3}g_s^2 L_{\nu u,ijkl}^{T,LL} + \frac{8}{9}e^2 L_{\nu u,ijkl}^{T,LL} + \frac{1652}{27}\alpha_s^2 L_{\nu u,ijkl}^{T,LL} - \frac{608}{27}\alpha_s \alpha L_{\nu u,ijkl}^{T,LL} \\ & - \frac{4864}{243}\alpha^2 L_{\nu u,ijkl}^{T,LL} ; \end{aligned}$$

$$\dot{L}_{\nu e,ijkl}^{S,LR} = \frac{353}{9}\alpha^2 L_{\nu e,ijkl}^{S,LR} - 6e^2 L_{\nu e,ijkl}^{S,LR} ;$$

$$\dot{L}_{\nu e,ijkl}^{S,LL} = \frac{353}{9}\alpha^2 L_{\nu e,ijkl}^{S,LL} - 6e^2 L_{\nu e,ijkl}^{S,LL} ;$$

$$\dot{L}_{\nu e,ijkl}^{T,LL} = 2e^2 L_{\nu e,ijkl}^{T,LL} - \frac{1501}{27}\alpha^2 L_{\nu e,ijkl}^{T,LL} ;$$

$$\dot{L}_{\nu e d u,ijkl}^{V,RR} = -4e^2 L_{\nu e d u,ijkl}^{V,RR} + 4\alpha_s \alpha L_{\nu e d u,ijkl}^{V,RR} - \frac{152}{27}\alpha^2 L_{\nu e d u,ijkl}^{V,RR} ;$$

$$\begin{aligned}
\dot{L}_{\nu edu}^{V,RL} &= -2e^2 L_{\nu edu}^{V,RL} - 4\alpha_s \alpha L_{\nu edu}^{V,RL} - \frac{469}{27} \alpha^2 L_{\nu edu}^{V,RL} ; \\
\dot{L}_{\nu edu}^{S,LR} &= -8g_s^2 L_{\nu edu}^{S,LR} + \frac{4}{3} e^2 L_{\nu edu}^{S,LR} - \frac{1012}{9} \alpha_s^2 L_{\nu edu}^{S,LR} + 12\alpha_s \alpha L_{\nu edu}^{S,LR} \\
&\quad - \frac{3832}{81} \alpha^2 L_{\nu edu}^{S,LR} ; \\
\dot{L}_{\nu edu}^{S,LL} &= -8g_s^2 L_{\nu edu}^{S,LL} + e^2 \left[ \frac{4}{3} L_{\nu edu}^{S,LL} + 8L_{\nu edu}^{T,LL} \right] - \frac{1012}{9} \alpha_s^2 L_{\nu edu}^{S,LL} \\
&\quad + \alpha_s \alpha \left[ 12L_{\nu edu}^{S,LL} - \frac{448}{9} L_{\nu edu}^{T,LL} \right] + \alpha^2 \left[ -\frac{3805}{81} L_{\nu edu}^{S,LL} - \frac{1064}{9} L_{\nu edu}^{T,LL} \right] ; \\
\dot{L}_{\nu edu}^{T,LL} &= \frac{8}{3} g_s^2 L_{\nu edu}^{T,LL} + e^2 \left[ \frac{1}{6} L_{\nu edu}^{S,LL} - \frac{40}{9} L_{\nu edu}^{T,LL} \right] + \frac{1652}{27} \alpha_s^2 L_{\nu edu}^{T,LL} \\
&\quad + \alpha_s \alpha \left[ \frac{4}{3} L_{\nu edu}^{T,LL} - \frac{4}{3} L_{\nu edu}^{S,LL} \right] + \alpha^2 \left[ \frac{3773}{243} L_{\nu edu}^{T,LL} - \frac{11}{162} L_{\nu edu}^{S,LL} \right] ;
\end{aligned}$$

## 2.11 $\Delta L = 4$ Transitions ( $\bar{\nu}_i^c \nu_j \bar{\nu}_k^c \nu_l$ )

$$\dot{L}_{\nu\nu}^{S,LL} = 0 ;$$

## 2.12 $|\Delta B| = |\Delta L| = 1$ Transitions: Baryon Number Violation

$$\begin{aligned}
\dot{L}_{ddd}^{S,LL} &= -4g_s^2 L_{ddd}^{S,LL} - \frac{4}{3} e^2 L_{ddd}^{S,LL} + \frac{370}{9} \alpha_s^2 L_{ddd}^{S,LL} + \alpha_s \alpha \left[ -\frac{260}{27} L_{ddd}^{S,LL} \right. \\
&\quad \left. - \frac{256}{27} L_{ddd}^{S,LL} \right] + \alpha^2 \left[ -\frac{10178}{243} L_{ddd}^{S,LL} - \frac{7616}{243} L_{ddd}^{S,LL} \right] ; \\
\dot{L}_{ddd}^{S,RR} &= -4g_s^2 L_{ddd}^{S,RR} - \frac{4}{3} e^2 L_{ddd}^{S,RR} + \frac{370}{9} \alpha_s^2 L_{ddd}^{S,RR} + \alpha_s \alpha \left[ -\frac{260}{27} L_{ddd}^{S,RR} \right. \\
&\quad \left. - \frac{256}{27} L_{ddd}^{S,RR} \right] + \alpha^2 \left[ -\frac{10178}{243} L_{ddd}^{S,RR} - \frac{7616}{243} L_{ddd}^{S,RR} \right] ; \\
\dot{L}_{ddd}^{S,LR} &= -4g_s^2 L_{ddd}^{S,LR} - \frac{4}{3} e^2 L_{ddd}^{S,LR} + \frac{250}{9} \alpha_s^2 L_{ddd}^{S,LR} - \frac{4}{9} \alpha_s \alpha L_{ddd}^{S,LR}
\end{aligned}$$

$$\begin{aligned}
& -\frac{4114}{81}\alpha^2 L_{ijkl}^{S,LR} ; \\
\dot{L}_{ijkl}^{S,RL} &= -4g_s^2 L_{ijkl}^{S,RL} - \frac{4}{3}e^2 L_{ijkl}^{S,RL} + \frac{250}{9}\alpha_s^2 L_{ijkl}^{S,RL} - \frac{4}{9}\alpha_s\alpha L_{ijkl}^{S,RL} \\
& -\frac{4114}{81}\alpha^2 L_{ijkl}^{S,RL} ; \\
\dot{L}_{ijkl}^{S,LL} &= -4g_s^2 L_{ijkl}^{S,LL} + e^2 \left[ -\frac{2}{3}L_{ijkl}^{S,LL} - \frac{4}{3}L_{ikjl}^{S,LL} \right] + \frac{370}{9}\alpha_s^2 L_{ijkl}^{S,LL} \\
& + \alpha_s\alpha \left[ \frac{16}{3}L_{ikjl}^{S,LL} - \frac{8}{3}L_{ijkl}^{S,LL} \right] + \alpha^2 \left[ \frac{119}{27}L_{ijkl}^{S,LL} + \frac{1568}{81}L_{ikjl}^{S,LL} \right] ; \\
\dot{L}_{ijkl}^{S,RR} &= -4g_s^2 L_{ijkl}^{S,RR} + e^2 \left[ -\frac{2}{3}L_{ijkl}^{S,RR} - \frac{4}{3}L_{ilkj}^{S,RR} \right] + \frac{370}{9}\alpha_s^2 L_{ijkl}^{S,RR} \\
& + \alpha_s\alpha \left[ -\frac{584}{27}L_{ijkl}^{S,RR} - \frac{304}{27}L_{ilkj}^{S,RR} \right] + \alpha^2 \left[ -\frac{6113}{243}L_{ijkl}^{S,RR} - \frac{1688}{243}L_{ilkj}^{S,RR} \right] ; \\
\dot{L}_{ijkl}^{S,LR} &= -4g_s^2 L_{ijkl}^{S,LR} - \frac{4}{3}e^2 L_{ijkl}^{S,LR} + \frac{250}{9}\alpha_s^2 L_{ijkl}^{S,LR} - \frac{184}{9}\alpha_s\alpha L_{ijkl}^{S,LR} \\
& -\frac{2368}{81}\alpha^2 L_{ijkl}^{S,LR} ; \\
\dot{L}_{ijkl}^{S,RL} &= -4g_s^2 L_{ijkl}^{S,RL} - \frac{4}{3}e^2 L_{ijkl}^{S,RL} + \frac{250}{9}\alpha_s^2 L_{ijkl}^{S,RL} + \frac{16}{9}\alpha_s\alpha L_{ijkl}^{S,RL} \\
& + \frac{1240}{81}\alpha^2 L_{ijkl}^{S,RL} ; \\
\dot{L}_{ijkl}^{S,LR} &= -4g_s^2 L_{ijkl}^{S,LR} + \frac{2}{3}e^2 L_{ijkl}^{S,LR} + \frac{250}{9}\alpha_s^2 L_{ijkl}^{S,LR} - \frac{8}{9}\alpha_s\alpha L_{ijkl}^{S,LR} \\
& -\frac{1367}{81}\alpha^2 L_{ijkl}^{S,LR} ; \\
\dot{L}_{ijkl}^{S,RL} &= -4g_s^2 L_{ijkl}^{S,RL} + \frac{2}{3}e^2 L_{ijkl}^{S,RL} + \frac{250}{9}\alpha_s^2 L_{ijkl}^{S,RL} - \frac{8}{9}\alpha_s\alpha L_{ijkl}^{S,RL} \\
& -\frac{1367}{81}\alpha^2 L_{ijkl}^{S,RL} ;
\end{aligned}$$

$$\begin{aligned}
\dot{L}_{\substack{uud \\ ijkl}}^{S,LR} &= -4g_s^2 L_{\substack{uud \\ ijkl}}^{S,LR} + \frac{14}{3} e^2 L_{\substack{uud \\ ijkl}}^{S,LR} + \frac{250}{9} \alpha_s^2 L_{\substack{uud \\ ijkl}}^{S,LR} - \frac{68}{9} \alpha_s \alpha L_{\substack{uud \\ ijkl}}^{S,LR} \\
&\quad - \frac{7967}{81} \alpha^2 L_{\substack{uud \\ ijkl}}^{S,LR} ; \\
\dot{L}_{\substack{uud \\ ijkl}}^{S,RL} &= -4g_s^2 L_{\substack{uud \\ ijkl}}^{S,RL} + \frac{14}{3} e^2 L_{\substack{uud \\ ijkl}}^{S,RL} + \frac{250}{9} \alpha_s^2 L_{\substack{uud \\ ijkl}}^{S,RL} - \frac{68}{9} \alpha_s \alpha L_{\substack{uud \\ ijkl}}^{S,RL} \\
&\quad - \frac{7967}{81} \alpha^2 L_{\substack{uud \\ ijkl}}^{S,RL} ; \\
\dot{L}_{\substack{duu \\ ijkl}}^{S,LL} &= -4g_s^2 L_{\substack{duu \\ ijkl}}^{S,LL} + e^2 \left[ -2L_{\substack{duu \\ ijkl}}^{S,LL} - \frac{20}{3} L_{\substack{duu \\ ikjl}}^{S,LL} \right] + \frac{370}{9} \alpha_s^2 L_{\substack{duu \\ ijkl}}^{S,LL} \\
&\quad + \alpha_s \alpha \left[ \frac{20}{3} L_{\substack{duu \\ ijkl}}^{S,LL} + 16L_{\substack{duu \\ ikjl}}^{S,LL} \right] + \alpha^2 \left[ \frac{1037}{81} L_{\substack{duu \\ ijkl}}^{S,LL} + \frac{8560}{81} L_{\substack{duu \\ ikjl}}^{S,LL} \right] ; \\
\dot{L}_{\substack{duu \\ ijkl}}^{S,RR} &= -4g_s^2 L_{\substack{duu \\ ijkl}}^{S,RR} + e^2 \left[ -2L_{\substack{duu \\ ijkl}}^{S,RR} - \frac{20}{3} L_{\substack{duu \\ ikjl}}^{S,RR} \right] + \frac{370}{9} \alpha_s^2 L_{\substack{duu \\ ijkl}}^{S,RR} \\
&\quad + \alpha_s \alpha \left[ \frac{20}{3} L_{\substack{duu \\ ijkl}}^{S,RR} + 16L_{\substack{duu \\ ikjl}}^{S,RR} \right] + \alpha^2 \left[ \frac{1037}{81} L_{\substack{duu \\ ijkl}}^{S,RR} + \frac{8560}{81} L_{\substack{duu \\ ikjl}}^{S,RR} \right] ; \\
\dot{L}_{\substack{duu \\ ijkl}}^{S,LR} &= -4g_s^2 L_{\substack{duu \\ ijkl}}^{S,LR} - \frac{16}{3} e^2 L_{\substack{duu \\ ijkl}}^{S,LR} + \frac{250}{9} \alpha_s^2 L_{\substack{duu \\ ijkl}}^{S,LR} + \frac{88}{9} \alpha_s \alpha L_{\substack{duu \\ ijkl}}^{S,LR} \\
&\quad - \frac{152}{81} \alpha^2 L_{\substack{duu \\ ijkl}}^{S,LR} ; \\
\dot{L}_{\substack{duu \\ ijkl}}^{S,RL} &= -4g_s^2 L_{\substack{duu \\ ijkl}}^{S,RL} - \frac{16}{3} e^2 L_{\substack{duu \\ ijkl}}^{S,RL} + \frac{250}{9} \alpha_s^2 L_{\substack{duu \\ ijkl}}^{S,RL} + \frac{88}{9} \alpha_s \alpha L_{\substack{duu \\ ijkl}}^{S,RL} \\
&\quad - \frac{152}{81} \alpha^2 L_{\substack{duu \\ ijkl}}^{S,RL} ;
\end{aligned}$$



### 3 Three Flavor LEFT

#### 3.1 $\Delta F = 2$ Transitions ( $\bar{f}_i f_j \bar{f}_i f_j$ )

##### 3.1.1 $\Delta F = 2$ : $d$ -type ( $\bar{d}_i d_j \bar{d}_i d_j$ )

$$\begin{aligned}
\dot{L}_{dd,ij}^{V,LL} &= 4g_s^2 L_{dd,ij}^{V,LL} + \frac{4}{3}e^2 L_{dd,ij}^{V,LL} - \frac{47}{9}\alpha_s^2 L_{dd,ij}^{V,LL} - \frac{148}{9}\alpha_s \alpha L_{dd,ij}^{V,LL} \\
&\quad - \frac{2}{9}\alpha^2 L_{dd,ij}^{V,LL} ; \\
\dot{L}_{dd,ij}^{V,RR} &= 4g_s^2 L_{dd,ij}^{V,RR} + \frac{4}{3}e^2 L_{dd,ij}^{V,RR} - \frac{47}{9}\alpha_s^2 L_{dd,ij}^{V,RR} - \frac{148}{9}\alpha_s \alpha L_{dd,ij}^{V,RR} \\
&\quad - \frac{2}{9}\alpha^2 L_{dd,ij}^{V,RR} ; \\
\dot{L}_{dd,ij}^{V1,LR} &= -\frac{8}{3}g_s^2 L_{dd,ij}^{V8,LR} - \frac{4}{3}e^2 L_{dd,ij}^{V1,LR} + \alpha_s^2 \left[ -\frac{28}{3}L_{dd,ij}^{V1,LR} - \frac{2132}{27}L_{dd,ij}^{V8,LR} \right] \\
&\quad + \alpha_s \alpha \left[ \frac{32}{3}L_{dd,ij}^{V1,LR} - \frac{8}{27}L_{dd,ij}^{V8,LR} \right] + \frac{362}{27}\alpha^2 L_{dd,ij}^{V1,LR} ; \\
\dot{L}_{dd,ij}^{V8,LR} &= g_s^2 \left[ -12L_{dd,ij}^{V1,LR} - 14L_{dd,ij}^{V8,LR} \right] - \frac{4}{3}e^2 L_{dd,ij}^{V8,LR} + \alpha_s^2 \left[ -\frac{418}{3}L_{dd,ij}^{V1,LR} \right. \\
&\quad \left. - \frac{3067}{18}L_{dd,ij}^{V8,LR} \right] + \alpha_s \alpha \left[ -\frac{4}{3}L_{dd,ij}^{V1,LR} - \frac{26}{9}L_{dd,ij}^{V8,LR} \right] + \frac{362}{27}\alpha^2 L_{dd,ij}^{V8,LR} ; \\
\dot{L}_{dd,ij}^{S1,RR} &= g_s^2 \left[ \frac{160}{27}L_{dd,ij}^{S8,RR} - \frac{80}{9}L_{dd,ij}^{S1,RR} \right] + e^2 \left[ \frac{4}{27}L_{dd,ij}^{S1,RR} + \frac{64}{81}L_{dd,ij}^{S8,RR} \right] \\
&\quad + \alpha_s^2 \left[ \frac{19520}{243}L_{dd,ij}^{S8,RR} - \frac{10264}{81}L_{dd,ij}^{S1,RR} \right] + \alpha_s \alpha \left[ \frac{352}{243}L_{dd,ij}^{S8,RR} - \frac{1040}{81}L_{dd,ij}^{S1,RR} \right] \\
&\quad + \alpha^2 \left[ \frac{266}{81}L_{dd,ij}^{S1,RR} - \frac{256}{243}L_{dd,ij}^{S8,RR} \right] ; \\
\dot{L}_{dd,ij}^{S8,RR} &= g_s^2 \left[ \frac{8}{3}L_{dd,ij}^{S1,RR} + \frac{92}{9}L_{dd,ij}^{S8,RR} \right] + e^2 \left[ \frac{32}{9}L_{dd,ij}^{S1,RR} - \frac{28}{27}L_{dd,ij}^{S8,RR} \right] \\
&\quad + \alpha_s^2 \left[ \frac{7129}{81}L_{dd,ij}^{S8,RR} - \frac{104}{27}L_{dd,ij}^{S1,RR} \right] + \alpha_s \alpha \left[ -\frac{1840}{27}L_{dd,ij}^{S1,RR} - \frac{208}{81}L_{dd,ij}^{S8,RR} \right]
\end{aligned}$$

$$+ \alpha^2 \left[ \frac{394}{81} L_{ijij}^{S8,RR} - \frac{128}{27} L_{ijij}^{S1,RR} \right] ;$$

### 3.1.2 $\Delta F = 2$ : $e$ -type ( $\bar{e}_i e_j \bar{e}_i e_j$ )

$$\dot{L}_{ijij}^{V,LL} = 12e^2 L_{ijij}^{V,LL} - \frac{310}{3} \alpha^2 L_{ijij}^{V,LL} ;$$

$$\dot{L}_{ijij}^{V,RR} = 12e^2 L_{ijij}^{V,RR} - \frac{310}{3} \alpha^2 L_{ijij}^{V,RR} ;$$

$$\dot{L}_{ijij}^{V,LR} = \frac{442}{3} \alpha^2 L_{ijij}^{V,LR} - 12e^2 L_{ijij}^{V,LR} ;$$

$$\dot{L}_{ijij}^{S,RR} = 12e^2 L_{ijij}^{S,RR} - 374 \alpha^2 L_{ijij}^{S,RR} ;$$

### 3.1.3 $\Delta F = 2$ : $\nu$ -type ( $\bar{\nu}_i \nu_j \bar{\nu}_i \nu_j$ )

$$\dot{L}_{ijij}^{V,LL} = 0 ;$$

## 3.2 $\Delta F = 1.5$ Transitions ( $\bar{f}_i f_j \bar{f}_k f_j$ )

### 3.2.1 $\Delta F = 2$ : $\nu$ -type ( $\bar{\nu}_i \nu_j \bar{\nu}_k \nu_j$ )

$$\dot{L}_{ijkj}^{V,LL} = 0 ;$$

$$\dot{L}_{jijk}^{V,LL} = 0 ;$$

## 3.3 $\Delta F = 1$ Transitions ( $\bar{f}_i f_j \bar{f}_k' f_l'$ )

### 3.3.1 $\Delta F = 1$ : $ed$ -type ( $\bar{e}_i e_j \bar{d}_k d_l$ )

$$\dot{L}_{ijkl}^{V,LL} = 4e^2 L_{ijkl}^{V,LL} - 16\alpha_s \alpha L_{ijkl}^{V,LL} - \frac{130}{9} \alpha^2 L_{ijkl}^{V,LL} ;$$

$$\dot{L}_{ijkl}^{V,RR} = 4e^2 L_{ijkl}^{V,RR} - 16\alpha_s \alpha L_{ijkl}^{V,RR} - \frac{130}{9} \alpha^2 L_{ijkl}^{V,RR} ;$$

$$\dot{L}_{ijkl}^{V,LR} = -4e^2 L_{ijkl}^{V,LR} + 16\alpha_s \alpha L_{ijkl}^{V,LR} + \frac{430}{9} \alpha^2 L_{ijkl}^{V,LR} ;$$

$$\dot{L}_{klij}^{V,LR} = -4e^2 L_{klij}^{V,LR} + 16\alpha_s \alpha L_{klij}^{V,LR} + \frac{430}{9} \alpha^2 L_{klij}^{V,LR} ;$$

$$\begin{aligned}
\dot{L}_{ed}^{S,RL} &= -8g_s^2 L_{ijkl}^{S,RL} - \frac{20}{3} e^2 L_{ijkl}^{S,RL} - \frac{1052}{9} \alpha_s^2 L_{ijkl}^{S,RL} - \frac{8}{9} \alpha_s \alpha L_{ijkl}^{S,RL} \\
&\quad + \frac{1402}{27} \alpha^2 L_{ijkl}^{S,RL} ; \\
\dot{L}_{ed}^{S,RR} &= -8g_s^2 L_{ijkl}^{S,RR} + e^2 \left[ -\frac{20}{3} L_{ijkl}^{S,RR} - 32 L_{ijkl}^{T,RR} \right] - \frac{1052}{9} \alpha_s^2 L_{ijkl}^{S,RR} \\
&\quad + \alpha_s \alpha \left[ \frac{1792}{9} L_{ijkl}^{T,RR} - \frac{8}{9} L_{ijkl}^{S,RR} \right] + \alpha^2 \left[ \frac{94}{27} L_{ijkl}^{S,RR} + \frac{14080}{27} L_{ijkl}^{T,RR} \right] ; \\
\dot{L}_{ed}^{T,RR} &= \frac{8}{3} g_s^2 L_{ijkl}^{T,RR} + e^2 \left[ \frac{20}{9} L_{ijkl}^{T,RR} - \frac{2}{3} L_{ijkl}^{S,RR} \right] + \frac{1756}{27} \alpha_s^2 L_{ijkl}^{T,RR} \\
&\quad + \alpha_s \alpha \left[ \frac{16}{3} L_{ijkl}^{S,RR} - \frac{152}{27} L_{ijkl}^{T,RR} \right] + \alpha^2 \left[ \frac{112}{27} L_{ijkl}^{S,RR} - \frac{1766}{81} L_{ijkl}^{T,RR} \right] ;
\end{aligned}$$

### 3.3.2 $\Delta F = 1$ : $\nu d$ -type ( $\bar{\nu}_i \nu_j \bar{d}_k d_l$ )

$$\begin{aligned}
\dot{L}_{\nu d}^{V,LL} &= 0 ; \\
\dot{L}_{\nu d}^{V,LR} &= 0 ;
\end{aligned}$$

### 3.3.3 $\Delta F = 1$ : $\nu e$ -type ( $\bar{\nu}_i \nu_j \bar{e}_k e_l$ )

$$\begin{aligned}
\dot{L}_{\nu e}^{V,LL} &= 0 ; \\
\dot{L}_{\nu e}^{V,LR} &= 0 ;
\end{aligned}$$

### 3.3.4 $\Delta F = 1$ : $\nu edu$ -type ( $\bar{\nu}_i e_j \bar{d}_k u_l$ )

$$\begin{aligned}
\dot{L}_{\nu edu}^{V,LL} &= -4e^2 L_{ijkl}^{V,LL} + 4\alpha_s \alpha L_{ijkl}^{V,LL} - \frac{32}{9} \alpha^2 L_{ijkl}^{V,LL} ; \\
\dot{L}_{\nu edu}^{V,LR} &= -2e^2 L_{ijkl}^{V,LR} - 4\alpha_s \alpha L_{ijkl}^{V,LR} - \frac{91}{9} \alpha^2 L_{ijkl}^{V,LR} ; \\
\dot{L}_{\nu edu}^{S,RL} &= -8g_s^2 L_{ijkl}^{S,RL} + \frac{4}{3} e^2 L_{ijkl}^{S,RL} - \frac{1052}{9} \alpha_s^2 L_{ijkl}^{S,RL} + 12\alpha_s \alpha L_{ijkl}^{S,RL} \\
&\quad - \frac{848}{27} \alpha^2 L_{ijkl}^{S,RL} ;
\end{aligned}$$

$$\begin{aligned}
\dot{L}_{\nu edu}^{S,RR}{}_{ijkl} &= -8g_s^2 L_{\nu edu}^{S,RR}{}_{ijkl} + e^2 \left[ \frac{4}{3} L_{\nu edu}^{S,RR}{}_{ijkl} + 8 L_{\nu edu}^{T,RR}{}_{ijkl} \right] - \frac{1052}{9} \alpha_s^2 L_{\nu edu}^{S,RR}{}_{ijkl} \\
&\quad + \alpha_s \alpha \left[ 12 L_{\nu edu}^{S,RR}{}_{ijkl} - \frac{448}{9} L_{\nu edu}^{T,RR}{}_{ijkl} \right] + \alpha^2 \left[ -\frac{923}{27} L_{\nu edu}^{S,RR}{}_{ijkl} - \frac{1960}{27} L_{\nu edu}^{T,RR}{}_{ijkl} \right]; \\
\dot{L}_{\nu edu}^{T,RR}{}_{ijkl} &= \frac{8}{3} g_s^2 L_{\nu edu}^{T,RR}{}_{ijkl} + e^2 \left[ \frac{1}{6} L_{\nu edu}^{S,RR}{}_{ijkl} - \frac{40}{9} L_{\nu edu}^{T,RR}{}_{ijkl} \right] + \frac{1756}{27} \alpha_s^2 L_{\nu edu}^{T,RR}{}_{ijkl} \\
&\quad + \alpha_s \alpha \left[ \frac{4}{3} L_{\nu edu}^{T,RR}{}_{ijkl} - \frac{4}{3} L_{\nu edu}^{S,RR}{}_{ijkl} \right] + \alpha^2 \left[ \frac{1}{54} L_{\nu edu}^{S,RR}{}_{ijkl} + \frac{763}{81} L_{\nu edu}^{T,RR}{}_{ijkl} \right];
\end{aligned}$$

### 3.4 $\Delta F = 1^{\bar{f}f}$ Transitions ( $\bar{f}_i f_j \bar{f}'_k f'_k$ )

### 3.5 $\Delta F = 1^{\bar{f}f}$ : $d$ -type ( $\bar{d}_i d_j \bar{f}_k f_k$ )

$$\begin{aligned}
\dot{L}_{ed}^{V,LL}{}_{11ij} &= e^2 \left[ \frac{4}{3} L_{dd}^{V1,LR}{}_{ijii} + \frac{4}{3} L_{dd}^{V1,LR}{}_{ijjj} + \frac{32}{9} L_{dd}^{V,LL}{}_{ijii} + \frac{32}{9} L_{dd}^{V,LL}{}_{ijjj} + \frac{4}{3} L_{de}^{V,LR}{}_{ij11} \right. \\
&\quad \left. + \frac{4}{3} L_{de}^{V,LR}{}_{ij22} - \frac{8}{3} L_{du}^{V1,LR}{}_{ij11} + \frac{16}{3} L_{ed}^{V,LL}{}_{11ij} + \frac{4}{3} L_{ed}^{V,LL}{}_{22ij} - \frac{8}{3} L_{ud}^{V1,LL}{}_{11ij} \right] + \alpha_s \alpha \left[ \frac{16}{3} L_{dd}^{V1,LR}{}_{ijii} \right. \\
&\quad \left. + \frac{16}{3} L_{dd}^{V1,LR}{}_{ijjj} - \frac{992}{243} L_{dd}^{V8,LR}{}_{ijii} - \frac{992}{243} L_{dd}^{V8,LR}{}_{ijjj} + \frac{1120}{81} L_{dd}^{V,LL}{}_{ijii} + \frac{1120}{81} L_{dd}^{V,LL}{}_{ijjj} - \frac{32}{3} L_{du}^{V1,LR}{}_{ij11} \right. \\
&\quad \left. + \frac{1384}{243} L_{du}^{V8,LR}{}_{ij11} - 16 L_{ed}^{V,LL}{}_{11ij} - \frac{32}{3} L_{ud}^{V1,LL}{}_{11ij} - \frac{56}{243} L_{ud}^{V8,LL}{}_{11ij} \right] + \alpha^2 \left[ -\frac{1288}{243} L_{dd}^{V1,LR}{}_{ijii} \right. \\
&\quad \left. - \frac{1288}{243} L_{dd}^{V1,LR}{}_{ijjj} + \frac{4864}{243} L_{dd}^{V,LL}{}_{ijii} + \frac{4864}{243} L_{dd}^{V,LL}{}_{ijjj} - \frac{3160}{243} L_{de}^{V,LR}{}_{ij11} - \frac{3160}{243} L_{de}^{V,LR}{}_{ij22} \right. \\
&\quad \left. - \frac{6280}{243} L_{du}^{V1,LR}{}_{ij11} + \frac{242}{243} L_{ed}^{V,LL}{}_{11ij} + \frac{3752}{243} L_{ed}^{V,LL}{}_{22ij} + \frac{2936}{243} L_{ud}^{V1,LL}{}_{11ij} \right]; \\
\dot{L}_{ed}^{V,LL}{}_{22ij} &= e^2 \left[ \frac{4}{3} L_{dd}^{V1,LR}{}_{ijii} + \frac{4}{3} L_{dd}^{V1,LR}{}_{ijjj} + \frac{32}{9} L_{dd}^{V,LL}{}_{ijii} + \frac{32}{9} L_{dd}^{V,LL}{}_{ijjj} + \frac{4}{3} L_{de}^{V,LR}{}_{ij11} \right. \\
&\quad \left. + \frac{4}{3} L_{de}^{V,LR}{}_{ij22} - \frac{8}{3} L_{du}^{V1,LR}{}_{ij11} + \frac{4}{3} L_{ed}^{V,LL}{}_{11ij} + \frac{16}{3} L_{ed}^{V,LL}{}_{22ij} - \frac{8}{3} L_{ud}^{V1,LL}{}_{11ij} \right] + \alpha_s \alpha \left[ \frac{16}{3} L_{dd}^{V1,LR}{}_{ijii} \right. \\
&\quad \left. + \frac{16}{3} L_{dd}^{V1,LR}{}_{ijjj} - \frac{992}{243} L_{dd}^{V8,LR}{}_{ijii} - \frac{992}{243} L_{dd}^{V8,LR}{}_{ijjj} + \frac{1120}{81} L_{dd}^{V,LL}{}_{ijii} + \frac{1120}{81} L_{dd}^{V,LL}{}_{ijjj} - \frac{32}{3} L_{du}^{V1,LR}{}_{ij11} \right. \\
&\quad \left. + \frac{1384}{243} L_{du}^{V8,LR}{}_{ij11} - 16 L_{ed}^{V,LL}{}_{11ij} - \frac{32}{3} L_{ud}^{V1,LL}{}_{11ij} - \frac{56}{243} L_{ud}^{V8,LL}{}_{11ij} \right] + \alpha^2 \left[ -\frac{1288}{243} L_{dd}^{V1,LR}{}_{ijii} \right. \\
&\quad \left. - \frac{1288}{243} L_{dd}^{V1,LR}{}_{ijjj} + \frac{4864}{243} L_{dd}^{V,LL}{}_{ijii} + \frac{4864}{243} L_{dd}^{V,LL}{}_{ijjj} - \frac{3160}{243} L_{de}^{V,LR}{}_{ij11} - \frac{3160}{243} L_{de}^{V,LR}{}_{ij22} \right. \\
&\quad \left. - \frac{6280}{243} L_{du}^{V1,LR}{}_{ij11} + \frac{242}{243} L_{ed}^{V,LL}{}_{11ij} + \frac{3752}{243} L_{ed}^{V,LL}{}_{22ij} + \frac{2936}{243} L_{ud}^{V1,LL}{}_{11ij} \right];
\end{aligned}$$

$$\begin{aligned}
& + \frac{1384}{243} L_{ij11}^{V8,LR} - 16 L_{22ij}^{V,LL} - \frac{32}{3} L_{11ij}^{V1,LL} - \frac{56}{243} L_{11ij}^{V8,LL} \Big] + \alpha^2 \Big[ - \frac{1288}{243} L_{ijii}^{V1,LR} \\
& - \frac{1288}{243} L_{ijjj}^{V1,LR} + \frac{4864}{243} L_{ijii}^{V,LL} + \frac{4864}{243} L_{ijjj}^{V,LL} - \frac{3160}{243} L_{ij11}^{V,LR} - \frac{3160}{243} L_{ij22}^{V,LR} \\
& - \frac{6280}{243} L_{ij11}^{V1,LR} + \frac{3752}{243} L_{11ij}^{V,LL} + \frac{242}{243} L_{22ij}^{V,LL} + \frac{2936}{243} L_{11ij}^{V1,LL} \Big] ; \\
\dot{L}_{11ij}^{V1,LL} & = \frac{8}{3} g_s^2 L_{11ij}^{V8,LL} + e^2 \Big[ - \frac{8}{9} L_{ijii}^{V1,LR} - \frac{8}{9} L_{ijjj}^{V1,LR} - \frac{64}{27} L_{ijii}^{V,LL} - \frac{64}{27} L_{ijjj}^{V,LL} \\
& - \frac{8}{9} L_{ij11}^{V,LR} - \frac{8}{9} L_{ij22}^{V,LR} + \frac{16}{9} L_{ij11}^{V1,LR} - \frac{8}{9} L_{11ij}^{V,LL} - \frac{8}{9} L_{22ij}^{V,LL} - \frac{8}{9} L_{11ij}^{V1,LL} \Big] \\
& + \alpha_s^2 \Big[ - 8 L_{ijii}^{V1,LR} - 8 L_{ijjj}^{V1,LR} + \frac{4}{27} L_{ijii}^{V8,LR} + \frac{4}{27} L_{ijjj}^{V8,LR} + \frac{328}{9} L_{ijii}^{V,LL} \\
& + \frac{328}{9} L_{ijjj}^{V,LL} - 8 L_{ij11}^{V1,LR} + \frac{4}{27} L_{ij11}^{V8,LR} - \frac{4}{3} L_{11ij}^{V1,LL} + \frac{26}{9} L_{11ij}^{V8,LL} \Big] + \alpha_s \alpha \Big[ - \frac{32}{9} L_{ijii}^{V1,LR} \\
& - \frac{32}{9} L_{ijjj}^{V1,LR} + \frac{1984}{729} L_{ijii}^{V8,LR} + \frac{1984}{729} L_{ijjj}^{V8,LR} - \frac{2240}{243} L_{ijii}^{V,LL} - \frac{2240}{243} L_{ijjj}^{V,LL} \\
& + \frac{64}{9} L_{ij11}^{V1,LR} - \frac{2768}{729} L_{ij11}^{V8,LR} + \frac{256}{9} L_{11ij}^{V1,LL} - \frac{104}{729} L_{11ij}^{V8,LL} \Big] + \alpha^2 \Big[ - \frac{304}{729} L_{ijii}^{V1,LR} \\
& - \frac{304}{729} L_{ijjj}^{V1,LR} + \frac{8272}{729} L_{ijii}^{V,LL} + \frac{8272}{729} L_{ijjj}^{V,LL} - \frac{3040}{729} L_{ij11}^{V,LR} - \frac{3040}{729} L_{ij22}^{V,LR} \\
& - \frac{1120}{729} L_{ij11}^{V1,LR} + \frac{2576}{729} L_{11ij}^{V,LL} + \frac{2576}{729} L_{22ij}^{V,LL} + \frac{6368}{729} L_{11ij}^{V1,LL} \Big] ; \\
\dot{L}_{11ij}^{V8,LL} & = g_s^2 \Big[ \frac{2}{3} L_{ijii}^{V8,LR} + \frac{2}{3} L_{ijjj}^{V8,LR} + \frac{8}{3} L_{ijii}^{V,LL} + \frac{8}{3} L_{ijjj}^{V,LL} + \frac{2}{3} L_{ij11}^{V8,LR} \\
& + 12 L_{11ij}^{V1,LL} - \frac{10}{3} L_{11ij}^{V8,LL} \Big] - \frac{8}{3} e^2 L_{11ij}^{V8,LL} + \alpha_s^2 \Big[ - \frac{22}{3} L_{ijii}^{V1,LR} - \frac{22}{3} L_{ijjj}^{V1,LR} \\
& + \frac{169}{81} L_{ijii}^{V8,LR} + \frac{169}{81} L_{ijjj}^{V8,LR} + \frac{1930}{27} L_{ijii}^{V,LL} + \frac{1930}{27} L_{ijjj}^{V,LL} - \frac{22}{3} L_{ij11}^{V1,LR} + \frac{169}{81} L_{ij11}^{V8,LR} \\
& + \frac{35}{3} L_{11ij}^{V1,LL} - \frac{290}{81} L_{11ij}^{V8,LL} \Big] + \alpha_s \alpha \Big[ - \frac{208}{81} L_{ijii}^{V1,LR} - \frac{208}{81} L_{ijjj}^{V1,LR} + \frac{52}{27} L_{ijii}^{V8,LR}
\end{aligned}$$

$$\begin{aligned}
& + \frac{52}{27} L_{ijjj}^{V8,LR} - \frac{3200}{81} L_{ijii}^{V,LL} - \frac{3200}{81} L_{ijjj}^{V,LL} - \frac{208}{81} L_{ij11}^{V,LR} - \frac{208}{81} L_{ij22}^{V,LR} + \frac{416}{81} L_{ij11}^{V1,LR} \\
& - \frac{80}{27} L_{ij11}^{V8,LR} - \frac{208}{81} L_{11ij}^{V,LL} - \frac{208}{81} L_{22ij}^{V,LL} + \frac{308}{81} L_{11ij}^{V1,LL} + L_{11ij}^{V8,LL} \Big] ; \\
\dot{L}_{ijjj}^{V,LL} = & g_s^2 \left[ \frac{1}{9} L_{ijii}^{V8,LR} + \frac{1}{9} L_{ijjj}^{V8,LR} + \frac{4}{9} L_{ijii}^{V,LL} + \frac{40}{9} L_{ijjj}^{V,LL} + \frac{1}{9} L_{ij11}^{V8,LR} \right. \\
& + \left. \frac{1}{9} L_{11ij}^{V8,LL} \right] + e^2 \left[ \frac{2}{9} L_{ijii}^{V1,LR} + \frac{2}{9} L_{ijjj}^{V1,LR} + \frac{16}{27} L_{ijii}^{V,LL} + \frac{52}{27} L_{ijjj}^{V,LL} \right. \\
& + \left. \frac{2}{9} L_{ij11}^{V,LR} + \frac{2}{9} L_{ij22}^{V,LR} - \frac{4}{9} L_{ij11}^{V1,LR} + \frac{2}{9} L_{11ij}^{V,LL} + \frac{2}{9} L_{22ij}^{V,LL} - \frac{4}{9} L_{11ij}^{V1,LL} \right] \\
& + \alpha_s^2 \left[ -\frac{47}{9} L_{ijii}^{V1,LR} - \frac{47}{9} L_{ijjj}^{V1,LR} + \frac{205}{486} L_{ijii}^{V8,LR} + \frac{205}{486} L_{ijjj}^{V8,LR} + \frac{2441}{81} L_{ijii}^{V,LL} \right. \\
& + \left. \frac{2018}{81} L_{ijjj}^{V,LL} - \frac{47}{9} L_{ij11}^{V1,LR} + \frac{205}{486} L_{ij11}^{V8,LR} + \frac{35}{9} L_{11ij}^{V1,LL} + \frac{835}{486} L_{11ij}^{V8,LL} \right] \\
& + \alpha_s \alpha \left[ \frac{166}{243} L_{ijii}^{V1,LR} + \frac{166}{243} L_{ijjj}^{V1,LR} - \frac{721}{729} L_{ijii}^{V8,LR} - \frac{721}{729} L_{ijjj}^{V8,LR} + \frac{958}{243} L_{ijii}^{V,LL} \right. \\
& - \frac{3038}{243} L_{ijjj}^{V,LL} - \frac{50}{243} L_{ij11}^{V,LR} - \frac{50}{243} L_{ij22}^{V,LR} - \frac{332}{243} L_{ij11}^{V1,LR} + \frac{1331}{729} L_{ij11}^{V8,LR} \\
& - \frac{50}{243} L_{11ij}^{V,LL} - \frac{50}{243} L_{22ij}^{V,LL} - \frac{332}{243} L_{11ij}^{V1,LL} - \frac{217}{729} L_{11ij}^{V8,LL} \Big] + \alpha^2 \left[ -\frac{356}{729} L_{ijii}^{V1,LR} \right. \\
& - \frac{356}{729} L_{ijjj}^{V1,LR} + \frac{632}{729} L_{ijii}^{V,LL} + \frac{470}{729} L_{ijjj}^{V,LL} - \frac{644}{729} L_{ij11}^{V,LR} - \frac{644}{729} L_{ij22}^{V,LR} \\
& - \frac{1772}{729} L_{ij11}^{V1,LR} + \frac{868}{729} L_{11ij}^{V,LL} + \frac{868}{729} L_{22ij}^{V,LL} + \frac{244}{729} L_{11ij}^{V1,LL} \Big] ; \\
\dot{L}_{ijii}^{V,LL} = & g_s^2 \left[ \frac{1}{9} L_{ijii}^{V8,LR} + \frac{1}{9} L_{ijjj}^{V8,LR} + \frac{40}{9} L_{ijii}^{V,LL} + \frac{4}{9} L_{ijjj}^{V,LL} + \frac{1}{9} L_{ij11}^{V8,LR} \right. \\
& + \left. \frac{1}{9} L_{11ij}^{V8,LL} \right] + e^2 \left[ \frac{2}{9} L_{ijii}^{V1,LR} + \frac{2}{9} L_{ijjj}^{V1,LR} + \frac{52}{27} L_{ijii}^{V,LL} + \frac{16}{27} L_{ijjj}^{V,LL} \right. \\
& + \left. \frac{2}{9} L_{ij11}^{V,LR} + \frac{2}{9} L_{ij22}^{V,LR} - \frac{4}{9} L_{ij11}^{V1,LR} + \frac{2}{9} L_{11ij}^{V,LL} + \frac{2}{9} L_{22ij}^{V,LL} - \frac{4}{9} L_{11ij}^{V1,LL} \right]
\end{aligned}$$

$$\begin{aligned}
& + \alpha_s^2 \left[ -\frac{47}{9} L_{ij\bar{i}}^{V1,LR} - \frac{47}{9} L_{ij\bar{j}}^{V1,LR} + \frac{205}{486} L_{ij\bar{i}}^{V8,LR} + \frac{205}{486} L_{ij\bar{j}}^{V8,LR} + \frac{2018}{81} L_{ij\bar{i}}^{V,LL} \right. \\
& + \frac{2441}{81} L_{ij\bar{j}}^{V,LL} - \frac{47}{9} L_{ij11}^{V1,LR} + \frac{205}{486} L_{ij11}^{V8,LR} + \frac{35}{9} L_{11ij}^{V1,LL} + \left. \frac{835}{486} L_{11ij}^{V8,LL} \right] \\
& + \alpha_s \alpha \left[ \frac{166}{243} L_{ij\bar{i}}^{V1,LR} + \frac{166}{243} L_{ij\bar{j}}^{V1,LR} - \frac{721}{729} L_{ij\bar{i}}^{V8,LR} - \frac{721}{729} L_{ij\bar{j}}^{V8,LR} - \frac{3038}{243} L_{ij\bar{i}}^{V,LL} \right. \\
& + \frac{958}{243} L_{ij\bar{j}}^{V,LL} - \frac{50}{243} L_{ij11}^{V,LR} - \frac{50}{243} L_{ij22}^{V,LR} - \frac{332}{243} L_{ij11}^{V1,LR} + \frac{1331}{729} L_{ij11}^{V8,LR} \\
& - \frac{50}{243} L_{11ij}^{V,LL} - \frac{50}{243} L_{22ij}^{V,LL} - \frac{332}{243} L_{11ij}^{V1,LL} - \left. \frac{217}{729} L_{11ij}^{V8,LL} \right] + \alpha^2 \left[ -\frac{356}{729} L_{ij\bar{i}}^{V1,LR} \right. \\
& - \frac{356}{729} L_{ij\bar{j}}^{V1,LR} + \frac{470}{729} L_{ij\bar{i}}^{V,LL} + \frac{632}{729} L_{ij\bar{j}}^{V,LL} - \frac{644}{729} L_{ij11}^{V,LR} - \frac{644}{729} L_{ij22}^{V,LR} \\
& - \left. \frac{1772}{729} L_{ij11}^{V1,LR} + \frac{868}{729} L_{ij11}^{V,LL} + \frac{868}{729} L_{22ij}^{V,LL} + \frac{244}{729} L_{11ij}^{V1,LL} \right] ;
\end{aligned}$$

$$\begin{aligned}
\dot{L}_{ij11}^{V,LR} & = e^2 \left[ \frac{4}{3} L_{ij\bar{i}}^{V1,LR} + \frac{4}{3} L_{ij\bar{j}}^{V1,LR} + \frac{32}{9} L_{ij\bar{i}}^{V,LL} + \frac{32}{9} L_{ij\bar{j}}^{V,LL} - \frac{8}{3} L_{ij11}^{V,LR} \right. \\
& + \frac{4}{3} L_{ij22}^{V,LR} - \frac{8}{3} L_{ij11}^{V1,LR} + \frac{4}{3} L_{11ij}^{V,LL} + \frac{4}{3} L_{22ij}^{V,LL} - \left. \frac{8}{3} L_{11ij}^{V1,LL} \right] + \alpha_s \alpha \left[ \frac{16}{3} L_{ij\bar{i}}^{V1,LR} \right. \\
& + \frac{16}{3} L_{ij\bar{j}}^{V1,LR} - \frac{992}{243} L_{ij\bar{i}}^{V8,LR} - \frac{992}{243} L_{ij\bar{j}}^{V8,LR} + \frac{1120}{81} L_{ij\bar{i}}^{V,LL} + \frac{1120}{81} L_{ij\bar{j}}^{V,LL} + 16 L_{ij11}^{V,LR} \\
& - \frac{32}{3} L_{ij11}^{V1,LR} + \frac{1384}{243} L_{ij11}^{V8,LR} - \frac{32}{3} L_{11ij}^{V1,LL} - \frac{56}{243} L_{11ij}^{V8,LL} \left. \right] + \alpha^2 \left[ \frac{1736}{243} L_{ij\bar{i}}^{V1,LR} \right. \\
& + \frac{1736}{243} L_{ij\bar{j}}^{V1,LR} - \frac{752}{243} L_{ij\bar{i}}^{V,LL} - \frac{752}{243} L_{ij\bar{j}}^{V,LL} + \frac{15362}{243} L_{ij11}^{V,LR} + \frac{3752}{243} L_{ij22}^{V,LR} \\
& - \left. \frac{664}{243} L_{ij11}^{V1,LR} - \frac{1000}{243} L_{11ij}^{V,LL} - \frac{1000}{243} L_{22ij}^{V,LL} - \frac{7000}{243} L_{11ij}^{V1,LL} \right] ;
\end{aligned}$$

$$\begin{aligned}
\dot{L}_{ij22}^{V,LR} & = e^2 \left[ \frac{4}{3} L_{ij\bar{i}}^{V1,LR} + \frac{4}{3} L_{ij\bar{j}}^{V1,LR} + \frac{32}{9} L_{ij\bar{i}}^{V,LL} + \frac{32}{9} L_{ij\bar{j}}^{V,LL} + \frac{4}{3} L_{ij11}^{V,LR} \right. \\
& - \frac{8}{3} L_{ij22}^{V,LR} - \frac{8}{3} L_{ij11}^{V1,LR} + \frac{4}{3} L_{11ij}^{V,LL} + \frac{4}{3} L_{22ij}^{V,LL} - \left. \frac{8}{3} L_{11ij}^{V1,LL} \right] + \alpha_s \alpha \left[ \frac{16}{3} L_{ij\bar{i}}^{V1,LR} \right.
\end{aligned}$$

$$\begin{aligned}
& + \frac{16}{3} L_{ijj}^{V1,LR} - \frac{992}{243} L_{ijii}^{V8,LR} - \frac{992}{243} L_{ijjj}^{V8,LR} + \frac{1120}{81} L_{ijii}^{V,LL} + \frac{1120}{81} L_{ijjj}^{V,LL} + 16 L_{ij22}^{V,LR} \\
& - \frac{32}{3} L_{ij11}^{V1,LR} + \frac{1384}{243} L_{ij11}^{V8,LR} - \frac{32}{3} L_{11ij}^{V1,LL} - \frac{56}{243} L_{11ij}^{V8,LL} \left] + \alpha^2 \left[ \frac{1736}{243} L_{ijii}^{V1,LR} \right. \right. \\
& + \frac{1736}{243} L_{ijjj}^{V1,LR} - \frac{752}{243} L_{ijii}^{V,LL} - \frac{752}{243} L_{ijjj}^{V,LL} + \frac{3752}{243} L_{ij11}^{V,LR} + \frac{15362}{243} L_{ij22}^{V,LR} \\
& \left. \left. - \frac{664}{243} L_{ij11}^{V1,LR} - \frac{1000}{243} L_{11ij}^{V,LL} - \frac{1000}{243} L_{22ij}^{V,LL} - \frac{7000}{243} L_{11ij}^{V1,LL} \right] ; \right. \\
\dot{L}_{ij11}^{V1,LR} & = - \frac{8}{3} g_s^2 L_{ij11}^{V8,LR} + e^2 \left[ - \frac{8}{9} L_{ijii}^{V1,LR} - \frac{8}{9} L_{ijjj}^{V1,LR} - \frac{64}{27} L_{ijii}^{V,LL} - \frac{64}{27} L_{ijjj}^{V,LL} \right. \\
& - \frac{8}{9} L_{ij11}^{V,LR} - \frac{8}{9} L_{ij22}^{V,LR} + \frac{40}{9} L_{ij11}^{V1,LR} - \frac{8}{9} L_{11ij}^{V,LL} - \frac{8}{9} L_{22ij}^{V,LL} + \frac{16}{9} L_{11ij}^{V1,LL} \left. \right] \\
& + \alpha_s^2 \left[ 8 L_{ijii}^{V1,LR} + 8 L_{ijjj}^{V1,LR} + \frac{44}{27} L_{ijii}^{V8,LR} + \frac{44}{27} L_{ijjj}^{V8,LR} - \frac{232}{9} L_{ijii}^{V,LL} \right. \\
& - \frac{232}{9} L_{ijjj}^{V,LL} - \frac{4}{3} L_{ij11}^{V1,LR} - \frac{232}{3} L_{ij11}^{V8,LR} - 8 L_{11ij}^{V1,LL} + \frac{44}{27} L_{11ij}^{V8,LL} \left. \right] + \alpha_s \alpha \left[ - \frac{32}{9} L_{ijii}^{V1,LR} \right. \\
& - \frac{32}{9} L_{ijjj}^{V1,LR} + \frac{1984}{729} L_{ijii}^{V8,LR} + \frac{1984}{729} L_{ijjj}^{V8,LR} - \frac{2240}{243} L_{ijii}^{V,LL} - \frac{2240}{243} L_{ijjj}^{V,LL} \\
& - \frac{128}{9} L_{ij11}^{V1,LR} + \frac{3496}{729} L_{ij11}^{V8,LR} + \frac{64}{9} L_{11ij}^{V1,LL} + \frac{112}{729} L_{11ij}^{V8,LL} \left. \right] + \alpha^2 \left[ \frac{3728}{729} L_{ijii}^{V1,LR} \right. \\
& + \frac{3728}{729} L_{ijjj}^{V1,LR} + \frac{784}{729} L_{ijii}^{V,LL} + \frac{784}{729} L_{ijjj}^{V,LL} + \frac{6176}{729} L_{ij11}^{V,LR} + \frac{6176}{729} L_{ij22}^{V,LR} \\
& \left. \left. - \frac{17392}{729} L_{ij11}^{V1,LR} - \frac{3760}{729} L_{11ij}^{V,LL} - \frac{3760}{729} L_{22ij}^{V,LL} - \frac{6880}{729} L_{11ij}^{V1,LL} \right] ; \right. \\
\dot{L}_{ij11}^{V8,LR} & = g_s^2 \left[ \frac{2}{3} L_{ijii}^{V8,LR} + \frac{2}{3} L_{ijjj}^{V8,LR} + \frac{8}{3} L_{ijii}^{V,LL} + \frac{8}{3} L_{ijjj}^{V,LL} - 12 L_{ij11}^{V1,LR} \right. \\
& - \frac{40}{3} L_{ij11}^{V8,LR} + \frac{2}{3} L_{11ij}^{V8,LL} \left. \right] + \frac{8}{3} e^2 L_{ij11}^{V8,LR} + \alpha_s^2 \left[ - \frac{22}{3} L_{ijii}^{V1,LR} - \frac{22}{3} L_{ijjj}^{V1,LR} \right. \\
& + \frac{799}{81} L_{ijii}^{V8,LR} + \frac{799}{81} L_{ijjj}^{V8,LR} + \frac{1210}{27} L_{ijii}^{V,LL} + \frac{1210}{27} L_{ijjj}^{V,LL} - \frac{440}{3} L_{ij11}^{V1,LR} - \frac{26005}{162} L_{ij11}^{V8,LR} \\
& \left. \left. - \frac{440}{3} L_{11ij}^{V,LL} - \frac{26005}{162} L_{11ij}^{V8,LL} \right] ; \right.
\end{aligned}$$



$$\begin{aligned}
& -\frac{2}{3}L_{11ij}^{V1,LL} + \frac{619}{81}L_{11ij}^{V8,LL} \Big] + \alpha_s \alpha \Big[ -\frac{928}{81}L_{ijii}^{V1,LR} - \frac{928}{81}L_{ijjj}^{V1,LR} - \frac{44}{9}L_{ijii}^{V8,LR} \\
& -\frac{44}{9}L_{ijjj}^{V8,LR} - \frac{2192}{81}L_{ijii}^{V,LL} - \frac{2192}{81}L_{ijjj}^{V,LL} - \frac{928}{81}L_{ij11}^{V,LR} - \frac{928}{81}L_{ij22}^{V,LR} + \frac{4988}{81}L_{ij11}^{V1,LR} \\
& + 27L_{ij11}^{V8,LR} - \frac{928}{81}L_{11ij}^{V,LL} - \frac{928}{81}L_{22ij}^{V,LL} + \frac{1856}{81}L_{11ij}^{V1,LL} - \frac{160}{27}L_{11ij}^{V8,LL} \Big] \\
& -\frac{880}{27}\alpha^2 L_{ij11}^{V8,LR} ; \\
\dot{L}_{ijjj}^{V1,LR} = & -\frac{8}{3}g_s^2 L_{ijjj}^{V8,LR} + e^2 \Big[ \frac{4}{9}L_{ijii}^{V1,LR} - \frac{8}{9}L_{ijjj}^{V1,LR} + \frac{32}{27}L_{ijii}^{V,LL} + \frac{32}{27}L_{ijjj}^{V,LL} \\
& + \frac{4}{9}L_{ij11}^{V,LR} + \frac{4}{9}L_{ij22}^{V,LR} - \frac{8}{9}L_{ij11}^{V1,LR} + \frac{4}{9}L_{11ij}^{V,LL} + \frac{4}{9}L_{22ij}^{V,LL} - \frac{8}{9}L_{11ij}^{V1,LL} \Big] \\
& + \alpha_s^2 \Big[ 8L_{ijii}^{V1,LR} - \frac{4}{3}L_{ijjj}^{V1,LR} + \frac{44}{27}L_{ijii}^{V8,LR} - \frac{232}{3}L_{ijjj}^{V8,LR} - \frac{232}{9}L_{ijii}^{V,LL} \\
& - \frac{232}{9}L_{ijjj}^{V,LL} + 8L_{ij11}^{V1,LR} + \frac{44}{27}L_{ij11}^{V8,LR} - 8L_{11ij}^{V1,LL} + \frac{44}{27}L_{11ij}^{V8,LL} \Big] + \alpha_s \alpha \Big[ \frac{16}{9}L_{ijii}^{V1,LR} \\
& + \frac{112}{9}L_{ijjj}^{V1,LR} - \frac{992}{729}L_{ijii}^{V8,LR} - \frac{1208}{729}L_{ijjj}^{V8,LR} + \frac{1120}{243}L_{ijii}^{V,LL} + \frac{1120}{243}L_{ijjj}^{V,LL} \\
& - \frac{32}{9}L_{ij11}^{V1,LR} + \frac{1384}{729}L_{ij11}^{V8,LR} - \frac{32}{9}L_{11ij}^{V1,LL} - \frac{56}{729}L_{11ij}^{V8,LL} \Big] + \alpha^2 \Big[ \frac{296}{729}L_{ijii}^{V1,LR} \\
& + \frac{10070}{729}L_{ijjj}^{V1,LR} - \frac{608}{729}L_{ijii}^{V,LL} - \frac{608}{729}L_{ijjj}^{V,LL} + \frac{1016}{729}L_{ij11}^{V,LR} + \frac{1016}{729}L_{ij22}^{V,LR} \\
& - \frac{1672}{729}L_{ij11}^{V1,LR} + \frac{152}{729}L_{11ij}^{V,LL} + \frac{152}{729}L_{22ij}^{V,LL} - \frac{2824}{729}L_{11ij}^{V1,LL} \Big] ; \\
\dot{L}_{ijjj}^{V8,LR} = & g_s^2 \Big[ -12L_{ijjj}^{V1,LR} + \frac{2}{3}L_{ijii}^{V8,LR} - \frac{40}{3}L_{ijjj}^{V8,LR} + \frac{8}{3}L_{ijii}^{V,LL} + \frac{8}{3}L_{ijjj}^{V,LL} \\
& + \frac{2}{3}L_{ij11}^{V8,LR} + \frac{2}{3}L_{11ij}^{V8,LL} \Big] - \frac{4}{3}e^2 L_{ijjj}^{V8,LR} + \alpha_s^2 \Big[ -\frac{22}{3}L_{ijii}^{V1,LR} - \frac{440}{3}L_{ijjj}^{V1,LR} \\
& + \frac{799}{81}L_{ijii}^{V8,LR} - \frac{26005}{162}L_{ijjj}^{V8,LR} + \frac{1210}{27}L_{ijii}^{V,LL} + \frac{1210}{27}L_{ijjj}^{V,LL} - \frac{22}{3}L_{ij11}^{V1,LR}
\end{aligned}$$

$$\begin{aligned}
& + \frac{799}{81} L_{ij11}^{V8,LR} - \frac{2}{3} L_{11ij}^{V1,LL} + \frac{619}{81} L_{11ij}^{V8,LL} \left] + \alpha_s \alpha \left[ \frac{260}{81} L_{ijii}^{V1,LR} + \frac{152}{81} L_{ijjj}^{V1,LR} \right. \right. \\
& + \frac{14}{9} L_{ijii}^{V8,LR} - \frac{4}{3} L_{ijjj}^{V8,LR} + \frac{292}{81} L_{ijii}^{V,LL} + \frac{292}{81} L_{ijjj}^{V,LL} + \frac{260}{81} L_{ij11}^{V,LR} + \frac{260}{81} L_{ij22}^{V,LR} \\
& \left. - \frac{520}{81} L_{ij11}^{V1,LR} + \frac{2}{3} L_{ij11}^{V8,LR} + \frac{260}{81} L_{11ij}^{V,LL} + \frac{260}{81} L_{22ij}^{V,LL} - \frac{520}{81} L_{11ij}^{V1,LL} + \frac{122}{27} L_{11ij}^{V8,LL} \right] \\
& + \frac{362}{27} \alpha^2 L_{ijjj}^{V8,LR} ; \\
\dot{L}_{ijii}^{V1,LR} = & - \frac{8}{3} g_s^2 L_{ijii}^{V8,LR} + e^2 \left[ - \frac{8}{9} L_{ijii}^{V1,LR} + \frac{4}{9} L_{ijjj}^{V1,LR} + \frac{32}{27} L_{ijii}^{V,LL} + \frac{32}{27} L_{ijjj}^{V,LL} \right. \\
& + \frac{4}{9} L_{ij11}^{V,LR} + \frac{4}{9} L_{ij22}^{V,LR} - \frac{8}{9} L_{ij11}^{V1,LR} + \frac{4}{9} L_{11ij}^{V,LL} + \frac{4}{9} L_{22ij}^{V,LL} - \frac{8}{9} L_{11ij}^{V1,LL} \left. \right] \\
& + \alpha_s^2 \left[ - \frac{4}{3} L_{ijii}^{V1,LR} + 8 L_{ijjj}^{V1,LR} - \frac{232}{3} L_{ijii}^{V8,LR} + \frac{44}{27} L_{ijjj}^{V8,LR} - \frac{232}{9} L_{ijii}^{V,LL} \right. \\
& - \frac{232}{9} L_{ijjj}^{V,LL} + 8 L_{ij11}^{V1,LR} + \frac{44}{27} L_{ij11}^{V8,LR} - 8 L_{11ij}^{V1,LL} + \frac{44}{27} L_{11ij}^{V8,LL} \left. \right] + \alpha_s \alpha \left[ \frac{112}{9} L_{ijii}^{V1,LR} \right. \\
& + \frac{16}{9} L_{ijjj}^{V1,LR} - \frac{1208}{729} L_{ijii}^{V8,LR} - \frac{992}{729} L_{ijjj}^{V8,LR} + \frac{1120}{243} L_{ijii}^{V,LL} + \frac{1120}{243} L_{ijjj}^{V,LL} \\
& - \frac{32}{9} L_{ij11}^{V1,LR} + \frac{1384}{729} L_{ij11}^{V8,LR} - \frac{32}{9} L_{11ij}^{V1,LL} - \frac{56}{729} L_{11ij}^{V8,LL} \left. \right] + \alpha^2 \left[ \frac{10070}{729} L_{ijii}^{V1,LR} \right. \\
& + \frac{296}{729} L_{ijjj}^{V1,LR} - \frac{608}{729} L_{ijii}^{V,LL} - \frac{608}{729} L_{ijjj}^{V,LL} + \frac{1016}{729} L_{ij11}^{V,LR} + \frac{1016}{729} L_{ij22}^{V,LR} \\
& \left. - \frac{1672}{729} L_{ij11}^{V1,LR} + \frac{152}{729} L_{11ij}^{V,LL} + \frac{152}{729} L_{22ij}^{V,LL} - \frac{2824}{729} L_{11ij}^{V1,LL} \right] ; \\
\dot{L}_{ijii}^{V8,LR} = & g_s^2 \left[ - 12 L_{ijii}^{V1,LR} - \frac{40}{3} L_{ijii}^{V8,LR} + \frac{2}{3} L_{ijjj}^{V8,LR} + \frac{8}{3} L_{ijii}^{V,LL} + \frac{8}{3} L_{ijjj}^{V,LL} \right. \\
& + \frac{2}{3} L_{ij11}^{V8,LR} + \frac{2}{3} L_{11ij}^{V8,LL} \left. \right] - \frac{4}{3} e^2 L_{ijii}^{V8,LR} + \alpha_s^2 \left[ - \frac{440}{3} L_{ijii}^{V1,LR} - \frac{22}{3} L_{ijjj}^{V1,LR} \right. \\
& \left. - \frac{26005}{162} L_{ijii}^{V8,LR} + \frac{799}{81} L_{ijjj}^{V8,LR} + \frac{1210}{27} L_{ijii}^{V,LL} + \frac{1210}{27} L_{ijjj}^{V,LL} - \frac{22}{3} L_{ij11}^{V1,LR} \right.
\end{aligned}$$

$$\begin{aligned}
& + \frac{799}{81} L_{ij11}^{V8,LR} - \frac{2}{3} L_{11ij}^{V1,LL} + \frac{619}{81} L_{11ij}^{V8,LL} \left] + \alpha_s \alpha \left[ \frac{152}{81} L_{ijii}^{V1,LR} + \frac{260}{81} L_{ijjj}^{V1,LR} \right. \right. \\
& - \frac{4}{3} L_{ijii}^{V8,LR} + \frac{14}{9} L_{ijjj}^{V8,LR} + \frac{292}{81} L_{ijii}^{V,LL} + \frac{292}{81} L_{ijjj}^{V,LL} + \frac{260}{81} L_{ij11}^{V,LR} + \frac{260}{81} L_{ij22}^{V,LR} \\
& - \frac{520}{81} L_{ij11}^{V1,LR} + \frac{2}{3} L_{ij11}^{V8,LR} + \frac{260}{81} L_{11ij}^{V,LL} + \frac{260}{81} L_{22ij}^{V,LL} - \frac{520}{81} L_{11ij}^{V1,LL} + \frac{122}{27} L_{11ij}^{V8,LL} \left. \right] \\
& + \frac{362}{27} \alpha^2 L_{ijii}^{V8,LR} ; \\
\dot{L}_{11ij}^{S,RL} & = -8g_s^2 L_{11ij}^{S,RL} - \frac{20}{3} e^2 L_{11ij}^{S,RL} - \frac{1052}{9} \alpha_s^2 L_{11ij}^{S,RL} - \frac{8}{9} \alpha_s \alpha L_{11ij}^{S,RL} \\
& + \frac{1402}{27} \alpha^2 L_{11ij}^{S,RL} ; \\
\dot{L}_{22ij}^{S,RL} & = -8g_s^2 L_{22ij}^{S,RL} - \frac{20}{3} e^2 L_{22ij}^{S,RL} - \frac{1052}{9} \alpha_s^2 L_{22ij}^{S,RL} - \frac{8}{9} \alpha_s \alpha L_{22ij}^{S,RL} \\
& + \frac{1402}{27} \alpha^2 L_{22ij}^{S,RL} ; \\
\dot{L}_{1ji1}^{V1,LR} & = -\frac{8}{3} g_s^2 L_{1ji1}^{V8,LR} - \frac{10}{3} e^2 L_{1ji1}^{V1,LR} + \alpha_s^2 \left[ -\frac{28}{3} L_{1ji1}^{V1,LR} - \frac{2132}{27} L_{1ji1}^{V8,LR} \right] \\
& + \alpha_s \alpha \left[ \frac{8}{3} L_{1ji1}^{V1,LR} - \frac{128}{27} L_{1ji1}^{V8,LR} \right] + \frac{47}{27} \alpha^2 L_{1ji1}^{V1,LR} ; \\
\dot{L}_{1ji1}^{V8,LR} & = g_s^2 \left[ -12 L_{1ji1}^{V1,LR} - 14 L_{1ji1}^{V8,LR} \right] - \frac{10}{3} e^2 L_{1ji1}^{V8,LR} + \alpha_s^2 \left[ -\frac{418}{3} L_{1ji1}^{V1,LR} \right. \\
& \left. - \frac{3067}{18} L_{1ji1}^{V8,LR} \right] + \alpha_s \alpha \left[ \frac{16}{9} L_{1ji1}^{V8,LR} - \frac{64}{3} L_{1ji1}^{V1,LR} \right] + \frac{47}{27} \alpha^2 L_{1ji1}^{V8,LR} ; \\
\dot{L}_{11ij}^{S,RR} & = -8g_s^2 L_{11ij}^{S,RR} + e^2 \left[ -\frac{20}{3} L_{11ij}^{S,RR} - 32 L_{11ij}^{T,RR} \right] - \frac{1052}{9} \alpha_s^2 L_{11ij}^{S,RR} \\
& + \alpha_s \alpha \left[ \frac{1792}{9} L_{11ij}^{T,RR} - \frac{8}{9} L_{11ij}^{S,RR} \right] + \alpha^2 \left[ \frac{94}{27} L_{11ij}^{S,RR} + \frac{14080}{27} L_{11ij}^{T,RR} \right] ; \\
\dot{L}_{11ij}^{T,RR} & = \frac{8}{3} g_s^2 L_{11ij}^{T,RR} + e^2 \left[ \frac{20}{9} L_{11ij}^{T,RR} - \frac{2}{3} L_{11ij}^{S,RR} \right] + \frac{1756}{27} \alpha_s^2 L_{11ij}^{T,RR}
\end{aligned}$$

$$\begin{aligned}
& + \alpha_s \alpha \left[ \frac{16}{3} L_{11ij}^{S,RR} - \frac{152}{27} L_{11ij}^{T,RR} \right] + \alpha^2 \left[ \frac{112}{27} L_{11ij}^{S,RR} - \frac{1766}{81} L_{11ij}^{T,RR} \right]; \\
\dot{L}_{ed,22ij}^{S,RR} & = -8g_s^2 L_{ed,22ij}^{S,RR} + e^2 \left[ -\frac{20}{3} L_{ed,22ij}^{S,RR} - 32 L_{ed,22ij}^{T,RR} \right] - \frac{1052}{9} \alpha_s^2 L_{ed,22ij}^{S,RR} \\
& + \alpha_s \alpha \left[ \frac{1792}{9} L_{ed,22ij}^{T,RR} - \frac{8}{9} L_{ed,22ij}^{S,RR} \right] + \alpha^2 \left[ \frac{94}{27} L_{ed,22ij}^{S,RR} + \frac{14080}{27} L_{ed,22ij}^{T,RR} \right]; \\
\dot{L}_{ed,22ij}^{T,RR} & = \frac{8}{3} g_s^2 L_{ed,22ij}^{T,RR} + e^2 \left[ \frac{20}{9} L_{ed,22ij}^{T,RR} - \frac{2}{3} L_{ed,22ij}^{S,RR} \right] + \frac{1756}{27} \alpha_s^2 L_{ed,22ij}^{T,RR} \\
& + \alpha_s \alpha \left[ \frac{16}{3} L_{ed,22ij}^{S,RR} - \frac{152}{27} L_{ed,22ij}^{T,RR} \right] + \alpha^2 \left[ \frac{112}{27} L_{ed,22ij}^{S,RR} - \frac{1766}{81} L_{ed,22ij}^{T,RR} \right]; \\
\dot{L}_{ud,11ij}^{S1,RR} & = g_s^2 \left[ \frac{64}{9} L_{uddu,1ji1}^{S1,RR} + \frac{112}{27} L_{uddu,1ji1}^{S8,RR} - 16 L_{ud,11ij}^{S1,RR} + \frac{16}{9} L_{ud,11ij}^{S8,RR} \right] \\
& + e^2 \left[ \frac{4}{27} L_{uddu,1ji1}^{S1,RR} + \frac{16}{81} L_{uddu,1ji1}^{S8,RR} - \frac{46}{9} L_{ud,11ij}^{S1,RR} \right] + \alpha_s^2 \left[ \frac{9536}{81} L_{uddu,1ji1}^{S1,RR} + \frac{16688}{243} L_{uddu,1ji1}^{S8,RR} \right. \\
& - \frac{2200}{9} L_{ud,11ij}^{S1,RR} + \frac{944}{81} L_{ud,11ij}^{S8,RR} \left. \right] + \alpha_s \alpha \left[ \frac{1888}{81} L_{uddu,1ji1}^{S1,RR} + \frac{3808}{243} L_{uddu,1ji1}^{S8,RR} + \frac{136}{27} L_{ud,11ij}^{S1,RR} \right. \\
& + \frac{224}{81} L_{ud,11ij}^{S8,RR} \left. \right] + \alpha^2 \left[ \frac{2}{9} L_{uddu,1ji1}^{S1,RR} + \frac{8}{27} L_{uddu,1ji1}^{S8,RR} + \frac{415}{27} L_{ud,11ij}^{S1,RR} \right]; \\
\dot{L}_{ud,11ij}^{S8,RR} & = g_s^2 \left[ -\frac{16}{3} L_{uddu,1ji1}^{S1,RR} + \frac{44}{9} L_{uddu,1ji1}^{S8,RR} + 8 L_{ud,11ij}^{S1,RR} + \frac{16}{3} L_{ud,11ij}^{S8,RR} \right] \\
& + e^2 \left[ \frac{8}{9} L_{uddu,1ji1}^{S1,RR} - \frac{4}{27} L_{uddu,1ji1}^{S8,RR} - \frac{46}{9} L_{ud,11ij}^{S8,RR} \right] + \alpha_s^2 \left[ -\frac{872}{27} L_{uddu,1ji1}^{S1,RR} - \frac{2462}{81} L_{uddu,1ji1}^{S8,RR} \right. \\
& + \frac{256}{9} L_{ud,11ij}^{S1,RR} + \frac{3197}{27} L_{ud,11ij}^{S8,RR} \left. \right] + \alpha_s \alpha \left[ -\frac{868}{27} L_{uddu,1ji1}^{S1,RR} + \frac{1370}{81} L_{uddu,1ji1}^{S8,RR} + \frac{112}{9} L_{ud,11ij}^{S1,RR} \right. \\
& + \frac{224}{9} L_{ud,11ij}^{S8,RR} \left. \right] + \alpha^2 \left[ \frac{4}{3} L_{uddu,1ji1}^{S1,RR} - \frac{2}{9} L_{uddu,1ji1}^{S8,RR} + \frac{415}{27} L_{ud,11ij}^{S8,RR} \right]; \\
\dot{L}_{uddu,1ji1}^{S1,RR} & = g_s^2 \left[ -16 L_{uddu,1ji1}^{S1,RR} + \frac{16}{9} L_{uddu,1ji1}^{S8,RR} + \frac{64}{9} L_{ud,11ij}^{S1,RR} + \frac{112}{27} L_{ud,11ij}^{S8,RR} \right]
\end{aligned}$$

$$\begin{aligned}
& + e^2 \left[ \frac{26}{9} L_{1ji1}^{S1,RR} - \frac{32}{27} L_{11ij}^{S1,RR} - \frac{128}{81} L_{11ij}^{S8,RR} \right] + \alpha_s^2 \left[ -\frac{2200}{9} L_{1ji1}^{S1,RR} + \frac{944}{81} L_{1ji1}^{S8,RR} \right. \\
& + \frac{9536}{81} L_{11ij}^{S1,RR} + \frac{16688}{243} L_{11ij}^{S8,RR} \left. \right] + \alpha_s \alpha \left[ \frac{712}{27} L_{1ji1}^{S1,RR} - \frac{64}{81} L_{1ji1}^{S8,RR} - \frac{2144}{81} L_{11ij}^{S1,RR} \right. \\
& - \frac{7784}{243} L_{11ij}^{S8,RR} \left. \right] + \alpha^2 \left[ -\frac{1025}{27} L_{1ji1}^{S1,RR} + \frac{176}{27} L_{11ij}^{S1,RR} + \frac{704}{81} L_{11ij}^{S8,RR} \right] ; \\
\dot{L}_{1ji1}^{S8,RR} & = g_s^2 \left[ 8 L_{1ji1}^{S1,RR} + \frac{16}{3} L_{1ji1}^{S8,RR} - \frac{16}{3} L_{11ij}^{S1,RR} + \frac{44}{9} L_{11ij}^{S8,RR} \right] \\
& + e^2 \left[ \frac{26}{9} L_{1ji1}^{S8,RR} - \frac{64}{9} L_{11ij}^{S1,RR} + \frac{32}{27} L_{11ij}^{S8,RR} \right] + \alpha_s^2 \left[ \frac{256}{9} L_{1ji1}^{S1,RR} + \frac{3197}{27} L_{1ji1}^{S8,RR} \right. \\
& - \frac{872}{27} L_{11ij}^{S1,RR} - \frac{2462}{81} L_{11ij}^{S8,RR} \left. \right] + \alpha_s \alpha \left[ -\frac{32}{9} L_{1ji1}^{S1,RR} - \frac{400}{9} L_{1ji1}^{S8,RR} + \frac{3704}{27} L_{11ij}^{S1,RR} \right. \\
& - \frac{2050}{81} L_{11ij}^{S8,RR} \left. \right] + \alpha^2 \left[ -\frac{1025}{27} L_{1ji1}^{S8,RR} + \frac{352}{9} L_{11ij}^{S1,RR} - \frac{176}{27} L_{11ij}^{S8,RR} \right] ; \\
\dot{L}_{ijj}^{S1,RR} & = g_s^2 \left[ \frac{160}{27} L_{ijj}^{S8,RR} - \frac{80}{9} L_{ijj}^{S1,RR} \right] + e^2 \left[ \frac{4}{27} L_{ijj}^{S1,RR} + \frac{64}{81} L_{ijj}^{S8,RR} \right] \\
& + \alpha_s^2 \left[ \frac{19520}{243} L_{ijj}^{S8,RR} - \frac{10264}{81} L_{ijj}^{S1,RR} \right] + \alpha_s \alpha \left[ \frac{352}{243} L_{ijj}^{S8,RR} - \frac{1040}{81} L_{ijj}^{S1,RR} \right] \\
& + \alpha^2 \left[ \frac{266}{81} L_{ijj}^{S1,RR} - \frac{256}{243} L_{ijj}^{S8,RR} \right] ; \\
\dot{L}_{ijj}^{S8,RR} & = g_s^2 \left[ \frac{8}{3} L_{ijj}^{S1,RR} + \frac{92}{9} L_{ijj}^{S8,RR} \right] + e^2 \left[ \frac{32}{9} L_{ijj}^{S1,RR} - \frac{28}{27} L_{ijj}^{S8,RR} \right] \\
& + \alpha_s^2 \left[ \frac{7129}{81} L_{ijj}^{S8,RR} - \frac{104}{27} L_{ijj}^{S1,RR} \right] + \alpha_s \alpha \left[ -\frac{1840}{27} L_{ijj}^{S1,RR} - \frac{208}{81} L_{ijj}^{S8,RR} \right] \\
& + \alpha^2 \left[ \frac{394}{81} L_{ijj}^{S8,RR} - \frac{128}{27} L_{ijj}^{S1,RR} \right] ; \\
\dot{L}_{iji}^{S1,RR} & = g_s^2 \left[ \frac{160}{27} L_{iji}^{S8,RR} - \frac{80}{9} L_{iji}^{S1,RR} \right] + e^2 \left[ \frac{4}{27} L_{iji}^{S1,RR} + \frac{64}{81} L_{iji}^{S8,RR} \right]
\end{aligned}$$

$$\begin{aligned}
& + \alpha_s^2 \left[ \frac{19520}{243} L_{ij\bar{i}\bar{i}}^{S8,RR} - \frac{10264}{81} L_{ij\bar{i}\bar{i}}^{S1,RR} \right] + \alpha_s \alpha \left[ \frac{352}{243} L_{ij\bar{i}\bar{i}}^{S8,RR} - \frac{1040}{81} L_{ij\bar{i}\bar{i}}^{S1,RR} \right] \\
& + \alpha^2 \left[ \frac{266}{81} L_{ij\bar{i}\bar{i}}^{S1,RR} - \frac{256}{243} L_{ij\bar{i}\bar{i}}^{S8,RR} \right]; \\
\dot{L}_{ij\bar{i}\bar{i}}^{S8,RR} & = g_s^2 \left[ \frac{8}{3} L_{ij\bar{i}\bar{i}}^{S1,RR} + \frac{92}{9} L_{ij\bar{i}\bar{i}}^{S8,RR} \right] + e^2 \left[ \frac{32}{9} L_{ij\bar{i}\bar{i}}^{S1,RR} - \frac{28}{27} L_{ij\bar{i}\bar{i}}^{S8,RR} \right] \\
& + \alpha_s^2 \left[ \frac{7129}{81} L_{ij\bar{i}\bar{i}}^{S8,RR} - \frac{104}{27} L_{ij\bar{i}\bar{i}}^{S1,RR} \right] + \alpha_s \alpha \left[ -\frac{1840}{27} L_{ij\bar{i}\bar{i}}^{S1,RR} - \frac{208}{81} L_{ij\bar{i}\bar{i}}^{S8,RR} \right] \\
& + \alpha^2 \left[ \frac{394}{81} L_{ij\bar{i}\bar{i}}^{S8,RR} - \frac{128}{27} L_{ij\bar{i}\bar{i}}^{S1,RR} \right]; \\
\dot{L}_{11ij}^{V,RR} & = e^2 \left[ \frac{4}{3} L_{ii\bar{j}}^{V1,LR} + \frac{4}{3} L_{jj\bar{i}\bar{j}}^{V1,LR} + \frac{32}{9} L_{ij\bar{i}\bar{i}}^{V,RR} + \frac{32}{9} L_{ij\bar{j}\bar{j}}^{V,RR} + \frac{4}{3} L_{11ij}^{V,LR} \right. \\
& + \frac{4}{3} L_{22ij}^{V,LR} + \frac{16}{3} L_{11ij}^{V,RR} + \frac{4}{3} L_{22ij}^{V,RR} - \frac{8}{3} L_{11ij}^{V1,LR} - \frac{8}{3} L_{11ij}^{V1,RR} \left. \right] + \alpha_s \alpha \left[ \frac{16}{3} L_{ii\bar{j}}^{V1,LR} \right. \\
& + \frac{16}{3} L_{jj\bar{i}\bar{j}}^{V1,LR} - \frac{992}{243} L_{ii\bar{j}}^{V8,LR} - \frac{992}{243} L_{jj\bar{i}\bar{j}}^{V8,LR} + \frac{1120}{81} L_{ij\bar{i}\bar{i}}^{V,RR} + \frac{1120}{81} L_{ij\bar{j}\bar{j}}^{V,RR} - 16 L_{11ij}^{V,RR} \\
& - \frac{32}{3} L_{11ij}^{V1,LR} - \frac{32}{3} L_{11ij}^{V1,RR} + \frac{1384}{243} L_{11ij}^{V8,LR} - \frac{56}{243} L_{11ij}^{V8,RR} \left. \right] + \alpha^2 \left[ -\frac{1288}{243} L_{ii\bar{j}}^{V1,LR} \right. \\
& - \frac{1288}{243} L_{jj\bar{i}\bar{j}}^{V1,LR} + \frac{4864}{243} L_{ij\bar{i}\bar{i}}^{V,RR} + \frac{4864}{243} L_{ij\bar{j}\bar{j}}^{V,RR} - \frac{3160}{243} L_{11ij}^{V,LR} - \frac{3160}{243} L_{22ij}^{V,LR} \\
& + \frac{242}{243} L_{11ij}^{V,RR} + \frac{3752}{243} L_{22ij}^{V,RR} - \frac{6280}{243} L_{11ij}^{V1,LR} + \frac{2936}{243} L_{11ij}^{V1,RR} \left. \right]; \\
\dot{L}_{22ij}^{V,RR} & = e^2 \left[ \frac{4}{3} L_{ii\bar{j}}^{V1,LR} + \frac{4}{3} L_{jj\bar{i}\bar{j}}^{V1,LR} + \frac{32}{9} L_{ij\bar{i}\bar{i}}^{V,RR} + \frac{32}{9} L_{ij\bar{j}\bar{j}}^{V,RR} + \frac{4}{3} L_{11ij}^{V,LR} \right. \\
& + \frac{4}{3} L_{22ij}^{V,LR} + \frac{4}{3} L_{11ij}^{V,RR} + \frac{16}{3} L_{22ij}^{V,RR} - \frac{8}{3} L_{11ij}^{V1,LR} - \frac{8}{3} L_{11ij}^{V1,RR} \left. \right] + \alpha_s \alpha \left[ \frac{16}{3} L_{ii\bar{j}}^{V1,LR} \right. \\
& + \frac{16}{3} L_{jj\bar{i}\bar{j}}^{V1,LR} - \frac{992}{243} L_{ii\bar{j}}^{V8,LR} - \frac{992}{243} L_{jj\bar{i}\bar{j}}^{V8,LR} + \frac{1120}{81} L_{ij\bar{i}\bar{i}}^{V,RR} + \frac{1120}{81} L_{ij\bar{j}\bar{j}}^{V,RR} - 16 L_{22ij}^{V,RR} \\
& - \frac{32}{3} L_{11ij}^{V1,LR} - \frac{32}{3} L_{11ij}^{V1,RR} + \frac{1384}{243} L_{11ij}^{V8,LR} - \frac{56}{243} L_{11ij}^{V8,RR} \left. \right] + \alpha^2 \left[ -\frac{1288}{243} L_{ii\bar{j}}^{V1,LR} \right.
\end{aligned}$$

$$\begin{aligned}
& -\frac{1288}{243}L_{jjj}^{V1,LR} + \frac{4864}{243}L_{ijj}^{V,RR} + \frac{4864}{243}L_{ijj}^{V,RR} - \frac{3160}{243}L_{11j}^{V,LR} - \frac{3160}{243}L_{22j}^{V,LR} \\
& + \frac{3752}{243}L_{11j}^{V,RR} + \frac{242}{243}L_{22j}^{V,RR} - \frac{6280}{243}L_{11j}^{V1,LR} + \frac{2936}{243}L_{11j}^{V1,RR} \Bigg]; \\
\dot{L}_{11j}^{V1,RR} &= \frac{8}{3}g_s^2 L_{11j}^{V8,RR} + e^2 \Bigg[ -\frac{8}{9}L_{iii}^{V1,LR} - \frac{8}{9}L_{jjj}^{V1,LR} - \frac{64}{27}L_{ijj}^{V,RR} - \frac{64}{27}L_{ijj}^{V,RR} \\
& -\frac{8}{9}L_{11j}^{V,LR} - \frac{8}{9}L_{22j}^{V,LR} - \frac{8}{9}L_{11j}^{V,RR} - \frac{8}{9}L_{22j}^{V,RR} + \frac{16}{9}L_{11j}^{V1,LR} - \frac{8}{9}L_{11j}^{V1,RR} \Bigg] \\
& + \alpha_s^2 \Bigg[ -8L_{iii}^{V1,LR} - 8L_{jjj}^{V1,LR} + \frac{4}{27}L_{iii}^{V8,LR} + \frac{4}{27}L_{jjj}^{V8,LR} + \frac{328}{9}L_{ijj}^{V,RR} \\
& + \frac{328}{9}L_{ijj}^{V,RR} - 8L_{11j}^{V1,LR} - \frac{4}{3}L_{11j}^{V1,RR} + \frac{4}{27}L_{11j}^{V8,LR} + \frac{26}{9}L_{11j}^{V8,RR} \Bigg] + \alpha_s \alpha \Bigg[ -\frac{32}{9}L_{iii}^{V1,LR} \\
& -\frac{32}{9}L_{jjj}^{V1,LR} + \frac{1984}{729}L_{iii}^{V8,LR} + \frac{1984}{729}L_{jjj}^{V8,LR} - \frac{2240}{243}L_{ijj}^{V,RR} - \frac{2240}{243}L_{ijj}^{V,RR} \\
& + \frac{64}{9}L_{11j}^{V1,LR} + \frac{256}{9}L_{11j}^{V1,RR} - \frac{2768}{729}L_{11j}^{V8,LR} - \frac{104}{729}L_{11j}^{V8,RR} \Bigg] + \alpha^2 \Bigg[ -\frac{304}{729}L_{iii}^{V1,LR} \\
& -\frac{304}{729}L_{jjj}^{V1,LR} + \frac{8272}{729}L_{ijj}^{V,RR} + \frac{8272}{729}L_{ijj}^{V,RR} - \frac{3040}{729}L_{11j}^{V,LR} - \frac{3040}{729}L_{22j}^{V,LR} \\
& + \frac{2576}{729}L_{11j}^{V,RR} + \frac{2576}{729}L_{22j}^{V,RR} - \frac{1120}{729}L_{11j}^{V1,LR} + \frac{6368}{729}L_{11j}^{V1,RR} \Bigg]; \\
\dot{L}_{11j}^{V8,RR} &= g_s^2 \Bigg[ \frac{2}{3}L_{iii}^{V8,LR} + \frac{2}{3}L_{jjj}^{V8,LR} + \frac{8}{3}L_{ijj}^{V,RR} + \frac{8}{3}L_{ijj}^{V,RR} + 12L_{11j}^{V1,RR} \\
& + \frac{2}{3}L_{11j}^{V8,LR} - \frac{10}{3}L_{11j}^{V8,RR} \Bigg] - \frac{8}{3}e^2 L_{11j}^{V8,RR} + \alpha_s^2 \Bigg[ -\frac{22}{3}L_{iii}^{V1,LR} - \frac{22}{3}L_{jjj}^{V1,LR} \\
& + \frac{169}{81}L_{iii}^{V8,LR} + \frac{169}{81}L_{jjj}^{V8,LR} + \frac{1930}{27}L_{ijj}^{V,RR} + \frac{1930}{27}L_{ijj}^{V,RR} - \frac{22}{3}L_{11j}^{V1,LR} + \frac{35}{3}L_{11j}^{V1,RR} \\
& + \frac{169}{81}L_{11j}^{V8,LR} - \frac{290}{81}L_{11j}^{V8,RR} \Bigg] + \alpha_s \alpha \Bigg[ -\frac{208}{81}L_{iii}^{V1,LR} - \frac{208}{81}L_{jjj}^{V1,LR} + \frac{52}{27}L_{ijj}^{V8,LR} \\
& + \frac{52}{27}L_{jjj}^{V8,LR} - \frac{3200}{81}L_{ijj}^{V,RR} - \frac{3200}{81}L_{ijj}^{V,RR} - \frac{208}{81}L_{11j}^{V,LR} - \frac{208}{81}L_{22j}^{V,LR} - \frac{208}{81}L_{11j}^{V,RR}
\end{aligned}$$

$$\begin{aligned}
& -\frac{208}{81}L_{22ij}^{V,RR} + \frac{416}{81}L_{11ij}^{V1,LR} + \frac{308}{81}L_{11ij}^{V1,RR} - \frac{80}{27}L_{11ij}^{V8,LR} + L_{11ij}^{V8,RR} \Big] ; \\
\dot{L}_{ijjj}^{V,RR} &= g_s^2 \left[ \frac{1}{9}L_{iiij}^{V8,LR} + \frac{1}{9}L_{jjij}^{V8,LR} + \frac{4}{9}L_{ijii}^{V,RR} + \frac{40}{9}L_{ijjj}^{V,RR} + \frac{1}{9}L_{11ij}^{V8,LR} \right. \\
& + \left. \frac{1}{9}L_{11ij}^{V8,RR} \right] + e^2 \left[ \frac{2}{9}L_{iiij}^{V1,LR} + \frac{2}{9}L_{jjij}^{V1,LR} + \frac{16}{27}L_{ijii}^{V,RR} + \frac{52}{27}L_{ijjj}^{V,RR} \right. \\
& + \left. \frac{2}{9}L_{11ij}^{V,LR} + \frac{2}{9}L_{22ij}^{V,LR} + \frac{2}{9}L_{11ij}^{V,RR} + \frac{2}{9}L_{22ij}^{V,RR} - \frac{4}{9}L_{11ij}^{V1,LR} - \frac{4}{9}L_{11ij}^{V1,RR} \right] \\
& + \alpha_s^2 \left[ -\frac{47}{9}L_{iiij}^{V1,LR} - \frac{47}{9}L_{jjij}^{V1,LR} + \frac{205}{486}L_{iiij}^{V8,LR} + \frac{205}{486}L_{jjij}^{V8,LR} + \frac{2441}{81}L_{ijii}^{V,RR} \right. \\
& + \left. \frac{2018}{81}L_{ijjj}^{V,RR} - \frac{47}{9}L_{11ij}^{V1,LR} + \frac{35}{9}L_{11ij}^{V1,RR} + \frac{205}{486}L_{11ij}^{V8,LR} + \frac{835}{486}L_{11ij}^{V8,RR} \right] \\
& + \alpha_s \alpha \left[ \frac{166}{243}L_{iiij}^{V1,LR} + \frac{166}{243}L_{jjij}^{V1,LR} - \frac{721}{729}L_{iiij}^{V8,LR} - \frac{721}{729}L_{jjij}^{V8,LR} + \frac{958}{243}L_{ijii}^{V,RR} \right. \\
& - \frac{3038}{243}L_{ijjj}^{V,RR} - \frac{50}{243}L_{11ij}^{V,LR} - \frac{50}{243}L_{22ij}^{V,LR} - \frac{50}{243}L_{11ij}^{V,RR} - \frac{50}{243}L_{22ij}^{V,RR} - \frac{332}{243}L_{11ij}^{V1,LR} \\
& - \frac{332}{243}L_{11ij}^{V1,RR} + \frac{1331}{729}L_{11ij}^{V8,LR} - \frac{217}{729}L_{11ij}^{V8,RR} \Big] + \alpha^2 \left[ -\frac{356}{729}L_{iiij}^{V1,LR} - \frac{356}{729}L_{jjij}^{V1,LR} \right. \\
& + \frac{632}{729}L_{ijii}^{V,RR} + \frac{470}{729}L_{ijjj}^{V,RR} - \frac{644}{729}L_{11ij}^{V,LR} - \frac{644}{729}L_{22ij}^{V,LR} + \frac{868}{729}L_{11ij}^{V,RR} + \frac{868}{729}L_{22ij}^{V,RR} \\
& - \left. \frac{1772}{729}L_{11ij}^{V1,LR} + \frac{244}{729}L_{11ij}^{V1,RR} \right] ; \\
\dot{L}_{ijii}^{V,RR} &= g_s^2 \left[ \frac{1}{9}L_{iiij}^{V8,LR} + \frac{1}{9}L_{jjij}^{V8,LR} + \frac{40}{9}L_{ijii}^{V,RR} + \frac{4}{9}L_{ijjj}^{V,RR} + \frac{1}{9}L_{11ij}^{V8,LR} \right. \\
& + \left. \frac{1}{9}L_{11ij}^{V8,RR} \right] + e^2 \left[ \frac{2}{9}L_{iiij}^{V1,LR} + \frac{2}{9}L_{jjij}^{V1,LR} + \frac{52}{27}L_{ijii}^{V,RR} + \frac{16}{27}L_{ijjj}^{V,RR} \right. \\
& + \left. \frac{2}{9}L_{11ij}^{V,LR} + \frac{2}{9}L_{22ij}^{V,LR} + \frac{2}{9}L_{11ij}^{V,RR} + \frac{2}{9}L_{22ij}^{V,RR} - \frac{4}{9}L_{11ij}^{V1,LR} - \frac{4}{9}L_{11ij}^{V1,RR} \right] \\
& + \alpha_s^2 \left[ -\frac{47}{9}L_{iiij}^{V1,LR} - \frac{47}{9}L_{jjij}^{V1,LR} + \frac{205}{486}L_{iiij}^{V8,LR} + \frac{205}{486}L_{jjij}^{V8,LR} + \frac{2018}{81}L_{ijii}^{V,RR} \right.
\end{aligned}$$



$$\begin{aligned}
& + \frac{2441}{81} L_{ijj}^{V,RR} - \frac{47}{9} L_{11ij}^{V1,LR} + \frac{35}{9} L_{11ij}^{V1,RR} + \frac{205}{486} L_{11ij}^{V8,LR} + \frac{835}{486} L_{11ij}^{V8,RR} \Big] \\
& + \alpha_s \alpha \left[ \frac{166}{243} L_{iii}^{V1,LR} + \frac{166}{243} L_{jjj}^{V1,LR} - \frac{721}{729} L_{iii}^{V8,LR} - \frac{721}{729} L_{jjj}^{V8,LR} - \frac{3038}{243} L_{ijj}^{V,RR} \right. \\
& + \frac{958}{243} L_{ijj}^{V,RR} - \frac{50}{243} L_{11ij}^{V,LR} - \frac{50}{243} L_{22ij}^{V,LR} - \frac{50}{243} L_{11ij}^{V,RR} - \frac{50}{243} L_{22ij}^{V,RR} - \frac{332}{243} L_{11ij}^{V1,LR} \\
& - \frac{332}{243} L_{11ij}^{V1,RR} + \frac{1331}{729} L_{11ij}^{V8,LR} - \frac{217}{729} L_{11ij}^{V8,RR} \Big] + \alpha^2 \left[ - \frac{356}{729} L_{iii}^{V1,LR} - \frac{356}{729} L_{jjj}^{V1,LR} \right. \\
& + \frac{470}{729} L_{ijj}^{V,RR} + \frac{632}{729} L_{ijj}^{V,RR} - \frac{644}{729} L_{11ij}^{V,LR} - \frac{644}{729} L_{22ij}^{V,LR} + \frac{868}{729} L_{11ij}^{V,RR} + \frac{868}{729} L_{22ij}^{V,RR} \\
& \left. - \frac{1772}{729} L_{11ij}^{V1,LR} + \frac{244}{729} L_{11ij}^{V1,RR} \right] ; \\
\dot{L}_{ed,11ij}^{V,LR} & = e^2 \left[ \frac{4}{3} L_{iii}^{V1,LR} + \frac{4}{3} L_{jjj}^{V1,LR} + \frac{32}{9} L_{ijj}^{V,RR} + \frac{32}{9} L_{ijj}^{V,RR} - \frac{8}{3} L_{11ij}^{V,LR} \right. \\
& + \frac{4}{3} L_{22ij}^{V,LR} + \frac{4}{3} L_{11ij}^{V,RR} + \frac{4}{3} L_{22ij}^{V,RR} - \frac{8}{3} L_{11ij}^{V1,LR} - \frac{8}{3} L_{11ij}^{V1,RR} \Big] + \alpha_s \alpha \left[ \frac{16}{3} L_{iii}^{V1,LR} \right. \\
& + \frac{16}{3} L_{jjj}^{V1,LR} - \frac{992}{243} L_{iii}^{V8,LR} - \frac{992}{243} L_{jjj}^{V8,LR} + \frac{1120}{81} L_{ijj}^{V,RR} + \frac{1120}{81} L_{ijj}^{V,RR} + 16 L_{11ij}^{V,LR} \\
& - \frac{32}{3} L_{11ij}^{V1,LR} - \frac{32}{3} L_{11ij}^{V1,RR} + \frac{1384}{243} L_{11ij}^{V8,LR} - \frac{56}{243} L_{11ij}^{V8,RR} \Big] + \alpha^2 \left[ \frac{1736}{243} L_{iii}^{V1,LR} \right. \\
& + \frac{1736}{243} L_{jjj}^{V1,LR} - \frac{752}{243} L_{ijj}^{V,RR} - \frac{752}{243} L_{ijj}^{V,RR} + \frac{15362}{243} L_{11ij}^{V,LR} + \frac{3752}{243} L_{22ij}^{V,LR} \\
& \left. - \frac{1000}{243} L_{11ij}^{V,RR} - \frac{1000}{243} L_{22ij}^{V,RR} - \frac{664}{243} L_{11ij}^{V1,LR} - \frac{7000}{243} L_{11ij}^{V1,RR} \right] ; \\
\dot{L}_{ed,22ij}^{V,LR} & = e^2 \left[ \frac{4}{3} L_{iii}^{V1,LR} + \frac{4}{3} L_{jjj}^{V1,LR} + \frac{32}{9} L_{ijj}^{V,RR} + \frac{32}{9} L_{ijj}^{V,RR} + \frac{4}{3} L_{11ij}^{V,LR} \right. \\
& - \frac{8}{3} L_{22ij}^{V,LR} + \frac{4}{3} L_{ed,11ij}^{V,RR} + \frac{4}{3} L_{ed,22ij}^{V,RR} - \frac{8}{3} L_{11ij}^{V1,LR} - \frac{8}{3} L_{11ij}^{V1,RR} \Big] + \alpha_s \alpha \left[ \frac{16}{3} L_{iii}^{V1,LR} \right. \\
& + \frac{16}{3} L_{jjj}^{V1,LR} - \frac{992}{243} L_{iii}^{V8,LR} - \frac{992}{243} L_{jjj}^{V8,LR} + \frac{1120}{81} L_{ijj}^{V,RR} + \frac{1120}{81} L_{ijj}^{V,RR} + 16 L_{22ij}^{V,LR} \\
& \left. - \frac{1000}{243} L_{ed,11ij}^{V,RR} - \frac{1000}{243} L_{ed,22ij}^{V,RR} - \frac{664}{243} L_{11ij}^{V1,LR} - \frac{7000}{243} L_{11ij}^{V1,RR} \right] ;
\end{aligned}$$

$$\begin{aligned}
& -\frac{32}{3}L_{11ij}^{V1,LR} - \frac{32}{3}L_{11ij}^{V1,RR} + \frac{1384}{243}L_{11ij}^{V8,LR} - \frac{56}{243}L_{11ij}^{V8,RR} \Big] + \alpha^2 \Big[ \frac{1736}{243}L_{iiij}^{V1,LR} \\
& + \frac{1736}{243}L_{jjij}^{V1,LR} - \frac{752}{243}L_{ijii}^{V,RR} - \frac{752}{243}L_{ijjj}^{V,RR} + \frac{3752}{243}L_{11ij}^{V,LR} + \frac{15362}{243}L_{22ij}^{V,LR} \\
& - \frac{1000}{243}L_{11ij}^{V,RR} - \frac{1000}{243}L_{22ij}^{V,RR} - \frac{664}{243}L_{11ij}^{V1,LR} - \frac{7000}{243}L_{11ij}^{V1,RR} \Big] ; \\
\dot{L}_{11ij}^{V1,LR} = & -\frac{8}{3}g_s^2 L_{11ij}^{V8,LR} + e^2 \Big[ -\frac{8}{9}L_{iiij}^{V1,LR} - \frac{8}{9}L_{jjij}^{V1,LR} - \frac{64}{27}L_{ijii}^{V,RR} - \frac{64}{27}L_{ijjj}^{V,RR} \\
& - \frac{8}{9}L_{11ij}^{V,LR} - \frac{8}{9}L_{22ij}^{V,LR} - \frac{8}{9}L_{11ij}^{V,RR} - \frac{8}{9}L_{22ij}^{V,RR} + \frac{40}{9}L_{11ij}^{V1,LR} + \frac{16}{9}L_{11ij}^{V1,RR} \Big] \\
& + \alpha_s^2 \Big[ 8L_{iiij}^{V1,LR} + 8L_{jjij}^{V1,LR} + \frac{44}{27}L_{iiij}^{V8,LR} + \frac{44}{27}L_{jjij}^{V8,LR} - \frac{232}{9}L_{ijii}^{V,RR} \\
& - \frac{232}{9}L_{ijjj}^{V,RR} - \frac{4}{3}L_{11ij}^{V1,LR} - 8L_{11ij}^{V1,RR} - \frac{232}{3}L_{11ij}^{V8,LR} + \frac{44}{27}L_{11ij}^{V8,RR} \Big] + \alpha_s \alpha \Big[ -\frac{32}{9}L_{iiij}^{V1,LR} \\
& - \frac{32}{9}L_{jjij}^{V1,LR} + \frac{1984}{729}L_{iiij}^{V8,LR} + \frac{1984}{729}L_{jjij}^{V8,LR} - \frac{2240}{243}L_{ijii}^{V,RR} - \frac{2240}{243}L_{ijjj}^{V,RR} \\
& - \frac{128}{9}L_{11ij}^{V1,LR} + \frac{64}{9}L_{11ij}^{V1,RR} + \frac{3496}{729}L_{11ij}^{V8,LR} + \frac{112}{729}L_{11ij}^{V8,RR} \Big] + \alpha^2 \Big[ \frac{3728}{729}L_{iiij}^{V1,LR} \\
& + \frac{3728}{729}L_{jjij}^{V1,LR} + \frac{784}{729}L_{ijii}^{V,RR} + \frac{784}{729}L_{ijjj}^{V,RR} + \frac{6176}{729}L_{11ij}^{V,LR} + \frac{6176}{729}L_{22ij}^{V,LR} \\
& - \frac{3760}{729}L_{11ij}^{V,RR} - \frac{3760}{729}L_{22ij}^{V,RR} - \frac{17392}{729}L_{11ij}^{V1,LR} - \frac{6880}{729}L_{11ij}^{V1,RR} \Big] ; \\
\dot{L}_{11ij}^{V8,LR} = & g_s^2 \Big[ \frac{2}{3}L_{iiij}^{V8,LR} + \frac{2}{3}L_{jjij}^{V8,LR} + \frac{8}{3}L_{ijii}^{V,RR} + \frac{8}{3}L_{ijjj}^{V,RR} - 12L_{11ij}^{V1,LR} \\
& - \frac{40}{3}L_{11ij}^{V8,LR} + \frac{2}{3}L_{11ij}^{V8,RR} \Big] + \frac{8}{3}e^2 L_{11ij}^{V8,LR} + \alpha_s^2 \Big[ -\frac{22}{3}L_{iiij}^{V1,LR} - \frac{22}{3}L_{jjij}^{V1,LR} \\
& + \frac{799}{81}L_{iiij}^{V8,LR} + \frac{799}{81}L_{jjij}^{V8,LR} + \frac{1210}{27}L_{ijii}^{V,RR} + \frac{1210}{27}L_{ijjj}^{V,RR} - \frac{440}{3}L_{11ij}^{V1,LR} - \frac{2}{3}L_{11ij}^{V1,RR} \\
& - \frac{26005}{162}L_{11ij}^{V8,LR} + \frac{619}{81}L_{11ij}^{V8,RR} \Big] + \alpha_s \alpha \Big[ -\frac{928}{81}L_{iiij}^{V1,LR} - \frac{928}{81}L_{jjij}^{V1,LR} - \frac{44}{9}L_{iiij}^{V8,LR}
\end{aligned}$$

$$\begin{aligned}
& -\frac{44}{9}L_{jjij}^{V8,LR} - \frac{2192}{81}L_{ijii}^{V,RR} - \frac{2192}{81}L_{ijjj}^{V,RR} - \frac{928}{81}L_{11ij}^{V,LR} - \frac{928}{81}L_{22ij}^{V,LR} - \frac{928}{81}L_{11ij}^{V,RR} \\
& - \frac{928}{81}L_{22ij}^{V,RR} + \frac{4988}{81}L_{11ij}^{V1,LR} + \frac{1856}{81}L_{11ij}^{V1,RR} + 27L_{11ij}^{V8,LR} - \frac{160}{27}L_{11ij}^{V8,RR} \Big] \\
& - \frac{880}{27}\alpha^2 L_{11ij}^{V8,LR} ; \\
\dot{L}_{jjij}^{V1,LR} = & -\frac{8}{3}g_s^2 L_{jjij}^{V8,LR} + e^2 \Big[ \frac{4}{9}L_{iiij}^{V1,LR} - \frac{8}{9}L_{jjij}^{V1,LR} + \frac{32}{27}L_{ijii}^{V,RR} + \frac{32}{27}L_{ijjj}^{V,RR} \\
& + \frac{4}{9}L_{11ij}^{V,LR} + \frac{4}{9}L_{22ij}^{V,LR} + \frac{4}{9}L_{11ij}^{V,RR} + \frac{4}{9}L_{22ij}^{V,RR} - \frac{8}{9}L_{11ij}^{V1,LR} - \frac{8}{9}L_{11ij}^{V1,RR} \Big] \\
& + \alpha_s^2 \Big[ 8L_{iiij}^{V1,LR} - \frac{4}{3}L_{jjij}^{V1,LR} + \frac{44}{27}L_{iiij}^{V8,LR} - \frac{232}{3}L_{jjij}^{V8,LR} - \frac{232}{9}L_{ijii}^{V,RR} \\
& - \frac{232}{9}L_{ijjj}^{V,RR} + 8L_{11ij}^{V1,LR} - 8L_{11ij}^{V1,RR} + \frac{44}{27}L_{11ij}^{V8,LR} + \frac{44}{27}L_{11ij}^{V8,RR} \Big] + \alpha_s \alpha \Big[ \frac{16}{9}L_{iiij}^{V1,LR} \\
& + \frac{112}{9}L_{jjij}^{V1,LR} - \frac{992}{729}L_{iiij}^{V8,LR} - \frac{1208}{729}L_{jjij}^{V8,LR} + \frac{1120}{243}L_{ijii}^{V,RR} + \frac{1120}{243}L_{ijjj}^{V,RR} \\
& - \frac{32}{9}L_{11ij}^{V1,LR} - \frac{32}{9}L_{11ij}^{V1,RR} + \frac{1384}{729}L_{11ij}^{V8,LR} - \frac{56}{729}L_{11ij}^{V8,RR} \Big] + \alpha^2 \Big[ \frac{296}{729}L_{iiij}^{V1,LR} \\
& + \frac{10070}{729}L_{jjij}^{V1,LR} - \frac{608}{729}L_{iiij}^{V,RR} - \frac{608}{729}L_{ijjj}^{V,RR} + \frac{1016}{729}L_{11ij}^{V,LR} + \frac{1016}{729}L_{22ij}^{V,LR} \\
& + \frac{152}{729}L_{11ij}^{V,RR} + \frac{152}{729}L_{22ij}^{V,RR} - \frac{1672}{729}L_{11ij}^{V1,LR} - \frac{2824}{729}L_{11ij}^{V1,RR} \Big] ; \\
\dot{L}_{jjij}^{V8,LR} = & g_s^2 \Big[ -12L_{jjij}^{V1,LR} + \frac{2}{3}L_{iiij}^{V8,LR} - \frac{40}{3}L_{jjij}^{V8,LR} + \frac{8}{3}L_{ijii}^{V,RR} + \frac{8}{3}L_{ijjj}^{V,RR} \\
& + \frac{2}{3}L_{11ij}^{V8,LR} + \frac{2}{3}L_{11ij}^{V8,RR} \Big] - \frac{4}{3}e^2 L_{jjij}^{V8,LR} + \alpha_s^2 \Big[ -\frac{22}{3}L_{iiij}^{V1,LR} - \frac{440}{3}L_{jjij}^{V1,LR} \\
& + \frac{799}{81}L_{iiij}^{V8,LR} - \frac{26005}{162}L_{jjij}^{V8,LR} + \frac{1210}{27}L_{ijii}^{V,RR} + \frac{1210}{27}L_{ijjj}^{V,RR} - \frac{22}{3}L_{11ij}^{V1,LR} \\
& - \frac{2}{3}L_{11ij}^{V1,RR} + \frac{799}{81}L_{11ij}^{V8,LR} + \frac{619}{81}L_{11ij}^{V8,RR} \Big] + \alpha_s \alpha \Big[ \frac{260}{81}L_{iiij}^{V1,LR} + \frac{152}{81}L_{jjij}^{V1,LR}
\end{aligned}$$

$$\begin{aligned}
& + \frac{14}{9} L_{\ddot{ii}j}^{V8,LR} - \frac{4}{3} L_{\ddot{jj}j}^{V8,LR} + \frac{292}{81} L_{\ddot{ij}i}^{V,RR} + \frac{292}{81} L_{\ddot{ij}j}^{V,RR} + \frac{260}{81} L_{\ddot{11}ij}^{V,LR} + \frac{260}{81} L_{\ddot{22}ij}^{V,LR} \\
& + \frac{260}{81} L_{\ddot{11}ij}^{V,RR} + \frac{260}{81} L_{\ddot{22}ij}^{V,RR} - \frac{520}{81} L_{\ddot{11}ij}^{V1,LR} - \frac{520}{81} L_{\ddot{11}ij}^{V1,RR} + \frac{2}{3} L_{\ddot{11}ij}^{V8,LR} + \frac{122}{27} L_{\ddot{11}ij}^{V8,RR} \Big] \\
& + \frac{362}{27} \alpha^2 L_{\ddot{jj}ij}^{V8,LR} ; \\
\dot{L}_{\ddot{ii}j}^{V1,LR} = & - \frac{8}{3} g_s^2 L_{\ddot{iii}j}^{V8,LR} + e^2 \Big[ - \frac{8}{9} L_{\ddot{iii}j}^{V1,LR} + \frac{4}{9} L_{\ddot{jj}ij}^{V1,LR} + \frac{32}{27} L_{\ddot{ij}ii}^{V,RR} + \frac{32}{27} L_{\ddot{ij}jj}^{V,RR} \\
& + \frac{4}{9} L_{\ddot{11}ij}^{V,LR} + \frac{4}{9} L_{\ddot{22}ij}^{V,LR} + \frac{4}{9} L_{\ddot{11}ij}^{V,RR} + \frac{4}{9} L_{\ddot{22}ij}^{V,RR} - \frac{8}{9} L_{\ddot{11}ij}^{V1,LR} - \frac{8}{9} L_{\ddot{11}ij}^{V1,RR} \Big] \\
& + \alpha_s^2 \Big[ - \frac{4}{3} L_{\ddot{iii}j}^{V1,LR} + 8 L_{\ddot{jj}ij}^{V1,LR} - \frac{232}{3} L_{\ddot{iii}j}^{V8,LR} + \frac{44}{27} L_{\ddot{jj}ij}^{V8,LR} - \frac{232}{9} L_{\ddot{ij}ii}^{V,RR} \\
& - \frac{232}{9} L_{\ddot{ij}jj}^{V,RR} + 8 L_{\ddot{ud}11ij}^{V1,LR} - 8 L_{\ddot{ud}11ij}^{V1,RR} + \frac{44}{27} L_{\ddot{ud}11ij}^{V8,LR} + \frac{44}{27} L_{\ddot{ud}11ij}^{V8,RR} \Big] + \alpha_s \alpha \Big[ \frac{112}{9} L_{\ddot{iii}j}^{V1,LR} \\
& + \frac{16}{9} L_{\ddot{jj}ij}^{V1,LR} - \frac{1208}{729} L_{\ddot{iii}j}^{V8,LR} - \frac{992}{729} L_{\ddot{jj}ij}^{V8,LR} + \frac{1120}{243} L_{\ddot{ij}ii}^{V,RR} + \frac{1120}{243} L_{\ddot{ij}jj}^{V,RR} \\
& - \frac{32}{9} L_{\ddot{11}ij}^{V1,LR} - \frac{32}{9} L_{\ddot{11}ij}^{V1,RR} + \frac{1384}{729} L_{\ddot{ud}11ij}^{V8,LR} - \frac{56}{729} L_{\ddot{ud}11ij}^{V8,RR} \Big] + \alpha^2 \Big[ \frac{10070}{729} L_{\ddot{iii}j}^{V1,LR} \\
& + \frac{296}{729} L_{\ddot{jj}ij}^{V1,LR} - \frac{608}{729} L_{\ddot{ij}ii}^{V,RR} - \frac{608}{729} L_{\ddot{ij}jj}^{V,RR} + \frac{1016}{729} L_{\ddot{11}ij}^{V,LR} + \frac{1016}{729} L_{\ddot{22}ij}^{V,LR} \\
& + \frac{152}{729} L_{\ddot{11}ij}^{V,RR} + \frac{152}{729} L_{\ddot{22}ij}^{V,RR} - \frac{1672}{729} L_{\ddot{11}ij}^{V1,LR} - \frac{2824}{729} L_{\ddot{11}ij}^{V1,RR} \Big] ; \\
\dot{L}_{\ddot{ii}j}^{V8,LR} = & g_s^2 \Big[ - 12 L_{\ddot{iii}j}^{V1,LR} - \frac{40}{3} L_{\ddot{iii}j}^{V8,LR} + \frac{2}{3} L_{\ddot{jj}ij}^{V8,LR} + \frac{8}{3} L_{\ddot{ij}ii}^{V,RR} + \frac{8}{3} L_{\ddot{ij}jj}^{V,RR} \\
& + \frac{2}{3} L_{\ddot{11}ij}^{V8,LR} + \frac{2}{3} L_{\ddot{11}ij}^{V8,RR} \Big] - \frac{4}{3} e^2 L_{\ddot{iii}j}^{V8,LR} + \alpha_s^2 \Big[ - \frac{440}{3} L_{\ddot{iii}j}^{V1,LR} - \frac{22}{3} L_{\ddot{jj}ij}^{V1,LR} \\
& - \frac{26005}{162} L_{\ddot{iii}j}^{V8,LR} + \frac{799}{81} L_{\ddot{jj}ij}^{V8,LR} + \frac{1210}{27} L_{\ddot{ij}ii}^{V,RR} + \frac{1210}{27} L_{\ddot{ij}jj}^{V,RR} - \frac{22}{3} L_{\ddot{11}ij}^{V1,LR} \\
& - \frac{2}{3} L_{\ddot{11}ij}^{V1,RR} + \frac{799}{81} L_{\ddot{11}ij}^{V8,LR} + \frac{619}{81} L_{\ddot{11}ij}^{V8,RR} \Big] + \alpha_s \alpha \Big[ \frac{152}{81} L_{\ddot{iii}j}^{V1,LR} + \frac{260}{81} L_{\ddot{jj}ij}^{V1,LR}
\end{aligned}$$

$$\begin{aligned}
& -\frac{4}{3}L_{\substack{dd \\ iiij}}^{V8,LR} + \frac{14}{9}L_{\substack{dd \\ jjij}}^{V8,LR} + \frac{292}{81}L_{\substack{dd \\ ijii}}^{V,RR} + \frac{292}{81}L_{\substack{dd \\ ijjj}}^{V,RR} + \frac{260}{81}L_{\substack{ed \\ 11ij}}^{V,LR} + \frac{260}{81}L_{\substack{ed \\ 22ij}}^{V,LR} \\
& + \frac{260}{81}L_{\substack{ed \\ 11ij}}^{V,RR} + \frac{260}{81}L_{\substack{ed \\ 22ij}}^{V,RR} - \frac{520}{81}L_{\substack{ud \\ 11ij}}^{V1,LR} - \frac{520}{81}L_{\substack{ud \\ 11ij}}^{V1,RR} + \frac{2}{3}L_{\substack{ud \\ 11ij}}^{V8,LR} + \frac{122}{27}L_{\substack{ud \\ 11ij}}^{V8,RR} \Big] \\
& + \frac{362}{27}\alpha^2 L_{\substack{dd \\ iiij}}^{V8,LR} ;
\end{aligned}$$

$$\dot{L}_{\substack{\nu d \\ 11ij}}^{V,LL} = 0 ;$$

$$\dot{L}_{\substack{\nu d \\ 22ij}}^{V,LL} = 0 ;$$

$$\dot{L}_{\substack{\nu d \\ 33ij}}^{V,LL} = 0 ;$$

$$\dot{L}_{\substack{\nu d \\ 11ij}}^{V,LR} = 0 ;$$

$$\dot{L}_{\substack{\nu d \\ 22ij}}^{V,LR} = 0 ;$$

$$\dot{L}_{\substack{\nu d \\ 33ij}}^{V,LR} = 0 ;$$

$$\begin{aligned}
\dot{L}_{\substack{\nu d \\ 11ij}}^{S,LR} &= -8g_s^2 L_{\substack{\nu d \\ 11ij}}^{S,LR} - \frac{2}{3}e^2 L_{\substack{\nu d \\ 11ij}}^{S,LR} - \frac{1052}{9}\alpha_s^2 L_{\substack{\nu d \\ 11ij}}^{S,LR} - \frac{8}{9}\alpha_s \alpha L_{\substack{\nu d \\ 11ij}}^{S,LR} \\
&+ \frac{79}{27}\alpha^2 L_{\substack{\nu d \\ 11ij}}^{S,LR} ;
\end{aligned}$$

$$\begin{aligned}
\dot{L}_{\substack{\nu d \\ 22ij}}^{S,LR} &= -8g_s^2 L_{\substack{\nu d \\ 22ij}}^{S,LR} - \frac{2}{3}e^2 L_{\substack{\nu d \\ 22ij}}^{S,LR} - \frac{1052}{9}\alpha_s^2 L_{\substack{\nu d \\ 22ij}}^{S,LR} - \frac{8}{9}\alpha_s \alpha L_{\substack{\nu d \\ 22ij}}^{S,LR} \\
&+ \frac{79}{27}\alpha^2 L_{\substack{\nu d \\ 22ij}}^{S,LR} ;
\end{aligned}$$

$$\begin{aligned}
\dot{L}_{\substack{\nu d \\ 33ij}}^{S,LR} &= -8g_s^2 L_{\substack{\nu d \\ 33ij}}^{S,LR} - \frac{2}{3}e^2 L_{\substack{\nu d \\ 33ij}}^{S,LR} - \frac{1052}{9}\alpha_s^2 L_{\substack{\nu d \\ 33ij}}^{S,LR} - \frac{8}{9}\alpha_s \alpha L_{\substack{\nu d \\ 33ij}}^{S,LR} \\
&+ \frac{79}{27}\alpha^2 L_{\substack{\nu d \\ 33ij}}^{S,LR} ;
\end{aligned}$$

$$\begin{aligned}
\dot{L}_{\substack{\nu d \\ 11ij}}^{S,LL} &= -8g_s^2 L_{\substack{\nu d \\ 11ij}}^{S,LL} - \frac{2}{3}e^2 L_{\substack{\nu d \\ 11ij}}^{S,LL} - \frac{1052}{9}\alpha_s^2 L_{\substack{\nu d \\ 11ij}}^{S,LL} - \frac{8}{9}\alpha_s \alpha L_{\substack{\nu d \\ 11ij}}^{S,LL} \\
&+ \frac{79}{27}\alpha^2 L_{\substack{\nu d \\ 11ij}}^{S,LL} ;
\end{aligned}$$

$$\dot{L}_{\substack{\nu d \\ 11ij}}^{T,LL} = \frac{8}{3}g_s^2 L_{\substack{\nu d \\ 11ij}}^{T,LL} + \frac{2}{9}e^2 L_{\substack{\nu d \\ 11ij}}^{T,LL} + \frac{1756}{27}\alpha_s^2 L_{\substack{\nu d \\ 11ij}}^{T,LL} - \frac{152}{27}\alpha_s \alpha L_{\substack{\nu d \\ 11ij}}^{T,LL}$$

$$\begin{aligned}
& -\frac{227}{81}\alpha^2 L_{11ij}^{T,LL} ; \\
\dot{L}_{22ij}^{S,LL} &= -8g_s^2 L_{22ij}^{S,LL} - \frac{2}{3}e^2 L_{22ij}^{S,LL} - \frac{1052}{9}\alpha_s^2 L_{22ij}^{S,LL} - \frac{8}{9}\alpha_s\alpha L_{22ij}^{S,LL} \\
& + \frac{79}{27}\alpha^2 L_{22ij}^{S,LL} ; \\
\dot{L}_{22ij}^{T,LL} &= \frac{8}{3}g_s^2 L_{22ij}^{T,LL} + \frac{2}{9}e^2 L_{22ij}^{T,LL} + \frac{1756}{27}\alpha_s^2 L_{22ij}^{T,LL} - \frac{152}{27}\alpha_s\alpha L_{22ij}^{T,LL} \\
& - \frac{227}{81}\alpha^2 L_{22ij}^{T,LL} ; \\
\dot{L}_{33ij}^{S,LL} &= -8g_s^2 L_{33ij}^{S,LL} - \frac{2}{3}e^2 L_{33ij}^{S,LL} - \frac{1052}{9}\alpha_s^2 L_{33ij}^{S,LL} - \frac{8}{9}\alpha_s\alpha L_{33ij}^{S,LL} \\
& + \frac{79}{27}\alpha^2 L_{33ij}^{S,LL} ; \\
\dot{L}_{33ij}^{T,LL} &= \frac{8}{3}g_s^2 L_{33ij}^{T,LL} + \frac{2}{9}e^2 L_{33ij}^{T,LL} + \frac{1756}{27}\alpha_s^2 L_{33ij}^{T,LL} - \frac{152}{27}\alpha_s\alpha L_{33ij}^{T,LL} \\
& - \frac{227}{81}\alpha^2 L_{33ij}^{T,LL} ;
\end{aligned}$$

### 3.6 $\Delta F = 1^{\bar{f}f}$ : $e$ -type ( $\bar{e}_i e_j \bar{f}_k f_k$ )

$$\begin{aligned}
\dot{L}_{ij11}^{V,LL} &= e^2 \left[ \frac{40}{9}L_{ij11}^{V,LL} + \frac{4}{9}L_{ij22}^{V,LL} + \frac{4}{9}L_{ij11}^{V,LR} + \frac{4}{9}L_{ij22}^{V,LR} + \frac{16}{9}L_{ijii}^{V,LL} \right. \\
& + \frac{16}{9}L_{ijjj}^{V,LL} + \frac{4}{9}L_{ijii}^{V,LR} + \frac{4}{9}L_{ijjj}^{V,LR} - \frac{8}{9}L_{ij11}^{V,LL} - \frac{8}{9}L_{ij11}^{V,LR} \left. \right] + \alpha_s^2 \left[ 8L_{ij11}^{V,LL} \right. \\
& + 8L_{ij22}^{V,LL} - 8L_{ij11}^{V,LR} - 8L_{ij22}^{V,LR} + 8L_{ij11}^{V,LL} - 8L_{ij11}^{V,LR} \left. \right] + \alpha_s\alpha \left[ -\frac{128}{9}L_{ij11}^{V,LL} \right. \\
& + \frac{16}{9}L_{ij22}^{V,LL} + \frac{16}{9}L_{ij11}^{V,LR} + \frac{16}{9}L_{ij22}^{V,LR} - \frac{32}{9}L_{ij11}^{V,LL} - \frac{32}{9}L_{ij11}^{V,LR} \left. \right] + \alpha^2 \left[ -\frac{3614}{243}L_{ij11}^{V,LL} \right. \\
& - \frac{104}{243}L_{ij22}^{V,LL} - \frac{200}{243}L_{ij11}^{V,LR} - \frac{200}{243}L_{ij22}^{V,LR} + \frac{32}{81}L_{ijii}^{V,LL} + \frac{32}{81}L_{ijjj}^{V,LL} - \frac{520}{81}L_{ijii}^{V,LR} \\
& \left. - \frac{520}{81}L_{ijjj}^{V,LR} - \frac{1016}{243}L_{ij11}^{V,LL} - \frac{1400}{243}L_{ij11}^{V,LR} \right] ;
\end{aligned}$$

$$\begin{aligned}
\dot{L}_{ij22}^{V,LL} &= e^2 \left[ \frac{4}{9} L_{ij11}^{V,LL} + \frac{40}{9} L_{ij22}^{V,LL} + \frac{4}{9} L_{ij11}^{V,LR} + \frac{4}{9} L_{ij22}^{V,LR} + \frac{16}{9} L_{ijii}^{V,LL} \right. \\
&\quad + \frac{16}{9} L_{ijjj}^{V,LL} + \frac{4}{9} L_{ijii}^{V,LR} + \frac{4}{9} L_{ijjj}^{V,LR} - \frac{8}{9} L_{ij11}^{V,LL} - \frac{8}{9} L_{ij11}^{V,LR} \left. \right] + \alpha_s^2 \left[ 8 L_{ij11}^{V,LL} \right. \\
&\quad + 8 L_{ij22}^{V,LL} - 8 L_{ij11}^{V,LR} - 8 L_{ij22}^{V,LR} + 8 L_{ij11}^{V,LL} - 8 L_{ij11}^{V,LR} \left. \right] + \alpha_s \alpha \left[ \frac{16}{9} L_{ij11}^{V,LL} \right. \\
&\quad - \frac{128}{9} L_{ij22}^{V,LL} + \frac{16}{9} L_{ij11}^{V,LR} + \frac{16}{9} L_{ij22}^{V,LR} - \frac{32}{9} L_{ij11}^{V,LL} - \frac{32}{9} L_{ij11}^{V,LR} \left. \right] + \alpha^2 \left[ -\frac{104}{243} L_{ij11}^{V,LL} \right. \\
&\quad - \frac{3614}{243} L_{ij22}^{V,LL} - \frac{200}{243} L_{ij11}^{V,LR} - \frac{200}{243} L_{ij22}^{V,LR} + \frac{32}{81} L_{ijii}^{V,LL} + \frac{32}{81} L_{ijjj}^{V,LL} - \frac{520}{81} L_{ijii}^{V,LR} \\
&\quad \left. - \frac{520}{81} L_{ijjj}^{V,LR} - \frac{1016}{243} L_{ij11}^{V,LL} - \frac{1400}{243} L_{ij11}^{V,LR} \right] ;
\end{aligned}$$

$$\begin{aligned}
\dot{L}_{ij11}^{V,LL} &= e^2 \left[ -\frac{8}{9} L_{ij11}^{V,LL} - \frac{8}{9} L_{ij22}^{V,LL} - \frac{8}{9} L_{ij11}^{V,LR} - \frac{8}{9} L_{ij22}^{V,LR} - \frac{32}{9} L_{ijii}^{V,LL} \right. \\
&\quad - \frac{32}{9} L_{ijjj}^{V,LL} - \frac{8}{9} L_{ijii}^{V,LR} - \frac{8}{9} L_{ijjj}^{V,LR} - \frac{56}{9} L_{ij11}^{V,LL} + \frac{16}{9} L_{ij11}^{V,LR} \left. \right] + \alpha_s^2 \left[ 8 L_{ij11}^{V,LL} \right. \\
&\quad + 8 L_{ij22}^{V,LL} - 8 L_{ij11}^{V,LR} - 8 L_{ij22}^{V,LR} + 8 L_{ij11}^{V,LL} - 8 L_{ij11}^{V,LR} \left. \right] + \alpha_s \alpha \left[ -\frac{32}{9} L_{ij11}^{V,LL} \right. \\
&\quad - \frac{32}{9} L_{ij22}^{V,LL} - \frac{32}{9} L_{ij11}^{V,LR} - \frac{32}{9} L_{ij22}^{V,LR} + \frac{352}{9} L_{ij11}^{V,LL} + \frac{64}{9} L_{ij11}^{V,LR} \left. \right] + \alpha^2 \left[ \frac{2512}{243} L_{ij11}^{V,LL} \right. \\
&\quad + \frac{2512}{243} L_{ij22}^{V,LL} + \frac{1408}{243} L_{ij11}^{V,LR} + \frac{1408}{243} L_{ij22}^{V,LR} + \frac{3680}{81} L_{ijii}^{V,LL} + \frac{3680}{81} L_{ijjj}^{V,LL} \\
&\quad + \frac{464}{81} L_{ijii}^{V,LR} + \frac{464}{81} L_{ijjj}^{V,LR} + \frac{3472}{243} L_{ij11}^{V,LL} - \frac{3104}{243} L_{ij11}^{V,LR} \left. \right] ;
\end{aligned}$$

$$\begin{aligned}
\dot{L}_{ijjj}^{V,LL} &= e^2 \left[ \frac{2}{3} L_{ij11}^{V,LL} + \frac{2}{3} L_{ij22}^{V,LL} + \frac{2}{3} L_{ij11}^{V,LR} + \frac{2}{3} L_{ij22}^{V,LR} + \frac{8}{3} L_{ijii}^{V,LL} \right. \\
&\quad + \frac{44}{3} L_{ijjj}^{V,LL} + \frac{2}{3} L_{ijii}^{V,LR} + \frac{2}{3} L_{ijjj}^{V,LR} - \frac{4}{3} L_{ij11}^{V,LL} - \frac{4}{3} L_{ij11}^{V,LR} \left. \right] + \alpha_s \alpha \left[ \frac{8}{3} L_{ij11}^{V,LL} \right. \\
&\quad + \frac{8}{3} L_{ij22}^{V,LL} + \frac{8}{3} L_{ij11}^{V,LR} + \frac{8}{3} L_{ij22}^{V,LR} - \frac{16}{3} L_{ij11}^{V,LL} - \frac{16}{3} L_{ij11}^{V,LR} \left. \right] + \alpha^2 \left[ \frac{332}{81} L_{ij11}^{V,LL} \right.
\end{aligned}$$

$$\begin{aligned}
& + \frac{332}{81} L_{ed\,ij22}^{V,LL} + \frac{68}{81} L_{ed\,ij11}^{V,LR} + \frac{68}{81} L_{ed\,ij22}^{V,LR} + \frac{640}{27} L_{ee\,ijii}^{V,LL} - \frac{2150}{27} L_{ee\,ijjj}^{V,LL} - \frac{356}{27} L_{ee\,ijii}^{V,LR} \\
& - \frac{356}{27} L_{ee\,ijjj}^{V,LR} - \frac{628}{81} L_{eu\,ij11}^{V,LL} - \frac{1684}{81} L_{eu\,ij11}^{V,LR} \Big] ; \\
\dot{L}_{ee\,ijii}^{V,LL} & = e^2 \left[ \frac{2}{3} L_{ed\,ij11}^{V,LL} + \frac{2}{3} L_{ed\,ij22}^{V,LL} + \frac{2}{3} L_{ed\,ij11}^{V,LR} + \frac{2}{3} L_{ed\,ij22}^{V,LR} + \frac{44}{3} L_{ee\,ijii}^{V,LL} \right. \\
& + \frac{8}{3} L_{ee\,ijjj}^{V,LL} + \frac{2}{3} L_{ee\,ijii}^{V,LR} + \frac{2}{3} L_{ee\,ijjj}^{V,LR} - \frac{4}{3} L_{eu\,ij11}^{V,LL} - \frac{4}{3} L_{eu\,ij11}^{V,LR} \Big] + \alpha_s \alpha \left[ \frac{8}{3} L_{ed\,ij11}^{V,LL} \right. \\
& + \frac{8}{3} L_{ed\,ij22}^{V,LL} + \frac{8}{3} L_{ed\,ij11}^{V,LR} + \frac{8}{3} L_{ed\,ij22}^{V,LR} - \frac{16}{3} L_{eu\,ij11}^{V,LL} - \frac{16}{3} L_{eu\,ij11}^{V,LR} \Big] + \alpha^2 \left[ \frac{332}{81} L_{ed\,ij11}^{V,LL} \right. \\
& + \frac{332}{81} L_{ed\,ij22}^{V,LL} + \frac{68}{81} L_{ed\,ij11}^{V,LR} + \frac{68}{81} L_{ed\,ij22}^{V,LR} - \frac{2150}{27} L_{ee\,ijii}^{V,LL} + \frac{640}{27} L_{ee\,ijjj}^{V,LL} - \frac{356}{27} L_{ee\,ijii}^{V,LR} \\
& - \frac{356}{27} L_{ee\,ijjj}^{V,LR} - \frac{628}{81} L_{eu\,ij11}^{V,LL} - \frac{1684}{81} L_{eu\,ij11}^{V,LR} \Big] ; \\
\dot{L}_{ed\,ij11}^{V,LR} & = e^2 \left[ \frac{4}{9} L_{ed\,ij11}^{V,LL} + \frac{4}{9} L_{ed\,ij22}^{V,LL} - \frac{32}{9} L_{ed\,ij11}^{V,LR} + \frac{4}{9} L_{ed\,ij22}^{V,LR} + \frac{16}{9} L_{ee\,ijii}^{V,LL} \right. \\
& + \frac{16}{9} L_{ee\,ijjj}^{V,LL} + \frac{4}{9} L_{ee\,ijii}^{V,LR} + \frac{4}{9} L_{ee\,ijjj}^{V,LR} - \frac{8}{9} L_{eu\,ij11}^{V,LL} - \frac{8}{9} L_{eu\,ij11}^{V,LR} \Big] + \alpha_s^2 \left[ -8 L_{ed\,ij11}^{V,LL} \right. \\
& - 8 L_{ed\,ij22}^{V,LL} + 8 L_{ed\,ij11}^{V,LR} + 8 L_{ed\,ij22}^{V,LR} - 8 L_{eu\,ij11}^{V,LL} + 8 L_{eu\,ij11}^{V,LR} \Big] + \alpha_s \alpha \left[ \frac{16}{9} L_{ed\,ij11}^{V,LL} \right. \\
& + \frac{16}{9} L_{ed\,ij22}^{V,LL} + \frac{160}{9} L_{ed\,ij11}^{V,LR} + \frac{16}{9} L_{ed\,ij22}^{V,LR} - \frac{32}{9} L_{eu\,ij11}^{V,LL} - \frac{32}{9} L_{eu\,ij11}^{V,LR} \Big] + \alpha^2 \left[ -\frac{440}{243} L_{ed\,ij11}^{V,LL} \right. \\
& - \frac{440}{243} L_{ed\,ij22}^{V,LL} + \frac{11506}{243} L_{ed\,ij11}^{V,LR} - \frac{104}{243} L_{ed\,ij22}^{V,LR} - \frac{640}{81} L_{ee\,ijii}^{V,LL} - \frac{640}{81} L_{ee\,ijjj}^{V,LL} - \frac{184}{81} L_{ee\,ijii}^{V,LR} \\
& - \frac{184}{81} L_{ee\,ijjj}^{V,LR} - \frac{1640}{243} L_{eu\,ij11}^{V,LL} - \frac{296}{243} L_{eu\,ij11}^{V,LR} \Big] ; \\
\dot{L}_{ed\,ij22}^{V,LR} & = e^2 \left[ \frac{4}{9} L_{ed\,ij11}^{V,LL} + \frac{4}{9} L_{ed\,ij22}^{V,LL} + \frac{4}{9} L_{ed\,ij11}^{V,LR} - \frac{32}{9} L_{ed\,ij22}^{V,LR} + \frac{16}{9} L_{ee\,ijii}^{V,LL} \right. \\
& + \frac{16}{9} L_{ee\,ijjj}^{V,LL} + \frac{4}{9} L_{ee\,ijii}^{V,LR} + \frac{4}{9} L_{ee\,ijjj}^{V,LR} - \frac{8}{9} L_{eu\,ij11}^{V,LL} - \frac{8}{9} L_{eu\,ij11}^{V,LR} \Big] + \alpha_s^2 \left[ -8 L_{ed\,ij11}^{V,LL} \right.
\end{aligned}$$



$$\begin{aligned}
& -8L_{ed\,ij22}^{V,LL} + 8L_{ed\,ij11}^{V,LR} + 8L_{ed\,ij22}^{V,LR} - 8L_{eu\,ij11}^{V,LL} + 8L_{eu\,ij11}^{V,LR} \Big] + \alpha_s \alpha \Big[ \frac{16}{9} L_{ed\,ij11}^{V,LL} \\
& + \frac{16}{9} L_{ed\,ij22}^{V,LL} + \frac{16}{9} L_{ed\,ij11}^{V,LR} + \frac{160}{9} L_{ed\,ij22}^{V,LR} - \frac{32}{9} L_{eu\,ij11}^{V,LL} - \frac{32}{9} L_{eu\,ij11}^{V,LR} \Big] + \alpha^2 \Big[ -\frac{440}{243} L_{ed\,ij11}^{V,LL} \\
& - \frac{440}{243} L_{ed\,ij22}^{V,LL} - \frac{104}{243} L_{ed\,ij11}^{V,LR} + \frac{11506}{243} L_{ed\,ij22}^{V,LR} - \frac{640}{81} L_{ee\,ijii}^{V,LL} - \frac{640}{81} L_{ee\,ijjj}^{V,LL} - \frac{184}{81} L_{ee\,ijii}^{V,LR} \\
& - \frac{184}{81} L_{ee\,ijjj}^{V,LR} - \frac{1640}{243} L_{eu\,ij11}^{V,LL} - \frac{296}{243} L_{eu\,ij11}^{V,LR} \Big] ; \\
\dot{L}_{eu\,ij11}^{V,LR} &= e^2 \Big[ -\frac{8}{9} L_{ed\,ij11}^{V,LL} - \frac{8}{9} L_{ed\,ij22}^{V,LL} - \frac{8}{9} L_{ed\,ij11}^{V,LR} - \frac{8}{9} L_{ed\,ij22}^{V,LR} - \frac{32}{9} L_{ee\,ijii}^{V,LL} \\
& - \frac{32}{9} L_{ee\,ijjj}^{V,LL} - \frac{8}{9} L_{ee\,ijii}^{V,LR} - \frac{8}{9} L_{ee\,ijjj}^{V,LR} + \frac{16}{9} L_{eu\,ij11}^{V,LL} + \frac{88}{9} L_{eu\,ij11}^{V,LR} \Big] + \alpha_s^2 \Big[ -8L_{ed\,ij11}^{V,LL} \\
& - 8L_{ed\,ij22}^{V,LL} + 8L_{ed\,ij11}^{V,LR} + 8L_{ed\,ij22}^{V,LR} - 8L_{eu\,ij11}^{V,LL} + 8L_{eu\,ij11}^{V,LR} \Big] + \alpha_s \alpha \Big[ -\frac{32}{9} L_{ed\,ij11}^{V,LL} \\
& - \frac{32}{9} L_{ed\,ij22}^{V,LL} - \frac{32}{9} L_{ed\,ij11}^{V,LR} - \frac{32}{9} L_{ed\,ij22}^{V,LR} + \frac{64}{9} L_{eu\,ij11}^{V,LL} - \frac{224}{9} L_{eu\,ij11}^{V,LR} \Big] + \alpha^2 \Big[ \frac{1168}{243} L_{ed\,ij11}^{V,LL} \\
& + \frac{1168}{243} L_{ed\,ij22}^{V,LL} + \frac{1792}{243} L_{ed\,ij11}^{V,LR} + \frac{1792}{243} L_{ed\,ij22}^{V,LR} + \frac{992}{81} L_{ee\,ijii}^{V,LL} + \frac{992}{81} L_{ee\,ijjj}^{V,LL} \\
& + \frac{1808}{81} L_{ee\,ijii}^{V,LR} + \frac{1808}{81} L_{ee\,ijjj}^{V,LR} - \frac{1184}{243} L_{eu\,ij11}^{V,LL} - \frac{30656}{243} L_{eu\,ij11}^{V,LR} \Big] ; \\
\dot{L}_{ee\,ijjj}^{V,LR} &= e^2 \Big[ \frac{4}{3} L_{ed\,ij11}^{V,LL} + \frac{4}{3} L_{ed\,ij22}^{V,LL} + \frac{4}{3} L_{ed\,ij11}^{V,LR} + \frac{4}{3} L_{ed\,ij22}^{V,LR} + \frac{16}{3} L_{ee\,ijii}^{V,LL} \\
& + \frac{16}{3} L_{ee\,ijjj}^{V,LL} + \frac{4}{3} L_{ee\,ijii}^{V,LR} - \frac{32}{3} L_{ee\,ijjj}^{V,LR} - \frac{8}{3} L_{eu\,ij11}^{V,LL} - \frac{8}{3} L_{eu\,ij11}^{V,LR} \Big] + \alpha_s \alpha \Big[ \frac{16}{3} L_{ed\,ij11}^{V,LL} \\
& + \frac{16}{3} L_{ed\,ij22}^{V,LL} + \frac{16}{3} L_{ed\,ij11}^{V,LR} + \frac{16}{3} L_{ed\,ij22}^{V,LR} - \frac{32}{3} L_{eu\,ij11}^{V,LL} - \frac{32}{3} L_{eu\,ij11}^{V,LR} \Big] + \alpha^2 \Big[ -\frac{344}{81} L_{ed\,ij11}^{V,LL} \\
& - \frac{344}{81} L_{ed\,ij22}^{V,LL} + \frac{424}{81} L_{ed\,ij11}^{V,LR} + \frac{424}{81} L_{ed\,ij22}^{V,LR} - \frac{736}{27} L_{ee\,ijii}^{V,LL} - \frac{736}{27} L_{ee\,ijjj}^{V,LL} + \frac{296}{27} L_{ee\,ijii}^{V,LR} \\
& + \frac{4274}{27} L_{ee\,ijjj}^{V,LR} - \frac{3128}{81} L_{eu\,ij11}^{V,LL} - \frac{56}{81} L_{eu\,ij11}^{V,LR} \Big] ;
\end{aligned}$$

$$\begin{aligned}
\dot{L}_{ij\bar{i}\bar{i}}^{V,LR} = & e^2 \left[ \frac{4}{3} L_{ij11}^{V,LL} + \frac{4}{3} L_{ij22}^{V,LL} + \frac{4}{3} L_{ij11}^{V,LR} + \frac{4}{3} L_{ij22}^{V,LR} + \frac{16}{3} L_{ij\bar{i}\bar{i}}^{V,LL} \right. \\
& + \frac{16}{3} L_{ij\bar{j}\bar{j}}^{V,LL} - \frac{32}{3} L_{ij\bar{i}\bar{i}}^{V,LR} + \frac{4}{3} L_{ij\bar{j}\bar{j}}^{V,LR} - \frac{8}{3} L_{ij11}^{V,LL} - \frac{8}{3} L_{ij11}^{V,LR} \left. \right] + \alpha_s \alpha \left[ \frac{16}{3} L_{ij11}^{V,LL} \right. \\
& + \frac{16}{3} L_{ij22}^{V,LL} + \frac{16}{3} L_{ij11}^{V,LR} + \frac{16}{3} L_{ij22}^{V,LR} - \frac{32}{3} L_{ij11}^{V,LL} - \frac{32}{3} L_{ij11}^{V,LR} \left. \right] + \alpha^2 \left[ -\frac{344}{81} L_{ij11}^{V,LL} \right. \\
& - \frac{344}{81} L_{ij22}^{V,LL} + \frac{424}{81} L_{ij11}^{V,LR} + \frac{424}{81} L_{ij22}^{V,LR} - \frac{736}{27} L_{ij\bar{i}\bar{i}}^{V,LL} - \frac{736}{27} L_{ij\bar{j}\bar{j}}^{V,LL} + \frac{4274}{27} L_{ij\bar{i}\bar{i}}^{V,LR} \\
& \left. + \frac{296}{27} L_{ij\bar{j}\bar{j}}^{V,LR} - \frac{3128}{81} L_{ij11}^{V,LL} - \frac{56}{81} L_{ij11}^{V,LR} \right] ;
\end{aligned}$$

$$\begin{aligned}
\dot{L}_{ij11}^{S,RL} = & -8g_s^2 L_{ij11}^{S,RL} - \frac{20}{3} e^2 L_{ij11}^{S,RL} - \frac{1052}{9} \alpha_s^2 L_{ij11}^{S,RL} - \frac{8}{9} \alpha_s \alpha L_{ij11}^{S,RL} \\
& + \frac{1402}{27} \alpha^2 L_{ij11}^{S,RL} ;
\end{aligned}$$

$$\begin{aligned}
\dot{L}_{ij22}^{S,RL} = & -8g_s^2 L_{ij22}^{S,RL} - \frac{20}{3} e^2 L_{ij22}^{S,RL} - \frac{1052}{9} \alpha_s^2 L_{ij22}^{S,RL} - \frac{8}{9} \alpha_s \alpha L_{ij22}^{S,RL} \\
& + \frac{1402}{27} \alpha^2 L_{ij22}^{S,RL} ;
\end{aligned}$$

$$\begin{aligned}
\dot{L}_{ij11}^{S,RL} = & -8g_s^2 L_{ij11}^{S,RL} - \frac{26}{3} e^2 L_{ij11}^{S,RL} - \frac{1052}{9} \alpha_s^2 L_{ij11}^{S,RL} - \frac{32}{9} \alpha_s \alpha L_{ij11}^{S,RL} \\
& + \frac{223}{27} \alpha^2 L_{ij11}^{S,RL} ;
\end{aligned}$$

$$\begin{aligned}
\dot{L}_{ij11}^{S,RR} = & -8g_s^2 L_{ij11}^{S,RR} + e^2 \left[ -\frac{20}{3} L_{ij11}^{S,RR} - 32 L_{ij11}^{T,RR} \right] - \frac{1052}{9} \alpha_s^2 L_{ij11}^{S,RR} \\
& + \alpha_s \alpha \left[ \frac{1792}{9} L_{ij11}^{T,RR} - \frac{8}{9} L_{ij11}^{S,RR} \right] + \alpha^2 \left[ \frac{94}{27} L_{ij11}^{S,RR} + \frac{14080}{27} L_{ij11}^{T,RR} \right] ;
\end{aligned}$$

$$\begin{aligned}
\dot{L}_{ij11}^{T,RR} = & \frac{8}{3} g_s^2 L_{ij11}^{T,RR} + e^2 \left[ \frac{20}{9} L_{ij11}^{T,RR} - \frac{2}{3} L_{ij11}^{S,RR} \right] + \frac{1756}{27} \alpha_s^2 L_{ij11}^{T,RR} \\
& + \alpha_s \alpha \left[ \frac{16}{3} L_{ij11}^{S,RR} - \frac{152}{27} L_{ij11}^{T,RR} \right] + \alpha^2 \left[ \frac{112}{27} L_{ij11}^{S,RR} - \frac{1766}{81} L_{ij11}^{T,RR} \right] ;
\end{aligned}$$

$$\begin{aligned}
\dot{L}_{ij22}^{S,RR} = & -8g_s^2 L_{ij22}^{S,RR} + e^2 \left[ -\frac{20}{3} L_{ij22}^{S,RR} - 32 L_{ij22}^{T,RR} \right] - \frac{1052}{9} \alpha_s^2 L_{ij22}^{S,RR}
\end{aligned}$$

$$\begin{aligned}
& + \alpha_s \alpha \left[ \frac{1792}{9} L_{ij22}^{T,RR} - \frac{8}{9} L_{ij22}^{S,RR} \right] + \alpha^2 \left[ \frac{94}{27} L_{ij22}^{S,RR} + \frac{14080}{27} L_{ij22}^{T,RR} \right]; \\
\dot{L}_{ij22}^{T,RR} &= \frac{8}{3} g_s^2 L_{ij22}^{T,RR} + e^2 \left[ \frac{20}{9} L_{ij22}^{T,RR} - \frac{2}{3} L_{ij22}^{S,RR} \right] + \frac{1756}{27} \alpha_s^2 L_{ij22}^{T,RR} \\
& + \alpha_s \alpha \left[ \frac{16}{3} L_{ij22}^{S,RR} - \frac{152}{27} L_{ij22}^{T,RR} \right] + \alpha^2 \left[ \frac{112}{27} L_{ij22}^{S,RR} - \frac{1766}{81} L_{ij22}^{T,RR} \right]; \\
\dot{L}_{ij11}^{S,RR} &= -8g_s^2 L_{ij11}^{S,RR} + e^2 \left[ 64 L_{ij11}^{T,RR} - \frac{26}{3} L_{ij11}^{S,RR} \right] - \frac{1052}{9} \alpha_s^2 L_{ij11}^{S,RR} \\
& + \alpha_s \alpha \left[ -\frac{32}{9} L_{ij11}^{S,RR} - \frac{3584}{9} L_{ij11}^{T,RR} \right] + \alpha^2 \left[ -\frac{1553}{27} L_{ij11}^{S,RR} - \frac{23936}{27} L_{ij11}^{T,RR} \right]; \\
\dot{L}_{ij11}^{T,RR} &= \frac{8}{3} g_s^2 L_{ij11}^{T,RR} + e^2 \left[ \frac{4}{3} L_{ij11}^{S,RR} + \frac{26}{9} L_{ij11}^{T,RR} \right] + \frac{1756}{27} \alpha_s^2 L_{ij11}^{T,RR} \\
& + \alpha_s \alpha \left[ -\frac{32}{3} L_{ij11}^{S,RR} - \frac{608}{27} L_{ij11}^{T,RR} \right] + \alpha^2 \left[ -\frac{440}{27} L_{ij11}^{S,RR} - \frac{3971}{81} L_{ij11}^{T,RR} \right]; \\
\dot{L}_{ijjj}^{S,RR} &= -4e^2 L_{ijjj}^{S,RR} - \frac{851}{9} \alpha^2 L_{ijjj}^{S,RR}; \\
\dot{L}_{ijii}^{S,RR} &= -4e^2 L_{ijii}^{S,RR} - \frac{851}{9} \alpha^2 L_{ijii}^{S,RR}; \\
\dot{L}_{ij11}^{V,RR} &= e^2 \left[ \frac{4}{9} L_{11ij}^{V,LR} + \frac{4}{9} L_{22ij}^{V,LR} + \frac{40}{9} L_{ij11}^{V,RR} + \frac{4}{9} L_{ij22}^{V,RR} + \frac{4}{9} L_{iijj}^{V,LR} \right. \\
& + \frac{4}{9} L_{jjij}^{V,LR} + \frac{16}{9} L_{ijii}^{V,RR} + \frac{16}{9} L_{ijjj}^{V,RR} - \frac{8}{9} L_{ij11}^{V,RR} - \frac{8}{9} L_{11ij}^{V,LR} \left. \right] + \alpha_s^2 \left[ -8 L_{11ij}^{V,LR} \right. \\
& - 8 L_{22ij}^{V,LR} + 8 L_{ed}^{V,RR} + 8 L_{ij11}^{V,RR} + 8 L_{ij22}^{V,RR} + 8 L_{ij11}^{V,RR} - 8 L_{11ij}^{V,LR} \left. \right] + \alpha_s \alpha \left[ \frac{16}{9} L_{11ij}^{V,LR} \right. \\
& + \frac{16}{9} L_{22ij}^{V,LR} - \frac{128}{9} L_{ij11}^{V,RR} + \frac{16}{9} L_{ij22}^{V,RR} - \frac{32}{9} L_{ij11}^{V,RR} - \frac{32}{9} L_{11ij}^{V,LR} \left. \right] + \alpha^2 \left[ -\frac{200}{243} L_{11ij}^{V,LR} \right. \\
& - \frac{200}{243} L_{22ij}^{V,LR} - \frac{3614}{243} L_{ij11}^{V,RR} - \frac{104}{243} L_{ij22}^{V,RR} - \frac{520}{81} L_{iijj}^{V,LR} - \frac{520}{81} L_{jjij}^{V,LR} + \frac{32}{81} L_{ijii}^{V,RR} \\
& \left. + \frac{32}{81} L_{ijjj}^{V,RR} - \frac{1016}{243} L_{ij11}^{V,RR} - \frac{1400}{243} L_{11ij}^{V,LR} \right];
\end{aligned}$$

$$\begin{aligned}
\dot{L}_{ed\ ij22}^{V,RR} = & e^2 \left[ \frac{4}{9} L_{11ij}^{V,LR} + \frac{4}{9} L_{22ij}^{V,LR} + \frac{4}{9} L_{ij11}^{V,RR} + \frac{40}{9} L_{ij22}^{V,RR} + \frac{4}{9} L_{iij}^{V,LR} \right. \\
& + \frac{4}{9} L_{jjij}^{V,LR} + \frac{16}{9} L_{ijii}^{V,RR} + \frac{16}{9} L_{ijjj}^{V,RR} - \frac{8}{9} L_{ij11}^{V,RR} - \frac{8}{9} L_{11ij}^{V,LR} \left. \right] + \alpha_s^2 \left[ -8 L_{11ij}^{V,LR} \right. \\
& - 8 L_{22ij}^{V,LR} + 8 L_{ed\ ij11}^{V,RR} + 8 L_{ed\ ij22}^{V,RR} + 8 L_{eu\ ij11}^{V,RR} - 8 L_{ue\ 11ij}^{V,LR} \left. \right] + \alpha_s \alpha \left[ \frac{16}{9} L_{11ij}^{V,LR} \right. \\
& + \frac{16}{9} L_{22ij}^{V,LR} + \frac{16}{9} L_{ed\ ij11}^{V,RR} - \frac{128}{9} L_{ed\ ij22}^{V,RR} - \frac{32}{9} L_{eu\ ij11}^{V,RR} - \frac{32}{9} L_{ue\ 11ij}^{V,LR} \left. \right] + \alpha^2 \left[ -\frac{200}{243} L_{11ij}^{V,LR} \right. \\
& - \frac{200}{243} L_{22ij}^{V,LR} - \frac{104}{243} L_{ed\ ij11}^{V,RR} - \frac{3614}{243} L_{ed\ ij22}^{V,RR} - \frac{520}{81} L_{iij}^{V,LR} - \frac{520}{81} L_{jjij}^{V,LR} + \frac{32}{81} L_{ijii}^{V,RR} \\
& \left. + \frac{32}{81} L_{ijjj}^{V,RR} - \frac{1016}{243} L_{eu\ ij11}^{V,RR} - \frac{1400}{243} L_{ue\ 11ij}^{V,LR} \right] ;
\end{aligned}$$

$$\begin{aligned}
\dot{L}_{eu\ ij11}^{V,RR} = & e^2 \left[ -\frac{8}{9} L_{11ij}^{V,LR} - \frac{8}{9} L_{22ij}^{V,LR} - \frac{8}{9} L_{ij11}^{V,RR} - \frac{8}{9} L_{ij22}^{V,RR} - \frac{8}{9} L_{iij}^{V,LR} \right. \\
& - \frac{8}{9} L_{jjij}^{V,LR} - \frac{32}{9} L_{ijii}^{V,RR} - \frac{32}{9} L_{ijjj}^{V,RR} - \frac{56}{9} L_{eu\ ij11}^{V,RR} + \frac{16}{9} L_{ue\ 11ij}^{V,LR} \left. \right] + \alpha_s^2 \left[ -8 L_{11ij}^{V,LR} \right. \\
& - 8 L_{22ij}^{V,LR} + 8 L_{ed\ ij11}^{V,RR} + 8 L_{ed\ ij22}^{V,RR} + 8 L_{eu\ ij11}^{V,RR} - 8 L_{ue\ 11ij}^{V,LR} \left. \right] + \alpha_s \alpha \left[ -\frac{32}{9} L_{11ij}^{V,LR} \right. \\
& - \frac{32}{9} L_{22ij}^{V,LR} - \frac{32}{9} L_{ed\ ij11}^{V,RR} - \frac{32}{9} L_{ed\ ij22}^{V,RR} + \frac{352}{9} L_{eu\ ij11}^{V,RR} + \frac{64}{9} L_{ue\ 11ij}^{V,LR} \left. \right] + \alpha^2 \left[ \frac{1408}{243} L_{11ij}^{V,LR} \right. \\
& + \frac{1408}{243} L_{22ij}^{V,LR} + \frac{2512}{243} L_{ed\ ij11}^{V,RR} + \frac{2512}{243} L_{ed\ ij22}^{V,RR} + \frac{464}{81} L_{iij}^{V,LR} + \frac{464}{81} L_{jjij}^{V,LR} \\
& \left. + \frac{3680}{81} L_{ijii}^{V,RR} + \frac{3680}{81} L_{ijjj}^{V,RR} + \frac{3472}{243} L_{eu\ ij11}^{V,RR} - \frac{3104}{243} L_{ue\ 11ij}^{V,LR} \right] ;
\end{aligned}$$

$$\begin{aligned}
\dot{L}_{ee\ ijjj}^{V,RR} = & e^2 \left[ \frac{2}{3} L_{11ij}^{V,LR} + \frac{2}{3} L_{22ij}^{V,LR} + \frac{2}{3} L_{ij11}^{V,RR} + \frac{2}{3} L_{ij22}^{V,RR} + \frac{2}{3} L_{iij}^{V,LR} \right. \\
& + \frac{2}{3} L_{jjij}^{V,LR} + \frac{8}{3} L_{ijii}^{V,RR} + \frac{44}{3} L_{ijjj}^{V,RR} - \frac{4}{3} L_{eu\ ij11}^{V,RR} - \frac{4}{3} L_{ue\ 11ij}^{V,LR} \left. \right] + \alpha_s \alpha \left[ \frac{8}{3} L_{11ij}^{V,LR} \right. \\
& + \frac{8}{3} L_{22ij}^{V,LR} + \frac{8}{3} L_{ed\ ij11}^{V,RR} + \frac{8}{3} L_{ed\ ij22}^{V,RR} - \frac{16}{3} L_{eu\ ij11}^{V,RR} - \frac{16}{3} L_{ue\ 11ij}^{V,LR} \left. \right] + \alpha^2 \left[ \frac{68}{81} L_{11ij}^{V,LR} \right.
\end{aligned}$$

$$\begin{aligned}
& + \frac{68}{81} L_{22ij}^{V,LR} + \frac{332}{81} L_{ij11}^{V,RR} + \frac{332}{81} L_{ij22}^{V,RR} - \frac{356}{27} L_{iij}^{V,LR} - \frac{356}{27} L_{jjj}^{V,LR} + \frac{640}{27} L_{ijii}^{V,RR} \\
& - \frac{2150}{27} L_{ijjj}^{V,RR} - \frac{628}{81} L_{ij11}^{V,RR} - \frac{1684}{81} L_{11ij}^{V,LR} \Big] ;
\end{aligned}$$

$$\begin{aligned}
\dot{L}_{ijii}^{V,RR} = & e^2 \left[ \frac{2}{3} L_{11ij}^{V,LR} + \frac{2}{3} L_{22ij}^{V,LR} + \frac{2}{3} L_{ij11}^{V,RR} + \frac{2}{3} L_{ij22}^{V,RR} + \frac{2}{3} L_{iij}^{V,LR} \right. \\
& + \frac{2}{3} L_{jjj}^{V,LR} + \frac{44}{3} L_{ijii}^{V,RR} + \frac{8}{3} L_{ijjj}^{V,RR} - \frac{4}{3} L_{ij11}^{V,RR} - \frac{4}{3} L_{11ij}^{V,LR} \Big] + \alpha_s \alpha \left[ \frac{8}{3} L_{11ij}^{V,LR} \right. \\
& + \frac{8}{3} L_{22ij}^{V,LR} + \frac{8}{3} L_{ij11}^{V,RR} + \frac{8}{3} L_{ij22}^{V,RR} - \frac{16}{3} L_{ij11}^{V,RR} - \frac{16}{3} L_{11ij}^{V,LR} \Big] + \alpha^2 \left[ \frac{68}{81} L_{11ij}^{V,LR} \right. \\
& + \frac{68}{81} L_{22ij}^{V,LR} + \frac{332}{81} L_{ij11}^{V,RR} + \frac{332}{81} L_{ij22}^{V,RR} - \frac{356}{27} L_{iij}^{V,LR} - \frac{356}{27} L_{jjj}^{V,LR} - \frac{2150}{27} L_{ijii}^{V,RR} \\
& + \frac{640}{27} L_{ijjj}^{V,RR} - \frac{628}{81} L_{ij11}^{V,RR} - \frac{1684}{81} L_{11ij}^{V,LR} \Big] ;
\end{aligned}$$

$$\begin{aligned}
\dot{L}_{11ij}^{V,LR} = & e^2 \left[ -\frac{32}{9} L_{11ij}^{V,LR} + \frac{4}{9} L_{22ij}^{V,LR} + \frac{4}{9} L_{ij11}^{V,RR} + \frac{4}{9} L_{ij22}^{V,RR} + \frac{4}{9} L_{iij}^{V,LR} \right. \\
& + \frac{4}{9} L_{jjj}^{V,LR} + \frac{16}{9} L_{ijii}^{V,RR} + \frac{16}{9} L_{ijjj}^{V,RR} - \frac{8}{9} L_{ij11}^{V,RR} - \frac{8}{9} L_{11ij}^{V,LR} \Big] + \alpha_s^2 \left[ 8 L_{11ij}^{V,LR} \right. \\
& + 8 L_{22ij}^{V,LR} - 8 L_{ij11}^{V,RR} - 8 L_{ij22}^{V,RR} + 8 L_{11ij}^{V,LR} \Big] + \alpha_s \alpha \left[ \frac{160}{9} L_{11ij}^{V,LR} \right. \\
& + \frac{16}{9} L_{22ij}^{V,LR} + \frac{16}{9} L_{ij11}^{V,RR} + \frac{16}{9} L_{ij22}^{V,RR} - \frac{32}{9} L_{ij11}^{V,RR} - \frac{32}{9} L_{11ij}^{V,LR} \Big] + \alpha^2 \left[ \frac{11506}{243} L_{11ij}^{V,LR} \right. \\
& - \frac{104}{243} L_{22ij}^{V,LR} - \frac{440}{243} L_{ij11}^{V,RR} - \frac{440}{243} L_{ij22}^{V,RR} - \frac{184}{81} L_{iij}^{V,LR} - \frac{184}{81} L_{jjj}^{V,LR} - \frac{640}{81} L_{ijii}^{V,RR} \\
& - \frac{640}{81} L_{ijjj}^{V,RR} - \frac{1640}{243} L_{ij11}^{V,RR} - \frac{296}{243} L_{11ij}^{V,LR} \Big] ;
\end{aligned}$$

$$\begin{aligned}
\dot{L}_{22ij}^{V,LR} = & e^2 \left[ \frac{4}{9} L_{11ij}^{V,LR} - \frac{32}{9} L_{22ij}^{V,LR} + \frac{4}{9} L_{ij11}^{V,RR} + \frac{4}{9} L_{ij22}^{V,RR} + \frac{4}{9} L_{iij}^{V,LR} \right. \\
& + \frac{4}{9} L_{jjj}^{V,LR} + \frac{16}{9} L_{ijii}^{V,RR} + \frac{16}{9} L_{ijjj}^{V,RR} - \frac{8}{9} L_{ij11}^{V,RR} - \frac{8}{9} L_{11ij}^{V,LR} \Big] + \alpha_s^2 \left[ 8 L_{11ij}^{V,LR} \right.
\end{aligned}$$

$$\begin{aligned}
& + 8L_{22ij}^{V,LR} - 8L_{ij11}^{V,RR} - 8L_{ij22}^{V,RR} - 8L_{ij11}^{V,RR} + 8L_{11ij}^{V,LR} \Big] + \alpha_s \alpha \left[ \frac{16}{9} L_{11ij}^{V,LR} \right. \\
& + \frac{160}{9} L_{22ij}^{V,LR} + \frac{16}{9} L_{ij11}^{V,RR} + \frac{16}{9} L_{ij22}^{V,RR} - \frac{32}{9} L_{ij11}^{V,RR} - \frac{32}{9} L_{11ij}^{V,LR} \Big] + \alpha^2 \left[ -\frac{104}{243} L_{11ij}^{V,LR} \right. \\
& + \frac{11506}{243} L_{22ij}^{V,LR} - \frac{440}{243} L_{ij11}^{V,RR} - \frac{440}{243} L_{ij22}^{V,RR} - \frac{184}{81} L_{iiij}^{V,LR} - \frac{184}{81} L_{jjij}^{V,LR} - \frac{640}{81} L_{ijii}^{V,RR} \\
& \left. - \frac{640}{81} L_{ijjj}^{V,RR} - \frac{1640}{243} L_{ij11}^{V,RR} - \frac{296}{243} L_{11ij}^{V,LR} \right] ; \\
\dot{L}_{11ij}^{V,LR} & = e^2 \left[ -\frac{8}{9} L_{11ij}^{V,LR} - \frac{8}{9} L_{22ij}^{V,LR} - \frac{8}{9} L_{ij11}^{V,RR} - \frac{8}{9} L_{ij22}^{V,RR} - \frac{8}{9} L_{iiij}^{V,LR} \right. \\
& - \frac{8}{9} L_{jjij}^{V,LR} - \frac{32}{9} L_{ijii}^{V,RR} - \frac{32}{9} L_{ijjj}^{V,RR} + \frac{16}{9} L_{ij11}^{V,RR} + \frac{88}{9} L_{11ij}^{V,LR} \Big] + \alpha_s^2 \left[ 8L_{11ij}^{V,LR} \right. \\
& + 8L_{22ij}^{V,LR} - 8L_{ij11}^{V,RR} - 8L_{ij22}^{V,RR} - 8L_{ij11}^{V,RR} + 8L_{11ij}^{V,LR} \Big] + \alpha_s \alpha \left[ -\frac{32}{9} L_{11ij}^{V,LR} \right. \\
& - \frac{32}{9} L_{22ij}^{V,LR} - \frac{32}{9} L_{ij11}^{V,RR} - \frac{32}{9} L_{ij22}^{V,RR} + \frac{64}{9} L_{ij11}^{V,RR} - \frac{224}{9} L_{11ij}^{V,LR} \Big] + \alpha^2 \left[ \frac{1792}{243} L_{11ij}^{V,LR} \right. \\
& + \frac{1792}{243} L_{22ij}^{V,LR} + \frac{1168}{243} L_{ij11}^{V,RR} + \frac{1168}{243} L_{ij22}^{V,RR} + \frac{1808}{81} L_{iiij}^{V,LR} + \frac{1808}{81} L_{jjij}^{V,LR} \\
& \left. + \frac{992}{81} L_{ijii}^{V,RR} + \frac{992}{81} L_{ijjj}^{V,RR} - \frac{1184}{243} L_{ij11}^{V,RR} - \frac{30656}{243} L_{11ij}^{V,LR} \right] ; \\
\dot{L}_{jjij}^{V,LR} & = e^2 \left[ \frac{4}{3} L_{11ij}^{V,LR} + \frac{4}{3} L_{22ij}^{V,LR} + \frac{4}{3} L_{ij11}^{V,RR} + \frac{4}{3} L_{ij22}^{V,RR} + \frac{4}{3} L_{iiij}^{V,LR} \right. \\
& - \frac{32}{3} L_{jjij}^{V,LR} + \frac{16}{3} L_{ijii}^{V,RR} + \frac{16}{3} L_{ijjj}^{V,RR} - \frac{8}{3} L_{ij11}^{V,RR} - \frac{8}{3} L_{11ij}^{V,LR} \Big] + \alpha_s \alpha \left[ \frac{16}{3} L_{11ij}^{V,LR} \right. \\
& + \frac{16}{3} L_{22ij}^{V,LR} + \frac{16}{3} L_{ij11}^{V,RR} + \frac{16}{3} L_{ij22}^{V,RR} - \frac{32}{3} L_{ij11}^{V,RR} - \frac{32}{3} L_{11ij}^{V,LR} \Big] + \alpha^2 \left[ \frac{424}{81} L_{11ij}^{V,LR} \right. \\
& + \frac{424}{81} L_{22ij}^{V,LR} - \frac{344}{81} L_{ij11}^{V,RR} - \frac{344}{81} L_{ij22}^{V,RR} + \frac{296}{27} L_{iiij}^{V,LR} + \frac{4274}{27} L_{jjij}^{V,LR} - \frac{736}{27} L_{ijii}^{V,RR} \\
& \left. - \frac{736}{27} L_{ijjj}^{V,RR} - \frac{3128}{81} L_{ij11}^{V,RR} - \frac{56}{81} L_{11ij}^{V,LR} \right] ;
\end{aligned}$$

$$\begin{aligned}
\dot{L}_{\bar{ii}j}^{V,LR} = & e^2 \left[ \frac{4}{3} L_{11ij}^{V,LR} + \frac{4}{3} L_{22ij}^{V,LR} + \frac{4}{3} L_{ij11}^{V,RR} + \frac{4}{3} L_{ij22}^{V,RR} - \frac{32}{3} L_{\bar{ii}j}^{V,LR} \right. \\
& + \frac{4}{3} L_{jjij}^{V,LR} + \frac{16}{3} L_{ijii}^{V,RR} + \frac{16}{3} L_{ijjj}^{V,RR} - \frac{8}{3} L_{ij11}^{V,RR} - \frac{8}{3} L_{11ij}^{V,LR} \left. \right] + \alpha_s \alpha \left[ \frac{16}{3} L_{11ij}^{V,LR} \right. \\
& + \frac{16}{3} L_{22ij}^{V,LR} + \frac{16}{3} L_{ij11}^{V,RR} + \frac{16}{3} L_{ij22}^{V,RR} - \frac{32}{3} L_{ij11}^{V,RR} - \frac{32}{3} L_{11ij}^{V,LR} \left. \right] + \alpha^2 \left[ \frac{424}{81} L_{11ij}^{V,LR} \right. \\
& + \frac{424}{81} L_{22ij}^{V,LR} - \frac{344}{81} L_{ij11}^{V,RR} - \frac{344}{81} L_{ij22}^{V,RR} + \frac{4274}{27} L_{\bar{ii}j}^{V,LR} + \frac{296}{27} L_{jjij}^{V,LR} - \frac{736}{27} L_{ijii}^{V,RR} \\
& \left. - \frac{736}{27} L_{ijjj}^{V,RR} - \frac{3128}{81} L_{ij11}^{V,RR} - \frac{56}{81} L_{11ij}^{V,LR} \right] ;
\end{aligned}$$

$$\dot{L}_{\bar{\nu}e}^{V,LL} = 0 ;$$

$$\dot{L}_{22ij}^{V,LL} = 0 ;$$

$$\dot{L}_{33ij}^{V,LL} = 0 ;$$

$$\dot{L}_{11ij}^{V,LR} = 0 ;$$

$$\dot{L}_{22ij}^{V,LR} = 0 ;$$

$$\dot{L}_{33ij}^{V,LR} = 0 ;$$

$$\dot{L}_{11ij}^{S,LR} = \frac{71}{3} \alpha^2 L_{11ij}^{S,LR} - 6e^2 L_{11ij}^{S,LR} ;$$

$$\dot{L}_{22ij}^{S,LR} = \frac{71}{3} \alpha^2 L_{22ij}^{S,LR} - 6e^2 L_{22ij}^{S,LR} ;$$

$$\dot{L}_{33ij}^{S,LR} = \frac{71}{3} \alpha^2 L_{33ij}^{S,LR} - 6e^2 L_{33ij}^{S,LR} ;$$

$$\dot{L}_{11ij}^{S,LL} = \frac{71}{3} \alpha^2 L_{11ij}^{S,LL} - 6e^2 L_{11ij}^{S,LL} ;$$

$$\dot{L}_{11ij}^{T,LL} = 2e^2 L_{11ij}^{T,LL} - \frac{379}{9} \alpha^2 L_{11ij}^{T,LL} ;$$

$$\dot{L}_{22ij}^{S,LL} = \frac{71}{3} \alpha^2 L_{22ij}^{S,LL} - 6e^2 L_{22ij}^{S,LL} ;$$

$$\dot{L}_{22ij}^{T,LL} = 2e^2 L_{22ij}^{T,LL} - \frac{379}{9} \alpha^2 L_{22ij}^{T,LL} ;$$

$$\begin{aligned}\dot{L}_{33ij}^{S,LL} &= \frac{71}{3}\alpha^2 L_{33ij}^{S,LL} - 6e^2 L_{33ij}^{S,LL} ; \\ \dot{L}_{33ij}^{T,LL} &= 2e^2 L_{33ij}^{T,LL} - \frac{379}{9}\alpha^2 L_{33ij}^{T,LL} ;\end{aligned}$$

### 3.7 $\Delta F = 1^{ff}$ : $\nu$ -type ( $\bar{\nu}_i \nu_j \bar{f}_k f_k$ )

$$\begin{aligned}\dot{L}_{ij11}^{V,LL} &= e^2 \left[ \frac{4}{3} L_{ij11}^{V,LL} + \frac{4}{3} L_{ij22}^{V,LL} + \frac{4}{3} L_{ij11}^{V,LR} + \frac{4}{3} L_{ij22}^{V,LR} + \frac{4}{3} L_{ij11}^{V,LL} \right. \\ &\quad \left. + \frac{4}{3} L_{ij22}^{V,LL} + \frac{4}{3} L_{ij11}^{V,LR} + \frac{4}{3} L_{ij22}^{V,LR} - \frac{8}{3} L_{ij11}^{V,LL} - \frac{8}{3} L_{ij11}^{V,LR} \right] \\ &\quad + \alpha_s \alpha \left[ \frac{16}{3} L_{ij11}^{V,LL} + \frac{16}{3} L_{ij22}^{V,LL} + \frac{16}{3} L_{ij11}^{V,LR} + \frac{16}{3} L_{ij22}^{V,LR} - \frac{32}{3} L_{ij11}^{V,LL} \right. \\ &\quad \left. - \frac{32}{3} L_{ij11}^{V,LR} \right] + \alpha^2 \left[ \frac{40}{9} L_{ij11}^{V,LL} + \frac{40}{9} L_{ij22}^{V,LL} - \frac{32}{9} L_{ij11}^{V,LR} - \frac{32}{9} L_{ij22}^{V,LR} \right. \\ &\quad \left. + 16 L_{ij11}^{V,LL} + 16 L_{ij22}^{V,LL} - 8 L_{ij11}^{V,LR} - 8 L_{ij22}^{V,LR} + \frac{112}{9} L_{ij11}^{V,LL} - \frac{176}{9} L_{ij11}^{V,LR} \right] ; \\ \dot{L}_{ij22}^{V,LL} &= e^2 \left[ \frac{4}{3} L_{ij11}^{V,LL} + \frac{4}{3} L_{ij22}^{V,LL} + \frac{4}{3} L_{ij11}^{V,LR} + \frac{4}{3} L_{ij22}^{V,LR} + \frac{4}{3} L_{ij11}^{V,LL} \right. \\ &\quad \left. + \frac{4}{3} L_{ij22}^{V,LL} + \frac{4}{3} L_{ij11}^{V,LR} + \frac{4}{3} L_{ij22}^{V,LR} - \frac{8}{3} L_{ij11}^{V,LL} - \frac{8}{3} L_{ij11}^{V,LR} \right] \\ &\quad + \alpha_s \alpha \left[ \frac{16}{3} L_{ij11}^{V,LL} + \frac{16}{3} L_{ij22}^{V,LL} + \frac{16}{3} L_{ij11}^{V,LR} + \frac{16}{3} L_{ij22}^{V,LR} - \frac{32}{3} L_{ij11}^{V,LL} \right. \\ &\quad \left. - \frac{32}{3} L_{ij11}^{V,LR} \right] + \alpha^2 \left[ \frac{40}{9} L_{ij11}^{V,LL} + \frac{40}{9} L_{ij22}^{V,LL} - \frac{32}{9} L_{ij11}^{V,LR} - \frac{32}{9} L_{ij22}^{V,LR} \right. \\ &\quad \left. + 16 L_{ij11}^{V,LL} + 16 L_{ij22}^{V,LL} - 8 L_{ij11}^{V,LR} - 8 L_{ij22}^{V,LR} + \frac{112}{9} L_{ij11}^{V,LL} - \frac{176}{9} L_{ij11}^{V,LR} \right] ; \\ \dot{L}_{ij11}^{V,LL} &= e^2 \left[ \frac{4}{9} L_{ij11}^{V,LL} + \frac{4}{9} L_{ij22}^{V,LL} + \frac{4}{9} L_{ij11}^{V,LR} + \frac{4}{9} L_{ij22}^{V,LR} + \frac{4}{9} L_{ij11}^{V,LL} \right. \\ &\quad \left. + \frac{4}{9} L_{ij22}^{V,LL} + \frac{4}{9} L_{ij11}^{V,LR} + \frac{4}{9} L_{ij22}^{V,LR} - \frac{8}{9} L_{ij11}^{V,LL} - \frac{8}{9} L_{ij11}^{V,LR} \right] \\ &\quad + \alpha_s \alpha \left[ \frac{16}{3} L_{ij11}^{V,LL} + \frac{16}{3} L_{ij22}^{V,LL} + \frac{16}{3} L_{ij11}^{V,LR} + \frac{16}{3} L_{ij22}^{V,LR} - \frac{32}{3} L_{ij11}^{V,LL} \right. \\ &\quad \left. - \frac{32}{3} L_{ij11}^{V,LR} \right] + \alpha^2 \left[ \frac{40}{9} L_{ij11}^{V,LL} + \frac{40}{9} L_{ij22}^{V,LL} - \frac{32}{9} L_{ij11}^{V,LR} - \frac{32}{9} L_{ij22}^{V,LR} \right. \\ &\quad \left. + 16 L_{ij11}^{V,LL} + 16 L_{ij22}^{V,LL} - 8 L_{ij11}^{V,LR} - 8 L_{ij22}^{V,LR} + \frac{112}{9} L_{ij11}^{V,LL} - \frac{176}{9} L_{ij11}^{V,LR} \right] ;\end{aligned}$$



$$\begin{aligned}
& + \alpha_s^2 \left[ 8L_{ij11}^{V,LL} + 8L_{ij22}^{V,LL} - 8L_{ij11}^{V,LR} - 8L_{ij22}^{V,LR} + 8L_{ij11}^{V,LL} \right. \\
& \left. - 8L_{ij11}^{V,LR} \right] + \alpha_s \alpha \left[ \frac{16}{9}L_{ij11}^{V,LL} + \frac{16}{9}L_{ij22}^{V,LL} + \frac{16}{9}L_{ij11}^{V,LR} + \frac{16}{9}L_{ij22}^{V,LR} \right. \\
& \left. - \frac{32}{9}L_{ij11}^{V,LL} - \frac{32}{9}L_{ij11}^{V,LR} \right] + \alpha^2 \left[ \frac{16}{27}L_{ij11}^{V,LL} + \frac{16}{27}L_{ij22}^{V,LL} - \frac{8}{27}L_{ij11}^{V,LR} \right. \\
& \left. - \frac{8}{27}L_{ij22}^{V,LR} + \frac{8}{3}L_{ij11}^{V,LL} + \frac{8}{3}L_{ij22}^{V,LL} + \frac{16}{27}L_{ij11}^{V,LL} - \frac{80}{27}L_{ij11}^{V,LR} \right]; \\
\dot{L}_{ij22}^{V,LL} & = e^2 \left[ \frac{4}{9}L_{ij11}^{V,LL} + \frac{4}{9}L_{ij22}^{V,LL} + \frac{4}{9}L_{ij11}^{V,LR} + \frac{4}{9}L_{ij22}^{V,LR} + \frac{4}{9}L_{ij11}^{V,LL} \right. \\
& \left. + \frac{4}{9}L_{ij22}^{V,LL} + \frac{4}{9}L_{ij11}^{V,LR} + \frac{4}{9}L_{ij22}^{V,LR} - \frac{8}{9}L_{ij11}^{V,LL} - \frac{8}{9}L_{ij11}^{V,LR} \right] \\
& + \alpha_s^2 \left[ 8L_{ij11}^{V,LL} + 8L_{ij22}^{V,LL} - 8L_{ij11}^{V,LR} - 8L_{ij22}^{V,LR} + 8L_{ij11}^{V,LL} \right. \\
& \left. - 8L_{ij11}^{V,LR} \right] + \alpha_s \alpha \left[ \frac{16}{9}L_{ij11}^{V,LL} + \frac{16}{9}L_{ij22}^{V,LL} + \frac{16}{9}L_{ij11}^{V,LR} + \frac{16}{9}L_{ij22}^{V,LR} \right. \\
& \left. - \frac{32}{9}L_{ij11}^{V,LL} - \frac{32}{9}L_{ij11}^{V,LR} \right] + \alpha^2 \left[ \frac{16}{27}L_{ij11}^{V,LL} + \frac{16}{27}L_{ij22}^{V,LL} - \frac{8}{27}L_{ij11}^{V,LR} \right. \\
& \left. - \frac{8}{27}L_{ij22}^{V,LR} + \frac{8}{3}L_{ij11}^{V,LL} + \frac{8}{3}L_{ij22}^{V,LL} + \frac{16}{27}L_{ij11}^{V,LL} - \frac{80}{27}L_{ij11}^{V,LR} \right]; \\
\dot{L}_{ij11}^{V,LL} & = e^2 \left[ -\frac{8}{9}L_{ij11}^{V,LL} - \frac{8}{9}L_{ij22}^{V,LL} - \frac{8}{9}L_{ij11}^{V,LR} - \frac{8}{9}L_{ij22}^{V,LR} - \frac{8}{9}L_{ij11}^{V,LL} \right. \\
& \left. - \frac{8}{9}L_{ij22}^{V,LL} - \frac{8}{9}L_{ij11}^{V,LR} - \frac{8}{9}L_{ij22}^{V,LR} + \frac{16}{9}L_{ij11}^{V,LL} + \frac{16}{9}L_{ij11}^{V,LR} \right] \\
& + \alpha_s^2 \left[ 8L_{ij11}^{V,LL} + 8L_{ij22}^{V,LL} - 8L_{ij11}^{V,LR} - 8L_{ij22}^{V,LR} + 8L_{ij11}^{V,LL} \right. \\
& \left. - 8L_{ij11}^{V,LR} \right] + \alpha_s \alpha \left[ -\frac{32}{9}L_{ij11}^{V,LL} - \frac{32}{9}L_{ij22}^{V,LL} - \frac{32}{9}L_{ij11}^{V,LR} - \frac{32}{9}L_{ij22}^{V,LR} \right. \\
& \left. - \frac{32}{9}L_{ij11}^{V,LL} - \frac{32}{9}L_{ij22}^{V,LL} - \frac{32}{9}L_{ij11}^{V,LR} - \frac{32}{9}L_{ij22}^{V,LR} \right]
\end{aligned}$$

$$\begin{aligned}
& + \frac{64}{9} L_{ij11}^{V,LL} + \frac{64}{9} L_{ij11}^{V,LR} \Big] + \alpha^2 \Big[ \frac{40}{27} L_{ij11}^{V,LL} + \frac{40}{27} L_{ij22}^{V,LL} - \frac{56}{27} L_{ij11}^{V,LR} \\
& - \frac{56}{27} L_{ij22}^{V,LR} + \frac{8}{3} L_{ij11}^{V,LL} + \frac{8}{3} L_{ij22}^{V,LL} - 8 L_{ij11}^{V,LR} - 8 L_{ij22}^{V,LR} + \frac{256}{27} L_{ij11}^{V,LL} \\
& - \frac{128}{27} L_{ij11}^{V,LR} \Big] ;
\end{aligned}$$

$$\begin{aligned}
\dot{L}_{ij11}^{V,LR} &= e^2 \Big[ \frac{4}{3} L_{ij11}^{V,LL} + \frac{4}{3} L_{ij22}^{V,LL} + \frac{4}{3} L_{ij11}^{V,LR} + \frac{4}{3} L_{ij22}^{V,LR} + \frac{4}{3} L_{ij11}^{V,LL} \\
& + \frac{4}{3} L_{ij22}^{V,LL} + \frac{4}{3} L_{ij11}^{V,LR} + \frac{4}{3} L_{ij22}^{V,LR} - \frac{8}{3} L_{ij11}^{V,LL} - \frac{8}{3} L_{ij11}^{V,LR} \Big] \\
& + \alpha_s \alpha \Big[ \frac{16}{3} L_{ij11}^{V,LL} + \frac{16}{3} L_{ij22}^{V,LL} + \frac{16}{3} L_{ij11}^{V,LR} + \frac{16}{3} L_{ij22}^{V,LR} - \frac{32}{3} L_{ij11}^{V,LL} \\
& - \frac{32}{3} L_{ij11}^{V,LR} \Big] + \alpha^2 \Big[ - \frac{32}{9} L_{ij11}^{V,LL} - \frac{32}{9} L_{ij22}^{V,LL} + \frac{40}{9} L_{ij11}^{V,LR} + \frac{40}{9} L_{ij22}^{V,LR} \\
& - 8 L_{ij11}^{V,LL} - 8 L_{ij22}^{V,LL} + 16 L_{ij11}^{V,LR} + 16 L_{ij22}^{V,LR} - \frac{176}{9} L_{ij11}^{V,LL} + \frac{112}{9} L_{ij11}^{V,LR} \Big] ;
\end{aligned}$$

$$\begin{aligned}
\dot{L}_{ij22}^{V,LR} &= e^2 \Big[ \frac{4}{3} L_{ij11}^{V,LL} + \frac{4}{3} L_{ij22}^{V,LL} + \frac{4}{3} L_{ij11}^{V,LR} + \frac{4}{3} L_{ij22}^{V,LR} + \frac{4}{3} L_{ij11}^{V,LL} \\
& + \frac{4}{3} L_{ij22}^{V,LL} + \frac{4}{3} L_{ij11}^{V,LR} + \frac{4}{3} L_{ij22}^{V,LR} - \frac{8}{3} L_{ij11}^{V,LL} - \frac{8}{3} L_{ij11}^{V,LR} \Big] \\
& + \alpha_s \alpha \Big[ \frac{16}{3} L_{ij11}^{V,LL} + \frac{16}{3} L_{ij22}^{V,LL} + \frac{16}{3} L_{ij11}^{V,LR} + \frac{16}{3} L_{ij22}^{V,LR} - \frac{32}{3} L_{ij11}^{V,LL} \\
& - \frac{32}{3} L_{ij11}^{V,LR} \Big] + \alpha^2 \Big[ - \frac{32}{9} L_{ij11}^{V,LL} - \frac{32}{9} L_{ij22}^{V,LL} + \frac{40}{9} L_{ij11}^{V,LR} + \frac{40}{9} L_{ij22}^{V,LR} \\
& - 8 L_{ij11}^{V,LL} - 8 L_{ij22}^{V,LL} + 16 L_{ij11}^{V,LR} + 16 L_{ij22}^{V,LR} - \frac{176}{9} L_{ij11}^{V,LL} + \frac{112}{9} L_{ij11}^{V,LR} \Big] ;
\end{aligned}$$

$$\dot{L}_{ij11}^{V,LR} = e^2 \Big[ \frac{4}{9} L_{ij11}^{V,LL} + \frac{4}{9} L_{ij22}^{V,LL} + \frac{4}{9} L_{ij11}^{V,LR} + \frac{4}{9} L_{ij22}^{V,LR} + \frac{4}{9} L_{ij11}^{V,LL}$$

$$\begin{aligned}
& + \frac{4}{9} L_{ij22}^{V,LL} + \frac{4}{9} L_{ij11}^{V,LR} + \frac{4}{9} L_{ij22}^{V,LR} - \frac{8}{9} L_{ij11}^{V,LL} - \frac{8}{9} L_{ij11}^{V,LR} \Big] \\
& + \alpha_s^2 \left[ -8 L_{ij11}^{V,LL} - 8 L_{ij22}^{V,LL} + 8 L_{ij11}^{V,LR} + 8 L_{ij22}^{V,LR} - 8 L_{ij11}^{V,LL} \right. \\
& + 8 L_{ij11}^{V,LR} \Big] + \alpha_s \alpha \left[ \frac{16}{9} L_{ij11}^{V,LL} + \frac{16}{9} L_{ij22}^{V,LL} + \frac{16}{9} L_{ij11}^{V,LR} + \frac{16}{9} L_{ij22}^{V,LR} \right. \\
& - \frac{32}{9} L_{ij11}^{V,LL} - \frac{32}{9} L_{ij11}^{V,LR} \Big] + \alpha^2 \left[ -\frac{8}{27} L_{ij11}^{V,LL} - \frac{8}{27} L_{ij22}^{V,LL} + \frac{16}{27} L_{ij11}^{V,LR} \right. \\
& + \frac{16}{27} L_{ij22}^{V,LR} + \frac{8}{3} L_{ij11}^{V,LR} + \frac{8}{3} L_{ij22}^{V,LR} - \frac{80}{27} L_{ij11}^{V,LL} + \frac{16}{27} L_{ij11}^{V,LR} \Big] ; \\
\dot{L}_{ij22}^{V,LR} & = e^2 \left[ \frac{4}{9} L_{ij11}^{V,LL} + \frac{4}{9} L_{ij22}^{V,LL} + \frac{4}{9} L_{ij11}^{V,LR} + \frac{4}{9} L_{ij22}^{V,LR} + \frac{4}{9} L_{ij11}^{V,LL} \right. \\
& + \frac{4}{9} L_{ij22}^{V,LL} + \frac{4}{9} L_{ij11}^{V,LR} + \frac{4}{9} L_{ij22}^{V,LR} - \frac{8}{9} L_{ij11}^{V,LL} - \frac{8}{9} L_{ij11}^{V,LR} \Big] \\
& + \alpha_s^2 \left[ -8 L_{ij11}^{V,LL} - 8 L_{ij22}^{V,LL} + 8 L_{ij11}^{V,LR} + 8 L_{ij22}^{V,LR} - 8 L_{ij11}^{V,LL} \right. \\
& + 8 L_{ij11}^{V,LR} \Big] + \alpha_s \alpha \left[ \frac{16}{9} L_{ij11}^{V,LL} + \frac{16}{9} L_{ij22}^{V,LL} + \frac{16}{9} L_{ij11}^{V,LR} + \frac{16}{9} L_{ij22}^{V,LR} \right. \\
& - \frac{32}{9} L_{ij11}^{V,LL} - \frac{32}{9} L_{ij11}^{V,LR} \Big] + \alpha^2 \left[ -\frac{8}{27} L_{ij11}^{V,LL} - \frac{8}{27} L_{ij22}^{V,LL} + \frac{16}{27} L_{ij11}^{V,LR} \right. \\
& + \frac{16}{27} L_{ij22}^{V,LR} + \frac{8}{3} L_{ij11}^{V,LR} + \frac{8}{3} L_{ij22}^{V,LR} - \frac{80}{27} L_{ij11}^{V,LL} + \frac{16}{27} L_{ij11}^{V,LR} \Big] ; \\
\dot{L}_{ij11}^{V,LR} & = e^2 \left[ -\frac{8}{9} L_{ij11}^{V,LL} - \frac{8}{9} L_{ij22}^{V,LL} - \frac{8}{9} L_{ij11}^{V,LR} - \frac{8}{9} L_{ij22}^{V,LR} - \frac{8}{9} L_{ij11}^{V,LL} \right. \\
& - \frac{8}{9} L_{ij22}^{V,LL} - \frac{8}{9} L_{ij11}^{V,LR} - \frac{8}{9} L_{ij22}^{V,LR} + \frac{16}{9} L_{ij11}^{V,LL} + \frac{16}{9} L_{ij11}^{V,LR} \Big] \\
& + \alpha_s^2 \left[ -8 L_{ij11}^{V,LL} - 8 L_{ij22}^{V,LL} + 8 L_{ij11}^{V,LR} + 8 L_{ij22}^{V,LR} - 8 L_{ij11}^{V,LL} \right.
\end{aligned}$$

$$\begin{aligned}
& + 8L_{ij11}^{V,LR} \Big] + \alpha_s \alpha \Big[ -\frac{32}{9}L_{ij11}^{V,LL} - \frac{32}{9}L_{ij22}^{V,LL} - \frac{32}{9}L_{ij11}^{V,LR} - \frac{32}{9}L_{ij22}^{V,LR} \\
& + \frac{64}{9}L_{ij11}^{V,LL} + \frac{64}{9}L_{ij11}^{V,LR} \Big] + \alpha^2 \Big[ -\frac{56}{27}L_{ij11}^{V,LL} - \frac{56}{27}L_{ij22}^{V,LL} + \frac{40}{27}L_{ij11}^{V,LR} \\
& + \frac{40}{27}L_{ij22}^{V,LR} - 8L_{ij11}^{V,LL} - 8L_{ij22}^{V,LL} + \frac{8}{3}L_{ij11}^{V,LR} + \frac{8}{3}L_{ij22}^{V,LR} - \frac{128}{27}L_{ij11}^{V,LL} \\
& + \frac{256}{27}L_{ij11}^{V,LR} \Big] ;
\end{aligned}$$

$$\dot{L}_{ij11}^{S,LR} = \frac{71}{3}\alpha^2 L_{ij11}^{S,LR} - 6e^2 L_{ij11}^{S,LR} ;$$

$$\dot{L}_{ij22}^{S,LR} = \frac{71}{3}\alpha^2 L_{ij22}^{S,LR} - 6e^2 L_{ij22}^{S,LR} ;$$

$$\begin{aligned}
\dot{L}_{ij11}^{S,LR} = & -8g_s^2 L_{ij11}^{S,LR} - \frac{2}{3}e^2 L_{ij11}^{S,LR} - \frac{1052}{9}\alpha_s^2 L_{ij11}^{S,LR} - \frac{8}{9}\alpha_s \alpha L_{ij11}^{S,LR} \\
& + \frac{79}{27}\alpha^2 L_{ij11}^{S,LR} ;
\end{aligned}$$

$$\begin{aligned}
\dot{L}_{ij22}^{S,LR} = & -8g_s^2 L_{ij22}^{S,LR} - \frac{2}{3}e^2 L_{ij22}^{S,LR} - \frac{1052}{9}\alpha_s^2 L_{ij22}^{S,LR} - \frac{8}{9}\alpha_s \alpha L_{ij22}^{S,LR} \\
& + \frac{79}{27}\alpha^2 L_{ij22}^{S,LR} ;
\end{aligned}$$

$$\begin{aligned}
\dot{L}_{ij11}^{S,LR} = & -8g_s^2 L_{ij11}^{S,LR} - \frac{8}{3}e^2 L_{ij11}^{S,LR} - \frac{1052}{9}\alpha_s^2 L_{ij11}^{S,LR} - \frac{32}{9}\alpha_s \alpha L_{ij11}^{S,LR} \\
& + \frac{304}{27}\alpha^2 L_{ij11}^{S,LR} ;
\end{aligned}$$

$$\dot{L}_{ij11}^{S,LL} = \frac{71}{3}\alpha^2 L_{ij11}^{S,LL} - 6e^2 L_{ij11}^{S,LL} ;$$

$$\dot{L}_{ij11}^{T,LL} = 2e^2 L_{ij11}^{T,LL} - \frac{379}{9}\alpha^2 L_{ij11}^{T,LL} ;$$

$$\dot{L}_{ij22}^{S,LL} = \frac{71}{3}\alpha^2 L_{ij22}^{S,LL} - 6e^2 L_{ij22}^{S,LL} ;$$

$$\dot{L}_{ij22}^{T,LL} = 2e^2 L_{ij22}^{T,LL} - \frac{379}{9}\alpha^2 L_{ij22}^{T,LL} ;$$

$$\begin{aligned}
\dot{L}_{ij11}^{S,LL} = & -8g_s^2 L_{ij11}^{S,LL} - \frac{2}{3}e^2 L_{ij11}^{S,LL} - \frac{1052}{9}\alpha_s^2 L_{ij11}^{S,LL} - \frac{8}{9}\alpha_s \alpha L_{ij11}^{S,LL} \\
& + \frac{79}{27}\alpha^2 L_{ij11}^{S,LL} ;
\end{aligned}$$

$$\begin{aligned}
\dot{L}_{ij11}^{T,LL} &= \frac{8}{3}g_s^2 L_{ij11}^{T,LL} + \frac{2}{9}e^2 L_{ij11}^{T,LL} + \frac{1756}{27}\alpha_s^2 L_{ij11}^{T,LL} - \frac{152}{27}\alpha_s \alpha L_{ij11}^{T,LL} \\
&\quad - \frac{227}{81}\alpha^2 L_{ij11}^{T,LL} ; \\
\dot{L}_{ij22}^{S,LL} &= -8g_s^2 L_{ij22}^{S,LL} - \frac{2}{3}e^2 L_{ij22}^{S,LL} - \frac{1052}{9}\alpha_s^2 L_{ij22}^{S,LL} - \frac{8}{9}\alpha_s \alpha L_{ij22}^{S,LL} \\
&\quad + \frac{79}{27}\alpha^2 L_{ij22}^{S,LL} ; \\
\dot{L}_{ij22}^{T,LL} &= \frac{8}{3}g_s^2 L_{ij22}^{T,LL} + \frac{2}{9}e^2 L_{ij22}^{T,LL} + \frac{1756}{27}\alpha_s^2 L_{ij22}^{T,LL} - \frac{152}{27}\alpha_s \alpha L_{ij22}^{T,LL} \\
&\quad - \frac{227}{81}\alpha^2 L_{ij22}^{T,LL} ; \\
\dot{L}_{ij11}^{S,LL} &= -8g_s^2 L_{ij11}^{S,LL} - \frac{8}{3}e^2 L_{ij11}^{S,LL} - \frac{1052}{9}\alpha_s^2 L_{ij11}^{S,LL} - \frac{32}{9}\alpha_s \alpha L_{ij11}^{S,LL} \\
&\quad + \frac{304}{27}\alpha^2 L_{ij11}^{S,LL} ; \\
\dot{L}_{ij11}^{T,LL} &= \frac{8}{3}g_s^2 L_{ij11}^{T,LL} + \frac{8}{9}e^2 L_{ij11}^{T,LL} + \frac{1756}{27}\alpha_s^2 L_{ij11}^{T,LL} - \frac{608}{27}\alpha_s \alpha L_{ij11}^{T,LL} \\
&\quad - \frac{1136}{81}\alpha^2 L_{ij11}^{T,LL} ; \\
\dot{L}_{ijkk}^{V,LL} &= 0 ; \\
\dot{L}_{ijjj}^{V,LL} &= 0 ; \\
\dot{L}_{ijii}^{V,LL} &= 0 ; \\
\dot{L}_{ijkk}^{S,LL} &= 0 ; \\
\dot{L}_{ikkj}^{S,LL} &= 0 ; \\
\dot{L}_{ijjj}^{S,LL} &= 0 ; \\
\dot{L}_{ijii}^{S,LL} &= 0 ;
\end{aligned}$$

### 3.8 $\Delta F = 0$ Transitions ( $\bar{f}_i f_i \bar{f}_j f_j$ )

$$\dot{L}_{ijjj}^{S,RL} = -8g_s^2 L_{ijjj}^{S,RL} - \frac{20}{3}e^2 L_{ijjj}^{S,RL} - \frac{1052}{9}\alpha_s^2 L_{ijjj}^{S,RL} - \frac{8}{9}\alpha_s \alpha L_{ijjj}^{S,RL}$$

$$\begin{aligned}
& + \frac{1402}{27} \alpha^2 L_{ijj}^{S,RL,ed} ; \\
\dot{L}_{ijj}^{S,RL,eu} & = -8g_s^2 L_{ijj}^{S,RL,eu} - \frac{26}{3} e^2 L_{ijj}^{S,RL,eu} - \frac{1052}{9} \alpha_s^2 L_{ijj}^{S,RL,eu} - \frac{32}{9} \alpha_s \alpha L_{ijj}^{S,RL,eu} \\
& + \frac{223}{27} \alpha^2 L_{ijj}^{S,RL,eu} ; \\
\dot{L}_{ijj}^{S,LR,\nu e} & = -6e^2 L_{ijj}^{S,LR,\nu e} ; \\
\dot{L}_{ijj}^{S,LR,\nu d} & = -8g_s^2 L_{ijj}^{S,LR,\nu d} - \frac{2}{3} e^2 L_{ijj}^{S,LR,\nu d} - \frac{1052}{9} \alpha_s^2 L_{ijj}^{S,LR,\nu d} - \frac{8}{9} \alpha_s \alpha L_{ijj}^{S,LR,\nu d} \\
& + \frac{79}{27} \alpha^2 L_{ijj}^{S,LR,\nu d} ; \\
\dot{L}_{ijj}^{S,LR,\nu u} & = -8g_s^2 L_{ijj}^{S,LR,\nu u} - \frac{8}{3} e^2 L_{ijj}^{S,LR,\nu u} - \frac{1052}{9} \alpha_s^2 L_{ijj}^{S,LR,\nu u} - \frac{32}{9} \alpha_s \alpha L_{ijj}^{S,LR,\nu u} \\
& + \frac{304}{27} \alpha^2 L_{ijj}^{S,LR,\nu u} ; \\
\dot{L}_{ijji}^{V1,LR,uddu} & = -\frac{8}{3} g_s^2 L_{ijji}^{V8,LR,uddu} - \frac{10}{3} e^2 L_{ijji}^{V1,LR,uddu} + \alpha_s^2 \left[ -\frac{28}{3} L_{ijji}^{V1,LR,uddu} - \frac{2132}{27} L_{ijji}^{V8,LR,uddu} \right] \\
& + \alpha_s \alpha \left[ \frac{8}{3} L_{ijji}^{V1,LR,uddu} - \frac{128}{27} L_{ijji}^{V8,LR,uddu} \right] + \frac{47}{27} \alpha^2 L_{ijji}^{V1,LR,uddu} ; \\
\dot{L}_{ijji}^{V8,LR,uddu} & = g_s^2 \left[ -12 L_{ijji}^{V1,LR,uddu} - 14 L_{ijji}^{V8,LR,uddu} \right] - \frac{10}{3} e^2 L_{ijji}^{V8,LR,uddu} + \alpha_s^2 \left[ -\frac{418}{3} L_{ijji}^{V1,LR,uddu} \right. \\
& \left. - \frac{3067}{18} L_{ijji}^{V8,LR,uddu} \right] + \alpha_s \alpha \left[ \frac{16}{9} L_{ijji}^{V8,LR,uddu} - \frac{64}{3} L_{ijji}^{V1,LR,uddu} \right] + \frac{47}{27} \alpha^2 L_{ijji}^{V8,LR,uddu} ; \\
\dot{L}_{ijji}^{V1,LR,dd} & = -\frac{8}{3} g_s^2 L_{ijji}^{V8,LR,dd} - \frac{4}{3} e^2 L_{ijji}^{V1,LR,dd} + \alpha_s^2 \left[ -\frac{28}{3} L_{ijji}^{V1,LR,dd} - \frac{2132}{27} L_{ijji}^{V8,LR,dd} \right] \\
& + \alpha_s \alpha \left[ \frac{32}{3} L_{ijji}^{V1,LR,dd} - \frac{8}{27} L_{ijji}^{V8,LR,dd} \right] + \frac{362}{27} \alpha^2 L_{ijji}^{V1,LR,dd} ; \\
\dot{L}_{ijji}^{V8,LR,dd} & = g_s^2 \left[ -12 L_{ijji}^{V1,LR,dd} - 14 L_{ijji}^{V8,LR,dd} \right] - \frac{4}{3} e^2 L_{ijji}^{V8,LR,dd} + \alpha_s^2 \left[ -\frac{418}{3} L_{ijji}^{V1,LR,dd} \right. \\
& \left. - \frac{3067}{18} L_{ijji}^{V8,LR,dd} \right] + \alpha_s \alpha \left[ -\frac{4}{3} L_{ijji}^{V1,LR,dd} - \frac{26}{9} L_{ijji}^{V8,LR,dd} \right] + \frac{362}{27} \alpha^2 L_{ijji}^{V8,LR,dd} ;
\end{aligned}$$

$$\begin{aligned}
\dot{L}_{ee}^{V,LR}{}_{ijji} &= \frac{442}{3}\alpha^2 L_{ee}^{V,LR}{}_{ijji} - 12e^2 L_{ee}^{V,LR}{}_{ijji} ; \\
\dot{L}_{ed}^{S,RL}{}_{jjii} &= -8g_s^2 L_{ed}^{S,RL}{}_{jjii} - \frac{20}{3}e^2 L_{ed}^{S,RL}{}_{jjii} - \frac{1052}{9}\alpha_s^2 L_{ed}^{S,RL}{}_{jjii} - \frac{8}{9}\alpha_s \alpha L_{ed}^{S,RL}{}_{jjii} \\
&\quad + \frac{1402}{27}\alpha^2 L_{ed}^{S,RL}{}_{jjii} ; \\
\dot{L}_{eu}^{S,RL}{}_{jjii} &= -8g_s^2 L_{eu}^{S,RL}{}_{jjii} - \frac{26}{3}e^2 L_{eu}^{S,RL}{}_{jjii} - \frac{1052}{9}\alpha_s^2 L_{eu}^{S,RL}{}_{jjii} - \frac{32}{9}\alpha_s \alpha L_{eu}^{S,RL}{}_{jjii} \\
&\quad + \frac{223}{27}\alpha^2 L_{eu}^{S,RL}{}_{jjii} ; \\
\dot{L}_{\nu e}^{S,LR}{}_{jjii} &= -6e^2 L_{\nu e}^{S,LR}{}_{jjii} ; \\
\dot{L}_{\nu d}^{S,LR}{}_{jjii} &= -8g_s^2 L_{\nu d}^{S,LR}{}_{jjii} - \frac{2}{3}e^2 L_{\nu d}^{S,LR}{}_{jjii} - \frac{1052}{9}\alpha_s^2 L_{\nu d}^{S,LR}{}_{jjii} - \frac{8}{9}\alpha_s \alpha L_{\nu d}^{S,LR}{}_{jjii} \\
&\quad + \frac{79}{27}\alpha^2 L_{\nu d}^{S,LR}{}_{jjii} ; \\
\dot{L}_{\nu u}^{S,LR}{}_{jjii} &= -8g_s^2 L_{\nu u}^{S,LR}{}_{jjii} - \frac{8}{3}e^2 L_{\nu u}^{S,LR}{}_{jjii} - \frac{1052}{9}\alpha_s^2 L_{\nu u}^{S,LR}{}_{jjii} - \frac{32}{9}\alpha_s \alpha L_{\nu u}^{S,LR}{}_{jjii} \\
&\quad + \frac{304}{27}\alpha^2 L_{\nu u}^{S,LR}{}_{jjii} ; \\
\dot{L}_{uddu}^{V1,LR}{}_{jii j} &= -\frac{8}{3}g_s^2 L_{uddu}^{V8,LR}{}_{jii j} - \frac{10}{3}e^2 L_{uddu}^{V1,LR}{}_{jii j} + \alpha_s^2 \left[ -\frac{28}{3}L_{uddu}^{V1,LR}{}_{jii j} - \frac{2132}{27}L_{uddu}^{V8,LR}{}_{jii j} \right] \\
&\quad + \alpha_s \alpha \left[ \frac{8}{3}L_{uddu}^{V1,LR}{}_{jii j} - \frac{128}{27}L_{uddu}^{V8,LR}{}_{jii j} \right] + \frac{47}{27}\alpha^2 L_{uddu}^{V1,LR}{}_{jii j} ; \\
\dot{L}_{uddu}^{V8,LR}{}_{jii j} &= g_s^2 \left[ -12L_{uddu}^{V1,LR}{}_{jii j} - 14L_{uddu}^{V8,LR}{}_{jii j} \right] - \frac{10}{3}e^2 L_{uddu}^{V8,LR}{}_{jii j} + \alpha_s^2 \left[ -\frac{418}{3}L_{uddu}^{V1,LR}{}_{jii j} \right. \\
&\quad \left. - \frac{3067}{18}L_{uddu}^{V8,LR}{}_{jii j} \right] + \alpha_s \alpha \left[ \frac{16}{9}L_{uddu}^{V8,LR}{}_{jii j} - \frac{64}{3}L_{uddu}^{V1,LR}{}_{jii j} \right] + \frac{47}{27}\alpha^2 L_{uddu}^{V8,LR}{}_{jii j} ; \\
\dot{L}_{dd}^{V1,LR}{}_{jii j} &= -\frac{8}{3}g_s^2 L_{dd}^{V8,LR}{}_{jii j} - \frac{4}{3}e^2 L_{dd}^{V1,LR}{}_{jii j} + \alpha_s^2 \left[ -\frac{28}{3}L_{dd}^{V1,LR}{}_{jii j} - \frac{2132}{27}L_{dd}^{V8,LR}{}_{jii j} \right] \\
&\quad + \alpha_s \alpha \left[ \frac{32}{3}L_{dd}^{V1,LR}{}_{jii j} - \frac{8}{27}L_{dd}^{V8,LR}{}_{jii j} \right] + \frac{362}{27}\alpha^2 L_{dd}^{V1,LR}{}_{jii j} ; \\
\dot{L}_{dd}^{V8,LR}{}_{jii j} &= g_s^2 \left[ -12L_{dd}^{V1,LR}{}_{jii j} - 14L_{dd}^{V8,LR}{}_{jii j} \right] - \frac{4}{3}e^2 L_{dd}^{V8,LR}{}_{jii j} + \alpha_s^2 \left[ -\frac{418}{3}L_{dd}^{V1,LR}{}_{jii j} \right.
\end{aligned}$$

$$\begin{aligned}
& -\frac{3067}{18}L_{jj}^{V8,LR} \Big] + \alpha_s \alpha \left[ -\frac{4}{3}L_{jj}^{V1,LR} - \frac{26}{9}L_{jj}^{V8,LR} \right] + \frac{362}{27}\alpha^2 L_{jj}^{V8,LR} ; \\
\dot{L}_{jj}^{V,LR} &= \frac{442}{3}\alpha^2 L_{jj}^{V,LR} - 12e^2 L_{jj}^{V,LR} ; \\
\dot{L}_{ij}^{S,RR} &= -8g_s^2 L_{ij}^{S,RR} + e^2 \left[ -\frac{20}{3}L_{ij}^{S,RR} - 32L_{ij}^{T,RR} \right] - \frac{1052}{9}\alpha^2 L_{ij}^{S,RR} \\
&+ \alpha_s \alpha \left[ \frac{1792}{9}L_{ij}^{T,RR} - \frac{8}{9}L_{ij}^{S,RR} \right] + \alpha^2 \left[ \frac{94}{27}L_{ij}^{S,RR} + \frac{14080}{27}L_{ij}^{T,RR} \right] ; \\
\dot{L}_{ij}^{T,RR} &= \frac{8}{3}g_s^2 L_{ij}^{T,RR} + e^2 \left[ \frac{20}{9}L_{ij}^{T,RR} - \frac{2}{3}L_{ij}^{S,RR} \right] + \frac{1756}{27}\alpha^2 L_{ij}^{T,RR} \\
&+ \alpha_s \alpha \left[ \frac{16}{3}L_{ij}^{S,RR} - \frac{152}{27}L_{ij}^{T,RR} \right] + \alpha^2 \left[ \frac{112}{27}L_{ij}^{S,RR} - \frac{1766}{81}L_{ij}^{T,RR} \right] ; \\
\dot{L}_{ij}^{S,RR} &= -8g_s^2 L_{ij}^{S,RR} + e^2 \left[ 64L_{ij}^{T,RR} - \frac{26}{3}L_{ij}^{S,RR} \right] - \frac{1052}{9}\alpha^2 L_{ij}^{S,RR} \\
&+ \alpha_s \alpha \left[ -\frac{32}{9}L_{ij}^{S,RR} - \frac{3584}{9}L_{ij}^{T,RR} \right] + \alpha^2 \left[ -\frac{1553}{27}L_{ij}^{S,RR} - \frac{23936}{27}L_{ij}^{T,RR} \right] ; \\
\dot{L}_{ij}^{T,RR} &= \frac{8}{3}g_s^2 L_{ij}^{T,RR} + e^2 \left[ \frac{4}{3}L_{ij}^{S,RR} + \frac{26}{9}L_{ij}^{T,RR} \right] + \frac{1756}{27}\alpha^2 L_{ij}^{T,RR} \\
&+ \alpha_s \alpha \left[ -\frac{32}{3}L_{ij}^{S,RR} - \frac{608}{27}L_{ij}^{T,RR} \right] + \alpha^2 \left[ -\frac{440}{27}L_{ij}^{S,RR} - \frac{3971}{81}L_{ij}^{T,RR} \right] ; \\
\dot{L}_{ij}^{S,LL} &= \frac{71}{3}\alpha^2 L_{ij}^{S,LL} - 6e^2 L_{ij}^{S,LL} ; \\
\dot{L}_{ij}^{T,LL} &= 2e^2 L_{ij}^{T,LL} - \frac{379}{9}\alpha^2 L_{ij}^{T,LL} ; \\
\dot{L}_{ij}^{S,LL} &= -8g_s^2 L_{ij}^{S,LL} - \frac{2}{3}e^2 L_{ij}^{S,LL} - \frac{1052}{9}\alpha^2 L_{ij}^{S,LL} - \frac{8}{9}\alpha_s \alpha L_{ij}^{S,LL} \\
&+ \frac{79}{27}\alpha^2 L_{ij}^{S,LL} ; \\
\dot{L}_{ij}^{T,LL} &= \frac{8}{3}g_s^2 L_{ij}^{T,LL} + \frac{2}{9}e^2 L_{ij}^{T,LL} + \frac{1756}{27}\alpha^2 L_{ij}^{T,LL} - \frac{152}{27}\alpha_s \alpha L_{ij}^{T,LL} \\
&- \frac{227}{81}\alpha^2 L_{ij}^{T,LL} ;
\end{aligned}$$



$$\begin{aligned}
\dot{L}_{\nu u}^{S,LL}{}_{ijj} &= -8g_s^2 L_{\nu u}^{S,LL}{}_{ijj} - \frac{8}{3}e^2 L_{\nu u}^{S,LL}{}_{ijj} - \frac{1052}{9}\alpha_s^2 L_{\nu u}^{S,LL}{}_{ijj} - \frac{32}{9}\alpha_s\alpha L_{\nu u}^{S,LL}{}_{ijj} \\
&\quad + \frac{304}{27}\alpha^2 L_{\nu u}^{S,LL}{}_{ijj} ; \\
\dot{L}_{\nu u}^{T,LL}{}_{ijj} &= \frac{8}{3}g_s^2 L_{\nu u}^{T,LL}{}_{ijj} + \frac{8}{9}e^2 L_{\nu u}^{T,LL}{}_{ijj} + \frac{1756}{27}\alpha_s^2 L_{\nu u}^{T,LL}{}_{ijj} - \frac{608}{27}\alpha_s\alpha L_{\nu u}^{T,LL}{}_{ijj} \\
&\quad - \frac{1136}{81}\alpha^2 L_{\nu u}^{T,LL}{}_{ijj} ; \\
\dot{L}_{ud}^{S1,RR}{}_{ijj} &= g_s^2 \left[ \frac{64}{9} L_{uddu}^{S1,RR}{}_{ijji} + \frac{112}{27} L_{uddu}^{S8,RR}{}_{ijji} - 16 L_{ud}^{S1,RR}{}_{ijj} + \frac{16}{9} L_{ud}^{S8,RR}{}_{ijj} \right] \\
&\quad + e^2 \left[ \frac{4}{27} L_{uddu}^{S1,RR}{}_{ijji} + \frac{16}{81} L_{uddu}^{S8,RR}{}_{ijji} - \frac{46}{9} L_{ud}^{S1,RR}{}_{ijj} \right] + \alpha_s^2 \left[ \frac{9536}{81} L_{uddu}^{S1,RR}{}_{ijji} + \frac{16688}{243} L_{uddu}^{S8,RR}{}_{ijji} \right. \\
&\quad \left. - \frac{2200}{9} L_{ud}^{S1,RR}{}_{ijj} + \frac{944}{81} L_{ud}^{S8,RR}{}_{ijj} \right] + \alpha_s\alpha \left[ \frac{1888}{81} L_{uddu}^{S1,RR}{}_{ijji} + \frac{3808}{243} L_{uddu}^{S8,RR}{}_{ijji} + \frac{136}{27} L_{ud}^{S1,RR}{}_{ijj} \right. \\
&\quad \left. + \frac{224}{81} L_{ud}^{S8,RR}{}_{ijj} \right] + \alpha^2 \left[ \frac{2}{9} L_{uddu}^{S1,RR}{}_{ijji} + \frac{8}{27} L_{uddu}^{S8,RR}{}_{ijji} + \frac{415}{27} L_{ud}^{S1,RR}{}_{ijj} \right] ; \\
\dot{L}_{ud}^{S8,RR}{}_{ijj} &= g_s^2 \left[ -\frac{16}{3} L_{uddu}^{S1,RR}{}_{ijji} + \frac{44}{9} L_{uddu}^{S8,RR}{}_{ijji} + 8 L_{ud}^{S1,RR}{}_{ijj} + \frac{16}{3} L_{ud}^{S8,RR}{}_{ijj} \right] \\
&\quad + e^2 \left[ \frac{8}{9} L_{uddu}^{S1,RR}{}_{ijji} - \frac{4}{27} L_{uddu}^{S8,RR}{}_{ijji} - \frac{46}{9} L_{ud}^{S8,RR}{}_{ijj} \right] + \alpha_s^2 \left[ -\frac{872}{27} L_{uddu}^{S1,RR}{}_{ijji} - \frac{2462}{81} L_{uddu}^{S8,RR}{}_{ijji} \right. \\
&\quad \left. + \frac{256}{9} L_{ud}^{S1,RR}{}_{ijj} + \frac{3197}{27} L_{ud}^{S8,RR}{}_{ijj} \right] + \alpha_s\alpha \left[ -\frac{868}{27} L_{uddu}^{S1,RR}{}_{ijji} + \frac{1370}{81} L_{uddu}^{S8,RR}{}_{ijji} + \frac{112}{9} L_{ud}^{S1,RR}{}_{ijj} \right. \\
&\quad \left. + \frac{224}{9} L_{ud}^{S8,RR}{}_{ijj} \right] + \alpha^2 \left[ \frac{4}{3} L_{uddu}^{S1,RR}{}_{ijji} - \frac{2}{9} L_{uddu}^{S8,RR}{}_{ijji} + \frac{415}{27} L_{ud}^{S8,RR}{}_{ijj} \right] ; \\
\dot{L}_{uddu}^{S1,RR}{}_{ijji} &= g_s^2 \left[ -16 L_{uddu}^{S1,RR}{}_{ijji} + \frac{16}{9} L_{uddu}^{S8,RR}{}_{ijji} + \frac{64}{9} L_{ud}^{S1,RR}{}_{ijj} + \frac{112}{27} L_{ud}^{S8,RR}{}_{ijj} \right] \\
&\quad + e^2 \left[ \frac{26}{9} L_{uddu}^{S1,RR}{}_{ijji} - \frac{32}{27} L_{ud}^{S1,RR}{}_{ijj} - \frac{128}{81} L_{ud}^{S8,RR}{}_{ijj} \right] + \alpha_s^2 \left[ -\frac{2200}{9} L_{uddu}^{S1,RR}{}_{ijji} + \frac{944}{81} L_{uddu}^{S8,RR}{}_{ijji} \right. \\
&\quad \left. + \frac{9536}{81} L_{ud}^{S1,RR}{}_{ijj} + \frac{16688}{243} L_{ud}^{S8,RR}{}_{ijj} \right] + \alpha_s\alpha \left[ \frac{712}{27} L_{uddu}^{S1,RR}{}_{ijji} - \frac{64}{81} L_{uddu}^{S8,RR}{}_{ijji} - \frac{2144}{81} L_{ud}^{S1,RR}{}_{ijj} \right.
\end{aligned}$$

$$\begin{aligned}
& -\frac{7784}{243}L_{ijj}^{S8,RR} \Big] + \alpha^2 \Big[ -\frac{1025}{27}L_{ijji}^{S1,RR} + \frac{176}{27}L_{ijj}^{S1,RR} + \frac{704}{81}L_{ijj}^{S8,RR} \Big] ; \\
\dot{L}_{ijji}^{S8,RR} &= g_s^2 \Big[ 8L_{ijji}^{S1,RR} + \frac{16}{3}L_{ijji}^{S8,RR} - \frac{16}{3}L_{ijj}^{S1,RR} + \frac{44}{9}L_{ijj}^{S8,RR} \Big] \\
&+ e^2 \Big[ \frac{26}{9}L_{ijji}^{S8,RR} - \frac{64}{9}L_{ijj}^{S1,RR} + \frac{32}{27}L_{ijj}^{S8,RR} \Big] + \alpha_s^2 \Big[ \frac{256}{9}L_{ijji}^{S1,RR} + \frac{3197}{27}L_{ijji}^{S8,RR} \\
&- \frac{872}{27}L_{ijj}^{S1,RR} - \frac{2462}{81}L_{ijj}^{S8,RR} \Big] + \alpha_s \alpha \Big[ -\frac{32}{9}L_{ijji}^{S1,RR} - \frac{400}{9}L_{ijji}^{S8,RR} + \frac{3704}{27}L_{ijj}^{S1,RR} \\
&- \frac{2050}{81}L_{ijj}^{S8,RR} \Big] + \alpha^2 \Big[ -\frac{1025}{27}L_{ijji}^{S8,RR} + \frac{352}{9}L_{ijj}^{S1,RR} - \frac{176}{27}L_{ijj}^{S8,RR} \Big] ; \\
\dot{L}_{jjii}^{S,RR} &= -8g_s^2L_{jjii}^{S,RR} + e^2 \Big[ -\frac{20}{3}L_{jjii}^{S,RR} - 32L_{jjii}^{T,RR} \Big] - \frac{1052}{9}\alpha_s^2L_{jjii}^{S,RR} \\
&+ \alpha_s \alpha \Big[ \frac{1792}{9}L_{jjii}^{T,RR} - \frac{8}{9}L_{jjii}^{S,RR} \Big] + \alpha^2 \Big[ \frac{94}{27}L_{jjii}^{S,RR} + \frac{14080}{27}L_{jjii}^{T,RR} \Big] ; \\
\dot{L}_{jjii}^{T,RR} &= \frac{8}{3}g_s^2L_{jjii}^{T,RR} + e^2 \Big[ \frac{20}{9}L_{jjii}^{T,RR} - \frac{2}{3}L_{jjii}^{S,RR} \Big] + \frac{1756}{27}\alpha_s^2L_{jjii}^{T,RR} \\
&+ \alpha_s \alpha \Big[ \frac{16}{3}L_{jjii}^{S,RR} - \frac{152}{27}L_{jjii}^{T,RR} \Big] + \alpha^2 \Big[ \frac{112}{27}L_{jjii}^{S,RR} - \frac{1766}{81}L_{jjii}^{T,RR} \Big] ; \\
\dot{L}_{jjii}^{S,RR} &= -8g_s^2L_{jjii}^{S,RR} + e^2 \Big[ 64L_{jjii}^{T,RR} - \frac{26}{3}L_{jjii}^{S,RR} \Big] - \frac{1052}{9}\alpha_s^2L_{jjii}^{S,RR} \\
&+ \alpha_s \alpha \Big[ -\frac{32}{9}L_{jjii}^{S,RR} - \frac{3584}{9}L_{jjii}^{T,RR} \Big] + \alpha^2 \Big[ -\frac{1553}{27}L_{jjii}^{S,RR} - \frac{23936}{27}L_{jjii}^{T,RR} \Big] ; \\
\dot{L}_{jjii}^{T,RR} &= \frac{8}{3}g_s^2L_{jjii}^{T,RR} + e^2 \Big[ \frac{4}{3}L_{jjii}^{S,RR} + \frac{26}{9}L_{jjii}^{T,RR} \Big] + \frac{1756}{27}\alpha_s^2L_{jjii}^{T,RR} \\
&+ \alpha_s \alpha \Big[ -\frac{32}{3}L_{jjii}^{S,RR} - \frac{608}{27}L_{jjii}^{T,RR} \Big] + \alpha^2 \Big[ -\frac{440}{27}L_{jjii}^{S,RR} - \frac{3971}{81}L_{jjii}^{T,RR} \Big] ; \\
\dot{L}_{jjii}^{S,LL} &= \frac{71}{3}\alpha^2L_{jjii}^{S,LL} - 6e^2L_{jjii}^{S,LL} ; \\
\dot{L}_{jjii}^{T,LL} &= 2e^2L_{jjii}^{T,LL} - \frac{379}{9}\alpha^2L_{jjii}^{T,LL} ;
\end{aligned}$$

$$\begin{aligned}\dot{L}_{\nu d}^{S,LL} &= -8g_s^2 L_{\nu d}^{S,LL} - \frac{2}{3}e^2 L_{\nu d}^{S,LL} - \frac{1052}{9}\alpha_s^2 L_{\nu d}^{S,LL} - \frac{8}{9}\alpha_s\alpha L_{\nu d}^{S,LL} \\ &\quad + \frac{79}{27}\alpha^2 L_{\nu d}^{S,LL};\end{aligned}$$

$$\begin{aligned}\dot{L}_{\nu d}^{T,LL} &= \frac{8}{3}g_s^2 L_{\nu d}^{T,LL} + \frac{2}{9}e^2 L_{\nu d}^{T,LL} + \frac{1756}{27}\alpha_s^2 L_{\nu d}^{T,LL} - \frac{152}{27}\alpha_s\alpha L_{\nu d}^{T,LL} \\ &\quad - \frac{227}{81}\alpha^2 L_{\nu d}^{T,LL};\end{aligned}$$

$$\begin{aligned}\dot{L}_{\nu u}^{S,LL} &= -8g_s^2 L_{\nu u}^{S,LL} - \frac{8}{3}e^2 L_{\nu u}^{S,LL} - \frac{1052}{9}\alpha_s^2 L_{\nu u}^{S,LL} - \frac{32}{9}\alpha_s\alpha L_{\nu u}^{S,LL} \\ &\quad + \frac{304}{27}\alpha^2 L_{\nu u}^{S,LL};\end{aligned}$$

$$\begin{aligned}\dot{L}_{\nu u}^{T,LL} &= \frac{8}{3}g_s^2 L_{\nu u}^{T,LL} + \frac{8}{9}e^2 L_{\nu u}^{T,LL} + \frac{1756}{27}\alpha_s^2 L_{\nu u}^{T,LL} - \frac{608}{27}\alpha_s\alpha L_{\nu u}^{T,LL} \\ &\quad - \frac{1136}{81}\alpha^2 L_{\nu u}^{T,LL};\end{aligned}$$

$$\begin{aligned}\dot{L}_{ud}^{S1,RR} &= g_s^2 \left[ \frac{64}{9} L_{uddu}^{S1,RR} + \frac{112}{27} L_{uudj}^{S8,RR} - 16 L_{ud}^{S1,RR} + \frac{16}{9} L_{ud}^{S8,RR} \right] \\ &\quad + e^2 \left[ \frac{4}{27} L_{uddu}^{S1,RR} + \frac{16}{81} L_{uudj}^{S8,RR} - \frac{46}{9} L_{ud}^{S1,RR} \right] + \alpha_s^2 \left[ \frac{9536}{81} L_{uddu}^{S1,RR} + \frac{16688}{243} L_{uudj}^{S8,RR} \right. \\ &\quad \left. - \frac{2200}{9} L_{ud}^{S1,RR} + \frac{944}{81} L_{ud}^{S8,RR} \right] + \alpha_s\alpha \left[ \frac{1888}{81} L_{uddu}^{S1,RR} + \frac{3808}{243} L_{uudj}^{S8,RR} + \frac{136}{27} L_{ud}^{S1,RR} \right. \\ &\quad \left. + \frac{224}{81} L_{ud}^{S8,RR} \right] + \alpha^2 \left[ \frac{2}{9} L_{uddu}^{S1,RR} + \frac{8}{27} L_{uudj}^{S8,RR} + \frac{415}{27} L_{ud}^{S1,RR} \right];\end{aligned}$$

$$\begin{aligned}\dot{L}_{ud}^{S8,RR} &= g_s^2 \left[ -\frac{16}{3} L_{uddu}^{S1,RR} + \frac{44}{9} L_{uudj}^{S8,RR} + 8 L_{ud}^{S1,RR} + \frac{16}{3} L_{ud}^{S8,RR} \right] \\ &\quad + e^2 \left[ \frac{8}{9} L_{uddu}^{S1,RR} - \frac{4}{27} L_{uudj}^{S8,RR} - \frac{46}{9} L_{ud}^{S8,RR} \right] + \alpha_s^2 \left[ -\frac{872}{27} L_{uddu}^{S1,RR} - \frac{2462}{81} L_{uudj}^{S8,RR} \right. \\ &\quad \left. + \frac{256}{9} L_{ud}^{S1,RR} + \frac{3197}{27} L_{ud}^{S8,RR} \right] + \alpha_s\alpha \left[ -\frac{868}{27} L_{uddu}^{S1,RR} + \frac{1370}{81} L_{uudj}^{S8,RR} + \frac{112}{9} L_{ud}^{S1,RR} \right. \\ &\quad \left. + \frac{224}{9} L_{ud}^{S8,RR} \right] + \alpha^2 \left[ \frac{4}{3} L_{uddu}^{S1,RR} - \frac{2}{9} L_{uudj}^{S8,RR} + \frac{415}{27} L_{ud}^{S8,RR} \right];\end{aligned}$$

$$\begin{aligned}
\dot{L}_{uddu}^{S1,RR} = & g_s^2 \left[ -16L_{uddu}^{S1,RR} + \frac{16}{9}L_{uddu}^{S8,RR} + \frac{64}{9}L_{ud}^{S1,RR} + \frac{112}{27}L_{ud}^{S8,RR} \right] \\
& + e^2 \left[ \frac{26}{9}L_{uddu}^{S1,RR} - \frac{32}{27}L_{ud}^{S1,RR} - \frac{128}{81}L_{ud}^{S8,RR} \right] + \alpha_s^2 \left[ -\frac{2200}{9}L_{uddu}^{S1,RR} + \frac{944}{81}L_{uddu}^{S8,RR} \right. \\
& + \frac{9536}{81}L_{ud}^{S1,RR} + \frac{16688}{243}L_{ud}^{S8,RR} \left. \right] + \alpha_s \alpha \left[ \frac{712}{27}L_{uddu}^{S1,RR} - \frac{64}{81}L_{uddu}^{S8,RR} - \frac{2144}{81}L_{ud}^{S1,RR} \right. \\
& \left. - \frac{7784}{243}L_{ud}^{S8,RR} \right] + \alpha^2 \left[ -\frac{1025}{27}L_{uddu}^{S1,RR} + \frac{176}{27}L_{ud}^{S1,RR} + \frac{704}{81}L_{ud}^{S8,RR} \right];
\end{aligned}$$

$$\begin{aligned}
\dot{L}_{jii}^{S8,RR} = & g_s^2 \left[ 8L_{uddu}^{S1,RR} + \frac{16}{3}L_{uddu}^{S8,RR} - \frac{16}{3}L_{ud}^{S1,RR} + \frac{44}{9}L_{ud}^{S8,RR} \right] \\
& + e^2 \left[ \frac{26}{9}L_{uddu}^{S8,RR} - \frac{64}{9}L_{ud}^{S1,RR} + \frac{32}{27}L_{ud}^{S8,RR} \right] + \alpha_s^2 \left[ \frac{256}{9}L_{uddu}^{S1,RR} + \frac{3197}{27}L_{uddu}^{S8,RR} \right. \\
& \left. - \frac{872}{27}L_{ud}^{S1,RR} - \frac{2462}{81}L_{ud}^{S8,RR} \right] + \alpha_s \alpha \left[ -\frac{32}{9}L_{uddu}^{S1,RR} - \frac{400}{9}L_{uddu}^{S8,RR} + \frac{3704}{27}L_{ud}^{S1,RR} \right. \\
& \left. - \frac{2050}{81}L_{ud}^{S8,RR} \right] + \alpha^2 \left[ -\frac{1025}{27}L_{uddu}^{S8,RR} + \frac{352}{9}L_{ud}^{S1,RR} - \frac{176}{27}L_{ud}^{S8,RR} \right];
\end{aligned}$$

$$\begin{aligned}
\dot{L}_{iij}^{S1,RR} = & g_s^2 \left[ -16L_{dd}^{S1,RR} + \frac{64}{9}L_{dd}^{S1,RR} + \frac{16}{9}L_{dd}^{S8,RR} + \frac{112}{27}L_{dd}^{S8,RR} \right] \\
& + e^2 \left[ -\frac{4}{9}L_{dd}^{S1,RR} + \frac{16}{27}L_{dd}^{S1,RR} + \frac{64}{81}L_{dd}^{S8,RR} \right] + \alpha_s^2 \left[ -\frac{2200}{9}L_{dd}^{S1,RR} + \frac{9536}{81}L_{dd}^{S1,RR} \right. \\
& + \frac{944}{81}L_{dd}^{S8,RR} + \frac{16688}{243}L_{dd}^{S8,RR} \left. \right] + \alpha_s \alpha \left[ -\frac{176}{27}L_{dd}^{S1,RR} - \frac{512}{81}L_{dd}^{S1,RR} - \frac{256}{81}L_{dd}^{S8,RR} \right. \\
& \left. + \frac{1120}{243}L_{dd}^{S8,RR} \right] + \alpha^2 \left[ \frac{110}{27}L_{dd}^{S1,RR} - \frac{64}{81}L_{dd}^{S1,RR} - \frac{256}{243}L_{dd}^{S8,RR} \right];
\end{aligned}$$

$$\begin{aligned}
\dot{L}_{iij}^{S8,RR} = & g_s^2 \left[ 8L_{dd}^{S1,RR} - \frac{16}{3}L_{dd}^{S1,RR} + \frac{16}{3}L_{dd}^{S8,RR} + \frac{44}{9}L_{dd}^{S8,RR} \right] + e^2 \left[ \frac{32}{9}L_{dd}^{S1,RR} \right. \\
& \left. - \frac{4}{9}L_{dd}^{S8,RR} - \frac{16}{27}L_{dd}^{S8,RR} \right] + \alpha_s^2 \left[ \frac{256}{9}L_{dd}^{S1,RR} - \frac{872}{27}L_{dd}^{S1,RR} + \frac{3197}{27}L_{dd}^{S8,RR} \right.
\end{aligned}$$

$$\begin{aligned}
& -\frac{2462}{81}L_{ijji}^{S8,RR} \Big] + \alpha_s \alpha \Big[ -\frac{128}{9}L_{ijj}^{S1,RR} - \frac{1456}{27}L_{ijji}^{S1,RR} - \frac{16}{9}L_{ijj}^{S8,RR} - \frac{64}{81}L_{ijji}^{S8,RR} \Big] \\
& + \alpha^2 \Big[ -\frac{128}{27}L_{ijji}^{S1,RR} + \frac{110}{27}L_{ijj}^{S8,RR} + \frac{64}{81}L_{ijji}^{S8,RR} \Big] ; \\
\dot{L}_{ijji}^{S1,RR} & = g_s^2 \Big[ \frac{64}{9}L_{ijj}^{S1,RR} - 16L_{ijji}^{S1,RR} + \frac{112}{27}L_{ijj}^{S8,RR} + \frac{16}{9}L_{ijji}^{S8,RR} \Big] \\
& + e^2 \Big[ \frac{16}{27}L_{ijj}^{S1,RR} - \frac{4}{9}L_{ijji}^{S1,RR} + \frac{64}{81}L_{ijj}^{S8,RR} \Big] + \alpha_s^2 \Big[ \frac{9536}{81}L_{ijj}^{S1,RR} - \frac{2200}{9}L_{ijji}^{S1,RR} \\
& + \frac{16688}{243}L_{ijj}^{S8,RR} + \frac{944}{81}L_{ijji}^{S8,RR} \Big] + \alpha_s \alpha \Big[ -\frac{512}{81}L_{ijj}^{S1,RR} - \frac{176}{27}L_{ijji}^{S1,RR} + \frac{1120}{243}L_{ijj}^{S8,RR} \\
& - \frac{256}{81}L_{ijji}^{S8,RR} \Big] + \alpha^2 \Big[ -\frac{64}{81}L_{ijj}^{S1,RR} + \frac{110}{27}L_{ijji}^{S1,RR} - \frac{256}{243}L_{ijj}^{S8,RR} \Big] ; \\
\dot{L}_{ijji}^{S8,RR} & = g_s^2 \Big[ -\frac{16}{3}L_{ijj}^{S1,RR} + 8L_{ijji}^{S1,RR} + \frac{44}{9}L_{ijj}^{S8,RR} + \frac{16}{3}L_{ijji}^{S8,RR} \Big] \\
& + e^2 \Big[ \frac{32}{9}L_{ijj}^{S1,RR} - \frac{16}{27}L_{ijj}^{S8,RR} - \frac{4}{9}L_{ijji}^{S8,RR} \Big] + \alpha_s^2 \Big[ -\frac{872}{27}L_{ijj}^{S1,RR} + \frac{256}{9}L_{ijji}^{S1,RR} \\
& - \frac{2462}{81}L_{ijj}^{S8,RR} + \frac{3197}{27}L_{ijji}^{S8,RR} \Big] + \alpha_s \alpha \Big[ -\frac{1456}{27}L_{ijj}^{S1,RR} - \frac{128}{9}L_{ijji}^{S1,RR} - \frac{64}{81}L_{ijj}^{S8,RR} \\
& - \frac{16}{9}L_{ijji}^{S8,RR} \Big] + \alpha^2 \Big[ -\frac{128}{27}L_{ijj}^{S1,RR} + \frac{64}{81}L_{ijj}^{S8,RR} + \frac{110}{27}L_{ijji}^{S8,RR} \Big] ; \\
\dot{L}_{iii}^{S1,RR} & = g_s^2 \Big[ \frac{160}{27}L_{iii}^{S8,RR} - \frac{80}{9}L_{iii}^{S1,RR} \Big] + e^2 \Big[ \frac{4}{27}L_{iii}^{S1,RR} + \frac{64}{81}L_{iii}^{S8,RR} \Big] \\
& + \alpha_s^2 \Big[ \frac{19520}{243}L_{iii}^{S8,RR} - \frac{10264}{81}L_{iii}^{S1,RR} \Big] + \alpha_s \alpha \Big[ \frac{352}{243}L_{iii}^{S8,RR} - \frac{1040}{81}L_{iii}^{S1,RR} \Big] \\
& + \alpha^2 \Big[ \frac{266}{81}L_{iii}^{S1,RR} - \frac{256}{243}L_{iii}^{S8,RR} \Big] ; \\
\dot{L}_{iii}^{S8,RR} & = g_s^2 \Big[ \frac{8}{3}L_{iii}^{S1,RR} + \frac{92}{9}L_{iii}^{S8,RR} \Big] + e^2 \Big[ \frac{32}{9}L_{iii}^{S1,RR} - \frac{28}{27}L_{iii}^{S8,RR} \Big]
\end{aligned}$$

$$\begin{aligned}
& + \alpha_s^2 \left[ \frac{7129}{81} L_{\bar{d}\bar{d}}^{S8,RR} - \frac{104}{27} L_{\bar{d}\bar{d}}^{S1,RR} \right] + \alpha_s \alpha \left[ -\frac{1840}{27} L_{\bar{d}\bar{d}}^{S1,RR} - \frac{208}{81} L_{\bar{d}\bar{d}}^{S8,RR} \right] \\
& + \alpha^2 \left[ \frac{394}{81} L_{\bar{d}\bar{d}}^{S8,RR} - \frac{128}{27} L_{\bar{d}\bar{d}}^{S1,RR} \right] ; \\
\dot{L}_{\bar{u}\bar{u}}^{S1,RR} &= g_s^2 \left[ \frac{160}{27} L_{\bar{u}\bar{u}}^{S8,RR} - \frac{80}{9} L_{\bar{u}\bar{u}}^{S1,RR} \right] + e^2 \left[ \frac{16}{27} L_{\bar{u}\bar{u}}^{S1,RR} + \frac{256}{81} L_{\bar{u}\bar{u}}^{S8,RR} \right] \\
& + \alpha_s^2 \left[ \frac{19520}{243} L_{\bar{u}\bar{u}}^{S8,RR} - \frac{10264}{81} L_{\bar{u}\bar{u}}^{S1,RR} \right] + \alpha_s \alpha \left[ \frac{1408}{243} L_{\bar{u}\bar{u}}^{S8,RR} - \frac{4160}{81} L_{\bar{u}\bar{u}}^{S1,RR} \right] \\
& + \alpha^2 \left[ -\frac{224}{81} L_{\bar{u}\bar{u}}^{S1,RR} - \frac{2048}{243} L_{\bar{u}\bar{u}}^{S8,RR} \right] ; \\
\dot{L}_{\bar{u}\bar{u}}^{S8,RR} &= g_s^2 \left[ \frac{8}{3} L_{\bar{u}\bar{u}}^{S1,RR} + \frac{92}{9} L_{\bar{u}\bar{u}}^{S8,RR} \right] + e^2 \left[ \frac{128}{9} L_{\bar{u}\bar{u}}^{S1,RR} - \frac{112}{27} L_{\bar{u}\bar{u}}^{S8,RR} \right] \\
& + \alpha_s^2 \left[ \frac{7129}{81} L_{\bar{u}\bar{u}}^{S8,RR} - \frac{104}{27} L_{\bar{u}\bar{u}}^{S1,RR} \right] + \alpha_s \alpha \left[ -\frac{7360}{27} L_{\bar{u}\bar{u}}^{S1,RR} - \frac{832}{81} L_{\bar{u}\bar{u}}^{S8,RR} \right] \\
& + \alpha^2 \left[ \frac{800}{81} L_{\bar{u}\bar{u}}^{S8,RR} - \frac{1024}{27} L_{\bar{u}\bar{u}}^{S1,RR} \right] ; \\
\dot{L}_{\bar{e}\bar{e}}^{S,RR} &= e^2 \left[ 16 L_{\bar{e}\bar{e}}^{S,RR} - 4 L_{\bar{e}\bar{e}}^{S,RR} \right] - \frac{2086}{9} \alpha^2 L_{\bar{e}\bar{e}}^{S,RR} ; \\
\dot{L}_{\bar{e}\bar{e}}^{S,RR} &= e^2 \left[ 16 L_{\bar{e}\bar{e}}^{S,RR} - 4 L_{\bar{e}\bar{e}}^{S,RR} \right] + \frac{128}{3} \alpha^2 L_{\bar{e}\bar{e}}^{S,RR} ; \\
\dot{L}_{\bar{e}\bar{e}}^{S,RR} &= 12 e^2 L_{\bar{e}\bar{e}}^{S,RR} - \frac{851}{9} \alpha^2 L_{\bar{e}\bar{e}}^{S,RR} ; \\
\dot{L}_{\bar{\nu}\bar{\nu}}^{S,LL} &= 0 ; \\
\dot{L}_{\bar{\nu}\bar{\nu}}^{S,LL} &= 0 ; \\
\dot{L}_{\bar{\nu}\bar{\nu}}^{S,LL} &= 0 ;
\end{aligned}$$

$$\begin{aligned}
\dot{L}_{ijj}^{V,LL} = & e^2 \left[ 4L_{ijj}^{V,LL} + \frac{16}{9}L_{ijj}^{V,LL} + \frac{4}{9}L_{ijj}^{V,LR} + \frac{4}{9}L_{ii1}^{V,LL} + \frac{4}{9}L_{ii2}^{V,LL} \right. \\
& + \frac{4}{9}L_{ii1}^{V,LR} + \frac{4}{9}L_{ii2}^{V,LR} + \frac{16}{9}L_{iii}^{V,LL} + \frac{4}{9}L_{iii}^{V,LR} - \frac{8}{9}L_{ii1}^{V,LL} - \frac{8}{9}L_{ii1}^{V,LR} \\
& + \frac{8}{3}L_{jjj}^{V1,LR} + \frac{64}{9}L_{jjj}^{V,LL} + \frac{4}{3}L_{jj1}^{V,LR} + \frac{4}{3}L_{jj2}^{V,LR} - \frac{8}{3}L_{jj1}^{V1,LR} + \frac{4}{3}L_{11jj}^{V,LL} \\
& \left. + \frac{4}{3}L_{22jj}^{V,LL} - \frac{8}{3}L_{11jj}^{V1,LL} \right] + \alpha_s^2 \left[ 8L_{ii1}^{V,LL} + 8L_{ii2}^{V,LL} - 8L_{ii1}^{V,LR} \right. \\
& - 8L_{ii2}^{V,LR} + 8L_{ii1}^{V,LL} - 8L_{ii1}^{V,LR} \left. \right] + \alpha_s \alpha \left[ -16L_{ijj}^{V,LL} + \frac{16}{9}L_{ii1}^{V,LL} \right. \\
& + \frac{16}{9}L_{ii2}^{V,LL} + \frac{16}{9}L_{ii1}^{V,LR} + \frac{16}{9}L_{ii2}^{V,LR} - \frac{32}{9}L_{ii1}^{V,LL} - \frac{32}{9}L_{ii1}^{V,LR} + \frac{32}{3}L_{jjj}^{V1,LR} \\
& - \frac{2044}{243}L_{jjj}^{V8,LR} + \frac{5152}{243}L_{jjj}^{V,LL} - \frac{32}{3}L_{jj1}^{V1,LR} + \frac{1354}{243}L_{jj1}^{V8,LR} - \frac{32}{3}L_{11jj}^{V1,LL} \\
& - \frac{86}{243}L_{11jj}^{V8,LL} \left. \right] + \alpha^2 \left[ -\frac{130}{9}L_{ijj}^{V,LL} + \frac{224}{81}L_{ijj}^{V,LL} - \frac{520}{81}L_{ijj}^{V,LR} - \frac{104}{243}L_{ii1}^{V,LL} \right. \\
& - \frac{104}{243}L_{ii2}^{V,LL} - \frac{200}{243}L_{ii1}^{V,LR} - \frac{200}{243}L_{ii2}^{V,LR} + \frac{32}{81}L_{iii}^{V,LL} - \frac{520}{81}L_{iii}^{V,LR} - \frac{1016}{243}L_{ii1}^{V,LL} \\
& - \frac{1400}{243}L_{ii1}^{V,LR} - \frac{2624}{243}L_{jjj}^{V1,LR} + \frac{23296}{729}L_{jjj}^{V,LL} - \frac{3184}{243}L_{jj1}^{V,LR} - \frac{3184}{243}L_{jj2}^{V,LR} \\
& \left. - \frac{6232}{243}L_{jj1}^{V1,LR} + \frac{3728}{243}L_{11jj}^{V,LL} + \frac{3728}{243}L_{22jj}^{V,LL} + \frac{2984}{243}L_{11jj}^{V1,LL} \right];
\end{aligned}$$

$$\begin{aligned}
\dot{L}_{ijj}^{V,LL} = & e^2 \left[ -\frac{32}{9}L_{ijj}^{V,LL} - \frac{8}{9}L_{ijj}^{V,LR} - 8L_{ijj}^{V,LL} - \frac{8}{9}L_{ii1}^{V,LL} - \frac{8}{9}L_{ii2}^{V,LL} \right. \\
& - \frac{8}{9}L_{ii1}^{V,LR} - \frac{8}{9}L_{ii2}^{V,LR} - \frac{32}{9}L_{iii}^{V,LL} - \frac{8}{9}L_{iii}^{V,LR} + \frac{16}{9}L_{ii1}^{V,LL} + \frac{16}{9}L_{ii1}^{V,LR} \\
& + \frac{4}{3}L_{11jj}^{V,LL} + \frac{4}{3}L_{22jj}^{V,LL} + \frac{4}{3}L_{jj1}^{V1,LL} + \frac{4}{3}L_{jj2}^{V1,LL} + \frac{4}{3}L_{jj1}^{V1,LR} + \frac{4}{3}L_{jj2}^{V1,LR} \\
& \left. + \frac{4}{3}L_{jj1}^{V,LR} + \frac{4}{3}L_{jj2}^{V,LR} - \frac{8}{3}L_{jjj}^{V1,LR} - \frac{64}{9}L_{jjj}^{V,LL} \right] + \alpha_s^2 \left[ 8L_{ii1}^{V,LL} \right. \\
& \left. + 8L_{ii2}^{V,LL} - 8L_{ii1}^{V,LR} - 8L_{ii2}^{V,LR} + 8L_{ii1}^{V,LL} - 8L_{ii1}^{V,LR} \right] + \alpha_s \alpha \left[ 32L_{ii1}^{V,LL} \right.
\end{aligned}$$

$$\begin{aligned}
& -\frac{32}{9}L_{ed\ i11}^{V,LL} - \frac{32}{9}L_{ed\ i22}^{V,LL} - \frac{32}{9}L_{ed\ i11}^{V,LR} - \frac{32}{9}L_{ed\ i22}^{V,LR} + \frac{64}{9}L_{eu\ i11}^{V,LL} + \frac{64}{9}L_{eu\ i11}^{V,LR} \\
& + \frac{16}{3}L_{ud\ jj11}^{V1,LL} + \frac{16}{3}L_{ud\ jj22}^{V1,LL} + \frac{16}{3}L_{ud\ jj11}^{V1,LR} - \frac{32}{3}L_{ud\ jj22}^{V1,LR} + \frac{352}{243}L_{ud\ jj11}^{V8,LL} + \frac{352}{243}L_{ud\ jj22}^{V8,LL} \\
& - \frac{368}{243}L_{ud\ jj11}^{V8,LR} + \frac{2008}{243}L_{ud\ jj22}^{V8,LR} - \frac{32}{3}L_{uu\ jjjj}^{V1,LR} + \frac{2008}{243}L_{uu\ jjjj}^{V8,LR} - \frac{2144}{81}L_{uu\ jjjj}^{V,LL} \Big] \\
& + \alpha^2 \Big[ \frac{2432}{81}L_{ee\ ij\ j}^{V,LL} + \frac{464}{81}L_{ee\ ij\ j}^{V,LR} + \frac{80}{9}L_{eu\ ij\ j}^{V,LL} + \frac{2512}{243}L_{ed\ i11}^{V,LL} + \frac{2512}{243}L_{ed\ i22}^{V,LL} \\
& + \frac{1408}{243}L_{ed\ i11}^{V,LR} + \frac{1408}{243}L_{ed\ i22}^{V,LR} + \frac{3680}{81}L_{ee\ iii}^{V,LL} + \frac{464}{81}L_{ee\ iii}^{V,LR} + \frac{1312}{243}L_{eu\ i11}^{V,LL} \\
& - \frac{3104}{243}L_{eu\ i11}^{V,LR} + \frac{3248}{243}L_{eu\ 11\ jj}^{V,LL} + \frac{3248}{243}L_{eu\ 22\ jj}^{V,LL} + \frac{296}{243}L_{ud\ jj11}^{V1,LL} + \frac{296}{243}L_{ud\ jj22}^{V1,LL} \\
& - \frac{928}{243}L_{ud\ jj11}^{V1,LR} + \frac{416}{243}L_{ud\ jj22}^{V1,LR} - \frac{424}{243}L_{ue\ jj11}^{V,LR} - \frac{424}{243}L_{ue\ jj22}^{V,LR} + \frac{128}{243}L_{uu\ jjjj}^{V1,LR} \\
& + \frac{26272}{243}L_{uu\ jjjj}^{V,LL} \Big] ;
\end{aligned}$$

$$\begin{aligned}
\dot{L}_{\nu_e\ ij\ j}^{V,LL} & = e^2 \Big[ \frac{4}{3}L_{\nu d\ i11}^{V,LL} + \frac{4}{3}L_{\nu d\ i22}^{V,LL} + \frac{4}{3}L_{\nu d\ i11}^{V,LR} + \frac{4}{3}L_{\nu d\ i22}^{V,LR} + \frac{4}{3}L_{\nu e\ i11}^{V,LL} \\
& + \frac{4}{3}L_{\nu e\ i22}^{V,LL} + \frac{4}{3}L_{\nu e\ i11}^{V,LR} + \frac{4}{3}L_{\nu e\ i22}^{V,LR} - \frac{8}{3}L_{\nu u\ i11}^{V,LL} - \frac{8}{3}L_{\nu u\ i11}^{V,LR} \Big] \\
& + \alpha_s \alpha \Big[ \frac{16}{3}L_{\nu d\ i11}^{V,LL} + \frac{16}{3}L_{\nu d\ i22}^{V,LL} + \frac{16}{3}L_{\nu d\ i11}^{V,LR} + \frac{16}{3}L_{\nu d\ i22}^{V,LR} - \frac{32}{3}L_{\nu u\ i11}^{V,LL} \\
& - \frac{32}{3}L_{\nu u\ i11}^{V,LR} \Big] + \alpha^2 \Big[ \frac{40}{9}L_{\nu d\ i11}^{V,LL} + \frac{40}{9}L_{\nu d\ i22}^{V,LL} - \frac{32}{9}L_{\nu d\ i11}^{V,LR} - \frac{32}{9}L_{\nu d\ i22}^{V,LR} \\
& + 16L_{\nu e\ i11}^{V,LL} + 16L_{\nu e\ i22}^{V,LL} - 8L_{\nu e\ i11}^{V,LR} - 8L_{\nu e\ i22}^{V,LR} + \frac{112}{9}L_{\nu u\ i11}^{V,LL} - \frac{176}{9}L_{\nu u\ i11}^{V,LR} \Big] ;
\end{aligned}$$

$$\begin{aligned}
\dot{L}_{\nu d\ ij\ j}^{V,LL} & = e^2 \Big[ \frac{4}{9}L_{\nu d\ i11}^{V,LL} + \frac{4}{9}L_{\nu d\ i22}^{V,LL} + \frac{4}{9}L_{\nu d\ i11}^{V,LR} + \frac{4}{9}L_{\nu d\ i22}^{V,LR} + \frac{4}{9}L_{\nu e\ i11}^{V,LL} \\
& + \frac{4}{9}L_{\nu e\ i22}^{V,LL} + \frac{4}{9}L_{\nu e\ i11}^{V,LR} + \frac{4}{9}L_{\nu e\ i22}^{V,LR} - \frac{8}{9}L_{\nu u\ i11}^{V,LL} - \frac{8}{9}L_{\nu u\ i11}^{V,LR} \Big]
\end{aligned}$$



$$\begin{aligned}
& + \alpha_s^2 \left[ 8L_{\nu d, ii11}^{V,LL} + 8L_{\nu d, ii22}^{V,LL} - 8L_{\nu d, ii11}^{V,LR} - 8L_{\nu d, ii22}^{V,LR} + 8L_{\nu u, ii11}^{V,LL} \right. \\
& \left. - 8L_{\nu u, ii11}^{V,LR} \right] + \alpha_s \alpha \left[ \frac{16}{9} L_{\nu d, ii11}^{V,LL} + \frac{16}{9} L_{\nu d, ii22}^{V,LL} + \frac{16}{9} L_{\nu d, ii11}^{V,LR} + \frac{16}{9} L_{\nu d, ii22}^{V,LR} \right. \\
& \left. - \frac{32}{9} L_{\nu u, ii11}^{V,LL} - \frac{32}{9} L_{\nu u, ii11}^{V,LR} \right] + \alpha^2 \left[ \frac{16}{27} L_{\nu d, ii11}^{V,LL} + \frac{16}{27} L_{\nu d, ii22}^{V,LL} - \frac{8}{27} L_{\nu d, ii11}^{V,LR} \right. \\
& \left. - \frac{8}{27} L_{\nu d, ii22}^{V,LR} + \frac{8}{3} L_{\nu e, ii11}^{V,LL} + \frac{8}{3} L_{\nu e, ii22}^{V,LL} + \frac{16}{27} L_{\nu u, ii11}^{V,LL} - \frac{80}{27} L_{\nu u, ii11}^{V,LR} \right]; \\
\dot{L}_{\nu u, ij\bar{j}}^{V,LL} & = e^2 \left[ -\frac{8}{9} L_{\nu d, ii11}^{V,LL} - \frac{8}{9} L_{\nu d, ii22}^{V,LL} - \frac{8}{9} L_{\nu d, ii11}^{V,LR} - \frac{8}{9} L_{\nu d, ii22}^{V,LR} - \frac{8}{9} L_{\nu e, ii11}^{V,LL} \right. \\
& \left. - \frac{8}{9} L_{\nu e, ii22}^{V,LL} - \frac{8}{9} L_{\nu e, ii11}^{V,LR} - \frac{8}{9} L_{\nu e, ii22}^{V,LR} + \frac{16}{9} L_{\nu u, ii11}^{V,LL} + \frac{16}{9} L_{\nu u, ii11}^{V,LR} \right] \\
& + \alpha_s^2 \left[ 8L_{\nu d, ii11}^{V,LL} + 8L_{\nu d, ii22}^{V,LL} - 8L_{\nu d, ii11}^{V,LR} - 8L_{\nu d, ii22}^{V,LR} + 8L_{\nu u, ii11}^{V,LL} \right. \\
& \left. - 8L_{\nu u, ii11}^{V,LR} \right] + \alpha_s \alpha \left[ -\frac{32}{9} L_{\nu d, ii11}^{V,LL} - \frac{32}{9} L_{\nu d, ii22}^{V,LL} - \frac{32}{9} L_{\nu d, ii11}^{V,LR} - \frac{32}{9} L_{\nu d, ii22}^{V,LR} \right. \\
& + \frac{64}{9} L_{\nu u, ii11}^{V,LL} + \frac{64}{9} L_{\nu u, ii11}^{V,LR} \left] + \alpha^2 \left[ \frac{40}{27} L_{\nu d, ii11}^{V,LL} + \frac{40}{27} L_{\nu d, ii22}^{V,LL} - \frac{56}{27} L_{\nu d, ii11}^{V,LR} \right. \right. \\
& \left. - \frac{56}{27} L_{\nu d, ii22}^{V,LR} + \frac{8}{3} L_{\nu e, ii11}^{V,LL} + \frac{8}{3} L_{\nu e, ii22}^{V,LL} - 8L_{\nu e, ii11}^{V,LR} - 8L_{\nu e, ii22}^{V,LR} + \frac{256}{27} L_{\nu u, ii11}^{V,LL} \right. \\
& \left. - \frac{128}{27} L_{\nu u, ii11}^{V,LR} \right]; \\
\dot{L}_{ud, ij\bar{j}}^{V1,LL} & = \frac{8}{3} g_s^2 L_{ud, ij\bar{j}}^{V8,LL} + e^2 \left[ -\frac{8}{3} L_{ud, ij\bar{j}}^{V1,LL} + \frac{4}{9} L_{eu, 11ii}^{V,LL} + \frac{4}{9} L_{eu, 22ii}^{V,LL} + \frac{4}{9} L_{ud, ii11}^{V1,LL} \right. \\
& + \frac{4}{9} L_{ud, ii22}^{V1,LL} + \frac{4}{9} L_{ud, ii11}^{V1,LR} + \frac{4}{9} L_{ud, ii22}^{V1,LR} + \frac{4}{9} L_{ue, ii11}^{V,LR} + \frac{4}{9} L_{ue, ii22}^{V,LR} - \frac{8}{9} L_{uu, iii}^{V1,LR} \\
& - \frac{64}{27} L_{uu, iii}^{V,LL} - \frac{16}{9} L_{dd, jj\bar{j}\bar{j}}^{V1,LR} - \frac{128}{27} L_{dd, jj\bar{j}\bar{j}}^{V,LL} - \frac{8}{9} L_{de, jj11}^{V,LR} - \frac{8}{9} L_{de, jj22}^{V,LR} + \frac{16}{9} L_{du, jj11}^{V1,LR} \\
& \left. - \frac{8}{9} L_{ed, 11jj}^{V,LL} - \frac{8}{9} L_{ed, 22jj}^{V,LL} + \frac{16}{9} L_{ud, 11jj}^{V1,LL} \right] + \alpha_s^2 \left[ -\frac{28}{3} L_{ud, ij\bar{j}}^{V1,LL} + \frac{74}{27} L_{ud, ij\bar{j}}^{V8,LL} \right]
\end{aligned}$$

$$\begin{aligned}
& + 8L_{ii11}^{V1,LL} + 8L_{ii22}^{V1,LL} - 8L_{ii11}^{V1,LR} - 8L_{ii22}^{V1,LR} + \frac{4}{27}L_{ii11}^{V8,LL} + \frac{4}{27}L_{ii22}^{V8,LL} \\
& + \frac{4}{27}L_{ii11}^{V8,LR} + \frac{4}{27}L_{ii22}^{V8,LR} - 8L_{iii}^{V1,LR} + \frac{4}{27}L_{iii}^{V8,LR} + \frac{328}{9}L_{iii}^{V,LL} - 16L_{jjj}^{V1,LR} \\
& + \frac{8}{27}L_{jjj}^{V8,LR} + \frac{1672}{27}L_{jjj}^{V,LL} - 8L_{jj11}^{V1,LR} + \frac{4}{27}L_{jj11}^{V8,LR} + 8L_{11jj}^{V1,LL} + \frac{4}{27}L_{11jj}^{V8,LL} \Big] \\
& + \alpha_s \alpha \left[ \frac{64}{3}L_{ijj}^{V1,LL} - \frac{8}{27}L_{ijj}^{V8,LL} + \frac{16}{9}L_{ii11}^{V1,LL} + \frac{16}{9}L_{ii22}^{V1,LL} + \frac{16}{9}L_{ii11}^{V1,LR} \right. \\
& - \frac{32}{9}L_{ii22}^{V1,LR} + \frac{352}{729}L_{ii11}^{V8,LL} + \frac{352}{729}L_{ii22}^{V8,LL} - \frac{368}{729}L_{ii11}^{V8,LR} + \frac{2008}{729}L_{ii22}^{V8,LR} \\
& - \frac{32}{9}L_{iii}^{V1,LR} + \frac{2008}{729}L_{iii}^{V8,LR} - \frac{2144}{243}L_{iii}^{V,LL} - \frac{64}{9}L_{jjj}^{V1,LR} + \frac{4088}{729}L_{jjj}^{V8,LR} \\
& \left. - \frac{10304}{729}L_{jjj}^{V,LL} + \frac{64}{9}L_{jj11}^{V1,LR} - \frac{2708}{729}L_{jj11}^{V8,LR} + \frac{64}{9}L_{11jj}^{V1,LL} + \frac{172}{729}L_{11jj}^{V8,LL} \right] \\
& + \alpha^2 \left[ \frac{1448}{729}L_{11ii}^{V,LL} + \frac{1448}{729}L_{22ii}^{V,LL} - \frac{208}{729}L_{ii11}^{V1,LL} - \frac{208}{729}L_{ii22}^{V1,LL} - \frac{136}{729}L_{ii11}^{V1,LR} \right. \\
& + \frac{2720}{729}L_{ii22}^{V1,LR} + \frac{1664}{729}L_{ii11}^{V,LR} + \frac{1664}{729}L_{ii22}^{V,LR} + \frac{2432}{729}L_{iii}^{V1,LR} + \frac{11872}{729}L_{iii}^{V,LL} \\
& - \frac{512}{729}L_{jjj}^{V1,LR} + \frac{40528}{2187}L_{jjj}^{V,LL} - \frac{2992}{729}L_{jj11}^{V,LR} - \frac{2992}{729}L_{jj22}^{V,LR} - \frac{1216}{729}L_{jj11}^{V1,LR} \\
& \left. + \frac{2624}{729}L_{11jj}^{V,LL} + \frac{2624}{729}L_{22jj}^{V,LL} + \frac{6272}{729}L_{11jj}^{V1,LL} \right] ;
\end{aligned}$$

$$\begin{aligned}
\dot{L}_{ijj}^{V8,LL} & = g_s^2 \left[ 12L_{ijj}^{V1,LL} - 4L_{ijj}^{V8,LL} + \frac{2}{3}L_{ii11}^{V8,LL} + \frac{2}{3}L_{ii22}^{V8,LL} + \frac{2}{3}L_{ii11}^{V8,LR} \right. \\
& + \frac{2}{3}L_{ii22}^{V8,LR} + \frac{2}{3}L_{iii}^{V8,LR} + \frac{8}{3}L_{iii}^{V,LL} + \frac{4}{3}L_{jjj}^{V8,LR} + \frac{16}{3}L_{jjj}^{V,LL} + \frac{2}{3}L_{jj11}^{V8,LR} \\
& \left. + \frac{2}{3}L_{11jj}^{V8,LL} \right] - \frac{8}{3}e^2L_{ijj}^{V8,LL} + \alpha_s^2 \left[ \frac{37}{3}L_{ijj}^{V1,LL} - \frac{121}{9}L_{ijj}^{V8,LL} - \frac{2}{3}L_{ii11}^{V1,LL} \right. \\
& - \frac{2}{3}L_{ii22}^{V1,LL} - \frac{22}{3}L_{ii11}^{V1,LR} - \frac{22}{3}L_{ii22}^{V1,LR} + \frac{805}{81}L_{ii11}^{V8,LL} + \frac{805}{81}L_{ii22}^{V8,LL} + \frac{175}{81}L_{ii11}^{V8,LR} \\
& \left. + \frac{175}{81}L_{ii22}^{V8,LR} - \frac{22}{3}L_{iii}^{V1,LR} + \frac{175}{81}L_{iii}^{V8,LR} + \frac{1942}{27}L_{iii}^{V,LL} - \frac{44}{3}L_{jjj}^{V1,LR} + \frac{314}{81}L_{jjj}^{V8,LR} \right]
\end{aligned}$$

$$\begin{aligned}
& + \frac{10246}{81} L_{jjjj}^{V,LL} - \frac{22}{3} L_{jj11}^{V1,LR} + \frac{157}{81} L_{jj11}^{V8,LR} - \frac{2}{3} L_{11jj}^{V1,LL} + \frac{787}{81} L_{11jj}^{V8,LL} \Bigg] \\
& + \alpha_s \alpha \left[ -\frac{4}{3} L_{ijjj}^{V1,LL} - \frac{47}{9} L_{ijjj}^{V8,LL} + \frac{284}{81} L_{11ii}^{V,LL} + \frac{284}{81} L_{22ii}^{V,LL} + \frac{284}{81} L_{ii11}^{V1,LL} \right. \\
& + \frac{284}{81} L_{ii22}^{V1,LL} + \frac{284}{81} L_{ii11}^{V1,LR} - \frac{496}{81} L_{ii22}^{V1,LR} + \frac{14}{9} L_{ii11}^{V8,LL} + \frac{14}{9} L_{ii22}^{V8,LL} + \frac{10}{27} L_{ii11}^{V8,LR} \\
& + \frac{4}{27} L_{ii22}^{V8,LR} + \frac{284}{81} L_{ii11}^{V,LR} + \frac{284}{81} L_{ii22}^{V,LR} - \frac{568}{81} L_{iii}^{V1,LR} + \frac{4}{27} L_{iii}^{V8,LR} - \frac{4616}{81} L_{iii}^{V,LL} \\
& - \frac{392}{81} L_{jjjj}^{V1,LR} + \frac{104}{27} L_{jjjj}^{V8,LR} - \frac{15728}{243} L_{jjjj}^{V,LL} - \frac{196}{81} L_{jj11}^{V,LR} - \frac{196}{81} L_{jj22}^{V,LR} + \frac{392}{81} L_{jj11}^{V1,LR} \\
& \left. - \frac{80}{27} L_{jj11}^{V8,LR} - \frac{196}{81} L_{11jj}^{V,LL} - \frac{196}{81} L_{22jj}^{V,LL} + \frac{392}{81} L_{11jj}^{V1,LL} + \frac{56}{9} L_{11jj}^{V8,LL} \right] ; \\
\dot{L}_{ed}^{V,LL} & = e^2 \left[ \frac{4}{3} L_{ijjj}^{V1,LR} + \frac{8}{3} L_{ijjj}^{V,LL} + \frac{8}{9} L_{ijji}^{V,LL} + 4 L_{jjii}^{V,LL} + \frac{4}{3} L_{iii}^{V1,LR} \right. \\
& + \frac{32}{9} L_{iii}^{V,LL} + \frac{4}{3} L_{ii11}^{V,LR} + \frac{4}{3} L_{ii22}^{V,LR} - \frac{8}{3} L_{ii11}^{V1,LR} + \frac{4}{3} L_{11ii}^{V,LL} + \frac{4}{3} L_{22ii}^{V,LL} \\
& - \frac{8}{3} L_{11ii}^{V1,LL} + \frac{4}{9} L_{jj11}^{V,LL} + \frac{4}{9} L_{jj22}^{V,LL} + \frac{4}{9} L_{jj11}^{V,LR} + \frac{4}{9} L_{jj22}^{V,LR} + \frac{8}{3} L_{jjjj}^{V,LL} \\
& \left. + \frac{8}{9} L_{jjjj}^{V,LR} - \frac{8}{9} L_{jj11}^{V,LL} - \frac{8}{9} L_{jj11}^{V,LR} \right] + \alpha_s^2 \left[ 8 L_{jj11}^{V,LL} + 8 L_{jj22}^{V,LL} \right. \\
& \left. - 8 L_{jj11}^{V,LR} - 8 L_{jj22}^{V,LR} + 8 L_{jj11}^{V,LL} - 8 L_{jj11}^{V,LR} \right] + \alpha_s \alpha \left[ \frac{16}{3} L_{ijjj}^{V1,LR} \right. \\
& - \frac{1022}{243} L_{ijjj}^{V8,LR} + 8 L_{ijjj}^{V,LL} + \frac{64}{243} L_{ijji}^{V,LL} - 16 L_{jjii}^{V,LL} + \frac{16}{3} L_{iii}^{V1,LR} - \frac{1022}{243} L_{iii}^{V8,LR} \\
& + \frac{1048}{81} L_{iii}^{V,LL} - \frac{32}{3} L_{ii11}^{V1,LR} + \frac{1354}{243} L_{ii11}^{V8,LR} - \frac{32}{3} L_{11ii}^{V1,LL} - \frac{86}{243} L_{11ii}^{V8,LL} + \frac{16}{9} L_{jj11}^{V,LL} \\
& + \frac{16}{9} L_{jj22}^{V,LL} + \frac{16}{9} L_{jj11}^{V,LR} + \frac{16}{9} L_{jj22}^{V,LR} - \frac{32}{9} L_{jj11}^{V,LL} - \frac{32}{9} L_{jj11}^{V,LR} \Bigg] + \alpha^2 \left[ -\frac{1312}{243} L_{ijjj}^{V1,LR} \right. \\
& + \frac{1984}{243} L_{ijjj}^{V,LL} + \frac{2896}{729} L_{ijji}^{V,LL} - \frac{130}{9} L_{jjii}^{V,LL} - \frac{1312}{243} L_{iii}^{V1,LR} + \frac{4816}{243} L_{iii}^{V,LL} \\
& \left. - \frac{3184}{243} L_{ii11}^{V,LR} - \frac{3184}{243} L_{ii22}^{V,LR} - \frac{6232}{243} L_{ii11}^{V1,LR} + \frac{3728}{243} L_{11ii}^{V,LL} + \frac{3728}{243} L_{22ii}^{V,LL} \right]
\end{aligned}$$

$$\begin{aligned}
& + \frac{2984}{243} L_{11ii}^{V1,LL} - \frac{104}{243} L_{jj11}^{V,LL} - \frac{104}{243} L_{jj22}^{V,LL} - \frac{200}{243} L_{jj11}^{V,LR} - \frac{200}{243} L_{jj22}^{V,LR} \\
& + \frac{16}{9} L_{jjjj}^{V,LL} - \frac{1040}{81} L_{jjjj}^{V,LR} - \frac{1016}{243} L_{jj11}^{V,LL} - \frac{1400}{243} L_{jj11}^{V,LR} \Big] ; \\
\dot{L}_{jjii}^{V,LL} = & e^2 \left[ -8 L_{jjii}^{V,LL} + \frac{4}{3} L_{11ii}^{V,LL} + \frac{4}{3} L_{22ii}^{V,LL} + \frac{4}{3} L_{ii11}^{V1,LL} + \frac{4}{3} L_{ii22}^{V1,LL} \right. \\
& + \frac{4}{3} L_{ii11}^{V1,LR} + \frac{4}{3} L_{ii22}^{V1,LR} + \frac{4}{3} L_{ii11}^{V,LR} + \frac{4}{3} L_{ii22}^{V,LR} - \frac{8}{3} L_{iiii}^{V1,LR} - \frac{64}{9} L_{iiii}^{V,LL} \\
& - \frac{8}{9} L_{jj11}^{V,LL} - \frac{8}{9} L_{jj22}^{V,LL} - \frac{8}{9} L_{jj11}^{V,LR} - \frac{8}{9} L_{jj22}^{V,LR} - \frac{16}{3} L_{jjjj}^{V,LL} - \frac{16}{9} L_{jjjj}^{V,LR} \\
& + \frac{16}{9} L_{jj11}^{V,LL} + \frac{16}{9} L_{jj11}^{V,LR} \Big] + \alpha_s^2 \left[ 8 L_{jj11}^{V,LL} + 8 L_{jj22}^{V,LL} - 8 L_{jj11}^{V,LR} \right. \\
& - 8 L_{jj22}^{V,LR} + 8 L_{jj11}^{V,LL} - 8 L_{jj11}^{V,LR} \Big] + \alpha_s \alpha \left[ 32 L_{jjii}^{V,LL} + \frac{16}{3} L_{ii11}^{V1,LL} \right. \\
& + \frac{16}{3} L_{ii22}^{V1,LL} + \frac{16}{3} L_{ii11}^{V1,LR} - \frac{32}{3} L_{ii22}^{V1,LR} + \frac{352}{243} L_{ii11}^{V8,LL} + \frac{352}{243} L_{ii22}^{V8,LL} - \frac{368}{243} L_{ii11}^{V8,LR} \\
& + \frac{2008}{243} L_{ii22}^{V8,LR} - \frac{32}{3} L_{iiii}^{V1,LR} + \frac{2008}{243} L_{iiii}^{V8,LR} - \frac{2144}{81} L_{iiii}^{V,LL} - \frac{32}{9} L_{jj11}^{V,LL} - \frac{32}{9} L_{jj22}^{V,LL} \\
& - \frac{32}{9} L_{jj11}^{V,LR} - \frac{32}{9} L_{jj22}^{V,LR} + \frac{64}{9} L_{jj11}^{V,LL} + \frac{64}{9} L_{jj11}^{V,LR} \Big] + \alpha^2 \left[ \frac{80}{9} L_{jjii}^{V,LL} \right. \\
& + \frac{3248}{243} L_{11ii}^{V,LL} + \frac{3248}{243} L_{22ii}^{V,LL} + \frac{296}{243} L_{ii11}^{V1,LL} + \frac{296}{243} L_{ii22}^{V1,LL} - \frac{928}{243} L_{ii11}^{V1,LR} \\
& + \frac{416}{243} L_{ii22}^{V1,LR} - \frac{424}{243} L_{ii11}^{V,LR} - \frac{424}{243} L_{ii22}^{V,LR} + \frac{128}{243} L_{iiii}^{V1,LR} + \frac{26272}{243} L_{iiii}^{V,LL} \\
& + \frac{2512}{243} L_{jj11}^{V,LL} + \frac{2512}{243} L_{jj22}^{V,LL} + \frac{1408}{243} L_{jj11}^{V,LR} + \frac{1408}{243} L_{jj22}^{V,LR} + \frac{544}{9} L_{jjjj}^{V,LL} \\
& + \frac{928}{81} L_{jjjj}^{V,LR} + \frac{1312}{243} L_{jj11}^{V,LL} - \frac{3104}{243} L_{jj11}^{V,LR} \Big] ; \\
\dot{L}_{jjii}^{V,LL} = & e^2 \left[ \frac{4}{3} L_{jj11}^{V,LL} + \frac{4}{3} L_{jj22}^{V,LL} + \frac{4}{3} L_{jj11}^{V,LR} + \frac{4}{3} L_{jj22}^{V,LR} + \frac{4}{3} L_{jj11}^{V,LL} \right. \\
& + \frac{4}{3} L_{jj22}^{V,LL} + \frac{4}{3} L_{jj11}^{V,LR} + \frac{4}{3} L_{jj22}^{V,LR} - \frac{8}{3} L_{jj11}^{V,LL} - \frac{8}{3} L_{jj11}^{V,LR} \Big]
\end{aligned}$$

$$\begin{aligned}
& + \alpha_s \alpha \left[ \frac{16}{3} L_{jj11}^{V,LL} + \frac{16}{3} L_{jj22}^{V,LL} + \frac{16}{3} L_{jj11}^{V,LR} + \frac{16}{3} L_{jj22}^{V,LR} - \frac{32}{3} L_{jj11}^{V,LL} \right. \\
& \quad \left. - \frac{32}{3} L_{jj11}^{V,LR} \right] + \alpha^2 \left[ \frac{40}{9} L_{jj11}^{V,LL} + \frac{40}{9} L_{jj22}^{V,LL} - \frac{32}{9} L_{jj11}^{V,LR} - \frac{32}{9} L_{jj22}^{V,LR} \right. \\
& \quad \left. + 16 L_{jj11}^{V,LL} + 16 L_{jj22}^{V,LL} - 8 L_{jj11}^{V,LR} - 8 L_{jj22}^{V,LR} + \frac{112}{9} L_{jj11}^{V,LL} - \frac{176}{9} L_{jj11}^{V,LR} \right] ; \\
\dot{L}_{jj\bar{i}}^{V,LL} & = e^2 \left[ \frac{4}{9} L_{jj11}^{V,LL} + \frac{4}{9} L_{jj22}^{V,LL} + \frac{4}{9} L_{jj11}^{V,LR} + \frac{4}{9} L_{jj22}^{V,LR} + \frac{4}{9} L_{jj11}^{V,LL} \right. \\
& \quad \left. + \frac{4}{9} L_{jj22}^{V,LL} + \frac{4}{9} L_{jj11}^{V,LR} + \frac{4}{9} L_{jj22}^{V,LR} - \frac{8}{9} L_{jj11}^{V,LL} - \frac{8}{9} L_{jj11}^{V,LR} \right] \\
& \quad + \alpha_s^2 \left[ 8 L_{jj11}^{V,LL} + 8 L_{jj22}^{V,LL} - 8 L_{jj11}^{V,LR} - 8 L_{jj22}^{V,LR} + 8 L_{jj11}^{V,LL} \right. \\
& \quad \left. - 8 L_{jj11}^{V,LR} \right] + \alpha_s \alpha \left[ \frac{16}{9} L_{jj11}^{V,LL} + \frac{16}{9} L_{jj22}^{V,LL} + \frac{16}{9} L_{jj11}^{V,LR} + \frac{16}{9} L_{jj22}^{V,LR} \right. \\
& \quad \left. - \frac{32}{9} L_{jj11}^{V,LL} - \frac{32}{9} L_{jj11}^{V,LR} \right] + \alpha^2 \left[ \frac{16}{27} L_{jj11}^{V,LL} + \frac{16}{27} L_{jj22}^{V,LL} - \frac{8}{27} L_{jj11}^{V,LR} \right. \\
& \quad \left. - \frac{8}{27} L_{jj22}^{V,LR} + \frac{8}{3} L_{jj11}^{V,LL} + \frac{8}{3} L_{jj22}^{V,LL} + \frac{16}{27} L_{jj11}^{V,LL} - \frac{80}{27} L_{jj11}^{V,LR} \right] ; \\
\dot{L}_{jj\bar{i}}^{V,LL} & = e^2 \left[ -\frac{8}{9} L_{jj11}^{V,LL} - \frac{8}{9} L_{jj22}^{V,LL} - \frac{8}{9} L_{jj11}^{V,LR} - \frac{8}{9} L_{jj22}^{V,LR} - \frac{8}{9} L_{jj11}^{V,LL} \right. \\
& \quad \left. - \frac{8}{9} L_{jj22}^{V,LL} - \frac{8}{9} L_{jj11}^{V,LR} - \frac{8}{9} L_{jj22}^{V,LR} + \frac{16}{9} L_{jj11}^{V,LL} + \frac{16}{9} L_{jj11}^{V,LR} \right] \\
& \quad + \alpha_s^2 \left[ 8 L_{jj11}^{V,LL} + 8 L_{jj22}^{V,LL} - 8 L_{jj11}^{V,LR} - 8 L_{jj22}^{V,LR} + 8 L_{jj11}^{V,LL} \right. \\
& \quad \left. - 8 L_{jj11}^{V,LR} \right] + \alpha_s \alpha \left[ -\frac{32}{9} L_{jj11}^{V,LL} - \frac{32}{9} L_{jj22}^{V,LL} - \frac{32}{9} L_{jj11}^{V,LR} - \frac{32}{9} L_{jj22}^{V,LR} \right. \\
& \quad \left. + \frac{64}{9} L_{jj11}^{V,LL} + \frac{64}{9} L_{jj11}^{V,LR} \right] + \alpha^2 \left[ \frac{40}{27} L_{jj11}^{V,LL} + \frac{40}{27} L_{jj22}^{V,LL} - \frac{56}{27} L_{jj11}^{V,LR} \right.
\end{aligned}$$

$$\begin{aligned}
& -\frac{56}{27}L_{jj22}^{V,LR} + \frac{8}{3}L_{jj11}^{V,LL} + \frac{8}{3}L_{jj22}^{V,LL} - 8L_{jj11}^{V,LR} - 8L_{jj22}^{V,LR} + \frac{256}{27}L_{jj11}^{V,LL} \\
& - \frac{128}{27}L_{jj11}^{V,LR} \Big] ;
\end{aligned}$$

$$\begin{aligned}
\dot{L}_{jjii}^{V1,LL} = & \frac{8}{3}L_{jjii}^{V8,LL}g_s^2 + e^2 \Bigg[ -\frac{8}{9}L_{iii}^{V1,LR} - \frac{8}{9}L_{ijj}^{V1,LR} - \frac{64}{27}L_{iii}^{V,LL} - \frac{16}{9}L_{ijj}^{V,LL} \\
& - \frac{16}{27}L_{ijji}^{V,LL} - \frac{8}{9}L_{ii11}^{V,LR} - \frac{8}{9}L_{ii22}^{V,LR} + \frac{16}{9}L_{ii11}^{V1,LR} - \frac{8}{9}L_{11ii}^{V,LL} - \frac{8}{9}L_{22ii}^{V,LL} \\
& + \frac{4}{9}L_{11jj}^{V,LL} + \frac{4}{9}L_{22jj}^{V,LL} + \frac{16}{9}L_{11ii}^{V1,LL} + \frac{4}{9}L_{jj11}^{V1,LL} + \frac{4}{9}L_{jj22}^{V1,LL} - \frac{8}{3}L_{jjii}^{V1,LL} \\
& + \frac{4}{9}L_{jj11}^{V1,LR} + \frac{4}{9}L_{jj22}^{V1,LR} + \frac{4}{9}L_{jj11}^{V,LR} + \frac{4}{9}L_{jj22}^{V,LR} - \frac{8}{9}L_{jjjj}^{V1,LR} - \frac{64}{27}L_{jjjj}^{V,LL} \Bigg] \\
& + \alpha_s^2 \Bigg[ -8L_{iii}^{V1,LR} - 8L_{ijj}^{V1,LR} + \frac{4}{27}L_{iii}^{V8,LR} + \frac{4}{27}L_{ijj}^{V8,LR} + \frac{328}{9}L_{iii}^{V,LL} \\
& + 16L_{ijj}^{V,LL} + \frac{256}{27}L_{ijji}^{V,LL} - 8L_{ii11}^{V1,LR} + \frac{4}{27}L_{ii11}^{V8,LR} + 8L_{11ii}^{V1,LL} + 8L_{jj11}^{V1,LL} \\
& + 8L_{jj22}^{V1,LL} - \frac{28}{3}L_{jjii}^{V1,LL} - 8L_{jj11}^{V1,LR} - 8L_{jj22}^{V1,LR} + \frac{4}{27}L_{11ii}^{V8,LL} + \frac{4}{27}L_{jj11}^{V8,LL} \\
& + \frac{4}{27}L_{jj22}^{V8,LL} + \frac{74}{27}L_{jjii}^{V8,LL} + \frac{4}{27}L_{jj11}^{V8,LR} + \frac{4}{27}L_{jj22}^{V8,LR} - 8L_{jjjj}^{V1,LR} + \frac{4}{27}L_{jjjj}^{V8,LR} \\
& + \frac{328}{9}L_{jjjj}^{V,LL} \Bigg] + \alpha_s\alpha \Bigg[ -\frac{32}{9}L_{iii}^{V1,LR} - \frac{32}{9}L_{ijj}^{V1,LR} + \frac{2044}{729}L_{iii}^{V8,LR} + \frac{2044}{729}L_{ijj}^{V8,LR} \\
& - \frac{2096}{243}L_{iii}^{V,LL} - \frac{16}{3}L_{ijj}^{V,LL} - \frac{128}{729}L_{ijji}^{V,LL} + \frac{64}{9}L_{ii11}^{V1,LR} - \frac{2708}{729}L_{ii11}^{V8,LR} + \frac{64}{9}L_{11ii}^{V1,LL} \\
& + \frac{16}{9}L_{jj11}^{V1,LL} + \frac{16}{9}L_{jj22}^{V1,LL} + \frac{64}{3}L_{jjii}^{V1,LL} + \frac{16}{9}L_{jj11}^{V1,LR} - \frac{32}{9}L_{jj22}^{V1,LR} + \frac{172}{729}L_{11ii}^{V8,LL} \\
& + \frac{352}{729}L_{jj11}^{V8,LL} + \frac{352}{729}L_{jj22}^{V8,LL} - \frac{8}{27}L_{jjii}^{V8,LL} - \frac{368}{729}L_{jj11}^{V8,LR} + \frac{2008}{729}L_{jj22}^{V8,LR} \\
& - \frac{32}{9}L_{jjjj}^{V1,LR} + \frac{2008}{729}L_{jjjj}^{V8,LR} - \frac{2144}{243}L_{jjjj}^{V,LL} \Bigg] + \alpha^2 \Bigg[ -\frac{256}{729}L_{iii}^{V1,LR} - \frac{256}{729}L_{ijj}^{V1,LR} \\
& + \frac{8368}{729}L_{iii}^{V,LL} + \frac{3232}{729}L_{ijj}^{V,LL} + \frac{5728}{2187}L_{ijji}^{V,LL} - \frac{2992}{729}L_{ii11}^{V,LR} - \frac{2992}{729}L_{ii22}^{V,LR}
\end{aligned}$$

$$\begin{aligned}
& -\frac{1216}{729}L_{\substack{du \\ ii11}}^{V1,LR} + \frac{2624}{729}L_{\substack{ed \\ 11ii}}^{V,LL} + \frac{2624}{729}L_{\substack{ed \\ 22ii}}^{V,LL} + \frac{1448}{729}L_{\substack{eu \\ 11jj}}^{V,LL} + \frac{1448}{729}L_{\substack{eu \\ 22jj}}^{V,LL} \\
& + \frac{6272}{729}L_{\substack{ud \\ 11ii}}^{V1,LL} - \frac{208}{729}L_{\substack{ud \\ jj11}}^{V1,LL} - \frac{208}{729}L_{\substack{ud \\ jj22}}^{V1,LL} - \frac{136}{729}L_{\substack{ud \\ jj11}}^{V1,LR} + \frac{2720}{729}L_{\substack{ud \\ jj22}}^{V1,LR} \\
& + \frac{1664}{729}L_{\substack{ue \\ jj11}}^{V,LR} + \frac{1664}{729}L_{\substack{ue \\ jj22}}^{V,LR} + \frac{2432}{729}L_{\substack{uu \\ jjjj}}^{V1,LR} + \frac{11872}{729}L_{\substack{uu \\ jjjj}}^{V,LL} \Big] ;
\end{aligned}$$

$$\begin{aligned}
\dot{L}_{\substack{ud \\ jjii}}^{V8,LL} = & g_s^2 \left[ \frac{2}{3}L_{\substack{dd \\ iijj}}^{V8,LR} + \frac{8}{3}L_{\substack{dd \\ ijji}}^{V,LL} + 12L_{\substack{ud \\ jjii}}^{V1,LL} - 4L_{\substack{ud \\ jjii}}^{V8,LL} + \frac{2}{3}L_{\substack{dd \\ iiii}}^{V8,LR} \right. \\
& + \frac{8}{3}L_{\substack{dd \\ iiii}}^{V,LL} + \frac{2}{3}L_{\substack{du \\ ii11}}^{V8,LR} + \frac{2}{3}L_{\substack{du \\ 11ii}}^{V8,LL} + \frac{2}{3}L_{\substack{ud \\ jj11}}^{V8,LL} + \frac{2}{3}L_{\substack{ud \\ jj22}}^{V8,LL} + \frac{2}{3}L_{\substack{ud \\ jj11}}^{V8,LR} \\
& + \frac{2}{3}L_{\substack{ud \\ jj22}}^{V8,LR} + \frac{2}{3}L_{\substack{uu \\ jjjj}}^{V8,LR} + \frac{8}{3}L_{\substack{uu \\ jjjj}}^{V,LL} \Big] - \frac{8}{3}e^2L_{\substack{ud \\ jjii}}^{V8,LL} + \alpha_s^2 \left[ -\frac{22}{3}L_{\substack{ud \\ iijj}}^{V1,LR} \right. \\
& + \frac{157}{81}L_{\substack{dd \\ iijj}}^{V8,LR} - \frac{28}{3}L_{\substack{dd \\ iijj}}^{V,LL} + \frac{5248}{81}L_{\substack{dd \\ ijji}}^{V,LL} + \frac{37}{3}L_{\substack{ud \\ jjii}}^{V1,LL} - \frac{121}{9}L_{\substack{ud \\ jjii}}^{V8,LL} - \frac{22}{3}L_{\substack{ud \\ iiii}}^{V1,LR} \\
& + \frac{157}{81}L_{\substack{dd \\ iiii}}^{V8,LR} + \frac{1918}{27}L_{\substack{dd \\ iiii}}^{V,LL} - \frac{22}{3}L_{\substack{du \\ ii11}}^{V1,LR} + \frac{157}{81}L_{\substack{du \\ ii11}}^{V8,LR} - \frac{2}{3}L_{\substack{ud \\ 11ii}}^{V1,LL} + \frac{787}{81}L_{\substack{ud \\ 11ii}}^{V8,LL} \\
& - \frac{2}{3}L_{\substack{ud \\ jj11}}^{V1,LL} - \frac{2}{3}L_{\substack{ud \\ jj22}}^{V1,LL} - \frac{22}{3}L_{\substack{ud \\ jj11}}^{V1,LR} - \frac{22}{3}L_{\substack{ud \\ jj22}}^{V1,LR} + \frac{805}{81}L_{\substack{ud \\ jj11}}^{V8,LL} + \frac{805}{81}L_{\substack{ud \\ jj22}}^{V8,LL} \\
& + \frac{175}{81}L_{\substack{ud \\ jj11}}^{V8,LR} + \frac{175}{81}L_{\substack{ud \\ jj22}}^{V8,LR} - \frac{22}{3}L_{\substack{uu \\ jjjj}}^{V1,LR} + \frac{175}{81}L_{\substack{uu \\ jjjj}}^{V8,LR} + \frac{1942}{27}L_{\substack{uu \\ jjjj}}^{V,LL} \Big] \\
& + \alpha_s \alpha \left[ -\frac{196}{81}L_{\substack{dd \\ iijj}}^{V1,LR} + \frac{52}{27}L_{\substack{dd \\ iijj}}^{V8,LR} - \frac{392}{81}L_{\substack{dd \\ iijj}}^{V,LL} - \frac{5096}{243}L_{\substack{dd \\ ijji}}^{V,LL} - \frac{4}{3}L_{\substack{ud \\ jjii}}^{V1,LL} \right. \\
& - \frac{47}{9}L_{\substack{ud \\ jjii}}^{V8,LL} - \frac{196}{81}L_{\substack{dd \\ iiii}}^{V1,LR} + \frac{52}{27}L_{\substack{dd \\ iiii}}^{V8,LR} - \frac{3152}{81}L_{\substack{dd \\ iiii}}^{V,LL} - \frac{196}{81}L_{\substack{de \\ ii11}}^{V,LR} - \frac{196}{81}L_{\substack{de \\ ii22}}^{V,LR} \\
& + \frac{392}{81}L_{\substack{du \\ ii11}}^{V1,LR} - \frac{80}{27}L_{\substack{du \\ ii11}}^{V8,LR} - \frac{196}{81}L_{\substack{ed \\ 11ii}}^{V,LL} - \frac{196}{81}L_{\substack{ed \\ 22ii}}^{V,LL} + \frac{392}{81}L_{\substack{ud \\ 11ii}}^{V1,LL} + \frac{56}{9}L_{\substack{ud \\ 11ii}}^{V8,LL} \\
& + \frac{284}{81}L_{\substack{eu \\ 11jj}}^{V,LL} + \frac{284}{81}L_{\substack{eu \\ 22jj}}^{V,LL} + \frac{284}{81}L_{\substack{ud \\ jj11}}^{V1,LL} + \frac{284}{81}L_{\substack{ud \\ jj22}}^{V1,LL} + \frac{284}{81}L_{\substack{ud \\ jj11}}^{V1,LR} - \frac{496}{81}L_{\substack{ud \\ jj22}}^{V1,LR} \\
& + \frac{14}{9}L_{\substack{ud \\ jj11}}^{V8,LL} + \frac{14}{9}L_{\substack{ud \\ jj22}}^{V8,LL} + \frac{10}{27}L_{\substack{ud \\ jj11}}^{V8,LR} + \frac{4}{27}L_{\substack{ud \\ jj22}}^{V8,LR} + \frac{284}{81}L_{\substack{ue \\ jj11}}^{V,LR} + \frac{284}{81}L_{\substack{ue \\ jj22}}^{V,LR} \\
& - \frac{568}{81}L_{\substack{uu \\ jjjj}}^{V1,LR} + \frac{4}{27}L_{\substack{uu \\ jjjj}}^{V8,LR} - \frac{4616}{81}L_{\substack{uu \\ jjjj}}^{V,LL} \Big] ;
\end{aligned}$$

$$\begin{aligned}
\dot{L}_{ijj}^{V,LL} = & g_s^2 \left[ -\frac{1}{18} L_{iii}^{V8,LR} - \frac{1}{18} L_{ijj}^{V8,LR} - \frac{1}{9} L_{jjj}^{V8,LR} - \frac{2}{9} L_{iii}^{V,LL} - 2 L_{ijj}^{V,LL} \right. \\
& + \frac{52}{9} L_{ijj}^{V,LL} - \frac{4}{9} L_{jjj}^{V,LL} - \frac{1}{18} L_{ii1}^{V8,LR} - \frac{1}{18} L_{jj1}^{V8,LR} - \frac{1}{18} L_{11i}^{V8,LL} - \frac{1}{18} L_{11j}^{V8,LL} \left. \right] \\
& + e^2 \left[ \frac{2}{9} L_{iii}^{V1,LR} + \frac{2}{9} L_{ijj}^{V1,LR} + \frac{4}{9} L_{jjj}^{V1,LR} + \frac{16}{27} L_{iii}^{V,LL} + \frac{16}{9} L_{ijj}^{V,LL} + \frac{4}{27} L_{jjj}^{V,LL} \right. \\
& + \frac{32}{27} L_{jjj}^{V,LL} + \frac{2}{9} L_{de}^{V,LR} + \frac{2}{9} L_{de}^{V,LR} + \frac{2}{9} L_{de}^{V,LR} + \frac{2}{9} L_{de}^{V,LR} + \frac{2}{9} L_{de}^{V,LR} - \frac{4}{9} L_{ii1}^{V1,LR} \\
& - \frac{4}{9} L_{jj1}^{V1,LR} + \frac{2}{9} L_{ed}^{V,LL} + \frac{2}{9} L_{ed}^{V,LL} + \frac{2}{9} L_{ed}^{V,LL} + \frac{2}{9} L_{ed}^{V,LL} + \frac{2}{9} L_{ed}^{V,LL} - \frac{4}{9} L_{11i}^{V1,LL} \\
& \left. - \frac{4}{9} L_{11j}^{V1,LL} \right] + \alpha_s^2 \left[ -\frac{61}{18} L_{iii}^{V1,LR} - \frac{61}{18} L_{ijj}^{V1,LR} - \frac{61}{9} L_{jjj}^{V1,LR} - \frac{85}{972} L_{iii}^{V8,LR} \right. \\
& - \frac{85}{972} L_{ijj}^{V8,LR} - \frac{85}{486} L_{jjj}^{V8,LR} + \frac{1993}{162} L_{iii}^{V,LL} - \frac{47}{18} L_{ijj}^{V,LL} + \frac{2677}{486} L_{ijj}^{V,LL} + \frac{9925}{486} L_{jjj}^{V,LL} \\
& - \frac{61}{18} L_{ii1}^{V1,LR} - \frac{61}{18} L_{jj1}^{V1,LR} - \frac{85}{972} L_{ii1}^{V8,LR} - \frac{85}{972} L_{jj1}^{V8,LR} + \frac{73}{18} L_{11i}^{V1,LL} + \frac{73}{18} L_{11j}^{V1,LL} \\
& \left. - \frac{715}{972} L_{11i}^{V8,LL} - \frac{715}{972} L_{11j}^{V8,LL} \right] + \alpha_s \alpha \left[ \frac{238}{243} L_{iii}^{V1,LR} + \frac{238}{243} L_{ijj}^{V1,LR} + \frac{476}{243} L_{jjj}^{V1,LR} \right. \\
& - \frac{797}{1458} L_{iii}^{V8,LR} - \frac{797}{1458} L_{ijj}^{V8,LR} - \frac{797}{729} L_{jjj}^{V8,LR} + \frac{313}{243} L_{iii}^{V,LL} - \frac{1522}{243} L_{ijj}^{V,LL} \\
& - \frac{6740}{729} L_{ijj}^{V,LL} + \frac{1621}{729} L_{jjj}^{V,LL} + \frac{22}{243} L_{de}^{V,LR} + \frac{22}{243} L_{de}^{V,LR} + \frac{22}{243} L_{de}^{V,LR} + \frac{22}{243} L_{de}^{V,LR} \\
& - \frac{476}{243} L_{ii1}^{V1,LR} - \frac{476}{243} L_{jj1}^{V1,LR} + \frac{715}{1458} L_{ii1}^{V8,LR} + \frac{715}{1458} L_{jj1}^{V8,LR} + \frac{22}{243} L_{11i}^{V,LL} \\
& + \frac{22}{243} L_{11j}^{V,LL} + \frac{22}{243} L_{22i}^{V,LL} + \frac{22}{243} L_{22j}^{V,LL} - \frac{476}{243} L_{11i}^{V1,LL} - \frac{476}{243} L_{11j}^{V1,LL} + \frac{103}{1458} L_{11i}^{V8,LL} \\
& \left. + \frac{103}{1458} L_{11j}^{V8,LL} \right] + \alpha^2 \left[ -\frac{368}{729} L_{iii}^{V1,LR} - \frac{368}{729} L_{ijj}^{V1,LR} - \frac{736}{729} L_{jjj}^{V1,LR} + \frac{608}{729} L_{iii}^{V,LL} \right. \\
& + \frac{110}{729} L_{ijj}^{V,LL} + \frac{296}{2187} L_{ijj}^{V,LL} + \frac{2936}{2187} L_{jjj}^{V,LL} - \frac{656}{729} L_{de}^{V,LR} - \frac{656}{729} L_{de}^{V,LR} \\
& \left. - \frac{656}{729} L_{de}^{V,LR} - \frac{656}{729} L_{de}^{V,LR} - \frac{1748}{729} L_{ii1}^{V1,LR} - \frac{1748}{729} L_{jj1}^{V1,LR} + \frac{856}{729} L_{11i}^{V,LL} \right]
\end{aligned}$$



$$\begin{aligned}
& + \frac{856}{729} L_{11jj}^{V,LL,ed} + \frac{856}{729} L_{22ii}^{V,LL,ed} + \frac{856}{729} L_{22jj}^{V,LL,ed} + \frac{268}{729} L_{11ii}^{V1,LL} + \frac{268}{729} L_{11jj}^{V1,LL} \Big] ; \\
\dot{L}_{dd\,ijji}^{V,LL} = & g_s^2 \left[ \frac{1}{6} L_{dd\,ijji}^{V8,LR} + 6 L_{dd\,ijji}^{V,LL} - \frac{4}{3} L_{dd\,ijji}^{V,LL} + \frac{1}{6} L_{dd\,iiii}^{V8,LR} + \frac{2}{3} L_{dd\,iiii}^{V,LL} \right. \\
& + \frac{1}{6} L_{du\,ii11}^{V8,LR} + \frac{1}{6} L_{ud\,11ii}^{V8,LL} + \frac{1}{3} L_{dd\,jjjj}^{V8,LR} + \frac{4}{3} L_{dd\,jjjj}^{V,LL} + \frac{1}{6} L_{du\,jj11}^{V8,LR} + \frac{1}{6} L_{ud\,11jj}^{V8,LL} \Big] \\
& + \frac{4}{3} e^2 L_{dd\,ijji}^{V,LL} + \alpha_s^2 \left[ -\frac{11}{6} L_{dd\,ijji}^{V1,LR} + \frac{157}{324} L_{dd\,ijji}^{V8,LR} + \frac{23}{6} L_{dd\,ijji}^{V,LL} + \frac{779}{162} L_{dd\,ijji}^{V,LL} \right. \\
& - \frac{11}{6} L_{dd\,iiii}^{V1,LR} + \frac{157}{324} L_{dd\,iiii}^{V8,LR} + \frac{959}{54} L_{dd\,iiii}^{V,LL} - \frac{11}{6} L_{du\,ii11}^{V1,LR} + \frac{157}{324} L_{du\,ii11}^{V8,LR} - \frac{1}{6} L_{ud\,11ii}^{V1,LL} \\
& + \frac{787}{324} L_{ud\,11ii}^{V8,LL} - \frac{11}{3} L_{dd\,jjjj}^{V1,LR} + \frac{157}{162} L_{dd\,jjjj}^{V8,LR} + \frac{5123}{162} L_{dd\,jjjj}^{V,LL} - \frac{11}{6} L_{du\,jj11}^{V1,LR} + \frac{157}{324} L_{du\,jj11}^{V8,LR} \\
& - \frac{1}{6} L_{ud\,11jj}^{V1,LL} + \frac{787}{324} L_{ud\,11jj}^{V8,LL} \Big] + \alpha_s \alpha \left[ -\frac{22}{81} L_{dd\,ijji}^{V1,LR} - \frac{25}{54} L_{dd\,ijji}^{V8,LR} - \frac{746}{81} L_{dd\,ijji}^{V,LL} \right. \\
& - \frac{1436}{243} L_{dd\,ijji}^{V,LL} - \frac{22}{81} L_{dd\,iiii}^{V1,LR} - \frac{25}{54} L_{dd\,iiii}^{V8,LR} + \frac{211}{81} L_{dd\,iiii}^{V,LL} - \frac{22}{81} L_{de\,ii11}^{V,LR} - \frac{22}{81} L_{de\,ii22}^{V,LR} \\
& + \frac{44}{81} L_{du\,ii11}^{V1,LR} + \frac{71}{54} L_{du\,ii11}^{V8,LR} - \frac{22}{81} L_{ed\,11ii}^{V,LL} - \frac{22}{81} L_{ed\,22ii}^{V,LL} + \frac{44}{81} L_{ud\,11ii}^{V1,LL} - \frac{7}{18} L_{ud\,11ii}^{V8,LL} \\
& - \frac{44}{81} L_{dd\,jjjj}^{V1,LR} - \frac{25}{27} L_{dd\,jjjj}^{V8,LR} + \frac{955}{243} L_{dd\,jjjj}^{V,LL} - \frac{22}{81} L_{de\,jj11}^{V,LR} - \frac{22}{81} L_{de\,jj22}^{V,LR} + \frac{44}{81} L_{du\,jj11}^{V1,LR} \\
& + \frac{71}{54} L_{du\,jj11}^{V8,LR} - \frac{22}{81} L_{ed\,11jj}^{V,LL} - \frac{22}{81} L_{ed\,22jj}^{V,LL} + \frac{44}{81} L_{ud\,11jj}^{V1,LL} - \frac{7}{18} L_{ud\,11jj}^{V8,LL} \Big] - \frac{2}{9} \alpha^2 L_{dd\,ijji}^{V,LL} ; \\
\dot{L}_{dd\,iiii}^{V,LL} = & g_s^2 \left[ \frac{2}{9} L_{dd\,ijji}^{V8,LR} + \frac{8}{9} L_{dd\,ijji}^{V,LL} + \frac{2}{9} L_{dd\,iiii}^{V8,LR} + \frac{44}{9} L_{dd\,iiii}^{V,LL} + \frac{2}{9} L_{du\,ii11}^{V8,LR} \right. \\
& + \frac{2}{9} L_{ud\,11ii}^{V8,LL} \Big] + e^2 \left[ \frac{4}{9} L_{dd\,ijji}^{V1,LR} + \frac{8}{9} L_{dd\,ijji}^{V,LL} + \frac{8}{27} L_{dd\,ijji}^{V,LL} + \frac{4}{9} L_{dd\,iiii}^{V1,LR} \right. \\
& + \frac{68}{27} L_{dd\,iiii}^{V,LL} + \frac{4}{9} L_{de\,ii11}^{V,LR} + \frac{4}{9} L_{de\,ii22}^{V,LR} - \frac{8}{9} L_{du\,ii11}^{V1,LR} + \frac{4}{9} L_{ed\,11ii}^{V,LL} + \frac{4}{9} L_{ed\,22ii}^{V,LL} \\
& - \frac{8}{9} L_{ud\,11ii}^{V1,LL} \Big] + \alpha_s^2 \left[ -\frac{94}{9} L_{dd\,ijji}^{V1,LR} + \frac{193}{243} L_{dd\,ijji}^{V8,LR} + \frac{116}{9} L_{dd\,ijji}^{V,LL} + \frac{7552}{243} L_{dd\,ijji}^{V,LL} \right. \\
& - \frac{94}{9} L_{dd\,iiii}^{V1,LR} + \frac{193}{243} L_{dd\,iiii}^{V8,LR} + \frac{4447}{81} L_{dd\,iiii}^{V,LL} - \frac{94}{9} L_{du\,ii11}^{V1,LR} + \frac{193}{243} L_{du\,ii11}^{V8,LR} + \frac{70}{9} L_{ud\,11ii}^{V1,LL}
\end{aligned}$$

$$\begin{aligned}
& + \frac{823}{243} L_{11ii}^{V8,LL} \Big] + \alpha_s \alpha \Big[ \frac{344}{243} L_{iijj}^{V1,LR} - \frac{1472}{729} L_{iijj}^{V8,LR} + \frac{472}{243} L_{iijj}^{V,LL} + \frac{1880}{729} L_{ijji}^{V,LL} \\
& + \frac{344}{243} L_{iii}^{V1,LR} - \frac{1472}{729} L_{iii}^{V8,LR} - \frac{2104}{243} L_{iii}^{V,LL} - \frac{88}{243} L_{ii11}^{V,LR} - \frac{88}{243} L_{ii22}^{V,LR} \\
& - \frac{688}{243} L_{ii11}^{V1,LR} + \frac{2632}{729} L_{ii11}^{V8,LR} - \frac{88}{243} L_{11ii}^{V,LL} - \frac{88}{243} L_{22ii}^{V,LL} - \frac{688}{243} L_{11ii}^{V1,LL} \\
& - \frac{464}{729} L_{11ii}^{V8,LL} \Big] + \alpha^2 \Big[ - \frac{736}{729} L_{iijj}^{V1,LR} + \frac{544}{729} L_{iijj}^{V,LL} + \frac{592}{2187} L_{ijji}^{V,LL} - \frac{736}{729} L_{iii}^{V1,LR} \\
& + \frac{1054}{729} L_{iii}^{V,LL} - \frac{1312}{729} L_{ii11}^{V,LR} - \frac{1312}{729} L_{ii22}^{V,LR} - \frac{3496}{729} L_{ii11}^{V1,LR} + \frac{1712}{729} L_{11ii}^{V,LL} \\
& + \frac{1712}{729} L_{22ii}^{V,LL} + \frac{536}{729} L_{11ii}^{V1,LL} \Big] ;
\end{aligned}$$

$$\begin{aligned}
\dot{L}_{iii}^{V,LL} & = g_s^2 \Big[ \frac{2}{9} L_{ii11}^{V8,LL} + \frac{2}{9} L_{ii22}^{V8,LL} + \frac{2}{9} L_{ii11}^{V8,LR} + \frac{2}{9} L_{ii22}^{V8,LR} + \frac{2}{9} L_{iii}^{V8,LR} \\
& + \frac{44}{9} L_{iii}^{V,LL} \Big] + e^2 \Big[ - \frac{8}{9} L_{11ii}^{V,LL} - \frac{8}{9} L_{22ii}^{V,LL} - \frac{8}{9} L_{ii11}^{V1,LL} - \frac{8}{9} L_{ii22}^{V1,LL} \\
& - \frac{8}{9} L_{ii11}^{V1,LR} - \frac{8}{9} L_{ii22}^{V1,LR} - \frac{8}{9} L_{ii11}^{V,LR} - \frac{8}{9} L_{ii22}^{V,LR} + \frac{16}{9} L_{iii}^{V1,LR} + \frac{272}{27} L_{iii}^{V,LL} \Big] \\
& + \alpha_s^2 \Big[ \frac{70}{9} L_{ii11}^{V1,LL} + \frac{70}{9} L_{ii22}^{V1,LL} - \frac{94}{9} L_{ii11}^{V1,LR} - \frac{94}{9} L_{ii22}^{V1,LR} + \frac{841}{243} L_{ii11}^{V8,LL} \\
& + \frac{841}{243} L_{ii22}^{V8,LL} + \frac{211}{243} L_{ii11}^{V8,LR} + \frac{211}{243} L_{ii22}^{V8,LR} - \frac{94}{9} L_{iii}^{V1,LR} + \frac{211}{243} L_{iii}^{V8,LR} \\
& + \frac{4471}{81} L_{iii}^{V,LL} \Big] + \alpha_s \alpha \Big[ \frac{176}{243} L_{11ii}^{V,LL} + \frac{176}{243} L_{22ii}^{V,LL} - \frac{688}{243} L_{ii11}^{V1,LL} - \frac{688}{243} L_{ii22}^{V1,LL} \\
& - \frac{688}{243} L_{ii11}^{V1,LR} + \frac{1448}{243} L_{ii22}^{V1,LR} - \frac{1190}{729} L_{ii11}^{V8,LL} - \frac{1190}{729} L_{ii22}^{V8,LL} + \frac{1906}{729} L_{ii11}^{V8,LR} \\
& - \frac{5816}{729} L_{ii22}^{V8,LR} + \frac{176}{243} L_{ii11}^{V,LR} + \frac{176}{243} L_{ii22}^{V,LR} + \frac{1376}{243} L_{iii}^{V1,LR} - \frac{5816}{729} L_{iii}^{V8,LR} \\
& - \frac{8320}{243} L_{iii}^{V,LL} \Big] + \alpha^2 \Big[ \frac{2504}{729} L_{11ii}^{V,LL} + \frac{2504}{729} L_{22ii}^{V,LL} + \frac{1928}{729} L_{ii11}^{V1,LL} + \frac{1928}{729} L_{ii22}^{V1,LL} \\
& - \frac{2104}{729} L_{ii11}^{V1,LR} - \frac{12352}{729} L_{ii22}^{V1,LR} - \frac{9592}{729} L_{ii11}^{V,LR} - \frac{9592}{729} L_{ii22}^{V,LR} - \frac{11776}{729} L_{iii}^{V1,LR}
\end{aligned}$$

$$+ \frac{6496}{729} L_{iii}^{V,LL} \Big] ;$$

$$\begin{aligned} \dot{L}_{ijj}^{V,LL} = & e^2 \left[ \frac{40}{3} L_{ijj}^{V,LL} + \frac{1}{3} L_{ijj}^{V,LR} + \frac{1}{3} L_{ii1}^{V,LL} + \frac{1}{3} L_{ii2}^{V,LL} + \frac{1}{3} L_{ii1}^{V,LR} \right. \\ & + \frac{1}{3} L_{ii2}^{V,LR} + \frac{4}{3} L_{iii}^{V,LL} + \frac{1}{3} L_{iii}^{V,LR} - \frac{2}{3} L_{ii1}^{V,LL} - \frac{2}{3} L_{ii1}^{V,LR} + \frac{1}{3} L_{jj1}^{V,LL} \\ & + \frac{1}{3} L_{jj2}^{V,LL} + \frac{1}{3} L_{jj1}^{V,LR} + \frac{1}{3} L_{jj2}^{V,LR} + 2 L_{jjj}^{V,LL} + \frac{2}{3} L_{jjj}^{V,LR} - \frac{2}{3} L_{jj1}^{V,LL} \\ & \left. - \frac{2}{3} L_{jj1}^{V,LR} \right] + \alpha_s \alpha \left[ \frac{4}{3} L_{ii1}^{V,LL} + \frac{4}{3} L_{ii2}^{V,LL} + \frac{4}{3} L_{ii1}^{V,LR} + \frac{4}{3} L_{ii2}^{V,LR} \right. \\ & - \frac{8}{3} L_{ii1}^{V,LL} - \frac{8}{3} L_{ii1}^{V,LR} + \frac{4}{3} L_{jj1}^{V,LL} + \frac{4}{3} L_{jj2}^{V,LL} + \frac{4}{3} L_{jj1}^{V,LR} + \frac{4}{3} L_{jj2}^{V,LR} \\ & \left. - \frac{8}{3} L_{jj1}^{V,LL} - \frac{8}{3} L_{jj1}^{V,LR} \right] + \alpha^2 \left[ -\frac{2494}{27} L_{ijj}^{V,LL} - \frac{178}{27} L_{ijj}^{V,LR} + \frac{166}{81} L_{ii1}^{V,LL} \right. \\ & + \frac{166}{81} L_{ii2}^{V,LL} + \frac{34}{81} L_{ii1}^{V,LR} + \frac{34}{81} L_{ii2}^{V,LR} + \frac{320}{27} L_{iii}^{V,LL} - \frac{178}{27} L_{iii}^{V,LR} - \frac{314}{81} L_{ii1}^{V,LL} \\ & - \frac{842}{81} L_{ii1}^{V,LR} + \frac{166}{81} L_{jj1}^{V,LL} + \frac{166}{81} L_{jj2}^{V,LL} + \frac{34}{81} L_{jj1}^{V,LR} + \frac{34}{81} L_{jj2}^{V,LR} + \frac{52}{3} L_{jjj}^{V,LL} \\ & \left. - \frac{356}{27} L_{jjj}^{V,LR} - \frac{314}{81} L_{jj1}^{V,LL} - \frac{842}{81} L_{jj1}^{V,LR} \right] ; \end{aligned}$$

$$\begin{aligned} \dot{L}_{iii}^{V,LL} = & e^2 \left[ \frac{16}{3} L_{ijj}^{V,LL} + \frac{4}{3} L_{ijj}^{V,LR} + \frac{4}{3} L_{ii1}^{V,LL} + \frac{4}{3} L_{ii2}^{V,LL} + \frac{4}{3} L_{ii1}^{V,LR} \right. \\ & \left. + \frac{4}{3} L_{ii2}^{V,LR} + \frac{52}{3} L_{iii}^{V,LL} + \frac{4}{3} L_{iii}^{V,LR} - \frac{8}{3} L_{ii1}^{V,LL} - \frac{8}{3} L_{ii1}^{V,LR} \right] + \alpha_s \alpha \left[ \frac{16}{3} L_{ii1}^{V,LL} \right. \\ & + \frac{16}{3} L_{ii2}^{V,LL} + \frac{16}{3} L_{ii1}^{V,LR} + \frac{16}{3} L_{ii2}^{V,LR} - \frac{32}{3} L_{ii1}^{V,LL} - \frac{32}{3} L_{ii1}^{V,LR} \left. \right] + \alpha^2 \left[ \frac{1184}{27} L_{ijj}^{V,LL} \right. \\ & - \frac{712}{27} L_{ijj}^{V,LR} + \frac{664}{81} L_{ii1}^{V,LL} + \frac{664}{81} L_{ii2}^{V,LL} + \frac{136}{81} L_{ii1}^{V,LR} + \frac{136}{81} L_{ii2}^{V,LR} - \frac{1510}{27} L_{iii}^{V,LL} \\ & \left. - \frac{712}{27} L_{iii}^{V,LR} - \frac{1256}{81} L_{ii1}^{V,LL} - \frac{3368}{81} L_{ii1}^{V,LR} \right] ; \end{aligned}$$

$$\dot{L}_{ijj}^{V,LL} = 0 ;$$

$$\dot{L}_{\nu\nu iii}^{V,LL} = 0;$$

$$\begin{aligned} \dot{L}_{de ijj}^{V,LR} = & e^2 \left[ \frac{4}{3} L_{dd ijj}^{V1,LR} + \frac{8}{3} L_{dd ijj}^{V,LL} + \frac{8}{9} L_{dd ijj}^{V,LL} - 4 L_{de ijj}^{V,LR} + \frac{4}{3} L_{dd iii}^{V1,LR} \right. \\ & + \frac{32}{9} L_{dd iii}^{V,LL} + \frac{4}{3} L_{de i11}^{V,LR} + \frac{4}{3} L_{de i22}^{V,LR} - \frac{8}{3} L_{du i11}^{V1,LR} + \frac{4}{3} L_{ed 11ii}^{V,LL} + \frac{4}{3} L_{ed 22ii}^{V,LL} \\ & - \frac{8}{3} L_{ud 11ii}^{V1,LL} + \frac{4}{9} L_{de 11jj}^{V,LR} + \frac{4}{9} L_{de 22jj}^{V,LR} + \frac{4}{9} L_{ed jj11}^{V,RR} + \frac{4}{9} L_{ed jj22}^{V,RR} + \frac{8}{9} L_{jjjj}^{V,LR} \\ & \left. + \frac{8}{3} L_{jjjj}^{V,RR} - \frac{8}{9} L_{jj11}^{V,RR} - \frac{8}{9} L_{11jj}^{V,LR} \right] + \alpha_s^2 \left[ 8 L_{de 11jj}^{V,LR} + 8 L_{de 22jj}^{V,LR} \right. \\ & \left. - 8 L_{ed jj11}^{V,RR} - 8 L_{ed jj22}^{V,RR} - 8 L_{eu jj11}^{V,RR} + 8 L_{ue 11jj}^{V,LR} \right] + \alpha_s \alpha \left[ \frac{16}{3} L_{dd ijj}^{V1,LR} \right. \\ & - \frac{1022}{243} L_{dd ijj}^{V8,LR} + 8 L_{dd ijj}^{V,LL} + \frac{64}{243} L_{dd ijj}^{V,LL} + 16 L_{de ijj}^{V,LR} + \frac{16}{3} L_{dd iii}^{V1,LR} - \frac{1022}{243} L_{dd iii}^{V8,LR} \\ & + \frac{1048}{81} L_{dd iii}^{V,LL} - \frac{32}{3} L_{du i11}^{V1,LR} + \frac{1354}{243} L_{du i11}^{V8,LR} - \frac{32}{3} L_{ud 11ii}^{V1,LL} - \frac{86}{243} L_{ud 11ii}^{V8,LL} + \frac{16}{9} L_{de 11jj}^{V,LR} \\ & + \frac{16}{9} L_{de 22jj}^{V,LR} + \frac{16}{9} L_{ed jj11}^{V,RR} + \frac{16}{9} L_{ed jj22}^{V,RR} - \frac{32}{9} L_{eu jj11}^{V,RR} - \frac{32}{9} L_{ue 11jj}^{V,LR} \left. \right] + \alpha^2 \left[ \frac{1712}{243} L_{dd ijj}^{V1,LR} \right. \\ & + \frac{256}{243} L_{dd ijj}^{V,LL} - \frac{1424}{729} L_{dd ijj}^{V,LL} + \frac{430}{9} L_{de ijj}^{V,LR} + \frac{1712}{243} L_{dd iii}^{V1,LR} - \frac{800}{243} L_{dd iii}^{V,LL} \\ & + \frac{3728}{243} L_{de i11}^{V,LR} + \frac{3728}{243} L_{de i22}^{V,LR} - \frac{616}{243} L_{du i11}^{V1,LR} - \frac{1024}{243} L_{ed 11ii}^{V,LL} - \frac{1024}{243} L_{ed 22ii}^{V,LL} \\ & - \frac{6952}{243} L_{ud 11ii}^{V1,LL} - \frac{104}{243} L_{de 11jj}^{V,LR} - \frac{104}{243} L_{de 22jj}^{V,LR} - \frac{440}{243} L_{ed jj11}^{V,RR} - \frac{440}{243} L_{ed jj22}^{V,RR} \\ & \left. - \frac{368}{81} L_{jjjj}^{V,LR} - \frac{80}{9} L_{jjjj}^{V,RR} - \frac{1640}{243} L_{eu jj11}^{V,RR} - \frac{296}{243} L_{ue 11jj}^{V,LR} \right]; \end{aligned}$$

$$\begin{aligned} \dot{L}_{ue ijj}^{V,LR} = & e^2 \left[ 8 L_{ue ijj}^{V,LR} + \frac{4}{3} L_{eu 11ii}^{V,LL} + \frac{4}{3} L_{eu 22ii}^{V,LL} + \frac{4}{3} L_{ud i11}^{V1,LL} + \frac{4}{3} L_{ud i22}^{V1,LL} \right. \\ & + \frac{4}{3} L_{ud i11}^{V1,LR} + \frac{4}{3} L_{ud i22}^{V1,LR} + \frac{4}{3} L_{ue i11}^{V,LR} + \frac{4}{3} L_{ue i22}^{V,LR} - \frac{8}{3} L_{uu iii}^{V1,LR} - \frac{64}{9} L_{uu iii}^{V,LL} \\ & \left. - \frac{8}{9} L_{de 11jj}^{V,LR} - \frac{8}{9} L_{de 22jj}^{V,LR} - \frac{8}{9} L_{ed jj11}^{V,RR} - \frac{8}{9} L_{ed jj22}^{V,RR} - \frac{16}{9} L_{jjjj}^{V,LR} - \frac{16}{3} L_{jjjj}^{V,RR} \right] \end{aligned}$$

$$\begin{aligned}
& + \frac{16}{9} L_{jj11}^{V,RR} + \frac{16}{9} L_{11jj}^{V,LR} \Big] + \alpha_s^2 \Big[ 8L_{11jj}^{V,LR} + 8L_{22jj}^{V,LR} - 8L_{jj11}^{V,RR} \\
& - 8L_{jj22}^{V,RR} - 8L_{jj11}^{V,RR} + 8L_{11jj}^{V,LR} \Big] + \alpha_s \alpha \Big[ -32L_{ijjj}^{V,LR} + \frac{16}{3} L_{ii11}^{V1,LL} \\
& + \frac{16}{3} L_{ii22}^{V1,LL} + \frac{16}{3} L_{ii11}^{V1,LR} - \frac{32}{3} L_{ii22}^{V1,LR} + \frac{352}{243} L_{ii11}^{V8,LL} + \frac{352}{243} L_{ii22}^{V8,LL} - \frac{368}{243} L_{ii11}^{V8,LR} \\
& + \frac{2008}{243} L_{ii22}^{V8,LR} - \frac{32}{3} L_{iii}^{V1,LR} + \frac{2008}{243} L_{iii}^{V8,LR} - \frac{2144}{81} L_{iii}^{V,LL} - \frac{32}{9} L_{11jj}^{V,LR} - \frac{32}{9} L_{22jj}^{V,LR} \\
& - \frac{32}{9} L_{jj11}^{V,RR} - \frac{32}{9} L_{jj22}^{V,RR} + \frac{64}{9} L_{jj11}^{V,RR} + \frac{64}{9} L_{11jj}^{V,LR} \Big] + \alpha^2 \Big[ -\frac{1184}{9} L_{ijjj}^{V,LR} \\
& - \frac{4744}{243} L_{11ii}^{V,LL} - \frac{4744}{243} L_{22ii}^{V,LL} - \frac{3808}{243} L_{ii11}^{V1,LL} - \frac{3808}{243} L_{ii22}^{V1,LL} - \frac{1144}{243} L_{ii11}^{V1,LR} \\
& + \frac{12512}{243} L_{ii22}^{V1,LR} + \frac{3248}{243} L_{ii11}^{V,LR} + \frac{3248}{243} L_{ii22}^{V,LR} + \frac{12224}{243} L_{iii}^{V1,LR} + \frac{3808}{243} L_{iii}^{V,LL} \\
& + \frac{1792}{243} L_{11jj}^{V,LR} + \frac{1792}{243} L_{22jj}^{V,LR} + \frac{1168}{243} L_{jj11}^{V,RR} + \frac{1168}{243} L_{jj22}^{V,RR} + \frac{3616}{81} L_{jjjj}^{V,RR} \\
& + \frac{160}{9} L_{jjjj}^{V,RR} - \frac{1184}{243} L_{jj11}^{V,RR} + \frac{1312}{243} L_{11jj}^{V,LR} \Big] ;
\end{aligned}$$

$$\begin{aligned}
\dot{L}_{ijjj}^{V,LR} &= e^2 \Big[ \frac{4}{3} L_{ii11}^{V,LL} + \frac{4}{3} L_{ii22}^{V,LL} + \frac{4}{3} L_{ii11}^{V,LR} + \frac{4}{3} L_{ii22}^{V,LR} + \frac{4}{3} L_{ii11}^{V,LL} \\
& + \frac{4}{3} L_{ii22}^{V,LL} + \frac{4}{3} L_{ii11}^{V,LR} + \frac{4}{3} L_{ii22}^{V,LR} - \frac{8}{3} L_{ii11}^{V,LL} - \frac{8}{3} L_{ii11}^{V,LR} \Big] \\
& + \alpha_s \alpha \Big[ \frac{16}{3} L_{ii11}^{V,LL} + \frac{16}{3} L_{ii22}^{V,LL} + \frac{16}{3} L_{ii11}^{V,LR} + \frac{16}{3} L_{ii22}^{V,LR} - \frac{32}{3} L_{ii11}^{V,LL} \\
& - \frac{32}{3} L_{ii11}^{V,LR} \Big] + \alpha^2 \Big[ -\frac{32}{9} L_{ii11}^{V,LL} - \frac{32}{9} L_{ii22}^{V,LL} + \frac{40}{9} L_{ii11}^{V,LR} + \frac{40}{9} L_{ii22}^{V,LR} \\
& - 8L_{ii11}^{V,LL} - 8L_{ii22}^{V,LL} + 16L_{ii11}^{V,LR} + 16L_{ii22}^{V,LR} - \frac{176}{9} L_{ii11}^{V,LL} + \frac{112}{9} L_{ii11}^{V,LR} \Big] ;
\end{aligned}$$

$$\dot{L}_{ijjj}^{V,LR} = e^2 \Big[ \frac{4}{9} L_{ii11}^{V,LL} + \frac{4}{9} L_{ii22}^{V,LL} + \frac{4}{9} L_{ii11}^{V,LR} + \frac{4}{9} L_{ii22}^{V,LR} + \frac{4}{9} L_{ii11}^{V,LL}$$

$$\begin{aligned}
& + \frac{4}{9} L_{\nu e, ii22}^{V,LL} + \frac{4}{9} L_{\nu e, ii11}^{V,LR} + \frac{4}{9} L_{\nu e, ii22}^{V,LR} - \frac{8}{9} L_{\nu u, ii11}^{V,LL} - \frac{8}{9} L_{\nu u, ii11}^{V,LR} \Big] \\
& + \alpha_s^2 \Big[ -8 L_{\nu d, ii11}^{V,LL} - 8 L_{\nu d, ii22}^{V,LL} + 8 L_{\nu d, ii11}^{V,LR} + 8 L_{\nu d, ii22}^{V,LR} - 8 L_{\nu u, ii11}^{V,LL} \\
& + 8 L_{\nu u, ii11}^{V,LR} \Big] + \alpha_s \alpha \Big[ \frac{16}{9} L_{\nu d, ii11}^{V,LL} + \frac{16}{9} L_{\nu d, ii22}^{V,LL} + \frac{16}{9} L_{\nu d, ii11}^{V,LR} + \frac{16}{9} L_{\nu d, ii22}^{V,LR} \\
& - \frac{32}{9} L_{\nu u, ii11}^{V,LL} - \frac{32}{9} L_{\nu u, ii11}^{V,LR} \Big] + \alpha^2 \Big[ -\frac{8}{27} L_{\nu d, ii11}^{V,LL} - \frac{8}{27} L_{\nu d, ii22}^{V,LL} + \frac{16}{27} L_{\nu d, ii11}^{V,LR} \\
& + \frac{16}{27} L_{\nu d, ii22}^{V,LR} + \frac{8}{3} L_{\nu e, ii11}^{V,LR} + \frac{8}{3} L_{\nu e, ii22}^{V,LR} - \frac{80}{27} L_{\nu u, ii11}^{V,LL} + \frac{16}{27} L_{\nu u, ii11}^{V,LR} \Big] ; \\
\dot{L}_{\nu u, ij\bar{j}}^{V,LR} & = e^2 \Big[ -\frac{8}{9} L_{\nu d, ii11}^{V,LL} - \frac{8}{9} L_{\nu d, ii22}^{V,LL} - \frac{8}{9} L_{\nu d, ii11}^{V,LR} - \frac{8}{9} L_{\nu d, ii22}^{V,LR} - \frac{8}{9} L_{\nu e, ii11}^{V,LL} \\
& - \frac{8}{9} L_{\nu e, ii22}^{V,LL} - \frac{8}{9} L_{\nu e, ii11}^{V,LR} - \frac{8}{9} L_{\nu e, ii22}^{V,LR} + \frac{16}{9} L_{\nu u, ii11}^{V,LL} + \frac{16}{9} L_{\nu u, ii11}^{V,LR} \Big] \\
& + \alpha_s^2 \Big[ -8 L_{\nu d, ii11}^{V,LL} - 8 L_{\nu d, ii22}^{V,LL} + 8 L_{\nu d, ii11}^{V,LR} + 8 L_{\nu d, ii22}^{V,LR} - 8 L_{\nu u, ii11}^{V,LL} \\
& + 8 L_{\nu u, ii11}^{V,LR} \Big] + \alpha_s \alpha \Big[ -\frac{32}{9} L_{\nu d, ii11}^{V,LL} - \frac{32}{9} L_{\nu d, ii22}^{V,LL} - \frac{32}{9} L_{\nu d, ii11}^{V,LR} - \frac{32}{9} L_{\nu d, ii22}^{V,LR} \\
& + \frac{64}{9} L_{\nu u, ii11}^{V,LL} + \frac{64}{9} L_{\nu u, ii11}^{V,LR} \Big] + \alpha^2 \Big[ -\frac{56}{27} L_{\nu d, ii11}^{V,LL} - \frac{56}{27} L_{\nu d, ii22}^{V,LL} + \frac{40}{27} L_{\nu d, ii11}^{V,LR} \\
& + \frac{40}{27} L_{\nu d, ii22}^{V,LR} - 8 L_{\nu e, ii11}^{V,LL} - 8 L_{\nu e, ii22}^{V,LL} + \frac{8}{3} L_{\nu e, ii11}^{V,LR} + \frac{8}{3} L_{\nu e, ii22}^{V,LR} - \frac{128}{27} L_{\nu u, ii11}^{V,LL} \\
& + \frac{256}{27} L_{\nu u, ii11}^{V,LR} \Big] ; \\
\dot{L}_{du, ij\bar{j}}^{V1,LR} & = -\frac{8}{3} L_{du, ij\bar{j}}^{V8,LR} g_s^2 + e^2 \Big[ -\frac{8}{9} L_{dd, iii}^{V1,LR} - \frac{8}{9} L_{dd, ij\bar{j}}^{V1,LR} - \frac{64}{27} L_{dd, iii}^{V,LL} - \frac{16}{9} L_{dd, ij\bar{j}}^{V,LL} \\
& - \frac{16}{27} L_{dd, ij\bar{j}}^{V,LL} - \frac{8}{9} L_{de, ii11}^{V,LR} - \frac{8}{9} L_{de, ii22}^{V,LR} + \frac{4}{9} L_{du, 11j\bar{j}}^{V1,LR} + \frac{4}{9} L_{du, 22j\bar{j}}^{V1,LR} + \frac{16}{9} L_{du, ii11}^{V1,LR} \\
& + \frac{8}{3} L_{du, ij\bar{j}}^{V1,LR} - \frac{8}{9} L_{ed, 11ii}^{V,LL} - \frac{8}{9} L_{ed, 22ii}^{V,LL} + \frac{4}{9} L_{eu, 11j\bar{j}}^{V,LR} + \frac{4}{9} L_{eu, 22j\bar{j}}^{V,LR} + \frac{4}{9} L_{eu, 11j\bar{j}}^{V1,LR}
\end{aligned}$$

$$\begin{aligned}
& + \frac{4}{9} L_{22jj}^{V,RR} + \frac{16}{9} L_{11ii}^{V1,LL} + \frac{4}{9} L_{jj11}^{V1,RR} + \frac{4}{9} L_{jj22}^{V1,RR} - \frac{8}{9} L_{jjjj}^{V1,LR} - \frac{64}{27} L_{jjjj}^{V,RR} \Big] \\
& + \alpha_s^2 \Bigg[ 8 L_{iii}^{V1,LR} + 8 L_{ijj}^{V1,LR} + \frac{44}{27} L_{iii}^{V8,LR} + \frac{44}{27} L_{ijj}^{V8,LR} - \frac{232}{9} L_{iii}^{V,LL} \\
& - 16 L_{ijj}^{V,LL} - \frac{64}{27} L_{ijji}^{V,LL} + 8 L_{11jj}^{V1,LR} + 8 L_{22jj}^{V1,LR} + 8 L_{ii11}^{V1,LR} - \frac{28}{3} L_{ijj}^{V1,LR} \\
& + \frac{44}{27} L_{11jj}^{V8,LR} + \frac{44}{27} L_{22jj}^{V8,LR} + \frac{44}{27} L_{ii11}^{V8,LR} - \frac{2132}{27} L_{ijj}^{V8,LR} - 8 L_{11ii}^{V1,LL} - 8 L_{jj11}^{V1,RR} \\
& - 8 L_{jj22}^{V1,RR} + \frac{44}{27} L_{11ii}^{V8,LL} + \frac{44}{27} L_{jj11}^{V8,RR} + \frac{44}{27} L_{jj22}^{V8,RR} + 8 L_{jjjj}^{V1,LR} + \frac{44}{27} L_{jjjj}^{V8,LR} \\
& - \frac{232}{9} L_{jjjj}^{V,RR} \Big] + \alpha_s \alpha \Bigg[ - \frac{32}{9} L_{iii}^{V1,LR} - \frac{32}{9} L_{ijj}^{V1,LR} + \frac{2044}{729} L_{iii}^{V8,LR} + \frac{2044}{729} L_{ijj}^{V8,LR} \\
& - \frac{2096}{243} L_{iii}^{V,LL} - \frac{16}{3} L_{ijj}^{V,LL} - \frac{128}{729} L_{ijji}^{V,LL} + \frac{16}{9} L_{11jj}^{V1,LR} - \frac{32}{9} L_{22jj}^{V1,LR} + \frac{64}{9} L_{ii11}^{V1,LR} \\
& - \frac{64}{3} L_{ijj}^{V1,LR} - \frac{368}{729} L_{11jj}^{V8,LR} + \frac{2008}{729} L_{22jj}^{V8,LR} - \frac{2708}{729} L_{ii11}^{V8,LR} + \frac{232}{27} L_{ijj}^{V8,LR} \\
& + \frac{64}{9} L_{11ii}^{V1,LL} + \frac{16}{9} L_{jj11}^{V1,RR} + \frac{16}{9} L_{jj22}^{V1,RR} + \frac{172}{729} L_{11ii}^{V8,LL} + \frac{352}{729} L_{jj11}^{V8,RR} + \frac{352}{729} L_{jj22}^{V8,RR} \\
& - \frac{32}{9} L_{jjjj}^{V1,LR} + \frac{2008}{729} L_{jjjj}^{V8,LR} - \frac{2144}{243} L_{jjjj}^{V,RR} \Big] + \alpha^2 \Bigg[ \frac{3776}{729} L_{iii}^{V1,LR} + \frac{3776}{729} L_{ijj}^{V1,LR} \\
& + \frac{880}{729} L_{iii}^{V,LL} + \frac{928}{729} L_{ijj}^{V,LL} - \frac{32}{2187} L_{ijji}^{V,LL} + \frac{6224}{729} L_{ii11}^{V,LR} + \frac{6224}{729} L_{ii22}^{V,LR} \\
& - \frac{208}{729} L_{11jj}^{V1,LR} + \frac{6752}{729} L_{22jj}^{V1,LR} + \frac{6272}{729} L_{ii11}^{V1,LR} - \frac{880}{27} L_{ijj}^{V1,LR} - \frac{3712}{729} L_{11ii}^{V,LL} \\
& - \frac{3712}{729} L_{22ii}^{V,LL} + \frac{2888}{729} L_{11jj}^{V,LR} + \frac{2888}{729} L_{22jj}^{V,LR} - \frac{1216}{729} L_{11jj}^{V,RR} - \frac{1216}{729} L_{22jj}^{V,RR} \\
& - \frac{6976}{729} L_{11ii}^{V1,LL} - \frac{1576}{729} L_{jj11}^{V1,RR} - \frac{1576}{729} L_{jj22}^{V1,RR} + \frac{6464}{729} L_{jjjj}^{V1,LR} + \frac{4384}{729} L_{jjjj}^{V,RR} \Big] ;
\end{aligned}$$

$$\begin{aligned}
\dot{L}_{ijj}^{V8,LR} & = g_s^2 \Bigg[ \frac{2}{3} L_{ijj}^{V8,LR} + \frac{8}{3} L_{ijji}^{V,LL} - 12 L_{ijj}^{V1,LR} - 14 L_{ijj}^{V8,LR} + \frac{2}{3} L_{iii}^{V8,LR} \\
& + \frac{8}{3} L_{iii}^{V,LL} + \frac{2}{3} L_{ii11}^{V8,LR} + \frac{2}{3} L_{11ii}^{V8,LL} + \frac{2}{3} L_{11jj}^{V8,LR} + \frac{2}{3} L_{22jj}^{V8,LR} + \frac{2}{3} L_{jj11}^{V8,RR} \Big]
\end{aligned}$$

$$\begin{aligned}
& + \frac{2}{3} L_{jj22}^{V8,RR} + \frac{2}{3} L_{jjjj}^{V8,LR} + \frac{8}{3} L_{jjjj}^{V,RR} \Big] + \frac{8}{3} e^2 L_{ijjj}^{V8,LR} + \alpha_s^2 \Bigg[ - \frac{22}{3} L_{ijjj}^{V1,LR} \\
& + \frac{787}{81} L_{ijjj}^{V8,LR} - \frac{28}{3} L_{ijjj}^{V,LL} + \frac{3448}{81} L_{ijji}^{V,LL} - \frac{418}{3} L_{ijjj}^{V1,LR} - \frac{3067}{18} L_{ijjj}^{V8,LR} - \frac{22}{3} L_{iiii}^{V1,LR} \\
& + \frac{787}{81} L_{iiii}^{V8,LR} + \frac{1198}{27} L_{iiii}^{V,LL} - \frac{22}{3} L_{ii11}^{V1,LR} + \frac{787}{81} L_{ii11}^{V8,LR} - \frac{2}{3} L_{11ii}^{V1,LL} + \frac{607}{81} L_{11ii}^{V8,LL} \\
& - \frac{22}{3} L_{11jj}^{V1,LR} - \frac{22}{3} L_{22jj}^{V1,LR} + \frac{805}{81} L_{11jj}^{V8,LR} + \frac{805}{81} L_{22jj}^{V8,LR} - \frac{2}{3} L_{jj11}^{V1,RR} - \frac{2}{3} L_{jj22}^{V1,RR} \\
& + \frac{625}{81} L_{jj11}^{V8,RR} + \frac{625}{81} L_{jj22}^{V8,RR} - \frac{22}{3} L_{jjjj}^{V1,LR} + \frac{805}{81} L_{jjjj}^{V8,LR} + \frac{1222}{27} L_{jjjj}^{V,RR} \Big] \\
& + \alpha_s \alpha \Bigg[ - \frac{916}{81} L_{ijjj}^{V1,LR} - \frac{44}{9} L_{ijjj}^{V8,LR} - \frac{1832}{81} L_{ijjj}^{V,LL} + \frac{664}{243} L_{ijji}^{V,LL} + \frac{116}{3} L_{ijjj}^{V1,LR} \\
& + \frac{187}{9} L_{ijjj}^{V8,LR} - \frac{916}{81} L_{iiii}^{V1,LR} - \frac{44}{9} L_{iiii}^{V8,LR} - \frac{2144}{81} L_{iiii}^{V,LL} - \frac{916}{81} L_{ii11}^{V,LR} - \frac{916}{81} L_{ii22}^{V,LR} \\
& + \frac{1832}{81} L_{ii11}^{V1,LR} + \frac{56}{9} L_{ii11}^{V8,LR} - \frac{916}{81} L_{ii11}^{V,LL} - \frac{916}{81} L_{22ii}^{V,LL} + \frac{1832}{81} L_{11ii}^{V1,LL} - \frac{160}{27} L_{11ii}^{V8,LL} \\
& + \frac{644}{81} L_{11jj}^{V1,LR} - \frac{1216}{81} L_{22jj}^{V1,LR} + \frac{14}{9} L_{11jj}^{V8,LR} - \frac{20}{3} L_{22jj}^{V8,LR} + \frac{644}{81} L_{11jj}^{V,LR} + \frac{644}{81} L_{22jj}^{V,LR} \\
& + \frac{644}{81} L_{11jj}^{V,RR} + \frac{644}{81} L_{22jj}^{V,RR} + \frac{644}{81} L_{jj11}^{V1,RR} + \frac{644}{81} L_{jj22}^{V1,RR} - \frac{70}{27} L_{jj11}^{V8,RR} - \frac{70}{27} L_{jj22}^{V8,RR} \\
& - \frac{1288}{81} L_{jjjj}^{V1,LR} - \frac{20}{3} L_{jjjj}^{V8,LR} - \frac{3608}{81} L_{jjjj}^{V,RR} \Big] - \frac{880}{27} \alpha^2 L_{ijjj}^{V8,LR} ;
\end{aligned}$$

$$\begin{aligned}
\dot{L}_{jjii}^{V,LR} & = e^2 \Bigg[ - 4 L_{jjii}^{V,LR} + \frac{4}{9} L_{jjii}^{V,RR} + \frac{16}{9} L_{ijjj}^{V,RR} + \frac{4}{9} L_{11ii}^{V,LR} + \frac{4}{9} L_{22ii}^{V,LR} \\
& + \frac{4}{9} L_{ii11}^{V,RR} + \frac{4}{9} L_{ii22}^{V,RR} + \frac{4}{9} L_{ii11}^{V,LR} + \frac{16}{9} L_{iiii}^{V,RR} - \frac{8}{9} L_{ii11}^{V,RR} - \frac{8}{9} L_{11ii}^{V,LR} \\
& + \frac{8}{3} L_{jjjj}^{V1,LR} + \frac{64}{9} L_{jjjj}^{V,LL} + \frac{4}{3} L_{jj11}^{V,LR} + \frac{4}{3} L_{jj22}^{V,LR} - \frac{8}{3} L_{jj11}^{V1,LR} + \frac{4}{3} L_{11jj}^{V,LL} \\
& + \frac{4}{3} L_{22jj}^{V,LL} - \frac{8}{3} L_{11jj}^{V1,LL} \Big] + \alpha_s^2 \Bigg[ 8 L_{11ii}^{V,LR} + 8 L_{22ii}^{V,LR} - 8 L_{ii11}^{V,RR} \\
& - 8 L_{ed22}^{V,RR} - 8 L_{ii11}^{V,RR} + 8 L_{11ii}^{V,LR} \Big] + \alpha_s \alpha \Bigg[ 16 L_{jjii}^{V,LR} + \frac{16}{9} L_{11ii}^{V,LR}
\end{aligned}$$



$$\begin{aligned}
& + \frac{16}{9} L_{22ii}^{V,LR} + \frac{16}{9} L_{ii11}^{V,RR} + \frac{16}{9} L_{ii22}^{V,RR} - \frac{32}{9} L_{ii11}^{V,RR} - \frac{32}{9} L_{11ii}^{V,LR} + \frac{32}{3} L_{jjjj}^{V1,LR} \\
& - \frac{2044}{243} L_{jjjj}^{V8,LR} + \frac{5152}{243} L_{jjjj}^{V,LL} - \frac{32}{3} L_{jj11}^{V1,LR} + \frac{1354}{243} L_{jj11}^{V8,LR} - \frac{32}{3} L_{11jj}^{V1,LL} \\
& - \frac{86}{243} L_{11jj}^{V8,LL} \Big] + \alpha^2 \Big[ \frac{430}{9} L_{jjii}^{V,LR} - \frac{184}{81} L_{jjii}^{V,LR} - \frac{160}{81} L_{iijj}^{V,RR} - \frac{104}{243} L_{11ii}^{V,LR} \\
& - \frac{104}{243} L_{22ii}^{V,LR} - \frac{440}{243} L_{ii11}^{V,RR} - \frac{440}{243} L_{ii22}^{V,RR} - \frac{184}{81} L_{iii}^{V,LR} - \frac{640}{81} L_{iii}^{V,RR} - \frac{1640}{243} L_{ii11}^{V,RR} \\
& - \frac{296}{243} L_{11ii}^{V,LR} + \frac{3424}{243} L_{jjjj}^{V1,LR} - \frac{3056}{729} L_{jjjj}^{V,LL} + \frac{3728}{243} L_{jj11}^{V,LR} + \frac{3728}{243} L_{jj22}^{V,LR} \\
& - \frac{616}{243} L_{jj11}^{V1,LR} - \frac{1024}{243} L_{11jj}^{V,LL} - \frac{1024}{243} L_{22jj}^{V,LL} - \frac{6952}{243} L_{11jj}^{V1,LL} \Big] ; \\
\dot{L}_{jjii}^{V,LR} & = e^2 \Big[ -\frac{8}{9} L_{jjii}^{V,LR} - \frac{32}{9} L_{iijj}^{V,RR} + 8 L_{jjii}^{V,LR} - \frac{8}{9} L_{11ii}^{V,LR} - \frac{8}{9} L_{22ii}^{V,LR} \\
& - \frac{8}{9} L_{ii11}^{V,RR} - \frac{8}{9} L_{ii22}^{V,RR} - \frac{8}{9} L_{iii}^{V,LR} - \frac{32}{9} L_{iii}^{V,RR} + \frac{16}{9} L_{ii11}^{V,RR} + \frac{16}{9} L_{11ii}^{V,LR} \\
& + \frac{4}{3} L_{11jj}^{V,LL} + \frac{4}{3} L_{22jj}^{V,LL} + \frac{4}{3} L_{jj11}^{V1,LL} + \frac{4}{3} L_{jj22}^{V1,LL} + \frac{4}{3} L_{jj11}^{V1,LR} + \frac{4}{3} L_{jj22}^{V1,LR} \\
& + \frac{4}{3} L_{jj11}^{V,LR} + \frac{4}{3} L_{jj22}^{V,LR} - \frac{8}{3} L_{jjjj}^{V1,LR} - \frac{64}{9} L_{jjjj}^{V,LL} \Big] + \alpha_s^2 \Big[ 8 L_{11ii}^{V,LR} \\
& + 8 L_{22ii}^{V,LR} - 8 L_{ii11}^{V,RR} - 8 L_{ii22}^{V,RR} - 8 L_{iii}^{V,RR} + 8 L_{ii11}^{V,RR} + 8 L_{11ii}^{V,LR} \Big] + \alpha_s \alpha \Big[ -32 L_{jjii}^{V,LR} \\
& - \frac{32}{9} L_{11ii}^{V,LR} - \frac{32}{9} L_{22ii}^{V,LR} - \frac{32}{9} L_{ii11}^{V,RR} - \frac{32}{9} L_{ii22}^{V,RR} + \frac{64}{9} L_{ii11}^{V,RR} + \frac{64}{9} L_{11ii}^{V,LR} \\
& + \frac{16}{3} L_{jj11}^{V1,LL} + \frac{16}{3} L_{jj22}^{V1,LL} + \frac{16}{3} L_{jj11}^{V1,LR} - \frac{32}{3} L_{jj22}^{V1,LR} + \frac{352}{243} L_{jj11}^{V8,LL} + \frac{352}{243} L_{jj22}^{V8,LL} \\
& - \frac{368}{243} L_{jj11}^{V8,LR} + \frac{2008}{243} L_{jj22}^{V8,LR} - \frac{32}{3} L_{jjjj}^{V1,LR} + \frac{2008}{243} L_{jjjj}^{V8,LR} - \frac{2144}{81} L_{jjjj}^{V,LL} \Big] \\
& + \alpha^2 \Big[ \frac{1808}{81} L_{jjii}^{V,LR} + \frac{896}{81} L_{iijj}^{V,RR} - \frac{1184}{9} L_{jjii}^{V,LR} + \frac{1792}{243} L_{11ii}^{V,LR} + \frac{1792}{243} L_{22ii}^{V,LR} \\
& + \frac{1168}{243} L_{ii11}^{V,RR} + \frac{1168}{243} L_{ii22}^{V,RR} + \frac{1808}{81} L_{iii}^{V,LR} + \frac{992}{81} L_{iii}^{V,RR} - \frac{1184}{243} L_{ii11}^{V,RR}
\end{aligned}$$

$$\begin{aligned}
& + \frac{1312}{243} L_{11ii}^{V,LR} - \frac{4744}{243} L_{11jj}^{V,LL} - \frac{4744}{243} L_{22jj}^{V,LL} - \frac{3808}{243} L_{jj11}^{V1,LL} - \frac{3808}{243} L_{jj22}^{V1,LL} \\
& - \frac{1144}{243} L_{jj11}^{V1,LR} + \frac{12512}{243} L_{jj22}^{V1,LR} + \frac{3248}{243} L_{jj11}^{V,LR} + \frac{3248}{243} L_{jj22}^{V,LR} + \frac{12224}{243} L_{jjjj}^{V1,LR} \\
& + \frac{3808}{243} L_{jjjj}^{V,LL} \Big] ;
\end{aligned}$$

$$\begin{aligned}
\dot{L}_{jj\bar{i}}^{V,LR} &= e^2 \left[ \frac{4}{3} L_{jj11}^{V,LL} + \frac{4}{3} L_{jj22}^{V,LL} + \frac{4}{3} L_{jj11}^{V,LR} + \frac{4}{3} L_{jj22}^{V,LR} + \frac{4}{3} L_{jj11}^{V,LL} \right. \\
& + \frac{4}{3} L_{jj22}^{V,LL} + \frac{4}{3} L_{jj11}^{V,LR} + \frac{4}{3} L_{jj22}^{V,LR} - \frac{8}{3} L_{jj11}^{V,LL} - \frac{8}{3} L_{jj11}^{V,LR} \Big] \\
& + \alpha_s \alpha \left[ \frac{16}{3} L_{jj11}^{V,LL} + \frac{16}{3} L_{jj22}^{V,LL} + \frac{16}{3} L_{jj11}^{V,LR} + \frac{16}{3} L_{jj22}^{V,LR} - \frac{32}{3} L_{jj11}^{V,LL} \right. \\
& - \frac{32}{3} L_{jj11}^{V,LR} \Big] + \alpha^2 \left[ -\frac{32}{9} L_{jj11}^{V,LL} - \frac{32}{9} L_{jj22}^{V,LL} + \frac{40}{9} L_{jj11}^{V,LR} + \frac{40}{9} L_{jj22}^{V,LR} \right. \\
& - 8 L_{jj11}^{V,LL} - 8 L_{jj22}^{V,LL} + 16 L_{jj11}^{V,LR} + 16 L_{jj22}^{V,LR} - \frac{176}{9} L_{jj11}^{V,LL} + \frac{112}{9} L_{jj11}^{V,LR} \Big] ;
\end{aligned}$$

$$\begin{aligned}
\dot{L}_{jj\bar{i}}^{V,LR} &= e^2 \left[ \frac{4}{9} L_{jj11}^{V,LL} + \frac{4}{9} L_{jj22}^{V,LL} + \frac{4}{9} L_{jj11}^{V,LR} + \frac{4}{9} L_{jj22}^{V,LR} + \frac{4}{9} L_{jj11}^{V,LL} \right. \\
& + \frac{4}{9} L_{jj22}^{V,LL} + \frac{4}{9} L_{jj11}^{V,LR} + \frac{4}{9} L_{jj22}^{V,LR} - \frac{8}{9} L_{jj11}^{V,LL} - \frac{8}{9} L_{jj11}^{V,LR} \Big] \\
& + \alpha_s^2 \left[ -8 L_{jj11}^{V,LL} - 8 L_{jj22}^{V,LL} + 8 L_{jj11}^{V,LR} + 8 L_{jj22}^{V,LR} - 8 L_{jj11}^{V,LL} \right. \\
& + 8 L_{jj11}^{V,LR} \Big] + \alpha_s \alpha \left[ \frac{16}{9} L_{jj11}^{V,LL} + \frac{16}{9} L_{jj22}^{V,LL} + \frac{16}{9} L_{jj11}^{V,LR} + \frac{16}{9} L_{jj22}^{V,LR} \right. \\
& - \frac{32}{9} L_{jj11}^{V,LL} - \frac{32}{9} L_{jj11}^{V,LR} \Big] + \alpha^2 \left[ -\frac{8}{27} L_{jj11}^{V,LL} - \frac{8}{27} L_{jj22}^{V,LL} + \frac{16}{27} L_{jj11}^{V,LR} \right. \\
& + \frac{16}{27} L_{jj22}^{V,LR} + \frac{8}{3} L_{jj11}^{V,LR} + \frac{8}{3} L_{jj22}^{V,LR} - \frac{80}{27} L_{jj11}^{V,LL} + \frac{16}{27} L_{jj11}^{V,LR} \Big] ;
\end{aligned}$$

$$\dot{L}_{jj\bar{i}}^{V,LR} = e^2 \left[ -\frac{8}{9} L_{jj11}^{V,LL} - \frac{8}{9} L_{jj22}^{V,LL} - \frac{8}{9} L_{jj11}^{V,LR} - \frac{8}{9} L_{jj22}^{V,LR} - \frac{8}{9} L_{jj11}^{V,LL} \right]$$

$$\begin{aligned}
& -\frac{8}{9}L_{jj22}^{V,LL} - \frac{8}{9}L_{jj11}^{V,LR} - \frac{8}{9}L_{jj22}^{V,LR} + \frac{16}{9}L_{jj11}^{V,LL} + \frac{16}{9}L_{jj11}^{V,LR} \Big] \\
& + \alpha_s^2 \Big[ -8L_{jj11}^{V,LL} - 8L_{jj22}^{V,LL} + 8L_{jj11}^{V,LR} + 8L_{jj22}^{V,LR} - 8L_{jj11}^{V,LL} \\
& + 8L_{jj11}^{V,LR} \Big] + \alpha_s \alpha \Big[ -\frac{32}{9}L_{jj11}^{V,LL} - \frac{32}{9}L_{jj22}^{V,LL} - \frac{32}{9}L_{jj11}^{V,LR} - \frac{32}{9}L_{jj22}^{V,LR} \\
& + \frac{64}{9}L_{jj11}^{V,LL} + \frac{64}{9}L_{jj11}^{V,LR} \Big] + \alpha^2 \Big[ -\frac{56}{27}L_{jj11}^{V,LL} - \frac{56}{27}L_{jj22}^{V,LL} + \frac{40}{27}L_{jj11}^{V,LR} \\
& + \frac{40}{27}L_{jj22}^{V,LR} - 8L_{jj11}^{V,LL} - 8L_{jj22}^{V,LL} + \frac{8}{3}L_{jj11}^{V,LR} + \frac{8}{3}L_{jj22}^{V,LR} - \frac{128}{27}L_{jj11}^{V,LL} \\
& + \frac{256}{27}L_{jj11}^{V,LR} \Big] ;
\end{aligned}$$

$$\begin{aligned}
\dot{L}_{jjii}^{V1,LR} = & -\frac{8}{3}g_s^2 L_{jjii}^{V8,LR} + e^2 \Big[ \frac{8}{3}L_{jjii}^{V1,LR} + \frac{4}{9}L_{11ii}^{V1,LR} + \frac{4}{9}L_{22ii}^{V1,LR} + \frac{4}{9}L_{11ii}^{V,LR} \\
& + \frac{4}{9}L_{22ii}^{V,LR} + \frac{4}{9}L_{11ii}^{V,RR} + \frac{4}{9}L_{22ii}^{V,RR} + \frac{4}{9}L_{ii11}^{V1,RR} + \frac{4}{9}L_{ii22}^{V1,RR} - \frac{8}{9}L_{iii}^{V1,LR} \\
& - \frac{64}{27}L_{iii}^{V,RR} - \frac{16}{9}L_{jjj}^{V1,LR} - \frac{128}{27}L_{jjj}^{V,LL} - \frac{8}{9}L_{jj11}^{V,LR} - \frac{8}{9}L_{jj22}^{V,LR} + \frac{16}{9}L_{jj11}^{V1,LR} \\
& - \frac{8}{9}L_{11jj}^{V,LL} - \frac{8}{9}L_{22jj}^{V,LL} + \frac{16}{9}L_{11jj}^{V1,LL} \Big] + \alpha_s^2 \Big[ -\frac{28}{3}L_{jjii}^{V1,LR} - \frac{2132}{27}L_{jjii}^{V8,LR} \\
& + 8L_{11ii}^{V1,LR} + 8L_{22ii}^{V1,LR} + \frac{44}{27}L_{11ii}^{V8,LR} + \frac{44}{27}L_{22ii}^{V8,LR} - 8L_{ii11}^{V1,RR} - 8L_{ii22}^{V1,RR} \\
& + \frac{44}{27}L_{ii11}^{V8,RR} + \frac{44}{27}L_{ii22}^{V8,RR} + 8L_{iii}^{V1,LR} + \frac{44}{27}L_{iii}^{V8,LR} - \frac{232}{9}L_{iii}^{V,RR} + 16L_{jjj}^{V1,LR} \\
& + \frac{88}{27}L_{jjj}^{V8,LR} - \frac{1192}{27}L_{jjj}^{V,LL} + 8L_{jj11}^{V1,LR} + \frac{44}{27}L_{jj11}^{V8,LR} - 8L_{11jj}^{V1,LL} + \frac{44}{27}L_{11jj}^{V8,LL} \Big] \\
& + \alpha_s \alpha \Big[ -\frac{64}{3}L_{jjii}^{V1,LR} + \frac{232}{27}L_{jjii}^{V8,LR} + \frac{16}{9}L_{11ii}^{V1,LR} - \frac{32}{9}L_{22ii}^{V1,LR} - \frac{368}{729}L_{11ii}^{V8,LR} \\
& + \frac{2008}{729}L_{22ii}^{V8,LR} + \frac{16}{9}L_{ii11}^{V1,RR} + \frac{16}{9}L_{ii22}^{V1,RR} + \frac{352}{729}L_{ii11}^{V8,RR} + \frac{352}{729}L_{ii22}^{V8,RR} - \frac{32}{9}L_{iii}^{V1,LR} \\
& + \frac{2008}{729}L_{iii}^{V8,LR} - \frac{2144}{243}L_{iii}^{V,RR} - \frac{64}{9}L_{jjj}^{V1,LR} + \frac{4088}{729}L_{jjj}^{V8,LR} - \frac{10304}{729}L_{jjj}^{V,LL}
\end{aligned}$$

$$\begin{aligned}
& + \frac{64}{9} L_{jj11}^{V1,LR} - \frac{2708}{729} L_{jj11}^{V8,LR} + \frac{64}{9} L_{11jj}^{V1,LL} + \frac{172}{729} L_{11jj}^{V8,LL} \Big] + \alpha^2 \Big[ - \frac{880}{27} L_{jjii}^{V1,LR} \\
& - \frac{208}{729} L_{11ii}^{V1,LR} + \frac{6752}{729} L_{22ii}^{V1,LR} + \frac{2888}{729} L_{11ii}^{V,LR} + \frac{2888}{729} L_{22ii}^{V,LR} - \frac{1216}{729} L_{11ii}^{V,RR} \\
& - \frac{1216}{729} L_{22ii}^{V,RR} - \frac{1576}{729} L_{ii11}^{V1,RR} - \frac{1576}{729} L_{ii22}^{V1,RR} + \frac{6464}{729} L_{iii}^{V1,LR} + \frac{4384}{729} L_{iii}^{V,RR} \\
& + \frac{7552}{729} L_{jjjj}^{V1,LR} + \frac{5392}{2187} L_{jjjj}^{V,LL} + \frac{6224}{729} L_{jj11}^{V,LR} + \frac{6224}{729} L_{jj22}^{V,LR} + \frac{6272}{729} L_{jj11}^{V1,LR} \\
& - \frac{3712}{729} L_{11jj}^{V,LL} - \frac{3712}{729} L_{22jj}^{V,LL} - \frac{6976}{729} L_{11jj}^{V1,LL} \Big] ;
\end{aligned}$$

$$\begin{aligned}
\dot{L}_{jjii}^{V8,LR} &= g_s^2 \Big[ -12 L_{jjii}^{V1,LR} - 14 L_{jjii}^{V8,LR} + \frac{2}{3} L_{11ii}^{V8,LR} + \frac{2}{3} L_{22ii}^{V8,LR} + \frac{2}{3} L_{ii11}^{V8,RR} \\
& + \frac{2}{3} L_{ii22}^{V8,RR} + \frac{2}{3} L_{iii}^{V8,LR} + \frac{8}{3} L_{iii}^{V,RR} + \frac{4}{3} L_{jjjj}^{V8,LR} + \frac{16}{3} L_{jjjj}^{V,LL} + \frac{2}{3} L_{jj11}^{V8,LR} \\
& + \frac{2}{3} L_{11jj}^{V8,LL} \Big] + \frac{8}{3} e^2 L_{jjii}^{V8,LR} + \alpha_s^2 \Big[ - \frac{418}{3} L_{jjii}^{V1,LR} - \frac{3067}{18} L_{jjii}^{V8,LR} - \frac{22}{3} L_{11ii}^{V1,LR} \\
& - \frac{22}{3} L_{22ii}^{V1,LR} + \frac{805}{81} L_{11ii}^{V8,LR} + \frac{805}{81} L_{22ii}^{V8,LR} - \frac{2}{3} L_{ii11}^{V1,RR} - \frac{2}{3} L_{ii22}^{V1,RR} + \frac{625}{81} L_{ii11}^{V8,RR} \\
& + \frac{625}{81} L_{ii22}^{V8,RR} - \frac{22}{3} L_{iii}^{V1,LR} + \frac{805}{81} L_{iii}^{V8,LR} + \frac{1222}{27} L_{iii}^{V,RR} - \frac{44}{3} L_{jjjj}^{V1,LR} + \frac{1574}{81} L_{jjjj}^{V8,LR} \\
& + \frac{6286}{81} L_{jjjj}^{V,LL} - \frac{22}{3} L_{jj11}^{V1,LR} + \frac{787}{81} L_{jj11}^{V8,LR} - \frac{2}{3} L_{11jj}^{V1,LL} + \frac{607}{81} L_{11jj}^{V8,LL} \Big] \\
& + \alpha_s \alpha \Big[ \frac{116}{3} L_{jjii}^{V1,LR} + \frac{187}{9} L_{jjii}^{V8,LR} + \frac{644}{81} L_{11ii}^{V1,LR} - \frac{1216}{81} L_{22ii}^{V1,LR} + \frac{14}{9} L_{11ii}^{V8,LR} \\
& - \frac{20}{3} L_{22ii}^{V8,LR} + \frac{644}{81} L_{11ii}^{V,LR} + \frac{644}{81} L_{22ii}^{V,LR} + \frac{644}{81} L_{11ii}^{V,RR} + \frac{644}{81} L_{22ii}^{V,RR} + \frac{644}{81} L_{ii11}^{V1,RR} \\
& + \frac{644}{81} L_{ii22}^{V1,RR} - \frac{70}{27} L_{ii11}^{V8,RR} - \frac{70}{27} L_{ii22}^{V8,RR} - \frac{1288}{81} L_{iii}^{V1,LR} - \frac{20}{3} L_{iii}^{V8,LR} - \frac{3608}{81} L_{iii}^{V,RR} \\
& - \frac{1832}{81} L_{jjjj}^{V1,LR} - \frac{88}{9} L_{jjjj}^{V8,LR} - \frac{11264}{243} L_{jjjj}^{V,LL} - \frac{916}{81} L_{jj11}^{V,LR} - \frac{916}{81} L_{jj22}^{V,LR} + \frac{1832}{81} L_{jj11}^{V1,LR} \\
& + \frac{56}{9} L_{jj11}^{V8,LR} - \frac{916}{81} L_{11jj}^{V,LL} - \frac{916}{81} L_{22jj}^{V,LL} + \frac{1832}{81} L_{11jj}^{V1,LL} - \frac{160}{27} L_{11jj}^{V8,LL} \Big]
\end{aligned}$$

$$\begin{aligned}
& -\frac{880}{27}\alpha^2 L_{jj\bar{i}\bar{i}}^{V8,LR}; \\
\dot{L}_{dd\bar{i}\bar{j}\bar{j}}^{V1,LR} = & -\frac{8}{3}g_s^2 L_{\bar{i}\bar{j}\bar{j}}^{V8,LR} + e^2 \left[ -\frac{8}{9}L_{\bar{i}\bar{j}\bar{j}}^{V1,LR} + \frac{8}{9}L_{\bar{i}\bar{j}\bar{j}}^{V,LL} + \frac{8}{27}L_{\bar{i}\bar{j}\bar{j}i}^{V,LL} + \frac{4}{9}L_{\bar{i}\bar{i}\bar{i}}^{V1,LR} \right. \\
& + \frac{32}{27}L_{\bar{i}\bar{i}\bar{i}}^{V,LL} + \frac{4}{9}L_{\bar{i}i11}^{V,LR} + \frac{4}{9}L_{\bar{i}i22}^{V,LR} - \frac{8}{9}L_{\bar{i}i11}^{V1,LR} + \frac{4}{9}L_{11\bar{i}\bar{i}}^{V,LL} + \frac{4}{9}L_{22\bar{i}\bar{i}}^{V,LL} \\
& - \frac{8}{9}L_{11\bar{i}\bar{i}}^{V1,LL} + \frac{8}{9}L_{\bar{j}\bar{j}\bar{j}}^{V1,LR} + \frac{64}{27}L_{\bar{j}\bar{j}\bar{j}}^{V,RR} + \frac{4}{9}L_{\bar{j}\bar{j}\bar{j}}^{V,LR} + \frac{4}{9}L_{22\bar{j}\bar{j}}^{V,LR} + \frac{4}{9}L_{11\bar{j}\bar{j}}^{V,RR} \\
& + \frac{4}{9}L_{22\bar{j}\bar{j}}^{V,RR} - \frac{8}{9}L_{\bar{j}\bar{j}\bar{j}}^{V1,LR} - \frac{8}{9}L_{\bar{j}\bar{j}\bar{j}}^{V1,RR} \left. \right] + \alpha_s^2 \left[ -\frac{4}{3}L_{\bar{i}\bar{j}\bar{j}}^{V1,LR} - \frac{232}{3}L_{\bar{i}\bar{j}\bar{j}}^{V8,LR} \right. \\
& - 16L_{\bar{i}\bar{j}\bar{j}}^{V,LL} - \frac{64}{27}L_{\bar{i}\bar{j}\bar{j}i}^{V,LL} + 8L_{\bar{i}\bar{i}\bar{i}}^{V1,LR} + \frac{44}{27}L_{\bar{i}\bar{i}\bar{i}}^{V8,LR} - \frac{232}{9}L_{\bar{i}\bar{i}\bar{i}}^{V,LL} + 8L_{\bar{i}i11}^{V1,LR} \\
& + \frac{44}{27}L_{\bar{i}i11}^{V8,LR} - 8L_{11\bar{i}\bar{i}}^{V1,LL} + \frac{44}{27}L_{\bar{i}i11}^{V8,LL} + 16L_{\bar{j}\bar{j}\bar{j}}^{V1,LR} + \frac{88}{27}L_{\bar{j}\bar{j}\bar{j}}^{V8,LR} - \frac{1192}{27}L_{\bar{j}\bar{j}\bar{j}}^{V,RR} \\
& + 8L_{\bar{j}\bar{j}\bar{j}}^{V1,LR} - 8L_{\bar{j}\bar{j}\bar{j}}^{V1,RR} + \frac{44}{27}L_{\bar{j}\bar{j}\bar{j}}^{V8,LR} + \frac{44}{27}L_{\bar{j}\bar{j}\bar{j}}^{V8,RR} \left. \right] + \alpha_s \alpha \left[ \frac{112}{9}L_{\bar{i}\bar{j}\bar{j}}^{V1,LR} \right. \\
& - \frac{1238}{729}L_{\bar{i}\bar{j}\bar{j}}^{V8,LR} + \frac{8}{3}L_{\bar{i}\bar{j}\bar{j}}^{V,LL} + \frac{64}{729}L_{\bar{i}\bar{j}\bar{j}i}^{V,LL} + \frac{16}{9}L_{\bar{i}\bar{i}\bar{i}}^{V1,LR} - \frac{1022}{729}L_{\bar{i}\bar{i}\bar{i}}^{V8,LR} + \frac{1048}{243}L_{\bar{i}\bar{i}\bar{i}}^{V,LL} \\
& - \frac{32}{9}L_{\bar{i}i11}^{V1,LR} + \frac{1354}{729}L_{\bar{i}i11}^{V8,LR} - \frac{32}{9}L_{\bar{i}i11}^{V1,LL} - \frac{86}{729}L_{11\bar{i}\bar{i}}^{V8,LL} + \frac{32}{9}L_{\bar{j}\bar{j}\bar{j}}^{V1,LR} - \frac{2044}{729}L_{\bar{j}\bar{j}\bar{j}}^{V8,LR} \\
& + \frac{5152}{729}L_{\bar{j}\bar{j}\bar{j}}^{V,RR} - \frac{32}{9}L_{\bar{j}\bar{j}\bar{j}}^{V1,LR} - \frac{32}{9}L_{\bar{j}\bar{j}\bar{j}}^{V1,RR} + \frac{1354}{729}L_{\bar{j}\bar{j}\bar{j}}^{V8,LR} - \frac{86}{729}L_{\bar{j}\bar{j}\bar{j}}^{V8,RR} \left. \right] \\
& + \alpha^2 \left[ \frac{10046}{729}L_{\bar{i}\bar{j}\bar{j}}^{V1,LR} - \frac{32}{729}L_{\bar{i}\bar{j}\bar{j}}^{V,LL} - \frac{848}{2187}L_{\bar{i}\bar{j}\bar{j}i}^{V,LL} + \frac{272}{729}L_{\bar{i}\bar{i}\bar{i}}^{V1,LR} - \frac{656}{729}L_{\bar{i}\bar{i}\bar{i}}^{V,LL} \right. \\
& + \frac{992}{729}L_{\bar{i}i11}^{V,LR} + \frac{992}{729}L_{\bar{i}i22}^{V,LR} - \frac{1624}{729}L_{\bar{i}i11}^{V1,LR} + \frac{128}{729}L_{11\bar{i}\bar{i}}^{V,LL} + \frac{128}{729}L_{22\bar{i}\bar{i}}^{V,LL} \\
& - \frac{2776}{729}L_{11\bar{i}\bar{i}}^{V1,LL} + \frac{544}{729}L_{\bar{j}\bar{j}\bar{j}}^{V1,LR} - \frac{2912}{2187}L_{\bar{j}\bar{j}\bar{j}}^{V,RR} + \frac{992}{729}L_{\bar{j}\bar{j}\bar{j}}^{V,LR} + \frac{992}{729}L_{22\bar{j}\bar{j}}^{V,LR} \\
& + \frac{128}{729}L_{11\bar{j}\bar{j}}^{V,RR} + \frac{128}{729}L_{22\bar{j}\bar{j}}^{V,RR} - \frac{1624}{729}L_{\bar{j}\bar{j}\bar{j}}^{V1,LR} - \frac{2776}{729}L_{\bar{j}\bar{j}\bar{j}}^{V1,RR} \left. \right]; \\
\dot{L}_{dd\bar{i}\bar{j}\bar{j}}^{V8,LR} = & g_s^2 \left[ -12L_{\bar{i}\bar{j}\bar{j}}^{V1,LR} - \frac{40}{3}L_{\bar{i}\bar{j}\bar{j}}^{V8,LR} + \frac{8}{3}L_{\bar{i}\bar{j}\bar{j}i}^{V,LL} + \frac{2}{3}L_{\bar{i}\bar{i}\bar{i}}^{V8,LR} + \frac{8}{3}L_{\bar{i}\bar{i}\bar{i}}^{V,LL} \right.
\end{aligned}$$

$$\begin{aligned}
& + \frac{2}{3} L_{\frac{du}{ii11}}^{V8,LR} + \frac{2}{3} L_{\frac{dd}{11ii}}^{V8,LL} + \frac{4}{3} L_{\frac{dd}{jjjj}}^{V8,LR} + \frac{16}{3} L_{\frac{dd}{jjjj}}^{V,RR} + \frac{2}{3} L_{\frac{ud}{11jj}}^{V8,LR} + \frac{2}{3} L_{\frac{ud}{11jj}}^{V8,RR} \Big] \\
& - \frac{4}{3} e^2 L_{\frac{dd}{ijjj}}^{V8,LR} + \alpha_s^2 \Bigg[ - \frac{440}{3} L_{\frac{dd}{ijjj}}^{V1,LR} - \frac{26029}{162} L_{\frac{dd}{ijjj}}^{V8,LR} - \frac{28}{3} L_{\frac{dd}{ijjj}}^{V,LL} + \frac{3448}{81} L_{\frac{dd}{ijji}}^{V,LL} \\
& - \frac{22}{3} L_{\frac{dd}{iiii}}^{V1,LR} + \frac{787}{81} L_{\frac{dd}{iiii}}^{V8,LR} + \frac{1198}{27} L_{\frac{dd}{iiii}}^{V,LL} - \frac{22}{3} L_{\frac{du}{ii11}}^{V1,LR} + \frac{787}{81} L_{\frac{du}{ii11}}^{V8,LR} - \frac{2}{3} L_{\frac{ud}{11ii}}^{V1,LL} \\
& + \frac{607}{81} L_{\frac{ud}{11ii}}^{V8,LL} - \frac{44}{3} L_{\frac{dd}{jjjj}}^{V1,LR} + \frac{1574}{81} L_{\frac{dd}{jjjj}}^{V8,LR} + \frac{6286}{81} L_{\frac{dd}{jjjj}}^{V,RR} - \frac{22}{3} L_{\frac{ud}{11jj}}^{V1,LR} - \frac{2}{3} L_{\frac{ud}{11jj}}^{V1,RR} \\
& + \frac{787}{81} L_{\frac{ud}{11jj}}^{V8,LR} + \frac{607}{81} L_{\frac{ud}{11jj}}^{V8,RR} \Bigg] + \alpha_s \alpha \Bigg[ \frac{164}{81} L_{\frac{dd}{ijjj}}^{V1,LR} - \frac{4}{3} L_{\frac{dd}{ijjj}}^{V8,LR} + \frac{544}{81} L_{\frac{dd}{ijji}}^{V,LL} \\
& - \frac{1064}{243} L_{\frac{dd}{ijji}}^{V,LL} + \frac{272}{81} L_{\frac{dd}{iiii}}^{V1,LR} + \frac{14}{9} L_{\frac{dd}{iiii}}^{V8,LR} + \frac{340}{81} L_{\frac{dd}{iiii}}^{V,LL} + \frac{272}{81} L_{\frac{de}{ii11}}^{V,LR} + \frac{272}{81} L_{\frac{de}{ii22}}^{V,LR} \\
& - \frac{544}{81} L_{\frac{du}{ii11}}^{V1,LR} + \frac{2}{3} L_{\frac{du}{ii11}}^{V8,LR} + \frac{272}{81} L_{\frac{ed}{11ii}}^{V,LL} + \frac{272}{81} L_{\frac{ed}{22ii}}^{V,LL} - \frac{544}{81} L_{\frac{ud}{11ii}}^{V1,LL} + \frac{122}{27} L_{\frac{ud}{11ii}}^{V8,LL} \\
& + \frac{544}{81} L_{\frac{dd}{jjjj}}^{V1,LR} + \frac{28}{9} L_{\frac{dd}{jjjj}}^{V8,LR} + \frac{1588}{243} L_{\frac{dd}{jjjj}}^{V,RR} + \frac{272}{81} L_{\frac{ed}{11jj}}^{V,LR} + \frac{272}{81} L_{\frac{ed}{22jj}}^{V,LR} + \frac{272}{81} L_{\frac{ed}{11jj}}^{V,RR} \\
& + \frac{272}{81} L_{\frac{ed}{22jj}}^{V,RR} - \frac{544}{81} L_{\frac{ud}{11jj}}^{V1,LR} - \frac{544}{81} L_{\frac{ud}{11jj}}^{V1,RR} + \frac{2}{3} L_{\frac{ud}{11jj}}^{V8,LR} + \frac{122}{27} L_{\frac{ud}{11jj}}^{V8,RR} \Bigg] \\
& + \frac{362}{27} \alpha^2 L_{\frac{dd}{ijjj}}^{V8,LR} ;
\end{aligned}$$

$$\begin{aligned}
\dot{L}_{\frac{dd}{iiii}}^{V1,LR} = & - \frac{8}{3} g_s^2 L_{\frac{dd}{iiii}}^{V8,LR} + e^2 \Bigg[ \frac{4}{9} L_{\frac{dd}{ijjj}}^{V1,LR} + \frac{4}{9} L_{\frac{dd}{jjii}}^{V1,LR} + \frac{8}{9} L_{\frac{dd}{ijjj}}^{V,LL} + \frac{8}{27} L_{\frac{dd}{ijji}}^{V,LL} \\
& + \frac{8}{9} L_{\frac{dd}{ijjj}}^{V,RR} + \frac{8}{27} L_{\frac{dd}{ijji}}^{V,RR} - \frac{4}{9} L_{\frac{dd}{iiii}}^{V1,LR} + \frac{32}{27} L_{\frac{dd}{iiii}}^{V,LL} + \frac{32}{27} L_{\frac{dd}{iiii}}^{V,RR} + \frac{4}{9} L_{\frac{de}{ii11}}^{V,LR} \\
& + \frac{4}{9} L_{\frac{de}{ii22}}^{V,LR} - \frac{8}{9} L_{\frac{du}{ii11}}^{V1,LR} + \frac{4}{9} L_{\frac{ed}{11ii}}^{V,LL} + \frac{4}{9} L_{\frac{ed}{22ii}}^{V,LL} + \frac{4}{9} L_{\frac{ed}{11ii}}^{V,LR} + \frac{4}{9} L_{\frac{ed}{22ii}}^{V,LR} \\
& + \frac{4}{9} L_{\frac{ed}{11ii}}^{V,RR} + \frac{4}{9} L_{\frac{ed}{22ii}}^{V,RR} - \frac{8}{9} L_{\frac{ud}{11ii}}^{V1,LL} - \frac{8}{9} L_{\frac{ud}{11ii}}^{V1,LR} - \frac{8}{9} L_{\frac{ud}{11ii}}^{V1,RR} \Bigg] + \alpha_s^2 \Bigg[ 8 L_{\frac{dd}{ijjj}}^{V1,LR} \\
& + 8 L_{\frac{dd}{jjii}}^{V1,LR} + \frac{44}{27} L_{\frac{dd}{ijjj}}^{V8,LR} + \frac{44}{27} L_{\frac{dd}{jjii}}^{V8,LR} - 16 L_{\frac{dd}{ijjj}}^{V,LL} - \frac{64}{27} L_{\frac{dd}{ijji}}^{V,LL} - 16 L_{\frac{dd}{ijjj}}^{V,RR} \\
& - \frac{64}{27} L_{\frac{dd}{ijji}}^{V,RR} + \frac{20}{3} L_{\frac{dd}{iiii}}^{V1,LR} - \frac{2044}{27} L_{\frac{dd}{iiii}}^{V8,LR} - \frac{232}{9} L_{\frac{dd}{iiii}}^{V,LL} - \frac{232}{9} L_{\frac{dd}{iiii}}^{V,RR} + 8 L_{\frac{du}{ii11}}^{V1,LR} \\
& + \frac{44}{27} L_{\frac{du}{ii11}}^{V8,LR} - 8 L_{\frac{ud}{11ii}}^{V1,LL} + 8 L_{\frac{ud}{11ii}}^{V1,LR} - 8 L_{\frac{ud}{11ii}}^{V1,RR} + \frac{44}{27} L_{\frac{ud}{11ii}}^{V8,LL} + \frac{44}{27} L_{\frac{ud}{11ii}}^{V8,LR}
\end{aligned}$$

$$\begin{aligned}
& + \frac{44}{27} L_{11ii}^{V8,RR} \Big] + \alpha_s \alpha \Bigg[ \frac{16}{9} L_{ijj}^{V1,LR} + \frac{16}{9} L_{jji}^{V1,LR} - \frac{1022}{729} L_{ijj}^{V8,LR} - \frac{1022}{729} L_{jji}^{V8,LR} \\
& + \frac{8}{3} L_{ijj}^{V,LL} + \frac{64}{729} L_{ijji}^{V,LL} + \frac{8}{3} L_{ijj}^{V,RR} + \frac{64}{729} L_{ijji}^{V,RR} + \frac{128}{9} L_{iii}^{V1,LR} - \frac{2260}{729} L_{iii}^{V8,LR} \\
& + \frac{1048}{243} L_{iii}^{V,LL} + \frac{1048}{243} L_{iii}^{V,RR} - \frac{32}{9} L_{ii11}^{V1,LR} + \frac{1354}{729} L_{ii11}^{V8,LR} - \frac{32}{9} L_{11ii}^{V1,LL} - \frac{32}{9} L_{11ii}^{V1,LR} \\
& - \frac{32}{9} L_{11ii}^{V1,RR} - \frac{86}{729} L_{11ii}^{V8,LL} + \frac{1354}{729} L_{11ii}^{V8,LR} - \frac{86}{729} L_{11ii}^{V8,RR} \Big] + \alpha^2 \Bigg[ \frac{272}{729} L_{ijj}^{V1,LR} \\
& + \frac{272}{729} L_{jji}^{V1,LR} - \frac{32}{729} L_{ijj}^{V,LL} - \frac{848}{2187} L_{ijji}^{V,LL} - \frac{32}{729} L_{ijj}^{V,RR} - \frac{848}{2187} L_{ijji}^{V,RR} \\
& + \frac{10318}{729} L_{iii}^{V1,LR} - \frac{656}{729} L_{iii}^{V,LL} - \frac{656}{729} L_{iii}^{V,RR} + \frac{992}{729} L_{ii11}^{V,LR} + \frac{992}{729} L_{ii22}^{V,LR} \\
& - \frac{1624}{729} L_{ii11}^{V1,LR} + \frac{128}{729} L_{11ii}^{V,LL} + \frac{128}{729} L_{22ii}^{V,LL} + \frac{992}{729} L_{11ii}^{V,LR} + \frac{992}{729} L_{22ii}^{V,LR} \\
& + \frac{128}{729} L_{11ii}^{V,RR} + \frac{128}{729} L_{22ii}^{V,RR} - \frac{2776}{729} L_{11ii}^{V1,LL} - \frac{1624}{729} L_{11ii}^{V1,LR} - \frac{2776}{729} L_{11ii}^{V1,RR} \Big] ;
\end{aligned}$$

$$\begin{aligned}
\dot{L}_{iii}^{V8,LR} &= g_s^2 \Bigg[ \frac{2}{3} L_{ijj}^{V8,LR} + \frac{2}{3} L_{jji}^{V8,LR} + \frac{8}{3} L_{ijji}^{V,LL} + \frac{8}{3} L_{ijji}^{V,RR} - 12 L_{iii}^{V1,LR} \\
& - \frac{38}{3} L_{iii}^{V8,LR} + \frac{8}{3} L_{iii}^{V,LL} + \frac{8}{3} L_{iii}^{V,RR} + \frac{2}{3} L_{ii11}^{V8,LR} + \frac{2}{3} L_{11ii}^{V8,LL} + \frac{2}{3} L_{11ii}^{V8,LR} \\
& + \frac{2}{3} L_{11ii}^{V8,RR} \Big] - \frac{4}{3} e^2 L_{iii}^{V8,LR} + \alpha_s^2 \Bigg[ - \frac{22}{3} L_{ijj}^{V1,LR} - \frac{22}{3} L_{jji}^{V1,LR} + \frac{787}{81} L_{ijj}^{V8,LR} \\
& + \frac{787}{81} L_{jji}^{V8,LR} - \frac{28}{3} L_{ijj}^{V,LL} + \frac{3448}{81} L_{ijji}^{V,LL} - \frac{28}{3} L_{ijj}^{V,RR} + \frac{3448}{81} L_{ijji}^{V,RR} - 154 L_{iii}^{V1,LR} \\
& - \frac{24455}{162} L_{iii}^{V8,LR} + \frac{1198}{27} L_{iii}^{V,LL} + \frac{1198}{27} L_{iii}^{V,RR} - \frac{22}{3} L_{ii11}^{V1,LR} + \frac{787}{81} L_{ii11}^{V8,LR} \\
& - \frac{2}{3} L_{11ii}^{V1,LL} - \frac{22}{3} L_{11ii}^{V1,LR} - \frac{2}{3} L_{11ii}^{V1,RR} + \frac{607}{81} L_{11ii}^{V8,LL} + \frac{787}{81} L_{11ii}^{V8,LR} + \frac{607}{81} L_{11ii}^{V8,RR} \Big] \\
& + \alpha_s \alpha \Bigg[ \frac{272}{81} L_{ijj}^{V1,LR} + \frac{272}{81} L_{jji}^{V1,LR} + \frac{14}{9} L_{ijj}^{V8,LR} + \frac{14}{9} L_{jji}^{V8,LR} + \frac{544}{81} L_{ijj}^{V,LL} \\
& - \frac{1064}{243} L_{ijji}^{V,LL} + \frac{544}{81} L_{ijji}^{V,RR} - \frac{1064}{243} L_{ijji}^{V,RR} + \frac{436}{81} L_{iii}^{V1,LR} + \frac{2}{9} L_{iii}^{V8,LR} + \frac{340}{81} L_{iii}^{V,LL}
\end{aligned}$$

$$\begin{aligned}
& + \frac{340}{81} L_{iii}^{V,RR} + \frac{272}{81} L_{ii1}^{V,LR} + \frac{272}{81} L_{ii2}^{V,LR} - \frac{544}{81} L_{ii1}^{V1,LR} + \frac{2}{3} L_{ii1}^{V8,LR} + \frac{272}{81} L_{1ii}^{V,LL} \\
& + \frac{272}{81} L_{2ii}^{V,LL} + \frac{272}{81} L_{1ii}^{V,LR} + \frac{272}{81} L_{2ii}^{V,LR} + \frac{272}{81} L_{1ii}^{V,RR} + \frac{272}{81} L_{2ii}^{V,RR} - \frac{544}{81} L_{1ii}^{V1,LL} \\
& - \frac{544}{81} L_{1ii}^{V1,LR} - \frac{544}{81} L_{1ii}^{V1,RR} + \frac{122}{27} L_{1ii}^{V8,LL} + \frac{2}{3} L_{1ii}^{V8,LR} + \frac{122}{27} L_{1ii}^{V8,RR} \Big] \\
& + \frac{362}{27} \alpha^2 L_{iii}^{V8,LR} ; \\
\dot{L}_{iii}^{V1,LR} = & - \frac{8}{3} g_s^2 L_{iii}^{V8,LR} + e^2 \Bigg[ - \frac{8}{9} L_{1ii}^{V1,LR} - \frac{8}{9} L_{2ii}^{V1,LR} - \frac{8}{9} L_{1ii}^{V1,LL} - \frac{8}{9} L_{2ii}^{V1,LL} \\
& - \frac{8}{9} L_{1ii}^{V,LR} - \frac{8}{9} L_{2ii}^{V,LR} - \frac{8}{9} L_{1ii}^{V,RR} - \frac{8}{9} L_{2ii}^{V,RR} - \frac{8}{9} L_{ii1}^{V1,LL} - \frac{8}{9} L_{ii2}^{V1,LL} \\
& - \frac{8}{9} L_{ii1}^{V1,LR} - \frac{8}{9} L_{ii2}^{V1,LR} - \frac{8}{9} L_{ii1}^{V1,RR} - \frac{8}{9} L_{ii2}^{V1,RR} - \frac{8}{9} L_{ii1}^{V,LR} - \frac{8}{9} L_{ii2}^{V,LR} \\
& - \frac{16}{9} L_{iii}^{V1,LR} + \frac{128}{27} L_{iii}^{V,LL} + \frac{128}{27} L_{iii}^{V,RR} \Big] + \alpha_s^2 \Bigg[ 8 L_{1ii}^{V1,LR} + 8 L_{2ii}^{V1,LR} \\
& + \frac{44}{27} L_{1ii}^{V8,LR} + \frac{44}{27} L_{2ii}^{V8,LR} - 8 L_{ii1}^{V1,LL} - 8 L_{ii2}^{V1,LL} + 8 L_{ii1}^{V1,LR} + 8 L_{ii2}^{V1,LR} \\
& - 8 L_{ii1}^{V1,RR} - 8 L_{ii2}^{V1,RR} + \frac{44}{27} L_{ii1}^{V8,LL} + \frac{44}{27} L_{ii2}^{V8,LL} + \frac{44}{27} L_{ii1}^{V8,LR} + \frac{44}{27} L_{ii2}^{V8,LR} \\
& + \frac{44}{27} L_{ii1}^{V8,RR} + \frac{44}{27} L_{ii2}^{V8,RR} + \frac{20}{3} L_{iii}^{V1,LR} - \frac{2044}{27} L_{iii}^{V8,LR} - \frac{232}{9} L_{iii}^{V1,LL} - \frac{232}{9} L_{iii}^{V,RR} \Big] \\
& + \alpha_s \alpha \Bigg[ - \frac{32}{9} L_{1ii}^{V1,LR} + \frac{64}{9} L_{2ii}^{V1,LR} + \frac{736}{729} L_{1ii}^{V8,LR} - \frac{4016}{729} L_{2ii}^{V8,LR} - \frac{32}{9} L_{ii1}^{V1,LL} \\
& - \frac{32}{9} L_{ii2}^{V1,LL} - \frac{32}{9} L_{ii1}^{V1,LR} + \frac{64}{9} L_{ii2}^{V1,LR} - \frac{32}{9} L_{ii1}^{V1,RR} - \frac{32}{9} L_{ii2}^{V1,RR} - \frac{704}{729} L_{ii1}^{V8,LL} \\
& - \frac{704}{729} L_{ii2}^{V8,LL} + \frac{736}{729} L_{ii1}^{V8,LR} - \frac{4016}{729} L_{ii2}^{V8,LR} - \frac{704}{729} L_{ii1}^{V8,RR} - \frac{704}{729} L_{ii2}^{V8,RR} \\
& + \frac{512}{9} L_{iii}^{V1,LR} - \frac{8896}{729} L_{iii}^{V8,LR} + \frac{4288}{243} L_{iii}^{V,LL} + \frac{4288}{243} L_{iii}^{V,RR} \Big] + \alpha^2 \Bigg[ - \frac{2392}{729} L_{1ii}^{V1,LR} \\
& + \frac{3776}{729} L_{2ii}^{V1,LR} - \frac{8152}{729} L_{1ii}^{V,LL} - \frac{8152}{729} L_{2ii}^{V,LL} - \frac{4696}{729} L_{1ii}^{V,LR} - \frac{4696}{729} L_{2ii}^{V,LR} \\
& - \frac{8152}{729} L_{1ii}^{V,RR} - \frac{8152}{729} L_{2ii}^{V,RR} - \frac{3544}{729} L_{ii1}^{V1,LL} - \frac{3544}{729} L_{ii2}^{V1,LL} - \frac{2392}{729} L_{ii1}^{V1,LR}
\end{aligned}$$



$$\begin{aligned}
& + \frac{3776}{729} L_{ud\,ii22}^{V1,LR} - \frac{3544}{729} L_{ud\,ii11}^{V1,RR} - \frac{3544}{729} L_{ud\,ii22}^{V1,RR} - \frac{4696}{729} L_{ue\,ii11}^{V,LR} - \frac{4696}{729} L_{ue\,ii22}^{V,LR} \\
& + \frac{51040}{729} L_{uu\,iii}^{V1,LR} - \frac{10496}{729} L_{uu\,iii}^{V,LL} - \frac{10496}{729} L_{uu\,iii}^{V,RR} \Big] ; \\
\dot{L}_{uu\,iii}^{V8,LR} = & g_s^2 \left[ \frac{2}{3} L_{du\,11ii}^{V8,LR} + \frac{2}{3} L_{du\,22ii}^{V8,LR} + \frac{2}{3} L_{ud\,ii11}^{V8,LL} + \frac{2}{3} L_{ud\,ii22}^{V8,LL} + \frac{2}{3} L_{ud\,ii11}^{V8,LR} \right. \\
& + \frac{2}{3} L_{ud\,ii22}^{V8,LR} + \frac{2}{3} L_{ud\,ii11}^{V8,RR} + \frac{2}{3} L_{ud\,ii22}^{V8,RR} - 12 L_{uu\,iii}^{V1,LR} - \frac{38}{3} L_{uu\,iii}^{V8,LR} + \frac{8}{3} L_{uu\,iii}^{V,LL} \\
& + \left. \frac{8}{3} L_{uu\,iii}^{V,RR} \right] - \frac{16}{3} e^2 L_{uu\,iii}^{V8,LR} + \alpha_s^2 \left[ -\frac{22}{3} L_{du\,11ii}^{V1,LR} - \frac{22}{3} L_{du\,22ii}^{V1,LR} + \frac{805}{81} L_{du\,11ii}^{V8,LR} \right. \\
& + \frac{805}{81} L_{du\,22ii}^{V8,LR} - \frac{2}{3} L_{ud\,ii11}^{V1,LL} - \frac{2}{3} L_{ud\,ii22}^{V1,LL} - \frac{22}{3} L_{ud\,ii11}^{V1,LR} - \frac{22}{3} L_{ud\,ii22}^{V1,LR} - \frac{2}{3} L_{ud\,ii11}^{V1,RR} \\
& - \frac{2}{3} L_{ud\,ii22}^{V1,RR} + \frac{625}{81} L_{ud\,ii11}^{V8,LL} + \frac{625}{81} L_{ud\,ii22}^{V8,LL} + \frac{805}{81} L_{ud\,ii11}^{V8,LR} + \frac{805}{81} L_{ud\,ii22}^{V8,LR} + \frac{625}{81} L_{ud\,ii11}^{V8,RR} \\
& + \left. \frac{625}{81} L_{ud\,ii22}^{V8,RR} - 154 L_{uu\,iii}^{V1,LR} - \frac{24383}{162} L_{uu\,iii}^{V8,LR} + \frac{1222}{27} L_{uu\,iii}^{V,LL} + \frac{1222}{27} L_{uu\,iii}^{V,RR} \right] \\
& + \alpha_s \alpha \left[ -\frac{544}{81} L_{du\,11ii}^{V1,LR} + \frac{1160}{81} L_{du\,22ii}^{V1,LR} + \frac{22}{9} L_{du\,11ii}^{V8,LR} + \frac{56}{9} L_{du\,22ii}^{V8,LR} - \frac{544}{81} L_{eu\,11ii}^{V,LL} \right. \\
& - \frac{544}{81} L_{eu\,22ii}^{V,LL} - \frac{544}{81} L_{eu\,11ii}^{V,LR} - \frac{544}{81} L_{eu\,22ii}^{V,LR} - \frac{544}{81} L_{eu\,11ii}^{V,RR} - \frac{544}{81} L_{eu\,22ii}^{V,RR} - \frac{544}{81} L_{ud\,ii11}^{V1,LL} \\
& - \frac{544}{81} L_{ud\,ii22}^{V1,LL} - \frac{544}{81} L_{ud\,ii11}^{V1,LR} + \frac{1160}{81} L_{ud\,ii22}^{V1,LR} - \frac{544}{81} L_{ud\,ii11}^{V1,RR} - \frac{544}{81} L_{ud\,ii22}^{V1,RR} \\
& + \frac{170}{27} L_{ud\,ii11}^{V8,LL} + \frac{170}{27} L_{ud\,ii22}^{V8,LL} + \frac{22}{9} L_{ud\,ii11}^{V8,LR} + \frac{56}{9} L_{ud\,ii22}^{V8,LR} + \frac{170}{27} L_{ud\,ii11}^{V8,RR} + \frac{170}{27} L_{ud\,ii22}^{V8,RR} \\
& - \frac{544}{81} L_{ue\,ii11}^{V,LR} - \frac{544}{81} L_{ue\,ii22}^{V,LR} + \frac{1744}{81} L_{uu\,iii}^{V1,LR} + \frac{8}{9} L_{uu\,iii}^{V8,LR} + \frac{1360}{81} L_{uu\,iii}^{V,LL} + \frac{1360}{81} L_{uu\,iii}^{V,RR} \Big] \\
& + \frac{1568}{27} \alpha^2 L_{uu\,iii}^{V8,LR} ; \\
\dot{L}_{ee\,ijj}^{V,LR} = & e^2 \left[ \frac{16}{3} L_{ee\,ijj}^{V,LL} - \frac{32}{3} L_{ee\,ijj}^{V,LR} + \frac{4}{3} L_{ed\,ii11}^{V,LL} + \frac{4}{3} L_{ed\,ii22}^{V,LL} + \frac{4}{3} L_{ed\,ii11}^{V,LR} \right. \\
& + \frac{4}{3} L_{ed\,ii22}^{V,LR} + \frac{16}{3} L_{ee\,iii}^{V,LL} + \frac{4}{3} L_{ee\,iii}^{V,LR} - \frac{8}{3} L_{eu\,ii11}^{V,LL} - \frac{8}{3} L_{eu\,ii11}^{V,LR} + \frac{4}{3} L_{de\,11jj}^{V,LR} \\
& + \left. \frac{4}{3} L_{de\,22jj}^{V,LR} \right]
\end{aligned}$$

$$\begin{aligned}
& + \frac{4}{3}L_{22jj}^{V,LR} + \frac{4}{3}L_{jj11}^{V,RR} + \frac{4}{3}L_{jj22}^{V,RR} + \frac{8}{3}L_{jjjj}^{V,LR} + 8L_{jjjj}^{V,RR} - \frac{8}{3}L_{jj11}^{V,RR} \\
& - \frac{8}{3}L_{11jj}^{V,LR} \Big] + \alpha_s \alpha \left[ \frac{16}{3}L_{ii11}^{V,LL} + \frac{16}{3}L_{ii22}^{V,LL} + \frac{16}{3}L_{ii11}^{V,LR} + \frac{16}{3}L_{ii22}^{V,LR} \right. \\
& - \frac{32}{3}L_{ii11}^{V,LL} - \frac{32}{3}L_{ii11}^{V,LR} + \frac{16}{3}L_{11jj}^{V,LR} + \frac{16}{3}L_{22jj}^{V,LR} + \frac{16}{3}L_{jj11}^{V,RR} + \frac{16}{3}L_{jj22}^{V,RR} \\
& \left. - \frac{32}{3}L_{jj11}^{V,RR} - \frac{32}{3}L_{11jj}^{V,LR} \right] + \alpha^2 \left[ \frac{32}{27}L_{iijj}^{V,LL} + \frac{4274}{27}L_{iijj}^{V,LR} - \frac{344}{81}L_{ii11}^{V,LL} \right. \\
& - \frac{344}{81}L_{ii22}^{V,LL} + \frac{424}{81}L_{ii11}^{V,LR} + \frac{424}{81}L_{ii22}^{V,LR} - \frac{736}{27}L_{iii}^{V,LL} + \frac{296}{27}L_{iii}^{V,LR} - \frac{3128}{81}L_{ii11}^{V,LL} \\
& - \frac{56}{81}L_{ii11}^{V,LR} + \frac{424}{81}L_{11jj}^{V,LR} + \frac{424}{81}L_{22jj}^{V,LR} - \frac{344}{81}L_{jj11}^{V,RR} - \frac{344}{81}L_{jj22}^{V,RR} + \frac{592}{27}L_{jjjj}^{V,LR} \\
& \left. - \frac{80}{3}L_{jjjj}^{V,RR} - \frac{3128}{81}L_{jj11}^{V,RR} - \frac{56}{81}L_{11jj}^{V,LR} \right] ;
\end{aligned}$$

$$\begin{aligned}
\dot{L}_{ee}^{V,LR} = & e^2 \left[ \frac{16}{3}L_{iijj}^{V,LL} + \frac{4}{3}L_{iijj}^{V,LR} + \frac{4}{3}L_{jjii}^{V,LR} + \frac{16}{3}L_{iijj}^{V,RR} + \frac{4}{3}L_{11ii}^{V,LR} \right. \\
& + \frac{4}{3}L_{22ii}^{V,LR} + \frac{4}{3}L_{ii11}^{V,LL} + \frac{4}{3}L_{ii22}^{V,LL} + \frac{4}{3}L_{ii11}^{V,LR} + \frac{4}{3}L_{ii22}^{V,LR} + \frac{4}{3}L_{ii11}^{V,RR} \\
& + \frac{4}{3}L_{ii22}^{V,RR} + \frac{16}{3}L_{iii}^{V,LL} - \frac{28}{3}L_{iii}^{V,LR} + \frac{16}{3}L_{iii}^{V,RR} - \frac{8}{3}L_{ii11}^{V,LL} - \frac{8}{3}L_{ii11}^{V,LR} \\
& \left. - \frac{8}{3}L_{ii11}^{V,RR} - \frac{8}{3}L_{11ii}^{V,LR} \right] + \alpha_s \alpha \left[ \frac{16}{3}L_{11ii}^{V,LR} + \frac{16}{3}L_{22ii}^{V,LR} + \frac{16}{3}L_{ii11}^{V,LL} \right. \\
& + \frac{16}{3}L_{ii22}^{V,LL} + \frac{16}{3}L_{ii11}^{V,LR} + \frac{16}{3}L_{ii22}^{V,LR} + \frac{16}{3}L_{ii11}^{V,RR} + \frac{16}{3}L_{ii22}^{V,RR} - \frac{32}{3}L_{ii11}^{V,LL} \\
& \left. - \frac{32}{3}L_{ii11}^{V,LR} - \frac{32}{3}L_{ii11}^{V,RR} - \frac{32}{3}L_{11ii}^{V,LR} \right] + \alpha^2 \left[ \frac{32}{27}L_{iijj}^{V,LL} + \frac{296}{27}L_{iijj}^{V,LR} \right. \\
& + \frac{296}{27}L_{jjii}^{V,LR} + \frac{32}{27}L_{iijj}^{V,RR} + \frac{424}{81}L_{11ii}^{V,LR} + \frac{424}{81}L_{22ii}^{V,LR} - \frac{344}{81}L_{ii11}^{V,LL} - \frac{344}{81}L_{ii22}^{V,LL} \\
& + \frac{424}{81}L_{ii11}^{V,LR} + \frac{424}{81}L_{ii22}^{V,LR} - \frac{344}{81}L_{ii11}^{V,RR} - \frac{344}{81}L_{ii22}^{V,RR} - \frac{736}{27}L_{iii}^{V,LL} + \frac{4570}{27}L_{iii}^{V,LR} \\
& \left. - \frac{736}{27}L_{iii}^{V,RR} - \frac{3128}{81}L_{ii11}^{V,LL} - \frac{56}{81}L_{ii11}^{V,LR} - \frac{3128}{81}L_{ii11}^{V,RR} - \frac{56}{81}L_{11ii}^{V,LR} \right] ;
\end{aligned}$$

$$\begin{aligned}
\dot{L}_{ijj}^{V,RR} = & e^2 \left[ 4L_{ijj}^{V,RR} + \frac{4}{9}L_{jji}^{V,LR} + \frac{16}{9}L_{ijj}^{V,RR} + \frac{4}{9}L_{11ii}^{V,LR} + \frac{4}{9}L_{22ii}^{V,LR} \right. \\
& + \frac{4}{9}L_{ii11}^{V,RR} + \frac{4}{9}L_{ed}^{V,RR} + \frac{4}{9}L_{iii}^{V,LR} + \frac{16}{9}L_{iii}^{V,RR} - \frac{8}{9}L_{ii11}^{V,RR} - \frac{8}{9}L_{ue}^{V,LR} \\
& + \frac{8}{3}L_{jjj}^{V1,LR} + \frac{64}{9}L_{jjj}^{V,RR} + \frac{4}{3}L_{11jj}^{V,LR} + \frac{4}{3}L_{22jj}^{V,LR} + \frac{4}{3}L_{11jj}^{V,RR} + \frac{4}{3}L_{22jj}^{V,RR} \\
& \left. - \frac{8}{3}L_{11jj}^{V1,LR} - \frac{8}{3}L_{11jj}^{V1,RR} \right] + \alpha_s^2 \left[ -8L_{11ii}^{V,LR} - 8L_{22ii}^{V,LR} + 8L_{ii11}^{V,RR} \right. \\
& + 8L_{ii22}^{V,RR} + 8L_{ii11}^{V,RR} - 8L_{ue}^{V,LR} \left. \right] + \alpha_s \alpha \left[ -16L_{ijj}^{V,RR} + \frac{16}{9}L_{11ii}^{V,LR} \right. \\
& + \frac{16}{9}L_{22ii}^{V,LR} + \frac{16}{9}L_{ii11}^{V,RR} + \frac{16}{9}L_{ed}^{V,RR} - \frac{32}{9}L_{ii11}^{V,RR} - \frac{32}{9}L_{ue}^{V,LR} + \frac{32}{3}L_{jjj}^{V1,LR} \\
& - \frac{2044}{243}L_{jjj}^{V8,LR} + \frac{5152}{243}L_{jjj}^{V,RR} - \frac{32}{3}L_{11jj}^{V1,LR} - \frac{32}{3}L_{11jj}^{V1,RR} + \frac{1354}{243}L_{11jj}^{V8,LR} \\
& \left. - \frac{86}{243}L_{11jj}^{V8,RR} \right] + \alpha^2 \left[ -\frac{130}{9}L_{ijj}^{V,RR} - \frac{520}{81}L_{jji}^{V,LR} + \frac{224}{81}L_{ijj}^{V,RR} - \frac{200}{243}L_{11ii}^{V,LR} \right. \\
& - \frac{200}{243}L_{22ii}^{V,LR} - \frac{104}{243}L_{ii11}^{V,RR} - \frac{104}{243}L_{ii22}^{V,RR} - \frac{520}{81}L_{iii}^{V,LR} + \frac{32}{81}L_{iii}^{V,RR} - \frac{1016}{243}L_{ii11}^{V,RR} \\
& - \frac{1400}{243}L_{11ii}^{V,LR} - \frac{2624}{243}L_{jjj}^{V1,LR} + \frac{23296}{729}L_{jjj}^{V,RR} - \frac{3184}{243}L_{11jj}^{V,LR} - \frac{3184}{243}L_{22jj}^{V,LR} \\
& \left. + \frac{3728}{243}L_{11jj}^{V,RR} + \frac{3728}{243}L_{22jj}^{V,RR} - \frac{6232}{243}L_{11jj}^{V1,LR} + \frac{2984}{243}L_{11jj}^{V1,RR} \right] ;
\end{aligned}$$

$$\begin{aligned}
\dot{L}_{ijj}^{V,RR} = & e^2 \left[ -\frac{8}{9}L_{jji}^{V,LR} - \frac{32}{9}L_{ijj}^{V,RR} - 8L_{ijj}^{V,RR} - \frac{8}{9}L_{11ii}^{V,LR} - \frac{8}{9}L_{22ii}^{V,LR} \right. \\
& - \frac{8}{9}L_{ii11}^{V,RR} - \frac{8}{9}L_{ed}^{V,RR} - \frac{8}{9}L_{iii}^{V,LR} - \frac{32}{9}L_{iii}^{V,RR} + \frac{16}{9}L_{ii11}^{V,RR} + \frac{16}{9}L_{11ii}^{V,LR} \\
& + \frac{4}{3}L_{11jj}^{V1,LR} + \frac{4}{3}L_{22jj}^{V1,LR} + \frac{4}{3}L_{11jj}^{V,LR} + \frac{4}{3}L_{22jj}^{V,LR} + \frac{4}{3}L_{11jj}^{V,RR} + \frac{4}{3}L_{22jj}^{V,RR} \\
& \left. + \frac{4}{3}L_{11jj}^{V1,RR} + \frac{4}{3}L_{22jj}^{V1,RR} - \frac{8}{3}L_{jjj}^{V1,LR} - \frac{64}{9}L_{jjj}^{V,RR} \right] + \alpha_s^2 \left[ -8L_{11ii}^{V,LR} \right. \\
& \left. - 8L_{22ii}^{V,LR} + 8L_{ii11}^{V,RR} + 8L_{ii22}^{V,RR} + 8L_{ue}^{V,RR} - 8L_{ue}^{V,LR} \right] + \alpha_s \alpha \left[ 32L_{ijj}^{V,RR} \right.
\end{aligned}$$

$$\begin{aligned}
& -\frac{32}{9}L_{11ii}^{V,LR} - \frac{32}{9}L_{22ii}^{V,LR} - \frac{32}{9}L_{ii11}^{V,RR} - \frac{32}{9}L_{ii22}^{V,RR} + \frac{64}{9}L_{ii11}^{V,RR} + \frac{64}{9}L_{11ii}^{V,LR} \\
& + \frac{16}{3}L_{11jj}^{V1,LR} - \frac{32}{3}L_{22jj}^{V1,LR} - \frac{368}{243}L_{11jj}^{V8,LR} + \frac{2008}{243}L_{22jj}^{V8,LR} + \frac{16}{3}L_{jj11}^{V1,RR} + \frac{16}{3}L_{jj22}^{V1,RR} \\
& + \frac{352}{243}L_{jj11}^{V8,RR} + \frac{352}{243}L_{jj22}^{V8,RR} - \frac{32}{3}L_{jjjj}^{V1,LR} + \frac{2008}{243}L_{jjjj}^{V8,LR} - \frac{2144}{81}L_{jjjj}^{V,RR} \Big] \\
& + \alpha^2 \Bigg[ \frac{464}{81}L_{jjii}^{V,LR} + \frac{2432}{81}L_{iijj}^{V,RR} + \frac{80}{9}L_{ijjj}^{V,RR} + \frac{1408}{243}L_{11ii}^{V,LR} + \frac{1408}{243}L_{22ii}^{V,LR} \\
& + \frac{2512}{243}L_{ii11}^{V,RR} + \frac{2512}{243}L_{ii22}^{V,RR} + \frac{464}{81}L_{iii}^{V,LR} + \frac{3680}{81}L_{iii}^{V,RR} + \frac{1312}{243}L_{ii11}^{V,RR} \\
& - \frac{3104}{243}L_{11ii}^{V,LR} - \frac{928}{243}L_{11jj}^{V1,LR} + \frac{416}{243}L_{22jj}^{V1,LR} - \frac{424}{243}L_{11jj}^{V,LR} - \frac{424}{243}L_{22jj}^{V,LR} \\
& + \frac{3248}{243}L_{11jj}^{V,RR} + \frac{3248}{243}L_{22jj}^{V,RR} + \frac{296}{243}L_{jj11}^{V1,RR} + \frac{296}{243}L_{jj22}^{V1,RR} + \frac{128}{243}L_{jjjj}^{V1,LR} \\
& + \frac{26272}{243}L_{jjjj}^{V,RR} \Bigg] ;
\end{aligned}$$

$$\begin{aligned}
\dot{L}_{ijj}^{V1,RR} &= \frac{8}{3}g_s^2 L_{ijj}^{V8,RR} + e^2 \Bigg[ -\frac{8}{3}L_{ijj}^{V1,RR} + \frac{4}{9}L_{11ii}^{V1,LR} + \frac{4}{9}L_{22ii}^{V1,LR} + \frac{4}{9}L_{11ii}^{V,LR} \\
& + \frac{4}{9}L_{22ii}^{V,RR} + \frac{4}{9}L_{11ii}^{V,RR} + \frac{4}{9}L_{22ii}^{V,RR} + \frac{4}{9}L_{ii11}^{V1,RR} + \frac{4}{9}L_{ii22}^{V1,RR} - \frac{8}{9}L_{iii}^{V1,LR} \\
& - \frac{64}{27}L_{iii}^{V,RR} - \frac{16}{9}L_{jjjj}^{V1,LR} - \frac{128}{27}L_{jjjj}^{V,RR} - \frac{8}{9}L_{11jj}^{V,LR} - \frac{8}{9}L_{22jj}^{V,LR} - \frac{8}{9}L_{11jj}^{V,RR} \\
& - \frac{8}{9}L_{22jj}^{V,RR} + \frac{16}{9}L_{11jj}^{V1,LR} + \frac{16}{9}L_{11jj}^{V1,RR} \Bigg] + \alpha_s^2 \Bigg[ -\frac{28}{3}L_{ijj}^{V1,RR} + \frac{74}{27}L_{ijj}^{V8,RR} \\
& - 8L_{11ii}^{V1,LR} - 8L_{22ii}^{V1,LR} + \frac{4}{27}L_{11ii}^{V8,LR} + \frac{4}{27}L_{22ii}^{V8,LR} + 8L_{ii11}^{V1,RR} + 8L_{ii22}^{V1,RR} \\
& + \frac{4}{27}L_{ii11}^{V8,RR} + \frac{4}{27}L_{ii22}^{V8,RR} - 8L_{iii}^{V1,LR} + \frac{4}{27}L_{iii}^{V8,LR} + \frac{328}{9}L_{iii}^{V,RR} - 16L_{jjjj}^{V1,LR} \\
& + \frac{8}{27}L_{jjjj}^{V8,LR} + \frac{1672}{27}L_{jjjj}^{V,RR} - 8L_{11jj}^{V1,LR} + 8L_{11jj}^{V1,RR} + \frac{4}{27}L_{11jj}^{V8,LR} + \frac{4}{27}L_{11jj}^{V8,RR} \Bigg] \\
& + \alpha_s \alpha \Bigg[ \frac{64}{3}L_{ijj}^{V1,RR} - \frac{8}{27}L_{ijj}^{V8,RR} + \frac{16}{9}L_{11ii}^{V1,LR} - \frac{32}{9}L_{22ii}^{V1,LR} - \frac{368}{729}L_{11ii}^{V8,LR}
\end{aligned}$$

$$\begin{aligned}
& + \frac{2008}{729} L_{22ii}^{V8,LR} + \frac{16}{9} L_{ii11}^{V1,RR} + \frac{16}{9} L_{ii22}^{V1,RR} + \frac{352}{729} L_{ii11}^{V8,RR} + \frac{352}{729} L_{ii22}^{V8,RR} - \frac{32}{9} L_{iii}^{V1,LR} \\
& + \frac{2008}{729} L_{iii}^{V8,LR} - \frac{2144}{243} L_{iii}^{V,RR} - \frac{64}{9} L_{jjj}^{V1,LR} + \frac{4088}{729} L_{jjj}^{V8,LR} - \frac{10304}{729} L_{jjj}^{V,RR} \\
& + \frac{64}{9} L_{11jj}^{V1,LR} + \frac{64}{9} L_{11jj}^{V1,RR} - \frac{2708}{729} L_{11jj}^{V8,LR} + \frac{172}{729} L_{11jj}^{V8,RR} \Big] + \alpha^2 \Big[ - \frac{136}{729} L_{11ii}^{V1,LR} \\
& + \frac{2720}{729} L_{22ii}^{V1,LR} + \frac{1664}{729} L_{11ii}^{V,LR} + \frac{1664}{729} L_{22ii}^{V,LR} + \frac{1448}{729} L_{11ii}^{V,RR} + \frac{1448}{729} L_{22ii}^{V,RR} \\
& - \frac{208}{729} L_{ii11}^{V1,RR} - \frac{208}{729} L_{ii22}^{V1,RR} + \frac{2432}{729} L_{iii}^{V1,LR} + \frac{11872}{729} L_{iii}^{V,RR} - \frac{512}{729} L_{jjj}^{V1,LR} \\
& + \frac{40528}{2187} L_{jjj}^{V,RR} - \frac{2992}{729} L_{11jj}^{V,LR} - \frac{2992}{729} L_{22jj}^{V,LR} + \frac{2624}{729} L_{11jj}^{V,RR} + \frac{2624}{729} L_{22jj}^{V,RR} \\
& - \frac{1216}{729} L_{11jj}^{V1,LR} + \frac{6272}{729} L_{11jj}^{V1,RR} \Big] ;
\end{aligned}$$

$$\begin{aligned}
\dot{L}_{ijj}^{V8,RR} & = g_s^2 \Big[ 12 L_{ijj}^{V1,RR} - 4 L_{ijj}^{V8,RR} + \frac{2}{3} L_{11ii}^{V8,LR} + \frac{2}{3} L_{22ii}^{V8,LR} + \frac{2}{3} L_{ii11}^{V8,RR} \\
& + \frac{2}{3} L_{ii22}^{V8,RR} + \frac{2}{3} L_{iii}^{V8,LR} + \frac{8}{3} L_{iii}^{V,RR} + \frac{4}{3} L_{jjj}^{V8,LR} + \frac{16}{3} L_{jjj}^{V,RR} + \frac{2}{3} L_{11jj}^{V8,LR} \\
& + \frac{2}{3} L_{11jj}^{V8,RR} \Big] - \frac{8}{3} e^2 L_{ijj}^{V8,RR} + \alpha_s^2 \Big[ \frac{37}{3} L_{ijj}^{V1,RR} - \frac{121}{9} L_{ijj}^{V8,RR} - \frac{22}{3} L_{11ii}^{V1,LR} \\
& - \frac{22}{3} L_{22ii}^{V1,LR} + \frac{175}{81} L_{11ii}^{V8,LR} + \frac{175}{81} L_{22ii}^{V8,LR} - \frac{2}{3} L_{ii11}^{V1,RR} - \frac{2}{3} L_{ii22}^{V1,RR} + \frac{805}{81} L_{ii11}^{V8,RR} \\
& + \frac{805}{81} L_{ii22}^{V8,RR} - \frac{22}{3} L_{iii}^{V1,LR} + \frac{175}{81} L_{iii}^{V8,LR} + \frac{1942}{27} L_{iii}^{V,RR} - \frac{44}{3} L_{jjj}^{V1,LR} + \frac{314}{81} L_{jjj}^{V8,LR} \\
& + \frac{10246}{81} L_{jjj}^{V,RR} - \frac{22}{3} L_{11jj}^{V1,LR} - \frac{2}{3} L_{11jj}^{V1,RR} + \frac{157}{81} L_{11jj}^{V8,LR} + \frac{787}{81} L_{11jj}^{V8,RR} \Big] \\
& + \alpha_s \alpha \Big[ - \frac{4}{3} L_{ijj}^{V1,RR} - \frac{47}{9} L_{ijj}^{V8,RR} + \frac{284}{81} L_{11ii}^{V1,LR} - \frac{496}{81} L_{22ii}^{V1,LR} + \frac{10}{27} L_{11ii}^{V8,LR} \\
& + \frac{4}{27} L_{22ii}^{V8,LR} + \frac{284}{81} L_{11ii}^{V,LR} + \frac{284}{81} L_{22ii}^{V,LR} + \frac{284}{81} L_{11ii}^{V,RR} + \frac{284}{81} L_{22ii}^{V,RR} + \frac{284}{81} L_{ii11}^{V1,RR} \\
& + \frac{284}{81} L_{ii22}^{V1,RR} + \frac{14}{9} L_{ii11}^{V8,RR} + \frac{14}{9} L_{ii22}^{V8,RR} - \frac{568}{81} L_{iii}^{V1,LR} + \frac{4}{27} L_{iii}^{V8,LR} - \frac{4616}{81} L_{iii}^{V,RR} \\
& - \frac{392}{81} L_{jjj}^{V1,LR} + \frac{104}{27} L_{jjj}^{V8,LR} - \frac{15728}{243} L_{jjj}^{V,RR} - \frac{196}{81} L_{11jj}^{V,LR} - \frac{196}{81} L_{22jj}^{V,LR} - \frac{196}{81} L_{11jj}^{V,RR}
\end{aligned}$$

$$\begin{aligned}
& -\frac{196}{81}L_{22jj}^{V,RR} + \frac{392}{81}L_{11jj}^{V1,LR} + \frac{392}{81}L_{11jj}^{V1,RR} - \frac{80}{27}L_{11jj}^{V8,LR} + \frac{56}{9}L_{11jj}^{V8,RR} \Big] ; \\
\dot{L}_{ed}^{V,RR}{}_{jji} &= e^2 \left[ \frac{4}{3}L_{jji}^{V1,LR} + \frac{8}{3}L_{ijj}^{V,RR} + \frac{8}{9}L_{ijji}^{V,RR} + 4L_{jji}^{V,RR} + \frac{4}{3}L_{iii}^{V1,LR} \right. \\
& + \frac{32}{9}L_{iii}^{V,RR} + \frac{4}{3}L_{11ii}^{V,LR} + \frac{4}{3}L_{ed}^{V,LR}{}_{22ii} + \frac{4}{3}L_{11ii}^{V,RR} + \frac{4}{3}L_{ed}^{V,RR}{}_{22ii} - \frac{8}{3}L_{11ii}^{V1,LR} \\
& - \frac{8}{3}L_{11ii}^{V1,RR} + \frac{4}{9}L_{11jj}^{V,LR} + \frac{4}{9}L_{22jj}^{V,LR} + \frac{4}{9}L_{jj11}^{V,RR} + \frac{4}{9}L_{jj22}^{V,RR} + \frac{8}{9}L_{jjjj}^{V,LR} \\
& \left. + \frac{8}{3}L_{jjjj}^{V,RR} - \frac{8}{9}L_{jj11}^{V,RR} - \frac{8}{9}L_{11jj}^{V,LR} \right] + \alpha_s^2 \left[ -8L_{11jj}^{V,LR}{}_{de} - 8L_{22jj}^{V,LR}{}_{de} \right. \\
& + 8L_{jj11}^{V,RR}{}_{ed} + 8L_{jj22}^{V,RR}{}_{ed} + 8L_{jj11}^{V,RR}{}_{eu} - 8L_{11jj}^{V,LR}{}_{ue} \Big] + \alpha_s \alpha \left[ \frac{16}{3}L_{jji}^{V1,LR}{}_{dd} \right. \\
& - \frac{1022}{243}L_{jji}^{V8,LR}{}_{dd} + 8L_{ijj}^{V,RR}{}_{dd} + \frac{64}{243}L_{ijji}^{V,RR}{}_{dd} - 16L_{jji}^{V,RR}{}_{ed} + \frac{16}{3}L_{iii}^{V1,LR}{}_{dd} - \frac{1022}{243}L_{iii}^{V8,LR}{}_{dd} \\
& + \frac{1048}{81}L_{iii}^{V,RR}{}_{dd} - \frac{32}{3}L_{11ii}^{V1,LR}{}_{ud} - \frac{32}{3}L_{11ii}^{V1,RR}{}_{ud} + \frac{1354}{243}L_{11ii}^{V8,LR}{}_{ud} - \frac{86}{243}L_{11ii}^{V8,RR}{}_{ud} + \frac{16}{9}L_{11jj}^{V,LR}{}_{de} \\
& + \frac{16}{9}L_{22jj}^{V,LR}{}_{de} + \frac{16}{9}L_{jj11}^{V,RR}{}_{ed} + \frac{16}{9}L_{jj22}^{V,RR}{}_{ed} - \frac{32}{9}L_{jj11}^{V,RR}{}_{eu} - \frac{32}{9}L_{11jj}^{V,LR}{}_{ue} \Big] + \alpha^2 \left[ -\frac{1312}{243}L_{jji}^{V1,LR}{}_{dd} \right. \\
& + \frac{1984}{243}L_{ijj}^{V,RR}{}_{dd} + \frac{2896}{729}L_{ijji}^{V,RR}{}_{dd} - \frac{130}{9}L_{jji}^{V,RR}{}_{ed} - \frac{1312}{243}L_{iii}^{V1,LR}{}_{dd} + \frac{4816}{243}L_{iii}^{V,RR}{}_{dd} \\
& - \frac{3184}{243}L_{11ii}^{V,LR}{}_{ed} - \frac{3184}{243}L_{22ii}^{V,LR}{}_{ed} + \frac{3728}{243}L_{11ii}^{V,RR}{}_{ed} + \frac{3728}{243}L_{22ii}^{V,RR}{}_{ed} - \frac{6232}{243}L_{11ii}^{V1,LR}{}_{ud} \\
& + \frac{2984}{243}L_{11ii}^{V1,RR}{}_{ud} - \frac{200}{243}L_{11jj}^{V,LR}{}_{de} - \frac{200}{243}L_{22jj}^{V,LR}{}_{de} - \frac{104}{243}L_{jj11}^{V,RR}{}_{ed} - \frac{104}{243}L_{jj22}^{V,RR}{}_{ed} \\
& \left. - \frac{1040}{81}L_{jjjj}^{V,LR}{}_{ee} + \frac{16}{9}L_{jjjj}^{V,RR}{}_{ee} - \frac{1016}{243}L_{jj11}^{V,RR}{}_{eu} - \frac{1400}{243}L_{11jj}^{V,LR}{}_{ue} \right] ; \\
\dot{L}_{eu}^{V,RR}{}_{jji} &= e^2 \left[ -8L_{jji}^{V,RR}{}_{eu} + \frac{4}{3}L_{11ii}^{V1,LR}{}_{du} + \frac{4}{3}L_{22ii}^{V1,LR}{}_{du} + \frac{4}{3}L_{11ii}^{V,LR}{}_{eu} + \frac{4}{3}L_{22ii}^{V,LR}{}_{eu} \right. \\
& + \frac{4}{3}L_{11ii}^{V,RR}{}_{eu} + \frac{4}{3}L_{22ii}^{V,RR}{}_{eu} + \frac{4}{3}L_{ii11}^{V1,RR}{}_{ud} + \frac{4}{3}L_{ii22}^{V1,RR}{}_{ud} - \frac{8}{3}L_{iii}^{V1,LR}{}_{uu} - \frac{64}{9}L_{iii}^{V,RR}{}_{uu} \\
& - \frac{8}{9}L_{11jj}^{V,LR}{}_{de} - \frac{8}{9}L_{22jj}^{V,LR}{}_{de} - \frac{8}{9}L_{jj11}^{V,RR}{}_{ed} - \frac{8}{9}L_{jj22}^{V,RR}{}_{ed} - \frac{16}{9}L_{jjjj}^{V,LR}{}_{ee} - \frac{16}{3}L_{jjjj}^{V,RR}{}_{ee} \Big] ;
\end{aligned}$$

$$\begin{aligned}
& + \frac{16}{9} L_{jj11}^{V,RR} + \frac{16}{9} L_{11jj}^{V,LR} \Big] + \alpha_s^2 \Big[ -8 L_{11jj}^{V,LR} - 8 L_{22jj}^{V,LR} + 8 L_{jj11}^{V,RR} \\
& + 8 L_{ed22}^{V,RR} + 8 L_{jj11}^{V,RR} - 8 L_{11jj}^{V,LR} \Big] + \alpha_s \alpha \Big[ 32 L_{jjii}^{V,RR} + \frac{16}{3} L_{11ii}^{V1,LR} \\
& - \frac{32}{3} L_{22ii}^{V1,LR} - \frac{368}{243} L_{11ii}^{V8,LR} + \frac{2008}{243} L_{22ii}^{V8,LR} + \frac{16}{3} L_{ii11}^{V1,RR} + \frac{16}{3} L_{ii22}^{V1,RR} + \frac{352}{243} L_{ii11}^{V8,RR} \\
& + \frac{352}{243} L_{ii22}^{V8,RR} - \frac{32}{3} L_{iiii}^{V1,LR} + \frac{2008}{243} L_{iiii}^{V8,LR} - \frac{2144}{81} L_{iiii}^{V,RR} - \frac{32}{9} L_{11jj}^{V,LR} - \frac{32}{9} L_{22jj}^{V,LR} \\
& - \frac{32}{9} L_{ed11}^{V,RR} - \frac{32}{9} L_{jj22}^{V,RR} + \frac{64}{9} L_{jj11}^{V,RR} + \frac{64}{9} L_{11jj}^{V,LR} \Big] + \alpha^2 \Big[ \frac{80}{9} L_{jjii}^{V,RR} \\
& - \frac{928}{243} L_{11ii}^{V1,LR} + \frac{416}{243} L_{22ii}^{V1,LR} - \frac{424}{243} L_{11ii}^{V,LR} - \frac{424}{243} L_{22ii}^{V,LR} + \frac{3248}{243} L_{11ii}^{V,RR} \\
& + \frac{3248}{243} L_{22ii}^{V,RR} + \frac{296}{243} L_{ii11}^{V1,RR} + \frac{296}{243} L_{ii22}^{V1,RR} + \frac{128}{243} L_{iiii}^{V1,LR} + \frac{26272}{243} L_{iiii}^{V,RR} \\
& + \frac{1408}{243} L_{11jj}^{V,LR} + \frac{1408}{243} L_{22jj}^{V,LR} + \frac{2512}{243} L_{jj11}^{V,RR} + \frac{2512}{243} L_{jj22}^{V,RR} + \frac{928}{81} L_{jjjj}^{V,LR} \\
& + \frac{544}{9} L_{jjjj}^{V,RR} + \frac{1312}{243} L_{jj11}^{V,RR} - \frac{3104}{243} L_{11jj}^{V,LR} \Big] ;
\end{aligned}$$

$$\begin{aligned}
\dot{L}_{ud,jjii}^{V1,RR} &= \frac{8}{3} L_{ud,jjii}^{V8,RR} g_s^2 + e^2 \Big[ -\frac{8}{9} L_{dd,iiii}^{V1,LR} - \frac{8}{9} L_{jjii}^{V1,LR} - \frac{64}{27} L_{iiii}^{V,RR} - \frac{16}{9} L_{ijjj}^{V,RR} \\
& - \frac{16}{27} L_{dd,ijji}^{V,RR} + \frac{4}{9} L_{du,11jj}^{V1,LR} + \frac{4}{9} L_{du,22jj}^{V1,LR} - \frac{8}{9} L_{ed,11ii}^{V,LR} - \frac{8}{9} L_{ed,22ii}^{V,LR} - \frac{8}{9} L_{ed,11ii}^{V,RR} \\
& - \frac{8}{9} L_{ed,22ii}^{V,RR} + \frac{4}{9} L_{eu,11jj}^{V,LR} + \frac{4}{9} L_{eu,22jj}^{V,LR} + \frac{4}{9} L_{eu,11jj}^{V,RR} + \frac{4}{9} L_{eu,22jj}^{V,RR} + \frac{16}{9} L_{ud,11ii}^{V1,LR} \\
& + \frac{16}{9} L_{ud,11ii}^{V1,RR} + \frac{4}{9} L_{ud,jj11}^{V1,RR} + \frac{4}{9} L_{ud,jj22}^{V1,RR} - \frac{8}{3} L_{ud,jjii}^{V1,RR} - \frac{8}{9} L_{uu,jjjj}^{V1,LR} - \frac{64}{27} L_{uu,jjjj}^{V,RR} \Big] \\
& + \alpha_s^2 \Big[ -8 L_{dd,iiii}^{V1,LR} - 8 L_{dd,jjii}^{V1,LR} + \frac{4}{27} L_{dd,iiii}^{V8,LR} + \frac{4}{27} L_{dd,jjii}^{V8,LR} + \frac{328}{9} L_{dd,iiii}^{V,RR} \\
& + 16 L_{dd,ijjj}^{V,RR} + \frac{256}{27} L_{dd,ijji}^{V,RR} - 8 L_{du,11jj}^{V1,LR} - 8 L_{du,22jj}^{V1,LR} + \frac{4}{27} L_{du,11jj}^{V8,LR} + \frac{4}{27} L_{du,22jj}^{V8,LR} \\
& - 8 L_{11ii}^{V1,LR} + 8 L_{11ii}^{V1,RR} + 8 L_{jj11}^{V1,RR} + 8 L_{jj22}^{V1,RR} - \frac{28}{3} L_{jjii}^{V1,RR} + \frac{4}{27} L_{11ii}^{V8,LR}
\end{aligned}$$

$$\begin{aligned}
& + \frac{4}{27} L_{11ii}^{V8,RR} + \frac{4}{27} L_{jj11}^{V8,RR} + \frac{4}{27} L_{jj22}^{V8,RR} + \frac{74}{27} L_{jjii}^{V8,RR} - 8 L_{jjjj}^{V1,LR} + \frac{4}{27} L_{jjjj}^{V8,LR} \\
& + \frac{328}{9} L_{jjjj}^{V,RR} \Big] + \alpha_s \alpha \Bigg[ - \frac{32}{9} L_{iii}^{V1,LR} - \frac{32}{9} L_{jjii}^{V1,LR} + \frac{2044}{729} L_{iii}^{V8,LR} + \frac{2044}{729} L_{jjii}^{V8,LR} \\
& - \frac{2096}{243} L_{iii}^{V,RR} - \frac{16}{3} L_{ijjj}^{V,RR} - \frac{128}{729} L_{ijji}^{V,RR} + \frac{16}{9} L_{11jj}^{V1,LR} - \frac{32}{9} L_{22jj}^{V1,LR} - \frac{368}{729} L_{11jj}^{V8,LR} \\
& + \frac{2008}{729} L_{22jj}^{V8,LR} + \frac{64}{9} L_{11ii}^{V1,LR} + \frac{64}{9} L_{11ii}^{V1,RR} + \frac{16}{9} L_{jj11}^{V1,RR} + \frac{16}{9} L_{jj22}^{V1,RR} + \frac{64}{3} L_{jjii}^{V1,RR} \\
& - \frac{2708}{729} L_{11ii}^{V8,LR} + \frac{172}{729} L_{11ii}^{V8,RR} + \frac{352}{729} L_{jj11}^{V8,RR} + \frac{352}{729} L_{jj22}^{V8,RR} - \frac{8}{27} L_{jjii}^{V8,RR} \\
& - \frac{32}{9} L_{jjjj}^{V1,LR} + \frac{2008}{729} L_{jjjj}^{V8,LR} - \frac{2144}{243} L_{jjjj}^{V,RR} \Big] + \alpha^2 \Bigg[ - \frac{256}{729} L_{iii}^{V1,LR} - \frac{256}{729} L_{jjii}^{V1,LR} \\
& + \frac{8368}{729} L_{iii}^{V,RR} + \frac{3232}{729} L_{ijjj}^{V,RR} + \frac{5728}{2187} L_{ijji}^{V,RR} - \frac{136}{729} L_{11jj}^{V1,LR} + \frac{2720}{729} L_{22jj}^{V1,LR} \\
& - \frac{2992}{729} L_{11ii}^{V,LR} - \frac{2992}{729} L_{22ii}^{V,LR} + \frac{2624}{729} L_{11ii}^{V,RR} + \frac{2624}{729} L_{22ii}^{V,RR} + \frac{1664}{729} L_{11jj}^{V,LR} \\
& + \frac{1664}{729} L_{22jj}^{V,LR} + \frac{1448}{729} L_{11jj}^{V,RR} + \frac{1448}{729} L_{22jj}^{V,RR} - \frac{1216}{729} L_{11ii}^{V1,LR} + \frac{6272}{729} L_{11ii}^{V1,RR} \\
& - \frac{208}{729} L_{jj11}^{V1,RR} - \frac{208}{729} L_{jj22}^{V1,RR} + \frac{2432}{729} L_{jjjj}^{V1,LR} + \frac{11872}{729} L_{jjjj}^{V,RR} \Big] ;
\end{aligned}$$

$$\begin{aligned}
\dot{L}_{jjii}^{V8,RR} & = g_s^2 \Bigg[ \frac{2}{3} L_{jjii}^{V8,LR} + \frac{8}{3} L_{ijji}^{V,RR} + 12 L_{jjii}^{V1,RR} - 4 L_{jjii}^{V8,RR} + \frac{2}{3} L_{iii}^{V8,LR} \\
& + \frac{8}{3} L_{iii}^{V,RR} + \frac{2}{3} L_{11ii}^{V8,LR} + \frac{2}{3} L_{11ii}^{V8,RR} + \frac{2}{3} L_{11jj}^{V8,LR} + \frac{2}{3} L_{22jj}^{V8,LR} + \frac{2}{3} L_{jj11}^{V8,RR} \\
& + \frac{2}{3} L_{jj22}^{V8,RR} + \frac{2}{3} L_{jjjj}^{V8,LR} + \frac{8}{3} L_{jjjj}^{V,RR} \Big] - \frac{8}{3} e^2 L_{jjii}^{V8,RR} + \alpha_s^2 \Bigg[ - \frac{22}{3} L_{jjii}^{V1,LR} \\
& + \frac{157}{81} L_{jjii}^{V8,LR} - \frac{28}{3} L_{ijjj}^{V,RR} + \frac{5248}{81} L_{ijji}^{V,RR} + \frac{37}{3} L_{jjii}^{V1,RR} - \frac{121}{9} L_{jjii}^{V8,RR} - \frac{22}{3} L_{iii}^{V1,LR} \\
& + \frac{157}{81} L_{iii}^{V8,LR} + \frac{1918}{27} L_{iii}^{V,RR} - \frac{22}{3} L_{11ii}^{V1,LR} - \frac{2}{3} L_{11ii}^{V1,RR} + \frac{157}{81} L_{11ii}^{V8,LR} + \frac{787}{81} L_{11ii}^{V8,RR} \\
& - \frac{22}{3} L_{11jj}^{V1,LR} - \frac{22}{3} L_{22jj}^{V1,LR} + \frac{175}{81} L_{11jj}^{V8,LR} + \frac{175}{81} L_{22jj}^{V8,LR} - \frac{2}{3} L_{jj11}^{V1,RR} - \frac{2}{3} L_{jj22}^{V1,RR}
\end{aligned}$$



$$\begin{aligned}
& + \frac{805}{81} L_{\frac{ud}{jj11}}^{V8,RR} + \frac{805}{81} L_{\frac{ud}{jj22}}^{V8,RR} - \frac{22}{3} L_{\frac{uu}{jjjj}}^{V1,LR} + \frac{175}{81} L_{\frac{uu}{jjjj}}^{V8,LR} + \frac{1942}{27} L_{\frac{uu}{jjjj}}^{V,RR} \Bigg] \\
& + \alpha_s \alpha \Bigg[ - \frac{196}{81} L_{\frac{dd}{jjii}}^{V1,LR} + \frac{52}{27} L_{\frac{dd}{jjii}}^{V8,LR} - \frac{392}{81} L_{\frac{dd}{ijjj}}^{V,RR} - \frac{5096}{243} L_{\frac{dd}{ijji}}^{V,RR} - \frac{4}{3} L_{\frac{ud}{jjii}}^{V1,RR} \\
& - \frac{47}{9} L_{\frac{ud}{jjii}}^{V8,RR} - \frac{196}{81} L_{\frac{dd}{iiii}}^{V1,LR} + \frac{52}{27} L_{\frac{dd}{iiii}}^{V8,LR} - \frac{3152}{81} L_{\frac{dd}{iiii}}^{V,RR} - \frac{196}{81} L_{\frac{ud}{11ii}}^{V,LR} - \frac{196}{81} L_{\frac{ed}{22ii}}^{V,LR} \\
& - \frac{196}{81} L_{\frac{ed}{11ii}}^{V,RR} - \frac{196}{81} L_{\frac{ed}{22ii}}^{V,RR} + \frac{392}{81} L_{\frac{ud}{11ii}}^{V1,LR} + \frac{392}{81} L_{\frac{ud}{11ii}}^{V1,RR} - \frac{80}{27} L_{\frac{ud}{11ii}}^{V8,LR} + \frac{56}{9} L_{\frac{ud}{11ii}}^{V8,RR} \\
& + \frac{284}{81} L_{\frac{du}{11jj}}^{V1,LR} - \frac{496}{81} L_{\frac{du}{22jj}}^{V1,LR} + \frac{10}{27} L_{\frac{du}{11jj}}^{V8,LR} + \frac{4}{27} L_{\frac{du}{22jj}}^{V8,LR} + \frac{284}{81} L_{\frac{eu}{11jj}}^{V,LR} + \frac{284}{81} L_{\frac{eu}{22jj}}^{V,LR} \\
& + \frac{284}{81} L_{\frac{eu}{11jj}}^{V,RR} + \frac{284}{81} L_{\frac{eu}{22jj}}^{V,RR} + \frac{284}{81} L_{\frac{ud}{jj11}}^{V1,RR} + \frac{284}{81} L_{\frac{ud}{jj22}}^{V1,RR} + \frac{14}{9} L_{\frac{ud}{jj11}}^{V8,RR} + \frac{14}{9} L_{\frac{ud}{jj22}}^{V8,RR} \\
& - \frac{568}{81} L_{\frac{uu}{jjjj}}^{V1,LR} + \frac{4}{27} L_{\frac{uu}{jjjj}}^{V8,LR} - \frac{4616}{81} L_{\frac{uu}{jjjj}}^{V,RR} \Bigg] ;
\end{aligned}$$

$$\begin{aligned}
\dot{L}_{\frac{dd}{ijj}}^{V,RR} & = g_s^2 \Bigg[ - \frac{1}{18} L_{\frac{dd}{iiii}}^{V8,LR} - \frac{1}{18} L_{\frac{dd}{jjii}}^{V8,LR} - \frac{1}{9} L_{\frac{dd}{jjjj}}^{V8,LR} - \frac{2}{9} L_{\frac{dd}{iiii}}^{V,RR} - 2 L_{\frac{dd}{ijj}}^{V,RR} \\
& + \frac{52}{9} L_{\frac{dd}{ijji}}^{V,RR} - \frac{4}{9} L_{\frac{dd}{jjjj}}^{V,RR} - \frac{1}{18} L_{\frac{ud}{11ii}}^{V8,LR} - \frac{1}{18} L_{\frac{ud}{11jj}}^{V8,LR} - \frac{1}{18} L_{\frac{ud}{11ii}}^{V8,RR} - \frac{1}{18} L_{\frac{ud}{11jj}}^{V8,RR} \Bigg] \\
& + e^2 \Bigg[ \frac{2}{9} L_{\frac{dd}{iiii}}^{V1,LR} + \frac{2}{9} L_{\frac{dd}{jjii}}^{V1,LR} + \frac{4}{9} L_{\frac{dd}{jjjj}}^{V1,LR} + \frac{16}{27} L_{\frac{dd}{iiii}}^{V,RR} + \frac{16}{9} L_{\frac{dd}{ijji}}^{V,RR} + \frac{4}{27} L_{\frac{dd}{ijji}}^{V,RR} \\
& + \frac{32}{27} L_{\frac{dd}{jjjj}}^{V,RR} + \frac{2}{9} L_{\frac{ed}{11ii}}^{V,LR} + \frac{2}{9} L_{\frac{ed}{11jj}}^{V,LR} + \frac{2}{9} L_{\frac{ed}{22ii}}^{V,LR} + \frac{2}{9} L_{\frac{ed}{22jj}}^{V,LR} + \frac{2}{9} L_{\frac{ed}{11ii}}^{V,RR} \\
& + \frac{2}{9} L_{\frac{ed}{11jj}}^{V,RR} + \frac{2}{9} L_{\frac{ed}{22ii}}^{V,RR} + \frac{2}{9} L_{\frac{ed}{22jj}}^{V,RR} - \frac{4}{9} L_{\frac{ud}{11ii}}^{V1,LR} - \frac{4}{9} L_{\frac{ud}{11jj}}^{V1,LR} - \frac{4}{9} L_{\frac{ud}{11ii}}^{V1,RR} \\
& - \frac{4}{9} L_{\frac{ud}{11jj}}^{V1,RR} \Bigg] + \alpha_s^2 \Bigg[ - \frac{61}{18} L_{\frac{dd}{iiii}}^{V1,LR} - \frac{61}{18} L_{\frac{dd}{jjii}}^{V1,LR} - \frac{61}{9} L_{\frac{dd}{jjjj}}^{V1,LR} - \frac{85}{972} L_{\frac{dd}{iiii}}^{V8,LR} \\
& - \frac{85}{972} L_{\frac{dd}{jjii}}^{V8,LR} - \frac{85}{486} L_{\frac{dd}{jjjj}}^{V8,LR} + \frac{1993}{162} L_{\frac{dd}{iiii}}^{V,RR} - \frac{47}{18} L_{\frac{dd}{ijji}}^{V,RR} + \frac{2677}{486} L_{\frac{dd}{ijji}}^{V,RR} + \frac{9925}{486} L_{\frac{dd}{jjjj}}^{V,RR} \\
& - \frac{61}{18} L_{\frac{ud}{11ii}}^{V1,LR} - \frac{61}{18} L_{\frac{ud}{11jj}}^{V1,LR} + \frac{73}{18} L_{\frac{ud}{11ii}}^{V1,RR} + \frac{73}{18} L_{\frac{ud}{11jj}}^{V1,RR} - \frac{85}{972} L_{\frac{ud}{11ii}}^{V8,LR} - \frac{85}{972} L_{\frac{ud}{11jj}}^{V8,LR} \\
& - \frac{715}{972} L_{\frac{ud}{11ii}}^{V8,RR} - \frac{715}{972} L_{\frac{ud}{11jj}}^{V8,RR} \Bigg] + \alpha_s \alpha \Bigg[ \frac{238}{243} L_{\frac{dd}{iiii}}^{V1,LR} + \frac{238}{243} L_{\frac{dd}{jjii}}^{V1,LR} + \frac{476}{243} L_{\frac{dd}{jjjj}}^{V1,LR}
\end{aligned}$$

$$\begin{aligned}
& -\frac{797}{1458}L_{\bar{u}\bar{u}\bar{u}}^{V8,LR} - \frac{797}{1458}L_{\bar{u}\bar{u}\bar{d}}^{V8,LR} - \frac{797}{729}L_{\bar{u}\bar{d}\bar{d}}^{V8,LR} + \frac{313}{243}L_{\bar{u}\bar{u}\bar{u}}^{V,RR} - \frac{1522}{243}L_{\bar{u}\bar{d}\bar{d}}^{V,RR} \\
& - \frac{6740}{729}L_{\bar{u}\bar{d}\bar{d}}^{V,RR} + \frac{1621}{729}L_{\bar{u}\bar{d}\bar{u}}^{V,RR} + \frac{22}{243}L_{\bar{u}\bar{d}\bar{u}}^{V,LR} + \frac{22}{243}L_{\bar{u}\bar{d}\bar{d}}^{V,LR} + \frac{22}{243}L_{\bar{u}\bar{d}\bar{u}}^{V,LR} + \frac{22}{243}L_{\bar{u}\bar{d}\bar{d}}^{V,LR} \\
& + \frac{22}{243}L_{\bar{u}\bar{d}\bar{u}}^{V,RR} + \frac{22}{243}L_{\bar{u}\bar{d}\bar{d}}^{V,RR} + \frac{22}{243}L_{\bar{u}\bar{d}\bar{u}}^{V,RR} + \frac{22}{243}L_{\bar{u}\bar{d}\bar{d}}^{V,RR} - \frac{476}{243}L_{\bar{u}\bar{d}\bar{u}}^{V1,LR} - \frac{476}{243}L_{\bar{u}\bar{d}\bar{d}}^{V1,LR} \\
& - \frac{476}{243}L_{\bar{u}\bar{d}\bar{u}}^{V1,RR} - \frac{476}{243}L_{\bar{u}\bar{d}\bar{d}}^{V1,RR} + \frac{715}{1458}L_{\bar{u}\bar{d}\bar{u}}^{V8,LR} + \frac{715}{1458}L_{\bar{u}\bar{d}\bar{d}}^{V8,LR} + \frac{103}{1458}L_{\bar{u}\bar{d}\bar{u}}^{V8,RR} \\
& + \frac{103}{1458}L_{\bar{u}\bar{d}\bar{d}}^{V8,RR} \Big] + \alpha^2 \Big[ -\frac{368}{729}L_{\bar{u}\bar{d}\bar{u}}^{V1,LR} - \frac{368}{729}L_{\bar{u}\bar{d}\bar{d}}^{V1,LR} - \frac{736}{729}L_{\bar{u}\bar{d}\bar{u}}^{V1,LR} + \frac{608}{729}L_{\bar{u}\bar{d}\bar{d}}^{V,RR} \\
& + \frac{110}{729}L_{\bar{u}\bar{d}\bar{u}}^{V,RR} + \frac{296}{2187}L_{\bar{u}\bar{d}\bar{u}}^{V,RR} + \frac{2936}{2187}L_{\bar{u}\bar{d}\bar{u}}^{V,RR} - \frac{656}{729}L_{\bar{u}\bar{d}\bar{u}}^{V,LR} - \frac{656}{729}L_{\bar{u}\bar{d}\bar{d}}^{V,LR} \\
& - \frac{656}{729}L_{\bar{u}\bar{d}\bar{u}}^{V,LR} - \frac{656}{729}L_{\bar{u}\bar{d}\bar{d}}^{V,LR} + \frac{856}{729}L_{\bar{u}\bar{d}\bar{u}}^{V,RR} + \frac{856}{729}L_{\bar{u}\bar{d}\bar{d}}^{V,RR} + \frac{856}{729}L_{\bar{u}\bar{d}\bar{u}}^{V,RR} + \frac{856}{729}L_{\bar{u}\bar{d}\bar{d}}^{V,RR} \\
& - \frac{1748}{729}L_{\bar{u}\bar{d}\bar{u}}^{V1,LR} - \frac{1748}{729}L_{\bar{u}\bar{d}\bar{d}}^{V1,LR} + \frac{268}{729}L_{\bar{u}\bar{d}\bar{u}}^{V1,RR} + \frac{268}{729}L_{\bar{u}\bar{d}\bar{d}}^{V1,RR} \Big] ;
\end{aligned}$$

$$\begin{aligned}
\dot{L}_{\bar{u}\bar{d}\bar{d}}^{V,RR} &= g_s^2 \Big[ \frac{1}{6}L_{\bar{u}\bar{d}\bar{u}}^{V8,LR} + 6L_{\bar{u}\bar{d}\bar{u}}^{V,RR} - \frac{4}{3}L_{\bar{u}\bar{d}\bar{u}}^{V,RR} + \frac{1}{6}L_{\bar{u}\bar{d}\bar{u}}^{V8,LR} + \frac{2}{3}L_{\bar{u}\bar{d}\bar{u}}^{V,RR} \\
& + \frac{1}{6}L_{\bar{u}\bar{d}\bar{u}}^{V8,LR} + \frac{1}{6}L_{\bar{u}\bar{d}\bar{u}}^{V8,RR} + \frac{1}{3}L_{\bar{u}\bar{d}\bar{u}}^{V8,LR} + \frac{4}{3}L_{\bar{u}\bar{d}\bar{u}}^{V,RR} + \frac{1}{6}L_{\bar{u}\bar{d}\bar{u}}^{V8,LR} + \frac{1}{6}L_{\bar{u}\bar{d}\bar{u}}^{V8,RR} \Big] \\
& + \frac{4}{3}e^2L_{\bar{u}\bar{d}\bar{u}}^{V,RR} + \alpha_s^2 \Big[ -\frac{11}{6}L_{\bar{u}\bar{d}\bar{u}}^{V1,LR} + \frac{157}{324}L_{\bar{u}\bar{d}\bar{u}}^{V8,LR} + \frac{23}{6}L_{\bar{u}\bar{d}\bar{u}}^{V,RR} + \frac{779}{162}L_{\bar{u}\bar{d}\bar{u}}^{V,RR} \\
& - \frac{11}{6}L_{\bar{u}\bar{d}\bar{u}}^{V1,LR} + \frac{157}{324}L_{\bar{u}\bar{d}\bar{u}}^{V8,LR} + \frac{959}{54}L_{\bar{u}\bar{d}\bar{u}}^{V,RR} - \frac{11}{6}L_{\bar{u}\bar{d}\bar{u}}^{V1,LR} - \frac{1}{6}L_{\bar{u}\bar{d}\bar{u}}^{V1,RR} + \frac{157}{324}L_{\bar{u}\bar{d}\bar{u}}^{V8,LR} \\
& + \frac{787}{324}L_{\bar{u}\bar{d}\bar{u}}^{V8,RR} - \frac{11}{3}L_{\bar{u}\bar{d}\bar{u}}^{V1,LR} + \frac{157}{162}L_{\bar{u}\bar{d}\bar{u}}^{V8,LR} + \frac{5123}{162}L_{\bar{u}\bar{d}\bar{u}}^{V,RR} - \frac{11}{6}L_{\bar{u}\bar{d}\bar{u}}^{V1,LR} - \frac{1}{6}L_{\bar{u}\bar{d}\bar{u}}^{V1,RR} \\
& + \frac{157}{324}L_{\bar{u}\bar{d}\bar{u}}^{V8,LR} + \frac{787}{324}L_{\bar{u}\bar{d}\bar{u}}^{V8,RR} \Big] + \alpha_s \alpha \Big[ -\frac{22}{81}L_{\bar{u}\bar{d}\bar{u}}^{V1,LR} - \frac{25}{54}L_{\bar{u}\bar{d}\bar{u}}^{V8,LR} - \frac{746}{81}L_{\bar{u}\bar{d}\bar{u}}^{V,RR} \\
& - \frac{1436}{243}L_{\bar{u}\bar{d}\bar{u}}^{V,RR} - \frac{22}{81}L_{\bar{u}\bar{d}\bar{u}}^{V1,LR} - \frac{25}{54}L_{\bar{u}\bar{d}\bar{u}}^{V8,LR} + \frac{211}{81}L_{\bar{u}\bar{d}\bar{u}}^{V,RR} - \frac{22}{81}L_{\bar{u}\bar{d}\bar{u}}^{V,LR} - \frac{22}{81}L_{\bar{u}\bar{d}\bar{u}}^{V,LR} \\
& - \frac{22}{81}L_{\bar{u}\bar{d}\bar{u}}^{V,RR} - \frac{22}{81}L_{\bar{u}\bar{d}\bar{u}}^{V,RR} + \frac{44}{81}L_{\bar{u}\bar{d}\bar{u}}^{V1,LR} + \frac{44}{81}L_{\bar{u}\bar{d}\bar{u}}^{V1,RR} + \frac{71}{54}L_{\bar{u}\bar{d}\bar{u}}^{V8,LR} - \frac{7}{18}L_{\bar{u}\bar{d}\bar{u}}^{V8,RR}
\end{aligned}$$

$$\begin{aligned}
& -\frac{44}{81}L_{jjj}^{V1,LR} - \frac{25}{27}L_{jjj}^{V8,LR} + \frac{955}{243}L_{jjj}^{V,RR} - \frac{22}{81}L_{11jj}^{V,LR} - \frac{22}{81}L_{22jj}^{V,LR} - \frac{22}{81}L_{11jj}^{V,RR} \\
& - \frac{22}{81}L_{22jj}^{V,RR} + \frac{44}{81}L_{11jj}^{V1,LR} + \frac{44}{81}L_{11jj}^{V1,RR} + \frac{71}{54}L_{11jj}^{V8,LR} - \frac{7}{18}L_{11jj}^{V8,RR} \Big] - \frac{2}{9}\alpha^2 L_{ijji}^{V,RR} ; \\
\dot{L}_{dd}^{V,RR}{}_{iii} &= g_s^2 \left[ \frac{2}{9}L_{jjii}^{V8,LR} + \frac{8}{9}L_{ijji}^{V,RR} + \frac{2}{9}L_{iii}^{V8,LR} + \frac{44}{9}L_{iii}^{V,RR} + \frac{2}{9}L_{11ii}^{V8,LR} \right. \\
& + \left. \frac{2}{9}L_{11ii}^{V8,RR} \right] + e^2 \left[ \frac{4}{9}L_{jjii}^{V1,LR} + \frac{8}{9}L_{ijji}^{V,RR} + \frac{8}{27}L_{ijji}^{V,RR} + \frac{4}{9}L_{iii}^{V1,LR} \right. \\
& + \frac{68}{27}L_{iii}^{V,RR} + \frac{4}{9}L_{11ii}^{V,LR} + \frac{4}{9}L_{22ii}^{V,LR} + \frac{4}{9}L_{11ii}^{V,RR} + \frac{4}{9}L_{22ii}^{V,RR} - \frac{8}{9}L_{11ii}^{V1,LR} \\
& - \left. \frac{8}{9}L_{11ii}^{V1,RR} \right] + \alpha_s^2 \left[ -\frac{94}{9}L_{jjii}^{V1,LR} + \frac{193}{243}L_{jjii}^{V8,LR} + \frac{116}{9}L_{ijji}^{V,RR} + \frac{7552}{243}L_{ijji}^{V,RR} \right. \\
& - \frac{94}{9}L_{iii}^{V1,LR} + \frac{193}{243}L_{iii}^{V8,LR} + \frac{4447}{81}L_{iii}^{V,RR} - \frac{94}{9}L_{11ii}^{V1,LR} + \frac{70}{9}L_{11ii}^{V1,RR} + \frac{193}{243}L_{11ii}^{V8,LR} \\
& + \left. \frac{823}{243}L_{11ii}^{V8,RR} \right] + \alpha_s \alpha \left[ \frac{344}{243}L_{jjii}^{V1,LR} - \frac{1472}{729}L_{jjii}^{V8,LR} + \frac{472}{243}L_{ijji}^{V,RR} + \frac{1880}{729}L_{ijji}^{V,RR} \right. \\
& + \frac{344}{243}L_{iii}^{V1,LR} - \frac{1472}{729}L_{iii}^{V8,LR} - \frac{2104}{243}L_{iii}^{V,RR} - \frac{88}{243}L_{11ii}^{V,LR} - \frac{88}{243}L_{22ii}^{V,LR} \\
& - \frac{88}{243}L_{11ii}^{V,RR} - \frac{88}{243}L_{22ii}^{V,RR} - \frac{688}{243}L_{11ii}^{V1,LR} - \frac{688}{243}L_{11ii}^{V1,RR} + \frac{2632}{729}L_{11ii}^{V8,LR} \\
& - \left. \frac{464}{729}L_{11ii}^{V8,RR} \right] + \alpha^2 \left[ -\frac{736}{729}L_{jjii}^{V1,LR} + \frac{544}{729}L_{ijji}^{V,RR} + \frac{592}{2187}L_{ijji}^{V,RR} - \frac{736}{729}L_{iii}^{V1,LR} \right. \\
& + \frac{1054}{729}L_{iii}^{V,RR} - \frac{1312}{729}L_{11ii}^{V,LR} - \frac{1312}{729}L_{22ii}^{V,LR} + \frac{1712}{729}L_{11ii}^{V,RR} + \frac{1712}{729}L_{22ii}^{V,RR} \\
& - \left. \frac{3496}{729}L_{11ii}^{V1,LR} + \frac{536}{729}L_{11ii}^{V1,RR} \right] ; \\
\dot{L}_{uu}^{V,RR}{}_{iii} &= g_s^2 \left[ \frac{2}{9}L_{du}^{V8,LR}{}_{11ii} + \frac{2}{9}L_{22ii}^{V8,LR} + \frac{2}{9}L_{ii11}^{V8,RR} + \frac{2}{9}L_{ii22}^{V8,RR} + \frac{2}{9}L_{iii}^{V8,LR} \right. \\
& + \left. \frac{44}{9}L_{iii}^{V,RR} \right] + e^2 \left[ -\frac{8}{9}L_{11ii}^{V1,LR} - \frac{8}{9}L_{22ii}^{V1,LR} - \frac{8}{9}L_{11ii}^{V,LR} - \frac{8}{9}L_{22ii}^{V,LR} \right. \\
& - \frac{8}{9}L_{11ii}^{V,RR} - \frac{8}{9}L_{22ii}^{V,RR} - \frac{8}{9}L_{ii11}^{V1,RR} - \frac{8}{9}L_{ii22}^{V1,RR} + \frac{16}{9}L_{iii}^{V1,LR} + \frac{272}{27}L_{iii}^{V,RR} \Big]
\end{aligned}$$

$$\begin{aligned}
& + \alpha_s^2 \left[ -\frac{94}{9} L_{11ii}^{V1,LR} - \frac{94}{9} L_{22ii}^{V1,LR} + \frac{211}{243} L_{11ii}^{V8,LR} + \frac{211}{243} L_{22ii}^{V8,LR} + \frac{70}{9} L_{ii11}^{V1,RR} \right. \\
& + \frac{70}{9} L_{ud\ ii22}^{V1,RR} + \frac{841}{243} L_{ii11}^{V8,RR} + \frac{841}{243} L_{ud\ ii22}^{V8,RR} - \frac{94}{9} L_{uu\ iii}^{V1,LR} + \frac{211}{243} L_{uu\ iii}^{V8,LR} + \frac{4471}{81} L_{uu\ iii}^{V,RR} \left. \right] \\
& + \alpha_s \alpha \left[ -\frac{688}{243} L_{11ii}^{V1,LR} + \frac{1448}{243} L_{22ii}^{V1,LR} + \frac{1906}{729} L_{11ii}^{V8,LR} - \frac{5816}{729} L_{22ii}^{V8,LR} + \frac{176}{243} L_{11ii}^{V,LR} \right. \\
& + \frac{176}{243} L_{22ii}^{V,LR} + \frac{176}{243} L_{11ii}^{V,RR} + \frac{176}{243} L_{22ii}^{V,RR} - \frac{688}{243} L_{ud\ ii11}^{V1,RR} - \frac{688}{243} L_{ii22}^{V1,RR} \\
& - \frac{1190}{729} L_{ud\ ii11}^{V8,RR} - \frac{1190}{729} L_{ii22}^{V8,RR} + \frac{1376}{243} L_{uu\ iii}^{V1,LR} - \frac{5816}{729} L_{uu\ iii}^{V8,LR} - \frac{8320}{243} L_{uu\ iii}^{V,RR} \left. \right] \\
& + \alpha^2 \left[ -\frac{2104}{729} L_{11ii}^{V1,LR} - \frac{12352}{729} L_{22ii}^{V1,LR} - \frac{9592}{729} L_{11ii}^{V,LR} - \frac{9592}{729} L_{22ii}^{V,LR} + \frac{2504}{729} L_{11ii}^{V,RR} \right. \\
& + \frac{2504}{729} L_{22ii}^{V,RR} + \frac{1928}{729} L_{ud\ ii11}^{V1,RR} + \frac{1928}{729} L_{ii22}^{V1,RR} - \frac{11776}{729} L_{uu\ iii}^{V1,LR} + \frac{6496}{729} L_{uu\ iii}^{V,RR} \left. \right];
\end{aligned}$$

$$\begin{aligned}
\dot{L}_{ee\ ij}^{V,RR} &= e^2 \left[ \frac{1}{3} L_{jjii}^{V,LR} + \frac{40}{3} L_{ijj}^{V,RR} + \frac{1}{3} L_{11ii}^{V,LR} + \frac{1}{3} L_{22ii}^{V,LR} + \frac{1}{3} L_{ii11}^{V,RR} \right. \\
& + \frac{1}{3} L_{ii22}^{V,RR} + \frac{1}{3} L_{iii}^{V,LR} + \frac{4}{3} L_{iii}^{V,RR} - \frac{2}{3} L_{ii11}^{V,RR} - \frac{2}{3} L_{11ii}^{V,LR} + \frac{1}{3} L_{11jj}^{V,LR} \\
& + \frac{1}{3} L_{22jj}^{V,LR} + \frac{1}{3} L_{jj11}^{V,RR} + \frac{1}{3} L_{jj22}^{V,RR} + \frac{2}{3} L_{jjjj}^{V,LR} + 2 L_{jjjj}^{V,RR} - \frac{2}{3} L_{jj11}^{V,RR} \\
& - \frac{2}{3} L_{11jj}^{V,LR} \left. \right] + \alpha_s \alpha \left[ \frac{4}{3} L_{11ii}^{V,LR} + \frac{4}{3} L_{22ii}^{V,LR} + \frac{4}{3} L_{ii11}^{V,RR} + \frac{4}{3} L_{ii22}^{V,RR} \right. \\
& - \frac{8}{3} L_{ii11}^{V,RR} - \frac{8}{3} L_{11ii}^{V,LR} + \frac{4}{3} L_{11jj}^{V,LR} + \frac{4}{3} L_{22jj}^{V,LR} + \frac{4}{3} L_{jj11}^{V,RR} + \frac{4}{3} L_{jj22}^{V,RR} \\
& - \frac{8}{3} L_{jj11}^{V,RR} - \frac{8}{3} L_{11jj}^{V,LR} \left. \right] + \alpha^2 \left[ -\frac{178}{27} L_{jjii}^{V,LR} - \frac{2494}{27} L_{ijj}^{V,RR} + \frac{34}{81} L_{11ii}^{V,LR} \right. \\
& + \frac{34}{81} L_{22ii}^{V,LR} + \frac{166}{81} L_{ii11}^{V,RR} + \frac{166}{81} L_{ii22}^{V,RR} - \frac{178}{27} L_{iii}^{V,LR} + \frac{320}{27} L_{iii}^{V,RR} - \frac{314}{81} L_{ii11}^{V,RR} \\
& - \frac{842}{81} L_{11ii}^{V,LR} + \frac{34}{81} L_{11jj}^{V,LR} + \frac{34}{81} L_{22jj}^{V,LR} + \frac{166}{81} L_{jj11}^{V,RR} + \frac{166}{81} L_{jj22}^{V,RR} - \frac{356}{27} L_{jjjj}^{V,LR} \left. \right]
\end{aligned}$$

$$\begin{aligned}
& + \frac{52}{3} L_{jjjj}^{V,RR} - \frac{314}{81} L_{jj11}^{V,RR} - \frac{842}{81} L_{11jj}^{V,LR} \Big] ; \\
\dot{L}_{iii}^{V,RR} &= e^2 \left[ \frac{4}{3} L_{jjii}^{V,LR} + \frac{16}{3} L_{ijij}^{V,RR} + \frac{4}{3} L_{11ii}^{V,LR} + \frac{4}{3} L_{22ii}^{V,LR} + \frac{4}{3} L_{ii11}^{V,RR} \right. \\
& + \frac{4}{3} L_{edii22}^{V,RR} + \frac{4}{3} L_{iii}^{V,LR} + \frac{52}{3} L_{iii}^{V,RR} - \frac{8}{3} L_{ii11}^{V,RR} - \frac{8}{3} L_{11ii}^{V,LR} \Big] + \alpha_s \alpha \left[ \frac{16}{3} L_{11ii}^{V,LR} \right. \\
& + \frac{16}{3} L_{de22ii}^{V,LR} + \frac{16}{3} L_{edii11}^{V,RR} + \frac{16}{3} L_{edii22}^{V,RR} - \frac{32}{3} L_{ii11}^{V,RR} - \frac{32}{3} L_{11ii}^{V,LR} \Big] + \alpha^2 \left[ -\frac{712}{27} L_{jjii}^{V,LR} \right. \\
& + \frac{1184}{27} L_{ijij}^{V,RR} + \frac{136}{81} L_{de11ii}^{V,LR} + \frac{136}{81} L_{de22ii}^{V,LR} + \frac{664}{81} L_{edii11}^{V,RR} + \frac{664}{81} L_{edii22}^{V,RR} - \frac{712}{27} L_{iii}^{V,LR} \\
& \left. - \frac{1510}{27} L_{iii}^{V,RR} - \frac{1256}{81} L_{ii11}^{V,RR} - \frac{3368}{81} L_{11ii}^{V,LR} \right] ; \\
\dot{L}_{ijj}^{V,LR} &= e^2 \left[ -4 L_{edijj}^{V,LR} + \frac{16}{9} L_{ijij}^{V,LL} + \frac{4}{9} L_{ijij}^{V,LR} + \frac{4}{9} L_{ii11}^{V,LL} + \frac{4}{9} L_{ii22}^{V,LL} \right. \\
& + \frac{4}{9} L_{edii11}^{V,LR} + \frac{4}{9} L_{edii22}^{V,LR} + \frac{16}{9} L_{iii}^{V,LL} + \frac{4}{9} L_{iii}^{V,LR} - \frac{8}{9} L_{ii11}^{V,LL} - \frac{8}{9} L_{ii11}^{V,LR} \\
& + \frac{8}{3} L_{jjjj}^{V1,LR} + \frac{64}{9} L_{jjjj}^{V,RR} + \frac{4}{3} L_{11jj}^{V,LR} + \frac{4}{3} L_{22jj}^{V,LR} + \frac{4}{3} L_{11jj}^{V,RR} + \frac{4}{3} L_{22jj}^{V,RR} \\
& \left. - \frac{8}{3} L_{11jj}^{V1,LR} - \frac{8}{3} L_{11jj}^{V1,RR} \right] + \alpha_s^2 \left[ -8 L_{edii11}^{V,LL} - 8 L_{edii22}^{V,LL} + 8 L_{edii11}^{V,LR} \right. \\
& + 8 L_{edii22}^{V,LR} - 8 L_{ii11}^{V,LL} + 8 L_{ii11}^{V,LR} \Big] + \alpha_s \alpha \left[ 16 L_{edijj}^{V,LR} + \frac{16}{9} L_{edii11}^{V,LL} \right. \\
& + \frac{16}{9} L_{edii22}^{V,LL} + \frac{16}{9} L_{edii11}^{V,LR} + \frac{16}{9} L_{edii22}^{V,LR} - \frac{32}{9} L_{ii11}^{V,LL} - \frac{32}{9} L_{ii11}^{V,LR} + \frac{32}{3} L_{jjjj}^{V1,LR} \\
& - \frac{2044}{243} L_{jjjj}^{V8,LR} + \frac{5152}{243} L_{jjjj}^{V,RR} - \frac{32}{3} L_{11jj}^{V1,LR} - \frac{32}{3} L_{11jj}^{V1,RR} + \frac{1354}{243} L_{11jj}^{V8,LR} \\
& \left. - \frac{86}{243} L_{11jj}^{V8,RR} \right] + \alpha^2 \left[ \frac{430}{9} L_{edijj}^{V,LR} - \frac{160}{81} L_{ijij}^{V,LL} - \frac{184}{81} L_{ijij}^{V,LR} - \frac{440}{243} L_{edii11}^{V,LL} \right. \\
& - \frac{440}{243} L_{edii22}^{V,LL} - \frac{104}{243} L_{edii11}^{V,LR} - \frac{104}{243} L_{edii22}^{V,LR} - \frac{640}{81} L_{iii}^{V,LL} - \frac{184}{81} L_{iii}^{V,LR} - \frac{1640}{243} L_{ii11}^{V,LL} \\
& \left. - \frac{296}{243} L_{ii11}^{V,LR} + \frac{3424}{243} L_{jjjj}^{V1,LR} - \frac{3056}{729} L_{jjjj}^{V,RR} + \frac{3728}{243} L_{11jj}^{V,LR} + \frac{3728}{243} L_{22jj}^{V,LR} \right]
\end{aligned}$$

$$\begin{aligned}
& -\frac{1024}{243}L_{11jj}^{V,RR} - \frac{1024}{243}L_{22jj}^{V,RR} - \frac{616}{243}L_{11jj}^{V1,LR} - \frac{6952}{243}L_{11jj}^{V1,RR} \Big] ; \\
\dot{L}_{ijj}^{V,LR} = & e^2 \Bigg[ -\frac{32}{9}L_{ijj}^{V,LL} - \frac{8}{9}L_{ijj}^{V,LR} + 8L_{ijj}^{V,LR} - \frac{8}{9}L_{ii1}^{V,LL} - \frac{8}{9}L_{ii2}^{V,LL} \\
& - \frac{8}{9}L_{ii1}^{V,LR} - \frac{8}{9}L_{ii2}^{V,LR} - \frac{32}{9}L_{iii}^{V,LL} - \frac{8}{9}L_{iii}^{V,LR} + \frac{16}{9}L_{ii1}^{V,LL} + \frac{16}{9}L_{ii1}^{V,LR} \\
& + \frac{4}{3}L_{11jj}^{V1,LR} + \frac{4}{3}L_{22jj}^{V1,LR} + \frac{4}{3}L_{11jj}^{V,LR} + \frac{4}{3}L_{22jj}^{V,LR} + \frac{4}{3}L_{11jj}^{V,RR} + \frac{4}{3}L_{22jj}^{V,RR} \\
& + \frac{4}{3}L_{jj11}^{V1,RR} + \frac{4}{3}L_{jj22}^{V1,RR} - \frac{8}{3}L_{jjjj}^{V1,LR} - \frac{64}{9}L_{jjjj}^{V,RR} \Big] + \alpha_s^2 \Bigg[ -8L_{ii1}^{V,LL} \\
& - 8L_{ii2}^{V,LL} + 8L_{ii1}^{V,LR} + 8L_{ii2}^{V,LR} - 8L_{ii1}^{V,LL} + 8L_{ii1}^{V,LR} \Big] + \alpha_s \alpha \Bigg[ -32L_{ijj}^{V,LR} \\
& - \frac{32}{9}L_{ii1}^{V,LL} - \frac{32}{9}L_{ii2}^{V,LL} - \frac{32}{9}L_{ii1}^{V,LR} - \frac{32}{9}L_{ii2}^{V,LR} + \frac{64}{9}L_{ii1}^{V,LL} + \frac{64}{9}L_{ii1}^{V,LR} \\
& + \frac{16}{3}L_{11jj}^{V1,LR} - \frac{32}{3}L_{22jj}^{V1,LR} - \frac{368}{243}L_{11jj}^{V8,LR} + \frac{2008}{243}L_{22jj}^{V8,LR} + \frac{16}{3}L_{jj11}^{V1,RR} + \frac{16}{3}L_{jj22}^{V1,RR} \\
& + \frac{352}{243}L_{jj11}^{V8,RR} + \frac{352}{243}L_{jj22}^{V8,RR} - \frac{32}{3}L_{jjjj}^{V1,LR} + \frac{2008}{243}L_{jjjj}^{V8,LR} - \frac{2144}{81}L_{jjjj}^{V,RR} \Big] \\
& + \alpha^2 \Bigg[ \frac{896}{81}L_{ijj}^{V,LL} + \frac{1808}{81}L_{ijj}^{V,LR} - \frac{1184}{9}L_{ijj}^{V,LR} + \frac{1168}{243}L_{ii1}^{V,LL} + \frac{1168}{243}L_{ii2}^{V,LL} \\
& + \frac{1792}{243}L_{ii1}^{V,LR} + \frac{1792}{243}L_{ii2}^{V,LR} + \frac{992}{81}L_{iii}^{V,LL} + \frac{1808}{81}L_{iii}^{V,LR} - \frac{1184}{243}L_{ii1}^{V,LL} \\
& + \frac{1312}{243}L_{ii1}^{V,LR} - \frac{1144}{243}L_{11jj}^{V1,LR} + \frac{12512}{243}L_{22jj}^{V1,LR} + \frac{3248}{243}L_{11jj}^{V,LR} + \frac{3248}{243}L_{22jj}^{V,LR} \\
& - \frac{4744}{243}L_{11jj}^{V,RR} - \frac{4744}{243}L_{22jj}^{V,RR} - \frac{3808}{243}L_{jj11}^{V1,RR} - \frac{3808}{243}L_{jj22}^{V1,RR} + \frac{12224}{243}L_{jjjj}^{V1,LR} \\
& + \frac{3808}{243}L_{jjjj}^{V,RR} \Big] ; \\
\dot{L}_{ijj}^{V1,LR} = & -\frac{8}{3}g_s^2L_{ijj}^{V8,LR} + e^2 \Bigg[ \frac{8}{3}L_{ijj}^{V1,LR} + \frac{4}{9}L_{11ii}^{V,LL} + \frac{4}{9}L_{22ii}^{V,LL} + \frac{4}{9}L_{ii1}^{V1,LL} \\
& + \frac{4}{9}L_{ii2}^{V1,LL} + \frac{4}{9}L_{ii1}^{V1,LR} + \frac{4}{9}L_{ii2}^{V1,LR} + \frac{4}{9}L_{ii1}^{V,LR} + \frac{4}{9}L_{ii2}^{V,LR} - \frac{8}{9}L_{iii}^{V1,LR} \\
& + \frac{4}{9}L_{ii2}^{V,RR} + \frac{4}{9}L_{ii1}^{V,RR} + \frac{4}{9}L_{ii2}^{V,RR} + \frac{4}{9}L_{ii1}^{V,RR} - \frac{8}{9}L_{iii}^{V1,LR} \Big]
\end{aligned}$$

$$\begin{aligned}
& -\frac{64}{27}L_{\bar{u}\bar{u}\bar{u}}^{V,LL} - \frac{16}{9}L_{\bar{d}\bar{d}\bar{d}}^{V1,LR} - \frac{128}{27}L_{\bar{d}\bar{d}\bar{d}}^{V,RR} - \frac{8}{9}L_{11\bar{d}}^{V,LR} - \frac{8}{9}L_{22\bar{d}}^{V,LR} - \frac{8}{9}L_{11\bar{d}}^{V,RR} \\
& - \frac{8}{9}L_{22\bar{d}}^{V,RR} + \frac{16}{9}L_{11\bar{d}}^{V1,LR} + \frac{16}{9}L_{11\bar{d}}^{V1,RR} \Big] + \alpha_s^2 \Big[ -\frac{28}{3}L_{\bar{u}\bar{u}\bar{d}}^{V1,LR} - \frac{2132}{27}L_{\bar{u}\bar{u}\bar{d}}^{V8,LR} \\
& - 8L_{\bar{u}\bar{u}\bar{d}}^{V1,LL} - 8L_{\bar{u}\bar{u}\bar{d}}^{V1,LL} + 8L_{\bar{u}\bar{u}\bar{d}}^{V1,LR} + 8L_{\bar{u}\bar{u}\bar{d}}^{V1,LR} + \frac{44}{27}L_{\bar{u}\bar{u}\bar{d}}^{V8,LL} + \frac{44}{27}L_{\bar{u}\bar{u}\bar{d}}^{V8,LL} \\
& + \frac{44}{27}L_{\bar{u}\bar{u}\bar{d}}^{V8,LR} + \frac{44}{27}L_{\bar{u}\bar{u}\bar{d}}^{V8,LR} + 8L_{\bar{u}\bar{u}\bar{u}}^{V1,LR} + \frac{44}{27}L_{\bar{u}\bar{u}\bar{u}}^{V8,LR} - \frac{232}{9}L_{\bar{u}\bar{u}\bar{u}}^{V,LL} + 16L_{\bar{d}\bar{d}\bar{d}}^{V1,LR} \\
& + \frac{88}{27}L_{\bar{d}\bar{d}\bar{d}}^{V8,LR} - \frac{1192}{27}L_{\bar{d}\bar{d}\bar{d}}^{V,RR} + 8L_{\bar{u}\bar{u}\bar{d}}^{V1,LR} - 8L_{\bar{u}\bar{u}\bar{d}}^{V1,RR} + \frac{44}{27}L_{\bar{u}\bar{u}\bar{d}}^{V8,LR} + \frac{44}{27}L_{\bar{u}\bar{u}\bar{d}}^{V8,RR} \Big] \\
& + \alpha_s \alpha \Big[ -\frac{64}{3}L_{\bar{u}\bar{u}\bar{d}}^{V1,LR} + \frac{232}{27}L_{\bar{u}\bar{u}\bar{d}}^{V8,LR} + \frac{16}{9}L_{\bar{u}\bar{u}\bar{d}}^{V1,LL} + \frac{16}{9}L_{\bar{u}\bar{u}\bar{d}}^{V1,LL} + \frac{16}{9}L_{\bar{u}\bar{u}\bar{d}}^{V1,LR} \\
& - \frac{32}{9}L_{\bar{u}\bar{u}\bar{d}}^{V1,LR} + \frac{352}{729}L_{\bar{u}\bar{u}\bar{d}}^{V8,LL} + \frac{352}{729}L_{\bar{u}\bar{u}\bar{d}}^{V8,LL} - \frac{368}{729}L_{\bar{u}\bar{u}\bar{d}}^{V8,LR} + \frac{2008}{729}L_{\bar{u}\bar{u}\bar{d}}^{V8,LR} \\
& - \frac{32}{9}L_{\bar{u}\bar{u}\bar{u}}^{V1,LR} + \frac{2008}{729}L_{\bar{u}\bar{u}\bar{u}}^{V8,LR} - \frac{2144}{243}L_{\bar{u}\bar{u}\bar{u}}^{V,LL} - \frac{64}{9}L_{\bar{d}\bar{d}\bar{d}}^{V1,LR} + \frac{4088}{729}L_{\bar{d}\bar{d}\bar{d}}^{V8,LR} \\
& - \frac{10304}{729}L_{\bar{d}\bar{d}\bar{d}}^{V,RR} + \frac{64}{9}L_{\bar{u}\bar{u}\bar{d}}^{V1,LR} + \frac{64}{9}L_{\bar{u}\bar{u}\bar{d}}^{V1,RR} - \frac{2708}{729}L_{\bar{u}\bar{u}\bar{d}}^{V8,LR} + \frac{172}{729}L_{\bar{u}\bar{u}\bar{d}}^{V8,RR} \Big] \\
& + \alpha^2 \Big[ -\frac{880}{27}L_{\bar{u}\bar{u}\bar{d}}^{V1,LR} - \frac{1216}{729}L_{11\bar{u}}^{V,LL} - \frac{1216}{729}L_{22\bar{u}}^{V,LL} - \frac{1576}{729}L_{\bar{u}\bar{u}\bar{d}}^{V1,LL} - \frac{1576}{729}L_{\bar{u}\bar{u}\bar{d}}^{V1,LL} \\
& - \frac{208}{729}L_{\bar{u}\bar{u}\bar{d}}^{V1,LR} + \frac{6752}{729}L_{\bar{u}\bar{u}\bar{d}}^{V1,LR} + \frac{2888}{729}L_{\bar{u}\bar{u}\bar{d}}^{V,LR} + \frac{2888}{729}L_{\bar{u}\bar{u}\bar{d}}^{V,LR} + \frac{6464}{729}L_{\bar{u}\bar{u}\bar{u}}^{V1,LR} \\
& + \frac{4384}{729}L_{\bar{u}\bar{u}\bar{u}}^{V,LL} + \frac{7552}{729}L_{\bar{d}\bar{d}\bar{d}}^{V1,LR} + \frac{5392}{2187}L_{\bar{d}\bar{d}\bar{d}}^{V,RR} + \frac{6224}{729}L_{\bar{d}\bar{d}\bar{d}}^{V,LR} + \frac{6224}{729}L_{\bar{d}\bar{d}\bar{d}}^{V,LR} \\
& - \frac{3712}{729}L_{\bar{d}\bar{d}\bar{d}}^{V,RR} - \frac{3712}{729}L_{\bar{d}\bar{d}\bar{d}}^{V,RR} + \frac{6272}{729}L_{\bar{u}\bar{u}\bar{d}}^{V1,LR} - \frac{6976}{729}L_{\bar{u}\bar{u}\bar{d}}^{V1,RR} \Big] ; \\
\dot{L}_{\bar{u}\bar{u}\bar{d}}^{V8,LR} & = g_s^2 \Big[ -12L_{\bar{u}\bar{u}\bar{d}}^{V1,LR} - 14L_{\bar{u}\bar{u}\bar{d}}^{V8,LR} + \frac{2}{3}L_{\bar{u}\bar{u}\bar{d}}^{V8,LL} + \frac{2}{3}L_{\bar{u}\bar{u}\bar{d}}^{V8,LL} + \frac{2}{3}L_{\bar{u}\bar{u}\bar{d}}^{V8,LR} \\
& + \frac{2}{3}L_{\bar{u}\bar{u}\bar{d}}^{V8,LR} + \frac{2}{3}L_{\bar{u}\bar{u}\bar{u}}^{V8,LR} + \frac{8}{3}L_{\bar{u}\bar{u}\bar{u}}^{V,LL} + \frac{4}{3}L_{\bar{d}\bar{d}\bar{d}}^{V8,LR} + \frac{16}{3}L_{\bar{d}\bar{d}\bar{d}}^{V,RR} + \frac{2}{3}L_{\bar{u}\bar{u}\bar{d}}^{V8,LR} \\
& + \frac{2}{3}L_{\bar{u}\bar{u}\bar{d}}^{V8,RR} \Big] + \frac{8}{3}e^2L_{\bar{u}\bar{u}\bar{d}}^{V8,LR} + \alpha_s^2 \Big[ -\frac{418}{3}L_{\bar{u}\bar{u}\bar{d}}^{V1,LR} - \frac{3067}{18}L_{\bar{u}\bar{u}\bar{d}}^{V8,LR} - \frac{2}{3}L_{\bar{u}\bar{u}\bar{d}}^{V1,LL}
\end{aligned}$$

$$\begin{aligned}
& -\frac{2}{3}L_{\substack{ud \\ ii22}}^{V1,LL} - \frac{22}{3}L_{\substack{ud \\ ii11}}^{V1,LR} - \frac{22}{3}L_{\substack{ud \\ ii22}}^{V1,LR} + \frac{625}{81}L_{\substack{ud \\ ii11}}^{V8,LL} + \frac{625}{81}L_{\substack{ud \\ ii22}}^{V8,LL} + \frac{805}{81}L_{\substack{ud \\ ii11}}^{V8,LR} \\
& + \frac{805}{81}L_{\substack{ud \\ ii22}}^{V8,LR} - \frac{22}{3}L_{\substack{uu \\ iii}}^{V1,LR} + \frac{805}{81}L_{\substack{uu \\ iii}}^{V8,LR} + \frac{1222}{27}L_{\substack{uu \\ iii}}^{V,LL} - \frac{44}{3}L_{\substack{dd \\ jjj}}^{V1,LR} + \frac{1574}{81}L_{\substack{dd \\ jjj}}^{V8,LR} \\
& + \frac{6286}{81}L_{\substack{dd \\ jjj}}^{V,RR} - \frac{22}{3}L_{\substack{ud \\ 11jj}}^{V1,LR} - \frac{2}{3}L_{\substack{ud \\ 11jj}}^{V1,RR} + \frac{787}{81}L_{\substack{ud \\ 11jj}}^{V8,LR} + \frac{607}{81}L_{\substack{ud \\ 11jj}}^{V8,RR} \Big] \\
& + \alpha_s \alpha \left[ \frac{116}{3}L_{\substack{ud \\ ijj}}^{V1,LR} + \frac{187}{9}L_{\substack{ud \\ ijj}}^{V8,LR} + \frac{644}{81}L_{\substack{eu \\ 11ii}}^{V,LL} + \frac{644}{81}L_{\substack{eu \\ 22ii}}^{V,LL} + \frac{644}{81}L_{\substack{ud \\ ii11}}^{V1,LL} \right. \\
& + \frac{644}{81}L_{\substack{ud \\ ii22}}^{V1,LL} + \frac{644}{81}L_{\substack{ud \\ ii11}}^{V1,LR} - \frac{1216}{81}L_{\substack{ud \\ ii22}}^{V1,LR} - \frac{70}{27}L_{\substack{ud \\ ii11}}^{V8,LL} - \frac{70}{27}L_{\substack{ud \\ ii22}}^{V8,LL} + \frac{14}{9}L_{\substack{ud \\ ii11}}^{V8,LR} \\
& - \frac{20}{3}L_{\substack{ud \\ ii22}}^{V8,LR} + \frac{644}{81}L_{\substack{ue \\ ii11}}^{V,LR} + \frac{644}{81}L_{\substack{ue \\ ii22}}^{V,LR} - \frac{1288}{81}L_{\substack{uu \\ iii}}^{V1,LR} - \frac{20}{3}L_{\substack{uu \\ iii}}^{V8,LR} - \frac{3608}{81}L_{\substack{uu \\ iii}}^{V,LL} \\
& - \frac{1832}{81}L_{\substack{dd \\ jjj}}^{V1,LR} - \frac{88}{9}L_{\substack{dd \\ jjj}}^{V8,LR} - \frac{11264}{243}L_{\substack{dd \\ jjj}}^{V,RR} - \frac{916}{81}L_{\substack{ed \\ 11jj}}^{V,LR} - \frac{916}{81}L_{\substack{ed \\ 22jj}}^{V,LR} - \frac{916}{81}L_{\substack{ed \\ 11jj}}^{V,RR} \\
& - \frac{916}{81}L_{\substack{ed \\ 22jj}}^{V,RR} + \frac{1832}{81}L_{\substack{ud \\ 11jj}}^{V1,LR} + \frac{1832}{81}L_{\substack{ud \\ 11jj}}^{V1,RR} + \frac{56}{9}L_{\substack{ud \\ 11jj}}^{V8,LR} - \frac{160}{27}L_{\substack{ud \\ 11jj}}^{V8,RR} \Big] \\
& - \frac{880}{27}\alpha^2 L_{\substack{ud \\ ijj}}^{V8,LR} ;
\end{aligned}$$

$$\begin{aligned}
\dot{L}_{\substack{ed \\ jj\bar{i}}}^{V,LR} & = e^2 \left[ \frac{4}{3}L_{\substack{dd \\ jj\bar{i}}}^{V1,LR} + \frac{8}{3}L_{\substack{dd \\ ijj}}^{V,RR} + \frac{8}{9}L_{\substack{dd \\ ijj}}^{V,RR} - 4L_{\substack{ed \\ jj\bar{i}}}^{V,LR} + \frac{4}{3}L_{\substack{dd \\ iii}}^{V1,LR} \right. \\
& + \frac{32}{9}L_{\substack{dd \\ iii}}^{V,RR} + \frac{4}{3}L_{\substack{ed \\ 11ii}}^{V,LR} + \frac{4}{3}L_{\substack{ed \\ 22ii}}^{V,LR} + \frac{4}{3}L_{\substack{ed \\ 11ii}}^{V,RR} + \frac{4}{3}L_{\substack{ed \\ 22ii}}^{V,RR} - \frac{8}{3}L_{\substack{ud \\ 11ii}}^{V1,LR} \\
& - \frac{8}{3}L_{\substack{ud \\ 11ii}}^{V1,RR} + \frac{4}{9}L_{\substack{ed \\ jj11}}^{V,LL} + \frac{4}{9}L_{\substack{ed \\ jj22}}^{V,LL} + \frac{4}{9}L_{\substack{ed \\ jj11}}^{V,LR} + \frac{4}{9}L_{\substack{ed \\ jj22}}^{V,LR} + \frac{8}{3}L_{\substack{ee \\ jjj}}^{V,LL} \\
& + \frac{8}{9}L_{\substack{ee \\ jjj}}^{V,LR} - \frac{8}{9}L_{\substack{eu \\ jj11}}^{V,LL} - \frac{8}{9}L_{\substack{eu \\ jj11}}^{V,LR} \Big] + \alpha_s^2 \left[ -8L_{\substack{ed \\ jj11}}^{V,LL} - 8L_{\substack{ed \\ jj22}}^{V,LL} \right. \\
& + 8L_{\substack{ed \\ jj11}}^{V,LR} + 8L_{\substack{ed \\ jj22}}^{V,LR} - 8L_{\substack{eu \\ jj11}}^{V,LL} + 8L_{\substack{eu \\ jj11}}^{V,LR} \Big] + \alpha_s \alpha \left[ \frac{16}{3}L_{\substack{dd \\ jj\bar{i}}}^{V1,LR} \right. \\
& - \frac{1022}{243}L_{\substack{dd \\ jj\bar{i}}}^{V8,LR} + 8L_{\substack{dd \\ ijj}}^{V,RR} + \frac{64}{243}L_{\substack{dd \\ ijj}}^{V,RR} + 16L_{\substack{ed \\ jj\bar{i}}}^{V,LR} + \frac{16}{3}L_{\substack{dd \\ iii}}^{V1,LR} - \frac{1022}{243}L_{\substack{dd \\ iii}}^{V8,LR} \\
& + \frac{1048}{81}L_{\substack{dd \\ iii}}^{V,RR} - \frac{32}{3}L_{\substack{ud \\ 11ii}}^{V1,LR} - \frac{32}{3}L_{\substack{ud \\ 11ii}}^{V1,RR} + \frac{1354}{243}L_{\substack{ud \\ 11ii}}^{V8,LR} - \frac{86}{243}L_{\substack{ud \\ 11ii}}^{V8,RR} + \frac{16}{9}L_{\substack{ed \\ jj11}}^{V,LL}
\end{aligned}$$



$$\begin{aligned}
& + \frac{16}{9} L_{jj22}^{V,LL} + \frac{16}{9} L_{jj11}^{V,LR} + \frac{16}{9} L_{jj22}^{V,LR} - \frac{32}{9} L_{jj11}^{V,LL} - \frac{32}{9} L_{jj11}^{V,LR} \Big] + \alpha^2 \Bigg[ \frac{1712}{243} L_{jjii}^{V1,LR} \\
& + \frac{256}{243} L_{ijjj}^{V,RR} - \frac{1424}{729} L_{ijji}^{V,RR} + \frac{430}{9} L_{jjii}^{V,LR} + \frac{1712}{243} L_{iiii}^{V1,LR} - \frac{800}{243} L_{iiii}^{V,RR} \\
& + \frac{3728}{243} L_{11ii}^{V,LR} + \frac{3728}{243} L_{22ii}^{V,LR} - \frac{1024}{243} L_{11ii}^{V,RR} - \frac{1024}{243} L_{22ii}^{V,RR} - \frac{616}{243} L_{11ii}^{V1,LR} \\
& - \frac{6952}{243} L_{11ii}^{V1,RR} - \frac{440}{243} L_{jj11}^{V,LL} - \frac{440}{243} L_{jj22}^{V,LL} - \frac{104}{243} L_{jj11}^{V,LR} - \frac{104}{243} L_{jj22}^{V,LR} \\
& - \frac{80}{9} L_{jjjj}^{V,LL} - \frac{368}{81} L_{jjjj}^{V,LR} - \frac{1640}{243} L_{jj11}^{V,LL} - \frac{296}{243} L_{jj11}^{V,LR} \Big] ; \\
\dot{L}_{jjii}^{V,LR} & = e^2 \Bigg[ 8 L_{jjii}^{V,LR} + \frac{4}{3} L_{11ii}^{V1,LR} + \frac{4}{3} L_{22ii}^{V1,LR} + \frac{4}{3} L_{11ii}^{V,LR} + \frac{4}{3} L_{22ii}^{V,LR} \\
& + \frac{4}{3} L_{11ii}^{V,RR} + \frac{4}{3} L_{22ii}^{V,RR} + \frac{4}{3} L_{ii11}^{V1,RR} + \frac{4}{3} L_{ii22}^{V1,RR} - \frac{8}{3} L_{iiii}^{V1,LR} - \frac{64}{9} L_{iiii}^{V,RR} \\
& - \frac{8}{9} L_{jj11}^{V,LL} - \frac{8}{9} L_{jj22}^{V,LL} - \frac{8}{9} L_{jj11}^{V,LR} - \frac{8}{9} L_{jj22}^{V,LR} - \frac{16}{3} L_{jjjj}^{V,LL} - \frac{16}{9} L_{jjjj}^{V,LR} \\
& + \frac{16}{9} L_{jj11}^{V,LL} + \frac{16}{9} L_{jj11}^{V,LR} \Big] + \alpha_s^2 \Bigg[ - 8 L_{jj11}^{V,LL} - 8 L_{jj22}^{V,LL} + 8 L_{jj11}^{V,LR} \\
& + 8 L_{jj22}^{V,LR} - 8 L_{jj11}^{V,LL} + 8 L_{jj11}^{V,LR} \Big] + \alpha_s \alpha \Bigg[ - 32 L_{jjii}^{V,LR} + \frac{16}{3} L_{11ii}^{V1,LR} \\
& - \frac{32}{3} L_{22ii}^{V1,LR} - \frac{368}{243} L_{11ii}^{V8,LR} + \frac{2008}{243} L_{22ii}^{V8,LR} + \frac{16}{3} L_{ii11}^{V1,RR} + \frac{16}{3} L_{ii22}^{V1,RR} + \frac{352}{243} L_{ii11}^{V8,RR} \\
& + \frac{352}{243} L_{ii22}^{V8,RR} - \frac{32}{3} L_{iiii}^{V1,LR} + \frac{2008}{243} L_{iiii}^{V8,LR} - \frac{2144}{81} L_{iiii}^{V,RR} - \frac{32}{9} L_{jj11}^{V,LL} - \frac{32}{9} L_{jj22}^{V,LL} \\
& - \frac{32}{9} L_{jj11}^{V,LR} - \frac{32}{9} L_{jj22}^{V,LR} + \frac{64}{9} L_{jj11}^{V,LL} + \frac{64}{9} L_{jj11}^{V,LR} \Big] + \alpha^2 \Bigg[ - \frac{1184}{9} L_{jjii}^{V,LR} \\
& - \frac{1144}{243} L_{11ii}^{V1,LR} + \frac{12512}{243} L_{22ii}^{V1,LR} + \frac{3248}{243} L_{11ii}^{V,LR} + \frac{3248}{243} L_{22ii}^{V,LR} - \frac{4744}{243} L_{11ii}^{V,RR} \\
& - \frac{4744}{243} L_{22ii}^{V,RR} - \frac{3808}{243} L_{ii11}^{V1,RR} - \frac{3808}{243} L_{ii22}^{V1,RR} + \frac{12224}{243} L_{iiii}^{V1,LR} + \frac{3808}{243} L_{iiii}^{V,RR} \\
& + \frac{1168}{243} L_{jj11}^{V,LL} + \frac{1168}{243} L_{jj22}^{V,LL} + \frac{1792}{243} L_{jj11}^{V,LR} + \frac{1792}{243} L_{jj22}^{V,LR} + \frac{160}{9} L_{jjjj}^{V,LL}
\end{aligned}$$

$$\begin{aligned}
& + \frac{3616}{81} L_{jjjj}^{V,LR} - \frac{1184}{243} L_{jj11}^{V,LL} + \frac{1312}{243} L_{jj11}^{V,LR} \Big] ; \\
\dot{L}_{jj\bar{i}i}^{V1,LR} = & - \frac{8}{3} L_{jj\bar{i}i}^{V8,LR} g_s^2 + e^2 \Bigg[ - \frac{8}{9} L_{iii}^{V1,LR} - \frac{8}{9} L_{jj\bar{i}i}^{V1,LR} - \frac{64}{27} L_{iii}^{V,RR} - \frac{16}{9} L_{ijj}^{V,RR} \\
& - \frac{16}{27} L_{ijj}^{V,RR} - \frac{8}{9} L_{11\bar{i}i}^{V,LR} - \frac{8}{9} L_{ed}^{V,LR} - \frac{8}{9} L_{22\bar{i}i}^{V,LR} - \frac{8}{9} L_{11\bar{i}i}^{V,RR} - \frac{8}{9} L_{22\bar{i}i}^{V,RR} + \frac{4}{9} L_{11jj}^{V,LL} \\
& + \frac{4}{9} L_{22jj}^{V,LL} + \frac{4}{9} L_{ud}^{V1,LL} + \frac{4}{9} L_{jj11}^{V1,LL} + \frac{16}{9} L_{ud}^{V1,LL} + \frac{16}{9} L_{jj11}^{V1,LR} + \frac{4}{9} L_{ud}^{V1,LR} + \frac{4}{9} L_{jj22}^{V1,LR} \\
& + \frac{8}{3} L_{jj\bar{i}i}^{V1,LR} + \frac{16}{9} L_{11\bar{i}i}^{V1,RR} + \frac{4}{9} L_{ue}^{V,LR} + \frac{4}{9} L_{jj22}^{V,LR} - \frac{8}{9} L_{jjj}^{V1,LR} - \frac{64}{27} L_{jjj}^{V,LL} \Bigg] \\
& + \alpha_s^2 \Bigg[ 8 L_{iii}^{V1,LR} + 8 L_{jj\bar{i}i}^{V1,LR} + \frac{44}{27} L_{iii}^{V8,LR} + \frac{44}{27} L_{jj\bar{i}i}^{V8,LR} - \frac{232}{9} L_{iii}^{V,RR} \\
& - 16 L_{ijj}^{V,RR} - \frac{64}{27} L_{ijj}^{V,RR} - 8 L_{jj11}^{V1,LL} - 8 L_{jj22}^{V1,LL} + 8 L_{11\bar{i}i}^{V1,LR} + 8 L_{jj11}^{V1,LR} \\
& + 8 L_{jj22}^{V1,LR} - \frac{28}{3} L_{jj\bar{i}i}^{V1,LR} - 8 L_{11\bar{i}i}^{V1,RR} + \frac{44}{27} L_{jj11}^{V8,LL} + \frac{44}{27} L_{jj22}^{V8,LL} + \frac{44}{27} L_{11\bar{i}i}^{V8,LR} \\
& + \frac{44}{27} L_{jj11}^{V8,LR} + \frac{44}{27} L_{jj22}^{V8,LR} - \frac{2132}{27} L_{jj\bar{i}i}^{V8,LR} + \frac{44}{27} L_{11\bar{i}i}^{V8,RR} + 8 L_{jjj}^{V1,LR} + \frac{44}{27} L_{jjj}^{V8,LR} \\
& - \frac{232}{9} L_{jjj}^{V,LL} \Bigg] + \alpha_s \alpha \Bigg[ - \frac{32}{9} L_{iii}^{V1,LR} - \frac{32}{9} L_{jj\bar{i}i}^{V1,LR} + \frac{2044}{729} L_{iii}^{V8,LR} + \frac{2044}{729} L_{jj\bar{i}i}^{V8,LR} \\
& - \frac{2096}{243} L_{iii}^{V,RR} - \frac{16}{3} L_{ijj}^{V,RR} - \frac{128}{729} L_{ijj}^{V,RR} + \frac{16}{9} L_{jj11}^{V1,LL} + \frac{16}{9} L_{jj22}^{V1,LL} + \frac{64}{9} L_{11\bar{i}i}^{V1,LR} \\
& + \frac{16}{9} L_{jj11}^{V1,LR} - \frac{32}{9} L_{jj22}^{V1,LR} - \frac{64}{3} L_{jj\bar{i}i}^{V1,LR} + \frac{64}{9} L_{11\bar{i}i}^{V1,RR} + \frac{352}{729} L_{jj11}^{V8,LL} + \frac{352}{729} L_{jj22}^{V8,LL} \\
& - \frac{2708}{729} L_{11\bar{i}i}^{V8,LR} - \frac{368}{729} L_{jj11}^{V8,LR} + \frac{2008}{729} L_{jj22}^{V8,LR} + \frac{232}{27} L_{jj\bar{i}i}^{V8,LR} + \frac{172}{729} L_{11\bar{i}i}^{V8,RR} \\
& - \frac{32}{9} L_{jjj}^{V1,LR} + \frac{2008}{729} L_{jjj}^{V8,LR} - \frac{2144}{243} L_{jjj}^{V,LL} \Bigg] + \alpha^2 \Bigg[ \frac{3776}{729} L_{iii}^{V1,LR} + \frac{3776}{729} L_{jj\bar{i}i}^{V1,LR} \\
& + \frac{880}{729} L_{iii}^{V,RR} + \frac{928}{729} L_{ijj}^{V,RR} - \frac{32}{2187} L_{ijj}^{V,RR} + \frac{6224}{729} L_{11\bar{i}i}^{V,LR} + \frac{6224}{729} L_{22\bar{i}i}^{V,LR} \\
& - \frac{3712}{729} L_{11\bar{i}i}^{V,RR} - \frac{3712}{729} L_{22\bar{i}i}^{V,RR} - \frac{1216}{729} L_{11jj}^{V,LL} - \frac{1216}{729} L_{22jj}^{V,LL} - \frac{1576}{729} L_{jj11}^{V1,LR}
\end{aligned}$$

$$\begin{aligned}
& -\frac{1576}{729}L_{jj22}^{V1,LL} + \frac{6272}{729}L_{11ii}^{V1,LR} - \frac{208}{729}L_{jj11}^{V1,LR} + \frac{6752}{729}L_{jj22}^{V1,LR} - \frac{880}{27}L_{jjii}^{V1,LR} \\
& -\frac{6976}{729}L_{11ii}^{V1,RR} + \frac{2888}{729}L_{jj11}^{V,LR} + \frac{2888}{729}L_{jj22}^{V,LR} + \frac{6464}{729}L_{jjjj}^{V1,LR} + \frac{4384}{729}L_{jjjj}^{V,LL} \Big] ; \\
\dot{L}_{jjii}^{V8,LR} = & g_s^2 \left[ \frac{2}{3}L_{jjii}^{V8,LR} + \frac{8}{3}L_{ijji}^{V,RR} - 12L_{jjii}^{V1,LR} - 14L_{jjii}^{V8,LR} + \frac{2}{3}L_{iii}^{V8,LR} \right. \\
& + \frac{8}{3}L_{iii}^{V,RR} + \frac{2}{3}L_{11ii}^{V8,LR} + \frac{2}{3}L_{11ii}^{V8,RR} + \frac{2}{3}L_{jj11}^{V8,LL} + \frac{2}{3}L_{jj22}^{V8,LL} + \frac{2}{3}L_{jj11}^{V8,LR} \\
& \left. + \frac{2}{3}L_{jj22}^{V8,LR} + \frac{2}{3}L_{jjjj}^{V8,LR} + \frac{8}{3}L_{jjjj}^{V,LL} \right] + \frac{8}{3}e^2L_{jjii}^{V8,LR} + \alpha_s^2 \left[ -\frac{22}{3}L_{jjii}^{V1,LR} \right. \\
& + \frac{787}{81}L_{jjii}^{V8,LR} - \frac{28}{3}L_{ijji}^{V,RR} + \frac{3448}{81}L_{ijji}^{V,RR} - \frac{418}{3}L_{jjii}^{V1,LR} - \frac{3067}{18}L_{jjii}^{V8,LR} - \frac{22}{3}L_{iii}^{V1,LR} \\
& + \frac{787}{81}L_{iii}^{V8,LR} + \frac{1198}{27}L_{iii}^{V,RR} - \frac{22}{3}L_{11ii}^{V1,LR} - \frac{2}{3}L_{11ii}^{V1,RR} + \frac{787}{81}L_{11ii}^{V8,LR} + \frac{607}{81}L_{11ii}^{V8,RR} \\
& - \frac{2}{3}L_{jj11}^{V1,LL} - \frac{2}{3}L_{jj22}^{V1,LL} - \frac{22}{3}L_{jj11}^{V1,LR} - \frac{22}{3}L_{jj22}^{V1,LR} + \frac{625}{81}L_{jj11}^{V8,LL} + \frac{625}{81}L_{jj22}^{V8,LL} \\
& \left. + \frac{805}{81}L_{jj11}^{V8,LR} + \frac{805}{81}L_{jj22}^{V8,LR} - \frac{22}{3}L_{jjjj}^{V1,LR} + \frac{805}{81}L_{jjjj}^{V8,LR} + \frac{1222}{27}L_{jjjj}^{V,LL} \right] \\
& + \alpha_s \alpha \left[ -\frac{916}{81}L_{jjii}^{V1,LR} - \frac{44}{9}L_{jjii}^{V8,LR} - \frac{1832}{81}L_{ijji}^{V,RR} + \frac{664}{243}L_{ijji}^{V,RR} + \frac{116}{3}L_{jjii}^{V1,LR} \right. \\
& + \frac{187}{9}L_{jjii}^{V8,LR} - \frac{916}{81}L_{iii}^{V1,LR} - \frac{44}{9}L_{iii}^{V8,LR} - \frac{2144}{81}L_{iii}^{V,RR} - \frac{916}{81}L_{11ii}^{V,LR} - \frac{916}{81}L_{22ii}^{V,LR} \\
& - \frac{916}{81}L_{11ii}^{V,RR} - \frac{916}{81}L_{22ii}^{V,RR} + \frac{1832}{81}L_{11ii}^{V1,LR} + \frac{1832}{81}L_{11ii}^{V1,RR} + \frac{56}{9}L_{11ii}^{V8,LR} - \frac{160}{27}L_{11ii}^{V8,RR} \\
& + \frac{644}{81}L_{11jj}^{V,LL} + \frac{644}{81}L_{22jj}^{V,LL} + \frac{644}{81}L_{jj11}^{V1,LL} + \frac{644}{81}L_{jj22}^{V1,LL} + \frac{644}{81}L_{jj11}^{V1,LR} - \frac{1216}{81}L_{jj22}^{V1,LR} \\
& - \frac{70}{27}L_{jj11}^{V8,LL} - \frac{70}{27}L_{jj22}^{V8,LL} + \frac{14}{9}L_{jj11}^{V8,LR} - \frac{20}{3}L_{jj22}^{V8,LR} + \frac{644}{81}L_{jj11}^{V,LR} + \frac{644}{81}L_{jj22}^{V,LR} \\
& \left. - \frac{1288}{81}L_{jjjj}^{V1,LR} - \frac{20}{3}L_{jjjj}^{V8,LR} - \frac{3608}{81}L_{jjjj}^{V,LL} \right] - \frac{880}{27}\alpha^2L_{jjii}^{V8,LR} ; \\
\dot{L}_{jjii}^{V1,LR} = & -\frac{8}{3}g_s^2L_{jjii}^{V8,LR} + e^2 \left[ -\frac{8}{9}L_{jjii}^{V1,LR} + \frac{8}{9}L_{ijji}^{V,RR} + \frac{8}{27}L_{ijji}^{V,RR} + \frac{4}{9}L_{iii}^{V1,LR} \right.
\end{aligned}$$

$$\begin{aligned}
& + \frac{32}{27} L_{iii}^{V,RR} + \frac{4}{9} L_{11ii}^{V,LR} + \frac{4}{9} L_{22ii}^{V,LR} + \frac{4}{9} L_{11ii}^{V,RR} + \frac{4}{9} L_{22ii}^{V,RR} - \frac{8}{9} L_{11ii}^{V1,LR} \\
& - \frac{8}{9} L_{11ii}^{V1,RR} + \frac{8}{9} L_{jjjj}^{V1,LR} + \frac{64}{27} L_{jjjj}^{V,LL} + \frac{4}{9} L_{jj11}^{V,LR} + \frac{4}{9} L_{jj22}^{V,LR} - \frac{8}{9} L_{jj11}^{V1,LR} \\
& + \frac{4}{9} L_{11jj}^{V,LL} + \frac{4}{9} L_{22jj}^{V,LL} - \frac{8}{9} L_{11jj}^{V1,LL} \Big] + \alpha_s^2 \Big[ - \frac{4}{3} L_{jjii}^{V1,LR} - \frac{232}{3} L_{jjii}^{V8,LR} \\
& - 16 L_{ijjj}^{V,RR} - \frac{64}{27} L_{ijji}^{V,RR} + 8 L_{iiii}^{V1,LR} + \frac{44}{27} L_{iiii}^{V8,LR} - \frac{232}{9} L_{iiii}^{V,RR} + 8 L_{11ii}^{V1,LR} \\
& - 8 L_{11ii}^{V1,RR} + \frac{44}{27} L_{11ii}^{V8,LR} + \frac{44}{27} L_{11ii}^{V8,RR} + 16 L_{jjjj}^{V1,LR} + \frac{88}{27} L_{jjjj}^{V8,LR} - \frac{1192}{27} L_{jjjj}^{V,LL} \\
& + 8 L_{jj11}^{V1,LR} + \frac{44}{27} L_{jj11}^{V8,LR} - 8 L_{11jj}^{V1,LL} + \frac{44}{27} L_{11jj}^{V8,LL} \Big] + \alpha_s \alpha \Big[ \frac{112}{9} L_{jjii}^{V1,LR} \\
& - \frac{1238}{729} L_{jjii}^{V8,LR} + \frac{8}{3} L_{ijjj}^{V,RR} + \frac{64}{729} L_{ijji}^{V,RR} + \frac{16}{9} L_{iiii}^{V1,LR} - \frac{1022}{729} L_{iiii}^{V8,LR} + \frac{1048}{243} L_{iiii}^{V,RR} \\
& - \frac{32}{9} L_{11ii}^{V1,LR} - \frac{32}{9} L_{11ii}^{V1,RR} + \frac{1354}{729} L_{11ii}^{V8,LR} - \frac{86}{729} L_{11ii}^{V8,RR} + \frac{32}{9} L_{jjjj}^{V1,LR} - \frac{2044}{729} L_{jjjj}^{V8,LR} \\
& + \frac{5152}{729} L_{jjjj}^{V,LL} - \frac{32}{9} L_{jj11}^{V1,LR} + \frac{1354}{729} L_{jj11}^{V8,LR} - \frac{32}{9} L_{11jj}^{V1,LL} - \frac{86}{729} L_{11jj}^{V8,LL} \Big] \\
& + \alpha^2 \Big[ \frac{10046}{729} L_{jjii}^{V1,LR} - \frac{32}{729} L_{ijjj}^{V,RR} - \frac{848}{2187} L_{ijji}^{V,RR} + \frac{272}{729} L_{iiii}^{V1,LR} - \frac{656}{729} L_{iiii}^{V,RR} \\
& + \frac{992}{729} L_{11ii}^{V,LR} + \frac{992}{729} L_{22ii}^{V,LR} + \frac{128}{729} L_{11ii}^{V,RR} + \frac{128}{729} L_{22ii}^{V,RR} - \frac{1624}{729} L_{11ii}^{V1,LR} \\
& - \frac{2776}{729} L_{11ii}^{V1,RR} + \frac{544}{729} L_{jjjj}^{V1,LR} - \frac{2912}{2187} L_{jjjj}^{V,LL} + \frac{992}{729} L_{jj11}^{V,LR} + \frac{992}{729} L_{jj22}^{V,LR} \\
& - \frac{1624}{729} L_{jj11}^{V1,LR} + \frac{128}{729} L_{11jj}^{V,LL} + \frac{128}{729} L_{22jj}^{V,LL} - \frac{2776}{729} L_{11jj}^{V1,LL} \Big] ; \\
\dot{L}_{jjii}^{V8,LR} & = g_s^2 \Big[ - 12 L_{jjii}^{V1,LR} - \frac{40}{3} L_{jjii}^{V8,LR} + \frac{8}{3} L_{ijji}^{V,RR} + \frac{2}{3} L_{iiii}^{V8,LR} + \frac{8}{3} L_{iiii}^{V,RR} \\
& + \frac{2}{3} L_{11ii}^{V8,LR} + \frac{2}{3} L_{11ii}^{V8,RR} + \frac{4}{3} L_{jjjj}^{V8,LR} + \frac{16}{3} L_{jjjj}^{V,LL} + \frac{2}{3} L_{jj11}^{V8,LR} + \frac{2}{3} L_{11jj}^{V8,LL} \Big] \\
& - \frac{4}{3} e^2 L_{jjii}^{V8,LR} + \alpha_s^2 \Big[ - \frac{440}{3} L_{jjii}^{V1,LR} - \frac{26029}{162} L_{jjii}^{V8,LR} - \frac{28}{3} L_{ijji}^{V,RR} + \frac{3448}{81} L_{ijji}^{V,RR}
\end{aligned}$$

$$\begin{aligned}
& -\frac{22}{3}L_{\overline{iii}}^{V1,LR} + \frac{787}{81}L_{\overline{iii}}^{V8,LR} + \frac{1198}{27}L_{\overline{iii}}^{V,RR} - \frac{22}{3}L_{1\overline{ii}}^{V1,LR} - \frac{2}{3}L_{1\overline{ii}}^{V1,RR} + \frac{787}{81}L_{1\overline{ii}}^{V8,LR} \\
& + \frac{607}{81}L_{1\overline{ii}}^{V8,RR} - \frac{44}{3}L_{jjj}^{V1,LR} + \frac{1574}{81}L_{jjj}^{V8,LR} + \frac{6286}{81}L_{jjj}^{V,LL} - \frac{22}{3}L_{jj1}^{V1,LR} + \frac{787}{81}L_{jj1}^{V8,LR} \\
& - \frac{2}{3}L_{1jj}^{V1,LL} + \frac{607}{81}L_{1jj}^{V8,LL} \Big] + \alpha_s \alpha \Big[ \frac{164}{81}L_{jj\overline{ii}}^{V1,LR} - \frac{4}{3}L_{jj\overline{ii}}^{V8,LR} + \frac{544}{81}L_{i\overline{jj}}^{V,RR} \\
& - \frac{1064}{243}L_{ij\overline{ii}}^{V,RR} + \frac{272}{81}L_{\overline{iii}}^{V1,LR} + \frac{14}{9}L_{\overline{iii}}^{V8,LR} + \frac{340}{81}L_{\overline{iii}}^{V,RR} + \frac{272}{81}L_{1\overline{ii}}^{V,LR} + \frac{272}{81}L_{2\overline{ii}}^{V,LR} \\
& + \frac{272}{81}L_{1\overline{ii}}^{V,RR} + \frac{272}{81}L_{2\overline{ii}}^{V,RR} - \frac{544}{81}L_{1\overline{ii}}^{V1,LR} - \frac{544}{81}L_{1\overline{ii}}^{V1,RR} + \frac{2}{3}L_{1\overline{ii}}^{V8,LR} + \frac{122}{27}L_{1\overline{ii}}^{V8,RR} \\
& + \frac{544}{81}L_{jjj}^{V1,LR} + \frac{28}{9}L_{jjj}^{V8,LR} + \frac{1588}{243}L_{jjj}^{V,LL} + \frac{272}{81}L_{jj1}^{V,LR} + \frac{272}{81}L_{jj2}^{V,LR} - \frac{544}{81}L_{jj1}^{V1,LR} \\
& + \frac{2}{3}L_{jj1}^{V8,LR} + \frac{272}{81}L_{1jj}^{V,LL} + \frac{272}{81}L_{2jj}^{V,LL} - \frac{544}{81}L_{1jj}^{V1,LL} + \frac{122}{27}L_{1jj}^{V8,LL} \Big] \\
& + \frac{362}{27}\alpha^2 L_{jj\overline{ii}}^{V8,LR} ;
\end{aligned}$$

$$\begin{aligned}
\dot{L}_{jj\overline{ii}}^{V,LR} &= e^2 \Big[ -\frac{32}{3}L_{jj\overline{ii}}^{V,LR} + \frac{16}{3}L_{i\overline{jj}}^{V,RR} + \frac{4}{3}L_{1\overline{ii}}^{V,LR} + \frac{4}{3}L_{2\overline{ii}}^{V,LR} + \frac{4}{3}L_{i\overline{11}}^{V,RR} \\
& + \frac{4}{3}L_{ed}^{V,RR} + \frac{4}{3}L_{\overline{iii}}^{V,LR} + \frac{16}{3}L_{\overline{iii}}^{V,RR} - \frac{8}{3}L_{i\overline{11}}^{V,RR} - \frac{8}{3}L_{1\overline{ii}}^{V,LR} + \frac{4}{3}L_{jj1}^{V,LL} \\
& + \frac{4}{3}L_{jj2}^{V,LL} + \frac{4}{3}L_{jj1}^{V,LR} + \frac{4}{3}L_{jj2}^{V,LR} + 8L_{jjj}^{V,LL} + \frac{8}{3}L_{jjj}^{V,LR} - \frac{8}{3}L_{jj1}^{V,LL} \\
& - \frac{8}{3}L_{jj1}^{V,LR} \Big] + \alpha_s \alpha \Big[ \frac{16}{3}L_{1\overline{ii}}^{V,LR} + \frac{16}{3}L_{2\overline{ii}}^{V,LR} + \frac{16}{3}L_{i\overline{11}}^{V,RR} + \frac{16}{3}L_{i\overline{22}}^{V,RR} \\
& - \frac{32}{3}L_{i\overline{11}}^{V,RR} - \frac{32}{3}L_{1\overline{ii}}^{V,LR} + \frac{16}{3}L_{jj1}^{V,LL} + \frac{16}{3}L_{jj2}^{V,LL} + \frac{16}{3}L_{jj1}^{V,LR} + \frac{16}{3}L_{jj2}^{V,LR} \\
& - \frac{32}{3}L_{jj1}^{V,LL} - \frac{32}{3}L_{jj1}^{V,LR} \Big] + \alpha^2 \Big[ \frac{4274}{27}L_{jj\overline{ii}}^{V,LR} + \frac{32}{27}L_{i\overline{jj}}^{V,RR} + \frac{424}{81}L_{1\overline{ii}}^{V,LR} \\
& + \frac{424}{81}L_{2\overline{ii}}^{V,LR} - \frac{344}{81}L_{i\overline{11}}^{V,RR} - \frac{344}{81}L_{i\overline{22}}^{V,RR} + \frac{296}{27}L_{\overline{iii}}^{V,LR} - \frac{736}{27}L_{\overline{iii}}^{V,RR} - \frac{3128}{81}L_{i\overline{11}}^{V,RR} \\
& - \frac{56}{81}L_{1\overline{ii}}^{V,LR} - \frac{344}{81}L_{1\overline{ii}}^{V,LL} - \frac{344}{81}L_{jj2}^{V,LL} + \frac{424}{81}L_{jj1}^{V,LR} + \frac{424}{81}L_{jj2}^{V,LR} - \frac{80}{3}L_{jjj}^{V,LL}
\end{aligned}$$

$$+ \frac{592}{27} L_{jjjj}^{V,LR} - \frac{3128}{81} L_{jj11}^{V,LL} - \frac{56}{81} L_{jj11}^{V,LR} \Big] ;$$

### 3.9 $\Delta L = 2$ Transitions ( $\bar{\nu}_i^c \nu_j f_k f_l$ or $\bar{\nu}_i^c e_j \bar{d}_k u_l$ )

$$\begin{aligned} \dot{L}_{\nu d,ijkl}^{S,LR} &= -8g_s^2 L_{\nu d,ijkl}^{S,LR} - \frac{2}{3} e^2 L_{\nu d,ijkl}^{S,LR} - \frac{1052}{9} \alpha_s^2 L_{\nu d,ijkl}^{S,LR} - \frac{8}{9} \alpha_s \alpha L_{\nu d,ijkl}^{S,LR} \\ &\quad + \frac{79}{27} \alpha^2 L_{\nu d,ijkl}^{S,LR} ; \end{aligned}$$

$$\begin{aligned} \dot{L}_{\nu d,ijkl}^{S,LL} &= -8g_s^2 L_{\nu d,ijkl}^{S,LL} - \frac{2}{3} e^2 L_{\nu d,ijkl}^{S,LL} - \frac{1052}{9} \alpha_s^2 L_{\nu d,ijkl}^{S,LL} - \frac{8}{9} \alpha_s \alpha L_{\nu d,ijkl}^{S,LL} \\ &\quad + \frac{79}{27} \alpha^2 L_{\nu d,ijkl}^{S,LL} ; \end{aligned}$$

$$\begin{aligned} \dot{L}_{\nu d,ijkl}^{T,LL} &= \frac{8}{3} g_s^2 L_{\nu d,ijkl}^{T,LL} + \frac{2}{9} e^2 L_{\nu d,ijkl}^{T,LL} + \frac{1756}{27} \alpha_s^2 L_{\nu d,ijkl}^{T,LL} - \frac{152}{27} \alpha_s \alpha L_{\nu d,ijkl}^{T,LL} \\ &\quad - \frac{227}{81} \alpha^2 L_{\nu d,ijkl}^{T,LL} ; \end{aligned}$$

$$\dot{L}_{\nu e,ijkl}^{S,LR} = \frac{71}{3} \alpha^2 L_{\nu e,ijkl}^{S,LR} - 6e^2 L_{\nu e,ijkl}^{S,LR} ;$$

$$\dot{L}_{\nu e,ijkl}^{S,LL} = \frac{71}{3} \alpha^2 L_{\nu e,ijkl}^{S,LL} - 6e^2 L_{\nu e,ijkl}^{S,LL} ;$$

$$\dot{L}_{\nu e,ijkl}^{T,LL} = 2e^2 L_{\nu e,ijkl}^{T,LL} - \frac{379}{9} \alpha^2 L_{\nu e,ijkl}^{T,LL} ;$$

$$\dot{L}_{\nu du,ijkl}^{V,RR} = -4e^2 L_{\nu du,ijkl}^{V,RR} + 4\alpha_s \alpha L_{\nu du,ijkl}^{V,RR} - \frac{32}{9} \alpha^2 L_{\nu du,ijkl}^{V,RR} ;$$

$$\dot{L}_{\nu du,ijkl}^{V,RL} = -2e^2 L_{\nu du,ijkl}^{V,RL} - 4\alpha_s \alpha L_{\nu du,ijkl}^{V,RL} - \frac{91}{9} \alpha^2 L_{\nu du,ijkl}^{V,RL} ;$$

$$\begin{aligned} \dot{L}_{\nu du,ijkl}^{S,LR} &= -8g_s^2 L_{\nu du,ijkl}^{S,LR} + \frac{4}{3} e^2 L_{\nu du,ijkl}^{S,LR} - \frac{1052}{9} \alpha_s^2 L_{\nu du,ijkl}^{S,LR} + 12\alpha_s \alpha L_{\nu du,ijkl}^{S,LR} \\ &\quad - \frac{848}{27} \alpha^2 L_{\nu du,ijkl}^{S,LR} ; \end{aligned}$$

$$\begin{aligned}
\dot{L}_{\nu edu}^{S,LL} &= -8g_s^2 L_{\nu edu}^{S,LL} + e^2 \left[ \frac{4}{3} L_{ijkl}^{S,LL} + 8 L_{\nu edu}^{T,LL} \right] - \frac{1052}{9} \alpha_s^2 L_{\nu edu}^{S,LL} \\
&\quad + \alpha_s \alpha \left[ 12 L_{\nu edu}^{S,LL} - \frac{448}{9} L_{\nu edu}^{T,LL} \right] + \alpha^2 \left[ -\frac{923}{27} L_{\nu edu}^{S,LL} - \frac{1960}{27} L_{\nu edu}^{T,LL} \right]; \\
\dot{L}_{\nu edu}^{T,LL} &= \frac{8}{3} g_s^2 L_{\nu edu}^{T,LL} + e^2 \left[ \frac{1}{6} L_{\nu edu}^{S,LL} - \frac{40}{9} L_{\nu edu}^{T,LL} \right] + \frac{1756}{27} \alpha_s^2 L_{\nu edu}^{T,LL} \\
&\quad + \alpha_s \alpha \left[ \frac{4}{3} L_{\nu edu}^{T,LL} - \frac{4}{3} L_{\nu edu}^{S,LL} \right] + \alpha^2 \left[ \frac{1}{54} L_{\nu edu}^{S,LL} + \frac{763}{81} L_{\nu edu}^{T,LL} \right];
\end{aligned}$$

### 3.10 $\Delta L = 4$ Transitions ( $\bar{\nu}_i^c \nu_j \bar{\nu}_k^c \nu_l$ )

$$\dot{L}_{\nu\nu}^{S,LL} = 0;$$

### 3.11 $|\Delta B| = |\Delta L| = 1$ Transitions: Baryon Number Violation

$$\begin{aligned}
\dot{L}_{ddd}^{S,LL} &= -4g_s^2 L_{ddd}^{S,LL} - \frac{4}{3} e^2 L_{ddd}^{S,LL} + \frac{374}{9} \alpha_s^2 L_{ddd}^{S,LL} + \alpha_s \alpha \left[ -\frac{260}{27} L_{ddd}^{S,LL} \right. \\
&\quad \left. - \frac{256}{27} L_{iljk}^{S,LL} \right] + \alpha^2 \left[ -\frac{826}{27} L_{ijk}^{S,LL} - \frac{1792}{81} L_{iljk}^{S,LL} \right]; \\
\dot{L}_{ddd}^{S,RR} &= -4g_s^2 L_{ddd}^{S,RR} - \frac{4}{3} e^2 L_{ddd}^{S,RR} + \frac{374}{9} \alpha_s^2 L_{ddd}^{S,RR} + \alpha_s \alpha \left[ -\frac{260}{27} L_{ddd}^{S,RR} \right. \\
&\quad \left. - \frac{256}{27} L_{iljk}^{S,RR} \right] + \alpha^2 \left[ -\frac{826}{27} L_{ijk}^{S,RR} - \frac{1792}{81} L_{iljk}^{S,RR} \right]; \\
\dot{L}_{ddd}^{S,LR} &= -4g_s^2 L_{ddd}^{S,LR} - \frac{4}{3} e^2 L_{ddd}^{S,LR} + \frac{254}{9} \alpha_s^2 L_{ddd}^{S,LR} - \frac{4}{9} \alpha_s \alpha L_{ddd}^{S,LR} \\
&\quad - \frac{314}{9} \alpha^2 L_{ijk}^{S,LR}; \\
\dot{L}_{ddd}^{S,RL} &= -4g_s^2 L_{ddd}^{S,RL} - \frac{4}{3} e^2 L_{ddd}^{S,RL} + \frac{254}{9} \alpha_s^2 L_{ddd}^{S,RL} - \frac{4}{9} \alpha_s \alpha L_{ddd}^{S,RL} \\
&\quad - \frac{314}{9} \alpha^2 L_{ijk}^{S,RL};
\end{aligned}$$

$$\begin{aligned}
\dot{L}_{ijkl}^{S,LL} &= -4g_s^2 L_{ijkl}^{S,LL} + e^2 \left[ -\frac{2}{3} L_{ijkl}^{S,LL} - \frac{4}{3} L_{ikjl}^{S,LL} \right] + \frac{374}{9} \alpha_s^2 L_{ijkl}^{S,LL} \\
&\quad + \alpha_s \alpha \left[ \frac{16}{3} L_{ikjl}^{S,LL} - \frac{8}{3} L_{ijkl}^{S,LL} \right] + \alpha^2 \left[ \frac{7}{3} L_{ijkl}^{S,LL} + \frac{280}{27} L_{ikjl}^{S,LL} \right]; \\
\dot{L}_{ijkl}^{S,RR} &= -4g_s^2 L_{ijkl}^{S,RR} + e^2 \left[ -\frac{2}{3} L_{ijkl}^{S,RR} - \frac{4}{3} L_{ilkj}^{S,RR} \right] + \frac{374}{9} \alpha_s^2 L_{ijkl}^{S,RR} \\
&\quad + \alpha_s \alpha \left[ -\frac{584}{27} L_{ijkl}^{S,RR} - \frac{304}{27} L_{ilkj}^{S,RR} \right] + \alpha^2 \left[ -\frac{449}{27} L_{ijkl}^{S,RR} - \frac{376}{81} L_{ilkj}^{S,RR} \right]; \\
\dot{L}_{ijkl}^{S,LR} &= -4g_s^2 L_{ijkl}^{S,LR} - \frac{4}{3} e^2 L_{ijkl}^{S,LR} + \frac{254}{9} \alpha_s^2 L_{ijkl}^{S,LR} - \frac{184}{9} \alpha_s \alpha L_{ijkl}^{S,LR} \\
&\quad - \frac{176}{9} \alpha^2 L_{ijkl}^{S,LR}; \\
\dot{L}_{ijkl}^{S,RL} &= -4g_s^2 L_{ijkl}^{S,RL} - \frac{4}{3} e^2 L_{ijkl}^{S,RL} + \frac{254}{9} \alpha_s^2 L_{ijkl}^{S,RL} + \frac{16}{9} \alpha_s \alpha L_{ijkl}^{S,RL} \\
&\quad + \frac{88}{9} \alpha^2 L_{ijkl}^{S,RL}; \\
\dot{L}_{ijkl}^{S,LR} &= -4g_s^2 L_{ddu}^{S,LR} + \frac{2}{3} e^2 L_{ddu}^{S,LR} + \frac{254}{9} \alpha_s^2 L_{ddu}^{S,LR} - \frac{8}{9} \alpha_s \alpha L_{ddu}^{S,LR} \\
&\quad - 11 \alpha^2 L_{ddu}^{S,LR}; \\
\dot{L}_{ijlk}^{S,RL} &= -4g_s^2 L_{ddu}^{S,RL} + \frac{2}{3} e^2 L_{ddu}^{S,RL} + \frac{254}{9} \alpha_s^2 L_{ddu}^{S,RL} - \frac{8}{9} \alpha_s \alpha L_{ddu}^{S,RL} \\
&\quad - 11 \alpha^2 L_{ddu}^{S,RL}; \\
\dot{L}_{ijkl}^{S,LR} &= -4g_s^2 L_{uud}^{S,LR} + \frac{14}{3} e^2 L_{uud}^{S,LR} + \frac{254}{9} \alpha_s^2 L_{uud}^{S,LR} - \frac{68}{9} \alpha_s \alpha L_{uud}^{S,LR} \\
&\quad - \frac{209}{3} \alpha^2 L_{uud}^{S,LR}; \\
\dot{L}_{ijkl}^{S,RL} &= -4g_s^2 L_{uud}^{S,RL} + \frac{14}{3} e^2 L_{uud}^{S,RL} + \frac{254}{9} \alpha_s^2 L_{uud}^{S,RL} - \frac{68}{9} \alpha_s \alpha L_{uud}^{S,RL}
\end{aligned}$$



$$- \frac{209}{3} \alpha^2 L_{ijkl}^{S,RL} ;$$

$$\begin{aligned} \dot{L}_{duu}^{S,LL} = & -4g_s^2 L_{ijkl}^{S,LL} + e^2 \left[ -2L_{duu}^{S,LL} - \frac{20}{3} L_{ikjl}^{S,LL} \right] + \frac{374}{9} \alpha_s^2 L_{ijkl}^{S,LL} \\ & + \alpha_s \alpha \left[ \frac{20}{3} L_{duu}^{S,LL} + 16L_{ikjl}^{S,LL} \right] + \alpha^2 \left[ \frac{47}{27} L_{ijkl}^{S,LL} + \frac{1640}{27} L_{ikjl}^{S,LL} \right] ; \end{aligned}$$

$$\begin{aligned} \dot{L}_{duu}^{S,RR} = & -4g_s^2 L_{duu}^{S,RR} + e^2 \left[ -2L_{duu}^{S,RR} - \frac{20}{3} L_{ikjl}^{S,RR} \right] + \frac{374}{9} \alpha_s^2 L_{ijkl}^{S,RR} \\ & + \alpha_s \alpha \left[ \frac{20}{3} L_{duu}^{S,RR} + 16L_{ikjl}^{S,RR} \right] + \alpha^2 \left[ \frac{47}{27} L_{duu}^{S,RR} + \frac{1640}{27} L_{ikjl}^{S,RR} \right] ; \end{aligned}$$

$$\begin{aligned} \dot{L}_{duu}^{S,LR} = & -4g_s^2 L_{duu}^{S,LR} - \frac{16}{3} e^2 L_{ijkl}^{S,LR} + \frac{254}{9} \alpha_s^2 L_{ijkl}^{S,LR} + \frac{88}{9} \alpha_s \alpha L_{ijkl}^{S,LR} \\ & + \frac{8}{9} \alpha^2 L_{ijkl}^{S,LR} ; \end{aligned}$$

$$\begin{aligned} \dot{L}_{duu}^{S,RL} = & -4g_s^2 L_{duu}^{S,RL} - \frac{16}{3} e^2 L_{duu}^{S,RL} + \frac{254}{9} \alpha_s^2 L_{duu}^{S,RL} + \frac{88}{9} \alpha_s \alpha L_{duu}^{S,RL} \\ & + \frac{8}{9} \alpha^2 L_{duu}^{S,RL} ; \end{aligned}$$
