# Supplementary material for: Two-Loop Anomalous Dimensions in the LEFT: Dimension-Six Four-Fermion Operators in NDR
Source: arXiv:2501.08384 ancillary file (2026-01-17)
Supplement: Supplementary file 2 [file C_Penguin_ADM_Seeds.pdf]

# Two Loop Anomalous Dimensions in the LEFT: Dimension-Six Four-Fermion Operators in NDR

---

Jason Aebischer, Pol Morell, Marko Pesut and Javier Virto

## C Penguin ADM Seeds

In this appendix we provide the set of two-loop penguin ADM seeds required for the derivation of the complete four-fermion ADM at NLO in the JMS basis. They are given as matrices in the format of Eq.(4.29) and (4.31). Let us first generalize their definition in order to include both the lepton and down-quark bases in Eqs.(4.27)-(4.28). The generalized  $(n + m)$ -loop ADMs for these bases read:

$$\hat{\gamma}_p^{(n,m)} \Big|_{\text{Lepton Basis}} = \begin{pmatrix} 0_{4 \times 4} & \hat{O}_{P_e}^{(n,m)} & \hat{O}_{P_u}^{(n,m)} & \hat{O}_{P_d}^{(n,m)} \\ 0_{6 \times 4} & \hat{X}_e^{(n,m)} & \hat{X}_u^{(n,m)} & \hat{X}_d^{(n,m)} \end{pmatrix}, \quad (\text{C.1})$$

$$\hat{\gamma}_p^{(n,m)} \Big|_{\text{Down-Quark Basis}} = \begin{pmatrix} 0_{6 \times 6} & \hat{Q}_{P_e}^{(n,m)} & \hat{Q}_{P_u}^{(n,m)} & \hat{Q}_{P_d}^{(n,m)} \\ 0_{10 \times 6} & \hat{Y}_e^{(n,m)} & \hat{Y}_u^{(n,m)} & \hat{Y}_d^{(n,m)} \end{pmatrix}, \quad (\text{C.2})$$

while the corresponding results for the alternative bases in Eqs. (??) and (??) read:

$$\hat{\gamma}_p^{(n,m)} \Big|_{\text{Alt. Lep. Basis}} = \begin{pmatrix} 0_{4 \times 4} & \hat{C}_{P_e}^{(n,m)} & \hat{C}_{P_u}^{(n,m)} & \hat{C}_{P_d}^{(n,m)} \\ 0_{6 \times 4} & \hat{X}_e^{(n,m)} & \hat{X}_u^{(n,m)} & \hat{X}_d^{(n,m)} \end{pmatrix}, \quad (\text{C.3})$$

$$\hat{\gamma}_p^{(n,m)} \Big|_{\text{Alt. Down-Quark Basis}} = \begin{pmatrix} 0_{6 \times 6} & \hat{K}_{P_e}^{(n,m)} & \hat{K}_{P_u}^{(n,m)} & \hat{K}_{P_d}^{(n,m)} \\ 0_{10 \times 6} & \hat{Y}_e^{(n,m)} & \hat{Y}_u^{(n,m)} & \hat{Y}_d^{(n,m)} \end{pmatrix}. \quad (\text{C.4})$$

Note that the structure of all penguin contributions mixing only into  $\mathcal{O}_{5-10}^{(\ell)}$  or  $\mathcal{O}_{7-16}^{(d)}$  is maintained. Due to the structure of the penguin operators the corresponding seeds depend the fermion charges  $Q_f$  that characterize the  $\Delta F = 1$  transition,  $d_{i,j}$  or  $\ell_{i,j}$  in Eqs.(4.27)-(4.28), i.e. the “outer flavors”, as well as on the charges of the “inner” flavors. Neutrinos are included in the leptonic case, but their charge should be put to zero ( $Q_\ell \rightarrow Q_\nu = 0$ ).

The matrices  $\hat{X}_{e,u,d}^{(n,m)}$  and  $\hat{Y}_{e,u,d}^{(n,m)}$  are not relevant for our purposes, since they do not affect the change of basis. For completeness, we report them in the following as a function

of the penguin seeds

$$\hat{X}_\psi^{(n,m)} = \begin{pmatrix} \hat{M}_C \left( n_e \hat{C}_{P_\psi}^{(n,m)} + 2 \hat{O}_{P_\psi}^{(n,m)} \right) \Big|_{Q_f \rightarrow Q_e} \\ n_u \hat{N}_C \hat{C}_{P_\psi}^{(n,m)} \Big|_{Q_f \rightarrow Q_u} \\ n_d \hat{N}_C \hat{C}_{P_\psi}^{(n,m)} \Big|_{Q_f \rightarrow Q_d} \end{pmatrix}, \quad (\text{C.5})$$

$$\hat{Y}_\psi^{(n,m)} = \begin{pmatrix} \hat{M}_K \hat{K}_{P_\psi}^{(n,m)} \Big|_{Q_f \rightarrow Q_e} \\ \hat{N}_K \left( n_u \hat{K}_{P_\psi}^{(n,m)} + 2 \delta_{qu} \hat{N}_K \hat{Q}_{P_\psi}^{(n,m)} \right) \Big|_{Q_f \rightarrow Q_u} \\ \hat{N}_K \left( n_d \hat{K}_{P_\psi}^{(n,m)} + 2 \delta_{qd} \hat{N}_K \hat{Q}_{P_\psi}^{(n,m)} \right) \Big|_{Q_f \rightarrow Q_d} \end{pmatrix}, \quad (\text{C.6})$$

where  $\psi = e, u, d$  and where the matrices  $\hat{M}_i$  and  $\hat{N}_i$  are given by

$$\begin{aligned} \hat{M}_C &= \begin{pmatrix} \hat{1}_{2 \times 2} & 0_{2 \times 2} \end{pmatrix}, & \hat{M}_K &= \begin{pmatrix} \hat{1}_{2 \times 2} & 0_{2 \times 4} \end{pmatrix}, \\ \hat{N}_C &= \begin{pmatrix} 0_{2 \times 2} & \hat{1}_{2 \times 2} \end{pmatrix}, & \hat{N}_K &= \begin{pmatrix} 0_{4 \times 2} & \hat{1}_{4 \times 4} \end{pmatrix}. \end{aligned} \quad (\text{C.7})$$

The explicit lepton-basis and quark-basis penguin seeds,  $\hat{O}_{P_f}$ ,  $\hat{Q}_{P_f}$ ,  $\hat{C}_{P_f}$  and  $\hat{K}_{P_f}$ , are given below.

### C.1 Lepton Basis Penguin Seeds

Starting with the lepton penguin basis, the penguin ADM seeds read:

$$\hat{O}_{P_u}^{(2,0)} = \hat{O}_{P_d}^{(2,0)} = \begin{pmatrix} 0 & 0 \\ 0 & 0 \\ 8 & -8 \\ 4 & -4 \end{pmatrix}, \quad \hat{C}_{P_u}^{(2,0)} = \hat{C}_{P_d}^{(2,0)} = \begin{pmatrix} 0 & 0 \\ 0 & 0 \\ 8 & -8 \\ -8 & 8 \end{pmatrix}, \quad \hat{O}_{P_e}^{(2,0)} = \hat{C}_{P_e}^{(2,0)} = 0_{4 \times 2}, \quad (\text{C.8})$$

$$\hat{O}_{P_e}^{(1,1)} = \begin{pmatrix} 0 & 0 \\ 0 & 0 \\ -16Q_q & -16Q_q \\ 8Q_q & 8Q_q \end{pmatrix}, \quad \hat{C}_{P_e}^{(1,1)} = \begin{pmatrix} 0 & 0 \\ 0 & 0 \\ -16Q_q & -16Q_q \\ -16Q_q & -16Q_q \end{pmatrix}, \quad \hat{O}_{P_u}^{(1,1)} = \begin{pmatrix} 0 & 0 \\ 0 & 0 \\ \frac{32}{3}Q_q & \frac{32}{3}Q_q \\ -\frac{16}{3}Q_q & -\frac{16}{3}Q_q \end{pmatrix}, \quad (\text{C.9})$$

$$\hat{O}_{P_d}^{(1,1)} = \begin{pmatrix} 0 & 0 \\ 0 & 0 \\ -\frac{16}{3}Q_q & -\frac{16}{3}Q_q \\ \frac{8}{3}Q_q & \frac{8}{3}Q_q \end{pmatrix}, \quad \hat{C}_{P_d}^{(1,1)} = \begin{pmatrix} 0 & 0 \\ 0 & 0 \\ -\frac{16}{3}Q_q & -\frac{16}{3}Q_q \\ -\frac{16}{3}Q_q & -\frac{16}{3}Q_q \end{pmatrix}, \quad \hat{C}_{P_u}^{(1,1)} = \begin{pmatrix} 0 & 0 \\ 0 & 0 \\ \frac{32}{3}Q_q & \frac{32}{3}Q_q \\ \frac{32}{3}Q_q & \frac{32}{3}Q_q \end{pmatrix}, \quad (\text{C.10})$$

$$\hat{O}_{P_e}^{(0,2)} = \begin{pmatrix} \frac{88}{27}Q_f^2Q_l + \frac{28}{3}Q_fQ_l^2 + \frac{28}{3}Q_fQ_l - 4Q_l^3 + 12Q_l^2 & \frac{88}{27}Q_f^2Q_l + \frac{28}{3}Q_fQ_l^2 + \frac{20}{3}Q_fQ_l - 4Q_l^3 - 12Q_l^2 \\ -\frac{68}{27}Q_f^2Q_l - \frac{22}{3}Q_fQ_l^2 - \frac{22}{3}Q_fQ_l + 2Q_l^3 - 6Q_l^2 & -\frac{68}{27}Q_f^2Q_l - \frac{22}{3}Q_fQ_l^2 - \frac{22}{3}Q_fQ_l + 2Q_l^3 - 6Q_l^2 \\ \frac{88}{9}Q_f^2Q_q + 28Q_fQ_q^2 + 28Q_fQ_q - 12Q_q^3 + 36Q_q^2 & \frac{88}{9}Q_f^2Q_q + 28Q_fQ_q^2 + 20Q_fQ_q - 12Q_q^3 - 36Q_q^2 \\ -\frac{68}{9}Q_f^2Q_q - 22Q_fQ_q^2 - 2Q_fQ_q + 6Q_q^3 + 18Q_q^2 & -\frac{68}{9}Q_f^2Q_q - 22Q_fQ_q^2 - 22Q_fQ_q + 6Q_q^3 - 18Q_q^2 \end{pmatrix}, \quad (\text{C.11})$$

$$\hat{C}_{P_e}^{(0,2)} = \begin{pmatrix} \frac{88}{27}Q_f^2Q_l + \frac{4}{3}Q_fQ_l^2 + \frac{4}{3}Q_fQ_l - 4Q_l^3 + 12Q_l^2 & \frac{88}{27}Q_f^2Q_l + \frac{4}{3}Q_fQ_l^2 + \frac{44}{3}Q_fQ_l - 4Q_l^3 - 12Q_l^2 \\ \frac{136}{27}Q_f^2Q_l + \frac{44}{3}Q_fQ_l^2 + \frac{44}{3}Q_fQ_l - 4Q_l^3 + 12Q_l^2 & \frac{136}{27}Q_f^2Q_l + \frac{44}{3}Q_fQ_l^2 + \frac{44}{3}Q_fQ_l - 4Q_l^3 + 12Q_l^2 \\ \frac{88}{9}Q_f^2Q_q + \frac{92}{3}Q_fQ_q^2 + \frac{92}{3}Q_fQ_q - 12Q_q^3 + 36Q_q^2 & \frac{88}{9}Q_f^2Q_q + \frac{92}{3}Q_fQ_q^2 + \frac{52}{3}Q_fQ_q - 12Q_q^3 - 36Q_q^2 \\ \frac{136}{9}Q_f^2Q_q + \frac{52}{3}Q_fQ_q^2 + \frac{92}{3}Q_fQ_q - 12Q_q^3 - 36Q_q^2 & \frac{136}{9}Q_f^2Q_q + \frac{52}{3}Q_fQ_q^2 + \frac{52}{3}Q_fQ_q - 12Q_q^3 + 36Q_q^2 \end{pmatrix}, \quad (\text{C.12})$$

$$\hat{O}_{P_u}^{(0,2)} = \begin{pmatrix} -\frac{176}{81}Q_f^2Q_l - \frac{56}{9}Q_fQ_l^2 + \frac{112}{27}Q_fQ_l + \frac{8}{3}Q_l^3 + \frac{16}{3}Q_l^2 & -\frac{176}{81}Q_f^2Q_l - \frac{56}{9}Q_fQ_l^2 + \frac{80}{27}Q_fQ_l + \frac{8}{3}Q_l^3 - \frac{16}{3}Q_l^2 \\ \frac{136}{81}Q_f^2Q_l + \frac{44}{9}Q_fQ_l^2 - \frac{8}{27}Q_fQ_l - \frac{4}{3}Q_l^3 + \frac{8}{3}Q_l^2 & \frac{136}{81}Q_f^2Q_l + \frac{44}{9}Q_fQ_l^2 - \frac{88}{27}Q_fQ_l - \frac{4}{3}Q_l^3 - \frac{8}{3}Q_l^2 \\ -\frac{176}{27}Q_f^2Q_q - \frac{56}{3}Q_fQ_q^2 + \frac{112}{9}Q_fQ_q + 8Q_q^3 + 16Q_q^2 & -\frac{176}{27}Q_f^2Q_q - \frac{56}{3}Q_fQ_q^2 + \frac{80}{9}Q_fQ_q + 8Q_q^3 - 16Q_q^2 \\ \frac{136}{27}Q_f^2Q_q + \frac{44}{3}Q_fQ_q^2 - \frac{8}{9}Q_fQ_q - 4Q_q^3 + 8Q_q^2 & \frac{136}{27}Q_f^2Q_q + \frac{44}{3}Q_fQ_q^2 - \frac{88}{9}Q_fQ_q - 4Q_q^3 - 8Q_q^2 \end{pmatrix}, \quad (\text{C.13})$$

$$\hat{O}_{P_u}^{(0,2)} = \begin{pmatrix} -\frac{176}{81}Q_f^2Q_l - \frac{8}{9}Q_fQ_l^2 + \frac{16}{27}Q_fQ_l + \frac{8}{3}Q_l^3 + \frac{16}{3}Q_l^2 & -\frac{176}{81}Q_f^2Q_l - \frac{8}{9}Q_fQ_l^2 + \frac{176}{27}Q_fQ_l + \frac{8}{3}Q_l^3 - \frac{16}{3}Q_l^2 \\ -\frac{272}{81}Q_f^2Q_l - \frac{88}{9}Q_fQ_l^2 + \frac{16}{27}Q_fQ_l + \frac{8}{3}Q_l^3 - \frac{16}{3}Q_l^2 & -\frac{272}{81}Q_f^2Q_l - \frac{88}{9}Q_fQ_l^2 + \frac{176}{27}Q_fQ_l + \frac{8}{3}Q_l^3 + \frac{16}{3}Q_l^2 \\ 8Q_d^3 - \frac{184}{9}Q_d^2Q_f + 16Q_d^2 - \frac{176}{27}Q_dQ_f^2 + \frac{368}{27}Q_dQ_f & 8Q_d^3 - \frac{184}{9}Q_d^2Q_f - 16Q_d^2 - \frac{176}{27}Q_dQ_f^2 + \frac{208}{27}Q_dQ_f \\ 8Q_d^3 - \frac{104}{9}Q_d^2Q_f - 16Q_d^2 - \frac{272}{27}Q_dQ_f^2 + \frac{368}{27}Q_dQ_f & 8Q_d^3 - \frac{104}{9}Q_d^2Q_f + 16Q_d^2 - \frac{272}{27}Q_dQ_f^2 + \frac{208}{27}Q_dQ_f \end{pmatrix}, \quad (\text{C.14})$$

$$\hat{O}_{P_d}^{(0,2)} = \begin{pmatrix} \frac{88}{81}Q_f^2Q_l + \frac{28}{9}Q_fQ_l^2 + \frac{28}{27}Q_fQ_l - \frac{4}{3}Q_l^3 + \frac{4}{3}Q_l^2 & \frac{88}{81}Q_f^2Q_l + \frac{28}{9}Q_fQ_l^2 + \frac{20}{27}Q_fQ_l - \frac{4}{3}Q_l^3 - \frac{4}{3}Q_l^2 \\ -\frac{68}{81}Q_f^2Q_l - \frac{22}{9}Q_fQ_l^2 - \frac{2}{27}Q_fQ_l + \frac{2}{3}Q_l^3 + \frac{2}{3}Q_l^2 & -\frac{68}{81}Q_f^2Q_l - \frac{22}{9}Q_fQ_l^2 - \frac{22}{27}Q_fQ_l + \frac{2}{3}Q_l^3 - \frac{2}{3}Q_l^2 \\ \frac{88}{27}Q_f^2Q_q + \frac{28}{3}Q_fQ_q^2 + \frac{28}{9}Q_fQ_q - 4Q_q^3 + 4Q_q^2 & \frac{88}{27}Q_f^2Q_q + \frac{28}{3}Q_fQ_q^2 + \frac{20}{9}Q_fQ_q - 4Q_q^3 - 4Q_q^2 \\ -\frac{68}{27}Q_f^2Q_q - \frac{22}{3}Q_fQ_q^2 - \frac{2}{9}Q_fQ_q + 2Q_q^3 + 2Q_q^2 & -\frac{68}{27}Q_f^2Q_q - \frac{22}{3}Q_fQ_q^2 - \frac{22}{9}Q_fQ_q + 2Q_q^3 - 2Q_q^2 \end{pmatrix}, \quad (\text{C.15})$$

$$\hat{O}_{P_d}^{(0,2)} = \begin{pmatrix} \frac{88}{81}Q_f^2Q_l + \frac{4}{9}Q_fQ_l^2 + \frac{4}{27}Q_fQ_l - \frac{4}{3}Q_l^3 + \frac{4}{3}Q_l^2 & \frac{88}{81}Q_f^2Q_l + \frac{4}{9}Q_fQ_l^2 + \frac{44}{27}Q_fQ_l - \frac{4}{3}Q_l^3 - \frac{4}{3}Q_l^2 \\ \frac{136}{81}Q_f^2Q_l + \frac{44}{9}Q_fQ_l^2 + \frac{4}{27}Q_fQ_l - \frac{4}{3}Q_l^3 - \frac{4}{3}Q_l^2 & \frac{136}{81}Q_f^2Q_l + \frac{44}{9}Q_fQ_l^2 + \frac{44}{27}Q_fQ_l - \frac{4}{3}Q_l^3 + \frac{4}{3}Q_l^2 \\ \frac{88}{27}Q_f^2Q_q + \frac{92}{9}Q_fQ_q^2 + \frac{92}{27}Q_fQ_q - 4Q_q^3 + 4Q_q^2 & \frac{88}{27}Q_f^2Q_q + \frac{92}{9}Q_fQ_q^2 + \frac{52}{27}Q_fQ_q - 4Q_q^3 - 4Q_q^2 \\ \frac{136}{27}Q_f^2Q_q + \frac{52}{9}Q_fQ_q^2 + \frac{92}{27}Q_fQ_q - 4Q_q^3 - 4Q_q^2 & \frac{136}{27}Q_f^2Q_q + \frac{52}{9}Q_fQ_q^2 + \frac{52}{27}Q_fQ_q - 4Q_q^3 + 4Q_q^2 \end{pmatrix}, \quad (\text{C.16})$$

## C.2 Quark Basis Penguin Seeds

The ADM seeds for the quark penguin basis are:

$$\begin{aligned}
\hat{Q}_{P_u}^{(2,0)} = \hat{Q}_{P_d}^{(2,0)} = & \begin{pmatrix} 0 & 0 & 0 & 0 \\ 0 & 0 & 0 & 0 \\ -\frac{202}{243} & \frac{1354}{81} & -\frac{1192}{243} & \frac{904}{81} \\ \frac{79}{9} & -\frac{7}{3} & -\frac{65}{9} & -\frac{7}{3} \\ \frac{341}{243} & -\frac{53}{81} & -\frac{352}{243} & -\frac{368}{81} \\ \frac{61}{18} & \frac{11}{6} & -\frac{83}{18} & \frac{11}{6} \end{pmatrix}, \quad \hat{K}_{P_u}^{(2,0)} = \hat{K}_{P_d}^{(2,0)} = \begin{pmatrix} 0 & 0 & 0 & 0 \\ 0 & 0 & 0 & 0 \\ \frac{73}{9} & -\frac{1}{3} & -\frac{71}{9} & -\frac{1}{3} \\ -\frac{106}{243} & \frac{826}{81} & -\frac{502}{243} & \frac{646}{81} \\ -\frac{61}{9} & -\frac{11}{3} & \frac{83}{9} & -\frac{11}{3} \\ -\frac{682}{243} & \frac{106}{81} & \frac{704}{243} & \frac{736}{81} \end{pmatrix}, \quad \hat{Q}_{P_e}^{(2,0)} = \hat{K}_{P_e}^{(2,0)} = 0_{6 \times 2}, \quad (\text{C.17})
\end{aligned}$$

$$\begin{aligned}
\hat{Q}_{P_e}^{(1,1)} = & \begin{pmatrix} 0 & 0 & 0 \\ 0 & 0 & 0 \\ \frac{352}{81} Q_f + \frac{64}{9} Q_q & \frac{352}{81} Q_f + \frac{64}{9} Q_q & -16 Q_q \\ -16 Q_q & -16 Q_q & -16 Q_q \\ -\frac{272}{81} Q_f - \frac{64}{9} Q_q & -\frac{272}{81} Q_f - \frac{64}{9} Q_q & 8 Q_q \end{pmatrix}, \quad \hat{K}_{P_e}^{(1,1)} = \begin{pmatrix} 0 & 0 & 0 \\ 0 & 0 & 0 \\ -16 Q_q & -16 Q_q & -16 Q_q \\ \frac{544}{81} Q_f - \frac{32}{9} Q_q & \frac{544}{81} Q_f - \frac{32}{9} Q_q & -16 Q_q \\ -16 Q_q & -16 Q_q & -16 Q_q \\ \frac{544}{81} Q_f + \frac{128}{9} Q_q & \frac{544}{81} Q_f + \frac{128}{9} Q_q & \frac{544}{81} Q_f + \frac{128}{9} Q_q \end{pmatrix}, \quad (\text{C.18})
\end{aligned}$$

$$\begin{aligned}
\hat{Q}_{P_u}^{(1,1)} = & \begin{pmatrix} \frac{44}{81} Q_f Q_l - \frac{28}{27} Q_l & \frac{28}{9} Q_l - \frac{44}{27} Q_f Q_l & \frac{44}{81} Q_f Q_l - \frac{20}{27} Q_l \\ \frac{2}{27} Q_l - \frac{34}{81} Q_f Q_l & \frac{34}{27} Q_f Q_l - \frac{2}{9} Q_l & \frac{22}{27} Q_l - \frac{34}{81} Q_f Q_l \\ \frac{170}{81} Q_f Q_q - \frac{956}{243} Q_f - \frac{2}{3} Q_q^2 - \frac{76}{9} Q_q & -\frac{170}{27} Q_f Q_q + \frac{28}{9} Q_f + 2 Q_q^2 + \frac{100}{9} Q_q & \frac{170}{81} Q_f Q_q - \frac{884}{243} Q_f - \frac{2}{3} Q_q^2 - \frac{76}{27} Q_q \\ \frac{44}{27} Q_f Q_q + \frac{68}{9} Q_q & \frac{28}{3} Q_q - \frac{44}{9} Q_f Q_q & \frac{44}{27} Q_f Q_q + \frac{76}{9} Q_q \\ -\frac{133}{81} Q_f Q_q + \frac{562}{243} Q_f + \frac{Q_q^2}{3} + \frac{94}{27} Q_q & \frac{133}{27} Q_f Q_q - \frac{2}{9} Q_f - Q_q^2 + \frac{34}{9} Q_q & -\frac{133}{81} Q_f Q_q + \frac{742}{243} Q_f + \frac{Q_q^2}{3} + \frac{62}{9} Q_q \\ -\frac{34}{27} Q_f Q_q - \frac{46}{9} Q_q & \frac{34}{9} Q_f Q_q - \frac{2}{3} Q_q & -\frac{34}{27} Q_f Q_q - \frac{26}{9} Q_q \end{pmatrix}, \quad (\text{C.19})
\end{aligned}$$

$$\hat{K}_{P_u}^{(1,1)} = \begin{pmatrix} \frac{68}{81}Q_fQ_l - \frac{4}{27}Q_l & \frac{4}{9}Q_l - \frac{68}{27}Q_fQ_l & \frac{68}{81}Q_fQ_l - \frac{44}{27}Q_l & \frac{44}{9}Q_l - \frac{68}{27}Q_fQ_l \\ \frac{68}{81}Q_fQ_l - \frac{4}{27}Q_l & \frac{4}{9}Q_l - \frac{68}{27}Q_fQ_l & \frac{68}{81}Q_fQ_l - \frac{44}{27}Q_l & \frac{44}{9}Q_l - \frac{68}{27}Q_fQ_l \\ \frac{68}{27}Q_fQ_q + \frac{92}{9}Q_q & \frac{4}{3}Q_q - \frac{68}{9}Q_fQ_q & \frac{68}{27}Q_fQ_q + \frac{52}{9}Q_q & \frac{44}{3}Q_q - \frac{68}{9}Q_fQ_q \\ \frac{86}{81}Q_fQ_q - \frac{1124}{243}Q_f - \frac{2}{3}Q_q^2 - \frac{4}{9}Q_q & -\frac{86}{27}Q_fQ_q + \frac{4}{9}Q_f + 2Q_q^2 + \frac{76}{9}Q_q & \frac{86}{81}Q_fQ_q - \frac{1484}{243}Q_f - \frac{2}{3}Q_q^2 + \frac{92}{27}Q_q & -\frac{86}{27}Q_fQ_q + \frac{44}{9}Q_f + 2Q_q^2 - \frac{28}{9}Q_q \end{pmatrix},$$

$$\begin{pmatrix} \frac{68}{27}Q_fQ_q + \frac{92}{9}Q_q & \frac{4}{3}Q_q - \frac{68}{9}Q_fQ_q & \frac{68}{27}Q_fQ_q + \frac{52}{9}Q_q & \frac{44}{3}Q_q - \frac{68}{9}Q_fQ_q \\ \frac{266}{81}Q_fQ_q - \frac{1124}{243}Q_f - \frac{2}{3}Q_q^2 - \frac{188}{27}Q_q & -\frac{266}{27}Q_fQ_q + \frac{4}{9}Q_f + 2Q_q^2 - \frac{68}{9}Q_q & \frac{266}{81}Q_fQ_q - \frac{1484}{243}Q_f - \frac{2}{3}Q_q^2 - \frac{124}{9}Q_q & -\frac{266}{27}Q_fQ_q + \frac{44}{9}Q_f + 2Q_q^2 + \frac{116}{9}Q_q \end{pmatrix} \quad (C.20)$$

$$\hat{Q}_{P_d}^{(1,1)} = \begin{pmatrix} \frac{44}{81}Q_fQ_l + \frac{14}{27}Q_l & -\frac{44}{27}Q_fQ_l - \frac{14}{9}Q_l & \frac{44}{81}Q_fQ_l + \frac{10}{27}Q_l & -\frac{44}{27}Q_fQ_l - \frac{10}{9}Q_l \\ -\frac{34}{81}Q_fQ_l - \frac{Q_l}{27} & \frac{34}{27}Q_fQ_l + \frac{Q_l}{9} & -\frac{34}{81}Q_fQ_l - \frac{11}{27}Q_l & \frac{34}{27}Q_fQ_l + \frac{11}{9}Q_l \\ \frac{170}{81}Q_fQ_q + \frac{478}{243}Q_f - \frac{2}{3}Q_q^2 + \frac{38}{9}Q_q & -\frac{170}{27}Q_fQ_q - \frac{14}{9}Q_f + 2Q_q^2 - \frac{50}{9}Q_q & \frac{170}{81}Q_fQ_q + \frac{442}{243}Q_f - \frac{2}{3}Q_q^2 + \frac{38}{27}Q_q & -\frac{170}{27}Q_fQ_q - \frac{10}{9}Q_f + 2Q_q^2 + \frac{26}{9}Q_q \\ -\frac{133}{81}Q_fQ_q - \frac{281}{243}Q_f + \frac{Q_q^2}{3} - \frac{47}{27}Q_q & \frac{133}{27}Q_fQ_q + \frac{Q_f}{9} - Q_q^2 - \frac{17}{9}Q_q & -\frac{133}{81}Q_fQ_q - \frac{371}{243}Q_f + \frac{Q_q^2}{3} - \frac{31}{9}Q_q & \frac{133}{27}Q_fQ_q + \frac{11}{9}Q_f - Q_q^2 + \frac{29}{9}Q_q \end{pmatrix},$$

$$\begin{pmatrix} \frac{44}{27}Q_fQ_q - \frac{34}{9}Q_q & -\frac{44}{9}Q_fQ_q - \frac{14}{3}Q_q & \frac{44}{27}Q_fQ_q - \frac{38}{9}Q_q & -\frac{44}{9}Q_fQ_q - \frac{10}{3}Q_q \\ \frac{23}{9}Q_q - \frac{34}{27}Q_fQ_q & \frac{34}{9}Q_fQ_q + \frac{Q_q}{3} & \frac{13}{9}Q_q - \frac{34}{27}Q_fQ_q & \frac{34}{9}Q_fQ_q + \frac{11}{3}Q_q \end{pmatrix} \quad (C.21)$$

$$\hat{K}_{P_d}^{(1,1)} = \begin{pmatrix} \frac{68}{81}Q_fQ_l + \frac{2}{27}Q_l & -\frac{68}{27}Q_fQ_l - \frac{2}{9}Q_l & \frac{68}{81}Q_fQ_l + \frac{22}{27}Q_l & -\frac{68}{27}Q_fQ_l - \frac{22}{9}Q_l \\ \frac{68}{81}Q_fQ_l + \frac{2}{27}Q_l & -\frac{68}{27}Q_fQ_l - \frac{2}{9}Q_l & \frac{68}{81}Q_fQ_l + \frac{22}{27}Q_l & -\frac{68}{27}Q_fQ_l - \frac{22}{9}Q_l \\ \frac{68}{27}Q_fQ_q - \frac{46}{9}Q_q & -\frac{68}{9}Q_fQ_q - \frac{2}{3}Q_q & \frac{68}{27}Q_fQ_q - \frac{26}{9}Q_q & -\frac{68}{9}Q_fQ_q - \frac{22}{3}Q_q \\ \frac{86}{81}Q_fQ_q + \frac{562}{243}Q_f - \frac{2}{3}Q_q^2 + \frac{2}{9}Q_q & -\frac{86}{27}Q_fQ_q - \frac{2}{9}Q_f + 2Q_q^2 - \frac{38}{9}Q_q & \frac{86}{81}Q_fQ_q + \frac{742}{243}Q_f - \frac{2}{3}Q_q^2 - \frac{46}{27}Q_q & -\frac{86}{27}Q_fQ_q - \frac{22}{9}Q_f + 2Q_q^2 + \frac{14}{9}Q_q \end{pmatrix},$$

$$\begin{pmatrix} \frac{68}{27}Q_fQ_q - \frac{46}{9}Q_q & -\frac{68}{9}Q_fQ_q - \frac{2}{3}Q_q & \frac{68}{27}Q_fQ_q - \frac{26}{9}Q_q & -\frac{68}{9}Q_fQ_q - \frac{22}{3}Q_q \\ \frac{266}{81}Q_fQ_q + \frac{562}{243}Q_f - \frac{2}{3}Q_q^2 + \frac{94}{27}Q_q & -\frac{266}{27}Q_fQ_q - \frac{2}{9}Q_f + 2Q_q^2 + \frac{34}{9}Q_q & \frac{266}{81}Q_fQ_q + \frac{742}{243}Q_f - \frac{2}{3}Q_q^2 + \frac{62}{9}Q_q & -\frac{266}{27}Q_fQ_q - \frac{22}{9}Q_f + 2Q_q^2 - \frac{58}{9}Q_q \end{pmatrix} \quad (C.22)$$

$$\hat{Q}_{P_e}^{(0,2)} = \begin{pmatrix} \frac{88}{27}Q_f^2Q_l + \frac{28}{3}Q_fQ_l^2 + \frac{28}{3}Q_fQ_l - 4Q_l^3 + 12Q_l^2 & \frac{88}{27}Q_f^2Q_l + \frac{28}{3}Q_fQ_l^2 + \frac{20}{3}Q_fQ_l - 4Q_l^3 - 12Q_l^2 \\ -\frac{68}{27}Q_f^2Q_l - \frac{22}{3}Q_fQ_l^2 - \frac{22}{3}Q_fQ_l + 2Q_l^3 + 6Q_l^2 & -\frac{68}{27}Q_f^2Q_l - \frac{22}{3}Q_fQ_l^2 - \frac{22}{3}Q_fQ_l + 2Q_l^3 - 6Q_l^2 \\ \frac{88}{27}Q_f^2Q_q + \frac{28}{3}Q_fQ_q^2 + \frac{28}{3}Q_fQ_q - 4Q_q^3 + 12Q_q^2 & \frac{88}{27}Q_f^2Q_q + \frac{28}{3}Q_fQ_q^2 + \frac{20}{3}Q_fQ_q - 4Q_q^3 - 12Q_q^2 \\ \frac{88}{9}Q_f^2Q_q + 28Q_fQ_q^2 + 28Q_fQ_q - 12Q_q^3 + 36Q_q^2 & \frac{88}{9}Q_f^2Q_q + 28Q_fQ_q^2 + 20Q_fQ_q - 12Q_q^3 - 36Q_q^2 \\ -\frac{68}{27}Q_f^2Q_q - \frac{22}{3}Q_fQ_q^2 - \frac{22}{3}Q_fQ_q + 2Q_q^3 + 6Q_q^2 & -\frac{68}{27}Q_f^2Q_q - \frac{22}{3}Q_fQ_q^2 - \frac{22}{3}Q_fQ_q + 2Q_q^3 - 6Q_q^2 \\ -\frac{68}{9}Q_f^2Q_q - 22Q_fQ_q^2 - 22Q_fQ_q + 6Q_q^3 - 18Q_q^2 & -\frac{68}{9}Q_f^2Q_q - 22Q_fQ_q^2 - 22Q_fQ_q + 6Q_q^3 - 18Q_q^2 \end{pmatrix}, \quad (\text{C.23})$$

$$\hat{K}_{P_e}^{(0,2)} = \begin{pmatrix} \frac{136}{27}Q_f^2Q_l + \frac{4}{3}Q_fQ_l^2 + \frac{44}{3}Q_fQ_l - 4Q_l^3 + 12Q_l^2 & \frac{136}{27}Q_f^2Q_l + \frac{4}{3}Q_fQ_l^2 + \frac{44}{3}Q_fQ_l - 4Q_l^3 - 12Q_l^2 \\ \frac{136}{27}Q_f^2Q_l + \frac{44}{3}Q_fQ_l^2 + \frac{44}{3}Q_fQ_l - 4Q_l^3 + 12Q_l^2 & \frac{136}{27}Q_f^2Q_l + \frac{44}{3}Q_fQ_l^2 + \frac{44}{3}Q_fQ_l - 4Q_l^3 + 12Q_l^2 \\ \frac{136}{9}Q_f^2Q_q + 4Q_fQ_q^2 + 44Q_fQ_q - 12Q_q^3 - 36Q_q^2 & \frac{136}{9}Q_f^2Q_q + 4Q_fQ_q^2 + 44Q_fQ_q - 12Q_q^3 - 36Q_q^2 \\ \frac{136}{27}Q_f^2Q_q + \frac{4}{3}Q_fQ_q^2 + \frac{44}{3}Q_fQ_q - 4Q_q^3 - 12Q_q^2 & \frac{136}{27}Q_f^2Q_q + \frac{4}{3}Q_fQ_q^2 + \frac{44}{3}Q_fQ_q - 4Q_q^3 - 12Q_q^2 \\ \frac{136}{9}Q_f^2Q_q + 44Q_fQ_q^2 + 44Q_fQ_q - 12Q_q^3 + 36Q_q^2 & \frac{136}{9}Q_f^2Q_q + 44Q_fQ_q^2 + 44Q_fQ_q - 12Q_q^3 + 36Q_q^2 \\ \frac{136}{27}Q_f^2Q_q + \frac{44}{3}Q_fQ_q^2 + \frac{44}{3}Q_fQ_q - 4Q_q^3 + 12Q_q^2 & \frac{136}{27}Q_f^2Q_q + \frac{44}{3}Q_fQ_q^2 + \frac{44}{3}Q_fQ_q - 4Q_q^3 + 12Q_q^2 \end{pmatrix}, \quad (\text{C.24})$$

$$\hat{Q}_{P_u}^{(0,2)} = \begin{pmatrix} -\frac{176}{81}Q_f^2Q_l - \frac{56}{9}Q_fQ_l^2 + \frac{112}{27}Q_fQ_l + \frac{8}{3}Q_l^3 + \frac{16}{3}Q_l^2 & 0 \\ \frac{136}{81}Q_f^2Q_l + \frac{44}{9}Q_fQ_l^2 - \frac{8}{27}Q_fQ_l - \frac{4}{3}Q_l^3 + \frac{8}{3}Q_l^2 & 0 \\ -\frac{176}{81}Q_f^2Q_q - \frac{56}{9}Q_fQ_q^2 + \frac{112}{27}Q_fQ_q + \frac{8}{3}Q_q^3 + \frac{16}{3}Q_q^2 & 0 \\ -\frac{176}{27}Q_f^2Q_q - \frac{56}{3}Q_fQ_q^2 + \frac{112}{9}Q_fQ_q + 8Q_q^3 + 16Q_q^2 & 0 \\ \frac{136}{81}Q_f^2Q_q + \frac{44}{9}Q_fQ_q^2 - \frac{8}{27}Q_fQ_q - \frac{4}{3}Q_q^3 + \frac{8}{3}Q_q^2 & 0 \\ \frac{136}{27}Q_f^2Q_q + \frac{44}{3}Q_fQ_q^2 - \frac{8}{9}Q_fQ_q - 4Q_q^3 + 8Q_q^2 & 0 \end{pmatrix}, \quad (\text{C.25})$$

$$\hat{K}_{P_u}^{(0,2)} = \begin{pmatrix} -\frac{272}{81}Q_f^2Q_l - \frac{8}{9}Q_fQ_l^2 + \frac{16}{27}Q_fQ_l + \frac{8}{3}Q_l^3 + \frac{16}{3}Q_l^2 & 0 \\ -\frac{272}{81}Q_f^2Q_l - \frac{8}{9}Q_fQ_l^2 + \frac{16}{27}Q_fQ_l + \frac{8}{3}Q_l^3 - \frac{16}{3}Q_l^2 & 0 \\ -\frac{272}{27}Q_f^2Q_q - \frac{8}{3}Q_fQ_q^2 + \frac{16}{9}Q_fQ_q + 8Q_q^3 + 16Q_q^2 & 0 \\ -\frac{272}{27}Q_f^2Q_q - \frac{8}{3}Q_fQ_q^2 + \frac{16}{9}Q_fQ_q + \frac{8}{3}Q_q^3 + \frac{16}{3}Q_q^2 & 0 \\ -\frac{272}{27}Q_f^2Q_q - \frac{88}{3}Q_fQ_q^2 + \frac{16}{9}Q_fQ_q + 8Q_q^3 - 16Q_q^2 & 0 \\ -\frac{272}{81}Q_f^2Q_q - \frac{88}{9}Q_fQ_q^2 + \frac{16}{27}Q_fQ_q + \frac{8}{3}Q_q^3 - \frac{16}{3}Q_q^2 & 0 \end{pmatrix}, \quad (\text{C.26})$$

$$\begin{aligned}
\hat{Q}_{Pd}^{(0,2)} &= \begin{pmatrix} \frac{88}{81}Q_f^2Q_l + \frac{28}{9}Q_fQ_l^2 + \frac{28}{27}Q_fQ_l - \frac{4}{3}Q_l^3 + \frac{4}{3}Q_l^2 & 0 & \frac{88}{81}Q_f^2Q_l + \frac{28}{9}Q_fQ_l^2 + \frac{20}{27}Q_fQ_l - \frac{4}{3}Q_l^3 - \frac{4}{3}Q_l^2 & 0 \\ -\frac{68}{81}Q_f^2Q_l - \frac{22}{9}Q_fQ_l^2 - \frac{2}{27}Q_fQ_l + \frac{2}{3}Q_l^3 + \frac{2}{3}Q_l^2 & 0 & -\frac{68}{81}Q_f^2Q_l - \frac{22}{9}Q_fQ_l^2 - \frac{22}{27}Q_fQ_l + \frac{2}{3}Q_l^3 - \frac{2}{3}Q_l^2 & 0 \\ \frac{88}{81}Q_f^2Q_q + \frac{28}{9}Q_fQ_q^2 + \frac{28}{27}Q_fQ_q - \frac{4}{3}Q_q^3 + \frac{4}{3}Q_q^2 & 0 & \frac{88}{81}Q_f^2Q_q + \frac{28}{9}Q_fQ_q^2 + \frac{20}{27}Q_fQ_q - \frac{4}{3}Q_q^3 - \frac{4}{3}Q_q^2 & 0 \\ \frac{88}{27}Q_f^2Q_q + \frac{28}{3}Q_fQ_q^2 + \frac{28}{9}Q_fQ_q - 4Q_q^3 + 4Q_q^2 & 0 & \frac{88}{27}Q_f^2Q_q + \frac{28}{3}Q_fQ_q^2 + \frac{20}{9}Q_fQ_q - 4Q_q^3 - 4Q_q^2 & 0 \\ -\frac{68}{81}Q_f^2Q_q - \frac{22}{9}Q_fQ_q^2 - \frac{2}{27}Q_fQ_q + \frac{2}{3}Q_q^3 + \frac{2}{3}Q_q^2 & 0 & -\frac{68}{81}Q_f^2Q_q - \frac{22}{9}Q_fQ_q^2 - \frac{22}{27}Q_fQ_q + \frac{2}{3}Q_q^3 - \frac{2}{3}Q_q^2 & 0 \\ -\frac{68}{27}Q_f^2Q_q - \frac{22}{3}Q_fQ_q^2 - \frac{2}{9}Q_fQ_q + 2Q_q^3 + 2Q_q^2 & 0 & -\frac{68}{27}Q_f^2Q_q - \frac{22}{3}Q_fQ_q^2 - \frac{22}{9}Q_fQ_q + 2Q_q^3 - 2Q_q^2 & 0 \end{pmatrix}, \\
&\quad (C.27) \\
\hat{K}_{Pd}^{(0,2)} &= \begin{pmatrix} \frac{136}{81}Q_f^2Q_l + \frac{4}{9}Q_fQ_l^2 + \frac{4}{27}Q_fQ_l - \frac{4}{3}Q_l^3 + \frac{4}{3}Q_l^2 & 0 & \frac{136}{81}Q_f^2Q_l + \frac{4}{9}Q_fQ_l^2 + \frac{44}{27}Q_fQ_l - \frac{4}{3}Q_l^3 - \frac{4}{3}Q_l^2 & 0 \\ \frac{136}{81}Q_f^2Q_l + \frac{44}{9}Q_fQ_l^2 + \frac{4}{27}Q_fQ_l - \frac{4}{3}Q_l^3 - \frac{4}{3}Q_l^2 & 0 & \frac{136}{81}Q_f^2Q_l + \frac{44}{9}Q_fQ_l^2 + \frac{44}{27}Q_fQ_l - \frac{4}{3}Q_l^3 + \frac{4}{3}Q_l^2 & 0 \\ \frac{136}{27}Q_f^2Q_q + \frac{4}{3}Q_fQ_q^2 + \frac{4}{9}Q_fQ_q - 4Q_q^3 + 4Q_q^2 & 0 & \frac{136}{27}Q_f^2Q_q + \frac{4}{3}Q_fQ_q^2 + \frac{44}{9}Q_fQ_q - 4Q_q^3 - 4Q_q^2 & 0 \\ \frac{136}{81}Q_f^2Q_q + \frac{4}{9}Q_fQ_q^2 + \frac{4}{27}Q_fQ_q - \frac{4}{3}Q_q^3 + \frac{4}{3}Q_q^2 & 0 & \frac{136}{81}Q_f^2Q_q + \frac{4}{9}Q_fQ_q^2 + \frac{44}{27}Q_fQ_q - \frac{4}{3}Q_q^3 - \frac{4}{3}Q_q^2 & 0 \\ \frac{136}{27}Q_f^2Q_q + \frac{44}{3}Q_fQ_q^2 + \frac{4}{9}Q_fQ_q - 4Q_q^3 - 4Q_q^2 & 0 & \frac{136}{27}Q_f^2Q_q + \frac{44}{3}Q_fQ_q^2 + \frac{44}{9}Q_fQ_q - 4Q_q^3 + 4Q_q^2 & 0 \\ \frac{136}{81}Q_f^2Q_q + \frac{44}{9}Q_fQ_q^2 + \frac{4}{27}Q_fQ_q - \frac{4}{3}Q_q^3 - \frac{4}{3}Q_q^2 & 0 & \frac{136}{81}Q_f^2Q_q + \frac{44}{9}Q_fQ_q^2 + \frac{44}{27}Q_fQ_q - \frac{4}{3}Q_q^3 + \frac{4}{3}Q_q^2 & 0 \end{pmatrix}. \\
&\quad (C.28)
\end{aligned}$$
